# Supplementary material for: Hydride Units Filled B--C Clathrate: A New Pathway for High-Temperature Superconductivity at Ambient Pressure
Source: arXiv:2311.01656 source file (2024-07-09)
Supplement: Supplementary file 1 [file SI.pdf]

# Supplemental Material of “Hydride Units Filled B–C Clathrate: A New Pathway for High-Temperature Superconductivity at Ambient Pressure”

Ying Sun and Li Zhu\*

*Department of Physics, Rutgers University, Newark, New Jersey 07102, United States*

## CONTENTS

|                                                                                             |     |
|---------------------------------------------------------------------------------------------|-----|
| I. Supplementary Figures                                                                    | 2   |
| 1.1 $\text{SrNH}_4\text{B}_6\text{C}_6$                                                     | 2   |
| 1.2 $\text{NaNH}_4\text{B}_6\text{C}_6$                                                     | 4   |
| 1.3 $\text{KNH}_4\text{B}_6\text{C}_6$                                                      | 5   |
| 1.4 $\text{CaNH}_4\text{B}_6\text{C}_6$                                                     | 6   |
| 1.5 $\text{YNH}_4\text{B}_6\text{C}_6$                                                      | 7   |
| 1.6 $\text{PbNH}_4\text{B}_6\text{C}_6$                                                     | 8   |
| 1.7 $\text{LaNH}_4\text{B}_6\text{C}_6$                                                     | 9   |
| 1.8 $\text{PrNH}_4\text{B}_6\text{C}_6$                                                     | 10  |
| 1.9 $\text{NdNH}_4\text{B}_6\text{C}_6$                                                     | 11  |
| 1.10 $\text{PmNH}_4\text{B}_6\text{C}_6$                                                    | 12  |
| 1.11 $\text{SmNH}_4\text{B}_6\text{C}_6$                                                    | 13  |
| 1.12 $\text{EuNH}_4\text{B}_6\text{C}_6$                                                    | 14  |
| 1.13 $\text{GdNH}_4\text{B}_6\text{C}_6$                                                    | 15  |
| 1.14 $\text{TbNH}_4\text{B}_6\text{C}_6$                                                    | 16  |
| 1.15 $\text{DyNH}_4\text{B}_6\text{C}_6$                                                    | 17  |
| 1.16 $\text{HoNH}_4\text{B}_6\text{C}_6$                                                    | 18  |
| 1.17 $\text{ErNH}_4\text{B}_6\text{C}_6$                                                    | 19  |
| 1.18 $\text{TmNH}_4\text{B}_6\text{C}_6$                                                    | 20  |
| 1.19 $\text{YbNH}_4\text{B}_6\text{C}_6$                                                    | 21  |
| 1.20 $\text{LuNH}_4\text{B}_6\text{C}_6$                                                    | 22  |
| 1.21 $\text{AcNH}_4\text{B}_6\text{C}_6$                                                    | 23  |
| 1.22 $\text{ThNH}_4\text{B}_6\text{C}_6$                                                    | 24  |
| 1.23 $\text{PaNH}_4\text{B}_6\text{C}_6$                                                    | 25  |
| 1.24 $\text{UNH}_4\text{B}_6\text{C}_6$                                                     | 26  |
| II. Supplementary Tables                                                                    | 27  |
| 2.1 Electron-phonon interaction properties of $\text{MNH}_4\text{B}_6\text{C}_6$ compounds. | 27  |
| III. Supplementary Information                                                              | 28  |
| 3.1 Structure parameters of $\text{MNH}_4\text{B}_6\text{C}_6$ compounds.                   | 28  |
| 3.2 Possible synthesis paths of $\text{MNH}_4\text{B}_6\text{C}_6$ materials.               | 43  |
| References                                                                                  | 109 |

## I. SUPPLEMENTARY FIGURES

1.1  $\text{SrNH}_4\text{B}_6\text{C}_6$ 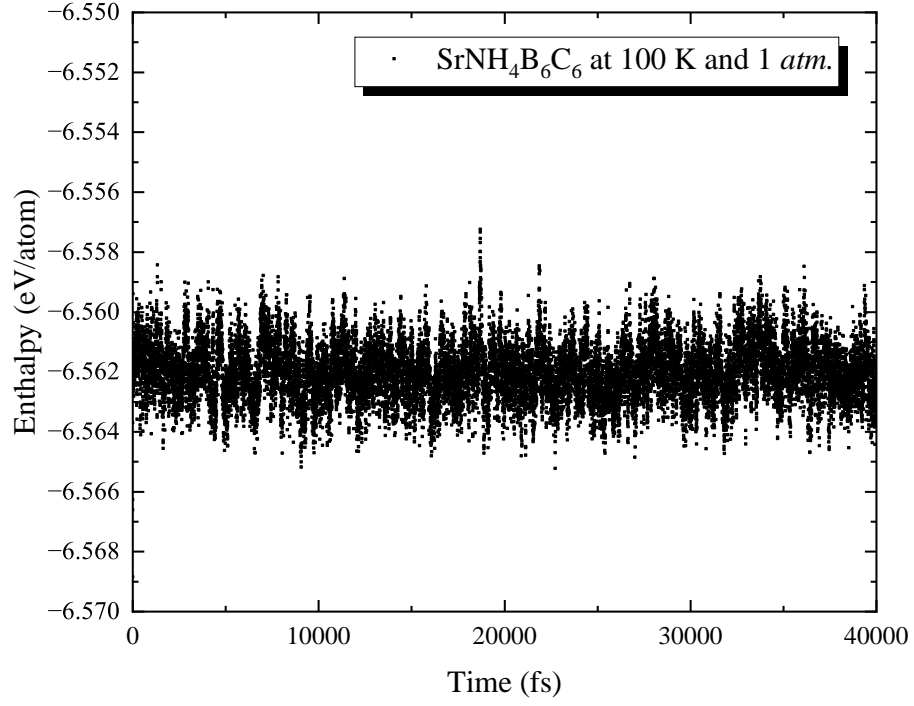

FIG. S1. Enthalpy evolution of  $\text{SrNH}_4\text{B}_6\text{C}_6$  during the 100 K metadynamics simulations at ambient pressure.

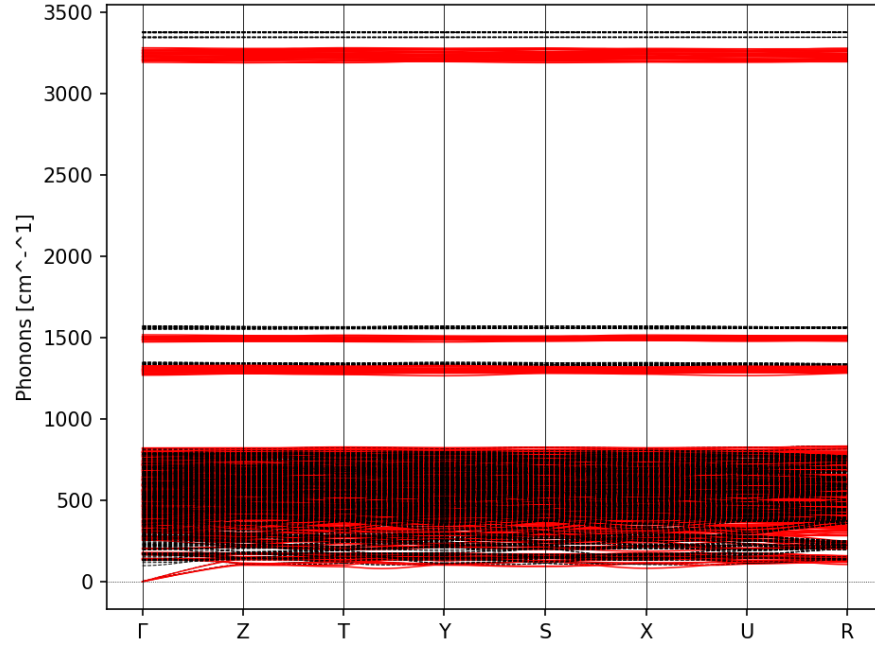

FIG. S2. Comparison between the SSCHA anharmonic (red lines) and the harmonic (black dash lines) phonon dispersion of  $Fmmm - \text{SrNH}_4\text{B}_6\text{C}_6$  at 0 K and ambient pressure.

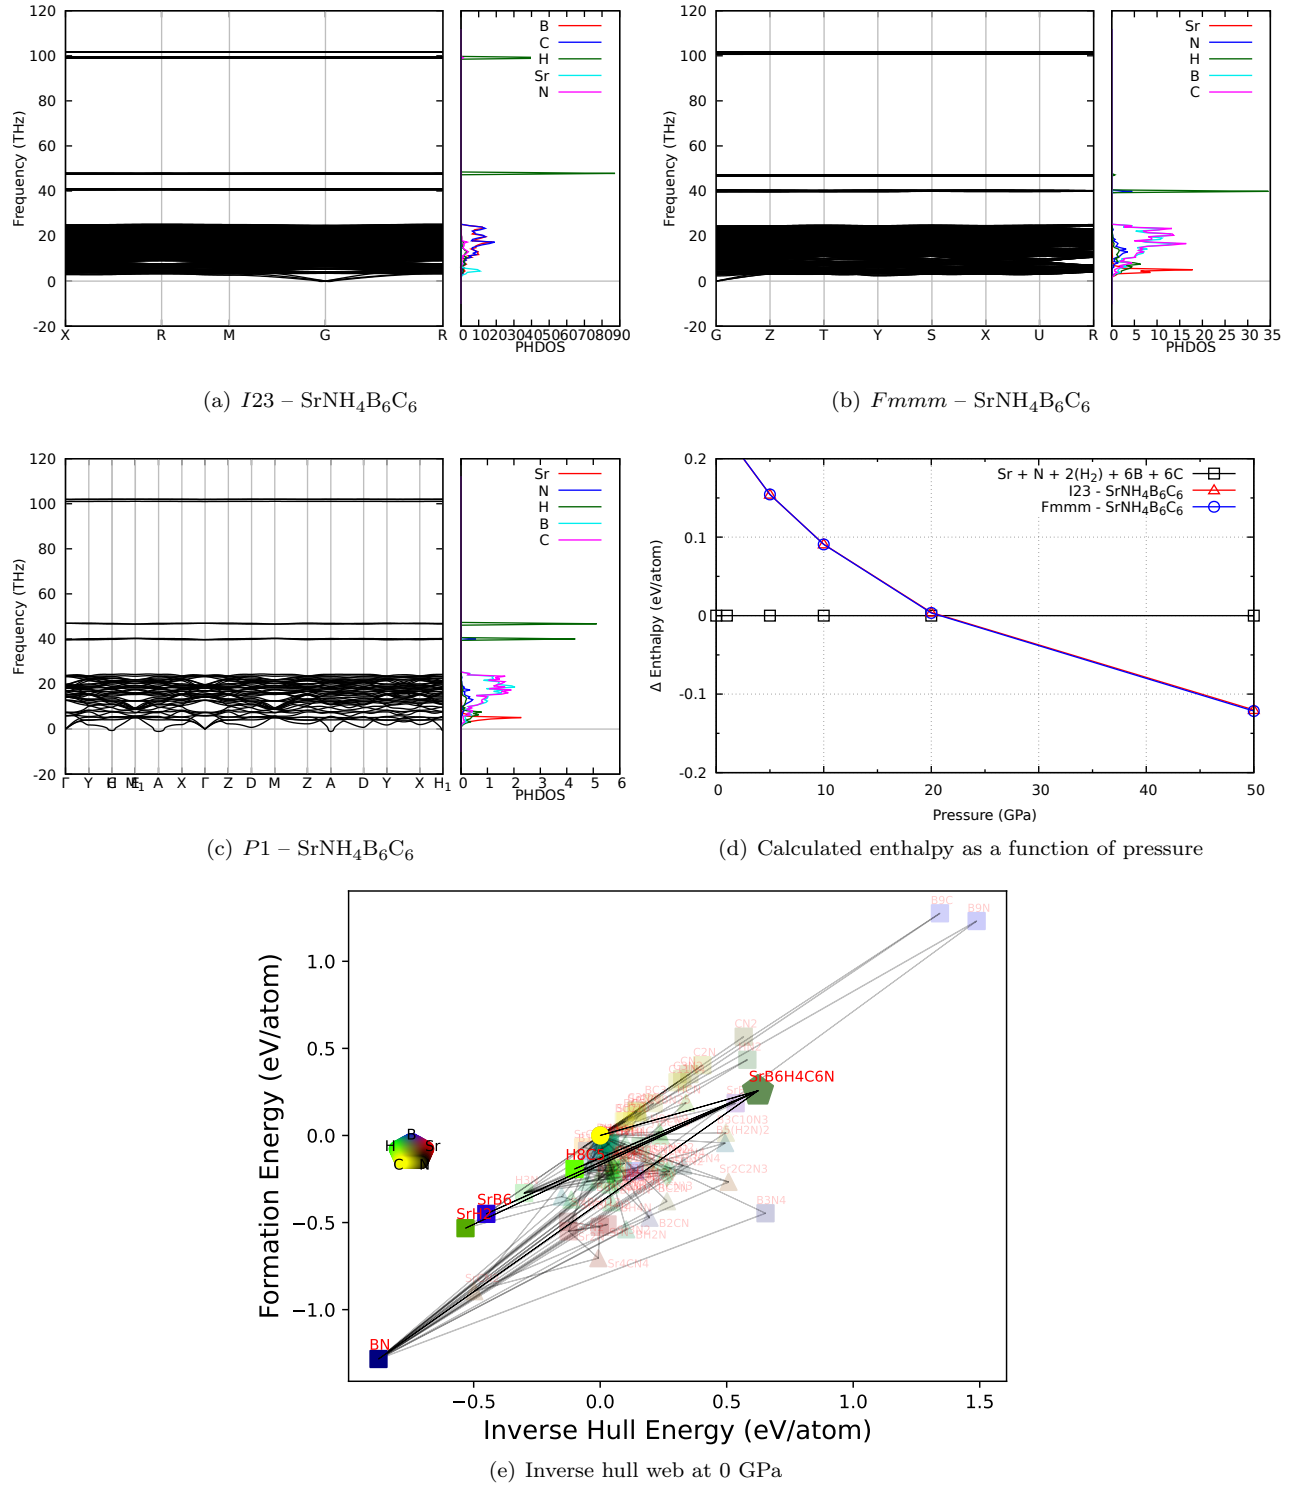

FIG. S3. (a-c) Phonon dispersion (left panel) and projected phonon densities of states (PHDOS, right panel) of different  $\text{SrNH}_4\text{B}_6\text{C}_6$  phases at ambient pressure. The absence of an imaginary frequency in the phonon spectra indicates that the structures are dynamically stable at ambient pressure. (d) Calculated enthalpy as a function of pressure for  $\text{SrNH}_4\text{B}_6\text{C}_6$  relative to simple elemental substance, and the phase transition pressure is  $\sim 20.8$  GPa. (e) Inverse hull web of Sr-N-H-B-C system at 0 K and ambient pressure. Compounds located in the positive range of the inverse-hull-energy axis indicates that they are metastable, while the others located in the negative range of the inverse-hull-energy axis are stable ones. We leave the  $\text{SrNH}_4\text{B}_6\text{C}_6$  compound and its hull reactants opaque, while we make all other phases partially transparent. Ground state structures of simple substances and other compounds were collected from the Inorganic Crystal Structure Database (ICSD) [1].

## 1.2 $\text{NaNH}_4\text{B}_6\text{C}_6$

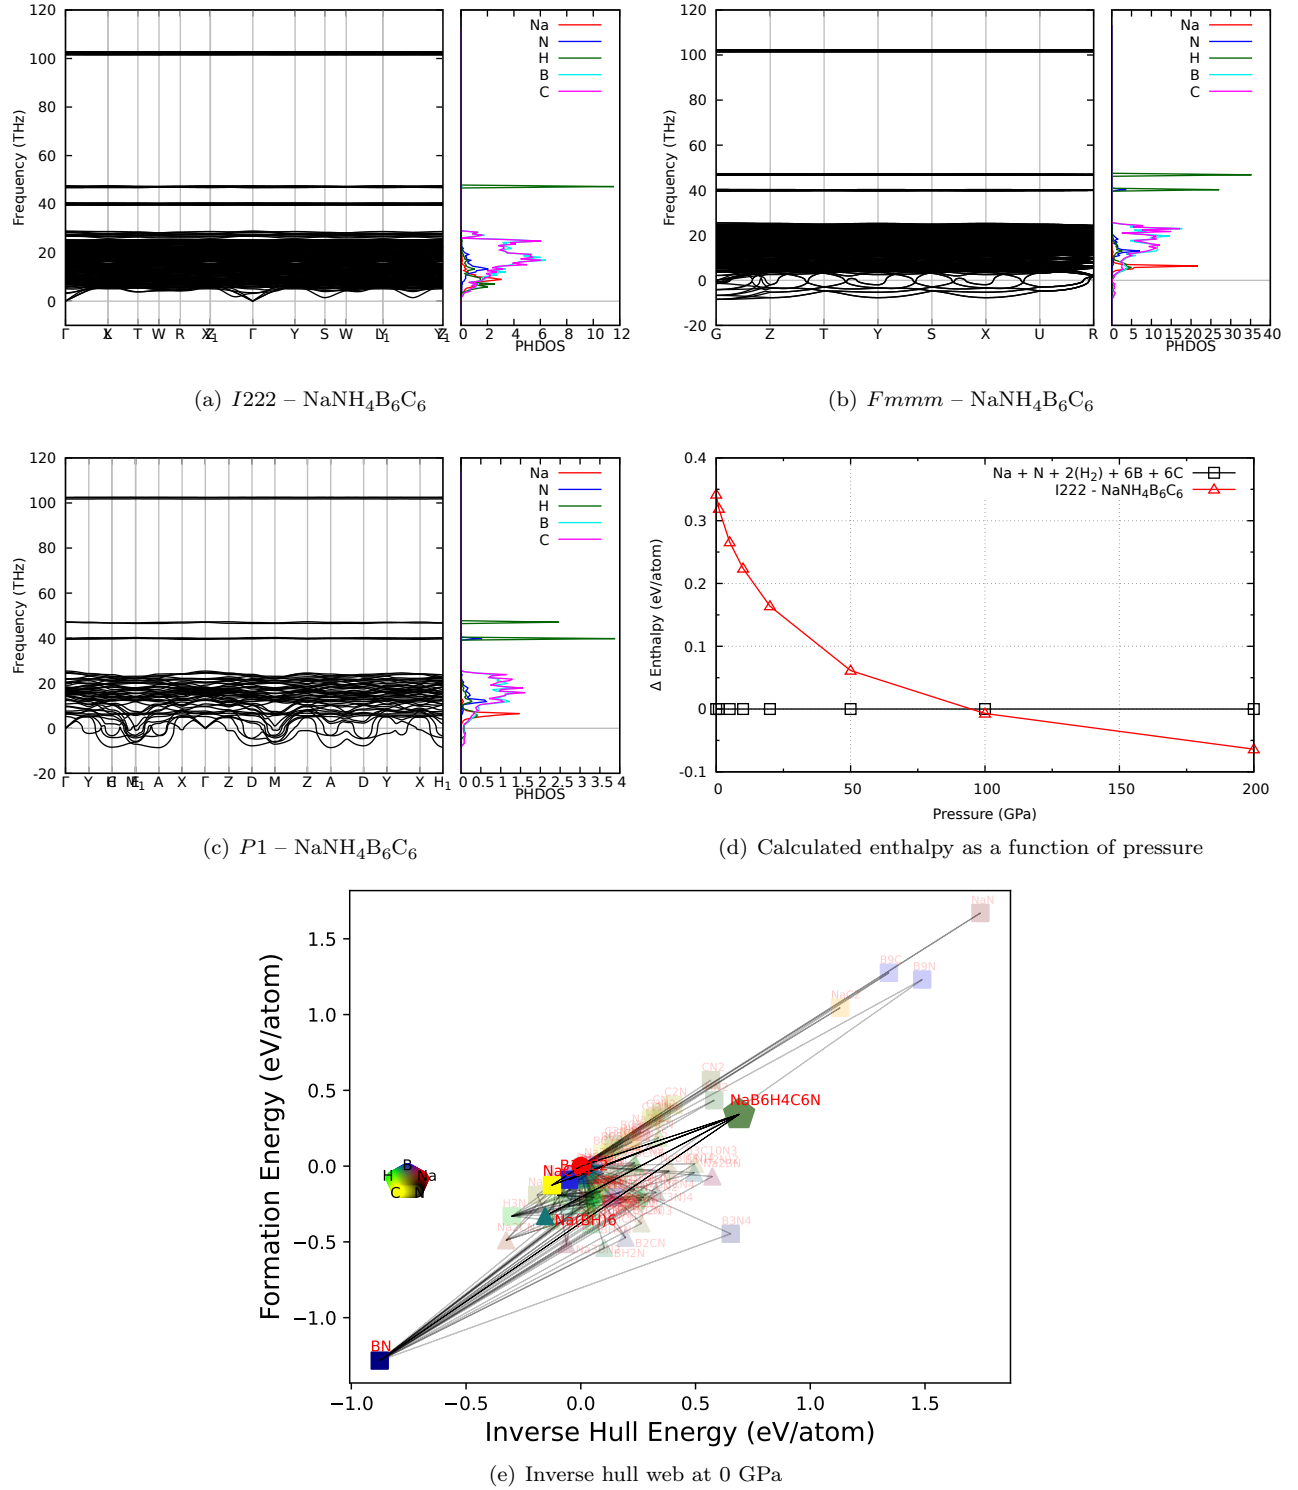

FIG. S4. (a–c) Phonon dispersion (left panel) and projected phonon densities of states (PHDOS, right panel) of different  $\text{NaNH}_4\text{B}_6\text{C}_6$  phases at ambient pressure. The absence of an imaginary frequency in the phonon spectra indicates that the structures are dynamically stable at ambient pressure. (d) Calculated enthalpy as a function of pressure for  $\text{NaNH}_4\text{B}_6\text{C}_6$  relative to simple elemental substance, and the phase transition pressure is  $\sim 95$  GPa. (e) Inverse hull web of Na-N-H-B-C system at 0 K and ambient pressure. Compounds located in the positive range of the inverse-hull-energy axis indicates that they are metastable, while the others located in the negative range of the inverse-hull-energy axis are stable ones. We leave the  $\text{NaNH}_4\text{B}_6\text{C}_6$  compound and its hull reactants opaque, while we make all other phases partially transparent. Ground state structures of simple substances and other compounds were collected from the Inorganic Crystal Structure Database (ICSD) [1].



1.3  $\text{KNH}_4\text{B}_6\text{C}_6$ 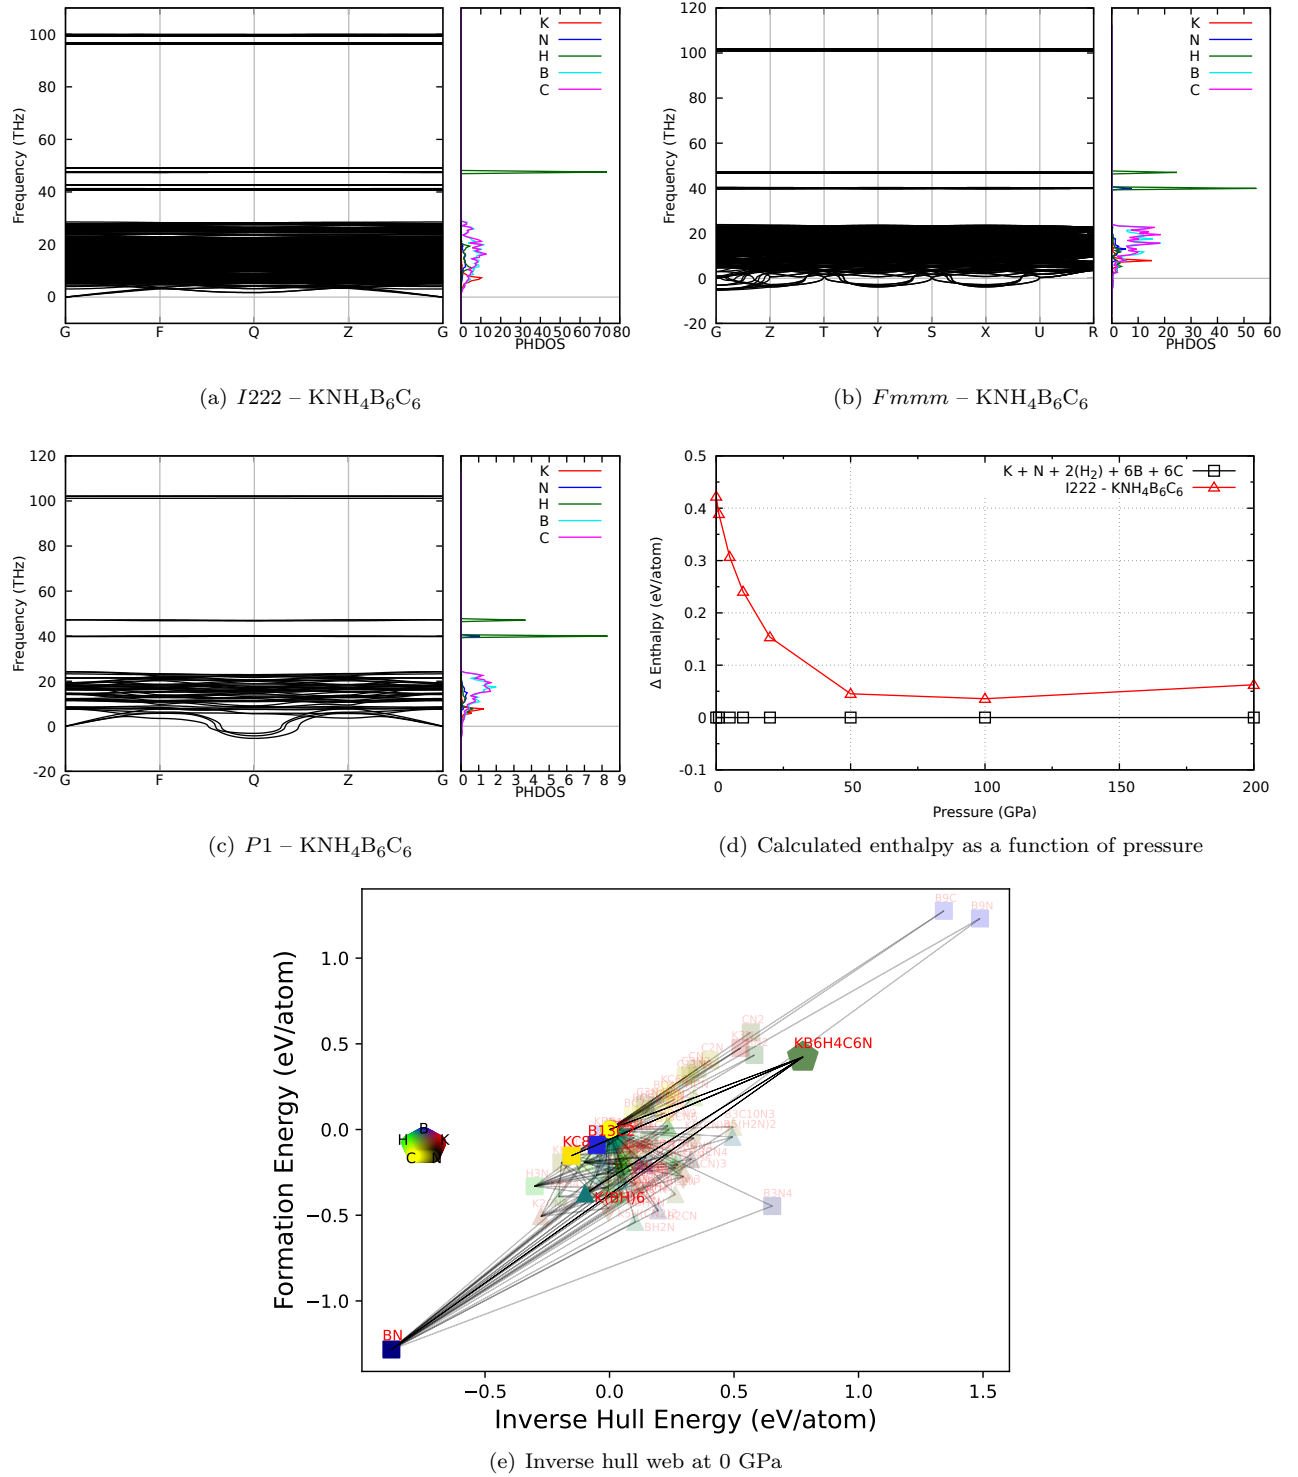

FIG. S5. (a-c) Phonon dispersion (left panel) and projected phonon densities of states (PHDOS, right panel) of different  $\text{KNH}_4\text{B}_6\text{C}_6$  phases at ambient pressure. The absence of an imaginary frequency in the phonon spectra indicates that the structures are dynamically stable at ambient pressure. (d) Calculated enthalpy as a function of pressure for  $\text{KNH}_4\text{B}_6\text{C}_6$  relative to simple elemental substance. (e) Inverse hull web of K-N-H-B-C system at 0 K and ambient pressure. Compounds located in the positive range of the inverse-hull-energy axis indicates that they are metastable, while the others located in the negative range of the inverse-hull-energy axis are stable ones. We leave the  $\text{KNH}_4\text{B}_6\text{C}_6$  compound and its hull reactants opaque, while we make all other phases partially transparent. Ground state structures of simple substances and other compounds were collected from the Inorganic Crystal Structure Database (ICSD) [1].

### 1.4 $\text{CaNH}_4\text{B}_6\text{C}_6$

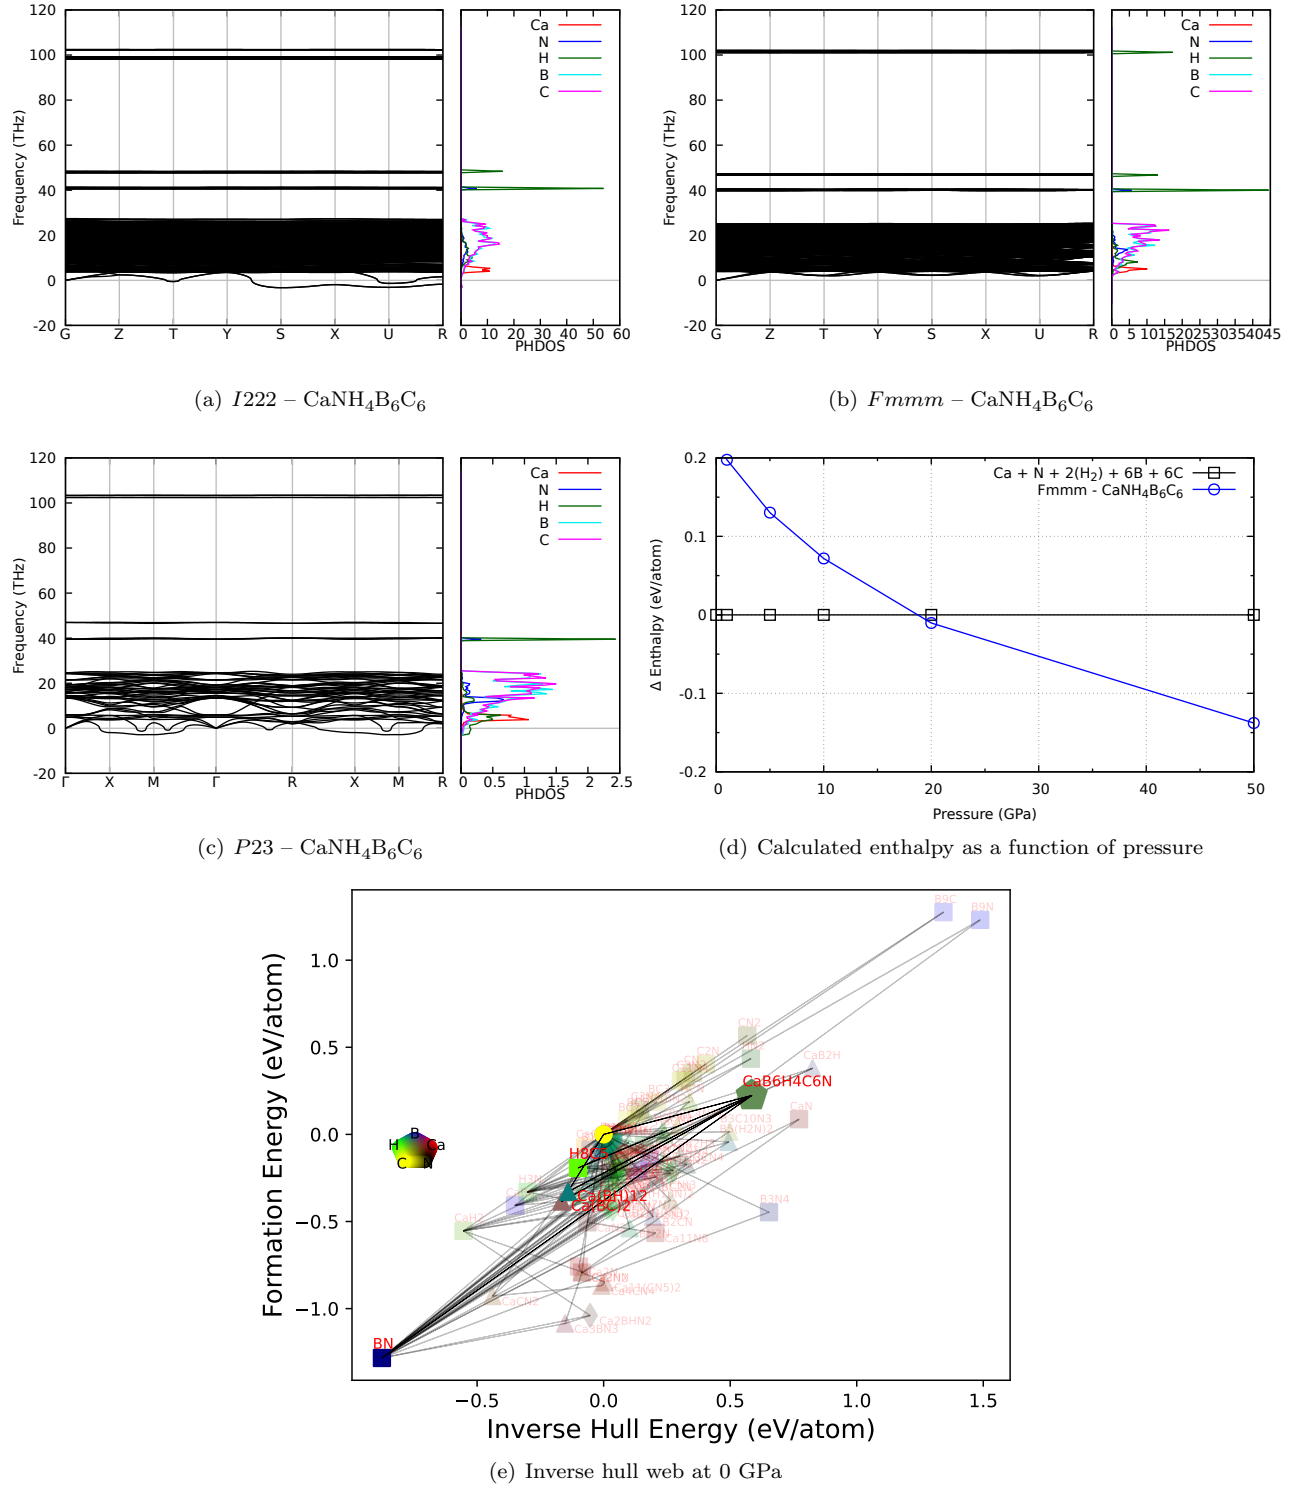

FIG. S6. (a–c) Phonon dispersion (left panel) and projected phonon densities of states (PHDOS, right panel) of different  $\text{CaNH}_4\text{B}_6\text{C}_6$  phases at ambient pressure. The absence of an imaginary frequency in the phonon spectra indicates that the structures are dynamically stable at ambient pressure. (d) Calculated enthalpy as a function of pressure for  $\text{CaNH}_4\text{B}_6\text{C}_6$  relative to simple elemental substance, and the phase transition pressure is  $\sim 18.7$  GPa. (e) Inverse hull web of Ca-N-H-B-C system at 0 K and ambient pressure. Compounds located in the positive range of the inverse-hull-energy axis indicates that they are metastable, while the others located in the negative range of the inverse-hull-energy axis are stable ones. We leave the  $\text{CaNH}_4\text{B}_6\text{C}_6$  compound and its hull reactants opaque, while we make all other phases partially transparent. Ground state structures of simple substances and other compounds were collected from the Inorganic Crystal Structure Database (ICSD) [1].

# 1.5 YNH<sub>4</sub>B<sub>6</sub>C<sub>6</sub>

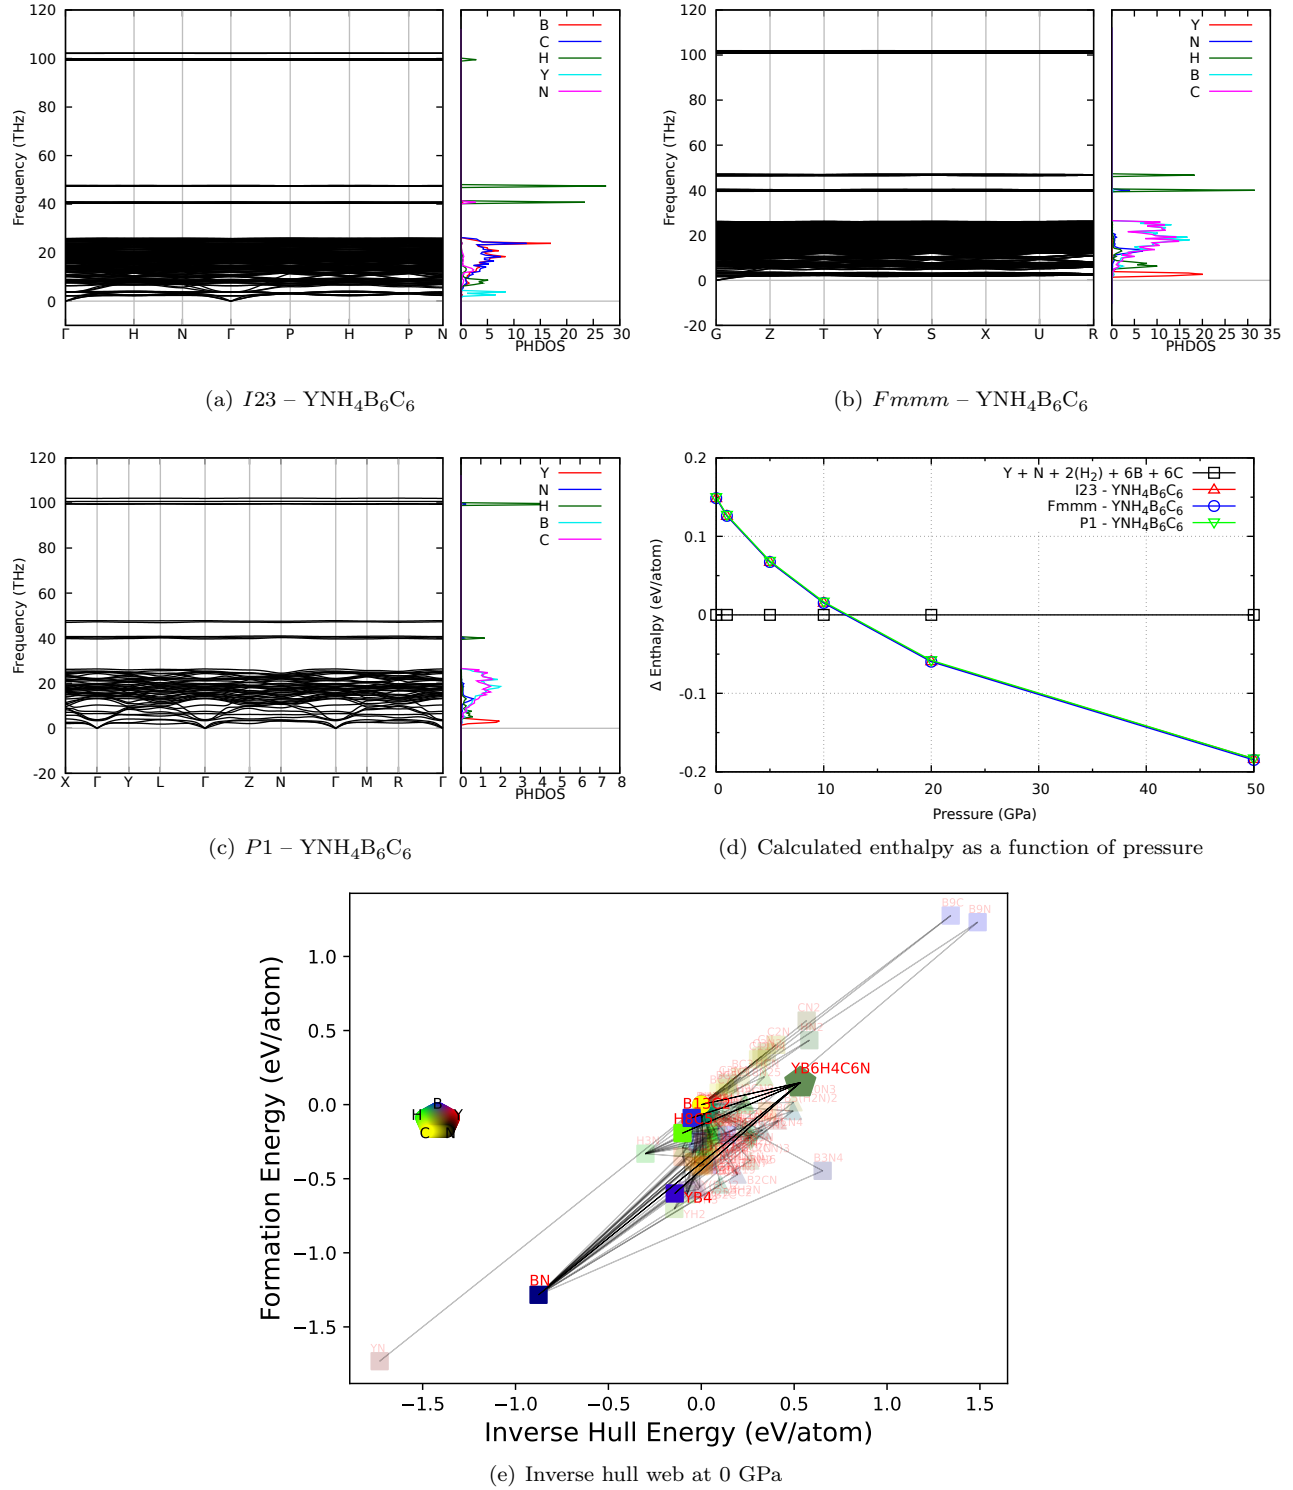

FIG. S7. (a–c) Phonon dispersion (left panel) and projected phonon densities of states (PHDOS, right panel) of different YNH<sub>4</sub>B<sub>6</sub>C<sub>6</sub> phases at ambient pressure. The absence of an imaginary frequency in the phonon spectra indicates that the structures are dynamically stable at ambient pressure. (d) Calculated enthalpy as a function of pressure for YNH<sub>4</sub>B<sub>6</sub>C<sub>6</sub> relative to simple elemental substance, and the phase transition pressure is  $\sim 12.1$  GPa. (e) Inverse hull web of Y-N-H-B-C system at 0 K and ambient pressure. Compounds located in the positive range of the inverse-hull-energy axis indicates that they are metastable, while the others located in the negative range of the inverse-hull-energy axis are stable. We leave the YNH<sub>4</sub>B<sub>6</sub>C<sub>6</sub> compound and its hull reactants opaque, while we make all other phases partially transparent. Ground state structures of simple substances and other compounds were collected from the Inorganic Crystal Structure Database (ICSD) [1].

### 1.6 $\text{PbNH}_4\text{B}_6\text{C}_6$

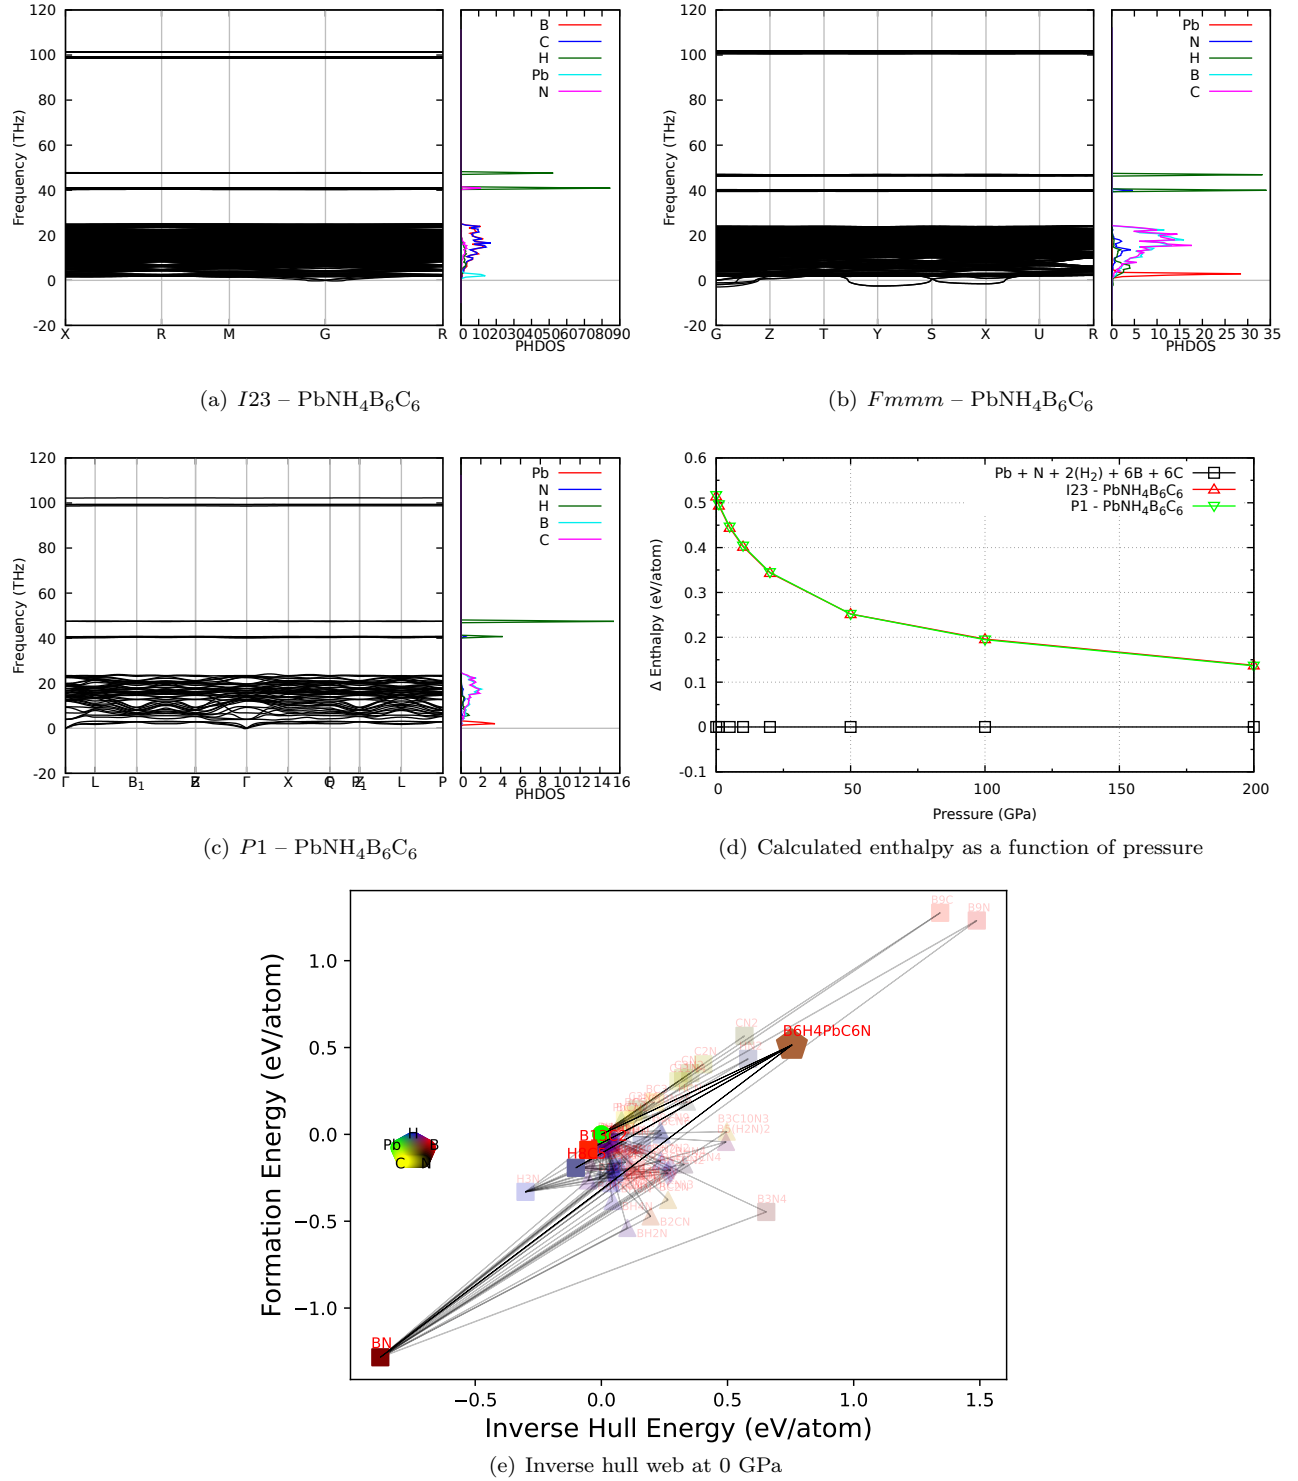

FIG. S8. (a–c) Phonon dispersion (left panel) and projected phonon densities of states (PHDOS, right panel) of different  $\text{PbNH}_4\text{B}_6\text{C}_6$  phases at ambient pressure. The absence of an imaginary frequency in the phonon spectra indicates that the structures are dynamically stable at ambient pressure. (d) Calculated enthalpy as a function of pressure for  $\text{PbNH}_4\text{B}_6\text{C}_6$  relative to simple elemental substance. (e) Inverse hull web of Pb-N-H-B-C system at 0 K and ambient pressure. Compounds located in the positive range of the inverse-hull-energy axis indicates that they are metastable, while the others located in the negative range of the inverse-hull-energy axis are stable ones. We leave the  $\text{PbNH}_4\text{B}_6\text{C}_6$  compound and its hull reactants opaque, while we make all other phases partially transparent. Ground state structures of simple substances and other compounds were collected from the Inorganic Crystal Structure Database (ICSD) [1].

### 1.7 $\text{LaNH}_4\text{B}_6\text{C}_6$

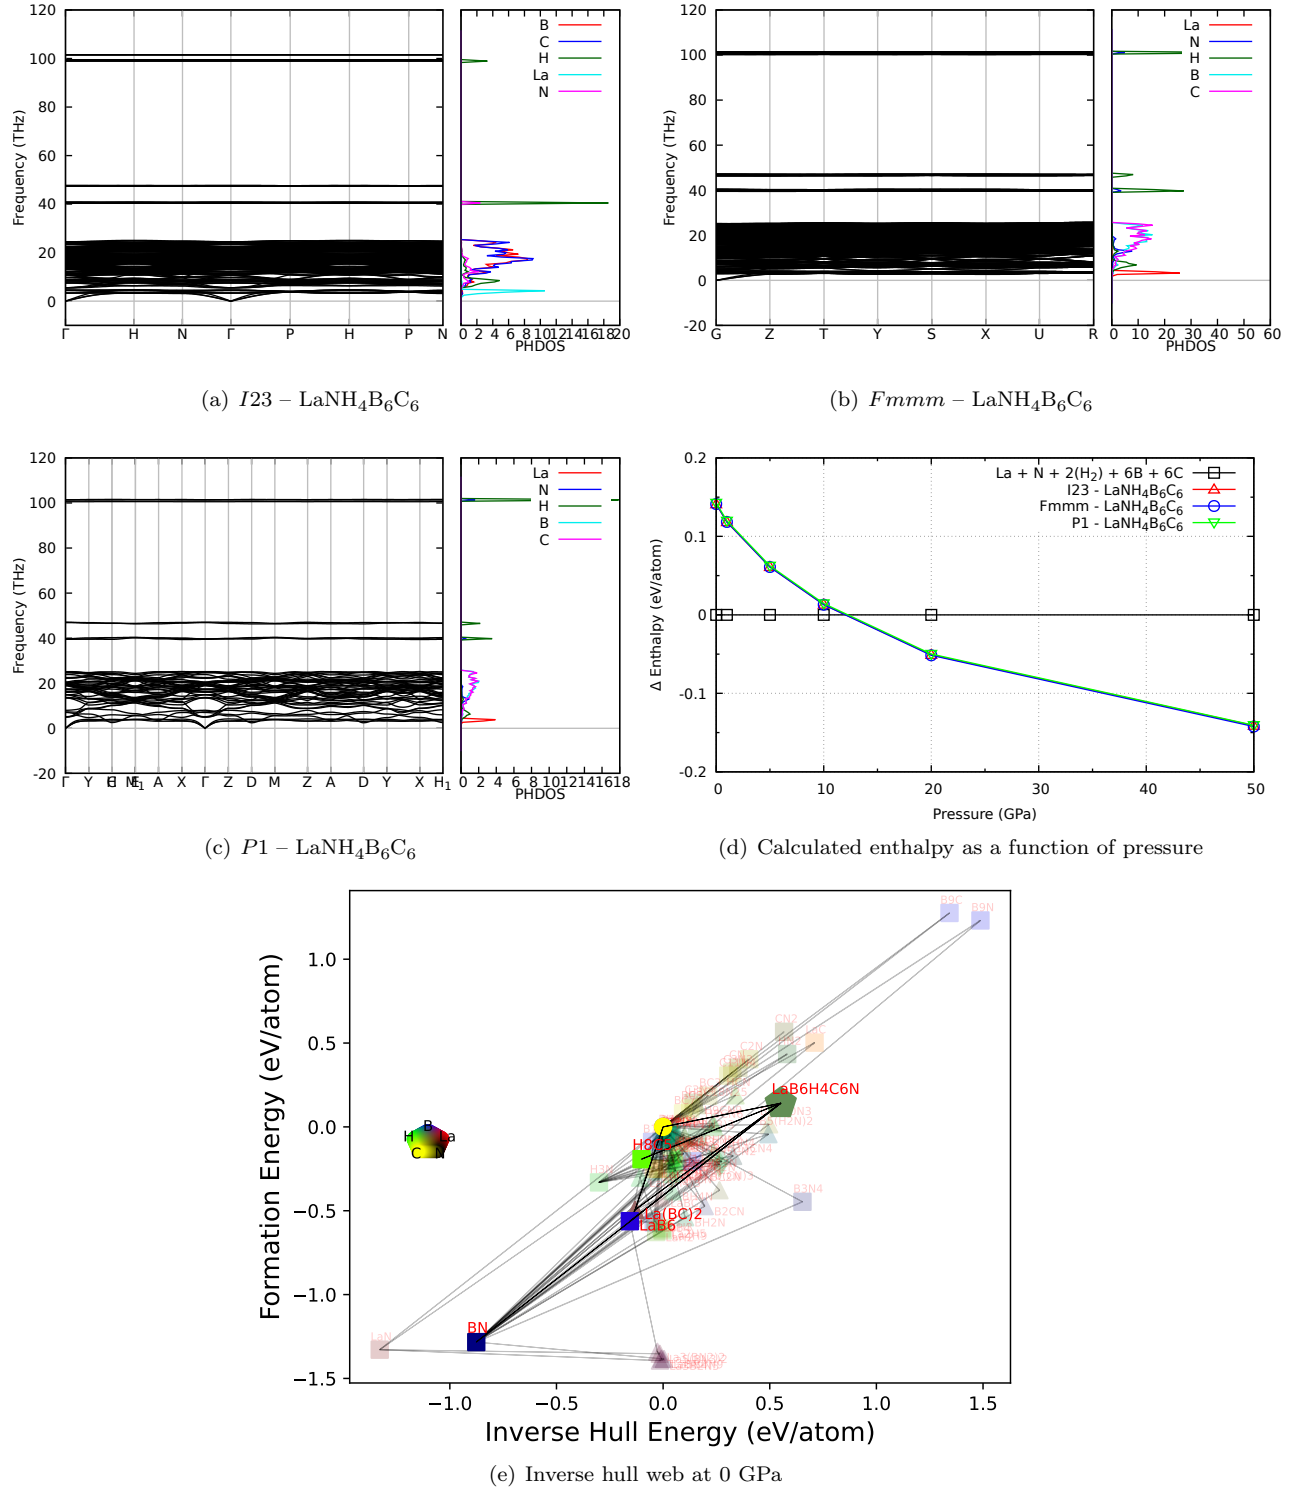

FIG. S9. (a–c) Phonon dispersion (left panel) and projected phonon densities of states (PHDOS, right panel) of different  $\text{LaNH}_4\text{B}_6\text{C}_6$  phases at ambient pressure. The absence of an imaginary frequency in the phonon spectra indicates that the structures are dynamically stable at ambient pressure. (d) Calculated enthalpy as a function of pressure for  $\text{LaNH}_4\text{B}_6\text{C}_6$  relative to simple elemental substance, and the phase transition pressure is  $\sim 12.0$  GPa. (e) Inverse hull web of La-N-H-B-C system at 0 K and ambient pressure. Compounds located in the positive range of the inverse-hull-energy axis indicates that they are metastable, while the others located in the negative range of the inverse-hull-energy axis are stable ones. We leave the  $\text{LaNH}_4\text{B}_6\text{C}_6$  compound and its hull reactants opaque, while we make all other phases partially transparent. Ground state structures of simple substances and other compounds were collected from the Inorganic Crystal Structure Database (ICSD) [1].

### 1.8 $\text{PrNH}_4\text{B}_6\text{C}_6$

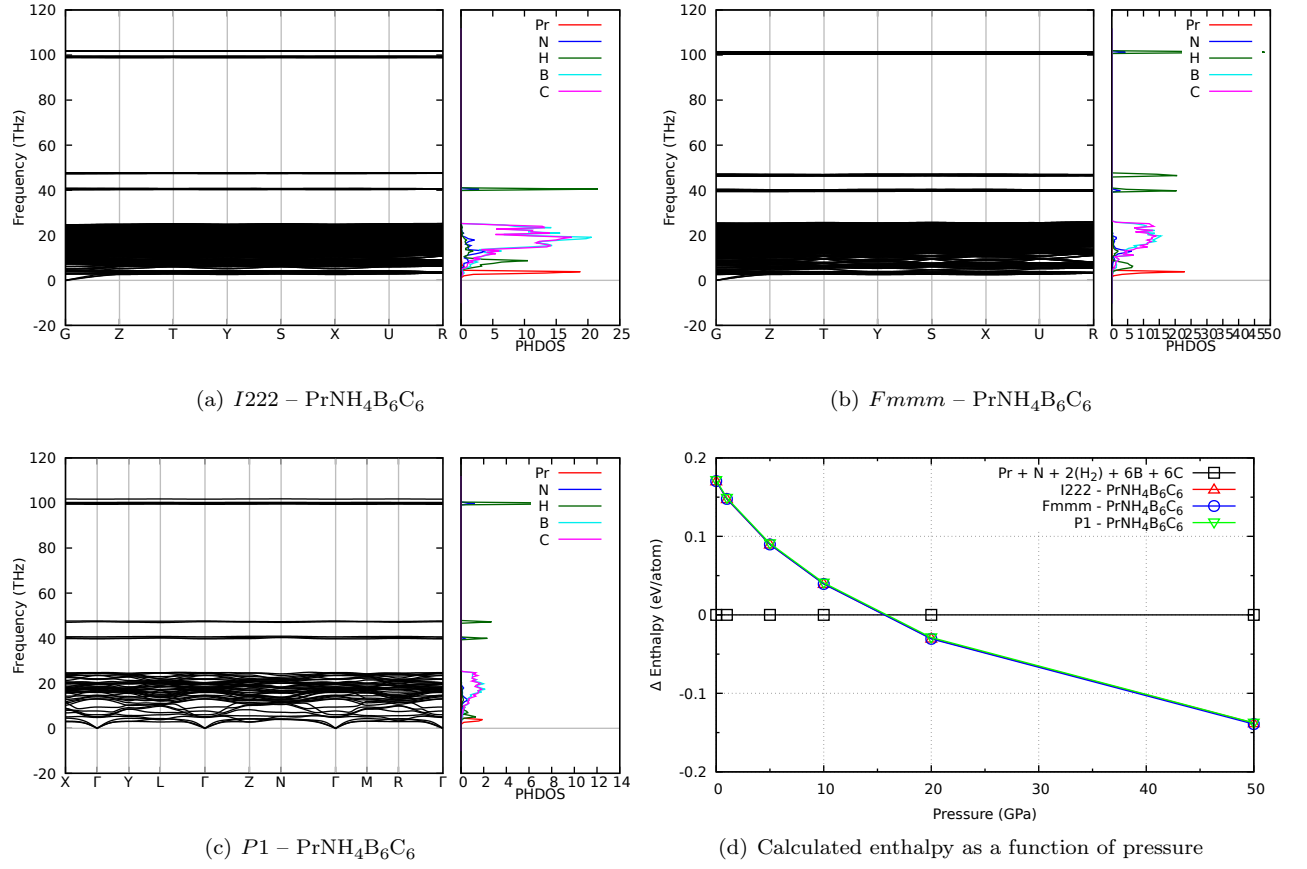

FIG. S10. (a–c) Phonon dispersion (left panel) and projected phonon densities of states (PHDOS, right panel) of different  $\text{PrNH}_4\text{B}_6\text{C}_6$  phases at ambient pressure. The absence of an imaginary frequency in the phonon spectra indicates that the structures are dynamically stable at ambient pressure. (d) Calculated enthalpy as a function of pressure for  $\text{PrNH}_4\text{B}_6\text{C}_6$  relative to simple elemental substance, and the phase transition pressure is  $\sim 15.7$  GPa. Ground state structures of simple substances were collected from the Inorganic Crystal Structure Database (ICSD) [1].

### 1.9 $\text{NdNH}_4\text{B}_6\text{C}_6$

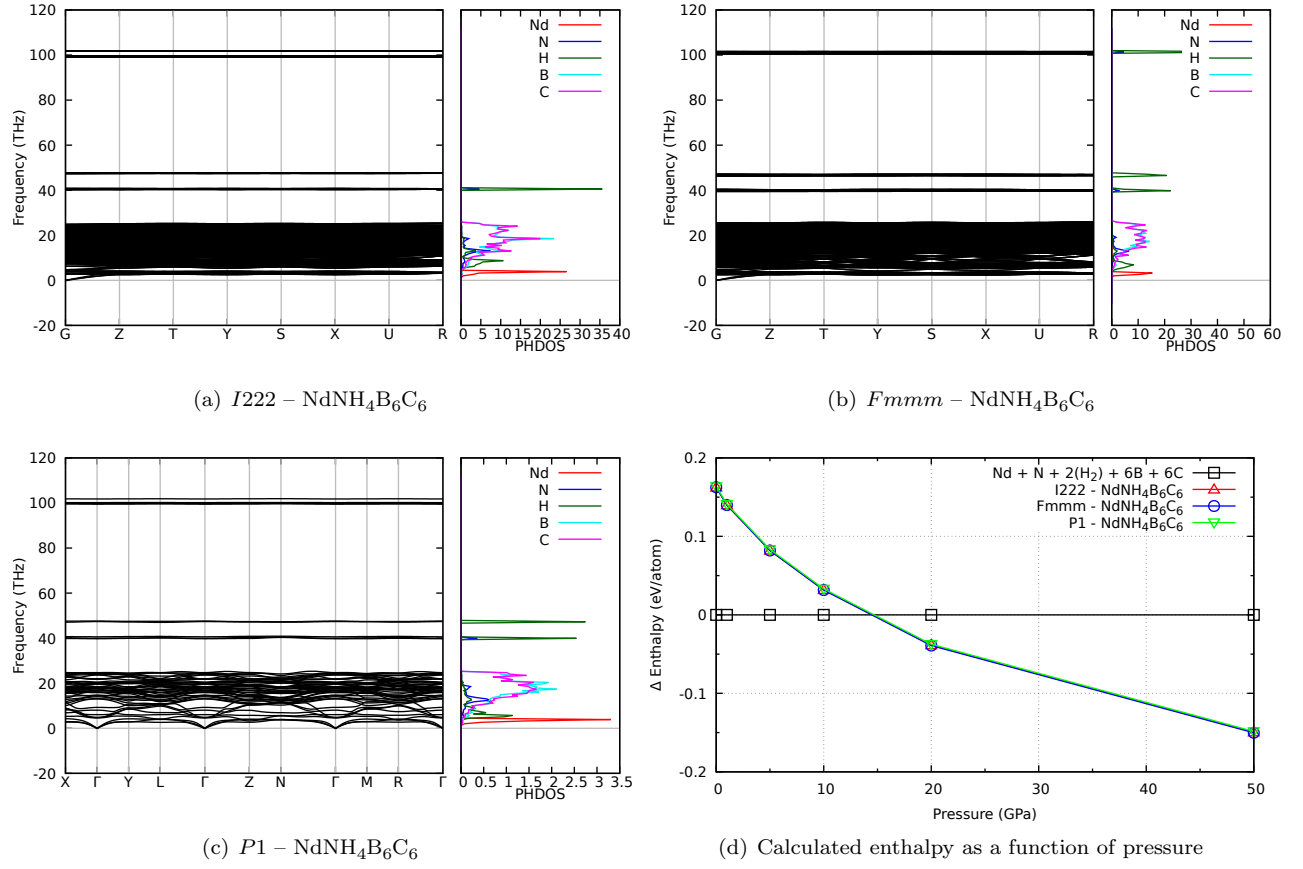

FIG. S11. (a–c) Phonon dispersion (left panel) and projected phonon densities of states (PHDOS, right panel) of different  $\text{NdNH}_4\text{B}_6\text{C}_6$  phases at ambient pressure. The absence of an imaginary frequency in the phonon spectra indicates that the structures are dynamically stable at ambient pressure. (d) Calculated enthalpy as a function of pressure for  $\text{NdNH}_4\text{B}_6\text{C}_6$  relative to simple elemental substance, and the phase transition pressure is  $\sim 14.6$  GPa. Ground state structures of simple substances were collected from the Inorganic Crystal Structure Database (ICSD) [1].

1.10  $\text{PmNH}_4\text{B}_6\text{C}_6$ 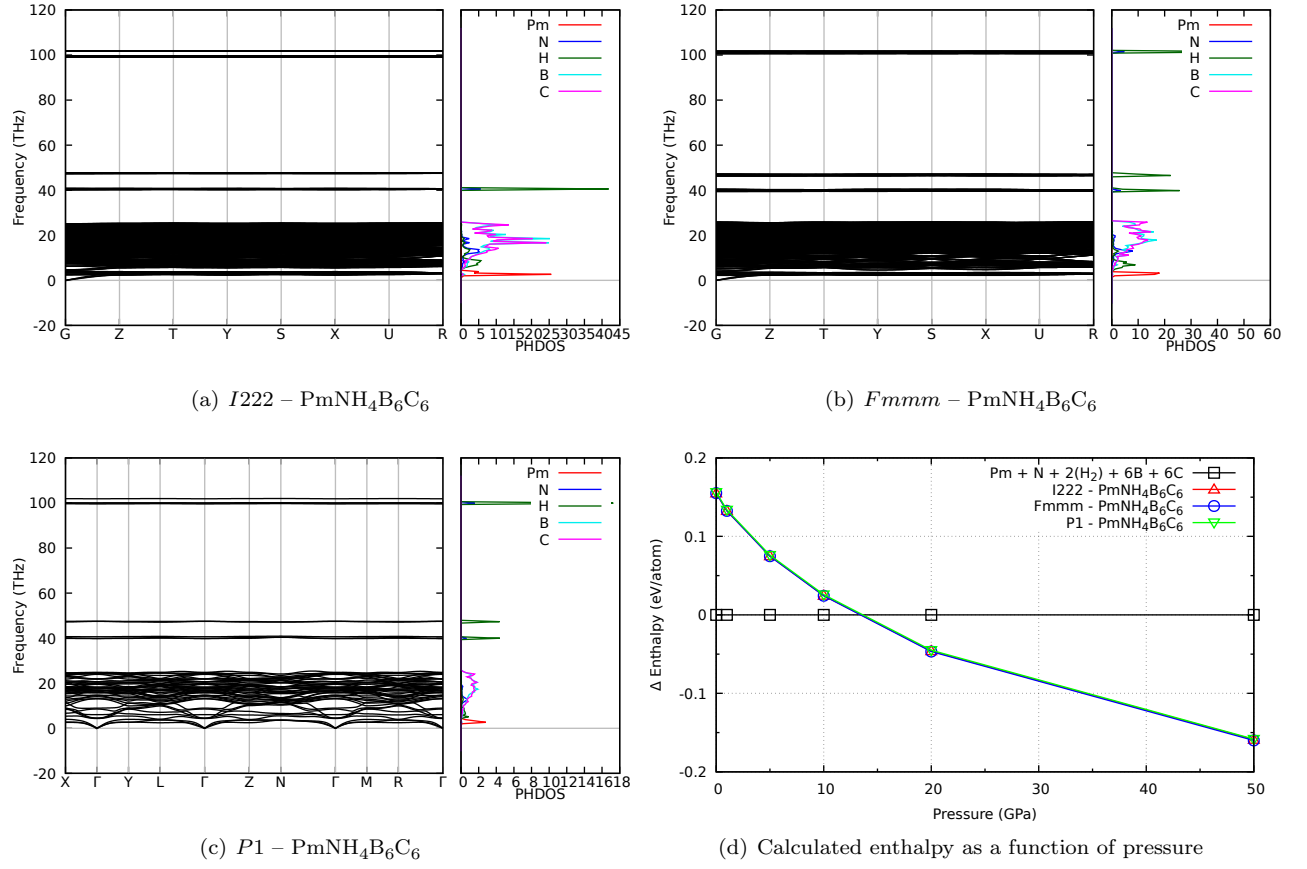

FIG. S12. (a–c) Phonon dispersion (left panel) and projected phonon densities of states (PHDOS, right panel) of different  $\text{PmNH}_4\text{B}_6\text{C}_6$  phases at ambient pressure. The absence of an imaginary frequency in the phonon spectra indicates that the structures are dynamically stable at ambient pressure. (d) Calculated enthalpy as a function of pressure for  $\text{PmNH}_4\text{B}_6\text{C}_6$  relative to simple elemental substance, and the phase transition pressure is  $\sim 13.6$  GPa. Ground state structures of simple substances were collected from the Inorganic Crystal Structure Database (ICSD) [1].



1.11  $\text{SmNH}_4\text{B}_6\text{C}_6$ 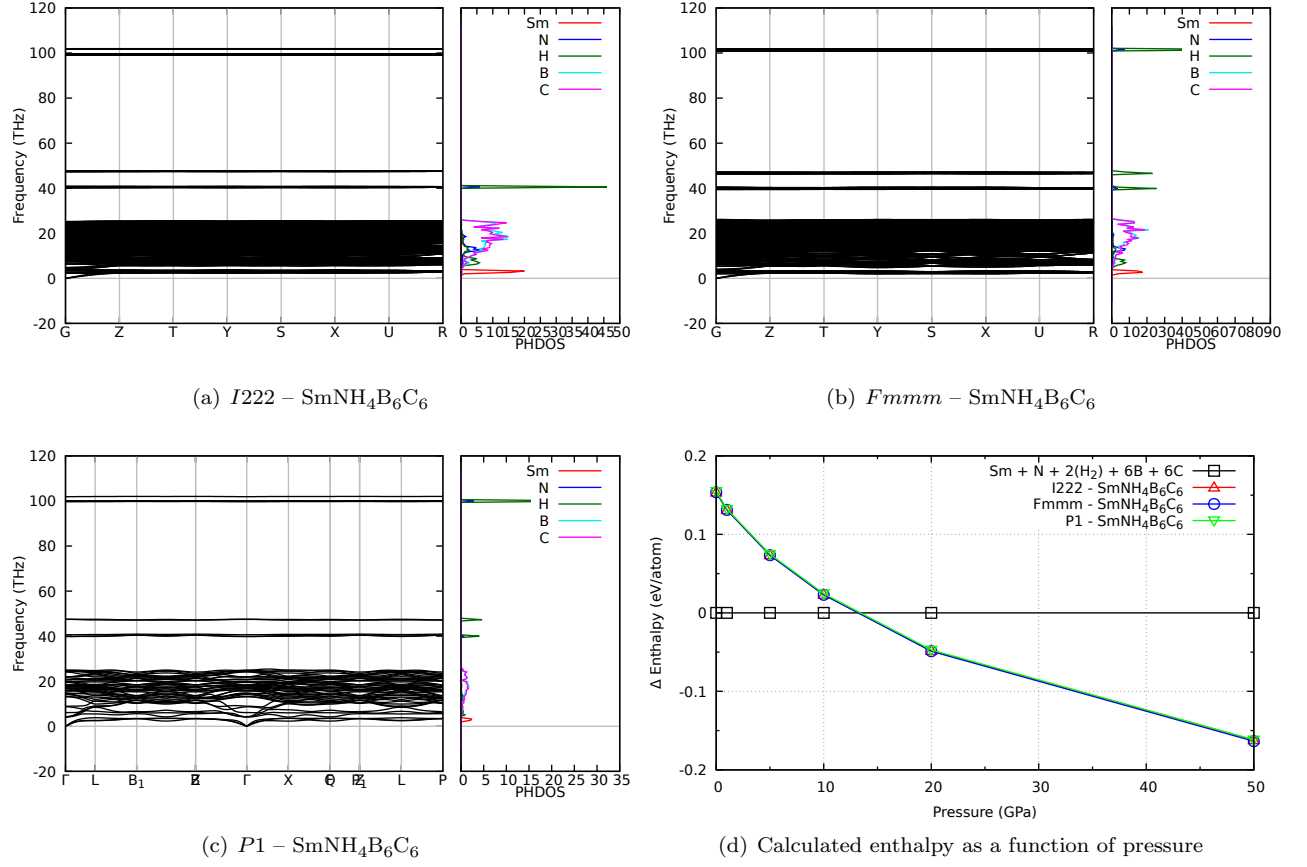

FIG. S13. (a–c) Phonon dispersion (left panel) and projected phonon densities of states (PHDOS, right panel) of different  $\text{SmNH}_4\text{B}_6\text{C}_6$  phases at ambient pressure. The absence of an imaginary frequency in the phonon spectra indicates that the structures are dynamically stable at ambient pressure. (d) Calculated enthalpy as a function of pressure for  $\text{SmNH}_4\text{B}_6\text{C}_6$  relative to simple elemental substance, and the phase transition pressure is  $\sim 13.3$  GPa. Ground state structures of simple substances were collected from the Inorganic Crystal Structure Database (ICSD) [1].

1.12  $\text{EuNH}_4\text{B}_6\text{C}_6$ 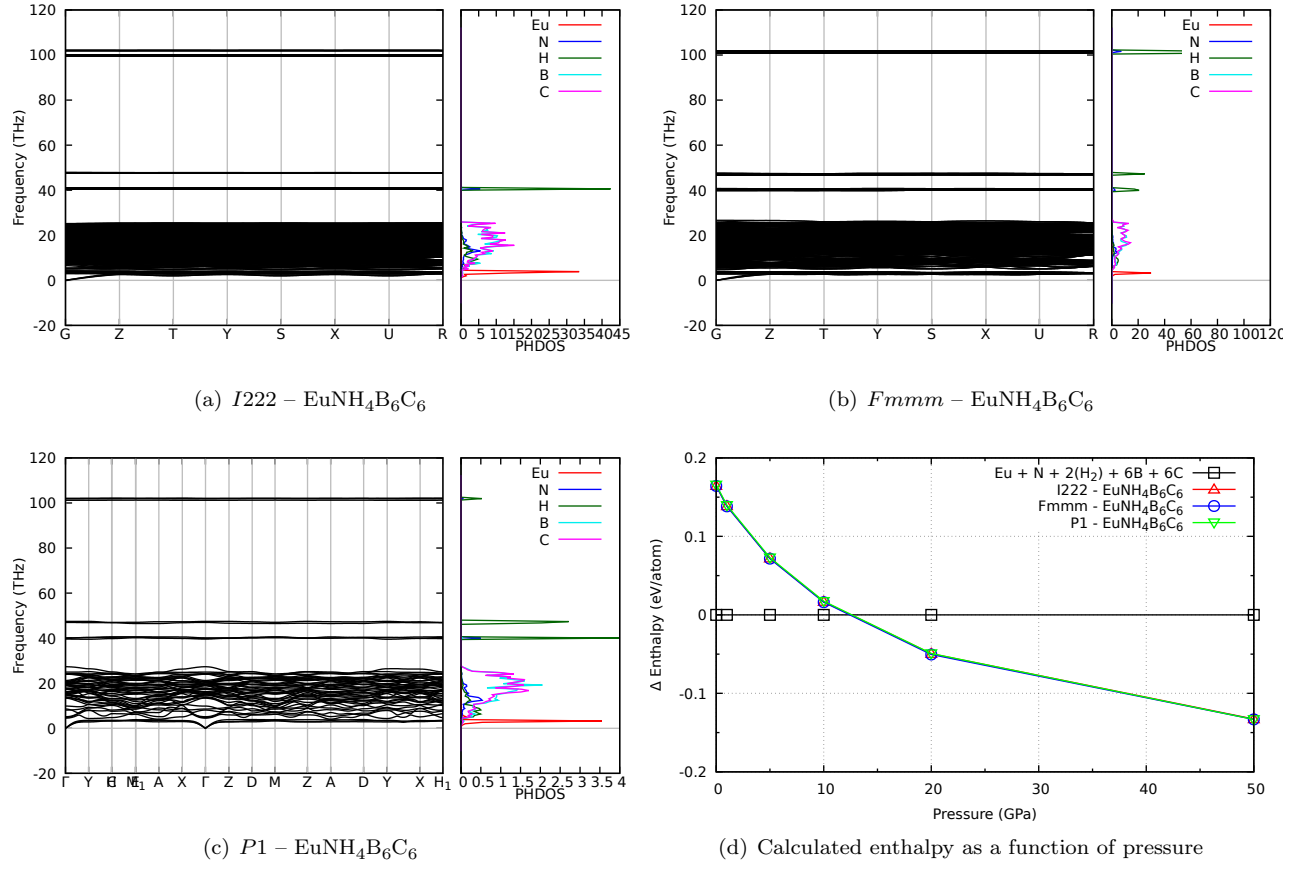

FIG. S14. (a–c) Phonon dispersion (left panel) and projected phonon densities of states (PHDOS, right panel) of different  $\text{EuNH}_4\text{B}_6\text{C}_6$  phases at ambient pressure. The absence of an imaginary frequency in the phonon spectra indicates that the structures are dynamically stable at ambient pressure. (d) Calculated enthalpy as a function of pressure for  $\text{EuNH}_4\text{B}_6\text{C}_6$  relative to simple elemental substance, and the phase transition pressure is  $\sim 12.5$  GPa. Ground state structures of simple substances were collected from the Inorganic Crystal Structure Database (ICSD) [1].

1.13  $\text{GdNH}_4\text{B}_6\text{C}_6$ 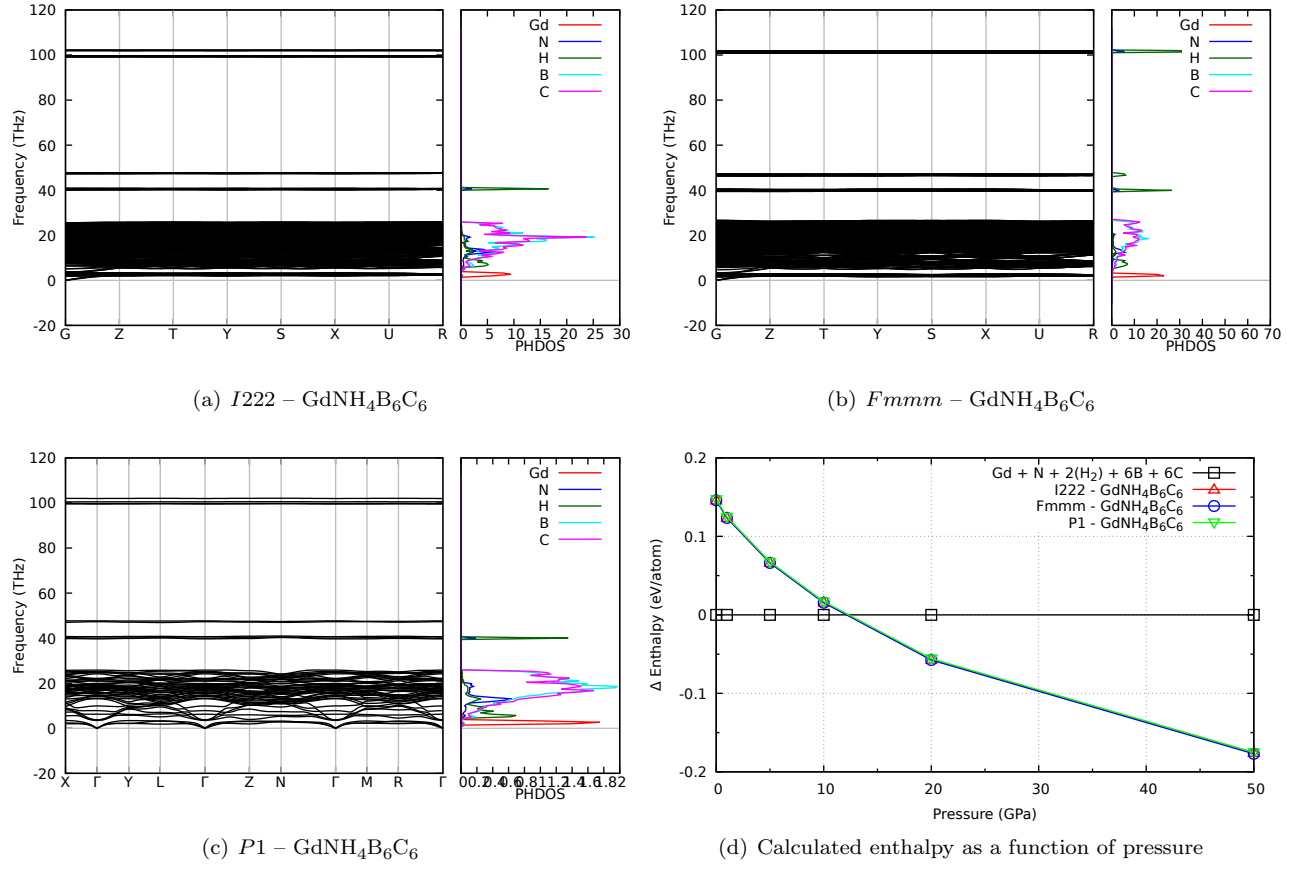

FIG. S15. (a–c) Phonon dispersion (left panel) and projected phonon densities of states (PHDOS, right panel) of different  $\text{GdNH}_4\text{B}_6\text{C}_6$  phases at ambient pressure. The absence of an imaginary frequency in the phonon spectra indicates that the structures are dynamically stable at ambient pressure. (d) Calculated enthalpy as a function of pressure for  $\text{GdNH}_4\text{B}_6\text{C}_6$  relative to simple elemental substance, and the phase transition pressure is  $\sim 12.3$  GPa. Ground state structures of simple substances were collected from the Inorganic Crystal Structure Database (ICSD) [1].

1.14  $\text{TbNH}_4\text{B}_6\text{C}_6$ 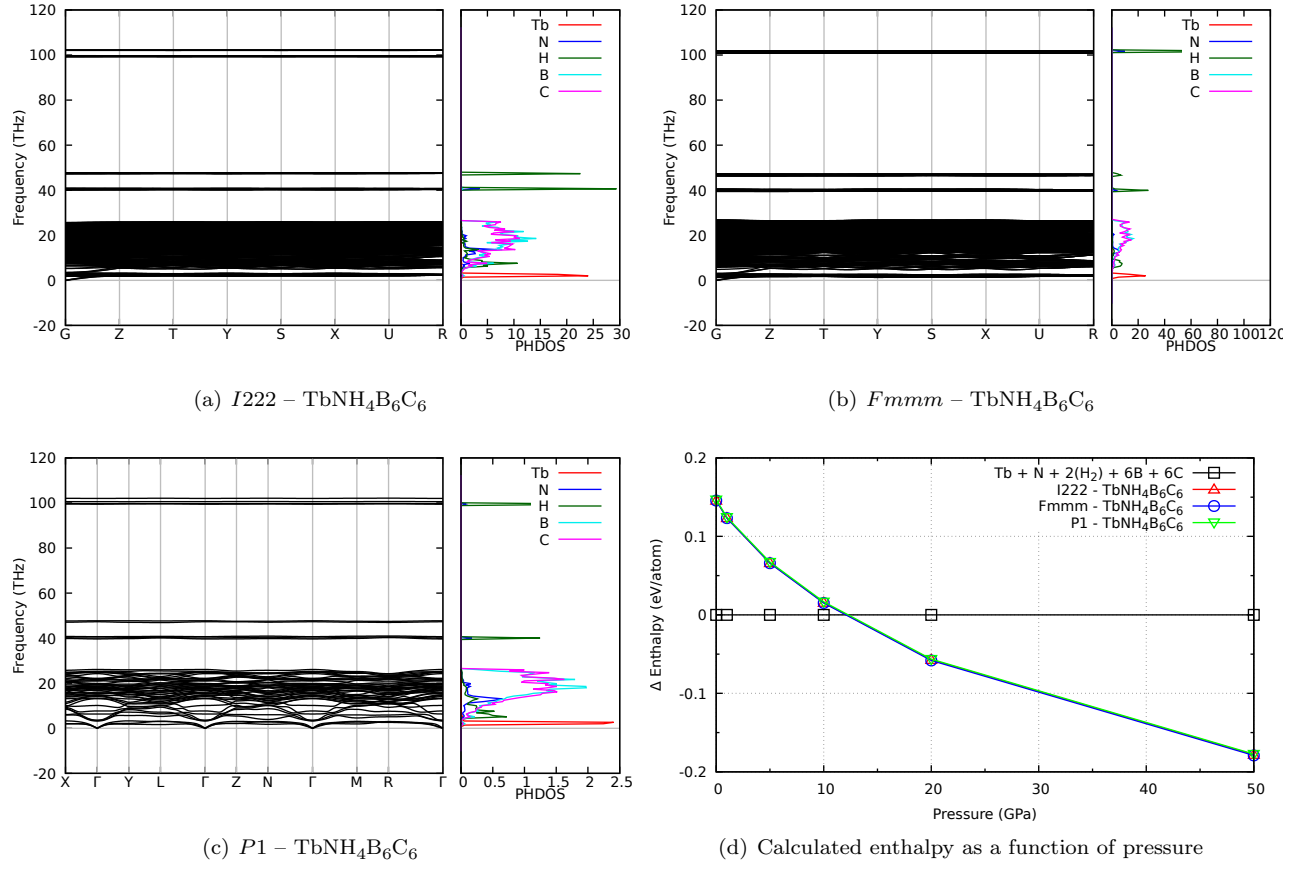

FIG. S16. (a–c) Phonon dispersion (left panel) and projected phonon densities of states (PHDOS, right panel) of different  $\text{TbNH}_4\text{B}_6\text{C}_6$  phases at ambient pressure. The absence of an imaginary frequency in the phonon spectra indicates that the structures are dynamically stable at ambient pressure. (d) Calculated enthalpy as a function of pressure for  $\text{TbNH}_4\text{B}_6\text{C}_6$  relative to simple elemental substance, and the phase transition pressure is  $\sim 12.2$  GPa. Ground state structures of simple substances were collected from the Inorganic Crystal Structure Database (ICSD) [1].

1.15  $\text{DyNH}_4\text{B}_6\text{C}_6$ 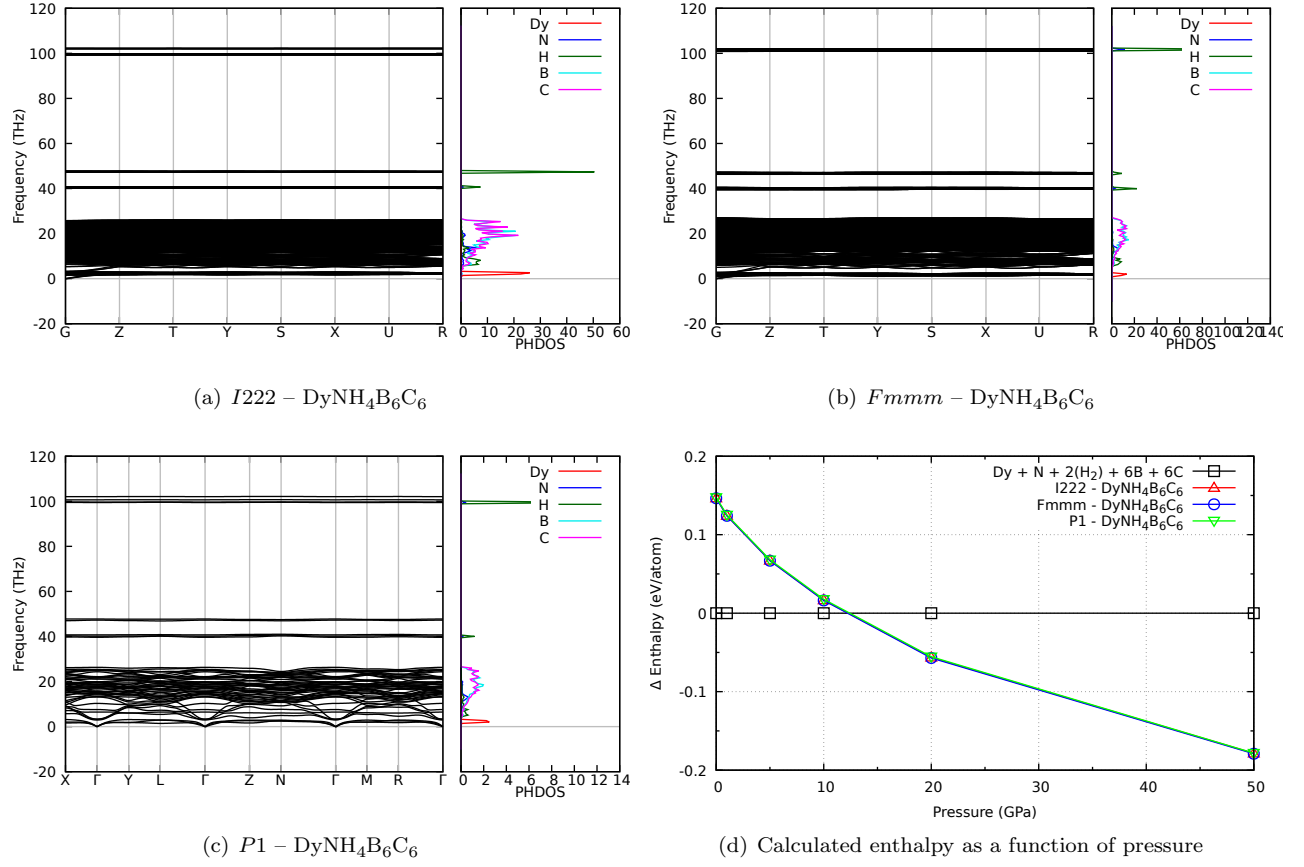

FIG. S17. (a–c) Phonon dispersion (left panel) and projected phonon densities of states (PHDOS, right panel) of different  $\text{DyNH}_4\text{B}_6\text{C}_6$  phases at ambient pressure. The absence of an imaginary frequency in the phonon spectra indicates that the structures are dynamically stable at ambient pressure. (d) Calculated enthalpy as a function of pressure for  $\text{DyNH}_4\text{B}_6\text{C}_6$  relative to simple elemental substance, and the phase transition pressure is  $\sim 12.3$  GPa. Ground state structures of simple substances were collected from the Inorganic Crystal Structure Database (ICSD) [1].

1.16  $\text{HoNH}_4\text{B}_6\text{C}_6$ 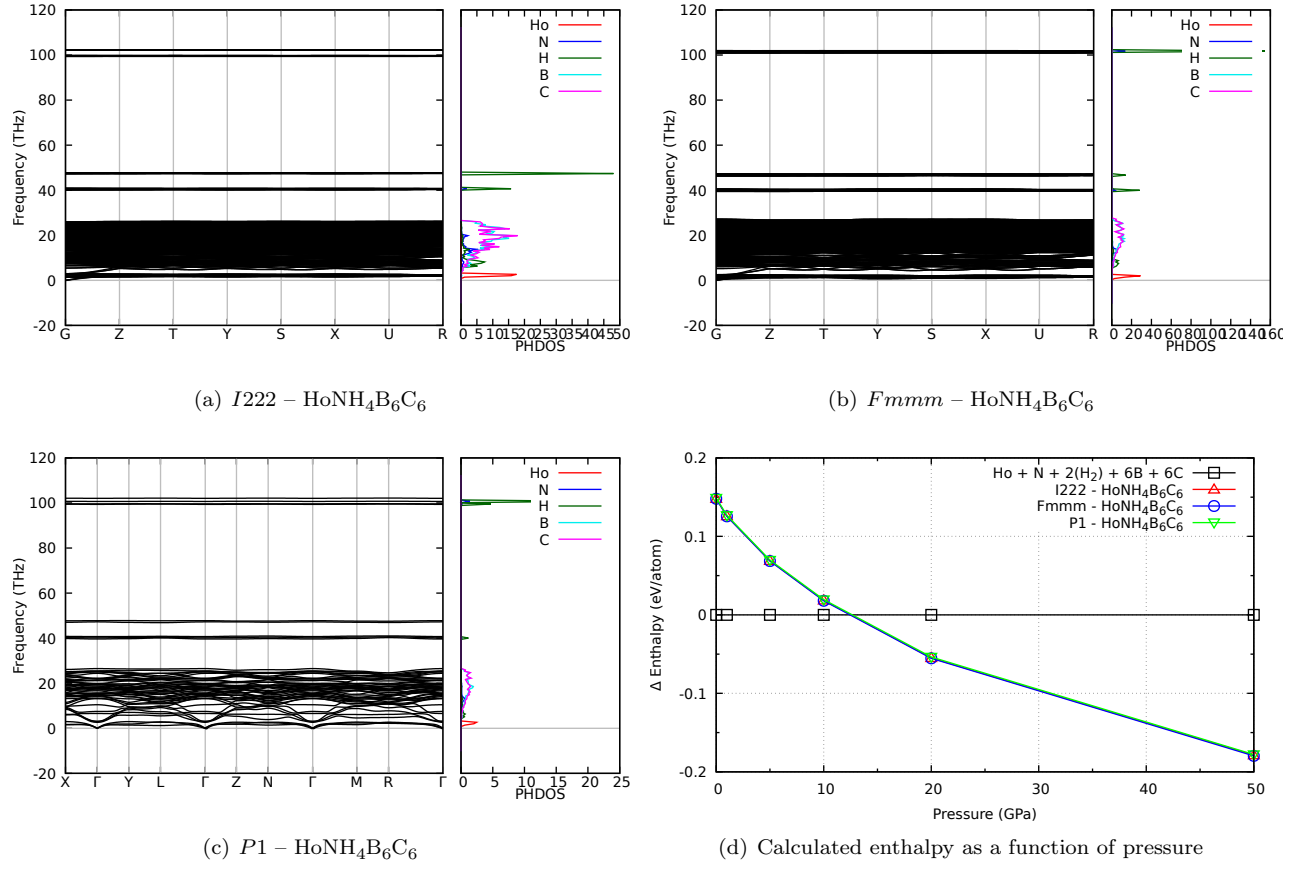

FIG. S18. (a–c) Phonon dispersion (left panel) and projected phonon densities of states (PHDOS, right panel) of different  $\text{HoNH}_4\text{B}_6\text{C}_6$  phases at ambient pressure. The absence of an imaginary frequency in the phonon spectra indicates that the structures are dynamically stable at ambient pressure. (d) Calculated enthalpy as a function of pressure for  $\text{HoNH}_4\text{B}_6\text{C}_6$  relative to simple elemental substance, and the phase transition pressure is  $\sim 12.5$  GPa. Ground state structures of simple substances were collected from the Inorganic Crystal Structure Database (ICSD) [1].

1.17  $\text{ErNH}_4\text{B}_6\text{C}_6$ 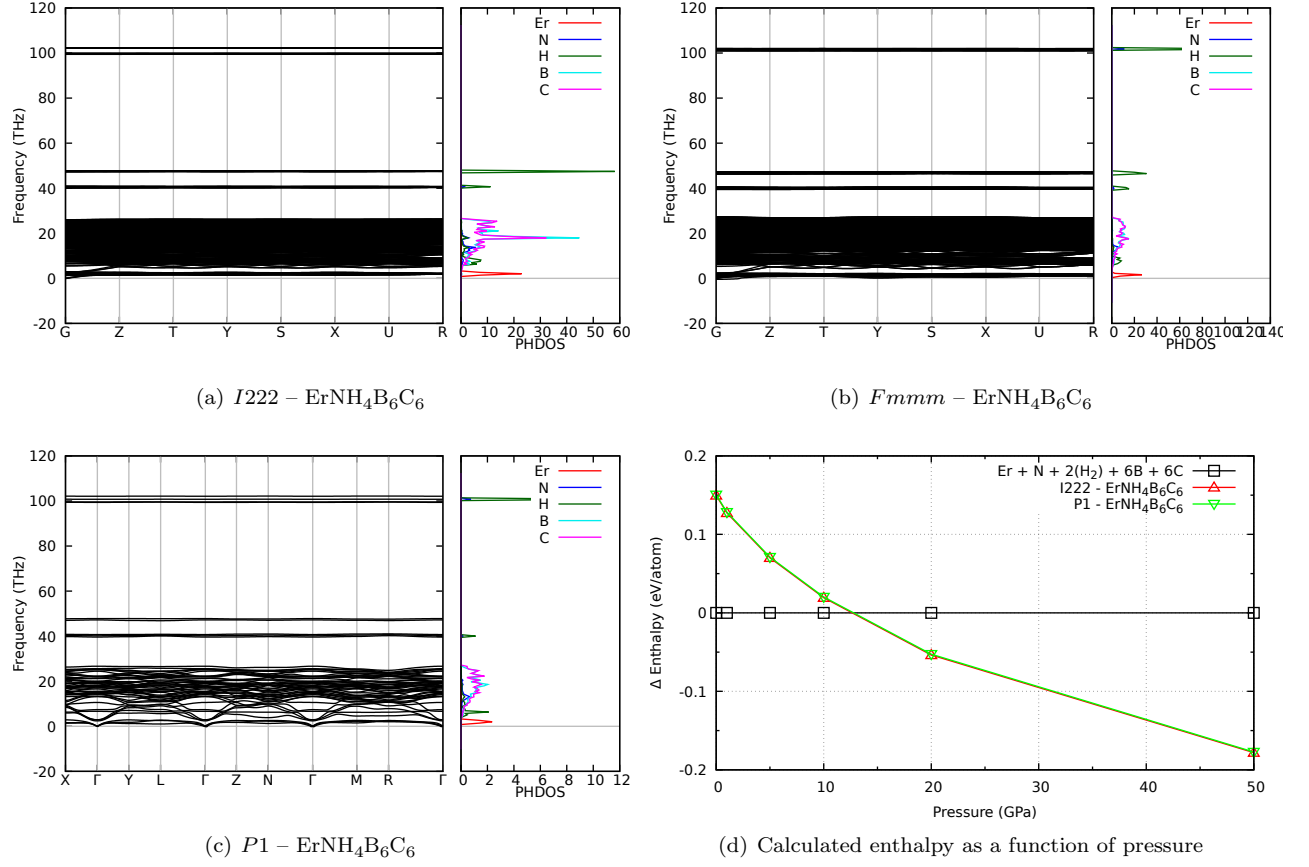

FIG. S19. (a–c) Phonon dispersion (left panel) and projected phonon densities of states (PHDOS, right panel) of different  $\text{ErNH}_4\text{B}_6\text{C}_6$  phases at ambient pressure. The absence of an imaginary frequency in the phonon spectra indicates that the structures are dynamically stable at ambient pressure. (d) Calculated enthalpy as a function of pressure for  $\text{ErNH}_4\text{B}_6\text{C}_6$  relative to simple elemental substance, and the phase transition pressure is  $\sim 12.7$  GPa. Ground state structures of simple substances were collected from the Inorganic Crystal Structure Database (ICSD) [1].

1.18  $\text{TmNH}_4\text{B}_6\text{C}_6$ 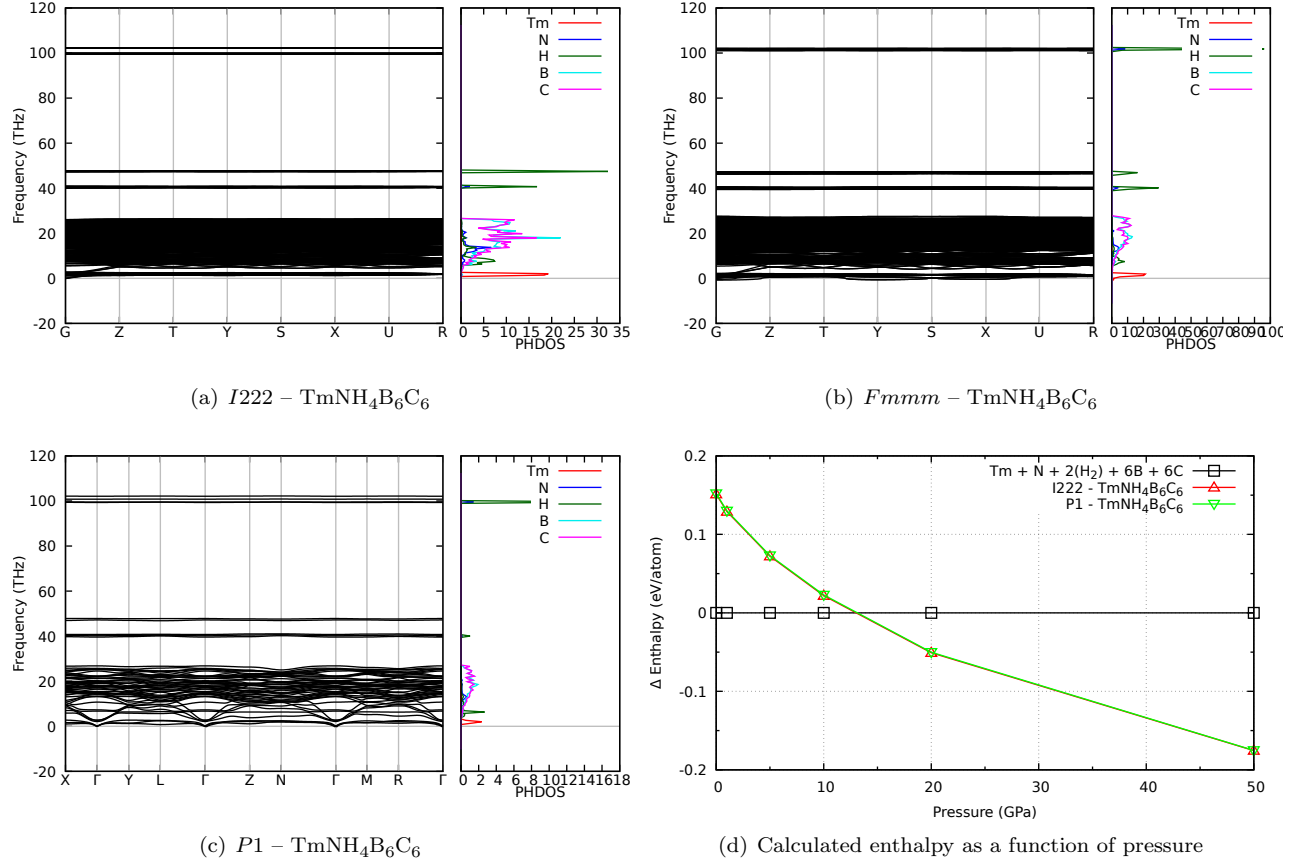

FIG. S20. (a–c) Phonon dispersion (left panel) and projected phonon densities of states (PHDOS, right panel) of different  $\text{TmNH}_4\text{B}_6\text{C}_6$  phases at ambient pressure. The absence of an imaginary frequency in the phonon spectra indicates that the structures are dynamically stable at ambient pressure. (d) Calculated enthalpy as a function of pressure for  $\text{TmNH}_4\text{B}_6\text{C}_6$  relative to simple elemental substance, and the phase transition pressure is  $\sim 13.0$  GPa. Ground state structures of simple substances were collected from the Inorganic Crystal Structure Database (ICSD) [1].



1.19  $\text{YbNH}_4\text{B}_6\text{C}_6$ 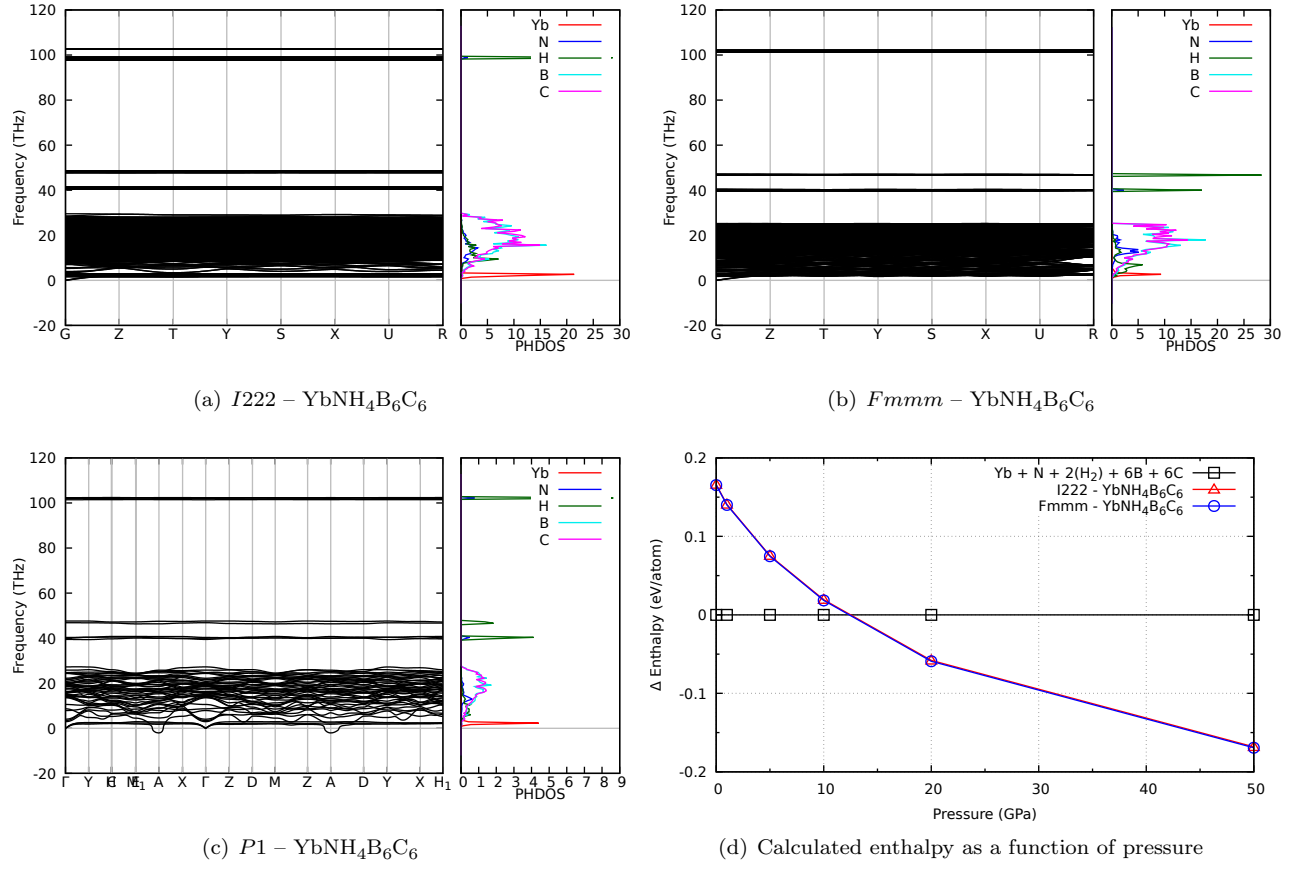

FIG. S21. (a–c) Phonon dispersion (left panel) and projected phonon densities of states (PHDOS, right panel) of different  $\text{YbNH}_4\text{B}_6\text{C}_6$  phases at ambient pressure. The absence of an imaginary frequency in the phonon spectra indicates that the structures are dynamically stable at ambient pressure. (d) Calculated enthalpy as a function of pressure for  $\text{YbNH}_4\text{B}_6\text{C}_6$  relative to simple elemental substance, and the phase transition pressure is  $\sim 12.4$  GPa. Ground state structures of simple substances were collected from the Inorganic Crystal Structure Database (ICSD) [1].

1.20  $\text{LuNH}_4\text{B}_6\text{C}_6$ 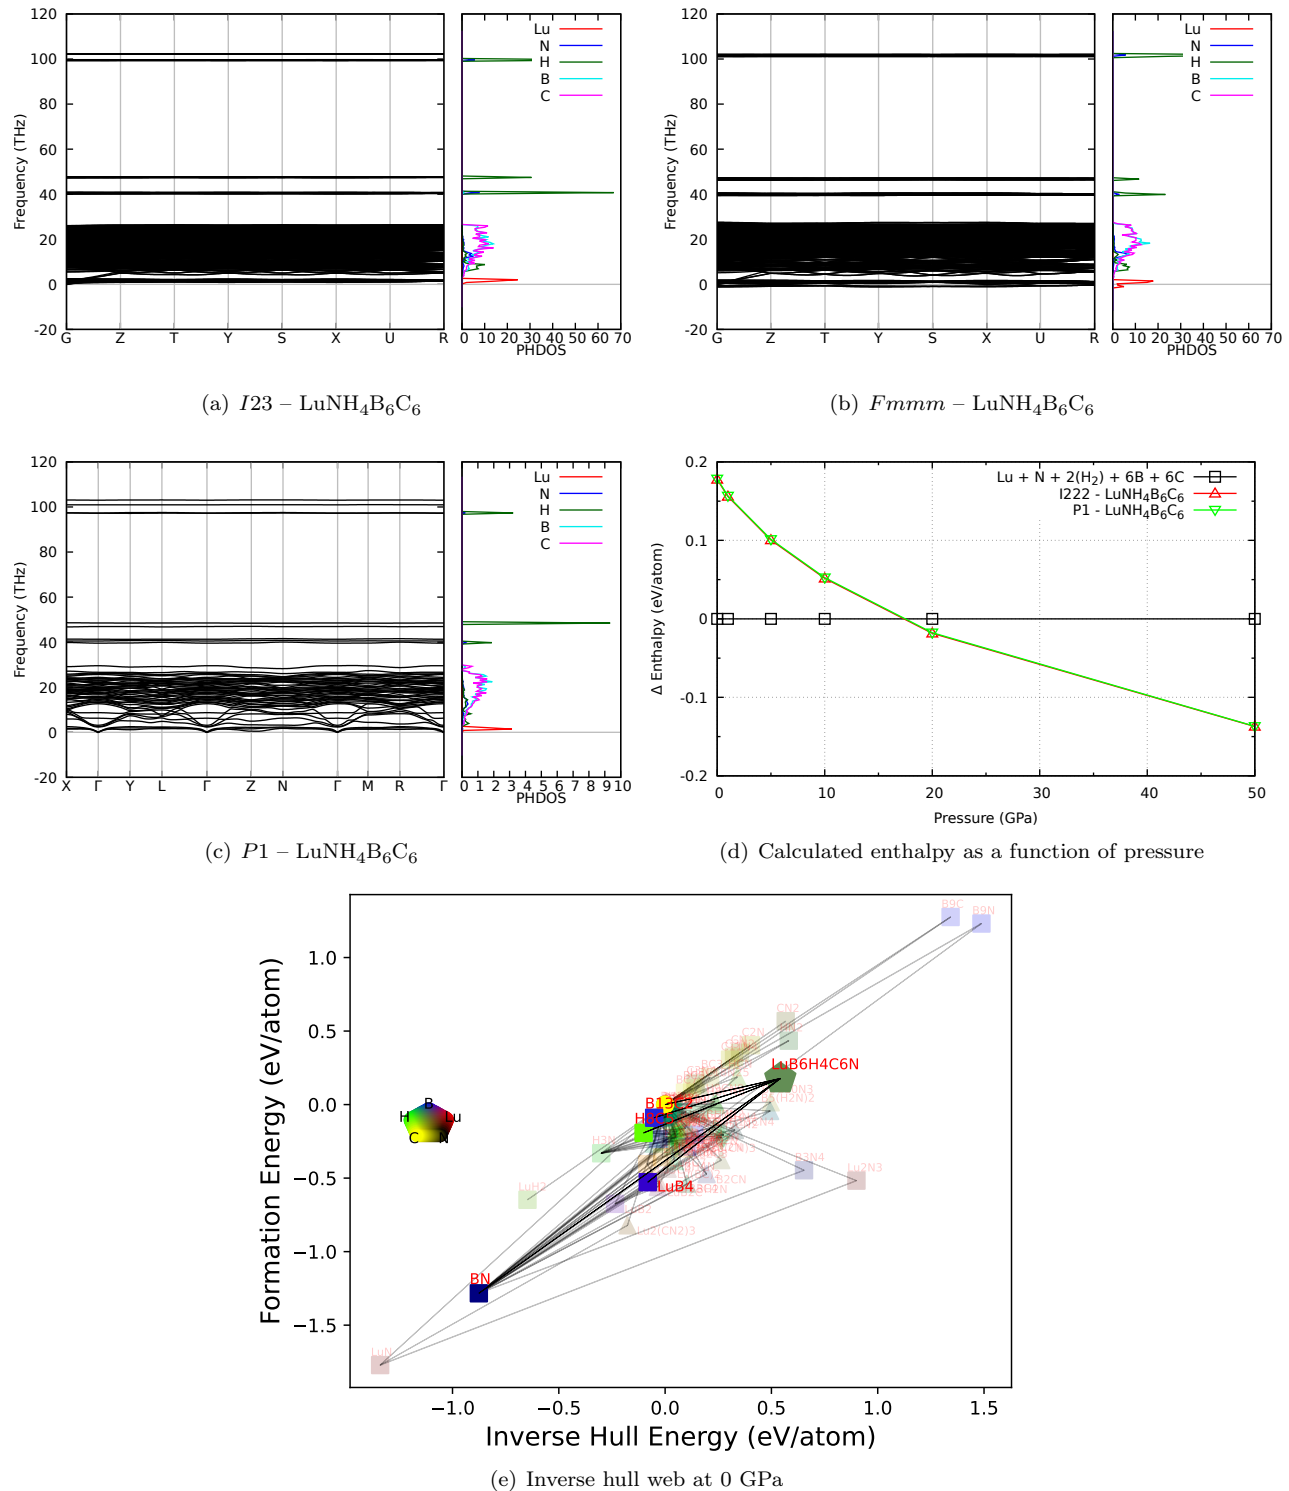

FIG. S22. (a-c) Phonon dispersion (left panel) and projected phonon densities of states (PHDOS, right panel) of different  $\text{LuNH}_4\text{B}_6\text{C}_6$  phases at ambient pressure. The absence of an imaginary frequency in the phonon spectra indicates that the structures are dynamically stable at ambient pressure. (d) Calculated enthalpy as a function of pressure for  $\text{LuNH}_4\text{B}_6\text{C}_6$  relative to simple elemental substance, and the phase transition pressure is  $\sim 17.4$  GPa. (e) Inverse hull web of Lu-N-H-B-C system at 0 K and ambient pressure. Compounds located in the positive range of the inverse-hull-energy axis indicates that they are metastable, while the others located in the negative range of the inverse-hull-energy axis are stable ones. We leave the  $\text{LuNH}_4\text{B}_6\text{C}_6$  compound and its hull reactants opaque, while we make all other phases partially transparent. Ground state structures of simple substances and other compounds were collected from the Inorganic Crystal Structure Database (ICSD) [1].

1.21  $\text{AcNH}_4\text{B}_6\text{C}_6$ 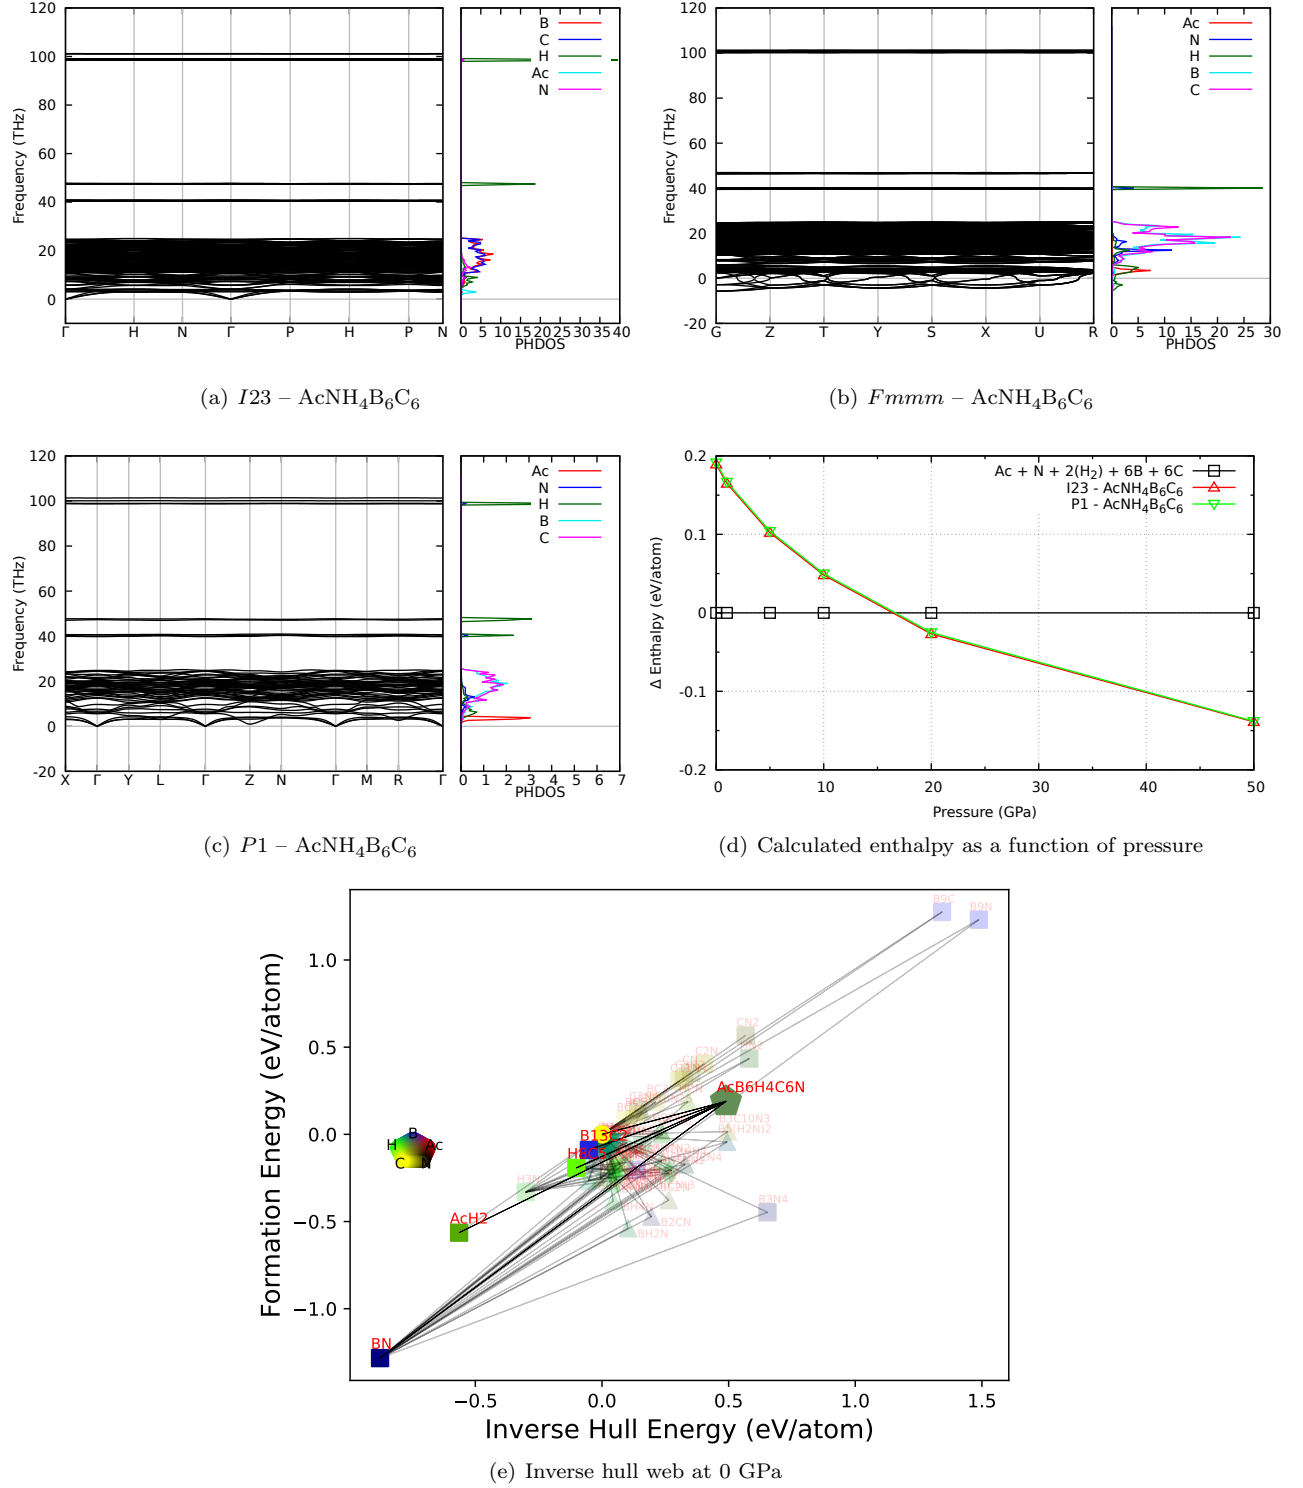

FIG. S23. (a–c) Phonon dispersion (left panel) and projected phonon densities of states (PHDOS, right panel) of different  $\text{AcNH}_4\text{B}_6\text{C}_6$  phases at ambient pressure. The absence of an imaginary frequency in the phonon spectra indicates that the structures are dynamically stable at ambient pressure. (d) Calculated enthalpy as a function of pressure for  $\text{AcNH}_4\text{B}_6\text{C}_6$  relative to simple elemental substance, and the phase transition pressure is  $\sim 16.4$  GPa. (e) Inverse hull web of Ac-N-H-B-C system at 0 K and ambient pressure. Compounds located in the positive range of the inverse-hull-energy axis indicates that they are metastable, while the others located in the negative range of the inverse-hull-energy axis are stable ones. We leave the  $\text{AcNH}_4\text{B}_6\text{C}_6$  compound and its hull reactants opaque, while we make all other phases partially transparent. Ground state structures of simple substances and other compounds were collected from the Inorganic Crystal Structure Database (ICSD) [1].

1.22  $\text{ThNH}_4\text{B}_6\text{C}_6$ 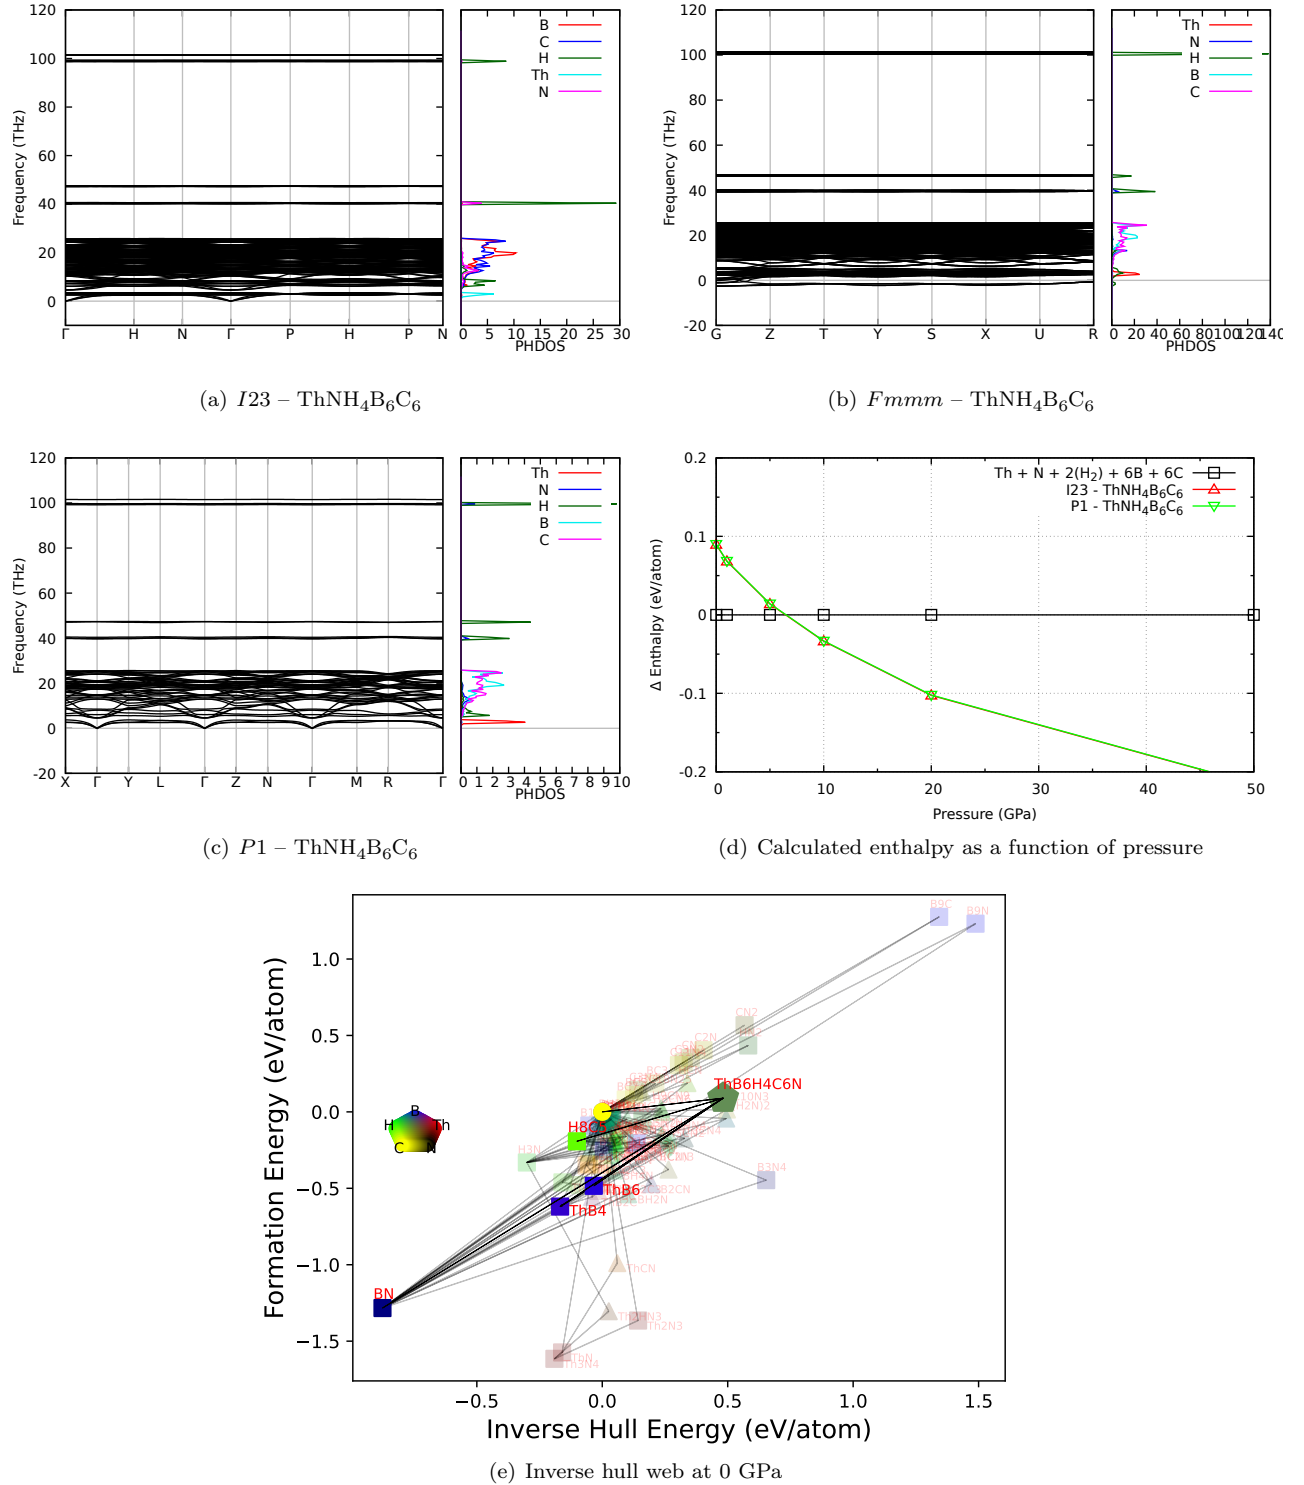

FIG. S24. (a–c) Phonon dispersion (left panel) and projected phonon densities of states (PHDOS, right panel) of different  $\text{ThNH}_4\text{B}_6\text{C}_6$  phases at ambient pressure. The absence of an imaginary frequency in the phonon spectra indicates that the structures are dynamically stable at ambient pressure. (d) Calculated enthalpy as a function of pressure for  $\text{ThNH}_4\text{B}_6\text{C}_6$  relative to simple elemental substance, and the phase transition pressure is  $\sim 6.4$  GPa. (e) Inverse hull web of Th-N-H-B-C system at 0 K and ambient pressure. Compounds located in the positive range of the inverse-hull-energy axis indicates that they are metastable, while the others located in the negative range of the inverse-hull-energy axis are stable ones. We leave the  $\text{ThNH}_4\text{B}_6\text{C}_6$  compound and its hull reactants opaque, while we make all other phases partially transparent. Ground state structures of simple substances and other compounds were collected from the Inorganic Crystal Structure Database (ICSD) [1].

### 1.23 $\text{PaNH}_4\text{B}_6\text{C}_6$

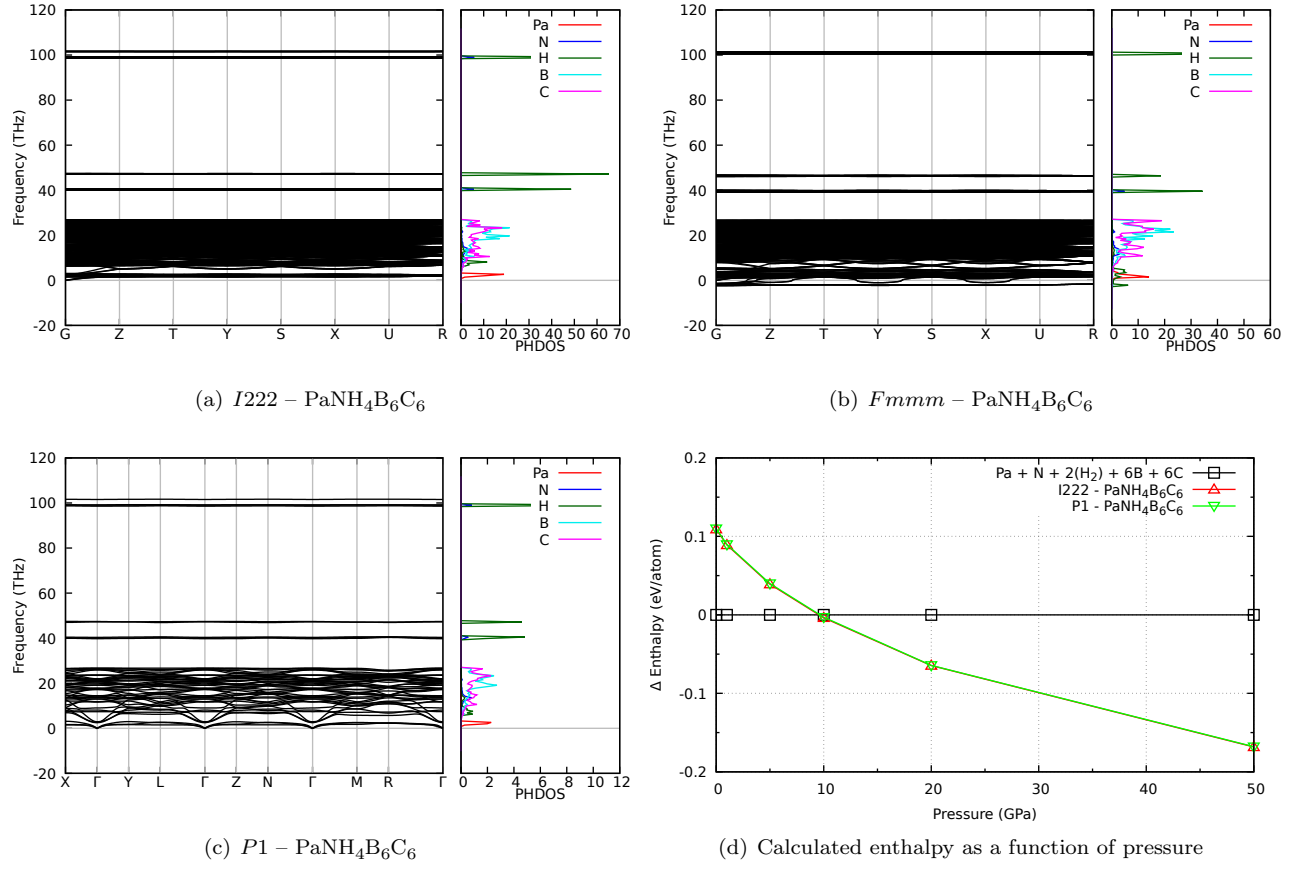

FIG. S25. (a–c) Phonon dispersion (left panel) and projected phonon densities of states (PHDOS, right panel) of different  $\text{PaNH}_4\text{B}_6\text{C}_6$  phases at ambient pressure. The absence of an imaginary frequency in the phonon spectra indicates that the structures are dynamically stable at ambient pressure. (d) Calculated enthalpy as a function of pressure for  $\text{PaNH}_4\text{B}_6\text{C}_6$  relative to simple elemental substance, and the phase transition pressure is  $\sim 9.8$  GPa. Ground state structures of simple substances were collected from the Inorganic Crystal Structure Database (ICSD) [1].

1.24  $\text{UNH}_4\text{B}_6\text{C}_6$ 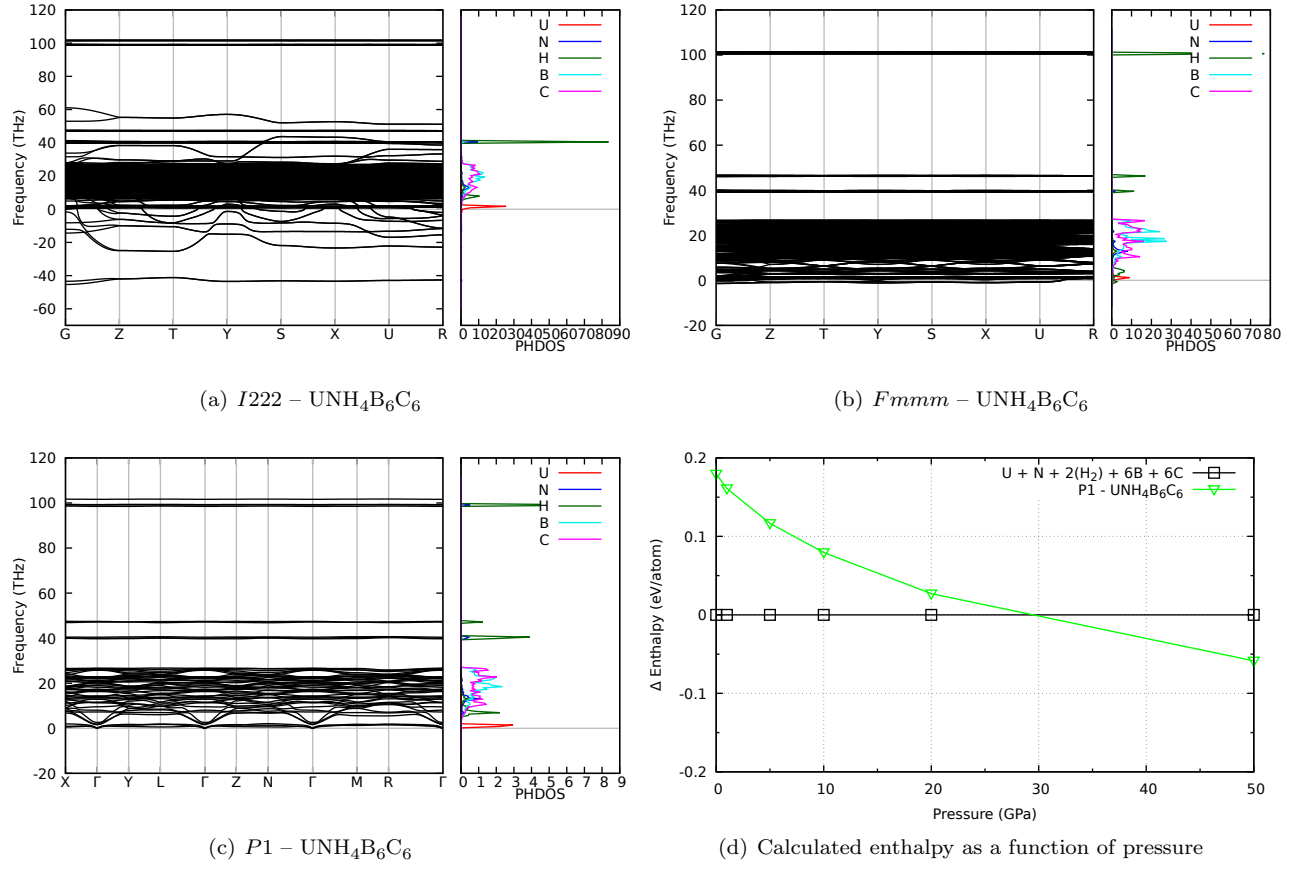

FIG. S26. (a–c) Phonon dispersion (left panel) and projected phonon densities of states (PHDOS, right panel) of different  $\text{UNH}_4\text{B}_6\text{C}_6$  phases at ambient pressure. The absence of an imaginary frequency in the phonon spectra indicates that the structures are dynamically stable at ambient pressure. (d) Calculated enthalpy as a function of pressure for  $\text{UNH}_4\text{B}_6\text{C}_6$  relative to simple elemental substance, and the phase transition pressure is  $\sim 29.5$  GPa. Ground state structures of simple substances were collected from the Inorganic Crystal Structure Database (ICSD) [1].

## II. SUPPLEMENTARY TABLES

### 2.1 Electron-phonon interaction properties of $\text{MNH}_4\text{B}_6\text{C}_6$ compounds.

TABLE S1: Summary of electron-phonon interaction properties for different phases of  $\text{MNH}_4\text{B}_6\text{C}_6$  at ambient pressure. The properties were computed using the Interpolation over the Brillouin Zone method and the Optimized Tetrahedron method, respectively. The phases are categorized by their compound and space group (S.G.). Listed values include the electronic density of states at the Fermi level ( $N(E_f)$  in states/Ry/f.u.), electron-phonon coupling constant ( $\lambda$ ), logarithmically averaged phonon frequency ( $\omega_{log}$  in K), and the critical temperature ( $T_c$  in K) estimated using Coulomb pseudopotential values of  $\mu^* = 0.10$ – $0.13$ , derived from solving the AD-McMillan (AD-M) equation and Eliashberg (E) equations. The computational demand was extraordinarily high, but in particular with  $I222$ - $\text{LuNH}_4\text{B}_6\text{C}_6$  and  $P1$ - $\text{LaNH}_4\text{B}_6\text{C}_6$ . Attempts to compute the electron-phonon coupling properties of  $I222$ - $\text{LuNH}_4\text{B}_6\text{C}_6$  and  $P1$ - $\text{LaNH}_4\text{B}_6\text{C}_6$  phases using 64-core nodes over 14 days (the maximum allowable computation time) for some single q-points did not yield results, leading us to abandon using the tetrahedron method for these phases.

| Compound                            | S.G.   | Interpolation over the Brillouin Zone |           |                |              |           | Optimized tetrahedron method |           |                |              |           |
|-------------------------------------|--------|---------------------------------------|-----------|----------------|--------------|-----------|------------------------------|-----------|----------------|--------------|-----------|
|                                     |        | $N(E_f)$                              | $\lambda$ | $\omega_{log}$ | $T_c$ (AD-M) | $T_c$ (E) | $N(E_f)$                     | $\lambda$ | $\omega_{log}$ | $T_c$ (AD-M) | $T_c$ (E) |
| $\text{NaNH}_4\text{B}_6\text{C}_6$ | $I222$ | 16.97                                 | 0.95      | 481.60         | 28–33        | 29–34     | 19.69                        | 1.43      | 446.16         | 49–55        | 53–58     |
| $\text{KNH}_4\text{B}_6\text{C}_6$  | $I222$ | 19.52                                 | 2.34      | 272.37         | 52–56        | 59–63     | 23.84                        | 3.71      | 191.22         | 56–62        | 71–76     |
| $\text{SrNH}_4\text{B}_6\text{C}_6$ | $I23$  | 18.25                                 | 1.79      | 422.67         | 60–66        | 65–70     | 19.51                        | 3.02      | 301.52         | 70–77        | 80–85     |
| $\text{YNH}_4\text{B}_6\text{C}_6$  | $I23$  | 13.85                                 | 2.10      | 192.57         | 33–36        | 42–47     | 12.18                        | 3.12      | 148.07         | 37–41        | 51–56     |
| $\text{LaNH}_4\text{B}_6\text{C}_6$ | $I23$  | 14.34                                 | 1.01      | 534.06         | 35–41        | 37–42     | 13.11                        | 1.07      | 513.51         | 37–43        | 39–44     |
| $\text{LuNH}_4\text{B}_6\text{C}_6$ | $I222$ | 13.90                                 | 1.54      | 252.71         | 31–34        | 39–44     | –                            | –         | –              | –            | –         |
| $\text{PbNH}_4\text{B}_6\text{C}_6$ | $I23$  | 18.82                                 | 2.31      | 318.72         | 59–64        | 67–72     | 18.78                        | 3.76      | 355.95         | 96–104       | 109–115   |
| $\text{AcNH}_4\text{B}_6\text{C}_6$ | $I23$  | 14.84                                 | 1.10      | 515.00         | 38–44        | 41–47     | 12.64                        | 1.42      | 481.26         | 52–58        | 56–62     |
| $\text{ThNH}_4\text{B}_6\text{C}_6$ | $I23$  | 12.14                                 | 0.81      | 635.46         | 26–32        | 28–33     | 11.42                        | 0.99      | 594.10         | 37–43        | 40–46     |
| $\text{CaNH}_4\text{B}_6\text{C}_6$ | $Fmmm$ | 17.85                                 | 2.52      | 250.19         | 51–56        | 68–73     | 21.47                        | 3.42      | 187.6          | 51–57        | 73–79     |
| $\text{SrNH}_4\text{B}_6\text{C}_6$ | $Fmmm$ | 18.44                                 | 2.01      | 377.43         | 61–66        | 68–73     | 22.58                        | 3.53      | 203.86         | 57–63        | 77–83     |
| $\text{YNH}_4\text{B}_6\text{C}_6$  | $Fmmm$ | 13.68                                 | 1.98      | 162.90         | 26–29        | 42–47     | 12.68                        | 3.6       | 109.85         | 31–35        | 44–49     |
| $\text{LaNH}_4\text{B}_6\text{C}_6$ | $Fmmm$ | 14.10                                 | 1.02      | 525.15         | 35–41        | 37–42     | 13.22                        | 1.16      | 408.1          | 34–39        | 36–40     |
| $\text{YNH}_4\text{B}_6\text{C}_6$  | $P1$   | 13.85                                 | 2.55      | 221.40         | 46–51        | 55–60     | 14.18                        | 1.17      | 333.78         | 28–32        | 29–33     |
| $\text{LaNH}_4\text{B}_6\text{C}_6$ | $P1$   | 14.13                                 | 1.23      | 480.22         | 43–49        | 46–51     | –                            | –         | –              | –            | –         |
| $\text{LuNH}_4\text{B}_6\text{C}_6$ | $P1$   | 12.60                                 | 1.26      | 351.16         | 33–38        | 37–42     | 10.69                        | 1.26      | 375.04         | 35–40        | 38–43     |
| $\text{PbNH}_4\text{B}_6\text{C}_6$ | $P1$   | 20.13                                 | 3.73      | 223.81         | 65–72        | 80–86     | 22.53                        | 3.91      | 180.57         | 56–62        | 78–84     |
| $\text{AcNH}_4\text{B}_6\text{C}_6$ | $P1$   | 14.88                                 | 1.22      | 508.39         | 45–51        | 48–54     | 14.50                        | 0.94      | 468.24         | 27–32        | 28–33     |
| $\text{ThNH}_4\text{B}_6\text{C}_6$ | $P1$   | 12.21                                 | 0.68      | 666.47         | 17–22        | 18–24     | 12.96                        | 0.82      | 567.11         | 24–29        | 25–31     |

### III. SUPPLEMENTARY INFORMATION

#### 3.1 Structure parameters of $\text{MNH}_4\text{B}_6\text{C}_6$ compounds.

TABLE S2: Structural parameters of proposed  $\text{MNH}_4\text{B}_6\text{C}_6$  compounds at ambient pressure.

| Compound<br>S.G.(Setting)                               | Lattice<br>(Å, °) | Atomic coordinates (fractional) |        |        |        |
|---------------------------------------------------------|-------------------|---------------------------------|--------|--------|--------|
|                                                         |                   | Atoms                           | X      | Y      | Z      |
| $\text{AcNH}_4\text{B}_6\text{C}_6$<br><i>I</i> 23 (1)  | a = 9.9078        | Ac(2a)                          | 0.0000 | 0.0000 | 0.0000 |
|                                                         | b = 9.9078        | Ac(6b)                          | 0.0000 | 0.5000 | 0.5000 |
|                                                         | c = 9.9078        | B(24f)                          | 0.1279 | 0.0004 | 0.7503 |
|                                                         | $\alpha = 90$     | B(24f)                          | 0.3710 | 0.9960 | 0.7505 |
|                                                         | $\beta = 90$      | C(24f)                          | 0.1229 | 0.7499 | 0.9989 |
|                                                         | $\gamma = 90$     | C(24f)                          | 0.8763 | 0.2498 | 0.5027 |
|                                                         |                   | H(24f)                          | 0.2213 | 0.8304 | 0.6933 |
|                                                         |                   | H(8c)                           | 0.3107 | 0.3107 | 0.3107 |
|                                                         |                   | N(8c)                           | 0.2513 | 0.2513 | 0.2513 |
| $\text{AcNH}_4\text{B}_6\text{C}_6$<br><i>P</i> 1 (1)   | a = 4.9198        | Ac(1a)                          | 0.1948 | 0.8082 | 0.1951 |
|                                                         | b = 4.9205        | N(1a)                           | 0.6918 | 0.3057 | 0.6918 |
|                                                         | c = 4.9838        | H(1a)                           | 0.8536 | 0.1923 | 0.7592 |
|                                                         | $\alpha = 89.9$   | H(1a)                           | 0.5711 | 0.1838 | 0.5797 |
|                                                         | $\beta = 89.9$    | H(1a)                           | 0.7567 | 0.4616 | 0.5732 |
|                                                         | $\gamma = 89.1$   | H(1a)                           | 0.5817 | 0.3806 | 0.8496 |
|                                                         |                   | B(1a)                           | 0.9339 | 0.8031 | 0.6956 |
|                                                         |                   | B(1a)                           | 0.1925 | 0.3088 | 0.9385 |
|                                                         |                   | B(1a)                           | 0.6937 | 0.0617 | 0.1921 |
|                                                         |                   | B(1a)                           | 0.4546 | 0.8063 | 0.6958 |
|                                                         |                   | B(1a)                           | 0.1921 | 0.3088 | 0.4510 |
|                                                         |                   | B(1a)                           | 0.6971 | 0.5544 | 0.1920 |
|                                                         |                   | C(1a)                           | 0.1955 | 0.0545 | 0.6947 |
|                                                         |                   | C(1a)                           | 0.6945 | 0.8073 | 0.9481 |
|                                                         |                   | C(1a)                           | 0.9483 | 0.3080 | 0.1940 |
|                                                         |                   | C(1a)                           | 0.1934 | 0.5600 | 0.6947 |
|                                                         |                   | C(1a)                           | 0.6945 | 0.8078 | 0.4403 |
|                                                         |                   | C(1a)                           | 0.4400 | 0.3074 | 0.1945 |
| $\text{CaNH}_4\text{B}_6\text{C}_6$<br><i>Fm</i> mm (1) | a = 9.7007        | B(16m)                          | 0.0000 | 0.6255 | 0.7518 |
|                                                         | b = 9.6567        | B(16n)                          | 0.7478 | 0.0000 | 0.1260 |
|                                                         | c = 9.6568        | B(16o)                          | 0.8743 | 0.2519 | 0.0000 |
|                                                         | $\alpha = 90$     | C(16o)                          | 0.7488 | 0.1218 | 0.0000 |
|                                                         | $\beta = 90$      | C(16m)                          | 0.0000 | 0.2510 | 0.1214 |
|                                                         | $\gamma = 90$     | C(16n)                          | 0.3784 | 0.0000 | 0.7513 |
|                                                         |                   | Ca(4a)                          | 0.0000 | 0.0000 | 0.0000 |
|                                                         |                   | Ca(4b)                          | 0.0000 | 0.0000 | 0.5000 |
|                                                         |                   | H(32p)                          | 0.6895 | 0.8107 | 0.3107 |
| $\text{DyNH}_4\text{B}_6\text{C}_6$<br><i>Fm</i> mm (1) |                   | N(8f)                           | 0.2500 | 0.2500 | 0.2500 |
|                                                         | a = 9.6964        | B(16m)                          | 0.0000 | 0.2515 | 0.1258 |
|                                                         | b = 9.5719        | B(16o)                          | 0.7516 | 0.6284 | 0.0000 |
|                                                         | c = 9.5761        | B(16n)                          | 0.6268 | 0.0000 | 0.7517 |
|                                                         | $\alpha = 90$     | C(16n)                          | 0.2510 | 0.0000 | 0.1205 |
|                                                         | $\beta = 90$      | C(16m)                          | 0.0000 | 0.6198 | 0.7510 |
|                                                         | $\gamma = 90$     | C(16o)                          | 0.6202 | 0.7507 | 0.0000 |
|                                                         |                   | Dy(4a)                          | 0.0000 | 0.0000 | 0.0000 |
|                                                         |                   | Dy(4b)                          | 0.0000 | 0.0000 | 0.5000 |
| $\text{DyNH}_4\text{B}_6\text{C}_6$<br><i>I</i> 222 (1) |                   | H(32p)                          | 0.8107 | 0.8111 | 0.8113 |
|                                                         |                   | N(8f)                           | 0.2500 | 0.2500 | 0.2500 |
|                                                         | a = 9.6986        | B(8k)                           | 0.2497 | 0.9997 | 0.8740 |
|                                                         | b = 9.7007        | B(8k)                           | 0.9998 | 0.1260 | 0.7503 |
|                                                         | c = 9.7008        | B(8k)                           | 0.1260 | 0.2497 | 0.0002 |
|                                                         | $\alpha = 90$     | B(8k)                           | 0.2493 | 0.0025 | 0.6265 |
|                                                         | $\beta = 90$      | B(8k)                           | 0.0025 | 0.3735 | 0.7507 |
|                                                         | $\gamma = 90$     | B(8k)                           | 0.3735 | 0.2493 | 0.9975 |
|                                                         |                   | C(8k)                           | 0.0009 | 0.2502 | 0.8801 |

Continued on next page



Continued

| Compound<br>S.G.(Setting)                                   | Lattice<br>(Å,°) | Atomic coordinates (fractional) |        |        |        |
|-------------------------------------------------------------|------------------|---------------------------------|--------|--------|--------|
|                                                             |                  | Atoms                           | X      | Y      | Z      |
|                                                             |                  | C(8k)                           | 0.2502 | 0.1199 | 0.9991 |
|                                                             |                  | C(8k)                           | 0.1199 | 0.0009 | 0.7498 |
|                                                             |                  | C(8k)                           | 0.9985 | 0.2504 | 0.6205 |
|                                                             |                  | C(8k)                           | 0.2504 | 0.3795 | 0.0015 |
|                                                             |                  | C(8k)                           | 0.3795 | 0.9985 | 0.7496 |
|                                                             |                  | Dy(2a)                          | 0.0000 | 0.0000 | 0.0000 |
|                                                             |                  | Dy(2c)                          | 0.0000 | 0.0000 | 0.5000 |
|                                                             |                  | Dy(2d)                          | 0.0000 | 0.5000 | 0.0000 |
|                                                             |                  | Dy(2b)                          | 0.5000 | 0.0000 | 0.0000 |
|                                                             |                  | H(8k)                           | 0.3080 | 0.1687 | 0.7806 |
|                                                             |                  | H(8k)                           | 0.1687 | 0.2194 | 0.6919 |
|                                                             |                  | H(8k)                           | 0.2194 | 0.3081 | 0.8313 |
|                                                             |                  | H(8k)                           | 0.3118 | 0.3117 | 0.6883 |
|                                                             |                  | N(8k)                           | 0.2512 | 0.2512 | 0.7488 |
| DyNH <sub>4</sub> B <sub>6</sub> C <sub>6</sub><br>P1 (1)   | a = 4.8228       | Dy(1a)                          | 0.8094 | 0.8098 | 0.8095 |
|                                                             | b = 4.8460       | N(1a)                           | 0.3053 | 0.3055 | 0.3049 |
|                                                             | c = 4.8924       | H(1a)                           | 0.1789 | 0.1830 | 0.1924 |
|                                                             | $\alpha = 89.7$  | H(1a)                           | 0.3736 | 0.4634 | 0.1839 |
|                                                             | $\beta = 89.9$   | H(1a)                           | 0.4680 | 0.1893 | 0.3723 |
|                                                             | $\gamma = 89.9$  | H(1a)                           | 0.1959 | 0.3813 | 0.4662 |
|                                                             |                  | B(1a)                           | 0.3091 | 0.0564 | 0.8056 |
|                                                             |                  | B(1a)                           | 0.0637 | 0.8046 | 0.3095 |
|                                                             |                  | B(1a)                           | 0.8051 | 0.3092 | 0.0606 |
|                                                             |                  | B(1a)                           | 0.3090 | 0.5595 | 0.8057 |
|                                                             |                  | B(1a)                           | 0.5517 | 0.8047 | 0.3091 |
|                                                             |                  | B(1a)                           | 0.8057 | 0.3095 | 0.5551 |
|                                                             |                  | C(1a)                           | 0.3080 | 0.8077 | 0.0472 |
|                                                             |                  | C(1a)                           | 0.0463 | 0.3078 | 0.8078 |
|                                                             |                  | C(1a)                           | 0.8078 | 0.0474 | 0.3082 |
|                                                             |                  | C(1a)                           | 0.3077 | 0.8076 | 0.5668 |
|                                                             |                  | C(1a)                           | 0.5674 | 0.3077 | 0.8075 |
|                                                             |                  | C(1a)                           | 0.8074 | 0.5655 | 0.3076 |
| ErNH <sub>4</sub> B <sub>6</sub> C <sub>6</sub><br>I222 (1) | a = 9.6816       | B(8k)                           | 0.2497 | 0.9997 | 0.8741 |
|                                                             | b = 9.6837       | B(8k)                           | 0.9998 | 0.1259 | 0.7503 |
|                                                             | c = 9.6838       | B(8k)                           | 0.1259 | 0.2497 | 0.0002 |
|                                                             | $\alpha = 90$    | B(8k)                           | 0.2493 | 0.0025 | 0.6263 |
|                                                             | $\beta = 90$     | B(8k)                           | 0.0025 | 0.3736 | 0.7507 |
|                                                             | $\gamma = 90$    | B(8k)                           | 0.3737 | 0.2493 | 0.9975 |
|                                                             |                  | C(8k)                           | 0.0009 | 0.2502 | 0.8803 |
|                                                             |                  | C(8k)                           | 0.2502 | 0.1197 | 0.9991 |
|                                                             |                  | C(8k)                           | 0.1197 | 0.0009 | 0.7498 |
|                                                             |                  | C(8k)                           | 0.9985 | 0.2504 | 0.6204 |
|                                                             |                  | C(8k)                           | 0.2504 | 0.3797 | 0.0015 |
|                                                             |                  | C(8k)                           | 0.3796 | 0.9985 | 0.7496 |
|                                                             |                  | Er(2a)                          | 0.0000 | 0.0000 | 0.0000 |
|                                                             |                  | Er(2c)                          | 0.0000 | 0.0000 | 0.5000 |
|                                                             |                  | Er(2d)                          | 0.0000 | 0.5000 | 0.0000 |
|                                                             |                  | Er(2b)                          | 0.5000 | 0.0000 | 0.0000 |
|                                                             |                  | H(8k)                           | 0.3081 | 0.1687 | 0.7808 |
|                                                             |                  | H(8k)                           | 0.1687 | 0.2192 | 0.6918 |
|                                                             |                  | H(8k)                           | 0.2192 | 0.3082 | 0.8313 |
|                                                             |                  | H(8k)                           | 0.3118 | 0.3118 | 0.6882 |
|                                                             |                  | N(8k)                           | 0.2512 | 0.2512 | 0.7488 |
| ErNH <sub>4</sub> B <sub>6</sub> C <sub>6</sub><br>P1 (1)   | a = 4.8093       | Er(1a)                          | 0.8099 | 0.8106 | 0.8102 |
|                                                             | b = 4.8387       | N(1a)                           | 0.3053 | 0.3054 | 0.3048 |
|                                                             | c = 4.8922       | H(1a)                           | 0.1775 | 0.1828 | 0.1938 |
|                                                             | $\alpha = 89.6$  | H(1a)                           | 0.3727 | 0.4635 | 0.1828 |
|                                                             | $\beta = 89.8$   | H(1a)                           | 0.4690 | 0.1889 | 0.3710 |
|                                                             | $\gamma = 89.9$  | H(1a)                           | 0.1971 | 0.3816 | 0.4668 |

Continued on next page

Continued

| Compound<br>S.G.(Setting)                                          | Lattice<br>(Å, °) | Atomic coordinates (fractional) |        |        |        |
|--------------------------------------------------------------------|-------------------|---------------------------------|--------|--------|--------|
|                                                                    |                   | Atoms                           | X      | Y      | Z      |
|                                                                    |                   | B(1a)                           | 0.3092 | 0.0557 | 0.8055 |
|                                                                    |                   | B(1a)                           | 0.0639 | 0.8045 | 0.3097 |
|                                                                    |                   | B(1a)                           | 0.8051 | 0.3093 | 0.0603 |
|                                                                    |                   | B(1a)                           | 0.3091 | 0.5602 | 0.8057 |
|                                                                    |                   | B(1a)                           | 0.5514 | 0.8045 | 0.3091 |
|                                                                    |                   | B(1a)                           | 0.8057 | 0.3098 | 0.5553 |
|                                                                    |                   | C(1a)                           | 0.3080 | 0.8076 | 0.0468 |
|                                                                    |                   | C(1a)                           | 0.0458 | 0.3078 | 0.8078 |
|                                                                    |                   | C(1a)                           | 0.8078 | 0.0470 | 0.3083 |
|                                                                    |                   | C(1a)                           | 0.3077 | 0.8076 | 0.5672 |
|                                                                    |                   | C(1a)                           | 0.5677 | 0.3077 | 0.8075 |
|                                                                    |                   | C(1a)                           | 0.8074 | 0.5655 | 0.3074 |
| EuNH <sub>4</sub> B <sub>6</sub> C <sub>6</sub><br><i>Fmmm</i> (1) | a = 9.7160        | B(16m)                          | 0.0000 | 0.2515 | 0.1258 |
|                                                                    | b = 9.5980        | B(16o)                          | 0.7520 | 0.6272 | 0.0000 |
|                                                                    | c = 9.5987        | B(16n)                          | 0.6263 | 0.0000 | 0.7516 |
|                                                                    | $\alpha = 90$     | C(16n)                          | 0.2510 | 0.0000 | 0.1226 |
|                                                                    | $\beta = 90$      | C(16m)                          | 0.0000 | 0.6217 | 0.7508 |
|                                                                    | $\gamma = 90$     | C(16o)                          | 0.6220 | 0.7511 | 0.0000 |
|                                                                    |                   | Eu(4a)                          | 0.0000 | 0.0000 | 0.0000 |
|                                                                    |                   | Eu(4b)                          | 0.0000 | 0.0000 | 0.5000 |
|                                                                    |                   | H(32p)                          | 0.8105 | 0.8110 | 0.8111 |
|                                                                    |                   | N(8f)                           | 0.2500 | 0.2500 | 0.2500 |
| EuNH <sub>4</sub> B <sub>6</sub> C <sub>6</sub><br><i>I222</i> (1) | a = 9.7223        | B(8k)                           | 0.6254 | 0.4993 | 0.7495 |
|                                                                    | b = 9.7223        | B(8k)                           | 0.2495 | 0.1254 | 0.9993 |
|                                                                    | c = 9.7198        | B(8k)                           | 0.9993 | 0.2495 | 0.1254 |
|                                                                    | $\alpha = 90$     | B(8k)                           | 0.3735 | 0.0045 | 0.2497 |
|                                                                    | $\beta = 90$      | B(8k)                           | 0.7497 | 0.8735 | 0.5045 |
|                                                                    | $\gamma = 90$     | B(8k)                           | 0.0045 | 0.2497 | 0.3735 |
|                                                                    |                   | C(8k)                           | 0.6219 | 0.7500 | 0.5007 |
|                                                                    |                   | C(8k)                           | 0.0007 | 0.1219 | 0.2500 |
|                                                                    |                   | C(8k)                           | 0.2500 | 0.0007 | 0.1219 |
|                                                                    |                   | C(8k)                           | 0.3774 | 0.2504 | 0.9971 |
|                                                                    |                   | C(8k)                           | 0.9971 | 0.3774 | 0.2504 |
|                                                                    |                   | C(8k)                           | 0.7504 | 0.4971 | 0.8774 |
|                                                                    |                   | Eu(2a)                          | 0.0000 | 0.0000 | 0.0000 |
|                                                                    |                   | Eu(2b)                          | 0.5000 | 0.0000 | 0.0000 |
|                                                                    |                   | Eu(2d)                          | 0.0000 | 0.5000 | 0.0000 |
|                                                                    |                   | Eu(2c)                          | 0.0000 | 0.0000 | 0.5000 |
|                                                                    |                   | H(8k)                           | 0.7183 | 0.6693 | 0.8080 |
|                                                                    |                   | H(8k)                           | 0.3080 | 0.2183 | 0.1693 |
|                                                                    |                   | H(8k)                           | 0.1693 | 0.3080 | 0.2183 |
|                                                                    |                   | H(8k)                           | 0.3114 | 0.3114 | 0.3114 |
|                                                                    |                   | N(8k)                           | 0.2510 | 0.2510 | 0.2510 |
| EuNH <sub>4</sub> B <sub>6</sub> C <sub>6</sub><br><i>P1</i> (1)   | a = 6.8172        | Eu(1a)                          | 0.8067 | 0.8069 | 0.6134 |
|                                                                    | b = 4.7757        | N(1a)                           | 0.3067 | 0.3070 | 0.6134 |
|                                                                    | c = 4.8523        | H(1a)                           | 0.1841 | 0.1844 | 0.3730 |
|                                                                    | $\alpha = 90$     | H(1a)                           | 0.1874 | 0.4289 | 0.6189 |
|                                                                    | $\beta = 135$     | H(1a)                           | 0.4258 | 0.4291 | 0.6077 |
|                                                                    | $\gamma = 90$     | H(1a)                           | 0.4294 | 0.1844 | 0.8538 |
|                                                                    |                   | B(1a)                           | 0.8070 | 0.3067 | 0.8643 |
|                                                                    |                   | B(1a)                           | 0.3067 | 0.0598 | 0.1133 |
|                                                                    |                   | B(1a)                           | 0.0614 | 0.8063 | 0.3672 |
|                                                                    |                   | B(1a)                           | 0.8063 | 0.3068 | 0.3623 |
|                                                                    |                   | B(1a)                           | 0.3067 | 0.5536 | 0.1133 |
|                                                                    |                   | B(1a)                           | 0.5519 | 0.8062 | 0.8594 |
|                                                                    |                   | C(1a)                           | 0.0498 | 0.3067 | 0.8562 |
|                                                                    |                   | C(1a)                           | 0.8067 | 0.0510 | 0.1133 |
|                                                                    |                   | C(1a)                           | 0.3072 | 0.8067 | 0.3593 |
|                                                                    |                   | C(1a)                           | 0.5635 | 0.3067 | 0.3705 |

Continued on next page

Continued

| Compound<br>S.G.(Setting)                                          | Lattice<br>(Å,°)                                                                               | Atomic coordinates (fractional) |        |        |        |
|--------------------------------------------------------------------|------------------------------------------------------------------------------------------------|---------------------------------|--------|--------|--------|
|                                                                    |                                                                                                | Atoms                           | X      | Y      | Z      |
| GdNH <sub>4</sub> B <sub>6</sub> C <sub>6</sub><br><i>Fmmm</i> (1) | a = 9.7162<br>b = 9.5961<br>c = 9.5997<br>$\alpha = 90$<br>$\beta = 90$<br>$\gamma = 90$       | C(1a)                           | 0.8067 | 0.5623 | 0.1133 |
|                                                                    |                                                                                                | C(1a)                           | 0.3062 | 0.8067 | 0.8674 |
|                                                                    |                                                                                                | B(16m)                          | 0.0000 | 0.2515 | 0.1260 |
|                                                                    |                                                                                                | B(16o)                          | 0.7516 | 0.6284 | 0.0000 |
|                                                                    |                                                                                                | B(16n)                          | 0.6270 | 0.0000 | 0.7517 |
|                                                                    |                                                                                                | C(16n)                          | 0.2510 | 0.0000 | 0.1207 |
|                                                                    |                                                                                                | C(16m)                          | 0.0000 | 0.6201 | 0.7509 |
|                                                                    |                                                                                                | C(16o)                          | 0.6204 | 0.7507 | 0.0000 |
|                                                                    |                                                                                                | Gd(4a)                          | 0.0000 | 0.0000 | 0.0000 |
|                                                                    |                                                                                                | Gd(4b)                          | 0.0000 | 0.0000 | 0.5000 |
|                                                                    |                                                                                                | H(32p)                          | 0.8105 | 0.8110 | 0.8112 |
|                                                                    |                                                                                                | N(8f)                           | 0.2500 | 0.2500 | 0.2500 |
| GdNH <sub>4</sub> B <sub>6</sub> C <sub>6</sub><br><i>I222</i> (1) | a = 9.7207<br>b = 9.7207<br>c = 9.7186<br>$\alpha = 90$<br>$\beta = 90$<br>$\gamma = 90$       | B(8k)                           | 0.1261 | 0.9998 | 0.2497 |
|                                                                    |                                                                                                | B(8k)                           | 0.2497 | 0.1261 | 0.9998 |
|                                                                    |                                                                                                | B(8k)                           | 0.9998 | 0.2497 | 0.1261 |
|                                                                    |                                                                                                | B(8k)                           | 0.3734 | 0.0026 | 0.2493 |
|                                                                    |                                                                                                | B(8k)                           | 0.2493 | 0.3734 | 0.0026 |
|                                                                    |                                                                                                | B(8k)                           | 0.0026 | 0.2493 | 0.3734 |
|                                                                    |                                                                                                | C(8k)                           | 0.1201 | 0.2502 | 0.0009 |
|                                                                    |                                                                                                | C(8k)                           | 0.0009 | 0.1201 | 0.2502 |
|                                                                    |                                                                                                | C(8k)                           | 0.2502 | 0.0009 | 0.1201 |
|                                                                    |                                                                                                | C(8k)                           | 0.3793 | 0.2503 | 0.9984 |
|                                                                    |                                                                                                | C(8k)                           | 0.9984 | 0.3793 | 0.2503 |
|                                                                    |                                                                                                | C(8k)                           | 0.2503 | 0.9984 | 0.3793 |
|                                                                    |                                                                                                | Gd(2a)                          | 0.0000 | 0.0000 | 0.0000 |
|                                                                    |                                                                                                | Gd(2b)                          | 0.5000 | 0.0000 | 0.0000 |
|                                                                    |                                                                                                | Gd(2d)                          | 0.0000 | 0.5000 | 0.0000 |
|                                                                    |                                                                                                | Gd(2c)                          | 0.0000 | 0.0000 | 0.5000 |
|                                                                    |                                                                                                | H(8k)                           | 0.2196 | 0.1688 | 0.3079 |
|                                                                    |                                                                                                | H(8k)                           | 0.3079 | 0.2196 | 0.1688 |
|                                                                    |                                                                                                | H(8k)                           | 0.1688 | 0.3079 | 0.2196 |
|                                                                    |                                                                                                | H(8k)                           | 0.3116 | 0.3116 | 0.3116 |
|                                                                    |                                                                                                | N(8k)                           | 0.2512 | 0.2512 | 0.2512 |
| GdNH <sub>4</sub> B <sub>6</sub> C <sub>6</sub><br><i>P1</i> (1)   | a = 4.8393<br>b = 4.8546<br>c = 4.8920<br>$\alpha = 89.8$<br>$\beta = 89.9$<br>$\gamma = 89.9$ | Gd(1a)                          | 0.8090 | 0.8093 | 0.8091 |
|                                                                    |                                                                                                | N(1a)                           | 0.3053 | 0.3055 | 0.3050 |
|                                                                    |                                                                                                | H(1a)                           | 0.1807 | 0.1833 | 0.1907 |
|                                                                    |                                                                                                | H(1a)                           | 0.3747 | 0.4633 | 0.1853 |
|                                                                    |                                                                                                | H(1a)                           | 0.4669 | 0.1897 | 0.3740 |
|                                                                    |                                                                                                | H(1a)                           | 0.1944 | 0.3809 | 0.4654 |
|                                                                    |                                                                                                | B(1a)                           | 0.3091 | 0.0574 | 0.8055 |
|                                                                    |                                                                                                | B(1a)                           | 0.0634 | 0.8048 | 0.3094 |
|                                                                    |                                                                                                | B(1a)                           | 0.8052 | 0.3092 | 0.0608 |
|                                                                    |                                                                                                | B(1a)                           | 0.3089 | 0.5585 | 0.8057 |
|                                                                    |                                                                                                | B(1a)                           | 0.5521 | 0.8049 | 0.3090 |
|                                                                    |                                                                                                | B(1a)                           | 0.8057 | 0.3092 | 0.5550 |
|                                                                    |                                                                                                | C(1a)                           | 0.3079 | 0.8077 | 0.0477 |
|                                                                    |                                                                                                | C(1a)                           | 0.0468 | 0.3078 | 0.8078 |
|                                                                    |                                                                                                | C(1a)                           | 0.8078 | 0.0478 | 0.3081 |
|                                                                    |                                                                                                | C(1a)                           | 0.3077 | 0.8076 | 0.5664 |
|                                                                    |                                                                                                | C(1a)                           | 0.5669 | 0.3078 | 0.8076 |
|                                                                    |                                                                                                | C(1a)                           | 0.8075 | 0.5655 | 0.3078 |
| HoNH <sub>4</sub> B <sub>6</sub> C <sub>6</sub><br><i>Fmmm</i> (1) | a = 9.6877<br>b = 9.5613<br>c = 9.5663<br>$\alpha = 90$<br>$\beta = 90$<br>$\gamma = 90$       | B(16m)                          | 0.0000 | 0.2516 | 0.1257 |
|                                                                    |                                                                                                | B(16o)                          | 0.7516 | 0.6284 | 0.0000 |
|                                                                    |                                                                                                | B(16n)                          | 0.6268 | 0.0000 | 0.7517 |
|                                                                    |                                                                                                | C(16n)                          | 0.2510 | 0.0000 | 0.1205 |
|                                                                    |                                                                                                | C(16m)                          | 0.0000 | 0.6197 | 0.7510 |
|                                                                    |                                                                                                | C(16o)                          | 0.6201 | 0.7507 | 0.0000 |
|                                                                    |                                                                                                | H(32p)                          | 0.8107 | 0.8111 | 0.8114 |
|                                                                    |                                                                                                | Ho(4a)                          | 0.0000 | 0.0000 | 0.0000 |

Continued on next page

Continued

| Compound<br>S.G.(Setting)                                           | Lattice<br>(Å, °)                                                                              | Atomic coordinates (fractional) |        |        |        |
|---------------------------------------------------------------------|------------------------------------------------------------------------------------------------|---------------------------------|--------|--------|--------|
|                                                                     |                                                                                                | Atoms                           | X      | Y      | Z      |
| HoNH <sub>4</sub> B <sub>6</sub> C <sub>6</sub><br><i>I</i> 222 (1) | a = 9.6900<br>b = 9.6922<br>c = 9.6922<br>$\alpha$ = 90<br>$\beta$ = 90<br>$\gamma$ = 90       | Ho(4b)                          | 0.0000 | 0.0000 | 0.5000 |
|                                                                     |                                                                                                | N(8f)                           | 0.2500 | 0.2500 | 0.2500 |
|                                                                     |                                                                                                | B(8k)                           | 0.2497 | 0.9997 | 0.8741 |
|                                                                     |                                                                                                | B(8k)                           | 0.9998 | 0.1260 | 0.7503 |
|                                                                     |                                                                                                | B(8k)                           | 0.1259 | 0.2497 | 0.0002 |
|                                                                     |                                                                                                | B(8k)                           | 0.2493 | 0.0025 | 0.6264 |
|                                                                     |                                                                                                | B(8k)                           | 0.0025 | 0.3736 | 0.7507 |
|                                                                     |                                                                                                | B(8k)                           | 0.3736 | 0.2493 | 0.9975 |
|                                                                     |                                                                                                | C(8k)                           | 0.0009 | 0.2502 | 0.8802 |
|                                                                     |                                                                                                | C(8k)                           | 0.2502 | 0.1198 | 0.9991 |
|                                                                     |                                                                                                | C(8k)                           | 0.1198 | 0.0009 | 0.7498 |
|                                                                     |                                                                                                | C(8k)                           | 0.9985 | 0.2504 | 0.6204 |
|                                                                     |                                                                                                | C(8k)                           | 0.2504 | 0.3796 | 0.0015 |
|                                                                     |                                                                                                | C(8k)                           | 0.3796 | 0.9985 | 0.7496 |
|                                                                     |                                                                                                | H(8k)                           | 0.3081 | 0.1687 | 0.7807 |
|                                                                     |                                                                                                | H(8k)                           | 0.1687 | 0.2194 | 0.6918 |
|                                                                     |                                                                                                | H(8k)                           | 0.2193 | 0.3081 | 0.8313 |
|                                                                     |                                                                                                | H(8k)                           | 0.3118 | 0.3117 | 0.6883 |
|                                                                     |                                                                                                | Ho(2a)                          | 0.0000 | 0.0000 | 0.0000 |
|                                                                     |                                                                                                | Ho(2c)                          | 0.0000 | 0.0000 | 0.5000 |
|                                                                     |                                                                                                | Ho(2d)                          | 0.0000 | 0.5000 | 0.0000 |
|                                                                     |                                                                                                | Ho(2b)                          | 0.5000 | 0.0000 | 0.0000 |
|                                                                     |                                                                                                | N(8k)                           | 0.2512 | 0.2512 | 0.7488 |
| HoNH <sub>4</sub> B <sub>6</sub> C <sub>6</sub><br><i>P</i> 1 (1)   | a = 4.8159<br>b = 4.8423<br>c = 4.8924<br>$\alpha$ = 89.6<br>$\beta$ = 89.9<br>$\gamma$ = 89.9 | Ho(1a)                          | 0.8096 | 0.8102 | 0.8098 |
|                                                                     |                                                                                                | N(1a)                           | 0.3053 | 0.3054 | 0.3048 |
|                                                                     |                                                                                                | H(1a)                           | 0.1782 | 0.1829 | 0.1931 |
|                                                                     |                                                                                                | H(1a)                           | 0.3731 | 0.4635 | 0.1834 |
|                                                                     |                                                                                                | H(1a)                           | 0.4685 | 0.1891 | 0.3716 |
|                                                                     |                                                                                                | H(1a)                           | 0.1966 | 0.3815 | 0.4665 |
|                                                                     |                                                                                                | B(1a)                           | 0.3092 | 0.0560 | 0.8056 |
|                                                                     |                                                                                                | B(1a)                           | 0.0638 | 0.8046 | 0.3096 |
|                                                                     |                                                                                                | B(1a)                           | 0.8051 | 0.3093 | 0.0605 |
|                                                                     |                                                                                                | B(1a)                           | 0.3090 | 0.5599 | 0.8057 |
|                                                                     |                                                                                                | B(1a)                           | 0.5515 | 0.8046 | 0.3091 |
|                                                                     |                                                                                                | B(1a)                           | 0.8057 | 0.3096 | 0.5552 |
|                                                                     |                                                                                                | C(1a)                           | 0.3080 | 0.8076 | 0.0470 |
|                                                                     |                                                                                                | C(1a)                           | 0.0460 | 0.3078 | 0.8078 |
|                                                                     |                                                                                                | C(1a)                           | 0.8078 | 0.0472 | 0.3083 |
|                                                                     |                                                                                                | C(1a)                           | 0.3077 | 0.8076 | 0.5670 |
|                                                                     |                                                                                                | C(1a)                           | 0.5676 | 0.3077 | 0.8075 |
|                                                                     |                                                                                                | C(1a)                           | 0.8074 | 0.5655 | 0.3075 |
| KNH <sub>4</sub> B <sub>6</sub> C <sub>6</sub><br><i>I</i> 222 (1)  | a = 9.6857<br>b = 9.7888<br>c = 9.7939<br>$\alpha$ = 90<br>$\beta$ = 90<br>$\gamma$ = 90       | B(8k)                           | 0.0000 | 0.2500 | 0.1348 |
|                                                                     |                                                                                                | B(8k)                           | 0.1273 | 0.0085 | 0.2539 |
|                                                                     |                                                                                                | B(8k)                           | 0.7451 | 0.6269 | 0.4868 |
|                                                                     |                                                                                                | B(8k)                           | 0.5000 | 0.7500 | 0.8864 |
|                                                                     |                                                                                                | B(8k)                           | 0.3728 | 0.0085 | 0.2461 |
|                                                                     |                                                                                                | B(8k)                           | 0.2451 | 0.3731 | 0.0132 |
|                                                                     |                                                                                                | C(8k)                           | 0.2476 | 0.9941 | 0.1260 |
|                                                                     |                                                                                                | C(8k)                           | 0.1112 | 0.2500 | 0.0000 |
|                                                                     |                                                                                                | C(8k)                           | 0.5072 | 0.6256 | 0.7556 |
|                                                                     |                                                                                                | C(8k)                           | 0.2524 | 0.9941 | 0.3740 |
|                                                                     |                                                                                                | C(8k)                           | 0.8663 | 0.7500 | 0.5000 |
|                                                                     |                                                                                                | C(8k)                           | 0.9928 | 0.3744 | 0.2556 |
|                                                                     |                                                                                                | H(8k)                           | 0.1642 | 0.3104 | 0.2525 |
|                                                                     |                                                                                                | H(8k)                           | 0.2514 | 0.1869 | 0.3332 |
|                                                                     |                                                                                                | H(8k)                           | 0.7486 | 0.6869 | 0.6668 |
|                                                                     |                                                                                                | H(8k)                           | 0.8358 | 0.8104 | 0.7475 |
|                                                                     |                                                                                                | K(2a)                           | 0.0000 | 0.0000 | 0.0000 |
|                                                                     |                                                                                                | K(2c)                           | 0.0000 | 0.0000 | 0.5000 |

Continued on next page

Continued

| Compound<br>S.G.(Setting)                                          | Lattice<br>(Å,°)                                                                          | Atomic coordinates (fractional) |        |        |        |
|--------------------------------------------------------------------|-------------------------------------------------------------------------------------------|---------------------------------|--------|--------|--------|
|                                                                    |                                                                                           | Atoms                           | X      | Y      | Z      |
| LaNH <sub>4</sub> B <sub>6</sub> C <sub>6</sub><br><i>Fmmm</i> (1) | a = 9.8075<br>b = 9.6993<br>c = 9.7018<br>$\alpha = 90$<br>$\beta = 90$<br>$\gamma = 90$  | K(2b)                           | 0.5000 | 0.0000 | 0.0000 |
|                                                                    |                                                                                           | K(2d)                           | 0.0000 | 0.5000 | 0.0000 |
|                                                                    |                                                                                           | N(8k)                           | 0.2500 | 0.2494 | 0.2500 |
|                                                                    |                                                                                           | B(16m)                          | 0.0000 | 0.2513 | 0.1272 |
|                                                                    |                                                                                           | B(16o)                          | 0.7514 | 0.6290 | 0.0000 |
|                                                                    |                                                                                           | B(16n)                          | 0.6278 | 0.0000 | 0.7514 |
|                                                                    |                                                                                           | C(16n)                          | 0.2508 | 0.0000 | 0.1223 |
|                                                                    |                                                                                           | C(16m)                          | 0.0000 | 0.6218 | 0.7507 |
|                                                                    |                                                                                           | C(16o)                          | 0.6219 | 0.7507 | 0.0000 |
|                                                                    |                                                                                           | H(32p)                          | 0.8100 | 0.8105 | 0.8106 |
|                                                                    |                                                                                           | La(4a)                          | 0.0000 | 0.0000 | 0.0000 |
|                                                                    |                                                                                           | La(4b)                          | 0.0000 | 0.0000 | 0.5000 |
|                                                                    |                                                                                           | N(8f)                           | 0.2500 | 0.2500 | 0.2500 |
|                                                                    |                                                                                           |                                 |        |        |        |
| LaNH <sub>4</sub> B <sub>6</sub> C <sub>6</sub><br><i>I23</i> (1)  | a = 9.8112<br>b = 9.8112<br>c = 9.8112<br>$\alpha = 90$<br>$\beta = 90$<br>$\gamma = 90$  | B(24f)                          | 0.7497 | 0.5003 | 0.6268 |
|                                                                    |                                                                                           | B(24f)                          | 0.2495 | 0.9969 | 0.3724 |
|                                                                    |                                                                                           | C(24f)                          | 0.5009 | 0.2499 | 0.6216 |
|                                                                    |                                                                                           | C(24f)                          | 0.4980 | 0.2497 | 0.8778 |
|                                                                    |                                                                                           | H(24f)                          | 0.8074 | 0.3305 | 0.7197 |
|                                                                    |                                                                                           | H(8c)                           | 0.1889 | 0.1889 | 0.1889 |
|                                                                    |                                                                                           | La(2a)                          | 0.0000 | 0.0000 | 0.0000 |
|                                                                    |                                                                                           | La(6b)                          | 0.0000 | 0.5000 | 0.5000 |
|                                                                    |                                                                                           | N(8c)                           | 0.2488 | 0.2488 | 0.2488 |
|                                                                    |                                                                                           |                                 |        |        |        |
|                                                                    |                                                                                           |                                 |        |        |        |
| LaNH <sub>4</sub> B <sub>6</sub> C <sub>6</sub><br><i>P1</i> (1)   | a = 6.8830<br>b = 4.8444<br>c = 4.8762<br>$\alpha = 90$<br>$\beta = 135$<br>$\gamma = 90$ | La(1a)                          | 0.1933 | 0.1932 | 0.3866 |
|                                                                    |                                                                                           | N(1a)                           | 0.6933 | 0.6933 | 0.3867 |
|                                                                    |                                                                                           | H(1a)                           | 0.8130 | 0.8145 | 0.6273 |
|                                                                    |                                                                                           | H(1a)                           | 0.5715 | 0.5725 | 0.3847 |
|                                                                    |                                                                                           | H(1a)                           | 0.8151 | 0.5722 | 0.3887 |
|                                                                    |                                                                                           | H(1a)                           | 0.5737 | 0.8144 | 0.1459 |
|                                                                    |                                                                                           | B(1a)                           | 0.9391 | 0.6933 | 0.1323 |
|                                                                    |                                                                                           | B(1a)                           | 0.1933 | 0.9368 | 0.8867 |
|                                                                    |                                                                                           | B(1a)                           | 0.6936 | 0.1934 | 0.6295 |
|                                                                    |                                                                                           | B(1a)                           | 0.4475 | 0.6933 | 0.6410 |
|                                                                    |                                                                                           | B(1a)                           | 0.1933 | 0.4498 | 0.8867 |
|                                                                    |                                                                                           | B(1a)                           | 0.6931 | 0.1935 | 0.1438 |
|                                                                    |                                                                                           | C(1a)                           | 0.1933 | 0.6933 | 0.1430 |
|                                                                    |                                                                                           | C(1a)                           | 0.6933 | 0.9493 | 0.8867 |
|                                                                    |                                                                                           | C(1a)                           | 0.9491 | 0.1933 | 0.6423 |
|                                                                    |                                                                                           | C(1a)                           | 0.1933 | 0.6933 | 0.6303 |
|                                                                    |                                                                                           | C(1a)                           | 0.6933 | 0.4374 | 0.8867 |
|                                                                    |                                                                                           | C(1a)                           | 0.4376 | 0.1933 | 0.1310 |
|                                                                    |                                                                                           |                                 |        |        |        |
|                                                                    |                                                                                           |                                 |        |        |        |
| LuNH <sub>4</sub> B <sub>6</sub> C <sub>6</sub><br><i>I222</i> (1) | a = 9.6804<br>b = 9.6804<br>c = 9.6780<br>$\alpha = 90$<br>$\beta = 90$<br>$\gamma = 90$  | B(8k)                           | 0.4998 | 0.3743 | 0.7497 |
|                                                                    |                                                                                           | B(8k)                           | 0.6257 | 0.2503 | 0.4998 |
|                                                                    |                                                                                           | B(8k)                           | 0.7497 | 0.5002 | 0.6257 |
|                                                                    |                                                                                           | B(8k)                           | 0.5025 | 0.1261 | 0.7492 |
|                                                                    |                                                                                           | B(8k)                           | 0.8739 | 0.2508 | 0.5025 |
|                                                                    |                                                                                           | B(8k)                           | 0.7492 | 0.4975 | 0.8739 |
|                                                                    |                                                                                           | C(8k)                           | 0.7502 | 0.3804 | 0.5009 |
|                                                                    |                                                                                           | C(8k)                           | 0.6196 | 0.4991 | 0.7502 |
|                                                                    |                                                                                           | C(8k)                           | 0.5009 | 0.2498 | 0.6196 |
|                                                                    |                                                                                           | C(8k)                           | 0.7504 | 0.1203 | 0.4985 |
|                                                                    |                                                                                           | C(8k)                           | 0.8797 | 0.5015 | 0.7504 |
|                                                                    |                                                                                           | C(8k)                           | 0.4985 | 0.2496 | 0.8797 |
|                                                                    |                                                                                           | H(8k)                           | 0.6683 | 0.2802 | 0.8081 |
|                                                                    |                                                                                           | H(8k)                           | 0.7198 | 0.1919 | 0.6683 |
|                                                                    |                                                                                           | H(8k)                           | 0.8081 | 0.3317 | 0.7198 |
|                                                                    |                                                                                           | H(8k)                           | 0.8118 | 0.1882 | 0.8118 |
|                                                                    |                                                                                           | Lu(2a)                          | 0.0000 | 0.0000 | 0.0000 |
|                                                                    |                                                                                           | Lu(2d)                          | 0.0000 | 0.5000 | 0.0000 |
|                                                                    |                                                                                           | Lu(2b)                          | 0.5000 | 0.0000 | 0.0000 |

Continued on next page

Continued

| Compound<br>S.G.(Setting)                                          | Lattice<br>(Å, °)                                                                              | Atomic coordinates (fractional) |        |        |        |
|--------------------------------------------------------------------|------------------------------------------------------------------------------------------------|---------------------------------|--------|--------|--------|
|                                                                    |                                                                                                | Atoms                           | X      | Y      | Z      |
| LuNH <sub>4</sub> B <sub>6</sub> C <sub>6</sub><br><i>P1</i> (1)   | a = 4.7214<br>b = 4.7727<br>c = 4.9437<br>$\alpha$ = 89.4<br>$\beta$ = 89.7<br>$\gamma$ = 89.8 | Lu(2c)                          | 0.0000 | 0.0000 | 0.5000 |
|                                                                    |                                                                                                | N(8k)                           | 0.7512 | 0.2488 | 0.7512 |
|                                                                    |                                                                                                | Lu(1a)                          | 0.8136 | 0.8176 | 0.8625 |
|                                                                    |                                                                                                | N(1a)                           | 0.3045 | 0.3055 | 0.2983 |
|                                                                    |                                                                                                | H(1a)                           | 0.1694 | 0.1778 | 0.2002 |
|                                                                    |                                                                                                | H(1a)                           | 0.3501 | 0.4704 | 0.1724 |
|                                                                    |                                                                                                | H(1a)                           | 0.4812 | 0.1912 | 0.3438 |
|                                                                    |                                                                                                | H(1a)                           | 0.2087 | 0.3737 | 0.4702 |
|                                                                    |                                                                                                | B(1a)                           | 0.3107 | 0.0497 | 0.8019 |
|                                                                    |                                                                                                | B(1a)                           | 0.0707 | 0.8042 | 0.3165 |
|                                                                    |                                                                                                | B(1a)                           | 0.8059 | 0.3121 | 0.0567 |
|                                                                    |                                                                                                | B(1a)                           | 0.3105 | 0.5651 | 0.8021 |
|                                                                    |                                                                                                | B(1a)                           | 0.5429 | 0.8019 | 0.3141 |
|                                                                    |                                                                                                | B(1a)                           | 0.8055 | 0.3099 | 0.5509 |
|                                                                    |                                                                                                | C(1a)                           | 0.3092 | 0.8069 | 0.0459 |
|                                                                    |                                                                                                | C(1a)                           | 0.0444 | 0.3080 | 0.8032 |
|                                                                    |                                                                                                | C(1a)                           | 0.8081 | 0.0495 | 0.3077 |
|                                                                    |                                                                                                | C(1a)                           | 0.3073 | 0.8078 | 0.5651 |
|                                                                    |                                                                                                | C(1a)                           | 0.5699 | 0.3073 | 0.8041 |
|                                                                    |                                                                                                | C(1a)                           | 0.8075 | 0.5615 | 0.3044 |
| NaNH <sub>4</sub> B <sub>6</sub> C <sub>6</sub><br><i>I222</i> (1) | a = 9.6463<br>b = 9.5936<br>c = 9.5825<br>$\alpha$ = 90<br>$\beta$ = 90<br>$\gamma$ = 90       | B(8k)                           | 0.2478 | 0.3886 | 0.4993 |
|                                                                    |                                                                                                | B(8k)                           | 0.9999 | 0.7504 | 0.1106 |
|                                                                    |                                                                                                | B(8k)                           | 0.8838 | 0.0003 | 0.2482 |
|                                                                    |                                                                                                | B(8k)                           | 0.7404 | 0.6368 | 0.0001 |
|                                                                    |                                                                                                | B(8k)                           | 0.5003 | 0.2418 | 0.8623 |
|                                                                    |                                                                                                | B(8k)                           | 0.6333 | 0.9996 | 0.2617 |
|                                                                    |                                                                                                | C(8k)                           | 0.4999 | 0.3711 | 0.7465 |
|                                                                    |                                                                                                | C(8k)                           | 0.7508 | 0.0003 | 0.1336 |
|                                                                    |                                                                                                | C(8k)                           | 0.8663 | 0.7547 | 0.0001 |
|                                                                    |                                                                                                | C(8k)                           | 0.0006 | 0.6119 | 0.2400 |
|                                                                    |                                                                                                | C(8k)                           | 0.7546 | 0.0003 | 0.3932 |
|                                                                    |                                                                                                | C(8k)                           | 0.1058 | 0.2575 | 0.4997 |
|                                                                    |                                                                                                | H(8k)                           | 0.6927 | 0.8153 | 0.1896 |
|                                                                    |                                                                                                | H(8k)                           | 0.8086 | 0.6891 | 0.1867 |
|                                                                    |                                                                                                | H(8k)                           | 0.3150 | 0.3091 | 0.8087 |
|                                                                    |                                                                                                | H(8k)                           | 0.6879 | 0.6910 | 0.3109 |
|                                                                    |                                                                                                | N(8k)                           | 0.7501 | 0.7502 | 0.2498 |
|                                                                    |                                                                                                | Na(2a)                          | 0.0000 | 0.0000 | 0.0000 |
|                                                                    |                                                                                                | Na(2d)                          | 0.0000 | 0.5000 | 0.0000 |
|                                                                    |                                                                                                | Na(2c)                          | 0.0000 | 0.0000 | 0.5000 |
|                                                                    |                                                                                                | Na(2b)                          | 0.5000 | 0.0000 | 0.0000 |
| NdNH <sub>4</sub> B <sub>6</sub> C <sub>6</sub><br><i>Fmmm</i> (1) | a = 9.7764<br>b = 9.6671<br>c = 9.6692<br>$\alpha$ = 90<br>$\beta$ = 90<br>$\gamma$ = 90       | B(16m)                          | 0.0000 | 0.2514 | 0.1266 |
|                                                                    |                                                                                                | B(16o)                          | 0.7515 | 0.6286 | 0.0000 |
|                                                                    |                                                                                                | B(16n)                          | 0.6274 | 0.0000 | 0.7515 |
|                                                                    |                                                                                                | C(16n)                          | 0.2509 | 0.0000 | 0.1214 |
|                                                                    |                                                                                                | C(16m)                          | 0.0000 | 0.6208 | 0.7508 |
|                                                                    |                                                                                                | C(16o)                          | 0.6210 | 0.7507 | 0.0000 |
|                                                                    |                                                                                                | H(32p)                          | 0.8102 | 0.8106 | 0.8108 |
|                                                                    |                                                                                                | N(8f)                           | 0.2500 | 0.2500 | 0.2500 |
|                                                                    |                                                                                                | Nd(4a)                          | 0.0000 | 0.0000 | 0.0000 |
|                                                                    |                                                                                                | Nd(4b)                          | 0.0000 | 0.0000 | 0.5000 |
| NdNH <sub>4</sub> B <sub>6</sub> C <sub>6</sub><br><i>I222</i> (1) | a = 9.7787<br>b = 9.7807<br>c = 9.7807<br>$\alpha$ = 90<br>$\beta$ = 90<br>$\gamma$ = 90       | B(8k)                           | 0.2497 | 0.1264 | 0.9997 |
|                                                                    |                                                                                                | B(8k)                           | 0.4998 | 0.7497 | 0.6265 |
|                                                                    |                                                                                                | B(8k)                           | 0.1265 | 0.9998 | 0.2497 |
|                                                                    |                                                                                                | B(8k)                           | 0.2494 | 0.3729 | 0.0029 |
|                                                                    |                                                                                                | B(8k)                           | 0.0029 | 0.2494 | 0.3729 |
|                                                                    |                                                                                                | B(8k)                           | 0.8729 | 0.5029 | 0.7494 |
|                                                                    |                                                                                                | C(8k)                           | 0.0009 | 0.1207 | 0.2502 |
|                                                                    |                                                                                                | C(8k)                           | 0.7502 | 0.5009 | 0.6207 |

Continued on next page

Continued

| Compound<br>S.G.(Setting)                                          | Lattice<br>(Å,°) | Atomic coordinates (fractional) |        |        |        |
|--------------------------------------------------------------------|------------------|---------------------------------|--------|--------|--------|
|                                                                    |                  | Atoms                           | X      | Y      | Z      |
|                                                                    |                  | C(8k)                           | 0.1207 | 0.2502 | 0.0009 |
|                                                                    |                  | C(8k)                           | 0.4982 | 0.8786 | 0.7503 |
|                                                                    |                  | C(8k)                           | 0.2503 | 0.9982 | 0.3786 |
|                                                                    |                  | C(8k)                           | 0.3786 | 0.2503 | 0.9982 |
|                                                                    |                  | H(8k)                           | 0.3074 | 0.2203 | 0.1689 |
|                                                                    |                  | H(8k)                           | 0.6689 | 0.8075 | 0.7204 |
|                                                                    |                  | H(8k)                           | 0.2203 | 0.1690 | 0.3075 |
|                                                                    |                  | H(8k)                           | 0.8114 | 0.8113 | 0.8113 |
|                                                                    |                  | N(8k)                           | 0.2513 | 0.2513 | 0.2513 |
|                                                                    |                  | Nd(2a)                          | 0.0000 | 0.0000 | 0.0000 |
|                                                                    |                  | Nd(2d)                          | 0.0000 | 0.5000 | 0.0000 |
|                                                                    |                  | Nd(2c)                          | 0.0000 | 0.0000 | 0.5000 |
|                                                                    |                  | Nd(2b)                          | 0.5000 | 0.0000 | 0.0000 |
| NdNH <sub>4</sub> B <sub>6</sub> C <sub>6</sub><br><i>P1</i> (1)   | a = 4.8788       | Nd(1a)                          | 0.8085 | 0.8087 | 0.8086 |
|                                                                    | b = 4.8814       | N(1a)                           | 0.3053 | 0.3054 | 0.3051 |
|                                                                    | c = 4.9073       | H(1a)                           | 0.1833 | 0.1839 | 0.1887 |
|                                                                    | $\alpha = 89.9$  | H(1a)                           | 0.4650 | 0.1908 | 0.3757 |
|                                                                    | $\beta = 89.9$   | H(1a)                           | 0.1928 | 0.3794 | 0.4641 |
|                                                                    | $\gamma = 89.9$  | H(1a)                           | 0.3757 | 0.4631 | 0.1876 |
|                                                                    |                  | B(1a)                           | 0.0633 | 0.8050 | 0.3092 |
|                                                                    |                  | B(1a)                           | 0.8053 | 0.3091 | 0.0614 |
|                                                                    |                  | B(1a)                           | 0.3091 | 0.0597 | 0.8054 |
|                                                                    |                  | B(1a)                           | 0.5524 | 0.8052 | 0.3089 |
|                                                                    |                  | B(1a)                           | 0.8057 | 0.3089 | 0.5545 |
|                                                                    |                  | B(1a)                           | 0.3087 | 0.5562 | 0.8056 |
|                                                                    |                  | C(1a)                           | 0.8078 | 0.0491 | 0.3080 |
|                                                                    |                  | C(1a)                           | 0.3079 | 0.8078 | 0.0490 |
|                                                                    |                  | C(1a)                           | 0.0485 | 0.3078 | 0.8078 |
|                                                                    |                  | C(1a)                           | 0.8075 | 0.5647 | 0.3079 |
|                                                                    |                  | C(1a)                           | 0.3078 | 0.8075 | 0.5652 |
|                                                                    |                  | C(1a)                           | 0.5656 | 0.3078 | 0.8075 |
| PaNH <sub>4</sub> B <sub>6</sub> C <sub>6</sub><br><i>I222</i> (1) | a = 9.7037       | B(8k)                           | 0.2497 | 0.9999 | 0.8741 |
|                                                                    | b = 9.7061       | B(8k)                           | 0.9999 | 0.1259 | 0.7503 |
|                                                                    | c = 9.7062       | B(8k)                           | 0.1259 | 0.2497 | 0.0001 |
|                                                                    | $\alpha = 90$    | B(8k)                           | 0.2493 | 0.0016 | 0.6265 |
|                                                                    | $\beta = 90$     | B(8k)                           | 0.0016 | 0.3734 | 0.7507 |
|                                                                    | $\gamma = 90$    | B(8k)                           | 0.3734 | 0.2493 | 0.9984 |
|                                                                    |                  | C(8k)                           | 0.0007 | 0.2501 | 0.8802 |
|                                                                    |                  | C(8k)                           | 0.2501 | 0.1198 | 0.9993 |
|                                                                    |                  | C(8k)                           | 0.1198 | 0.0007 | 0.7499 |
|                                                                    |                  | C(8k)                           | 0.9993 | 0.2506 | 0.6202 |
|                                                                    |                  | C(8k)                           | 0.2506 | 0.3799 | 0.0007 |
|                                                                    |                  | C(8k)                           | 0.3798 | 0.9993 | 0.7494 |
|                                                                    |                  | H(8k)                           | 0.3078 | 0.1683 | 0.7804 |
|                                                                    |                  | H(8k)                           | 0.1683 | 0.2197 | 0.6921 |
|                                                                    |                  | H(8k)                           | 0.2196 | 0.3078 | 0.8316 |
|                                                                    |                  | H(8k)                           | 0.3118 | 0.3117 | 0.6883 |
|                                                                    |                  | N(8k)                           | 0.2512 | 0.2512 | 0.7488 |
|                                                                    |                  | Pa(2a)                          | 0.0000 | 0.0000 | 0.0000 |
|                                                                    |                  | Pa(2c)                          | 0.0000 | 0.0000 | 0.5000 |
|                                                                    |                  | Pa(2d)                          | 0.0000 | 0.5000 | 0.0000 |
|                                                                    |                  | Pa(2b)                          | 0.5000 | 0.0000 | 0.0000 |
| PaNH <sub>4</sub> B <sub>6</sub> C <sub>6</sub><br><i>P1</i> (1)   | a = 4.8393       | Pa(1a)                          | 0.1907 | 0.1907 | 0.1903 |
|                                                                    | b = 4.8653       | N(1a)                           | 0.6947 | 0.6950 | 0.6950 |
|                                                                    | c = 4.8666       | H(1a)                           | 0.8183 | 0.8144 | 0.8135 |
|                                                                    | $\alpha = 89.6$  | H(1a)                           | 0.6283 | 0.8094 | 0.5312 |
|                                                                    | $\beta = 89.9$   | H(1a)                           | 0.5305 | 0.6312 | 0.8109 |
|                                                                    | $\gamma = 89.9$  | H(1a)                           | 0.8072 | 0.5302 | 0.6292 |
|                                                                    |                  | B(1a)                           | 0.6907 | 0.1946 | 0.9406 |

Continued on next page

Continued

| Compound<br>S.G.(Setting)                                           | Lattice<br>(Å, °) | Atomic coordinates (fractional) |        |        |        |
|---------------------------------------------------------------------|-------------------|---------------------------------|--------|--------|--------|
|                                                                     |                   | Atoms                           | X      | Y      | Z      |
|                                                                     |                   | B(1a)                           | 0.9393 | 0.6906 | 0.1948 |
|                                                                     |                   | B(1a)                           | 0.1948 | 0.9391 | 0.6908 |
|                                                                     |                   | B(1a)                           | 0.6911 | 0.1941 | 0.4435 |
|                                                                     |                   | B(1a)                           | 0.4449 | 0.6910 | 0.1945 |
|                                                                     |                   | B(1a)                           | 0.1945 | 0.4451 | 0.6906 |
|                                                                     |                   | C(1a)                           | 0.6920 | 0.9533 | 0.1921 |
|                                                                     |                   | C(1a)                           | 0.9529 | 0.1922 | 0.6919 |
|                                                                     |                   | C(1a)                           | 0.1922 | 0.6914 | 0.9528 |
|                                                                     |                   | C(1a)                           | 0.6925 | 0.4323 | 0.1924 |
|                                                                     |                   | C(1a)                           | 0.4330 | 0.1924 | 0.6925 |
|                                                                     |                   | C(1a)                           | 0.1924 | 0.6930 | 0.4332 |
| PbNH <sub>4</sub> B <sub>6</sub> C <sub>6</sub><br><i>I</i> 23 (1)  | a = 9.8705        | B(24f)                          | 0.2487 | 0.9985 | 0.8768 |
|                                                                     | b = 9.8705        | B(24f)                          | 0.7513 | 0.5080 | 0.1287 |
|                                                                     | c = 9.8705        | C(24f)                          | 0.0006 | 0.2490 | 0.8756 |
|                                                                     | $\alpha = 90$     | C(24f)                          | 0.9942 | 0.2508 | 0.6235 |
|                                                                     | $\beta = 90$      | H(24f)                          | 0.3059 | 0.1682 | 0.7788 |
|                                                                     | $\gamma = 90$     | H(8c)                           | 0.6897 | 0.6897 | 0.6897 |
|                                                                     |                   | N(8c)                           | 0.7493 | 0.7493 | 0.7493 |
|                                                                     |                   | Pb(2a)                          | 0.0000 | 0.0000 | 0.0000 |
| PbNH <sub>4</sub> B <sub>6</sub> C <sub>6</sub><br><i>P</i> 1 (1)   | a = 4.8946        | Pb(6b)                          | 0.0000 | 0.5000 | 0.5000 |
|                                                                     | b = 4.8946        | B(1a)                           | 0.6962 | 0.9433 | 0.8045 |
|                                                                     | c = 4.8946        | B(1a)                           | 0.9436 | 0.1913 | 0.3095 |
|                                                                     | $\alpha = 89.8$   | B(1a)                           | 0.1935 | 0.6970 | 0.0590 |
|                                                                     | $\beta = 89.8$    | B(1a)                           | 0.6972 | 0.4460 | 0.8070 |
|                                                                     | $\gamma = 89.8$   | B(1a)                           | 0.4458 | 0.1935 | 0.3105 |
|                                                                     |                   | B(1a)                           | 0.1913 | 0.6964 | 0.5570 |
|                                                                     |                   | C(1a)                           | 0.6953 | 0.1953 | 0.0548 |
|                                                                     |                   | C(1a)                           | 0.9473 | 0.6951 | 0.8080 |
|                                                                     |                   | C(1a)                           | 0.1947 | 0.9474 | 0.3084 |
|                                                                     |                   | C(1a)                           | 0.6951 | 0.1947 | 0.5604 |
|                                                                     |                   | C(1a)                           | 0.4414 | 0.6953 | 0.8086 |
|                                                                     |                   | C(1a)                           | 0.1952 | 0.4413 | 0.3086 |
|                                                                     |                   | H(1a)                           | 0.7469 | 0.8585 | 0.1932 |
|                                                                     |                   | H(1a)                           | 0.5720 | 0.5715 | 0.1846 |
|                                                                     |                   | H(1a)                           | 0.5794 | 0.7465 | 0.4715 |
|                                                                     |                   | H(1a)                           | 0.8581 | 0.5799 | 0.3607 |
|                                                                     |                   | N(1a)                           | 0.6910 | 0.6910 | 0.3044 |
|                                                                     |                   | Pb(1a)                          | 0.1959 | 0.1959 | 0.8092 |
| PmNH <sub>4</sub> B <sub>6</sub> C <sub>6</sub><br><i>Fmm</i> (1)   | a = 9.7573        | B(16m)                          | 0.0000 | 0.2514 | 0.1264 |
|                                                                     | b = 9.6450        | B(16o)                          | 0.7515 | 0.6286 | 0.0000 |
|                                                                     | c = 9.6476        | B(16n)                          | 0.6272 | 0.0000 | 0.7516 |
|                                                                     | $\alpha = 90$     | C(16n)                          | 0.2509 | 0.0000 | 0.1212 |
|                                                                     | $\beta = 90$      | C(16m)                          | 0.0000 | 0.6206 | 0.7509 |
|                                                                     | $\gamma = 90$     | C(16o)                          | 0.6208 | 0.7507 | 0.0000 |
|                                                                     |                   | H(32p)                          | 0.8103 | 0.8107 | 0.8109 |
|                                                                     |                   | N(8f)                           | 0.2500 | 0.2500 | 0.2500 |
|                                                                     |                   | Pm(4a)                          | 0.0000 | 0.0000 | 0.0000 |
|                                                                     |                   | Pm(4b)                          | 0.0000 | 0.0000 | 0.5000 |
| PmNH <sub>4</sub> B <sub>6</sub> C <sub>6</sub><br><i>I</i> 222 (1) | a = 9.7621        | B(8k)                           | 0.1263 | 0.9998 | 0.2497 |
|                                                                     | b = 9.7621        | B(8k)                           | 0.2497 | 0.1263 | 0.9998 |
|                                                                     | c = 9.7597        | B(8k)                           | 0.4998 | 0.7497 | 0.6263 |
|                                                                     | $\alpha = 90$     | B(8k)                           | 0.8730 | 0.5028 | 0.7494 |
|                                                                     | $\beta = 90$      | B(8k)                           | 0.2494 | 0.3730 | 0.0028 |
|                                                                     | $\gamma = 90$     | B(8k)                           | 0.0028 | 0.2494 | 0.3730 |
|                                                                     |                   | C(8k)                           | 0.1205 | 0.2502 | 0.0009 |
|                                                                     |                   | C(8k)                           | 0.0009 | 0.1205 | 0.2502 |
|                                                                     |                   | C(8k)                           | 0.7502 | 0.5009 | 0.6205 |
|                                                                     |                   | C(8k)                           | 0.3789 | 0.2503 | 0.9982 |
|                                                                     |                   | C(8k)                           | 0.4982 | 0.8789 | 0.7503 |

Continued on next page



Continued

| Compound<br>S.G.(Setting)                                          | Lattice<br>(Å,°)                                                                               | Atomic coordinates (fractional) |        |        |        |
|--------------------------------------------------------------------|------------------------------------------------------------------------------------------------|---------------------------------|--------|--------|--------|
|                                                                    |                                                                                                | Atoms                           | X      | Y      | Z      |
| PmNH <sub>4</sub> B <sub>6</sub> C <sub>6</sub><br><i>P1</i> (1)   | a = 4.8771<br>b = 4.8780<br>c = 4.8870<br>$\alpha$ = 89.9<br>$\beta$ = 89.9<br>$\gamma$ = 89.9 | C(8k)                           | 0.2503 | 0.9982 | 0.3789 |
|                                                                    |                                                                                                | H(8k)                           | 0.2201 | 0.1689 | 0.3076 |
|                                                                    |                                                                                                | H(8k)                           | 0.3076 | 0.2201 | 0.1689 |
|                                                                    |                                                                                                | H(8k)                           | 0.6689 | 0.8076 | 0.7201 |
|                                                                    |                                                                                                | H(8k)                           | 0.3114 | 0.3114 | 0.3114 |
|                                                                    |                                                                                                | N(8k)                           | 0.2513 | 0.2513 | 0.2513 |
|                                                                    |                                                                                                | Pm(2a)                          | 0.0000 | 0.0000 | 0.0000 |
|                                                                    |                                                                                                | Pm(2b)                          | 0.5000 | 0.0000 | 0.0000 |
|                                                                    |                                                                                                | Pm(2d)                          | 0.0000 | 0.5000 | 0.0000 |
|                                                                    |                                                                                                | Pm(2c)                          | 0.0000 | 0.0000 | 0.5000 |
|                                                                    |                                                                                                | Pm(1a)                          | 0.8087 | 0.8087 | 0.8087 |
|                                                                    |                                                                                                | N(1a)                           | 0.3052 | 0.3053 | 0.3052 |
|                                                                    |                                                                                                | H(1a)                           | 0.1846 | 0.1846 | 0.1863 |
|                                                                    |                                                                                                | H(1a)                           | 0.4647 | 0.1904 | 0.3766 |
|                                                                    |                                                                                                | H(1a)                           | 0.1909 | 0.3777 | 0.4643 |
|                                                                    |                                                                                                | H(1a)                           | 0.3764 | 0.4641 | 0.1892 |
|                                                                    |                                                                                                | B(1a)                           | 0.0618 | 0.8051 | 0.3092 |
|                                                                    |                                                                                                | B(1a)                           | 0.8052 | 0.3091 | 0.0611 |
|                                                                    |                                                                                                | B(1a)                           | 0.3091 | 0.0605 | 0.8053 |
| PrNH <sub>4</sub> B <sub>6</sub> C <sub>6</sub><br><i>Fmmm</i> (1) | a = 9.7965<br>b = 9.6901<br>c = 9.6919<br>$\alpha$ = 90<br>$\beta$ = 90<br>$\gamma$ = 90       | B(1a)                           | 0.5539 | 0.8054 | 0.3089 |
|                                                                    |                                                                                                | B(1a)                           | 0.8055 | 0.3089 | 0.5547 |
|                                                                    |                                                                                                | B(1a)                           | 0.3089 | 0.5553 | 0.8055 |
|                                                                    |                                                                                                | C(1a)                           | 0.8078 | 0.0485 | 0.3079 |
|                                                                    |                                                                                                | C(1a)                           | 0.3079 | 0.8078 | 0.0485 |
|                                                                    |                                                                                                | C(1a)                           | 0.0483 | 0.3079 | 0.8078 |
|                                                                    |                                                                                                | C(1a)                           | 0.8075 | 0.5654 | 0.3078 |
|                                                                    |                                                                                                | C(1a)                           | 0.3078 | 0.8075 | 0.5655 |
|                                                                    |                                                                                                | C(1a)                           | 0.5657 | 0.3078 | 0.8075 |
|                                                                    |                                                                                                | B(16m)                          | 0.0000 | 0.2514 | 0.1268 |
|                                                                    |                                                                                                | B(16o)                          | 0.7515 | 0.6287 | 0.0000 |
|                                                                    |                                                                                                | B(16n)                          | 0.6275 | 0.0000 | 0.7515 |
|                                                                    |                                                                                                | C(16n)                          | 0.2509 | 0.0000 | 0.1216 |
|                                                                    |                                                                                                | C(16m)                          | 0.0000 | 0.6211 | 0.7508 |
| PrNH <sub>4</sub> B <sub>6</sub> C <sub>6</sub><br><i>I222</i> (1) | a = 9.8010<br>b = 9.8010<br>c = 9.7989<br>$\alpha$ = 90<br>$\beta$ = 90<br>$\gamma$ = 90       | C(16o)                          | 0.6212 | 0.7507 | 0.0000 |
|                                                                    |                                                                                                | H(32p)                          | 0.8101 | 0.8105 | 0.8107 |
|                                                                    |                                                                                                | N(8f)                           | 0.2500 | 0.2500 | 0.2500 |
|                                                                    |                                                                                                | Pr(4a)                          | 0.0000 | 0.0000 | 0.0000 |
|                                                                    |                                                                                                | Pr(4b)                          | 0.0000 | 0.0000 | 0.5000 |
|                                                                    |                                                                                                | B(8k)                           | 0.1266 | 0.9998 | 0.2497 |
|                                                                    |                                                                                                | B(8k)                           | 0.2497 | 0.1266 | 0.9998 |
|                                                                    |                                                                                                | B(8k)                           | 0.4998 | 0.7497 | 0.6266 |
|                                                                    |                                                                                                | B(8k)                           | 0.8727 | 0.5030 | 0.7494 |
|                                                                    |                                                                                                | B(8k)                           | 0.2494 | 0.3727 | 0.0030 |
|                                                                    |                                                                                                | B(8k)                           | 0.0030 | 0.2494 | 0.3727 |
|                                                                    |                                                                                                | C(8k)                           | 0.1210 | 0.2501 | 0.0010 |
|                                                                    |                                                                                                | C(8k)                           | 0.0010 | 0.1210 | 0.2501 |
|                                                                    |                                                                                                | C(8k)                           | 0.7501 | 0.5010 | 0.6210 |
|                                                                    |                                                                                                | C(8k)                           | 0.3784 | 0.2503 | 0.9981 |
|                                                                    |                                                                                                | C(8k)                           | 0.4981 | 0.8784 | 0.7503 |
|                                                                    |                                                                                                | C(8k)                           | 0.2503 | 0.9981 | 0.3784 |
|                                                                    |                                                                                                | H(8k)                           | 0.2206 | 0.1690 | 0.3073 |
|                                                                    |                                                                                                | H(8k)                           | 0.3073 | 0.2206 | 0.1690 |
|                                                                    |                                                                                                | H(8k)                           | 0.6690 | 0.8073 | 0.7206 |
|                                                                    |                                                                                                | H(8k)                           | 0.3113 | 0.3113 | 0.3113 |
|                                                                    |                                                                                                | N(8k)                           | 0.2513 | 0.2513 | 0.2513 |
|                                                                    |                                                                                                | Pr(2a)                          | 0.0000 | 0.0000 | 0.0000 |
|                                                                    |                                                                                                | Pr(2b)                          | 0.5000 | 0.0000 | 0.0000 |
|                                                                    |                                                                                                | Pr(2d)                          | 0.0000 | 0.5000 | 0.0000 |
|                                                                    |                                                                                                | Pr(2c)                          | 0.0000 | 0.0000 | 0.5000 |

Continued on next page

Continued

| Compound<br>S.G.(Setting)                                          | Lattice<br>(Å, °) | Atomic coordinates (fractional) |        |        |        |
|--------------------------------------------------------------------|-------------------|---------------------------------|--------|--------|--------|
|                                                                    |                   | Atoms                           | X      | Y      | Z      |
| PrNH <sub>4</sub> B <sub>6</sub> C <sub>6</sub><br><i>P1</i> (1)   | a = 4.8829        | Pr(1a)                          | 0.1916 | 0.1914 | 0.8085 |
|                                                                    | b = 4.8861        | N(1a)                           | 0.6947 | 0.6945 | 0.3050 |
|                                                                    | c = 4.9232        | H(1a)                           | 0.8177 | 0.8164 | 0.1904 |
|                                                                    | $\alpha = 90.1$   | H(1a)                           | 0.5352 | 0.8090 | 0.3753 |
|                                                                    | $\beta = 90.1$    | H(1a)                           | 0.8058 | 0.6191 | 0.4636 |
|                                                                    | $\gamma = 90$     | H(1a)                           | 0.6243 | 0.5379 | 0.1866 |
|                                                                    |                   | B(1a)                           | 0.9357 | 0.1953 | 0.3091 |
|                                                                    |                   | B(1a)                           | 0.1947 | 0.6909 | 0.0617 |
|                                                                    |                   | B(1a)                           | 0.6908 | 0.9406 | 0.8055 |
|                                                                    |                   | B(1a)                           | 0.4487 | 0.1948 | 0.3089 |
|                                                                    |                   | B(1a)                           | 0.1942 | 0.6912 | 0.5542 |
|                                                                    |                   | B(1a)                           | 0.6916 | 0.4435 | 0.8057 |
|                                                                    |                   | C(1a)                           | 0.1923 | 0.9503 | 0.3080 |
|                                                                    |                   | C(1a)                           | 0.6921 | 0.1923 | 0.0495 |
|                                                                    |                   | C(1a)                           | 0.9510 | 0.6922 | 0.8078 |
|                                                                    |                   | C(1a)                           | 0.1926 | 0.4359 | 0.3079 |
|                                                                    |                   | C(1a)                           | 0.6922 | 0.1926 | 0.5648 |
|                                                                    |                   | C(1a)                           | 0.4347 | 0.6922 | 0.8075 |
| SmNH <sub>4</sub> B <sub>6</sub> C <sub>6</sub><br><i>Fmmm</i> (1) | a = 9.7453        | B(16m)                          | 0.0000 | 0.2514 | 0.1263 |
|                                                                    | b = 9.6303        | B(16o)                          | 0.7515 | 0.6285 | 0.0000 |
|                                                                    | c = 9.6332        | B(16n)                          | 0.6271 | 0.0000 | 0.7516 |
|                                                                    | $\alpha = 90$     | C(16n)                          | 0.2509 | 0.0000 | 0.1210 |
|                                                                    | $\beta = 90$      | C(16m)                          | 0.0000 | 0.6204 | 0.7509 |
|                                                                    | $\gamma = 90$     | C(16o)                          | 0.6207 | 0.7507 | 0.0000 |
|                                                                    |                   | H(32p)                          | 0.8104 | 0.8108 | 0.8110 |
|                                                                    |                   | N(8f)                           | 0.2500 | 0.2500 | 0.2500 |
|                                                                    |                   | Sm(4a)                          | 0.0000 | 0.0000 | 0.0000 |
|                                                                    |                   | Sm(4b)                          | 0.0000 | 0.0000 | 0.5000 |
| SmNH <sub>4</sub> B <sub>6</sub> C <sub>6</sub><br><i>I222</i> (1) | a = 9.7498        | B(8k)                           | 0.1262 | 0.9998 | 0.2497 |
|                                                                    | b = 9.7498        | B(8k)                           | 0.2497 | 0.1262 | 0.9998 |
|                                                                    | c = 9.7474        | B(8k)                           | 0.9998 | 0.2497 | 0.1262 |
|                                                                    | $\alpha = 90$     | B(8k)                           | 0.3731 | 0.0027 | 0.2494 |
|                                                                    | $\beta = 90$      | B(8k)                           | 0.2494 | 0.3731 | 0.0027 |
|                                                                    | $\gamma = 90$     | B(8k)                           | 0.0027 | 0.2494 | 0.3731 |
|                                                                    |                   | C(8k)                           | 0.1204 | 0.2502 | 0.0009 |
|                                                                    |                   | C(8k)                           | 0.0009 | 0.1204 | 0.2502 |
|                                                                    |                   | C(8k)                           | 0.2502 | 0.0009 | 0.1204 |
|                                                                    |                   | C(8k)                           | 0.3790 | 0.2503 | 0.9983 |
|                                                                    |                   | C(8k)                           | 0.9983 | 0.3790 | 0.2503 |
|                                                                    |                   | C(8k)                           | 0.2503 | 0.9983 | 0.3790 |
|                                                                    |                   | H(8k)                           | 0.2199 | 0.1689 | 0.3077 |
|                                                                    |                   | H(8k)                           | 0.3077 | 0.2199 | 0.1689 |
|                                                                    |                   | H(8k)                           | 0.1689 | 0.3077 | 0.2199 |
|                                                                    |                   | H(8k)                           | 0.3115 | 0.3115 | 0.3115 |
|                                                                    |                   | N(8k)                           | 0.2513 | 0.2513 | 0.2513 |
|                                                                    |                   | Sm(2a)                          | 0.0000 | 0.0000 | 0.0000 |
|                                                                    |                   | Sm(2b)                          | 0.5000 | 0.0000 | 0.0000 |
|                                                                    |                   | Sm(2d)                          | 0.0000 | 0.5000 | 0.0000 |
|                                                                    |                   | Sm(2c)                          | 0.0000 | 0.0000 | 0.5000 |
| SmNH <sub>4</sub> B <sub>6</sub> C <sub>6</sub><br><i>P1</i> (1)   | a = 4.8706        | Sm(1a)                          | 0.8088 | 0.8088 | 0.8088 |
|                                                                    | b = 4.8769        | N(1a)                           | 0.3053 | 0.3052 | 0.3052 |
|                                                                    | c = 4.8769        | H(1a)                           | 0.1843 | 0.1853 | 0.1855 |
|                                                                    | $\alpha = 89.9$   | H(1a)                           | 0.3770 | 0.4644 | 0.1898 |
|                                                                    | $\beta = 89.9$    | H(1a)                           | 0.4647 | 0.1896 | 0.3763 |
|                                                                    | $\gamma = 89.9$   | H(1a)                           | 0.1907 | 0.3772 | 0.4648 |
|                                                                    |                   | B(1a)                           | 0.3091 | 0.0605 | 0.8053 |
|                                                                    |                   | B(1a)                           | 0.0610 | 0.8052 | 0.3092 |
|                                                                    |                   | B(1a)                           | 0.8052 | 0.3092 | 0.0613 |
|                                                                    |                   | B(1a)                           | 0.3089 | 0.5553 | 0.8055 |

Continued on next page

Continued

| Compound<br>S.G.(Setting)                                          | Lattice<br>(Å,°) | Atomic coordinates (fractional) |        |        |        |
|--------------------------------------------------------------------|------------------|---------------------------------|--------|--------|--------|
|                                                                    |                  | Atoms                           | X      | Y      | Z      |
|                                                                    |                  | B(1a)                           | 0.5548 | 0.8054 | 0.3089 |
|                                                                    |                  | B(1a)                           | 0.8055 | 0.3089 | 0.5544 |
|                                                                    |                  | C(1a)                           | 0.3079 | 0.8078 | 0.0481 |
|                                                                    |                  | C(1a)                           | 0.0480 | 0.3079 | 0.8078 |
|                                                                    |                  | C(1a)                           | 0.8078 | 0.0482 | 0.3079 |
|                                                                    |                  | C(1a)                           | 0.3078 | 0.8075 | 0.5659 |
|                                                                    |                  | C(1a)                           | 0.5658 | 0.3078 | 0.8075 |
|                                                                    |                  | C(1a)                           | 0.8075 | 0.5657 | 0.3078 |
| SrNH <sub>4</sub> B <sub>6</sub> C <sub>6</sub><br><i>Fmmm</i> (1) | a = 9.7937       | B(16m)                          | 0.0000 | 0.2516 | 0.1263 |
|                                                                    | b = 9.7372       | B(16o)                          | 0.7519 | 0.6269 | 0.0000 |
|                                                                    | c = 9.7374       | B(16n)                          | 0.6265 | 0.0000 | 0.7517 |
|                                                                    | $\alpha = 90$    | C(16n)                          | 0.2510 | 0.0000 | 0.1230 |
|                                                                    | $\beta = 90$     | C(16m)                          | 0.0000 | 0.6225 | 0.7509 |
|                                                                    | $\gamma = 90$    | C(16o)                          | 0.6227 | 0.7511 | 0.0000 |
|                                                                    |                  | H(32p)                          | 0.8100 | 0.8102 | 0.8103 |
|                                                                    |                  | N(8f)                           | 0.2500 | 0.2500 | 0.2500 |
|                                                                    |                  | Sr(4a)                          | 0.0000 | 0.0000 | 0.0000 |
|                                                                    |                  | Sr(4b)                          | 0.0000 | 0.0000 | 0.5000 |
| SrBH <sub>4</sub> B <sub>6</sub> C <sub>6</sub><br><i>I23</i> (1)  | a = 9.8013       | B(24f)                          | 0.2493 | 0.9990 | 0.8747 |
|                                                                    | b = 9.8013       | B(24f)                          | 0.7501 | 0.5061 | 0.1276 |
|                                                                    | c = 9.8013       | C(24f)                          | 0.0008 | 0.2497 | 0.8772 |
|                                                                    | $\alpha = 90$    | C(24f)                          | 0.9958 | 0.2505 | 0.6234 |
|                                                                    | $\beta = 90$     | H(24f)                          | 0.3069 | 0.1685 | 0.7792 |
|                                                                    | $\gamma = 90$    | H(8c)                           | 0.6890 | 0.6890 | 0.6890 |
|                                                                    |                  | N(8c)                           | 0.7490 | 0.7490 | 0.7490 |
|                                                                    |                  | Sr(2a)                          | 0.0000 | 0.0000 | 0.0000 |
|                                                                    |                  | Sr(6b)                          | 0.0000 | 0.5000 | 0.5000 |
| TbNH <sub>4</sub> B <sub>6</sub> C <sub>6</sub><br><i>Fmmm</i> (1) | a = 9.7057       | B(16m)                          | 0.0000 | 0.2515 | 0.1259 |
|                                                                    | b = 9.5834       | B(16o)                          | 0.7516 | 0.6284 | 0.0000 |
|                                                                    | c = 9.5873       | B(16n)                          | 0.6269 | 0.0000 | 0.7517 |
|                                                                    | $\alpha = 90$    | C(16n)                          | 0.2510 | 0.0000 | 0.1206 |
|                                                                    | $\beta = 90$     | C(16m)                          | 0.0000 | 0.6200 | 0.7510 |
|                                                                    | $\gamma = 90$    | C(16o)                          | 0.6203 | 0.7507 | 0.0000 |
|                                                                    |                  | H(32p)                          | 0.8106 | 0.8110 | 0.8112 |
|                                                                    |                  | N(8f)                           | 0.2500 | 0.2500 | 0.2500 |
|                                                                    |                  | Tb(4a)                          | 0.0000 | 0.0000 | 0.0000 |
|                                                                    |                  | Tb(4b)                          | 0.0000 | 0.0000 | 0.5000 |
| TbNH <sub>4</sub> B <sub>6</sub> C <sub>6</sub><br><i>I222</i> (1) | a = 9.7078       | B(8k)                           | 0.2497 | 0.9997 | 0.8740 |
|                                                                    | b = 9.7101       | B(8k)                           | 0.9998 | 0.1260 | 0.7503 |
|                                                                    | c = 9.7102       | B(8k)                           | 0.1260 | 0.2497 | 0.0002 |
|                                                                    | $\alpha = 90$    | B(8k)                           | 0.2493 | 0.0026 | 0.6265 |
|                                                                    | $\beta = 90$     | B(8k)                           | 0.0026 | 0.3734 | 0.7507 |
|                                                                    | $\gamma = 90$    | B(8k)                           | 0.3734 | 0.2493 | 0.9974 |
|                                                                    |                  | C(8k)                           | 0.0009 | 0.2502 | 0.8800 |
|                                                                    |                  | C(8k)                           | 0.2502 | 0.1200 | 0.9991 |
|                                                                    |                  | C(8k)                           | 0.1200 | 0.0009 | 0.7498 |
|                                                                    |                  | C(8k)                           | 0.9984 | 0.2503 | 0.6206 |
|                                                                    |                  | C(8k)                           | 0.2503 | 0.3794 | 0.0016 |
|                                                                    |                  | C(8k)                           | 0.3794 | 0.9984 | 0.7497 |
|                                                                    |                  | H(8k)                           | 0.3079 | 0.1687 | 0.7806 |
|                                                                    |                  | H(8k)                           | 0.1688 | 0.2195 | 0.6920 |
|                                                                    |                  | H(8k)                           | 0.2194 | 0.3080 | 0.8312 |
|                                                                    |                  | H(8k)                           | 0.3117 | 0.3116 | 0.6884 |
|                                                                    |                  | N(8k)                           | 0.2512 | 0.2512 | 0.7488 |
|                                                                    |                  | Tb(2a)                          | 0.0000 | 0.0000 | 0.0000 |
|                                                                    |                  | Tb(2c)                          | 0.0000 | 0.0000 | 0.5000 |
|                                                                    |                  | Tb(2d)                          | 0.0000 | 0.5000 | 0.0000 |
|                                                                    |                  | Tb(2b)                          | 0.5000 | 0.0000 | 0.0000 |
| TbNH <sub>4</sub> B <sub>6</sub> C <sub>6</sub>                    | a = 4.8304       | Tb(1a)                          | 0.8092 | 0.8095 | 0.8093 |

Continued on next page

Continued

| Compound<br>S.G.(Setting)                         | Lattice<br>(Å, °) | Atomic coordinates (fractional) |        |        |        |
|---------------------------------------------------|-------------------|---------------------------------|--------|--------|--------|
|                                                   |                   | Atoms                           | X      | Y      | Z      |
| $P1$ (1)                                          | $b = 4.8500$      | N(1a)                           | 0.3053 | 0.3055 | 0.3049 |
|                                                   | $c = 4.8923$      | H(1a)                           | 0.1797 | 0.1831 | 0.1917 |
|                                                   | $\alpha = 89.7$   | H(1a)                           | 0.3742 | 0.4633 | 0.1845 |
|                                                   | $\beta = 89.9$    | H(1a)                           | 0.4675 | 0.1895 | 0.3732 |
|                                                   | $\gamma = 89.9$   | H(1a)                           | 0.1952 | 0.3812 | 0.4658 |
|                                                   |                   | B(1a)                           | 0.3091 | 0.0569 | 0.8056 |
|                                                   |                   | B(1a)                           | 0.0635 | 0.8047 | 0.3094 |
|                                                   |                   | B(1a)                           | 0.8052 | 0.3092 | 0.0607 |
|                                                   |                   | B(1a)                           | 0.3090 | 0.5590 | 0.8057 |
|                                                   |                   | B(1a)                           | 0.5519 | 0.8048 | 0.3090 |
|                                                   |                   | B(1a)                           | 0.8057 | 0.3093 | 0.5550 |
|                                                   |                   | C(1a)                           | 0.3080 | 0.8077 | 0.0474 |
|                                                   |                   | C(1a)                           | 0.0465 | 0.3078 | 0.8078 |
|                                                   |                   | C(1a)                           | 0.8078 | 0.0476 | 0.3081 |
|                                                   |                   | C(1a)                           | 0.3077 | 0.8076 | 0.5666 |
|                                                   |                   | C(1a)                           | 0.5672 | 0.3077 | 0.8076 |
|                                                   |                   | C(1a)                           | 0.8075 | 0.5655 | 0.3077 |
| $\text{ThNH}_4\text{B}_6\text{C}_6$<br>$I23$ (1)  | $a = 9.7868$      | B(24f)                          | 0.7497 | 0.3728 | 0.5001 |
|                                                   | $b = 9.7868$      | B(24f)                          | 0.2495 | 0.6279 | 0.9980 |
|                                                   | $c = 9.7868$      | C(24f)                          | 0.5009 | 0.3791 | 0.2499 |
|                                                   | $\alpha = 90$     | C(24f)                          | 0.9988 | 0.6213 | 0.7497 |
|                                                   | $\beta = 90$      | H(24f)                          | 0.8076 | 0.2805 | 0.3307 |
|                                                   | $\gamma = 90$     | H(8c)                           | 0.8113 | 0.8113 | 0.8113 |
|                                                   |                   | N(8c)                           | 0.7513 | 0.7513 | 0.7513 |
|                                                   |                   | Th(2a)                          | 0.0000 | 0.0000 | 0.0000 |
|                                                   |                   | Th(6b)                          | 0.0000 | 0.5000 | 0.5000 |
|                                                   |                   |                                 |        |        |        |
| $\text{ThNH}_4\text{B}_6\text{C}_6$<br>$P1$ (1)   | $a = 4.8855$      | Th(1a)                          | 0.1919 | 0.1918 | 0.8081 |
|                                                   | $b = 4.8860$      | N(1a)                           | 0.6946 | 0.6947 | 0.3052 |
|                                                   | $c = 4.8989$      | H(1a)                           | 0.8160 | 0.8152 | 0.1868 |
|                                                   | $\alpha = 90.1$   | H(1a)                           | 0.5352 | 0.8093 | 0.3758 |
|                                                   | $\beta = 90.1$    | H(1a)                           | 0.8082 | 0.6226 | 0.4646 |
|                                                   | $\gamma = 90.1$   | H(1a)                           | 0.6235 | 0.5357 | 0.1896 |
|                                                   |                   | B(1a)                           | 0.9366 | 0.1948 | 0.3089 |
|                                                   |                   | B(1a)                           | 0.1947 | 0.6911 | 0.0629 |
|                                                   |                   | B(1a)                           | 0.6909 | 0.9373 | 0.8054 |
|                                                   |                   | B(1a)                           | 0.4476 | 0.1943 | 0.3087 |
|                                                   |                   | B(1a)                           | 0.1942 | 0.6913 | 0.5529 |
|                                                   |                   | B(1a)                           | 0.6917 | 0.4469 | 0.8058 |
|                                                   |                   | C(1a)                           | 0.1923 | 0.9507 | 0.3078 |
|                                                   |                   | C(1a)                           | 0.6922 | 0.1922 | 0.0492 |
|                                                   |                   | C(1a)                           | 0.9509 | 0.6923 | 0.8078 |
|                                                   |                   | C(1a)                           | 0.1925 | 0.4351 | 0.3077 |
|                                                   |                   | C(1a)                           | 0.6923 | 0.1925 | 0.5652 |
|                                                   |                   | C(1a)                           | 0.4348 | 0.6922 | 0.8076 |
| $\text{TmNH}_4\text{B}_6\text{C}_6$<br>$I222$ (1) | $a = 9.6759$      | B(8k)                           | 0.3741 | 0.4997 | 0.2503 |
|                                                   | $b = 9.6759$      | B(8k)                           | 0.7503 | 0.1259 | 0.0003 |
|                                                   | $c = 9.6734$      | B(8k)                           | 0.0003 | 0.2497 | 0.8741 |
|                                                   | $\alpha = 90$     | B(8k)                           | 0.6263 | 0.0025 | 0.7507 |
|                                                   | $\beta = 90$      | B(8k)                           | 0.2507 | 0.8737 | 0.4975 |
|                                                   | $\gamma = 90$     | B(8k)                           | 0.9975 | 0.2493 | 0.6263 |
|                                                   |                   | C(8k)                           | 0.3804 | 0.7502 | 0.4991 |
|                                                   |                   | C(8k)                           | 0.9991 | 0.1196 | 0.7498 |
|                                                   |                   | C(8k)                           | 0.7498 | 0.0009 | 0.8804 |
|                                                   |                   | C(8k)                           | 0.6203 | 0.2504 | 0.0015 |
|                                                   |                   | C(8k)                           | 0.0015 | 0.3797 | 0.7496 |
|                                                   |                   | C(8k)                           | 0.2496 | 0.4985 | 0.1203 |
|                                                   |                   | H(8k)                           | 0.2809 | 0.6687 | 0.1917 |
|                                                   |                   | H(8k)                           | 0.6917 | 0.2191 | 0.8313 |
|                                                   |                   | H(8k)                           | 0.8313 | 0.3083 | 0.7809 |
|                                                   |                   |                                 |        |        |        |
|                                                   |                   |                                 |        |        |        |

Continued on next page

Continued

| Compound<br>S.G.(Setting)                                          | Lattice<br>(Å,°)                                                                               | Atomic coordinates (fractional) |        |        |        |
|--------------------------------------------------------------------|------------------------------------------------------------------------------------------------|---------------------------------|--------|--------|--------|
|                                                                    |                                                                                                | Atoms                           | X      | Y      | Z      |
| TmNH <sub>4</sub> B <sub>6</sub> C <sub>6</sub><br><i>P1</i> (1)   | a = 4.8029<br>b = 4.8351<br>c = 4.8921<br>$\alpha$ = 89.6<br>$\beta$ = 89.8<br>$\gamma$ = 89.9 | H(8k)                           | 0.6882 | 0.3118 | 0.6882 |
|                                                                    |                                                                                                | N(8k)                           | 0.7488 | 0.2512 | 0.7488 |
|                                                                    |                                                                                                | Tm(2a)                          | 0.0000 | 0.0000 | 0.0000 |
|                                                                    |                                                                                                | Tm(2b)                          | 0.5000 | 0.0000 | 0.0000 |
|                                                                    |                                                                                                | Tm(2d)                          | 0.0000 | 0.5000 | 0.0000 |
|                                                                    |                                                                                                | Tm(2c)                          | 0.0000 | 0.0000 | 0.5000 |
|                                                                    |                                                                                                | Tm(1a)                          | 0.8102 | 0.8112 | 0.8108 |
|                                                                    |                                                                                                | N(1a)                           | 0.3053 | 0.3054 | 0.3047 |
|                                                                    |                                                                                                | H(1a)                           | 0.1768 | 0.1826 | 0.1945 |
|                                                                    |                                                                                                | H(1a)                           | 0.3722 | 0.4635 | 0.1822 |
|                                                                    |                                                                                                | H(1a)                           | 0.4694 | 0.1888 | 0.3704 |
|                                                                    |                                                                                                | H(1a)                           | 0.1977 | 0.3819 | 0.4670 |
|                                                                    |                                                                                                | B(1a)                           | 0.3093 | 0.0553 | 0.8055 |
|                                                                    |                                                                                                | B(1a)                           | 0.0639 | 0.8044 | 0.3097 |
|                                                                    |                                                                                                | B(1a)                           | 0.8050 | 0.3094 | 0.0602 |
|                                                                    |                                                                                                | B(1a)                           | 0.3091 | 0.5605 | 0.8057 |
|                                                                    |                                                                                                | B(1a)                           | 0.5512 | 0.8044 | 0.3092 |
|                                                                    |                                                                                                | B(1a)                           | 0.8057 | 0.3099 | 0.5554 |
|                                                                    |                                                                                                | C(1a)                           | 0.3080 | 0.8075 | 0.0466 |
| UNH <sub>4</sub> B <sub>6</sub> C <sub>6</sub><br><i>P1</i> (1)    | a = 4.8159<br>b = 4.8604<br>c = 4.8618<br>$\alpha$ = 89.5<br>$\beta$ = 89.9<br>$\gamma$ = 89.8 | C(1a)                           | 0.0455 | 0.3078 | 0.8077 |
|                                                                    |                                                                                                | C(1a)                           | 0.8078 | 0.0468 | 0.3084 |
|                                                                    |                                                                                                | C(1a)                           | 0.3076 | 0.8076 | 0.5673 |
|                                                                    |                                                                                                | C(1a)                           | 0.5679 | 0.3076 | 0.8075 |
|                                                                    |                                                                                                | C(1a)                           | 0.8074 | 0.5655 | 0.3073 |
|                                                                    |                                                                                                | U(1a)                           | 0.1897 | 0.1888 | 0.1877 |
|                                                                    |                                                                                                | N(1a)                           | 0.6947 | 0.6952 | 0.6951 |
|                                                                    |                                                                                                | H(1a)                           | 0.8202 | 0.8135 | 0.8131 |
|                                                                    |                                                                                                | H(1a)                           | 0.6268 | 0.8106 | 0.5322 |
|                                                                    |                                                                                                | H(1a)                           | 0.5305 | 0.6313 | 0.8125 |
|                                                                    |                                                                                                | H(1a)                           | 0.8064 | 0.5302 | 0.6276 |
|                                                                    |                                                                                                | B(1a)                           | 0.6906 | 0.1949 | 0.9427 |
|                                                                    |                                                                                                | B(1a)                           | 0.9403 | 0.6904 | 0.1952 |
|                                                                    |                                                                                                | B(1a)                           | 0.1951 | 0.9399 | 0.6905 |
|                                                                    |                                                                                                | B(1a)                           | 0.6910 | 0.1942 | 0.4417 |
|                                                                    |                                                                                                | B(1a)                           | 0.4441 | 0.6908 | 0.1950 |
|                                                                    |                                                                                                | B(1a)                           | 0.1947 | 0.4447 | 0.6903 |
|                                                                    |                                                                                                | C(1a)                           | 0.6920 | 0.9544 | 0.1924 |
|                                                                    |                                                                                                | C(1a)                           | 0.9539 | 0.1924 | 0.6919 |
| YbNH <sub>4</sub> B <sub>6</sub> C <sub>6</sub><br><i>Fmmm</i> (1) | a = 9.6618<br>b = 9.6618<br>c = 9.6588<br>$\alpha$ = 90<br>$\beta$ = 90<br>$\gamma$ = 90       | C(1a)                           | 0.1923 | 0.6910 | 0.9537 |
|                                                                    |                                                                                                | C(1a)                           | 0.6926 | 0.4317 | 0.1926 |
|                                                                    |                                                                                                | C(1a)                           | 0.4326 | 0.1926 | 0.6926 |
|                                                                    |                                                                                                | C(1a)                           | 0.1926 | 0.6935 | 0.4332 |
|                                                                    |                                                                                                | B(16o)                          | 0.1255 | 0.2520 | 0.0000 |
|                                                                    |                                                                                                | B(16m)                          | 0.0000 | 0.1255 | 0.7480 |
|                                                                    |                                                                                                | B(16n)                          | 0.7520 | 0.0000 | 0.3745 |
|                                                                    |                                                                                                | C(16n)                          | 0.1213 | 0.0000 | 0.7488 |
|                                                                    |                                                                                                | C(16o)                          | 0.2512 | 0.1213 | 0.0000 |
|                                                                    |                                                                                                | C(16m)                          | 0.0000 | 0.2512 | 0.8787 |
| YbNH <sub>4</sub> B <sub>6</sub> C <sub>6</sub><br><i>I222</i> (1) | a = 9.5213<br>b = 9.5304<br>c = 9.6621<br>$\alpha$ = 90<br>$\beta$ = 90<br>$\gamma$ = 90       | H(32p)                          | 0.8107 | 0.3107 | 0.6893 |
|                                                                    |                                                                                                | N(8f)                           | 0.2500 | 0.2500 | 0.2500 |
|                                                                    |                                                                                                | Yb(4a)                          | 0.0000 | 0.0000 | 0.0000 |
|                                                                    |                                                                                                | Yb(4b)                          | 0.0000 | 0.0000 | 0.5000 |
|                                                                    |                                                                                                | B(8k)                           | 0.1347 | 0.0008 | 0.2531 |
|                                                                    |                                                                                                | B(8k)                           | 0.2497 | 0.1245 | 0.0001 |
|                                                                    |                                                                                                | B(8k)                           | 0.4996 | 0.7455 | 0.6333 |
|                                                                    |                                                                                                | B(8k)                           | 0.8795 | 0.5025 | 0.7464 |
|                                                                    |                                                                                                | B(8k)                           | 0.2429 | 0.3747 | 0.0034 |
|                                                                    |                                                                                                | B(8k)                           | 0.0025 | 0.2470 | 0.3810 |
|                                                                    |                                                                                                | C(8k)                           | 0.1112 | 0.2492 | 0.0008 |
|                                                                    |                                                                                                |                                 |        |        |        |

Continued on next page

Continued

| Compound<br>S.G.(Setting)                                         | Lattice<br>(Å, °) | Atomic coordinates (fractional) |        |        |        |
|-------------------------------------------------------------------|-------------------|---------------------------------|--------|--------|--------|
|                                                                   |                   | Atoms                           | X      | Y      | Z      |
|                                                                   |                   | C(8k)                           | 0.0011 | 0.1123 | 0.2529 |
|                                                                   |                   | C(8k)                           | 0.7522 | 0.5015 | 0.6210 |
|                                                                   |                   | C(8k)                           | 0.3717 | 0.2524 | 0.9983 |
|                                                                   |                   | C(8k)                           | 0.4982 | 0.8712 | 0.7545 |
|                                                                   |                   | C(8k)                           | 0.2558 | 0.9977 | 0.3782 |
|                                                                   |                   | H(8k)                           | 0.2314 | 0.1655 | 0.3111 |
|                                                                   |                   | H(8k)                           | 0.3080 | 0.2271 | 0.1660 |
|                                                                   |                   | H(8k)                           | 0.6630 | 0.8056 | 0.7295 |
|                                                                   |                   | H(8k)                           | 0.8115 | 0.8170 | 0.8119 |
|                                                                   |                   | N(8k)                           | 0.2526 | 0.2519 | 0.2528 |
|                                                                   |                   | Yb(2a)                          | 0.0000 | 0.0000 | 0.0000 |
|                                                                   |                   | Yb(2b)                          | 0.5000 | 0.0000 | 0.0000 |
|                                                                   |                   | Yb(2d)                          | 0.0000 | 0.5000 | 0.0000 |
|                                                                   |                   | Yb(2c)                          | 0.0000 | 0.0000 | 0.5000 |
| YNH <sub>4</sub> B <sub>6</sub> C <sub>6</sub><br><i>Fmmm</i> (1) | a = 9.6985        | B(16m)                          | 0.0000 | 0.2516 | 0.1261 |
|                                                                   | b = 9.6332        | B(16o)                          | 0.7517 | 0.6273 | 0.0000 |
|                                                                   | c = 9.6341        | B(16n)                          | 0.6266 | 0.0000 | 0.7517 |
|                                                                   | $\alpha = 90$     | C(16n)                          | 0.2510 | 0.0000 | 0.1203 |
|                                                                   | $\beta = 90$      | C(16m)                          | 0.0000 | 0.6199 | 0.7510 |
|                                                                   | $\gamma = 90$     | C(16o)                          | 0.6201 | 0.7509 | 0.0000 |
|                                                                   |                   | H(32p)                          | 0.8106 | 0.8108 | 0.8109 |
|                                                                   |                   | N(8f)                           | 0.2500 | 0.2500 | 0.2500 |
|                                                                   |                   | Y(4a)                           | 0.0000 | 0.0000 | 0.0000 |
|                                                                   |                   | Y(4b)                           | 0.0000 | 0.0000 | 0.5000 |
| YNH <sub>4</sub> B <sub>6</sub> C <sub>6</sub><br><i>I23</i> (1)  | a = 9.7023        | B(24f)                          | 0.7497 | 0.5002 | 0.6260 |
|                                                                   | b = 9.7023        | B(24f)                          | 0.2493 | 0.9975 | 0.3736 |
|                                                                   | c = 9.7023        | C(24f)                          | 0.5009 | 0.2498 | 0.6199 |
|                                                                   | $\alpha = 90$     | C(24f)                          | 0.4984 | 0.2496 | 0.8795 |
|                                                                   | $\beta = 90$      | H(24f)                          | 0.8080 | 0.3313 | 0.7195 |
|                                                                   | $\gamma = 90$     | H(8c)                           | 0.6883 | 0.6883 | 0.6883 |
|                                                                   |                   | N(8c)                           | 0.7488 | 0.7488 | 0.7488 |
|                                                                   |                   | Y(2a)                           | 0.0000 | 0.0000 | 0.0000 |
|                                                                   |                   | Y(6b)                           | 0.0000 | 0.5000 | 0.5000 |
| YNH <sub>4</sub> B <sub>6</sub> C <sub>6</sub><br><i>P1</i> (1)   | a = 4.8234        | Y(1a)                           | 0.8095 | 0.8099 | 0.8096 |
|                                                                   | b = 4.8451        | N(1a)                           | 0.3053 | 0.3055 | 0.3048 |
|                                                                   | c = 4.8948        | H(1a)                           | 0.1787 | 0.1828 | 0.1928 |
|                                                                   | $\alpha = 89.7$   | H(1a)                           | 0.3731 | 0.4634 | 0.1837 |
|                                                                   | $\beta = 89.9$    | H(1a)                           | 0.4683 | 0.1895 | 0.3719 |
|                                                                   | $\gamma = 89.9$   | H(1a)                           | 0.1962 | 0.3814 | 0.4663 |
|                                                                   |                   | B(1a)                           | 0.3091 | 0.0563 | 0.8056 |
|                                                                   |                   | B(1a)                           | 0.0638 | 0.8046 | 0.3095 |
|                                                                   |                   | B(1a)                           | 0.8051 | 0.3093 | 0.0605 |
|                                                                   |                   | B(1a)                           | 0.3090 | 0.5596 | 0.8057 |
|                                                                   |                   | B(1a)                           | 0.5515 | 0.8047 | 0.3091 |
|                                                                   |                   | B(1a)                           | 0.8057 | 0.3095 | 0.5553 |
|                                                                   |                   | C(1a)                           | 0.3080 | 0.8077 | 0.0472 |
|                                                                   |                   | C(1a)                           | 0.0462 | 0.3078 | 0.8078 |
|                                                                   |                   | C(1a)                           | 0.8078 | 0.0474 | 0.3082 |
|                                                                   |                   | C(1a)                           | 0.3077 | 0.8076 | 0.5668 |
|                                                                   |                   | C(1a)                           | 0.5675 | 0.3077 | 0.8075 |
|                                                                   |                   | C(1a)                           | 0.8074 | 0.5655 | 0.3076 |

### 3.2 Possible synthesis paths of $\text{MNH}_4\text{B}_6\text{C}_6$ materials.

TABLE S3: Possible synthesis paths of  $\text{MNH}_4\text{B}_6\text{C}_6$  materials at ambient pressure when the reactants are elemental and binary compounds and the calculated reaction energy values.

| Compound                           | Chemical reaction                                                                                                                                                               | Reaction energy(eV) |
|------------------------------------|---------------------------------------------------------------------------------------------------------------------------------------------------------------------------------|---------------------|
| $\text{KNH}_4\text{B}_6\text{C}_6$ | $15 \text{ B}_{13}\text{C}_2 + 95 \text{ N}_2 + 4 \text{ KH} \rightarrow 3 \text{ KC}_8 + 189 \text{ BN} + \text{KB}_6\text{H}_4\text{C}_6\text{N}$                             | -459.9543           |
| $\text{KNH}_4\text{B}_6\text{C}_6$ | $3 \text{ B}_{13}\text{C}_2 + 16.71 \text{ KN}_3 + 1.792 \text{ B}_9\text{H}_{11} \rightarrow 49.12 \text{ BN} + 15.71 \text{ KH} + \text{KB}_6\text{H}_4\text{C}_6\text{N}$    | -107.1112           |
| $\text{KNH}_4\text{B}_6\text{C}_6$ | $3 \text{ B}_{13}\text{C}_2 + 15.81 \text{ KN}_3 + 2.688 \text{ B}_5\text{H}_7 \rightarrow 46.44 \text{ BN} + 14.81 \text{ KH} + \text{KB}_6\text{H}_4\text{C}_6\text{N}$       | -100.8526           |
| $\text{KNH}_4\text{B}_6\text{C}_6$ | $3 \text{ B}_{13}\text{C}_2 + 0.3636 \text{ B}_9\text{H}_{11} + \text{KB}_6 + 21.64 \text{ N}_2 \rightarrow 42.27 \text{ BN} + \text{KB}_6\text{H}_4\text{C}_6\text{N}$         | -96.0256            |
| $\text{KNH}_4\text{B}_6\text{C}_6$ | $3 \text{ B}_{13}\text{C}_2 + 0.5714 \text{ B}_5\text{H}_7 + \text{KB}_6 + 21.43 \text{ N}_2 \rightarrow 41.86 \text{ BN} + \text{KB}_6\text{H}_4\text{C}_6\text{N}$            | -95.0212            |
| $\text{KNH}_4\text{B}_6\text{C}_6$ | $3 \text{ B}_{13}\text{C}_2 + 2 \text{ H}_2 + \text{KB}_6 + 20 \text{ N}_2 \rightarrow 39 \text{ BN} + \text{KB}_6\text{H}_4\text{C}_6\text{N}$                                 | -88.2848            |
| $\text{KNH}_4\text{B}_6\text{C}_6$ | $3 \text{ B}_{13}\text{C}_2 + 1.333 \text{ H}_3\text{N} + \text{KB}_6 + 19.33 \text{ N}_2 \rightarrow 39 \text{ BN} + \text{KB}_6\text{H}_4\text{C}_6\text{N}$                  | -86.5193            |
| $\text{KNH}_4\text{B}_6\text{C}_6$ | $3 \text{ B}_{13}\text{C}_2 + 0.3636 \text{ B}_9\text{H}_{11} + \text{K} + 18.64 \text{ N}_2 \rightarrow 36.27 \text{ BN} + \text{KB}_6\text{H}_4\text{C}_6\text{N}$            | -80.8122            |
| $\text{KNH}_4\text{B}_6\text{C}_6$ | $3 \text{ B}_{13}\text{C}_2 + \text{KN}_3 + 0.3636 \text{ B}_9\text{H}_{11} + 17.14 \text{ N}_2 \rightarrow 36.27 \text{ BN} + \text{KB}_6\text{H}_4\text{C}_6\text{N}$         | -80.2030            |
| $\text{KNH}_4\text{B}_6\text{C}_6$ | $3 \text{ B}_{13}\text{C}_2 + 0.5714 \text{ B}_5\text{H}_7 + \text{K} + 18.43 \text{ N}_2 \rightarrow 35.86 \text{ BN} + \text{KB}_6\text{H}_4\text{C}_6\text{N}$               | -79.8078            |
| $\text{KNH}_4\text{B}_6\text{C}_6$ | $3 \text{ B}_{13}\text{C}_2 + \text{KN}_3 + 0.5714 \text{ B}_5\text{H}_7 + 16.93 \text{ N}_2 \rightarrow 35.86 \text{ BN} + \text{KB}_6\text{H}_4\text{C}_6\text{N}$            | -79.1985            |
| $\text{KNH}_4\text{B}_6\text{C}_6$ | $3 \text{ B}_{13}\text{C}_2 + 0.2727 \text{ B}_9\text{H}_{11} + 18.23 \text{ N}_2 + \text{KH} \rightarrow 35.45 \text{ BN} + \text{KB}_6\text{H}_4\text{C}_6\text{N}$           | -78.4900            |
| $\text{KNH}_4\text{B}_6\text{C}_6$ | $3 \text{ B}_{13}\text{C}_2 + 0.4286 \text{ B}_5\text{H}_7 + 18.07 \text{ N}_2 + \text{KH} \rightarrow 35.14 \text{ BN} + \text{KB}_6\text{H}_4\text{C}_6\text{N}$              | -77.7367            |
| $\text{KNH}_4\text{B}_6\text{C}_6$ | $1.2 \text{ H}_8\text{C}_5 + 6.6 \text{ KB}_6 + 17.3 \text{ N}_2 \rightarrow 33.6 \text{ BN} + 5.6 \text{ KH} + \text{KB}_6\text{H}_4\text{C}_6\text{N}$                        | -76.5682            |
| $\text{KNH}_4\text{B}_6\text{C}_6$ | $3 \text{ B}_{13}\text{C}_2 + 21.5 \text{ N}_2 + 4 \text{ KH} \rightarrow 3 \text{ KN}_3 + 33 \text{ BN} + \text{KB}_6\text{H}_4\text{C}_6\text{N}$                             | -73.3510            |
| $\text{KNH}_4\text{B}_6\text{C}_6$ | $3 \text{ B}_{13}\text{C}_2 + 12.42 \text{ KN}_3 + 0.3636 \text{ B}_9\text{H}_{11} \rightarrow 11.42 \text{ K} + 36.27 \text{ BN} + \text{KB}_6\text{H}_4\text{C}_6\text{N}$    | -73.2432            |
| $\text{KNH}_4\text{B}_6\text{C}_6$ | $3 \text{ B}_{13}\text{C}_2 + 2 \text{ H}_2 + \text{K} + 17 \text{ N}_2 \rightarrow 33 \text{ BN} + \text{KB}_6\text{H}_4\text{C}_6\text{N}$                                    | -73.0713            |
| $\text{KNH}_4\text{B}_6\text{C}_6$ | $3 \text{ B}_{13}\text{C}_2 + 1.5 \text{ H}_2 + 17 \text{ N}_2 + \text{KH} \rightarrow 33 \text{ BN} + \text{KB}_6\text{H}_4\text{C}_6\text{N}$                                 | -72.6843            |
| $\text{KNH}_4\text{B}_6\text{C}_6$ | $3 \text{ B}_{13}\text{C}_2 + \text{KN}_3 + 2 \text{ H}_2 + 15.5 \text{ N}_2 \rightarrow 33 \text{ BN} + \text{KB}_6\text{H}_4\text{C}_6\text{N}$                               | -72.4621            |
| $\text{KNH}_4\text{B}_6\text{C}_6$ | $3 \text{ B}_{13}\text{C}_2 + 12.29 \text{ KN}_3 + 0.5714 \text{ B}_5\text{H}_7 \rightarrow 11.29 \text{ K} + 35.86 \text{ BN} + \text{KB}_6\text{H}_4\text{C}_6\text{N}$       | -72.3232            |
| $\text{KNH}_4\text{B}_6\text{C}_6$ | $3 \text{ B}_{13}\text{C}_2 + 17 \text{ N}_2 + 4 \text{ KH} \rightarrow 3 \text{ K} + 33 \text{ BN} + \text{KB}_6\text{H}_4\text{C}_6\text{N}$                                  | -71.5234            |
| $\text{KNH}_4\text{B}_6\text{C}_6$ | $3 \text{ B}_{13}\text{C}_2 + \text{H}_3\text{N} + 16.5 \text{ N}_2 + \text{KH} \rightarrow 33 \text{ BN} + \text{KB}_6\text{H}_4\text{C}_6\text{N}$                            | -71.3603            |
| $\text{KNH}_4\text{B}_6\text{C}_6$ | $3 \text{ B}_{13}\text{C}_2 + 1.333 \text{ H}_3\text{N} + \text{K} + 16.33 \text{ N}_2 \rightarrow 33 \text{ BN} + \text{KB}_6\text{H}_4\text{C}_6\text{N}$                     | -71.3059            |
| $\text{KNH}_4\text{B}_6\text{C}_6$ | $3 \text{ B}_{13}\text{C}_2 + \text{KN}_3 + 1.333 \text{ H}_3\text{N} + 14.83 \text{ N}_2 \rightarrow 33 \text{ BN} + \text{KB}_6\text{H}_4\text{C}_6\text{N}$                  | -70.6967            |
| $\text{KNH}_4\text{B}_6\text{C}_6$ | $3 \text{ B}_{13}\text{C}_2 + 11.33 \text{ KN}_3 + 7.167 \text{ H}_2 \rightarrow 33 \text{ BN} + 10.33 \text{ KH} + \text{KB}_6\text{H}_4\text{C}_6\text{N}$                    | -70.1657            |
| $\text{KNH}_4\text{B}_6\text{C}_6$ | $3 \text{ B}_{13}\text{C}_2 + 11.33 \text{ KN}_3 + 2 \text{ H}_2 \rightarrow 10.33 \text{ K} + 33 \text{ BN} + \text{KB}_6\text{H}_4\text{C}_6\text{N}$                         | -66.1669            |
| $\text{KNH}_4\text{B}_6\text{C}_6$ | $3 \text{ B}_{13}\text{C}_2 + 34 \text{ H}_3\text{N} + 99 \text{ K} \rightarrow 33 \text{ BN} + 98 \text{ KH} + \text{KB}_6\text{H}_4\text{C}_6\text{N}$                        | -65.9770            |
| $\text{KNH}_4\text{B}_6\text{C}_6$ | $3 \text{ B}_{13}\text{C}_2 + 9.9 \text{ KN}_3 + 4.3 \text{ H}_3\text{N} \rightarrow 33 \text{ BN} + 8.9 \text{ KH} + \text{KB}_6\text{H}_4\text{C}_6\text{N}$                  | -64.7908            |
| $\text{KNH}_4\text{B}_6\text{C}_6$ | $3 \text{ B}_{13}\text{C}_2 + 10.89 \text{ KN}_3 + 1.333 \text{ H}_3\text{N} \rightarrow 9.889 \text{ K} + 33 \text{ BN} + \text{KB}_6\text{H}_4\text{C}_6\text{N}$             | -64.6723            |
| $\text{KNH}_4\text{B}_6\text{C}_6$ | $3 \text{ B}_{13}\text{C}_2 + 11.33 \text{ KN}_3 + 4 \text{ KH} \rightarrow 14.33 \text{ K} + 33 \text{ BN} + \text{KB}_6\text{H}_4\text{C}_6\text{N}$                          | -64.6190            |
| $\text{KNH}_4\text{B}_6\text{C}_6$ | $1.75 \text{ B}_{13}\text{C}_2 + 0.5 \text{ H}_8\text{C}_5 + \text{KB}_6 + 11.88 \text{ N}_2 \rightarrow 22.75 \text{ BN} + \text{KB}_6\text{H}_4\text{C}_6\text{N}$            | -47.0019            |
| $\text{KNH}_4\text{B}_6\text{C}_6$ | $2.062 \text{ B}_{13}\text{C}_2 + 0.375 \text{ H}_8\text{C}_5 + 10.91 \text{ N}_2 + \text{KH} \rightarrow 20.81 \text{ BN} + \text{KB}_6\text{H}_4\text{C}_6\text{N}$           | -41.7222            |
| $\text{KNH}_4\text{B}_6\text{C}_6$ | $6.6 \text{ KN}_3 + 1.2 \text{ H}_8\text{C}_5 + 24.8 \text{ B} \rightarrow 18.8 \text{ BN} + 5.6 \text{ KH} + \text{KB}_6\text{H}_4\text{C}_6\text{N}$                          | -35.7943            |
| $\text{KNH}_4\text{B}_6\text{C}_6$ | $3 \text{ B}_{13}\text{C}_2 + 40 \text{ H}_3\text{N} + \text{KB}_6 \rightarrow 58 \text{ H}_2 + 39 \text{ BN} + \text{KB}_6\text{H}_4\text{C}_6\text{N}$                        | -35.3220            |
| $\text{KNH}_4\text{B}_6\text{C}_6$ | $1.75 \text{ B}_{13}\text{C}_2 + 0.5 \text{ H}_8\text{C}_5 + \text{K} + 8.875 \text{ N}_2 \rightarrow 16.75 \text{ BN} + \text{KB}_6\text{H}_4\text{C}_6\text{N}$               | -31.7884            |
| $\text{KNH}_4\text{B}_6\text{C}_6$ | $3 \text{ B}_{13}\text{C}_2 + \text{KN}_3 + 31 \text{ H}_3\text{N} \rightarrow 44.5 \text{ H}_2 + 33 \text{ BN} + \text{KB}_6\text{H}_4\text{C}_6\text{N}$                      | -31.4159            |
| $\text{KNH}_4\text{B}_6\text{C}_6$ | $1.75 \text{ B}_{13}\text{C}_2 + \text{KN}_3 + 0.5 \text{ H}_8\text{C}_5 + 7.375 \text{ N}_2 \rightarrow 16.75 \text{ BN} + \text{KB}_6\text{H}_4\text{C}_6\text{N}$            | -31.1792            |
| $\text{KNH}_4\text{B}_6\text{C}_6$ | $1.75 \text{ B}_{13}\text{C}_2 + 5.917 \text{ KN}_3 + 0.5 \text{ H}_8\text{C}_5 \rightarrow 4.917 \text{ K} + 16.75 \text{ BN} + \text{KB}_6\text{H}_4\text{C}_6\text{N}$       | -28.1839            |
| $\text{KNH}_4\text{B}_6\text{C}_6$ | $3 \text{ B}_{13}\text{C}_2 + 34 \text{ H}_3\text{N} + \text{K} \rightarrow 49 \text{ H}_2 + 33 \text{ BN} + \text{KB}_6\text{H}_4\text{C}_6\text{N}$                           | -28.0529            |
| $\text{KNH}_4\text{B}_6\text{C}_6$ | $3 \text{ B}_{13}\text{C}_2 + 34 \text{ H}_3\text{N} + \text{KH} \rightarrow 49.5 \text{ H}_2 + 33 \text{ BN} + \text{KB}_6\text{H}_4\text{C}_6\text{N}$                        | -27.6660            |
| $\text{KNH}_4\text{B}_6\text{C}_6$ | $3 \text{ B}_{13}\text{C}_2 + 8 \text{ N}_2 + 4 \text{ KH} \rightarrow 3 \text{ KB}_6 + 15 \text{ BN} + \text{KB}_6\text{H}_4\text{C}_6\text{N}$                                | -25.8831            |
| $\text{KNH}_4\text{B}_6\text{C}_6$ | $14.33 \text{ KN}_3 + 1.2 \text{ H}_8\text{C}_5 + 17.2 \text{ B}_5\text{H}_7 \rightarrow 42 \text{ H}_3\text{N} + 13.33 \text{ KB}_6 + \text{KB}_6\text{H}_4\text{C}_6\text{N}$ | -20.7923            |
| $\text{KNH}_4\text{B}_6\text{C}_6$ | $3 \text{ B}_{13}\text{C}_2 + 4.808 \text{ KN}_3 + 0.3636 \text{ B}_9\text{H}_{11} \rightarrow 3.808 \text{ KB}_6 + 13.42 \text{ BN} + \text{KB}_6\text{H}_4\text{C}_6\text{N}$ | -19.9491            |
| $\text{KNH}_4\text{B}_6\text{C}_6$ | $3 \text{ B}_{13}\text{C}_2 + 4.762 \text{ KN}_3 + 0.5714 \text{ B}_5\text{H}_7 \rightarrow 3.762 \text{ KB}_6 + 13.29 \text{ BN} + \text{KB}_6\text{H}_4\text{C}_6\text{N}$    | -19.6752            |
| $\text{KNH}_4\text{B}_6\text{C}_6$ | $3 \text{ B}_{13}\text{C}_2 + 4.296 \text{ KN}_3 + 1.333 \text{ H}_3\text{N} \rightarrow 3.296 \text{ KB}_6 + 13.22 \text{ BN} + \text{KB}_6\text{H}_4\text{C}_6\text{N}$       | -18.5405            |
| $\text{KNH}_4\text{B}_6\text{C}_6$ | $3 \text{ B}_{13}\text{C}_2 + 4.444 \text{ KN}_3 + 2 \text{ H}_2 \rightarrow 3.444 \text{ KB}_6 + 12.33 \text{ BN} + \text{KB}_6\text{H}_4\text{C}_6\text{N}$                   | -17.9619            |
| $\text{KNH}_4\text{B}_6\text{C}_6$ | $3.844 \text{ KN}_3 + 1.2 \text{ H}_8\text{C}_5 + 2.756 \text{ KB}_6 \rightarrow 10.53 \text{ BN} + 5.6 \text{ KH} + \text{KB}_6\text{H}_4\text{C}_6\text{N}$                   | -15.7389            |
| $\text{KNH}_4\text{B}_6\text{C}_6$ | $3 \text{ B}_{13}\text{C}_2 + \text{KN}_3 + 10.77 \text{ H}_3\text{N} \rightarrow 4.045 \text{ B}_5\text{H}_7 + 12.77 \text{ BN} + \text{KB}_6\text{H}_4\text{C}_6\text{N}$     | -10.5073            |
| $\text{KNH}_4\text{B}_6\text{C}_6$ | $3 \text{ B}_{13}\text{C}_2 + 6.5 \text{ KN}_3 + 29.75 \text{ H}_2 \rightarrow 18.5 \text{ H}_3\text{N} + 5.5 \text{ KB}_6 + \text{KB}_6\text{H}_4\text{C}_6\text{N}$           | -9.9328             |
| $\text{KNH}_4\text{B}_6\text{C}_6$ | $3 \text{ B}_{13}\text{C}_2 + \text{KN}_3 + 9.921 \text{ H}_3\text{N} \rightarrow 2.342 \text{ B}_9\text{H}_{11} + 11.92 \text{ BN} + \text{KB}_6\text{H}_4\text{C}_6\text{N}$  | -9.4686             |
| $\text{KNH}_4\text{B}_6\text{C}_6$ | $8.833 \text{ KN}_3 + 11.5 \text{ B}_5\text{H}_7 + 0.75 \text{ KC}_8 \rightarrow 25.5 \text{ H}_3\text{N} + 8.583 \text{ KB}_6 + \text{KB}_6\text{H}_4\text{C}_6\text{N}$       | -9.3349             |
| $\text{KNH}_4\text{B}_6\text{C}_6$ | $1.097 \text{ B}_{13}\text{C}_2 + 3.088 \text{ KN}_3 + 0.7611 \text{ H}_8\text{C}_5 \rightarrow 8.265 \text{ BN} + 2.088 \text{ KH} + \text{KB}_6\text{H}_4\text{C}_6\text{N}$  | -9.1603             |
| $\text{KNH}_4\text{B}_6\text{C}_6$ | $3 \text{ B}_{13}\text{C}_2 + 13.64 \text{ H}_3\text{N} + \text{KB}_6 \rightarrow 5.273 \text{ B}_5\text{H}_7 + 12.64 \text{ BN} + \text{KB}_6\text{H}_4\text{C}_6\text{N}$     | -8.0703             |
| $\text{KNH}_4\text{B}_6\text{C}_6$ | $3 \text{ B}_{13}\text{C}_2 + 12.53 \text{ H}_3\text{N} + \text{KB}_6 \rightarrow 3.053 \text{ B}_9\text{H}_{11} + 11.53 \text{ BN} + \text{KB}_6\text{H}_4\text{C}_6\text{N}$  | -6.7164             |
| $\text{KNH}_4\text{B}_6\text{C}_6$ | $3 \text{ B}_{13}\text{C}_2 + 74.3 \text{ N}_2 + 50.2 \text{ KH} \rightarrow 49.2 \text{ KN}_3 + 6.6 \text{ B}_5\text{H}_7 + \text{KB}_6\text{H}_4\text{C}_6\text{N}$           | -5.8122             |
| $\text{KNH}_4\text{B}_6\text{C}_6$ | $1.75 \text{ B}_{13}\text{C}_2 + 2.639 \text{ KN}_3 + 0.5 \text{ H}_8\text{C}_5 \rightarrow 1.639 \text{ KB}_6 + 6.917 \text{ BN} + \text{KB}_6\text{H}_4\text{C}_6\text{N}$    | -5.2476             |

Continued on next page

Continued

| Compound                                       | Chemical reaction                                                                                                                                                                      | Reaction energy(eV) |
|------------------------------------------------|----------------------------------------------------------------------------------------------------------------------------------------------------------------------------------------|---------------------|
| KNH <sub>4</sub> B <sub>6</sub> C <sub>6</sub> | $3 \text{ B}_{13}\text{C}_2 + 11.73 \text{ H}_3\text{N} + \text{K} \rightarrow 4.455 \text{ B}_5\text{H}_7 + 10.73 \text{ BN} + \text{KB}_6\text{H}_4\text{C}_6\text{N}$               | -5.0300             |
| KNH <sub>4</sub> B <sub>6</sub> C <sub>6</sub> | $3 \text{ B}_{13}\text{C}_2 + 11.5 \text{ H}_3\text{N} + \text{KH} \rightarrow 4.5 \text{ B}_5\text{H}_7 + 10.5 \text{ BN} + \text{KB}_6\text{H}_4\text{C}_6\text{N}$                  | -4.4081             |
| KNH <sub>4</sub> B <sub>6</sub> C <sub>6</sub> | $3 \text{ B}_{13}\text{C}_2 + 65.5 \text{ N}_2 + 44.33 \text{ KH} \rightarrow 43.33 \text{ KN}_3 + 3.667 \text{ B}_9\text{H}_{11} + \text{KB}_6\text{H}_4\text{C}_6\text{N}$           | -4.2605             |
| KNH <sub>4</sub> B <sub>6</sub> C <sub>6</sub> | $3 \text{ B}_{13}\text{C}_2 + 10.79 \text{ H}_3\text{N} + \text{K} \rightarrow 2.579 \text{ B}_9\text{H}_{11} + 9.789 \text{ BN} + \text{KB}_6\text{H}_4\text{C}_6\text{N}$            | -3.8862             |
| KNH <sub>4</sub> B <sub>6</sub> C <sub>6</sub> | $3 \text{ B}_{13}\text{C}_2 + 10.55 \text{ H}_3\text{N} + \text{KH} \rightarrow 2.605 \text{ B}_9\text{H}_{11} + 9.553 \text{ BN} + \text{KB}_6\text{H}_4\text{C}_6\text{N}$           | -3.2526             |
| KNH <sub>4</sub> B <sub>6</sub> C <sub>6</sub> | $150 \text{ C} + 6 \text{ BN} + 19 \text{ KH} \rightarrow 5 \text{ H}_3\text{N} + 18 \text{ KC}_8 + \text{KB}_6\text{H}_4\text{C}_6\text{N}$                                           | -1.0066             |
| YNH <sub>4</sub> B <sub>6</sub> C <sub>6</sub> | $3 \text{ B}_{13}\text{C}_2 + 251 \text{ H}_3\text{N} + 251 \text{ YB}_2 \rightarrow 107 \text{ B}_5\text{H}_7 + 250 \text{ YN} + \text{YB}_6\text{H}_4\text{C}_6\text{N}$             | -202.7686           |
| YNH <sub>4</sub> B <sub>6</sub> C <sub>6</sub> | $3 \text{ B}_{13}\text{C}_2 + 50 \text{ Y} + 34 \text{ H}_3\text{N} \rightarrow 49 \text{ YH}_2 + 33 \text{ BN} + \text{YB}_6\text{H}_4\text{C}_6\text{N}$                             | -136.4286           |
| YNH <sub>4</sub> B <sub>6</sub> C <sub>6</sub> | $0.3636 \text{ B}_9\text{H}_{11} + 3 \text{ B}_{13}\text{C}_2 + \text{YB}_{12} + 24.64 \text{ N}_2 \rightarrow 48.27 \text{ BN} + \text{YB}_6\text{H}_4\text{C}_6\text{N}$             | -113.3094           |
| YNH <sub>4</sub> B <sub>6</sub> C <sub>6</sub> | $3 \text{ B}_{13}\text{C}_2 + \text{YB}_{12} + 0.5714 \text{ B}_5\text{H}_7 + 24.43 \text{ N}_2 \rightarrow 47.86 \text{ BN} + \text{YB}_6\text{H}_4\text{C}_6\text{N}$                | -112.3050           |
| YNH <sub>4</sub> B <sub>6</sub> C <sub>6</sub> | $3 \text{ B}_{13}\text{C}_2 + 33.67 \text{ Y} + 34 \text{ H}_3\text{N} \rightarrow 32.67 \text{ YH}_3 + 33 \text{ BN} + \text{YB}_6\text{H}_4\text{C}_6\text{N}$                       | -112.0542           |
| YNH <sub>4</sub> B <sub>6</sub> C <sub>6</sub> | $3 \text{ B}_{13}\text{C}_2 + \text{YB}_{12} + 23 \text{ N}_2 + 2 \text{ H}_2 \rightarrow 45 \text{ BN} + \text{YB}_6\text{H}_4\text{C}_6\text{N}$                                     | -105.5686           |
| YNH <sub>4</sub> B <sub>6</sub> C <sub>6</sub> | $56 \text{ H}_3\text{N} + 15.5 \text{ Y}_4\text{C}_7 + 6 \text{ BN} \rightarrow 20.5 \text{ H}_8\text{C}_5 + 61 \text{ YN} + \text{YB}_6\text{H}_4\text{C}_6\text{N}$                  | -104.3911           |
| YNH <sub>4</sub> B <sub>6</sub> C <sub>6</sub> | $3 \text{ B}_{13}\text{C}_2 + 1.333 \text{ H}_3\text{N} + \text{YB}_{12} + 22.33 \text{ N}_2 \rightarrow 45 \text{ BN} + \text{YB}_6\text{H}_4\text{C}_6\text{N}$                      | -103.8031           |
| YNH <sub>4</sub> B <sub>6</sub> C <sub>6</sub> | $2 \text{ YH}_2 + 3.875 \text{ B}_{13}\text{C}_2 + 22.69 \text{ N}_2 \rightarrow 0.25 \text{ Y}_4\text{C}_7 + 44.37 \text{ BN} + \text{YB}_6\text{H}_4\text{C}_6\text{N}$              | -102.8619           |
| YNH <sub>4</sub> B <sub>6</sub> C <sub>6</sub> | $2 \text{ YH}_2 + 3.625 \text{ B}_{13}\text{C}_2 + 21.06 \text{ N}_2 \rightarrow 0.25 \text{ Y}_4\text{C}_5 + 41.12 \text{ BN} + \text{YB}_6\text{H}_4\text{C}_6\text{N}$              | -94.7323            |
| YNH <sub>4</sub> B <sub>6</sub> C <sub>6</sub> | $0.3636 \text{ B}_9\text{H}_{11} + 3 \text{ B}_{13}\text{C}_2 + 20.64 \text{ N}_2 + \text{YB}_4 \rightarrow 40.27 \text{ BN} + \text{YB}_6\text{H}_4\text{C}_6\text{N}$                | -93.0087            |
| YNH <sub>4</sub> B <sub>6</sub> C <sub>6</sub> | $3 \text{ B}_{13}\text{C}_2 + 0.5714 \text{ B}_5\text{H}_7 + 20.43 \text{ N}_2 + \text{YB}_4 \rightarrow 39.86 \text{ BN} + \text{YB}_6\text{H}_4\text{C}_6\text{N}$                   | -92.0043            |
| YNH <sub>4</sub> B <sub>6</sub> C <sub>6</sub> | $3.8 \text{ YB}_{12} + 1.2 \text{ H}_8\text{C}_5 + 20.3 \text{ N}_2 \rightarrow 2.8 \text{ YH}_2 + 39.6 \text{ BN} + \text{YB}_6\text{H}_4\text{C}_6\text{N}$                          | -89.5966            |
| YNH <sub>4</sub> B <sub>6</sub> C <sub>6</sub> | $0.3636 \text{ B}_9\text{H}_{11} + 3 \text{ B}_{13}\text{C}_2 + 19.64 \text{ N}_2 + \text{YB}_2 \rightarrow 38.27 \text{ BN} + \text{YB}_6\text{H}_4\text{C}_6\text{N}$                | -89.1369            |
| YNH <sub>4</sub> B <sub>6</sub> C <sub>6</sub> | $3 \text{ B}_{13}\text{C}_2 + 0.5714 \text{ B}_5\text{H}_7 + 19.43 \text{ N}_2 + \text{YB}_2 \rightarrow 37.86 \text{ BN} + \text{YB}_6\text{H}_4\text{C}_6\text{N}$                   | -88.1325            |
| YNH <sub>4</sub> B <sub>6</sub> C <sub>6</sub> | $0.3636 \text{ B}_9\text{H}_{11} + 3 \text{ B}_{13}\text{C}_2 + \text{Y} + 18.64 \text{ N}_2 \rightarrow 36.27 \text{ BN} + \text{YB}_6\text{H}_4\text{C}_6\text{N}$                   | -85.7395            |
| YNH <sub>4</sub> B <sub>6</sub> C <sub>6</sub> | $3 \text{ B}_{13}\text{C}_2 + 19 \text{ N}_2 + 2 \text{ H}_2 + \text{YB}_4 \rightarrow 37 \text{ BN} + \text{YB}_6\text{H}_4\text{C}_6\text{N}$                                        | -85.2679            |
| YNH <sub>4</sub> B <sub>6</sub> C <sub>6</sub> | $3 \text{ B}_{13}\text{C}_2 + \text{Y} + 0.5714 \text{ B}_5\text{H}_7 + 18.43 \text{ N}_2 \rightarrow 35.86 \text{ BN} + \text{YB}_6\text{H}_4\text{C}_6\text{N}$                      | -84.7351            |
| YNH <sub>4</sub> B <sub>6</sub> C <sub>6</sub> | $1.333 \text{ YH}_3 + 3.292 \text{ B}_{13}\text{C}_2 + 18.9 \text{ N}_2 \rightarrow 0.08333 \text{ Y}_4\text{C}_7 + 36.79 \text{ BN} + \text{YB}_6\text{H}_4\text{C}_6\text{N}$        | -84.4664            |
| YNH <sub>4</sub> B <sub>6</sub> C <sub>6</sub> | $3 \text{ B}_{13}\text{C}_2 + 1.333 \text{ H}_3\text{N} + 18.33 \text{ N}_2 + \text{YB}_4 \rightarrow 37 \text{ BN} + \text{YB}_6\text{H}_4\text{C}_6\text{N}$                         | -83.5024            |
| YNH <sub>4</sub> B <sub>6</sub> C <sub>6</sub> | $2 \text{ YH}_2 + 3.25 \text{ B}_{13}\text{C}_2 + 18.62 \text{ N}_2 \rightarrow 0.5 \text{ Y}_2\text{C} + 36.25 \text{ BN} + \text{YB}_6\text{H}_4\text{C}_6\text{N}$                  | -82.3105            |
| YNH <sub>4</sub> B <sub>6</sub> C <sub>6</sub> | $0.3636 \text{ B}_9\text{H}_{11} + 3 \text{ B}_{13}\text{C}_2 + 18.14 \text{ N}_2 + \text{YN} \rightarrow 36.27 \text{ BN} + \text{YB}_6\text{H}_4\text{C}_6\text{N}$                  | -82.2765            |
| YNH <sub>4</sub> B <sub>6</sub> C <sub>6</sub> | $1.333 \text{ YH}_3 + 3.208 \text{ B}_{13}\text{C}_2 + 18.35 \text{ N}_2 \rightarrow 0.08333 \text{ Y}_4\text{C}_5 + 35.71 \text{ BN} + \text{YB}_6\text{H}_4\text{C}_6\text{N}$       | -81.7565            |
| YNH <sub>4</sub> B <sub>6</sub> C <sub>6</sub> | $3 \text{ B}_{13}\text{C}_2 + 18 \text{ N}_2 + 2 \text{ H}_2 + \text{YB}_2 \rightarrow 35 \text{ BN} + \text{YB}_6\text{H}_4\text{C}_6\text{N}$                                        | -81.3961            |
| YNH <sub>4</sub> B <sub>6</sub> C <sub>6</sub> | $3 \text{ B}_{13}\text{C}_2 + 0.5714 \text{ B}_5\text{H}_7 + 17.93 \text{ N}_2 + \text{YN} \rightarrow 35.86 \text{ BN} + \text{YB}_6\text{H}_4\text{C}_6\text{N}$                     | -81.2721            |
| YNH <sub>4</sub> B <sub>6</sub> C <sub>6</sub> | $6 \text{ Y}_2\text{C} + 27.6 \text{ B}_5\text{H}_7 + 32.03 \text{ N}_2 \rightarrow 63.07 \text{ H}_3\text{N} + 11 \text{ YB}_{12} + \text{YB}_6\text{H}_4\text{C}_6\text{N}$          | -81.1942            |
| YNH <sub>4</sub> B <sub>6</sub> C <sub>6</sub> | $0.1818 \text{ B}_9\text{H}_{11} + \text{YH}_2 + 3 \text{ B}_{13}\text{C}_2 + 17.82 \text{ N}_2 \rightarrow 34.64 \text{ BN} + \text{YB}_6\text{H}_4\text{C}_6\text{N}$                | -79.7579            |
| YNH <sub>4</sub> B <sub>6</sub> C <sub>6</sub> | $3 \text{ B}_{13}\text{C}_2 + 1.333 \text{ H}_3\text{N} + 17.33 \text{ N}_2 + \text{YB}_2 \rightarrow 35 \text{ BN} + \text{YB}_6\text{H}_4\text{C}_6\text{N}$                         | -79.6306            |
| YNH <sub>4</sub> B <sub>6</sub> C <sub>6</sub> | $\text{YH}_2 + 3 \text{ B}_{13}\text{C}_2 + 0.2857 \text{ B}_5\text{H}_7 + 17.71 \text{ N}_2 \rightarrow 34.43 \text{ BN} + \text{YB}_6\text{H}_4\text{C}_6\text{N}$                   | -79.2557            |
| YNH <sub>4</sub> B <sub>6</sub> C <sub>6</sub> | $3 \text{ B}_{13}\text{C}_2 + \text{Y} + 17 \text{ N}_2 + 2 \text{ H}_2 \rightarrow 33 \text{ BN} + \text{YB}_6\text{H}_4\text{C}_6\text{N}$                                           | -77.9987            |
| YNH <sub>4</sub> B <sub>6</sub> C <sub>6</sub> | $1.333 \text{ YH}_3 + 3.083 \text{ B}_{13}\text{C}_2 + 17.54 \text{ N}_2 \rightarrow 0.1667 \text{ Y}_2\text{C} + 34.08 \text{ BN} + \text{YB}_6\text{H}_4\text{C}_6\text{N}$          | -77.6159            |
| YNH <sub>4</sub> B <sub>6</sub> C <sub>6</sub> | $\text{YH}_3 + 0.09091 \text{ B}_9\text{H}_{11} + 3 \text{ B}_{13}\text{C}_2 + 17.41 \text{ N}_2 \rightarrow 33.82 \text{ BN} + \text{YB}_6\text{H}_4\text{C}_6\text{N}$               | -77.5133            |
| YNH <sub>4</sub> B <sub>6</sub> C <sub>6</sub> | $\text{YH}_3 + 3 \text{ B}_{13}\text{C}_2 + 0.1429 \text{ B}_5\text{H}_7 + 17.36 \text{ N}_2 \rightarrow 33.71 \text{ BN} + \text{YB}_6\text{H}_4\text{C}_6\text{N}$                   | -77.2622            |
| YNH <sub>4</sub> B <sub>6</sub> C <sub>6</sub> | $2 \text{ YH}_2 + 3 \text{ B}_{13}\text{C}_2 + 17.5 \text{ N}_2 \rightarrow \text{YN} + 33 \text{ BN} + \text{YB}_6\text{H}_4\text{C}_6\text{N}$                                       | -77.2393            |
| YNH <sub>4</sub> B <sub>6</sub> C <sub>6</sub> | $0.3636 \text{ B}_9\text{H}_{11} + 2.75 \text{ B}_{13}\text{C}_2 + 0.5 \text{ Y}_2\text{C} + 17.01 \text{ N}_2 \rightarrow 33.02 \text{ BN} + \text{YB}_6\text{H}_4\text{C}_6\text{N}$ | -77.2053            |
| YNH <sub>4</sub> B <sub>6</sub> C <sub>6</sub> | $3 \text{ B}_{13}\text{C}_2 + \text{Y} + 1.333 \text{ H}_3\text{N} + 16.33 \text{ N}_2 \rightarrow 33 \text{ BN} + \text{YB}_6\text{H}_4\text{C}_6\text{N}$                            | -76.2332            |
| YNH <sub>4</sub> B <sub>6</sub> C <sub>6</sub> | $2.75 \text{ B}_{13}\text{C}_2 + 0.5 \text{ Y}_2\text{C} + 0.5714 \text{ B}_5\text{H}_7 + 16.8 \text{ N}_2 \rightarrow 32.61 \text{ BN} + \text{YB}_6\text{H}_4\text{C}_6\text{N}$     | -76.2009            |
| YNH <sub>4</sub> B <sub>6</sub> C <sub>6</sub> | $1.333 \text{ YH}_3 + 3 \text{ B}_{13}\text{C}_2 + 17.17 \text{ N}_2 \rightarrow 0.3333 \text{ YN} + 33 \text{ BN} + \text{YB}_6\text{H}_4\text{C}_6\text{N}$                          | -75.9255            |
| YNH <sub>4</sub> B <sub>6</sub> C <sub>6</sub> | $\text{YH}_2 + 3 \text{ B}_{13}\text{C}_2 + 17 \text{ N}_2 + \text{H}_2 \rightarrow 33 \text{ BN} + \text{YB}_6\text{H}_4\text{C}_6\text{N}$                                           | -75.8875            |
| YNH <sub>4</sub> B <sub>6</sub> C <sub>6</sub> | $\text{YH}_3 + 3 \text{ B}_{13}\text{C}_2 + 17 \text{ N}_2 + 0.5 \text{ H}_2 \rightarrow 33 \text{ BN} + \text{YB}_6\text{H}_4\text{C}_6\text{N}$                                      | -75.5780            |
| YNH <sub>4</sub> B <sub>6</sub> C <sub>6</sub> | $2 \text{ YH}_3 + 3 \text{ B}_{13}\text{C}_2 + 17 \text{ N}_2 \rightarrow \text{YH}_2 + 33 \text{ BN} + \text{YB}_6\text{H}_4\text{C}_6\text{N}$                                       | -75.2686            |
| YNH <sub>4</sub> B <sub>6</sub> C <sub>6</sub> | $\text{YH}_3 + 3 \text{ B}_{13}\text{C}_2 + 0.3333 \text{ H}_3\text{N} + 16.83 \text{ N}_2 \rightarrow 33 \text{ BN} + \text{YB}_6\text{H}_4\text{C}_6\text{N}$                        | -75.1367            |
| YNH <sub>4</sub> B <sub>6</sub> C <sub>6</sub> | $\text{YH}_2 + 3 \text{ B}_{13}\text{C}_2 + 0.6667 \text{ H}_3\text{N} + 16.67 \text{ N}_2 \rightarrow 33 \text{ BN} + \text{YB}_6\text{H}_4\text{C}_6\text{N}$                        | -75.0048            |
| YNH <sub>4</sub> B <sub>6</sub> C <sub>6</sub> | $1.333 \text{ YH}_3 + 3 \text{ B}_{13}\text{C}_2 + 17 \text{ N}_2 \rightarrow 0.3333 \text{ Y} + 33 \text{ BN} + \text{YB}_6\text{H}_4\text{C}_6\text{N}$                              | -74.7712            |
| YNH <sub>4</sub> B <sub>6</sub> C <sub>6</sub> | $3 \text{ B}_{13}\text{C}_2 + 16.5 \text{ N}_2 + \text{YN} + 2 \text{ H}_2 \rightarrow 33 \text{ BN} + \text{YB}_6\text{H}_4\text{C}_6\text{N}$                                        | -74.5356            |
| YNH <sub>4</sub> B <sub>6</sub> C <sub>6</sub> | $3.364 \text{ B}_9\text{H}_{11} + 6 \text{ Y}_2\text{C} + 12.64 \text{ N}_2 \rightarrow 11 \text{ YH}_3 + 24.27 \text{ BN} + \text{YB}_6\text{H}_4\text{C}_6\text{N}$                  | -73.8183            |
| YNH <sub>4</sub> B <sub>6</sub> C <sub>6</sub> | $2 \text{ YH}_2 + 3 \text{ B}_{13}\text{C}_2 + 17 \text{ N}_2 \rightarrow \text{Y} + 33 \text{ BN} + \text{YB}_6\text{H}_4\text{C}_6\text{N}$                                          | -73.7763            |
| YNH <sub>4</sub> B <sub>6</sub> C <sub>6</sub> | $1.333 \text{ YH}_3 + 3 \text{ B}_{13}\text{C}_2 + 16.67 \text{ N}_2 \rightarrow 32.33 \text{ BN} + 0.3333 \text{ YB}_2 + \text{YB}_6\text{H}_4\text{C}_6\text{N}$                     | -73.6387            |
| YNH <sub>4</sub> B <sub>6</sub> C <sub>6</sub> | $3 \text{ B}_{13}\text{C}_2 + 1.333 \text{ H}_3\text{N} + 15.83 \text{ N}_2 + \text{YN} \rightarrow 33 \text{ BN} + \text{YB}_6\text{H}_4\text{C}_6\text{N}$                           | -72.7702            |
| YNH <sub>4</sub> B <sub>6</sub> C <sub>6</sub> | $1.333 \text{ YH}_3 + 3 \text{ B}_{13}\text{C}_2 + 16.33 \text{ N}_2 \rightarrow 31.67 \text{ BN} + 0.3333 \text{ YB}_4 + \text{YB}_6\text{H}_4\text{C}_6\text{N}$                     | -72.3481            |
| YNH <sub>4</sub> B <sub>6</sub> C <sub>6</sub> | $15.33 \text{ B}_9\text{H}_{11} + 6 \text{ Y}_2\text{C} + 27.94 \text{ N}_2 \rightarrow 54.89 \text{ H}_3\text{N} + 11 \text{ YB}_{12} + \text{YB}_6\text{H}_4\text{C}_6\text{N}$      | -71.4032            |
| YNH <sub>4</sub> B <sub>6</sub> C <sub>6</sub> | $2 \text{ YH}_2 + 3 \text{ B}_{13}\text{C}_2 + 16 \text{ N}_2 \rightarrow 31 \text{ BN} + \text{YB}_2 + \text{YB}_6\text{H}_4\text{C}_6\text{N}$                                       | -70.3789            |
| YNH <sub>4</sub> B <sub>6</sub> C <sub>6</sub> | $2.75 \text{ B}_{13}\text{C}_2 + 0.5 \text{ Y}_2\text{C} + 15.37 \text{ N}_2 + 2 \text{ H}_2 \rightarrow 29.75 \text{ BN} + \text{YB}_6\text{H}_4\text{C}_6\text{N}$                   | -69.4645            |
| YNH <sub>4</sub> B <sub>6</sub> C <sub>6</sub> | $12.8 \text{ B}_9\text{H}_{11} + 22.8 \text{ Y}_2\text{C} + \text{YN} \rightarrow 45.6 \text{ YH}_3 + 8.4 \text{ B}_{13}\text{C}_2 + \text{YB}_6\text{H}_4\text{C}_6\text{N}$          | -68.2358            |

Continued on next page



Continued

| Compound                                       | Chemical reaction                                                                                                                                                                                             | Reaction energy(eV) |
|------------------------------------------------|---------------------------------------------------------------------------------------------------------------------------------------------------------------------------------------------------------------|---------------------|
| YNH <sub>4</sub> B <sub>6</sub> C <sub>6</sub> | 2.75 B <sub>13</sub> C <sub>2</sub> + 0.5 Y <sub>2</sub> C + 1.333 H <sub>3</sub> N + 14.71 N <sub>2</sub> → 29.75 BN + YB <sub>6</sub> H <sub>4</sub> C <sub>6</sub> N                                       | -67.6990            |
| YNH <sub>4</sub> B <sub>6</sub> C <sub>6</sub> | 2 YH <sub>2</sub> + 3 B <sub>13</sub> C <sub>2</sub> + 15 N <sub>2</sub> → 29 BN + YB <sub>4</sub> + YB <sub>6</sub> H <sub>4</sub> C <sub>6</sub> N                                                          | -66.5071            |
| YNH <sub>4</sub> B <sub>6</sub> C <sub>6</sub> | 1.333 YH <sub>3</sub> + 3 B <sub>13</sub> C <sub>2</sub> + 15 N <sub>2</sub> → 0.3333 YB <sub>12</sub> + 29 BN + YB <sub>6</sub> H <sub>4</sub> C <sub>6</sub> N                                              | -65.5812            |
| YNH <sub>4</sub> B <sub>6</sub> C <sub>6</sub> | YH <sub>3</sub> + 2.687 B <sub>13</sub> C <sub>2</sub> + 0.125 H <sub>8</sub> C <sub>5</sub> + 14.97 N <sub>2</sub> → 28.94 BN + YB <sub>6</sub> H <sub>4</sub> C <sub>6</sub> N                              | -65.2573            |
| YNH <sub>4</sub> B <sub>6</sub> C <sub>6</sub> | 0.3636 B <sub>9</sub> H <sub>11</sub> + 2.375 B <sub>13</sub> C <sub>2</sub> + 0.25 Y <sub>4</sub> C <sub>5</sub> + 14.57 N <sub>2</sub> → 28.15 BN + YB <sub>6</sub> H <sub>4</sub> C <sub>6</sub> N         | -64.7835            |
| YNH <sub>4</sub> B <sub>6</sub> C <sub>6</sub> | 6 Y <sub>2</sub> C + 5.286 B <sub>5</sub> H <sub>7</sub> + 10.71 N <sub>2</sub> → 11 YH <sub>3</sub> + 20.43 BN + YB <sub>6</sub> H <sub>4</sub> C <sub>6</sub> N                                             | -64.5273            |
| YNH <sub>4</sub> B <sub>6</sub> C <sub>6</sub> | 11.69 B <sub>9</sub> H <sub>11</sub> + 21.26 Y <sub>2</sub> C + 0.5 N <sub>2</sub> → 41.51 YH <sub>3</sub> + 7.629 B <sub>13</sub> C <sub>2</sub> + YB <sub>6</sub> H <sub>4</sub> C <sub>6</sub> N           | -64.4227            |
| YNH <sub>4</sub> B <sub>6</sub> C <sub>6</sub> | 1.75 B <sub>13</sub> C <sub>2</sub> + YB <sub>12</sub> + 0.5 H <sub>8</sub> C <sub>5</sub> + 14.88 N <sub>2</sub> → 28.75 BN + YB <sub>6</sub> H <sub>4</sub> C <sub>6</sub> N                                | -64.2857            |
| YNH <sub>4</sub> B <sub>6</sub> C <sub>6</sub> | 12.03 B <sub>9</sub> H <sub>11</sub> + 21.89 Y <sub>2</sub> C + BN → 42.77 YH <sub>3</sub> + 7.943 B <sub>13</sub> C <sub>2</sub> + YB <sub>6</sub> H <sub>4</sub> C <sub>6</sub> N                           | -64.0356            |
| YNH <sub>4</sub> B <sub>6</sub> C <sub>6</sub> | 6 Y <sub>2</sub> C + 29.67 H <sub>3</sub> N + 17.33 YB <sub>2</sub> → 28.33 YH <sub>3</sub> + 28.67 BN + YB <sub>6</sub> H <sub>4</sub> C <sub>6</sub> N                                                      | -63.7802            |
| YNH <sub>4</sub> B <sub>6</sub> C <sub>6</sub> | 2.375 B <sub>13</sub> C <sub>2</sub> + 0.25 Y <sub>4</sub> C <sub>5</sub> + 0.5714 B <sub>5</sub> H <sub>7</sub> + 14.37 N <sub>2</sub> → 27.73 BN + YB <sub>6</sub> H <sub>4</sub> C <sub>6</sub> N          | -63.7791            |
| YNH <sub>4</sub> B <sub>6</sub> C <sub>6</sub> | 2.867 YB <sub>12</sub> + 1.2 H <sub>8</sub> C <sub>5</sub> + 14.7 N <sub>2</sub> → 1.867 YH <sub>3</sub> + 28.4 BN + YB <sub>6</sub> H <sub>4</sub> C <sub>6</sub> N                                          | -62.4719            |
| YNH <sub>4</sub> B <sub>6</sub> C <sub>6</sub> | 101 YH <sub>2</sub> + 3 B <sub>13</sub> C <sub>2</sub> + 34 H <sub>3</sub> N → 100 YH <sub>3</sub> + 33 BN + YB <sub>6</sub> H <sub>4</sub> C <sub>6</sub> N                                                  | -61.8131            |
| YNH <sub>4</sub> B <sub>6</sub> C <sub>6</sub> | 3 B <sub>13</sub> C <sub>2</sub> + 79.8 H <sub>3</sub> N + 79.8 YB <sub>2</sub> → 21.4 B <sub>9</sub> H <sub>11</sub> + 78.8 YN + YB <sub>6</sub> H <sub>4</sub> C <sub>6</sub> N                             | -60.7882            |
| YNH <sub>4</sub> B <sub>6</sub> C <sub>6</sub> | 10.57 B <sub>9</sub> H <sub>11</sub> + 19.71 Y <sub>2</sub> C + H <sub>3</sub> N → 38.43 YH <sub>3</sub> + 6.857 B <sub>13</sub> C <sub>2</sub> + YB <sub>6</sub> H <sub>4</sub> C <sub>6</sub> N             | -58.2431            |
| YNH <sub>4</sub> B <sub>6</sub> C <sub>6</sub> | 2.375 B <sub>13</sub> C <sub>2</sub> + 0.25 Y <sub>4</sub> C <sub>5</sub> + 12.94 N <sub>2</sub> + 2 H <sub>2</sub> → 24.88 BN + YB <sub>6</sub> H <sub>4</sub> C <sub>6</sub> N                              | -57.0426            |
| YNH <sub>4</sub> B <sub>6</sub> C <sub>6</sub> | 0.3636 B <sub>9</sub> H <sub>11</sub> + 2.125 B <sub>13</sub> C <sub>2</sub> + 12.95 N <sub>2</sub> + 0.25 Y <sub>4</sub> C <sub>7</sub> → 24.9 BN + YB <sub>6</sub> H <sub>4</sub> C <sub>6</sub> N          | -56.6540            |
| YNH <sub>4</sub> B <sub>6</sub> C <sub>6</sub> | 2.125 B <sub>13</sub> C <sub>2</sub> + 0.5714 B <sub>5</sub> H <sub>7</sub> + 12.74 N <sub>2</sub> + 0.25 Y <sub>4</sub> C <sub>7</sub> → 24.48 BN + YB <sub>6</sub> H <sub>4</sub> C <sub>6</sub> N          | -55.6495            |
| YNH <sub>4</sub> B <sub>6</sub> C <sub>6</sub> | 2.375 B <sub>13</sub> C <sub>2</sub> + 1.333 H <sub>3</sub> N + 0.25 Y <sub>4</sub> C <sub>5</sub> + 12.27 N <sub>2</sub> → 24.88 BN + YB <sub>6</sub> H <sub>4</sub> C <sub>6</sub> N                        | -55.2772            |
| YNH <sub>4</sub> B <sub>6</sub> C <sub>6</sub> | YH <sub>2</sub> + 2.375 B <sub>13</sub> C <sub>2</sub> + 0.25 H <sub>8</sub> C <sub>5</sub> + 12.94 N <sub>2</sub> → 24.88 BN + YB <sub>6</sub> H <sub>4</sub> C <sub>6</sub> N                               | -55.2460            |
| YNH <sub>4</sub> B <sub>6</sub> C <sub>6</sub> | 2.364 B <sub>9</sub> H <sub>11</sub> + 6 Y <sub>2</sub> C + 8.136 N <sub>2</sub> → 11 YH <sub>2</sub> + 15.27 BN + YB <sub>6</sub> H <sub>4</sub> C <sub>6</sub> N                                            | -49.1271            |
| YNH <sub>4</sub> B <sub>6</sub> C <sub>6</sub> | 2.125 B <sub>13</sub> C <sub>2</sub> + 11.31 N <sub>2</sub> + 0.25 Y <sub>4</sub> C <sub>7</sub> + 2 H <sub>2</sub> → 21.62 BN + YB <sub>6</sub> H <sub>4</sub> C <sub>6</sub> N                              | -48.9131            |
| YNH <sub>4</sub> B <sub>6</sub> C <sub>6</sub> | 2.125 B <sub>13</sub> C <sub>2</sub> + 1.333 H <sub>3</sub> N + 10.65 N <sub>2</sub> + 0.25 Y <sub>4</sub> C <sub>7</sub> → 21.62 BN + YB <sub>6</sub> H <sub>4</sub> C <sub>6</sub> N                        | -47.1477            |
| YNH <sub>4</sub> B <sub>6</sub> C <sub>6</sub> | 16.19 Y <sub>2</sub> C + 14.45 B <sub>5</sub> H <sub>7</sub> + YN → 32.39 YH <sub>3</sub> + 5.097 B <sub>13</sub> C <sub>2</sub> + YB <sub>6</sub> H <sub>4</sub> C <sub>6</sub> N                            | -46.9016            |
| YNH <sub>4</sub> B <sub>6</sub> C <sub>6</sub> | 2 YH <sub>2</sub> + 3 B <sub>13</sub> C <sub>2</sub> + 11 N <sub>2</sub> → YB <sub>12</sub> + 21 BN + YB <sub>6</sub> H <sub>4</sub> C <sub>6</sub> N                                                         | -46.2064            |
| YNH <sub>4</sub> B <sub>6</sub> C <sub>6</sub> | 8.75 Y <sub>2</sub> C + 1.2 B <sub>5</sub> H <sub>7</sub> + 8.75 N <sub>2</sub> → 0.55 H <sub>8</sub> C <sub>5</sub> + 16.5 YN + YB <sub>6</sub> H <sub>4</sub> C <sub>6</sub> N                              | -45.3484            |
| YNH <sub>4</sub> B <sub>6</sub> C <sub>6</sub> | 15.23 Y <sub>2</sub> C + 13.19 B <sub>5</sub> H <sub>7</sub> + 0.5 N <sub>2</sub> → 29.45 YH <sub>3</sub> + 4.613 B <sub>13</sub> C <sub>2</sub> + YB <sub>6</sub> H <sub>4</sub> C <sub>6</sub> N            | -44.9458            |
| YNH <sub>4</sub> B <sub>6</sub> C <sub>6</sub> | 3 B <sub>13</sub> C <sub>2</sub> + 46 H <sub>3</sub> N + YB <sub>12</sub> → 67 H <sub>2</sub> + 45 BN + YB <sub>6</sub> H <sub>4</sub> C <sub>6</sub> N                                                       | -44.6613            |
| YNH <sub>4</sub> B <sub>6</sub> C <sub>6</sub> | 15.68 Y <sub>2</sub> C + 13.58 B <sub>5</sub> H <sub>7</sub> + BN → 30.35 YH <sub>3</sub> + 4.839 B <sub>13</sub> C <sub>2</sub> + YB <sub>6</sub> H <sub>4</sub> C <sub>6</sub> N                            | -43.9872            |
| YNH <sub>4</sub> B <sub>6</sub> C <sub>6</sub> | 1.75 B <sub>13</sub> C <sub>2</sub> + 0.5 H <sub>8</sub> C <sub>5</sub> + 10.88 N <sub>2</sub> + YB <sub>4</sub> → 20.75 BN + YB <sub>6</sub> H <sub>4</sub> C <sub>6</sub> N                                 | -43.9850            |
| YNH <sub>4</sub> B <sub>6</sub> C <sub>6</sub> | 6 Y <sub>2</sub> C + 10 B <sub>5</sub> H <sub>7</sub> + 11.5 N <sub>2</sub> → 22 H <sub>3</sub> N + 11 YB <sub>4</sub> + YB <sub>6</sub> H <sub>4</sub> C <sub>6</sub> N                                      | -42.6445            |
| YNH <sub>4</sub> B <sub>6</sub> C <sub>6</sub> | 6 Y <sub>2</sub> C + 3.714 B <sub>5</sub> H <sub>7</sub> + 6.786 N <sub>2</sub> → 11 YH <sub>2</sub> + 12.57 BN + YB <sub>6</sub> H <sub>4</sub> C <sub>6</sub> N                                             | -42.5982            |
| YNH <sub>4</sub> B <sub>6</sub> C <sub>6</sub> | 0.6667 B <sub>9</sub> H <sub>11</sub> + 8.083 Y <sub>2</sub> C + 8.083 N <sub>2</sub> → 0.4167 H <sub>8</sub> C <sub>5</sub> + 15.17 YN + YB <sub>6</sub> H <sub>4</sub> C <sub>6</sub> N                     | -41.1462            |
| YNH <sub>4</sub> B <sub>6</sub> C <sub>6</sub> | 14.26 Y <sub>2</sub> C + H <sub>3</sub> N + 11.94 B <sub>5</sub> H <sub>7</sub> → 27.52 YH <sub>3</sub> + 4.129 B <sub>13</sub> C <sub>2</sub> + YB <sub>6</sub> H <sub>4</sub> C <sub>6</sub> N              | -40.6234            |
| YNH <sub>4</sub> B <sub>6</sub> C <sub>6</sub> | 3 B <sub>13</sub> C <sub>2</sub> + 34 YN + 51.5 H <sub>2</sub> → 33 YH <sub>3</sub> + 33 BN + YB <sub>6</sub> H <sub>4</sub> C <sub>6</sub> N                                                                 | -40.1354            |
| YNH <sub>4</sub> B <sub>6</sub> C <sub>6</sub> | 1.75 B <sub>13</sub> C <sub>2</sub> + 0.5 H <sub>8</sub> C <sub>5</sub> + 9.875 N <sub>2</sub> + YB <sub>2</sub> → 18.75 BN + YB <sub>6</sub> H <sub>4</sub> C <sub>6</sub> N                                 | -40.1132            |
| YNH <sub>4</sub> B <sub>6</sub> C <sub>6</sub> | 5.556 B <sub>9</sub> H <sub>11</sub> + 6 Y <sub>2</sub> C + 10.02 N <sub>2</sub> → 19.04 H <sub>3</sub> N + 11 YB <sub>4</sub> + YB <sub>6</sub> H <sub>4</sub> C <sub>6</sub> N                              | -39.0970            |
| YNH <sub>4</sub> B <sub>6</sub> C <sub>6</sub> | 2 YH <sub>2</sub> + 6 Y <sub>2</sub> C + 8.5 N <sub>2</sub> + 3 YB <sub>2</sub> → 16 YN + YB <sub>6</sub> H <sub>4</sub> C <sub>6</sub> N                                                                     | -36.9670            |
| YNH <sub>4</sub> B <sub>6</sub> C <sub>6</sub> | 1.75 B <sub>13</sub> C <sub>2</sub> + Y + 0.5 H <sub>8</sub> C <sub>5</sub> + 8.875 N <sub>2</sub> → 16.75 BN + YB <sub>6</sub> H <sub>4</sub> C <sub>6</sub> N                                               | -36.7158            |
| YNH <sub>4</sub> B <sub>6</sub> C <sub>6</sub> | 1.333 YH <sub>3</sub> + 6 Y <sub>2</sub> C + 8.167 N <sub>2</sub> + 3 YB <sub>2</sub> → 15.33 YN + YB <sub>6</sub> H <sub>4</sub> C <sub>6</sub> N                                                            | -35.6532            |
| YNH <sub>4</sub> B <sub>6</sub> C <sub>6</sub> | 3 B <sub>13</sub> C <sub>2</sub> + 17.17 H <sub>3</sub> N + 16.83 YN → 15.83 YH <sub>3</sub> + 33 BN + YB <sub>6</sub> H <sub>4</sub> C <sub>6</sub> N                                                        | -35.3006            |
| YNH <sub>4</sub> B <sub>6</sub> C <sub>6</sub> | 3 B <sub>13</sub> C <sub>2</sub> + 38 H <sub>3</sub> N + YB <sub>4</sub> → 55 H <sub>2</sub> + 37 BN + YB <sub>6</sub> H <sub>4</sub> C <sub>6</sub> N                                                        | -34.9532            |
| YNH <sub>4</sub> B <sub>6</sub> C <sub>6</sub> | 6 Y <sub>2</sub> C + 15.5 H <sub>3</sub> N + 10.25 YB <sub>2</sub> → 21.25 YH <sub>2</sub> + 14.5 BN + YB <sub>6</sub> H <sub>4</sub> C <sub>6</sub> N                                                        | -34.7512            |
| YNH <sub>4</sub> B <sub>6</sub> C <sub>6</sub> | 6 Y <sub>2</sub> C + 7.5 N <sub>2</sub> + 2 H <sub>2</sub> + 3 YB <sub>2</sub> → 14 YN + YB <sub>6</sub> H <sub>4</sub> C <sub>6</sub> N                                                                      | -34.2633            |
| YNH <sub>4</sub> B <sub>6</sub> C <sub>6</sub> | 6 Y <sub>2</sub> C + 18.11 H <sub>3</sub> N + 5.778 YB <sub>4</sub> → 16.78 YH <sub>3</sub> + 17.11 BN + YB <sub>6</sub> H <sub>4</sub> C <sub>6</sub> N                                                      | -34.2205            |
| YNH <sub>4</sub> B <sub>6</sub> C <sub>6</sub> | 8.875 B <sub>9</sub> H <sub>11</sub> + H <sub>3</sub> N + 9.484 Y <sub>4</sub> C <sub>7</sub> → 12.08 H <sub>8</sub> C <sub>5</sub> + 36.94 YB <sub>2</sub> + YB <sub>6</sub> H <sub>4</sub> C <sub>6</sub> N | -33.9156            |
| YNH <sub>4</sub> B <sub>6</sub> C <sub>6</sub> | 3 B <sub>13</sub> C <sub>2</sub> + 36 H <sub>3</sub> N + YB <sub>2</sub> → 52 H <sub>2</sub> + 35 BN + YB <sub>6</sub> H <sub>4</sub> C <sub>6</sub> N                                                        | -33.7295            |
| YNH <sub>4</sub> B <sub>6</sub> C <sub>6</sub> | 1.75 B <sub>13</sub> C <sub>2</sub> + 0.5 H <sub>8</sub> C <sub>5</sub> + 8.375 N <sub>2</sub> + YN → 16.75 BN + YB <sub>6</sub> H <sub>4</sub> C <sub>6</sub> N                                              | -33.2527            |
| YNH <sub>4</sub> B <sub>6</sub> C <sub>6</sub> | 3 B <sub>13</sub> C <sub>2</sub> + Y + 34 H <sub>3</sub> N → 49 H <sub>2</sub> + 33 BN + YB <sub>6</sub> H <sub>4</sub> C <sub>6</sub> N                                                                      | -32.9803            |
| YNH <sub>4</sub> B <sub>6</sub> C <sub>6</sub> | 3 B <sub>13</sub> C <sub>2</sub> + 16.73 Y + 16.73 H <sub>3</sub> N → 6.6 B <sub>5</sub> H <sub>7</sub> + 15.73 YN + YB <sub>6</sub> H <sub>4</sub> C <sub>6</sub> N                                          | -32.5222            |
| YNH <sub>4</sub> B <sub>6</sub> C <sub>6</sub> | 6 Y <sub>2</sub> C + 1.333 H <sub>3</sub> N + 6.833 N <sub>2</sub> + 3 YB <sub>2</sub> → 14 YN + YB <sub>6</sub> H <sub>4</sub> C <sub>6</sub> N                                                              | -32.4979            |
| YNH <sub>4</sub> B <sub>6</sub> C <sub>6</sub> | 2 YH <sub>2</sub> + 6 Y <sub>2</sub> C + 7.75 N <sub>2</sub> + 1.5 YB <sub>4</sub> → 14.5 YN + YB <sub>6</sub> H <sub>4</sub> C <sub>6</sub> N                                                                | -32.4841            |
| YNH <sub>4</sub> B <sub>6</sub> C <sub>6</sub> | 2 YH <sub>2</sub> + 6 Y <sub>2</sub> C + 0.5 YB <sub>12</sub> + 7.25 N <sub>2</sub> → 13.5 YN + YB <sub>6</sub> H <sub>4</sub> C <sub>6</sub> N                                                               | -31.9022            |
| YNH <sub>4</sub> B <sub>6</sub> C <sub>6</sub> | 2 YH <sub>2</sub> + 6 Y <sub>2</sub> C + 7 N <sub>2</sub> + 6 B → 13 YN + YB <sub>6</sub> H <sub>4</sub> C <sub>6</sub> N                                                                                     | -31.7863            |
| YNH <sub>4</sub> B <sub>6</sub> C <sub>6</sub> | 8.75 B <sub>9</sub> H <sub>11</sub> + YN + 9.094 Y <sub>4</sub> C <sub>7</sub> → 11.53 H <sub>8</sub> C <sub>5</sub> + 36.38 YB <sub>2</sub> + YB <sub>6</sub> H <sub>4</sub> C <sub>6</sub> N                | -31.3197            |
| YNH <sub>4</sub> B <sub>6</sub> C <sub>6</sub> | 6 Y <sub>2</sub> C + 0.5714 B <sub>5</sub> H <sub>7</sub> + 6.786 N <sub>2</sub> + 1.571 YB <sub>2</sub> → 12.57 YN + YB <sub>6</sub> H <sub>4</sub> C <sub>6</sub> N                                         | -31.1991            |
| YNH <sub>4</sub> B <sub>6</sub> C <sub>6</sub> | 1.333 YH <sub>3</sub> + 6 Y <sub>2</sub> C + 7.417 N <sub>2</sub> + 1.5 YB <sub>4</sub> → 13.83 YN + YB <sub>6</sub> H <sub>4</sub> C <sub>6</sub> N                                                          | -31.1702            |
| YNH <sub>4</sub> B <sub>6</sub> C <sub>6</sub> | 6 Y <sub>2</sub> C + 13.91 H <sub>3</sub> N + 1.576 YB <sub>12</sub> → 12.58 YH <sub>3</sub> + 12.91 BN + YB <sub>6</sub> H <sub>4</sub> C <sub>6</sub> N                                                     | -31.0564            |
| YNH <sub>4</sub> B <sub>6</sub> C <sub>6</sub> | YH <sub>2</sub> + 3 B <sub>13</sub> C <sub>2</sub> + 34 H <sub>3</sub> N → 50 H <sub>2</sub> + 33 BN + YB <sub>6</sub> H <sub>4</sub> C <sub>6</sub> N                                                        | -30.8691            |
| YNH <sub>4</sub> B <sub>6</sub> C <sub>6</sub> | 3 B <sub>13</sub> C <sub>2</sub> + 33 H <sub>3</sub> N + YN → 47.5 H <sub>2</sub> + 33 BN + YB <sub>6</sub> H <sub>4</sub> C <sub>6</sub> N                                                                   | -30.8413            |

Continued on next page

Continued

| Compound                                       | Chemical reaction                                                                                                                                                                                          | Reaction energy(eV) |
|------------------------------------------------|------------------------------------------------------------------------------------------------------------------------------------------------------------------------------------------------------------|---------------------|
| YNH <sub>4</sub> B <sub>6</sub> C <sub>6</sub> | 0.3636 B <sub>9</sub> H <sub>11</sub> + 6 Y <sub>2</sub> C + 6.682 N <sub>2</sub> + 1.364 YB <sub>2</sub> → 12.36 YN + YB <sub>6</sub> H <sub>4</sub> C <sub>6</sub> N                                     | -30.7780            |
| YNH <sub>4</sub> B <sub>6</sub> C <sub>6</sub> | 25.1 YH <sub>2</sub> + 3 B <sub>13</sub> C <sub>2</sub> + 12.55 N <sub>2</sub> → 6.6 B <sub>5</sub> H <sub>7</sub> + 24.1 YN + YB <sub>6</sub> H <sub>4</sub> C <sub>6</sub> N                             | -30.6617            |
| YNH <sub>4</sub> B <sub>6</sub> C <sub>6</sub> | 1.333 YH <sub>3</sub> + 6 Y <sub>2</sub> C + 0.5 YB <sub>12</sub> + 6.917 N <sub>2</sub> → 12.83 YN + YB <sub>6</sub> H <sub>4</sub> C <sub>6</sub> N                                                      | -30.5883            |
| YNH <sub>4</sub> B <sub>6</sub> C <sub>6</sub> | YH <sub>3</sub> + 3 B <sub>13</sub> C <sub>2</sub> + 34 H <sub>3</sub> N → 50.5 H <sub>2</sub> + 33 BN + YB <sub>6</sub> H <sub>4</sub> C <sub>6</sub> N                                                   | -30.5597            |
| YNH <sub>4</sub> B <sub>6</sub> C <sub>6</sub> | 1.333 YH <sub>3</sub> + 6 Y <sub>2</sub> C + 6.667 N <sub>2</sub> + 6 B → 12.33 YN + YB <sub>6</sub> H <sub>4</sub> C <sub>6</sub> N                                                                       | -30.4724            |
| YNH <sub>4</sub> B <sub>6</sub> C <sub>6</sub> | 6 Y <sub>2</sub> C + 12.33 H <sub>3</sub> N + 17.33 B → 11 YH <sub>3</sub> + 11.33 BN + YB <sub>6</sub> H <sub>4</sub> C <sub>6</sub> N                                                                    | -30.3755            |
| YNH <sub>4</sub> B <sub>6</sub> C <sub>6</sub> | 3 B <sub>13</sub> C <sub>2</sub> + 14 H <sub>3</sub> N + 20 YN → 19 YH <sub>2</sub> + 33 BN + YB <sub>6</sub> H <sub>4</sub> C <sub>6</sub> N                                                              | -30.3131            |
| YNH <sub>4</sub> B <sub>6</sub> C <sub>6</sub> | 3 B <sub>13</sub> C <sub>2</sub> + 34 YN + 35 H <sub>2</sub> → 33 YH <sub>2</sub> + 33 BN + YB <sub>6</sub> H <sub>4</sub> C <sub>6</sub> N                                                                | -29.9239            |
| YNH <sub>4</sub> B <sub>6</sub> C <sub>6</sub> | 6 Y <sub>2</sub> C + 6.75 N <sub>2</sub> + 2 H <sub>2</sub> + 1.5 YB <sub>4</sub> → 12.5 YN + YB <sub>6</sub> H <sub>4</sub> C <sub>6</sub> N                                                              | -29.7803            |
| YNH <sub>4</sub> B <sub>6</sub> C <sub>6</sub> | 6 Y <sub>2</sub> C + 1.2 B <sub>5</sub> H <sub>7</sub> + 6.733 N <sub>2</sub> → 1.467 H <sub>3</sub> N + 11 YN + YB <sub>6</sub> H <sub>4</sub> C <sub>6</sub> N                                           | -29.7705            |
| YNH <sub>4</sub> B <sub>6</sub> C <sub>6</sub> | 0.6667 B <sub>9</sub> H <sub>11</sub> + 6 Y <sub>2</sub> C + 6.556 N <sub>2</sub> → 1.111 H <sub>3</sub> N + 11 YN + YB <sub>6</sub> H <sub>4</sub> C <sub>6</sub> N                                       | -29.3448            |
| YNH <sub>4</sub> B <sub>6</sub> C <sub>6</sub> | 6 Y <sub>2</sub> C + 0.5 YB <sub>12</sub> + 6.25 N <sub>2</sub> + 2 H <sub>2</sub> → 11.5 YN + YB <sub>6</sub> H <sub>4</sub> C <sub>6</sub> N                                                             | -29.1984            |
| YNH <sub>4</sub> B <sub>6</sub> C <sub>6</sub> | 6 Y <sub>2</sub> C + 6 N <sub>2</sub> + 2 H <sub>2</sub> + 6 B → 11 YN + YB <sub>6</sub> H <sub>4</sub> C <sub>6</sub> N                                                                                   | -29.0825            |
| YNH <sub>4</sub> B <sub>6</sub> C <sub>6</sub> | 6 Y <sub>2</sub> C + 0.5714 B <sub>5</sub> H <sub>7</sub> + 6.393 N <sub>2</sub> + 0.7857 YB <sub>4</sub> → 11.79 YN + YB <sub>6</sub> H <sub>4</sub> C <sub>6</sub> N                                     | -28.8509            |
| YNH <sub>4</sub> B <sub>6</sub> C <sub>6</sub> | 2 YH <sub>2</sub> + 6 Y <sub>2</sub> C + 0.5 N <sub>2</sub> + 162 B → 13 YB <sub>12</sub> + YB <sub>6</sub> H <sub>4</sub> C <sub>6</sub> N                                                                | -28.7725            |
| YNH <sub>4</sub> B <sub>6</sub> C <sub>6</sub> | 2.75 B <sub>13</sub> C <sub>2</sub> + 0.5 Y <sub>2</sub> C + 30.75 H <sub>3</sub> N → 44.12 H <sub>2</sub> + 29.75 BN + YB <sub>6</sub> H <sub>4</sub> C <sub>6</sub> N                                    | -28.7493            |
| YNH <sub>4</sub> B <sub>6</sub> C <sub>6</sub> | 0.3636 B <sub>9</sub> H <sub>11</sub> + 6 Y <sub>2</sub> C + 6.341 N <sub>2</sub> + 0.6818 YB <sub>4</sub> → 11.68 YN + YB <sub>6</sub> H <sub>4</sub> C <sub>6</sub> N                                    | -28.7403            |
| YNH <sub>4</sub> B <sub>6</sub> C <sub>6</sub> | 6 Y <sub>2</sub> C + 0.2619 YB <sub>12</sub> + 0.5714 B <sub>5</sub> H <sub>7</sub> + 6.131 N <sub>2</sub> → 11.26 YN + YB <sub>6</sub> H <sub>4</sub> C <sub>6</sub> N                                    | -28.5461            |
| YNH <sub>4</sub> B <sub>6</sub> C <sub>6</sub> | 2 YH <sub>2</sub> + 6 Y <sub>2</sub> C + YN + 174 B → 14 YB <sub>12</sub> + YB <sub>6</sub> H <sub>4</sub> C <sub>6</sub> N                                                                                | -28.5406            |
| YNH <sub>4</sub> B <sub>6</sub> C <sub>6</sub> | 6 Y <sub>2</sub> C + 0.5714 B <sub>5</sub> H <sub>7</sub> + 6 N <sub>2</sub> + 3.143 B → 11 YN + YB <sub>6</sub> H <sub>4</sub> C <sub>6</sub> N                                                           | -28.4854            |
| YNH <sub>4</sub> B <sub>6</sub> C <sub>6</sub> | 0.3636 B <sub>9</sub> H <sub>11</sub> + 6 Y <sub>2</sub> C + 0.2273 YB <sub>12</sub> + 6.114 N <sub>2</sub> → 11.23 YN + YB <sub>6</sub> H <sub>4</sub> C <sub>6</sub> N                                   | -28.4758            |
| YNH <sub>4</sub> B <sub>6</sub> C <sub>6</sub> | 0.3636 B <sub>9</sub> H <sub>11</sub> + 6 Y <sub>2</sub> C + 6 N <sub>2</sub> + 2.727 B → 11 YN + YB <sub>6</sub> H <sub>4</sub> C <sub>6</sub> N                                                          | -28.4231            |
| YNH <sub>4</sub> B <sub>6</sub> C <sub>6</sub> | 1.5 B <sub>13</sub> C <sub>2</sub> + 0.5 Y <sub>2</sub> C + 0.5 H <sub>8</sub> C <sub>5</sub> + 7.25 N <sub>2</sub> → 13.5 BN + YB <sub>6</sub> H <sub>4</sub> C <sub>6</sub> N                            | -28.1816            |
| YNH <sub>4</sub> B <sub>6</sub> C <sub>6</sub> | 3 B <sub>13</sub> C <sub>2</sub> + 14.78 Y + 14.78 H <sub>3</sub> N → 3.667 B <sub>9</sub> H <sub>11</sub> + 13.78 YN + YB <sub>6</sub> H <sub>4</sub> C <sub>6</sub> N                                    | -28.0913            |
| YNH <sub>4</sub> B <sub>6</sub> C <sub>6</sub> | 6 Y <sub>2</sub> C + 1.333 H <sub>3</sub> N + 6.083 N <sub>2</sub> + 1.5 YB <sub>4</sub> → 12.5 YN + YB <sub>6</sub> H <sub>4</sub> C <sub>6</sub> N                                                       | -28.0149            |
| YNH <sub>4</sub> B <sub>6</sub> C <sub>6</sub> | 2.75 B <sub>9</sub> H <sub>11</sub> + 6 Y <sub>2</sub> C + 6 N <sub>2</sub> → 3.75 B <sub>5</sub> H <sub>7</sub> + 11 YN + YB <sub>6</sub> H <sub>4</sub> C <sub>6</sub> N                                 | -28.0145            |
| YNH <sub>4</sub> B <sub>6</sub> C <sub>6</sub> | 0.6667 B <sub>9</sub> H <sub>11</sub> + 6 Y <sub>2</sub> C + 6 N <sub>2</sub> → 11 YN + 1.667 H <sub>2</sub> + YB <sub>6</sub> H <sub>4</sub> C <sub>6</sub> N                                             | -27.8736            |
| YNH <sub>4</sub> B <sub>6</sub> C <sub>6</sub> | 6 Y <sub>2</sub> C + 1.2 B <sub>5</sub> H <sub>7</sub> + 6 N <sub>2</sub> → 11 YN + 2.2 H <sub>2</sub> + YB <sub>6</sub> H <sub>4</sub> C <sub>6</sub> N                                                   | -27.8285            |
| YNH <sub>4</sub> B <sub>6</sub> C <sub>6</sub> | 1.333 YH <sub>3</sub> + 6 Y <sub>2</sub> C + 0.5 N <sub>2</sub> + 154 B → 12.33 YB <sub>12</sub> + YB <sub>6</sub> H <sub>4</sub> C <sub>6</sub> N                                                         | -27.6132            |
| YNH <sub>4</sub> B <sub>6</sub> C <sub>6</sub> | 6 Y <sub>2</sub> C + 1.333 H <sub>3</sub> N + 0.5 YB <sub>12</sub> + 5.583 N <sub>2</sub> → 11.5 YN + YB <sub>6</sub> H <sub>4</sub> C <sub>6</sub> N                                                      | -27.4330            |
| YNH <sub>4</sub> B <sub>6</sub> C <sub>6</sub> | 1.333 YH <sub>3</sub> + 6 Y <sub>2</sub> C + YN + 166 B → 13.33 YB <sub>12</sub> + YB <sub>6</sub> H <sub>4</sub> C <sub>6</sub> N                                                                         | -27.3814            |
| YNH <sub>4</sub> B <sub>6</sub> C <sub>6</sub> | 6 Y <sub>2</sub> C + 1.333 H <sub>3</sub> N + 5.333 N <sub>2</sub> + 6 B → 11 YN + YB <sub>6</sub> H <sub>4</sub> C <sub>6</sub> N                                                                         | -27.3171            |
| YNH <sub>4</sub> B <sub>6</sub> C <sub>6</sub> | 0.6667 B <sub>9</sub> H <sub>11</sub> + 6 Y <sub>2</sub> C + 5.444 N <sub>2</sub> → 1.111 YH <sub>3</sub> + 9.889 YN + YB <sub>6</sub> H <sub>4</sub> C <sub>6</sub> N                                     | -26.7153            |
| YNH <sub>4</sub> B <sub>6</sub> C <sub>6</sub> | 6 Y <sub>2</sub> C + 0.5 N <sub>2</sub> + 2 H <sub>2</sub> + 138 B → 11 YB <sub>12</sub> + YB <sub>6</sub> H <sub>4</sub> C <sub>6</sub> N                                                                 | -26.5324            |
| YNH <sub>4</sub> B <sub>6</sub> C <sub>6</sub> | 22.17 YH <sub>2</sub> + 3 B <sub>13</sub> C <sub>2</sub> + 11.08 N <sub>2</sub> → 3.667 B <sub>9</sub> H <sub>11</sub> + 21.17 YN + YB <sub>6</sub> H <sub>4</sub> C <sub>6</sub> N                        | -26.4482            |
| YNH <sub>4</sub> B <sub>6</sub> C <sub>6</sub> | 6 Y <sub>2</sub> C + YN + 2 H <sub>2</sub> + 150 B → 12 YB <sub>12</sub> + YB <sub>6</sub> H <sub>4</sub> C <sub>6</sub> N                                                                                 | -26.3006            |
| YNH <sub>4</sub> B <sub>6</sub> C <sub>6</sub> | 6 Y <sub>2</sub> C + 1.2 B <sub>5</sub> H <sub>7</sub> + 5.267 N <sub>2</sub> → 1.467 YH <sub>3</sub> + 9.533 YN + YB <sub>6</sub> H <sub>4</sub> C <sub>6</sub> N                                         | -26.2996            |
| YNH <sub>4</sub> B <sub>6</sub> C <sub>6</sub> | 2 YH <sub>2</sub> + 6 Y <sub>2</sub> C + BN + 161 B → 13 YB <sub>12</sub> + YB <sub>6</sub> H <sub>4</sub> C <sub>6</sub> N                                                                                | -26.2057            |
| YNH <sub>4</sub> B <sub>6</sub> C <sub>6</sub> | 6 Y <sub>2</sub> C + 0.5714 B <sub>5</sub> H <sub>7</sub> + 0.5 N <sub>2</sub> + 135.1 B → 11 YB <sub>12</sub> + YB <sub>6</sub> H <sub>4</sub> C <sub>6</sub> N                                           | -25.9352            |
| YNH <sub>4</sub> B <sub>6</sub> C <sub>6</sub> | 0.3636 B <sub>9</sub> H <sub>11</sub> + 6 Y <sub>2</sub> C + 0.5 N <sub>2</sub> + 134.7 B → 11 YB <sub>12</sub> + YB <sub>6</sub> H <sub>4</sub> C <sub>6</sub> N                                          | -25.8730            |
| YNH <sub>4</sub> B <sub>6</sub> C <sub>6</sub> | 0.5 YH <sub>2</sub> + 6 Y <sub>2</sub> C + H <sub>3</sub> N + 144 B → 11.5 YB <sub>12</sub> + YB <sub>6</sub> H <sub>4</sub> C <sub>6</sub> N                                                              | -25.7683            |
| YNH <sub>4</sub> B <sub>6</sub> C <sub>6</sub> | 2 YH <sub>2</sub> + 0.4615 B <sub>13</sub> C <sub>2</sub> + 5.077 Y <sub>2</sub> C + 6.077 N <sub>2</sub> → 11.15 YN + YB <sub>6</sub> H <sub>4</sub> C <sub>6</sub> N                                     | -25.7478            |
| YNH <sub>4</sub> B <sub>6</sub> C <sub>6</sub> | 2 YH <sub>2</sub> + 6 Y <sub>2</sub> C + 0.5 N <sub>2</sub> + 58 B → 13 YB <sub>4</sub> + YB <sub>6</sub> H <sub>4</sub> C <sub>6</sub> N                                                                  | -25.7385            |
| YNH <sub>4</sub> B <sub>6</sub> C <sub>6</sub> | 6 Y <sub>2</sub> C + 0.5714 B <sub>5</sub> H <sub>7</sub> + YN + 147.1 B → 12 YB <sub>12</sub> + YB <sub>6</sub> H <sub>4</sub> C <sub>6</sub> N                                                           | -25.7034            |
| YNH <sub>4</sub> B <sub>6</sub> C <sub>6</sub> | 0.3636 B <sub>9</sub> H <sub>11</sub> + 0.2098 B <sub>13</sub> C <sub>2</sub> + 5.58 Y <sub>2</sub> C + 5.58 N <sub>2</sub> → 10.16 YN + YB <sub>6</sub> H <sub>4</sub> C <sub>6</sub> N                   | -25.6783            |
| YNH <sub>4</sub> B <sub>6</sub> C <sub>6</sub> | 0.3636 B <sub>9</sub> H <sub>11</sub> + 6 Y <sub>2</sub> C + YN + 146.7 B → 12 YB <sub>12</sub> + YB <sub>6</sub> H <sub>4</sub> C <sub>6</sub> N                                                          | -25.6411            |
| YNH <sub>4</sub> B <sub>6</sub> C <sub>6</sub> | 6 Y <sub>2</sub> C + 1.333 H <sub>3</sub> N + 138.3 B → 11 YB <sub>12</sub> + 0.3333 BN + YB <sub>6</sub> H <sub>4</sub> C <sub>6</sub> N                                                                  | -25.6226            |
| YNH <sub>4</sub> B <sub>6</sub> C <sub>6</sub> | 0.6667 B <sub>9</sub> H <sub>11</sub> + 6 Y <sub>2</sub> C + 5.167 N <sub>2</sub> → 1.667 YH <sub>2</sub> + 9.333 YN + YB <sub>6</sub> H <sub>4</sub> C <sub>6</sub> N                                     | -25.6204            |
| YNH <sub>4</sub> B <sub>6</sub> C <sub>6</sub> | 7 B <sub>9</sub> H <sub>11</sub> + 0.5 N <sub>2</sub> + 7.375 Y <sub>4</sub> C <sub>7</sub> → 9.125 H <sub>8</sub> C <sub>5</sub> + 28.5 YB <sub>2</sub> + YB <sub>6</sub> H <sub>4</sub> C <sub>6</sub> N | -25.5736            |
| YNH <sub>4</sub> B <sub>6</sub> C <sub>6</sub> | 0.3333 YH <sub>3</sub> + 6 Y <sub>2</sub> C + H <sub>3</sub> N + 142 B → 11.33 YB <sub>12</sub> + YB <sub>6</sub> H <sub>4</sub> C <sub>6</sub> N                                                          | -25.4785            |
| YNH <sub>4</sub> B <sub>6</sub> C <sub>6</sub> | 15.27 H <sub>3</sub> N + 1.2 Y <sub>4</sub> C <sub>5</sub> + 10.13 YB <sub>2</sub> → 13.93 YH <sub>3</sub> + 14.27 BN + YB <sub>6</sub> H <sub>4</sub> C <sub>6</sub> N                                    | -25.3498            |
| YNH <sub>4</sub> B <sub>6</sub> C <sub>6</sub> | 0.2418 B <sub>13</sub> C <sub>2</sub> + 5.516 Y <sub>2</sub> C + 0.5714 B <sub>5</sub> H <sub>7</sub> + 5.516 N <sub>2</sub> → 10.03 YN + YB <sub>6</sub> H <sub>4</sub> C <sub>6</sub> N                  | -25.3224            |
| YNH <sub>4</sub> B <sub>6</sub> C <sub>6</sub> | 2 YH <sub>2</sub> + 6 Y <sub>2</sub> C + YN + 62 B → 14 YB <sub>4</sub> + YB <sub>6</sub> H <sub>4</sub> C <sub>6</sub> N                                                                                  | -25.2733            |
| YNH <sub>4</sub> B <sub>6</sub> C <sub>6</sub> | 6 Y <sub>2</sub> C + H <sub>3</sub> N + 0.5 H <sub>2</sub> + 138 B → 11 YB <sub>12</sub> + YB <sub>6</sub> H <sub>4</sub> C <sub>6</sub> N                                                                 | -25.2083            |
| YNH <sub>4</sub> B <sub>6</sub> C <sub>6</sub> | 6 Y <sub>2</sub> C + H <sub>3</sub> N + 0.1429 B <sub>5</sub> H <sub>7</sub> + 137.3 B → 11 YB <sub>12</sub> + YB <sub>6</sub> H <sub>4</sub> C <sub>6</sub> N                                             | -25.0590            |
| YNH <sub>4</sub> B <sub>6</sub> C <sub>6</sub> | 1.333 YH <sub>3</sub> + 6 Y <sub>2</sub> C + BN + 153 B → 12.33 YB <sub>12</sub> + YB <sub>6</sub> H <sub>4</sub> C <sub>6</sub> N                                                                         | -25.0464            |
| YNH <sub>4</sub> B <sub>6</sub> C <sub>6</sub> | 0.09091 B <sub>9</sub> H <sub>11</sub> + 6 Y <sub>2</sub> C + H <sub>3</sub> N + 137.2 B → 11 YB <sub>12</sub> + YB <sub>6</sub> H <sub>4</sub> C <sub>6</sub> N                                           | -25.0435            |
| YNH <sub>4</sub> B <sub>6</sub> C <sub>6</sub> | 4.085 B <sub>9</sub> H <sub>11</sub> + 10.73 Y <sub>2</sub> C + 0.5 N <sub>2</sub> → 20.46 YH <sub>2</sub> + 2.366 B <sub>13</sub> C <sub>2</sub> + YB <sub>6</sub> H <sub>4</sub> C <sub>6</sub> N        | -24.9676            |
| YNH <sub>4</sub> B <sub>6</sub> C <sub>6</sub> | 4.451 B <sub>9</sub> H <sub>11</sub> + 11.24 Y <sub>2</sub> C + YN → 22.48 YH <sub>2</sub> + 2.62 B <sub>13</sub> C <sub>2</sub> + YB <sub>6</sub> H <sub>4</sub> C <sub>6</sub> N                         | -24.8976            |
| YNH <sub>4</sub> B <sub>6</sub> C <sub>6</sub> | 6 Y <sub>2</sub> C + 1.2 B <sub>5</sub> H <sub>7</sub> + 4.9 N <sub>2</sub> → 2.2 YH <sub>2</sub> + 8.8 YN + YB <sub>6</sub> H <sub>4</sub> C <sub>6</sub> N                                               | -24.8544            |

Continued on next page

Continued

| Compound                                       | Chemical reaction                                                                                                                                                                                 | Reaction energy(eV) |
|------------------------------------------------|---------------------------------------------------------------------------------------------------------------------------------------------------------------------------------------------------|---------------------|
| YNH <sub>4</sub> B <sub>6</sub> C <sub>6</sub> | 6 Y <sub>2</sub> C + 1.333 H <sub>3</sub> N + 134 B → 10.67 YB <sub>12</sub> + 0.3333 YN + YB <sub>6</sub> H <sub>4</sub> C <sub>6</sub> N                                                        | -24.8442            |
| YNH <sub>4</sub> B <sub>6</sub> C <sub>6</sub> | 6 Y <sub>2</sub> C + 1.333 H <sub>3</sub> N + 138 B → 11 YB <sub>12</sub> + 0.1667 N <sub>2</sub> + YB <sub>6</sub> H <sub>4</sub> C <sub>6</sub> N                                               | -24.7670            |
| YNH <sub>4</sub> B <sub>6</sub> C <sub>6</sub> | 1.333 YH <sub>3</sub> + 6 Y <sub>2</sub> C + 0.5 N <sub>2</sub> + 55.33 B → 12.33 YB <sub>4</sub> + YB <sub>6</sub> H <sub>4</sub> C <sub>6</sub> N                                               | -24.7348            |
| YNH <sub>4</sub> B <sub>6</sub> C <sub>6</sub> | 1.333 YH <sub>3</sub> + 0.4615 B <sub>13</sub> C <sub>2</sub> + 5.077 Y <sub>2</sub> C + 5.744 N <sub>2</sub> → 10.49 YN + YB <sub>6</sub> H <sub>4</sub> C <sub>6</sub> N                        | -24.4340            |
| YNH <sub>4</sub> B <sub>6</sub> C <sub>6</sub> | 1.2 Y <sub>4</sub> C <sub>5</sub> + 10.32 B <sub>5</sub> H <sub>7</sub> + 11.87 N <sub>2</sub> → 22.75 H <sub>3</sub> N + 3.8 YB <sub>12</sub> + YB <sub>6</sub> H <sub>4</sub> C <sub>6</sub> N  | -24.4223            |
| YNH <sub>4</sub> B <sub>6</sub> C <sub>6</sub> | 1.333 YH <sub>3</sub> + 6 Y <sub>2</sub> C + YN + 59.33 B → 13.33 YB <sub>4</sub> + YB <sub>6</sub> H <sub>4</sub> C <sub>6</sub> N                                                               | -24.2696            |
| YNH <sub>4</sub> B <sub>6</sub> C <sub>6</sub> | 0.3636 B <sub>9</sub> H <sub>11</sub> + 3 B <sub>13</sub> C <sub>2</sub> + 19.14 Y + 0.5 N <sub>2</sub> → 18.14 YB <sub>2</sub> + YB <sub>6</sub> H <sub>4</sub> C <sub>6</sub> N                 | -24.1232            |
| YNH <sub>4</sub> B <sub>6</sub> C <sub>6</sub> | 2 YH <sub>2</sub> + 6 Y <sub>2</sub> C + 7.25 YB <sub>12</sub> + 0.5 N <sub>2</sub> → 20.25 YB <sub>4</sub> + YB <sub>6</sub> H <sub>4</sub> C <sub>6</sub> N                                     | -24.0465            |
| YNH <sub>4</sub> B <sub>6</sub> C <sub>6</sub> | 6 Y <sub>2</sub> C + 2 H <sub>2</sub> + BN + 137 B → 11 YB <sub>12</sub> + YB <sub>6</sub> H <sub>4</sub> C <sub>6</sub> N                                                                        | -23.9656            |
| YNH <sub>4</sub> B <sub>6</sub> C <sub>6</sub> | 6 Y <sub>2</sub> C + 0.5 N <sub>2</sub> + 2 H <sub>2</sub> + 50 B → 11 YB <sub>4</sub> + YB <sub>6</sub> H <sub>4</sub> C <sub>6</sub> N                                                          | -23.9652            |
| YNH <sub>4</sub> B <sub>6</sub> C <sub>6</sub> | 3 B <sub>13</sub> C <sub>2</sub> + 18.93 Y + 0.5714 B <sub>5</sub> H <sub>7</sub> + 0.5 N <sub>2</sub> → 17.93 YB <sub>2</sub> + YB <sub>6</sub> H <sub>4</sub> C <sub>6</sub> N                  | -23.8248            |
| YNH <sub>4</sub> B <sub>6</sub> C <sub>6</sub> | 6 Y <sub>2</sub> C + YN + 2 H <sub>2</sub> + 54 B → 12 YB <sub>4</sub> + YB <sub>6</sub> H <sub>4</sub> C <sub>6</sub> N                                                                          | -23.5000            |
| YNH <sub>4</sub> B <sub>6</sub> C <sub>6</sub> | 2 YH <sub>2</sub> + 6 Y <sub>2</sub> C + 7.75 YB <sub>12</sub> + YN → 21.75 YB <sub>4</sub> + YB <sub>6</sub> H <sub>4</sub> C <sub>6</sub> N                                                     | -23.4646            |
| YNH <sub>4</sub> B <sub>6</sub> C <sub>6</sub> | 4.197 B <sub>9</sub> H <sub>11</sub> + 11.04 Y <sub>2</sub> C + BN → 21.08 YH <sub>2</sub> + 2.521 B <sub>13</sub> C <sub>2</sub> + YB <sub>6</sub> H <sub>4</sub> C <sub>6</sub> N               | -23.3857            |
| YNH <sub>4</sub> B <sub>6</sub> C <sub>6</sub> | 6 Y <sub>2</sub> C + 0.5714 B <sub>5</sub> H <sub>7</sub> + BN + 134.1 B → 11 YB <sub>12</sub> + YB <sub>6</sub> H <sub>4</sub> C <sub>6</sub> N                                                  | -23.3685            |
| YNH <sub>4</sub> B <sub>6</sub> C <sub>6</sub> | 6 Y <sub>2</sub> C + 0.5714 B <sub>5</sub> H <sub>7</sub> + 0.5 N <sub>2</sub> + 47.14 B → 11 YB <sub>4</sub> + YB <sub>6</sub> H <sub>4</sub> C <sub>6</sub> N                                   | -23.3680            |
| YNH <sub>4</sub> B <sub>6</sub> C <sub>6</sub> | 0.3636 B <sub>9</sub> H <sub>11</sub> + 6 Y <sub>2</sub> C + BN + 133.7 B → 11 YB <sub>12</sub> + YB <sub>6</sub> H <sub>4</sub> C <sub>6</sub> N                                                 | -23.3062            |
| YNH <sub>4</sub> B <sub>6</sub> C <sub>6</sub> | 0.3636 B <sub>9</sub> H <sub>11</sub> + 6 Y <sub>2</sub> C + 0.5 N <sub>2</sub> + 46.73 B → 11 YB <sub>4</sub> + YB <sub>6</sub> H <sub>4</sub> C <sub>6</sub> N                                  | -23.3058            |
| YNH <sub>4</sub> B <sub>6</sub> C <sub>6</sub> | 2 YH <sub>2</sub> + 6 Y <sub>2</sub> C + BN + 57 B → 13 YB <sub>4</sub> + YB <sub>6</sub> H <sub>4</sub> C <sub>6</sub> N                                                                         | -23.1718            |
| YNH <sub>4</sub> B <sub>6</sub> C <sub>6</sub> | 1.333 YH <sub>3</sub> + 6 Y <sub>2</sub> C + 6.917 YB <sub>12</sub> + 0.5 N <sub>2</sub> → 19.25 YB <sub>4</sub> + YB <sub>6</sub> H <sub>4</sub> C <sub>6</sub> N                                | -23.1206            |
| YNH <sub>4</sub> B <sub>6</sub> C <sub>6</sub> | 0.5 YH <sub>2</sub> + 6 Y <sub>2</sub> C + H <sub>3</sub> N + 52 B → 11.5 YB <sub>4</sub> + YB <sub>6</sub> H <sub>4</sub> C <sub>6</sub> N                                                       | -23.0845            |
| YNH <sub>4</sub> B <sub>6</sub> C <sub>6</sub> | 6 Y <sub>2</sub> C + 1.333 H <sub>3</sub> N + 50.33 B → 0.3333 BN + 11 YB <sub>4</sub> + YB <sub>6</sub> H <sub>4</sub> C <sub>6</sub> N                                                          | -23.0554            |
| YNH <sub>4</sub> B <sub>6</sub> C <sub>6</sub> | 0.4615 B <sub>13</sub> C <sub>2</sub> + 5.077 Y <sub>2</sub> C + 5.077 N <sub>2</sub> + 2 H <sub>2</sub> → 9.154 YN + YB <sub>6</sub> H <sub>4</sub> C <sub>6</sub> N                             | -23.0441            |
| YNH <sub>4</sub> B <sub>6</sub> C <sub>6</sub> | 6 Y <sub>2</sub> C + 0.5714 B <sub>5</sub> H <sub>7</sub> + YN + 51.14 B → 12 YB <sub>4</sub> + YB <sub>6</sub> H <sub>4</sub> C <sub>6</sub> N                                                   | -22.9028            |
| YNH <sub>4</sub> B <sub>6</sub> C <sub>6</sub> | 0.3636 B <sub>9</sub> H <sub>11</sub> + 6 Y <sub>2</sub> C + YN + 50.73 B → 12 YB <sub>4</sub> + YB <sub>6</sub> H <sub>4</sub> C <sub>6</sub> N                                                  | -22.8406            |
| YNH <sub>4</sub> B <sub>6</sub> C <sub>6</sub> | 0.3333 YH <sub>3</sub> + 6 Y <sub>2</sub> C + H <sub>3</sub> N + 51.33 B → 11.33 YB <sub>4</sub> + YB <sub>6</sub> H <sub>4</sub> C <sub>6</sub> N                                                | -22.8335            |
| YNH <sub>4</sub> B <sub>6</sub> C <sub>6</sub> | 2.375 B <sub>13</sub> C <sub>2</sub> + 25.88 H <sub>3</sub> N + 0.25 Y <sub>4</sub> C <sub>5</sub> → 36.81 H <sub>2</sub> + 24.87 BN + YB <sub>6</sub> H <sub>4</sub> C <sub>6</sub> N            | -22.7823            |
| YNH <sub>4</sub> B <sub>6</sub> C <sub>6</sub> | 6 Y <sub>2</sub> C + H <sub>3</sub> N + 0.5 H <sub>2</sub> + 50 B → 11 YB <sub>4</sub> + YB <sub>6</sub> H <sub>4</sub> C <sub>6</sub> N                                                          | -22.6411            |
| YNH <sub>4</sub> B <sub>6</sub> C <sub>6</sub> | 1.333 YH <sub>3</sub> + 6 Y <sub>2</sub> C + 7.417 YB <sub>12</sub> + YN → 20.75 YB <sub>4</sub> + YB <sub>6</sub> H <sub>4</sub> C <sub>6</sub> N                                                | -22.5387            |
| YNH <sub>4</sub> B <sub>6</sub> C <sub>6</sub> | 6 Y <sub>2</sub> C + 6.25 YB <sub>12</sub> + 0.5 N <sub>2</sub> + 2 H <sub>2</sub> → 17.25 YB <sub>4</sub> + YB <sub>6</sub> H <sub>4</sub> C <sub>6</sub> N                                      | -22.5066            |
| YNH <sub>4</sub> B <sub>6</sub> C <sub>6</sub> | 6 Y <sub>2</sub> C + H <sub>3</sub> N + 0.1429 B <sub>5</sub> H <sub>7</sub> + 49.29 B → 11 YB <sub>4</sub> + YB <sub>6</sub> H <sub>4</sub> C <sub>6</sub> N                                     | -22.4919            |
| YNH <sub>4</sub> B <sub>6</sub> C <sub>6</sub> | 0.09091 B <sub>9</sub> H <sub>11</sub> + 6 Y <sub>2</sub> C + H <sub>3</sub> N + 49.18 B → 11 YB <sub>4</sub> + YB <sub>6</sub> H <sub>4</sub> C <sub>6</sub> N                                   | -22.4763            |
| YNH <sub>4</sub> B <sub>6</sub> C <sub>6</sub> | 0.3636 B <sub>9</sub> H <sub>11</sub> + 3 B <sub>13</sub> C <sub>2</sub> + 19.64 Y + BN → 18.64 YB <sub>2</sub> + YB <sub>6</sub> H <sub>4</sub> C <sub>6</sub> N                                 | -22.4246            |
| YNH <sub>4</sub> B <sub>6</sub> C <sub>6</sub> | 6 Y <sub>2</sub> C + 8.667 H <sub>3</sub> N + 13.67 B → 11 YH <sub>2</sub> + 7.667 BN + YB <sub>6</sub> H <sub>4</sub> C <sub>6</sub> N                                                           | -22.4152            |
| YNH <sub>4</sub> B <sub>6</sub> C <sub>6</sub> | 6 Y <sub>2</sub> C + 1.333 H <sub>3</sub> N + 48.67 B → 0.3333 YN + 10.67 YB <sub>4</sub> + YB <sub>6</sub> H <sub>4</sub> C <sub>6</sub> N                                                       | -22.3549            |
| YNH <sub>4</sub> B <sub>6</sub> C <sub>6</sub> | 6 Y <sub>2</sub> C + 1.333 H <sub>3</sub> N + 50 B → 0.1667 N <sub>2</sub> + 11 YB <sub>4</sub> + YB <sub>6</sub> H <sub>4</sub> C <sub>6</sub> N                                                 | -22.1998            |
| YNH <sub>4</sub> B <sub>6</sub> C <sub>6</sub> | 6 Y <sub>2</sub> C + 11.4 H <sub>3</sub> N + 4.1 YB <sub>4</sub> → 15.1 YH <sub>2</sub> + 10.4 BN + YB <sub>6</sub> H <sub>4</sub> C <sub>6</sub> N                                               | -22.1765            |
| YNH <sub>4</sub> B <sub>6</sub> C <sub>6</sub> | 1.333 YH <sub>3</sub> + 6 Y <sub>2</sub> C + BN + 54.33 B → 12.33 YB <sub>4</sub> + YB <sub>6</sub> H <sub>4</sub> C <sub>6</sub> N                                                               | -22.1681            |
| YNH <sub>4</sub> B <sub>6</sub> C <sub>6</sub> | 3 B <sub>13</sub> C <sub>2</sub> + 19.43 Y + 0.5714 B <sub>5</sub> H <sub>7</sub> + BN → 18.43 YB <sub>2</sub> + YB <sub>6</sub> H <sub>4</sub> C <sub>6</sub> N                                  | -22.1261            |
| YNH <sub>4</sub> B <sub>6</sub> C <sub>6</sub> | 6 Y <sub>2</sub> C + 9.471 H <sub>3</sub> N + 1.206 YB <sub>12</sub> → 12.21 YH <sub>2</sub> + 8.471 BN + YB <sub>6</sub> H <sub>4</sub> C <sub>6</sub> N                                         | -22.0636            |
| YNH <sub>4</sub> B <sub>6</sub> C <sub>6</sub> | 6 Y <sub>2</sub> C + 5.893 YB <sub>12</sub> + 0.5714 B <sub>5</sub> H <sub>7</sub> + 0.5 N <sub>2</sub> → 16.89 YB <sub>4</sub> + YB <sub>6</sub> H <sub>4</sub> C <sub>6</sub> N                 | -21.9928            |
| YNH <sub>4</sub> B <sub>6</sub> C <sub>6</sub> | 0.3636 B <sub>9</sub> H <sub>11</sub> + 6 Y <sub>2</sub> C + 5.841 YB <sub>12</sub> + 0.5 N <sub>2</sub> → 16.84 YB <sub>4</sub> + YB <sub>6</sub> H <sub>4</sub> C <sub>6</sub> N                | -21.9426            |
| YNH <sub>4</sub> B <sub>6</sub> C <sub>6</sub> | 3 B <sub>13</sub> C <sub>2</sub> + 17.5 Y + 0.5 N <sub>2</sub> + 2 H <sub>2</sub> → 16.5 YB <sub>2</sub> + YB <sub>6</sub> H <sub>4</sub> C <sub>6</sub> N                                        | -21.9417            |
| YNH <sub>4</sub> B <sub>6</sub> C <sub>6</sub> | 6 Y <sub>2</sub> C + 6.75 YB <sub>12</sub> + YN + 2 H <sub>2</sub> → 18.75 YB <sub>4</sub> + YB <sub>6</sub> H <sub>4</sub> C <sub>6</sub> N                                                      | -21.9247            |
| YNH <sub>4</sub> B <sub>6</sub> C <sub>6</sub> | 3.535 B <sub>9</sub> H <sub>11</sub> + 9.972 Y <sub>2</sub> C + H <sub>3</sub> N → 18.94 YH <sub>2</sub> + 1.986 B <sub>13</sub> C <sub>2</sub> + YB <sub>6</sub> H <sub>4</sub> C <sub>6</sub> N | -21.7206            |
| YNH <sub>4</sub> B <sub>6</sub> C <sub>6</sub> | 1.368 B <sub>9</sub> H <sub>11</sub> + 6 Y <sub>2</sub> C + 7.316 H <sub>3</sub> N → 11 YH <sub>3</sub> + 6.316 BN + YB <sub>6</sub> H <sub>4</sub> C <sub>6</sub> N                              | -21.6588            |
| YNH <sub>4</sub> B <sub>6</sub> C <sub>6</sub> | 6 Y <sub>2</sub> C + 1.333 H <sub>3</sub> N + 6.292 YB <sub>12</sub> → 0.3333 BN + 17.29 YB <sub>4</sub> + YB <sub>6</sub> H <sub>4</sub> C <sub>6</sub> N                                        | -21.5870            |
| YNH <sub>4</sub> B <sub>6</sub> C <sub>6</sub> | 0.5 YH <sub>2</sub> + 6 Y <sub>2</sub> C + H <sub>3</sub> N + 6.5 YB <sub>12</sub> → 18 YB <sub>4</sub> + YB <sub>6</sub> H <sub>4</sub> C <sub>6</sub> N                                         | -21.5675            |
| YNH <sub>4</sub> B <sub>6</sub> C <sub>6</sub> | 5.375 Y <sub>2</sub> C + H <sub>3</sub> N + 0.125 H <sub>8</sub> C <sub>5</sub> + 123 B → 9.75 YB <sub>12</sub> + YB <sub>6</sub> H <sub>4</sub> C <sub>6</sub> N                                 | -21.5163            |
| YNH <sub>4</sub> B <sub>6</sub> C <sub>6</sub> | 9.451 Y <sub>2</sub> C + 5.686 B <sub>5</sub> H <sub>7</sub> + 0.5 N <sub>2</sub> → 17.9 YH <sub>2</sub> + 1.725 B <sub>13</sub> C <sub>2</sub> + YB <sub>6</sub> H <sub>4</sub> C <sub>6</sub> N | -21.5142            |
| YNH <sub>4</sub> B <sub>6</sub> C <sub>6</sub> | 2 YH <sub>2</sub> + 6 Y <sub>2</sub> C + 7.125 YB <sub>12</sub> + BN → 20.12 YB <sub>4</sub> + YB <sub>6</sub> H <sub>4</sub> C <sub>6</sub> N                                                    | -21.5089            |
| YNH <sub>4</sub> B <sub>6</sub> C <sub>6</sub> | 0.3636 B <sub>9</sub> H <sub>11</sub> + 6 Y <sub>2</sub> C + 4.636 N <sub>2</sub> + 2.727 BN → 11 YN + YB <sub>6</sub> H <sub>4</sub> C <sub>6</sub> N                                            | -21.4228            |
| YNH <sub>4</sub> B <sub>6</sub> C <sub>6</sub> | 6 Y <sub>2</sub> C + 6.393 YB <sub>12</sub> + 0.5714 B <sub>5</sub> H <sub>7</sub> + YN → 18.39 YB <sub>4</sub> + YB <sub>6</sub> H <sub>4</sub> C <sub>6</sub> N                                 | -21.4109            |
| YNH <sub>4</sub> B <sub>6</sub> C <sub>6</sub> | 6 Y <sub>2</sub> C + 2 H <sub>2</sub> + BN + 49 B → 11 YB <sub>4</sub> + YB <sub>6</sub> H <sub>4</sub> C <sub>6</sub> N                                                                          | -21.3984            |
| YNH <sub>4</sub> B <sub>6</sub> C <sub>6</sub> | 0.3636 B <sub>9</sub> H <sub>11</sub> + 6 Y <sub>2</sub> C + 6.341 YB <sub>12</sub> + YN → 18.34 YB <sub>4</sub> + YB <sub>6</sub> H <sub>4</sub> C <sub>6</sub> N                                | -21.3607            |
| YNH <sub>4</sub> B <sub>6</sub> C <sub>6</sub> | 0.3333 YH <sub>3</sub> + 6 Y <sub>2</sub> C + H <sub>3</sub> N + 6.417 YB <sub>12</sub> → 17.75 YB <sub>4</sub> + YB <sub>6</sub> H <sub>4</sub> C <sub>6</sub> N                                 | -21.3360            |
| YNH <sub>4</sub> B <sub>6</sub> C <sub>6</sub> | 3 B <sub>13</sub> C <sub>2</sub> + 17.83 Y + 1.333 H <sub>3</sub> N → 0.3333 YN + 16.5 YB <sub>2</sub> + YB <sub>6</sub> H <sub>4</sub> C <sub>6</sub> N                                          | -21.3307            |
| YNH <sub>4</sub> B <sub>6</sub> C <sub>6</sub> | 0.4615 B <sub>13</sub> C <sub>2</sub> + 5.077 Y <sub>2</sub> C + 1.333 H <sub>3</sub> N + 4.41 N <sub>2</sub> → 9.154 YN + YB <sub>6</sub> H <sub>4</sub> C <sub>6</sub> N                        | -21.2786            |
| YNH <sub>4</sub> B <sub>6</sub> C <sub>6</sub> | 6 Y <sub>2</sub> C + H <sub>3</sub> N + 6.25 YB <sub>12</sub> + 0.5 H <sub>2</sub> → 17.25 YB <sub>4</sub> + YB <sub>6</sub> H <sub>4</sub> C <sub>6</sub> N                                      | -21.1825            |
| YNH <sub>4</sub> B <sub>6</sub> C <sub>6</sub> | 0.09091 B <sub>9</sub> H <sub>11</sub> + 3 B <sub>13</sub> C <sub>2</sub> + 17.91 Y + H <sub>3</sub> N → 16.91 YB <sub>2</sub> + YB <sub>6</sub> H <sub>4</sub> C <sub>6</sub> N                  | -21.1630            |

Continued on next page

Continued

| Compound                                       | Chemical reaction                                                                                                                                                                                 | Reaction energy(eV) |
|------------------------------------------------|---------------------------------------------------------------------------------------------------------------------------------------------------------------------------------------------------|---------------------|
| YNH <sub>4</sub> B <sub>6</sub> C <sub>6</sub> | 9.843 Y <sub>2</sub> C + 6.196 B <sub>5</sub> H <sub>7</sub> + YN → 19.69 YH <sub>2</sub> + 1.922 B <sub>13</sub> C <sub>2</sub> + YB <sub>6</sub> H <sub>4</sub> C <sub>6</sub> N                | -21.1347            |
| YNH <sub>4</sub> B <sub>6</sub> C <sub>6</sub> | 3 B <sub>13</sub> C <sub>2</sub> + 17.86 Y + H <sub>3</sub> N + 0.1429 B <sub>5</sub> H <sub>7</sub> → 16.86 YB <sub>2</sub> + YB <sub>6</sub> H <sub>4</sub> C <sub>6</sub> N                    | -21.0884            |
| YNH <sub>4</sub> B <sub>6</sub> C <sub>6</sub> | 6 Y <sub>2</sub> C + H <sub>3</sub> N + 6.161 YB <sub>12</sub> + 0.1429 B <sub>5</sub> H <sub>7</sub> → 17.16 YB <sub>4</sub> + YB <sub>6</sub> H <sub>4</sub> C <sub>6</sub> N                   | -21.0541            |
| YNH <sub>4</sub> B <sub>6</sub> C <sub>6</sub> | 6 Y <sub>2</sub> C + 6.818 H <sub>3</sub> N + 2.364 B <sub>5</sub> H <sub>7</sub> → 11 YH <sub>3</sub> + 5.818 BN + YB <sub>6</sub> H <sub>4</sub> C <sub>6</sub> N                               | -21.0518            |
| YNH <sub>4</sub> B <sub>6</sub> C <sub>6</sub> | 0.09091 B <sub>9</sub> H <sub>11</sub> + 6 Y <sub>2</sub> C + H <sub>3</sub> N + 6.148 YB <sub>12</sub> → 17.15 YB <sub>4</sub> + YB <sub>6</sub> H <sub>4</sub> C <sub>6</sub> N                 | -21.0415            |
| YNH <sub>4</sub> B <sub>6</sub> C <sub>6</sub> | 6 Y <sub>2</sub> C + 1.333 H <sub>3</sub> N + 6.083 YB <sub>12</sub> → 0.3333 YN + 16.75 YB <sub>4</sub> + YB <sub>6</sub> H <sub>4</sub> C <sub>6</sub> N                                        | -20.9351            |
| YNH <sub>4</sub> B <sub>6</sub> C <sub>6</sub> | 6 Y <sub>2</sub> C + 0.5714 B <sub>5</sub> H <sub>7</sub> + BN + 46.14 B → 11 YB <sub>4</sub> + YB <sub>6</sub> H <sub>4</sub> C <sub>6</sub> N                                                   | -20.8013            |
| YNH <sub>4</sub> B <sub>6</sub> C <sub>6</sub> | 5.733 B <sub>9</sub> H <sub>11</sub> + 1.2 Y <sub>4</sub> C <sub>5</sub> + 10.34 N <sub>2</sub> → 19.69 H <sub>3</sub> N + 3.8 YB <sub>12</sub> + YB <sub>6</sub> H <sub>4</sub> C <sub>6</sub> N | -20.7613            |
| YNH <sub>4</sub> B <sub>6</sub> C <sub>6</sub> | 3 B <sub>13</sub> C <sub>2</sub> + 17.33 Y + 1.333 H <sub>3</sub> N → 0.3333 BN + 16.33 YB <sub>2</sub> + YB <sub>6</sub> H <sub>4</sub> C <sub>6</sub> N                                         | -20.7425            |
| YNH <sub>4</sub> B <sub>6</sub> C <sub>6</sub> | 6 Y <sub>2</sub> C + 1.333 H <sub>3</sub> N + 6.25 YB <sub>12</sub> → 0.1667 N <sub>2</sub> + 17.25 YB <sub>4</sub> + YB <sub>6</sub> H <sub>4</sub> C <sub>6</sub> N                             | -20.7412            |
| YNH <sub>4</sub> B <sub>6</sub> C <sub>6</sub> | 0.3636 B <sub>9</sub> H <sub>11</sub> + 6 Y <sub>2</sub> C + BN + 45.73 B → 11 YB <sub>4</sub> + YB <sub>6</sub> H <sub>4</sub> C <sub>6</sub> N                                                  | -20.7390            |
| YNH <sub>4</sub> B <sub>6</sub> C <sub>6</sub> | 0.3636 B <sub>9</sub> H <sub>11</sub> + 3 B <sub>13</sub> C <sub>2</sub> + 18.14 Y + YN → 18.14 YB <sub>2</sub> + YB <sub>6</sub> H <sub>4</sub> C <sub>6</sub> N                                 | -20.6602            |
| YNH <sub>4</sub> B <sub>6</sub> C <sub>6</sub> | 3 B <sub>13</sub> C <sub>2</sub> + 17.5 Y + H <sub>3</sub> N + 0.5 H <sub>2</sub> → 16.5 YB <sub>2</sub> + YB <sub>6</sub> H <sub>4</sub> C <sub>6</sub> N                                        | -20.6177            |
| YNH <sub>4</sub> B <sub>6</sub> C <sub>6</sub> | 1.333 YH <sub>3</sub> + 6 Y <sub>2</sub> C + 6.792 YB <sub>12</sub> + BN → 19.12 YB <sub>4</sub> + YB <sub>6</sub> H <sub>4</sub> C <sub>6</sub> N                                                | -20.5830            |
| YNH <sub>4</sub> B <sub>6</sub> C <sub>6</sub> | 6 Y <sub>2</sub> C + 0.5714 B <sub>5</sub> H <sub>7</sub> + 4.429 N <sub>2</sub> + 3.143 BN → 11 YN + YB <sub>6</sub> H <sub>4</sub> C <sub>6</sub> N                                             | -20.4184            |
| YNH <sub>4</sub> B <sub>6</sub> C <sub>6</sub> | 3 B <sub>13</sub> C <sub>2</sub> + 17.93 Y + 0.5714 B <sub>5</sub> H <sub>7</sub> + YN → 17.93 YB <sub>2</sub> + YB <sub>6</sub> H <sub>4</sub> C <sub>6</sub> N                                  | -20.3617            |
| YNH <sub>4</sub> B <sub>6</sub> C <sub>6</sub> | 3 B <sub>13</sub> C <sub>2</sub> + 18 Y + 2 H <sub>2</sub> + BN → 17 YB <sub>2</sub> + YB <sub>6</sub> H <sub>4</sub> C <sub>6</sub> N                                                            | -20.2430            |
| YNH <sub>4</sub> B <sub>6</sub> C <sub>6</sub> | 3 B <sub>13</sub> C <sub>2</sub> + 17.5 Y + 1.333 H <sub>3</sub> N → 0.1667 N <sub>2</sub> + 16.5 YB <sub>2</sub> + YB <sub>6</sub> H <sub>4</sub> C <sub>6</sub> N                               | -20.1763            |
| YNH <sub>4</sub> B <sub>6</sub> C <sub>6</sub> | 6 Y <sub>2</sub> C + 6.125 YB <sub>12</sub> + 2 H <sub>2</sub> + BN → 17.12 YB <sub>4</sub> + YB <sub>6</sub> H <sub>4</sub> C <sub>6</sub> N                                                     | -19.9690            |
| YNH <sub>4</sub> B <sub>6</sub> C <sub>6</sub> | 9.725 Y <sub>2</sub> C + 5.843 B <sub>5</sub> H <sub>7</sub> + BN → 18.45 YH <sub>2</sub> + 1.863 B <sub>13</sub> C <sub>2</sub> + YB <sub>6</sub> H <sub>4</sub> C <sub>6</sub> N                | -19.8371            |
| YNH <sub>4</sub> B <sub>6</sub> C <sub>6</sub> | 0.3636 B <sub>9</sub> H <sub>11</sub> + 3 B <sub>13</sub> C <sub>2</sub> + 10.07 Y + 0.5 N <sub>2</sub> → 9.068 YB <sub>4</sub> + YB <sub>6</sub> H <sub>4</sub> C <sub>6</sub> N                 | -19.8212            |
| YNH <sub>4</sub> B <sub>6</sub> C <sub>6</sub> | 0.3333 YH <sub>3</sub> + 3 B <sub>13</sub> C <sub>2</sub> + 17.17 Y + H <sub>3</sub> N → 16.5 YB <sub>2</sub> + YB <sub>6</sub> H <sub>4</sub> C <sub>6</sub> N                                   | -19.8108            |
| YNH <sub>4</sub> B <sub>6</sub> C <sub>6</sub> | 6 Y <sub>2</sub> C + 5.6 B <sub>5</sub> H <sub>7</sub> + 6.367 N <sub>2</sub> → 11.73 H <sub>3</sub> N + 11 YB <sub>2</sub> + YB <sub>6</sub> H <sub>4</sub> C <sub>6</sub> N                     | -19.7699            |
| YNH <sub>4</sub> B <sub>6</sub> C <sub>6</sub> | 6 Y <sub>2</sub> C + 0.5 N <sub>2</sub> + 23 H <sub>2</sub> + 3 YB <sub>2</sub> → 14 YH <sub>3</sub> + YB <sub>6</sub> H <sub>4</sub> C <sub>6</sub> N                                            | -19.6693            |
| YNH <sub>4</sub> B <sub>6</sub> C <sub>6</sub> | 3 B <sub>13</sub> C <sub>2</sub> + 9.964 Y + 0.5714 B <sub>5</sub> H <sub>7</sub> + 0.5 N <sub>2</sub> → 8.964 YB <sub>4</sub> + YB <sub>6</sub> H <sub>4</sub> C <sub>6</sub> N                  | -19.5720            |
| YNH <sub>4</sub> B <sub>6</sub> C <sub>6</sub> | 0.5 YH <sub>2</sub> + 3 B <sub>13</sub> C <sub>2</sub> + 17 Y + H <sub>3</sub> N → 16.5 YB <sub>2</sub> + YB <sub>6</sub> H <sub>4</sub> C <sub>6</sub> N                                         | -19.5621            |
| YNH <sub>4</sub> B <sub>6</sub> C <sub>6</sub> | 6 Y <sub>2</sub> C + 5.768 YB <sub>12</sub> + 0.5714 B <sub>5</sub> H <sub>7</sub> + BN → 16.77 YB <sub>4</sub> + YB <sub>6</sub> H <sub>4</sub> C <sub>6</sub> N                                 | -19.4552            |
| YNH <sub>4</sub> B <sub>6</sub> C <sub>6</sub> | 0.3636 B <sub>9</sub> H <sub>11</sub> + 6 Y <sub>2</sub> C + 5.716 YB <sub>12</sub> + BN → 16.72 YB <sub>4</sub> + YB <sub>6</sub> H <sub>4</sub> C <sub>6</sub> N                                | -19.4050            |
| YNH <sub>4</sub> B <sub>6</sub> C <sub>6</sub> | 6.125 B <sub>9</sub> H <sub>11</sub> + 6.516 Y <sub>4</sub> C <sub>7</sub> + BN → 7.922 H <sub>8</sub> C <sub>5</sub> + 25.06 YB <sub>2</sub> + YB <sub>6</sub> H <sub>4</sub> C <sub>6</sub> N   | -19.2703            |
| YNH <sub>4</sub> B <sub>6</sub> C <sub>6</sub> | 5.375 Y <sub>2</sub> C + H <sub>3</sub> N + 0.125 H <sub>8</sub> C <sub>5</sub> + 45 B → 9.75 YB <sub>4</sub> + YB <sub>6</sub> H <sub>4</sub> C <sub>6</sub> N                                   | -19.2408            |
| YNH <sub>4</sub> B <sub>6</sub> C <sub>6</sub> | 2.125 B <sub>13</sub> C <sub>2</sub> + 22.62 H <sub>3</sub> N + 0.25 Y <sub>4</sub> C <sub>7</sub> → 31.94 H <sub>2</sub> + 21.62 BN + YB <sub>6</sub> H <sub>4</sub> C <sub>6</sub> N            | -18.9560            |
| YNH <sub>4</sub> B <sub>6</sub> C <sub>6</sub> | 8.863 Y <sub>2</sub> C + H <sub>3</sub> N + 4.922 B <sub>5</sub> H <sub>7</sub> → 16.73 YH <sub>2</sub> + 1.431 B <sub>13</sub> C <sub>2</sub> + YB <sub>6</sub> H <sub>4</sub> C <sub>6</sub> N  | -18.7317            |
| YNH <sub>4</sub> B <sub>6</sub> C <sub>6</sub> | 1.333 YH <sub>3</sub> + 3 B <sub>13</sub> C <sub>2</sub> + 16.17 Y + 0.5 N <sub>2</sub> → 16.5 YB <sub>2</sub> + YB <sub>6</sub> H <sub>4</sub> C <sub>6</sub> N                                  | -18.7142            |
| YNH <sub>4</sub> B <sub>6</sub> C <sub>6</sub> | 6 Y <sub>2</sub> C + YN + 24.5 H <sub>2</sub> + 3 YB <sub>2</sub> → 15 YH <sub>3</sub> + YB <sub>6</sub> H <sub>4</sub> C <sub>6</sub> N                                                          | -18.6269            |
| YNH <sub>4</sub> B <sub>6</sub> C <sub>6</sub> | 12.52 H <sub>3</sub> N + 0.8571 Y <sub>4</sub> C <sub>7</sub> + 8.762 YB <sub>2</sub> → 11.19 YH <sub>3</sub> + 11.52 BN + YB <sub>6</sub> H <sub>4</sub> C <sub>6</sub> N                        | -18.5499            |
| YNH <sub>4</sub> B <sub>6</sub> C <sub>6</sub> | 3 B <sub>13</sub> C <sub>2</sub> + 16.5 Y + YN + 2 H <sub>2</sub> → 16.5 YB <sub>2</sub> + YB <sub>6</sub> H <sub>4</sub> C <sub>6</sub> N                                                        | -18.4787            |
| YNH <sub>4</sub> B <sub>6</sub> C <sub>6</sub> | 6 Y <sub>2</sub> C + 12 H <sub>3</sub> N + 32.18 B → 2.909 B <sub>9</sub> H <sub>11</sub> + 11 YN + YB <sub>6</sub> H <sub>4</sub> C <sub>6</sub> N                                               | -18.4691            |
| YNH <sub>4</sub> B <sub>6</sub> C <sub>6</sub> | 6 Y <sub>2</sub> C + H <sub>3</sub> N + 21.5 H <sub>2</sub> + 3 YB <sub>2</sub> → 14 YH <sub>3</sub> + YB <sub>6</sub> H <sub>4</sub> C <sub>6</sub> N                                            | -18.3452            |
| YNH <sub>4</sub> B <sub>6</sub> C <sub>6</sub> | 3.5 Y <sub>2</sub> C + 0.5 H <sub>8</sub> C <sub>5</sub> + 5 N <sub>2</sub> + 3 YB <sub>2</sub> → 9 YN + YB <sub>6</sub> H <sub>4</sub> C <sub>6</sub> N                                          | -18.3361            |
| YNH <sub>4</sub> B <sub>6</sub> C <sub>6</sub> | 3 B <sub>13</sub> C <sub>2</sub> + 9.25 Y + 0.5 N <sub>2</sub> + 2 H <sub>2</sub> → 8.25 YB <sub>4</sub> + YB <sub>6</sub> H <sub>4</sub> C <sub>6</sub> N                                        | -18.0279            |
| YNH <sub>4</sub> B <sub>6</sub> C <sub>6</sub> | 0.3636 B <sub>9</sub> H <sub>11</sub> + 3 B <sub>13</sub> C <sub>2</sub> + 10.32 Y + BN → 9.318 YB <sub>4</sub> + YB <sub>6</sub> H <sub>4</sub> C <sub>6</sub> N                                 | -18.0039            |
| YNH <sub>4</sub> B <sub>6</sub> C <sub>6</sub> | 6 Y <sub>2</sub> C + 12 H <sub>3</sub> N + 28.86 B → 4.571 B <sub>5</sub> H <sub>7</sub> + 11 YN + YB <sub>6</sub> H <sub>4</sub> C <sub>6</sub> N                                                | -17.9710            |
| YNH <sub>4</sub> B <sub>6</sub> C <sub>6</sub> | 5.375 Y <sub>2</sub> C + H <sub>3</sub> N + 5.625 YB <sub>12</sub> + 0.125 H <sub>8</sub> C <sub>5</sub> → 15.37 YB <sub>4</sub> + YB <sub>6</sub> H <sub>4</sub> C <sub>6</sub> N                | -17.9281            |
| YNH <sub>4</sub> B <sub>6</sub> C <sub>6</sub> | 3.111 B <sub>9</sub> H <sub>11</sub> + 6 Y <sub>2</sub> C + 5.537 N <sub>2</sub> → 10.07 H <sub>3</sub> N + 11 YB <sub>2</sub> + YB <sub>6</sub> H <sub>4</sub> C <sub>6</sub> N                  | -17.7833            |
| YNH <sub>4</sub> B <sub>6</sub> C <sub>6</sub> | 3 B <sub>13</sub> C <sub>2</sub> + 10.21 Y + 0.5714 B <sub>5</sub> H <sub>7</sub> + BN → 9.214 YB <sub>4</sub> + YB <sub>6</sub> H <sub>4</sub> C <sub>6</sub> N                                  | -17.7547            |
| YNH <sub>4</sub> B <sub>6</sub> C <sub>6</sub> | 2 YH <sub>2</sub> + 3 B <sub>13</sub> C <sub>2</sub> + 15.5 Y + 0.5 N <sub>2</sub> → 16.5 YB <sub>2</sub> + YB <sub>6</sub> H <sub>4</sub> C <sub>6</sub> N                                       | -17.7194            |
| YNH <sub>4</sub> B <sub>6</sub> C <sub>6</sub> | 6 Y <sub>2</sub> C + 0.5 N <sub>2</sub> + 18.5 H <sub>2</sub> + 6 B → 11 YH <sub>3</sub> + YB <sub>6</sub> H <sub>4</sub> C <sub>6</sub> N                                                        | -17.6158            |
| YNH <sub>4</sub> B <sub>6</sub> C <sub>6</sub> | 3 B <sub>13</sub> C <sub>2</sub> + 9.583 Y + 1.333 H <sub>3</sub> N → 0.3333 YN + 8.25 YB <sub>4</sub> + YB <sub>6</sub> H <sub>4</sub> C <sub>6</sub> N                                          | -17.4168            |
| YNH <sub>4</sub> B <sub>6</sub> C <sub>6</sub> | 0.3636 B <sub>9</sub> H <sub>11</sub> + 6 C + YB <sub>12</sub> + 5.136 N <sub>2</sub> → 9.273 BN + YB <sub>6</sub> H <sub>4</sub> C <sub>6</sub> N                                                | -17.2327            |
| YNH <sub>4</sub> B <sub>6</sub> C <sub>6</sub> | 6 Y <sub>2</sub> C + 0.5 YB <sub>12</sub> + 0.5 N <sub>2</sub> + 19.25 H <sub>2</sub> → 11.5 YH <sub>3</sub> + YB <sub>6</sub> H <sub>4</sub> C <sub>6</sub> N                                    | -17.2105            |
| YNH <sub>4</sub> B <sub>6</sub> C <sub>6</sub> | 2.687 B <sub>13</sub> C <sub>2</sub> + 15.47 Y + H <sub>3</sub> N + 0.125 H <sub>8</sub> C <sub>5</sub> → 14.47 YB <sub>2</sub> + YB <sub>6</sub> H <sub>4</sub> C <sub>6</sub> N                 | -17.1979            |
| YNH <sub>4</sub> B <sub>6</sub> C <sub>6</sub> | 0.09091 B <sub>9</sub> H <sub>11</sub> + 3 B <sub>13</sub> C <sub>2</sub> + 9.455 Y + H <sub>3</sub> N → 8.455 YB <sub>4</sub> + YB <sub>6</sub> H <sub>4</sub> C <sub>6</sub> N                  | -17.1521            |
| YNH <sub>4</sub> B <sub>6</sub> C <sub>6</sub> | 3 B <sub>13</sub> C <sub>2</sub> + 9.429 Y + H <sub>3</sub> N + 0.1429 B <sub>5</sub> H <sub>7</sub> → 8.429 YB <sub>4</sub> + YB <sub>6</sub> H <sub>4</sub> C <sub>6</sub> N                    | -17.0898            |
| YNH <sub>4</sub> B <sub>6</sub> C <sub>6</sub> | 1.333 YH <sub>3</sub> + 3 B <sub>13</sub> C <sub>2</sub> + 16.67 Y + BN → 17 YB <sub>2</sub> + YB <sub>6</sub> H <sub>4</sub> C <sub>6</sub> N                                                    | -17.0155            |
| YNH <sub>4</sub> B <sub>6</sub> C <sub>6</sub> | 3 B <sub>13</sub> C <sub>2</sub> + 9.167 Y + 1.333 H <sub>3</sub> N → 0.3333 BN + 8.167 YB <sub>4</sub> + YB <sub>6</sub> H <sub>4</sub> C <sub>6</sub> N                                         | -16.8682            |
| YNH <sub>4</sub> B <sub>6</sub> C <sub>6</sub> | 6 Y <sub>2</sub> C + 22.25 H <sub>2</sub> + BN + 2.5 YB <sub>2</sub> → 13.5 YH <sub>3</sub> + YB <sub>6</sub> H <sub>4</sub> C <sub>6</sub> N                                                     | -16.7603            |
| YNH <sub>4</sub> B <sub>6</sub> C <sub>6</sub> | 6 Y <sub>2</sub> C + 0.5 N <sub>2</sub> + 20.75 H <sub>2</sub> + 1.5 YB <sub>4</sub> → 12.5 YH <sub>3</sub> + YB <sub>6</sub> H <sub>4</sub> C <sub>6</sub> N                                     | -16.7500            |
| YNH <sub>4</sub> B <sub>6</sub> C <sub>6</sub> | 3 B <sub>13</sub> C <sub>2</sub> + 9.25 Y + H <sub>3</sub> N + 0.5 H <sub>2</sub> → 8.25 YB <sub>4</sub> + YB <sub>6</sub> H <sub>4</sub> C <sub>6</sub> N                                        | -16.7038            |
| YNH <sub>4</sub> B <sub>6</sub> C <sub>6</sub> | 6 Y <sub>2</sub> C + YN + 20 H <sub>2</sub> + 6 B → 12 YH <sub>3</sub> + YB <sub>6</sub> H <sub>4</sub> C <sub>6</sub> N                                                                          | -16.5734            |
| YNH <sub>4</sub> B <sub>6</sub> C <sub>6</sub> | 6 Y <sub>2</sub> C + 15.37 H <sub>3</sub> N + 3.371 YB <sub>12</sub> → 3.829 B <sub>9</sub> H <sub>11</sub> + 14.37 YN + YB <sub>6</sub> H <sub>4</sub> C <sub>6</sub> N                          | -16.4541            |

Continued on next page

Continued

| Compound                                       | Chemical reaction                                                                                                                                                                                     | Reaction energy(eV) |
|------------------------------------------------|-------------------------------------------------------------------------------------------------------------------------------------------------------------------------------------------------------|---------------------|
| YNH <sub>4</sub> B <sub>6</sub> C <sub>6</sub> | 1.4 B <sub>9</sub> H <sub>11</sub> + 1.2 Y <sub>4</sub> C <sub>5</sub> + 3.8 N <sub>2</sub> → 3.8 YH <sub>3</sub> + 6.6 BN + YB <sub>6</sub> H <sub>4</sub> C <sub>6</sub> N                          | -16.4104            |
| YNH <sub>4</sub> B <sub>6</sub> C <sub>6</sub> | 0.6667 B <sub>9</sub> H <sub>11</sub> + 6 Y <sub>2</sub> C + 0.5 N <sub>2</sub> + 14.83 H <sub>2</sub> → 11 YH <sub>3</sub> + YB <sub>6</sub> H <sub>4</sub> C <sub>6</sub> N                         | -16.4068            |
| YNH <sub>4</sub> B <sub>6</sub> C <sub>6</sub> | 2 YH <sub>2</sub> + 6 Y <sub>2</sub> C + 4 N <sub>2</sub> + 6 BN → 13 YN + YB <sub>6</sub> H <sub>4</sub> C <sub>6</sub> N                                                                            | -16.3857            |
| YNH <sub>4</sub> B <sub>6</sub> C <sub>6</sub> | 6 Y <sub>2</sub> C + 1.2 B <sub>5</sub> H <sub>7</sub> + 0.5 N <sub>2</sub> + 14.3 H <sub>2</sub> → 11 YH <sub>3</sub> + YB <sub>6</sub> H <sub>4</sub> C <sub>6</sub> N                              | -16.3618            |
| YNH <sub>4</sub> B <sub>6</sub> C <sub>6</sub> | 0.3636 B <sub>9</sub> H <sub>11</sub> + 3 B <sub>13</sub> C <sub>2</sub> + 9.068 Y + YN → 9.068 YB <sub>4</sub> + YB <sub>6</sub> H <sub>4</sub> C <sub>6</sub> N                                     | -16.3581            |
| YNH <sub>4</sub> B <sub>6</sub> C <sub>6</sub> | 6 Y <sub>2</sub> C + 8.167 H <sub>3</sub> N + 3 YB <sub>2</sub> → 6.833 YH <sub>3</sub> + 7.167 YN + YB <sub>6</sub> H <sub>4</sub> C <sub>6</sub> N                                                  | -16.3268            |
| YNH <sub>4</sub> B <sub>6</sub> C <sub>6</sub> | 41.25 B <sub>9</sub> H <sub>11</sub> + 6 Y <sub>2</sub> C + 0.5 N <sub>2</sub> → 64.25 B <sub>5</sub> H <sub>7</sub> + 11 YB <sub>4</sub> + YB <sub>6</sub> H <sub>4</sub> C <sub>6</sub> N           | -16.3044            |
| YNH <sub>4</sub> B <sub>6</sub> C <sub>6</sub> | 6 Y <sub>2</sub> C + H <sub>3</sub> N + 17 H <sub>2</sub> + 6 B → 11 YH <sub>3</sub> + YB <sub>6</sub> H <sub>4</sub> C <sub>6</sub> N                                                                | -16.2917            |
| YNH <sub>4</sub> B <sub>6</sub> C <sub>6</sub> | 3 B <sub>13</sub> C <sub>2</sub> + 9.25 Y + 1.333 H <sub>3</sub> N → 0.1667 N <sub>2</sub> + 8.25 YB <sub>4</sub> + YB <sub>6</sub> H <sub>4</sub> C <sub>6</sub> N                                   | -16.2624            |
| YNH <sub>4</sub> B <sub>6</sub> C <sub>6</sub> | 6 C + YB <sub>12</sub> + 0.5714 B <sub>5</sub> H <sub>7</sub> + 4.929 N <sub>2</sub> → 8.857 BN + YB <sub>6</sub> H <sub>4</sub> C <sub>6</sub> N                                                     | -16.2283            |
| YNH <sub>4</sub> B <sub>6</sub> C <sub>6</sub> | 1.02 B <sub>13</sub> C <sub>2</sub> + 3.961 Y <sub>2</sub> C + 8.255 H <sub>3</sub> N → 6.922 YH <sub>3</sub> + 7.255 BN + YB <sub>6</sub> H <sub>4</sub> C <sub>6</sub> N                            | -16.2189            |
| YNH <sub>4</sub> B <sub>6</sub> C <sub>6</sub> | 3 B <sub>13</sub> C <sub>2</sub> + 9.5 Y + 2 H <sub>2</sub> + BN → 8.5 YB <sub>4</sub> + YB <sub>6</sub> H <sub>4</sub> C <sub>6</sub> N                                                              | -16.2106            |
| YNH <sub>4</sub> B <sub>6</sub> C <sub>6</sub> | 6 Y <sub>2</sub> C + 0.5 YB <sub>12</sub> + YN + 20.75 H <sub>2</sub> → 12.5 YH <sub>3</sub> + YB <sub>6</sub> H <sub>4</sub> C <sub>6</sub> N                                                        | -16.1681            |
| YNH <sub>4</sub> B <sub>6</sub> C <sub>6</sub> | 3 B <sub>13</sub> C <sub>2</sub> + 8.964 Y + 0.5714 B <sub>5</sub> H <sub>7</sub> + YN → 8.964 YB <sub>4</sub> + YB <sub>6</sub> H <sub>4</sub> C <sub>6</sub> N                                      | -16.1090            |
| YNH <sub>4</sub> B <sub>6</sub> C <sub>6</sub> | 6 Y <sub>2</sub> C + 14.93 H <sub>3</sub> N + 2.928 YB <sub>12</sub> → 5.826 B <sub>5</sub> H <sub>7</sub> + 13.93 YN + YB <sub>6</sub> H <sub>4</sub> C <sub>6</sub> N                               | -16.0845            |
| YNH <sub>4</sub> B <sub>6</sub> C <sub>6</sub> | 2 YH <sub>2</sub> + 3 B <sub>13</sub> C <sub>2</sub> + 16 Y + BN → 17 YB <sub>2</sub> + YB <sub>6</sub> H <sub>4</sub> C <sub>6</sub> N                                                               | -16.0207            |
| YNH <sub>4</sub> B <sub>6</sub> C <sub>6</sub> | 0.3333 YH <sub>3</sub> + 3 B <sub>13</sub> C <sub>2</sub> + 8.917 Y + H <sub>3</sub> N → 8.25 YB <sub>4</sub> + YB <sub>6</sub> H <sub>4</sub> C <sub>6</sub> N                                       | -15.8969            |
| YNH <sub>4</sub> B <sub>6</sub> C <sub>6</sub> | 6 Y <sub>2</sub> C + H <sub>3</sub> N + 0.5 YB <sub>12</sub> + 17.75 H <sub>2</sub> → 11.5 YH <sub>3</sub> + YB <sub>6</sub> H <sub>4</sub> C <sub>6</sub> N                                          | -15.8864            |
| YNH <sub>4</sub> B <sub>6</sub> C <sub>6</sub> | 1.125 B <sub>13</sub> C <sub>2</sub> + 0.25 Y <sub>4</sub> C <sub>5</sub> + 0.5 H <sub>8</sub> C <sub>5</sub> + 4.812 N <sub>2</sub> → 8.625 BN + YB <sub>6</sub> H <sub>4</sub> C <sub>6</sub> N     | -15.7597            |
| YNH <sub>4</sub> B <sub>6</sub> C <sub>6</sub> | 6 Y <sub>2</sub> C + YN + 22.25 H <sub>2</sub> + 1.5 YB <sub>4</sub> → 13.5 YH <sub>3</sub> + YB <sub>6</sub> H <sub>4</sub> C <sub>6</sub> N                                                         | -15.7075            |
| YNH <sub>4</sub> B <sub>6</sub> C <sub>6</sub> | 0.5 YH <sub>2</sub> + 3 B <sub>13</sub> C <sub>2</sub> + 8.75 Y + H <sub>3</sub> N → 8.25 YB <sub>4</sub> + YB <sub>6</sub> H <sub>4</sub> C <sub>6</sub> N                                           | -15.6482            |
| YNH <sub>4</sub> B <sub>6</sub> C <sub>6</sub> | 2.338 B <sub>9</sub> H <sub>11</sub> + 6 Y <sub>2</sub> C + 0.5 N <sub>2</sub> → 7.239 YH <sub>3</sub> + 3.761 YB <sub>4</sub> + YB <sub>6</sub> H <sub>4</sub> C <sub>6</sub> N                      | -15.5466            |
| YNH <sub>4</sub> B <sub>6</sub> C <sub>6</sub> | 1.079 B <sub>9</sub> H <sub>11</sub> + 6 Y <sub>2</sub> C + 4.711 H <sub>3</sub> N → 11 YH <sub>2</sub> + 3.711 BN + YB <sub>6</sub> H <sub>4</sub> C <sub>6</sub> N                                  | -15.5423            |
| YNH <sub>4</sub> B <sub>6</sub> C <sub>6</sub> | 6 Y <sub>2</sub> C + 3.86 B <sub>5</sub> H <sub>7</sub> + 0.5 N <sub>2</sub> → 7.674 YH <sub>3</sub> + 3.326 YB <sub>4</sub> + YB <sub>6</sub> H <sub>4</sub> C <sub>6</sub> N                        | -15.5011            |
| YNH <sub>4</sub> B <sub>6</sub> C <sub>6</sub> | 6 Y <sub>2</sub> C + H <sub>3</sub> N + 19.25 H <sub>2</sub> + 1.5 YB <sub>4</sub> → 12.5 YH <sub>3</sub> + YB <sub>6</sub> H <sub>4</sub> C <sub>6</sub> N                                           | -15.4259            |
| YNH <sub>4</sub> B <sub>6</sub> C <sub>6</sub> | 0.6667 B <sub>9</sub> H <sub>11</sub> + 6 Y <sub>2</sub> C + YN + 16.33 H <sub>2</sub> → 12 YH <sub>3</sub> + YB <sub>6</sub> H <sub>4</sub> C <sub>6</sub> N                                         | -15.3644            |
| YNH <sub>4</sub> B <sub>6</sub> C <sub>6</sub> | 6 Y <sub>2</sub> C + 0.5 N <sub>2</sub> + 16 H <sub>2</sub> + 3 YB <sub>2</sub> → 14 YH <sub>2</sub> + YB <sub>6</sub> H <sub>4</sub> C <sub>6</sub> N                                                | -15.3371            |
| YNH <sub>4</sub> B <sub>6</sub> C <sub>6</sub> | 6 Y <sub>2</sub> C + 1.2 B <sub>5</sub> H <sub>7</sub> + YN + 15.8 H <sub>2</sub> → 12 YH <sub>3</sub> + YB <sub>6</sub> H <sub>4</sub> C <sub>6</sub> N                                              | -15.3193            |
| YNH <sub>4</sub> B <sub>6</sub> C <sub>6</sub> | 1.333 YH <sub>3</sub> + 3 B <sub>13</sub> C <sub>2</sub> + 15.17 Y + YN → 16.5 YB <sub>2</sub> + YB <sub>6</sub> H <sub>4</sub> C <sub>6</sub> N                                                      | -15.2512            |
| YNH <sub>4</sub> B <sub>6</sub> C <sub>6</sub> | 44.75 B <sub>9</sub> H <sub>11</sub> + 6 Y <sub>2</sub> C + YN → 69.75 B <sub>5</sub> H <sub>7</sub> + 12 YB <sub>4</sub> + YB <sub>6</sub> H <sub>4</sub> C <sub>6</sub> N                           | -15.2399            |
| YNH <sub>4</sub> B <sub>6</sub> C <sub>6</sub> | 6 Y <sub>2</sub> C + 33.38 B <sub>5</sub> H <sub>7</sub> + 0.5 N <sub>2</sub> → 11 YH <sub>3</sub> + 17.88 B <sub>9</sub> H <sub>11</sub> + YB <sub>6</sub> H <sub>4</sub> C <sub>6</sub> N           | -15.1530            |
| YNH <sub>4</sub> B <sub>6</sub> C <sub>6</sub> | 43.12 B <sub>9</sub> H <sub>11</sub> + 6 Y <sub>2</sub> C + H <sub>3</sub> N → 67.62 B <sub>5</sub> H <sub>7</sub> + 11 YB <sub>4</sub> + YB <sub>6</sub> H <sub>4</sub> C <sub>6</sub> N             | -15.1071            |
| YNH <sub>4</sub> B <sub>6</sub> C <sub>6</sub> | 0.6667 B <sub>9</sub> H <sub>11</sub> + 6 Y <sub>2</sub> C + H <sub>3</sub> N + 13.33 H <sub>2</sub> → 11 YH <sub>3</sub> + YB <sub>6</sub> H <sub>4</sub> C <sub>6</sub> N                           | -15.0828            |
| YNH <sub>4</sub> B <sub>6</sub> C <sub>6</sub> | 1.333 YH <sub>3</sub> + 6 Y <sub>2</sub> C + 3.667 N <sub>2</sub> + 6 BN → 12.33 YN + YB <sub>6</sub> H <sub>4</sub> C <sub>6</sub> N                                                                 | -15.0719            |
| YNH <sub>4</sub> B <sub>6</sub> C <sub>6</sub> | 6 Y <sub>2</sub> C + 4.318 H <sub>3</sub> N + 1.864 B <sub>5</sub> H <sub>7</sub> → 11 YH <sub>2</sub> + 3.318 BN + YB <sub>6</sub> H <sub>4</sub> C <sub>6</sub> N                                   | -15.0638            |
| YNH <sub>4</sub> B <sub>6</sub> C <sub>6</sub> | 6 Y <sub>2</sub> C + 18.5 H <sub>2</sub> + BN + 5 B → 11 YH <sub>3</sub> + YB <sub>6</sub> H <sub>4</sub> C <sub>6</sub> N                                                                            | -15.0490            |
| YNH <sub>4</sub> B <sub>6</sub> C <sub>6</sub> | 0.3636 B <sub>9</sub> H <sub>11</sub> + 3 B <sub>13</sub> C <sub>2</sub> + 0.5 N <sub>2</sub> + 20.14 YB <sub>2</sub> → 19.14 YB <sub>4</sub> + YB <sub>6</sub> H <sub>4</sub> C <sub>6</sub> N       | -15.0448            |
| YNH <sub>4</sub> B <sub>6</sub> C <sub>6</sub> | 6 Y <sub>2</sub> C + H <sub>3</sub> N + 1.2 B <sub>5</sub> H <sub>7</sub> + 12.8 H <sub>2</sub> → 11 YH <sub>3</sub> + YB <sub>6</sub> H <sub>4</sub> C <sub>6</sub> N                                | -15.0377            |
| YNH <sub>4</sub> B <sub>6</sub> C <sub>6</sub> | 3 B <sub>13</sub> C <sub>2</sub> + 0.5714 B <sub>5</sub> H <sub>7</sub> + 0.5 N <sub>2</sub> + 19.93 YB <sub>2</sub> → 18.93 YB <sub>4</sub> + YB <sub>6</sub> H <sub>4</sub> C <sub>6</sub> N        | -14.8449            |
| YNH <sub>4</sub> B <sub>6</sub> C <sub>6</sub> | 1.333 YH <sub>3</sub> + 3 B <sub>13</sub> C <sub>2</sub> + 7.917 Y + 0.5 N <sub>2</sub> → 8.25 YB <sub>4</sub> + YB <sub>6</sub> H <sub>4</sub> C <sub>6</sub> N                                      | -14.8003            |
| YNH <sub>4</sub> B <sub>6</sub> C <sub>6</sub> | 6 Y <sub>2</sub> C + 0.4167 YB <sub>12</sub> + 19.12 H <sub>2</sub> + BN → 11.42 YH <sub>3</sub> + YB <sub>6</sub> H <sub>4</sub> C <sub>6</sub> N                                                    | -14.7113            |
| YNH <sub>4</sub> B <sub>6</sub> C <sub>6</sub> | 6 Y <sub>2</sub> C + 6.667 H <sub>3</sub> N + 6 B → 5.333 YH <sub>3</sub> + 5.667 YN + YB <sub>6</sub> H <sub>4</sub> C <sub>6</sub> N                                                                | -14.6958            |
| YNH <sub>4</sub> B <sub>6</sub> C <sub>6</sub> | 3 B <sub>13</sub> C <sub>2</sub> + 8.25 Y + YN + 2 H <sub>2</sub> → 8.25 YB <sub>4</sub> + YB <sub>6</sub> H <sub>4</sub> C <sub>6</sub> N                                                            | -14.5648            |
| YNH <sub>4</sub> B <sub>6</sub> C <sub>6</sub> | 2.507 B <sub>9</sub> H <sub>11</sub> + 6 Y <sub>2</sub> C + YN → 7.859 YH <sub>3</sub> + 4.141 YB <sub>4</sub> + YB <sub>6</sub> H <sub>4</sub> C <sub>6</sub> N                                      | -14.4172            |
| YNH <sub>4</sub> B <sub>6</sub> C <sub>6</sub> | 6 Y <sub>2</sub> C + 15 H <sub>3</sub> N + 3 YB <sub>2</sub> → 14 YN + 20.5 H <sub>2</sub> + YB <sub>6</sub> H <sub>4</sub> C <sub>6</sub> N                                                          | -14.4023            |
| YNH <sub>4</sub> B <sub>6</sub> C <sub>6</sub> | 6 Y <sub>2</sub> C + 4.14 B <sub>5</sub> H <sub>7</sub> + YN → 8.326 YH <sub>3</sub> + 3.674 YB <sub>4</sub> + YB <sub>6</sub> H <sub>4</sub> C <sub>6</sub> N                                        | -14.3684            |
| YNH <sub>4</sub> B <sub>6</sub> C <sub>6</sub> | 6 Y <sub>2</sub> C + 20.38 H <sub>2</sub> + BN + 1.25 YB <sub>4</sub> → 12.25 YH <sub>3</sub> + YB <sub>6</sub> H <sub>4</sub> C <sub>6</sub> N                                                       | -14.3275            |
| YNH <sub>4</sub> B <sub>6</sub> C <sub>6</sub> | 2.169 B <sub>9</sub> H <sub>11</sub> + 6 Y <sub>2</sub> C + H <sub>3</sub> N → 7.62 YH <sub>3</sub> + 3.38 YB <sub>4</sub> + YB <sub>6</sub> H <sub>4</sub> C <sub>6</sub> N                          | -14.3095            |
| YNH <sub>4</sub> B <sub>6</sub> C <sub>6</sub> | 6 Y <sub>2</sub> C + H <sub>3</sub> N + 3.581 B <sub>5</sub> H <sub>7</sub> → 8.023 YH <sub>3</sub> + 2.977 YB <sub>4</sub> + YB <sub>6</sub> H <sub>4</sub> C <sub>6</sub> N                         | -14.2673            |
| YNH <sub>4</sub> B <sub>6</sub> C <sub>6</sub> | 2 YH <sub>2</sub> + 3 B <sub>13</sub> C <sub>2</sub> + 14.5 Y + YN → 16.5 YB <sub>2</sub> + YB <sub>6</sub> H <sub>4</sub> C <sub>6</sub> N                                                           | -14.2563            |
| YNH <sub>4</sub> B <sub>6</sub> C <sub>6</sub> | 6 Y <sub>2</sub> C + 6.917 H <sub>3</sub> N + 0.5 YB <sub>12</sub> → 5.583 YH <sub>3</sub> + 5.917 YN + YB <sub>6</sub> H <sub>4</sub> C <sub>6</sub> N                                               | -14.2201            |
| YNH <sub>4</sub> B <sub>6</sub> C <sub>6</sub> | 6 Y <sub>2</sub> C + 0.5 N <sub>2</sub> + 13 H <sub>2</sub> + 6 B → 11 YH <sub>2</sub> + YB <sub>6</sub> H <sub>4</sub> C <sub>6</sub> N                                                              | -14.2119            |
| YNH <sub>4</sub> B <sub>6</sub> C <sub>6</sub> | 6 Y <sub>2</sub> C + 6.8 H <sub>3</sub> N + 3 YB <sub>2</sub> → 8.2 YH <sub>2</sub> + 5.8 YN + YB <sub>6</sub> H <sub>4</sub> C <sub>6</sub> N                                                        | -14.1743            |
| YNH <sub>4</sub> B <sub>6</sub> C <sub>6</sub> | 16.73 YH <sub>3</sub> + 3 B <sub>13</sub> C <sub>2</sub> + 8.367 N <sub>2</sub> → 6.6 B <sub>5</sub> H <sub>7</sub> + 15.73 YN + YB <sub>6</sub> H <sub>4</sub> C <sub>6</sub> N                      | -14.1731            |
| YNH <sub>4</sub> B <sub>6</sub> C <sub>6</sub> | 7.029 B <sub>5</sub> H <sub>7</sub> + 8.033 N <sub>2</sub> + 0.8571 Y <sub>4</sub> C <sub>7</sub> → 15.07 H <sub>3</sub> N + 2.429 YB <sub>12</sub> + YB <sub>6</sub> H <sub>4</sub> C <sub>6</sub> N | -14.1288            |
| YNH <sub>4</sub> B <sub>6</sub> C <sub>6</sub> | 0.5556 B <sub>9</sub> H <sub>11</sub> + 6 Y <sub>2</sub> C + 15.44 H <sub>2</sub> + BN → 11 YH <sub>3</sub> + YB <sub>6</sub> H <sub>4</sub> C <sub>6</sub> N                                         | -14.0416            |
| YNH <sub>4</sub> B <sub>6</sub> C <sub>6</sub> | 6 Y <sub>2</sub> C + H <sub>3</sub> N + 14.5 H <sub>2</sub> + 3 YB <sub>2</sub> → 14 YH <sub>2</sub> + YB <sub>6</sub> H <sub>4</sub> C <sub>6</sub> N                                                | -14.0131            |
| YNH <sub>4</sub> B <sub>6</sub> C <sub>6</sub> | 6 Y <sub>2</sub> C + B <sub>5</sub> H <sub>7</sub> + 15 H <sub>2</sub> + BN → 11 YH <sub>3</sub> + YB <sub>6</sub> H <sub>4</sub> C <sub>6</sub> N                                                    | -14.0040            |
| YNH <sub>4</sub> B <sub>6</sub> C <sub>6</sub> | 6 Y <sub>2</sub> C + YN + 17 H <sub>2</sub> + 3 YB <sub>2</sub> → 15 YH <sub>2</sub> + YB <sub>6</sub> H <sub>4</sub> C <sub>6</sub> N                                                                | -13.9853            |
| YNH <sub>4</sub> B <sub>6</sub> C <sub>6</sub> | 6 Y <sub>2</sub> C + 36.75 B <sub>5</sub> H <sub>7</sub> + YN → 12 YH <sub>3</sub> + 19.75 B <sub>9</sub> H <sub>11</sub> + YB <sub>6</sub> H <sub>4</sub> C <sub>6</sub> N                           | -13.9837            |

Continued on next page

Continued

| Compound                                       | Chemical reaction                                                                                                                                                                   | Reaction energy(eV) |
|------------------------------------------------|-------------------------------------------------------------------------------------------------------------------------------------------------------------------------------------|---------------------|
| YNH <sub>4</sub> B <sub>6</sub> C <sub>6</sub> | $6 \text{ Y}_2\text{C} + \text{H}_3\text{N} + 30 \text{ B}_5\text{H}_7 \rightarrow 11 \text{ YH}_3 + 16 \text{ B}_9\text{H}_{11} + \text{YB}_6\text{H}_4\text{C}_6\text{N}$         | -13.9557            |
| YNH <sub>4</sub> B <sub>6</sub> C <sub>6</sub> | $6 \text{ Y}_2\text{C} + 4.667 \text{ B}_5\text{H}_7 + 0.5 \text{ N}_2 \rightarrow 9.556 \text{ YH}_3 + 1.444 \text{ YB}_{12} + \text{YB}_6\text{H}_4\text{C}_6\text{N}$            | -13.9099            |
| YNH <sub>4</sub> B <sub>6</sub> C <sub>6</sub> | $5.556 \text{ B}_9\text{H}_{11} + 6 \text{ Y}_2\text{C} + 0.5 \text{ N}_2 \rightarrow 28.56 \text{ H}_2 + 11 \text{ YB}_4 + \text{YB}_6\text{H}_4\text{C}_6\text{N}$                | -13.8906            |
| YNH <sub>4</sub> B <sub>6</sub> C <sub>6</sub> | $40.37 \text{ B}_9\text{H}_{11} + 6 \text{ Y}_2\text{C} + \text{BN} \rightarrow 62.87 \text{ B}_5\text{H}_7 + 11 \text{ YB}_4 + \text{YB}_6\text{H}_4\text{C}_6\text{N}$            | -13.8875            |
| YNH <sub>4</sub> B <sub>6</sub> C <sub>6</sub> | $2 \text{ YH}_2 + 1.2 \text{ Y}_4\text{C}_5 + 4.9 \text{ N}_2 + 3 \text{ YB}_2 \rightarrow 8.8 \text{ YN} + \text{YB}_6\text{H}_4\text{C}_6\text{N}$                                | -13.8543            |
| YNH <sub>4</sub> B <sub>6</sub> C <sub>6</sub> | $3.5 \text{ Y}_2\text{C} + 0.5 \text{ H}_8\text{C}_5 + 4.25 \text{ N}_2 + 1.5 \text{ YB}_4 \rightarrow 7.5 \text{ YN} + \text{YB}_6\text{H}_4\text{C}_6\text{N}$                    | -13.8531            |
| YNH <sub>4</sub> B <sub>6</sub> C <sub>6</sub> | $6 \text{ Y}_2\text{C} + 5.267 \text{ H}_3\text{N} + 1.2 \text{ B}_5\text{H}_7 \rightarrow 6.733 \text{ YH}_3 + 4.267 \text{ YN} + \text{YB}_6\text{H}_4\text{C}_6\text{N}$         | -13.8360            |
| YNH <sub>4</sub> B <sub>6</sub> C <sub>6</sub> | $0.6667 \text{ B}_9\text{H}_{11} + 6 \text{ Y}_2\text{C} + 5.444 \text{ H}_3\text{N} \rightarrow 6.556 \text{ YH}_3 + 4.444 \text{ YN} + \text{YB}_6\text{H}_4\text{C}_6\text{N}$   | -13.8310            |
| YNH <sub>4</sub> B <sub>6</sub> C <sub>6</sub> | $2 \text{ YH}_2 + 3 \text{ B}_{13}\text{C}_2 + 7.25 \text{ Y} + 0.5 \text{ N}_2 \rightarrow 8.25 \text{ YB}_4 + \text{YB}_6\text{H}_4\text{C}_6\text{N}$                            | -13.8055            |
| YNH <sub>4</sub> B <sub>6</sub> C <sub>6</sub> | $2.687 \text{ B}_{13}\text{C}_2 + 8.234 \text{ Y} + \text{H}_3\text{N} + 0.125 \text{ H}_8\text{C}_5 \rightarrow 7.234 \text{ YB}_4 + \text{YB}_6\text{H}_4\text{C}_6\text{N}$      | -13.7658            |
| YNH <sub>4</sub> B <sub>6</sub> C <sub>6</sub> | $2.906 \text{ B}_9\text{H}_{11} + 6 \text{ Y}_2\text{C} + 0.5 \text{ N}_2 \rightarrow 9.321 \text{ YH}_3 + 1.679 \text{ YB}_{12} + \text{YB}_6\text{H}_4\text{C}_6\text{N}$         | -13.7078            |
| YNH <sub>4</sub> B <sub>6</sub> C <sub>6</sub> | $6 \text{ Y}_2\text{C} + 3 \text{ N}_2 + 2 \text{ H}_2 + 6 \text{ BN} \rightarrow 11 \text{ YN} + \text{YB}_6\text{H}_4\text{C}_6\text{N}$                                          | -13.6820            |
| YNH <sub>4</sub> B <sub>6</sub> C <sub>6</sub> | $6 \text{ Y}_2\text{C} + 0.5 \text{ YB}_{12} + 0.5 \text{ N}_2 + 13.5 \text{ H}_2 \rightarrow 11.5 \text{ YH}_2 + \text{YB}_6\text{H}_4\text{C}_6\text{N}$                          | -13.6519            |
| YNH <sub>4</sub> B <sub>6</sub> C <sub>6</sub> | $25.25 \text{ B}_9\text{H}_{11} + 6 \text{ Y}_2\text{C} + 12 \text{ H}_3\text{N} \rightarrow 44.25 \text{ B}_5\text{H}_7 + 11 \text{ YN} + \text{YB}_6\text{H}_4\text{C}_6\text{N}$ | -13.6472            |
| YNH <sub>4</sub> B <sub>6</sub> C <sub>6</sub> | $3 \text{ B}_{13}\text{C}_2 + 0.5 \text{ N}_2 + 2 \text{ H}_2 + 18.5 \text{ YB}_2 \rightarrow 17.5 \text{ YB}_4 + \text{YB}_6\text{H}_4\text{C}_6\text{N}$                          | -13.6396            |
| YNH <sub>4</sub> B <sub>6</sub> C <sub>6</sub> | $6 \text{ Y}_2\text{C} + 7.417 \text{ H}_3\text{N} + 1.5 \text{ YB}_4 \rightarrow 6.083 \text{ YH}_3 + 6.417 \text{ YN} + \text{YB}_6\text{H}_4\text{C}_6\text{N}$                  | -13.6187            |
| YNH <sub>4</sub> B <sub>6</sub> C <sub>6</sub> | $6 \text{ Y}_2\text{C} + 10 \text{ B}_5\text{H}_7 + 0.5 \text{ N}_2 \rightarrow 33 \text{ H}_2 + 11 \text{ YB}_4 + \text{YB}_6\text{H}_4\text{C}_6\text{N}$                         | -13.5149            |
| YNH <sub>4</sub> B <sub>6</sub> C <sub>6</sub> | $0.4615 \text{ B}_{13}\text{C}_2 + 5.077 \text{ Y}_2\text{C} + 0.5 \text{ N}_2 + 15.73 \text{ H}_2 \rightarrow 9.154 \text{ YH}_3 + \text{YB}_6\text{H}_4\text{C}_6\text{N}$        | -13.5018            |
| YNH <sub>4</sub> B <sub>6</sub> C <sub>6</sub> | $3.5 \text{ Y}_2\text{C} + 0.5 \text{ YB}_{12} + 0.5 \text{ H}_8\text{C}_5 + 3.75 \text{ N}_2 \rightarrow 6.5 \text{ YN} + \text{YB}_6\text{H}_4\text{C}_6\text{N}$                 | -13.2712            |
| YNH <sub>4</sub> B <sub>6</sub> C <sub>6</sub> | $1.871 \text{ B}_9\text{H}_{11} + 6 \text{ Y}_2\text{C} + 0.5 \text{ N}_2 \rightarrow 8.29 \text{ YH}_2 + 2.71 \text{ YB}_4 + \text{YB}_6\text{H}_4\text{C}_6\text{N}$              | -13.2216            |
| YNH <sub>4</sub> B <sub>6</sub> C <sub>6</sub> | $6 \text{ Y}_2\text{C} + 12 \text{ H}_3\text{N} + 6 \text{ B} \rightarrow 11 \text{ YN} + 16 \text{ H}_2 + \text{YB}_6\text{H}_4\text{C}_6\text{N}$                                 | -13.1937            |
| YNH <sub>4</sub> B <sub>6</sub> C <sub>6</sub> | $3 \text{ B}_{13}\text{C}_2 + 15.55 \text{ H}_3\text{N} + \text{YB}_{12} \rightarrow 6.091 \text{ B}_5\text{H}_7 + 14.55 \text{ BN} + \text{YB}_6\text{H}_4\text{C}_6\text{N}$      | -13.1810            |
| YNH <sub>4</sub> B <sub>6</sub> C <sub>6</sub> | $3.5 \text{ Y}_2\text{C} + 0.5 \text{ H}_8\text{C}_5 + 3.5 \text{ N}_2 + 6 \text{ B} \rightarrow 6 \text{ YN} + \text{YB}_6\text{H}_4\text{C}_6\text{N}$                            | -13.1553            |
| YNH <sub>4</sub> B <sub>6</sub> C <sub>6</sub> | $2.296 \text{ B}_9\text{H}_{11} + 6 \text{ Y}_2\text{C} + \text{BN} \rightarrow 7.085 \text{ YH}_3 + 3.915 \text{ YB}_4 + \text{YB}_6\text{H}_4\text{C}_6\text{N}$                  | -13.1459            |
| YNH <sub>4</sub> B <sub>6</sub> C <sub>6</sub> | $0.3636 \text{ B}_9\text{H}_{11} + 3 \text{ B}_{13}\text{C}_2 + \text{BN} + 20.64 \text{ YB}_2 \rightarrow 19.64 \text{ YB}_4 + \text{YB}_6\text{H}_4\text{C}_6\text{N}$            | -13.1089            |
| YNH <sub>4</sub> B <sub>6</sub> C <sub>6</sub> | $6 \text{ Y}_2\text{C} + 3.791 \text{ B}_5\text{H}_7 + \text{BN} \rightarrow 7.512 \text{ YH}_3 + 3.488 \text{ YB}_4 + \text{YB}_6\text{H}_4\text{C}_6\text{N}$                     | -13.1012            |
| YNH <sub>4</sub> B <sub>6</sub> C <sub>6</sub> | $6 \text{ Y}_2\text{C} + 3.053 \text{ B}_5\text{H}_7 + 0.5 \text{ N}_2 \rightarrow 8.684 \text{ YH}_2 + 2.316 \text{ YB}_4 + \text{YB}_6\text{H}_4\text{C}_6\text{N}$               | -13.0752            |
| YNH <sub>4</sub> B <sub>6</sub> C <sub>6</sub> | $1.2 \text{ H}_8\text{C}_5 + 5.867 \text{ B}_5\text{H}_7 + 24.33 \text{ YN} \rightarrow 23.33 \text{ YH}_2 + 23.33 \text{ BN} + \text{YB}_6\text{H}_4\text{C}_6\text{N}$            | -13.0738            |
| YNH <sub>4</sub> B <sub>6</sub> C <sub>6</sub> | $6 \text{ Y}_2\text{C} + 5.6 \text{ H}_3\text{N} + 6 \text{ B} \rightarrow 6.4 \text{ YH}_2 + 4.6 \text{ YN} + \text{YB}_6\text{H}_4\text{C}_6\text{N}$                             | -13.0158            |
| YNH <sub>4</sub> B <sub>6</sub> C <sub>6</sub> | $0.6667 \text{ B}_9\text{H}_{11} + 6 \text{ Y}_2\text{C} + 0.5 \text{ N}_2 + 9.333 \text{ H}_2 \rightarrow 11 \text{ YH}_2 + \text{YB}_6\text{H}_4\text{C}_6\text{N}$               | -13.0030            |
| YNH <sub>4</sub> B <sub>6</sub> C <sub>6</sub> | $1.333 \text{ YH}_3 + 3 \text{ B}_{13}\text{C}_2 + 8.167 \text{ Y} + \text{BN} \rightarrow 8.5 \text{ YB}_4 + \text{YB}_6\text{H}_4\text{C}_6\text{N}$                              | -12.9830            |
| YNH <sub>4</sub> B <sub>6</sub> C <sub>6</sub> | $6 \text{ Y}_2\text{C} + 1.2 \text{ B}_5\text{H}_7 + 0.5 \text{ N}_2 + 8.8 \text{ H}_2 \rightarrow 11 \text{ YH}_2 + \text{YB}_6\text{H}_4\text{C}_6\text{N}$                       | -12.9579            |
| YNH <sub>4</sub> B <sub>6</sub> C <sub>6</sub> | $3 \text{ B}_{13}\text{C}_2 + 0.5714 \text{ B}_5\text{H}_7 + \text{BN} + 20.43 \text{ YB}_2 \rightarrow 19.43 \text{ YB}_4 + \text{YB}_6\text{H}_4\text{C}_6\text{N}$               | -12.9090            |
| YNH <sub>4</sub> B <sub>6</sub> C <sub>6</sub> | $6 \text{ Y}_2\text{C} + \text{H}_3\text{N} + 11.5 \text{ H}_2 + 6 \text{ B} \rightarrow 11 \text{ YH}_2 + \text{YB}_6\text{H}_4\text{C}_6\text{N}$                                 | -12.8879            |
| YNH <sub>4</sub> B <sub>6</sub> C <sub>6</sub> | $6 \text{ Y}_2\text{C} + 0.5 \text{ N}_2 + 14.5 \text{ H}_2 + 1.5 \text{ YB}_4 \rightarrow 12.5 \text{ YH}_2 + \text{YB}_6\text{H}_4\text{C}_6\text{N}$                             | -12.8820            |
| YNH <sub>4</sub> B <sub>6</sub> C <sub>6</sub> | $3 \text{ B}_{13}\text{C}_2 + 1.333 \text{ H}_3\text{N} + 19.17 \text{ YB}_2 \rightarrow 0.3333 \text{ YN} + 17.83 \text{ YB}_4 + \text{YB}_6\text{H}_4\text{C}_6\text{N}$          | -12.8703            |
| YNH <sub>4</sub> B <sub>6</sub> C <sub>6</sub> | $6 \text{ Y}_2\text{C} + \text{YN} + 14 \text{ H}_2 + 6 \text{ B} \rightarrow 12 \text{ YH}_2 + \text{YB}_6\text{H}_4\text{C}_6\text{N}$                                            | -12.8601            |
| YNH <sub>4</sub> B <sub>6</sub> C <sub>6</sub> | $6 \text{ Y}_2\text{C} + \text{H}_3\text{N} + 4.303 \text{ B}_5\text{H}_7 \rightarrow 9.707 \text{ YH}_3 + 1.293 \text{ YB}_{12} + \text{YB}_6\text{H}_4\text{C}_6\text{N}$         | -12.8430            |
| YNH <sub>4</sub> B <sub>6</sub> C <sub>6</sub> | $0.8723 \text{ B}_{13}\text{C}_2 + 4.255 \text{ Y}_2\text{C} + 6.34 \text{ H}_3\text{N} \rightarrow 7.511 \text{ YH}_2 + 5.34 \text{ BN} + \text{YB}_6\text{H}_4\text{C}_6\text{N}$ | -12.8284            |
| YNH <sub>4</sub> B <sub>6</sub> C <sub>6</sub> | $6 \text{ Y}_2\text{C} + 34.75 \text{ B}_5\text{H}_7 + \text{BN} \rightarrow 11 \text{ YH}_3 + 18.75 \text{ B}_9\text{H}_{11} + \text{YB}_6\text{H}_4\text{C}_6\text{N}$            | -12.7360            |
| YNH <sub>4</sub> B <sub>6</sub> C <sub>6</sub> | $0.09091 \text{ B}_9\text{H}_{11} + 3 \text{ B}_{13}\text{C}_2 + \text{H}_3\text{N} + 18.91 \text{ YB}_2 \rightarrow 17.91 \text{ YB}_4 + \text{YB}_6\text{H}_4\text{C}_6\text{N}$  | -12.6668            |
| YNH <sub>4</sub> B <sub>6</sub> C <sub>6</sub> | $2.679 \text{ B}_9\text{H}_{11} + 6 \text{ Y}_2\text{C} + \text{H}_3\text{N} \rightarrow 9.491 \text{ YH}_3 + 1.509 \text{ YB}_{12} + \text{YB}_6\text{H}_4\text{C}_6\text{N}$      | -12.6566            |
| YNH <sub>4</sub> B <sub>6</sub> C <sub>6</sub> | $6 \text{ Y}_2\text{C} + 12.5 \text{ H}_3\text{N} + 0.5 \text{ YB}_{12} \rightarrow 11.5 \text{ YN} + 16.75 \text{ H}_2 + \text{YB}_6\text{H}_4\text{C}_6\text{N}$                  | -12.6476            |
| YNH <sub>4</sub> B <sub>6</sub> C <sub>6</sub> | $6 \text{ B}_9\text{H}_{11} + 6 \text{ Y}_2\text{C} + \text{YN} \rightarrow 31 \text{ H}_2 + 12 \text{ YB}_4 + \text{YB}_6\text{H}_4\text{C}_6\text{N}$                             | -12.6194            |
| YNH <sub>4</sub> B <sub>6</sub> C <sub>6</sub> | $3 \text{ B}_{13}\text{C}_2 + \text{H}_3\text{N} + 0.1429 \text{ B}_5\text{H}_7 + 18.86 \text{ YB}_2 \rightarrow 17.86 \text{ YB}_4 + \text{YB}_6\text{H}_4\text{C}_6\text{N}$      | -12.6168            |
| YNH <sub>4</sub> B <sub>6</sub> C <sub>6</sub> | $6 \text{ Y}_2\text{C} + 5.03 \text{ B}_5\text{H}_7 + \text{YN} \rightarrow 10.4 \text{ YH}_3 + 1.596 \text{ YB}_{12} + \text{YB}_6\text{H}_4\text{C}_6\text{N}$                    | -12.6102            |
| YNH <sub>4</sub> B <sub>6</sub> C <sub>6</sub> | $6 \text{ Y}_2\text{C} + 15.5 \text{ H}_2 + \text{BN} + 2.5 \text{ YB}_2 \rightarrow 13.5 \text{ YH}_2 + \text{YB}_6\text{H}_4\text{C}_6\text{N}$                                   | -12.5828            |
| YNH <sub>4</sub> B <sub>6</sub> C <sub>6</sub> | $5.556 \text{ B}_9\text{H}_{11} + 6 \text{ Y}_2\text{C} + \text{H}_3\text{N} \rightarrow 30.06 \text{ H}_2 + 11 \text{ YB}_4 + \text{YB}_6\text{H}_4\text{C}_6\text{N}$             | -12.5665            |
| YNH <sub>4</sub> B <sub>6</sub> C <sub>6</sub> | $1.2 \text{ Y}_4\text{C}_5 + 2.2 \text{ B}_5\text{H}_7 + 3 \text{ N}_2 \rightarrow 3.8 \text{ YH}_3 + 5 \text{ BN} + \text{YB}_6\text{H}_4\text{C}_6\text{N}$                       | -12.5433            |
| YNH <sub>4</sub> B <sub>6</sub> C <sub>6</sub> | $1.333 \text{ YH}_3 + 1.2 \text{ Y}_4\text{C}_5 + 4.567 \text{ N}_2 + 3 \text{ YB}_2 \rightarrow 8.133 \text{ YN} + \text{YB}_6\text{H}_4\text{C}_6\text{N}$                        | -12.5405            |
| YNH <sub>4</sub> B <sub>6</sub> C <sub>6</sub> | $3 \text{ B}_{13}\text{C}_2 + 1.333 \text{ H}_3\text{N} + 18.33 \text{ YB}_2 \rightarrow 0.3333 \text{ BN} + 17.33 \text{ YB}_4 + \text{YB}_6\text{H}_4\text{C}_6\text{N}$          | -12.5194            |
| YNH <sub>4</sub> B <sub>6</sub> C <sub>6</sub> | $6 \text{ Y}_2\text{C} + 5.8 \text{ H}_3\text{N} + 0.5 \text{ YB}_{12} \rightarrow 6.7 \text{ YH}_2 + 4.8 \text{ YN} + \text{YB}_6\text{H}_4\text{C}_6\text{N}$                     | -12.4613            |
| YNH <sub>4</sub> B <sub>6</sub> C <sub>6</sub> | $0.4615 \text{ B}_{13}\text{C}_2 + 5.077 \text{ Y}_2\text{C} + \text{YN} + 17.23 \text{ H}_2 \rightarrow 10.15 \text{ YH}_3 + \text{YB}_6\text{H}_4\text{C}_6\text{N}$              | -12.4594            |
| YNH <sub>4</sub> B <sub>6</sub> C <sub>6</sub> | $1.2 \text{ H}_8\text{C}_5 + 5.1 \text{ N}_2 + 3.8 \text{ YB}_4 \rightarrow 2.8 \text{ YH}_2 + 9.2 \text{ BN} + \text{YB}_6\text{H}_4\text{C}_6\text{N}$                            | -12.4540            |
| YNH <sub>4</sub> B <sub>6</sub> C <sub>6</sub> | $3.132 \text{ B}_9\text{H}_{11} + 6 \text{ Y}_2\text{C} + \text{YN} \rightarrow 10.15 \text{ YH}_3 + 1.849 \text{ YB}_{12} + \text{YB}_6\text{H}_4\text{C}_6\text{N}$               | -12.3924            |
| YNH <sub>4</sub> B <sub>6</sub> C <sub>6</sub> | $6 \text{ Y}_2\text{C} + \text{H}_3\text{N} + 0.5 \text{ YB}_{12} + 12 \text{ H}_2 \rightarrow 11.5 \text{ YH}_2 + \text{YB}_6\text{H}_4\text{C}_6\text{N}$                         | -12.3279            |
| YNH <sub>4</sub> B <sub>6</sub> C <sub>6</sub> | $3 \text{ B}_{13}\text{C}_2 + \text{H}_3\text{N} + 0.5 \text{ H}_2 + 18.5 \text{ YB}_2 \rightarrow 17.5 \text{ YB}_4 + \text{YB}_6\text{H}_4\text{C}_6\text{N}$                     | -12.3155            |
| YNH <sub>4</sub> B <sub>6</sub> C <sub>6</sub> | $6 \text{ Y}_2\text{C} + 0.5 \text{ YB}_{12} + \text{YN} + 14.5 \text{ H}_2 \rightarrow 12.5 \text{ YH}_2 + \text{YB}_6\text{H}_4\text{C}_6\text{N}$                                | -12.3001            |
| YNH <sub>4</sub> B <sub>6</sub> C <sub>6</sub> | $6 \text{ Y}_2\text{C} + 21 \text{ B}_5\text{H}_7 + 0.5 \text{ N}_2 \rightarrow 11 \text{ B}_9\text{H}_{11} + 11 \text{ YH}_2 + \text{YB}_6\text{H}_4\text{C}_6\text{N}$            | -12.2141            |
| YNH <sub>4</sub> B <sub>6</sub> C <sub>6</sub> | $6 \text{ Y}_2\text{C} + 10.8 \text{ B}_5\text{H}_7 + \text{YN} \rightarrow 35.8 \text{ H}_2 + 12 \text{ YB}_4 + \text{YB}_6\text{H}_4\text{C}_6\text{N}$                           | -12.2137            |

Continued on next page

Continued

| Compound                                       | Chemical reaction                                                                                                                                                                           | Reaction energy(eV) |
|------------------------------------------------|---------------------------------------------------------------------------------------------------------------------------------------------------------------------------------------------|---------------------|
| YNH <sub>4</sub> B <sub>6</sub> C <sub>6</sub> | $6 \text{ Y}_2\text{C} + \text{H}_3\text{N} + 10 \text{ B}_5\text{H}_7 \rightarrow 34.5 \text{ H}_2 + 11 \text{ YB}_4 + \text{YB}_6\text{H}_4\text{C}_6\text{N}$                            | -12.1908            |
| YNH <sub>4</sub> B <sub>6</sub> C <sub>6</sub> | $0.4615 \text{ B}_{13}\text{C}_2 + 5.077 \text{ Y}_2\text{C} + \text{H}_3\text{N} + 14.23 \text{ H}_2 \rightarrow 9.154 \text{ YH}_3 + \text{YB}_6\text{H}_4\text{C}_6\text{N}$             | -12.1777            |
| YNH <sub>4</sub> B <sub>6</sub> C <sub>6</sub> | $6 \text{ Y}_2\text{C} + 5.286 \text{ B}_5\text{H}_7 + 0.5 \text{ N}_2 \rightarrow 11 \text{ YH}_3 + 20.43 \text{ B} + \text{YB}_6\text{H}_4\text{C}_6\text{N}$                             | -12.0921            |
| YNH <sub>4</sub> B <sub>6</sub> C <sub>6</sub> | $0.3636 \text{ B}_9\text{H}_{11} + 3 \text{ B}_{13}\text{C}_2 + \text{YN} + 18.14 \text{ YB}_2 \rightarrow 18.14 \text{ YB}_4 + \text{YB}_6\text{H}_4\text{C}_6\text{N}$                    | -12.0561            |
| YNH <sub>4</sub> B <sub>6</sub> C <sub>6</sub> | $2 \text{ YH}_2 + 3 \text{ B}_{13}\text{C}_2 + 7.5 \text{ Y} + \text{BN} \rightarrow 8.5 \text{ YB}_4 + \text{YB}_6\text{H}_4\text{C}_6\text{N}$                                            | -11.9882            |
| YNH <sub>4</sub> B <sub>6</sub> C <sub>6</sub> | $0.6667 \text{ B}_9\text{H}_{11} + 6 \text{ Y}_2\text{C} + 12 \text{ H}_3\text{N} \rightarrow 11 \text{ YN} + 19.67 \text{ H}_2 + \text{YB}_6\text{H}_4\text{C}_6\text{N}$                  | -11.9847            |
| YNH <sub>4</sub> B <sub>6</sub> C <sub>6</sub> | $6 \text{ Y}_2\text{C} + 12 \text{ H}_3\text{N} + 1.2 \text{ B}_5\text{H}_7 \rightarrow 11 \text{ YN} + 20.2 \text{ H}_2 + \text{YB}_6\text{H}_4\text{C}_6\text{N}$                         | -11.9396            |
| YNH <sub>4</sub> B <sub>6</sub> C <sub>6</sub> | $6 \text{ Y}_2\text{C} + 1.333 \text{ H}_3\text{N} + 2.333 \text{ N}_2 + 6 \text{ BN} \rightarrow 11 \text{ YN} + \text{YB}_6\text{H}_4\text{C}_6\text{N}$                                  | -11.9165            |
| YNH <sub>4</sub> B <sub>6</sub> C <sub>6</sub> | $6 \text{ Y}_2\text{C} + 13.5 \text{ H}_3\text{N} + 1.5 \text{ YB}_4 \rightarrow 12.5 \text{ YN} + 18.25 \text{ H}_2 + \text{YB}_6\text{H}_4\text{C}_6\text{N}$                             | -11.9054            |
| YNH <sub>4</sub> B <sub>6</sub> C <sub>6</sub> | $2 \text{ B}_9\text{H}_{11} + 6 \text{ Y}_2\text{C} + \text{YN} \rightarrow 9 \text{ YH}_2 + 3 \text{ YB}_4 + \text{YB}_6\text{H}_4\text{C}_6\text{N}$                                      | -11.8932            |
| YNH <sub>4</sub> B <sub>6</sub> C <sub>6</sub> | $14.78 \text{ YH}_3 + 3 \text{ B}_{13}\text{C}_2 + 7.389 \text{ N}_2 \rightarrow 3.667 \text{ B}_9\text{H}_{11} + 13.78 \text{ YN} + \text{YB}_6\text{H}_4\text{C}_6\text{N}$               | -11.8866            |
| YNH <sub>4</sub> B <sub>6</sub> C <sub>6</sub> | $3 \text{ B}_{13}\text{C}_2 + 1.333 \text{ H}_3\text{N} + 18.5 \text{ YB}_2 \rightarrow 0.1667 \text{ N}_2 + 17.5 \text{ YB}_4 + \text{YB}_6\text{H}_4\text{C}_6\text{N}$                   | -11.8741            |
| YNH <sub>4</sub> B <sub>6</sub> C <sub>6</sub> | $1.677 \text{ B}_9\text{H}_{11} + 6 \text{ Y}_2\text{C} + \text{H}_3\text{N} \rightarrow 8.726 \text{ YH}_2 + 2.274 \text{ YB}_4 + \text{YB}_6\text{H}_4\text{C}_6\text{N}$                 | -11.8624            |
| YNH <sub>4</sub> B <sub>6</sub> C <sub>6</sub> | $3 \text{ B}_{13}\text{C}_2 + 0.5714 \text{ B}_5\text{H}_7 + \text{YN} + 17.93 \text{ YB}_2 \rightarrow 17.93 \text{ YB}_4 + \text{YB}_6\text{H}_4\text{C}_6\text{N}$                       | -11.8562            |
| YNH <sub>4</sub> B <sub>6</sub> C <sub>6</sub> | $0.6667 \text{ B}_9\text{H}_{11} + 6 \text{ Y}_2\text{C} + 4.133 \text{ H}_3\text{N} \rightarrow 7.867 \text{ YH}_2 + 3.133 \text{ YN} + \text{YB}_6\text{H}_4\text{C}_6\text{N}$           | -11.7660            |
| YNH <sub>4</sub> B <sub>6</sub> C <sub>6</sub> | $3.5 \text{ Y}_2\text{C} + 0.5 \text{ H}_8\text{C}_5 + 0.5 \text{ N}_2 + 78 \text{ B} \rightarrow 6 \text{ YB}_{12} + \text{YB}_6\text{H}_4\text{C}_6\text{N}$                              | -11.7643            |
| YNH <sub>4</sub> B <sub>6</sub> C <sub>6</sub> | $6 \text{ Y}_2\text{C} + 3.263 \text{ B}_5\text{H}_7 + \text{YN} \rightarrow 9.421 \text{ YH}_2 + 2.579 \text{ YB}_4 + \text{YB}_6\text{H}_4\text{C}_6\text{N}$                             | -11.7366            |
| YNH <sub>4</sub> B <sub>6</sub> C <sub>6</sub> | $6 \text{ Y}_2\text{C} + \text{H}_3\text{N} + 2.737 \text{ B}_5\text{H}_7 \rightarrow 9.079 \text{ YH}_2 + 1.921 \text{ YB}_4 + \text{YB}_6\text{H}_4\text{C}_6\text{N}$                    | -11.7311            |
| YNH <sub>4</sub> B <sub>6</sub> C <sub>6</sub> | $6 \text{ Y}_2\text{C} + 3.92 \text{ H}_3\text{N} + 1.2 \text{ B}_5\text{H}_7 \rightarrow 8.08 \text{ YH}_2 + 2.92 \text{ YN} + \text{YB}_6\text{H}_4\text{C}_6\text{N}$                    | -11.7150            |
| YNH <sub>4</sub> B <sub>6</sub> C <sub>6</sub> | $3 \text{ B}_{13}\text{C}_2 + 2 \text{ H}_2 + \text{BN} + 19 \text{ YB}_2 \rightarrow 18 \text{ YB}_4 + \text{YB}_6\text{H}_4\text{C}_6\text{N}$                                            | -11.7037            |
| YNH <sub>4</sub> B <sub>6</sub> C <sub>6</sub> | $6 \text{ Y}_2\text{C} + 6.2 \text{ H}_3\text{N} + 1.5 \text{ YB}_4 \rightarrow 7.3 \text{ YH}_2 + 5.2 \text{ YN} + \text{YB}_6\text{H}_4\text{C}_6\text{N}$                                | -11.7024            |
| YNH <sub>4</sub> B <sub>6</sub> C <sub>6</sub> | $0.6667 \text{ B}_9\text{H}_{11} + 6 \text{ Y}_2\text{C} + \text{H}_3\text{N} + 7.833 \text{ H}_2 \rightarrow 11 \text{ YH}_2 + \text{YB}_6\text{H}_4\text{C}_6\text{N}$                    | -11.6789            |
| YNH <sub>4</sub> B <sub>6</sub> C <sub>6</sub> | $0.3333 \text{ YH}_3 + 3 \text{ B}_{13}\text{C}_2 + \text{H}_3\text{N} + 17.83 \text{ YB}_2 \rightarrow 17.17 \text{ YB}_4 + \text{YB}_6\text{H}_4\text{C}_6\text{N}$                       | -11.6668            |
| YNH <sub>4</sub> B <sub>6</sub> C <sub>6</sub> | $6 \text{ Y}_2\text{C} + 3.447 \text{ B}_5\text{H}_7 + 0.5 \text{ N}_2 \rightarrow 10.06 \text{ YH}_2 + 0.9362 \text{ YB}_{12} + \text{YB}_6\text{H}_4\text{C}_6\text{N}$                   | -11.6585            |
| YNH <sub>4</sub> B <sub>6</sub> C <sub>6</sub> | $0.6667 \text{ B}_9\text{H}_{11} + 6 \text{ Y}_2\text{C} + \text{YN} + 10.33 \text{ H}_2 \rightarrow 12 \text{ YH}_2 + \text{YB}_6\text{H}_4\text{C}_6\text{N}$                             | -11.6511            |
| YNH <sub>4</sub> B <sub>6</sub> C <sub>6</sub> | $6 \text{ Y}_2\text{C} + 13 \text{ H}_2 + \text{BN} + 5 \text{ B} \rightarrow 11 \text{ YH}_2 + \text{YB}_6\text{H}_4\text{C}_6\text{N}$                                                    | -11.6452            |
| YNH <sub>4</sub> B <sub>6</sub> C <sub>6</sub> | $1.75 \text{ Y}_4\text{C}_5 + 1.2 \text{ B}_5\text{H}_7 + 3.5 \text{ N}_2 \rightarrow 0.55 \text{ H}_8\text{C}_5 + 6 \text{ YN} + \text{YB}_6\text{H}_4\text{C}_6\text{N}$                  | -11.6424            |
| YNH <sub>4</sub> B <sub>6</sub> C <sub>6</sub> | $3.905 \text{ B}_9\text{H}_{11} + 6.992 \text{ N}_2 + 0.8571 \text{ Y}_4\text{C}_7 \rightarrow 12.98 \text{ H}_3\text{N} + 2.429 \text{ YB}_{12} + \text{YB}_6\text{H}_4\text{C}_6\text{N}$ | -11.6354            |
| YNH <sub>4</sub> B <sub>6</sub> C <sub>6</sub> | $6 \text{ Y}_2\text{C} + \text{H}_3\text{N} + 1.2 \text{ B}_5\text{H}_7 + 7.3 \text{ H}_2 \rightarrow 11 \text{ YH}_2 + \text{YB}_6\text{H}_4\text{C}_6\text{N}$                            | -11.6338            |
| YNH <sub>4</sub> B <sub>6</sub> C <sub>6</sub> | $0.3846 \text{ B}_{13}\text{C}_2 + 5.231 \text{ Y}_2\text{C} + 16.19 \text{ H}_2 + \text{BN} \rightarrow 9.462 \text{ YH}_3 + \text{YB}_6\text{H}_4\text{C}_6\text{N}$                      | -11.6207            |
| YNH <sub>4</sub> B <sub>6</sub> C <sub>6</sub> | $3 \text{ B}_{13}\text{C}_2 + 14.26 \text{ H}_3\text{N} + \text{YB}_{12} \rightarrow 3.526 \text{ B}_9\text{H}_{11} + 13.26 \text{ BN} + \text{YB}_6\text{H}_4\text{C}_6\text{N}$           | -11.6170            |
| YNH <sub>4</sub> B <sub>6</sub> C <sub>6</sub> | $6 \text{ Y}_2\text{C} + 1.2 \text{ B}_5\text{H}_7 + \text{YN} + 9.8 \text{ H}_2 \rightarrow 12 \text{ YH}_2 + \text{YB}_6\text{H}_4\text{C}_6\text{N}$                                     | -11.6060            |
| YNH <sub>4</sub> B <sub>6</sub> C <sub>6</sub> | $6 \text{ Y}_2\text{C} + 27.54 \text{ H}_3\text{N} + 15.54 \text{ YB}_4 \rightarrow 11.23 \text{ B}_5\text{H}_7 + 26.54 \text{ YN} + \text{YB}_6\text{H}_4\text{C}_6\text{N}$               | -11.5848            |
| YNH <sub>4</sub> B <sub>6</sub> C <sub>6</sub> | $6 \text{ Y}_2\text{C} + \text{H}_3\text{N} + 13 \text{ H}_2 + 1.5 \text{ YB}_4 \rightarrow 12.5 \text{ YH}_2 + \text{YB}_6\text{H}_4\text{C}_6\text{N}$                                    | -11.5579            |
| YNH <sub>4</sub> B <sub>6</sub> C <sub>6</sub> | $2.16 \text{ B}_9\text{H}_{11} + 6 \text{ Y}_2\text{C} + 0.5 \text{ N}_2 \rightarrow 9.88 \text{ YH}_2 + 1.12 \text{ YB}_{12} + \text{YB}_6\text{H}_4\text{C}_6\text{N}$                    | -11.5494            |
| YNH <sub>4</sub> B <sub>6</sub> C <sub>6</sub> | $3.5 \text{ Y}_2\text{C} + 0.5 \text{ H}_8\text{C}_5 + \text{YN} + 90 \text{ B} \rightarrow 7 \text{ YB}_{12} + \text{YB}_6\text{H}_4\text{C}_6\text{N}$                                    | -11.5325            |
| YNH <sub>4</sub> B <sub>6</sub> C <sub>6</sub> | $6 \text{ Y}_2\text{C} + \text{YN} + 15.5 \text{ H}_2 + 1.5 \text{ YB}_4 \rightarrow 13.5 \text{ YH}_2 + \text{YB}_6\text{H}_4\text{C}_6\text{N}$                                           | -11.5301            |
| YNH <sub>4</sub> B <sub>6</sub> C <sub>6</sub> | $5.444 \text{ B}_9\text{H}_{11} + 6 \text{ Y}_2\text{C} + \text{BN} \rightarrow 27.94 \text{ H}_2 + 11 \text{ YB}_4 + \text{YB}_6\text{H}_4\text{C}_6\text{N}$                              | -11.5253            |
| YNH <sub>4</sub> B <sub>6</sub> C <sub>6</sub> | $3.364 \text{ B}_9\text{H}_{11} + 6 \text{ Y}_2\text{C} + 0.5 \text{ N}_2 \rightarrow 11 \text{ YH}_3 + 24.27 \text{ B} + \text{YB}_6\text{H}_4\text{C}_6\text{N}$                          | -11.5161            |
| YNH <sub>4</sub> B <sub>6</sub> C <sub>6</sub> | $0.5 \text{ YH}_2 + 3 \text{ B}_{13}\text{C}_2 + \text{H}_3\text{N} + 17.5 \text{ YB}_2 \rightarrow 17 \text{ YB}_4 + \text{YB}_6\text{H}_4\text{C}_6\text{N}$                              | -11.4971            |
| YNH <sub>4</sub> B <sub>6</sub> C <sub>6</sub> | $6 \text{ Y}_2\text{C} + 4.636 \text{ B}_5\text{H}_7 + \text{BN} \rightarrow 9.485 \text{ YH}_3 + 1.515 \text{ YB}_{12} + \text{YB}_6\text{H}_4\text{C}_6\text{N}$                          | -11.4321            |
| YNH <sub>4</sub> B <sub>6</sub> C <sub>6</sub> | $1.333 \text{ YH}_3 + 3 \text{ B}_{13}\text{C}_2 + 6.917 \text{ Y} + \text{YN} \rightarrow 8.25 \text{ YB}_4 + \text{YB}_6\text{H}_4\text{C}_6\text{N}$                                     | -11.3373            |
| YNH <sub>4</sub> B <sub>6</sub> C <sub>6</sub> | $2.887 \text{ B}_9\text{H}_{11} + 6 \text{ Y}_2\text{C} + \text{BN} \rightarrow 9.252 \text{ YH}_3 + 1.748 \text{ YB}_{12} + \text{YB}_6\text{H}_4\text{C}_6\text{N}$                       | -11.2313            |
| YNH <sub>4</sub> B <sub>6</sub> C <sub>6</sub> | $6 \text{ Y}_2\text{C} + \text{H}_3\text{N} + 4.857 \text{ B}_5\text{H}_7 \rightarrow 11 \text{ YH}_3 + 18.29 \text{ B} + \text{YB}_6\text{H}_4\text{C}_6\text{N}$                          | -11.2159            |
| YNH <sub>4</sub> B <sub>6</sub> C <sub>6</sub> | $6 \text{ Y}_2\text{C} + 0.4167 \text{ YB}_{12} + 13.42 \text{ H}_2 + \text{BN} \rightarrow 11.42 \text{ YH}_2 + \text{YB}_6\text{H}_4\text{C}_6\text{N}$                                   | -11.1785            |
| YNH <sub>4</sub> B <sub>6</sub> C <sub>6</sub> | $6 \text{ Y}_2\text{C} + 9.8 \text{ B}_5\text{H}_7 + \text{BN} \rightarrow 32.3 \text{ H}_2 + 11 \text{ YB}_4 + \text{YB}_6\text{H}_4\text{C}_6\text{N}$                                    | -11.1572            |
| YNH <sub>4</sub> B <sub>6</sub> C <sub>6</sub> | $1.2 \text{ Y}_4\text{C}_5 + 4.24 \text{ B}_5\text{H}_7 + 4.78 \text{ N}_2 \rightarrow 8.56 \text{ H}_3\text{N} + 3.8 \text{ YB}_4 + \text{YB}_6\text{H}_4\text{C}_6\text{N}$               | -11.1506            |
| YNH <sub>4</sub> B <sub>6</sub> C <sub>6</sub> | $8.3 \text{ H}_3\text{N} + 1.2 \text{ Y}_4\text{C}_5 + 6.65 \text{ YB}_2 \rightarrow 10.45 \text{ YH}_2 + 7.3 \text{ BN} + \text{YB}_6\text{H}_4\text{C}_6\text{N}$                         | -11.1051            |
| YNH <sub>4</sub> B <sub>6</sub> C <sub>6</sub> | $1.333 \text{ YH}_3 + 3 \text{ B}_{13}\text{C}_2 + 0.5 \text{ N}_2 + 15.83 \text{ YB}_2 \rightarrow 16.17 \text{ YB}_4 + \text{YB}_6\text{H}_4\text{C}_6\text{N}$                           | -11.0744            |
| YNH <sub>4</sub> B <sub>6</sub> C <sub>6</sub> | $6 \text{ Y}_2\text{C} + \text{H}_3\text{N} + 17.62 \text{ B}_5\text{H}_7 \rightarrow 9.125 \text{ B}_9\text{H}_{11} + 11 \text{ YH}_2 + \text{YB}_6\text{H}_4\text{C}_6\text{N}$           | -11.0446            |
| YNH <sub>4</sub> B <sub>6</sub> C <sub>6</sub> | $6 \text{ Y}_2\text{C} + 3.172 \text{ B}_5\text{H}_7 + 0.5 \text{ N}_2 \rightarrow 6.069 \text{ YH}_3 + 4.931 \text{ YB}_2 + \text{YB}_6\text{H}_4\text{C}_6\text{N}$                       | -11.0168            |
| YNH <sub>4</sub> B <sub>6</sub> C <sub>6</sub> | $6 \text{ Y}_2\text{C} + 32.82 \text{ H}_3\text{N} + 20.82 \text{ YB}_4 \rightarrow 8.588 \text{ B}_9\text{H}_{11} + 31.82 \text{ YN} + \text{YB}_6\text{H}_4\text{C}_6\text{N}$            | -10.9252            |
| YNH <sub>4</sub> B <sub>6</sub> C <sub>6</sub> | $1.839 \text{ B}_9\text{H}_{11} + 6 \text{ Y}_2\text{C} + \text{BN} \rightarrow 8.113 \text{ YH}_2 + 2.887 \text{ YB}_4 + \text{YB}_6\text{H}_4\text{C}_6\text{N}$                          | -10.8833            |
| YNH <sub>4</sub> B <sub>6</sub> C <sub>6</sub> | $0.4615 \text{ B}_{13}\text{C}_2 + 5.077 \text{ Y}_2\text{C} + 5.744 \text{ H}_3\text{N} \rightarrow 4.41 \text{ YH}_3 + 4.744 \text{ YN} + \text{YB}_6\text{H}_4\text{C}_6\text{N}$        | -10.8707            |
| YNH <sub>4</sub> B <sub>6</sub> C <sub>6</sub> | $6 \text{ Y}_2\text{C} + 23.25 \text{ B}_5\text{H}_7 + \text{YN} \rightarrow 12.25 \text{ B}_9\text{H}_{11} + 12 \text{ YH}_2 + \text{YB}_6\text{H}_4\text{C}_6\text{N}$                    | -10.8418            |
| YNH <sub>4</sub> B <sub>6</sub> C <sub>6</sub> | $6 \text{ Y}_2\text{C} + 3 \text{ B}_5\text{H}_7 + \text{BN} \rightarrow 8.5 \text{ YH}_2 + 2.5 \text{ YB}_4 + \text{YB}_6\text{H}_4\text{C}_6\text{N}$                                     | -10.7777            |
| YNH <sub>4</sub> B <sub>6</sub> C <sub>6</sub> | $3.091 \text{ B}_9\text{H}_{11} + 6 \text{ Y}_2\text{C} + \text{H}_3\text{N} \rightarrow 11 \text{ YH}_3 + 21.82 \text{ B} + \text{YB}_6\text{H}_4\text{C}_6\text{N}$                       | -10.7267            |
| YNH <sub>4</sub> B <sub>6</sub> C <sub>6</sub> | $0.4615 \text{ B}_{13}\text{C}_2 + 5.077 \text{ Y}_2\text{C} + 0.5 \text{ N}_2 + 11.15 \text{ H}_2 \rightarrow 9.154 \text{ YH}_2 + \text{YB}_6\text{H}_4\text{C}_6\text{N}$                | -10.6866            |
| YNH <sub>4</sub> B <sub>6</sub> C <sub>6</sub> | $3 \text{ B}_{13}\text{C}_2 + \text{YN} + 2 \text{ H}_2 + 16.5 \text{ YB}_2 \rightarrow 16.5 \text{ YB}_4 + \text{YB}_6\text{H}_4\text{C}_6\text{N}$                                        | -10.6693            |
| YNH <sub>4</sub> B <sub>6</sub> C <sub>6</sub> |                                                                                                                                                                                             | -10.6509            |

Continued on next page

Continued

| Compound                                       | Chemical reaction                                                                                                                                                                                      | Reaction energy(eV) |
|------------------------------------------------|--------------------------------------------------------------------------------------------------------------------------------------------------------------------------------------------------------|---------------------|
| YNH <sub>4</sub> B <sub>6</sub> C <sub>6</sub> | 0.5556 B <sub>9</sub> H <sub>11</sub> + 6 Y <sub>2</sub> C + 9.944 H <sub>2</sub> + BN → 11 YH <sub>2</sub> + YB <sub>6</sub> H <sub>4</sub> C <sub>6</sub> N                                          | -10.6377            |
| YNH <sub>4</sub> B <sub>6</sub> C <sub>6</sub> | 6 Y <sub>2</sub> C + 5.714 B <sub>5</sub> H <sub>7</sub> + YN → 12 YH <sub>3</sub> + 22.57 B + YB <sub>6</sub> H <sub>4</sub> C <sub>6</sub> N                                                         | -10.6018            |
| YNH <sub>4</sub> B <sub>6</sub> C <sub>6</sub> | 6 Y <sub>2</sub> C + B <sub>5</sub> H <sub>7</sub> + 9.5 H <sub>2</sub> + BN → 11 YH <sub>2</sub> + YB <sub>6</sub> H <sub>4</sub> C <sub>6</sub> N                                                    | -10.6002            |
| YNH <sub>4</sub> B <sub>6</sub> C <sub>6</sub> | 6 Y <sub>2</sub> C + H <sub>3</sub> N + 3.064 B <sub>5</sub> H <sub>7</sub> → 10.22 YH <sub>2</sub> + 0.7766 YB <sub>12</sub> + YB <sub>6</sub> H <sub>4</sub> C <sub>6</sub> N                        | -10.5559            |
| YNH <sub>4</sub> B <sub>6</sub> C <sub>6</sub> | 6 Y <sub>2</sub> C + 14.25 H <sub>2</sub> + BN + 1.25 YB <sub>4</sub> → 12.25 YH <sub>2</sub> + YB <sub>6</sub> H <sub>4</sub> C <sub>6</sub> N                                                        | -10.5369            |
| YNH <sub>4</sub> B <sub>6</sub> C <sub>6</sub> | 1.878 B <sub>9</sub> H <sub>11</sub> + 6 Y <sub>2</sub> C + 0.5 N <sub>2</sub> → 5.551 YH <sub>3</sub> + 5.449 YB <sub>2</sub> + YB <sub>6</sub> H <sub>4</sub> C <sub>6</sub> N                       | -10.4812            |
| YNH <sub>4</sub> B <sub>6</sub> C <sub>6</sub> | 1.92 B <sub>9</sub> H <sub>11</sub> + 6 Y <sub>2</sub> C + H <sub>3</sub> N → 10.06 YH <sub>2</sub> + 0.94 YB <sub>12</sub> + YB <sub>6</sub> H <sub>4</sub> C <sub>6</sub> N                          | -10.4589            |
| YNH <sub>4</sub> B <sub>6</sub> C <sub>6</sub> | 2 YH <sub>2</sub> + 3 B <sub>13</sub> C <sub>2</sub> + 0.5 N <sub>2</sub> + 14.5 YB <sub>2</sub> → 15.5 YB <sub>4</sub> + YB <sub>6</sub> H <sub>4</sub> C <sub>6</sub> N                              | -10.3660            |
| YNH <sub>4</sub> B <sub>6</sub> C <sub>6</sub> | 3.5 Y <sub>2</sub> C + 0.5 H <sub>8</sub> C <sub>5</sub> + 0.5 N <sub>2</sub> + 30 B → 6 YB <sub>4</sub> + YB <sub>6</sub> H <sub>4</sub> C <sub>6</sub> N                                             | -10.3640            |
| YNH <sub>4</sub> B <sub>6</sub> C <sub>6</sub> | 2 YH <sub>2</sub> + 3 B <sub>13</sub> C <sub>2</sub> + 6.25 Y + YN → 8.25 YB <sub>4</sub> + YB <sub>6</sub> H <sub>4</sub> C <sub>6</sub> N                                                            | -10.3424            |
| YNH <sub>4</sub> B <sub>6</sub> C <sub>6</sub> | 6 Y <sub>2</sub> C + 3.714 B <sub>5</sub> H <sub>7</sub> + 0.5 N <sub>2</sub> → 11 YH <sub>2</sub> + 12.57 B + YB <sub>6</sub> H <sub>4</sub> C <sub>6</sub> N                                         | -10.3304            |
| YNH <sub>4</sub> B <sub>6</sub> C <sub>6</sub> | 6 Y <sub>2</sub> C + H <sub>3</sub> N + 2.966 B <sub>5</sub> H <sub>7</sub> → 6.586 YH <sub>3</sub> + 4.414 YB <sub>2</sub> + YB <sub>6</sub> H <sub>4</sub> C <sub>6</sub> N                          | -10.1714            |
| YNH <sub>4</sub> B <sub>6</sub> C <sub>6</sub> | 6 Y <sub>2</sub> C + 3.702 B <sub>5</sub> H <sub>7</sub> + YN → 10.96 YH <sub>2</sub> + 1.043 YB <sub>12</sub> + YB <sub>6</sub> H <sub>4</sub> C <sub>6</sub> N                                       | -10.1589            |
| YNH <sub>4</sub> B <sub>6</sub> C <sub>6</sub> | 6 Y <sub>2</sub> C + 0.5 N <sub>2</sub> + 2 H <sub>2</sub> + 28 B → 11 YB <sub>2</sub> + YB <sub>6</sub> H <sub>4</sub> C <sub>6</sub> N                                                               | -10.0863            |
| YNH <sub>4</sub> B <sub>6</sub> C <sub>6</sub> | 6 Y <sub>2</sub> C + 2.667 B <sub>5</sub> H <sub>7</sub> + 0.5 N <sub>2</sub> → 7.333 YH <sub>2</sub> + 3.667 YB <sub>2</sub> + YB <sub>6</sub> H <sub>4</sub> C <sub>6</sub> N                        | -10.0500            |
| YNH <sub>4</sub> B <sub>6</sub> C <sub>6</sub> | 2.32 B <sub>9</sub> H <sub>11</sub> + 6 Y <sub>2</sub> C + YN → 10.76 YH <sub>2</sub> + 1.24 YB <sub>12</sub> + YB <sub>6</sub> H <sub>4</sub> C <sub>6</sub> N                                        | -10.0418            |
| YNH <sub>4</sub> B <sub>6</sub> C <sub>6</sub> | 0.6667 B <sub>9</sub> H <sub>11</sub> + 1.617 Y <sub>4</sub> C <sub>5</sub> + 3.233 N <sub>2</sub> → 0.4167 H <sub>8</sub> C <sub>5</sub> + 5.467 YN + YB <sub>6</sub> H <sub>4</sub> C <sub>6</sub> N | -10.0083            |
| YNH <sub>4</sub> B <sub>6</sub> C <sub>6</sub> | 3.636 B <sub>9</sub> H <sub>11</sub> + 6 Y <sub>2</sub> C + YN → 12 YH <sub>3</sub> + 26.73 B + YB <sub>6</sub> H <sub>4</sub> C <sub>6</sub> N                                                        | -9.9791             |
| YNH <sub>4</sub> B <sub>6</sub> C <sub>6</sub> | 2 YH <sub>2</sub> + 4.214 N <sub>2</sub> + 0.8571 Y <sub>4</sub> C <sub>7</sub> + 3 YB <sub>2</sub> → 7.429 YN + YB <sub>6</sub> H <sub>4</sub> C <sub>6</sub> N                                       | -9.9721             |
| YNH <sub>4</sub> B <sub>6</sub> C <sub>6</sub> | 3 B <sub>13</sub> C <sub>2</sub> + Y + 11.73 H <sub>3</sub> N → 4.455 B <sub>5</sub> H <sub>7</sub> + 10.73 BN + YB <sub>6</sub> H <sub>4</sub> C <sub>6</sub> N                                       | -9.9573             |
| YNH <sub>4</sub> B <sub>6</sub> C <sub>6</sub> | 2.364 B <sub>9</sub> H <sub>11</sub> + 6 Y <sub>2</sub> C + 0.5 N <sub>2</sub> → 11 YH <sub>2</sub> + 15.27 B + YB <sub>6</sub> H <sub>4</sub> C <sub>6</sub> N                                        | -9.9257             |
| YNH <sub>4</sub> B <sub>6</sub> C <sub>6</sub> | 3.5 Y <sub>2</sub> C + 0.5 H <sub>8</sub> C <sub>5</sub> + YN + 34 B → 7 YB <sub>4</sub> + YB <sub>6</sub> H <sub>4</sub> C <sub>6</sub> N                                                             | -9.8988             |
| YNH <sub>4</sub> B <sub>6</sub> C <sub>6</sub> | 2.688 B <sub>13</sub> C <sub>2</sub> + H <sub>3</sub> N + 0.125 H <sub>8</sub> C <sub>5</sub> + 16.47 YB <sub>2</sub> → 15.47 YB <sub>4</sub> + YB <sub>6</sub> H <sub>4</sub> C <sub>6</sub> N        | -9.8594             |
| YNH <sub>4</sub> B <sub>6</sub> C <sub>6</sub> | 6 Y <sub>2</sub> C + 22.37 B <sub>5</sub> H <sub>7</sub> + BN → 11.87 B <sub>9</sub> H <sub>11</sub> + 11 YH <sub>2</sub> + YB <sub>6</sub> H <sub>4</sub> C <sub>6</sub> N                            | -9.7971             |
| YNH <sub>4</sub> B <sub>6</sub> C <sub>6</sub> | 1.755 B <sub>9</sub> H <sub>11</sub> + 6 Y <sub>2</sub> C + H <sub>3</sub> N → 6.102 YH <sub>3</sub> + 4.898 YB <sub>2</sub> + YB <sub>6</sub> H <sub>4</sub> C <sub>6</sub> N                         | -9.7563             |
| YNH <sub>4</sub> B <sub>6</sub> C <sub>6</sub> | 1.6 B <sub>9</sub> H <sub>11</sub> + 6 Y <sub>2</sub> C + 0.5 N <sub>2</sub> → 6.8 YH <sub>2</sub> + 4.2 YB <sub>2</sub> + YB <sub>6</sub> H <sub>4</sub> C <sub>6</sub> N                             | -9.7352             |
| YNH <sub>4</sub> B <sub>6</sub> C <sub>6</sub> | 9.5 Y + H <sub>3</sub> N + 1.2 H <sub>8</sub> C <sub>5</sub> + 1.2 B <sub>5</sub> H <sub>7</sub> → 8.5 YH <sub>2</sub> + YB <sub>6</sub> H <sub>4</sub> C <sub>6</sub> N                               | -9.6873             |
| YNH <sub>4</sub> B <sub>6</sub> C <sub>6</sub> | 2.356 B <sub>9</sub> H <sub>11</sub> + 1.2 Y <sub>4</sub> C <sub>5</sub> + 4.152 N <sub>2</sub> → 7.304 H <sub>3</sub> N + 3.8 YB <sub>4</sub> + YB <sub>6</sub> H <sub>4</sub> C <sub>6</sub> N       | -9.6010             |
| YNH <sub>4</sub> B <sub>6</sub> C <sub>6</sub> | 0.4615 B <sub>13</sub> C <sub>2</sub> + 5.077 Y <sub>2</sub> C + 10.15 H <sub>3</sub> N → 9.154 YN + 13.23 H <sub>2</sub> + YB <sub>6</sub> H <sub>4</sub> C <sub>6</sub> N                            | -9.5997             |
| YNH <sub>4</sub> B <sub>6</sub> C <sub>6</sub> | 6 Y <sub>2</sub> C + 5.286 B <sub>5</sub> H <sub>7</sub> + BN → 11 YH <sub>3</sub> + 21.43 B + YB <sub>6</sub> H <sub>4</sub> C <sub>6</sub> N                                                         | -9.5253             |
| YNH <sub>4</sub> B <sub>6</sub> C <sub>6</sub> | 6 C + YB <sub>12</sub> + 3.5 N <sub>2</sub> + 2 H <sub>2</sub> → 6 BN + YB <sub>6</sub> H <sub>4</sub> C <sub>6</sub> N                                                                                | -9.4919             |
| YNH <sub>4</sub> B <sub>6</sub> C <sub>6</sub> | 6 Y <sub>2</sub> C + 0.5714 B <sub>5</sub> H <sub>7</sub> + 0.5 N <sub>2</sub> + 25.14 B → 11 YB <sub>2</sub> + YB <sub>6</sub> H <sub>4</sub> C <sub>6</sub> N                                        | -9.4891             |
| YNH <sub>4</sub> B <sub>6</sub> C <sub>6</sub> | 3.5 Y <sub>2</sub> C + 3.75 YB <sub>12</sub> + 0.5 H <sub>8</sub> C <sub>5</sub> + 0.5 N <sub>2</sub> → 9.75 YB <sub>4</sub> + YB <sub>6</sub> H <sub>4</sub> C <sub>6</sub> N                         | -9.4889             |
| YNH <sub>4</sub> B <sub>6</sub> C <sub>6</sub> | 6 Y <sub>2</sub> C + H <sub>3</sub> N + 3.286 B <sub>5</sub> H <sub>7</sub> → 11 YH <sub>2</sub> + 10.43 B + YB <sub>6</sub> H <sub>4</sub> C <sub>6</sub> N                                           | -9.4542             |
| YNH <sub>4</sub> B <sub>6</sub> C <sub>6</sub> | 0.4615 B <sub>13</sub> C <sub>2</sub> + 5.077 Y <sub>2</sub> C + 4.862 H <sub>3</sub> N → 5.292 YH <sub>2</sub> + 3.862 YN + YB <sub>6</sub> H <sub>4</sub> C <sub>6</sub> N                           | -9.4525             |
| YNH <sub>4</sub> B <sub>6</sub> C <sub>6</sub> | 0.3636 B <sub>9</sub> H <sub>11</sub> + 6 Y <sub>2</sub> C + 0.5 N <sub>2</sub> + 24.73 B → 11 YB <sub>2</sub> + YB <sub>6</sub> H <sub>4</sub> C <sub>6</sub> N                                       | -9.4269             |
| YNH <sub>4</sub> B <sub>6</sub> C <sub>6</sub> | 1.333 H <sub>3</sub> N + 1.2 Y <sub>4</sub> C <sub>5</sub> + 3.233 N <sub>2</sub> + 3 YB <sub>2</sub> → 6.8 YN + YB <sub>6</sub> H <sub>4</sub> C <sub>6</sub> N                                       | -9.3852             |
| YNH <sub>4</sub> B <sub>6</sub> C <sub>6</sub> | 2 YH <sub>2</sub> + 1.2 Y <sub>4</sub> C <sub>5</sub> + 4.15 N <sub>2</sub> + 1.5 YB <sub>4</sub> → 7.3 YN + YB <sub>6</sub> H <sub>4</sub> C <sub>6</sub> N                                           | -9.3714             |
| YNH <sub>4</sub> B <sub>6</sub> C <sub>6</sub> | 0.4615 B <sub>13</sub> C <sub>2</sub> + 5.077 Y <sub>2</sub> C + H <sub>3</sub> N + 9.654 H <sub>2</sub> → 9.154 YH <sub>2</sub> + YB <sub>6</sub> H <sub>4</sub> C <sub>6</sub> N                     | -9.3452             |
| YNH <sub>4</sub> B <sub>6</sub> C <sub>6</sub> | 2 YH <sub>2</sub> + 6 Y <sub>2</sub> C + 0.5 N <sub>2</sub> + 32 B → 13 YB <sub>2</sub> + YB <sub>6</sub> H <sub>4</sub> C <sub>6</sub> N                                                              | -9.3362             |
| YNH <sub>4</sub> B <sub>6</sub> C <sub>6</sub> | 0.4615 B <sub>13</sub> C <sub>2</sub> + 5.077 Y <sub>2</sub> C + YN + 12.15 H <sub>2</sub> → 10.15 YH <sub>2</sub> + YB <sub>6</sub> H <sub>4</sub> C <sub>6</sub> N                                   | -9.3174             |
| YNH <sub>4</sub> B <sub>6</sub> C <sub>6</sub> | 6 Y <sub>2</sub> C + 3.379 B <sub>5</sub> H <sub>7</sub> + YN → 6.552 YH <sub>3</sub> + 5.448 YB <sub>2</sub> + YB <sub>6</sub> H <sub>4</sub> C <sub>6</sub> N                                        | -9.3125             |
| YNH <sub>4</sub> B <sub>6</sub> C <sub>6</sub> | 3 B <sub>13</sub> C <sub>2</sub> + 12.36 H <sub>3</sub> N + YB <sub>2</sub> → 4.727 B <sub>5</sub> H <sub>7</sub> + 11.36 BN + YB <sub>6</sub> H <sub>4</sub> C <sub>6</sub> N                         | -9.2970             |
| YNH <sub>4</sub> B <sub>6</sub> C <sub>6</sub> | 6 Y <sub>2</sub> C + H <sub>3</sub> N + 2.417 B <sub>5</sub> H <sub>7</sub> → 7.958 YH <sub>2</sub> + 3.042 YB <sub>2</sub> + YB <sub>6</sub> H <sub>4</sub> C <sub>6</sub> N                          | -9.2216             |
| YNH <sub>4</sub> B <sub>6</sub> C <sub>6</sub> | 3.5 Y <sub>2</sub> C + 0.5 H <sub>8</sub> C <sub>5</sub> + BN + 77 B → 6 YB <sub>12</sub> + YB <sub>6</sub> H <sub>4</sub> C <sub>6</sub> N                                                            | -9.1976             |
| YNH <sub>4</sub> B <sub>6</sub> C <sub>6</sub> | 6 Y <sub>2</sub> C + 3.426 B <sub>5</sub> H <sub>7</sub> + BN → 9.989 YH <sub>2</sub> + 1.011 YB <sub>12</sub> + YB <sub>6</sub> H <sub>4</sub> C <sub>6</sub> N                                       | -9.1974             |
| YNH <sub>4</sub> B <sub>6</sub> C <sub>6</sub> | 6 Y <sub>2</sub> C + 1.333 H <sub>3</sub> N + 28.33 B → 0.3333 BN + 11 YB <sub>2</sub> + YB <sub>6</sub> H <sub>4</sub> C <sub>6</sub> N                                                               | -9.1764             |
| YNH <sub>4</sub> B <sub>6</sub> C <sub>6</sub> | 1.333 YH <sub>3</sub> + 6 Y <sub>2</sub> C + 0.5 N <sub>2</sub> + 30.67 B → 12.33 YB <sub>2</sub> + YB <sub>6</sub> H <sub>4</sub> C <sub>6</sub> N                                                    | -9.1736             |
| YNH <sub>4</sub> B <sub>6</sub> C <sub>6</sub> | 3 B <sub>13</sub> C <sub>2</sub> + 13 H <sub>3</sub> N + YB <sub>4</sub> → 5 B <sub>5</sub> H <sub>7</sub> + 12 BN + YB <sub>6</sub> H <sub>4</sub> C <sub>6</sub> N                                   | -9.1111             |
| YNH <sub>4</sub> B <sub>6</sub> C <sub>6</sub> | 1.333 YH <sub>3</sub> + 3 B <sub>13</sub> C <sub>2</sub> + BN + 16.33 YB <sub>2</sub> → 16.67 YB <sub>4</sub> + YB <sub>6</sub> H <sub>4</sub> C <sub>6</sub> N                                        | -9.1087             |
| YNH <sub>4</sub> B <sub>6</sub> C <sub>6</sub> | 2.091 B <sub>9</sub> H <sub>11</sub> + 6 Y <sub>2</sub> C + H <sub>3</sub> N → 11 YH <sub>2</sub> + 12.82 B + YB <sub>6</sub> H <sub>4</sub> C <sub>6</sub> N                                          | -9.0962             |
| YNH <sub>4</sub> B <sub>6</sub> C <sub>6</sub> | 2.147 B <sub>9</sub> H <sub>11</sub> + 6 Y <sub>2</sub> C + BN → 9.807 YH <sub>2</sub> + 1.193 YB <sub>12</sub> + YB <sub>6</sub> H <sub>4</sub> C <sub>6</sub> N                                      | -9.0889             |
| YNH <sub>4</sub> B <sub>6</sub> C <sub>6</sub> | YB <sub>12</sub> + 1.2 H <sub>8</sub> C <sub>5</sub> + 4.433 N <sub>2</sub> → 1.867 H <sub>3</sub> N + 6 BN + YB <sub>6</sub> H <sub>4</sub> C <sub>6</sub> N                                          | -8.9612             |
| YNH <sub>4</sub> B <sub>6</sub> C <sub>6</sub> | 3.364 B <sub>9</sub> H <sub>11</sub> + 6 Y <sub>2</sub> C + BN → 11 YH <sub>3</sub> + 25.27 B + YB <sub>6</sub> H <sub>4</sub> C <sub>6</sub> N                                                        | -8.9493             |
| YNH <sub>4</sub> B <sub>6</sub> C <sub>6</sub> | 1.45 B <sub>9</sub> H <sub>11</sub> + 6 Y <sub>2</sub> C + H <sub>3</sub> N → 7.475 YH <sub>2</sub> + 3.525 YB <sub>2</sub> + YB <sub>6</sub> H <sub>4</sub> C <sub>6</sub> N                          | -8.9363             |
| YNH <sub>4</sub> B <sub>6</sub> C <sub>6</sub> | 3.5 Y <sub>2</sub> C + 4.25 YB <sub>12</sub> + 0.5 H <sub>8</sub> C <sub>5</sub> + YN → 11.25 YB <sub>4</sub> + YB <sub>6</sub> H <sub>4</sub> C <sub>6</sub> N                                        | -8.9070             |
| YNH <sub>4</sub> B <sub>6</sub> C <sub>6</sub> | 6 Y <sub>2</sub> C + 1.333 H <sub>3</sub> N + 27.33 B → 0.3333 YN + 10.67 YB <sub>2</sub> + YB <sub>6</sub> H <sub>4</sub> C <sub>6</sub> N                                                            | -8.8965             |
| YNH <sub>4</sub> B <sub>6</sub> C <sub>6</sub> | 2 B <sub>9</sub> H <sub>11</sub> + 6 Y <sub>2</sub> C + YN → 6 YH <sub>3</sub> + 6 YB <sub>2</sub> + YB <sub>6</sub> H <sub>4</sub> C <sub>6</sub> N                                                   | -8.8395             |
| YNH <sub>4</sub> B <sub>6</sub> C <sub>6</sub> | 6 Y <sub>2</sub> C + 26 H <sub>2</sub> + 6 BN → 11 YH <sub>3</sub> + 5 H <sub>3</sub> N + YB <sub>6</sub> H <sub>4</sub> C <sub>6</sub> N                                                              | -8.8356             |
| YNH <sub>4</sub> B <sub>6</sub> C <sub>6</sub> | 3 B <sub>13</sub> C <sub>2</sub> + Y + 10.79 H <sub>3</sub> N → 2.579 B <sub>9</sub> H <sub>11</sub> + 9.789 BN + YB <sub>6</sub> H <sub>4</sub> C <sub>6</sub> N                                      | -8.8135             |

Continued on next page



Continued

| Compound                                       | Chemical reaction                                                                                                                                                                                 | Reaction energy(eV) |
|------------------------------------------------|---------------------------------------------------------------------------------------------------------------------------------------------------------------------------------------------------|---------------------|
| YNH <sub>4</sub> B <sub>6</sub> C <sub>6</sub> | 2 YH <sub>2</sub> + 1.2 Y <sub>4</sub> C <sub>5</sub> + 0.5 YB <sub>12</sub> + 3.65 N <sub>2</sub> → 6.3 YN + YB <sub>6</sub> H <sub>4</sub> C <sub>6</sub> N                                     | -8.7895             |
| YNH <sub>4</sub> B <sub>6</sub> C <sub>6</sub> | 6 Y <sub>2</sub> C + H <sub>3</sub> N + 0.5 H <sub>2</sub> + 28 B → 11 YB <sub>2</sub> + YB <sub>6</sub> H <sub>4</sub> C <sub>6</sub> N                                                          | -8.7622             |
| YNH <sub>4</sub> B <sub>6</sub> C <sub>6</sub> | 0.3846 B <sub>13</sub> C <sub>2</sub> + 5.231 Y <sub>2</sub> C + 11.46 H <sub>2</sub> + BN → 9.462 YH <sub>2</sub> + YB <sub>6</sub> H <sub>4</sub> C <sub>6</sub> N                              | -8.6929             |
| YNH <sub>4</sub> B <sub>6</sub> C <sub>6</sub> | 6 Y <sub>2</sub> C + 4 B <sub>5</sub> H <sub>7</sub> + YN → 12 YH <sub>2</sub> + 14 B + YB <sub>6</sub> H <sub>4</sub> C <sub>6</sub> N                                                           | -8.6800             |
| YNH <sub>4</sub> B <sub>6</sub> C <sub>6</sub> | 2 YH <sub>2</sub> + 1.2 Y <sub>4</sub> C <sub>5</sub> + 3.4 N <sub>2</sub> + 6 B → 5.8 YN + YB <sub>6</sub> H <sub>4</sub> C <sub>6</sub> N                                                       | -8.6735             |
| YNH <sub>4</sub> B <sub>6</sub> C <sub>6</sub> | 1.333 YH <sub>3</sub> + 3.881 N <sub>2</sub> + 0.8571 Y <sub>4</sub> C <sub>7</sub> + 3 YB <sub>2</sub> → 6.762 YN + YB <sub>6</sub> H <sub>4</sub> C <sub>6</sub> N                              | -8.6583             |
| YNH <sub>4</sub> B <sub>6</sub> C <sub>6</sub> | 6 Y <sub>2</sub> C + H <sub>3</sub> N + 0.1429 B <sub>5</sub> H <sub>7</sub> + 27.29 B → 11 YB <sub>2</sub> + YB <sub>6</sub> H <sub>4</sub> C <sub>6</sub> N                                     | -8.6129             |
| YNH <sub>4</sub> B <sub>6</sub> C <sub>6</sub> | 0.6667 B <sub>9</sub> H <sub>11</sub> + 8.967 Y + H <sub>3</sub> N + 1.2 H <sub>8</sub> C <sub>5</sub> → 7.967 YH <sub>2</sub> + YB <sub>6</sub> H <sub>4</sub> C <sub>6</sub> N                  | -8.6064             |
| YNH <sub>4</sub> B <sub>6</sub> C <sub>6</sub> | 0.09091 B <sub>9</sub> H <sub>11</sub> + 6 Y <sub>2</sub> C + H <sub>3</sub> N + 27.18 B → 11 YB <sub>2</sub> + YB <sub>6</sub> H <sub>4</sub> C <sub>6</sub> N                                   | -8.5974             |
| YNH <sub>4</sub> B <sub>6</sub> C <sub>6</sub> | 0.5 YH <sub>2</sub> + 6 Y <sub>2</sub> C + H <sub>3</sub> N + 29 B → 11.5 YB <sub>2</sub> + YB <sub>6</sub> H <sub>4</sub> C <sub>6</sub> N                                                       | -8.5747             |
| YNH <sub>4</sub> B <sub>6</sub> C <sub>6</sub> | 0.3333 YH <sub>3</sub> + 6 Y <sub>2</sub> C + H <sub>3</sub> N + 28.67 B → 11.33 YB <sub>2</sub> + YB <sub>6</sub> H <sub>4</sub> C <sub>6</sub> N                                                | -8.5341             |
| YNH <sub>4</sub> B <sub>6</sub> C <sub>6</sub> | 3 B <sub>13</sub> C <sub>2</sub> + 11.41 H <sub>3</sub> N + YN → 4.318 B <sub>5</sub> H <sub>7</sub> + 11.41 BN + YB <sub>6</sub> H <sub>4</sub> C <sub>6</sub> N                                 | -8.5231             |
| YNH <sub>4</sub> B <sub>6</sub> C <sub>6</sub> | 2 YH <sub>2</sub> + 3 B <sub>13</sub> C <sub>2</sub> + BN + 15 YB <sub>2</sub> → 16 YB <sub>4</sub> + YB <sub>6</sub> H <sub>4</sub> C <sub>6</sub> N                                             | -8.4301             |
| YNH <sub>4</sub> B <sub>6</sub> C <sub>6</sub> | 6 Y <sub>2</sub> C + 2.833 B <sub>5</sub> H <sub>7</sub> + YN → 7.917 YH <sub>2</sub> + 4.083 YB <sub>2</sub> + YB <sub>6</sub> H <sub>4</sub> C <sub>6</sub> N                                   | -8.3677             |
| YNH <sub>4</sub> B <sub>6</sub> C <sub>6</sub> | 6 Y <sub>2</sub> C + YN + 2 H <sub>2</sub> + 30 B → 12 YB <sub>2</sub> + YB <sub>6</sub> H <sub>4</sub> C <sub>6</sub> N                                                                          | -8.3594             |
| YNH <sub>4</sub> B <sub>6</sub> C <sub>6</sub> | 6 Y <sub>2</sub> C + 1.333 H <sub>3</sub> N + 28 B → 0.1667 N <sub>2</sub> + 11 YB <sub>2</sub> + YB <sub>6</sub> H <sub>4</sub> C <sub>6</sub> N                                                 | -8.3209             |
| YNH <sub>4</sub> B <sub>6</sub> C <sub>6</sub> | 6 Y <sub>2</sub> C + 3.069 B <sub>5</sub> H <sub>7</sub> + BN → 5.828 YH <sub>3</sub> + 5.172 YB <sub>2</sub> + YB <sub>6</sub> H <sub>4</sub> C <sub>6</sub> N                                   | -8.3014             |
| YNH <sub>4</sub> B <sub>6</sub> C <sub>6</sub> | 70 YH <sub>3</sub> + 3 B <sub>13</sub> C <sub>2</sub> + 34 YN → 103 YH <sub>2</sub> + 33 BN + YB <sub>6</sub> H <sub>4</sub> C <sub>6</sub> N                                                     | -8.2631             |
| YNH <sub>4</sub> B <sub>6</sub> C <sub>6</sub> | 1.75 B <sub>13</sub> C <sub>2</sub> + 9.375 Y + 0.5 H <sub>8</sub> C <sub>5</sub> + 0.5 N <sub>2</sub> → 8.375 YB <sub>2</sub> + YB <sub>6</sub> H <sub>4</sub> C <sub>6</sub> N                  | -8.2626             |
| YNH <sub>4</sub> B <sub>6</sub> C <sub>6</sub> | 2.545 B <sub>9</sub> H <sub>11</sub> + 6 Y <sub>2</sub> C + YN → 12 YH <sub>2</sub> + 16.91 B + YB <sub>6</sub> H <sub>4</sub> C <sub>6</sub> N                                                   | -8.2441             |
| YNH <sub>4</sub> B <sub>6</sub> C <sub>6</sub> | 3.5 C + YB <sub>12</sub> + 0.5 H <sub>8</sub> C <sub>5</sub> + 3.5 N <sub>2</sub> → 6 BN + YB <sub>6</sub> H <sub>4</sub> C <sub>6</sub> N                                                        | -8.2409             |
| YNH <sub>4</sub> B <sub>6</sub> C <sub>6</sub> | 1.2 Y <sub>4</sub> C <sub>5</sub> + 0.5714 B <sub>5</sub> H <sub>7</sub> + 3.186 N <sub>2</sub> + 1.571 YB <sub>2</sub> → 5.371 YN + YB <sub>6</sub> H <sub>4</sub> C <sub>6</sub> N              | -8.0864             |
| YNH <sub>4</sub> B <sub>6</sub> C <sub>6</sub> | 3 B <sub>13</sub> C <sub>2</sub> + 11.37 H <sub>3</sub> N + YB <sub>2</sub> → 2.737 B <sub>9</sub> H <sub>11</sub> + 10.37 BN + YB <sub>6</sub> H <sub>4</sub> C <sub>6</sub> N                   | -8.0832             |
| YNH <sub>4</sub> B <sub>6</sub> C <sub>6</sub> | 8.511 H <sub>3</sub> N + 1.2 Y <sub>4</sub> C <sub>5</sub> + 3.378 YB <sub>4</sub> → 7.178 YH <sub>3</sub> + 7.511 BN + YB <sub>6</sub> H <sub>4</sub> C <sub>6</sub> N                           | -8.0688             |
| YNH <sub>4</sub> B <sub>6</sub> C <sub>6</sub> | 1.333 YH <sub>3</sub> + 1.2 Y <sub>4</sub> C <sub>5</sub> + 3.817 N <sub>2</sub> + 1.5 YB <sub>4</sub> → 6.633 YN + YB <sub>6</sub> H <sub>4</sub> C <sub>6</sub> N                               | -8.0575             |
| YNH <sub>4</sub> B <sub>6</sub> C <sub>6</sub> | 1.333 YH <sub>3</sub> + 3 B <sub>13</sub> C <sub>2</sub> + YN + 13.83 YB <sub>2</sub> → 15.17 YB <sub>4</sub> + YB <sub>6</sub> H <sub>4</sub> C <sub>6</sub> N                                   | -8.0560             |
| YNH <sub>4</sub> B <sub>6</sub> C <sub>6</sub> | 1.7 B <sub>9</sub> H <sub>11</sub> + 6 Y <sub>2</sub> C + YN → 7.35 YH <sub>2</sub> + 4.65 YB <sub>2</sub> + YB <sub>6</sub> H <sub>4</sub> C <sub>6</sub> N                                      | -8.0332             |
| YNH <sub>4</sub> B <sub>6</sub> C <sub>6</sub> | 2.75 B <sub>13</sub> C <sub>2</sub> + 0.5 Y <sub>2</sub> C + 10.69 H <sub>3</sub> N → 4.011 B <sub>5</sub> H <sub>7</sub> + 9.693 BN + YB <sub>6</sub> H <sub>4</sub> C <sub>6</sub> N            | -8.0169             |
| YNH <sub>4</sub> B <sub>6</sub> C <sub>6</sub> | 1.055 B <sub>9</sub> H <sub>11</sub> + 1.2 Y <sub>4</sub> C <sub>5</sub> + 2.245 N <sub>2</sub> → 3.8 YH <sub>2</sub> + 3.491 BN + YB <sub>6</sub> H <sub>4</sub> C <sub>6</sub> N                | -7.8807             |
| YNH <sub>4</sub> B <sub>6</sub> C <sub>6</sub> | 1.816 B <sub>9</sub> H <sub>11</sub> + 6 Y <sub>2</sub> C + BN → 5.327 YH <sub>3</sub> + 5.673 YB <sub>2</sub> + YB <sub>6</sub> H <sub>4</sub> C <sub>6</sub> N                                  | -7.8718             |
| YNH <sub>4</sub> B <sub>6</sub> C <sub>6</sub> | 8 Y + 1.2 H <sub>8</sub> C <sub>5</sub> + 1.2 B <sub>5</sub> H <sub>7</sub> + 0.5 N <sub>2</sub> → 7 YH <sub>2</sub> + YB <sub>6</sub> H <sub>4</sub> C <sub>6</sub> N                            | -7.8446             |
| YNH <sub>4</sub> B <sub>6</sub> C <sub>6</sub> | 3 B <sub>13</sub> C <sub>2</sub> + 11.95 H <sub>3</sub> N + YB <sub>4</sub> → 2.895 B <sub>9</sub> H <sub>11</sub> + 10.95 BN + YB <sub>6</sub> H <sub>4</sub> C <sub>6</sub> N                   | -7.8273             |
| YNH <sub>4</sub> B <sub>6</sub> C <sub>6</sub> | 3.5 Y <sub>2</sub> C + 0.5 H <sub>8</sub> C <sub>5</sub> + BN + 29 B → 6 YB <sub>4</sub> + YB <sub>6</sub> H <sub>4</sub> C <sub>6</sub> N                                                        | -7.7973             |
| YNH <sub>4</sub> B <sub>6</sub> C <sub>6</sub> | 6 Y <sub>2</sub> C + 3.714 B <sub>5</sub> H <sub>7</sub> + BN → 11 YH <sub>2</sub> + 13.57 B + YB <sub>6</sub> H <sub>4</sub> C <sub>6</sub> N                                                    | -7.7637             |
| YNH <sub>4</sub> B <sub>6</sub> C <sub>6</sub> | 6 Y <sub>2</sub> C + 0.5714 B <sub>5</sub> H <sub>7</sub> + YN + 27.14 B → 12 YB <sub>2</sub> + YB <sub>6</sub> H <sub>4</sub> C <sub>6</sub> N                                                   | -7.7622             |
| YNH <sub>4</sub> B <sub>6</sub> C <sub>6</sub> | 6 C + 1.333 H <sub>3</sub> N + YB <sub>12</sub> + 2.833 N <sub>2</sub> → 6 BN + YB <sub>6</sub> H <sub>4</sub> C <sub>6</sub> N                                                                   | -7.7264             |
| YNH <sub>4</sub> B <sub>6</sub> C <sub>6</sub> | 0.3636 B <sub>9</sub> H <sub>11</sub> + 6 Y <sub>2</sub> C + YN + 26.73 B → 12 YB <sub>2</sub> + YB <sub>6</sub> H <sub>4</sub> C <sub>6</sub> N                                                  | -7.6999             |
| YNH <sub>4</sub> B <sub>6</sub> C <sub>6</sub> | 0.3636 B <sub>9</sub> H <sub>11</sub> + 1.2 Y <sub>4</sub> C <sub>5</sub> + 3.082 N <sub>2</sub> + 1.364 YB <sub>2</sub> → 5.164 YN + YB <sub>6</sub> H <sub>4</sub> C <sub>6</sub> N             | -7.6653             |
| YNH <sub>4</sub> B <sub>6</sub> C <sub>6</sub> | 0.875 B <sub>13</sub> C <sub>2</sub> + 0.5 H <sub>8</sub> C <sub>5</sub> + 3.187 N <sub>2</sub> + 0.25 Y <sub>4</sub> C <sub>7</sub> → 5.375 BN + YB <sub>6</sub> H <sub>4</sub> C <sub>6</sub> N | -7.6302             |
| YNH <sub>4</sub> B <sub>6</sub> C <sub>6</sub> | 2 YH <sub>2</sub> + 6 Y <sub>2</sub> C + YN + 34 B → 14 YB <sub>2</sub> + YB <sub>6</sub> H <sub>4</sub> C <sub>6</sub> N                                                                         | -7.6092             |
| YNH <sub>4</sub> B <sub>6</sub> C <sub>6</sub> | 6 Y <sub>2</sub> C + 2 H <sub>2</sub> + BN + 27 B → 11 YB <sub>2</sub> + YB <sub>6</sub> H <sub>4</sub> C <sub>6</sub> N                                                                          | -7.5195             |
| YNH <sub>4</sub> B <sub>6</sub> C <sub>6</sub> | 17.6 YH <sub>3</sub> + 6 Y <sub>2</sub> C + 1.2 B <sub>5</sub> H <sub>7</sub> + 0.5 N <sub>2</sub> → 28.6 YH <sub>2</sub> + YB <sub>6</sub> H <sub>4</sub> C <sub>6</sub> N                       | -7.5118             |
| YNH <sub>4</sub> B <sub>6</sub> C <sub>6</sub> | 1.333 YH <sub>3</sub> + 1.2 Y <sub>4</sub> C <sub>5</sub> + 0.5 YB <sub>12</sub> + 3.317 N <sub>2</sub> → 5.633 YN + YB <sub>6</sub> H <sub>4</sub> C <sub>6</sub> N                              | -7.4756             |
| YNH <sub>4</sub> B <sub>6</sub> C <sub>6</sub> | 6 Y <sub>2</sub> C + 2.583 B <sub>5</sub> H <sub>7</sub> + BN → 7.042 YH <sub>2</sub> + 3.958 YB <sub>2</sub> + YB <sub>6</sub> H <sub>4</sub> C <sub>6</sub> N                                   | -7.4609             |
| YNH <sub>4</sub> B <sub>6</sub> C <sub>6</sub> | 1.333 YH <sub>3</sub> + 6 Y <sub>2</sub> C + YN + 32.67 B → 13.33 YB <sub>2</sub> + YB <sub>6</sub> H <sub>4</sub> C <sub>6</sub> N                                                               | -7.4467             |
| YNH <sub>4</sub> B <sub>6</sub> C <sub>6</sub> | 6 Y <sub>2</sub> C + 11 H <sub>2</sub> + 6 BN → 6 YH <sub>3</sub> + 5 YN + YB <sub>6</sub> H <sub>4</sub> C <sub>6</sub> N                                                                        | -7.4274             |
| YNH <sub>4</sub> B <sub>6</sub> C <sub>6</sub> | 3 B <sub>13</sub> C <sub>2</sub> + 10.5 H <sub>3</sub> N + YN → 2.5 B <sub>9</sub> H <sub>11</sub> + 10.5 BN + YB <sub>6</sub> H <sub>4</sub> C <sub>6</sub> N                                    | -7.4144             |
| YNH <sub>4</sub> B <sub>6</sub> C <sub>6</sub> | 2 YH <sub>2</sub> + 3 B <sub>13</sub> C <sub>2</sub> + YN + 12.5 YB <sub>2</sub> → 14.5 YB <sub>4</sub> + YB <sub>6</sub> H <sub>4</sub> C <sub>6</sub> N                                         | -7.3774             |
| YNH <sub>4</sub> B <sub>6</sub> C <sub>6</sub> | YH <sub>2</sub> + 3 B <sub>13</sub> C <sub>2</sub> + 11.27 H <sub>3</sub> N → 4.545 B <sub>5</sub> H <sub>7</sub> + 10.27 BN + YB <sub>6</sub> H <sub>4</sub> C <sub>6</sub> N                    | -7.3763             |
| YNH <sub>4</sub> B <sub>6</sub> C <sub>6</sub> | 1.333 YH <sub>3</sub> + 1.2 Y <sub>4</sub> C <sub>5</sub> + 3.067 N <sub>2</sub> + 6 B → 5.133 YN + YB <sub>6</sub> H <sub>4</sub> C <sub>6</sub> N                                               | -7.3597             |
| YNH <sub>4</sub> B <sub>6</sub> C <sub>6</sub> | 2.364 B <sub>9</sub> H <sub>11</sub> + 6 Y <sub>2</sub> C + BN → 11 YH <sub>2</sub> + 16.27 B + YB <sub>6</sub> H <sub>4</sub> C <sub>6</sub> N                                                   | -7.3589             |
| YNH <sub>4</sub> B <sub>6</sub> C <sub>6</sub> | 2 YH <sub>2</sub> + 1.2 Y <sub>4</sub> C <sub>5</sub> + 0.5 N <sub>2</sub> + 75.6 B → 5.8 YB <sub>12</sub> + YB <sub>6</sub> H <sub>4</sub> C <sub>6</sub> N                                      | -7.3289             |
| YNH <sub>4</sub> B <sub>6</sub> C <sub>6</sub> | 3.214 N <sub>2</sub> + 0.8571 Y <sub>4</sub> C <sub>7</sub> + 2 H <sub>2</sub> + 3 YB <sub>2</sub> → 5.429 YN + YB <sub>6</sub> H <sub>4</sub> C <sub>6</sub> N                                   | -7.2684             |
| YNH <sub>4</sub> B <sub>6</sub> C <sub>6</sub> | 18.67 YH <sub>3</sub> + 0.6667 B <sub>9</sub> H <sub>11</sub> + 6 Y <sub>2</sub> C + 0.5 N <sub>2</sub> → 29.67 YH <sub>2</sub> + YB <sub>6</sub> H <sub>4</sub> C <sub>6</sub> N                 | -7.2268             |
| YNH <sub>4</sub> B <sub>6</sub> C <sub>6</sub> | 1.55 B <sub>9</sub> H <sub>11</sub> + 6 Y <sub>2</sub> C + BN → 6.525 YH <sub>2</sub> + 4.475 YB <sub>2</sub> + YB <sub>6</sub> H <sub>4</sub> C <sub>6</sub> N                                   | -7.1560             |
| YNH <sub>4</sub> B <sub>6</sub> C <sub>6</sub> | 0.4615 B <sub>13</sub> C <sub>2</sub> + 2.577 Y <sub>2</sub> C + 0.5 H <sub>8</sub> C <sub>5</sub> + 2.577 N <sub>2</sub> → 4.154 YN + YB <sub>6</sub> H <sub>4</sub> C <sub>6</sub> N            | -7.1168             |
| YNH <sub>4</sub> B <sub>6</sub> C <sub>6</sub> | 14.6 YH <sub>3</sub> + 6 Y <sub>2</sub> C + H <sub>3</sub> N + 1.2 B <sub>5</sub> H <sub>7</sub> → 25.6 YH <sub>2</sub> + YB <sub>6</sub> H <sub>4</sub> C <sub>6</sub> N                         | -7.1160             |
| YNH <sub>4</sub> B <sub>6</sub> C <sub>6</sub> | 2 YH <sub>2</sub> + 1.2 Y <sub>4</sub> C <sub>5</sub> + YN + 87.6 B → 6.8 YB <sub>12</sub> + YB <sub>6</sub> H <sub>4</sub> C <sub>6</sub> N                                                      | -7.0971             |
| YNH <sub>4</sub> B <sub>6</sub> C <sub>6</sub> | 6.929 H <sub>3</sub> N + 0.8571 Y <sub>4</sub> C <sub>7</sub> + 5.964 YB <sub>2</sub> → 8.393 YH <sub>2</sub> + 5.929 BN + YB <sub>6</sub> H <sub>4</sub> C <sub>6</sub> N                        | -7.0847             |
| YNH <sub>4</sub> B <sub>6</sub> C <sub>6</sub> | 2.75 B <sub>13</sub> C <sub>2</sub> + 0.5 Y <sub>2</sub> C + 9.849 H <sub>3</sub> N → 2.322 B <sub>9</sub> H <sub>11</sub> + 8.849 BN + YB <sub>6</sub> H <sub>4</sub> C <sub>6</sub> N           | -6.9869             |

Continued on next page

Continued

| Compound                                       | Chemical reaction                                                                                                                                                                              | Reaction energy(eV) |
|------------------------------------------------|------------------------------------------------------------------------------------------------------------------------------------------------------------------------------------------------|---------------------|
| YNH <sub>4</sub> B <sub>6</sub> C <sub>6</sub> | $3.5 \text{ Y}_2\text{C} + 3.625 \text{ YB}_{12} + 0.5 \text{ H}_8\text{C}_5 + \text{BN} \rightarrow 9.625 \text{ YB}_4 + \text{YB}_6\text{H}_4\text{C}_6\text{N}$                             | -6.9513             |
| YNH <sub>4</sub> B <sub>6</sub> C <sub>6</sub> | $5.375 \text{ Y}_2\text{C} + \text{H}_3\text{N} + 0.125 \text{ H}_8\text{C}_5 + 25.5 \text{ B} \rightarrow 9.75 \text{ YB}_2 + \text{YB}_6\text{H}_4\text{C}_6\text{N}$                        | -6.9391             |
| YNH <sub>4</sub> B <sub>6</sub> C <sub>6</sub> | $6 \text{ Y}_2\text{C} + 0.5714 \text{ B}_5\text{H}_7 + \text{BN} + 24.14 \text{ B} \rightarrow 11 \text{ YB}_2 + \text{YB}_6\text{H}_4\text{C}_6\text{N}$                                     | -6.9224             |
| YNH <sub>4</sub> B <sub>6</sub> C <sub>6</sub> | $0.3636 \text{ B}_9\text{H}_{11} + 6 \text{ Y}_2\text{C} + \text{BN} + 23.73 \text{ B} \rightarrow 11 \text{ YB}_2 + \text{YB}_6\text{H}_4\text{C}_6\text{N}$                                  | -6.8601             |
| YNH <sub>4</sub> B <sub>6</sub> C <sub>6</sub> | $\text{YH}_3 + 3 \text{ B}_{13}\text{C}_2 + 11.05 \text{ H}_3\text{N} \rightarrow 4.591 \text{ B}_5\text{H}_7 + 10.05 \text{ BN} + \text{YB}_6\text{H}_4\text{C}_6\text{N}$                    | -6.8319             |
| YNH <sub>4</sub> B <sub>6</sub> C <sub>6</sub> | $15.67 \text{ YH}_3 + 0.6667 \text{ B}_9\text{H}_{11} + 6 \text{ Y}_2\text{C} + \text{H}_3\text{N} \rightarrow 26.67 \text{ YH}_2 + \text{YB}_6\text{H}_4\text{C}_6\text{N}$                   | -6.8310             |
| YNH <sub>4</sub> B <sub>6</sub> C <sub>6</sub> | $2 \text{ YH}_2 + 6 \text{ Y}_2\text{C} + \text{BN} + 31 \text{ B} \rightarrow 13 \text{ YB}_2 + \text{YB}_6\text{H}_4\text{C}_6\text{N}$                                                      | -6.7694             |
| YNH <sub>4</sub> B <sub>6</sub> C <sub>6</sub> | $0.6667 \text{ B}_9\text{H}_{11} + 7.467 \text{ Y} + 1.2 \text{ H}_8\text{C}_5 + 0.5 \text{ N}_2 \rightarrow 6.467 \text{ YH}_2 + \text{YB}_6\text{H}_4\text{C}_6\text{N}$                     | -6.7637             |
| YNH <sub>4</sub> B <sub>6</sub> C <sub>6</sub> | $1.2 \text{ Y}_4\text{C}_5 + 3.15 \text{ N}_2 + 2 \text{ H}_2 + 1.5 \text{ YB}_4 \rightarrow 5.3 \text{ YN} + \text{YB}_6\text{H}_4\text{C}_6\text{N}$                                         | -6.6676             |
| YNH <sub>4</sub> B <sub>6</sub> C <sub>6</sub> | $1.2 \text{ Y}_4\text{C}_5 + 1.2 \text{ B}_5\text{H}_7 + 3.133 \text{ N}_2 \rightarrow 1.467 \text{ H}_3\text{N} + 3.8 \text{ YN} + \text{YB}_6\text{H}_4\text{C}_6\text{N}$                   | -6.6577             |
| YNH <sub>4</sub> B <sub>6</sub> C <sub>6</sub> | $1.333 \text{ YH}_3 + 6 \text{ Y}_2\text{C} + \text{BN} + 29.67 \text{ B} \rightarrow 12.33 \text{ YB}_2 + \text{YB}_6\text{H}_4\text{C}_6\text{N}$                                            | -6.6069             |
| YNH <sub>4</sub> B <sub>6</sub> C <sub>6</sub> | $1.75 \text{ B}_{13}\text{C}_2 + 9.875 \text{ Y} + 0.5 \text{ H}_8\text{C}_5 + \text{BN} \rightarrow 8.875 \text{ YB}_2 + \text{YB}_6\text{H}_4\text{C}_6\text{N}$                             | -6.5639             |
| YNH <sub>4</sub> B <sub>6</sub> C <sub>6</sub> | $2.514 \text{ B}_9\text{H}_{11} + 1.2 \text{ H}_8\text{C}_5 + 17.63 \text{ YN} \rightarrow 16.63 \text{ YH}_2 + 16.63 \text{ BN} + \text{YB}_6\text{H}_4\text{C}_6\text{N}$                    | -6.4996             |
| YNH <sub>4</sub> B <sub>6</sub> C <sub>6</sub> | $\text{YB}_{12} + 1.2 \text{ H}_8\text{C}_5 + 3.5 \text{ N}_2 \rightarrow 2.8 \text{ H}_2 + 6 \text{ BN} + \text{YB}_6\text{H}_4\text{C}_6\text{N}$                                            | -6.4896             |
| YNH <sub>4</sub> B <sub>6</sub> C <sub>6</sub> | $6 \text{ Y}_2\text{C} + 3.667 \text{ H}_3\text{N} + 6 \text{ BN} \rightarrow 2.333 \text{ YH}_3 + 8.667 \text{ YN} + \text{YB}_6\text{H}_4\text{C}_6\text{N}$                                 | -6.3947             |
| YNH <sub>4</sub> B <sub>6</sub> C <sub>6</sub> | $1.75 \text{ B}_{13}\text{C}_2 + 5.187 \text{ Y} + 0.5 \text{ H}_8\text{C}_5 + 0.5 \text{ N}_2 \rightarrow 4.187 \text{ YB}_4 + \text{YB}_6\text{H}_4\text{C}_6\text{N}$                       | -6.2760             |
| YNH <sub>4</sub> B <sub>6</sub> C <sub>6</sub> | $0.6667 \text{ B}_9\text{H}_{11} + 1.2 \text{ Y}_4\text{C}_5 + 2.956 \text{ N}_2 \rightarrow 1.111 \text{ H}_3\text{N} + 3.8 \text{ YN} + \text{YB}_6\text{H}_4\text{C}_6\text{N}$             | -6.2320             |
| YNH <sub>4</sub> B <sub>6</sub> C <sub>6</sub> | $6.055 \text{ H}_3\text{N} + 1.2 \text{ Y}_4\text{C}_5 + 0.9212 \text{ YB}_{12} \rightarrow 4.721 \text{ YH}_3 + 5.055 \text{ BN} + \text{YB}_6\text{H}_4\text{C}_6\text{N}$                   | -6.2190             |
| YNH <sub>4</sub> B <sub>6</sub> C <sub>6</sub> | $\text{YH}_2 + 3 \text{ B}_{13}\text{C}_2 + 10.32 \text{ H}_3\text{N} \rightarrow 2.632 \text{ B}_9\text{H}_{11} + 9.316 \text{ BN} + \text{YB}_6\text{H}_4\text{C}_6\text{N}$                 | -6.2092             |
| YNH <sub>4</sub> B <sub>6</sub> C <sub>6</sub> | $2 \text{ YH}_2 + 0.4615 \text{ B}_{13}\text{C}_2 + 1.015 \text{ Y}_4\text{C}_5 + 3.031 \text{ N}_2 \rightarrow 5.062 \text{ YN} + \text{YB}_6\text{H}_4\text{C}_6\text{N}$                    | -6.1909             |
| YNH <sub>4</sub> B <sub>6</sub> C <sub>6</sub> | $1.333 \text{ YH}_3 + 1.2 \text{ Y}_4\text{C}_5 + 0.5 \text{ N}_2 + 67.6 \text{ B} \rightarrow 5.133 \text{ YB}_{12} + \text{YB}_6\text{H}_4\text{C}_6\text{N}$                                | -6.1696             |
| YNH <sub>4</sub> B <sub>6</sub> C <sub>6</sub> | $26 \text{ YH}_3 + 6 \text{ Y}_2\text{C} + 0.5 \text{ N}_2 + 6 \text{ B} \rightarrow 37 \text{ YH}_2 + \text{YB}_6\text{H}_4\text{C}_6\text{N}$                                                | -6.1665             |
| YNH <sub>4</sub> B <sub>6</sub> C <sub>6</sub> | $9.25 \text{ YH}_3 + 3 \text{ B}_{13}\text{C}_2 + 4.458 \text{ N}_2 \rightarrow 7.917 \text{ H}_3\text{N} + 8.25 \text{ YB}_4 + \text{YB}_6\text{H}_4\text{C}_6\text{N}$                       | -6.1192             |
| YNH <sub>4</sub> B <sub>6</sub> C <sub>6</sub> | $1.2 \text{ Y}_4\text{C}_5 + 0.5 \text{ YB}_{12} + 2.65 \text{ N}_2 + 2 \text{ H}_2 \rightarrow 4.3 \text{ YN} + \text{YB}_6\text{H}_4\text{C}_6\text{N}$                                      | -6.0857             |
| YNH <sub>4</sub> B <sub>6</sub> C <sub>6</sub> | $6.4 \text{ H}_3\text{N} + 3.1 \text{ Y}_4\text{C}_5 + 6 \text{ BN} \rightarrow 1.9 \text{ H}_8\text{C}_5 + 11.4 \text{ YN} + \text{YB}_6\text{H}_4\text{C}_6\text{N}$                         | -6.0234             |
| YNH <sub>4</sub> B <sub>6</sub> C <sub>6</sub> | $1.026 \text{ B}_9\text{H}_{11} + 2.117 \text{ N}_2 + 0.8571 \text{ Y}_4\text{C}_7 \rightarrow 2.429 \text{ YH}_3 + 3.234 \text{ BN} + \text{YB}_6\text{H}_4\text{C}_6\text{N}$                | -5.9957             |
| YNH <sub>4</sub> B <sub>6</sub> C <sub>6</sub> | $1.2 \text{ B}_5\text{H}_7 + 2.5 \text{ N}_2 + 1.25 \text{ Y}_4\text{C}_7 \rightarrow 0.55 \text{ H}_8\text{C}_5 + 4 \text{ YN} + \text{YB}_6\text{H}_4\text{C}_6\text{N}$                     | -5.9808             |
| YNH <sub>4</sub> B <sub>6</sub> C <sub>6</sub> | $2 \text{ YH}_2 + 1.2 \text{ Y}_4\text{C}_5 + 0.5 \text{ N}_2 + 29.2 \text{ B} \rightarrow 5.8 \text{ YB}_4 + \text{YB}_6\text{H}_4\text{C}_6\text{N}$                                         | -5.9753             |
| YNH <sub>4</sub> B <sub>6</sub> C <sub>6</sub> | $1.2 \text{ Y}_4\text{C}_5 + 2.4 \text{ N}_2 + 2 \text{ H}_2 + 6 \text{ B} \rightarrow 3.8 \text{ YN} + \text{YB}_6\text{H}_4\text{C}_6\text{N}$                                               | -5.9698             |
| YNH <sub>4</sub> B <sub>6</sub> C <sub>6</sub> | $1.333 \text{ YH}_3 + 1.2 \text{ Y}_4\text{C}_5 + \text{YN} + 79.6 \text{ B} \rightarrow 6.133 \text{ YB}_{12} + \text{YB}_6\text{H}_4\text{C}_6\text{N}$                                      | -5.9378             |
| YNH <sub>4</sub> B <sub>6</sub> C <sub>6</sub> | $6 \text{ Y}_2\text{C} + 2.8 \text{ YB}_{12} + 0.5 \text{ N}_2 + 2 \text{ H}_2 \rightarrow 13.8 \text{ YB}_2 + \text{YB}_6\text{H}_4\text{C}_6\text{N}$                                        | -5.9000             |
| YNH <sub>4</sub> B <sub>6</sub> C <sub>6</sub> | $5.133 \text{ H}_3\text{N} + 1.2 \text{ Y}_4\text{C}_5 + 10.13 \text{ B} \rightarrow 3.8 \text{ YH}_3 + 4.133 \text{ BN} + \text{YB}_6\text{H}_4\text{C}_6\text{N}$                            | -5.8209             |
| YNH <sub>4</sub> B <sub>6</sub> C <sub>6</sub> | $23 \text{ YH}_3 + 6 \text{ Y}_2\text{C} + \text{H}_3\text{N} + 6 \text{ B} \rightarrow 34 \text{ YH}_2 + \text{YB}_6\text{H}_4\text{C}_6\text{N}$                                             | -5.7708             |
| YNH <sub>4</sub> B <sub>6</sub> C <sub>6</sub> | $1.2 \text{ Y}_4\text{C}_5 + 0.5714 \text{ B}_5\text{H}_7 + 2.793 \text{ N}_2 + 0.7857 \text{ YB}_4 \rightarrow 4.586 \text{ YN} + \text{YB}_6\text{H}_4\text{C}_6\text{N}$                    | -5.7382             |
| YNH <sub>4</sub> B <sub>6</sub> C <sub>6</sub> | $6 \text{ Y}_2\text{C} + 6 \text{ H}_3\text{N} + 6 \text{ BN} \rightarrow 11 \text{ YN} + 7 \text{ H}_2 + \text{YB}_6\text{H}_4\text{C}_6\text{N}$                                             | -5.7375             |
| YNH <sub>4</sub> B <sub>6</sub> C <sub>6</sub> | $6 \text{ Y}_2\text{C} + 2.514 \text{ YB}_{12} + 0.5714 \text{ B}_5\text{H}_7 + 0.5 \text{ N}_2 \rightarrow 13.51 \text{ YB}_2 + \text{YB}_6\text{H}_4\text{C}_6\text{N}$                      | -5.7300             |
| YNH <sub>4</sub> B <sub>6</sub> C <sub>6</sub> | $0.3636 \text{ B}_9\text{H}_{11} + 6 \text{ Y}_2\text{C} + 2.473 \text{ YB}_{12} + 0.5 \text{ N}_2 \rightarrow 13.47 \text{ YB}_2 + \text{YB}_6\text{H}_4\text{C}_6\text{N}$                   | -5.7299             |
| YNH <sub>4</sub> B <sub>6</sub> C <sub>6</sub> | $22 \text{ B}_9\text{H}_{11} + 6 \text{ Y}_2\text{C} + 0.5 \text{ N}_2 \rightarrow 34 \text{ B}_5\text{H}_7 + 11 \text{ YB}_2 + \text{YB}_6\text{H}_4\text{C}_6\text{N}$                       | -5.7218             |
| YNH <sub>4</sub> B <sub>6</sub> C <sub>6</sub> | $118.2 \text{ B}_9\text{H}_{11} + 6 \text{ Y}_2\text{C} + 0.5 \text{ N}_2 \rightarrow 11 \text{ YB}_{12} + 185.2 \text{ B}_5\text{H}_7 + \text{YB}_6\text{H}_4\text{C}_6\text{N}$              | -5.6861             |
| YNH <sub>4</sub> B <sub>6</sub> C <sub>6</sub> | $6 \text{ Y}_2\text{C} + 3.2 \text{ H}_3\text{N} + 6 \text{ BN} \rightarrow 2.8 \text{ YH}_2 + 8.2 \text{ YN} + \text{YB}_6\text{H}_4\text{C}_6\text{N}$                                       | -5.6597             |
| YNH <sub>4</sub> B <sub>6</sub> C <sub>6</sub> | $\text{YH}_3 + 3 \text{ B}_{13}\text{C}_2 + 10.08 \text{ H}_3\text{N} \rightarrow 2.658 \text{ B}_9\text{H}_{11} + 9.079 \text{ BN} + \text{YB}_6\text{H}_4\text{C}_6\text{N}$                 | -5.6531             |
| YNH <sub>4</sub> B <sub>6</sub> C <sub>6</sub> | $0.3636 \text{ B}_9\text{H}_{11} + 1.2 \text{ Y}_4\text{C}_5 + 2.741 \text{ N}_2 + 0.6818 \text{ YB}_4 \rightarrow 4.482 \text{ YN} + \text{YB}_6\text{H}_4\text{C}_6\text{N}$                 | -5.6276             |
| YNH <sub>4</sub> B <sub>6</sub> C <sub>6</sub> | $3.143 \text{ B}_5\text{H}_7 + 3.5 \text{ N}_2 + 0.8571 \text{ Y}_4\text{C}_7 \rightarrow 6 \text{ H}_3\text{N} + 2.429 \text{ YB}_4 + \text{YB}_6\text{H}_4\text{C}_6\text{N}$                | -5.6178             |
| YNH <sub>4</sub> B <sub>6</sub> C <sub>6</sub> | $6 \text{ Y}_2\text{C} + 8 \text{ H}_2 + 6 \text{ BN} \rightarrow 6 \text{ YH}_2 + 5 \text{ YN} + \text{YB}_6\text{H}_4\text{C}_6\text{N}$                                                     | -5.5707             |
| YNH <sub>4</sub> B <sub>6</sub> C <sub>6</sub> | $19.6 \text{ YH}_3 + 6 \text{ Y}_2\text{C} + 1.2 \text{ B}_5\text{H}_7 + \text{YN} \rightarrow 31.6 \text{ YH}_2 + \text{YB}_6\text{H}_4\text{C}_6\text{N}$                                    | -5.5410             |
| YNH <sub>4</sub> B <sub>6</sub> C <sub>6</sub> | $16.63 \text{ C} + 7 \text{ H}_3\text{N} + \text{YB}_{12} \rightarrow 2.125 \text{ H}_8\text{C}_5 + 6 \text{ BN} + \text{YB}_6\text{H}_4\text{C}_6\text{N}$                                    | -5.5398             |
| YNH <sub>4</sub> B <sub>6</sub> C <sub>6</sub> | $2 \text{ YH}_2 + 1.2 \text{ Y}_4\text{C}_5 + \text{YN} + 33.2 \text{ B} \rightarrow 6.8 \text{ YB}_4 + \text{YB}_6\text{H}_4\text{C}_6\text{N}$                                               | -5.5101             |
| YNH <sub>4</sub> B <sub>6</sub> C <sub>6</sub> | $1.333 \text{ H}_3\text{N} + 2.548 \text{ N}_2 + 0.8571 \text{ Y}_4\text{C}_7 + 3 \text{ YB}_2 \rightarrow 5.429 \text{ YN} + \text{YB}_6\text{H}_4\text{C}_6\text{N}$                         | -5.5029             |
| YNH <sub>4</sub> B <sub>6</sub> C <sub>6</sub> | $2 \text{ YH}_2 + 3.464 \text{ N}_2 + 0.8571 \text{ Y}_4\text{C}_7 + 1.5 \text{ YB}_4 \rightarrow 5.929 \text{ YN} + \text{YB}_6\text{H}_4\text{C}_6\text{N}$                                  | -5.4891             |
| YNH <sub>4</sub> B <sub>6</sub> C <sub>6</sub> | $2.375 \text{ B}_{13}\text{C}_2 + 9.142 \text{ H}_3\text{N} + 0.25 \text{ Y}_4\text{C}_5 \rightarrow 3.347 \text{ B}_5\text{H}_7 + 8.142 \text{ BN} + \text{YB}_6\text{H}_4\text{C}_6\text{N}$ | -5.4857             |
| YNH <sub>4</sub> B <sub>6</sub> C <sub>6</sub> | $6.667 \text{ Y} + \text{H}_3\text{N} + 1.2 \text{ H}_8\text{C}_5 + 1.2 \text{ B}_5\text{H}_7 \rightarrow 5.667 \text{ YH}_3 + \text{YB}_6\text{H}_4\text{C}_6\text{N}$                        | -5.4591             |
| YNH <sub>4</sub> B <sub>6</sub> C <sub>6</sub> | $32 \text{ YH}_3 + 6 \text{ Y}_2\text{C} + 0.5 \text{ N}_2 + 3 \text{ YB}_2 \rightarrow 46 \text{ YH}_2 + \text{YB}_6\text{H}_4\text{C}_6\text{N}$                                             | -5.4351             |
| YNH <sub>4</sub> B <sub>6</sub> C <sub>6</sub> | $1.2 \text{ Y}_4\text{C}_5 + 0.2619 \text{ YB}_{12} + 0.5714 \text{ B}_5\text{H}_7 + 2.531 \text{ N}_2 \rightarrow 4.062 \text{ YN} + \text{YB}_6\text{H}_4\text{C}_6\text{N}$                 | -5.4334             |
| YNH <sub>4</sub> B <sub>6</sub> C <sub>6</sub> | $6 \text{ Y}_2\text{C} + 20.5 \text{ H}_2 + 6 \text{ BN} \rightarrow 11 \text{ YH}_2 + 5 \text{ H}_3\text{N} + \text{YB}_6\text{H}_4\text{C}_6\text{N}$                                        | -5.4317             |
| YNH <sub>4</sub> B <sub>6</sub> C <sub>6</sub> | $1.2 \text{ Y}_4\text{C}_5 + 0.5714 \text{ B}_5\text{H}_7 + 2.4 \text{ N}_2 + 3.143 \text{ B} \rightarrow 3.8 \text{ YN} + \text{YB}_6\text{H}_4\text{C}_6\text{N}$                            | -5.3726             |
| YNH <sub>4</sub> B <sub>6</sub> C <sub>6</sub> | $0.3636 \text{ B}_9\text{H}_{11} + 1.2 \text{ Y}_4\text{C}_5 + 0.2273 \text{ YB}_{12} + 2.514 \text{ N}_2 \rightarrow 4.027 \text{ YN} + \text{YB}_6\text{H}_4\text{C}_6\text{N}$              | -5.3631             |
| YNH <sub>4</sub> B <sub>6</sub> C <sub>6</sub> | $0.3636 \text{ B}_9\text{H}_{11} + 1.2 \text{ Y}_4\text{C}_5 + 2.4 \text{ N}_2 + 2.727 \text{ B} \rightarrow 3.8 \text{ YN} + \text{YB}_6\text{H}_4\text{C}_6\text{N}$                         | -5.3104             |
| YNH <sub>4</sub> B <sub>6</sub> C <sub>6</sub> | $27 \text{ YH}_3 + 6 \text{ Y}_2\text{C} + 0.5 \text{ YB}_{12} + 0.5 \text{ N}_2 \rightarrow 38.5 \text{ YH}_2 + \text{YB}_6\text{H}_4\text{C}_6\text{N}$                                      | -5.2971             |
| YNH <sub>4</sub> B <sub>6</sub> C <sub>6</sub> | $20.67 \text{ YH}_3 + 0.6667 \text{ B}_9\text{H}_{11} + 6 \text{ Y}_2\text{C} + \text{YN} \rightarrow 32.67 \text{ YH}_2 + \text{YB}_6\text{H}_4\text{C}_6\text{N}$                            | -5.2560             |
| YNH <sub>4</sub> B <sub>6</sub> C <sub>6</sub> | $0.3636 \text{ B}_9\text{H}_{11} + 1.611 \text{ B}_{13}\text{C}_2 + 2.777 \text{ Y}_2\text{C} + 0.5 \text{ N}_2 \rightarrow 4.555 \text{ YB}_4 + \text{YB}_6\text{H}_4\text{C}_6\text{N}$      | -5.2231             |

Continued on next page

Continued

| Compound                                       | Chemical reaction                                                                                                                                                                                 | Reaction energy(eV) |
|------------------------------------------------|---------------------------------------------------------------------------------------------------------------------------------------------------------------------------------------------------|---------------------|
| YNH <sub>4</sub> B <sub>6</sub> C <sub>6</sub> | $6 \text{ Y}_2\text{C} + 5.867 \text{ H}_3\text{N} + 1.2 \text{ B}_5\text{H}_7 \rightarrow 11 \text{ YH}_2 + 2.433 \text{ N}_2 + \text{YB}_6\text{H}_4\text{C}_6\text{N}$                         | -5.1900             |
| YNH <sub>4</sub> B <sub>6</sub> C <sub>6</sub> | $1.338 \text{ B}_{13}\text{C}_2 + 3.325 \text{ Y}_2\text{C} + 6.649 \text{ H}_3\text{N} \rightarrow 2.278 \text{ B}_5\text{H}_7 + 5.649 \text{ YN} + \text{YB}_6\text{H}_4\text{C}_6\text{N}$     | -5.1573             |
| YNH <sub>4</sub> B <sub>6</sub> C <sub>6</sub> | $1.626 \text{ B}_{13}\text{C}_2 + 2.749 \text{ Y}_2\text{C} + 0.5714 \text{ B}_5\text{H}_7 + 0.5 \text{ N}_2 \rightarrow 4.498 \text{ YB}_4 + \text{YB}_6\text{H}_4\text{C}_6\text{N}$            | -5.1246             |
| YNH <sub>4</sub> B <sub>6</sub> C <sub>6</sub> | $2 \text{ YH}_2 + 1.2 \text{ Y}_4\text{C}_5 + 3.65 \text{ YB}_{12} + 0.5 \text{ N}_2 \rightarrow 9.45 \text{ YB}_4 + \text{YB}_6\text{H}_4\text{C}_6\text{N}$                                     | -5.1235             |
| YNH <sub>4</sub> B <sub>6</sub> C <sub>6</sub> | $1.2 \text{ Y}_4\text{C}_5 + 0.5 \text{ N}_2 + 2 \text{ H}_2 + 51.6 \text{ B} \rightarrow 3.8 \text{ YB}_{12} + \text{YB}_6\text{H}_4\text{C}_6\text{N}$                                          | -5.0888             |
| YNH <sub>4</sub> B <sub>6</sub> C <sub>6</sub> | $29 \text{ YH}_3 + 6 \text{ Y}_2\text{C} + \text{H}_3\text{N} + 3 \text{ YB}_2 \rightarrow 43 \text{ YH}_2 + \text{YB}_6\text{H}_4\text{C}_6\text{N}$                                             | -5.0393             |
| YNH <sub>4</sub> B <sub>6</sub> C <sub>6</sub> | $1.333 \text{ YH}_3 + 1.2 \text{ Y}_4\text{C}_5 + 0.5 \text{ N}_2 + 26.53 \text{ B} \rightarrow 5.133 \text{ YB}_4 + \text{YB}_6\text{H}_4\text{C}_6\text{N}$                                     | -4.9716             |
| YNH <sub>4</sub> B <sub>6</sub> C <sub>6</sub> | $1.2 \text{ Y}_4\text{C}_5 + 1.657 \text{ B}_5\text{H}_7 + 1.643 \text{ N}_2 \rightarrow 3.8 \text{ YH}_2 + 2.286 \text{ BN} + \text{YB}_6\text{H}_4\text{C}_6\text{N}$                           | -4.9678             |
| YNH <sub>4</sub> B <sub>6</sub> C <sub>6</sub> | $6 \text{ Y}_2\text{C} + 1.333 \text{ H}_3\text{N} + 2.833 \text{ YB}_{12} \rightarrow 0.3333 \text{ BN} + 13.83 \text{ YB}_2 + \text{YB}_6\text{H}_4\text{C}_6\text{N}$                          | -4.9403             |
| YNH <sub>4</sub> B <sub>6</sub> C <sub>6</sub> | $2 \text{ YH}_2 + 0.5 \text{ YB}_{12} + 2.964 \text{ N}_2 + 0.8571 \text{ Y}_4\text{C}_7 \rightarrow 4.929 \text{ YN} + \text{YB}_6\text{H}_4\text{C}_6\text{N}$                                  | -4.9072             |
| YNH <sub>4</sub> B <sub>6</sub> C <sub>6</sub> | $1.333 \text{ H}_3\text{N} + 1.2 \text{ Y}_4\text{C}_5 + 2.483 \text{ N}_2 + 1.5 \text{ YB}_4 \rightarrow 5.3 \text{ YN} + \text{YB}_6\text{H}_4\text{C}_6\text{N}$                               | -4.9022             |
| YNH <sub>4</sub> B <sub>6</sub> C <sub>6</sub> | $2.75 \text{ B}_9\text{H}_{11} + 1.2 \text{ Y}_4\text{C}_5 + 2.4 \text{ N}_2 \rightarrow 3.75 \text{ B}_5\text{H}_7 + 3.8 \text{ YN} + \text{YB}_6\text{H}_4\text{C}_6\text{N}$                   | -4.9017             |
| YNH <sub>4</sub> B <sub>6</sub> C <sub>6</sub> | $24 \text{ YH}_3 + 6 \text{ Y}_2\text{C} + \text{H}_3\text{N} + 0.5 \text{ YB}_{12} \rightarrow 35.5 \text{ YH}_2 + \text{YB}_6\text{H}_4\text{C}_6\text{N}$                                      | -4.9013             |
| YNH <sub>4</sub> B <sub>6</sub> C <sub>6</sub> | $9.25 \text{ YH}_2 + 3 \text{ B}_{13}\text{C}_2 + 2.917 \text{ N}_2 \rightarrow 4.833 \text{ H}_3\text{N} + 8.25 \text{ YB}_4 + \text{YB}_6\text{H}_4\text{C}_6\text{N}$                          | -4.8990             |
| YNH <sub>4</sub> B <sub>6</sub> C <sub>6</sub> | $1.333 \text{ YH}_3 + 0.4615 \text{ B}_{13}\text{C}_2 + 1.015 \text{ Y}_4\text{C}_5 + 2.697 \text{ N}_2 \rightarrow 4.395 \text{ YN} + \text{YB}_6\text{H}_4\text{C}_6\text{N}$                   | -4.8770             |
| YNH <sub>4</sub> B <sub>6</sub> C <sub>6</sub> | $1.2 \text{ Y}_4\text{C}_5 + \text{YN} + 2 \text{ H}_2 + 63.6 \text{ B} \rightarrow 4.8 \text{ YB}_{12} + \text{YB}_6\text{H}_4\text{C}_6\text{N}$                                                | -4.8570             |
| YNH <sub>4</sub> B <sub>6</sub> C <sub>6</sub> | $0.7 \text{ Y}_4\text{C}_5 + 0.5 \text{ H}_8\text{C}_5 + 2.9 \text{ N}_2 + 3 \text{ YB}_2 \rightarrow 4.8 \text{ YN} + \text{YB}_6\text{H}_4\text{C}_6\text{N}$                                   | -4.8537             |
| YNH <sub>4</sub> B <sub>6</sub> C <sub>6</sub> | $6 \text{ Y}_2\text{C} + 1.333 \text{ H}_3\text{N} + 2.733 \text{ YB}_{12} \rightarrow 0.3333 \text{ YN} + 13.4 \text{ YB}_2 + \text{YB}_6\text{H}_4\text{C}_6\text{N}$                           | -4.8099             |
| YNH <sub>4</sub> B <sub>6</sub> C <sub>6</sub> | $1.75 \text{ B}_{13}\text{C}_2 + 8.375 \text{ Y} + 0.5 \text{ H}_8\text{C}_5 + \text{YN} \rightarrow 8.375 \text{ YB}_2 + \text{YB}_6\text{H}_4\text{C}_6\text{N}$                                | -4.7996             |
| YNH <sub>4</sub> B <sub>6</sub> C <sub>6</sub> | $3 \text{ B}_{13}\text{C}_2 + 1.333 \text{ H}_3\text{N} + 7.333 \text{ YN} \rightarrow 7.667 \text{ BN} + 6.333 \text{ YB}_4 + \text{YB}_6\text{H}_4\text{C}_6\text{N}$                           | -4.7993             |
| YNH <sub>4</sub> B <sub>6</sub> C <sub>6</sub> | $2 \text{ YH}_2 + 2.714 \text{ N}_2 + 0.8571 \text{ Y}_4\text{C}_7 + 6 \text{ B} \rightarrow 4.429 \text{ YN} + \text{YB}_6\text{H}_4\text{C}_6\text{N}$                                          | -4.7913             |
| YNH <sub>4</sub> B <sub>6</sub> C <sub>6</sub> | $0.6667 \text{ B}_9\text{H}_{11} + 2.31 \text{ N}_2 + 1.155 \text{ Y}_4\text{C}_7 \rightarrow 0.4167 \text{ H}_8\text{C}_5 + 3.619 \text{ YN} + \text{YB}_6\text{H}_4\text{C}_6\text{N}$          | -4.7781             |
| YNH <sub>4</sub> B <sub>6</sub> C <sub>6</sub> | $0.6667 \text{ B}_9\text{H}_{11} + 6 \text{ Y}_2\text{C} + 6.222 \text{ H}_3\text{N} \rightarrow 11 \text{ YH}_2 + 2.611 \text{ N}_2 + \text{YB}_6\text{H}_4\text{C}_6\text{N}$                   | -4.7643             |
| YNH <sub>4</sub> B <sub>6</sub> C <sub>6</sub> | $2 \text{ YH}_2 + 1.2 \text{ Y}_4\text{C}_5 + \text{BN} + 74.6 \text{ B} \rightarrow 5.8 \text{ YB}_{12} + \text{YB}_6\text{H}_4\text{C}_6\text{N}$                                               | -4.7622             |
| YNH <sub>4</sub> B <sub>6</sub> C <sub>6</sub> | $0.6667 \text{ B}_9\text{H}_{11} + 1.2 \text{ Y}_4\text{C}_5 + 2.4 \text{ N}_2 \rightarrow 3.8 \text{ YN} + 1.667 \text{ H}_2 + \text{YB}_6\text{H}_4\text{C}_6\text{N}$                          | -4.7608             |
| YNH <sub>4</sub> B <sub>6</sub> C <sub>6</sub> | $19 \text{ YH}_3 + 6 \text{ Y}_2\text{C} + \text{B}_5\text{H}_7 + \text{BN} \rightarrow 30 \text{ YH}_2 + \text{YB}_6\text{H}_4\text{C}_6\text{N}$                                                | -4.7208             |
| YNH <sub>4</sub> B <sub>6</sub> C <sub>6</sub> | $1.2 \text{ Y}_4\text{C}_5 + 1.2 \text{ B}_5\text{H}_7 + 2.4 \text{ N}_2 \rightarrow 3.8 \text{ YN} + 2.2 \text{ H}_2 + \text{YB}_6\text{H}_4\text{C}_6\text{N}$                                  | -4.7158             |
| YNH <sub>4</sub> B <sub>6</sub> C <sub>6</sub> | $1.41 \text{ B}_{13}\text{C}_2 + 3.179 \text{ Y}_2\text{C} + 6.359 \text{ H}_3\text{N} \rightarrow 1.371 \text{ B}_9\text{H}_{11} + 5.359 \text{ YN} + \text{YB}_6\text{H}_4\text{C}_6\text{N}$   | -4.6965             |
| YNH <sub>4</sub> B <sub>6</sub> C <sub>6</sub> | $0.6667 \text{ B}_9\text{H}_{11} + 6.311 \text{ Y} + \text{H}_3\text{N} + 1.2 \text{ H}_8\text{C}_5 \rightarrow 5.311 \text{ YH}_3 + \text{YB}_6\text{H}_4\text{C}_6\text{N}$                     | -4.6435             |
| YNH <sub>4</sub> B <sub>6</sub> C <sub>6</sub> | $2.375 \text{ B}_{13}\text{C}_2 + 8.438 \text{ H}_3\text{N} + 0.25 \text{ Y}_4\text{C}_5 \rightarrow 1.938 \text{ B}_9\text{H}_{11} + 7.438 \text{ BN} + \text{YB}_6\text{H}_4\text{C}_6\text{N}$ | -4.6264             |
| YNH <sub>4</sub> B <sub>6</sub> C <sub>6</sub> | $1.724 \text{ B}_{13}\text{C}_2 + 2.552 \text{ Y}_2\text{C} + 0.5 \text{ N}_2 + 2 \text{ H}_2 \rightarrow 4.103 \text{ YB}_4 + \text{YB}_6\text{H}_4\text{C}_6\text{N}$                           | -4.6161             |
| YNH <sub>4</sub> B <sub>6</sub> C <sub>6</sub> | $1.333 \text{ YH}_3 + 6 \text{ Y}_2\text{C} + 3.067 \text{ YB}_{12} + 0.5 \text{ N}_2 \rightarrow 15.4 \text{ YB}_2 + \text{YB}_6\text{H}_4\text{C}_6\text{N}$                                    | -4.5887             |
| YNH <sub>4</sub> B <sub>6</sub> C <sub>6</sub> | $6 \text{ Y}_2\text{C} + \text{H}_3\text{N} + 2.8 \text{ YB}_{12} + 0.5 \text{ H}_2 \rightarrow 13.8 \text{ YB}_2 + \text{YB}_6\text{H}_4\text{C}_6\text{N}$                                      | -4.5759             |
| YNH <sub>4</sub> B <sub>6</sub> C <sub>6</sub> | $2 \text{ YH}_2 + 6 \text{ Y}_2\text{C} + 3.2 \text{ YB}_{12} + 0.5 \text{ N}_2 \rightarrow 16.2 \text{ YB}_2 + \text{YB}_6\text{H}_4\text{C}_6\text{N}$                                          | -4.5519             |
| YNH <sub>4</sub> B <sub>6</sub> C <sub>6</sub> | $2 \text{ YH}_2 + 1.2 \text{ Y}_4\text{C}_5 + 4.15 \text{ YB}_{12} + \text{YN} \rightarrow 10.95 \text{ YB}_4 + \text{YB}_6\text{H}_4\text{C}_6\text{N}$                                          | -4.5416             |
| YNH <sub>4</sub> B <sub>6</sub> C <sub>6</sub> | $6 \text{ Y}_2\text{C} + \text{H}_3\text{N} + 2.729 \text{ YB}_{12} + 0.1429 \text{ B}_5\text{H}_7 \rightarrow 13.73 \text{ YB}_2 + \text{YB}_6\text{H}_4\text{C}_6\text{N}$                      | -4.5334             |
| YNH <sub>4</sub> B <sub>6</sub> C <sub>6</sub> | $0.09091 \text{ B}_9\text{H}_{11} + 6 \text{ Y}_2\text{C} + \text{H}_3\text{N} + 2.718 \text{ YB}_{12} \rightarrow 13.72 \text{ YB}_2 + \text{YB}_6\text{H}_4\text{C}_6\text{N}$                  | -4.5334             |
| YNH <sub>4</sub> B <sub>6</sub> C <sub>6</sub> | $23.87 \text{ B}_9\text{H}_{11} + 6 \text{ Y}_2\text{C} + \text{H}_3\text{N} \rightarrow 37.37 \text{ B}_5\text{H}_7 + 11 \text{ YB}_2 + \text{YB}_6\text{H}_4\text{C}_6\text{N}$                 | -4.5246             |
| YNH <sub>4</sub> B <sub>6</sub> C <sub>6</sub> | $1.333 \text{ YH}_3 + 1.2 \text{ Y}_4\text{C}_5 + \text{YN} + 30.53 \text{ B} \rightarrow 6.133 \text{ YB}_4 + \text{YB}_6\text{H}_4\text{C}_6\text{N}$                                           | -4.5064             |
| YNH <sub>4</sub> B <sub>6</sub> C <sub>6</sub> | $1.746 \text{ B}_9\text{H}_{11} + 3.034 \text{ N}_2 + 0.8571 \text{ Y}_4\text{C}_7 \rightarrow 5.069 \text{ H}_3\text{N} + 2.429 \text{ YB}_4 + \text{YB}_6\text{H}_4\text{C}_6\text{N}$          | -4.5029             |
| YNH <sub>4</sub> B <sub>6</sub> C <sub>6</sub> | $1.2 \text{ Y}_4\text{C}_5 + 0.5714 \text{ B}_5\text{H}_7 + 0.5 \text{ N}_2 + 48.74 \text{ B} \rightarrow 3.8 \text{ YB}_{12} + \text{YB}_6\text{H}_4\text{C}_6\text{N}$                          | -4.4917             |
| YNH <sub>4</sub> B <sub>6</sub> C <sub>6</sub> | $120.1 \text{ B}_9\text{H}_{11} + 6 \text{ Y}_2\text{C} + \text{H}_3\text{N} \rightarrow 11 \text{ YB}_{12} + 188.6 \text{ B}_5\text{H}_7 + \text{YB}_6\text{H}_4\text{C}_6\text{N}$              | -4.4888             |
| YNH <sub>4</sub> B <sub>6</sub> C <sub>6</sub> | $19.89 \text{ YH}_3 + 0.5556 \text{ B}_9\text{H}_{11} + 6 \text{ Y}_2\text{C} + \text{BN} \rightarrow 30.89 \text{ YH}_2 + \text{YB}_6\text{H}_4\text{C}_6\text{N}$                               | -4.4833             |
| YNH <sub>4</sub> B <sub>6</sub> C <sub>6</sub> | $1.75 \text{ B}_{13}\text{C}_2 + 5.438 \text{ Y} + 0.5 \text{ H}_8\text{C}_5 + \text{BN} \rightarrow 4.438 \text{ YB}_4 + \text{YB}_6\text{H}_4\text{C}_6\text{N}$                                | -4.4587             |
| YNH <sub>4</sub> B <sub>6</sub> C <sub>6</sub> | $3.111 \text{ B}_9\text{H}_{11} + 6 \text{ Y}_2\text{C} + 0.5 \text{ N}_2 \rightarrow 15.11 \text{ H}_2 + 11 \text{ YB}_2 + \text{YB}_6\text{H}_4\text{C}_6\text{N}$                              | -4.4445             |
| YNH <sub>4</sub> B <sub>6</sub> C <sub>6</sub> | $0.3636 \text{ B}_9\text{H}_{11} + 1.2 \text{ Y}_4\text{C}_5 + 0.5 \text{ N}_2 + 48.33 \text{ B} \rightarrow 3.8 \text{ YB}_{12} + \text{YB}_6\text{H}_4\text{C}_6\text{N}$                       | -4.4294             |
| YNH <sub>4</sub> B <sub>6</sub> C <sub>6</sub> | $0.3636 \text{ B}_9\text{H}_{11} + 3 \text{ B}_{13}\text{C}_2 + 8.255 \text{ YN} \rightarrow 7.255 \text{ BN} + 7.255 \text{ YB}_4 + \text{YB}_6\text{H}_4\text{C}_6\text{N}$                     | -4.4189             |
| YNH <sub>4</sub> B <sub>6</sub> C <sub>6</sub> | $7 \text{ Y} + 1.2 \text{ H}_8\text{C}_5 + 1.2 \text{ B}_5\text{H}_7 + \text{YN} \rightarrow 7 \text{ YH}_2 + \text{YB}_6\text{H}_4\text{C}_6\text{N}$                                            | -4.3815             |
| YNH <sub>4</sub> B <sub>6</sub> C <sub>6</sub> | $5.667 \text{ Y} + 1.2 \text{ H}_8\text{C}_5 + 1.2 \text{ B}_5\text{H}_7 + 0.5 \text{ N}_2 \rightarrow 4.667 \text{ YH}_3 + \text{YB}_6\text{H}_4\text{C}_6\text{N}$                              | -4.3625             |
| YNH <sub>4</sub> B <sub>6</sub> C <sub>6</sub> | $0.5 \text{ YH}_2 + \text{H}_3\text{N} + 1.2 \text{ Y}_4\text{C}_5 + 57.6 \text{ B} \rightarrow 4.3 \text{ YB}_{12} + \text{YB}_6\text{H}_4\text{C}_6\text{N}$                                    | -4.3248             |
| YNH <sub>4</sub> B <sub>6</sub> C <sub>6</sub> | $1.333 \text{ H}_3\text{N} + 1.2 \text{ Y}_4\text{C}_5 + 0.5 \text{ YB}_{12} + 1.983 \text{ N}_2 \rightarrow 4.3 \text{ YN} + \text{YB}_6\text{H}_4\text{C}_6\text{N}$                            | -4.3203             |
| YNH <sub>4</sub> B <sub>6</sub> C <sub>6</sub> | $3 \text{ B}_{13}\text{C}_2 + 0.5714 \text{ B}_5\text{H}_7 + 8.171 \text{ YN} \rightarrow 7.171 \text{ BN} + 7.171 \text{ YB}_4 + \text{YB}_6\text{H}_4\text{C}_6\text{N}$                        | -4.3065             |
| YNH <sub>4</sub> B <sub>6</sub> C <sub>6</sub> | $1.2 \text{ H}_8\text{C}_5 + 3.233 \text{ N}_2 + 2.867 \text{ YB}_4 \rightarrow 1.867 \text{ YH}_3 + 5.467 \text{ BN} + \text{YB}_6\text{H}_4\text{C}_6\text{N}$                                  | -4.2766             |
| YNH <sub>4</sub> B <sub>6</sub> C <sub>6</sub> | $1.2 \text{ Y}_4\text{C}_5 + 0.5714 \text{ B}_5\text{H}_7 + \text{YN} + 60.74 \text{ B} \rightarrow 4.8 \text{ YB}_{12} + \text{YB}_6\text{H}_4\text{C}_6\text{N}$                                | -4.2599             |
| YNH <sub>4</sub> B <sub>6</sub> C <sub>6</sub> | $0.3333 \text{ YH}_3 + 6 \text{ Y}_2\text{C} + \text{H}_3\text{N} + 2.867 \text{ YB}_{12} \rightarrow 14.2 \text{ YB}_2 + \text{YB}_6\text{H}_4\text{C}_6\text{N}$                                | -4.2481             |
| YNH <sub>4</sub> B <sub>6</sub> C <sub>6</sub> | $0.5 \text{ YH}_2 + 6 \text{ Y}_2\text{C} + \text{H}_3\text{N} + 2.9 \text{ YB}_{12} \rightarrow 14.4 \text{ YB}_2 + \text{YB}_6\text{H}_4\text{C}_6\text{N}$                                     | -4.2389             |
| YNH <sub>4</sub> B <sub>6</sub> C <sub>6</sub> | $6 \text{ Y}_2\text{C} + 5.6 \text{ B}_5\text{H}_7 + 0.5 \text{ N}_2 \rightarrow 17.6 \text{ H}_2 + 11 \text{ YB}_2 + \text{YB}_6\text{H}_4\text{C}_6\text{N}$                                    | -4.2341             |
| YNH <sub>4</sub> B <sub>6</sub> C <sub>6</sub> | $1.333 \text{ H}_3\text{N} + 1.2 \text{ Y}_4\text{C}_5 + 1.733 \text{ N}_2 + 6 \text{ B} \rightarrow 3.8 \text{ YN} + \text{YB}_6\text{H}_4\text{C}_6\text{N}$                                    | -4.2044             |
| YNH <sub>4</sub> B <sub>6</sub> C <sub>6</sub> | $0.5714 \text{ B}_5\text{H}_7 + 2.5 \text{ N}_2 + 0.8571 \text{ Y}_4\text{C}_7 + 1.571 \text{ YB}_2 \rightarrow 4 \text{ YN} + \text{YB}_6\text{H}_4\text{C}_6\text{N}$                           | -4.2042             |
| YNH <sub>4</sub> B <sub>6</sub> C <sub>6</sub> | $1.2 \text{ Y}_4\text{C}_5 + 0.5 \text{ N}_2 + 2 \text{ H}_2 + 21.2 \text{ B} \rightarrow 3.8 \text{ YB}_4 + \text{YB}_6\text{H}_4\text{C}_6\text{N}$                                             | -4.2020             |

Continued on next page

Continued

| Compound                                       | Chemical reaction                                                                                                                                                                                       | Reaction energy(eV) |
|------------------------------------------------|---------------------------------------------------------------------------------------------------------------------------------------------------------------------------------------------------------|---------------------|
| YNH <sub>4</sub> B <sub>6</sub> C <sub>6</sub> | 0.3636 B <sub>9</sub> H <sub>11</sub> + 1.2 Y <sub>4</sub> C <sub>5</sub> + YN + 60.33 B → 4.8 YB <sub>12</sub> + YB <sub>6</sub> H <sub>4</sub> C <sub>6</sub> N                                       | -4.1976             |
| YNH <sub>4</sub> B <sub>6</sub> C <sub>6</sub> | 1.333 YH <sub>3</sub> + 1.2 Y <sub>4</sub> C <sub>5</sub> + 3.317 YB <sub>12</sub> + 0.5 N <sub>2</sub> → 8.45 YB <sub>4</sub> + YB <sub>6</sub> H <sub>4</sub> C <sub>6</sub> N                        | -4.1976             |
| YNH <sub>4</sub> B <sub>6</sub> C <sub>6</sub> | 28 YH <sub>3</sub> + 6 Y <sub>2</sub> C + YN + 6 B → 40 YH <sub>2</sub> + YB <sub>6</sub> H <sub>4</sub> C <sub>6</sub> N                                                                               | -4.1958             |
| YNH <sub>4</sub> B <sub>6</sub> C <sub>6</sub> | 0.3636 B <sub>9</sub> H <sub>11</sub> + 0.2098 B <sub>13</sub> C <sub>2</sub> + 1.116 Y <sub>4</sub> C <sub>5</sub> + 2.232 N <sub>2</sub> → 3.464 YN + YB <sub>6</sub> H <sub>4</sub> C <sub>6</sub> N | -4.1819             |
| YNH <sub>4</sub> B <sub>6</sub> C <sub>6</sub> | 1.333 H <sub>3</sub> N + 1.2 Y <sub>4</sub> C <sub>5</sub> + 51.93 B → 3.8 YB <sub>12</sub> + 0.3333 BN + YB <sub>6</sub> H <sub>4</sub> C <sub>6</sub> N                                               | -4.1790             |
| YNH <sub>4</sub> B <sub>6</sub> C <sub>6</sub> | 1.333 YH <sub>3</sub> + 3.131 N <sub>2</sub> + 0.8571 Y <sub>4</sub> C <sub>7</sub> + 1.5 YB <sub>4</sub> → 5.262 YN + YB <sub>6</sub> H <sub>4</sub> C <sub>6</sub> N                                  | -4.1753             |
| YNH <sub>4</sub> B <sub>6</sub> C <sub>6</sub> | 6 Y <sub>2</sub> C + 1.333 H <sub>3</sub> N + 2.8 YB <sub>12</sub> → 0.1667 N <sub>2</sub> + 13.8 YB <sub>2</sub> + YB <sub>6</sub> H <sub>4</sub> C <sub>6</sub> N                                     | -4.1346             |
| YNH <sub>4</sub> B <sub>6</sub> C <sub>6</sub> | 0.2418 B <sub>13</sub> C <sub>2</sub> + 1.103 Y <sub>4</sub> C <sub>5</sub> + 0.5714 B <sub>5</sub> H <sub>7</sub> + 2.207 N <sub>2</sub> → 3.413 YN + YB <sub>6</sub> H <sub>4</sub> C <sub>6</sub> N  | -4.0722             |
| YNH <sub>4</sub> B <sub>6</sub> C <sub>6</sub> | 1.2 Y <sub>4</sub> C <sub>5</sub> + 0.5 N <sub>2</sub> + 12.2 H <sub>2</sub> + 3 YB <sub>2</sub> → 6.8 YH <sub>3</sub> + YB <sub>6</sub> H <sub>4</sub> C <sub>6</sub> N                                | -4.0621             |
| YNH <sub>4</sub> B <sub>6</sub> C <sub>6</sub> | 0.3333 YH <sub>3</sub> + H <sub>3</sub> N + 1.2 Y <sub>4</sub> C <sub>5</sub> + 55.6 B → 4.133 YB <sub>12</sub> + YB <sub>6</sub> H <sub>4</sub> C <sub>6</sub> N                                       | -4.0350             |
| YNH <sub>4</sub> B <sub>6</sub> C <sub>6</sub> | 7.3 Y + 1.2 H <sub>8</sub> C <sub>5</sub> + B <sub>5</sub> H <sub>7</sub> + BN → 6.3 YH <sub>2</sub> + YB <sub>6</sub> H <sub>4</sub> C <sub>6</sub> N                                                  | -4.0090             |
| YNH <sub>4</sub> B <sub>6</sub> C <sub>6</sub> | 2.125 B <sub>13</sub> C <sub>2</sub> + 8.108 H <sub>3</sub> N + 0.25 Y <sub>4</sub> C <sub>7</sub> → 2.903 B <sub>5</sub> H <sub>7</sub> + 7.108 BN + YB <sub>6</sub> H <sub>4</sub> C <sub>6</sub> N   | -3.9500             |
| YNH <sub>4</sub> B <sub>6</sub> C <sub>6</sub> | 29 YH <sub>3</sub> + 6 Y <sub>2</sub> C + 0.5 N <sub>2</sub> + 1.5 YB <sub>4</sub> → 41.5 YH <sub>2</sub> + YB <sub>6</sub> H <sub>4</sub> C <sub>6</sub> N                                             | -3.9082             |
| YNH <sub>4</sub> B <sub>6</sub> C <sub>6</sub> | 6 Y <sub>2</sub> C + 3 YB <sub>12</sub> + YN + 2 H <sub>2</sub> → 15 YB <sub>2</sub> + YB <sub>6</sub> H <sub>4</sub> C <sub>6</sub> N                                                                  | -3.8741             |
| YNH <sub>4</sub> B <sub>6</sub> C <sub>6</sub> | 1.75 B <sub>13</sub> C <sub>2</sub> + 0.5 H <sub>8</sub> C <sub>5</sub> + 0.5 N <sub>2</sub> + 10.38 YB <sub>2</sub> → 9.375 YB <sub>4</sub> + YB <sub>6</sub> H <sub>4</sub> C <sub>6</sub> N          | -3.8150             |
| YNH <sub>4</sub> B <sub>6</sub> C <sub>6</sub> | 0.3636 B <sub>9</sub> H <sub>11</sub> + 2.396 N <sub>2</sub> + 0.8571 Y <sub>4</sub> C <sub>7</sub> + 1.364 YB <sub>2</sub> → 3.792 YN + YB <sub>6</sub> H <sub>4</sub> C <sub>6</sub> N                | -3.7831             |
| YNH <sub>4</sub> B <sub>6</sub> C <sub>6</sub> | 22.31 YH <sub>3</sub> + 0.4615 B <sub>13</sub> C <sub>2</sub> + 5.077 Y <sub>2</sub> C + 0.5 N <sub>2</sub> → 31.46 YH <sub>2</sub> + YB <sub>6</sub> H <sub>4</sub> C <sub>6</sub> N                   | -3.7664             |
| YNH <sub>4</sub> B <sub>6</sub> C <sub>6</sub> | H <sub>3</sub> N + 1.2 Y <sub>4</sub> C <sub>5</sub> + 0.5 H <sub>2</sub> + 51.6 B → 3.8 YB <sub>12</sub> + YB <sub>6</sub> H <sub>4</sub> C <sub>6</sub> N                                             | -3.7648             |
| YNH <sub>4</sub> B <sub>6</sub> C <sub>6</sub> | 2 YH <sub>2</sub> + 0.5 N <sub>2</sub> + 0.8571 Y <sub>4</sub> C <sub>7</sub> + 59.14 B → 4.429 YB <sub>12</sub> + YB <sub>6</sub> H <sub>4</sub> C <sub>6</sub> N                                      | -3.7646             |
| YNH <sub>4</sub> B <sub>6</sub> C <sub>6</sub> | 6 Y <sub>2</sub> C + 9.533 H <sub>3</sub> N + 1.2 B <sub>5</sub> H <sub>7</sub> → 11 YH <sub>3</sub> + 4.267 N <sub>2</sub> + YB <sub>6</sub> H <sub>4</sub> C <sub>6</sub> N                           | -3.7390             |
| YNH <sub>4</sub> B <sub>6</sub> C <sub>6</sub> | 1.2 Y <sub>4</sub> C <sub>5</sub> + YN + 2 H <sub>2</sub> + 25.2 B → 4.8 YB <sub>4</sub> + YB <sub>6</sub> H <sub>4</sub> C <sub>6</sub> N                                                              | -3.7368             |
| YNH <sub>4</sub> B <sub>6</sub> C <sub>6</sub> | 6 Y <sub>2</sub> C + 2.714 YB <sub>12</sub> + 0.5714 B <sub>5</sub> H <sub>7</sub> + YN → 14.71 YB <sub>2</sub> + YB <sub>6</sub> H <sub>4</sub> C <sub>6</sub> N                                       | -3.7041             |
| YNH <sub>4</sub> B <sub>6</sub> C <sub>6</sub> | 0.3636 B <sub>9</sub> H <sub>11</sub> + 6 Y <sub>2</sub> C + 2.673 YB <sub>12</sub> + YN → 14.67 YB <sub>2</sub> + YB <sub>6</sub> H <sub>4</sub> C <sub>6</sub> N                                      | -3.7039             |
| YNH <sub>4</sub> B <sub>6</sub> C <sub>6</sub> | 3 B <sub>13</sub> C <sub>2</sub> + 7.6 YN + 2 H <sub>2</sub> → 6.6 BN + 6.6 YB <sub>4</sub> + YB <sub>6</sub> H <sub>4</sub> C <sub>6</sub> N                                                           | -3.7028             |
| YNH <sub>4</sub> B <sub>6</sub> C <sub>6</sub> | 23.75 B <sub>9</sub> H <sub>11</sub> + 6 Y <sub>2</sub> C + YN → 36.75 B <sub>5</sub> H <sub>7</sub> + 12 YB <sub>2</sub> + YB <sub>6</sub> H <sub>4</sub> C <sub>6</sub> N                             | -3.6952             |
| YNH <sub>4</sub> B <sub>6</sub> C <sub>6</sub> | 128.7 B <sub>9</sub> H <sub>11</sub> + 6 Y <sub>2</sub> C + YN → 12 YB <sub>12</sub> + 201.7 B <sub>5</sub> H <sub>7</sub> + YB <sub>6</sub> H <sub>4</sub> C <sub>6</sub> N                            | -3.6562             |
| YNH <sub>4</sub> B <sub>6</sub> C <sub>6</sub> | 1.333 YH <sub>3</sub> + 1.2 Y <sub>4</sub> C <sub>5</sub> + 3.817 YB <sub>12</sub> + YN → 9.95 YB <sub>4</sub> + YB <sub>6</sub> H <sub>4</sub> C <sub>6</sub> N                                        | -3.6157             |
| YNH <sub>4</sub> B <sub>6</sub> C <sub>6</sub> | H <sub>3</sub> N + 1.2 Y <sub>4</sub> C <sub>5</sub> + 0.1429 B <sub>5</sub> H <sub>7</sub> + 50.89 B → 3.8 YB <sub>12</sub> + YB <sub>6</sub> H <sub>4</sub> C <sub>6</sub> N                          | -3.6155             |
| YNH <sub>4</sub> B <sub>6</sub> C <sub>6</sub> | 6.683 H <sub>3</sub> N + 0.8571 Y <sub>4</sub> C <sub>7</sub> + 2.921 YB <sub>4</sub> → 5.349 YH <sub>3</sub> + 5.683 BN + YB <sub>6</sub> H <sub>4</sub> C <sub>6</sub> N                              | -3.6077             |
| YNH <sub>4</sub> B <sub>6</sub> C <sub>6</sub> | 1.2 Y <sub>4</sub> C <sub>5</sub> + 0.5714 B <sub>5</sub> H <sub>7</sub> + 0.5 N <sub>2</sub> + 18.34 B → 3.8 YB <sub>4</sub> + YB <sub>6</sub> H <sub>4</sub> C <sub>6</sub> N                         | -3.6048             |
| YNH <sub>4</sub> B <sub>6</sub> C <sub>6</sub> | 1.333 YH <sub>3</sub> + 1.2 Y <sub>4</sub> C <sub>5</sub> + BN + 66.6 B → 5.133 YB <sub>12</sub> + YB <sub>6</sub> H <sub>4</sub> C <sub>6</sub> N                                                      | -3.6029             |
| YNH <sub>4</sub> B <sub>6</sub> C <sub>6</sub> | 0.6667 B <sub>9</sub> H <sub>11</sub> + 1.2 Y <sub>4</sub> C <sub>5</sub> + 1.844 N <sub>2</sub> → 1.111 YH <sub>3</sub> + 2.689 YN + YB <sub>6</sub> H <sub>4</sub> C <sub>6</sub> N                   | -3.6026             |
| YNH <sub>4</sub> B <sub>6</sub> C <sub>6</sub> | 0.09091 B <sub>9</sub> H <sub>11</sub> + H <sub>3</sub> N + 1.2 Y <sub>4</sub> C <sub>5</sub> + 50.78 B → 3.8 YB <sub>12</sub> + YB <sub>6</sub> H <sub>4</sub> C <sub>6</sub> N                        | -3.5999             |
| YNH <sub>4</sub> B <sub>6</sub> C <sub>6</sub> | 26 YH <sub>3</sub> + 6 Y <sub>2</sub> C + BN + 5 B → 37 YH <sub>2</sub> + YB <sub>6</sub> H <sub>4</sub> C <sub>6</sub> N                                                                               | -3.5998             |
| YNH <sub>4</sub> B <sub>6</sub> C <sub>6</sub> | 1.333 YH <sub>3</sub> + 0.5 YB <sub>12</sub> + 2.631 N <sub>2</sub> + 0.8571 Y <sub>4</sub> C <sub>7</sub> → 4.262 YN + YB <sub>6</sub> H <sub>4</sub> C <sub>6</sub> N                                 | -3.5934             |
| YNH <sub>4</sub> B <sub>6</sub> C <sub>6</sub> | 1.2 Y <sub>4</sub> C <sub>5</sub> + 2.65 YB <sub>12</sub> + 0.5 N <sub>2</sub> + 2 H <sub>2</sub> → 6.45 YB <sub>4</sub> + YB <sub>6</sub> H <sub>4</sub> C <sub>6</sub> N                              | -3.5835             |
| YNH <sub>4</sub> B <sub>6</sub> C <sub>6</sub> | 1.736 B <sub>13</sub> C <sub>2</sub> + 2.529 Y <sub>2</sub> C + 1.333 H <sub>3</sub> N → 0.3333 BN + 4.057 YB <sub>4</sub> + YB <sub>6</sub> H <sub>4</sub> C <sub>6</sub> N                            | -3.5773             |
| YNH <sub>4</sub> B <sub>6</sub> C <sub>6</sub> | 0.6667 B <sub>9</sub> H <sub>11</sub> + 5.311 Y + 1.2 H <sub>8</sub> C <sub>5</sub> + 0.5 N <sub>2</sub> → 4.311 YH <sub>3</sub> + YB <sub>6</sub> H <sub>4</sub> C <sub>6</sub> N                      | -3.5469             |
| YNH <sub>4</sub> B <sub>6</sub> C <sub>6</sub> | 0.3636 B <sub>9</sub> H <sub>11</sub> + 1.2 Y <sub>4</sub> C <sub>5</sub> + 0.5 N <sub>2</sub> + 17.93 B → 3.8 YB <sub>4</sub> + YB <sub>6</sub> H <sub>4</sub> C <sub>6</sub> N                        | -3.5426             |
| YNH <sub>4</sub> B <sub>6</sub> C <sub>6</sub> | 2 YH <sub>2</sub> + YN + 0.8571 Y <sub>4</sub> C <sub>7</sub> + 71.14 B → 5.429 YB <sub>12</sub> + YB <sub>6</sub> H <sub>4</sub> C <sub>6</sub> N                                                      | -3.5328             |
| YNH <sub>4</sub> B <sub>6</sub> C <sub>6</sub> | 1.678 B <sub>13</sub> C <sub>2</sub> + 2.644 Y <sub>2</sub> C + 1.333 H <sub>3</sub> N → 0.3333 YN + 3.954 YB <sub>4</sub> + YB <sub>6</sub> H <sub>4</sub> C <sub>6</sub> N                            | -3.5217             |
| YNH <sub>4</sub> B <sub>6</sub> C <sub>6</sub> | 26 YH <sub>3</sub> + 6 Y <sub>2</sub> C + H <sub>3</sub> N + 1.5 YB <sub>4</sub> → 38.5 YH <sub>2</sub> + YB <sub>6</sub> H <sub>4</sub> C <sub>6</sub> N                                               | -3.5124             |
| YNH <sub>4</sub> B <sub>6</sub> C <sub>6</sub> | 0.4615 B <sub>13</sub> C <sub>2</sub> + 1.015 Y <sub>4</sub> C <sub>5</sub> + 2.031 N <sub>2</sub> + 2 H <sub>2</sub> → 3.062 YN + YB <sub>6</sub> H <sub>4</sub> C <sub>6</sub> N                      | -3.4871             |
| YNH <sub>4</sub> B <sub>6</sub> C <sub>6</sub> | 6 Y <sub>2</sub> C + 2.7 YB <sub>12</sub> + 2 H <sub>2</sub> + BN → 13.7 YB <sub>2</sub> + YB <sub>6</sub> H <sub>4</sub> C <sub>6</sub> N                                                              | -3.4828             |
| YNH <sub>4</sub> B <sub>6</sub> C <sub>6</sub> | 1.333 YH <sub>3</sub> + 2.381 N <sub>2</sub> + 0.8571 Y <sub>4</sub> C <sub>7</sub> + 6 B → 3.762 YN + YB <sub>6</sub> H <sub>4</sub> C <sub>6</sub> N                                                  | -3.4775             |
| YNH <sub>4</sub> B <sub>6</sub> C <sub>6</sub> | 34 YH <sub>3</sub> + 6 Y <sub>2</sub> C + YN + 3 YB <sub>2</sub> → 49 YH <sub>2</sub> + YB <sub>6</sub> H <sub>4</sub> C <sub>6</sub> N                                                                 | -3.4643             |
| YNH <sub>4</sub> B <sub>6</sub> C <sub>6</sub> | 0.09091 B <sub>9</sub> H <sub>11</sub> + 1.696 B <sub>13</sub> C <sub>2</sub> + 2.608 Y <sub>2</sub> C + H <sub>3</sub> N → 4.216 YB <sub>4</sub> + YB <sub>6</sub> H <sub>4</sub> C <sub>6</sub> N     | -3.4438             |
| YNH <sub>4</sub> B <sub>6</sub> C <sub>6</sub> | 1.7 B <sub>13</sub> C <sub>2</sub> + 2.601 Y <sub>2</sub> C + H <sub>3</sub> N + 0.1429 B <sub>5</sub> H <sub>7</sub> → 4.202 YB <sub>4</sub> + YB <sub>6</sub> H <sub>4</sub> C <sub>6</sub> N         | -3.4191             |
| YNH <sub>4</sub> B <sub>6</sub> C <sub>6</sub> | 2 YH <sub>2</sub> + 1.2 Y <sub>4</sub> C <sub>5</sub> + BN + 28.2 B → 5.8 YB <sub>4</sub> + YB <sub>6</sub> H <sub>4</sub> C <sub>6</sub> N                                                             | -3.4086             |
| YNH <sub>4</sub> B <sub>6</sub> C <sub>6</sub> | 1.333 H <sub>3</sub> N + 1.2 Y <sub>4</sub> C <sub>5</sub> + 47.6 B → 3.467 YB <sub>12</sub> + 0.3333 YN + YB <sub>6</sub> H <sub>4</sub> C <sub>6</sub> N                                              | -3.4007             |
| YNH <sub>4</sub> B <sub>6</sub> C <sub>6</sub> | 19.31 YH <sub>3</sub> + 0.4615 B <sub>13</sub> C <sub>2</sub> + 5.077 Y <sub>2</sub> C + H <sub>3</sub> N → 28.46 YH <sub>2</sub> + YB <sub>6</sub> H <sub>4</sub> C <sub>6</sub> N                     | -3.3706             |
| YNH <sub>4</sub> B <sub>6</sub> C <sub>6</sub> | 29 YH <sub>3</sub> + 6 Y <sub>2</sub> C + 0.5 YB <sub>12</sub> + YN → 41.5 YH <sub>2</sub> + YB <sub>6</sub> H <sub>4</sub> C <sub>6</sub> N                                                            | -3.3263             |
| YNH <sub>4</sub> B <sub>6</sub> C <sub>6</sub> | 1.333 H <sub>3</sub> N + 1.2 Y <sub>4</sub> C <sub>5</sub> + 51.6 B → 3.8 YB <sub>12</sub> + 0.1667 N <sub>2</sub> + YB <sub>6</sub> H <sub>4</sub> C <sub>6</sub> N                                    | -3.3234             |
| YNH <sub>4</sub> B <sub>6</sub> C <sub>6</sub> | 1.333 YH <sub>3</sub> + 1.908 B <sub>13</sub> C <sub>2</sub> + 2.184 Y <sub>2</sub> C + 0.5 N <sub>2</sub> → 4.701 YB <sub>4</sub> + YB <sub>6</sub> H <sub>4</sub> C <sub>6</sub> N                    | -3.3218             |
| YNH <sub>4</sub> B <sub>6</sub> C <sub>6</sub> | 0.5 YH <sub>2</sub> + H <sub>3</sub> N + 1.2 Y <sub>4</sub> C <sub>5</sub> + 23.2 B → 4.3 YB <sub>4</sub> + YB <sub>6</sub> H <sub>4</sub> C <sub>6</sub> N                                             | -3.3213             |
| YNH <sub>4</sub> B <sub>6</sub> C <sub>6</sub> | 0.6667 B <sub>9</sub> H <sub>11</sub> + 6 Y <sub>2</sub> C + 9.889 H <sub>3</sub> N → 11 YH <sub>3</sub> + 4.444 N <sub>2</sub> + YB <sub>6</sub> H <sub>4</sub> C <sub>6</sub> N                       | -3.3133             |
| YNH <sub>4</sub> B <sub>6</sub> C <sub>6</sub> | 6 Y <sub>2</sub> C + 2.414 YB <sub>12</sub> + 0.5714 B <sub>5</sub> H <sub>7</sub> + BN → 13.41 YB <sub>2</sub> + YB <sub>6</sub> H <sub>4</sub> C <sub>6</sub> N                                       | -3.3128             |
| YNH <sub>4</sub> B <sub>6</sub> C <sub>6</sub> | 0.3636 B <sub>9</sub> H <sub>11</sub> + 6 Y <sub>2</sub> C + 2.373 YB <sub>12</sub> + BN → 13.37 YB <sub>2</sub> + YB <sub>6</sub> H <sub>4</sub> C <sub>6</sub> N                                      | -3.3126             |
| YNH <sub>4</sub> B <sub>6</sub> C <sub>6</sub> | 21.12 B <sub>9</sub> H <sub>11</sub> + 6 Y <sub>2</sub> C + BN → 32.62 B <sub>5</sub> H <sub>7</sub> + 11 YB <sub>2</sub> + YB <sub>6</sub> H <sub>4</sub> C <sub>6</sub> N                             | -3.3049             |
| YNH <sub>4</sub> B <sub>6</sub> C <sub>6</sub> | 0.6667 B <sub>9</sub> H <sub>11</sub> + 6.467 Y + 1.2 H <sub>8</sub> C <sub>5</sub> + YN → 6.467 YH <sub>2</sub> + YB <sub>6</sub> H <sub>4</sub> C <sub>6</sub> N                                      | -3.3006             |

Continued on next page

Continued

| Compound                                       | Chemical reaction                                                                                                                                                                       | Reaction energy(eV) |
|------------------------------------------------|-----------------------------------------------------------------------------------------------------------------------------------------------------------------------------------------|---------------------|
| YNH <sub>4</sub> B <sub>6</sub> C <sub>6</sub> | $2\text{YH}_2 + 2\text{B}_{13}\text{C}_2 + 2\text{Y}_2\text{C} + 0.5\text{N}_2 \rightarrow 5\text{YB}_4 + \text{YB}_6\text{H}_4\text{C}_6\text{N}$                                      | -3.2935             |
| YNH <sub>4</sub> B <sub>6</sub> C <sub>6</sub> | $1.333\text{H}_3\text{N} + 1.2\text{Y}_4\text{C}_5 + 21.53\text{B} \rightarrow 0.3333\text{BN} + 3.8\text{YB}_4 + \text{YB}_6\text{H}_4\text{C}_6\text{N}$                              | -3.2922             |
| YNH <sub>4</sub> B <sub>6</sub> C <sub>6</sub> | $1.724\text{B}_{13}\text{C}_2 + 2.552\text{Y}_2\text{C} + \text{H}_3\text{N} + 0.5\text{H}_2 \rightarrow 4.103\text{YB}_4 + \text{YB}_6\text{H}_4\text{C}_6\text{N}$                    | -3.2920             |
| YNH <sub>4</sub> B <sub>6</sub> C <sub>6</sub> | $117.4\text{B}_9\text{H}_{11} + 6\text{Y}_2\text{C} + \text{BN} \rightarrow 11\text{YB}_{12} + 183.9\text{B}_5\text{H}_7 + \text{YB}_6\text{H}_4\text{C}_6\text{N}$                     | -3.2692             |
| YNH <sub>4</sub> B <sub>6</sub> C <sub>6</sub> | $0.3636\text{B}_9\text{H}_{11} + 1.749\text{B}_{13}\text{C}_2 + 2.502\text{Y}_2\text{C} + \text{YN} \rightarrow 5.003\text{YB}_4 + \text{YB}_6\text{H}_4\text{C}_6\text{N}$             | -3.2100             |
| YNH <sub>4</sub> B <sub>6</sub> C <sub>6</sub> | $2.125\text{B}_{13}\text{C}_2 + 7.497\text{H}_3\text{N} + 0.25\text{Y}_4\text{C}_7 \rightarrow 1.681\text{B}_9\text{H}_{11} + 6.497\text{BN} + \text{YB}_6\text{H}_4\text{C}_6\text{N}$ | -3.2045             |
| YNH <sub>4</sub> B <sub>6</sub> C <sub>6</sub> | $1.2\text{Y}_4\text{C}_5 + 2.72\text{B}_5\text{H}_7 + 3.007\text{N}_2 \rightarrow 5.013\text{H}_3\text{N} + 3.8\text{YB}_2 + \text{YB}_6\text{H}_4\text{C}_6\text{N}$                   | -3.2030             |
| YNH <sub>4</sub> B <sub>6</sub> C <sub>6</sub> | $1.2\text{Y}_4\text{C}_5 + 1.2\text{B}_5\text{H}_7 + 1.667\text{N}_2 \rightarrow 1.467\text{YH}_3 + 2.333\text{YN} + \text{YB}_6\text{H}_4\text{C}_6\text{N}$                           | -3.1869             |
| YNH <sub>4</sub> B <sub>6</sub> C <sub>6</sub> | $1.612\text{B}_5\text{H}_7 + 1.531\text{N}_2 + 0.8571\text{Y}_4\text{C}_7 \rightarrow 2.429\text{YH}_3 + 2.061\text{BN} + \text{YB}_6\text{H}_4\text{C}_6\text{N}$                      | -3.1618             |
| YNH <sub>4</sub> B <sub>6</sub> C <sub>6</sub> | $1.2\text{Y}_4\text{C}_5 + 0.5714\text{B}_5\text{H}_7 + \text{YN} + 22.34\text{B} \rightarrow 4.8\text{YB}_4 + \text{YB}_6\text{H}_4\text{C}_6\text{N}$                                 | -3.1396             |
| YNH <sub>4</sub> B <sub>6</sub> C <sub>6</sub> | $5.375\text{Y}_2\text{C} + \text{H}_3\text{N} + 2.55\text{YB}_{12} + 0.125\text{H}_8\text{C}_5 \rightarrow 12.3\text{YB}_2 + \text{YB}_6\text{H}_4\text{C}_6\text{N}$                   | -3.1266             |
| YNH <sub>4</sub> B <sub>6</sub> C <sub>6</sub> | $3.111\text{B}_9\text{H}_{11} + 6\text{Y}_2\text{C} + \text{H}_3\text{N} \rightarrow 16.61\text{H}_2 + 11\text{YB}_2 + \text{YB}_6\text{H}_4\text{C}_6\text{N}$                         | -3.1204             |
| YNH <sub>4</sub> B <sub>6</sub> C <sub>6</sub> | $1.764\text{B}_{13}\text{C}_2 + 2.473\text{Y}_2\text{C} + 0.5714\text{B}_5\text{H}_7 + \text{YN} \rightarrow 4.946\text{YB}_4 + \text{YB}_6\text{H}_4\text{C}_6\text{N}$                | -3.1115             |
| YNH <sub>4</sub> B <sub>6</sub> C <sub>6</sub> | $0.5556\text{B}_9\text{H}_{11} + 6.856\text{Y} + 1.2\text{H}_8\text{C}_5 + \text{BN} \rightarrow 5.856\text{YH}_2 + \text{YB}_6\text{H}_4\text{C}_6\text{N}$                            | -3.1082             |
| YNH <sub>4</sub> B <sub>6</sub> C <sub>6</sub> | $0.3636\text{B}_9\text{H}_{11} + 1.2\text{Y}_4\text{C}_5 + \text{YN} + 21.93\text{B} \rightarrow 4.8\text{YB}_4 + \text{YB}_6\text{H}_4\text{C}_6\text{N}$                              | -3.0774             |
| YNH <sub>4</sub> B <sub>6</sub> C <sub>6</sub> | $3.867\text{H}_3\text{N} + 1.2\text{Y}_4\text{C}_5 + 8.867\text{B} \rightarrow 3.8\text{YH}_2 + 2.867\text{BN} + \text{YB}_6\text{H}_4\text{C}_6\text{N}$                               | -3.0710             |
| YNH <sub>4</sub> B <sub>6</sub> C <sub>6</sub> | $0.3333\text{YH}_3 + \text{H}_3\text{N} + 1.2\text{Y}_4\text{C}_5 + 22.53\text{B} \rightarrow 4.133\text{YB}_4 + \text{YB}_6\text{H}_4\text{C}_6\text{N}$                               | -3.0703             |
| YNH <sub>4</sub> B <sub>6</sub> C <sub>6</sub> | $1.2\text{Y}_4\text{C}_5 + 2.293\text{YB}_{12} + 0.5714\text{B}_5\text{H}_7 + 0.5\text{N}_2 \rightarrow 6.093\text{YB}_4 + \text{YB}_6\text{H}_4\text{C}_6\text{N}$                     | -3.0697             |
| YNH <sub>4</sub> B <sub>6</sub> C <sub>6</sub> | $0.3636\text{B}_9\text{H}_{11} + 1.577\text{B}_{13}\text{C}_2 + 2.846\text{Y}_2\text{C} + \text{BN} \rightarrow 4.693\text{YB}_4 + \text{YB}_6\text{H}_4\text{C}_6\text{N}$             | -3.0434             |
| YNH <sub>4</sub> B <sub>6</sub> C <sub>6</sub> | $6\text{C} + 5.667\text{H}_3\text{N} + 5.333\text{YB}_2 \rightarrow 4.333\text{YH}_3 + 4.667\text{BN} + \text{YB}_6\text{H}_4\text{C}_6\text{N}$                                        | -3.0277             |
| YNH <sub>4</sub> B <sub>6</sub> C <sub>6</sub> | $1.2\text{Y}_4\text{C}_5 + \text{YN} + 13.7\text{H}_2 + 3\text{YB}_2 \rightarrow 7.8\text{YH}_3 + \text{YB}_6\text{H}_4\text{C}_6\text{N}$                                              | -3.0196             |
| YNH <sub>4</sub> B <sub>6</sub> C <sub>6</sub> | $0.3636\text{B}_9\text{H}_{11} + 1.2\text{Y}_4\text{C}_5 + 2.241\text{YB}_{12} + 0.5\text{N}_2 \rightarrow 6.041\text{YB}_4 + \text{YB}_6\text{H}_4\text{C}_6\text{N}$                  | -3.0196             |
| YNH <sub>4</sub> B <sub>6</sub> C <sub>6</sub> | $1.2\text{Y}_4\text{C}_5 + 3.15\text{YB}_{12} + \text{YN} + 2\text{H}_2 \rightarrow 7.95\text{YB}_4 + \text{YB}_6\text{H}_4\text{C}_6\text{N}$                                          | -3.0016             |
| YNH <sub>4</sub> B <sub>6</sub> C <sub>6</sub> | $31\text{YH}_3 + 6\text{Y}_2\text{C} + \text{BN} + 2.5\text{YB}_2 \rightarrow 44.5\text{YH}_2 + \text{YB}_6\text{H}_4\text{C}_6\text{N}$                                                | -2.9902             |
| YNH <sub>4</sub> B <sub>6</sub> C <sub>6</sub> | $23.75\text{YH}_2 + 3\text{B}_{13}\text{C}_2 + 0.5\text{N}_2 \rightarrow 14.5\text{YH}_3 + 8.25\text{YB}_4 + \text{YB}_6\text{H}_4\text{C}_6\text{N}$                                   | -2.9862             |
| YNH <sub>4</sub> B <sub>6</sub> C <sub>6</sub> | $0.3333\text{YH}_3 + 1.77\text{B}_{13}\text{C}_2 + 2.46\text{Y}_2\text{C} + \text{H}_3\text{N} \rightarrow 4.253\text{YB}_4 + \text{YB}_6\text{H}_4\text{C}_6\text{N}$                  | -2.9684             |
| YNH <sub>4</sub> B <sub>6</sub> C <sub>6</sub> | $0.5\text{YH}_2 + 1.793\text{B}_{13}\text{C}_2 + 2.414\text{Y}_2\text{C} + \text{H}_3\text{N} \rightarrow 4.328\text{YB}_4 + \text{YB}_6\text{H}_4\text{C}_6\text{N}$                   | -2.9614             |
| YNH <sub>4</sub> B <sub>6</sub> C <sub>6</sub> | $1.591\text{B}_{13}\text{C}_2 + 2.818\text{Y}_2\text{C} + 0.5714\text{B}_5\text{H}_7 + \text{BN} \rightarrow 4.635\text{YB}_4 + \text{YB}_6\text{H}_4\text{C}_6\text{N}$                | -2.9448             |
| YNH <sub>4</sub> B <sub>6</sub> C <sub>6</sub> | $5.64\text{H}_3\text{N} + 1.2\text{Y}_4\text{C}_5 + 2.66\text{YB}_4 \rightarrow 6.46\text{YH}_2 + 4.64\text{BN} + \text{YB}_6\text{H}_4\text{C}_6\text{N}$                              | -2.9162             |
| YNH <sub>4</sub> B <sub>6</sub> C <sub>6</sub> | $6\text{Y}_2\text{C} + \text{H}_3\text{N} + 5.6\text{B}_5\text{H}_7 \rightarrow 19.1\text{H}_2 + 11\text{YB}_2 + \text{YB}_6\text{H}_4\text{C}_6\text{N}$                               | -2.9101             |
| YNH <sub>4</sub> B <sub>6</sub> C <sub>6</sub> | $2\text{YH}_2 + 0.4615\text{B}_{13}\text{C}_2 + 2.451\text{N}_2 + 0.7253\text{Y}_4\text{C}_7 \rightarrow 3.901\text{YN} + \text{YB}_6\text{H}_4\text{C}_6\text{N}$                      | -2.9059             |
| YNH <sub>4</sub> B <sub>6</sub> C <sub>6</sub> | $\text{H}_3\text{N} + 1.2\text{Y}_4\text{C}_5 + 0.5\text{H}_2 + 21.2\text{B} \rightarrow 3.8\text{YB}_4 + \text{YB}_6\text{H}_4\text{C}_6\text{N}$                                      | -2.8779             |
| YNH <sub>4</sub> B <sub>6</sub> C <sub>6</sub> | $26.83\text{YH}_3 + 6\text{Y}_2\text{C} + 0.4167\text{YB}_{12} + \text{BN} \rightarrow 38.25\text{YH}_2 + \text{YB}_6\text{H}_4\text{C}_6\text{N}$                                      | -2.8752             |
| YNH <sub>4</sub> B <sub>6</sub> C <sub>6</sub> | $1.724\text{B}_{13}\text{C}_2 + 2.552\text{Y}_2\text{C} + 1.333\text{H}_3\text{N} \rightarrow 0.1667\text{N}_2 + 4.103\text{YB}_4 + \text{YB}_6\text{H}_4\text{C}_6\text{N}$            | -2.8507             |
| YNH <sub>4</sub> B <sub>6</sub> C <sub>6</sub> | $4.388\text{H}_3\text{N} + 1.2\text{Y}_4\text{C}_5 + 0.7824\text{YB}_{12} \rightarrow 4.582\text{YH}_2 + 3.388\text{BN} + \text{YB}_6\text{H}_4\text{C}_6\text{N}$                      | -2.8429             |
| YNH <sub>4</sub> B <sub>6</sub> C <sub>6</sub> | $1.75\text{B}_{13}\text{C}_2 + 4.188\text{Y} + 0.5\text{H}_8\text{C}_5 + \text{YN} \rightarrow 4.188\text{YB}_4 + \text{YB}_6\text{H}_4\text{C}_6\text{N}$                              | -2.8130             |
| YNH <sub>4</sub> B <sub>6</sub> C <sub>6</sub> | $3.5\text{Y}_2\text{C} + 0.5\text{H}_8\text{C}_5 + 0.5\text{N}_2 + 18\text{B} \rightarrow 6\text{YB}_2 + \text{YB}_6\text{H}_4\text{C}_6\text{N}$                                       | -2.7937             |
| YNH <sub>4</sub> B <sub>6</sub> C <sub>6</sub> | $2.464\text{N}_2 + 0.8571\text{Y}_4\text{C}_7 + 2\text{H}_2 + 1.5\text{YB}_4 \rightarrow 3.929\text{YN} + \text{YB}_6\text{H}_4\text{C}_6\text{N}$                                      | -2.7854             |
| YNH <sub>4</sub> B <sub>6</sub> C <sub>6</sub> | $1.2\text{B}_5\text{H}_7 + 2.448\text{N}_2 + 0.8571\text{Y}_4\text{C}_7 \rightarrow 1.467\text{H}_3\text{N} + 2.429\text{YN} + \text{YB}_6\text{H}_4\text{C}_6\text{N}$                 | -2.7755             |
| YNH <sub>4</sub> B <sub>6</sub> C <sub>6</sub> | $\text{H}_3\text{N} + 1.2\text{Y}_4\text{C}_5 + 10.7\text{H}_2 + 3\text{YB}_2 \rightarrow 6.8\text{YH}_3 + \text{YB}_6\text{H}_4\text{C}_6\text{N}$                                     | -2.7380             |
| YNH <sub>4</sub> B <sub>6</sub> C <sub>6</sub> | $6\text{Y}_2\text{C} + 8.667\text{H}_3\text{N} + 6\text{B} \rightarrow 11\text{YH}_2 + 3.833\text{N}_2 + \text{YB}_6\text{H}_4\text{C}_6\text{N}$                                       | -2.7367             |
| YNH <sub>4</sub> B <sub>6</sub> C <sub>6</sub> | $2\text{YH}_2 + 0.5\text{N}_2 + 0.8571\text{Y}_4\text{C}_7 + 23.71\text{B} \rightarrow 4.429\text{YB}_4 + \text{YB}_6\text{H}_4\text{C}_6\text{N}$                                      | -2.7311             |
| YNH <sub>4</sub> B <sub>6</sub> C <sub>6</sub> | $\text{H}_3\text{N} + 1.2\text{Y}_4\text{C}_5 + 0.1429\text{B}_5\text{H}_7 + 20.49\text{B} \rightarrow 3.8\text{YB}_4 + \text{YB}_6\text{H}_4\text{C}_6\text{N}$                        | -2.7286             |
| YNH <sub>4</sub> B <sub>6</sub> C <sub>6</sub> | $0.09091\text{B}_9\text{H}_{11} + \text{H}_3\text{N} + 1.2\text{Y}_4\text{C}_5 + 20.38\text{B} \rightarrow 3.8\text{YB}_4 + \text{YB}_6\text{H}_4\text{C}_6\text{N}$                    | -2.7131             |
| YNH <sub>4</sub> B <sub>6</sub> C <sub>6</sub> | $1.333\text{H}_3\text{N} + 1.2\text{Y}_4\text{C}_5 + 2.692\text{YB}_{12} \rightarrow 0.3333\text{BN} + 6.492\text{YB}_4 + \text{YB}_6\text{H}_4\text{C}_6\text{N}$                      | -2.6640             |
| YNH <sub>4</sub> B <sub>6</sub> C <sub>6</sub> | $0.5\text{YH}_2 + \text{H}_3\text{N} + 1.2\text{Y}_4\text{C}_5 + 2.9\text{YB}_{12} \rightarrow 7.2\text{YB}_4 + \text{YB}_6\text{H}_4\text{C}_6\text{N}$                                | -2.6445             |
| YNH <sub>4</sub> B <sub>6</sub> C <sub>6</sub> | $1.333\text{YH}_3 + 0.5\text{N}_2 + 0.8571\text{Y}_4\text{C}_7 + 51.14\text{B} \rightarrow 3.762\text{YB}_{12} + \text{YB}_6\text{H}_4\text{C}_6\text{N}$                               | -2.6054             |
| YNH <sub>4</sub> B <sub>6</sub> C <sub>6</sub> | $1.862\text{B}_{13}\text{C}_2 + 2.276\text{Y}_2\text{C} + \text{YN} + 2\text{H}_2 \rightarrow 4.552\text{YB}_4 + \text{YB}_6\text{H}_4\text{C}_6\text{N}$                               | -2.6029             |
| YNH <sub>4</sub> B <sub>6</sub> C <sub>6</sub> | $1.333\text{H}_3\text{N} + 1.2\text{Y}_4\text{C}_5 + 19.87\text{B} \rightarrow 0.3333\text{YN} + 3.467\text{YB}_4 + \text{YB}_6\text{H}_4\text{C}_6\text{N}$                            | -2.5916             |
| YNH <sub>4</sub> B <sub>6</sub> C <sub>6</sub> | $26.75\text{YH}_2 + 3\text{B}_{13}\text{C}_2 + \text{H}_3\text{N} \rightarrow 17.5\text{YH}_3 + 8.25\text{YB}_4 + \text{YB}_6\text{H}_4\text{C}_6\text{N}$                              | -2.5905             |
| YNH <sub>4</sub> B <sub>6</sub> C <sub>6</sub> | $0.5\text{H}_8\text{C}_5 + 2.5\text{N}_2 + 0.5\text{Y}_4\text{C}_7 + 3\text{YB}_2 \rightarrow 4\text{YN} + \text{YB}_6\text{H}_4\text{C}_6\text{N}$                                     | -2.5890             |
| YNH <sub>4</sub> B <sub>6</sub> C <sub>6</sub> | $2\text{YH}_2 + 1.2\text{Y}_4\text{C}_5 + 3.525\text{YB}_{12} + \text{BN} \rightarrow 9.325\text{YB}_4 + \text{YB}_6\text{H}_4\text{C}_6\text{N}$                                       | -2.5859             |
| YNH <sub>4</sub> B <sub>6</sub> C <sub>6</sub> | $1.333\text{YH}_3 + 6\text{Y}_2\text{C} + 3.267\text{YB}_{12} + \text{YN} \rightarrow 16.6\text{YB}_2 + \text{YB}_6\text{H}_4\text{C}_6\text{N}$                                        | -2.5627             |
| YNH <sub>4</sub> B <sub>6</sub> C <sub>6</sub> | $6\text{C} + 4.7\text{Y} + \text{H}_3\text{N} + 1.2\text{B}_5\text{H}_7 \rightarrow 3.7\text{YH}_2 + \text{YB}_6\text{H}_4\text{C}_6\text{N}$                                           | -2.5558             |
| YNH <sub>4</sub> B <sub>6</sub> C <sub>6</sub> | $2\text{YH}_2 + 6\text{Y}_2\text{C} + 3.4\text{YB}_{12} + \text{YN} \rightarrow 17.4\text{YB}_2 + \text{YB}_6\text{H}_4\text{C}_6\text{N}$                                              | -2.5259             |
| YNH <sub>4</sub> B <sub>6</sub> C <sub>6</sub> | $1.2\text{Y}_4\text{C}_5 + 2\text{H}_2 + \text{BN} + 50.6\text{B} \rightarrow 3.8\text{YB}_{12} + \text{YB}_6\text{H}_4\text{C}_6\text{N}$                                              | -2.5221             |
| YNH <sub>4</sub> B <sub>6</sub> C <sub>6</sub> | $0.6667\text{B}_9\text{H}_{11} + 1.2\text{Y}_4\text{C}_5 + 1.567\text{N}_2 \rightarrow 1.667\text{YH}_2 + 2.133\text{YN} + \text{YB}_6\text{H}_4\text{C}_6\text{N}$                     | -2.5077             |
| YNH <sub>4</sub> B <sub>6</sub> C <sub>6</sub> | $1.2\text{Y}_4\text{C}_5 + 2.793\text{YB}_{12} + 0.5714\text{B}_5\text{H}_7 + \text{YN} \rightarrow 7.593\text{YB}_4 + \text{YB}_6\text{H}_4\text{C}_6\text{N}$                         | -2.4878             |
| YNH <sub>4</sub> B <sub>6</sub> C <sub>6</sub> | $6\text{Y}_2\text{C} + 2.818\text{H}_3\text{N} + 9.182\text{BN} \rightarrow 0.6364\text{B}_5\text{H}_7 + 11\text{YN} + \text{YB}_6\text{H}_4\text{C}_6\text{N}$                         | -2.4485             |
| YNH <sub>4</sub> B <sub>6</sub> C <sub>6</sub> | $0.3636\text{B}_9\text{H}_{11} + 1.2\text{Y}_4\text{C}_5 + 2.741\text{YB}_{12} + \text{YN} \rightarrow 7.541\text{YB}_4 + \text{YB}_6\text{H}_4\text{C}_6\text{N}$                      | -2.4377             |

Continued on next page

Continued

| Compound                                       | Chemical reaction                                                                                                                                                                                   | Reaction energy(eV) |
|------------------------------------------------|-----------------------------------------------------------------------------------------------------------------------------------------------------------------------------------------------------|---------------------|
| YNH <sub>4</sub> B <sub>6</sub> C <sub>6</sub> | 1.333 H <sub>3</sub> N + 1.2 Y <sub>4</sub> C <sub>5</sub> + 21.2 B → 0.1667 N <sub>2</sub> + 3.8 YB <sub>4</sub> + YB <sub>6</sub> H <sub>4</sub> C <sub>6</sub> N                                 | -2.4366             |
| YNH <sub>4</sub> B <sub>6</sub> C <sub>6</sub> | 1.69 B <sub>13</sub> C <sub>2</sub> + 2.621 Y <sub>2</sub> C + 2 H <sub>2</sub> + BN → 4.241 YB <sub>4</sub> + YB <sub>6</sub> H <sub>4</sub> C <sub>6</sub> N                                      | -2.4363             |
| YNH <sub>4</sub> B <sub>6</sub> C <sub>6</sub> | 0.3333 YH <sub>3</sub> + H <sub>3</sub> N + 1.2 Y <sub>4</sub> C <sub>5</sub> + 2.817 YB <sub>12</sub> → 6.95 YB <sub>4</sub> + YB <sub>6</sub> H <sub>4</sub> C <sub>6</sub> N                     | -2.4130             |
| YNH <sub>4</sub> B <sub>6</sub> C <sub>6</sub> | 1.333 YH <sub>3</sub> + 1.2 Y <sub>4</sub> C <sub>5</sub> + BN + 25.53 B → 5.133 YB <sub>4</sub> + YB <sub>6</sub> H <sub>4</sub> C <sub>6</sub> N                                                  | -2.4049             |
| YNH <sub>4</sub> B <sub>6</sub> C <sub>6</sub> | 0.3636 B <sub>9</sub> H <sub>11</sub> + 3 B <sub>13</sub> C <sub>2</sub> + 4.023 Y + 0.5 N <sub>2</sub> → 3.023 YB <sub>12</sub> + YB <sub>6</sub> H <sub>4</sub> C <sub>6</sub> N                  | -2.4033             |
| YNH <sub>4</sub> B <sub>6</sub> C <sub>6</sub> | 1.333 YH <sub>3</sub> + YN + 0.8571 Y <sub>4</sub> C <sub>7</sub> + 63.14 B → 4.762 YB <sub>12</sub> + YB <sub>6</sub> H <sub>4</sub> C <sub>6</sub> N                                              | -2.3735             |
| YNH <sub>4</sub> B <sub>6</sub> C <sub>6</sub> | 3 B <sub>13</sub> C <sub>2</sub> + 3.988 Y + 0.5714 B <sub>5</sub> H <sub>7</sub> + 0.5 N <sub>2</sub> → 2.988 YB <sub>12</sub> + YB <sub>6</sub> H <sub>4</sub> C <sub>6</sub> N                   | -2.3537             |
| YNH <sub>4</sub> B <sub>6</sub> C <sub>6</sub> | 0.6667 B <sub>9</sub> H <sub>11</sub> + 2.27 N <sub>2</sub> + 0.8571 Y <sub>4</sub> C <sub>7</sub> → 1.111 H <sub>3</sub> N + 2.429 YN + YB <sub>6</sub> H <sub>4</sub> C <sub>6</sub> N            | -2.3498             |
| YNH <sub>4</sub> B <sub>6</sub> C <sub>6</sub> | 3.333 B <sub>9</sub> H <sub>11</sub> + 6 Y <sub>2</sub> C + YN → 16.33 H <sub>2</sub> + 12 YB <sub>2</sub> + YB <sub>6</sub> H <sub>4</sub> C <sub>6</sub> N                                        | -2.3146             |
| YNH <sub>4</sub> B <sub>6</sub> C <sub>6</sub> | H <sub>3</sub> N + 1.075 Y <sub>4</sub> C <sub>5</sub> + 0.125 H <sub>8</sub> C <sub>5</sub> + 45.6 B → 3.3 YB <sub>12</sub> + YB <sub>6</sub> H <sub>4</sub> C <sub>6</sub> N                      | -2.3065             |
| YNH <sub>4</sub> B <sub>6</sub> C <sub>6</sub> | 6 Y <sub>2</sub> C + 2.684 H <sub>3</sub> N + 9.316 BN → 0.3684 B <sub>9</sub> H <sub>11</sub> + 11 YN + YB <sub>6</sub> H <sub>4</sub> C <sub>6</sub> N                                            | -2.2851             |
| YNH <sub>4</sub> B <sub>6</sub> C <sub>6</sub> | 2 YH <sub>2</sub> + YN + 0.8571 Y <sub>4</sub> C <sub>7</sub> + 27.71 B → 5.429 YB <sub>4</sub> + YB <sub>6</sub> H <sub>4</sub> C <sub>6</sub> N                                                   | -2.2659             |
| YNH <sub>4</sub> B <sub>6</sub> C <sub>6</sub> | H <sub>3</sub> N + 1.2 Y <sub>4</sub> C <sub>5</sub> + 2.65 YB <sub>12</sub> + 0.5 H <sub>2</sub> → 6.45 YB <sub>4</sub> + YB <sub>6</sub> H <sub>4</sub> C <sub>6</sub> N                          | -2.2595             |
| YNH <sub>4</sub> B <sub>6</sub> C <sub>6</sub> | 1.511 B <sub>9</sub> H <sub>11</sub> + 1.2 Y <sub>4</sub> C <sub>5</sub> + 2.604 N <sub>2</sub> → 4.207 H <sub>3</sub> N + 3.8 YB <sub>2</sub> + YB <sub>6</sub> H <sub>4</sub> C <sub>6</sub> N    | -2.2381             |
| YNH <sub>4</sub> B <sub>6</sub> C <sub>6</sub> | 1.333 YH <sub>3</sub> + 3 B <sub>13</sub> C <sub>2</sub> + 6.533 YN → 5.533 BN + 6.867 YB <sub>4</sub> + YB <sub>6</sub> H <sub>4</sub> C <sub>6</sub> N                                            | -2.2307             |
| YNH <sub>4</sub> B <sub>6</sub> C <sub>6</sub> | 6 Y <sub>2</sub> C + 18.5 H <sub>2</sub> + 6 BN → 11 YH <sub>3</sub> + 2.5 N <sub>2</sub> + YB <sub>6</sub> H <sub>4</sub> C <sub>6</sub> N                                                         | -2.2152             |
| YNH <sub>4</sub> B <sub>6</sub> C <sub>6</sub> | 0.5 YB <sub>12</sub> + 1.964 N <sub>2</sub> + 0.8571 Y <sub>4</sub> C <sub>7</sub> + 2 H <sub>2</sub> → 2.929 YN + YB <sub>6</sub> H <sub>4</sub> C <sub>6</sub> N                                  | -2.2035             |
| YNH <sub>4</sub> B <sub>6</sub> C <sub>6</sub> | 3 B <sub>13</sub> C <sub>2</sub> + 3.75 Y + 0.5 N <sub>2</sub> + 2 H <sub>2</sub> → 2.75 YB <sub>12</sub> + YB <sub>6</sub> H <sub>4</sub> C <sub>6</sub> N                                         | -2.1815             |
| YNH <sub>4</sub> B <sub>6</sub> C <sub>6</sub> | 1.333 YH <sub>3</sub> + 6 Y <sub>2</sub> C + 2.967 YB <sub>12</sub> + BN → 15.3 YB <sub>2</sub> + YB <sub>6</sub> H <sub>4</sub> C <sub>6</sub> N                                                   | -2.1714             |
| YNH <sub>4</sub> B <sub>6</sub> C <sub>6</sub> | 0.3636 B <sub>9</sub> H <sub>11</sub> + 1.177 B <sub>13</sub> C <sub>2</sub> + 3.645 Y <sub>2</sub> C + 0.5 N <sub>2</sub> → 6.29 YB <sub>2</sub> + YB <sub>6</sub> H <sub>4</sub> C <sub>6</sub> N | -2.1551             |
| YNH <sub>4</sub> B <sub>6</sub> C <sub>6</sub> | 8.8 Y + 1.2 H <sub>8</sub> C <sub>5</sub> + 6 BN → 2.8 YH <sub>2</sub> + 5 YN + YB <sub>6</sub> H <sub>4</sub> C <sub>6</sub> N                                                                     | -2.1463             |
| YNH <sub>4</sub> B <sub>6</sub> C <sub>6</sub> | 2 YH <sub>2</sub> + 6 Y <sub>2</sub> C + 3.1 YB <sub>12</sub> + BN → 16.1 YB <sub>2</sub> + YB <sub>6</sub> H <sub>4</sub> C <sub>6</sub> N                                                         | -2.1346             |
| YNH <sub>4</sub> B <sub>6</sub> C <sub>6</sub> | H <sub>3</sub> N + 1.2 Y <sub>4</sub> C <sub>5</sub> + 2.561 YB <sub>12</sub> + 0.1429 B <sub>5</sub> H <sub>7</sub> → 6.361 YB <sub>4</sub> + YB <sub>6</sub> H <sub>4</sub> C <sub>6</sub> N      | -2.1310             |
| YNH <sub>4</sub> B <sub>6</sub> C <sub>6</sub> | 0.09091 B <sub>9</sub> H <sub>11</sub> + H <sub>3</sub> N + 1.2 Y <sub>4</sub> C <sub>5</sub> + 2.548 YB <sub>12</sub> → 6.348 YB <sub>4</sub> + YB <sub>6</sub> H <sub>4</sub> C <sub>6</sub> N    | -2.1185             |
| YNH <sub>4</sub> B <sub>6</sub> C <sub>6</sub> | 2 YH <sub>2</sub> + 3 B <sub>13</sub> C <sub>2</sub> + 6 YN → 5 BN + 7 YB <sub>4</sub> + YB <sub>6</sub> H <sub>4</sub> C <sub>6</sub> N                                                            | -2.1136             |
| YNH <sub>4</sub> B <sub>6</sub> C <sub>6</sub> | 1.197 B <sub>13</sub> C <sub>2</sub> + 3.605 Y <sub>2</sub> C + 0.5714 B <sub>5</sub> H <sub>7</sub> + 0.5 N <sub>2</sub> → 6.211 YB <sub>2</sub> + YB <sub>6</sub> H <sub>4</sub> C <sub>6</sub> N | -2.0952             |
| YNH <sub>4</sub> B <sub>6</sub> C <sub>6</sub> | 6 C + 7.333 Y + 1.333 H <sub>3</sub> N + 6 BN → 6.333 YN + YB <sub>6</sub> H <sub>4</sub> C <sub>6</sub> N                                                                                          | -2.0892             |
| YNH <sub>4</sub> B <sub>6</sub> C <sub>6</sub> | 6 Y <sub>2</sub> C + 6 B <sub>5</sub> H <sub>7</sub> + YN → 19 H <sub>2</sub> + 12 YB <sub>2</sub> + YB <sub>6</sub> H <sub>4</sub> C <sub>6</sub> N                                                | -2.0892             |
| YNH <sub>4</sub> B <sub>6</sub> C <sub>6</sub> | 1.714 N <sub>2</sub> + 0.8571 Y <sub>4</sub> C <sub>7</sub> + 2 H <sub>2</sub> + 6 B → 2.429 YN + YB <sub>6</sub> H <sub>4</sub> C <sub>6</sub> N                                                   | -2.0876             |
| YNH <sub>4</sub> B <sub>6</sub> C <sub>6</sub> | 3 B <sub>9</sub> H <sub>11</sub> + 6 Y <sub>2</sub> C + BN → 14.5 H <sub>2</sub> + 11 YB <sub>2</sub> + YB <sub>6</sub> H <sub>4</sub> C <sub>6</sub> N                                             | -2.0792             |
| YNH <sub>4</sub> B <sub>6</sub> C <sub>6</sub> | 5.3 Y + H <sub>3</sub> N + 1.2 H <sub>8</sub> C <sub>5</sub> + 6 B → 4.3 YH <sub>2</sub> + YB <sub>6</sub> H <sub>4</sub> C <sub>6</sub> N                                                          | -2.0743             |
| YNH <sub>4</sub> B <sub>6</sub> C <sub>6</sub> | 3.393 Y <sub>2</sub> C + H <sub>3</sub> N + 0.5214 H <sub>8</sub> C <sub>5</sub> + 1.2 B <sub>5</sub> H <sub>7</sub> → 5.786 YH <sub>2</sub> + YB <sub>6</sub> H <sub>4</sub> C <sub>6</sub> N      | -2.0731             |
| YNH <sub>4</sub> B <sub>6</sub> C <sub>6</sub> | 2 YH <sub>2</sub> + 2.964 YB <sub>12</sub> + 0.5 N <sub>2</sub> + 0.8571 Y <sub>4</sub> C <sub>7</sub> → 7.393 YB <sub>4</sub> + YB <sub>6</sub> H <sub>4</sub> C <sub>6</sub> N                    | -2.0393             |
| YNH <sub>4</sub> B <sub>6</sub> C <sub>6</sub> | 1.333 H <sub>3</sub> N + 1.2 Y <sub>4</sub> C <sub>5</sub> + 2.483 YB <sub>12</sub> → 0.3333 YN + 5.95 YB <sub>4</sub> + YB <sub>6</sub> H <sub>4</sub> C <sub>6</sub> N                            | -2.0121             |
| YNH <sub>4</sub> B <sub>6</sub> C <sub>6</sub> | 1.2 Y <sub>4</sub> C <sub>5</sub> + 0.5 N <sub>2</sub> + 7.7 H <sub>2</sub> + 6 B → 3.8 YH <sub>3</sub> + YB <sub>6</sub> H <sub>4</sub> C <sub>6</sub> N                                           | -2.0086             |
| YNH <sub>4</sub> B <sub>6</sub> C <sub>6</sub> | 4.558 H <sub>3</sub> N + 0.7965 YB <sub>12</sub> + 0.8571 Y <sub>4</sub> C <sub>7</sub> → 3.225 YH <sub>3</sub> + 3.558 BN + YB <sub>6</sub> H <sub>4</sub> C <sub>6</sub> N                        | -2.0083             |
| YNH <sub>4</sub> B <sub>6</sub> C <sub>6</sub> | 1.2 Y <sub>4</sub> C <sub>5</sub> + 0.5 N <sub>2</sub> + 8.8 H <sub>2</sub> + 3 YB <sub>2</sub> → 6.8 YH <sub>2</sub> + YB <sub>6</sub> H <sub>4</sub> C <sub>6</sub> N                             | -1.9579             |
| YNH <sub>4</sub> B <sub>6</sub> C <sub>6</sub> | 31 YH <sub>3</sub> + 6 Y <sub>2</sub> C + YN + 1.5 YB <sub>4</sub> → 44.5 YH <sub>2</sub> + YB <sub>6</sub> H <sub>4</sub> C <sub>6</sub> N                                                         | -1.9374             |
| YNH <sub>4</sub> B <sub>6</sub> C <sub>6</sub> | 1.2 Y <sub>4</sub> C <sub>5</sub> + 0.5714 B <sub>5</sub> H <sub>7</sub> + BN + 47.74 B → 3.8 YB <sub>12</sub> + YB <sub>6</sub> H <sub>4</sub> C <sub>6</sub> N                                    | -1.9249             |
| YNH <sub>4</sub> B <sub>6</sub> C <sub>6</sub> | 6 Y <sub>2</sub> C + 1.333 H <sub>3</sub> N + 9.733 BN → 10.07 YN + 0.9333 YB <sub>4</sub> + YB <sub>6</sub> H <sub>4</sub> C <sub>6</sub> N                                                        | -1.8998             |
| YNH <sub>4</sub> B <sub>6</sub> C <sub>6</sub> | 1.75 B <sub>13</sub> C <sub>2</sub> + 0.5 H <sub>8</sub> C <sub>5</sub> + BN + 10.87 YB <sub>2</sub> → 9.875 YB <sub>4</sub> + YB <sub>6</sub> H <sub>4</sub> C <sub>6</sub> N                      | -1.8791             |
| YNH <sub>4</sub> B <sub>6</sub> C <sub>6</sub> | 6 Y <sub>2</sub> C + 5.4 B <sub>5</sub> H <sub>7</sub> + BN → 16.9 H <sub>2</sub> + 11 YB <sub>2</sub> + YB <sub>6</sub> H <sub>4</sub> C <sub>6</sub> N                                            | -1.8764             |
| YNH <sub>4</sub> B <sub>6</sub> C <sub>6</sub> | 0.6941 B <sub>13</sub> C <sub>2</sub> + 4.023 H <sub>3</sub> N + 0.9224 Y <sub>4</sub> C <sub>5</sub> → 2.689 YH <sub>3</sub> + 3.023 BN + YB <sub>6</sub> H <sub>4</sub> C <sub>6</sub> N          | -1.8651             |
| YNH <sub>4</sub> B <sub>6</sub> C <sub>6</sub> | 0.3636 B <sub>9</sub> H <sub>11</sub> + 1.2 Y <sub>4</sub> C <sub>5</sub> + BN + 47.33 B → 3.8 YB <sub>12</sub> + YB <sub>6</sub> H <sub>4</sub> C <sub>6</sub> N                                   | -1.8627             |
| YNH <sub>4</sub> B <sub>6</sub> C <sub>6</sub> | 0.5714 B <sub>5</sub> H <sub>7</sub> + 2.107 N <sub>2</sub> + 0.8571 Y <sub>4</sub> C <sub>7</sub> + 0.7857 YB <sub>4</sub> → 3.214 YN + YB <sub>6</sub> H <sub>4</sub> C <sub>6</sub> N            | -1.8559             |
| YNH <sub>4</sub> B <sub>6</sub> C <sub>6</sub> | 1.333 B <sub>13</sub> C <sub>2</sub> + 3.333 Y <sub>2</sub> C + 0.5 N <sub>2</sub> + 2 H <sub>2</sub> → 5.667 YB <sub>2</sub> + YB <sub>6</sub> H <sub>4</sub> C <sub>6</sub> N                     | -1.8521             |
| YNH <sub>4</sub> B <sub>6</sub> C <sub>6</sub> | 1.552 B <sub>13</sub> C <sub>2</sub> + 2.272 Y <sub>2</sub> C + H <sub>3</sub> N + 0.125 H <sub>8</sub> C <sub>5</sub> → 3.543 YB <sub>4</sub> + YB <sub>6</sub> H <sub>4</sub> C <sub>6</sub> N    | -1.8266             |
| YNH <sub>4</sub> B <sub>6</sub> C <sub>6</sub> | 1.333 H <sub>3</sub> N + 1.2 Y <sub>4</sub> C <sub>5</sub> + 2.65 YB <sub>12</sub> → 0.1667 N <sub>2</sub> + 6.45 YB <sub>4</sub> + YB <sub>6</sub> H <sub>4</sub> C <sub>6</sub> N                 | -1.8181             |
| YNH <sub>4</sub> B <sub>6</sub> C <sub>6</sub> | 24.31 YH <sub>3</sub> + 0.4615 B <sub>13</sub> C <sub>2</sub> + 5.077 Y <sub>2</sub> C + YN → 34.46 YH <sub>2</sub> + YB <sub>6</sub> H <sub>4</sub> C <sub>6</sub> N                               | -1.7956             |
| YNH <sub>4</sub> B <sub>6</sub> C <sub>6</sub> | 0.3636 B <sub>9</sub> H <sub>11</sub> + 2.055 N <sub>2</sub> + 0.8571 Y <sub>4</sub> C <sub>7</sub> + 0.6818 YB <sub>4</sub> → 3.11 YN + YB <sub>6</sub> H <sub>4</sub> C <sub>6</sub> N            | -1.7453             |
| YNH <sub>4</sub> B <sub>6</sub> C <sub>6</sub> | 2 YH <sub>2</sub> + 6 C + 2.5 N <sub>2</sub> + 3 YB <sub>2</sub> → 4 YN + YB <sub>6</sub> H <sub>4</sub> C <sub>6</sub> N                                                                           | -1.7440             |
| YNH <sub>4</sub> B <sub>6</sub> C <sub>6</sub> | 1.2 Y <sub>4</sub> C <sub>5</sub> + 1.2 B <sub>5</sub> H <sub>7</sub> + 1.3 N <sub>2</sub> → 2.2 YH <sub>2</sub> + 1.6 YN + YB <sub>6</sub> H <sub>4</sub> C <sub>6</sub> N                         | -1.7416             |
| YNH <sub>4</sub> B <sub>6</sub> C <sub>6</sub> | 6 Y <sub>2</sub> C + 9 H <sub>3</sub> N + 0.5 YB <sub>12</sub> → 11.5 YH <sub>2</sub> + 4 N <sub>2</sub> + YB <sub>6</sub> H <sub>4</sub> C <sub>6</sub> N                                          | -1.7353             |
| YNH <sub>4</sub> B <sub>6</sub> C <sub>6</sub> | 4.567 H <sub>3</sub> N + 1.2 Y <sub>4</sub> C <sub>5</sub> + 3 YB <sub>2</sub> → 3.233 YH <sub>3</sub> + 3.567 YN + YB <sub>6</sub> H <sub>4</sub> C <sub>6</sub> N                                 | -1.7335             |
| YNH <sub>4</sub> B <sub>6</sub> C <sub>6</sub> | 1.333 YH <sub>3</sub> + 0.5 N <sub>2</sub> + 0.8571 Y <sub>4</sub> C <sub>7</sub> + 21.05 B → 3.762 YB <sub>4</sub> + YB <sub>6</sub> H <sub>4</sub> C <sub>6</sub> N                               | -1.7274             |
| YNH <sub>4</sub> B <sub>6</sub> C <sub>6</sub> | 0.4615 B <sub>13</sub> C <sub>2</sub> + 1.333 H <sub>3</sub> N + 1.015 Y <sub>4</sub> C <sub>5</sub> + 1.364 N <sub>2</sub> → 3.062 YN + YB <sub>6</sub> H <sub>4</sub> C <sub>6</sub> N            | -1.7217             |
| YNH <sub>4</sub> B <sub>6</sub> C <sub>6</sub> | 28.5 YH <sub>3</sub> + 6 Y <sub>2</sub> C + BN + 1.25 YB <sub>4</sub> → 40.75 YH <sub>2</sub> + YB <sub>6</sub> H <sub>4</sub> C <sub>6</sub> N                                                     | -1.7178             |
| YNH <sub>4</sub> B <sub>6</sub> C <sub>6</sub> | 3.762 H <sub>3</sub> N + 0.8571 Y <sub>4</sub> C <sub>7</sub> + 8.762 B → 2.429 YH <sub>3</sub> + 2.762 BN + YB <sub>6</sub> H <sub>4</sub> C <sub>6</sub> N                                        | -1.6641             |
| YNH <sub>4</sub> B <sub>6</sub> C <sub>6</sub> | 1.333 YH <sub>3</sub> + 1.2 Y <sub>4</sub> C <sub>5</sub> + 3.192 YB <sub>12</sub> + BN → 8.325 YB <sub>4</sub> + YB <sub>6</sub> H <sub>4</sub> C <sub>6</sub> N                                   | -1.6600             |
| YNH <sub>4</sub> B <sub>6</sub> C <sub>6</sub> | 1.2 Y <sub>4</sub> C <sub>5</sub> + 2 H <sub>2</sub> + BN + 20.2 B → 3.8 YB <sub>4</sub> + YB <sub>6</sub> H <sub>4</sub> C <sub>6</sub> N                                                          | -1.6352             |

Continued on next page

Continued

| Compound                                       | Chemical reaction                                                                                                                                                                                                 | Reaction energy(eV) |
|------------------------------------------------|-------------------------------------------------------------------------------------------------------------------------------------------------------------------------------------------------------------------|---------------------|
| YNH <sub>4</sub> B <sub>6</sub> C <sub>6</sub> | 0.5 N <sub>2</sub> + 0.8571 Y <sub>4</sub> C <sub>7</sub> + 10.14 H <sub>2</sub> + 3 YB <sub>2</sub> → 5.429 YH <sub>3</sub> + YB <sub>6</sub> H <sub>4</sub> C <sub>6</sub> N                                    | -1.6095             |
| YNH <sub>4</sub> B <sub>6</sub> C <sub>6</sub> | 1.2 Y <sub>4</sub> C <sub>5</sub> + 0.5 YB <sub>12</sub> + 0.5 N <sub>2</sub> + 8.45 H <sub>2</sub> → 4.3 YH <sub>3</sub> + YB <sub>6</sub> H <sub>4</sub> C <sub>6</sub> N                                       | -1.6033             |
| YNH <sub>4</sub> B <sub>6</sub> C <sub>6</sub> | 22.92 YH <sub>3</sub> + 0.3846 B <sub>13</sub> C <sub>2</sub> + 5.231 Y <sub>2</sub> C + BN → 32.38 YH <sub>2</sub> + YB <sub>6</sub> H <sub>4</sub> C <sub>6</sub> N                                             | -1.5996             |
| YNH <sub>4</sub> B <sub>6</sub> C <sub>6</sub> | 1.717 B <sub>9</sub> H <sub>11</sub> + 1.491 Y <sub>4</sub> C <sub>5</sub> + 0.5 N <sub>2</sub> → 4.964 YH <sub>3</sub> + 0.7275 B <sub>13</sub> C <sub>2</sub> + YB <sub>6</sub> H <sub>4</sub> C <sub>6</sub> N | -1.5939             |
| YNH <sub>4</sub> B <sub>6</sub> C <sub>6</sub> | 1.333 YH <sub>3</sub> + 0.4615 B <sub>13</sub> C <sub>2</sub> + 2.117 N <sub>2</sub> + 0.7253 Y <sub>4</sub> C <sub>7</sub> → 3.234 YN + YB <sub>6</sub> H <sub>4</sub> C <sub>6</sub> N                          | -1.5921             |
| YNH <sub>4</sub> B <sub>6</sub> C <sub>6</sub> | 3 B <sub>13</sub> C <sub>2</sub> + 4.083 Y + 1.333 H <sub>3</sub> N → 2.75 YB <sub>12</sub> + 0.3333 YN + YB <sub>6</sub> H <sub>4</sub> C <sub>6</sub> N                                                         | -1.5704             |
| YNH <sub>4</sub> B <sub>6</sub> C <sub>6</sub> | 0.2619 YB <sub>12</sub> + 0.5714 B <sub>5</sub> H <sub>7</sub> + 1.845 N <sub>2</sub> + 0.8571 Y <sub>4</sub> C <sub>7</sub> → 2.69 YN + YB <sub>6</sub> H <sub>4</sub> C <sub>6</sub> N                          | -1.5511             |
| YNH <sub>4</sub> B <sub>6</sub> C <sub>6</sub> | H <sub>3</sub> N + 1.075 Y <sub>4</sub> C <sub>5</sub> + 0.125 H <sub>8</sub> C <sub>5</sub> + 19.2 B → 3.3 YB <sub>4</sub> + YB <sub>6</sub> H <sub>4</sub> C <sub>6</sub> N                                     | -1.5363             |
| YNH <sub>4</sub> B <sub>6</sub> C <sub>6</sub> | 0.5 N <sub>2</sub> + 0.8571 Y <sub>4</sub> C <sub>7</sub> + 2 H <sub>2</sub> + 35.14 B → 2.429 YB <sub>12</sub> + YB <sub>6</sub> H <sub>4</sub> C <sub>6</sub> N                                                 | -1.5246             |
| YNH <sub>4</sub> B <sub>6</sub> C <sub>6</sub> | 0.3636 B <sub>9</sub> H <sub>11</sub> + 6 Y <sub>2</sub> C + 10.15 BN → 9.145 YN + 1.855 YB <sub>4</sub> + YB <sub>6</sub> H <sub>4</sub> C <sub>6</sub> N                                                        | -1.5194             |
| YNH <sub>4</sub> B <sub>6</sub> C <sub>6</sub> | 0.5714 B <sub>5</sub> H <sub>7</sub> + 1.714 N <sub>2</sub> + 0.8571 Y <sub>4</sub> C <sub>7</sub> + 3.143 B → 2.429 YN + YB <sub>6</sub> H <sub>4</sub> C <sub>6</sub> N                                         | -1.4904             |
| YNH <sub>4</sub> B <sub>6</sub> C <sub>6</sub> | 0.3636 B <sub>9</sub> H <sub>11</sub> + 0.2273 YB <sub>12</sub> + 1.828 N <sub>2</sub> + 0.8571 Y <sub>4</sub> C <sub>7</sub> → 2.656 YN + YB <sub>6</sub> H <sub>4</sub> C <sub>6</sub> N                        | -1.4808             |
| YNH <sub>4</sub> B <sub>6</sub> C <sub>6</sub> | 0.6667 B <sub>9</sub> H <sub>11</sub> + 6 C + 4.167 Y + H <sub>3</sub> N → 3.167 YH <sub>2</sub> + YB <sub>6</sub> H <sub>4</sub> C <sub>6</sub> N                                                                | -1.4749             |
| YNH <sub>4</sub> B <sub>6</sub> C <sub>6</sub> | 2 YH <sub>2</sub> + 3.464 YB <sub>12</sub> + YN + 0.8571 Y <sub>4</sub> C <sub>7</sub> → 8.893 YB <sub>4</sub> + YB <sub>6</sub> H <sub>4</sub> C <sub>6</sub> N                                                  | -1.4574             |
| YNH <sub>4</sub> B <sub>6</sub> C <sub>6</sub> | 2.857 Y <sub>2</sub> C + 0.6286 H <sub>8</sub> C <sub>5</sub> + 1.2 B <sub>5</sub> H <sub>7</sub> + 0.5 N <sub>2</sub> → 4.714 YH <sub>2</sub> + YB <sub>6</sub> H <sub>4</sub> C <sub>6</sub> N                  | -1.4326             |
| YNH <sub>4</sub> B <sub>6</sub> C <sub>6</sub> | 0.3636 B <sub>9</sub> H <sub>11</sub> + 1.714 N <sub>2</sub> + 0.8571 Y <sub>4</sub> C <sub>7</sub> + 2.727 B → 2.429 YN + YB <sub>6</sub> H <sub>4</sub> C <sub>6</sub> N                                        | -1.4281             |
| YNH <sub>4</sub> B <sub>6</sub> C <sub>6</sub> | 0.6667 B <sub>9</sub> H <sub>11</sub> + 3.202 Y <sub>2</sub> C + H <sub>3</sub> N + 0.5595 H <sub>8</sub> C <sub>5</sub> → 5.405 YH <sub>2</sub> + YB <sub>6</sub> H <sub>4</sub> C <sub>6</sub> N                | -1.4197             |
| YNH <sub>4</sub> B <sub>6</sub> C <sub>6</sub> | 6 Y <sub>2</sub> C + 0.5714 B <sub>5</sub> H <sub>7</sub> + 10.23 BN → 9.229 YN + 1.771 YB <sub>4</sub> + YB <sub>6</sub> H <sub>4</sub> C <sub>6</sub> N                                                         | -1.4070             |
| YNH <sub>4</sub> B <sub>6</sub> C <sub>6</sub> | 7.037 Y <sub>2</sub> C + 1.333 H <sub>3</sub> N + 12.74 BN → 0.5185 B <sub>13</sub> C <sub>2</sub> + 13.07 YN + YB <sub>6</sub> H <sub>4</sub> C <sub>6</sub> N                                                   | -1.3986             |
| YNH <sub>4</sub> B <sub>6</sub> C <sub>6</sub> | 4.8 H <sub>3</sub> N + 1.2 Y <sub>4</sub> C <sub>5</sub> + 14.51 B → 0.9455 B <sub>9</sub> H <sub>11</sub> + 3.8 YN + YB <sub>6</sub> H <sub>4</sub> C <sub>6</sub> N                                             | -1.3288             |
| YNH <sub>4</sub> B <sub>6</sub> C <sub>6</sub> | 1.333 YH <sub>3</sub> + 2.046 B <sub>13</sub> C <sub>2</sub> + 1.908 Y <sub>2</sub> C + YN → 5.149 YB <sub>4</sub> + YB <sub>6</sub> H <sub>4</sub> C <sub>6</sub> N                                              | -1.3087             |
| YNH <sub>4</sub> B <sub>6</sub> C <sub>6</sub> | YN + 0.8571 Y <sub>4</sub> C <sub>7</sub> + 2 H <sub>2</sub> + 47.14 B → 3.429 YB <sub>12</sub> + YB <sub>6</sub> H <sub>4</sub> C <sub>6</sub> N                                                                 | -1.2927             |
| YNH <sub>4</sub> B <sub>6</sub> C <sub>6</sub> | 6 Y <sub>2</sub> C + 12.33 H <sub>3</sub> N + 6 B → 11 YH <sub>3</sub> + 5.667 N <sub>2</sub> + YB <sub>6</sub> H <sub>4</sub> C <sub>6</sub> N                                                                   | -1.2856             |
| YNH <sub>4</sub> B <sub>6</sub> C <sub>6</sub> | 2 YH <sub>2</sub> + 2.138 B <sub>13</sub> C <sub>2</sub> + 1.724 Y <sub>2</sub> C + YN → 5.448 YB <sub>4</sub> + YB <sub>6</sub> H <sub>4</sub> C <sub>6</sub> N                                                  | -1.2804             |
| YNH <sub>4</sub> B <sub>6</sub> C <sub>6</sub> | 1.409 Y <sub>4</sub> C <sub>5</sub> + 2.558 B <sub>5</sub> H <sub>7</sub> + 0.5 N <sub>2</sub> → 4.636 YH <sub>3</sub> + 0.5224 B <sub>13</sub> C <sub>2</sub> + YB <sub>6</sub> H <sub>4</sub> C <sub>6</sub> N  | -1.2738             |
| YNH <sub>4</sub> B <sub>6</sub> C <sub>6</sub> | 10.58 Y + 1.2 H <sub>8</sub> C <sub>5</sub> + 10.58 BN → 0.5091 B <sub>9</sub> H <sub>11</sub> + 9.582 YN + YB <sub>6</sub> H <sub>4</sub> C <sub>6</sub> N                                                       | -1.2649             |
| YNH <sub>4</sub> B <sub>6</sub> C <sub>6</sub> | 1.333 YH <sub>3</sub> + YN + 0.8571 Y <sub>4</sub> C <sub>7</sub> + 25.05 B → 4.762 YB <sub>4</sub> + YB <sub>6</sub> H <sub>4</sub> C <sub>6</sub> N                                                             | -1.2622             |
| YNH <sub>4</sub> B <sub>6</sub> C <sub>6</sub> | 6 Y <sub>2</sub> C + 1.333 H <sub>3</sub> N + 9.111 BN → 9.444 YN + 1.556 YB <sub>2</sub> + YB <sub>6</sub> H <sub>4</sub> C <sub>6</sub> N                                                                       | -1.2447             |
| YNH <sub>4</sub> B <sub>6</sub> C <sub>6</sub> | 6 Y <sub>2</sub> C + 10.67 H <sub>3</sub> N + 3 YB <sub>2</sub> → 14 YH <sub>2</sub> + 4.833 N <sub>2</sub> + YB <sub>6</sub> H <sub>4</sub> C <sub>6</sub> N                                                     | -1.2137             |
| YNH <sub>4</sub> B <sub>6</sub> C <sub>6</sub> | 2 YH <sub>2</sub> + 0.8571 Y <sub>4</sub> C <sub>7</sub> + BN + 58.14 B → 4.429 YB <sub>12</sub> + YB <sub>6</sub> H <sub>4</sub> C <sub>6</sub> N                                                                | -1.1979             |
| YNH <sub>4</sub> B <sub>6</sub> C <sub>6</sub> | 3 B <sub>13</sub> C <sub>2</sub> + 3.722 Y + 1.333 H <sub>3</sub> N → 2.722 YB <sub>12</sub> + 0.3333 BN + YB <sub>6</sub> H <sub>4</sub> C <sub>6</sub> N                                                        | -1.1819             |
| YNH <sub>4</sub> B <sub>6</sub> C <sub>6</sub> | 4.8 H <sub>3</sub> N + 1.2 Y <sub>4</sub> C <sub>5</sub> + 13.43 B → 1.486 B <sub>5</sub> H <sub>7</sub> + 3.8 YN + YB <sub>6</sub> H <sub>4</sub> C <sub>6</sub> N                                               | -1.1669             |
| YNH <sub>4</sub> B <sub>6</sub> C <sub>6</sub> | 1.2 Y <sub>4</sub> C <sub>5</sub> + 11.45 H <sub>2</sub> + BN + 2.5 YB <sub>2</sub> → 6.3 YH <sub>3</sub> + YB <sub>6</sub> H <sub>4</sub> C <sub>6</sub> N                                                       | -1.1531             |
| YNH <sub>4</sub> B <sub>6</sub> C <sub>6</sub> | 1.2 Y <sub>4</sub> C <sub>5</sub> + 0.5 N <sub>2</sub> + 9.95 H <sub>2</sub> + 1.5 YB <sub>4</sub> → 5.3 YH <sub>3</sub> + YB <sub>6</sub> H <sub>4</sub> C <sub>6</sub> N                                        | -1.1427             |
| YNH <sub>4</sub> B <sub>6</sub> C <sub>6</sub> | 1.333 YH <sub>3</sub> + 1.874 B <sub>13</sub> C <sub>2</sub> + 2.253 Y <sub>2</sub> C + BN → 4.839 YB <sub>4</sub> + YB <sub>6</sub> H <sub>4</sub> C <sub>6</sub> N                                              | -1.1420             |
| YNH <sub>4</sub> B <sub>6</sub> C <sub>6</sub> | 2 YH <sub>2</sub> + 1.966 B <sub>13</sub> C <sub>2</sub> + 2.069 Y <sub>2</sub> C + BN → 5.138 YB <sub>4</sub> + YB <sub>6</sub> H <sub>4</sub> C <sub>6</sub> N                                                  | -1.1138             |
| YNH <sub>4</sub> B <sub>6</sub> C <sub>6</sub> | 1.333 YH <sub>3</sub> + 2.631 YB <sub>12</sub> + 0.5 N <sub>2</sub> + 0.8571 Y <sub>4</sub> C <sub>7</sub> → 6.393 YB <sub>4</sub> + YB <sub>6</sub> H <sub>4</sub> C <sub>6</sub> N                              | -1.1134             |
| YNH <sub>4</sub> B <sub>6</sub> C <sub>6</sub> | 1.2 H <sub>8</sub> C <sub>5</sub> + 2.95 B <sub>5</sub> H <sub>7</sub> + 9.75 YN → 8.75 YH <sub>3</sub> + 8.75 BN + YB <sub>6</sub> H <sub>4</sub> C <sub>6</sub> N                                               | -1.1123             |
| YNH <sub>4</sub> B <sub>6</sub> C <sub>6</sub> | 3.5 Y <sub>2</sub> C + 0.5 H <sub>8</sub> C <sub>5</sub> + YN + 20 B → 7 YB <sub>2</sub> + YB <sub>6</sub> H <sub>4</sub> C <sub>6</sub> N                                                                        | -1.0668             |
| YNH <sub>4</sub> B <sub>6</sub> C <sub>6</sub> | 1.2 Y <sub>4</sub> C <sub>5</sub> + 2.525 YB <sub>12</sub> + 2 H <sub>2</sub> + BN → 6.325 YB <sub>4</sub> + YB <sub>6</sub> H <sub>4</sub> C <sub>6</sub> N                                                      | -1.0460             |
| YNH <sub>4</sub> B <sub>6</sub> C <sub>6</sub> | 1.2 Y <sub>4</sub> C <sub>5</sub> + 0.5714 B <sub>5</sub> H <sub>7</sub> + BN + 17.34 B → 3.8 YB <sub>4</sub> + YB <sub>6</sub> H <sub>4</sub> C <sub>6</sub> N                                                   | -1.0381             |
| YNH <sub>4</sub> B <sub>6</sub> C <sub>6</sub> | 1.333 H <sub>3</sub> N + 1.798 N <sub>2</sub> + 0.8571 Y <sub>4</sub> C <sub>7</sub> + 1.5 YB <sub>4</sub> → 3.929 YN + YB <sub>6</sub> H <sub>4</sub> C <sub>6</sub> N                                           | -1.0200             |
| YNH <sub>4</sub> B <sub>6</sub> C <sub>6</sub> | 2.75 B <sub>9</sub> H <sub>11</sub> + 1.714 N <sub>2</sub> + 0.8571 Y <sub>4</sub> C <sub>7</sub> → 3.75 B <sub>5</sub> H <sub>7</sub> + 2.429 YN + YB <sub>6</sub> H <sub>4</sub> C <sub>6</sub> N               | -1.0195             |
| YNH <sub>4</sub> B <sub>6</sub> C <sub>6</sub> | 20.75 YH <sub>2</sub> + 3 B <sub>13</sub> C <sub>2</sub> + YN → 12.5 YH <sub>3</sub> + 8.25 YB <sub>4</sub> + YB <sub>6</sub> H <sub>4</sub> C <sub>6</sub> N                                                     | -1.0155             |
| YNH <sub>4</sub> B <sub>6</sub> C <sub>6</sub> | 17.5 YH <sub>3</sub> + 3 B <sub>13</sub> C <sub>2</sub> + 8.583 N <sub>2</sub> → 16.17 H <sub>3</sub> N + 16.5 YB <sub>2</sub> + YB <sub>6</sub> H <sub>4</sub> C <sub>6</sub> N                                  | -0.9865             |
| YNH <sub>4</sub> B <sub>6</sub> C <sub>6</sub> | H <sub>3</sub> N + 1.075 Y <sub>4</sub> C <sub>5</sub> + 2.4 YB <sub>12</sub> + 0.125 H <sub>8</sub> C <sub>5</sub> → 5.7 YB <sub>4</sub> + YB <sub>6</sub> H <sub>4</sub> C <sub>6</sub> N                       | -0.9762             |
| YNH <sub>4</sub> B <sub>6</sub> C <sub>6</sub> | 0.3636 B <sub>9</sub> H <sub>11</sub> + 1.2 Y <sub>4</sub> C <sub>5</sub> + BN + 16.93 B → 3.8 YB <sub>4</sub> + YB <sub>6</sub> H <sub>4</sub> C <sub>6</sub> N                                                  | -0.9758             |
| YNH <sub>4</sub> B <sub>6</sub> C <sub>6</sub> | 1.2 Y <sub>4</sub> C <sub>5</sub> + YN + 9.2 H <sub>2</sub> + 6 B → 4.8 YH <sub>3</sub> + YB <sub>6</sub> H <sub>4</sub> C <sub>6</sub> N                                                                         | -0.9661             |
| YNH <sub>4</sub> B <sub>6</sub> C <sub>6</sub> | 0.5 N <sub>2</sub> + 0.8571 Y <sub>4</sub> C <sub>7</sub> + 2 H <sub>2</sub> + 15.71 B → 2.429 YB <sub>4</sub> + YB <sub>6</sub> H <sub>4</sub> C <sub>6</sub> N                                                  | -0.9578             |
| YNH <sub>4</sub> B <sub>6</sub> C <sub>6</sub> | 0.5714 B <sub>5</sub> H <sub>7</sub> + 0.5 N <sub>2</sub> + 0.8571 Y <sub>4</sub> C <sub>7</sub> + 32.29 B → 2.429 YB <sub>12</sub> + YB <sub>6</sub> H <sub>4</sub> C <sub>6</sub> N                             | -0.9274             |
| YNH <sub>4</sub> B <sub>6</sub> C <sub>6</sub> | 1.2 H <sub>8</sub> C <sub>5</sub> + 2.645 N <sub>2</sub> + 5.291 YB <sub>2</sub> → 0.5091 B <sub>9</sub> H <sub>11</sub> + 4.291 YN + YB <sub>6</sub> H <sub>4</sub> C <sub>6</sub> N                             | -0.9174             |
| YNH <sub>4</sub> B <sub>6</sub> C <sub>6</sub> | 0.09091 B <sub>9</sub> H <sub>11</sub> + 3 B <sub>13</sub> C <sub>2</sub> + 3.818 Y + H <sub>3</sub> N → 2.818 YB <sub>12</sub> + YB <sub>6</sub> H <sub>4</sub> C <sub>6</sub> N                                 | -0.9129             |
| YNH <sub>4</sub> B <sub>6</sub> C <sub>6</sub> | 3 B <sub>13</sub> C <sub>2</sub> + 3.81 Y + H <sub>3</sub> N + 0.1429 B <sub>5</sub> H <sub>7</sub> → 2.81 YB <sub>12</sub> + YB <sub>6</sub> H <sub>4</sub> C <sub>6</sub> N                                     | -0.9004             |
| YNH <sub>4</sub> B <sub>6</sub> C <sub>6</sub> | 4.667 Y + 1.2 H <sub>8</sub> C <sub>5</sub> + 1.2 B <sub>5</sub> H <sub>7</sub> + YN → 4.667 YH <sub>3</sub> + YB <sub>6</sub> H <sub>4</sub> C <sub>6</sub> N                                                    | -0.8995             |
| YNH <sub>4</sub> B <sub>6</sub> C <sub>6</sub> | 0.6667 B <sub>9</sub> H <sub>11</sub> + 1.714 N <sub>2</sub> + 0.8571 Y <sub>4</sub> C <sub>7</sub> → 2.429 YN + 1.667 H <sub>2</sub> + YB <sub>6</sub> H <sub>4</sub> C <sub>6</sub> N                           | -0.8786             |
| YNH <sub>4</sub> B <sub>6</sub> C <sub>6</sub> | 5.2 Y + 1.2 H <sub>8</sub> C <sub>5</sub> + B <sub>5</sub> H <sub>7</sub> + BN → 4.2 YH <sub>3</sub> + YB <sub>6</sub> H <sub>4</sub> C <sub>6</sub> N                                                            | -0.8751             |
| YNH <sub>4</sub> B <sub>6</sub> C <sub>6</sub> | 0.3636 B <sub>9</sub> H <sub>11</sub> + 0.5 N <sub>2</sub> + 0.8571 Y <sub>4</sub> C <sub>7</sub> + 31.87 B → 2.429 YB <sub>12</sub> + YB <sub>6</sub> H <sub>4</sub> C <sub>6</sub> N                            | -0.8651             |
| YNH <sub>4</sub> B <sub>6</sub> C <sub>6</sub> | 1.302 B <sub>13</sub> C <sub>2</sub> + 3.397 Y <sub>2</sub> C + 1.333 H <sub>3</sub> N → 0.3333 YN + 5.46 YB <sub>2</sub> + YB <sub>6</sub> H <sub>4</sub> C <sub>6</sub> N                                       | -0.8584             |
| YNH <sub>4</sub> B <sub>6</sub> C <sub>6</sub> | 3 B <sub>13</sub> C <sub>2</sub> + 3.75 Y + H <sub>3</sub> N + 0.5 H <sub>2</sub> → 2.75 YB <sub>12</sub> + YB <sub>6</sub> H <sub>4</sub> C <sub>6</sub> N                                                       | -0.8574             |
| YNH <sub>4</sub> B <sub>6</sub> C <sub>6</sub> | 16.05 B <sub>9</sub> H <sub>11</sub> + 1.2 Y <sub>4</sub> C <sub>5</sub> + 0.5 N <sub>2</sub> → 24.65 B <sub>5</sub> H <sub>7</sub> + 3.8 YB <sub>4</sub> + YB <sub>6</sub> H <sub>4</sub> C <sub>6</sub> N       | -0.8564             |

Continued on next page

Continued

| Compound                                       | Chemical reaction                                                                                                                                                                                           | Reaction energy(eV) |
|------------------------------------------------|-------------------------------------------------------------------------------------------------------------------------------------------------------------------------------------------------------------|---------------------|
| YNH <sub>4</sub> B <sub>6</sub> C <sub>6</sub> | 2.108 B <sub>9</sub> H <sub>11</sub> + 1.599 Y <sub>4</sub> C <sub>5</sub> + YN → 6.397 YH <sub>3</sub> + 0.998 B <sub>13</sub> C <sub>2</sub> + YB <sub>6</sub> H <sub>4</sub> C <sub>6</sub> N            | -0.8468             |
| YNH <sub>4</sub> B <sub>6</sub> C <sub>6</sub> | 1.349 B <sub>13</sub> C <sub>2</sub> + 3.302 Y <sub>2</sub> C + 1.333 H <sub>3</sub> N → 0.3333 BN + 5.603 YB <sub>2</sub> + YB <sub>6</sub> H <sub>4</sub> C <sub>6</sub> N                                | -0.8443             |
| YNH <sub>4</sub> B <sub>6</sub> C <sub>6</sub> | 1.2 B <sub>5</sub> H <sub>7</sub> + 1.714 N <sub>2</sub> + 0.8571 Y <sub>4</sub> C <sub>7</sub> → 2.429 YN + 2.2 H <sub>2</sub> + YB <sub>6</sub> H <sub>4</sub> C <sub>6</sub> N                           | -0.8335             |
| YNH <sub>4</sub> B <sub>6</sub> C <sub>6</sub> | 1.2 Y <sub>4</sub> C <sub>5</sub> + 0.5 N <sub>2</sub> + 5.8 H <sub>2</sub> + 6 B → 3.8 YH <sub>2</sub> + YB <sub>6</sub> H <sub>4</sub> C <sub>6</sub> N                                                   | -0.8327             |
| YNH <sub>4</sub> B <sub>6</sub> C <sub>6</sub> | 1.75 B <sub>13</sub> C <sub>2</sub> + 0.5 H <sub>8</sub> C <sub>5</sub> + YN + 8.375 YB <sub>2</sub> → 8.375 YB <sub>4</sub> + YB <sub>6</sub> H <sub>4</sub> C <sub>6</sub> N                              | -0.8264             |
| YNH <sub>4</sub> B <sub>6</sub> C <sub>6</sub> | 0.4615 B <sub>13</sub> C <sub>2</sub> + 5.077 Y <sub>2</sub> C + 7.436 H <sub>3</sub> N → 9.154 YH <sub>2</sub> + 3.218 N <sub>2</sub> + YB <sub>6</sub> H <sub>4</sub> C <sub>6</sub> N                    | -0.8236             |
| YNH <sub>4</sub> B <sub>6</sub> C <sub>6</sub> | 7.8 H <sub>3</sub> N + 1.2 Y <sub>4</sub> C <sub>5</sub> + 3 YB <sub>2</sub> → 6.8 YN + 9.7 H <sub>2</sub> + YB <sub>6</sub> H <sub>4</sub> C <sub>6</sub> N                                                | -0.8228             |
| YNH <sub>4</sub> B <sub>6</sub> C <sub>6</sub> | 6 Y <sub>2</sub> C + 2 H <sub>2</sub> + 10.8 BN → 9.8 YN + 1.2 YB <sub>4</sub> + YB <sub>6</sub> H <sub>4</sub> C <sub>6</sub> N                                                                            | -0.8033             |
| YNH <sub>4</sub> B <sub>6</sub> C <sub>6</sub> | 0.6667 B <sub>9</sub> H <sub>11</sub> + 1.2 Y <sub>4</sub> C <sub>5</sub> + 0.5 N <sub>2</sub> + 4.033 H <sub>2</sub> → 3.8 YH <sub>3</sub> + YB <sub>6</sub> H <sub>4</sub> C <sub>6</sub> N               | -0.7996             |
| YNH <sub>4</sub> B <sub>6</sub> C <sub>6</sub> | 24.5 YH <sub>2</sub> + 3 B <sub>13</sub> C <sub>2</sub> + BN → 15 YH <sub>3</sub> + 8.5 YB <sub>4</sub> + YB <sub>6</sub> H <sub>4</sub> C <sub>6</sub> N                                                   | -0.7959             |
| YNH <sub>4</sub> B <sub>6</sub> C <sub>6</sub> | 0.6667 B <sub>9</sub> H <sub>11</sub> + 2.667 Y <sub>2</sub> C + 0.6667 H <sub>8</sub> C <sub>5</sub> + 0.5 N <sub>2</sub> → 4.333 YH <sub>2</sub> + YB <sub>6</sub> H <sub>4</sub> C <sub>6</sub> N        | -0.7792             |
| YNH <sub>4</sub> B <sub>6</sub> C <sub>6</sub> | 6 Y <sub>2</sub> C + 1.333 H <sub>3</sub> N + 10.31 BN → 0.359 YB <sub>12</sub> + 10.64 YN + YB <sub>6</sub> H <sub>4</sub> C <sub>6</sub> N                                                                | -0.7765             |
| YNH <sub>4</sub> B <sub>6</sub> C <sub>6</sub> | 0.5 YH <sub>2</sub> + H <sub>3</sub> N + 0.8571 Y <sub>4</sub> C <sub>7</sub> + 41.14 B → 2.929 YB <sub>12</sub> + YB <sub>6</sub> H <sub>4</sub> C <sub>6</sub> N                                          | -0.7605             |
| YNH <sub>4</sub> B <sub>6</sub> C <sub>6</sub> | 1.2 Y <sub>4</sub> C <sub>5</sub> + 1.2 B <sub>5</sub> H <sub>7</sub> + 0.5 N <sub>2</sub> + 3.5 H <sub>2</sub> → 3.8 YH <sub>3</sub> + YB <sub>6</sub> H <sub>4</sub> C <sub>6</sub> N                     | -0.7545             |
| YNH <sub>4</sub> B <sub>6</sub> C <sub>6</sub> | 7.867 Y + 1.2 H <sub>8</sub> C <sub>5</sub> + 6 BN → 1.867 YH <sub>3</sub> + 5 YN + YB <sub>6</sub> H <sub>4</sub> C <sub>6</sub> N                                                                         | -0.7535             |
| YNH <sub>4</sub> B <sub>6</sub> C <sub>6</sub> | 0.8 B <sub>9</sub> H <sub>11</sub> + 2.2 H <sub>3</sub> N + 1.2 Y <sub>4</sub> C <sub>5</sub> → 3.8 YH <sub>3</sub> + 1.2 BN + YB <sub>6</sub> H <sub>4</sub> C <sub>6</sub> N                              | -0.7250             |
| YNH <sub>4</sub> B <sub>6</sub> C <sub>6</sub> | 6 C + 3.467 Y + H <sub>3</sub> N + 1.2 B <sub>5</sub> H <sub>7</sub> → 2.467 YH <sub>3</sub> + YB <sub>6</sub> H <sub>4</sub> C <sub>6</sub> N                                                              | -0.7153             |
| YNH <sub>4</sub> B <sub>6</sub> C <sub>6</sub> | 3.92 H <sub>3</sub> N + 1.2 Y <sub>4</sub> C <sub>5</sub> + 3 YB <sub>2</sub> → 3.88 YH <sub>2</sub> + 2.92 YN + YB <sub>6</sub> H <sub>4</sub> C <sub>6</sub> N                                            | -0.7150             |
| YNH <sub>4</sub> B <sub>6</sub> C <sub>6</sub> | 6 C + 3.2 Y + 1.2 B <sub>5</sub> H <sub>7</sub> + 0.5 N <sub>2</sub> → 2.2 YH <sub>2</sub> + YB <sub>6</sub> H <sub>4</sub> C <sub>6</sub> N                                                                | -0.7131             |
| YNH <sub>4</sub> B <sub>6</sub> C <sub>6</sub> | 0.5714 B <sub>5</sub> H <sub>7</sub> + YN + 0.8571 Y <sub>4</sub> C <sub>7</sub> + 44.29 B → 3.429 YB <sub>12</sub> + YB <sub>6</sub> H <sub>4</sub> C <sub>6</sub> N                                       | -0.6956             |
| YNH <sub>4</sub> B <sub>6</sub> C <sub>6</sub> | H <sub>3</sub> N + 1.2 Y <sub>4</sub> C <sub>5</sub> + 6.2 H <sub>2</sub> + 6 B → 3.8 YH <sub>3</sub> + YB <sub>6</sub> H <sub>4</sub> C <sub>6</sub> N                                                     | -0.6845             |
| YNH <sub>4</sub> B <sub>6</sub> C <sub>6</sub> | 10 Y + 1.2 H <sub>8</sub> C <sub>5</sub> + 10 BN → 0.8 B <sub>5</sub> H <sub>7</sub> + 9 YN + YB <sub>6</sub> H <sub>4</sub> C <sub>6</sub> N                                                               | -0.6562             |
| YNH <sub>4</sub> B <sub>6</sub> C <sub>6</sub> | H <sub>3</sub> N + 1.2 Y <sub>4</sub> C <sub>5</sub> + 7.3 H <sub>2</sub> + 3 YB <sub>2</sub> → 6.8 YH <sub>2</sub> + YB <sub>6</sub> H <sub>4</sub> C <sub>6</sub> N                                       | -0.6338             |
| YNH <sub>4</sub> B <sub>6</sub> C <sub>6</sub> | 0.3636 B <sub>9</sub> H <sub>11</sub> + YN + 0.8571 Y <sub>4</sub> C <sub>7</sub> + 43.87 B → 3.429 YB <sub>12</sub> + YB <sub>6</sub> H <sub>4</sub> C <sub>6</sub> N                                      | -0.6333             |
| YNH <sub>4</sub> B <sub>6</sub> C <sub>6</sub> | 16 YH <sub>3</sub> + 6 Y <sub>2</sub> C + 6 BN → 22 YH <sub>2</sub> + 5 YN + YB <sub>6</sub> H <sub>4</sub> C <sub>6</sub> N                                                                                | -0.6197             |
| YNH <sub>4</sub> B <sub>6</sub> C <sub>6</sub> | 1.333 H <sub>3</sub> N + 0.8571 Y <sub>4</sub> C <sub>7</sub> + 35.48 B → 2.429 YB <sub>12</sub> + 0.3333 BN + YB <sub>6</sub> H <sub>4</sub> C <sub>6</sub> N                                              | -0.6147             |
| YNH <sub>4</sub> B <sub>6</sub> C <sub>6</sub> | 1.2 Y <sub>4</sub> C <sub>5</sub> + YN + 9.8 H <sub>2</sub> + 3 YB <sub>2</sub> → 7.8 YH <sub>2</sub> + YB <sub>6</sub> H <sub>4</sub> C <sub>6</sub> N                                                     | -0.6060             |
| YNH <sub>4</sub> B <sub>6</sub> C <sub>6</sub> | 0.09091 B <sub>9</sub> H <sub>11</sub> + 1.294 B <sub>13</sub> C <sub>2</sub> + 3.411 Y <sub>2</sub> C + H <sub>3</sub> N → 5.823 YB <sub>2</sub> + YB <sub>6</sub> H <sub>4</sub> C <sub>6</sub> N         | -0.6038             |
| YNH <sub>4</sub> B <sub>6</sub> C <sub>6</sub> | 2.632 Y <sub>2</sub> C + H <sub>3</sub> N + 0.6737 H <sub>8</sub> C <sub>5</sub> + 1.2 B <sub>5</sub> H <sub>7</sub> → 4.263 YH <sub>3</sub> + YB <sub>6</sub> H <sub>4</sub> C <sub>6</sub> N              | -0.6006             |
| YNH <sub>4</sub> B <sub>6</sub> C <sub>6</sub> | 1.299 B <sub>13</sub> C <sub>2</sub> + 3.401 Y <sub>2</sub> C + H <sub>3</sub> N + 0.1429 B <sub>5</sub> H <sub>7</sub> → 5.803 YB <sub>2</sub> + YB <sub>6</sub> H <sub>4</sub> C <sub>6</sub> N           | -0.5888             |
| YNH <sub>4</sub> B <sub>6</sub> C <sub>6</sub> | 0.3636 B <sub>9</sub> H <sub>11</sub> + 0.2098 B <sub>13</sub> C <sub>2</sub> + 1.594 N <sub>2</sub> + 0.7972 Y <sub>4</sub> C <sub>7</sub> → 2.189 YN + YB <sub>6</sub> H <sub>4</sub> C <sub>6</sub> N    | -0.5712             |
| YNH <sub>4</sub> B <sub>6</sub> C <sub>6</sub> | 2.171 B <sub>5</sub> H <sub>7</sub> + 2.367 N <sub>2</sub> + 0.8571 Y <sub>4</sub> C <sub>7</sub> → 3.733 H <sub>3</sub> N + 2.429 YB <sub>2</sub> + YB <sub>6</sub> H <sub>4</sub> C <sub>6</sub> N        | -0.5676             |
| YNH <sub>4</sub> B <sub>6</sub> C <sub>6</sub> | YN + 0.8571 Y <sub>4</sub> C <sub>7</sub> + 11.64 H <sub>2</sub> + 3 YB <sub>2</sub> → 6.429 YH <sub>3</sub> + YB <sub>6</sub> H <sub>4</sub> C <sub>6</sub> N                                              | -0.5670             |
| YNH <sub>4</sub> B <sub>6</sub> C <sub>6</sub> | 1.121 B <sub>9</sub> H <sub>11</sub> + 1.2 Y <sub>4</sub> C <sub>5</sub> + 0.5 N <sub>2</sub> → 2.777 YH <sub>3</sub> + 1.023 YB <sub>4</sub> + YB <sub>6</sub> H <sub>4</sub> C <sub>6</sub> N             | -0.5657             |
| YNH <sub>4</sub> B <sub>6</sub> C <sub>6</sub> | 1.2 Y <sub>4</sub> C <sub>5</sub> + 0.5 YB <sub>12</sub> + YN + 9.95 H <sub>2</sub> → 5.3 YH <sub>3</sub> + YB <sub>6</sub> H <sub>4</sub> C <sub>6</sub> N                                                 | -0.5608             |
| YNH <sub>4</sub> B <sub>6</sub> C <sub>6</sub> | 0.8052 B <sub>9</sub> H <sub>11</sub> + 1.123 N <sub>2</sub> + 0.8571 Y <sub>4</sub> C <sub>7</sub> → 2.429 YH <sub>2</sub> + 1.247 BN + YB <sub>6</sub> H <sub>4</sub> C <sub>6</sub> N                    | -0.5444             |
| YNH <sub>4</sub> B <sub>6</sub> C <sub>6</sub> | 1.2 Y <sub>4</sub> C <sub>5</sub> + 1.851 B <sub>5</sub> H <sub>7</sub> + 0.5 N <sub>2</sub> → 2.986 YH <sub>3</sub> + 0.814 YB <sub>4</sub> + YB <sub>6</sub> H <sub>4</sub> C <sub>6</sub> N              | -0.5439             |
| YNH <sub>4</sub> B <sub>6</sub> C <sub>6</sub> | 1.2 Y <sub>4</sub> C <sub>5</sub> + 2.168 YB <sub>12</sub> + 0.5714 B <sub>5</sub> H <sub>7</sub> + BN → 5.968 YB <sub>4</sub> + YB <sub>6</sub> H <sub>4</sub> C <sub>6</sub> N                            | -0.5321             |
| YNH <sub>4</sub> B <sub>6</sub> C <sub>6</sub> | 1.333 YH <sub>3</sub> + 3.131 YB <sub>12</sub> + YN + 0.8571 Y <sub>4</sub> C <sub>7</sub> → 7.893 YB <sub>4</sub> + YB <sub>6</sub> H <sub>4</sub> C <sub>6</sub> N                                        | -0.5315             |
| YNH <sub>4</sub> B <sub>6</sub> C <sub>6</sub> | 1.333 B <sub>13</sub> C <sub>2</sub> + 3.333 Y <sub>2</sub> C + H <sub>3</sub> N + 0.5 H <sub>2</sub> → 5.667 YB <sub>2</sub> + YB <sub>6</sub> H <sub>4</sub> C <sub>6</sub> N                             | -0.5281             |
| YNH <sub>4</sub> B <sub>6</sub> C <sub>6</sub> | 0.3636 B <sub>9</sub> H <sub>11</sub> + 8.061 Y <sub>2</sub> C + 16.12 BN → 1.03 B <sub>13</sub> C <sub>2</sub> + 15.12 YN + YB <sub>6</sub> H <sub>4</sub> C <sub>6</sub> N                                | -0.5236             |
| YNH <sub>4</sub> B <sub>6</sub> C <sub>6</sub> | 0.2418 B <sub>13</sub> C <sub>2</sub> + 0.5714 B <sub>5</sub> H <sub>7</sub> + 1.576 N <sub>2</sub> + 0.7881 Y <sub>4</sub> C <sub>7</sub> → 2.152 YN + YB <sub>6</sub> H <sub>4</sub> C <sub>6</sub> N     | -0.5028             |
| YNH <sub>4</sub> B <sub>6</sub> C <sub>6</sub> | 1.964 YB <sub>12</sub> + 0.5 N <sub>2</sub> + 0.8571 Y <sub>4</sub> C <sub>7</sub> + 2 H <sub>2</sub> → 4.393 YB <sub>4</sub> + YB <sub>6</sub> H <sub>4</sub> C <sub>6</sub> N                             | -0.4994             |
| YNH <sub>4</sub> B <sub>6</sub> C <sub>6</sub> | YN + 0.8571 Y <sub>4</sub> C <sub>7</sub> + 2 H <sub>2</sub> + 19.71 B → 3.429 YB <sub>4</sub> + YB <sub>6</sub> H <sub>4</sub> C <sub>6</sub> N                                                            | -0.4926             |
| YNH <sub>4</sub> B <sub>6</sub> C <sub>6</sub> | 0.3636 B <sub>9</sub> H <sub>11</sub> + 1.2 Y <sub>4</sub> C <sub>5</sub> + 2.116 YB <sub>12</sub> + BN → 5.916 YB <sub>4</sub> + YB <sub>6</sub> H <sub>4</sub> C <sub>6</sub> N                           | -0.4820             |
| YNH <sub>4</sub> B <sub>6</sub> C <sub>6</sub> | 0.3333 YH <sub>3</sub> + H <sub>3</sub> N + 0.8571 Y <sub>4</sub> C <sub>7</sub> + 39.14 B → 2.762 YB <sub>12</sub> + YB <sub>6</sub> H <sub>4</sub> C <sub>6</sub> N                                       | -0.4707             |
| YNH <sub>4</sub> B <sub>6</sub> C <sub>6</sub> | 4.8 Y + H <sub>3</sub> N + 0.5 YB <sub>12</sub> + 1.2 H <sub>8</sub> C <sub>5</sub> → 4.3 YH <sub>2</sub> + YB <sub>6</sub> H <sub>4</sub> C <sub>6</sub> N                                                 | -0.4587             |
| YNH <sub>4</sub> B <sub>6</sub> C <sub>6</sub> | 1.2 Y <sub>4</sub> C <sub>5</sub> + 9.075 B <sub>5</sub> H <sub>7</sub> + 0.5 N <sub>2</sub> → 3.8 YH <sub>3</sub> + 4.375 B <sub>9</sub> H <sub>11</sub> + YB <sub>6</sub> H <sub>4</sub> C <sub>6</sub> N | -0.4587             |
| YNH <sub>4</sub> B <sub>6</sub> C <sub>6</sub> | 7.968 Y <sub>2</sub> C + 0.5714 B <sub>5</sub> H <sub>7</sub> + 15.94 BN → 0.9841 B <sub>13</sub> C <sub>2</sub> + 14.94 YN + YB <sub>6</sub> H <sub>4</sub> C <sub>6</sub> N                               | -0.4558             |
| YNH <sub>4</sub> B <sub>6</sub> C <sub>6</sub> | 1.499 Y <sub>4</sub> C <sub>5</sub> + 3.14 B <sub>5</sub> H <sub>7</sub> + YN → 5.994 YH <sub>3</sub> + 0.7463 B <sub>13</sub> C <sub>2</sub> + YB <sub>6</sub> H <sub>4</sub> C <sub>6</sub> N             | -0.4540             |
| YNH <sub>4</sub> B <sub>6</sub> C <sub>6</sub> | 1.333 H <sub>3</sub> N + 0.5 YB <sub>12</sub> + 1.298 N <sub>2</sub> + 0.8571 Y <sub>4</sub> C <sub>7</sub> → 2.929 YN + YB <sub>6</sub> H <sub>4</sub> C <sub>6</sub> N                                    | -0.4381             |
| YNH <sub>4</sub> B <sub>6</sub> C <sub>6</sub> | 1.333 YH <sub>3</sub> + 6 C + 2.167 N <sub>2</sub> + 3 YB <sub>2</sub> → 3.333 YN + YB <sub>6</sub> H <sub>4</sub> C <sub>6</sub> N                                                                         | -0.4302             |
| YNH <sub>4</sub> B <sub>6</sub> C <sub>6</sub> | 6.32 H <sub>3</sub> N + 1.2 Y <sub>4</sub> C <sub>5</sub> + 1.52 YB <sub>12</sub> → 1.36 B <sub>9</sub> H <sub>11</sub> + 5.32 YN + YB <sub>6</sub> H <sub>4</sub> C <sub>6</sub> N                         | -0.4203             |
| YNH <sub>4</sub> B <sub>6</sub> C <sub>6</sub> | 3 B <sub>13</sub> C <sub>2</sub> + 3.75 Y + 1.333 H <sub>3</sub> N → 2.75 YB <sub>12</sub> + 0.1667 N <sub>2</sub> + YB <sub>6</sub> H <sub>4</sub> C <sub>6</sub> N                                        | -0.4160             |
| YNH <sub>4</sub> B <sub>6</sub> C <sub>6</sub> | 0.7 Y <sub>4</sub> C <sub>5</sub> + 0.5 H <sub>8</sub> C <sub>5</sub> + 2.15 N <sub>2</sub> + 1.5 YB <sub>4</sub> → 3.3 YN + YB <sub>6</sub> H <sub>4</sub> C <sub>6</sub> N                                | -0.3707             |
| YNH <sub>4</sub> B <sub>6</sub> C <sub>6</sub> | 1.909 H <sub>3</sub> N + 1.2 Y <sub>4</sub> C <sub>5</sub> + 1.382 B <sub>5</sub> H <sub>7</sub> → 3.8 YH <sub>3</sub> + 0.9091 BN + YB <sub>6</sub> H <sub>4</sub> C <sub>6</sub> N                        | -0.3702             |
| YNH <sub>4</sub> B <sub>6</sub> C <sub>6</sub> | 0.5714 B <sub>5</sub> H <sub>7</sub> + 0.5 N <sub>2</sub> + 0.8571 Y <sub>4</sub> C <sub>7</sub> + 12.86 B → 2.429 YB <sub>4</sub> + YB <sub>6</sub> H <sub>4</sub> C <sub>6</sub> N                        | -0.3606             |
| YNH <sub>4</sub> B <sub>6</sub> C <sub>6</sub> | 0.4615 B <sub>13</sub> C <sub>2</sub> + 4.562 Y + H <sub>3</sub> N + 1.015 H <sub>8</sub> C <sub>5</sub> → 3.562 YH <sub>2</sub> + YB <sub>6</sub> H <sub>4</sub> C <sub>6</sub> N                          | -0.3576             |
| YNH <sub>4</sub> B <sub>6</sub> C <sub>6</sub> | 3 B <sub>13</sub> C <sub>2</sub> + 1.333 H <sub>3</sub> N + 11.56 YN → 11.89 BN + 10.56 YB <sub>2</sub> + YB <sub>6</sub> H <sub>4</sub> C <sub>6</sub> N                                                   | -0.3543             |
| YNH <sub>4</sub> B <sub>6</sub> C <sub>6</sub> | 1.2 H <sub>8</sub> C <sub>5</sub> + 2.5 N <sub>2</sub> + 5 YB <sub>2</sub> → 0.8 B <sub>5</sub> H <sub>7</sub> + 4 YN + YB <sub>6</sub> H <sub>4</sub> C <sub>6</sub> N                                     | -0.3279             |

Continued on next page



Continued

| Compound                                        | Chemical reaction                                                                                                                                                                                  | Reaction energy(eV) |
|-------------------------------------------------|----------------------------------------------------------------------------------------------------------------------------------------------------------------------------------------------------|---------------------|
| YNH <sub>4</sub> B <sub>6</sub> C <sub>6</sub>  | 1.333 H <sub>3</sub> N + 1.048 N <sub>2</sub> + 0.8571 Y <sub>4</sub> C <sub>7</sub> + 6 B → 2.429 YN + YB <sub>6</sub> H <sub>4</sub> C <sub>6</sub> N                                            | -0.3222             |
| YNH <sub>4</sub> B <sub>6</sub> C <sub>6</sub>  | 0.3636 B <sub>9</sub> H <sub>11</sub> + 0.5 N <sub>2</sub> + 0.8571 Y <sub>4</sub> C <sub>7</sub> + 12.44 B → 2.429 YB <sub>4</sub> + YB <sub>6</sub> H <sub>4</sub> C <sub>6</sub> N              | -0.2984             |
| YNH <sub>4</sub> B <sub>6</sub> C <sub>6</sub>  | 0.4615 B <sub>13</sub> C <sub>2</sub> + 1.015 Y <sub>4</sub> C <sub>5</sub> + 0.5 N <sub>2</sub> + 6.592 H <sub>2</sub> → 3.062 YH <sub>3</sub> + YB <sub>6</sub> H <sub>4</sub> C <sub>6</sub> N  | -0.2957             |
| YNH <sub>4</sub> B <sub>6</sub> C <sub>6</sub>  | 6.162 H <sub>3</sub> N + 1.2 Y <sub>4</sub> C <sub>5</sub> + 1.362 YB <sub>12</sub> → 2.07 B <sub>5</sub> H <sub>7</sub> + 5.162 YN + YB <sub>6</sub> H <sub>4</sub> C <sub>6</sub> N              | -0.2890             |
| YNH <sub>4</sub> B <sub>6</sub> C <sub>6</sub>  | H <sub>3</sub> N + 0.8571 Y <sub>4</sub> C <sub>7</sub> + 8.643 H <sub>2</sub> + 3 YB <sub>2</sub> → 5.429 YH <sub>3</sub> + YB <sub>6</sub> H <sub>4</sub> C <sub>6</sub> N                       | -0.2854             |
| YNH <sub>4</sub> B <sub>6</sub> C <sub>6</sub>  | H <sub>3</sub> N + 1.2 Y <sub>4</sub> C <sub>5</sub> + 0.5 YB <sub>12</sub> + 6.95 H <sub>2</sub> → 4.3 YH <sub>3</sub> + YB <sub>6</sub> H <sub>4</sub> C <sub>6</sub> N                          | -0.2792             |
| YNH <sub>4</sub> B <sub>6</sub> C <sub>6</sub>  | 1.2 Y <sub>4</sub> C <sub>5</sub> + 0.5 YB <sub>12</sub> + 0.5 N <sub>2</sub> + 6.3 H <sub>2</sub> → 4.3 YH <sub>2</sub> + YB <sub>6</sub> H <sub>4</sub> C <sub>6</sub> N                         | -0.2727             |
| YNH <sub>4</sub> B <sub>6</sub> C <sub>6</sub>  | 2.237 Y <sub>2</sub> C + 0.7526 H <sub>8</sub> C <sub>5</sub> + 1.2 B <sub>5</sub> H <sub>7</sub> + 0.5 N <sub>2</sub> → 3.474 YH <sub>3</sub> + YB <sub>6</sub> H <sub>4</sub> C <sub>6</sub> N   | -0.2328             |
| YNH <sub>4</sub> B <sub>6</sub> C <sub>6</sub>  | 3.8 Y + 1.2 H <sub>8</sub> C <sub>5</sub> + 0.5 N <sub>2</sub> + 6 B → 2.8 YH <sub>2</sub> + YB <sub>6</sub> H <sub>4</sub> C <sub>6</sub> N                                                       | -0.2316             |
| YNH <sub>4</sub> B <sub>6</sub> C <sub>6</sub>  | 3.5 Y <sub>2</sub> C + 0.5 H <sub>8</sub> C <sub>5</sub> + BN + 17 B → 6 YB <sub>2</sub> + YB <sub>6</sub> H <sub>4</sub> C <sub>6</sub> N                                                         | -0.2270             |
| YNH <sub>4</sub> B <sub>6</sub> C <sub>6</sub>  | 6 C + 7 H <sub>3</sub> N + YB <sub>12</sub> → 8.5 H <sub>2</sub> + 6 BN + YB <sub>6</sub> H <sub>4</sub> C <sub>6</sub> N                                                                          | -0.2234             |
| YNH <sub>4</sub> B <sub>6</sub> C <sub>6</sub>  | 6 Y <sub>2</sub> C + 12.83 H <sub>3</sub> N + 0.5 YB <sub>12</sub> → 11.5 YH <sub>3</sub> + 5.917 N <sub>2</sub> + YB <sub>6</sub> H <sub>4</sub> C <sub>6</sub> N                                 | -0.2183             |
| YNH <sub>4</sub> B <sub>6</sub> C <sub>6</sub>  | 0.3636 B <sub>9</sub> H <sub>11</sub> + 6 Y <sub>2</sub> C + 8.909 BN → 7.909 YN + 3.091 YB <sub>2</sub> + YB <sub>6</sub> H <sub>4</sub> C <sub>6</sub> N                                         | -0.2178             |
| YNH <sub>4</sub> B <sub>6</sub> C <sub>6</sub>  | 0.6303 B <sub>13</sub> C <sub>2</sub> + 3.194 H <sub>3</sub> N + 0.9479 Y <sub>4</sub> C <sub>5</sub> → 2.791 YH <sub>2</sub> + 2.194 BN + YB <sub>6</sub> H <sub>4</sub> C <sub>6</sub> N         | -0.2083             |
| YNH <sub>4</sub> B <sub>6</sub> C <sub>6</sub>  | 0.4615 B <sub>13</sub> C <sub>2</sub> + 1.451 N <sub>2</sub> + 0.7253 Y <sub>4</sub> C <sub>7</sub> + 2 H <sub>2</sub> → 1.901 YN + YB <sub>6</sub> H <sub>4</sub> C <sub>6</sub> N                | -0.2022             |
| YNH <sub>4</sub> B <sub>6</sub> C <sub>6</sub>  | H <sub>3</sub> N + 0.8571 Y <sub>4</sub> C <sub>7</sub> + 0.5 H <sub>2</sub> + 35.14 B → 2.429 YB <sub>12</sub> + YB <sub>6</sub> H <sub>4</sub> C <sub>6</sub> N                                  | -0.2005             |
| YNH <sub>4</sub> B <sub>6</sub> C <sub>6</sub>  | 0.5556 B <sub>9</sub> H <sub>11</sub> + 4.904 Y + 1.2 H <sub>8</sub> C <sub>5</sub> + BN → 3.904 YH <sub>3</sub> + YB <sub>6</sub> H <sub>4</sub> C <sub>6</sub> N                                 | -0.1955             |
| YNH <sub>4</sub> B <sub>6</sub> C <sub>6</sub>  | 3 B <sub>13</sub> C <sub>2</sub> + Y + 0.5 N <sub>2</sub> + 25.1 H <sub>2</sub> → 6.6 B <sub>5</sub> H <sub>7</sub> + YB <sub>6</sub> H <sub>4</sub> C <sub>6</sub> N                              | -0.1928             |
| YNH <sub>4</sub> B <sub>6</sub> C <sub>6</sub>  | 2 YH <sub>2</sub> + 0.8571 Y <sub>4</sub> C <sub>7</sub> + BN + 22.71 B → 4.429 YB <sub>4</sub> + YB <sub>6</sub> H <sub>4</sub> C <sub>6</sub> N                                                  | -0.1643             |
| YNH <sub>4</sub> B <sub>6</sub> C <sub>6</sub>  | 6 Y <sub>2</sub> C + 0.5714 B <sub>5</sub> H <sub>7</sub> + 9.048 BN → 8.048 YN + 2.952 YB <sub>2</sub> + YB <sub>6</sub> H <sub>4</sub> C <sub>6</sub> N                                          | -0.1637             |
| YNH <sub>4</sub> B <sub>6</sub> C <sub>6</sub>  | 7.333 Y <sub>2</sub> C + 2 H <sub>2</sub> + 14.67 BN → 0.6667 B <sub>13</sub> C <sub>2</sub> + 13.67 YN + YB <sub>6</sub> H <sub>4</sub> C <sub>6</sub> N                                          | -0.1589             |
| YNH <sub>4</sub> B <sub>6</sub> C <sub>6</sub>  | 1.333 YH <sub>3</sub> + 1.46 B <sub>13</sub> C <sub>2</sub> + 3.079 Y <sub>2</sub> C + 0.5 N <sub>2</sub> → 6.492 YB <sub>2</sub> + YB <sub>6</sub> H <sub>4</sub> C <sub>6</sub> N                | -0.1553             |
| YNH <sub>4</sub> B <sub>6</sub> C <sub>6</sub>  | 1.2 Y <sub>4</sub> C <sub>5</sub> + 2.048 B <sub>5</sub> H <sub>7</sub> + 0.5 N <sub>2</sub> → 3.446 YH <sub>3</sub> + 0.3535 YB <sub>12</sub> + YB <sub>6</sub> H <sub>4</sub> C <sub>6</sub> N   | -0.1544             |
| YNH <sub>4</sub> B <sub>6</sub> C <sub>6</sub>  | 0.3636 B <sub>9</sub> H <sub>11</sub> + 3 B <sub>13</sub> C <sub>2</sub> + 4.106 Y + BN → 3.106 YB <sub>12</sub> + YB <sub>6</sub> H <sub>4</sub> C <sub>6</sub> N                                 | -0.1058             |
| YNH <sub>4</sub> B <sub>6</sub> C <sub>6</sub>  | 0.3333 YH <sub>3</sub> + 1.365 B <sub>13</sub> C <sub>2</sub> + 3.27 Y <sub>2</sub> C + H <sub>3</sub> N → 5.873 YB <sub>2</sub> + YB <sub>6</sub> H <sub>4</sub> C <sub>6</sub> N                 | -0.1039             |
| YNH <sub>4</sub> B <sub>6</sub> C <sub>6</sub>  | 3.5 Y <sub>2</sub> C + 1.8 YB <sub>12</sub> + 0.5 H <sub>8</sub> C <sub>5</sub> + 0.5 N <sub>2</sub> → 7.8 YB <sub>2</sub> + YB <sub>6</sub> H <sub>4</sub> C <sub>6</sub> N                       | -0.1026             |
| YNH <sub>4</sub> B <sub>6</sub> C <sub>6</sub>  | 3.067 H <sub>3</sub> N + 1.2 Y <sub>4</sub> C <sub>5</sub> + 6 B → 1.733 YH <sub>3</sub> + 2.067 YN + YB <sub>6</sub> H <sub>4</sub> C <sub>6</sub> N                                              | -0.1024             |
| YNH <sub>4</sub> B <sub>6</sub> C <sub>6</sub>  | 1.2 Y <sub>4</sub> C <sub>5</sub> + YN + 11.45 H <sub>2</sub> + 1.5 YB <sub>4</sub> → 6.3 YH <sub>3</sub> + YB <sub>6</sub> H <sub>4</sub> C <sub>6</sub> N                                        | -0.1003             |
| YNH <sub>4</sub> B <sub>6</sub> C <sub>6</sub>  | 1.333 B <sub>13</sub> C <sub>2</sub> + 3.333 Y <sub>2</sub> C + 1.333 H <sub>3</sub> N → 0.1667 N <sub>2</sub> + 5.667 YB <sub>2</sub> + YB <sub>6</sub> H <sub>4</sub> C <sub>6</sub> N           | -0.0867             |
| YNH <sub>4</sub> B <sub>6</sub> C <sub>6</sub>  | 0.6667 B <sub>9</sub> H <sub>11</sub> + 4.311 Y + 1.2 H <sub>8</sub> C <sub>5</sub> + YN → 4.311 YH <sub>3</sub> + YB <sub>6</sub> H <sub>4</sub> C <sub>6</sub> N                                 | -0.0839             |
| YNH <sub>4</sub> B <sub>6</sub> C <sub>6</sub>  | 6 Y <sub>2</sub> C + 9.667 H <sub>3</sub> N + 1.5 YB <sub>4</sub> → 12.5 YH <sub>2</sub> + 4.333 N <sub>2</sub> + YB <sub>6</sub> H <sub>4</sub> C <sub>6</sub> N                                  | -0.0826             |
| YNH <sub>4</sub> B <sub>6</sub> C <sub>6</sub>  | 0.5 YH <sub>2</sub> + H <sub>3</sub> N + 0.8571 Y <sub>4</sub> C <sub>7</sub> + 17.71 B → 2.929 YB <sub>4</sub> + YB <sub>6</sub> H <sub>4</sub> C <sub>6</sub> N                                  | -0.0770             |
| YNH <sub>4</sub> B <sub>6</sub> C <sub>6</sub>  | 3.65 C + 2.35 Y <sub>2</sub> C + H <sub>3</sub> N + 1.2 B <sub>5</sub> H <sub>7</sub> → 3.7 YH <sub>2</sub> + YB <sub>6</sub> H <sub>4</sub> C <sub>6</sub> N                                      | -0.0751             |
| YNH <sub>4</sub> B <sub>6</sub> C <sub>6</sub>  | 1.275 B <sub>9</sub> H <sub>11</sub> + 1.2 Y <sub>4</sub> C <sub>5</sub> + 0.5 N <sub>2</sub> → 3.343 YH <sub>3</sub> + 0.4566 YB <sub>12</sub> + YB <sub>6</sub> H <sub>4</sub> C <sub>6</sub> N  | -0.0657             |
| YNH <sub>4</sub> B <sub>6</sub> C <sub>6</sub>  | 3 B <sub>13</sub> C <sub>2</sub> + 4.071 Y + 0.5714 B <sub>5</sub> H <sub>7</sub> + BN → 3.071 YB <sub>12</sub> + YB <sub>6</sub> H <sub>4</sub> C <sub>6</sub> N                                  | -0.0562             |
| YNH <sub>4</sub> B <sub>6</sub> C <sub>6</sub>  | H <sub>3</sub> N + 0.1429 B <sub>5</sub> H <sub>7</sub> + 0.8571 Y <sub>4</sub> C <sub>7</sub> + 34.43 B → 2.429 YB <sub>12</sub> + YB <sub>6</sub> H <sub>4</sub> C <sub>6</sub> N                | -0.0512             |
| YNH <sub>4</sub> B <sub>6</sub> C <sub>6</sub>  | 0.3333 YH <sub>3</sub> + 3 B <sub>13</sub> C <sub>2</sub> + 3.417 Y + H <sub>3</sub> N → 2.75 YB <sub>12</sub> + YB <sub>6</sub> H <sub>4</sub> C <sub>6</sub> N                                   | -0.0505             |
| YNH <sub>4</sub> B <sub>6</sub> C <sub>6</sub>  | 1.333 H <sub>3</sub> N + 0.8571 Y <sub>4</sub> C <sub>7</sub> + 16.05 B → 0.3333 BN + 2.429 YB <sub>4</sub> + YB <sub>6</sub> H <sub>4</sub> C <sub>6</sub> N                                      | -0.0479             |
| YNH <sub>4</sub> B <sub>6</sub> C <sub>6</sub>  | 0.5 YH <sub>2</sub> + 1.381 B <sub>13</sub> C <sub>2</sub> + 3.238 Y <sub>2</sub> C + H <sub>3</sub> N → 5.976 YB <sub>2</sub> + YB <sub>6</sub> H <sub>4</sub> C <sub>6</sub> N                   | -0.0465             |
| YNH <sub>4</sub> B <sub>6</sub> C <sub>6</sub>  | 0.6667 B <sub>9</sub> H <sub>11</sub> + 2.491 Y <sub>2</sub> C + H <sub>3</sub> N + 0.7018 H <sub>8</sub> C <sub>5</sub> → 3.982 YH <sub>3</sub> + YB <sub>6</sub> H <sub>4</sub> C <sub>6</sub> N | -0.0441             |
| YNH <sub>4</sub> B <sub>6</sub> C <sub>6</sub>  | 1.333 YH <sub>3</sub> + 0.8571 Y <sub>4</sub> C <sub>7</sub> + BN + 50.14 B → 3.762 YB <sub>12</sub> + YB <sub>6</sub> H <sub>4</sub> C <sub>6</sub> N                                             | -0.0386             |
| YNH <sub>4</sub> B <sub>6</sub> C <sub>6</sub>  | 0.09091 B <sub>9</sub> H <sub>11</sub> + H <sub>3</sub> N + 0.8571 Y <sub>4</sub> C <sub>7</sub> + 34.32 B → 2.429 YB <sub>12</sub> + YB <sub>6</sub> H <sub>4</sub> C <sub>6</sub> N              | -0.0356             |
| AcNH <sub>4</sub> B <sub>6</sub> C <sub>6</sub> | 34 H <sub>3</sub> N + 50 Ac + 3 B <sub>13</sub> C <sub>2</sub> → 33 BN + 49 AcH <sub>2</sub> + AcB <sub>6</sub> H <sub>4</sub> C <sub>6</sub> N                                                    | -115.1753           |
| AcNH <sub>4</sub> B <sub>6</sub> C <sub>6</sub> | 0.3636 B <sub>9</sub> H <sub>11</sub> + 18.64 N <sub>2</sub> + Ac + 3 B <sub>13</sub> C <sub>2</sub> → 36.27 BN + AcB <sub>6</sub> H <sub>4</sub> C <sub>6</sub> N                                 | -85.0094            |
| AcNH <sub>4</sub> B <sub>6</sub> C <sub>6</sub> | 0.5714 B <sub>5</sub> H <sub>7</sub> + 18.43 N <sub>2</sub> + Ac + 3 B <sub>13</sub> C <sub>2</sub> → 35.86 BN + AcB <sub>6</sub> H <sub>4</sub> C <sub>6</sub> N                                  | -84.0050            |
| AcNH <sub>4</sub> B <sub>6</sub> C <sub>6</sub> | 0.1818 B <sub>9</sub> H <sub>11</sub> + AcH <sub>2</sub> + 17.82 N <sub>2</sub> + 3 B <sub>13</sub> C <sub>2</sub> → 34.64 BN + AcB <sub>6</sub> H <sub>4</sub> C <sub>6</sub> N                   | -79.4466            |
| AcNH <sub>4</sub> B <sub>6</sub> C <sub>6</sub> | AcH <sub>2</sub> + 0.2857 B <sub>5</sub> H <sub>7</sub> + 17.71 N <sub>2</sub> + 3 B <sub>13</sub> C <sub>2</sub> → 34.43 BN + AcB <sub>6</sub> H <sub>4</sub> C <sub>6</sub> N                    | -78.9444            |
| AcNH <sub>4</sub> B <sub>6</sub> C <sub>6</sub> | 2 H <sub>2</sub> + 17 N <sub>2</sub> + Ac + 3 B <sub>13</sub> C <sub>2</sub> → 33 BN + AcB <sub>6</sub> H <sub>4</sub> C <sub>6</sub> N                                                            | -77.2685            |
| AcNH <sub>4</sub> B <sub>6</sub> C <sub>6</sub> | H <sub>2</sub> + AcH <sub>2</sub> + 17 N <sub>2</sub> + 3 B <sub>13</sub> C <sub>2</sub> → 33 BN + AcB <sub>6</sub> H <sub>4</sub> C <sub>6</sub> N                                                | -75.5762            |
| AcNH <sub>4</sub> B <sub>6</sub> C <sub>6</sub> | 1.333 H <sub>3</sub> N + 16.33 N <sub>2</sub> + Ac + 3 B <sub>13</sub> C <sub>2</sub> → 33 BN + AcB <sub>6</sub> H <sub>4</sub> C <sub>6</sub> N                                                   | -75.5031            |
| AcNH <sub>4</sub> B <sub>6</sub> C <sub>6</sub> | AcH <sub>2</sub> + 0.6667 H <sub>3</sub> N + 16.67 N <sub>2</sub> + 3 B <sub>13</sub> C <sub>2</sub> → 33 BN + AcB <sub>6</sub> H <sub>4</sub> C <sub>6</sub> N                                    | -74.6935            |
| AcNH <sub>4</sub> B <sub>6</sub> C <sub>6</sub> | 2 AcH <sub>2</sub> + 17 N <sub>2</sub> + 3 B <sub>13</sub> C <sub>2</sub> → 33 BN + Ac + AcB <sub>6</sub> H <sub>4</sub> C <sub>6</sub> N                                                          | -73.8838            |
| AcNH <sub>4</sub> B <sub>6</sub> C <sub>6</sub> | 0.25 H <sub>8</sub> C <sub>5</sub> + AcH <sub>2</sub> + 12.94 N <sub>2</sub> + 2.375 B <sub>13</sub> C <sub>2</sub> → 24.88 BN + AcB <sub>6</sub> H <sub>4</sub> C <sub>6</sub> N                  | -54.9347            |
| AcNH <sub>4</sub> B <sub>6</sub> C <sub>6</sub> | 0.5 H <sub>8</sub> C <sub>5</sub> + 8.875 N <sub>2</sub> + Ac + 1.75 B <sub>13</sub> C <sub>2</sub> → 16.75 BN + AcB <sub>6</sub> H <sub>4</sub> C <sub>6</sub> N                                  | -35.9856            |
| AcNH <sub>4</sub> B <sub>6</sub> C <sub>6</sub> | 34 H <sub>3</sub> N + Ac + 3 B <sub>13</sub> C <sub>2</sub> → 49 H <sub>2</sub> + 33 BN + AcB <sub>6</sub> H <sub>4</sub> C <sub>6</sub> N                                                         | -32.2502            |
| AcNH <sub>4</sub> B <sub>6</sub> C <sub>6</sub> | AcH <sub>2</sub> + 34 H <sub>3</sub> N + 3 B <sub>13</sub> C <sub>2</sub> → 50 H <sub>2</sub> + 33 BN + AcB <sub>6</sub> H <sub>4</sub> C <sub>6</sub> N                                           | -30.5578            |
| AcNH <sub>4</sub> B <sub>6</sub> C <sub>6</sub> | 11.73 H <sub>3</sub> N + Ac + 3 B <sub>13</sub> C <sub>2</sub> → 10.73 BN + 4.455 B <sub>5</sub> H <sub>7</sub> + AcB <sub>6</sub> H <sub>4</sub> C <sub>6</sub> N                                 | -9.2272             |
| AcNH <sub>4</sub> B <sub>6</sub> C <sub>6</sub> | 10.79 H <sub>3</sub> N + Ac + 3 B <sub>13</sub> C <sub>2</sub> → 2.579 B <sub>9</sub> H <sub>11</sub> + 9.789 BN + AcB <sub>6</sub> H <sub>4</sub> C <sub>6</sub> N                                | -8.0834             |
| AcNH <sub>4</sub> B <sub>6</sub> C <sub>6</sub> | AcH <sub>2</sub> + 11.27 H <sub>3</sub> N + 3 B <sub>13</sub> C <sub>2</sub> → 10.27 BN + 4.545 B <sub>5</sub> H <sub>7</sub> + AcB <sub>6</sub> H <sub>4</sub> C <sub>6</sub> N                   | -7.0650             |
| AcNH <sub>4</sub> B <sub>6</sub> C <sub>6</sub> | AcH <sub>2</sub> + 10.32 H <sub>3</sub> N + 3 B <sub>13</sub> C <sub>2</sub> → 2.632 B <sub>9</sub> H <sub>11</sub> + 9.316 BN + AcB <sub>6</sub> H <sub>4</sub> C <sub>6</sub> N                  | -5.8979             |

Continued on next page

Continued

| Compound                                        | Chemical reaction                                                                                                                                                                                      | Reaction energy(eV) |
|-------------------------------------------------|--------------------------------------------------------------------------------------------------------------------------------------------------------------------------------------------------------|---------------------|
| AcNH <sub>4</sub> B <sub>6</sub> C <sub>6</sub> | 1.2 H <sub>8</sub> C <sub>5</sub> + H <sub>3</sub> N + 1.2 B <sub>5</sub> H <sub>7</sub> + 9.5 Ac → 8.5 AcH <sub>2</sub> + AcB <sub>6</sub> H <sub>4</sub> C <sub>6</sub> N                            | -5.3970             |
| AcNH <sub>4</sub> B <sub>6</sub> C <sub>6</sub> | 0.6667 B <sub>9</sub> H <sub>11</sub> + 1.2 H <sub>8</sub> C <sub>5</sub> + H <sub>3</sub> N + 8.967 Ac → 7.967 AcH <sub>2</sub> + AcB <sub>6</sub> H <sub>4</sub> C <sub>6</sub> N                    | -4.5395             |
| AcNH <sub>4</sub> B <sub>6</sub> C <sub>6</sub> | 1.2 H <sub>8</sub> C <sub>5</sub> + 1.2 B <sub>5</sub> H <sub>7</sub> + 0.5 N <sub>2</sub> + 8 Ac → 7 AcH <sub>2</sub> + AcB <sub>6</sub> H <sub>4</sub> C <sub>6</sub> N                              | -4.1825             |
| AcNH <sub>4</sub> B <sub>6</sub> C <sub>6</sub> | 0.6667 B <sub>9</sub> H <sub>11</sub> + 1.2 H <sub>8</sub> C <sub>5</sub> + 0.5 N <sub>2</sub> + 7.467 Ac → 6.467 AcH <sub>2</sub> + AcB <sub>6</sub> H <sub>4</sub> C <sub>6</sub> N                  | -3.3250             |
| AcNH <sub>4</sub> B <sub>6</sub> C <sub>6</sub> | BN + 1.2 H <sub>8</sub> C <sub>5</sub> + B <sub>5</sub> H <sub>7</sub> + 7.3 Ac → 6.3 AcH <sub>2</sub> + AcB <sub>6</sub> H <sub>4</sub> C <sub>6</sub> N                                              | -0.6402             |
| AcNH <sub>4</sub> B <sub>6</sub> C <sub>6</sub> | 6 C + H <sub>3</sub> N + 1.2 B <sub>5</sub> H <sub>7</sub> + 4.7 Ac → 3.7 AcH <sub>2</sub> + AcB <sub>6</sub> H <sub>4</sub> C <sub>6</sub> N                                                          | -0.2760             |
| CaNH <sub>4</sub> B <sub>6</sub> C <sub>6</sub> | 3 B <sub>13</sub> C <sub>2</sub> + 98 CaN <sub>2</sub> + 18 B <sub>9</sub> H <sub>11</sub> → 97 CaH <sub>2</sub> + 195 BN + CaB <sub>6</sub> H <sub>4</sub> C <sub>6</sub> N                           | -472.6116           |
| CaNH <sub>4</sub> B <sub>6</sub> C <sub>6</sub> | 3 B <sub>13</sub> C <sub>2</sub> + 62 CaN <sub>2</sub> + 18 B <sub>5</sub> H <sub>7</sub> → 61 CaH <sub>2</sub> + 123 BN + CaB <sub>6</sub> H <sub>4</sub> C <sub>6</sub> N                            | -296.3304           |
| CaNH <sub>4</sub> B <sub>6</sub> C <sub>6</sub> | 34 H <sub>3</sub> N + 3 B <sub>13</sub> C <sub>2</sub> + 50 Ca → 49 CaH <sub>2</sub> + 33 BN + CaB <sub>6</sub> H <sub>4</sub> C <sub>6</sub> N                                                        | -113.0566           |
| CaNH <sub>4</sub> B <sub>6</sub> C <sub>6</sub> | 34 Ca <sub>2</sub> N + 69 H <sub>2</sub> + 3 B <sub>13</sub> C <sub>2</sub> → 67 CaH <sub>2</sub> + 33 BN + CaB <sub>6</sub> H <sub>4</sub> C <sub>6</sub> N                                           | -110.5865           |
| CaNH <sub>4</sub> B <sub>6</sub> C <sub>6</sub> | 2 CaH <sub>2</sub> + 4 B <sub>13</sub> C <sub>2</sub> + 23.5 N <sub>2</sub> → 46 BN + CaC <sub>2</sub> + CaB <sub>6</sub> H <sub>4</sub> C <sub>6</sub> N                                              | -105.5774           |
| CaNH <sub>4</sub> B <sub>6</sub> C <sub>6</sub> | 3 B <sub>13</sub> C <sub>2</sub> + 36.5 CaN <sub>2</sub> + 20 B <sub>9</sub> H <sub>11</sub> → 35.5 CaB <sub>6</sub> + 72 H <sub>3</sub> N + CaB <sub>6</sub> H <sub>4</sub> C <sub>6</sub> N          | -97.1859            |
| CaNH <sub>4</sub> B <sub>6</sub> C <sub>6</sub> | CaB <sub>6</sub> + 3 B <sub>13</sub> C <sub>2</sub> + 0.3636 B <sub>9</sub> H <sub>11</sub> + 21.64 N <sub>2</sub> → 42.27 BN + CaB <sub>6</sub> H <sub>4</sub> C <sub>6</sub> N                       | -96.9406            |
| CaNH <sub>4</sub> B <sub>6</sub> C <sub>6</sub> | CaB <sub>6</sub> + 3 B <sub>13</sub> C <sub>2</sub> + 0.5714 B <sub>5</sub> H <sub>7</sub> + 21.43 N <sub>2</sub> → 41.86 BN + CaB <sub>6</sub> H <sub>4</sub> C <sub>6</sub> N                        | -95.9362            |
| CaNH <sub>4</sub> B <sub>6</sub> C <sub>6</sub> | 52 H <sub>2</sub> + 3 B <sub>13</sub> C <sub>2</sub> + 17 Ca <sub>3</sub> N <sub>2</sub> → 50 CaH <sub>2</sub> + 33 BN + CaB <sub>6</sub> H <sub>4</sub> C <sub>6</sub> N                              | -92.2966            |
| CaNH <sub>4</sub> B <sub>6</sub> C <sub>6</sub> | CaB <sub>6</sub> + 2 H <sub>2</sub> + 3 B <sub>13</sub> C <sub>2</sub> + 20 N <sub>2</sub> → 39 BN + CaB <sub>6</sub> H <sub>4</sub> C <sub>6</sub> N                                                  | -89.1998            |
| CaNH <sub>4</sub> B <sub>6</sub> C <sub>6</sub> | CaB <sub>6</sub> + 1.333 H <sub>3</sub> N + 3 B <sub>13</sub> C <sub>2</sub> + 19.33 N <sub>2</sub> → 39 BN + CaB <sub>6</sub> H <sub>4</sub> C <sub>6</sub> N                                         | -87.4343            |
| CaNH <sub>4</sub> B <sub>6</sub> C <sub>6</sub> | 3 B <sub>13</sub> C <sub>2</sub> + 0.3636 B <sub>9</sub> H <sub>11</sub> + 18.64 N <sub>2</sub> + Ca → 36.27 BN + CaB <sub>6</sub> H <sub>4</sub> C <sub>6</sub> N                                     | -84.3975            |
| CaNH <sub>4</sub> B <sub>6</sub> C <sub>6</sub> | 3 B <sub>13</sub> C <sub>2</sub> + 0.5714 B <sub>5</sub> H <sub>7</sub> + 18.43 N <sub>2</sub> + Ca → 35.86 BN + CaB <sub>6</sub> H <sub>4</sub> C <sub>6</sub> N                                      | -83.3930            |
| CaNH <sub>4</sub> B <sub>6</sub> C <sub>6</sub> | 0.5 Ca <sub>2</sub> N + 3 B <sub>13</sub> C <sub>2</sub> + 0.3636 B <sub>9</sub> H <sub>11</sub> + 18.39 N <sub>2</sub> → 36.27 BN + CaB <sub>6</sub> H <sub>4</sub> C <sub>6</sub> N                  | -83.2593            |
| CaNH <sub>4</sub> B <sub>6</sub> C <sub>6</sub> | 3 B <sub>13</sub> C <sub>2</sub> + 0.3333 Ca <sub>3</sub> N <sub>2</sub> + 0.3636 B <sub>9</sub> H <sub>11</sub> + 18.3 N <sub>2</sub> → 36.27 BN + CaB <sub>6</sub> H <sub>4</sub> C <sub>6</sub> N   | -83.0751            |
| CaNH <sub>4</sub> B <sub>6</sub> C <sub>6</sub> | 3 B <sub>13</sub> C <sub>2</sub> + CaN <sub>2</sub> + 0.3636 B <sub>9</sub> H <sub>11</sub> + 17.64 N <sub>2</sub> → 36.27 BN + CaB <sub>6</sub> H <sub>4</sub> C <sub>6</sub> N                       | -82.8832            |
| CaNH <sub>4</sub> B <sub>6</sub> C <sub>6</sub> | 0.5 Ca <sub>2</sub> N + 3 B <sub>13</sub> C <sub>2</sub> + 0.5714 B <sub>5</sub> H <sub>7</sub> + 18.18 N <sub>2</sub> → 35.86 BN + CaB <sub>6</sub> H <sub>4</sub> C <sub>6</sub> N                   | -82.2548            |
| CaNH <sub>4</sub> B <sub>6</sub> C <sub>6</sub> | 3 B <sub>13</sub> C <sub>2</sub> + 0.3333 Ca <sub>3</sub> N <sub>2</sub> + 0.5714 B <sub>5</sub> H <sub>7</sub> + 18.1 N <sub>2</sub> → 35.86 BN + CaB <sub>6</sub> H <sub>4</sub> C <sub>6</sub> N    | -82.0707            |
| CaNH <sub>4</sub> B <sub>6</sub> C <sub>6</sub> | 3 B <sub>13</sub> C <sub>2</sub> + CaN <sub>2</sub> + 0.5714 B <sub>5</sub> H <sub>7</sub> + 17.43 N <sub>2</sub> → 35.86 BN + CaB <sub>6</sub> H <sub>4</sub> C <sub>6</sub> N                        | -81.8788            |
| CaNH <sub>4</sub> B <sub>6</sub> C <sub>6</sub> | CaH <sub>2</sub> + 3 B <sub>13</sub> C <sub>2</sub> + 0.1818 B <sub>9</sub> H <sub>11</sub> + 17.82 N <sub>2</sub> → 34.64 BN + CaB <sub>6</sub> H <sub>4</sub> C <sub>6</sub> N                       | -78.8654            |
| CaNH <sub>4</sub> B <sub>6</sub> C <sub>6</sub> | CaH <sub>2</sub> + 3 B <sub>13</sub> C <sub>2</sub> + 0.2857 B <sub>5</sub> H <sub>7</sub> + 17.71 N <sub>2</sub> → 34.43 BN + CaB <sub>6</sub> H <sub>4</sub> C <sub>6</sub> N                        | -78.3632            |
| CaNH <sub>4</sub> B <sub>6</sub> C <sub>6</sub> | 3 B <sub>13</sub> C <sub>2</sub> + 27.45 CaN <sub>2</sub> + 0.3636 B <sub>9</sub> H <sub>11</sub> → 8.818 Ca <sub>3</sub> N <sub>2</sub> + 36.27 BN + CaB <sub>6</sub> H <sub>4</sub> C <sub>6</sub> N | -77.8075            |
| CaNH <sub>4</sub> B <sub>6</sub> C <sub>6</sub> | 18 H <sub>2</sub> + 3 B <sub>13</sub> C <sub>2</sub> + 17 CaN <sub>2</sub> → 16 CaH <sub>2</sub> + 33 BN + CaB <sub>6</sub> H <sub>4</sub> C <sub>6</sub> N                                            | -77.5004            |
| CaNH <sub>4</sub> B <sub>6</sub> C <sub>6</sub> | 3 B <sub>13</sub> C <sub>2</sub> + 27.14 CaN <sub>2</sub> + 0.5714 B <sub>5</sub> H <sub>7</sub> → 8.714 Ca <sub>3</sub> N <sub>2</sub> + 35.86 BN + CaB <sub>6</sub> H <sub>4</sub> C <sub>6</sub> N  | -76.8629            |
| CaNH <sub>4</sub> B <sub>6</sub> C <sub>6</sub> | 2 H <sub>2</sub> + 3 B <sub>13</sub> C <sub>2</sub> + 17 N <sub>2</sub> + Ca → 33 BN + CaB <sub>6</sub> H <sub>4</sub> C <sub>6</sub> N                                                                | -76.6566            |
| CaNH <sub>4</sub> B <sub>6</sub> C <sub>6</sub> | 0.5 Ca <sub>2</sub> N + 2 H <sub>2</sub> + 3 B <sub>13</sub> C <sub>2</sub> + 16.75 N <sub>2</sub> → 33 BN + CaB <sub>6</sub> H <sub>4</sub> C <sub>6</sub> N                                          | -75.5184            |
| CaNH <sub>4</sub> B <sub>6</sub> C <sub>6</sub> | 2 H <sub>2</sub> + 3 B <sub>13</sub> C <sub>2</sub> + 0.3333 Ca <sub>3</sub> N <sub>2</sub> + 16.67 N <sub>2</sub> → 33 BN + CaB <sub>6</sub> H <sub>4</sub> C <sub>6</sub> N                          | -75.3342            |
| CaNH <sub>4</sub> B <sub>6</sub> C <sub>6</sub> | 2 H <sub>2</sub> + 3 B <sub>13</sub> C <sub>2</sub> + CaN <sub>2</sub> + 16 N <sub>2</sub> → 33 BN + CaB <sub>6</sub> H <sub>4</sub> C <sub>6</sub> N                                                  | -75.1424            |
| CaNH <sub>4</sub> B <sub>6</sub> C <sub>6</sub> | H <sub>2</sub> + CaH <sub>2</sub> + 3 B <sub>13</sub> C <sub>2</sub> + 17 N <sub>2</sub> → 33 BN + CaB <sub>6</sub> H <sub>4</sub> C <sub>6</sub> N                                                    | -74.9950            |
| CaNH <sub>4</sub> B <sub>6</sub> C <sub>6</sub> | 1.333 H <sub>3</sub> N + 3 B <sub>13</sub> C <sub>2</sub> + 16.33 N <sub>2</sub> + Ca → 33 BN + CaB <sub>6</sub> H <sub>4</sub> C <sub>6</sub> N                                                       | -74.8912            |
| CaNH <sub>4</sub> B <sub>6</sub> C <sub>6</sub> | 2 CaH <sub>2</sub> + 3 B <sub>13</sub> C <sub>2</sub> + 18 N <sub>2</sub> → CaN <sub>2</sub> + 33 BN + CaB <sub>6</sub> H <sub>4</sub> C <sub>6</sub> N                                                | -74.8476            |
| CaNH <sub>4</sub> B <sub>6</sub> C <sub>6</sub> | 2 CaH <sub>2</sub> + 3 B <sub>13</sub> C <sub>2</sub> + 17.33 N <sub>2</sub> → 0.3333 Ca <sub>3</sub> N <sub>2</sub> + 33 BN + CaB <sub>6</sub> H <sub>4</sub> C <sub>6</sub> N                        | -74.6557            |
| CaNH <sub>4</sub> B <sub>6</sub> C <sub>6</sub> | 2 CaH <sub>2</sub> + 3 B <sub>13</sub> C <sub>2</sub> + 17.25 N <sub>2</sub> → 0.5 Ca <sub>2</sub> N + 33 BN + CaB <sub>6</sub> H <sub>4</sub> C <sub>6</sub> N                                        | -74.4716            |
| CaNH <sub>4</sub> B <sub>6</sub> C <sub>6</sub> | CaH <sub>2</sub> + 0.6667 H <sub>3</sub> N + 3 B <sub>13</sub> C <sub>2</sub> + 16.67 N <sub>2</sub> → 33 BN + CaB <sub>6</sub> H <sub>4</sub> C <sub>6</sub> N                                        | -74.1123            |
| CaNH <sub>4</sub> B <sub>6</sub> C <sub>6</sub> | 3 B <sub>13</sub> C <sub>2</sub> + 24.52 CaN <sub>2</sub> + 0.3636 B <sub>9</sub> H <sub>11</sub> → 11.76 Ca <sub>2</sub> N + 36.27 BN + CaB <sub>6</sub> H <sub>4</sub> C <sub>6</sub> N              | -74.0410            |
| CaNH <sub>4</sub> B <sub>6</sub> C <sub>6</sub> | 0.5 Ca <sub>2</sub> N + 1.333 H <sub>3</sub> N + 3 B <sub>13</sub> C <sub>2</sub> + 16.08 N <sub>2</sub> → 33 BN + CaB <sub>6</sub> H <sub>4</sub> C <sub>6</sub> N                                    | -73.7530            |
| CaNH <sub>4</sub> B <sub>6</sub> C <sub>6</sub> | 1.333 H <sub>3</sub> N + 3 B <sub>13</sub> C <sub>2</sub> + 0.3333 Ca <sub>3</sub> N <sub>2</sub> + 16 N <sub>2</sub> → 33 BN + CaB <sub>6</sub> H <sub>4</sub> C <sub>6</sub> N                       | -73.5688            |
| CaNH <sub>4</sub> B <sub>6</sub> C <sub>6</sub> | 1.333 H <sub>3</sub> N + 3 B <sub>13</sub> C <sub>2</sub> + CaN <sub>2</sub> + 15.33 N <sub>2</sub> → 33 BN + CaB <sub>6</sub> H <sub>4</sub> C <sub>6</sub> N                                         | -73.3769            |
| CaNH <sub>4</sub> B <sub>6</sub> C <sub>6</sub> | 2 CaH <sub>2</sub> + 3 B <sub>13</sub> C <sub>2</sub> + 17 N <sub>2</sub> → 33 BN + Ca + CaB <sub>6</sub> H <sub>4</sub> C <sub>6</sub> N                                                              | -73.3334            |
| CaNH <sub>4</sub> B <sub>6</sub> C <sub>6</sub> | 3 B <sub>13</sub> C <sub>2</sub> + 24.24 CaN <sub>2</sub> + 0.5714 B <sub>5</sub> H <sub>7</sub> → 11.62 Ca <sub>2</sub> N + 35.86 BN + CaB <sub>6</sub> H <sub>4</sub> C <sub>6</sub> N               | -73.1407            |
| CaNH <sub>4</sub> B <sub>6</sub> C <sub>6</sub> | 2 H <sub>2</sub> + 3 B <sub>13</sub> C <sub>2</sub> + 25 CaN <sub>2</sub> → 8 Ca <sub>3</sub> N <sub>2</sub> + 33 BN + CaB <sub>6</sub> H <sub>4</sub> C <sub>6</sub> N                                | -70.5376            |
| CaNH <sub>4</sub> B <sub>6</sub> C <sub>6</sub> | 2 CaH <sub>2</sub> + 3 B <sub>13</sub> C <sub>2</sub> + 26 CaN <sub>2</sub> → 9 Ca <sub>3</sub> N <sub>2</sub> + 33 BN + CaB <sub>6</sub> H <sub>4</sub> C <sub>6</sub> N                              | -69.6672            |
| CaNH <sub>4</sub> B <sub>6</sub> C <sub>6</sub> | 1.333 H <sub>3</sub> N + 3 B <sub>13</sub> C <sub>2</sub> + 24 CaN <sub>2</sub> → 7.667 Ca <sub>3</sub> N <sub>2</sub> + 33 BN + CaB <sub>6</sub> H <sub>4</sub> C <sub>6</sub> N                      | -68.9640            |
| CaNH <sub>4</sub> B <sub>6</sub> C <sub>6</sub> | 2 H <sub>2</sub> + 3 B <sub>13</sub> C <sub>2</sub> + 22.33 CaN <sub>2</sub> → 10.67 Ca <sub>2</sub> N + 33 BN + CaB <sub>6</sub> H <sub>4</sub> C <sub>6</sub> N                                      | -67.1205            |
| CaNH <sub>4</sub> B <sub>6</sub> C <sub>6</sub> | 2 CaH <sub>2</sub> + 3 B <sub>13</sub> C <sub>2</sub> + 23 CaN <sub>2</sub> → 12 Ca <sub>2</sub> N + 33 BN + CaB <sub>6</sub> H <sub>4</sub> C <sub>6</sub> N                                          | -65.8230            |
| CaNH <sub>4</sub> B <sub>6</sub> C <sub>6</sub> | 1.333 H <sub>3</sub> N + 3 B <sub>13</sub> C <sub>2</sub> + 21.44 CaN <sub>2</sub> → 10.22 Ca <sub>2</sub> N + 33 BN + CaB <sub>6</sub> H <sub>4</sub> C <sub>6</sub> N                                | -65.6893            |
| CaNH <sub>4</sub> B <sub>6</sub> C <sub>6</sub> | 9 H <sub>3</sub> N + 3 B <sub>13</sub> C <sub>2</sub> + 12.5 CaN <sub>2</sub> → 11.5 CaH <sub>2</sub> + 33 BN + CaB <sub>6</sub> H <sub>4</sub> C <sub>6</sub> N                                       | -64.9206            |
| CaNH <sub>4</sub> B <sub>6</sub> C <sub>6</sub> | 14.29 Ca <sub>2</sub> N + 19.71 H <sub>3</sub> N + 3 B <sub>13</sub> C <sub>2</sub> → 27.57 CaH <sub>2</sub> + 33 BN + CaB <sub>6</sub> H <sub>4</sub> C <sub>6</sub> N                                | -63.8463            |
| CaNH <sub>4</sub> B <sub>6</sub> C <sub>6</sub> | 2 CaH <sub>2</sub> + 3 B <sub>13</sub> C <sub>2</sub> + 14 N <sub>2</sub> → CaB <sub>6</sub> + 27 BN + CaB <sub>6</sub> H <sub>4</sub> C <sub>6</sub> N                                                | -60.7902            |
| CaNH <sub>4</sub> B <sub>6</sub> C <sub>6</sub> | 17.33 H <sub>3</sub> N + 3 B <sub>13</sub> C <sub>2</sub> + 8.333 Ca <sub>3</sub> N <sub>2</sub> → 24 CaH <sub>2</sub> + 33 BN + CaB <sub>6</sub> H <sub>4</sub> C <sub>6</sub> N                      | -60.5256            |
| CaNH <sub>4</sub> B <sub>6</sub> C <sub>6</sub> | 3 B <sub>13</sub> C <sub>2</sub> + 23.17 CaN <sub>2</sub> + 20 B <sub>5</sub> H <sub>7</sub> → 22.17 CaB <sub>6</sub> + 45.33 H <sub>3</sub> N + CaB <sub>6</sub> H <sub>4</sub> C <sub>6</sub> N      | -59.3366            |
| CaNH <sub>4</sub> B <sub>6</sub> C <sub>6</sub> | 3 B <sub>13</sub> C <sub>2</sub> + 18.64 CaN <sub>2</sub> + 0.3636 B <sub>9</sub> H <sub>11</sub> → 36.27 BN + 17.64 Ca + CaB <sub>6</sub> H <sub>4</sub> C <sub>6</sub> N                             | -56.1779            |
| CaNH <sub>4</sub> B <sub>6</sub> C <sub>6</sub> | 3 B <sub>13</sub> C <sub>2</sub> + 18.43 CaN <sub>2</sub> + 0.5714 B <sub>5</sub> H <sub>7</sub> → 35.86 BN + 17.43 Ca + CaB <sub>6</sub> H <sub>4</sub> C <sub>6</sub> N                              | -55.4881            |
| CaNH <sub>4</sub> B <sub>6</sub> C <sub>6</sub> | CaH <sub>2</sub> + 2.375 B <sub>13</sub> C <sub>2</sub> + 12.94 N <sub>2</sub> + 0.25 H <sub>8</sub> C <sub>5</sub> → 24.88 BN + CaB <sub>6</sub> H <sub>4</sub> C <sub>6</sub> N                      | -54.3535            |

Continued on next page

Continued

| Compound                            | Chemical reaction                                                                                                                                                                        | Reaction energy(eV) |
|-------------------------------------|------------------------------------------------------------------------------------------------------------------------------------------------------------------------------------------|---------------------|
| $\text{CaNH}_4\text{B}_6\text{C}_6$ | $2\text{B}_{13}\text{C}_2 + 0.3636\text{B}_9\text{H}_{11} + 12.14\text{N}_2 + \text{CaC}_2 \rightarrow 23.27\text{BN} + \text{CaB}_6\text{H}_4\text{C}_6\text{N}$                        | -52.1534            |
| $\text{CaNH}_4\text{B}_6\text{C}_6$ | $2\text{B}_{13}\text{C}_2 + 0.5714\text{B}_5\text{H}_7 + 11.93\text{N}_2 + \text{CaC}_2 \rightarrow 22.86\text{BN} + \text{CaB}_6\text{H}_4\text{C}_6\text{N}$                           | -51.1490            |
| $\text{CaNH}_4\text{B}_6\text{C}_6$ | $2\text{H}_2 + 3\text{B}_{13}\text{C}_2 + 17\text{CaN}_2 \rightarrow 33\text{BN} + 16\text{Ca} + \text{CaB}_6\text{H}_4\text{C}_6\text{N}$                                               | -50.9148            |
| $\text{CaNH}_4\text{B}_6\text{C}_6$ | $1.333\text{H}_3\text{N} + 3\text{B}_{13}\text{C}_2 + 16.33\text{CaN}_2 \rightarrow 33\text{BN} + 15.33\text{Ca} + \text{CaB}_6\text{H}_4\text{C}_6\text{N}$                             | -50.1589            |
| $\text{CaNH}_4\text{B}_6\text{C}_6$ | $\text{CaB}_6 + 1.75\text{B}_{13}\text{C}_2 + 11.88\text{N}_2 + 0.5\text{H}_8\text{C}_5 \rightarrow 22.75\text{BN} + \text{CaB}_6\text{H}_4\text{C}_6\text{N}$                           | -47.9169            |
| $\text{CaNH}_4\text{B}_6\text{C}_6$ | $2\text{CaH}_2 + 3\text{B}_{13}\text{C}_2 + 17\text{CaN}_2 \rightarrow 33\text{BN} + 18\text{Ca} + \text{CaB}_6\text{H}_4\text{C}_6\text{N}$                                             | -47.5916            |
| $\text{CaNH}_4\text{B}_6\text{C}_6$ | $2\text{H}_2 + 2\text{B}_{13}\text{C}_2 + 10.5\text{N}_2 + \text{CaC}_2 \rightarrow 20\text{BN} + \text{CaB}_6\text{H}_4\text{C}_6\text{N}$                                              | -44.4125            |
| $\text{CaNH}_4\text{B}_6\text{C}_6$ | $1.333\text{H}_3\text{N} + 2\text{B}_{13}\text{C}_2 + 9.833\text{N}_2 + \text{CaC}_2 \rightarrow 20\text{BN} + \text{CaB}_6\text{H}_4\text{C}_6\text{N}$                                 | -42.6471            |
| $\text{CaNH}_4\text{B}_6\text{C}_6$ | $3\text{B}_{13}\text{C}_2 + 73.55\text{Ca}_3\text{N}_2 + 0.3636\text{B}_9\text{H}_{11} \rightarrow 109.8\text{Ca}_2\text{N} + 36.27\text{BN} + \text{CaB}_6\text{H}_4\text{C}_6\text{N}$ | -42.6272            |
| $\text{CaNH}_4\text{B}_6\text{C}_6$ | $3\text{B}_{13}\text{C}_2 + 72.71\text{Ca}_3\text{N}_2 + 0.5714\text{B}_5\text{H}_7 \rightarrow 108.6\text{Ca}_2\text{N} + 35.86\text{BN} + \text{CaB}_6\text{H}_4\text{C}_6\text{N}$    | -42.0820            |
| $\text{CaNH}_4\text{B}_6\text{C}_6$ | $2\text{H}_2 + 3\text{B}_{13}\text{C}_2 + 67\text{Ca}_3\text{N}_2 \rightarrow 100\text{Ca}_2\text{N} + 33\text{BN} + \text{CaB}_6\text{H}_4\text{C}_6\text{N}$                           | -38.5026            |
| $\text{CaNH}_4\text{B}_6\text{C}_6$ | $1.333\text{H}_3\text{N} + 3\text{B}_{13}\text{C}_2 + 64.33\text{Ca}_3\text{N}_2 \rightarrow 96\text{Ca}_2\text{N} + 33\text{BN} + \text{CaB}_6\text{H}_4\text{C}_6\text{N}$             | -38.2104            |
| $\text{CaNH}_4\text{B}_6\text{C}_6$ | $2\text{CaH}_2 + 3\text{B}_{13}\text{C}_2 + 69\text{Ca}_3\text{N}_2 \rightarrow 104\text{Ca}_2\text{N} + 33\text{BN} + \text{CaB}_6\text{H}_4\text{C}_6\text{N}$                         | -36.3508            |
| $\text{CaNH}_4\text{B}_6\text{C}_6$ | $\text{CaB}_6 + 40\text{H}_3\text{N} + 3\text{B}_{13}\text{C}_2 \rightarrow 58\text{H}_2 + 39\text{BN} + \text{CaB}_6\text{H}_4\text{C}_6\text{N}$                                       | -36.2370            |
| $\text{CaNH}_4\text{B}_6\text{C}_6$ | $1.75\text{B}_{13}\text{C}_2 + 8.875\text{N}_2 + \text{Ca} + 0.5\text{H}_8\text{C}_5 \rightarrow 16.75\text{BN} + \text{CaB}_6\text{H}_4\text{C}_6\text{N}$                              | -35.3737            |
| $\text{CaNH}_4\text{B}_6\text{C}_6$ | $0.5\text{Ca}_2\text{N} + 1.75\text{B}_{13}\text{C}_2 + 8.625\text{N}_2 + 0.5\text{H}_8\text{C}_5 \rightarrow 16.75\text{BN} + \text{CaB}_6\text{H}_4\text{C}_6\text{N}$                 | -34.2355            |
| $\text{CaNH}_4\text{B}_6\text{C}_6$ | $1.75\text{B}_{13}\text{C}_2 + 0.3333\text{Ca}_3\text{N}_2 + 8.542\text{N}_2 + 0.5\text{H}_8\text{C}_5 \rightarrow 16.75\text{BN} + \text{CaB}_6\text{H}_4\text{C}_6\text{N}$            | -34.0513            |
| $\text{CaNH}_4\text{B}_6\text{C}_6$ | $1.75\text{B}_{13}\text{C}_2 + \text{CaN}_2 + 7.875\text{N}_2 + 0.5\text{H}_8\text{C}_5 \rightarrow 16.75\text{BN} + \text{CaB}_6\text{H}_4\text{C}_6\text{N}$                           | -33.8595            |
| $\text{CaNH}_4\text{B}_6\text{C}_6$ | $32\text{H}_3\text{N} + 3\text{B}_{13}\text{C}_2 + \text{CaN}_2 \rightarrow 46\text{H}_2 + 33\text{BN} + \text{CaB}_6\text{H}_4\text{C}_6\text{N}$                                       | -32.7721            |
| $\text{CaNH}_4\text{B}_6\text{C}_6$ | $34\text{H}_3\text{N} + 3\text{B}_{13}\text{C}_2 + \text{Ca} \rightarrow 49\text{H}_2 + 33\text{BN} + \text{CaB}_6\text{H}_4\text{C}_6\text{N}$                                          | -31.6382            |
| $\text{CaNH}_4\text{B}_6\text{C}_6$ | $1.75\text{B}_{13}\text{C}_2 + 12.81\text{CaN}_2 + 0.5\text{H}_8\text{C}_5 \rightarrow 3.937\text{Ca}_3\text{N}_2 + 16.75\text{BN} + \text{CaB}_6\text{H}_4\text{C}_6\text{N}$           | -31.5930            |
| $\text{CaNH}_4\text{B}_6\text{C}_6$ | $33.33\text{H}_3\text{N} + 3\text{B}_{13}\text{C}_2 + 0.3333\text{Ca}_3\text{N}_2 \rightarrow 48\text{H}_2 + 33\text{BN} + \text{CaB}_6\text{H}_4\text{C}_6\text{N}$                     | -31.1986            |
| $\text{CaNH}_4\text{B}_6\text{C}_6$ | $0.5\text{Ca}_2\text{N} + 33.5\text{H}_3\text{N} + 3\text{B}_{13}\text{C}_2 \rightarrow 48.25\text{H}_2 + 33\text{BN} + \text{CaB}_6\text{H}_4\text{C}_6\text{N}$                        | -31.1620            |
| $\text{CaNH}_4\text{B}_6\text{C}_6$ | $\text{CaH}_2 + 34\text{H}_3\text{N} + 3\text{B}_{13}\text{C}_2 \rightarrow 50\text{H}_2 + 33\text{BN} + \text{CaB}_6\text{H}_4\text{C}_6\text{N}$                                       | -29.9766            |
| $\text{CaNH}_4\text{B}_6\text{C}_6$ | $1.75\text{B}_{13}\text{C}_2 + 11.5\text{CaN}_2 + 0.5\text{H}_8\text{C}_5 \rightarrow 5.25\text{Ca}_2\text{N} + 16.75\text{BN} + \text{CaB}_6\text{H}_4\text{C}_6\text{N}$               | -29.9112            |
| $\text{CaNH}_4\text{B}_6\text{C}_6$ | $3.8\text{CaB}_6 + 8.9\text{N}_2 + 1.2\text{H}_8\text{C}_5 \rightarrow 2.8\text{CaH}_2 + 16.8\text{BN} + \text{CaB}_6\text{H}_4\text{C}_6\text{N}$                                       | -29.8942            |
| $\text{CaNH}_4\text{B}_6\text{C}_6$ | $1.75\text{B}_{13}\text{C}_2 + 8.875\text{CaN}_2 + 0.5\text{H}_8\text{C}_5 \rightarrow 16.75\text{BN} + 7.875\text{Ca} + \text{CaB}_6\text{H}_4\text{C}_6\text{N}$                       | -21.9350            |
| $\text{CaNH}_4\text{B}_6\text{C}_6$ | $3\text{B}_{13}\text{C}_2 + 5.409\text{CaN}_2 + 0.3636\text{B}_9\text{H}_{11} \rightarrow 4.409\text{CaB}_6 + 9.818\text{BN} + \text{CaB}_6\text{H}_4\text{C}_6\text{N}$                 | -20.9029            |
| $\text{CaNH}_4\text{B}_6\text{C}_6$ | $3\text{B}_{13}\text{C}_2 + 5.357\text{CaN}_2 + 0.5714\text{B}_5\text{H}_7 \rightarrow 4.357\text{CaB}_6 + 9.714\text{BN} + \text{CaB}_6\text{H}_4\text{C}_6\text{N}$                    | -20.6287            |
| $\text{CaNH}_4\text{B}_6\text{C}_6$ | $1.333\text{H}_3\text{N} + 3\text{B}_{13}\text{C}_2 + 4.833\text{CaN}_2 \rightarrow 3.833\text{CaB}_6 + 10\text{BN} + \text{CaB}_6\text{H}_4\text{C}_6\text{N}$                          | -19.4902            |
| $\text{CaNH}_4\text{B}_6\text{C}_6$ | $2\text{H}_2 + 3\text{B}_{13}\text{C}_2 + 5\text{CaN}_2 \rightarrow 4\text{CaB}_6 + 9\text{BN} + \text{CaB}_6\text{H}_4\text{C}_6\text{N}$                                               | -18.9128            |
| $\text{CaNH}_4\text{B}_6\text{C}_6$ | $21\text{H}_3\text{N} + 2\text{B}_{13}\text{C}_2 + \text{CaC}_2 \rightarrow 29.5\text{H}_2 + 20\text{BN} + \text{CaB}_6\text{H}_4\text{C}_6\text{N}$                                     | -16.6070            |
| $\text{CaNH}_4\text{B}_6\text{C}_6$ | $4.25\text{CaN}_2 + 1.5\text{B}_9\text{H}_{11} + 3\text{CaC}_2 \rightarrow 6.25\text{CaH}_2 + 7.5\text{BN} + \text{CaB}_6\text{H}_4\text{C}_6\text{N}$                                   | -15.8050            |
| $\text{CaNH}_4\text{B}_6\text{C}_6$ | $1.75\text{B}_{13}\text{C}_2 + 34.5\text{Ca}_3\text{N}_2 + 0.5\text{H}_8\text{C}_5 \rightarrow 51.25\text{Ca}_2\text{N} + 16.75\text{BN} + \text{CaB}_6\text{H}_4\text{C}_6\text{N}$     | -15.1751            |
| $\text{CaNH}_4\text{B}_6\text{C}_6$ | $4.563\text{Ca}_3\text{N}_2 + 2.825\text{B}_5\text{H}_7 + 1.2\text{H}_8\text{C}_5 \rightarrow 12.69\text{CaH}_2 + 8.125\text{BN} + \text{CaB}_6\text{H}_4\text{C}_6\text{N}$             | -13.8627            |
| $\text{CaNH}_4\text{B}_6\text{C}_6$ | $20\text{H}_2 + 3\text{B}_{13}\text{C}_2 + 6.5\text{CaN}_2 \rightarrow 5.5\text{CaB}_6 + 12\text{H}_3\text{N} + \text{CaB}_6\text{H}_4\text{C}_6\text{N}$                                | -13.7155            |
| $\text{CaNH}_4\text{B}_6\text{C}_6$ | $16.73\text{H}_3\text{N} + 3\text{B}_{13}\text{C}_2 + 32.47\text{Ca} \rightarrow 15.73\text{Ca}_2\text{N} + 6.6\text{B}_5\text{H}_7 + \text{CaB}_6\text{H}_4\text{C}_6\text{N}$          | -12.5098            |
| $\text{CaNH}_4\text{B}_6\text{C}_6$ | $2\text{CaH}_2 + 3\text{B}_{13}\text{C}_2 + 3.5\text{CaN}_2 \rightarrow 4.5\text{CaB}_6 + 6\text{BN} + \text{CaB}_6\text{H}_4\text{C}_6\text{N}$                                         | -11.5893            |
| $\text{CaNH}_4\text{B}_6\text{C}_6$ | $11.09\text{H}_3\text{N} + 3\text{B}_{13}\text{C}_2 + \text{CaN}_2 \rightarrow 12.09\text{BN} + 4.182\text{B}_5\text{H}_7 + \text{CaB}_6\text{H}_4\text{C}_6\text{N}$                    | -11.1587            |
| $\text{CaNH}_4\text{B}_6\text{C}_6$ | $3\text{B}_{13}\text{C}_2 + 18.64\text{Ca}_3\text{N}_2 + 0.3636\text{B}_9\text{H}_{11} \rightarrow 36.27\text{BN} + 54.91\text{Ca} + \text{CaB}_6\text{H}_4\text{C}_6\text{N}$           | -10.4659            |
| $\text{CaNH}_4\text{B}_6\text{C}_6$ | $14.78\text{H}_3\text{N} + 3\text{B}_{13}\text{C}_2 + 28.56\text{Ca} \rightarrow 13.78\text{Ca}_2\text{N} + 3.667\text{B}_9\text{H}_{11} + \text{CaB}_6\text{H}_4\text{C}_6\text{N}$     | -10.3995            |
| $\text{CaNH}_4\text{B}_6\text{C}_6$ | $3\text{B}_{13}\text{C}_2 + 18.43\text{Ca}_3\text{N}_2 + 0.5714\text{B}_5\text{H}_7 \rightarrow 35.86\text{BN} + 54.29\text{Ca} + \text{CaB}_6\text{H}_4\text{C}_6\text{N}$              | -10.2858            |
| $\text{CaNH}_4\text{B}_6\text{C}_6$ | $1.333\text{H}_3\text{N} + 3\text{B}_{13}\text{C}_2 + 16.33\text{Ca}_3\text{N}_2 \rightarrow 33\text{BN} + 48\text{Ca} + \text{CaB}_6\text{H}_4\text{C}_6\text{N}$                       | -10.0958            |
| $\text{CaNH}_4\text{B}_6\text{C}_6$ | $10.21\text{H}_3\text{N} + 3\text{B}_{13}\text{C}_2 + \text{CaN}_2 \rightarrow 11.21\text{BN} + 2.421\text{B}_9\text{H}_{11} + \text{CaB}_6\text{H}_4\text{C}_6\text{N}$                 | -10.0850            |
| $\text{CaNH}_4\text{B}_6\text{C}_6$ | $3.856\text{Ca}_3\text{N}_2 + 1.413\text{B}_9\text{H}_{11} + 1.2\text{H}_8\text{C}_5 \rightarrow 10.57\text{CaH}_2 + 6.713\text{BN} + \text{CaB}_6\text{H}_4\text{C}_6\text{N}$          | -9.9092             |
| $\text{CaNH}_4\text{B}_6\text{C}_6$ | $2\text{H}_2 + 3\text{B}_{13}\text{C}_2 + 17\text{Ca}_3\text{N}_2 \rightarrow 33\text{BN} + 50\text{Ca} + \text{CaB}_6\text{H}_4\text{C}_6\text{N}$                                      | -9.2166             |
| $\text{CaNH}_4\text{B}_6\text{C}_6$ | $\text{CaB}_6 + 13.64\text{H}_3\text{N} + 3\text{B}_{13}\text{C}_2 \rightarrow 12.64\text{BN} + 5.273\text{B}_5\text{H}_7 + \text{CaB}_6\text{H}_4\text{C}_6\text{N}$                    | -8.9853             |
| $\text{CaNH}_4\text{B}_6\text{C}_6$ | $3.8\text{CaN}_2 + 12.6\text{B} + 1.2\text{H}_8\text{C}_5 \rightarrow 2.8\text{CaH}_2 + 6.6\text{BN} + \text{CaB}_6\text{H}_4\text{C}_6\text{N}$                                         | -8.8172             |
| $\text{CaNH}_4\text{B}_6\text{C}_6$ | $11.52\text{H}_3\text{N} + 3\text{B}_{13}\text{C}_2 + 0.3333\text{Ca}_3\text{N}_2 \rightarrow 11.18\text{BN} + 4.364\text{B}_5\text{H}_7 + \text{CaB}_6\text{H}_4\text{C}_6\text{N}$     | -8.6455             |
| $\text{CaNH}_4\text{B}_6\text{C}_6$ | $11.73\text{H}_3\text{N} + 3\text{B}_{13}\text{C}_2 + \text{Ca} \rightarrow 10.73\text{BN} + 4.455\text{B}_5\text{H}_7 + \text{CaB}_6\text{H}_4\text{C}_6\text{N}$                       | -8.6152             |
| $\text{CaNH}_4\text{B}_6\text{C}_6$ | $3\text{B}_{13}\text{C}_2 + 0.3636\text{B}_9\text{H}_{11} + 0.5\text{N}_2 + 7.045\text{Ca} \rightarrow 6.045\text{CaB}_6 + \text{CaB}_6\text{H}_4\text{C}_6\text{N}$                     | -8.5682             |
| $\text{CaNH}_4\text{B}_6\text{C}_6$ | $0.5\text{Ca}_2\text{N} + 11.57\text{H}_3\text{N} + 3\text{B}_{13}\text{C}_2 \rightarrow 11.07\text{BN} + 4.386\text{B}_5\text{H}_7 + \text{CaB}_6\text{H}_4\text{C}_6\text{N}$          | -8.4915             |
| $\text{CaNH}_4\text{B}_6\text{C}_6$ | $3\text{B}_{13}\text{C}_2 + 0.5714\text{B}_5\text{H}_7 + 0.5\text{N}_2 + 6.976\text{Ca} \rightarrow 5.976\text{CaB}_6 + \text{CaB}_6\text{H}_4\text{C}_6\text{N}$                        | -8.4326             |
| $\text{CaNH}_4\text{B}_6\text{C}_6$ | $16.73\text{H}_3\text{N} + 3\text{B}_{13}\text{C}_2 + 24.6\text{Ca} \rightarrow 7.867\text{Ca}_3\text{N}_2 + 6.6\text{B}_5\text{H}_7 + \text{CaB}_6\text{H}_4\text{C}_6\text{N}$         | -7.9021             |
| $\text{CaNH}_4\text{B}_6\text{C}_6$ | $3\text{B}_{13}\text{C}_2 + 0.5\text{CaN}_2 + 0.3636\text{B}_9\text{H}_{11} + 6.545\text{Ca} \rightarrow 6.045\text{CaB}_6 + \text{CaB}_6\text{H}_4\text{C}_6\text{N}$                   | -7.8111             |
| $\text{CaNH}_4\text{B}_6\text{C}_6$ | $3\text{B}_{13}\text{C}_2 + 0.5\text{CaN}_2 + 0.5714\text{B}_5\text{H}_7 + 6.476\text{Ca} \rightarrow 5.976\text{CaB}_6 + \text{CaB}_6\text{H}_4\text{C}_6\text{N}$                      | -7.6755             |
| $\text{CaNH}_4\text{B}_6\text{C}_6$ | $2\text{H}_2 + 3\text{B}_{13}\text{C}_2 + 0.5\text{N}_2 + 6.5\text{Ca} \rightarrow 5.5\text{CaB}_6 + \text{CaB}_6\text{H}_4\text{C}_6\text{N}$                                           | -7.6691             |
| $\text{CaNH}_4\text{B}_6\text{C}_6$ | $\text{CaB}_6 + 12.53\text{H}_3\text{N} + 3\text{B}_{13}\text{C}_2 \rightarrow 11.53\text{BN} + 3.053\text{B}_9\text{H}_{11} + \text{CaB}_6\text{H}_4\text{C}_6\text{N}$                 | -7.6314             |
| $\text{CaNH}_4\text{B}_6\text{C}_6$ | $10.6\text{H}_3\text{N} + 3\text{B}_{13}\text{C}_2 + 0.3333\text{Ca}_3\text{N}_2 \rightarrow 10.26\text{BN} + 2.526\text{B}_9\text{H}_{11} + \text{CaB}_6\text{H}_4\text{C}_6\text{N}$   | -7.5250             |
| $\text{CaNH}_4\text{B}_6\text{C}_6$ | $10.79\text{H}_3\text{N} + 3\text{B}_{13}\text{C}_2 + \text{Ca} \rightarrow 9.789\text{BN} + 2.579\text{B}_9\text{H}_{11} + \text{CaB}_6\text{H}_4\text{C}_6\text{N}$                    | -7.4715             |

Continued on next page

Continued

| Compound                                        | Chemical reaction                                                                                                                                                                                                       | Reaction energy(eV) |
|-------------------------------------------------|-------------------------------------------------------------------------------------------------------------------------------------------------------------------------------------------------------------------------|---------------------|
| CaNH <sub>4</sub> B <sub>6</sub> C <sub>6</sub> | 0.5 Ca <sub>2</sub> N + 10.64 H <sub>3</sub> N + 3 B <sub>13</sub> C <sub>2</sub> → 10.14 BN + 2.539 B <sub>9</sub> H <sub>11</sub> + CaB <sub>6</sub> H <sub>4</sub> C <sub>6</sub> N                                  | -7.3652             |
| CaNH <sub>4</sub> B <sub>6</sub> C <sub>6</sub> | 1.333 H <sub>3</sub> N + 3 B <sub>13</sub> C <sub>2</sub> + 1.933 Ca <sub>3</sub> N <sub>2</sub> → 4.8 CaB <sub>6</sub> + 4.2 BN + CaB <sub>6</sub> H <sub>4</sub> C <sub>6</sub> N                                     | -7.0142             |
| CaNH <sub>4</sub> B <sub>6</sub> C <sub>6</sub> | 3 B <sub>13</sub> C <sub>2</sub> + 2.164 Ca <sub>3</sub> N <sub>2</sub> + 0.3636 B <sub>9</sub> H <sub>11</sub> → 5.491 CaB <sub>6</sub> + 3.327 BN + CaB <sub>6</sub> H <sub>4</sub> C <sub>6</sub> N                  | -6.9407             |
| CaNH <sub>4</sub> B <sub>6</sub> C <sub>6</sub> | 2 H <sub>2</sub> + 3 B <sub>13</sub> C <sub>2</sub> + 0.5 CaN <sub>2</sub> + 6 Ca → 5.5 CaB <sub>6</sub> + CaB <sub>6</sub> H <sub>4</sub> C <sub>6</sub> N                                                             | -6.9120             |
| CaNH <sub>4</sub> B <sub>6</sub> C <sub>6</sub> | Ca <sub>2</sub> N + 2 CaH <sub>2</sub> + 42 B + 3 CaC <sub>2</sub> → 6 CaB <sub>6</sub> + CaB <sub>6</sub> H <sub>4</sub> C <sub>6</sub> N                                                                              | -6.8696             |
| CaNH <sub>4</sub> B <sub>6</sub> C <sub>6</sub> | 5.615 Ca <sub>2</sub> N + 2.123 B <sub>5</sub> H <sub>7</sub> + 1.2 H <sub>8</sub> C <sub>5</sub> → 10.23 CaH <sub>2</sub> + 4.615 BN + CaB <sub>6</sub> H <sub>4</sub> C <sub>6</sub> N                                | -6.8227             |
| CaNH <sub>4</sub> B <sub>6</sub> C <sub>6</sub> | 3 B <sub>13</sub> C <sub>2</sub> + 2.143 Ca <sub>3</sub> N <sub>2</sub> + 0.5714 B <sub>5</sub> H <sub>7</sub> → 5.429 CaB <sub>6</sub> + 3.286 BN + CaB <sub>6</sub> H <sub>4</sub> C <sub>6</sub> N                   | -6.8006             |
| CaNH <sub>4</sub> B <sub>6</sub> C <sub>6</sub> | 1.333 H <sub>3</sub> N + 3 B <sub>13</sub> C <sub>2</sub> + 7.167 Ca → 5.5 CaB <sub>6</sub> + 0.3333 Ca <sub>2</sub> N + CaB <sub>6</sub> H <sub>4</sub> C <sub>6</sub> N                                               | -6.6625             |
| CaNH <sub>4</sub> B <sub>6</sub> C <sub>6</sub> | 3 B <sub>13</sub> C <sub>2</sub> + 3.042 Ca <sub>3</sub> N <sub>2</sub> + 1.75 B <sub>9</sub> H <sub>11</sub> → 8.125 CaB <sub>6</sub> + 5.083 H <sub>3</sub> N + CaB <sub>6</sub> H <sub>4</sub> C <sub>6</sub> N      | -6.6604             |
| CaNH <sub>4</sub> B <sub>6</sub> C <sub>6</sub> | 3.6 B <sub>5</sub> H <sub>7</sub> + 4.033 N <sub>2</sub> + 3 CaC <sub>2</sub> → 2 CaB <sub>6</sub> + 7.067 H <sub>3</sub> N + CaB <sub>6</sub> H <sub>4</sub> C <sub>6</sub> N                                          | -6.6343             |
| CaNH <sub>4</sub> B <sub>6</sub> C <sub>6</sub> | 1.333 H <sub>3</sub> N + 3 B <sub>13</sub> C <sub>2</sub> + 6.444 Ca → 5.444 CaB <sub>6</sub> + 0.3333 BN + CaB <sub>6</sub> H <sub>4</sub> C <sub>6</sub> N                                                            | -6.6005             |
| CaNH <sub>4</sub> B <sub>6</sub> C <sub>6</sub> | 3 B <sub>13</sub> C <sub>2</sub> + 0.5 Ca <sub>3</sub> N <sub>2</sub> + 0.3636 B <sub>9</sub> H <sub>11</sub> + 5.545 Ca → 6.045 CaB <sub>6</sub> + CaB <sub>6</sub> H <sub>4</sub> C <sub>6</sub> N                    | -6.5847             |
| CaNH <sub>4</sub> B <sub>6</sub> C <sub>6</sub> | H <sub>3</sub> N + 3 B <sub>13</sub> C <sub>2</sub> + 0.09091 B <sub>9</sub> H <sub>11</sub> + 6.636 Ca → 5.636 CaB <sub>6</sub> + CaB <sub>6</sub> H <sub>4</sub> C <sub>6</sub> N                                     | -6.5698             |
| CaNH <sub>4</sub> B <sub>6</sub> C <sub>6</sub> | 1.333 H <sub>3</sub> N + 3 B <sub>13</sub> C <sub>2</sub> + 7 Ca → 5.5 CaB <sub>6</sub> + 0.1667 Ca <sub>3</sub> N <sub>2</sub> + CaB <sub>6</sub> H <sub>4</sub> C <sub>6</sub> N                                      | -6.5648             |
| CaNH <sub>4</sub> B <sub>6</sub> C <sub>6</sub> | H <sub>3</sub> N + 3 B <sub>13</sub> C <sub>2</sub> + 0.1429 B <sub>5</sub> H <sub>7</sub> + 6.619 Ca → 5.619 CaB <sub>6</sub> + CaB <sub>6</sub> H <sub>4</sub> C <sub>6</sub> N                                       | -6.5359             |
| CaNH <sub>4</sub> B <sub>6</sub> C <sub>6</sub> | CaH <sub>2</sub> + 11.27 H <sub>3</sub> N + 3 B <sub>13</sub> C <sub>2</sub> → 10.27 BN + 4.545 B <sub>5</sub> H <sub>7</sub> + CaB <sub>6</sub> H <sub>4</sub> C <sub>6</sub> N                                        | -6.4838             |
| CaNH <sub>4</sub> B <sub>6</sub> C <sub>6</sub> | 3 B <sub>13</sub> C <sub>2</sub> + BN + 0.3636 B <sub>9</sub> H <sub>11</sub> + 7.212 Ca → 6.212 CaB <sub>6</sub> + CaB <sub>6</sub> H <sub>4</sub> C <sub>6</sub> N                                                    | -6.4777             |
| CaNH <sub>4</sub> B <sub>6</sub> C <sub>6</sub> | 3 B <sub>13</sub> C <sub>2</sub> + 0.5 Ca <sub>3</sub> N <sub>2</sub> + 0.5714 B <sub>5</sub> H <sub>7</sub> + 5.476 Ca → 5.976 CaB <sub>6</sub> + CaB <sub>6</sub> H <sub>4</sub> C <sub>6</sub> N                     | -6.4491             |
| CaNH <sub>4</sub> B <sub>6</sub> C <sub>6</sub> | 14.78 H <sub>3</sub> N + 3 B <sub>13</sub> C <sub>2</sub> + 21.67 Ca → 6.889 Ca <sub>3</sub> N <sub>2</sub> + 3.667 B <sub>9</sub> H <sub>11</sub> + CaB <sub>6</sub> H <sub>4</sub> C <sub>6</sub> N                   | -6.3646             |
| CaNH <sub>4</sub> B <sub>6</sub> C <sub>6</sub> | 0.5 H <sub>2</sub> + H <sub>3</sub> N + 3 B <sub>13</sub> C <sub>2</sub> + 6.5 Ca → 5.5 CaB <sub>6</sub> + CaB <sub>6</sub> H <sub>4</sub> C <sub>6</sub> N                                                             | -6.3450             |
| CaNH <sub>4</sub> B <sub>6</sub> C <sub>6</sub> | 3 B <sub>13</sub> C <sub>2</sub> + BN + 0.5714 B <sub>5</sub> H <sub>7</sub> + 7.143 Ca → 6.143 CaB <sub>6</sub> + CaB <sub>6</sub> H <sub>4</sub> C <sub>6</sub> N                                                     | -6.3421             |
| CaNH <sub>4</sub> B <sub>6</sub> C <sub>6</sub> | Ca <sub>2</sub> N + 3 B <sub>13</sub> C <sub>2</sub> + 0.3636 B <sub>9</sub> H <sub>11</sub> + 5.045 Ca → 6.045 CaB <sub>6</sub> + CaB <sub>6</sub> H <sub>4</sub> C <sub>6</sub> N                                     | -6.2918             |
| CaNH <sub>4</sub> B <sub>6</sub> C <sub>6</sub> | 1.75 B <sub>13</sub> C <sub>2</sub> + 2.969 CaN <sub>2</sub> + 0.5 H <sub>8</sub> C <sub>5</sub> → 1.969 CaB <sub>6</sub> + 4.937 BN + CaB <sub>6</sub> H <sub>4</sub> C <sub>6</sub> N                                 | -6.1840             |
| CaNH <sub>4</sub> B <sub>6</sub> C <sub>6</sub> | Ca <sub>2</sub> N + 3 B <sub>13</sub> C <sub>2</sub> + 0.5714 B <sub>5</sub> H <sub>7</sub> + 4.976 Ca → 5.976 CaB <sub>6</sub> + CaB <sub>6</sub> H <sub>4</sub> C <sub>6</sub> N                                      | -6.1562             |
| CaNH <sub>4</sub> B <sub>6</sub> C <sub>6</sub> | 1.333 H <sub>3</sub> N + 3 B <sub>13</sub> C <sub>2</sub> + 6.667 Ca → 5.5 CaB <sub>6</sub> + 0.1667 CaN <sub>2</sub> + CaB <sub>6</sub> H <sub>4</sub> C <sub>6</sub> N                                                | -6.1560             |
| CaNH <sub>4</sub> B <sub>6</sub> C <sub>6</sub> | 2.974 Ca <sub>2</sub> N + 1.333 H <sub>3</sub> N + 3 B <sub>13</sub> C <sub>2</sub> → 4.949 CaB <sub>6</sub> + 3.308 BN + CaB <sub>6</sub> H <sub>4</sub> C <sub>6</sub> N                                              | -6.0477             |
| CaNH <sub>4</sub> B <sub>6</sub> C <sub>6</sub> | 3 B <sub>13</sub> C <sub>2</sub> + 2.896 Ca <sub>3</sub> N <sub>2</sub> + 2.625 B <sub>5</sub> H <sub>7</sub> → 7.687 CaB <sub>6</sub> + 4.792 H <sub>3</sub> N + CaB <sub>6</sub> H <sub>4</sub> C <sub>6</sub> N      | -6.0330             |
| CaNH <sub>4</sub> B <sub>6</sub> C <sub>6</sub> | 2 H <sub>2</sub> + 3 B <sub>13</sub> C <sub>2</sub> + 2 Ca <sub>3</sub> N <sub>2</sub> → 5 CaB <sub>6</sub> + 3 BN + CaB <sub>6</sub> H <sub>4</sub> C <sub>6</sub> N                                                   | -6.0066             |
| CaNH <sub>4</sub> B <sub>6</sub> C <sub>6</sub> | 1.333 H <sub>3</sub> N + 3 B <sub>13</sub> C <sub>2</sub> + 6.5 Ca → 5.5 CaB <sub>6</sub> + 0.1667 N <sub>2</sub> + CaB <sub>6</sub> H <sub>4</sub> C <sub>6</sub> N                                                    | -5.9037             |
| CaNH <sub>4</sub> B <sub>6</sub> C <sub>6</sub> | 2 CaH <sub>2</sub> + 3 B <sub>13</sub> C <sub>2</sub> + 17 Ca <sub>3</sub> N <sub>2</sub> → 33 BN + 52 Ca + CaB <sub>6</sub> H <sub>4</sub> C <sub>6</sub> N                                                            | -5.8934             |
| CaNH <sub>4</sub> B <sub>6</sub> C <sub>6</sub> | 3.329 Ca <sub>2</sub> N + 3 B <sub>13</sub> C <sub>2</sub> + 0.3636 B <sub>9</sub> H <sub>11</sub> → 5.657 CaB <sub>6</sub> + 2.329 BN + CaB <sub>6</sub> H <sub>4</sub> C <sub>6</sub> N                               | -5.8590             |
| CaNH <sub>4</sub> B <sub>6</sub> C <sub>6</sub> | 2 CaH <sub>2</sub> + 0.5 Ca <sub>3</sub> N <sub>2</sub> + 39 B + 3 CaC <sub>2</sub> → 5.5 CaB <sub>6</sub> + CaB <sub>6</sub> H <sub>4</sub> C <sub>6</sub> N                                                           | -5.7338             |
| CaNH <sub>4</sub> B <sub>6</sub> C <sub>6</sub> | 3.297 Ca <sub>2</sub> N + 3 B <sub>13</sub> C <sub>2</sub> + 0.5714 B <sub>5</sub> H <sub>7</sub> → 5.593 CaB <sub>6</sub> + 2.297 BN + CaB <sub>6</sub> H <sub>4</sub> C <sub>6</sub> N                                | -5.7293             |
| CaNH <sub>4</sub> B <sub>6</sub> C <sub>6</sub> | 2 H <sub>2</sub> + 3 B <sub>13</sub> C <sub>2</sub> + 0.5 Ca <sub>3</sub> N <sub>2</sub> + 5 Ca → 5.5 CaB <sub>6</sub> + CaB <sub>6</sub> H <sub>4</sub> C <sub>6</sub> N                                               | -5.6856             |
| CaNH <sub>4</sub> B <sub>6</sub> C <sub>6</sub> | 2 H <sub>2</sub> + 3 B <sub>13</sub> C <sub>2</sub> + BN + 6.667 Ca → 5.667 CaB <sub>6</sub> + CaB <sub>6</sub> H <sub>4</sub> C <sub>6</sub> N                                                                         | -5.5786             |
| CaNH <sub>4</sub> B <sub>6</sub> C <sub>6</sub> | 0.5 CaH <sub>2</sub> + H <sub>3</sub> N + 3 B <sub>13</sub> C <sub>2</sub> + 6 Ca → 5.5 CaB <sub>6</sub> + CaB <sub>6</sub> H <sub>4</sub> C <sub>6</sub> N                                                             | -5.5142             |
| CaNH <sub>4</sub> B <sub>6</sub> C <sub>6</sub> | 4.171 Ca <sub>2</sub> N + 3 B <sub>13</sub> C <sub>2</sub> + 1.229 B <sub>9</sub> H <sub>11</sub> → 7.343 CaB <sub>6</sub> + 3.171 H <sub>3</sub> N + CaB <sub>6</sub> H <sub>4</sub> C <sub>6</sub> N                  | -5.4103             |
| CaNH <sub>4</sub> B <sub>6</sub> C <sub>6</sub> | Ca <sub>2</sub> N + 2 H <sub>2</sub> + 3 B <sub>13</sub> C <sub>2</sub> + 4.5 Ca → 5.5 CaB <sub>6</sub> + CaB <sub>6</sub> H <sub>4</sub> C <sub>6</sub> N                                                              | -5.3927             |
| CaNH <sub>4</sub> B <sub>6</sub> C <sub>6</sub> | 2 B <sub>9</sub> H <sub>11</sub> + 3.5 N <sub>2</sub> + 3 CaC <sub>2</sub> → 2 CaB <sub>6</sub> + 6 H <sub>3</sub> N + CaB <sub>6</sub> H <sub>4</sub> C <sub>6</sub> N                                                 | -5.3573             |
| CaNH <sub>4</sub> B <sub>6</sub> C <sub>6</sub> | CaH <sub>2</sub> + 10.32 H <sub>3</sub> N + 3 B <sub>13</sub> C <sub>2</sub> → 9.316 BN + 2.632 B <sub>9</sub> H <sub>11</sub> + CaB <sub>6</sub> H <sub>4</sub> C <sub>6</sub> N                                       | -5.3167             |
| CaNH <sub>4</sub> B <sub>6</sub> C <sub>6</sub> | 8.667 H <sub>3</sub> N + 1.2 B <sub>5</sub> H <sub>7</sub> + 12.5 CaC <sub>2</sub> → 3.833 Ca <sub>3</sub> N <sub>2</sub> + 3.8 H <sub>8</sub> C <sub>5</sub> + CaB <sub>6</sub> H <sub>4</sub> C <sub>6</sub> N        | -5.2340             |
| CaNH <sub>4</sub> B <sub>6</sub> C <sub>6</sub> | 3.077 Ca <sub>2</sub> N + 2 H <sub>2</sub> + 3 B <sub>13</sub> C <sub>2</sub> → 5.154 CaB <sub>6</sub> + 2.077 BN + CaB <sub>6</sub> H <sub>4</sub> C <sub>6</sub> N                                                    | -5.0067             |
| CaNH <sub>4</sub> B <sub>6</sub> C <sub>6</sub> | 4.029 Ca <sub>2</sub> N + 3 B <sub>13</sub> C <sub>2</sub> + 1.87 B <sub>5</sub> H <sub>7</sub> → 7.058 CaB <sub>6</sub> + 3.029 H <sub>3</sub> N + CaB <sub>6</sub> H <sub>4</sub> C <sub>6</sub> N                    | -5.0061             |
| CaNH <sub>4</sub> B <sub>6</sub> C <sub>6</sub> | 4.936 Ca <sub>2</sub> N + 1.104 B <sub>9</sub> H <sub>11</sub> + 1.2 H <sub>8</sub> C <sub>5</sub> → 8.872 CaH <sub>2</sub> + 3.936 BN + CaB <sub>6</sub> H <sub>4</sub> C <sub>6</sub> N                               | -4.5844             |
| CaNH <sub>4</sub> B <sub>6</sub> C <sub>6</sub> | H <sub>3</sub> N + 1.2 B <sub>5</sub> H <sub>7</sub> + 9.5 Ca + 1.2 H <sub>8</sub> C <sub>5</sub> → 8.5 CaH <sub>2</sub> + CaB <sub>6</sub> H <sub>4</sub> C <sub>6</sub> N                                             | -4.5237             |
| CaNH <sub>4</sub> B <sub>6</sub> C <sub>6</sub> | H <sub>3</sub> N + 2.687 B <sub>13</sub> C <sub>2</sub> + 5.823 Ca + 0.125 H <sub>8</sub> C <sub>5</sub> → 4.823 CaB <sub>6</sub> + CaB <sub>6</sub> H <sub>4</sub> C <sub>6</sub> N                                    | -4.5171             |
| CaNH <sub>4</sub> B <sub>6</sub> C <sub>6</sub> | Ca <sub>2</sub> N + 2 H <sub>2</sub> + 30 B + 3 CaC <sub>2</sub> → 4 CaB <sub>6</sub> + CaB <sub>6</sub> H <sub>4</sub> C <sub>6</sub> N                                                                                | -4.4781             |
| CaNH <sub>4</sub> B <sub>6</sub> C <sub>6</sub> | 2 CaH <sub>2</sub> + 3 B <sub>13</sub> C <sub>2</sub> + 0.5 N <sub>2</sub> + 4.5 Ca → 5.5 CaB <sub>6</sub> + CaB <sub>6</sub> H <sub>4</sub> C <sub>6</sub> N                                                           | -4.3459             |
| CaNH <sub>4</sub> B <sub>6</sub> C <sub>6</sub> | 8.074 H <sub>3</sub> N + 0.6667 B <sub>9</sub> H <sub>11</sub> + 11.61 CaC <sub>2</sub> → 3.537 Ca <sub>3</sub> N <sub>2</sub> + 3.444 H <sub>8</sub> C <sub>5</sub> + CaB <sub>6</sub> H <sub>4</sub> C <sub>6</sub> N | -4.1930             |
| CaNH <sub>4</sub> B <sub>6</sub> C <sub>6</sub> | 2 CaH <sub>2</sub> + 0.5 CaN <sub>2</sub> + 33 B + 3 CaC <sub>2</sub> → 4.5 CaB <sub>6</sub> + CaB <sub>6</sub> H <sub>4</sub> C <sub>6</sub> N                                                                         | -4.1028             |
| CaNH <sub>4</sub> B <sub>6</sub> C <sub>6</sub> | Ca <sub>2</sub> N + 27.14 B + 0.5714 B <sub>5</sub> H <sub>7</sub> + 3 CaC <sub>2</sub> → 4 CaB <sub>6</sub> + CaB <sub>6</sub> H <sub>4</sub> C <sub>6</sub> N                                                         | -3.8809             |
| CaNH <sub>4</sub> B <sub>6</sub> C <sub>6</sub> | Ca <sub>2</sub> N + 26.73 B + 0.3636 B <sub>9</sub> H <sub>11</sub> + 3 CaC <sub>2</sub> → 4 CaB <sub>6</sub> + CaB <sub>6</sub> H <sub>4</sub> C <sub>6</sub> N                                                        | -3.8186             |
| CaNH <sub>4</sub> B <sub>6</sub> C <sub>6</sub> | H <sub>3</sub> N + 0.6667 B <sub>9</sub> H <sub>11</sub> + 8.967 Ca + 1.2 H <sub>8</sub> C <sub>5</sub> → 7.967 CaH <sub>2</sub> + CaB <sub>6</sub> H <sub>4</sub> C <sub>6</sub> N                                     | -3.6826             |
| CaNH <sub>4</sub> B <sub>6</sub> C <sub>6</sub> | 2 CaH <sub>2</sub> + 3 B <sub>13</sub> C <sub>2</sub> + 0.5 CaN <sub>2</sub> + 4 Ca → 5.5 CaB <sub>6</sub> + CaB <sub>6</sub> H <sub>4</sub> C <sub>6</sub> N                                                           | -3.5888             |
| CaNH <sub>4</sub> B <sub>6</sub> C <sub>6</sub> | 7 H <sub>2</sub> + 3 B <sub>13</sub> C <sub>2</sub> + 2.167 Ca <sub>3</sub> N <sub>2</sub> → 5.5 CaB <sub>6</sub> + 3.333 H <sub>3</sub> N + CaB <sub>6</sub> H <sub>4</sub> C <sub>6</sub> N                           | -3.4874             |
| CaNH <sub>4</sub> B <sub>6</sub> C <sub>6</sub> | 2 CaH <sub>2</sub> + 30 B + 0.5 N <sub>2</sub> + 3 CaC <sub>2</sub> → 4 CaB <sub>6</sub> + CaB <sub>6</sub> H <sub>4</sub> C <sub>6</sub> N                                                                             | -3.4312             |
| CaNH <sub>4</sub> B <sub>6</sub> C <sub>6</sub> | 1.2 B <sub>5</sub> H <sub>7</sub> + 0.5 N <sub>2</sub> + 8 Ca + 1.2 H <sub>8</sub> C <sub>5</sub> → 7 CaH <sub>2</sub> + CaB <sub>6</sub> H <sub>4</sub> C <sub>6</sub> N                                               | -3.3553             |
| CaNH <sub>4</sub> B <sub>6</sub> C <sub>6</sub> | 2 H <sub>2</sub> + 0.5 Ca <sub>3</sub> N <sub>2</sub> + 27 B + 3 CaC <sub>2</sub> → 3.5 CaB <sub>6</sub> + CaB <sub>6</sub> H <sub>4</sub> C <sub>6</sub> N                                                             | -3.3422             |
| CaNH <sub>4</sub> B <sub>6</sub> C <sub>6</sub> | 11.09 Ca <sub>2</sub> N + 3 B <sub>13</sub> C <sub>2</sub> + 0.3636 B <sub>9</sub> H <sub>11</sub> → 6.045 CaB <sub>6</sub> + 5.045 Ca <sub>3</sub> N <sub>2</sub> + CaB <sub>6</sub> H <sub>4</sub> C <sub>6</sub> N   | -3.3366             |
| CaNH <sub>4</sub> B <sub>6</sub> C <sub>6</sub> | 3.25 Ca <sub>2</sub> N + 5.375 H <sub>2</sub> + 3 B <sub>13</sub> C <sub>2</sub> → 5.5 CaB <sub>6</sub> + 2.25 H <sub>3</sub> N + CaB <sub>6</sub> H <sub>4</sub> C <sub>6</sub> N                                      | -3.2500             |

Continued on next page

Continued

| Compound                                        | Chemical reaction                                                                                                                                                                                                    | Reaction energy(eV) |
|-------------------------------------------------|----------------------------------------------------------------------------------------------------------------------------------------------------------------------------------------------------------------------|---------------------|
| CaNH <sub>4</sub> B <sub>6</sub> C <sub>6</sub> | 10.95 Ca <sub>2</sub> N + 3 B <sub>13</sub> C <sub>2</sub> + 0.5714 B <sub>5</sub> H <sub>7</sub> → 5.976 CaB <sub>6</sub> + 4.976 Ca <sub>3</sub> N <sub>2</sub> + CaB <sub>6</sub> H <sub>4</sub> C <sub>6</sub> N | -3.2415             |
| CaNH <sub>4</sub> B <sub>6</sub> C <sub>6</sub> | 0.75 B <sub>13</sub> C <sub>2</sub> + 2.375 N <sub>2</sub> + CaC <sub>2</sub> + 0.5 H <sub>8</sub> C <sub>5</sub> → 3.75 BN + CaB <sub>6</sub> H <sub>4</sub> C <sub>6</sub> N                                       | -3.1296             |
| CaNH <sub>4</sub> B <sub>6</sub> C <sub>6</sub> | 10 Ca <sub>2</sub> N + 2 H <sub>2</sub> + 3 B <sub>13</sub> C <sub>2</sub> → 5.5 CaB <sub>6</sub> + 4.5 Ca <sub>3</sub> N <sub>2</sub> + CaB <sub>6</sub> H <sub>4</sub> C <sub>6</sub> N                            | -2.7570             |
| CaNH <sub>4</sub> B <sub>6</sub> C <sub>6</sub> | 7.591 H <sub>3</sub> N + 2 B <sub>13</sub> C <sub>2</sub> + CaC <sub>2</sub> → 6.591 BN + 2.682 B <sub>5</sub> H <sub>7</sub> + CaB <sub>6</sub> H <sub>4</sub> C <sub>6</sub> N                                     | -2.7463             |
| CaNH <sub>4</sub> B <sub>6</sub> C <sub>6</sub> | 0.5 Ca <sub>3</sub> N <sub>2</sub> + 24.14 B + 0.5714 B <sub>5</sub> H <sub>7</sub> + 3 CaC <sub>2</sub> → 3.5 CaB <sub>6</sub> + CaB <sub>6</sub> H <sub>4</sub> C <sub>6</sub> N                                   | -2.7451             |
| CaNH <sub>4</sub> B <sub>6</sub> C <sub>6</sub> | 0.5 Ca <sub>3</sub> N <sub>2</sub> + 23.73 B + 0.3636 B <sub>9</sub> H <sub>11</sub> + 3 CaC <sub>2</sub> → 3.5 CaB <sub>6</sub> + CaB <sub>6</sub> H <sub>4</sub> C <sub>6</sub> N                                  | -2.6828             |
| CaNH <sub>4</sub> B <sub>6</sub> C <sub>6</sub> | 0.5 CaN <sub>2</sub> + 1.2 B <sub>5</sub> H <sub>7</sub> + 7.5 Ca + 1.2 H <sub>8</sub> C <sub>5</sub> → 7 CaH <sub>2</sub> + CaB <sub>6</sub> H <sub>4</sub> C <sub>6</sub> N                                        | -2.5982             |
| CaNH <sub>4</sub> B <sub>6</sub> C <sub>6</sub> | 2 CaH <sub>2</sub> + 3 B <sub>13</sub> C <sub>2</sub> + 1.4 Ca <sub>3</sub> N <sub>2</sub> → 5.2 CaB <sub>6</sub> + 1.8 BN + CaB <sub>6</sub> H <sub>4</sub> C <sub>6</sub> N                                        | -2.5550             |
| CaNH <sub>4</sub> B <sub>6</sub> C <sub>6</sub> | 0.6667 B <sub>9</sub> H <sub>11</sub> + 0.5 N <sub>2</sub> + 7.467 Ca + 1.2 H <sub>8</sub> C <sub>5</sub> → 6.467 CaH <sub>2</sub> + CaB <sub>6</sub> H <sub>4</sub> C <sub>6</sub> N                                | -2.5142             |
| CaNH <sub>4</sub> B <sub>6</sub> C <sub>6</sub> | 14 Ca <sub>2</sub> N + 1.333 H <sub>3</sub> N + 3 B <sub>13</sub> C <sub>2</sub> → 5.5 CaB <sub>6</sub> + 7.167 Ca <sub>3</sub> N <sub>2</sub> + CaB <sub>6</sub> H <sub>4</sub> C <sub>6</sub> N                    | -2.4648             |
| CaNH <sub>4</sub> B <sub>6</sub> C <sub>6</sub> | 2.867 Ca <sub>2</sub> N + 34.4 B + 1.2 H <sub>8</sub> C <sub>5</sub> → 4.733 CaB <sub>6</sub> + 1.867 H <sub>3</sub> N + CaB <sub>6</sub> H <sub>4</sub> C <sub>6</sub> N                                            | -2.4491             |
| CaNH <sub>4</sub> B <sub>6</sub> C <sub>6</sub> | 2 CaH <sub>2</sub> + 3 B <sub>13</sub> C <sub>2</sub> + 0.5 Ca <sub>3</sub> N <sub>2</sub> + 3 Ca → 5.5 CaB <sub>6</sub> + CaB <sub>6</sub> H <sub>4</sub> C <sub>6</sub> N                                          | -2.3624             |
| CaNH <sub>4</sub> B <sub>6</sub> C <sub>6</sub> | 2 CaH <sub>2</sub> + 3 B <sub>13</sub> C <sub>2</sub> + BN + 4.667 Ca → 5.667 CaB <sub>6</sub> + CaB <sub>6</sub> H <sub>4</sub> C <sub>6</sub> N                                                                    | -2.2554             |
| CaNH <sub>4</sub> B <sub>6</sub> C <sub>6</sub> | Ca <sub>2</sub> N + 2 CaH <sub>2</sub> + 3 B <sub>13</sub> C <sub>2</sub> + 2.5 Ca → 5.5 CaB <sub>6</sub> + CaB <sub>6</sub> H <sub>4</sub> C <sub>6</sub> N                                                         | -2.0695             |
| CaNH <sub>4</sub> B <sub>6</sub> C <sub>6</sub> | 7.026 H <sub>3</sub> N + 2 B <sub>13</sub> C <sub>2</sub> + CaC <sub>2</sub> → 6.026 BN + 1.553 B <sub>9</sub> H <sub>11</sub> + CaB <sub>6</sub> H <sub>4</sub> C <sub>6</sub> N                                    | -2.0577             |
| CaNH <sub>4</sub> B <sub>6</sub> C <sub>6</sub> | 0.7778 B <sub>13</sub> C <sub>2</sub> + 2.556 CaN <sub>2</sub> + 0.8889 H <sub>8</sub> C <sub>5</sub> → 1.556 CaH <sub>2</sub> + 4.111 BN + CaB <sub>6</sub> H <sub>4</sub> C <sub>6</sub> N                         | -1.9798             |
| CaNH <sub>4</sub> B <sub>6</sub> C <sub>6</sub> | 2.154 Ca <sub>2</sub> N + 2 CaH <sub>2</sub> + 3 B <sub>13</sub> C <sub>2</sub> → 5.308 CaB <sub>6</sub> + 1.154 BN + CaB <sub>6</sub> H <sub>4</sub> C <sub>6</sub> N                                               | -1.8550             |
| CaNH <sub>4</sub> B <sub>6</sub> C <sub>6</sub> | 0.5 CaN <sub>2</sub> + 0.6667 B <sub>9</sub> H <sub>11</sub> + 6.967 Ca + 1.2 H <sub>8</sub> C <sub>5</sub> → 6.467 CaH <sub>2</sub> + CaB <sub>6</sub> H <sub>4</sub> C <sub>6</sub> N                              | -1.7571             |
| CaNH <sub>4</sub> B <sub>6</sub> C <sub>6</sub> | 2 H <sub>2</sub> + 0.5 CaN <sub>2</sub> + 21 B + 3 CaC <sub>2</sub> → 2.5 CaB <sub>6</sub> + CaB <sub>6</sub> H <sub>4</sub> C <sub>6</sub> N                                                                        | -1.7113             |
| CaNH <sub>4</sub> B <sub>6</sub> C <sub>6</sub> | 5.059 H <sub>3</sub> N + 1.2 B <sub>5</sub> H <sub>7</sub> + 9.118 CaC <sub>2</sub> → 4.059 Ca <sub>2</sub> N + 2.447 H <sub>8</sub> C <sub>5</sub> + CaB <sub>6</sub> H <sub>4</sub> C <sub>6</sub> N               | -1.3976             |
| CaNH <sub>4</sub> B <sub>6</sub> C <sub>6</sub> | 0.5 Ca <sub>3</sub> N <sub>2</sub> + 1.2 B <sub>5</sub> H <sub>7</sub> + 6.5 Ca + 1.2 H <sub>8</sub> C <sub>5</sub> → 7 CaH <sub>2</sub> + CaB <sub>6</sub> H <sub>4</sub> C <sub>6</sub> N                          | -1.3718             |
| CaNH <sub>4</sub> B <sub>6</sub> C <sub>6</sub> | 4.364 Ca <sub>2</sub> N + 3 B <sub>13</sub> C <sub>2</sub> + 0.3636 B <sub>9</sub> H <sub>11</sub> → 6.045 CaB <sub>6</sub> + 1.682 CaN <sub>2</sub> + CaB <sub>6</sub> H <sub>4</sub> C <sub>6</sub> N              | -1.1815             |
| CaNH <sub>4</sub> B <sub>6</sub> C <sub>6</sub> | 4.317 Ca <sub>2</sub> N + 3 B <sub>13</sub> C <sub>2</sub> + 0.5714 B <sub>5</sub> H <sub>7</sub> → 5.976 CaB <sub>6</sub> + 1.659 CaN <sub>2</sub> + CaB <sub>6</sub> H <sub>4</sub> C <sub>6</sub> N               | -1.1160             |
| CaNH <sub>4</sub> B <sub>6</sub> C <sub>6</sub> | 1.25 CaN <sub>2</sub> + 1.5 B <sub>5</sub> H <sub>7</sub> + 3 CaC <sub>2</sub> → 3.25 CaH <sub>2</sub> + 1.5 BN + CaB <sub>6</sub> H <sub>4</sub> C <sub>6</sub> N                                                   | -1.1150             |
| CaNH <sub>4</sub> B <sub>6</sub> C <sub>6</sub> | 0.5 CaN <sub>2</sub> + 18.14 B + 0.5714 B <sub>5</sub> H <sub>7</sub> + 3 CaC <sub>2</sub> → 2.5 CaB <sub>6</sub> + CaB <sub>6</sub> H <sub>4</sub> C <sub>6</sub> N                                                 | -1.1141             |
| CaNH <sub>4</sub> B <sub>6</sub> C <sub>6</sub> | Ca <sub>2</sub> N + 1.2 B <sub>5</sub> H <sub>7</sub> + 6 Ca + 1.2 H <sub>8</sub> C <sub>5</sub> → 7 CaH <sub>2</sub> + CaB <sub>6</sub> H <sub>4</sub> C <sub>6</sub> N                                             | -1.0790             |
| CaNH <sub>4</sub> B <sub>6</sub> C <sub>6</sub> | 0.5 CaN <sub>2</sub> + 17.73 B + 0.3636 B <sub>9</sub> H <sub>11</sub> + 3 CaC <sub>2</sub> → 2.5 CaB <sub>6</sub> + CaB <sub>6</sub> H <sub>4</sub> C <sub>6</sub> N                                                | -1.0518             |
| CaNH <sub>4</sub> B <sub>6</sub> C <sub>6</sub> | 2 H <sub>2</sub> + 18 B + 0.5 N <sub>2</sub> + 3 CaC <sub>2</sub> → 2 CaB <sub>6</sub> + CaB <sub>6</sub> H <sub>4</sub> C <sub>6</sub> N                                                                            | -1.0397             |
| CaNH <sub>4</sub> B <sub>6</sub> C <sub>6</sub> | 2 CaH <sub>2</sub> + BN + 29 B + 3 CaC <sub>2</sub> → 4 CaB <sub>6</sub> + CaB <sub>6</sub> H <sub>4</sub> C <sub>6</sub> N                                                                                          | -0.8645             |
| CaNH <sub>4</sub> B <sub>6</sub> C <sub>6</sub> | CaB <sub>6</sub> + 6 C + 0.3636 B <sub>9</sub> H <sub>11</sub> + 2.136 N <sub>2</sub> → 3.273 BN + CaB <sub>6</sub> H <sub>4</sub> C <sub>6</sub> N                                                                  | -0.8639             |
| CaNH <sub>4</sub> B <sub>6</sub> C <sub>6</sub> | 6.5 CaH <sub>2</sub> + 3 B <sub>13</sub> C <sub>2</sub> + 2 N <sub>2</sub> → 5.5 CaB <sub>6</sub> + 3 H <sub>3</sub> N + CaB <sub>6</sub> H <sub>4</sub> C <sub>6</sub> N                                            | -0.8409             |
| CaNH <sub>4</sub> B <sub>6</sub> C <sub>6</sub> | 4 Ca <sub>2</sub> N + 2 H <sub>2</sub> + 3 B <sub>13</sub> C <sub>2</sub> → 5.5 CaB <sub>6</sub> + 1.5 CaN <sub>2</sub> + CaB <sub>6</sub> H <sub>4</sub> C <sub>6</sub> N                                           | -0.8349             |
| CaNH <sub>4</sub> B <sub>6</sub> C <sub>6</sub> | 4.745 H <sub>3</sub> N + 0.6667 B <sub>9</sub> H <sub>11</sub> + 8.49 CaC <sub>2</sub> → 3.745 Ca <sub>2</sub> N + 2.196 H <sub>8</sub> C <sub>5</sub> + CaB <sub>6</sub> H <sub>4</sub> C <sub>6</sub> N            | -0.6531             |
| CaNH <sub>4</sub> B <sub>6</sub> C <sub>6</sub> | 6 Ca <sub>2</sub> N + 2 CaH <sub>2</sub> + 3 B <sub>13</sub> C <sub>2</sub> → 5.5 CaB <sub>6</sub> + 2.5 Ca <sub>3</sub> N <sub>2</sub> + CaB <sub>6</sub> H <sub>4</sub> C <sub>6</sub> N                           | -0.6052             |
| CaNH <sub>4</sub> B <sub>6</sub> C <sub>6</sub> | 3.523 Ca <sub>2</sub> N + 3 B <sub>13</sub> C <sub>2</sub> + 0.3636 B <sub>9</sub> H <sub>11</sub> → 6.045 CaB <sub>6</sub> + 1.261 N <sub>2</sub> + CaB <sub>6</sub> H <sub>4</sub> C <sub>6</sub> N                | -0.5491             |
| CaNH <sub>4</sub> B <sub>6</sub> C <sub>6</sub> | 0.5 Ca <sub>3</sub> N <sub>2</sub> + 0.6667 B <sub>9</sub> H <sub>11</sub> + 5.967 Ca + 1.2 H <sub>8</sub> C <sub>5</sub> → 6.467 CaH <sub>2</sub> + CaB <sub>6</sub> H <sub>4</sub> C <sub>6</sub> N                | -0.5307             |
| CaNH <sub>4</sub> B <sub>6</sub> C <sub>6</sub> | 32.67 Ca <sub>2</sub> N + 1.333 H <sub>3</sub> N + 3 B <sub>13</sub> C <sub>2</sub> → 33 BN + 64.33 Ca + CaB <sub>6</sub> H <sub>4</sub> C <sub>6</sub> N                                                            | -0.5291             |
| CaNH <sub>4</sub> B <sub>6</sub> C <sub>6</sub> | 3.488 Ca <sub>2</sub> N + 3 B <sub>13</sub> C <sub>2</sub> + 0.5714 B <sub>5</sub> H <sub>7</sub> → 5.976 CaB <sub>6</sub> + 1.244 N <sub>2</sub> + CaB <sub>6</sub> H <sub>4</sub> C <sub>6</sub> N                 | -0.4923             |
| CaNH <sub>4</sub> B <sub>6</sub> C <sub>6</sub> | 15.14 B + 0.5714 B <sub>5</sub> H <sub>7</sub> + 0.5 N <sub>2</sub> + 3 CaC <sub>2</sub> → 2 CaB <sub>6</sub> + CaB <sub>6</sub> H <sub>4</sub> C <sub>6</sub> N                                                     | -0.4425             |
| CaNH <sub>4</sub> B <sub>6</sub> C <sub>6</sub> | 14.73 B + 0.3636 B <sub>9</sub> H <sub>11</sub> + 0.5 N <sub>2</sub> + 3 CaC <sub>2</sub> → 2 CaB <sub>6</sub> + CaB <sub>6</sub> H <sub>4</sub> C <sub>6</sub> N                                                    | -0.3803             |
| CaNH <sub>4</sub> B <sub>6</sub> C <sub>6</sub> | 1.75 B <sub>13</sub> C <sub>2</sub> + 0.5 N <sub>2</sub> + 3.792 Ca + 0.5 H <sub>8</sub> C <sub>5</sub> → 2.792 CaB <sub>6</sub> + CaB <sub>6</sub> H <sub>4</sub> C <sub>6</sub> N                                  | -0.3573             |
| CaNH <sub>4</sub> B <sub>6</sub> C <sub>6</sub> | 0.5 CaH <sub>2</sub> + H <sub>3</sub> N + 21 B + 3 CaC <sub>2</sub> → 2.5 CaB <sub>6</sub> + CaB <sub>6</sub> H <sub>4</sub> C <sub>6</sub> N                                                                        | -0.3135             |
| CaNH <sub>4</sub> B <sub>6</sub> C <sub>6</sub> | 3.25 Ca <sub>2</sub> N + 2 H <sub>2</sub> + 3 B <sub>13</sub> C <sub>2</sub> → 5.5 CaB <sub>6</sub> + 1.125 N <sub>2</sub> + CaB <sub>6</sub> H <sub>4</sub> C <sub>6</sub> N                                        | -0.2708             |
| CaNH <sub>4</sub> B <sub>6</sub> C <sub>6</sub> | 1.2 B <sub>5</sub> H <sub>7</sub> + 3.875 N <sub>2</sub> + 4.375 CaC <sub>2</sub> → 3.375 CaN <sub>2</sub> + 0.55 H <sub>8</sub> C <sub>5</sub> + CaB <sub>6</sub> H <sub>4</sub> C <sub>6</sub> N                   | -0.2570             |
| CaNH <sub>4</sub> B <sub>6</sub> C <sub>6</sub> | Ca <sub>2</sub> N + 0.6667 B <sub>9</sub> H <sub>11</sub> + 5.467 Ca + 1.2 H <sub>8</sub> C <sub>5</sub> → 6.467 CaH <sub>2</sub> + CaB <sub>6</sub> H <sub>4</sub> C <sub>6</sub> N                                 | -0.2379             |
| CaNH <sub>4</sub> B <sub>6</sub> C <sub>6</sub> | 1.75 B <sub>13</sub> C <sub>2</sub> + 8.875 Ca <sub>3</sub> N <sub>2</sub> + 0.5 H <sub>8</sub> C <sub>5</sub> → 16.75 BN + 25.62 Ca + CaB <sub>6</sub> H <sub>4</sub> C <sub>6</sub> N                              | -0.1660             |
| CaNH <sub>4</sub> B <sub>6</sub> C <sub>6</sub> | 1.333 H <sub>3</sub> N + 18.33 B + 3 CaC <sub>2</sub> → 2 CaB <sub>6</sub> + 0.3333 BN + CaB <sub>6</sub> H <sub>4</sub> C <sub>6</sub> N                                                                            | -0.1299             |
| LaNH <sub>4</sub> B <sub>6</sub> C <sub>6</sub> | 50 La + 34 H <sub>3</sub> N + 3 B <sub>13</sub> C <sub>2</sub> → 33 BN + 49 LaH <sub>2</sub> + LaB <sub>6</sub> H <sub>4</sub> C <sub>6</sub> N                                                                      | -125.2998           |
| LaNH <sub>4</sub> B <sub>6</sub> C <sub>6</sub> | 44.56 La + 34 H <sub>3</sub> N + 3 B <sub>13</sub> C <sub>2</sub> → 33 BN + 10.89 La <sub>4</sub> H <sub>9</sub> + LaB <sub>6</sub> H <sub>4</sub> C <sub>6</sub> N                                                  | -120.4946           |
| LaNH <sub>4</sub> B <sub>6</sub> C <sub>6</sub> | 40.2 La + 34 H <sub>3</sub> N + 3 B <sub>13</sub> C <sub>2</sub> → 33 BN + 19.6 La <sub>2</sub> H <sub>5</sub> + LaB <sub>6</sub> H <sub>4</sub> C <sub>6</sub> N                                                    | -116.0742           |
| LaNH <sub>4</sub> B <sub>6</sub> C <sub>6</sub> | 2 LaH <sub>2</sub> + 23.5 N <sub>2</sub> + 4 B <sub>13</sub> C <sub>2</sub> → LaC <sub>2</sub> + 46 BN + LaB <sub>6</sub> H <sub>4</sub> C <sub>6</sub> N                                                            | -107.1535           |
| LaNH <sub>4</sub> B <sub>6</sub> C <sub>6</sub> | 33.67 La + 34 H <sub>3</sub> N + 3 B <sub>13</sub> C <sub>2</sub> → 32.67 LaH <sub>3</sub> + 33 BN + LaB <sub>6</sub> H <sub>4</sub> C <sub>6</sub> N                                                                | -107.1373           |
| LaNH <sub>4</sub> B <sub>6</sub> C <sub>6</sub> | 70 LaC <sub>2</sub> + 70 H <sub>3</sub> N + 1.2 B <sub>5</sub> H <sub>7</sub> → 26.8 H <sub>8</sub> C <sub>5</sub> + 69 LaN + LaB <sub>6</sub> H <sub>4</sub> C <sub>6</sub> N                                       | -101.1075           |
| LaNH <sub>4</sub> B <sub>6</sub> C <sub>6</sub> | 0.4444 La <sub>4</sub> H <sub>9</sub> + 22.06 N <sub>2</sub> + 3.778 B <sub>13</sub> C <sub>2</sub> → 0.7778 LaC <sub>2</sub> + 43.11 BN + LaB <sub>6</sub> H <sub>4</sub> C <sub>6</sub> N                          | -100.0652           |
| LaNH <sub>4</sub> B <sub>6</sub> C <sub>6</sub> | 2 LaH <sub>2</sub> + 21.87 N <sub>2</sub> + 3.75 B <sub>13</sub> C <sub>2</sub> → 42.75 BN + 0.5 La <sub>2</sub> C <sub>3</sub> + LaB <sub>6</sub> H <sub>4</sub> C <sub>6</sub> N                                   | -99.0157            |
| LaNH <sub>4</sub> B <sub>6</sub> C <sub>6</sub> | LaB <sub>6</sub> + 0.3636 B <sub>9</sub> H <sub>11</sub> + 21.64 N <sub>2</sub> + 3 B <sub>13</sub> C <sub>2</sub> → 42.27 BN + LaB <sub>6</sub> H <sub>4</sub> C <sub>6</sub> N                                     | -97.3404            |
| LaNH <sub>4</sub> B <sub>6</sub> C <sub>6</sub> | LaB <sub>6</sub> + 0.5714 B <sub>5</sub> H <sub>7</sub> + 21.43 N <sub>2</sub> + 3 B <sub>13</sub> C <sub>2</sub> → 41.86 BN + LaB <sub>6</sub> H <sub>4</sub> C <sub>6</sub> N                                      | -96.3360            |
| LaNH <sub>4</sub> B <sub>6</sub> C <sub>6</sub> | 20.9 N <sub>2</sub> + 3.6 B <sub>13</sub> C <sub>2</sub> + 0.8 La <sub>2</sub> H <sub>5</sub> → 0.6 LaC <sub>2</sub> + 40.8 BN + LaB <sub>6</sub> H <sub>4</sub> C <sub>6</sub> N                                    | -94.4180            |
| LaNH <sub>4</sub> B <sub>6</sub> C <sub>6</sub> | 0.4444 La <sub>4</sub> H <sub>9</sub> + 20.79 N <sub>2</sub> + 3.583 B <sub>13</sub> C <sub>2</sub> → 40.58 BN + 0.3889 La <sub>2</sub> C <sub>3</sub> + LaB <sub>6</sub> H <sub>4</sub> C <sub>6</sub> N            | -93.7358            |
| LaNH <sub>4</sub> B <sub>6</sub> C <sub>6</sub> | 0.3636 B <sub>9</sub> H <sub>11</sub> + 20.64 N <sub>2</sub> + 3 B <sub>13</sub> C <sub>2</sub> + LaB <sub>4</sub> → 40.27 BN + LaB <sub>6</sub> H <sub>4</sub> C <sub>6</sub> N                                     | -93.2975            |

Continued on next page

Continued

| Compound                                        | Chemical reaction                                                                                                                                                                                   | Reaction energy(eV) |
|-------------------------------------------------|-----------------------------------------------------------------------------------------------------------------------------------------------------------------------------------------------------|---------------------|
| LaNH <sub>4</sub> B <sub>6</sub> C <sub>6</sub> | 64.67 LaC <sub>2</sub> + 64.67 H <sub>3</sub> N + 0.6667 B <sub>9</sub> H <sub>11</sub> → 24.67 H <sub>8</sub> C <sub>5</sub> + 63.67 LaN + LaB <sub>6</sub> H <sub>4</sub> C <sub>6</sub> N        | -92.7289            |
| LaNH <sub>4</sub> B <sub>6</sub> C <sub>6</sub> | 0.5714 B <sub>5</sub> H <sub>7</sub> + 20.43 N <sub>2</sub> + 3 B <sub>13</sub> C <sub>2</sub> + LaB <sub>4</sub> → 39.86 BN + LaB <sub>6</sub> H <sub>4</sub> C <sub>6</sub> N                     | -92.2931            |
| LaNH <sub>4</sub> B <sub>6</sub> C <sub>6</sub> | 2 H <sub>2</sub> + LaB <sub>6</sub> + 20 N <sub>2</sub> + 3 B <sub>13</sub> C <sub>2</sub> → 39 BN + LaB <sub>6</sub> H <sub>4</sub> C <sub>6</sub> N                                               | -89.5996            |
| LaNH <sub>4</sub> B <sub>6</sub> C <sub>6</sub> | 19.93 N <sub>2</sub> + 3.45 B <sub>13</sub> C <sub>2</sub> + 0.8 La <sub>2</sub> H <sub>5</sub> → 38.85 BN + 0.3 La <sub>2</sub> C <sub>3</sub> + LaB <sub>6</sub> H <sub>4</sub> C <sub>6</sub> N  | -89.5353            |
| LaNH <sub>4</sub> B <sub>6</sub> C <sub>6</sub> | LaB <sub>6</sub> + 1.333 H <sub>3</sub> N + 19.33 N <sub>2</sub> + 3 B <sub>13</sub> C <sub>2</sub> → 39 BN + LaB <sub>6</sub> H <sub>4</sub> C <sub>6</sub> N                                      | -87.8341            |
| LaNH <sub>4</sub> B <sub>6</sub> C <sub>6</sub> | 1.333 LaH <sub>3</sub> + 19.17 N <sub>2</sub> + 3.333 B <sub>13</sub> C <sub>2</sub> → 0.3333 LaC <sub>2</sub> + 37.33 BN + LaB <sub>6</sub> H <sub>4</sub> C <sub>6</sub> N                        | -86.0414            |
| LaNH <sub>4</sub> B <sub>6</sub> C <sub>6</sub> | La + 0.3636 B <sub>9</sub> H <sub>11</sub> + 18.64 N <sub>2</sub> + 3 B <sub>13</sub> C <sub>2</sub> → 36.27 BN + LaB <sub>6</sub> H <sub>4</sub> C <sub>6</sub> N                                  | -85.8768            |
| LaNH <sub>4</sub> B <sub>6</sub> C <sub>6</sub> | 2 H <sub>2</sub> + 19 N <sub>2</sub> + 3 B <sub>13</sub> C <sub>2</sub> + LaB <sub>4</sub> → 37 BN + LaB <sub>6</sub> H <sub>4</sub> C <sub>6</sub> N                                               | -85.5567            |
| LaNH <sub>4</sub> B <sub>6</sub> C <sub>6</sub> | La + 0.5714 B <sub>5</sub> H <sub>7</sub> + 18.43 N <sub>2</sub> + 3 B <sub>13</sub> C <sub>2</sub> → 35.86 BN + LaB <sub>6</sub> H <sub>4</sub> C <sub>6</sub> N                                   | -84.8724            |
| LaNH <sub>4</sub> B <sub>6</sub> C <sub>6</sub> | 1.333 H <sub>3</sub> N + 18.33 N <sub>2</sub> + 3 B <sub>13</sub> C <sub>2</sub> + LaB <sub>4</sub> → 37 BN + LaB <sub>6</sub> H <sub>4</sub> C <sub>6</sub> N                                      | -83.7912            |
| LaNH <sub>4</sub> B <sub>6</sub> C <sub>6</sub> | 1.333 LaH <sub>3</sub> + 18.63 N <sub>2</sub> + 3.25 B <sub>13</sub> C <sub>2</sub> → 36.25 BN + 0.1667 La <sub>2</sub> C <sub>3</sub> + LaB <sub>6</sub> H <sub>4</sub> C <sub>6</sub> N           | -83.3288            |
| LaNH <sub>4</sub> B <sub>6</sub> C <sub>6</sub> | LaN + 0.3636 B <sub>9</sub> H <sub>11</sub> + 18.14 N <sub>2</sub> + 3 B <sub>13</sub> C <sub>2</sub> → 36.27 BN + LaB <sub>6</sub> H <sub>4</sub> C <sub>6</sub> N                                 | -83.2195            |
| LaNH <sub>4</sub> B <sub>6</sub> C <sub>6</sub> | LaN + 0.5714 B <sub>5</sub> H <sub>7</sub> + 17.93 N <sub>2</sub> + 3 B <sub>13</sub> C <sub>2</sub> → 35.86 BN + LaB <sub>6</sub> H <sub>4</sub> C <sub>6</sub> N                                  | -82.2150            |
| LaNH <sub>4</sub> B <sub>6</sub> C <sub>6</sub> | 34 H <sub>3</sub> N + 401 LaH <sub>2</sub> + 3 B <sub>13</sub> C <sub>2</sub> → 33 BN + 100 La <sub>4</sub> H <sub>9</sub> + LaB <sub>6</sub> H <sub>4</sub> C <sub>6</sub> N                       | -81.1703            |
| LaNH <sub>4</sub> B <sub>6</sub> C <sub>6</sub> | 0.1818 B <sub>9</sub> H <sub>11</sub> + LaH <sub>2</sub> + 17.82 N <sub>2</sub> + 3 B <sub>13</sub> C <sub>2</sub> → 34.64 BN + LaB <sub>6</sub> H <sub>4</sub> C <sub>6</sub> N                    | -80.1251            |
| LaNH <sub>4</sub> B <sub>6</sub> C <sub>6</sub> | 0.2857 B <sub>5</sub> H <sub>7</sub> + LaH <sub>2</sub> + 17.71 N <sub>2</sub> + 3 B <sub>13</sub> C <sub>2</sub> → 34.43 BN + LaB <sub>6</sub> H <sub>4</sub> C <sub>6</sub> N                     | -79.6229            |
| LaNH <sub>4</sub> B <sub>6</sub> C <sub>6</sub> | 0.25 La <sub>4</sub> H <sub>9</sub> + 0.1591 B <sub>9</sub> H <sub>11</sub> + 17.72 N <sub>2</sub> + 3 B <sub>13</sub> C <sub>2</sub> → 34.43 BN + LaB <sub>6</sub> H <sub>4</sub> C <sub>6</sub> N | -79.5165            |
| LaNH <sub>4</sub> B <sub>6</sub> C <sub>6</sub> | 0.25 La <sub>4</sub> H <sub>9</sub> + 0.25 B <sub>5</sub> H <sub>7</sub> + 17.63 N <sub>2</sub> + 3 B <sub>13</sub> C <sub>2</sub> → 34.25 BN + LaB <sub>6</sub> H <sub>4</sub> C <sub>6</sub> N    | -79.0770            |
| LaNH <sub>4</sub> B <sub>6</sub> C <sub>6</sub> | 0.1364 B <sub>9</sub> H <sub>11</sub> + 17.61 N <sub>2</sub> + 3 B <sub>13</sub> C <sub>2</sub> + 0.5 La <sub>2</sub> H <sub>5</sub> → 34.23 BN + LaB <sub>6</sub> H <sub>4</sub> C <sub>6</sub> N  | -78.9225            |
| LaNH <sub>4</sub> B <sub>6</sub> C <sub>6</sub> | 0.2143 B <sub>5</sub> H <sub>7</sub> + 17.54 N <sub>2</sub> + 3 B <sub>13</sub> C <sub>2</sub> + 0.5 La <sub>2</sub> H <sub>5</sub> → 34.07 BN + LaB <sub>6</sub> H <sub>4</sub> C <sub>6</sub> N   | -78.5459            |
| LaNH <sub>4</sub> B <sub>6</sub> C <sub>6</sub> | 34 H <sub>3</sub> N + 201 LaH <sub>2</sub> + 3 B <sub>13</sub> C <sub>2</sub> → 33 BN + 100 La <sub>2</sub> H <sub>5</sub> + LaB <sub>6</sub> H <sub>4</sub> C <sub>6</sub> N                       | -78.2303            |
| LaNH <sub>4</sub> B <sub>6</sub> C <sub>6</sub> | 2 H <sub>2</sub> + La + 17 N <sub>2</sub> + 3 B <sub>13</sub> C <sub>2</sub> → 33 BN + LaB <sub>6</sub> H <sub>4</sub> C <sub>6</sub> N                                                             | -78.1359            |
| LaNH <sub>4</sub> B <sub>6</sub> C <sub>6</sub> | LaH <sub>3</sub> + 0.09091 B <sub>9</sub> H <sub>11</sub> + 17.41 N <sub>2</sub> + 3 B <sub>13</sub> C <sub>2</sub> → 33.82 BN + LaB <sub>6</sub> H <sub>4</sub> C <sub>6</sub> N                   | -77.8053            |
| LaNH <sub>4</sub> B <sub>6</sub> C <sub>6</sub> | LaH <sub>3</sub> + 0.1429 B <sub>5</sub> H <sub>7</sub> + 17.36 N <sub>2</sub> + 3 B <sub>13</sub> C <sub>2</sub> → 33.71 BN + LaB <sub>6</sub> H <sub>4</sub> C <sub>6</sub> N                     | -77.5542            |
| LaNH <sub>4</sub> B <sub>6</sub> C <sub>6</sub> | 2 LaH <sub>2</sub> + 17.5 N <sub>2</sub> + 3 B <sub>13</sub> C <sub>2</sub> → 33 BN + LaN + LaB <sub>6</sub> H <sub>4</sub> C <sub>6</sub> N                                                        | -77.0308            |
| LaNH <sub>4</sub> B <sub>6</sub> C <sub>6</sub> | 0.4444 La <sub>4</sub> H <sub>9</sub> + 17.39 N <sub>2</sub> + 3 B <sub>13</sub> C <sub>2</sub> → 33 BN + 0.7778 LaN + LaB <sub>6</sub> H <sub>4</sub> C <sub>6</sub> N                             | -76.6364            |
| LaNH <sub>4</sub> B <sub>6</sub> C <sub>6</sub> | La + 1.333 H <sub>3</sub> N + 16.33 N <sub>2</sub> + 3 B <sub>13</sub> C <sub>2</sub> → 33 BN + LaB <sub>6</sub> H <sub>4</sub> C <sub>6</sub> N                                                    | -76.3705            |
| LaNH <sub>4</sub> B <sub>6</sub> C <sub>6</sub> | 17.3 N <sub>2</sub> + 3 B <sub>13</sub> C <sub>2</sub> + 0.8 La <sub>2</sub> H <sub>5</sub> → 33 BN + 0.6 LaN + LaB <sub>6</sub> H <sub>4</sub> C <sub>6</sub> N                                    | -76.3444            |
| LaNH <sub>4</sub> B <sub>6</sub> C <sub>6</sub> | H <sub>2</sub> + LaH <sub>2</sub> + 17 N <sub>2</sub> + 3 B <sub>13</sub> C <sub>2</sub> → 33 BN + LaB <sub>6</sub> H <sub>4</sub> C <sub>6</sub> N                                                 | -76.2547            |
| LaNH <sub>4</sub> B <sub>6</sub> C <sub>6</sub> | 0.875 H <sub>2</sub> + 0.25 La <sub>4</sub> H <sub>9</sub> + 17 N <sub>2</sub> + 3 B <sub>13</sub> C <sub>2</sub> → 33 BN + LaB <sub>6</sub> H <sub>4</sub> C <sub>6</sub> N                        | -76.1298            |
| LaNH <sub>4</sub> B <sub>6</sub> C <sub>6</sub> | 0.75 H <sub>2</sub> + 17 N <sub>2</sub> + 3 B <sub>13</sub> C <sub>2</sub> + 0.5 La <sub>2</sub> H <sub>5</sub> → 33 BN + LaB <sub>6</sub> H <sub>4</sub> C <sub>6</sub> N                          | -76.0197            |
| LaNH <sub>4</sub> B <sub>6</sub> C <sub>6</sub> | 1.333 LaH <sub>3</sub> + 17.17 N <sub>2</sub> + 3 B <sub>13</sub> C <sub>2</sub> → 33 BN + 0.3333 LaN + LaB <sub>6</sub> H <sub>4</sub> C <sub>6</sub> N                                            | -76.0005            |
| LaNH <sub>4</sub> B <sub>6</sub> C <sub>6</sub> | LaH <sub>3</sub> + 0.5 H <sub>2</sub> + 17 N <sub>2</sub> + 3 B <sub>13</sub> C <sub>2</sub> → 33 BN + LaB <sub>6</sub> H <sub>4</sub> C <sub>6</sub> N                                             | -75.8700            |
| LaNH <sub>4</sub> B <sub>6</sub> C <sub>6</sub> | 3 LaH <sub>3</sub> + 17 N <sub>2</sub> + 3 B <sub>13</sub> C <sub>2</sub> → 33 BN + La <sub>2</sub> H <sub>5</sub> + LaB <sub>6</sub> H <sub>4</sub> C <sub>6</sub> N                               | -75.5707            |
| LaNH <sub>4</sub> B <sub>6</sub> C <sub>6</sub> | 2.333 LaH <sub>3</sub> + 17 N <sub>2</sub> + 3 B <sub>13</sub> C <sub>2</sub> → 33 BN + 0.3333 La <sub>4</sub> H <sub>9</sub> + LaB <sub>6</sub> H <sub>4</sub> C <sub>6</sub> N                    | -75.5236            |
| LaNH <sub>4</sub> B <sub>6</sub> C <sub>6</sub> | 2 LaH <sub>3</sub> + 17 N <sub>2</sub> + 3 B <sub>13</sub> C <sub>2</sub> → 33 BN + LaH <sub>2</sub> + LaB <sub>6</sub> H <sub>4</sub> C <sub>6</sub> N                                             | -75.4854            |
| LaNH <sub>4</sub> B <sub>6</sub> C <sub>6</sub> | 2 H <sub>2</sub> + LaN + 16.5 N <sub>2</sub> + 3 B <sub>13</sub> C <sub>2</sub> → 33 BN + LaB <sub>6</sub> H <sub>4</sub> C <sub>6</sub> N                                                          | -75.4786            |
| LaNH <sub>4</sub> B <sub>6</sub> C <sub>6</sub> | LaH <sub>3</sub> + 0.3333 H <sub>3</sub> N + 16.83 N <sub>2</sub> + 3 B <sub>13</sub> C <sub>2</sub> → 33 BN + LaB <sub>6</sub> H <sub>4</sub> C <sub>6</sub> N                                     | -75.4287            |
| LaNH <sub>4</sub> B <sub>6</sub> C <sub>6</sub> | 0.6667 H <sub>3</sub> N + LaH <sub>2</sub> + 16.67 N <sub>2</sub> + 3 B <sub>13</sub> C <sub>2</sub> → 33 BN + LaB <sub>6</sub> H <sub>4</sub> C <sub>6</sub> N                                     | -75.3720            |
| LaNH <sub>4</sub> B <sub>6</sub> C <sub>6</sub> | 17 N <sub>2</sub> + 3 B <sub>13</sub> C <sub>2</sub> + 3.5 La <sub>2</sub> H <sub>5</sub> → 33 BN + 1.5 La <sub>4</sub> H <sub>9</sub> + LaB <sub>6</sub> H <sub>4</sub> C <sub>6</sub> N           | -75.3589            |
| LaNH <sub>4</sub> B <sub>6</sub> C <sub>6</sub> | 0.5 H <sub>3</sub> N + 16.75 N <sub>2</sub> + 3 B <sub>13</sub> C <sub>2</sub> + 0.5 La <sub>2</sub> H <sub>5</sub> → 33 BN + LaB <sub>6</sub> H <sub>4</sub> C <sub>6</sub> N                      | -75.3577            |
| LaNH <sub>4</sub> B <sub>6</sub> C <sub>6</sub> | 0.25 La <sub>4</sub> H <sub>9</sub> + 0.5833 H <sub>3</sub> N + 16.71 N <sub>2</sub> + 3 B <sub>13</sub> C <sub>2</sub> → 33 BN + LaB <sub>6</sub> H <sub>4</sub> C <sub>6</sub> N                  | -75.3575            |
| LaNH <sub>4</sub> B <sub>6</sub> C <sub>6</sub> | 17 N <sub>2</sub> + 3 B <sub>13</sub> C <sub>2</sub> + 2 La <sub>2</sub> H <sub>5</sub> → 33 BN + 3 LaH <sub>2</sub> + LaB <sub>6</sub> H <sub>4</sub> C <sub>6</sub> N                             | -75.3148            |
| LaNH <sub>4</sub> B <sub>6</sub> C <sub>6</sub> | 100.5 La <sub>4</sub> H <sub>9</sub> + 34 H <sub>3</sub> N + 3 B <sub>13</sub> C <sub>2</sub> → 33 BN + 200.5 La <sub>2</sub> H <sub>5</sub> + LaB <sub>6</sub> H <sub>4</sub> C <sub>6</sub> N     | -75.2756            |
| LaNH <sub>4</sub> B <sub>6</sub> C <sub>6</sub> | 2 La <sub>4</sub> H <sub>9</sub> + 17 N <sub>2</sub> + 3 B <sub>13</sub> C <sub>2</sub> → 33 BN + 7 LaH <sub>2</sub> + LaB <sub>6</sub> H <sub>4</sub> C <sub>6</sub> N                             | -75.2560            |
| LaNH <sub>4</sub> B <sub>6</sub> C <sub>6</sub> | 1.333 LaH <sub>3</sub> + 17 N <sub>2</sub> + 3 B <sub>13</sub> C <sub>2</sub> → 0.3333 La + 33 BN + LaB <sub>6</sub> H <sub>4</sub> C <sub>6</sub> N                                                | -75.1147            |
| LaNH <sub>4</sub> B <sub>6</sub> C <sub>6</sub> | 17 N <sub>2</sub> + 3 B <sub>13</sub> C <sub>2</sub> + 0.8 La <sub>2</sub> H <sub>5</sub> → 0.6 La + 33 BN + LaB <sub>6</sub> H <sub>4</sub> C <sub>6</sub> N                                       | -74.7500            |
| LaNH <sub>4</sub> B <sub>6</sub> C <sub>6</sub> | 0.4444 La <sub>4</sub> H <sub>9</sub> + 15.44 N <sub>2</sub> + 3 B <sub>13</sub> C <sub>2</sub> → 0.7778 La + 33 BN + LaB <sub>6</sub> H <sub>4</sub> C <sub>6</sub> N                              | -74.5695            |
| LaNH <sub>4</sub> B <sub>6</sub> C <sub>6</sub> | 2 LaH <sub>2</sub> + 17 N <sub>2</sub> + 3 B <sub>13</sub> C <sub>2</sub> → La + 33 BN + LaB <sub>6</sub> H <sub>4</sub> C <sub>6</sub> N                                                           | -74.3734            |
| LaNH <sub>4</sub> B <sub>6</sub> C <sub>6</sub> | 1.333 H <sub>3</sub> N + LaN + 15.83 N <sub>2</sub> + 3 B <sub>13</sub> C <sub>2</sub> → 33 BN + LaB <sub>6</sub> H <sub>4</sub> C <sub>6</sub> N                                                   | -73.7132            |
| LaNH <sub>4</sub> B <sub>6</sub> C <sub>6</sub> | 1.333 LaH <sub>3</sub> + 16.33 N <sub>2</sub> + 3 B <sub>13</sub> C <sub>2</sub> → 31.67 BN + 0.3333 LaB <sub>4</sub> + LaB <sub>6</sub> H <sub>4</sub> C <sub>6</sub> N                            | -72.6412            |
| LaNH <sub>4</sub> B <sub>6</sub> C <sub>6</sub> | 1.333 LaH <sub>3</sub> + 16 N <sub>2</sub> + 3 B <sub>13</sub> C <sub>2</sub> → 0.3333 LaB <sub>6</sub> + 31 BN + LaB <sub>6</sub> H <sub>4</sub> C <sub>6</sub> N                                  | -71.2935            |
| LaNH <sub>4</sub> B <sub>6</sub> C <sub>6</sub> | 15.8 N <sub>2</sub> + 3 B <sub>13</sub> C <sub>2</sub> + 0.8 La <sub>2</sub> H <sub>5</sub> → 30.6 BN + 0.6 LaB <sub>4</sub> + LaB <sub>6</sub> H <sub>4</sub> C <sub>6</sub> N                     | -70.2975            |
| LaNH <sub>4</sub> B <sub>6</sub> C <sub>6</sub> | 34 H <sub>3</sub> N + 101 LaH <sub>2</sub> + 3 B <sub>13</sub> C <sub>2</sub> → 100 LaH <sub>3</sub> + 33 BN + LaB <sub>6</sub> H <sub>4</sub> C <sub>6</sub> N                                     | -69.7003            |
| LaNH <sub>4</sub> B <sub>6</sub> C <sub>6</sub> | 50.5 LaC <sub>2</sub> + 52 H <sub>3</sub> N + 1.5 LaB <sub>4</sub> → 19 H <sub>8</sub> C <sub>5</sub> + 51 LaN + LaB <sub>6</sub> H <sub>4</sub> C <sub>6</sub> N                                   | -69.2928            |
| LaNH <sub>4</sub> B <sub>6</sub> C <sub>6</sub> | 0.4444 La <sub>4</sub> H <sub>9</sub> + 15.44 N <sub>2</sub> + 3 B <sub>13</sub> C <sub>2</sub> → 29.89 BN + 0.7778 LaB <sub>4</sub> + LaB <sub>6</sub> H <sub>4</sub> C <sub>6</sub> N             | -68.7979            |
| LaNH <sub>4</sub> B <sub>6</sub> C <sub>6</sub> | 15.2 N <sub>2</sub> + 3 B <sub>13</sub> C <sub>2</sub> + 0.8 La <sub>2</sub> H <sub>5</sub> → 0.6 LaB <sub>6</sub> + 29.4 BN + LaB <sub>6</sub> H <sub>4</sub> C <sub>6</sub> N                     | -67.8718            |
| LaNH <sub>4</sub> B <sub>6</sub> C <sub>6</sub> | 2 LaH <sub>2</sub> + 15 N <sub>2</sub> + 3 B <sub>13</sub> C <sub>2</sub> → 29 BN + LaB <sub>4</sub> + LaB <sub>6</sub> H <sub>4</sub> C <sub>6</sub> N                                             | -66.9527            |
| LaNH <sub>4</sub> B <sub>6</sub> C <sub>6</sub> | 33.67 La <sub>4</sub> H <sub>9</sub> + 34 H <sub>3</sub> N + 3 B <sub>13</sub> C <sub>2</sub> → 133.7 LaH <sub>3</sub> + 33 BN + LaB <sub>6</sub> H <sub>4</sub> C <sub>6</sub> N                   | -65.8387            |
| LaNH <sub>4</sub> B <sub>6</sub> C <sub>6</sub> | 0.4444 La <sub>4</sub> H <sub>9</sub> + 14.67 N <sub>2</sub> + 3 B <sub>13</sub> C <sub>2</sub> → 0.7778 LaB <sub>6</sub> + 28.33 BN + LaB <sub>6</sub> H <sub>4</sub> C <sub>6</sub> N             | -65.6534            |

Continued on next page

Continued

| Compound                                        | Chemical reaction                                                                                                                                                                                      | Reaction energy(eV) |
|-------------------------------------------------|--------------------------------------------------------------------------------------------------------------------------------------------------------------------------------------------------------|---------------------|
| LaNH <sub>4</sub> B <sub>6</sub> C <sub>6</sub> | LaH <sub>3</sub> + 0.125 H <sub>8</sub> C <sub>5</sub> + 14.97 N <sub>2</sub> + 2.687 B <sub>13</sub> C <sub>2</sub> → 28.94 BN + LaB <sub>6</sub> H <sub>4</sub> C <sub>6</sub> N                     | -65.5493            |
| LaNH <sub>4</sub> B <sub>6</sub> C <sub>6</sub> | 2 LaH <sub>2</sub> + 14 N <sub>2</sub> + 3 B <sub>13</sub> C <sub>2</sub> → LaB <sub>6</sub> + 27 BN + LaB <sub>6</sub> H <sub>4</sub> C <sub>6</sub> N                                                | -62.9098            |
| LaNH <sub>4</sub> B <sub>6</sub> C <sub>6</sub> | 51.5 H <sub>2</sub> + 34 LaN + 3 B <sub>13</sub> C <sub>2</sub> → 33 LaH <sub>3</sub> + 33 BN + LaB <sub>6</sub> H <sub>4</sub> C <sub>6</sub> N                                                       | -62.5614            |
| LaNH <sub>4</sub> B <sub>6</sub> C <sub>6</sub> | 0.3636 B <sub>9</sub> H <sub>11</sub> + 0.5 La <sub>2</sub> C <sub>3</sub> + 13.76 N <sub>2</sub> + 2.25 B <sub>13</sub> C <sub>2</sub> → 26.52 BN + LaB <sub>6</sub> H <sub>4</sub> C <sub>6</sub> N  | -61.2345            |
| LaNH <sub>4</sub> B <sub>6</sub> C <sub>6</sub> | 34 H <sub>3</sub> N + 3 B <sub>13</sub> C <sub>2</sub> + 101 La <sub>2</sub> H <sub>5</sub> → 201 LaH <sub>3</sub> + 33 BN + LaB <sub>6</sub> H <sub>4</sub> C <sub>6</sub> N                          | -61.0850            |
| LaNH <sub>4</sub> B <sub>6</sub> C <sub>6</sub> | 0.1875 H <sub>8</sub> C <sub>5</sub> + 13.95 N <sub>2</sub> + 2.531 B <sub>13</sub> C <sub>2</sub> + 0.5 La <sub>2</sub> H <sub>5</sub> → 26.91 BN + LaB <sub>6</sub> H <sub>4</sub> C <sub>6</sub> N  | -60.5386            |
| LaNH <sub>4</sub> B <sub>6</sub> C <sub>6</sub> | 0.5 La <sub>2</sub> C <sub>3</sub> + 0.5714 B <sub>5</sub> H <sub>7</sub> + 13.55 N <sub>2</sub> + 2.25 B <sub>13</sub> C <sub>2</sub> → 26.11 BN + LaB <sub>6</sub> H <sub>4</sub> C <sub>6</sub> N   | -60.2301            |
| LaNH <sub>4</sub> B <sub>6</sub> C <sub>6</sub> | 0.2187 H <sub>8</sub> C <sub>5</sub> + 0.25 La <sub>4</sub> H <sub>9</sub> + 13.45 N <sub>2</sub> + 2.453 B <sub>13</sub> C <sub>2</sub> → 25.89 BN + LaB <sub>6</sub> H <sub>4</sub> C <sub>6</sub> N | -58.0686            |
| LaNH <sub>4</sub> B <sub>6</sub> C <sub>6</sub> | 43.25 H <sub>2</sub> + 34 LaN + 3 B <sub>13</sub> C <sub>2</sub> → 33 BN + 16.5 La <sub>2</sub> H <sub>5</sub> + LaB <sub>6</sub> H <sub>4</sub> C <sub>6</sub> N                                      | -57.6223            |
| LaNH <sub>4</sub> B <sub>6</sub> C <sub>6</sub> | 43 LaC <sub>2</sub> + LaB <sub>6</sub> + 44 H <sub>3</sub> N → 16 H <sub>8</sub> C <sub>5</sub> + 43 LaN + LaB <sub>6</sub> H <sub>4</sub> C <sub>6</sub> N                                            | -57.1128            |
| LaNH <sub>4</sub> B <sub>6</sub> C <sub>6</sub> | 0.25 H <sub>8</sub> C <sub>5</sub> + LaH <sub>2</sub> + 12.94 N <sub>2</sub> + 2.375 B <sub>13</sub> C <sub>2</sub> → 24.87 BN + LaB <sub>6</sub> H <sub>4</sub> C <sub>6</sub> N                      | -55.6132            |
| LaNH <sub>4</sub> B <sub>6</sub> C <sub>6</sub> | 39.12 H <sub>2</sub> + 34 LaN + 3 B <sub>13</sub> C <sub>2</sub> → 33 BN + 8.25 La <sub>4</sub> H <sub>9</sub> + LaB <sub>6</sub> H <sub>4</sub> C <sub>6</sub> N                                      | -53.9879            |
| LaNH <sub>4</sub> B <sub>6</sub> C <sub>6</sub> | 2 H <sub>2</sub> + 0.5 La <sub>2</sub> C <sub>3</sub> + 12.12 N <sub>2</sub> + 2.25 B <sub>13</sub> C <sub>2</sub> → 23.25 BN + LaB <sub>6</sub> H <sub>4</sub> C <sub>6</sub> N                       | -53.4936            |
| LaNH <sub>4</sub> B <sub>6</sub> C <sub>6</sub> | LaC <sub>2</sub> + 0.3636 B <sub>9</sub> H <sub>11</sub> + 12.14 N <sub>2</sub> + 2 B <sub>13</sub> C <sub>2</sub> → 23.27 BN + LaB <sub>6</sub> H <sub>4</sub> C <sub>6</sub> N                       | -53.0967            |
| LaNH <sub>4</sub> B <sub>6</sub> C <sub>6</sub> | LaC <sub>2</sub> + 0.5714 B <sub>5</sub> H <sub>7</sub> + 11.93 N <sub>2</sub> + 2 B <sub>13</sub> C <sub>2</sub> → 22.86 BN + LaB <sub>6</sub> H <sub>4</sub> C <sub>6</sub> N                        | -52.0923            |
| LaNH <sub>4</sub> B <sub>6</sub> C <sub>6</sub> | 1.333 H <sub>3</sub> N + 0.5 La <sub>2</sub> C <sub>3</sub> + 11.46 N <sub>2</sub> + 2.25 B <sub>13</sub> C <sub>2</sub> → 23.25 BN + LaB <sub>6</sub> H <sub>4</sub> C <sub>6</sub> N                 | -51.7282            |
| LaNH <sub>4</sub> B <sub>6</sub> C <sub>6</sub> | 35 H <sub>2</sub> + 34 LaN + 3 B <sub>13</sub> C <sub>2</sub> → 33 BN + 33 LaH <sub>2</sub> + LaB <sub>6</sub> H <sub>4</sub> C <sub>6</sub> N                                                         | -49.8683            |
| LaNH <sub>4</sub> B <sub>6</sub> C <sub>6</sub> | 0.5 H <sub>8</sub> C <sub>5</sub> + LaB <sub>6</sub> + 11.87 N <sub>2</sub> + 1.75 B <sub>13</sub> C <sub>2</sub> → 22.75 BN + LaB <sub>6</sub> H <sub>4</sub> C <sub>6</sub> N                        | -48.3167            |
| LaNH <sub>4</sub> B <sub>6</sub> C <sub>6</sub> | 17.17 H <sub>3</sub> N + 16.83 LaN + 3 B <sub>13</sub> C <sub>2</sub> → 15.83 LaH <sub>3</sub> + 33 BN + LaB <sub>6</sub> H <sub>4</sub> C <sub>6</sub> N                                              | -46.5511            |
| LaNH <sub>4</sub> B <sub>6</sub> C <sub>6</sub> | LaC <sub>2</sub> + 2 H <sub>2</sub> + 10.5 N <sub>2</sub> + 2 B <sub>13</sub> C <sub>2</sub> → 20 BN + LaB <sub>6</sub> H <sub>4</sub> C <sub>6</sub> N                                                | -45.3558            |
| LaNH <sub>4</sub> B <sub>6</sub> C <sub>6</sub> | 15.73 H <sub>3</sub> N + 18.27 LaN + 3 B <sub>13</sub> C <sub>2</sub> → 33 BN + 8.636 La <sub>2</sub> H <sub>5</sub> + LaB <sub>6</sub> H <sub>4</sub> C <sub>6</sub> N                                | -45.3083            |
| LaNH <sub>4</sub> B <sub>6</sub> C <sub>6</sub> | 0.5 H <sub>8</sub> C <sub>5</sub> + 10.87 N <sub>2</sub> + 1.75 B <sub>13</sub> C <sub>2</sub> + LaB <sub>4</sub> → 20.75 BN + LaB <sub>6</sub> H <sub>4</sub> C <sub>6</sub> N                        | -44.2738            |
| LaNH <sub>4</sub> B <sub>6</sub> C <sub>6</sub> | 14.9 H <sub>3</sub> N + 19.1 LaN + 3 B <sub>13</sub> C <sub>2</sub> → 33 BN + 4.524 La <sub>4</sub> H <sub>9</sub> + LaB <sub>6</sub> H <sub>4</sub> C <sub>6</sub> N                                  | -43.9594            |
| LaNH <sub>4</sub> B <sub>6</sub> C <sub>6</sub> | LaC <sub>2</sub> + 1.333 H <sub>3</sub> N + 9.833 N <sub>2</sub> + 2 B <sub>13</sub> C <sub>2</sub> → 20 BN + LaB <sub>6</sub> H <sub>4</sub> C <sub>6</sub> N                                         | -43.5904            |
| LaNH <sub>4</sub> B <sub>6</sub> C <sub>6</sub> | 14 H <sub>3</sub> N + 20 LaN + 3 B <sub>13</sub> C <sub>2</sub> → 33 BN + 19 LaH <sub>2</sub> + LaB <sub>6</sub> H <sub>4</sub> C <sub>6</sub> N                                                       | -42.1963            |
| LaNH <sub>4</sub> B <sub>6</sub> C <sub>6</sub> | 0.5 H <sub>8</sub> C <sub>5</sub> + La + 8.875 N <sub>2</sub> + 1.75 B <sub>13</sub> C <sub>2</sub> → 16.75 BN + LaB <sub>6</sub> H <sub>4</sub> C <sub>6</sub> N                                      | -36.8531            |
| LaNH <sub>4</sub> B <sub>6</sub> C <sub>6</sub> | LaB <sub>6</sub> + 40 H <sub>3</sub> N + 3 B <sub>13</sub> C <sub>2</sub> → 58 H <sub>2</sub> + 39 BN + LaB <sub>6</sub> H <sub>4</sub> C <sub>6</sub> N                                               | -36.6368            |
| LaNH <sub>4</sub> B <sub>6</sub> C <sub>6</sub> | 28 LaC <sub>2</sub> + 6 B + 28 H <sub>3</sub> N → 10 H <sub>8</sub> C <sub>5</sub> + 27 LaN + LaB <sub>6</sub> H <sub>4</sub> C <sub>6</sub> N                                                         | -36.0248            |
| LaNH <sub>4</sub> B <sub>6</sub> C <sub>6</sub> | 38 H <sub>3</sub> N + 3 B <sub>13</sub> C <sub>2</sub> + LaB <sub>4</sub> → 55 H <sub>2</sub> + 37 BN + LaB <sub>6</sub> H <sub>4</sub> C <sub>6</sub> N                                               | -35.2420            |
| LaNH <sub>4</sub> B <sub>6</sub> C <sub>6</sub> | 0.5 H <sub>8</sub> C <sub>5</sub> + LaN + 8.375 N <sub>2</sub> + 1.75 B <sub>13</sub> C <sub>2</sub> → 16.75 BN + LaB <sub>6</sub> H <sub>4</sub> C <sub>6</sub> N                                     | -34.1957            |
| LaNH <sub>4</sub> B <sub>6</sub> C <sub>6</sub> | La + 34 H <sub>3</sub> N + 3 B <sub>13</sub> C <sub>2</sub> → 49 H <sub>2</sub> + 33 BN + LaB <sub>6</sub> H <sub>4</sub> C <sub>6</sub> N                                                             | -33.1176            |
| LaNH <sub>4</sub> B <sub>6</sub> C <sub>6</sub> | 33 H <sub>3</sub> N + LaN + 3 B <sub>13</sub> C <sub>2</sub> → 47.5 H <sub>2</sub> + 33 BN + LaB <sub>6</sub> H <sub>4</sub> C <sub>6</sub> N                                                          | -31.7843            |
| LaNH <sub>4</sub> B <sub>6</sub> C <sub>6</sub> | 173 LaH <sub>3</sub> + 34 LaN + 3 B <sub>13</sub> C <sub>2</sub> → 33 BN + 103 La <sub>2</sub> H <sub>5</sub> + LaB <sub>6</sub> H <sub>4</sub> C <sub>6</sub> N                                       | -31.7294            |
| LaNH <sub>4</sub> B <sub>6</sub> C <sub>6</sub> | 34 H <sub>3</sub> N + LaH <sub>2</sub> + 3 B <sub>13</sub> C <sub>2</sub> → 50 H <sub>2</sub> + 33 BN + LaB <sub>6</sub> H <sub>4</sub> C <sub>6</sub> N                                               | -31.2363            |
| LaNH <sub>4</sub> B <sub>6</sub> C <sub>6</sub> | 0.25 La <sub>4</sub> H <sub>9</sub> + 34 H <sub>3</sub> N + 3 B <sub>13</sub> C <sub>2</sub> → 50.12 H <sub>2</sub> + 33 BN + LaB <sub>6</sub> H <sub>4</sub> C <sub>6</sub> N                         | -31.1115            |
| LaNH <sub>4</sub> B <sub>6</sub> C <sub>6</sub> | 34 H <sub>3</sub> N + 3 B <sub>13</sub> C <sub>2</sub> + 0.5 La <sub>2</sub> H <sub>5</sub> → 50.25 H <sub>2</sub> + 33 BN + LaB <sub>6</sub> H <sub>4</sub> C <sub>6</sub> N                          | -31.0013            |
| LaNH <sub>4</sub> B <sub>6</sub> C <sub>6</sub> | LaH <sub>3</sub> + 34 H <sub>3</sub> N + 3 B <sub>13</sub> C <sub>2</sub> → 50.5 H <sub>2</sub> + 33 BN + LaB <sub>6</sub> H <sub>4</sub> C <sub>6</sub> N                                             | -30.8517            |
| LaNH <sub>4</sub> B <sub>6</sub> C <sub>6</sub> | 1.2 H <sub>8</sub> C <sub>5</sub> + 3.8 LaB <sub>6</sub> + 8.9 N <sub>2</sub> → 16.8 BN + 2.8 LaH <sub>2</sub> + LaB <sub>6</sub> H <sub>4</sub> C <sub>6</sub> N                                      | -27.8863            |
| LaNH <sub>4</sub> B <sub>6</sub> C <sub>6</sub> | 1.2 H <sub>8</sub> C <sub>5</sub> + 24.33 LaN + 5.867 B <sub>5</sub> H <sub>7</sub> → 23.33 BN + 23.33 LaH <sub>2</sub> + LaB <sub>6</sub> H <sub>4</sub> C <sub>6</sub> N                             | -27.4521            |
| LaNH <sub>4</sub> B <sub>6</sub> C <sub>6</sub> | 104.3 LaH <sub>3</sub> + 34 LaN + 3 B <sub>13</sub> C <sub>2</sub> → 33 BN + 34.33 La <sub>4</sub> H <sub>9</sub> + LaB <sub>6</sub> H <sub>4</sub> C <sub>6</sub> N                                   | -26.8815            |
| LaNH <sub>4</sub> B <sub>6</sub> C <sub>6</sub> | 20.62 LaC <sub>2</sub> + 20.62 H <sub>3</sub> N + 0.4615 B <sub>13</sub> C <sub>2</sub> → 7.231 H <sub>8</sub> C <sub>5</sub> + 19.62 LaN + LaB <sub>6</sub> H <sub>4</sub> C <sub>6</sub> N           | -24.2035            |
| LaNH <sub>4</sub> B <sub>6</sub> C <sub>6</sub> | 1.2 H <sub>8</sub> C <sub>5</sub> + 3.489 LaB <sub>6</sub> + 7.967 N <sub>2</sub> → 14.93 BN + 0.6222 La <sub>4</sub> H <sub>9</sub> + LaB <sub>6</sub> H <sub>4</sub> C <sub>6</sub> N                | -24.0452            |
| LaNH <sub>4</sub> B <sub>6</sub> C <sub>6</sub> | 70 LaH <sub>3</sub> + 34 LaN + 3 B <sub>13</sub> C <sub>2</sub> → 33 BN + 103 LaH <sub>2</sub> + LaB <sub>6</sub> H <sub>4</sub> C <sub>6</sub> N                                                      | -22.9435            |
| LaNH <sub>4</sub> B <sub>6</sub> C <sub>6</sub> | 24.25 H <sub>3</sub> N + 0.5 La <sub>2</sub> C <sub>3</sub> + 2.25 B <sub>13</sub> C <sub>2</sub> → 34.37 H <sub>2</sub> + 23.25 BN + LaB <sub>6</sub> H <sub>4</sub> C <sub>6</sub> N                 | -21.3849            |
| LaNH <sub>4</sub> B <sub>6</sub> C <sub>6</sub> | 1.2 H <sub>8</sub> C <sub>5</sub> + 3.24 LaB <sub>6</sub> + 7.22 N <sub>2</sub> → 13.44 BN + 1.12 La <sub>2</sub> H <sub>5</sub> + LaB <sub>6</sub> H <sub>4</sub> C <sub>6</sub> N                    | -20.9395            |
| LaNH <sub>4</sub> B <sub>6</sub> C <sub>6</sub> | 16.73 La + 16.73 H <sub>3</sub> N + 3 B <sub>13</sub> C <sub>2</sub> → 15.73 LaN + 6.6 B <sub>5</sub> H <sub>7</sub> + LaB <sub>6</sub> H <sub>4</sub> C <sub>6</sub> N                                | -19.9828            |
| LaNH <sub>4</sub> B <sub>6</sub> C <sub>6</sub> | 34 LaN + 3 B <sub>13</sub> C <sub>2</sub> + 156.5 La <sub>2</sub> H <sub>5</sub> → 33 BN + 86.5 La <sub>4</sub> H <sub>9</sub> + LaB <sub>6</sub> H <sub>4</sub> C <sub>6</sub> N                      | -19.5156            |
| LaNH <sub>4</sub> B <sub>6</sub> C <sub>6</sub> | 1.2 H <sub>8</sub> C <sub>5</sub> + 17.47 LaN + 4.494 B <sub>5</sub> H <sub>7</sub> → 16.47 BN + 4.118 La <sub>4</sub> H <sub>9</sub> + LaB <sub>6</sub> H <sub>4</sub> C <sub>6</sub> N               | -18.6536            |
| LaNH <sub>4</sub> B <sub>6</sub> C <sub>6</sub> | 10.07 La + 0.3636 B <sub>9</sub> H <sub>11</sub> + 0.5 N <sub>2</sub> + 3 B <sub>13</sub> C <sub>2</sub> → 9.068 LaB <sub>4</sub> + LaB <sub>6</sub> H <sub>4</sub> C <sub>6</sub> N                   | -18.5845            |
| LaNH <sub>4</sub> B <sub>6</sub> C <sub>6</sub> | 9.964 La + 0.5714 B <sub>5</sub> H <sub>7</sub> + 0.5 N <sub>2</sub> + 3 B <sub>13</sub> C <sub>2</sub> → 8.964 LaB <sub>4</sub> + LaB <sub>6</sub> H <sub>4</sub> C <sub>6</sub> N                    | -18.3510            |
| LaNH <sub>4</sub> B <sub>6</sub> C <sub>6</sub> | LaC <sub>2</sub> + 21 H <sub>3</sub> N + 2 B <sub>13</sub> C <sub>2</sub> → 29.5 H <sub>2</sub> + 20 BN + LaB <sub>6</sub> H <sub>4</sub> C <sub>6</sub> N                                             | -17.5503            |
| LaNH <sub>4</sub> B <sub>6</sub> C <sub>6</sub> | 25.1 LaH <sub>2</sub> + 12.55 N <sub>2</sub> + 3 B <sub>13</sub> C <sub>2</sub> → 24.1 LaN + 6.6 B <sub>5</sub> H <sub>7</sub> + LaB <sub>6</sub> H <sub>4</sub> C <sub>6</sub> N                      | -17.1521            |
| LaNH <sub>4</sub> B <sub>6</sub> C <sub>6</sub> | 14.78 La + 14.78 H <sub>3</sub> N + 3 B <sub>13</sub> C <sub>2</sub> → 13.78 LaN + 3.667 B <sub>9</sub> H <sub>11</sub> + LaB <sub>6</sub> H <sub>4</sub> C <sub>6</sub> N                             | -17.1275            |
| LaNH <sub>4</sub> B <sub>6</sub> C <sub>6</sub> | 1.2 H <sub>8</sub> C <sub>5</sub> + 17.63 LaN + 2.514 B <sub>9</sub> H <sub>11</sub> → 16.63 BN + 16.63 LaH <sub>2</sub> + LaB <sub>6</sub> H <sub>4</sub> C <sub>6</sub> N                            | -17.0174            |
| LaNH <sub>4</sub> B <sub>6</sub> C <sub>6</sub> | 34 LaN + 3 B <sub>13</sub> C <sub>2</sub> + 70 La <sub>2</sub> H <sub>5</sub> → 33 BN + 173 LaH <sub>2</sub> + LaB <sub>6</sub> H <sub>4</sub> C <sub>6</sub> N                                        | -16.9725            |
| LaNH <sub>4</sub> B <sub>6</sub> C <sub>6</sub> | 2 H <sub>2</sub> + 9.25 La + 0.5 N <sub>2</sub> + 3 B <sub>13</sub> C <sub>2</sub> → 8.25 LaB <sub>4</sub> + LaB <sub>6</sub> H <sub>4</sub> C <sub>6</sub> N                                          | -16.9151            |
| LaNH <sub>4</sub> B <sub>6</sub> C <sub>6</sub> | 10.32 La + BN + 0.3636 B <sub>9</sub> H <sub>11</sub> + 3 B <sub>13</sub> C <sub>2</sub> → 9.318 LaB <sub>4</sub> + LaB <sub>6</sub> H <sub>4</sub> C <sub>6</sub> N                                   | -16.7293            |
| LaNH <sub>4</sub> B <sub>6</sub> C <sub>6</sub> | 7.045 La + 0.3636 B <sub>9</sub> H <sub>11</sub> + 0.5 N <sub>2</sub> + 3 B <sub>13</sub> C <sub>2</sub> → 6.045 LaB <sub>6</sub> + LaB <sub>6</sub> H <sub>4</sub> C <sub>6</sub> N                   | -16.5741            |
| LaNH <sub>4</sub> B <sub>6</sub> C <sub>6</sub> | 10.21 La + BN + 0.5714 B <sub>5</sub> H <sub>7</sub> + 3 B <sub>13</sub> C <sub>2</sub> → 9.214 LaB <sub>4</sub> + LaB <sub>6</sub> H <sub>4</sub> C <sub>6</sub> N                                    | -16.4958            |
| LaNH <sub>4</sub> B <sub>6</sub> C <sub>6</sub> | 6.976 La + 0.5714 B <sub>5</sub> H <sub>7</sub> + 0.5 N <sub>2</sub> + 3 B <sub>13</sub> C <sub>2</sub> → 5.976 LaB <sub>6</sub> + LaB <sub>6</sub> H <sub>4</sub> C <sub>6</sub> N                    | -16.3637            |

Continued on next page

Continued

| Compound                                        | Chemical reaction                                                                                                                                                                                  | Reaction energy(eV) |
|-------------------------------------------------|----------------------------------------------------------------------------------------------------------------------------------------------------------------------------------------------------|---------------------|
| LaNH <sub>4</sub> B <sub>6</sub> C <sub>6</sub> | 1.2 H <sub>8</sub> C <sub>5</sub> + 2.867 LaB <sub>6</sub> + 6.1 N <sub>2</sub> → 1.867 LaH <sub>3</sub> + 11.2 BN + LaB <sub>6</sub> H <sub>4</sub> C <sub>6</sub> N                              | -16.1490            |
| LaNH <sub>4</sub> B <sub>6</sub> C <sub>6</sub> | 9.583 La + 1.333 H <sub>3</sub> N + 3 B <sub>13</sub> C <sub>2</sub> → 0.3333 LaN + 8.25 LaB <sub>4</sub> + LaB <sub>6</sub> H <sub>4</sub> C <sub>6</sub> N                                       | -16.0354            |
| LaNH <sub>4</sub> B <sub>6</sub> C <sub>6</sub> | 9.455 La + H <sub>3</sub> N + 0.09091 B <sub>9</sub> H <sub>11</sub> + 3 B <sub>13</sub> C <sub>2</sub> → 8.455 LaB <sub>4</sub> + LaB <sub>6</sub> H <sub>4</sub> C <sub>6</sub> N                | -16.0084            |
| LaNH <sub>4</sub> B <sub>6</sub> C <sub>6</sub> | 9.429 La + H <sub>3</sub> N + 0.1429 B <sub>5</sub> H <sub>7</sub> + 3 B <sub>13</sub> C <sub>2</sub> → 8.429 LaB <sub>4</sub> + LaB <sub>6</sub> H <sub>4</sub> C <sub>6</sub> N                  | -15.9500            |
| LaNH <sub>4</sub> B <sub>6</sub> C <sub>6</sub> | 9.068 La + LaN + 0.3636 B <sub>9</sub> H <sub>11</sub> + 3 B <sub>13</sub> C <sub>2</sub> → 9.068 LaB <sub>4</sub> + LaB <sub>6</sub> H <sub>4</sub> C <sub>6</sub> N                              | -15.9271            |
| LaNH <sub>4</sub> B <sub>6</sub> C <sub>6</sub> | 9.167 La + 1.333 H <sub>3</sub> N + 3 B <sub>13</sub> C <sub>2</sub> → 0.3333 BN + 8.167 LaB <sub>4</sub> + LaB <sub>6</sub> H <sub>4</sub> C <sub>6</sub> N                                       | -15.7681            |
| LaNH <sub>4</sub> B <sub>6</sub> C <sub>6</sub> | 8.964 La + LaN + 0.5714 B <sub>5</sub> H <sub>7</sub> + 3 B <sub>13</sub> C <sub>2</sub> → 8.964 LaB <sub>4</sub> + LaB <sub>6</sub> H <sub>4</sub> C <sub>6</sub> N                               | -15.6937            |
| LaNH <sub>4</sub> B <sub>6</sub> C <sub>6</sub> | 0.5 H <sub>2</sub> + 9.25 La + H <sub>3</sub> N + 3 B <sub>13</sub> C <sub>2</sub> → 8.25 LaB <sub>4</sub> + LaB <sub>6</sub> H <sub>4</sub> C <sub>6</sub> N                                      | -15.5910            |
| LaNH <sub>4</sub> B <sub>6</sub> C <sub>6</sub> | 9.25 La + 1.333 H <sub>3</sub> N + 3 B <sub>13</sub> C <sub>2</sub> → 0.1667 N <sub>2</sub> + 8.25 LaB <sub>4</sub> + LaB <sub>6</sub> H <sub>4</sub> C <sub>6</sub> N                             | -15.1497            |
| LaNH <sub>4</sub> B <sub>6</sub> C <sub>6</sub> | 2 H <sub>2</sub> + 6.5 La + 0.5 N <sub>2</sub> + 3 B <sub>13</sub> C <sub>2</sub> → 5.5 LaB <sub>6</sub> + LaB <sub>6</sub> H <sub>4</sub> C <sub>6</sub> N                                        | -15.0861            |
| LaNH <sub>4</sub> B <sub>6</sub> C <sub>6</sub> | 2 H <sub>2</sub> + 9.5 La + BN + 3 B <sub>13</sub> C <sub>2</sub> → 8.5 LaB <sub>4</sub> + LaB <sub>6</sub> H <sub>4</sub> C <sub>6</sub> N                                                        | -15.0599            |
| LaNH <sub>4</sub> B <sub>6</sub> C <sub>6</sub> | 70 La <sub>4</sub> H <sub>9</sub> + 34 LaN + 3 B <sub>13</sub> C <sub>2</sub> → 33 BN + 313 LaH <sub>2</sub> + LaB <sub>6</sub> H <sub>4</sub> C <sub>6</sub> N                                    | -14.9145            |
| LaNH <sub>4</sub> B <sub>6</sub> C <sub>6</sub> | 0.3333 LaH <sub>3</sub> + 8.917 La + H <sub>3</sub> N + 3 B <sub>13</sub> C <sub>2</sub> → 8.25 LaB <sub>4</sub> + LaB <sub>6</sub> H <sub>4</sub> C <sub>6</sub> N                                | -14.8357            |
| LaNH <sub>4</sub> B <sub>6</sub> C <sub>6</sub> | 2 La <sub>2</sub> C <sub>3</sub> + 4.8 B <sub>5</sub> H <sub>7</sub> + 5.433 N <sub>2</sub> → 3 LaB <sub>6</sub> + 9.867 H <sub>3</sub> N + LaB <sub>6</sub> H <sub>4</sub> C <sub>6</sub> N       | -14.8262            |
| LaNH <sub>4</sub> B <sub>6</sub> C <sub>6</sub> | 8.85 La + H <sub>3</sub> N + 3 B <sub>13</sub> C <sub>2</sub> + 0.2 La <sub>2</sub> H <sub>5</sub> → 8.25 LaB <sub>4</sub> + LaB <sub>6</sub> H <sub>4</sub> C <sub>6</sub> N                      | -14.7445            |
| LaNH <sub>4</sub> B <sub>6</sub> C <sub>6</sub> | 8.806 La + 0.1111 La <sub>4</sub> H <sub>9</sub> + H <sub>3</sub> N + 3 B <sub>13</sub> C <sub>2</sub> → 8.25 LaB <sub>4</sub> + LaB <sub>6</sub> H <sub>4</sub> C <sub>6</sub> N                  | -14.6994            |
| LaNH <sub>4</sub> B <sub>6</sub> C <sub>6</sub> | 7.212 La + BN + 0.3636 B <sub>9</sub> H <sub>11</sub> + 3 B <sub>13</sub> C <sub>2</sub> → 6.212 LaB <sub>6</sub> + LaB <sub>6</sub> H <sub>4</sub> C <sub>6</sub> N                               | -14.6635            |
| LaNH <sub>4</sub> B <sub>6</sub> C <sub>6</sub> | 8.75 La + H <sub>3</sub> N + 0.5 LaH <sub>2</sub> + 3 B <sub>13</sub> C <sub>2</sub> → 8.25 LaB <sub>4</sub> + LaB <sub>6</sub> H <sub>4</sub> C <sub>6</sub> N                                    | -14.6504            |
| LaNH <sub>4</sub> B <sub>6</sub> C <sub>6</sub> | 22.17 LaH <sub>2</sub> + 11.08 N <sub>2</sub> + 3 B <sub>13</sub> C <sub>2</sub> → 21.17 LaN + 3.667 B <sub>9</sub> H <sub>11</sub> + LaB <sub>6</sub> H <sub>4</sub> C <sub>6</sub> N             | -14.6277            |
| LaNH <sub>4</sub> B <sub>6</sub> C <sub>6</sub> | 6 BN + 14.67 H <sub>3</sub> N + 10.33 La <sub>2</sub> C <sub>3</sub> → 5 H <sub>8</sub> C <sub>5</sub> + 19.67 LaN + LaB <sub>6</sub> H <sub>4</sub> C <sub>6</sub> N                              | -14.5320            |
| LaNH <sub>4</sub> B <sub>6</sub> C <sub>6</sub> | 7.143 La + BN + 0.5714 B <sub>5</sub> H <sub>7</sub> + 3 B <sub>13</sub> C <sub>2</sub> → 6.143 LaB <sub>6</sub> + LaB <sub>6</sub> H <sub>4</sub> C <sub>6</sub> N                                | -14.4531            |
| LaNH <sub>4</sub> B <sub>6</sub> C <sub>6</sub> | 2 H <sub>2</sub> + 8.25 La + LaN + 3 B <sub>13</sub> C <sub>2</sub> → 8.25 LaB <sub>4</sub> + LaB <sub>6</sub> H <sub>4</sub> C <sub>6</sub> N                                                     | -14.2578            |
| LaNH <sub>4</sub> B <sub>6</sub> C <sub>6</sub> | 6.833 La + 1.333 H <sub>3</sub> N + 3 B <sub>13</sub> C <sub>2</sub> → 5.5 LaB <sub>6</sub> + 0.3333 LaN + LaB <sub>6</sub> H <sub>4</sub> C <sub>6</sub> N                                        | -14.2064            |
| LaNH <sub>4</sub> B <sub>6</sub> C <sub>6</sub> | 6.636 La + H <sub>3</sub> N + 0.09091 B <sub>9</sub> H <sub>11</sub> + 3 B <sub>13</sub> C <sub>2</sub> → 5.636 LaB <sub>6</sub> + LaB <sub>6</sub> H <sub>4</sub> C <sub>6</sub> N                | -14.1340            |
| LaNH <sub>4</sub> B <sub>6</sub> C <sub>6</sub> | 6.619 La + H <sub>3</sub> N + 0.1429 B <sub>5</sub> H <sub>7</sub> + 3 B <sub>13</sub> C <sub>2</sub> → 5.619 LaB <sub>6</sub> + LaB <sub>6</sub> H <sub>4</sub> C <sub>6</sub> N                  | -14.0814            |
| LaNH <sub>4</sub> B <sub>6</sub> C <sub>6</sub> | 24.47 LaN + 6.765 B <sub>9</sub> H <sub>11</sub> + 3 B <sub>13</sub> C <sub>2</sub> → 23.47 H <sub>3</sub> N + 23.47 LaB <sub>4</sub> + LaB <sub>6</sub> H <sub>4</sub> C <sub>6</sub> N           | -14.0206            |
| LaNH <sub>4</sub> B <sub>6</sub> C <sub>6</sub> | 6.444 La + 1.333 H <sub>3</sub> N + 3 B <sub>13</sub> C <sub>2</sub> → 5.444 LaB <sub>6</sub> + 0.3333 BN + LaB <sub>6</sub> H <sub>4</sub> C <sub>6</sub> N                                       | -13.9575            |
| LaNH <sub>4</sub> B <sub>6</sub> C <sub>6</sub> | 6.045 La + LaN + 0.3636 B <sub>9</sub> H <sub>11</sub> + 3 B <sub>13</sub> C <sub>2</sub> → 6.045 LaB <sub>6</sub> + LaB <sub>6</sub> H <sub>4</sub> C <sub>6</sub> N                              | -13.9168            |
| LaNH <sub>4</sub> B <sub>6</sub> C <sub>6</sub> | 1.333 LaH <sub>3</sub> + 7.917 La + 0.5 N <sub>2</sub> + 3 B <sub>13</sub> C <sub>2</sub> → 8.25 LaB <sub>4</sub> + LaB <sub>6</sub> H <sub>4</sub> C <sub>6</sub> N                               | -13.8939            |
| LaNH <sub>4</sub> B <sub>6</sub> C <sub>6</sub> | 0.5 H <sub>2</sub> + 6.5 La + H <sub>3</sub> N + 3 B <sub>13</sub> C <sub>2</sub> → 5.5 LaB <sub>6</sub> + LaB <sub>6</sub> H <sub>4</sub> C <sub>6</sub> N                                        | -13.7620            |
| LaNH <sub>4</sub> B <sub>6</sub> C <sub>6</sub> | 5.976 La + LaN + 0.5714 B <sub>5</sub> H <sub>7</sub> + 3 B <sub>13</sub> C <sub>2</sub> → 5.976 LaB <sub>6</sub> + LaB <sub>6</sub> H <sub>4</sub> C <sub>6</sub> N                               | -13.7063            |
| LaNH <sub>4</sub> B <sub>6</sub> C <sub>6</sub> | 1.2 H <sub>8</sub> C <sub>5</sub> + 13.73 LaN + 3.745 B <sub>5</sub> H <sub>7</sub> → 12.73 BN + 6.364 La <sub>2</sub> H <sub>5</sub> + LaB <sub>6</sub> H <sub>4</sub> C <sub>6</sub> N           | -13.6672            |
| LaNH <sub>4</sub> B <sub>6</sub> C <sub>6</sub> | 7.65 La + 0.5 N <sub>2</sub> + 3 B <sub>13</sub> C <sub>2</sub> + 0.8 La <sub>2</sub> H <sub>5</sub> → 8.25 LaB <sub>4</sub> + LaB <sub>6</sub> H <sub>4</sub> C <sub>6</sub> N                    | -13.5291            |
| LaNH <sub>4</sub> B <sub>6</sub> C <sub>6</sub> | 7.472 La + 0.4444 La <sub>4</sub> H <sub>9</sub> + 0.5 N <sub>2</sub> + 3 B <sub>13</sub> C <sub>2</sub> → 8.25 LaB <sub>4</sub> + LaB <sub>6</sub> H <sub>4</sub> C <sub>6</sub> N                | -13.3487            |
| LaNH <sub>4</sub> B <sub>6</sub> C <sub>6</sub> | 6.5 La + 1.333 H <sub>3</sub> N + 3 B <sub>13</sub> C <sub>2</sub> → 5.5 LaB <sub>6</sub> + 0.1667 N <sub>2</sub> + LaB <sub>6</sub> H <sub>4</sub> C <sub>6</sub> N                               | -13.3207            |
| LaNH <sub>4</sub> B <sub>6</sub> C <sub>6</sub> | 2 H <sub>2</sub> + 6.667 La + BN + 3 B <sub>13</sub> C <sub>2</sub> → 5.667 LaB <sub>6</sub> + LaB <sub>6</sub> H <sub>4</sub> C <sub>6</sub> N                                                    | -13.1755            |
| LaNH <sub>4</sub> B <sub>6</sub> C <sub>6</sub> | 7.25 La + 2 LaH <sub>2</sub> + 0.5 N <sub>2</sub> + 3 B <sub>13</sub> C <sub>2</sub> → 8.25 LaB <sub>4</sub> + LaB <sub>6</sub> H <sub>4</sub> C <sub>6</sub> N                                    | -13.1526            |
| LaNH <sub>4</sub> B <sub>6</sub> C <sub>6</sub> | 2.667 B <sub>9</sub> H <sub>11</sub> + 2 La <sub>2</sub> C <sub>3</sub> + 4.722 N <sub>2</sub> → 3 LaB <sub>6</sub> + 8.444 H <sub>3</sub> N + LaB <sub>6</sub> H <sub>4</sub> C <sub>6</sub> N    | -13.1234            |
| LaNH <sub>4</sub> B <sub>6</sub> C <sub>6</sub> | 0.3333 LaH <sub>3</sub> + 6.167 La + H <sub>3</sub> N + 3 B <sub>13</sub> C <sub>2</sub> → 5.5 LaB <sub>6</sub> + LaB <sub>6</sub> H <sub>4</sub> C <sub>6</sub> N                                 | -13.0067            |
| LaNH <sub>4</sub> B <sub>6</sub> C <sub>6</sub> | 6.1 La + H <sub>3</sub> N + 3 B <sub>13</sub> C <sub>2</sub> + 0.2 La <sub>2</sub> H <sub>5</sub> → 5.5 LaB <sub>6</sub> + LaB <sub>6</sub> H <sub>4</sub> C <sub>6</sub> N                        | -12.9155            |
| LaNH <sub>4</sub> B <sub>6</sub> C <sub>6</sub> | 6.056 La + 0.1111 La <sub>4</sub> H <sub>9</sub> + H <sub>3</sub> N + 3 B <sub>13</sub> C <sub>2</sub> → 5.5 LaB <sub>6</sub> + LaB <sub>6</sub> H <sub>4</sub> C <sub>6</sub> N                   | -12.8704            |
| LaNH <sub>4</sub> B <sub>6</sub> C <sub>6</sub> | 6 La + H <sub>3</sub> N + 0.5 LaH <sub>2</sub> + 3 B <sub>13</sub> C <sub>2</sub> → 5.5 LaB <sub>6</sub> + LaB <sub>6</sub> H <sub>4</sub> C <sub>6</sub> N                                        | -12.8214            |
| LaNH <sub>4</sub> B <sub>6</sub> C <sub>6</sub> | 0.125 H <sub>8</sub> C <sub>5</sub> + 8.234 La + H <sub>3</sub> N + 2.687 B <sub>13</sub> C <sub>2</sub> → 7.234 LaB <sub>4</sub> + LaB <sub>6</sub> H <sub>4</sub> C <sub>6</sub> N               | -12.8070            |
| LaNH <sub>4</sub> B <sub>6</sub> C <sub>6</sub> | 1.2 H <sub>8</sub> C <sub>5</sub> + 5.1 N <sub>2</sub> + 3.8 LaB <sub>4</sub> → 9.2 BN + 2.8 LaH <sub>2</sub> + LaB <sub>6</sub> H <sub>4</sub> C <sub>6</sub> N                                   | -12.5232            |
| LaNH <sub>4</sub> B <sub>6</sub> C <sub>6</sub> | 2 H <sub>2</sub> + 5.5 La + LaN + 3 B <sub>13</sub> C <sub>2</sub> → 5.5 LaB <sub>6</sub> + LaB <sub>6</sub> H <sub>4</sub> C <sub>6</sub> N                                                       | -12.4288            |
| LaNH <sub>4</sub> B <sub>6</sub> C <sub>6</sub> | 0.5 H <sub>8</sub> C <sub>5</sub> + 0.5 La <sub>2</sub> C <sub>3</sub> + 4 N <sub>2</sub> + B <sub>13</sub> C <sub>2</sub> → 7 BN + LaB <sub>6</sub> H <sub>4</sub> C <sub>6</sub> N               | -12.2107            |
| LaNH <sub>4</sub> B <sub>6</sub> C <sub>6</sub> | 5.578 La <sub>4</sub> H <sub>9</sub> + 11.16 N <sub>2</sub> + 3 B <sub>13</sub> C <sub>2</sub> → 21.31 LaN + 6.6 B <sub>5</sub> H <sub>7</sub> + LaB <sub>6</sub> H <sub>4</sub> C <sub>6</sub> N  | -12.2025            |
| LaNH <sub>4</sub> B <sub>6</sub> C <sub>6</sub> | 42 B + LaN + 2 La <sub>2</sub> C <sub>3</sub> + 2 LaH <sub>2</sub> → 6 LaB <sub>6</sub> + LaB <sub>6</sub> H <sub>4</sub> C <sub>6</sub> N                                                         | -12.1691            |
| LaNH <sub>4</sub> B <sub>6</sub> C <sub>6</sub> | 1.2 H <sub>8</sub> C <sub>5</sub> + 13.58 LaN + 2.065 B <sub>9</sub> H <sub>11</sub> → 12.58 BN + 3.146 La <sub>4</sub> H <sub>9</sub> + LaB <sub>6</sub> H <sub>4</sub> C <sub>6</sub> N          | -12.1603            |
| LaNH <sub>4</sub> B <sub>6</sub> C <sub>6</sub> | 1.333 LaH <sub>3</sub> + 5.167 La + 0.5 N <sub>2</sub> + 3 B <sub>13</sub> C <sub>2</sub> → 5.5 LaB <sub>6</sub> + LaB <sub>6</sub> H <sub>4</sub> C <sub>6</sub> N                                | -12.0649            |
| LaNH <sub>4</sub> B <sub>6</sub> C <sub>6</sub> | 1.333 LaH <sub>3</sub> + 8.167 La + BN + 3 B <sub>13</sub> C <sub>2</sub> → 8.5 LaB <sub>4</sub> + LaB <sub>6</sub> H <sub>4</sub> C <sub>6</sub> N                                                | -12.0387            |
| LaNH <sub>4</sub> B <sub>6</sub> C <sub>6</sub> | 0.3636 B <sub>9</sub> H <sub>11</sub> + 0.5 N <sub>2</sub> + 3 B <sub>13</sub> C <sub>2</sub> + 21.14 LaB <sub>4</sub> → 20.14 LaB <sub>6</sub> + LaB <sub>6</sub> H <sub>4</sub> C <sub>6</sub> N | -11.8882            |
| LaNH <sub>4</sub> B <sub>6</sub> C <sub>6</sub> | 0.5714 B <sub>5</sub> H <sub>7</sub> + 0.5 N <sub>2</sub> + 3 B <sub>13</sub> C <sub>2</sub> + 20.93 LaB <sub>4</sub> → 19.93 LaB <sub>6</sub> + LaB <sub>6</sub> H <sub>4</sub> C <sub>6</sub> N  | -11.7239            |
| LaNH <sub>4</sub> B <sub>6</sub> C <sub>6</sub> | 4.9 La + 0.5 N <sub>2</sub> + 3 B <sub>13</sub> C <sub>2</sub> + 0.8 La <sub>2</sub> H <sub>5</sub> → 5.5 LaB <sub>6</sub> + LaB <sub>6</sub> H <sub>4</sub> C <sub>6</sub> N                      | -11.7001            |
| LaNH <sub>4</sub> B <sub>6</sub> C <sub>6</sub> | 11.23 LaN + 3.154 B <sub>9</sub> H <sub>11</sub> + 3 B <sub>13</sub> C <sub>2</sub> → 10.23 LaB <sub>6</sub> + 10.23 H <sub>3</sub> N + LaB <sub>6</sub> H <sub>4</sub> C <sub>6</sub> N           | -11.6939            |
| LaNH <sub>4</sub> B <sub>6</sub> C <sub>6</sub> | 7.9 La + BN + 3 B <sub>13</sub> C <sub>2</sub> + 0.8 La <sub>2</sub> H <sub>5</sub> → 8.5 LaB <sub>4</sub> + LaB <sub>6</sub> H <sub>4</sub> C <sub>6</sub> N                                      | -11.6739            |
| LaNH <sub>4</sub> B <sub>6</sub> C <sub>6</sub> | 1.182 B <sub>9</sub> H <sub>11</sub> + 2 La <sub>2</sub> C <sub>3</sub> + 2.818 N <sub>2</sub> → 3 LaH <sub>3</sub> + 4.636 BN + LaB <sub>6</sub> H <sub>4</sub> C <sub>6</sub> N                  | -11.5223            |
| LaNH <sub>4</sub> B <sub>6</sub> C <sub>6</sub> | 4.722 La + 0.4444 La <sub>4</sub> H <sub>9</sub> + 0.5 N <sub>2</sub> + 3 B <sub>13</sub> C <sub>2</sub> → 5.5 LaB <sub>6</sub> + LaB <sub>6</sub> H <sub>4</sub> C <sub>6</sub> N                 | -11.5197            |
| LaNH <sub>4</sub> B <sub>6</sub> C <sub>6</sub> | 7.722 La + BN + 0.4444 La <sub>4</sub> H <sub>9</sub> + 3 B <sub>13</sub> C <sub>2</sub> → 8.5 LaB <sub>4</sub> + LaB <sub>6</sub> H <sub>4</sub> C <sub>6</sub> N                                 | -11.4935            |
| LaNH <sub>4</sub> B <sub>6</sub> C <sub>6</sub> | 40.67 B + 0.4444 La <sub>4</sub> H <sub>9</sub> + LaN + 2 La <sub>2</sub> C <sub>3</sub> → 5.778 LaB <sub>6</sub> + LaB <sub>6</sub> H <sub>4</sub> C <sub>6</sub> N                               | -11.4904            |

Continued on next page



Continued

| Compound                                        | Chemical reaction                                                                                                                                                                                   | Reaction energy(eV) |
|-------------------------------------------------|-----------------------------------------------------------------------------------------------------------------------------------------------------------------------------------------------------|---------------------|
| LaNH <sub>4</sub> B <sub>6</sub> C <sub>6</sub> | 4.5 La + 2 LaH <sub>2</sub> + 0.5 N <sub>2</sub> + 3 B <sub>13</sub> C <sub>2</sub> → 5.5 LaB <sub>6</sub> + LaB <sub>6</sub> H <sub>4</sub> C <sub>6</sub> N                                       | -11.3236            |
| LaNH <sub>4</sub> B <sub>6</sub> C <sub>6</sub> | 7.5 La + BN + 2 LaH <sub>2</sub> + 3 B <sub>13</sub> C <sub>2</sub> → 8.5 LaB <sub>4</sub> + LaB <sub>6</sub> H <sub>4</sub> C <sub>6</sub> N                                                       | -11.2974            |
| LaNH <sub>4</sub> B <sub>6</sub> C <sub>6</sub> | 1.333 LaH <sub>3</sub> + 6.917 La + LaN + 3 B <sub>13</sub> C <sub>2</sub> → 8.25 LaB <sub>4</sub> + LaB <sub>6</sub> H <sub>4</sub> C <sub>6</sub> N                                               | -11.2365            |
| LaNH <sub>4</sub> B <sub>6</sub> C <sub>6</sub> | 0.125 H <sub>8</sub> C <sub>5</sub> + 5.823 La + H <sub>3</sub> N + 2.688 B <sub>13</sub> C <sub>2</sub> → 4.823 LaB <sub>6</sub> + LaB <sub>6</sub> H <sub>4</sub> C <sub>6</sub> N                | -11.2031            |
| LaNH <sub>4</sub> B <sub>6</sub> C <sub>6</sub> | 39.6 B + LaN + 2 La <sub>2</sub> C <sub>3</sub> + 0.8 La <sub>2</sub> H <sub>5</sub> → 5.6 LaB <sub>6</sub> + LaB <sub>6</sub> H <sub>4</sub> C <sub>6</sub> N                                      | -10.9709            |
| LaNH <sub>4</sub> B <sub>6</sub> C <sub>6</sub> | 36 B + 2 La <sub>2</sub> C <sub>3</sub> + 2 LaH <sub>2</sub> + 0.5 N <sub>2</sub> → 5 LaB <sub>6</sub> + LaB <sub>6</sub> H <sub>4</sub> C <sub>6</sub> N                                           | -10.8895            |
| LaNH <sub>4</sub> B <sub>6</sub> C <sub>6</sub> | 6.65 La + LaN + 3 B <sub>13</sub> C <sub>2</sub> + 0.8 La <sub>2</sub> H <sub>5</sub> → 8.25 LaB <sub>4</sub> + LaB <sub>6</sub> H <sub>4</sub> C <sub>6</sub> N                                    | -10.8718            |
| LaNH <sub>4</sub> B <sub>6</sub> C <sub>6</sub> | 2 H <sub>2</sub> + 0.5 N <sub>2</sub> + 3 B <sub>13</sub> C <sub>2</sub> + 19.5 LaB <sub>4</sub> → 18.5 LaB <sub>6</sub> + LaB <sub>6</sub> H <sub>4</sub> C <sub>6</sub> N                         | -10.7630            |
| LaNH <sub>4</sub> B <sub>6</sub> C <sub>6</sub> | 20.31 LaN + 8.846 B <sub>5</sub> H <sub>7</sub> + 3 B <sub>13</sub> C <sub>2</sub> → 19.31 H <sub>3</sub> N + 19.31 LaB <sub>4</sub> + LaB <sub>6</sub> H <sub>4</sub> C <sub>6</sub> N             | -10.7447            |
| LaNH <sub>4</sub> B <sub>6</sub> C <sub>6</sub> | 6.472 La + 0.4444 La <sub>4</sub> H <sub>9</sub> + LaN + 3 B <sub>13</sub> C <sub>2</sub> → 8.25 LaB <sub>4</sub> + LaB <sub>6</sub> H <sub>4</sub> C <sub>6</sub> N                                | -10.6913            |
| LaNH <sub>4</sub> B <sub>6</sub> C <sub>6</sub> | 6.25 La + LaN + 2 LaH <sub>2</sub> + 3 B <sub>13</sub> C <sub>2</sub> → 8.25 LaB <sub>4</sub> + LaB <sub>6</sub> H <sub>4</sub> C <sub>6</sub> N                                                    | -10.4952            |
| LaNH <sub>4</sub> B <sub>6</sub> C <sub>6</sub> | 1.333 LaH <sub>3</sub> + 38 B + LaN + 2 La <sub>2</sub> C <sub>3</sub> → 5.333 LaB <sub>6</sub> + LaB <sub>6</sub> H <sub>4</sub> C <sub>6</sub> N                                                  | -10.2858            |
| LaNH <sub>4</sub> B <sub>6</sub> C <sub>6</sub> | 4.926 La <sub>4</sub> H <sub>9</sub> + 9.852 N <sub>2</sub> + 3 B <sub>13</sub> C <sub>2</sub> → 18.7 LaN + 3.667 B <sub>9</sub> H <sub>11</sub> + LaB <sub>6</sub> H <sub>4</sub> C <sub>6</sub> N | -10.2565            |
| LaNH <sub>4</sub> B <sub>6</sub> C <sub>6</sub> | 10.3 LaN + 4.556 B <sub>5</sub> H <sub>7</sub> + 3 B <sub>13</sub> C <sub>2</sub> → 9.296 LaB <sub>6</sub> + 9.296 H <sub>3</sub> N + LaB <sub>6</sub> H <sub>4</sub> C <sub>6</sub> N              | -10.2194            |
| LaNH <sub>4</sub> B <sub>6</sub> C <sub>6</sub> | 34.67 B + 0.4444 La <sub>4</sub> H <sub>9</sub> + 2 La <sub>2</sub> C <sub>3</sub> + 0.5 N <sub>2</sub> → 4.778 LaB <sub>6</sub> + LaB <sub>6</sub> H <sub>4</sub> C <sub>6</sub> N                 | -10.2108            |
| LaNH <sub>4</sub> B <sub>6</sub> C <sub>6</sub> | 1.333 LaH <sub>3</sub> + 5.333 La + BN + 3 B <sub>13</sub> C <sub>2</sub> → 5.667 LaB <sub>6</sub> + LaB <sub>6</sub> H <sub>4</sub> C <sub>6</sub> N                                               | -10.1543            |
| LaNH <sub>4</sub> B <sub>6</sub> C <sub>6</sub> | 8.255 LaN + 0.3636 B <sub>9</sub> H <sub>11</sub> + 3 B <sub>13</sub> C <sub>2</sub> → 7.255 BN + 7.255 LaB <sub>4</sub> + LaB <sub>6</sub> H <sub>4</sub> C <sub>6</sub> N                         | -10.1078            |
| LaNH <sub>4</sub> B <sub>6</sub> C <sub>6</sub> | La + 11.73 H <sub>3</sub> N + 3 B <sub>13</sub> C <sub>2</sub> → 10.73 BN + 4.455 B <sub>5</sub> H <sub>7</sub> + LaB <sub>6</sub> H <sub>4</sub> C <sub>6</sub> N                                  | -10.0946            |
| LaNH <sub>4</sub> B <sub>6</sub> C <sub>6</sub> | 6.182 LaN + 0.3636 B <sub>9</sub> H <sub>11</sub> + 3 B <sub>13</sub> C <sub>2</sub> → 5.182 LaB <sub>6</sub> + 5.182 BN + LaB <sub>6</sub> H <sub>4</sub> C <sub>6</sub> N                         | -10.0473            |
| LaNH <sub>4</sub> B <sub>6</sub> C <sub>6</sub> | 8.171 LaN + 0.5714 B <sub>5</sub> H <sub>7</sub> + 3 B <sub>13</sub> C <sub>2</sub> → 7.171 BN + 7.171 LaB <sub>4</sub> + LaB <sub>6</sub> H <sub>4</sub> C <sub>6</sub> N                          | -9.9410             |
| LaNH <sub>4</sub> B <sub>6</sub> C <sub>6</sub> | 1.2 H <sub>8</sub> C <sub>5</sub> + 4.478 N <sub>2</sub> + 3.489 LaB <sub>4</sub> → 7.956 BN + 0.6222 La <sub>4</sub> H <sub>9</sub> + LaB <sub>6</sub> H <sub>4</sub> C <sub>6</sub> N             | -9.9400             |
| LaNH <sub>4</sub> B <sub>6</sub> C <sub>6</sub> | LaN + 0.3636 B <sub>9</sub> H <sub>11</sub> + 3 B <sub>13</sub> C <sub>2</sub> + 18.14 LaB <sub>4</sub> → 18.14 LaB <sub>6</sub> + LaB <sub>6</sub> H <sub>4</sub> C <sub>6</sub> N                 | -9.8960             |
| LaNH <sub>4</sub> B <sub>6</sub> C <sub>6</sub> | 1.333 H <sub>3</sub> N + 7.333 LaN + 3 B <sub>13</sub> C <sub>2</sub> → 7.667 BN + 6.333 LaB <sub>4</sub> + LaB <sub>6</sub> H <sub>4</sub> C <sub>6</sub> N                                        | -9.8855             |
| LaNH <sub>4</sub> B <sub>6</sub> C <sub>6</sub> | 6.122 LaN + 0.5714 B <sub>5</sub> H <sub>7</sub> + 3 B <sub>13</sub> C <sub>2</sub> → 5.122 LaB <sub>6</sub> + 5.122 BN + LaB <sub>6</sub> H <sub>4</sub> C <sub>6</sub> N                          | -9.8812             |
| LaNH <sub>4</sub> B <sub>6</sub> C <sub>6</sub> | BN + 0.3636 B <sub>9</sub> H <sub>11</sub> + 3 B <sub>13</sub> C <sub>2</sub> + 21.64 LaB <sub>4</sub> → 20.64 LaB <sub>6</sub> + LaB <sub>6</sub> H <sub>4</sub> C <sub>6</sub> N                  | -9.8668             |
| LaNH <sub>4</sub> B <sub>6</sub> C <sub>6</sub> | 1.333 H <sub>3</sub> N + 5.524 LaN + 3 B <sub>13</sub> C <sub>2</sub> → 4.524 LaB <sub>6</sub> + 5.857 BN + LaB <sub>6</sub> H <sub>4</sub> C <sub>6</sub> N                                        | -9.8327             |
| LaNH <sub>4</sub> B <sub>6</sub> C <sub>6</sub> | 5.067 La + BN + 3 B <sub>13</sub> C <sub>2</sub> + 0.8 La <sub>2</sub> H <sub>5</sub> → 5.667 LaB <sub>6</sub> + LaB <sub>6</sub> H <sub>4</sub> C <sub>6</sub> N                                   | -9.7895             |
| LaNH <sub>4</sub> B <sub>6</sub> C <sub>6</sub> | LaN + 0.5714 B <sub>5</sub> H <sub>7</sub> + 3 B <sub>13</sub> C <sub>2</sub> + 17.93 LaB <sub>4</sub> → 17.93 LaB <sub>6</sub> + LaB <sub>6</sub> H <sub>4</sub> C <sub>6</sub> N                  | -9.7316             |
| LaNH <sub>4</sub> B <sub>6</sub> C <sub>6</sub> | H <sub>3</sub> N + 0.09091 B <sub>9</sub> H <sub>11</sub> + 3 B <sub>13</sub> C <sub>2</sub> + 19.91 LaB <sub>4</sub> → 18.91 LaB <sub>6</sub> + LaB <sub>6</sub> H <sub>4</sub> C <sub>6</sub> N   | -9.7202             |
| LaNH <sub>4</sub> B <sub>6</sub> C <sub>6</sub> | BN + 0.5714 B <sub>5</sub> H <sub>7</sub> + 3 B <sub>13</sub> C <sub>2</sub> + 21.43 LaB <sub>4</sub> → 20.43 LaB <sub>6</sub> + LaB <sub>6</sub> H <sub>4</sub> C <sub>6</sub> N                   | -9.7024             |
| LaNH <sub>4</sub> B <sub>6</sub> C <sub>6</sub> | 33.6 B + 2 La <sub>2</sub> C <sub>3</sub> + 0.5 N <sub>2</sub> + 0.8 La <sub>2</sub> H <sub>5</sub> → 4.6 LaB <sub>6</sub> + LaB <sub>6</sub> H <sub>4</sub> C <sub>6</sub> N                       | -9.6913             |
| LaNH <sub>4</sub> B <sub>6</sub> C <sub>6</sub> | H <sub>3</sub> N + 0.1429 B <sub>5</sub> H <sub>7</sub> + 3 B <sub>13</sub> C <sub>2</sub> + 19.86 LaB <sub>4</sub> → 18.86 LaB <sub>6</sub> + LaB <sub>6</sub> H <sub>4</sub> C <sub>6</sub> N     | -9.6792             |
| LaNH <sub>4</sub> B <sub>6</sub> C <sub>6</sub> | 1.333 H <sub>3</sub> N + 3 B <sub>13</sub> C <sub>2</sub> + 19.33 LaB <sub>4</sub> → 18.33 LaB <sub>6</sub> + 0.3333 BN + LaB <sub>6</sub> H <sub>4</sub> C <sub>6</sub> N                          | -9.6714             |
| LaNH <sub>4</sub> B <sub>6</sub> C <sub>6</sub> | 1.333 H <sub>3</sub> N + 3 B <sub>13</sub> C <sub>2</sub> + 20.5 LaB <sub>4</sub> → 19.17 LaB <sub>6</sub> + 0.3333 LaN + LaB <sub>6</sub> H <sub>4</sub> C <sub>6</sub> N                          | -9.6617             |
| LaNH <sub>4</sub> B <sub>6</sub> C <sub>6</sub> | 4.889 La + BN + 0.4444 La <sub>4</sub> H <sub>9</sub> + 3 B <sub>13</sub> C <sub>2</sub> → 5.667 LaB <sub>6</sub> + LaB <sub>6</sub> H <sub>4</sub> C <sub>6</sub> N                                | -9.6091             |
| LaNH <sub>4</sub> B <sub>6</sub> C <sub>6</sub> | 11.41 H <sub>3</sub> N + LaN + 3 B <sub>13</sub> C <sub>2</sub> → 11.41 BN + 4.318 B <sub>5</sub> H <sub>7</sub> + LaB <sub>6</sub> H <sub>4</sub> C <sub>6</sub> N                                 | -9.4661             |
| LaNH <sub>4</sub> B <sub>6</sub> C <sub>6</sub> | 0.5 H <sub>2</sub> + H <sub>3</sub> N + 3 B <sub>13</sub> C <sub>2</sub> + 19.5 LaB <sub>4</sub> → 18.5 LaB <sub>6</sub> + LaB <sub>6</sub> H <sub>4</sub> C <sub>6</sub> N                         | -9.4389             |
| LaNH <sub>4</sub> B <sub>6</sub> C <sub>6</sub> | 4.667 La + BN + 2 LaH <sub>2</sub> + 3 B <sub>13</sub> C <sub>2</sub> → 5.667 LaB <sub>6</sub> + LaB <sub>6</sub> H <sub>4</sub> C <sub>6</sub> N                                                   | -9.4130             |
| LaNH <sub>4</sub> B <sub>6</sub> C <sub>6</sub> | 1.333 LaH <sub>3</sub> + 4.167 La + LaN + 3 B <sub>13</sub> C <sub>2</sub> → 5.5 LaB <sub>6</sub> + LaB <sub>6</sub> H <sub>4</sub> C <sub>6</sub> N                                                | -9.4075             |
| LaNH <sub>4</sub> B <sub>6</sub> C <sub>6</sub> | 13 H <sub>3</sub> N + 3 B <sub>13</sub> C <sub>2</sub> + LaB <sub>4</sub> → 12 BN + 5 B <sub>5</sub> H <sub>7</sub> + LaB <sub>6</sub> H <sub>4</sub> C <sub>6</sub> N                              | -9.3999             |
| LaNH <sub>4</sub> B <sub>6</sub> C <sub>6</sub> | LaB <sub>6</sub> + 13.64 H <sub>3</sub> N + 3 B <sub>13</sub> C <sub>2</sub> → 12.64 BN + 5.273 B <sub>5</sub> H <sub>7</sub> + LaB <sub>6</sub> H <sub>4</sub> C <sub>6</sub> N                    | -9.3851             |
| LaNH <sub>4</sub> B <sub>6</sub> C <sub>6</sub> | 2 La <sub>2</sub> C <sub>3</sub> + 3.6 B <sub>5</sub> H <sub>7</sub> + 4.033 N <sub>2</sub> → 7.067 H <sub>3</sub> N + 3 LaB <sub>4</sub> + LaB <sub>6</sub> H <sub>4</sub> C <sub>6</sub> N        | -9.1009             |
| LaNH <sub>4</sub> B <sub>6</sub> C <sub>6</sub> | 1.2 H <sub>8</sub> C <sub>5</sub> + 11.12 LaN + 1.791 B <sub>9</sub> H <sub>11</sub> → 10.12 BN + 5.061 La <sub>2</sub> H <sub>5</sub> + LaB <sub>6</sub> H <sub>4</sub> C <sub>6</sub> N           | -9.0550             |
| LaNH <sub>4</sub> B <sub>6</sub> C <sub>6</sub> | 3.9 La + LaN + 3 B <sub>13</sub> C <sub>2</sub> + 0.8 La <sub>2</sub> H <sub>5</sub> → 5.5 LaB <sub>6</sub> + LaB <sub>6</sub> H <sub>4</sub> C <sub>6</sub> N                                      | -9.0428             |
| LaNH <sub>4</sub> B <sub>6</sub> C <sub>6</sub> | 1.333 LaH <sub>3</sub> + 32 B + 2 La <sub>2</sub> C <sub>3</sub> + 0.5 N <sub>2</sub> → 4.333 LaB <sub>6</sub> + LaB <sub>6</sub> H <sub>4</sub> C <sub>6</sub> N                                   | -9.0062             |
| LaNH <sub>4</sub> B <sub>6</sub> C <sub>6</sub> | 1.333 H <sub>3</sub> N + 3 B <sub>13</sub> C <sub>2</sub> + 19.5 LaB <sub>4</sub> → 18.5 LaB <sub>6</sub> + 0.1667 N <sub>2</sub> + LaB <sub>6</sub> H <sub>4</sub> C <sub>6</sub> N                | -8.9976             |
| LaNH <sub>4</sub> B <sub>6</sub> C <sub>6</sub> | 2 H <sub>2</sub> + 7.6 LaN + 3 B <sub>13</sub> C <sub>2</sub> → 6.6 BN + 6.6 LaB <sub>4</sub> + LaB <sub>6</sub> H <sub>4</sub> C <sub>6</sub> N                                                    | -8.9635             |
| LaNH <sub>4</sub> B <sub>6</sub> C <sub>6</sub> | La + 10.79 H <sub>3</sub> N + 3 B <sub>13</sub> C <sub>2</sub> → 9.789 BN + 2.579 B <sub>9</sub> H <sub>11</sub> + LaB <sub>6</sub> H <sub>4</sub> C <sub>6</sub> N                                 | -8.9508             |
| LaNH <sub>4</sub> B <sub>6</sub> C <sub>6</sub> | 2 H <sub>2</sub> + 5.714 LaN + 3 B <sub>13</sub> C <sub>2</sub> → 4.714 LaB <sub>6</sub> + 4.714 BN + LaB <sub>6</sub> H <sub>4</sub> C <sub>6</sub> N                                              | -8.9084             |
| LaNH <sub>4</sub> B <sub>6</sub> C <sub>6</sub> | 0.3333 LaH <sub>3</sub> + H <sub>3</sub> N + 3 B <sub>13</sub> C <sub>2</sub> + 18.5 LaB <sub>4</sub> → 17.83 LaB <sub>6</sub> + LaB <sub>6</sub> H <sub>4</sub> C <sub>6</sub> N                   | -8.9053             |
| LaNH <sub>4</sub> B <sub>6</sub> C <sub>6</sub> | 3.722 La + 0.4444 La <sub>4</sub> H <sub>9</sub> + LaN + 3 B <sub>13</sub> C <sub>2</sub> → 5.5 LaB <sub>6</sub> + LaB <sub>6</sub> H <sub>4</sub> C <sub>6</sub> N                                 | -8.8623             |
| LaNH <sub>4</sub> B <sub>6</sub> C <sub>6</sub> | H <sub>3</sub> N + 3 B <sub>13</sub> C <sub>2</sub> + 0.2 La <sub>2</sub> H <sub>5</sub> + 18.3 LaB <sub>4</sub> → 17.7 LaB <sub>6</sub> + LaB <sub>6</sub> H <sub>4</sub> C <sub>6</sub> N         | -8.8585             |
| LaNH <sub>4</sub> B <sub>6</sub> C <sub>6</sub> | 0.1111 La <sub>4</sub> H <sub>9</sub> + H <sub>3</sub> N + 3 B <sub>13</sub> C <sub>2</sub> + 18.17 LaB <sub>4</sub> → 17.61 LaB <sub>6</sub> + LaB <sub>6</sub> H <sub>4</sub> C <sub>6</sub> N    | -8.8429             |
| LaNH <sub>4</sub> B <sub>6</sub> C <sub>6</sub> | H <sub>3</sub> N + 0.5 LaH <sub>2</sub> + 3 B <sub>13</sub> C <sub>2</sub> + 18 LaB <sub>4</sub> → 17.5 LaB <sub>6</sub> + LaB <sub>6</sub> H <sub>4</sub> C <sub>6</sub> N                         | -8.8309             |
| LaNH <sub>4</sub> B <sub>6</sub> C <sub>6</sub> | 2 H <sub>2</sub> + LaN + 3 B <sub>13</sub> C <sub>2</sub> + 16.5 LaB <sub>4</sub> → 16.5 LaB <sub>6</sub> + LaB <sub>6</sub> H <sub>4</sub> C <sub>6</sub> N                                        | -8.7708             |
| LaNH <sub>4</sub> B <sub>6</sub> C <sub>6</sub> | 2 H <sub>2</sub> + BN + 3 B <sub>13</sub> C <sub>2</sub> + 20 LaB <sub>4</sub> → 19 LaB <sub>6</sub> + LaB <sub>6</sub> H <sub>4</sub> C <sub>6</sub> N                                             | -8.7416             |
| LaNH <sub>4</sub> B <sub>6</sub> C <sub>6</sub> | 3.5 La + LaN + 2 LaH <sub>2</sub> + 3 B <sub>13</sub> C <sub>2</sub> → 5.5 LaB <sub>6</sub> + LaB <sub>6</sub> H <sub>4</sub> C <sub>6</sub> N                                                      | -8.6662             |
| LaNH <sub>4</sub> B <sub>6</sub> C <sub>6</sub> | 3 LaC <sub>2</sub> + 3.6 B <sub>5</sub> H <sub>7</sub> + 4.033 N <sub>2</sub> → 2 LaB <sub>6</sub> + 7.067 H <sub>3</sub> N + LaB <sub>6</sub> H <sub>4</sub> C <sub>6</sub> N                      | -8.6646             |
| LaNH <sub>4</sub> B <sub>6</sub> C <sub>6</sub> | 1.333 LaH <sub>3</sub> + 0.5 N <sub>2</sub> + 3 B <sub>13</sub> C <sub>2</sub> + 15.5 LaB <sub>4</sub> → 15.83 LaB <sub>6</sub> + LaB <sub>6</sub> H <sub>4</sub> C <sub>6</sub> N                  | -8.6286             |
| LaNH <sub>4</sub> B <sub>6</sub> C <sub>6</sub> | 10.04 N <sub>2</sub> + 3 B <sub>13</sub> C <sub>2</sub> + 10.04 La <sub>2</sub> H <sub>5</sub> → 19.08 LaN + 6.6 B <sub>5</sub> H <sub>7</sub> + LaB <sub>6</sub> H <sub>4</sub> C <sub>6</sub> N   | -8.5380             |

Continued on next page

Continued

| Compound                                        | Chemical reaction                                                                                                                                                                       | Reaction energy(eV) |
|-------------------------------------------------|-----------------------------------------------------------------------------------------------------------------------------------------------------------------------------------------|---------------------|
| LaNH <sub>4</sub> B <sub>6</sub> C <sub>6</sub> | $3 \text{LaC}_2 + 36 \text{B} + \text{LaN} + 2 \text{LaH}_2 \rightarrow 5 \text{LaB}_6 + \text{LaB}_6\text{H}_4\text{C}_6\text{N}$                                                      | -8.4610             |
| LaNH <sub>4</sub> B <sub>6</sub> C <sub>6</sub> | $0.5 \text{N}_2 + 3 \text{B}_{13}\text{C}_2 + 0.8 \text{La}_2\text{H}_5 + 14.7 \text{LaB}_4 \rightarrow 15.3 \text{LaB}_6 + \text{LaB}_6\text{H}_4\text{C}_6\text{N}$                   | -8.4412             |
| LaNH <sub>4</sub> B <sub>6</sub> C <sub>6</sub> | $0.4444 \text{La}_4\text{H}_9 + 0.5 \text{N}_2 + 3 \text{B}_{13}\text{C}_2 + 14.17 \text{LaB}_4 \rightarrow 14.94 \text{LaB}_6 + \text{LaB}_6\text{H}_4\text{C}_6\text{N}$              | -8.3790             |
| LaNH <sub>4</sub> B <sub>6</sub> C <sub>6</sub> | $10.5 \text{H}_3\text{N} + \text{LaN} + 3 \text{B}_{13}\text{C}_2 \rightarrow 10.5 \text{BN} + 2.5 \text{B}_9\text{H}_{11} + \text{LaB}_6\text{H}_4\text{C}_6\text{N}$                  | -8.3573             |
| LaNH <sub>4</sub> B <sub>6</sub> C <sub>6</sub> | $2 \text{LaH}_2 + 0.5 \text{N}_2 + 3 \text{B}_{13}\text{C}_2 + 13.5 \text{LaB}_4 \rightarrow 14.5 \text{LaB}_6 + \text{LaB}_6\text{H}_4\text{C}_6\text{N}$                              | -8.3307             |
| LaNH <sub>4</sub> B <sub>6</sub> C <sub>6</sub> | $35 \text{B} + \text{BN} + 2 \text{La}_2\text{C}_3 + 2 \text{LaH}_2 \rightarrow 5 \text{LaB}_6 + \text{LaB}_6\text{H}_4\text{C}_6\text{N}$                                              | -8.3228             |
| LaNH <sub>4</sub> B <sub>6</sub> C <sub>6</sub> | $2 \text{La}_2\text{C}_3 + 1.857 \text{B}_5\text{H}_7 + 2.143 \text{N}_2 \rightarrow 3 \text{LaH}_3 + 3.286 \text{BN} + \text{LaB}_6\text{H}_4\text{C}_6\text{N}$                       | -8.2579             |
| LaNH <sub>4</sub> B <sub>6</sub> C <sub>6</sub> | $1.045 \text{B}_9\text{H}_{11} + 2 \text{La}_2\text{C}_3 + 2.205 \text{N}_2 \rightarrow 3.409 \text{BN} + 1.5 \text{La}_2\text{H}_5 + \text{LaB}_6\text{H}_4\text{C}_6\text{N}$         | -8.1705             |
| LaNH <sub>4</sub> B <sub>6</sub> C <sub>6</sub> | $11.95 \text{H}_3\text{N} + 3 \text{B}_{13}\text{C}_2 + \text{LaB}_4 \rightarrow 10.95 \text{BN} + 2.895 \text{B}_9\text{H}_{11} + \text{LaB}_6\text{H}_4\text{C}_6\text{N}$            | -8.1161             |
| LaNH <sub>4</sub> B <sub>6</sub> C <sub>6</sub> | $2 \text{H}_2 + 30 \text{B} + \text{LaN} + 2 \text{La}_2\text{C}_3 \rightarrow 4 \text{LaB}_6 + \text{LaB}_6\text{H}_4\text{C}_6\text{N}$                                               | -8.0578             |
| LaNH <sub>4</sub> B <sub>6</sub> C <sub>6</sub> | $\text{LaB}_6 + 12.53 \text{H}_3\text{N} + 3 \text{B}_{13}\text{C}_2 \rightarrow 11.53 \text{BN} + 3.053 \text{B}_9\text{H}_{11} + \text{LaB}_6\text{H}_4\text{C}_6\text{N}$            | -8.0312             |
| LaNH <sub>4</sub> B <sub>6</sub> C <sub>6</sub> | $1.2 \text{H}_8\text{C}_5 + 9.5 \text{La} + \text{H}_3\text{N} + 1.2 \text{B}_5\text{H}_7 \rightarrow 8.5 \text{LaH}_2 + \text{LaB}_6\text{H}_4\text{C}_6\text{N}$                      | -7.8702             |
| LaNH <sub>4</sub> B <sub>6</sub> C <sub>6</sub> | $1.2 \text{H}_8\text{C}_5 + 3.98 \text{N}_2 + 3.24 \text{LaB}_4 \rightarrow 6.96 \text{BN} + 1.12 \text{La}_2\text{H}_5 + \text{LaB}_6\text{H}_4\text{C}_6\text{N}$                     | -7.8405             |
| LaNH <sub>4</sub> B <sub>6</sub> C <sub>6</sub> | $2 \text{B}_9\text{H}_{11} + 2 \text{La}_2\text{C}_3 + 3.5 \text{N}_2 \rightarrow 6 \text{H}_3\text{N} + 3 \text{LaB}_4 + \text{LaB}_6\text{H}_4\text{C}_6\text{N}$                     | -7.8238             |
| LaNH <sub>4</sub> B <sub>6</sub> C <sub>6</sub> | $3 \text{LaC}_2 + 34.67 \text{B} + 0.4444 \text{La}_4\text{H}_9 + \text{LaN} \rightarrow 4.778 \text{LaB}_6 + \text{LaB}_6\text{H}_4\text{C}_6\text{N}$                                 | -7.7822             |
| LaNH <sub>4</sub> B <sub>6</sub> C <sub>6</sub> | $1.2 \text{H}_8\text{C}_5 + 9.75 \text{LaN} + 2.95 \text{B}_5\text{H}_7 \rightarrow 8.75 \text{LaH}_3 + 8.75 \text{BN} + \text{LaB}_6\text{H}_4\text{C}_6\text{N}$                      | -7.7515             |
| LaNH <sub>4</sub> B <sub>6</sub> C <sub>6</sub> | $11.27 \text{H}_3\text{N} + \text{LaH}_2 + 3 \text{B}_{13}\text{C}_2 \rightarrow 10.27 \text{BN} + 4.545 \text{B}_5\text{H}_7 + \text{LaB}_6\text{H}_4\text{C}_6\text{N}$               | -7.7435             |
| LaNH <sub>4</sub> B <sub>6</sub> C <sub>6</sub> | $33.67 \text{B} + \text{BN} + 0.4444 \text{La}_4\text{H}_9 + 2 \text{La}_2\text{C}_3 \rightarrow 4.778 \text{LaB}_6 + \text{LaB}_6\text{H}_4\text{C}_6\text{N}$                         | -7.6440             |
| LaNH <sub>4</sub> B <sub>6</sub> C <sub>6</sub> | $0.25 \text{La}_4\text{H}_9 + 11.22 \text{H}_3\text{N} + 3 \text{B}_{13}\text{C}_2 \rightarrow 10.22 \text{BN} + 4.557 \text{B}_5\text{H}_7 + \text{LaB}_6\text{H}_4\text{C}_6\text{N}$ | -7.5599             |
| LaNH <sub>4</sub> B <sub>6</sub> C <sub>6</sub> | $\text{H}_3\text{N} + 54.5 \text{LaH}_2 + 3 \text{B}_{13}\text{C}_2 \rightarrow 5.5 \text{LaB}_6 + 12 \text{La}_4\text{H}_9 + \text{LaB}_6\text{H}_4\text{C}_6\text{N}$                 | -7.5259             |
| LaNH <sub>4</sub> B <sub>6</sub> C <sub>6</sub> | $27.14 \text{B} + \text{LaN} + 2 \text{La}_2\text{C}_3 + 0.5714 \text{B}_5\text{H}_7 \rightarrow 4 \text{LaB}_6 + \text{LaB}_6\text{H}_4\text{C}_6\text{N}$                             | -7.4606             |
| LaNH <sub>4</sub> B <sub>6</sub> C <sub>6</sub> | $26.73 \text{B} + \text{LaN} + 0.3636 \text{B}_9\text{H}_{11} + 2 \text{La}_2\text{C}_3 \rightarrow 4 \text{LaB}_6 + \text{LaB}_6\text{H}_4\text{C}_6\text{N}$                          | -7.3983             |
| LaNH <sub>4</sub> B <sub>6</sub> C <sub>6</sub> | $11.16 \text{H}_3\text{N} + 3 \text{B}_{13}\text{C}_2 + 0.5 \text{La}_2\text{H}_5 \rightarrow 10.16 \text{BN} + 4.568 \text{B}_5\text{H}_7 + \text{LaB}_6\text{H}_4\text{C}_6\text{N}$  | -7.3910             |
| LaNH <sub>4</sub> B <sub>6</sub> C <sub>6</sub> | $3 \text{LaC}_2 + 2 \text{B}_9\text{H}_{11} + 3.5 \text{N}_2 \rightarrow 2 \text{LaB}_6 + 6 \text{H}_3\text{N} + \text{LaB}_6\text{H}_4\text{C}_6\text{N}$                              | -7.3875             |
| LaNH <sub>4</sub> B <sub>6</sub> C <sub>6</sub> | $42.5 \text{LaH}_2 + 0.5 \text{N}_2 + 3 \text{B}_{13}\text{C}_2 \rightarrow 5.5 \text{LaB}_6 + 9 \text{La}_4\text{H}_9 + \text{LaB}_6\text{H}_4\text{C}_6\text{N}$                      | -7.3519             |
| LaNH <sub>4</sub> B <sub>6</sub> C <sub>6</sub> | $0.125 \text{H}_8\text{C}_5 + \text{H}_3\text{N} + 2.687 \text{B}_{13}\text{C}_2 + 17.47 \text{LaB}_4 \rightarrow 16.47 \text{LaB}_6 + \text{LaB}_6\text{H}_4\text{C}_6\text{N}$        | -7.3304             |
| LaNH <sub>4</sub> B <sub>6</sub> C <sub>6</sub> | $3 \text{LaC}_2 + 33.6 \text{B} + \text{LaN} + 0.8 \text{La}_2\text{H}_5 \rightarrow 4.6 \text{LaB}_6 + \text{LaB}_6\text{H}_4\text{C}_6\text{N}$                                       | -7.2627             |
| LaNH <sub>4</sub> B <sub>6</sub> C <sub>6</sub> | $6.5 \text{LaH}_3 + 3.083 \text{N}_2 + 3 \text{B}_{13}\text{C}_2 \rightarrow 5.5 \text{LaB}_6 + 5.167 \text{H}_3\text{N} + \text{LaB}_6\text{H}_4\text{C}_6\text{N}$                    | -7.1987             |
| LaNH <sub>4</sub> B <sub>6</sub> C <sub>6</sub> | $3 \text{LaC}_2 + 30 \text{B} + 2 \text{LaH}_2 + 0.5 \text{N}_2 \rightarrow 4 \text{LaB}_6 + \text{LaB}_6\text{H}_4\text{C}_6\text{N}$                                                  | -7.1814             |
| LaNH <sub>4</sub> B <sub>6</sub> C <sub>6</sub> | $\text{H}_3\text{N} + 30.5 \text{LaH}_2 + 3 \text{B}_{13}\text{C}_2 \rightarrow 5.5 \text{LaB}_6 + 12 \text{La}_2\text{H}_5 + \text{LaB}_6\text{H}_4\text{C}_6\text{N}$                 | -7.1731             |
| LaNH <sub>4</sub> B <sub>6</sub> C <sub>6</sub> | $32.6 \text{B} + \text{BN} + 2 \text{La}_2\text{C}_3 + 0.8 \text{La}_2\text{H}_5 \rightarrow 4.6 \text{LaB}_6 + \text{LaB}_6\text{H}_4\text{C}_6\text{N}$                               | -7.1245             |
| LaNH <sub>4</sub> B <sub>6</sub> C <sub>6</sub> | $\text{LaH}_3 + 11.05 \text{H}_3\text{N} + 3 \text{B}_{13}\text{C}_2 \rightarrow 10.05 \text{BN} + 4.591 \text{B}_5\text{H}_7 + \text{LaB}_6\text{H}_4\text{C}_6\text{N}$               | -7.1239             |
| LaNH <sub>4</sub> B <sub>6</sub> C <sub>6</sub> | $24.5 \text{LaH}_2 + 0.5 \text{N}_2 + 3 \text{B}_{13}\text{C}_2 \rightarrow 5.5 \text{LaB}_6 + 9 \text{La}_2\text{H}_5 + \text{LaB}_6\text{H}_4\text{C}_6\text{N}$                      | -7.0873             |
| LaNH <sub>4</sub> B <sub>6</sub> C <sub>6</sub> | $1.2 \text{H}_8\text{C}_5 + 8.556 \text{La} + \text{H}_3\text{N} + 1.2 \text{B}_5\text{H}_7 \rightarrow 1.889 \text{La}_4\text{H}_9 + \text{LaB}_6\text{H}_4\text{C}_6\text{N}$         | -7.0367             |
| LaNH <sub>4</sub> B <sub>6</sub> C <sub>6</sub> | $8.867 \text{N}_2 + 3 \text{B}_{13}\text{C}_2 + 8.867 \text{La}_2\text{H}_5 \rightarrow 16.73 \text{LaN} + 3.667 \text{B}_9\text{H}_{11} + \text{LaB}_6\text{H}_4\text{C}_6\text{N}$    | -7.0203             |
| LaNH <sub>4</sub> B <sub>6</sub> C <sub>6</sub> | $\text{H}_3\text{N} + 79.25 \text{LaH}_2 + 3 \text{B}_{13}\text{C}_2 \rightarrow 17.5 \text{La}_4\text{H}_9 + 8.25 \text{LaB}_4 + \text{LaB}_6\text{H}_4\text{C}_6\text{N}$             | -6.9277             |
| LaNH <sub>4</sub> B <sub>6</sub> C <sub>6</sub> | $1.2 \text{H}_8\text{C}_5 + 8.967 \text{La} + \text{H}_3\text{N} + 0.6667 \text{B}_9\text{H}_{11} \rightarrow 7.967 \text{LaH}_2 + \text{LaB}_6\text{H}_4\text{C}_6\text{N}$            | -6.9120             |
| LaNH <sub>4</sub> B <sub>6</sub> C <sub>6</sub> | $6.5 \text{LaH}_2 + 2 \text{N}_2 + 3 \text{B}_{13}\text{C}_2 \rightarrow 5.5 \text{LaB}_6 + 3 \text{H}_3\text{N} + \text{LaB}_6\text{H}_4\text{C}_6\text{N}$                            | -6.8300             |
| LaNH <sub>4</sub> B <sub>6</sub> C <sub>6</sub> | $1.333 \text{LaH}_3 + 6.533 \text{LaN} + 3 \text{B}_{13}\text{C}_2 \rightarrow 5.533 \text{BN} + 6.867 \text{LaB}_4 + \text{LaB}_6\text{H}_4\text{C}_6\text{N}$                         | -6.7979             |
| LaNH <sub>4</sub> B <sub>6</sub> C <sub>6</sub> | $2.917 \text{La}_2\text{C}_3 + 1.2 \text{B}_5\text{H}_7 + 2.917 \text{N}_2 \rightarrow 0.55 \text{H}_8\text{C}_5 + 4.833 \text{LaN} + \text{LaB}_6\text{H}_4\text{C}_6\text{N}$         | -6.7907             |
| LaNH <sub>4</sub> B <sub>6</sub> C <sub>6</sub> | $2 \text{H}_2 + 24 \text{B} + 2 \text{La}_2\text{C}_3 + 0.5 \text{N}_2 \rightarrow 3 \text{LaB}_6 + \text{LaB}_6\text{H}_4\text{C}_6\text{N}$                                           | -6.7782             |
| LaNH <sub>4</sub> B <sub>6</sub> C <sub>6</sub> | $67.25 \text{LaH}_2 + 0.5 \text{N}_2 + 3 \text{B}_{13}\text{C}_2 \rightarrow 14.5 \text{La}_4\text{H}_9 + 8.25 \text{LaB}_4 + \text{LaB}_6\text{H}_4\text{C}_6\text{N}$                 | -6.7538             |
| LaNH <sub>4</sub> B <sub>6</sub> C <sub>6</sub> | $1.333 \text{LaH}_3 + 4.571 \text{LaN} + 3 \text{B}_{13}\text{C}_2 \rightarrow 4.905 \text{LaB}_6 + 3.571 \text{BN} + \text{LaB}_6\text{H}_4\text{C}_6\text{N}$                         | -6.7406             |
| LaNH <sub>4</sub> B <sub>6</sub> C <sub>6</sub> | $2.542 \text{N}_2 + 3 \text{B}_{13}\text{C}_2 + 3.25 \text{La}_2\text{H}_5 \rightarrow 5.5 \text{LaB}_6 + 4.083 \text{H}_3\text{N} + \text{LaB}_6\text{H}_4\text{C}_6\text{N}$          | -6.7372             |
| LaNH <sub>4</sub> B <sub>6</sub> C <sub>6</sub> | $1.625 \text{La}_4\text{H}_9 + 2.271 \text{N}_2 + 3 \text{B}_{13}\text{C}_2 \rightarrow 5.5 \text{LaB}_6 + 3.542 \text{H}_3\text{N} + \text{LaB}_6\text{H}_4\text{C}_6\text{N}$         | -6.7358             |
| LaNH <sub>4</sub> B <sub>6</sub> C <sub>6</sub> | $12.25 \text{La}_4\text{H}_9 + 0.5 \text{N}_2 + 3 \text{B}_{13}\text{C}_2 \rightarrow 5.5 \text{LaB}_6 + 21.25 \text{La}_2\text{H}_5 + \text{LaB}_6\text{H}_4\text{C}_6\text{N}$        | -6.7272             |
| LaNH <sub>4</sub> B <sub>6</sub> C <sub>6</sub> | $15.25 \text{La}_4\text{H}_9 + \text{H}_3\text{N} + 3 \text{B}_{13}\text{C}_2 \rightarrow 5.5 \text{LaB}_6 + 27.25 \text{La}_2\text{H}_5 + \text{LaB}_6\text{H}_4\text{C}_6\text{N}$    | -6.7247             |
| LaNH <sub>4</sub> B <sub>6</sub> C <sub>6</sub> | $7.444 \text{H}_3\text{N} + 2 \text{La}_2\text{C}_3 + 3.111 \text{LaB}_4 \rightarrow 6.111 \text{LaH}_3 + 6.444 \text{BN} + \text{LaB}_6\text{H}_4\text{C}_6\text{N}$                   | -6.6437             |
| LaNH <sub>4</sub> B <sub>6</sub> C <sub>6</sub> | $1.333 \text{LaH}_3 + \text{LaN} + 3 \text{B}_{13}\text{C}_2 + 12.5 \text{LaB}_4 \rightarrow 13.83 \text{LaB}_6 + \text{LaB}_6\text{H}_4\text{C}_6\text{N}$                             | -6.6363             |
| LaNH <sub>4</sub> B <sub>6</sub> C <sub>6</sub> | $1.333 \text{LaH}_3 + \text{BN} + 3 \text{B}_{13}\text{C}_2 + 16 \text{LaB}_4 \rightarrow 16.33 \text{LaB}_6 + \text{LaB}_6\text{H}_4\text{C}_6\text{N}$                                | -6.6071             |
| LaNH <sub>4</sub> B <sub>6</sub> C <sub>6</sub> | $6.32 \text{LaN} + 3 \text{B}_{13}\text{C}_2 + 0.8 \text{La}_2\text{H}_5 \rightarrow 5.32 \text{BN} + 6.92 \text{LaB}_4 + \text{LaB}_6\text{H}_4\text{C}_6\text{N}$                     | -6.6043             |
| LaNH <sub>4</sub> B <sub>6</sub> C <sub>6</sub> | $3 \text{LaC}_2 + 1.333 \text{LaH}_3 + 32 \text{B} + \text{LaN} \rightarrow 4.333 \text{LaB}_6 + \text{LaB}_6\text{H}_4\text{C}_6\text{N}$                                              | -6.5777             |
| LaNH <sub>4</sub> B <sub>6</sub> C <sub>6</sub> | $10.32 \text{H}_3\text{N} + \text{LaH}_2 + 3 \text{B}_{13}\text{C}_2 \rightarrow 9.316 \text{BN} + 2.632 \text{B}_9\text{H}_{11} + \text{LaB}_6\text{H}_4\text{C}_6\text{N}$            | -6.5764             |
| LaNH <sub>4</sub> B <sub>6</sub> C <sub>6</sub> | $4.343 \text{LaN} + 3 \text{B}_{13}\text{C}_2 + 0.8 \text{La}_2\text{H}_5 \rightarrow 4.943 \text{LaB}_6 + 3.343 \text{BN} + \text{LaB}_6\text{H}_4\text{C}_6\text{N}$                  | -6.5465             |
| LaNH <sub>4</sub> B <sub>6</sub> C <sub>6</sub> | $0.4444 \text{La}_4\text{H}_9 + 6.178 \text{LaN} + 3 \text{B}_{13}\text{C}_2 \rightarrow 5.178 \text{BN} + 6.956 \text{LaB}_4 + \text{LaB}_6\text{H}_4\text{C}_6\text{N}$               | -6.5379             |
| LaNH <sub>4</sub> B <sub>6</sub> C <sub>6</sub> | $3 \text{LaC}_2 + 28.67 \text{B} + 0.4444 \text{La}_4\text{H}_9 + 0.5 \text{N}_2 \rightarrow 3.778 \text{LaB}_6 + \text{LaB}_6\text{H}_4\text{C}_6\text{N}$                             | -6.5026             |
| LaNH <sub>4</sub> B <sub>6</sub> C <sub>6</sub> | $6 \text{LaN} + 2 \text{LaH}_2 + 3 \text{B}_{13}\text{C}_2 \rightarrow 5 \text{BN} + 7 \text{LaB}_4 + \text{LaB}_6\text{H}_4\text{C}_6\text{N}$                                         | -6.4844             |
| LaNH <sub>4</sub> B <sub>6</sub> C <sub>6</sub> | $27 \text{B} + \text{H}_3\text{N} + 2 \text{La}_2\text{C}_3 + 0.5 \text{LaH}_2 \rightarrow 3.5 \text{LaB}_6 + \text{LaB}_6\text{H}_4\text{C}_6\text{N}$                                 | -6.4819             |
| LaNH <sub>4</sub> B <sub>6</sub> C <sub>6</sub> | $0.4444 \text{La}_4\text{H}_9 + 4.19 \text{LaN} + 3 \text{B}_{13}\text{C}_2 \rightarrow 4.968 \text{LaB}_6 + 3.19 \text{BN} + \text{LaB}_6\text{H}_4\text{C}_6\text{N}$                 | -6.4799             |
| LaNH <sub>4</sub> B <sub>6</sub> C <sub>6</sub> | $\text{LaN} + 3 \text{B}_{13}\text{C}_2 + 0.8 \text{La}_2\text{H}_5 + 11.7 \text{LaB}_4 \rightarrow 13.3 \text{LaB}_6 + \text{LaB}_6\text{H}_4\text{C}_6\text{N}$                       | -6.4489             |

Continued on next page

Continued

| Compound                                        | Chemical reaction                                                                                                                                                                                              | Reaction energy(eV) |
|-------------------------------------------------|----------------------------------------------------------------------------------------------------------------------------------------------------------------------------------------------------------------|---------------------|
| LaNH <sub>4</sub> B <sub>6</sub> C <sub>6</sub> | 1.333 LaH <sub>3</sub> + 31 B + BN + 2 La <sub>2</sub> C <sub>3</sub> → 4.333 LaB <sub>6</sub> + LaB <sub>6</sub> H <sub>4</sub> C <sub>6</sub> N                                                              | -6.4394             |
| LaNH <sub>4</sub> B <sub>6</sub> C <sub>6</sub> | 9.25 LaH <sub>3</sub> + 4.458 N <sub>2</sub> + 3 B <sub>13</sub> C <sub>2</sub> → 7.917 H <sub>3</sub> N + 8.25 LaB <sub>4</sub> + LaB <sub>6</sub> H <sub>4</sub> C <sub>6</sub> N                            | -6.4376             |
| LaNH <sub>4</sub> B <sub>6</sub> C <sub>6</sub> | 4 LaN + 2 LaH <sub>2</sub> + 3 B <sub>13</sub> C <sub>2</sub> → 5 LaB <sub>6</sub> + 3 BN + LaB <sub>6</sub> H <sub>4</sub> C <sub>6</sub> N                                                                   | -6.4260             |
| LaNH <sub>4</sub> B <sub>6</sub> C <sub>6</sub> | BN + 3 B <sub>13</sub> C <sub>2</sub> + 0.8 La <sub>2</sub> H <sub>5</sub> + 15.2 LaB <sub>4</sub> → 15.8 LaB <sub>6</sub> + LaB <sub>6</sub> H <sub>4</sub> C <sub>6</sub> N                                  | -6.4197             |
| LaNH <sub>4</sub> B <sub>6</sub> C <sub>6</sub> | H <sub>3</sub> N + 44.25 LaH <sub>2</sub> + 3 B <sub>13</sub> C <sub>2</sub> → 17.5 La <sub>2</sub> H <sub>5</sub> + 8.25 LaB <sub>4</sub> + LaB <sub>6</sub> H <sub>4</sub> C <sub>6</sub> N                  | -6.4132             |
| LaNH <sub>4</sub> B <sub>6</sub> C <sub>6</sub> | 0.25 La <sub>4</sub> H <sub>9</sub> + 10.26 H <sub>3</sub> N + 3 B <sub>13</sub> C <sub>2</sub> → 9.257 BN + 2.638 B <sub>9</sub> H <sub>11</sub> + LaB <sub>6</sub> H <sub>4</sub> C <sub>6</sub> N           | -6.3899             |
| LaNH <sub>4</sub> B <sub>6</sub> C <sub>6</sub> | 0.9773 B <sub>9</sub> H <sub>11</sub> + 2 La <sub>2</sub> C <sub>3</sub> + 1.898 N <sub>2</sub> → 2.795 BN + 0.75 La <sub>4</sub> H <sub>9</sub> + LaB <sub>6</sub> H <sub>4</sub> C <sub>6</sub> N            | -6.3887             |
| LaNH <sub>4</sub> B <sub>6</sub> C <sub>6</sub> | 0.4444 La <sub>4</sub> H <sub>9</sub> + LaN + 3 B <sub>13</sub> C <sub>2</sub> + 11.17 LaB <sub>4</sub> → 12.94 LaB <sub>6</sub> + LaB <sub>6</sub> H <sub>4</sub> C <sub>6</sub> N                            | -6.3867             |
| LaNH <sub>4</sub> B <sub>6</sub> C <sub>6</sub> | 1.2 H <sub>8</sub> C <sub>5</sub> + 8 La + 1.2 B <sub>5</sub> H <sub>7</sub> + 0.5 N <sub>2</sub> → 7 LaH <sub>2</sub> + LaB <sub>6</sub> H <sub>4</sub> C <sub>6</sub> N                                      | -6.3724             |
| LaNH <sub>4</sub> B <sub>6</sub> C <sub>6</sub> | BN + 0.4444 La <sub>4</sub> H <sub>9</sub> + 3 B <sub>13</sub> C <sub>2</sub> + 14.67 LaB <sub>4</sub> → 15.44 LaB <sub>6</sub> + LaB <sub>6</sub> H <sub>4</sub> C <sub>6</sub> N                             | -6.3575             |
| LaNH <sub>4</sub> B <sub>6</sub> C <sub>6</sub> | LaN + 2 LaH <sub>2</sub> + 3 B <sub>13</sub> C <sub>2</sub> + 10.5 LaB <sub>4</sub> → 12.5 LaB <sub>6</sub> + LaB <sub>6</sub> H <sub>4</sub> C <sub>6</sub> N                                                 | -6.3384             |
| LaNH <sub>4</sub> B <sub>6</sub> C <sub>6</sub> | 38.25 LaH <sub>2</sub> + 0.5 N <sub>2</sub> + 3 B <sub>13</sub> C <sub>2</sub> → 14.5 La <sub>2</sub> H <sub>5</sub> + 8.25 LaB <sub>4</sub> + LaB <sub>6</sub> H <sub>4</sub> C <sub>6</sub> N                | -6.3275             |
| LaNH <sub>4</sub> B <sub>6</sub> C <sub>6</sub> | 15.5 LaH <sub>2</sub> + 0.5 N <sub>2</sub> + 3 B <sub>13</sub> C <sub>2</sub> → 9 LaH <sub>3</sub> + 5.5 LaB <sub>6</sub> + LaB <sub>6</sub> H <sub>4</sub> C <sub>6</sub> N                                   | -6.3196             |
| LaNH <sub>4</sub> B <sub>6</sub> C <sub>6</sub> | 26.67 B + 0.1111 La <sub>4</sub> H <sub>9</sub> + H <sub>3</sub> N + 2 La <sub>2</sub> C <sub>3</sub> → 3.444 LaB <sub>6</sub> + LaB <sub>6</sub> H <sub>4</sub> C <sub>6</sub> N                              | -6.3122             |
| LaNH <sub>4</sub> B <sub>6</sub> C <sub>6</sub> | BN + 2 LaH <sub>2</sub> + 3 B <sub>13</sub> C <sub>2</sub> + 14 LaB <sub>4</sub> → 15 LaB <sub>6</sub> + LaB <sub>6</sub> H <sub>4</sub> C <sub>6</sub> N                                                      | -6.3092             |
| LaNH <sub>4</sub> B <sub>6</sub> C <sub>6</sub> | 1.2 H <sub>8</sub> C <sub>5</sub> + 7.8 La + H <sub>3</sub> N + 1.2 B <sub>5</sub> H <sub>7</sub> → 3.4 La <sub>2</sub> H <sub>5</sub> + LaB <sub>6</sub> H <sub>4</sub> C <sub>6</sub> N                      | -6.2699             |
| LaNH <sub>4</sub> B <sub>6</sub> C <sub>6</sub> | 10.2 H <sub>3</sub> N + 3 B <sub>13</sub> C <sub>2</sub> + 0.5 La <sub>2</sub> H <sub>5</sub> → 9.197 BN + 2.645 B <sub>9</sub> H <sub>11</sub> + LaB <sub>6</sub> H <sub>4</sub> C <sub>6</sub> N             | -6.2181             |
| LaNH <sub>4</sub> B <sub>6</sub> C <sub>6</sub> | 26.4 B + H <sub>3</sub> N + 2 La <sub>2</sub> C <sub>3</sub> + 0.2 La <sub>2</sub> H <sub>5</sub> → 3.4 LaB <sub>6</sub> + LaB <sub>6</sub> H <sub>4</sub> C <sub>6</sub> N                                    | -6.1824             |
| LaNH <sub>4</sub> B <sub>6</sub> C <sub>6</sub> | 21.14 B + 2 La <sub>2</sub> C <sub>3</sub> + 0.5714 B <sub>5</sub> H <sub>7</sub> + 0.5 N <sub>2</sub> → 3 LaB <sub>6</sub> + LaB <sub>6</sub> H <sub>4</sub> C <sub>6</sub> N                                 | -6.1810             |
| LaNH <sub>4</sub> B <sub>6</sub> C <sub>6</sub> | H <sub>3</sub> N + 18.5 LaH <sub>2</sub> + 3 B <sub>13</sub> C <sub>2</sub> → 12 LaH <sub>3</sub> + 5.5 LaB <sub>6</sub> + LaB <sub>6</sub> H <sub>4</sub> C <sub>6</sub> N                                    | -6.1495             |
| LaNH <sub>4</sub> B <sub>6</sub> C <sub>6</sub> | 1.2 H <sub>8</sub> C <sub>5</sub> + 8.081 La + H <sub>3</sub> N + 0.6667 B <sub>9</sub> H <sub>11</sub> → 1.77 La <sub>4</sub> H <sub>9</sub> + LaB <sub>6</sub> H <sub>4</sub> C <sub>6</sub> N               | -6.1307             |
| LaNH <sub>4</sub> B <sub>6</sub> C <sub>6</sub> | 20.73 B + 0.3636 B <sub>9</sub> H <sub>11</sub> + 2 La <sub>2</sub> C <sub>3</sub> + 0.5 N <sub>2</sub> → 3 LaB <sub>6</sub> + LaB <sub>6</sub> H <sub>4</sub> C <sub>6</sub> N                                | -6.1187             |
| LaNH <sub>4</sub> B <sub>6</sub> C <sub>6</sub> | 0.3333 LaH <sub>3</sub> + 26 B + H <sub>3</sub> N + 2 La <sub>2</sub> C <sub>3</sub> → 3.333 LaB <sub>6</sub> + LaB <sub>6</sub> H <sub>4</sub> C <sub>6</sub> N                                               | -6.0111             |
| LaNH <sub>4</sub> B <sub>6</sub> C <sub>6</sub> | 3 LaC <sub>2</sub> + 27.6 B + 0.5 N <sub>2</sub> + 0.8 La <sub>2</sub> H <sub>5</sub> → 3.6 LaB <sub>6</sub> + LaB <sub>6</sub> H <sub>4</sub> C <sub>6</sub> N                                                | -5.9831             |
| LaNH <sub>4</sub> B <sub>6</sub> C <sub>6</sub> | LaH <sub>3</sub> + 10.08 H <sub>3</sub> N + 3 B <sub>13</sub> C <sub>2</sub> → 9.079 BN + 2.658 B <sub>9</sub> H <sub>11</sub> + LaB <sub>6</sub> H <sub>4</sub> C <sub>6</sub> N                              | -5.9451             |
| LaNH <sub>4</sub> B <sub>6</sub> C <sub>6</sub> | 9.25 LaH <sub>2</sub> + 2.917 N <sub>2</sub> + 3 B <sub>13</sub> C <sub>2</sub> → 4.833 H <sub>3</sub> N + 8.25 LaB <sub>4</sub> + LaB <sub>6</sub> H <sub>4</sub> C <sub>6</sub> N                            | -5.9130             |
| LaNH <sub>4</sub> B <sub>6</sub> C <sub>6</sub> | 24.33 B + 1.333 H <sub>3</sub> N + 2 La <sub>2</sub> C <sub>3</sub> → 3 LaB <sub>6</sub> + 0.3333 BN + LaB <sub>6</sub> H <sub>4</sub> C <sub>6</sub> N                                                        | -5.8683             |
| LaNH <sub>4</sub> B <sub>6</sub> C <sub>6</sub> | 3.687 N <sub>2</sub> + 3 B <sub>13</sub> C <sub>2</sub> + 4.625 La <sub>2</sub> H <sub>5</sub> → 6.375 H <sub>3</sub> N + 8.25 LaB <sub>4</sub> + LaB <sub>6</sub> H <sub>4</sub> C <sub>6</sub> N             | -5.7808             |
| LaNH <sub>4</sub> B <sub>6</sub> C <sub>6</sub> | 2.312 La <sub>4</sub> H <sub>9</sub> + 3.302 N <sub>2</sub> + 3 B <sub>13</sub> C <sub>2</sub> → 5.604 H <sub>3</sub> N + 8.25 LaB <sub>4</sub> + LaB <sub>6</sub> H <sub>4</sub> C <sub>6</sub> N             | -5.7789             |
| LaNH <sub>4</sub> B <sub>6</sub> C <sub>6</sub> | 0.5 H <sub>8</sub> C <sub>5</sub> + 5.187 La + 0.5 N <sub>2</sub> + 1.75 B <sub>13</sub> C <sub>2</sub> → 4.187 LaB <sub>4</sub> + LaB <sub>6</sub> H <sub>4</sub> C <sub>6</sub> N                            | -5.7788             |
| LaNH <sub>4</sub> B <sub>6</sub> C <sub>6</sub> | 19.12 La <sub>4</sub> H <sub>9</sub> + 0.5 N <sub>2</sub> + 3 B <sub>13</sub> C <sub>2</sub> → 33.62 La <sub>2</sub> H <sub>5</sub> + 8.25 LaB <sub>4</sub> + LaB <sub>6</sub> H <sub>4</sub> C <sub>6</sub> N | -5.7652             |
| LaNH <sub>4</sub> B <sub>6</sub> C <sub>6</sub> | 22.13 La <sub>4</sub> H <sub>9</sub> + H <sub>3</sub> N + 3 B <sub>13</sub> C <sub>2</sub> → 39.63 La <sub>2</sub> H <sub>5</sub> + 8.25 LaB <sub>4</sub> + LaB <sub>6</sub> H <sub>4</sub> C <sub>6</sub> N   | -5.7627             |
| LaNH <sub>4</sub> B <sub>6</sub> C <sub>6</sub> | 5.167 La <sub>4</sub> H <sub>9</sub> + 0.5 N <sub>2</sub> + 3 B <sub>13</sub> C <sub>2</sub> → 14.17 LaH <sub>3</sub> + 5.5 LaB <sub>6</sub> + LaB <sub>6</sub> H <sub>4</sub> C <sub>6</sub> N                | -5.7270             |
| LaNH <sub>4</sub> B <sub>6</sub> C <sub>6</sub> | 1.2 H <sub>8</sub> C <sub>5</sub> + 7.222 La + 1.2 B <sub>5</sub> H <sub>7</sub> + 0.5 N <sub>2</sub> → 1.556 La <sub>4</sub> H <sub>9</sub> + LaB <sub>6</sub> H <sub>4</sub> C <sub>6</sub> N                | -5.6860             |
| LaNH <sub>4</sub> B <sub>6</sub> C <sub>6</sub> | 30 B + LaN + 2 La <sub>2</sub> C <sub>3</sub> + 2 LaH <sub>2</sub> → 6 LaB <sub>4</sub> + LaB <sub>6</sub> H <sub>4</sub> C <sub>6</sub> N                                                                     | -5.6254             |
| LaNH <sub>4</sub> B <sub>6</sub> C <sub>6</sub> | 0.6667 B <sub>9</sub> H <sub>11</sub> + 2.694 La <sub>2</sub> C <sub>3</sub> + 2.694 N <sub>2</sub> → 0.4167 H <sub>8</sub> C <sub>5</sub> + 4.389 LaN + LaB <sub>6</sub> H <sub>4</sub> C <sub>6</sub> N      | -5.5981             |
| LaNH <sub>4</sub> B <sub>6</sub> C <sub>6</sub> | LaN + 33.5 LaH <sub>2</sub> + 3 B <sub>13</sub> C <sub>2</sub> → 5.5 LaB <sub>6</sub> + 7 La <sub>4</sub> H <sub>9</sub> + LaB <sub>6</sub> H <sub>4</sub> C <sub>6</sub> N                                    | -5.5771             |
| LaNH <sub>4</sub> B <sub>6</sub> C <sub>6</sub> | 0.5 H <sub>2</sub> + 24 B + H <sub>3</sub> N + 2 La <sub>2</sub> C <sub>3</sub> → 3 LaB <sub>6</sub> + LaB <sub>6</sub> H <sub>4</sub> C <sub>6</sub> N                                                        | -5.4541             |
| LaNH <sub>4</sub> B <sub>6</sub> C <sub>6</sub> | 6.167 La <sub>4</sub> H <sub>9</sub> + H <sub>3</sub> N + 3 B <sub>13</sub> C <sub>2</sub> → 18.17 LaH <sub>3</sub> + 5.5 LaB <sub>6</sub> + LaB <sub>6</sub> H <sub>4</sub> C <sub>6</sub> N                  | -5.4421             |
| LaNH <sub>4</sub> B <sub>6</sub> C <sub>6</sub> | 26 B + 2 La <sub>2</sub> C <sub>3</sub> + 2 LaH <sub>2</sub> + 0.5 N <sub>2</sub> → 5 LaB <sub>4</sub> + LaB <sub>6</sub> H <sub>4</sub> C <sub>6</sub> N                                                      | -5.4364             |
| LaNH <sub>4</sub> B <sub>6</sub> C <sub>6</sub> | 1.2 H <sub>8</sub> C <sub>5</sub> + 7.467 La + 0.6667 B <sub>9</sub> H <sub>11</sub> + 0.5 N <sub>2</sub> → 6.467 LaH <sub>2</sub> + LaB <sub>6</sub> H <sub>4</sub> C <sub>6</sub> N                          | -5.4141             |
| LaNH <sub>4</sub> B <sub>6</sub> C <sub>6</sub> | 1.2 H <sub>8</sub> C <sub>5</sub> + 7.373 La + H <sub>3</sub> N + 0.6667 B <sub>9</sub> H <sub>11</sub> → 3.187 La <sub>2</sub> H <sub>5</sub> + LaB <sub>6</sub> H <sub>4</sub> C <sub>6</sub> N              | -5.4120             |
| LaNH <sub>4</sub> B <sub>6</sub> C <sub>6</sub> | LaN + 19.5 LaH <sub>2</sub> + 3 B <sub>13</sub> C <sub>2</sub> → 5.5 LaB <sub>6</sub> + 7 La <sub>2</sub> H <sub>5</sub> + LaB <sub>6</sub> H <sub>4</sub> C <sub>6</sub> N                                    | -5.3714             |
| LaNH <sub>4</sub> B <sub>6</sub> C <sub>6</sub> | 23.29 B + H <sub>3</sub> N + 2 La <sub>2</sub> C <sub>3</sub> + 0.1429 B <sub>5</sub> H <sub>7</sub> → 3 LaB <sub>6</sub> + LaB <sub>6</sub> H <sub>4</sub> C <sub>6</sub> N                                   | -5.3048             |
| LaNH <sub>4</sub> B <sub>6</sub> C <sub>6</sub> | 3 LaC <sub>2</sub> + 1.333 LaH <sub>3</sub> + 26 B + 0.5 N <sub>2</sub> → 3.333 LaB <sub>6</sub> + LaB <sub>6</sub> H <sub>4</sub> C <sub>6</sub> N                                                            | -5.2980             |
| LaNH <sub>4</sub> B <sub>6</sub> C <sub>6</sub> | BN + 44 LaH <sub>2</sub> + 3 B <sub>13</sub> C <sub>2</sub> → 5.667 LaB <sub>6</sub> + 9.333 La <sub>4</sub> H <sub>9</sub> + LaB <sub>6</sub> H <sub>4</sub> C <sub>6</sub> N                                 | -5.2942             |
| LaNH <sub>4</sub> B <sub>6</sub> C <sub>6</sub> | 23.18 B + H <sub>3</sub> N + 0.09091 B <sub>9</sub> H <sub>11</sub> + 2 La <sub>2</sub> C <sub>3</sub> → 3 LaB <sub>6</sub> + LaB <sub>6</sub> H <sub>4</sub> C <sub>6</sub> N                                 | -5.2892             |
| LaNH <sub>4</sub> B <sub>6</sub> C <sub>6</sub> | 2 La <sub>2</sub> C <sub>3</sub> + 1.643 B <sub>5</sub> H <sub>7</sub> + 1.607 N <sub>2</sub> → 2.214 BN + 1.5 La <sub>2</sub> H <sub>5</sub> + LaB <sub>6</sub> H <sub>4</sub> C <sub>6</sub> N               | -5.2827             |
| LaNH <sub>4</sub> B <sub>6</sub> C <sub>6</sub> | 8.625 H <sub>3</sub> N + 0.5 La <sub>2</sub> C <sub>3</sub> + 2.25 B <sub>13</sub> C <sub>2</sub> → 7.625 BN + 3.125 B <sub>5</sub> H <sub>7</sub> + LaB <sub>6</sub> H <sub>4</sub> C <sub>6</sub> N          | -5.2336             |
| LaNH <sub>4</sub> B <sub>6</sub> C <sub>6</sub> | 29.11 B + 0.4444 La <sub>4</sub> H <sub>9</sub> + LaN + 2 La <sub>2</sub> C <sub>3</sub> → 5.778 LaB <sub>4</sub> + LaB <sub>6</sub> H <sub>4</sub> C <sub>6</sub> N                                           | -5.1890             |
| LaNH <sub>4</sub> B <sub>6</sub> C <sub>6</sub> | 6 C + 8.333 LaN + 2.667 B <sub>5</sub> H <sub>7</sub> → 7.333 BN + 7.333 LaH <sub>2</sub> + LaB <sub>6</sub> H <sub>4</sub> C <sub>6</sub> N                                                                   | -5.1474             |
| LaNH <sub>4</sub> B <sub>6</sub> C <sub>6</sub> | 10.25 H <sub>2</sub> + 6.5 LaN + 3 B <sub>13</sub> C <sub>2</sub> → 5.5 LaB <sub>6</sub> + 5.5 H <sub>3</sub> N + LaB <sub>6</sub> H <sub>4</sub> C <sub>6</sub> N                                             | -5.0958             |
| LaNH <sub>4</sub> B <sub>6</sub> C <sub>6</sub> | 23.75 LaH <sub>2</sub> + 0.5 N <sub>2</sub> + 3 B <sub>13</sub> C <sub>2</sub> → 14.5 LaH <sub>3</sub> + 8.25 LaB <sub>4</sub> + LaB <sub>6</sub> H <sub>4</sub> C <sub>6</sub> N                              | -5.0906             |
| LaNH <sub>4</sub> B <sub>6</sub> C <sub>6</sub> | 9.75 La <sub>4</sub> H <sub>9</sub> + LaN + 3 B <sub>13</sub> C <sub>2</sub> → 5.5 LaB <sub>6</sub> + 16.75 La <sub>2</sub> H <sub>5</sub> + LaB <sub>6</sub> H <sub>4</sub> C <sub>6</sub> N                  | -5.0847             |
| LaNH <sub>4</sub> B <sub>6</sub> C <sub>6</sub> | 1.2 H <sub>8</sub> C <sub>5</sub> + 6.6 La + 1.2 B <sub>5</sub> H <sub>7</sub> + 0.5 N <sub>2</sub> → 2.8 La <sub>2</sub> H <sub>5</sub> + LaB <sub>6</sub> H <sub>4</sub> C <sub>6</sub> N                    | -5.0545             |
| LaNH <sub>4</sub> B <sub>6</sub> C <sub>6</sub> | BN + 25.33 LaH <sub>2</sub> + 3 B <sub>13</sub> C <sub>2</sub> → 5.667 LaB <sub>6</sub> + 9.333 La <sub>2</sub> H <sub>5</sub> + LaB <sub>6</sub> H <sub>4</sub> C <sub>6</sub> N                              | -5.0198             |
| LaNH <sub>4</sub> B <sub>6</sub> C <sub>6</sub> | 24 B + 1.333 H <sub>3</sub> N + 2 La <sub>2</sub> C <sub>3</sub> → 3 LaB <sub>6</sub> + 0.1667 N <sub>2</sub> + LaB <sub>6</sub> H <sub>4</sub> C <sub>6</sub> N                                               | -5.0127             |
| LaNH <sub>4</sub> B <sub>6</sub> C <sub>6</sub> | 25.11 B + 0.4444 La <sub>4</sub> H <sub>9</sub> + 2 La <sub>2</sub> C <sub>3</sub> + 0.5 N <sub>2</sub> → 4.778 LaB <sub>4</sub> + LaB <sub>6</sub> H <sub>4</sub> C <sub>6</sub> N                            | -5.0000             |
| LaNH <sub>4</sub> B <sub>6</sub> C <sub>6</sub> | 0.5 N <sub>2</sub> + 3 B <sub>13</sub> C <sub>2</sub> + 15.5 La <sub>2</sub> H <sub>5</sub> → 24.5 LaH <sub>3</sub> + 5.5 LaB <sub>6</sub> + LaB <sub>6</sub> H <sub>4</sub> C <sub>6</sub> N                  | -4.9974             |
| LaNH <sub>4</sub> B <sub>6</sub> C <sub>6</sub> | LaN + 58.25 LaH <sub>2</sub> + 3 B <sub>13</sub> C <sub>2</sub> → 12.5 La <sub>4</sub> H <sub>9</sub> + 8.25 LaB <sub>4</sub> + LaB <sub>6</sub> H <sub>4</sub> C <sub>6</sub> N                               | -4.9790             |

Continued on next page

Continued

| Compound                                        | Chemical reaction                                                                                                                                                                            | Reaction energy(eV) |
|-------------------------------------------------|----------------------------------------------------------------------------------------------------------------------------------------------------------------------------------------------|---------------------|
| LaNH <sub>4</sub> B <sub>6</sub> C <sub>6</sub> | $1.2 \text{H}_8\text{C}_5 + 8.275 \text{LaN} + 1.475 \text{B}_9\text{H}_{11} \rightarrow 7.275 \text{LaH}_3 + 7.275 \text{BN} + \text{LaB}_6\text{H}_4\text{C}_6\text{N}$                    | -4.9509             |
| LaNH <sub>4</sub> B <sub>6</sub> C <sub>6</sub> | $\text{H}_3\text{N} + 26.75 \text{LaH}_2 + 3 \text{B}_{13}\text{C}_2 \rightarrow 17.5 \text{LaH}_3 + 8.25 \text{LaB}_4 + \text{LaB}_6\text{H}_4\text{C}_6\text{N}$                           | -4.9205             |
| LaNH <sub>4</sub> B <sub>6</sub> C <sub>6</sub> | $28.4 \text{B} + \text{LaN} + 2 \text{La}_2\text{C}_3 + 0.8 \text{La}_2\text{H}_5 \rightarrow 5.6 \text{LaB}_4 + \text{LaB}_6\text{H}_4\text{C}_6\text{N}$                                   | -4.8634             |
| LaNH <sub>4</sub> B <sub>6</sub> C <sub>6</sub> | $0.5 \text{H}_8\text{C}_5 + 3.792 \text{La} + 0.5 \text{N}_2 + 1.75 \text{B}_{13}\text{C}_2 \rightarrow 2.792 \text{LaB}_6 + \text{LaB}_6\text{H}_4\text{C}_6\text{N}$                       | -4.8505             |
| LaNH <sub>4</sub> B <sub>6</sub> C <sub>6</sub> | $3 \text{LaC}_2 + 2.8 \text{B}_5\text{H}_7 + 3.1 \text{N}_2 \rightarrow 5.2 \text{H}_3\text{N} + 2 \text{LaB}_4 + \text{LaB}_6\text{H}_4\text{C}_6\text{N}$                                  | -4.8478             |
| LaNH <sub>4</sub> B <sub>6</sub> C <sub>6</sub> | $1.2 \text{H}_8\text{C}_5 + 6.748 \text{La} + 0.6667 \text{B}_9\text{H}_{11} + 0.5 \text{N}_2 \rightarrow 1.437 \text{La}_4\text{H}_9 + \text{LaB}_6\text{H}_4\text{C}_6\text{N}$            | -4.7800             |
| LaNH <sub>4</sub> B <sub>6</sub> C <sub>6</sub> | $\text{LaN} + 12.5 \text{LaH}_2 + 3 \text{B}_{13}\text{C}_2 \rightarrow 7 \text{LaH}_3 + 5.5 \text{LaB}_6 + \text{LaB}_6\text{H}_4\text{C}_6\text{N}$                                        | -4.7743             |
| LaNH <sub>4</sub> B <sub>6</sub> C <sub>6</sub> | $1.2 \text{H}_8\text{C}_5 + 6.667 \text{La} + \text{H}_3\text{N} + 1.2 \text{B}_5\text{H}_7 \rightarrow 5.667 \text{LaH}_3 + \text{LaB}_6\text{H}_4\text{C}_6\text{N}$                       | -4.7196             |
| LaNH <sub>4</sub> B <sub>6</sub> C <sub>6</sub> | $\text{BN} + 69.5 \text{LaH}_2 + 3 \text{B}_{13}\text{C}_2 \rightarrow 15 \text{La}_4\text{H}_9 + 8.5 \text{LaB}_4 + \text{LaB}_6\text{H}_4\text{C}_6\text{N}$                               | -4.6780             |
| LaNH <sub>4</sub> B <sub>6</sub> C <sub>6</sub> | $24.4 \text{B} + 2 \text{La}_2\text{C}_3 + 0.5 \text{N}_2 + 0.8 \text{La}_2\text{H}_5 \rightarrow 4.6 \text{LaB}_4 + \text{LaB}_6\text{H}_4\text{C}_6\text{N}$                               | -4.6744             |
| LaNH <sub>4</sub> B <sub>6</sub> C <sub>6</sub> | $\text{BN} + 12.67 \text{La}_4\text{H}_9 + 3 \text{B}_{13}\text{C}_2 \rightarrow 5.667 \text{LaB}_6 + 22 \text{La}_2\text{H}_5 + \text{LaB}_6\text{H}_4\text{C}_6\text{N}$                   | -4.6474             |
| LaNH <sub>4</sub> B <sub>6</sub> C <sub>6</sub> | $3 \text{LaC}_2 + 29 \text{B} + \text{BN} + 2 \text{LaH}_2 \rightarrow 4 \text{LaB}_6 + \text{LaB}_6\text{H}_4\text{C}_6\text{N}$                                                            | -4.6146             |
| LaNH <sub>4</sub> B <sub>6</sub> C <sub>6</sub> | $\text{LaN} + 33.25 \text{LaH}_2 + 3 \text{B}_{13}\text{C}_2 \rightarrow 12.5 \text{La}_2\text{H}_5 + 8.25 \text{LaB}_4 + \text{LaB}_6\text{H}_4\text{C}_6\text{N}$                          | -4.6115             |
| LaNH <sub>4</sub> B <sub>6</sub> C <sub>6</sub> | $22 \text{B} + 1.333 \text{H}_3\text{N} + 2 \text{La}_2\text{C}_3 \rightarrow 2.667 \text{LaB}_6 + 0.3333 \text{LaN} + \text{LaB}_6\text{H}_4\text{C}_6\text{N}$                             | -4.5862             |
| LaNH <sub>4</sub> B <sub>6</sub> C <sub>6</sub> | $9.333 \text{B} + 4.333 \text{H}_3\text{N} + 2 \text{La}_2\text{C}_3 \rightarrow 3 \text{LaH}_3 + 3.333 \text{BN} + \text{LaB}_6\text{H}_4\text{C}_6\text{N}$                                | -4.5833             |
| LaNH <sub>4</sub> B <sub>6</sub> C <sub>6</sub> | $\text{H}_3\text{N} + 3 \text{B}_{13}\text{C}_2 + 18.5 \text{LaH}_5 \rightarrow 30.5 \text{LaH}_3 + 5.5 \text{LaB}_6 + \text{LaB}_6\text{H}_4\text{C}_6\text{N}$                             | -4.5714             |
| LaNH <sub>4</sub> B <sub>6</sub> C <sub>6</sub> | $0.9091 \text{B}_9\text{H}_{11} + 2 \text{La}_2\text{C}_3 + 1.591 \text{N}_2 \rightarrow 2.182 \text{BN} + 3 \text{LaH}_2 + \text{LaB}_6\text{H}_4\text{C}_6\text{N}$                        | -4.5627             |
| LaNH <sub>4</sub> B <sub>6</sub> C <sub>6</sub> | $1.2 \text{H}_8\text{C}_5 + 3.233 \text{N}_2 + 2.867 \text{LaB}_4 \rightarrow 1.867 \text{LaH}_3 + 5.467 \text{BN} + \text{LaB}_6\text{H}_4\text{C}_6\text{N}$                               | -4.5594             |
| LaNH <sub>4</sub> B <sub>6</sub> C <sub>6</sub> | $6 \text{B} + 2 \text{La}_2\text{C}_3 + 2 \text{LaH}_2 + 3 \text{N}_2 \rightarrow 5 \text{LaN} + \text{LaB}_6\text{H}_4\text{C}_6\text{N}$                                                   | -4.4915             |
| LaNH <sub>4</sub> B <sub>6</sub> C <sub>6</sub> | $1.333 \text{LaH}_3 + 27.33 \text{B} + \text{LaN} + 2 \text{La}_2\text{C}_3 \rightarrow 5.333 \text{LaB}_4 + \text{LaB}_6\text{H}_4\text{C}_6\text{N}$                                       | -4.4692             |
| LaNH <sub>4</sub> B <sub>6</sub> C <sub>6</sub> | $7.967 \text{H}_3\text{N} + 0.5 \text{La}_2\text{C}_3 + 2.25 \text{B}_{13}\text{C}_2 \rightarrow 6.967 \text{BN} + 1.809 \text{B}_9\text{H}_{11} + \text{LaB}_6\text{H}_4\text{C}_6\text{N}$ | -4.4312             |
| LaNH <sub>4</sub> B <sub>6</sub> C <sub>6</sub> | $6.158 \text{H}_3\text{N} + 2 \text{La}_2\text{C}_3 + 2.789 \text{LaB}_4 \rightarrow 5.158 \text{BN} + 2.895 \text{La}_2\text{H}_5 + \text{LaB}_6\text{H}_4\text{C}_6\text{N}$               | -4.3650             |
| LaNH <sub>4</sub> B <sub>6</sub> C <sub>6</sub> | $3 \text{LaC}_2 + 2 \text{H}_2 + 24 \text{B} + \text{LaN} \rightarrow 3 \text{LaB}_6 + \text{LaB}_6\text{H}_4\text{C}_6\text{N}$                                                             | -4.3496             |
| LaNH <sub>4</sub> B <sub>6</sub> C <sub>6</sub> | $4.167 \text{La}_4\text{H}_9 + \text{LaN} + 3 \text{B}_{13}\text{C}_2 \rightarrow 11.17 \text{LaH}_3 + 5.5 \text{LaB}_6 + \text{LaB}_6\text{H}_4\text{C}_6\text{N}$                          | -4.2963             |
| LaNH <sub>4</sub> B <sub>6</sub> C <sub>6</sub> | $1.333 \text{LaH}_3 + 23.33 \text{B} + 2 \text{La}_2\text{C}_3 + 0.5 \text{N}_2 \rightarrow 4.333 \text{LaB}_4 + \text{LaB}_6\text{H}_4\text{C}_6\text{N}$                                   | -4.2802             |
| LaNH <sub>4</sub> B <sub>6</sub> C <sub>6</sub> | $\text{BN} + 39.5 \text{LaH}_2 + 3 \text{B}_{13}\text{C}_2 \rightarrow 15 \text{La}_2\text{H}_5 + 8.5 \text{LaB}_4 + \text{LaB}_6\text{H}_4\text{C}_6\text{N}$                               | -4.2369             |
| LaNH <sub>4</sub> B <sub>6</sub> C <sub>6</sub> | $\text{BN} + 16 \text{LaH}_2 + 3 \text{B}_{13}\text{C}_2 \rightarrow 9.333 \text{LaH}_3 + 5.667 \text{LaB}_6 + \text{LaB}_6\text{H}_4\text{C}_6\text{N}$                                     | -4.2237             |
| LaNH <sub>4</sub> B <sub>6</sub> C <sub>6</sub> | $16.73 \text{LaH}_3 + 8.367 \text{N}_2 + 3 \text{B}_{13}\text{C}_2 \rightarrow 15.73 \text{LaN} + 6.6 \text{B}_5\text{H}_7 + \text{LaB}_6\text{H}_4\text{C}_6\text{N}$                       | -4.2227             |
| LaNH <sub>4</sub> B <sub>6</sub> C <sub>6</sub> | $2 \text{H}_2 + 23 \text{B} + \text{BN} + 2 \text{La}_2\text{C}_3 \rightarrow 3 \text{LaB}_6 + \text{LaB}_6\text{H}_4\text{C}_6\text{N}$                                                     | -4.2114             |
| LaNH <sub>4</sub> B <sub>6</sub> C <sub>6</sub> | $2 \text{La}_2\text{C}_3 + 2 \text{LaH}_2 + 3.75 \text{N}_2 + 1.5 \text{LaB}_4 \rightarrow 6.5 \text{LaN} + \text{LaB}_6\text{H}_4\text{C}_6\text{N}$                                        | -4.2080             |
| LaNH <sub>4</sub> B <sub>6</sub> C <sub>6</sub> | $1.2 \text{H}_8\text{C}_5 + 6.173 \text{La} + 0.6667 \text{B}_9\text{H}_{11} + 0.5 \text{N}_2 \rightarrow 2.587 \text{La}_2\text{H}_5 + \text{LaB}_6\text{H}_4\text{C}_6\text{N}$            | -4.1966             |
| LaNH <sub>4</sub> B <sub>6</sub> C <sub>6</sub> | $7.917 \text{La}_4\text{H}_9 + 0.5 \text{N}_2 + 3 \text{B}_{13}\text{C}_2 \rightarrow 22.42 \text{LaH}_3 + 8.25 \text{LaB}_4 + \text{LaB}_6\text{H}_4\text{C}_6\text{N}$                     | -4.1826             |
| LaNH <sub>4</sub> B <sub>6</sub> C <sub>6</sub> | $16.63 \text{La}_4\text{H}_9 + \text{LaN} + 3 \text{B}_{13}\text{C}_2 \rightarrow 29.13 \text{La}_2\text{H}_5 + 8.25 \text{LaB}_4 + \text{LaB}_6\text{H}_4\text{C}_6\text{N}$                | -4.1228             |
| LaNH <sub>4</sub> B <sub>6</sub> C <sub>6</sub> | $6 \text{B} + 0.4444 \text{La}_4\text{H}_9 + 2 \text{La}_2\text{C}_3 + 2.889 \text{N}_2 \rightarrow 4.778 \text{LaN} + \text{LaB}_6\text{H}_4\text{C}_6\text{N}$                             | -4.0971             |
| LaNH <sub>4</sub> B <sub>6</sub> C <sub>6</sub> | $\text{LaC}_2 + 0.5 \text{H}_8\text{C}_5 + 2.375 \text{N}_2 + 0.75 \text{B}_{13}\text{C}_2 \rightarrow 3.75 \text{BN} + \text{LaB}_6\text{H}_4\text{C}_6\text{N}$                            | -4.0729             |
| LaNH <sub>4</sub> B <sub>6</sub> C <sub>6</sub> | $1.2 \text{H}_8\text{C}_5 + 6.311 \text{La} + \text{H}_3\text{N} + 0.6667 \text{B}_9\text{H}_{11} \rightarrow 5.311 \text{LaH}_3 + \text{LaB}_6\text{H}_4\text{C}_6\text{N}$                 | -3.9590             |
| LaNH <sub>4</sub> B <sub>6</sub> C <sub>6</sub> | $3 \text{LaC}_2 + 27.67 \text{B} + \text{BN} + 0.4444 \text{La}_4\text{H}_9 \rightarrow 3.778 \text{LaB}_6 + \text{LaB}_6\text{H}_4\text{C}_6\text{N}$                                       | -3.9358             |
| LaNH <sub>4</sub> B <sub>6</sub> C <sub>6</sub> | $0.5 \text{H}_8\text{C}_5 + 5.437 \text{La} + \text{BN} + 1.75 \text{B}_{13}\text{C}_2 \rightarrow 4.437 \text{LaB}_4 + \text{LaB}_6\text{H}_4\text{C}_6\text{N}$                            | -3.9237             |
| LaNH <sub>4</sub> B <sub>6</sub> C <sub>6</sub> | $8.917 \text{La}_4\text{H}_9 + \text{H}_3\text{N} + 3 \text{B}_{13}\text{C}_2 \rightarrow 26.42 \text{LaH}_3 + 8.25 \text{LaB}_4 + \text{LaB}_6\text{H}_4\text{C}_6\text{N}$                 | -3.8977             |
| LaNH <sub>4</sub> B <sub>6</sub> C <sub>6</sub> | $3 \text{LaC}_2 + 1.556 \text{B}_9\text{H}_{11} + 2.685 \text{N}_2 \rightarrow 4.37 \text{H}_3\text{N} + 2 \text{LaB}_4 + \text{LaB}_6\text{H}_4\text{C}_6\text{N}$                          | -3.8545             |
| LaNH <sub>4</sub> B <sub>6</sub> C <sub>6</sub> | $0.4444 \text{La}_4\text{H}_9 + 2 \text{La}_2\text{C}_3 + 3.639 \text{N}_2 + 1.5 \text{LaB}_4 \rightarrow 6.278 \text{LaN} + \text{LaB}_6\text{H}_4\text{C}_6\text{N}$                       | -3.8136             |
| LaNH <sub>4</sub> B <sub>6</sub> C <sub>6</sub> | $6 \text{B} + 2 \text{La}_2\text{C}_3 + 2.8 \text{N}_2 + 0.8 \text{La}_2\text{H}_5 \rightarrow 4.6 \text{LaN} + \text{LaB}_6\text{H}_4\text{C}_6\text{N}$                                    | -3.8051             |
| LaNH <sub>4</sub> B <sub>6</sub> C <sub>6</sub> | $1.867 \text{LaB}_6 + 6.2 \text{H}_3\text{N} + 2 \text{La}_2\text{C}_3 \rightarrow 4.867 \text{LaH}_3 + 5.2 \text{BN} + \text{LaB}_6\text{H}_4\text{C}_6\text{N}$                            | -3.7837             |
| LaNH <sub>4</sub> B <sub>6</sub> C <sub>6</sub> | $1.2 \text{H}_8\text{C}_5 + 5.667 \text{La} + 1.2 \text{B}_5\text{H}_7 + 0.5 \text{N}_2 \rightarrow 4.667 \text{LaH}_3 + \text{LaB}_6\text{H}_4\text{C}_6\text{N}$                           | -3.7778             |
| LaNH <sub>4</sub> B <sub>6</sub> C <sub>6</sub> | $0.125 \text{H}_8\text{C}_5 + 21.5 \text{B} + \text{H}_3\text{N} + 1.792 \text{La}_2\text{C}_3 \rightarrow 2.583 \text{LaB}_6 + \text{LaB}_6\text{H}_4\text{C}_6\text{N}$                    | -3.7606             |
| LaNH <sub>4</sub> B <sub>6</sub> C <sub>6</sub> | $3 \text{LaC}_2 + 21.14 \text{B} + \text{LaN} + 0.5714 \text{B}_5\text{H}_7 \rightarrow 3 \text{LaB}_6 + \text{LaB}_6\text{H}_4\text{C}_6\text{N}$                                           | -3.7524             |
| LaNH <sub>4</sub> B <sub>6</sub> C <sub>6</sub> | $1.2 \text{H}_8\text{C}_5 + 7 \text{La} + \text{LaN} + 1.2 \text{B}_5\text{H}_7 \rightarrow 7 \text{LaH}_2 + \text{LaB}_6\text{H}_4\text{C}_6\text{N}$                                       | -3.7151             |
| LaNH <sub>4</sub> B <sub>6</sub> C <sub>6</sub> | $\text{LaN} + 3 \text{B}_{13}\text{C}_2 + 12.5 \text{La}_2\text{H}_5 \rightarrow 19.5 \text{LaH}_3 + 5.5 \text{LaB}_6 + \text{LaB}_6\text{H}_4\text{C}_6\text{N}$                            | -3.7080             |
| LaNH <sub>4</sub> B <sub>6</sub> C <sub>6</sub> | $2 \text{H}_2 + 22 \text{B} + \text{LaN} + 2 \text{La}_2\text{C}_3 \rightarrow 4 \text{LaB}_4 + \text{LaB}_6\text{H}_4\text{C}_6\text{N}$                                                    | -3.6953             |
| LaNH <sub>4</sub> B <sub>6</sub> C <sub>6</sub> | $3 \text{LaC}_2 + 20.73 \text{B} + \text{LaN} + 0.3636 \text{B}_9\text{H}_{11} \rightarrow 3 \text{LaB}_6 + \text{LaB}_6\text{H}_4\text{C}_6\text{N}$                                        | -3.6902             |
| LaNH <sub>4</sub> B <sub>6</sub> C <sub>6</sub> | $\text{LaC}_2 + 7.591 \text{H}_3\text{N} + 2 \text{B}_{13}\text{C}_2 \rightarrow 6.591 \text{BN} + 2.682 \text{B}_5\text{H}_7 + \text{LaB}_6\text{H}_4\text{C}_6\text{N}$                    | -3.6896             |
| LaNH <sub>4</sub> B <sub>6</sub> C <sub>6</sub> | $2 \text{La}_2\text{C}_3 + 1.536 \text{B}_5\text{H}_7 + 1.339 \text{N}_2 \rightarrow 1.679 \text{BN} + 0.75 \text{La}_4\text{H}_9 + \text{LaB}_6\text{H}_4\text{C}_6\text{N}$                | -3.6892             |
| LaNH <sub>4</sub> B <sub>6</sub> C <sub>6</sub> | $3 \text{LaC}_2 + 0.9091 \text{B}_9\text{H}_{11} + 1.591 \text{N}_2 \rightarrow 2 \text{LaH}_3 + 2.182 \text{BN} + \text{LaB}_6\text{H}_4\text{C}_6\text{N}$                                 | -3.6795             |
| LaNH <sub>4</sub> B <sub>6</sub> C <sub>6</sub> | $\text{BN} + 19.75 \text{La}_4\text{H}_9 + 3 \text{B}_{13}\text{C}_2 \rightarrow 34.75 \text{La}_2\text{H}_5 + 8.5 \text{LaB}_4 + \text{LaB}_6\text{H}_4\text{C}_6\text{N}$                  | -3.6563             |
| LaNH <sub>4</sub> B <sub>6</sub> C <sub>6</sub> | $2 \text{La}_2\text{C}_3 + 1.2 \text{B}_5\text{H}_7 + 2.733 \text{N}_2 \rightarrow 1.467 \text{H}_3\text{N} + 3 \text{LaN} + \text{LaB}_6\text{H}_4\text{C}_6\text{N}$                       | -3.6273             |
| LaNH <sub>4</sub> B <sub>6</sub> C <sub>6</sub> | $20.14 \text{B} + \text{BN} + 2 \text{La}_2\text{C}_3 + 0.5714 \text{B}_5\text{H}_7 \rightarrow 3 \text{LaB}_6 + \text{LaB}_6\text{H}_4\text{C}_6\text{N}$                                   | -3.6142             |
| LaNH <sub>4</sub> B <sub>6</sub> C <sub>6</sub> | $\text{BN} + 5.333 \text{La}_4\text{H}_9 + 3 \text{B}_{13}\text{C}_2 \rightarrow 14.67 \text{LaH}_3 + 5.667 \text{LaB}_6 + \text{LaB}_6\text{H}_4\text{C}_6\text{N}$                         | -3.6119             |
| LaNH <sub>4</sub> B <sub>6</sub> C <sub>6</sub> | $19.73 \text{B} + \text{BN} + 0.3636 \text{B}_9\text{H}_{11} + 2 \text{La}_2\text{C}_3 \rightarrow 3 \text{LaB}_6 + \text{LaB}_6\text{H}_4\text{C}_6\text{N}$                                | -3.5520             |
| LaNH <sub>4</sub> B <sub>6</sub> C <sub>6</sub> | $\text{LaN} + 20.75 \text{LaH}_2 + 3 \text{B}_{13}\text{C}_2 \rightarrow 12.5 \text{LaH}_3 + 8.25 \text{LaB}_4 + \text{LaB}_6\text{H}_4\text{C}_6\text{N}$                                   | -3.5453             |
| LaNH <sub>4</sub> B <sub>6</sub> C <sub>6</sub> | $2 \text{La}_2\text{C}_3 + 3.55 \text{N}_2 + 0.8 \text{La}_2\text{H}_5 + 1.5 \text{LaB}_4 \rightarrow 6.1 \text{LaN} + \text{LaB}_6\text{H}_4\text{C}_6\text{N}$                             | -3.5216             |

Continued on next page

Continued

| Compound                                        | Chemical reaction                                                                                                                                                                                        | Reaction energy(eV) |
|-------------------------------------------------|----------------------------------------------------------------------------------------------------------------------------------------------------------------------------------------------------------|---------------------|
| LaNH <sub>4</sub> B <sub>6</sub> C <sub>6</sub> | 8.833 B + 3.833 H <sub>3</sub> N + 2 La <sub>2</sub> C <sub>3</sub> → 2.833 BN + 1.5 La <sub>2</sub> H <sub>5</sub> + LaB <sub>6</sub> H <sub>4</sub> C <sub>6</sub> N                                   | -3.5129             |
| LaNH <sub>4</sub> B <sub>6</sub> C <sub>6</sub> | 2 H <sub>2</sub> + 18 B + 2 La <sub>2</sub> C <sub>3</sub> + 0.5 N <sub>2</sub> → 3 LaB <sub>4</sub> + LaB <sub>6</sub> H <sub>4</sub> C <sub>6</sub> N                                                  | -3.5063             |
| LaNH <sub>4</sub> B <sub>6</sub> C <sub>6</sub> | 1.333 LaH <sub>3</sub> + 6 B + 2 La <sub>2</sub> C <sub>3</sub> + 2.667 N <sub>2</sub> → 4.333 LaN + LaB <sub>6</sub> H <sub>4</sub> C <sub>6</sub> N                                                    | -3.4612             |
| LaNH <sub>4</sub> B <sub>6</sub> C <sub>6</sub> | 3 LaC <sub>2</sub> + 26.6 B + BN + 0.8 La <sub>2</sub> H <sub>5</sub> → 3.6 LaB <sub>6</sub> + LaB <sub>6</sub> H <sub>4</sub> C <sub>6</sub> N                                                          | -3.4164             |
| LaNH <sub>4</sub> B <sub>6</sub> C <sub>6</sub> | LaN + 23.75 B <sub>9</sub> H <sub>11</sub> + 2 La <sub>2</sub> C <sub>3</sub> → 4 LaB <sub>6</sub> + 36.75 B <sub>5</sub> H <sub>7</sub> + LaB <sub>6</sub> H <sub>4</sub> C <sub>6</sub> N              | -3.3937             |
| LaNH <sub>4</sub> B <sub>6</sub> C <sub>6</sub> | 14.38 H <sub>2</sub> + 9.25 LaN + 3 B <sub>13</sub> C <sub>2</sub> → 8.25 H <sub>3</sub> N + 8.25 LaB <sub>4</sub> + LaB <sub>6</sub> H <sub>4</sub> C <sub>6</sub> N                                    | -3.2583             |
| LaNH <sub>4</sub> B <sub>6</sub> C <sub>6</sub> | 4.375 LaC <sub>2</sub> + 1.2 B <sub>5</sub> H <sub>7</sub> + 2.188 N <sub>2</sub> → 0.55 H <sub>8</sub> C <sub>5</sub> + 3.375 LaN + LaB <sub>6</sub> H <sub>4</sub> C <sub>6</sub> N                    | -3.2491             |
| LaNH <sub>4</sub> B <sub>6</sub> C <sub>6</sub> | LaB <sub>6</sub> + 2 La <sub>2</sub> C <sub>3</sub> + 2 LaH <sub>2</sub> + 3.5 N <sub>2</sub> → 6 LaN + LaB <sub>6</sub> H <sub>4</sub> C <sub>6</sub> N                                                 | -3.2119             |
| LaNH <sub>4</sub> B <sub>6</sub> C <sub>6</sub> | 14.78 LaH <sub>3</sub> + 7.389 N <sub>2</sub> + 3 B <sub>13</sub> C <sub>2</sub> → 13.78 LaN + 3.667 B <sub>9</sub> H <sub>11</sub> + LaB <sub>6</sub> H <sub>4</sub> C <sub>6</sub> N                   | -3.2092             |
| LaNH <sub>4</sub> B <sub>6</sub> C <sub>6</sub> | 0.6667 B <sub>9</sub> H <sub>11</sub> + 2 La <sub>2</sub> C <sub>3</sub> + 2.556 N <sub>2</sub> → 1.111 H <sub>3</sub> N + 3 LaN + LaB <sub>6</sub> H <sub>4</sub> C <sub>6</sub> N                      | -3.2016             |
| LaNH <sub>4</sub> B <sub>6</sub> C <sub>6</sub> | 1.333 LaH <sub>3</sub> + 2 La <sub>2</sub> C <sub>3</sub> + 3.417 N <sub>2</sub> + 1.5 LaB <sub>4</sub> → 5.833 LaN + LaB <sub>6</sub> H <sub>4</sub> C <sub>6</sub> N                                   | -3.1777             |
| LaNH <sub>4</sub> B <sub>6</sub> C <sub>6</sub> | 3 LaC <sub>2</sub> + 6.111 H <sub>3</sub> N + 2.778 LaB <sub>4</sub> → 4.778 LaH <sub>3</sub> + 5.111 BN + LaB <sub>6</sub> H <sub>4</sub> C <sub>6</sub> N                                              | -3.1431             |
| LaNH <sub>4</sub> B <sub>6</sub> C <sub>6</sub> | 0.5 H <sub>8</sub> C <sub>5</sub> + 4.187 La + LaN + 1.75 B <sub>13</sub> C <sub>2</sub> → 4.187 LaB <sub>4</sub> + LaB <sub>6</sub> H <sub>4</sub> C <sub>6</sub> N                                     | -3.1215             |
| LaNH <sub>4</sub> B <sub>6</sub> C <sub>6</sub> | 5.564 H <sub>3</sub> N + 2 La <sub>2</sub> C <sub>3</sub> + 2.641 LaB <sub>4</sub> → 4.564 BN + 1.41 La <sub>4</sub> H <sub>9</sub> + LaB <sub>6</sub> H <sub>4</sub> C <sub>6</sub> N                   | -3.1143             |
| LaNH <sub>4</sub> B <sub>6</sub> C <sub>6</sub> | 19.14 B + LaN + 2 La <sub>2</sub> C <sub>3</sub> + 0.5714 B <sub>5</sub> H <sub>7</sub> → 4 LaB <sub>4</sub> + LaB <sub>6</sub> H <sub>4</sub> C <sub>6</sub> N                                          | -3.0981             |
| LaNH <sub>4</sub> B <sub>6</sub> C <sub>6</sub> | 3 LaC <sub>2</sub> + 2 H <sub>2</sub> + 18 B + 0.5 N <sub>2</sub> → 2 LaB <sub>6</sub> + LaB <sub>6</sub> H <sub>4</sub> C <sub>6</sub> N                                                                | -3.0700             |
| LaNH <sub>4</sub> B <sub>6</sub> C <sub>6</sub> | 0.5 N <sub>2</sub> + 3 B <sub>13</sub> C <sub>2</sub> + 23.75 La <sub>2</sub> H <sub>5</sub> → 38.25 LaH <sub>3</sub> + 8.25 LaB <sub>4</sub> + LaB <sub>6</sub> H <sub>4</sub> C <sub>6</sub> N         | -3.0647             |
| LaNH <sub>4</sub> B <sub>6</sub> C <sub>6</sub> | 18.73 B + LaN + 0.3636 B <sub>9</sub> H <sub>11</sub> + 2 La <sub>2</sub> C <sub>3</sub> → 4 LaB <sub>4</sub> + LaB <sub>6</sub> H <sub>4</sub> C <sub>6</sub> N                                         | -3.0359             |
| LaNH <sub>4</sub> B <sub>6</sub> C <sub>6</sub> | 1.2 H <sub>8</sub> C <sub>5</sub> + 6.222 La + LaN + 1.2 B <sub>5</sub> H <sub>7</sub> → 1.556 La <sub>4</sub> H <sub>9</sub> + LaB <sub>6</sub> H <sub>4</sub> C <sub>6</sub> N                         | -3.0286             |
| LaNH <sub>4</sub> B <sub>6</sub> C <sub>6</sub> | 1.2 H <sub>8</sub> C <sub>5</sub> + 5.311 La + 0.6667 B <sub>9</sub> H <sub>11</sub> + 0.5 N <sub>2</sub> → 4.311 LaH <sub>3</sub> + LaB <sub>6</sub> H <sub>4</sub> C <sub>6</sub> N                    | -3.0172             |
| LaNH <sub>4</sub> B <sub>6</sub> C <sub>6</sub> | 18.5 B <sub>9</sub> H <sub>11</sub> + 2 La <sub>2</sub> C <sub>3</sub> + 0.5 N <sub>2</sub> → 3 LaB <sub>6</sub> + 28.5 B <sub>5</sub> H <sub>7</sub> + LaB <sub>6</sub> H <sub>4</sub> C <sub>6</sub> N | -3.0131             |
| LaNH <sub>4</sub> B <sub>6</sub> C <sub>6</sub> | 3 LaC <sub>2</sub> + 26 B + LaN + 2 LaH <sub>2</sub> → 5 LaB <sub>4</sub> + LaB <sub>6</sub> H <sub>4</sub> C <sub>6</sub> N                                                                             | -3.0079             |
| LaNH <sub>4</sub> B <sub>6</sub> C <sub>6</sub> | LaC <sub>2</sub> + 7.026 H <sub>3</sub> N + 2 B <sub>13</sub> C <sub>2</sub> → 6.026 BN + 1.553 B <sub>9</sub> H <sub>11</sub> + LaB <sub>6</sub> H <sub>4</sub> C <sub>6</sub> N                        | -3.0010             |
| LaNH <sub>4</sub> B <sub>6</sub> C <sub>6</sub> | BN + 24.5 LaH <sub>2</sub> + 3 B <sub>13</sub> C <sub>2</sub> → 15 LaH <sub>3</sub> + 8.5 LaB <sub>4</sub> + LaB <sub>6</sub> H <sub>4</sub> C <sub>6</sub> N                                            | -2.9574             |
| LaNH <sub>4</sub> B <sub>6</sub> C <sub>6</sub> | 0.5 H <sub>8</sub> C <sub>5</sub> + 3.958 La + BN + 1.75 B <sub>13</sub> C <sub>2</sub> → 2.958 LaB <sub>6</sub> + LaB <sub>6</sub> H <sub>4</sub> C <sub>6</sub> N                                      | -2.9399             |
| LaNH <sub>4</sub> B <sub>6</sub> C <sub>6</sub> | 2 H <sub>2</sub> + 6 B + 2 La <sub>2</sub> C <sub>3</sub> + 2 N <sub>2</sub> → 3 LaN + LaB <sub>6</sub> H <sub>4</sub> C <sub>6</sub> N                                                                  | -2.9393             |
| LaNH <sub>4</sub> B <sub>6</sub> C <sub>6</sub> | 15.14 B + 2 La <sub>2</sub> C <sub>3</sub> + 0.5714 B <sub>5</sub> H <sub>7</sub> + 0.5 N <sub>2</sub> → 3 LaB <sub>4</sub> + LaB <sub>6</sub> H <sub>4</sub> C <sub>6</sub> N                           | -2.9091             |
| LaNH <sub>4</sub> B <sub>6</sub> C <sub>6</sub> | 8.583 B + 3.583 H <sub>3</sub> N + 2 La <sub>2</sub> C <sub>3</sub> → 2.583 BN + 0.75 La <sub>4</sub> H <sub>9</sub> + LaB <sub>6</sub> H <sub>4</sub> C <sub>6</sub> N                                  | -2.8718             |
| LaNH <sub>4</sub> B <sub>6</sub> C <sub>6</sub> | 25 B + BN + 2 La <sub>2</sub> C <sub>3</sub> + 2 LaH <sub>2</sub> → 5 LaB <sub>4</sub> + LaB <sub>6</sub> H <sub>4</sub> C <sub>6</sub> N                                                                | -2.8696             |
| LaNH <sub>4</sub> B <sub>6</sub> C <sub>6</sub> | BN + 3 B <sub>13</sub> C <sub>2</sub> + 16 La <sub>2</sub> H <sub>5</sub> → 25.33 LaH <sub>3</sub> + 5.667 LaB <sub>6</sub> + LaB <sub>6</sub> H <sub>4</sub> C <sub>6</sub> N                           | -2.8589             |
| LaNH <sub>4</sub> B <sub>6</sub> C <sub>6</sub> | 6.5 LaH <sub>2</sub> + 0.5 N <sub>2</sub> + 3 B <sub>13</sub> C <sub>2</sub> → 4.5 H <sub>2</sub> + 5.5 LaB <sub>6</sub> + LaB <sub>6</sub> H <sub>4</sub> C <sub>6</sub> N                              | -2.8578             |
| LaNH <sub>4</sub> B <sub>6</sub> C <sub>6</sub> | 2.4 LaN + 4.1 LaH <sub>2</sub> + 3 B <sub>13</sub> C <sub>2</sub> → 5.5 LaB <sub>6</sub> + 1.4 H <sub>3</sub> N + LaB <sub>6</sub> H <sub>4</sub> C <sub>6</sub> N                                       | -2.8490             |
| LaNH <sub>4</sub> B <sub>6</sub> C <sub>6</sub> | 14.73 B + 0.3636 B <sub>9</sub> H <sub>11</sub> + 2 La <sub>2</sub> C <sub>3</sub> + 0.5 N <sub>2</sub> → 3 LaB <sub>4</sub> + LaB <sub>6</sub> H <sub>4</sub> C <sub>6</sub> N                          | -2.8469             |
| LaNH <sub>4</sub> B <sub>6</sub> C <sub>6</sub> | 3 LaC <sub>2</sub> + 22 B + 2 LaH <sub>2</sub> + 0.5 N <sub>2</sub> → 4 LaB <sub>4</sub> + LaB <sub>6</sub> H <sub>4</sub> C <sub>6</sub> N                                                              | -2.8189             |
| LaNH <sub>4</sub> B <sub>6</sub> C <sub>6</sub> | LaB <sub>6</sub> + 0.4444 La <sub>4</sub> H <sub>9</sub> + 2 La <sub>2</sub> C <sub>3</sub> + 3.389 N <sub>2</sub> → 5.778 LaN + LaB <sub>6</sub> H <sub>4</sub> C <sub>6</sub> N                        | -2.8175             |
| LaNH <sub>4</sub> B <sub>6</sub> C <sub>6</sub> | 3 LaC <sub>2</sub> + 21 B + H <sub>3</sub> N + 0.5 LaH <sub>2</sub> → 2.5 LaB <sub>6</sub> + LaB <sub>6</sub> H <sub>4</sub> C <sub>6</sub> N                                                            | -2.7738             |
| LaNH <sub>4</sub> B <sub>6</sub> C <sub>6</sub> | 1.2 H <sub>8</sub> C <sub>5</sub> + 6.467 La + LaN + 0.6667 B <sub>9</sub> H <sub>11</sub> → 6.467 LaH <sub>2</sub> + LaB <sub>6</sub> H <sub>4</sub> C <sub>6</sub> N                                   | -2.7568             |
| LaNH <sub>4</sub> B <sub>6</sub> C <sub>6</sub> | 6.917 La <sub>4</sub> H <sub>9</sub> + LaN + 3 B <sub>13</sub> C <sub>2</sub> → 19.42 LaH <sub>3</sub> + 8.25 LaB <sub>4</sub> + LaB <sub>6</sub> H <sub>4</sub> C <sub>6</sub> N                        | -2.7519             |
| LaNH <sub>4</sub> B <sub>6</sub> C <sub>6</sub> | 3 LaC <sub>2</sub> + 1.333 LaH <sub>3</sub> + 25 B + BN → 3.333 LaB <sub>6</sub> + LaB <sub>6</sub> H <sub>4</sub> C <sub>6</sub> N                                                                      | -2.7313             |
| LaNH <sub>4</sub> B <sub>6</sub> C <sub>6</sub> | 1.2 H <sub>8</sub> C <sub>5</sub> + 7.3 La + BN + B <sub>5</sub> H <sub>7</sub> → 6.3 LaH <sub>2</sub> + LaB <sub>6</sub> H <sub>4</sub> C <sub>6</sub> N                                                | -2.6978             |
| LaNH <sub>4</sub> B <sub>6</sub> C <sub>6</sub> | 20 B + H <sub>3</sub> N + 2 La <sub>2</sub> C <sub>3</sub> + 0.5 LaH <sub>2</sub> → 3.5 LaB <sub>4</sub> + LaB <sub>6</sub> H <sub>4</sub> C <sub>6</sub> N                                              | -2.6648             |
| LaNH <sub>4</sub> B <sub>6</sub> C <sub>6</sub> | 2 H <sub>2</sub> + 2 La <sub>2</sub> C <sub>3</sub> + 2.75 N <sub>2</sub> + 1.5 LaB <sub>4</sub> → 4.5 LaN + LaB <sub>6</sub> H <sub>4</sub> C <sub>6</sub> N                                            | -2.6558             |
| LaNH <sub>4</sub> B <sub>6</sub> C <sub>6</sub> | H <sub>3</sub> N + 3 B <sub>13</sub> C <sub>2</sub> + 26.75 La <sub>2</sub> H <sub>5</sub> → 44.25 LaH <sub>3</sub> + 8.25 LaB <sub>4</sub> + LaB <sub>6</sub> H <sub>4</sub> C <sub>6</sub> N           | -2.6387             |
| LaNH <sub>4</sub> B <sub>6</sub> C <sub>6</sub> | 1.692 La <sub>2</sub> C <sub>3</sub> + 2 LaH <sub>2</sub> + 2.692 N <sub>2</sub> + 0.4615 B <sub>13</sub> C <sub>2</sub> → 4.385 LaN + LaB <sub>6</sub> H <sub>4</sub> C <sub>6</sub> N                  | -2.6201             |
| LaNH <sub>4</sub> B <sub>6</sub> C <sub>6</sub> | 3 LaC <sub>2</sub> + 20.67 B + 0.1111 La <sub>4</sub> H <sub>9</sub> + H <sub>3</sub> N → 2.444 LaB <sub>6</sub> + LaB <sub>6</sub> H <sub>4</sub> C <sub>6</sub> N                                      | -2.6041             |
| LaNH <sub>4</sub> B <sub>6</sub> C <sub>6</sub> | 18.33 B + 1.333 H <sub>3</sub> N + 2 La <sub>2</sub> C <sub>3</sub> → 0.3333 BN + 3 LaB <sub>4</sub> + LaB <sub>6</sub> H <sub>4</sub> C <sub>6</sub> N                                                  | -2.5964             |
| LaNH <sub>4</sub> B <sub>6</sub> C <sub>6</sub> | 3 LaC <sub>2</sub> + 25.11 B + 0.4444 La <sub>4</sub> H <sub>9</sub> + LaN → 4.778 LaB <sub>4</sub> + LaB <sub>6</sub> H <sub>4</sub> C <sub>6</sub> N                                                   | -2.5715             |
| LaNH <sub>4</sub> B <sub>6</sub> C <sub>6</sub> | 19.78 B + 0.1111 La <sub>4</sub> H <sub>9</sub> + H <sub>3</sub> N + 2 La <sub>2</sub> C <sub>3</sub> → 3.444 LaB <sub>4</sub> + LaB <sub>6</sub> H <sub>4</sub> C <sub>6</sub> N                        | -2.5557             |
| LaNH <sub>4</sub> B <sub>6</sub> C <sub>6</sub> | LaB <sub>6</sub> + 2 La <sub>2</sub> C <sub>3</sub> + 3.3 N <sub>2</sub> + 0.8 La <sub>2</sub> H <sub>5</sub> → 5.6 LaN + LaB <sub>6</sub> H <sub>4</sub> C <sub>6</sub> N                               | -2.5255             |
| LaNH <sub>4</sub> B <sub>6</sub> C <sub>6</sub> | 19.6 B + H <sub>3</sub> N + 2 La <sub>2</sub> C <sub>3</sub> + 0.2 La <sub>2</sub> H <sub>5</sub> → 3.4 LaB <sub>4</sub> + LaB <sub>6</sub> H <sub>4</sub> C <sub>6</sub> N                              | -2.4743             |
| LaNH <sub>4</sub> B <sub>6</sub> C <sub>6</sub> | 3 LaC <sub>2</sub> + 20.4 B + H <sub>3</sub> N + 0.2 La <sub>2</sub> H <sub>5</sub> → 2.4 LaB <sub>6</sub> + LaB <sub>6</sub> H <sub>4</sub> C <sub>6</sub> N                                            | -2.4742             |
| LaNH <sub>4</sub> B <sub>6</sub> C <sub>6</sub> | 3 LaC <sub>2</sub> + 15.14 B + 0.5714 B <sub>5</sub> H <sub>7</sub> + 0.5 N <sub>2</sub> → 2 LaB <sub>6</sub> + LaB <sub>6</sub> H <sub>4</sub> C <sub>6</sub> N                                         | -2.4728             |
| LaNH <sub>4</sub> B <sub>6</sub> C <sub>6</sub> | 0.9762 La <sub>4</sub> H <sub>9</sub> + 2.595 LaN + 3 B <sub>13</sub> C <sub>2</sub> → 5.5 LaB <sub>6</sub> + 1.595 H <sub>3</sub> N + LaB <sub>6</sub> H <sub>4</sub> C <sub>6</sub> N                  | -2.4685             |
| LaNH <sub>4</sub> B <sub>6</sub> C <sub>6</sub> | 24.11 B + BN + 0.4444 La <sub>4</sub> H <sub>9</sub> + 2 La <sub>2</sub> C <sub>3</sub> → 4.778 LaB <sub>4</sub> + LaB <sub>6</sub> H <sub>4</sub> C <sub>6</sub> N                                      | -2.4333             |
| LaNH <sub>4</sub> B <sub>6</sub> C <sub>6</sub> | 3 LaC <sub>2</sub> + 14.73 B + 0.3636 B <sub>9</sub> H <sub>11</sub> + 0.5 N <sub>2</sub> → 2 LaB <sub>6</sub> + LaB <sub>6</sub> H <sub>4</sub> C <sub>6</sub> N                                        | -2.4106             |
| LaNH <sub>4</sub> B <sub>6</sub> C <sub>6</sub> | 1.2 H <sub>8</sub> C <sub>5</sub> + 5.6 La + LaN + 1.2 B <sub>5</sub> H <sub>7</sub> → 2.8 La <sub>2</sub> H <sub>5</sub> + LaB <sub>6</sub> H <sub>4</sub> C <sub>6</sub> N                             | -2.3971             |
| LaNH <sub>4</sub> B <sub>6</sub> C <sub>6</sub> | 3 LaC <sub>2</sub> + 21.11 B + 0.4444 La <sub>4</sub> H <sub>9</sub> + 0.5 N <sub>2</sub> → 3.778 LaB <sub>4</sub> + LaB <sub>6</sub> H <sub>4</sub> C <sub>6</sub> N                                    | -2.3825             |
| LaNH <sub>4</sub> B <sub>6</sub> C <sub>6</sub> | 6 C + 6.176 LaN + 2.235 B <sub>5</sub> H <sub>7</sub> → 5.176 BN + 1.294 La <sub>4</sub> H <sub>9</sub> + LaB <sub>6</sub> H <sub>4</sub> C <sub>6</sub> N                                               | -2.3822             |
| LaNH <sub>4</sub> B <sub>6</sub> C <sub>6</sub> | 0.3333 LaH <sub>3</sub> + 19.33 B + H <sub>3</sub> N + 2 La <sub>2</sub> C <sub>3</sub> → 3.333 LaB <sub>4</sub> + LaB <sub>6</sub> H <sub>4</sub> C <sub>6</sub> N                                      | -2.3757             |
| LaNH <sub>4</sub> B <sub>6</sub> C <sub>6</sub> | 3.143 B + 2 La <sub>2</sub> C <sub>3</sub> + 0.5714 B <sub>5</sub> H <sub>7</sub> + 2 N <sub>2</sub> → 3 LaN + LaB <sub>6</sub> H <sub>4</sub> C <sub>6</sub> N                                          | -2.3422             |

Continued on next page

Continued

| Compound                                        | Chemical reaction                                                                                                                                                                                          | Reaction energy(eV) |
|-------------------------------------------------|------------------------------------------------------------------------------------------------------------------------------------------------------------------------------------------------------------|---------------------|
| LaNH <sub>4</sub> B <sub>6</sub> C <sub>6</sub> | 0.5 H <sub>8</sub> C <sub>5</sub> + 0.5 N <sub>2</sub> + 1.75 B <sub>13</sub> C <sub>2</sub> + 11.38 LaB <sub>4</sub> → 10.38 LaB <sub>6</sub> + LaB <sub>6</sub> H <sub>4</sub> C <sub>6</sub> N          | -2.3287             |
| LaNH <sub>4</sub> B <sub>6</sub> C <sub>6</sub> | 4.042 LaC <sub>2</sub> + 0.6667 B <sub>9</sub> H <sub>11</sub> + 2.021 N <sub>2</sub> → 0.4167 H <sub>8</sub> C <sub>5</sub> + 3.042 LaN + LaB <sub>6</sub> H <sub>4</sub> C <sub>6</sub> N                | -2.3263             |
| LaNH <sub>4</sub> B <sub>6</sub> C <sub>6</sub> | 3 LaC <sub>2</sub> + 0.3333 LaH <sub>3</sub> + 20 B + H <sub>3</sub> N → 2.333 LaB <sub>6</sub> + LaB <sub>6</sub> H <sub>4</sub> C <sub>6</sub> N                                                         | -2.3029             |
| LaNH <sub>4</sub> B <sub>6</sub> C <sub>6</sub> | 2.727 B + 0.3636 B <sub>9</sub> H <sub>11</sub> + 2 La <sub>2</sub> C <sub>3</sub> + 2 N <sub>2</sub> → 3 LaN + LaB <sub>6</sub> H <sub>4</sub> C <sub>6</sub> N                                           | -2.2799             |
| LaNH <sub>4</sub> B <sub>6</sub> C <sub>6</sub> | 3 LaC <sub>2</sub> + 24.4 B + LaN + 0.8 La <sub>2</sub> H <sub>5</sub> → 4.6 LaB <sub>4</sub> + LaB <sub>6</sub> H <sub>4</sub> C <sub>6</sub> N                                                           | -2.2459             |
| LaNH <sub>4</sub> B <sub>6</sub> C <sub>6</sub> | 0.4444 La <sub>4</sub> H <sub>9</sub> + 1.692 La <sub>2</sub> C <sub>3</sub> + 2.581 N <sub>2</sub> + 0.4615 B <sub>13</sub> C <sub>2</sub> → 4.162 LaN + LaB <sub>6</sub> H <sub>4</sub> C <sub>6</sub> N | -2.2257             |
| LaNH <sub>4</sub> B <sub>6</sub> C <sub>6</sub> | 2 La <sub>2</sub> C <sub>3</sub> + 0.5714 B <sub>5</sub> H <sub>7</sub> + 2.393 N <sub>2</sub> + 0.7857 LaB <sub>4</sub> → 3.786 LaN + LaB <sub>6</sub> H <sub>4</sub> C <sub>6</sub> N                    | -2.1937             |
| LaNH <sub>4</sub> B <sub>6</sub> C <sub>6</sub> | 0.5 H <sub>8</sub> C <sub>5</sub> + 2.792 La + LaN + 1.75 B <sub>13</sub> C <sub>2</sub> → 2.792 LaB <sub>6</sub> + LaB <sub>6</sub> H <sub>4</sub> C <sub>6</sub> N                                       | -2.1931             |
| LaNH <sub>4</sub> B <sub>6</sub> C <sub>6</sub> | 8.333 B + 3.333 H <sub>3</sub> N + 2 La <sub>2</sub> C <sub>3</sub> → 2.333 BN + 3 LaH <sub>2</sub> + LaB <sub>6</sub> H <sub>4</sub> C <sub>6</sub> N                                                     | -2.1867             |
| LaNH <sub>4</sub> B <sub>6</sub> C <sub>6</sub> | 0.5 H <sub>2</sub> + 18 B + H <sub>3</sub> N + 2 La <sub>2</sub> C <sub>3</sub> → 3 LaB <sub>4</sub> + LaB <sub>6</sub> H <sub>4</sub> C <sub>6</sub> N                                                    | -2.1822             |
| LaNH <sub>4</sub> B <sub>6</sub> C <sub>6</sub> | 1.333 LaH <sub>3</sub> + LaB <sub>6</sub> + 2 La <sub>2</sub> C <sub>3</sub> + 3.167 N <sub>2</sub> → 5.333 LaN + LaB <sub>6</sub> H <sub>4</sub> C <sub>6</sub> N                                         | -2.1816             |
| LaNH <sub>4</sub> B <sub>6</sub> C <sub>6</sub> | 2.773 LaN + 3 B <sub>13</sub> C <sub>2</sub> + 1.864 La <sub>2</sub> H <sub>5</sub> → 5.5 LaB <sub>6</sub> + 1.773 H <sub>3</sub> N + LaB <sub>6</sub> H <sub>4</sub> C <sub>6</sub> N                     | -2.1774             |
| LaNH <sub>4</sub> B <sub>6</sub> C <sub>6</sub> | 1.71 LaB <sub>6</sub> + 5.258 H <sub>3</sub> N + 2 La <sub>2</sub> C <sub>3</sub> → 4.258 BN + 2.355 La <sub>2</sub> H <sub>5</sub> + LaB <sub>6</sub> H <sub>4</sub> C <sub>6</sub> N                     | -2.1706             |
| LaNH <sub>4</sub> B <sub>6</sub> C <sub>6</sub> | 5.635 LaH <sub>2</sub> + 0.5 N <sub>2</sub> + 3 B <sub>13</sub> C <sub>2</sub> → 4.635 LaB <sub>6</sub> + 1.038 B <sub>5</sub> H <sub>7</sub> + LaB <sub>6</sub> H <sub>4</sub> C <sub>6</sub> N           | -2.1641             |
| LaNH <sub>4</sub> B <sub>6</sub> C <sub>6</sub> | 3 LaC <sub>2</sub> + 18.33 B + 1.333 H <sub>3</sub> N → 2 LaB <sub>6</sub> + 0.3333 BN + LaB <sub>6</sub> H <sub>4</sub> C <sub>6</sub> N                                                                  | -2.1602             |
| LaNH <sub>4</sub> B <sub>6</sub> C <sub>6</sub> | 0.3636 B <sub>9</sub> H <sub>11</sub> + 2 La <sub>2</sub> C <sub>3</sub> + 2.341 N <sub>2</sub> + 0.6818 LaB <sub>4</sub> → 3.682 LaN + LaB <sub>6</sub> H <sub>4</sub> C <sub>6</sub> N                   | -2.1510             |
| LaNH <sub>4</sub> B <sub>6</sub> C <sub>6</sub> | 1.2 H <sub>8</sub> C <sub>5</sub> + 5.748 La + LaN + 0.6667 B <sub>9</sub> H <sub>11</sub> → 1.437 La <sub>4</sub> H <sub>9</sub> + LaB <sub>6</sub> H <sub>4</sub> C <sub>6</sub> N                       | -2.1227             |
| LaNH <sub>4</sub> B <sub>6</sub> C <sub>6</sub> | 23.4 B + BN + 2 La <sub>2</sub> C <sub>3</sub> + 0.8 La <sub>2</sub> H <sub>5</sub> → 4.6 LaB <sub>4</sub> + LaB <sub>6</sub> H <sub>4</sub> C <sub>6</sub> N                                              | -2.1077             |
| LaNH <sub>4</sub> B <sub>6</sub> C <sub>6</sub> | LaN + 5.5 LaH <sub>2</sub> + 3 B <sub>13</sub> C <sub>2</sub> → 3.5 H <sub>2</sub> + 5.5 LaB <sub>6</sub> + LaB <sub>6</sub> H <sub>4</sub> C <sub>6</sub> N                                               | -2.0818             |
| LaNH <sub>4</sub> B <sub>6</sub> C <sub>6</sub> | 1.2 H <sub>8</sub> C <sub>5</sub> + 6.6 La + BN + B <sub>5</sub> H <sub>7</sub> → 1.4 La <sub>4</sub> H <sub>9</sub> + LaB <sub>6</sub> H <sub>4</sub> C <sub>6</sub> N                                    | -2.0800             |
| LaNH <sub>4</sub> B <sub>6</sub> C <sub>6</sub> | 3 LaC <sub>2</sub> + 6 B + 2 LaH <sub>2</sub> + 2.5 N <sub>2</sub> → 4 LaN + LaB <sub>6</sub> H <sub>4</sub> C <sub>6</sub> N                                                                              | -2.0629             |
| LaNH <sub>4</sub> B <sub>6</sub> C <sub>6</sub> | 3 LaC <sub>2</sub> + 20.4 B + 0.5 N <sub>2</sub> + 0.8 La <sub>2</sub> H <sub>5</sub> → 3.6 LaB <sub>4</sub> + LaB <sub>6</sub> H <sub>4</sub> C <sub>6</sub> N                                            | -2.0569             |
| LaNH <sub>4</sub> B <sub>6</sub> C <sub>6</sub> | 2 La <sub>2</sub> C <sub>3</sub> + 1.429 B <sub>5</sub> H <sub>7</sub> + 1.071 N <sub>2</sub> → 1.143 BN + 3 LaH <sub>2</sub> + LaB <sub>6</sub> H <sub>4</sub> C <sub>6</sub> N                           | -2.0516             |
| LaNH <sub>4</sub> B <sub>6</sub> C <sub>6</sub> | 1.625 La <sub>4</sub> H <sub>9</sub> + 0.5 N <sub>2</sub> + 3 B <sub>13</sub> C <sub>2</sub> → 5.312 H <sub>2</sub> + 5.5 LaB <sub>6</sub> + LaB <sub>6</sub> H <sub>4</sub> C <sub>6</sub> N              | -2.0464             |
| LaNH <sub>4</sub> B <sub>6</sub> C <sub>6</sub> | 5.536 LaH <sub>2</sub> + 0.5 N <sub>2</sub> + 3 B <sub>13</sub> C <sub>2</sub> → 4.536 LaB <sub>6</sub> + 0.6429 B <sub>9</sub> H <sub>11</sub> + LaB <sub>6</sub> H <sub>4</sub> C <sub>6</sub> N         | -2.0414             |
| LaNH <sub>4</sub> B <sub>6</sub> C <sub>6</sub> | 17.29 B + H <sub>3</sub> N + 2 La <sub>2</sub> C <sub>3</sub> + 0.1429 B <sub>5</sub> H <sub>7</sub> → 3 LaB <sub>4</sub> + LaB <sub>6</sub> H <sub>4</sub> C <sub>6</sub> N                               | -2.0329             |
| LaNH <sub>4</sub> B <sub>6</sub> C <sub>6</sub> | BN + 8.167 La <sub>4</sub> H <sub>9</sub> + 3 B <sub>13</sub> C <sub>2</sub> → 23.17 LaH <sub>3</sub> + 8.5 LaB <sub>4</sub> + LaB <sub>6</sub> H <sub>4</sub> C <sub>6</sub> N                            | -2.0207             |
| LaNH <sub>4</sub> B <sub>6</sub> C <sub>6</sub> | 17.18 B + H <sub>3</sub> N + 0.09091 B <sub>9</sub> H <sub>11</sub> + 2 La <sub>2</sub> C <sub>3</sub> → 3 LaB <sub>4</sub> + LaB <sub>6</sub> H <sub>4</sub> C <sub>6</sub> N                             | -2.0174             |
| LaNH <sub>4</sub> B <sub>6</sub> C <sub>6</sub> | LaN + 3.333 B <sub>9</sub> H <sub>11</sub> + 2 La <sub>2</sub> C <sub>3</sub> → 16.33 H <sub>2</sub> + 4 LaB <sub>6</sub> + LaB <sub>6</sub> H <sub>4</sub> C <sub>6</sub> N                               | -2.0130             |
| LaNH <sub>4</sub> B <sub>6</sub> C <sub>6</sub> | 2.667 B <sub>9</sub> H <sub>11</sub> + 2 La <sub>2</sub> C <sub>3</sub> + 0.5 N <sub>2</sub> → 12.67 H <sub>2</sub> + 3 LaB <sub>6</sub> + LaB <sub>6</sub> H <sub>4</sub> C <sub>6</sub> N                | -1.9423             |
| LaNH <sub>4</sub> B <sub>6</sub> C <sub>6</sub> | 1.692 La <sub>2</sub> C <sub>3</sub> + 2.492 N <sub>2</sub> + 0.4615 B <sub>13</sub> C <sub>2</sub> + 0.8 La <sub>2</sub> H <sub>5</sub> → 3.985 LaN + LaB <sub>6</sub> H <sub>4</sub> C <sub>6</sub> N    | -1.9337             |
| LaNH <sub>4</sub> B <sub>6</sub> C <sub>6</sub> | 3.417 LaH <sub>3</sub> + 3.083 LaN + 3 B <sub>13</sub> C <sub>2</sub> → 5.5 LaB <sub>6</sub> + 2.083 H <sub>3</sub> N + LaB <sub>6</sub> H <sub>4</sub> C <sub>6</sub> N                                   | -1.9093             |
| LaNH <sub>4</sub> B <sub>6</sub> C <sub>6</sub> | 1.2 H <sub>8</sub> C <sub>5</sub> + 6.856 La + BN + 0.5556 B <sub>9</sub> H <sub>11</sub> → 5.856 LaH <sub>2</sub> + LaB <sub>6</sub> H <sub>4</sub> C <sub>6</sub> N                                      | -1.8992             |
| LaNH <sub>4</sub> B <sub>6</sub> C <sub>6</sub> | 2.75 B <sub>9</sub> H <sub>11</sub> + 2 La <sub>2</sub> C <sub>3</sub> + 2 N <sub>2</sub> → 3 LaN + 3.75 B <sub>5</sub> H <sub>7</sub> + LaB <sub>6</sub> H <sub>4</sub> C <sub>6</sub> N                  | -1.8712             |
| LaNH <sub>4</sub> B <sub>6</sub> C <sub>6</sub> | 3 LaC <sub>2</sub> + 1.333 LaH <sub>3</sub> + 23.33 B + LaN → 4.333 LaB <sub>4</sub> + LaB <sub>6</sub> H <sub>4</sub> C <sub>6</sub> N                                                                    | -1.8516             |
| LaNH <sub>4</sub> B <sub>6</sub> C <sub>6</sub> | 5 H <sub>3</sub> N + 2 La <sub>2</sub> C <sub>3</sub> + 2.5 LaB <sub>4</sub> → 4 BN + 5.5 LaH <sub>2</sub> + LaB <sub>6</sub> H <sub>4</sub> C <sub>6</sub> N                                              | -1.8451             |
| LaNH <sub>4</sub> B <sub>6</sub> C <sub>6</sub> | 6 C + 4.7 La + H <sub>3</sub> N + 1.2 B <sub>5</sub> H <sub>7</sub> → 3.7 LaH <sub>2</sub> + LaB <sub>6</sub> H <sub>4</sub> C <sub>6</sub> N                                                              | -1.8424             |
| LaNH <sub>4</sub> B <sub>6</sub> C <sub>6</sub> | H <sub>3</sub> N + 20.38 B <sub>9</sub> H <sub>11</sub> + 2 La <sub>2</sub> C <sub>3</sub> → 3 LaB <sub>6</sub> + 31.88 B <sub>5</sub> H <sub>7</sub> + LaB <sub>6</sub> H <sub>4</sub> C <sub>6</sub> N   | -1.8158             |
| LaNH <sub>4</sub> B <sub>6</sub> C <sub>6</sub> | LaN + 2 La <sub>2</sub> C <sub>3</sub> + 6 B <sub>5</sub> H <sub>7</sub> → 19 H <sub>2</sub> + 4 LaB <sub>6</sub> + LaB <sub>6</sub> H <sub>4</sub> C <sub>6</sub> N                                       | -1.7876             |
| LaNH <sub>4</sub> B <sub>6</sub> C <sub>6</sub> | 3 LaC <sub>2</sub> + 2 LaH <sub>2</sub> + 3.25 N <sub>2</sub> + 1.5 LaB <sub>4</sub> → 5.5 LaN + LaB <sub>6</sub> H <sub>4</sub> C <sub>6</sub> N                                                          | -1.7794             |
| LaNH <sub>4</sub> B <sub>6</sub> C <sub>6</sub> | LaN + 3 B <sub>13</sub> C <sub>2</sub> + 20.75 La <sub>2</sub> H <sub>5</sub> → 33.25 LaH <sub>3</sub> + 8.25 LaB <sub>4</sub> + LaB <sub>6</sub> H <sub>4</sub> C <sub>6</sub> N                          | -1.7753             |
| LaNH <sub>4</sub> B <sub>6</sub> C <sub>6</sub> | 6.5 H <sub>2</sub> + 6 B + 2 La <sub>2</sub> C <sub>3</sub> + 0.5 N <sub>2</sub> → 3 LaH <sub>3</sub> + LaB <sub>6</sub> H <sub>4</sub> C <sub>6</sub> N                                                   | -1.7650             |
| LaNH <sub>4</sub> B <sub>6</sub> C <sub>6</sub> | 2 La <sub>2</sub> C <sub>3</sub> + 4.8 B <sub>5</sub> H <sub>7</sub> + 0.5 N <sub>2</sub> → 14.8 H <sub>2</sub> + 3 LaB <sub>6</sub> + LaB <sub>6</sub> H <sub>4</sub> C <sub>6</sub> N                    | -1.7620             |
| LaNH <sub>4</sub> B <sub>6</sub> C <sub>6</sub> | 3 LaC <sub>2</sub> + 0.5 H <sub>2</sub> + 18 B + H <sub>3</sub> N → 2 LaB <sub>6</sub> + LaB <sub>6</sub> H <sub>4</sub> C <sub>6</sub> N                                                                  | -1.7459             |
| LaNH <sub>4</sub> B <sub>6</sub> C <sub>6</sub> | 18 B + 1.333 H <sub>3</sub> N + 2 La <sub>2</sub> C <sub>3</sub> → 0.1667 N <sub>2</sub> + 3 LaB <sub>4</sub> + LaB <sub>6</sub> H <sub>4</sub> C <sub>6</sub> N                                           | -1.7409             |
| LaNH <sub>4</sub> B <sub>6</sub> C <sub>6</sub> | 0.6667 B <sub>9</sub> H <sub>11</sub> + 2 La <sub>2</sub> C <sub>3</sub> + 2 N <sub>2</sub> → 1.667 H <sub>2</sub> + 3 LaN + LaB <sub>6</sub> H <sub>4</sub> C <sub>6</sub> N                              | -1.7304             |
| LaNH <sub>4</sub> B <sub>6</sub> C <sub>6</sub> | 1.333 LaH <sub>3</sub> + 22.33 B + BN + 2 La <sub>2</sub> C <sub>3</sub> → 4.333 LaB <sub>4</sub> + LaB <sub>6</sub> H <sub>4</sub> C <sub>6</sub> N                                                       | -1.7134             |
| LaNH <sub>4</sub> B <sub>6</sub> C <sub>6</sub> | 0.4545 LaB <sub>6</sub> + 0.3636 B <sub>9</sub> H <sub>11</sub> + 2 La <sub>2</sub> C <sub>3</sub> + 2.227 N <sub>2</sub> → 3.455 LaN + LaB <sub>6</sub> H <sub>4</sub> C <sub>6</sub> N                   | -1.6982             |
| LaNH <sub>4</sub> B <sub>6</sub> C <sub>6</sub> | 2 La <sub>2</sub> C <sub>3</sub> + 1.2 B <sub>5</sub> H <sub>7</sub> + 2 N <sub>2</sub> → 2.2 H <sub>2</sub> + 3 LaN + LaB <sub>6</sub> H <sub>4</sub> C <sub>6</sub> N                                    | -1.6853             |
| LaNH <sub>4</sub> B <sub>6</sub> C <sub>6</sub> | 16.67 B + 1.333 H <sub>3</sub> N + 2 La <sub>2</sub> C <sub>3</sub> → 0.3333 LaN + 2.667 LaB <sub>4</sub> + LaB <sub>6</sub> H <sub>4</sub> C <sub>6</sub> N                                               | -1.6779             |
| LaNH <sub>4</sub> B <sub>6</sub> C <sub>6</sub> | 0.5238 LaB <sub>6</sub> + 2 La <sub>2</sub> C <sub>3</sub> + 0.5714 B <sub>5</sub> H <sub>7</sub> + 2.262 N <sub>2</sub> → 3.524 LaN + LaB <sub>6</sub> H <sub>4</sub> C <sub>6</sub> N                    | -1.6719             |
| LaNH <sub>4</sub> B <sub>6</sub> C <sub>6</sub> | 3 LaC <sub>2</sub> + 6 B + 0.4444 La <sub>4</sub> H <sub>9</sub> + 2.389 N <sub>2</sub> → 3.778 LaN + LaB <sub>6</sub> H <sub>4</sub> C <sub>6</sub> N                                                     | -1.6685             |
| LaNH <sub>4</sub> B <sub>6</sub> C <sub>6</sub> | 3 LaC <sub>2</sub> + 1.333 LaH <sub>3</sub> + 19.33 B + 0.5 N <sub>2</sub> → 3.333 LaB <sub>4</sub> + LaB <sub>6</sub> H <sub>4</sub> C <sub>6</sub> N                                                     | -1.6626             |
| LaNH <sub>4</sub> B <sub>6</sub> C <sub>6</sub> | 2 H <sub>2</sub> + LaB <sub>6</sub> + 2 La <sub>2</sub> C <sub>3</sub> + 2.5 N <sub>2</sub> → 4 LaN + LaB <sub>6</sub> H <sub>4</sub> C <sub>6</sub> N                                                     | -1.6597             |
| LaNH <sub>4</sub> B <sub>6</sub> C <sub>6</sub> | 3 LaC <sub>2</sub> + 17.29 B + H <sub>3</sub> N + 0.1429 B <sub>5</sub> H <sub>7</sub> → 2 LaB <sub>6</sub> + LaB <sub>6</sub> H <sub>4</sub> C <sub>6</sub> N                                             | -1.5966             |
| LaNH <sub>4</sub> B <sub>6</sub> C <sub>6</sub> | 1.333 LaH <sub>3</sub> + 1.692 La <sub>2</sub> C <sub>3</sub> + 2.359 N <sub>2</sub> + 0.4615 B <sub>13</sub> C <sub>2</sub> → 3.718 LaN + LaB <sub>6</sub> H <sub>4</sub> C <sub>6</sub> N                | -1.5899             |
| LaNH <sub>4</sub> B <sub>6</sub> C <sub>6</sub> | 3 LaC <sub>2</sub> + 17.18 B + H <sub>3</sub> N + 0.09091 B <sub>9</sub> H <sub>11</sub> → 2 LaB <sub>6</sub> + LaB <sub>6</sub> H <sub>4</sub> C <sub>6</sub> N                                           | -1.5811             |
| LaNH <sub>4</sub> B <sub>6</sub> C <sub>6</sub> | LaN + 4.827 LaH <sub>2</sub> + 3 B <sub>13</sub> C <sub>2</sub> → 4.827 LaB <sub>6</sub> + 0.8077 B <sub>5</sub> H <sub>7</sub> + LaB <sub>6</sub> H <sub>4</sub> C <sub>6</sub> N                         | -1.5422             |
| LaNH <sub>4</sub> B <sub>6</sub> C <sub>6</sub> | 1.2 H <sub>8</sub> C <sub>5</sub> + 5.173 La + LaN + 0.6667 B <sub>9</sub> H <sub>11</sub> → 2.587 La <sub>2</sub> H <sub>5</sub> + LaB <sub>6</sub> H <sub>4</sub> C <sub>6</sub> N                       | -1.5393             |
| LaNH <sub>4</sub> B <sub>6</sub> C <sub>6</sub> | H <sub>3</sub> N + 6.5 LaH <sub>2</sub> + 3 B <sub>13</sub> C <sub>2</sub> → 6 H <sub>2</sub> + 5.5 LaB <sub>6</sub> + LaB <sub>6</sub> H <sub>4</sub> C <sub>6</sub> N                                    | -1.5338             |

Continued on next page

Continued

| Compound                                        | Chemical reaction                                                                                                                                                                              | Reaction energy(eV) |
|-------------------------------------------------|------------------------------------------------------------------------------------------------------------------------------------------------------------------------------------------------|---------------------|
| LaNH <sub>4</sub> B <sub>6</sub> C <sub>6</sub> | $1.2 \text{ H}_8\text{C}_5 + 6.04 \text{ La} + \text{BN} + \text{B}_5\text{H}_7 \rightarrow 2.52 \text{ La}_2\text{H}_5 + \text{LaB}_6\text{H}_4\text{C}_6\text{N}$                            | -1.5116             |
| LaNH <sub>4</sub> B <sub>6</sub> C <sub>6</sub> | $6 \text{ C} + 4.289 \text{ La} + \text{H}_3\text{N} + 1.2 \text{ B}_5\text{H}_7 \rightarrow 0.8222 \text{ La}_4\text{H}_9 + \text{LaB}_6\text{H}_4\text{C}_6\text{N}$                         | -1.4796             |
| LaNH <sub>4</sub> B <sub>6</sub> C <sub>6</sub> | $\text{LaN} + 4.75 \text{ LaH}_2 + 3 \text{ B}_{13}\text{C}_2 \rightarrow 4.75 \text{ LaB}_6 + 0.5 \text{ B}_9\text{H}_{11} + \text{LaB}_6\text{H}_4\text{C}_6\text{N}$                        | -1.4467             |
| LaNH <sub>4</sub> B <sub>6</sub> C <sub>6</sub> | $3 \text{ LaC}_2 + 0.8182 \text{ B}_9\text{H}_{11} + 1.182 \text{ N}_2 \rightarrow 1.364 \text{ BN} + \text{La}_2\text{H}_5 + \text{LaB}_6\text{H}_4\text{C}_6\text{N}$                        | -1.4450             |
| LaNH <sub>4</sub> B <sub>6</sub> C <sub>6</sub> | $0.3636 \text{ B}_9\text{H}_{11} + 1.86 \text{ La}_2\text{C}_3 + 1.86 \text{ N}_2 + 0.2098 \text{ B}_{13}\text{C}_2 \rightarrow 2.72 \text{ LaN} + \text{LaB}_6\text{H}_4\text{C}_6\text{N}$   | -1.4293             |
| LaNH <sub>4</sub> B <sub>6</sub> C <sub>6</sub> | $1.375 \text{ La}_4\text{H}_9 + \text{LaN} + 3 \text{ B}_{13}\text{C}_2 \rightarrow 4.188 \text{ H}_2 + 5.5 \text{ LaB}_6 + \text{LaB}_6\text{H}_4\text{C}_6\text{N}$                          | -1.3952             |
| LaNH <sub>4</sub> B <sub>6</sub> C <sub>6</sub> | $3 \text{ LaC}_2 + 0.4444 \text{ La}_4\text{H}_9 + 3.139 \text{ N}_2 + 1.5 \text{ LaB}_4 \rightarrow 5.278 \text{ LaN} + \text{LaB}_6\text{H}_4\text{C}_6\text{N}$                             | -1.3850             |
| LaNH <sub>4</sub> B <sub>6</sub> C <sub>6</sub> | $3 \text{ LaC}_2 + 6 \text{ B} + 2.3 \text{ N}_2 + 0.8 \text{ La}_2\text{H}_5 \rightarrow 3.6 \text{ LaN} + \text{LaB}_6\text{H}_4\text{C}_6\text{N}$                                          | -1.3765             |
| LaNH <sub>4</sub> B <sub>6</sub> C <sub>6</sub> | $8 \text{ H}_2 + 6 \text{ B} + \text{LaN} + 2 \text{ La}_2\text{C}_3 \rightarrow 4 \text{ LaH}_3 + \text{LaB}_6\text{H}_4\text{C}_6\text{N}$                                                   | -1.3736             |
| LaNH <sub>4</sub> B <sub>6</sub> C <sub>6</sub> | $1.376 \text{ La}_4\text{H}_9 + 0.5 \text{ N}_2 + 3 \text{ B}_{13}\text{C}_2 \rightarrow 4.502 \text{ LaB}_6 + 1.197 \text{ B}_5\text{H}_7 + \text{LaB}_6\text{H}_4\text{C}_6\text{N}$         | -1.3712             |
| LaNH <sub>4</sub> B <sub>6</sub> C <sub>6</sub> | $1.839 \text{ La}_2\text{C}_3 + 0.5714 \text{ B}_5\text{H}_7 + 1.839 \text{ N}_2 + 0.2418 \text{ B}_{13}\text{C}_2 \rightarrow 2.678 \text{ LaN} + \text{LaB}_6\text{H}_4\text{C}_6\text{N}$   | -1.3619             |
| LaNH <sub>4</sub> B <sub>6</sub> C <sub>6</sub> | $3 \text{ LaC}_2 + 5.105 \text{ H}_3\text{N} + 2.526 \text{ LaB}_4 \rightarrow 4.105 \text{ BN} + 2.263 \text{ La}_2\text{H}_5 + \text{LaB}_6\text{H}_4\text{C}_6\text{N}$                     | -1.3616             |
| LaNH <sub>4</sub> B <sub>6</sub> C <sub>6</sub> | $0.5 \text{ N}_2 + 3 \text{ B}_{13}\text{C}_2 + 3.25 \text{ La}_2\text{H}_5 \rightarrow 6.125 \text{ H}_2 + 5.5 \text{ LaB}_6 + \text{LaB}_6\text{H}_4\text{C}_6\text{N}$                      | -1.3305             |
| LaNH <sub>4</sub> B <sub>6</sub> C <sub>6</sub> | $1.2 \text{ H}_8\text{C}_5 + 6.205 \text{ La} + \text{BN} + 0.5556 \text{ B}_9\text{H}_{11} \rightarrow 1.301 \text{ La}_4\text{H}_9 + \text{LaB}_6\text{H}_4\text{C}_6\text{N}$               | -1.3250             |
| LaNH <sub>4</sub> B <sub>6</sub> C <sub>6</sub> | $5.75 \text{ H}_2 + 6 \text{ B} + 2 \text{ La}_2\text{C}_3 + 0.5 \text{ N}_2 \rightarrow 1.5 \text{ La}_2\text{H}_5 + \text{LaB}_6\text{H}_4\text{C}_6\text{N}$                                | -1.3160             |
| LaNH <sub>4</sub> B <sub>6</sub> C <sub>6</sub> | $3 \text{ LaC}_2 + 18 \text{ B} + 1.333 \text{ H}_3\text{N} \rightarrow 2 \text{ LaB}_6 + 0.1667 \text{ N}_2 + \text{LaB}_6\text{H}_4\text{C}_6\text{N}$                                       | -1.3046             |
| LaNH <sub>4</sub> B <sub>6</sub> C <sub>6</sub> | $3 \text{ LaC}_2 + 8.333 \text{ B} + 3.333 \text{ H}_3\text{N} \rightarrow 2 \text{ LaH}_3 + 2.333 \text{ BN} + \text{LaB}_6\text{H}_4\text{C}_6\text{N}$                                      | -1.3034             |
| LaNH <sub>4</sub> B <sub>6</sub> C <sub>6</sub> | $0.6667 \text{ B}_9\text{H}_{11} + 2 \text{ La}_2\text{C}_3 + 1.444 \text{ N}_2 \rightarrow 1.111 \text{ LaH}_3 + 1.889 \text{ LaN} + \text{LaB}_6\text{H}_4\text{C}_6\text{N}$                | -1.2954             |
| LaNH <sub>4</sub> B <sub>6</sub> C <sub>6</sub> | $0.5 \text{ H}_8\text{C}_5 + 20 \text{ B} + \text{LaN} + 1.167 \text{ La}_2\text{C}_3 \rightarrow 2.333 \text{ LaB}_6 + \text{LaB}_6\text{H}_4\text{C}_6\text{N}$                              | -1.2838             |
| LaNH <sub>4</sub> B <sub>6</sub> C <sub>6</sub> | $6 \text{ C} + \text{LaB}_6 + 0.3636 \text{ B}_9\text{H}_{11} + 2.136 \text{ N}_2 \rightarrow 3.273 \text{ BN} + \text{LaB}_6\text{H}_4\text{C}_6\text{N}$                                     | -1.2637             |
| LaNH <sub>4</sub> B <sub>6</sub> C <sub>6</sub> | $1.348 \text{ La}_4\text{H}_9 + 0.5 \text{ N}_2 + 3 \text{ B}_{13}\text{C}_2 \rightarrow 4.391 \text{ LaB}_6 + 0.7391 \text{ B}_9\text{H}_{11} + \text{LaB}_6\text{H}_4\text{C}_6\text{N}$     | -1.2461             |
| LaNH <sub>4</sub> B <sub>6</sub> C <sub>6</sub> | $1.635 \text{ LaB}_6 + 4.81 \text{ H}_3\text{N} + 2 \text{ La}_2\text{C}_3 \rightarrow 3.81 \text{ BN} + 1.159 \text{ La}_4\text{H}_9 + \text{LaB}_6\text{H}_4\text{C}_6\text{N}$              | -1.2388             |
| LaNH <sub>4</sub> B <sub>6</sub> C <sub>6</sub> | $1.2 \text{ H}_8\text{C}_5 + 6 \text{ B} + 5.3 \text{ La} + \text{H}_3\text{N} \rightarrow 4.3 \text{ LaH}_2 + \text{LaB}_6\text{H}_4\text{C}_6\text{N}$                                       | -1.2229             |
| LaNH <sub>4</sub> B <sub>6</sub> C <sub>6</sub> | $3.465 \text{ H}_3\text{N} + 1.566 \text{ La}_2\text{C}_3 + 0.6512 \text{ B}_{13}\text{C}_2 \rightarrow 2.132 \text{ LaH}_3 + 2.465 \text{ BN} + \text{LaB}_6\text{H}_4\text{C}_6\text{N}$     | -1.2040             |
| LaNH <sub>4</sub> B <sub>6</sub> C <sub>6</sub> | $3 \text{ LaC}_2 + 1.2 \text{ B}_5\text{H}_7 + 2.233 \text{ N}_2 \rightarrow 1.467 \text{ H}_3\text{N} + 2 \text{ LaN} + \text{LaB}_6\text{H}_4\text{C}_6\text{N}$                             | -1.1987             |
| LaNH <sub>4</sub> B <sub>6</sub> C <sub>6</sub> | $6 \text{ B} + 1.333 \text{ H}_3\text{N} + 2 \text{ La}_2\text{C}_3 + 1.333 \text{ N}_2 \rightarrow 3 \text{ LaN} + \text{LaB}_6\text{H}_4\text{C}_6\text{N}$                                  | -1.1739             |
| LaNH <sub>4</sub> B <sub>6</sub> C <sub>6</sub> | $3 \text{ LaC}_2 + 1.429 \text{ B}_5\text{H}_7 + 1.071 \text{ N}_2 \rightarrow 2 \text{ LaH}_3 + 1.143 \text{ BN} + \text{LaB}_6\text{H}_4\text{C}_6\text{N}$                                  | -1.1684             |
| LaNH <sub>4</sub> B <sub>6</sub> C <sub>6</sub> | $6 \text{ C} + 3.96 \text{ La} + \text{H}_3\text{N} + 1.2 \text{ B}_5\text{H}_7 \rightarrow 1.48 \text{ La}_2\text{H}_5 + \text{LaB}_6\text{H}_4\text{C}_6\text{N}$                            | -1.1458             |
| LaNH <sub>4</sub> B <sub>6</sub> C <sub>6</sub> | $1.2 \text{ H}_8\text{C}_5 + 4.667 \text{ La} + \text{LaN} + 1.2 \text{ B}_5\text{H}_7 \rightarrow 4.667 \text{ LaH}_3 + \text{LaB}_6\text{H}_4\text{C}_6\text{N}$                             | -1.1204             |
| LaNH <sub>4</sub> B <sub>6</sub> C <sub>6</sub> | $2 \text{ La}_2\text{C}_3 + 1.2 \text{ B}_5\text{H}_7 + 1.267 \text{ N}_2 \rightarrow 1.467 \text{ LaH}_3 + 1.533 \text{ LaN} + \text{LaB}_6\text{H}_4\text{C}_6\text{N}$                      | -1.1112             |
| LaNH <sub>4</sub> B <sub>6</sub> C <sub>6</sub> | $3 \text{ LaC}_2 + 3.05 \text{ N}_2 + 0.8 \text{ La}_2\text{H}_5 + 1.5 \text{ LaB}_4 \rightarrow 5.1 \text{ LaN} + \text{LaB}_6\text{H}_4\text{C}_6\text{N}$                                   | -1.0930             |
| LaNH <sub>4</sub> B <sub>6</sub> C <sub>6</sub> | $3 \text{ LaC}_2 + 2 \text{ H}_2 + 18 \text{ B} + \text{LaN} \rightarrow 3 \text{ LaB}_4 + \text{LaB}_6\text{H}_4\text{C}_6\text{N}$                                                           | -1.0777             |
| LaNH <sub>4</sub> B <sub>6</sub> C <sub>6</sub> | $2 \text{ H}_2 + 1.692 \text{ La}_2\text{C}_3 + 1.692 \text{ N}_2 + 0.4615 \text{ B}_{13}\text{C}_2 \rightarrow 2.385 \text{ LaN} + \text{LaB}_6\text{H}_4\text{C}_6\text{N}$                  | -1.0680             |
| LaNH <sub>4</sub> B <sub>6</sub> C <sub>6</sub> | $3 \text{ LaC}_2 + 1.333 \text{ LaH}_3 + 6 \text{ B} + 2.167 \text{ N}_2 \rightarrow 3.333 \text{ LaN} + \text{LaB}_6\text{H}_4\text{C}_6\text{N}$                                             | -1.0327             |
| LaNH <sub>4</sub> B <sub>6</sub> C <sub>6</sub> | $0.8571 \text{ La}_2\text{C}_3 + 2 \text{ LaH}_2 + 0.5 \text{ N}_2 + 1.714 \text{ B}_{13}\text{C}_2 \rightarrow 2.714 \text{ LaB}_6 + \text{LaB}_6\text{H}_4\text{C}_6\text{N}$                | -1.0139             |
| LaNH <sub>4</sub> B <sub>6</sub> C <sub>6</sub> | $0.6667 \text{ B}_9\text{H}_{11} + 2 \text{ La}_2\text{C}_3 + 1.333 \text{ N}_2 \rightarrow 1.667 \text{ LaN} + 0.6667 \text{ La}_2\text{H}_5 + \text{LaB}_6\text{H}_4\text{C}_6\text{N}$      | -1.0089             |
| LaNH <sub>4</sub> B <sub>6</sub> C <sub>6</sub> | $1.355 \text{ B}_9\text{H}_{11} + 2.318 \text{ La}_2\text{C}_3 + 0.5 \text{ N}_2 \rightarrow 3.636 \text{ LaH}_3 + 0.4766 \text{ B}_{13}\text{C}_2 + \text{LaB}_6\text{H}_4\text{C}_6\text{N}$ | -0.9914             |
| LaNH <sub>4</sub> B <sub>6</sub> C <sub>6</sub> | $5.375 \text{ H}_2 + 6 \text{ B} + 2 \text{ La}_2\text{C}_3 + 0.5 \text{ N}_2 \rightarrow 0.75 \text{ La}_4\text{H}_9 + \text{LaB}_6\text{H}_4\text{C}_6\text{N}$                              | -0.9856             |
| LaNH <sub>4</sub> B <sub>6</sub> C <sub>6</sub> | $0.125 \text{ H}_8\text{C}_5 + 16.33 \text{ B} + \text{H}_3\text{N} + 1.792 \text{ La}_2\text{C}_3 \rightarrow 2.583 \text{ LaB}_4 + \text{LaB}_6\text{H}_4\text{C}_6\text{N}$                 | -0.9432             |
| LaNH <sub>4</sub> B <sub>6</sub> C <sub>6</sub> | $2 \text{ H}_2 + 17 \text{ B} + \text{BN} + 2 \text{ La}_2\text{C}_3 \rightarrow 3 \text{ LaB}_4 + \text{LaB}_6\text{H}_4\text{C}_6\text{N}$                                                   | -0.9395             |
| LaNH <sub>4</sub> B <sub>6</sub> C <sub>6</sub> | $8.75 \text{ H}_2 + 2 \text{ La}_2\text{C}_3 + 0.5 \text{ N}_2 + 1.5 \text{ LaB}_4 \rightarrow 4.5 \text{ LaH}_3 + \text{LaB}_6\text{H}_4\text{C}_6\text{N}$                                   | -0.8944             |
| LaNH <sub>4</sub> B <sub>6</sub> C <sub>6</sub> | $1.333 \text{ H}_3\text{N} + 2 \text{ La}_2\text{C}_3 + 2.083 \text{ N}_2 + 1.5 \text{ LaB}_4 \rightarrow 4.5 \text{ LaN} + \text{LaB}_6\text{H}_4\text{C}_6\text{N}$                          | -0.8904             |
| LaNH <sub>4</sub> B <sub>6</sub> C <sub>6</sub> | $3 \text{ LaC}_2 + 2 \text{ H}_2 + 14 \text{ B} + 0.5 \text{ N}_2 \rightarrow 2 \text{ LaB}_4 + \text{LaB}_6\text{H}_4\text{C}_6\text{N}$                                                      | -0.8888             |
| LaNH <sub>4</sub> B <sub>6</sub> C <sub>6</sub> | $6 \text{ C} + 4.167 \text{ La} + \text{H}_3\text{N} + 0.6667 \text{ B}_9\text{H}_{11} \rightarrow 3.167 \text{ LaH}_2 + \text{LaB}_6\text{H}_4\text{C}_6\text{N}$                             | -0.8841             |
| LaNH <sub>4</sub> B <sub>6</sub> C <sub>6</sub> | $3 \text{ LaC}_2 + 16 \text{ B} + 1.333 \text{ H}_3\text{N} \rightarrow 1.667 \text{ LaB}_6 + 0.3333 \text{ LaN} + \text{LaB}_6\text{H}_4\text{C}_6\text{N}$                                   | -0.8780             |
| LaNH <sub>4</sub> B <sub>6</sub> C <sub>6</sub> | $\text{BN} + 3 \text{ B}_{13}\text{C}_2 + 24.5 \text{ La}_2\text{H}_5 \rightarrow 39.5 \text{ LaH}_3 + 8.5 \text{ LaB}_4 + \text{LaB}_6\text{H}_4\text{C}_6\text{N}$                           | -0.8676             |
| LaNH <sub>4</sub> B <sub>6</sub> C <sub>6</sub> | $1.178 \text{ La}_4\text{H}_9 + \text{LaN} + 3 \text{ B}_{13}\text{C}_2 \rightarrow 4.714 \text{ LaB}_6 + 0.9437 \text{ B}_5\text{H}_7 + \text{LaB}_6\text{H}_4\text{C}_6\text{N}$             | -0.8629             |
| LaNH <sub>4</sub> B <sub>6</sub> C <sub>6</sub> | $\text{LaN} + 1.72 \text{ B}_9\text{H}_{11} + 2.486 \text{ La}_2\text{C}_3 \rightarrow 4.972 \text{ LaH}_3 + 0.729 \text{ B}_{13}\text{C}_2 + \text{LaB}_6\text{H}_4\text{C}_6\text{N}$        | -0.8304             |
| LaNH <sub>4</sub> B <sub>6</sub> C <sub>6</sub> | $6 \text{ C} + 5 \text{ LaN} + 2 \text{ B}_5\text{H}_7 \rightarrow 4 \text{ BN} + 2 \text{ La}_2\text{H}_5 + \text{LaB}_6\text{H}_4\text{C}_6\text{N}$                                         | -0.8150             |
| LaNH <sub>4</sub> B <sub>6</sub> C <sub>6</sub> | $1.032 \text{ B}_9\text{H}_{11} + 2 \text{ La}_2\text{C}_3 + 0.5 \text{ N}_2 \rightarrow 2.452 \text{ LaH}_3 + 0.5484 \text{ LaB}_6 + \text{LaB}_6\text{H}_4\text{C}_6\text{N}$                | -0.8095             |
| LaNH <sub>4</sub> B <sub>6</sub> C <sub>6</sub> | $1.2 \text{ H}_8\text{C}_5 + 6 \text{ B} + 4.822 \text{ La} + \text{H}_3\text{N} \rightarrow 0.9556 \text{ La}_4\text{H}_9 + \text{LaB}_6\text{H}_4\text{C}_6\text{N}$                         | -0.8013             |
| LaNH <sub>4</sub> B <sub>6</sub> C <sub>6</sub> | $1.2 \text{ H}_8\text{C}_5 + 5.684 \text{ La} + \text{BN} + 0.5556 \text{ B}_9\text{H}_{11} \rightarrow 2.342 \text{ La}_2\text{H}_5 + \text{LaB}_6\text{H}_4\text{C}_6\text{N}$               | -0.7967             |
| LaNH <sub>4</sub> B <sub>6</sub> C <sub>6</sub> | $\text{LaN} + 3 \text{ B}_{13}\text{C}_2 + 2.75 \text{ La}_2\text{H}_5 \rightarrow 4.875 \text{ H}_2 + 5.5 \text{ LaB}_6 + \text{LaB}_6\text{H}_4\text{C}_6\text{N}$                           | -0.7894             |
| LaNH <sub>4</sub> B <sub>6</sub> C <sub>6</sub> | $3 \text{ LaC}_2 + \text{LaB}_6 + 2 \text{ LaH}_2 + 3 \text{ N}_2 \rightarrow 5 \text{ LaN} + \text{LaB}_6\text{H}_4\text{C}_6\text{N}$                                                        | -0.7833             |
| LaNH <sub>4</sub> B <sub>6</sub> C <sub>6</sub> | $2.216 \text{ La}_2\text{C}_3 + 2.042 \text{ B}_5\text{H}_7 + 0.5 \text{ N}_2 \rightarrow 3.432 \text{ LaH}_3 + 0.3239 \text{ B}_{13}\text{C}_2 + \text{LaB}_6\text{H}_4\text{C}_6\text{N}$    | -0.7752             |
| LaNH <sub>4</sub> B <sub>6</sub> C <sub>6</sub> | $7 \text{ H}_2 + 6 \text{ B} + \text{LaN} + 2 \text{ La}_2\text{C}_3 \rightarrow 2 \text{ La}_2\text{H}_5 + \text{LaB}_6\text{H}_4\text{C}_6\text{N}$                                          | -0.7749             |
| LaNH <sub>4</sub> B <sub>6</sub> C <sub>6</sub> | $3 \text{ LaC}_2 + 0.6667 \text{ B}_9\text{H}_{11} + 2.056 \text{ N}_2 \rightarrow 1.111 \text{ H}_3\text{N} + 2 \text{ LaN} + \text{LaB}_6\text{H}_4\text{C}_6\text{N}$                       | -0.7730             |
| LaNH <sub>4</sub> B <sub>6</sub> C <sub>6</sub> | $0.6667 \text{ B}_9\text{H}_{11} + 2 \text{ La}_2\text{C}_3 + 1.259 \text{ N}_2 \rightarrow 0.3704 \text{ La}_4\text{H}_9 + 1.519 \text{ LaN} + \text{LaB}_6\text{H}_4\text{C}_6\text{N}$      | -0.7656             |
| LaNH <sub>4</sub> B <sub>6</sub> C <sub>6</sub> | $1.157 \text{ La}_4\text{H}_9 + \text{LaN} + 3 \text{ B}_{13}\text{C}_2 \rightarrow 4.626 \text{ LaB}_6 + 0.5826 \text{ B}_9\text{H}_{11} + \text{LaB}_6\text{H}_4\text{C}_6\text{N}$          | -0.7643             |
| LaNH <sub>4</sub> B <sub>6</sub> C <sub>6</sub> | $3 \text{ LaC}_2 + 1.333 \text{ LaH}_3 + 2.917 \text{ N}_2 + 1.5 \text{ LaB}_4 \rightarrow 4.833 \text{ LaN} + \text{LaB}_6\text{H}_4\text{C}_6\text{N}$                                       | -0.7492             |

Continued on next page

Continued

| Compound                                        | Chemical reaction                                                                                                                                                                                  | Reaction energy(eV) |
|-------------------------------------------------|----------------------------------------------------------------------------------------------------------------------------------------------------------------------------------------------------|---------------------|
| LaNH <sub>4</sub> B <sub>6</sub> C <sub>6</sub> | $2 \text{La}_2\text{C}_3 + 1.2 \text{B}_5\text{H}_7 + 1.12 \text{N}_2 \rightarrow 1.24 \text{LaN} + 0.88 \text{La}_2\text{H}_5 + \text{LaB}_6\text{H}_4\text{C}_6\text{N}$                         | -0.7329             |
| LaNH <sub>4</sub> B <sub>6</sub> C <sub>6</sub> | $1.625 \text{La}_4\text{H}_9 + \text{H}_3\text{N} + 3 \text{B}_{13}\text{C}_2 \rightarrow 6.813 \text{H}_2 + 5.5 \text{LaB}_6 + \text{LaB}_6\text{H}_4\text{C}_6\text{N}$                          | -0.7223             |
| LaNH <sub>4</sub> B <sub>6</sub> C <sub>6</sub> | $0.4444 \text{La}_4\text{H}_9 + 0.8995 \text{La}_2\text{C}_3 + 0.5 \text{N}_2 + 1.651 \text{B}_{13}\text{C}_2 \rightarrow 2.577 \text{LaB}_6 + \text{LaB}_6\text{H}_4\text{C}_6\text{N}$           | -0.7010             |
| LaNH <sub>4</sub> B <sub>6</sub> C <sub>6</sub> | $0.5 \text{N}_2 + 3 \text{B}_{13}\text{C}_2 + 2.688 \text{La}_2\text{H}_5 \rightarrow 4.376 \text{LaB}_6 + 1.349 \text{B}_5\text{H}_7 + \text{LaB}_6\text{H}_4\text{C}_6\text{N}$                  | -0.6937             |
| LaNH <sub>4</sub> B <sub>6</sub> C <sub>6</sub> | $2 \text{La}_2\text{C}_3 + 1.684 \text{B}_5\text{H}_7 + 0.5 \text{N}_2 \rightarrow 2.596 \text{LaH}_3 + 0.4035 \text{LaB}_6 + \text{LaB}_6\text{H}_4\text{C}_6\text{N}$                            | -0.6793             |
| LaNH <sub>4</sub> B <sub>6</sub> C <sub>6</sub> | $\text{LaN} + 0.6667 \text{La}_2\text{C}_3 + 2 \text{LaH}_2 + 2 \text{B}_{13}\text{C}_2 \rightarrow 3.333 \text{LaB}_6 + \text{LaB}_6\text{H}_4\text{C}_6\text{N}$                                 | -0.6476             |
| LaNH <sub>4</sub> B <sub>6</sub> C <sub>6</sub> | $13.25 \text{B}_9\text{H}_{11} + 2 \text{La}_2\text{C}_3 + 0.5 \text{N}_2 \rightarrow 20.25 \text{B}_5\text{H}_7 + 3 \text{LaB}_4 + \text{LaB}_6\text{H}_4\text{C}_6\text{N}$                      | -0.6402             |
| LaNH <sub>4</sub> B <sub>6</sub> C <sub>6</sub> | $\text{BN} + 6.667 \text{LaH}_2 + 3 \text{B}_{13}\text{C}_2 \rightarrow 4.667 \text{H}_2 + 5.667 \text{LaB}_6 + \text{LaB}_6\text{H}_4\text{C}_6\text{N}$                                          | -0.6337             |
| LaNH <sub>4</sub> B <sub>6</sub> C <sub>6</sub> | $\text{H}_3\text{N} + 2.667 \text{B}_9\text{H}_{11} + 2 \text{La}_2\text{C}_3 \rightarrow 14.17 \text{H}_2 + 3 \text{LaB}_6 + \text{LaB}_6\text{H}_4\text{C}_6\text{N}$                            | -0.6183             |
| LaNH <sub>4</sub> B <sub>6</sub> C <sub>6</sub> | $5 \text{H}_2 + 6 \text{B} + 2 \text{La}_2\text{C}_3 + 0.5 \text{N}_2 \rightarrow 3 \text{LaH}_2 + \text{LaB}_6\text{H}_4\text{C}_6\text{N}$                                                       | -0.6111             |
| LaNH <sub>4</sub> B <sub>6</sub> C <sub>6</sub> | $\text{H}_3\text{N} + 5.346 \text{LaH}_2 + 3 \text{B}_{13}\text{C}_2 \rightarrow 4.346 \text{LaB}_6 + 1.385 \text{B}_5\text{H}_7 + \text{LaB}_6\text{H}_4\text{C}_6\text{N}$                       | -0.6088             |
| LaNH <sub>4</sub> B <sub>6</sub> C <sub>6</sub> | $\text{BN} + 17.63 \text{B}_9\text{H}_{11} + 2 \text{La}_2\text{C}_3 \rightarrow 3 \text{LaB}_6 + 27.13 \text{B}_5\text{H}_7 + \text{LaB}_6\text{H}_4\text{C}_6\text{N}$                           | -0.5961             |
| LaNH <sub>4</sub> B <sub>6</sub> C <sub>6</sub> | $3 \text{LaC}_2 + 8 \text{B} + 3 \text{H}_3\text{N} \rightarrow 2 \text{BN} + \text{La}_2\text{H}_5 + \text{LaB}_6\text{H}_4\text{C}_6\text{N}$                                                    | -0.5899             |
| LaNH <sub>4</sub> B <sub>6</sub> C <sub>6</sub> | $3 \text{LaC}_2 + 1.667 \text{LaB}_6 + 5 \text{H}_3\text{N} \rightarrow 3.667 \text{LaH}_3 + 4 \text{BN} + \text{LaB}_6\text{H}_4\text{C}_6\text{N}$                                               | -0.5895             |
| LaNH <sub>4</sub> B <sub>6</sub> C <sub>6</sub> | $3 \text{LaC}_2 + \text{LaN} + 18.5 \text{B}_9\text{H}_{11} \rightarrow 3 \text{LaB}_6 + 28.5 \text{B}_5\text{H}_7 + \text{LaB}_6\text{H}_4\text{C}_6\text{N}$                                     | -0.5845             |
| LaNH <sub>4</sub> B <sub>6</sub> C <sub>6</sub> | $6 \text{C} + 3.815 \text{La} + \text{H}_3\text{N} + 0.6667 \text{B}_9\text{H}_{11} \rightarrow 0.7037 \text{La}_4\text{H}_9 + \text{LaB}_6\text{H}_4\text{C}_6\text{N}$                           | -0.5736             |
| LaNH <sub>4</sub> B <sub>6</sub> C <sub>6</sub> | $0.5 \text{N}_2 + 3 \text{B}_{13}\text{C}_2 + 2.627 \text{La}_2\text{H}_5 \rightarrow 4.254 \text{LaB}_6 + 0.8305 \text{B}_9\text{H}_{11} + \text{LaB}_6\text{H}_4\text{C}_6\text{N}$              | -0.5684             |
| LaNH <sub>4</sub> B <sub>6</sub> C <sub>6</sub> | $2.538 \text{LaC}_2 + 2 \text{LaH}_2 + 2.269 \text{N}_2 + 0.4615 \text{B}_{13}\text{C}_2 \rightarrow 3.538 \text{LaN} + \text{LaB}_6\text{H}_4\text{C}_6\text{N}$                                  | -0.5652             |
| LaNH <sub>4</sub> B <sub>6</sub> C <sub>6</sub> | $3.138 \text{H}_3\text{N} + 1.583 \text{La}_2\text{C}_3 + 0.626 \text{B}_{13}\text{C}_2 \rightarrow 2.138 \text{BN} + 1.083 \text{La}_2\text{H}_5 + \text{LaB}_6\text{H}_4\text{C}_6\text{N}$      | -0.5621             |
| LaNH <sub>4</sub> B <sub>6</sub> C <sub>6</sub> | $\text{LaN} + 2.357 \text{La}_2\text{C}_3 + 2.592 \text{B}_5\text{H}_7 \rightarrow 4.714 \text{LaH}_3 + 0.5352 \text{B}_{13}\text{C}_2 + \text{LaB}_6\text{H}_4\text{C}_6\text{N}$                 | -0.5561             |
| LaNH <sub>4</sub> B <sub>6</sub> C <sub>6</sub> | $2.833 \text{H}_2 + 0.6667 \text{B}_9\text{H}_{11} + 2 \text{La}_2\text{C}_3 + 0.5 \text{N}_2 \rightarrow 3 \text{LaH}_3 + \text{LaB}_6\text{H}_4\text{C}_6\text{N}$                               | -0.5561             |
| LaNH <sub>4</sub> B <sub>6</sub> C <sub>6</sub> | $\text{LaN} + 1.226 \text{B}_9\text{H}_{11} + 2 \text{La}_2\text{C}_3 \rightarrow 3.161 \text{LaH}_3 + 0.8387 \text{LaB}_6 + \text{LaB}_6\text{H}_4\text{C}_6\text{N}$                             | -0.5522             |
| LaNH <sub>4</sub> B <sub>6</sub> C <sub>6</sub> | $2.3 \text{H}_2 + 2 \text{La}_2\text{C}_3 + 1.2 \text{B}_5\text{H}_7 + 0.5 \text{N}_2 \rightarrow 3 \text{LaH}_3 + \text{LaB}_6\text{H}_4\text{C}_6\text{N}$                                       | -0.5110             |
| LaNH <sub>4</sub> B <sub>6</sub> C <sub>6</sub> | $3 \text{LaC}_2 + 2 \text{H}_2 + 6 \text{B} + 1.5 \text{N}_2 \rightarrow 2 \text{LaN} + \text{LaB}_6\text{H}_4\text{C}_6\text{N}$                                                                  | -0.5108             |
| LaNH <sub>4</sub> B <sub>6</sub> C <sub>6</sub> | $3 \text{LaC}_2 + 2 \text{H}_2 + 17 \text{B} + \text{BN} \rightarrow 2 \text{LaB}_6 + \text{LaB}_6\text{H}_4\text{C}_6\text{N}$                                                                    | -0.5032             |
| LaNH <sub>4</sub> B <sub>6</sub> C <sub>6</sub> | $10.25 \text{H}_2 + \text{LaN} + 2 \text{La}_2\text{C}_3 + 1.5 \text{LaB}_4 \rightarrow 5.5 \text{LaH}_3 + \text{LaB}_6\text{H}_4\text{C}_6\text{N}$                                               | -0.5030             |
| LaNH <sub>4</sub> B <sub>6</sub> C <sub>6</sub> | $3 \text{LaC}_2 + 15.14 \text{B} + \text{LaN} + 0.5714 \text{B}_5\text{H}_7 \rightarrow 3 \text{LaB}_4 + \text{LaB}_6\text{H}_4\text{C}_6\text{N}$                                                 | -0.4806             |
| LaNH <sub>4</sub> B <sub>6</sub> C <sub>6</sub> | $0.9333 \text{La}_2\text{C}_3 + 0.5 \text{N}_2 + 1.6 \text{B}_{13}\text{C}_2 + 0.8 \text{La}_2\text{H}_5 \rightarrow 2.467 \text{LaB}_6 + \text{LaB}_6\text{H}_4\text{C}_6\text{N}$                | -0.4741             |
| LaNH <sub>4</sub> B <sub>6</sub> C <sub>6</sub> | $6 \text{C} + 3.467 \text{La} + \text{H}_3\text{N} + 1.2 \text{B}_5\text{H}_7 \rightarrow 2.467 \text{LaH}_3 + \text{LaB}_6\text{H}_4\text{C}_6\text{N}$                                           | -0.4709             |
| LaNH <sub>4</sub> B <sub>6</sub> C <sub>6</sub> | $\text{H}_3\text{N} + 5.214 \text{LaH}_2 + 3 \text{B}_{13}\text{C}_2 \rightarrow 4.214 \text{LaB}_6 + 0.8571 \text{B}_9\text{H}_{11} + \text{LaB}_6\text{H}_4\text{C}_6\text{N}$                   | -0.4451             |
| LaNH <sub>4</sub> B <sub>6</sub> C <sub>6</sub> | $5 \text{H}_2 + 6 \text{B} + \text{H}_3\text{N} + 2 \text{La}_2\text{C}_3 \rightarrow 3 \text{LaH}_3 + \text{LaB}_6\text{H}_4\text{C}_6\text{N}$                                                   | -0.4410             |
| LaNH <sub>4</sub> B <sub>6</sub> C <sub>6</sub> | $2.687 \text{LaC}_2 + 0.125 \text{H}_8\text{C}_5 + 16.12 \text{B} + \text{H}_3\text{N} \rightarrow 1.687 \text{LaB}_6 + \text{LaB}_6\text{H}_4\text{C}_6\text{N}$                                  | -0.4387             |
| LaNH <sub>4</sub> B <sub>6</sub> C <sub>6</sub> | $\text{H}_3\text{N} + 2 \text{La}_2\text{C}_3 + 4.8 \text{B}_5\text{H}_7 \rightarrow 16.3 \text{H}_2 + 3 \text{LaB}_6 + \text{LaB}_6\text{H}_4\text{C}_6\text{N}$                                  | -0.4379             |
| LaNH <sub>4</sub> B <sub>6</sub> C <sub>6</sub> | $0.6667 \text{B}_9\text{H}_{11} + 2 \text{La}_2\text{C}_3 + 1.167 \text{N}_2 \rightarrow 1.333 \text{LaN} + 1.667 \text{LaH}_2 + \text{LaB}_6\text{H}_4\text{C}_6\text{N}$                         | -0.4369             |
| LaNH <sub>4</sub> B <sub>6</sub> C <sub>6</sub> | $0.5 \text{H}_8\text{C}_5 + 4.35 \text{LaN} + 1.75 \text{B}_{13}\text{C}_2 \rightarrow 3.35 \text{BN} + 3.35 \text{LaB}_4 + \text{LaB}_6\text{H}_4\text{C}_6\text{N}$                              | -0.4342             |
| LaNH <sub>4</sub> B <sub>6</sub> C <sub>6</sub> | $0.3636 \text{B}_9\text{H}_{11} + 1.342 \text{La}_2\text{C}_3 + 0.5 \text{N}_2 + 0.987 \text{B}_{13}\text{C}_2 \rightarrow 1.684 \text{LaB}_6 + \text{LaB}_6\text{H}_4\text{C}_6\text{N}$          | -0.4328             |
| LaNH <sub>4</sub> B <sub>6</sub> C <sub>6</sub> | $3 \text{LaC}_2 + 14.73 \text{B} + \text{LaN} + 0.3636 \text{B}_9\text{H}_{11} \rightarrow 3 \text{LaB}_4 + \text{LaB}_6\text{H}_4\text{C}_6\text{N}$                                              | -0.4183             |
| LaNH <sub>4</sub> B <sub>6</sub> C <sub>6</sub> | $1.2 \text{H}_8\text{C}_5 + 6 \text{B} + 4.44 \text{La} + \text{H}_3\text{N} \rightarrow 1.72 \text{La}_2\text{H}_5 + \text{LaB}_6\text{H}_4\text{C}_6\text{N}$                                    | -0.4134             |
| LaNH <sub>4</sub> B <sub>6</sub> C <sub>6</sub> | $2 \text{La}_2\text{C}_3 + 1.2 \text{B}_5\text{H}_7 + 1.022 \text{N}_2 \rightarrow 0.4889 \text{La}_4\text{H}_9 + 1.044 \text{LaN} + \text{LaB}_6\text{H}_4\text{C}_6\text{N}$                     | -0.4118             |
| LaNH <sub>4</sub> B <sub>6</sub> C <sub>6</sub> | $0.5 \text{H}_8\text{C}_5 + 3.393 \text{LaN} + 1.75 \text{B}_{13}\text{C}_2 \rightarrow 2.393 \text{LaB}_6 + 2.393 \text{BN} + \text{LaB}_6\text{H}_4\text{C}_6\text{N}$                           | -0.4063             |
| LaNH <sub>4</sub> B <sub>6</sub> C <sub>6</sub> | $6 \text{C} + 5.286 \text{LaN} + 1.143 \text{B}_9\text{H}_{11} \rightarrow 4.286 \text{BN} + 4.286 \text{LaH}_2 + \text{LaB}_6\text{H}_4\text{C}_6\text{N}$                                        | -0.4044             |
| LaNH <sub>4</sub> B <sub>6</sub> C <sub>6</sub> | $\text{LaN} + 2 \text{La}_2\text{C}_3 + 2 \text{B}_5\text{H}_7 \rightarrow 3.333 \text{LaH}_3 + 0.6667 \text{LaB}_6 + \text{LaB}_6\text{H}_4\text{C}_6\text{N}$                                    | -0.3976             |
| LaNH <sub>4</sub> B <sub>6</sub> C <sub>6</sub> | $0.9859 \text{B}_9\text{H}_{11} + 2 \text{La}_2\text{C}_3 + 0.5 \text{N}_2 \rightarrow 2.282 \text{LaH}_3 + 0.7183 \text{LaB}_4 + \text{LaB}_6\text{H}_4\text{C}_6\text{N}$                        | -0.3941             |
| LaNH <sub>4</sub> B <sub>6</sub> C <sub>6</sub> | $3 \text{LaC}_2 + \text{LaB}_6 + 0.4444 \text{La}_4\text{H}_9 + 2.889 \text{N}_2 \rightarrow 4.778 \text{LaN} + \text{LaB}_6\text{H}_4\text{C}_6\text{N}$                                          | -0.3889             |
| LaNH <sub>4</sub> B <sub>6</sub> C <sub>6</sub> | $3 \text{LaC}_2 + 4.641 \text{H}_3\text{N} + 2.41 \text{LaB}_4 \rightarrow 3.641 \text{BN} + 1.103 \text{La}_4\text{H}_9 + \text{LaB}_6\text{H}_4\text{C}_6\text{N}$                               | -0.3837             |
| LaNH <sub>4</sub> B <sub>6</sub> C <sub>6</sub> | $1.329 \text{La}_2\text{C}_3 + 0.5714 \text{B}_5\text{H}_7 + 0.5 \text{N}_2 + 1.007 \text{B}_{13}\text{C}_2 \rightarrow 1.658 \text{LaB}_6 + \text{LaB}_6\text{H}_4\text{C}_6\text{N}$             | -0.3811             |
| LaNH <sub>4</sub> B <sub>6</sub> C <sub>6</sub> | $2 \text{La}_2\text{C}_3 + 1.628 \text{B}_5\text{H}_7 + 0.5 \text{N}_2 \rightarrow 2.465 \text{LaH}_3 + 0.5349 \text{LaB}_4 + \text{LaB}_6\text{H}_4\text{C}_6\text{N}$                            | -0.3743             |
| LaNH <sub>4</sub> B <sub>6</sub> C <sub>6</sub> | $0.9492 \text{B}_9\text{H}_{11} + 2 \text{La}_2\text{C}_3 + 0.5 \text{N}_2 \rightarrow 0.4237 \text{LaB}_6 + 1.288 \text{La}_2\text{H}_5 + \text{LaB}_6\text{H}_4\text{C}_6\text{N}$               | -0.3663             |
| LaNH <sub>4</sub> B <sub>6</sub> C <sub>6</sub> | $1.2 \text{H}_8\text{C}_5 + 5.2 \text{La} + \text{BN} + \text{B}_5\text{H}_7 \rightarrow 4.2 \text{LaH}_3 + \text{LaB}_6\text{H}_4\text{C}_6\text{N}$                                              | -0.3626             |
| LaNH <sub>4</sub> B <sub>6</sub> C <sub>6</sub> | $1.2 \text{H}_8\text{C}_5 + 4.311 \text{La} + \text{LaN} + 0.6667 \text{B}_9\text{H}_{11} \rightarrow 4.311 \text{LaH}_3 + \text{LaB}_6\text{H}_4\text{C}_6\text{N}$                               | -0.3599             |
| LaNH <sub>4</sub> B <sub>6</sub> C <sub>6</sub> | $6.5 \text{LaH}_3 + 0.5 \text{N}_2 + 3 \text{B}_{13}\text{C}_2 \rightarrow 7.75 \text{H}_2 + 5.5 \text{LaB}_6 + \text{LaB}_6\text{H}_4\text{C}_6\text{N}$                                          | -0.3577             |
| LaNH <sub>4</sub> B <sub>6</sub> C <sub>6</sub> | $6 \text{C} + 3.2 \text{La} + 1.2 \text{B}_5\text{H}_7 + 0.5 \text{N}_2 \rightarrow 2.2 \text{LaH}_2 + \text{LaB}_6\text{H}_4\text{C}_6\text{N}$                                                   | -0.3446             |
| LaNH <sub>4</sub> B <sub>6</sub> C <sub>6</sub> | $1.146 \text{B}_9\text{H}_{11} + 2.221 \text{La}_2\text{C}_3 + 0.5 \text{N}_2 \rightarrow 0.3319 \text{B}_{13}\text{C}_2 + 1.721 \text{La}_2\text{H}_5 + \text{LaB}_6\text{H}_4\text{C}_6\text{N}$ | -0.3439             |
| LaNH <sub>4</sub> B <sub>6</sub> C <sub>6</sub> | $14.14 \text{B} + \text{BN} + 2 \text{La}_2\text{C}_3 + 0.5714 \text{B}_5\text{H}_7 \rightarrow 3 \text{LaB}_4 + \text{LaB}_6\text{H}_4\text{C}_6\text{N}$                                         | -0.3424             |
| LaNH <sub>4</sub> B <sub>6</sub> C <sub>6</sub> | $0.5 \text{H}_8\text{C}_5 + \text{LaN} + 1.75 \text{B}_{13}\text{C}_2 + 8.375 \text{LaB}_4 \rightarrow 8.375 \text{LaB}_6 + \text{LaB}_6\text{H}_4\text{C}_6\text{N}$                              | -0.3364             |
| LaNH <sub>4</sub> B <sub>6</sub> C <sub>6</sub> | $0.4444 \text{La}_4\text{H}_9 + \text{LaN} + 0.709 \text{La}_2\text{C}_3 + 1.937 \text{B}_{13}\text{C}_2 \rightarrow 3.196 \text{LaB}_6 + \text{LaB}_6\text{H}_4\text{C}_6\text{N}$                | -0.3346             |
| LaNH <sub>4</sub> B <sub>6</sub> C <sub>6</sub> | $6.5 \text{H}_2 + 6 \text{B} + \text{LaN} + 2 \text{La}_2\text{C}_3 \rightarrow \text{La}_4\text{H}_9 + \text{LaB}_6\text{H}_4\text{C}_6\text{N}$                                                  | -0.3344             |
| LaNH <sub>4</sub> B <sub>6</sub> C <sub>6</sub> | $25.1 \text{H}_2 + \text{La} + 0.5 \text{N}_2 + 3 \text{B}_{13}\text{C}_2 \rightarrow 6.6 \text{B}_5\text{H}_7 + \text{LaB}_6\text{H}_4\text{C}_6\text{N}$                                         | -0.3301             |
| LaNH <sub>4</sub> B <sub>6</sub> C <sub>6</sub> | $2 \text{La}_2\text{C}_3 + 6.375 \text{B}_5\text{H}_7 + 0.5 \text{N}_2 \rightarrow 3 \text{LaH}_3 + 2.875 \text{B}_9\text{H}_{11} + \text{LaB}_6\text{H}_4\text{C}_6\text{N}$                      | -0.3166             |
| LaNH <sub>4</sub> B <sub>6</sub> C <sub>6</sub> | $0.5 \text{H}_8\text{C}_5 + \text{BN} + 1.75 \text{B}_{13}\text{C}_2 + 11.88 \text{LaB}_4 \rightarrow 10.88 \text{LaB}_6 + \text{LaB}_6\text{H}_4\text{C}_6\text{N}$                               | -0.3072             |

Continued on next page



Continued

| Compound                                        | Chemical reaction                                                                                                                                                                               | Reaction energy(eV) |
|-------------------------------------------------|-------------------------------------------------------------------------------------------------------------------------------------------------------------------------------------------------|---------------------|
| LaNH <sub>4</sub> B <sub>6</sub> C <sub>6</sub> | $3 \text{LaC}_2 + 11.14 \text{B} + 0.5714 \text{B}_5\text{H}_7 + 0.5 \text{N}_2 \rightarrow 2 \text{LaB}_4 + \text{LaB}_6\text{H}_4\text{C}_6\text{N}$                                          | -0.2916             |
| LaNH <sub>4</sub> B <sub>6</sub> C <sub>6</sub> | $6 \text{C} + 3.533 \text{La} + \text{H}_3\text{N} + 0.6667 \text{B}_9\text{H}_{11} \rightarrow 1.267 \text{La}_2\text{H}_5 + \text{LaB}_6\text{H}_4\text{C}_6\text{N}$                         | -0.2879             |
| LaNH <sub>4</sub> B <sub>6</sub> C <sub>6</sub> | $\text{LaN} + 3 \text{B}_{13}\text{C}_2 + 2.303 \text{La}_2\text{H}_5 \rightarrow 4.606 \text{LaB}_6 + 1.073 \text{B}_5\text{H}_7 + \text{LaB}_6\text{H}_4\text{C}_6\text{N}$                   | -0.2825             |
| LaNH <sub>4</sub> B <sub>6</sub> C <sub>6</sub> | $13.73 \text{B} + \text{BN} + 0.3636 \text{B}_9\text{H}_{11} + 2 \text{La}_2\text{C}_3 \rightarrow 3 \text{LaB}_4 + \text{LaB}_6\text{H}_4\text{C}_6\text{N}$                                   | -0.2801             |
| LaNH <sub>4</sub> B <sub>6</sub> C <sub>6</sub> | $1.563 \text{LaB}_6 + 4.375 \text{H}_3\text{N} + 2 \text{La}_2\text{C}_3 \rightarrow 3.375 \text{BN} + 4.563 \text{LaH}_2 + \text{LaB}_6\text{H}_4\text{C}_6\text{N}$                           | -0.2691             |
| LaNH <sub>4</sub> B <sub>6</sub> C <sub>6</sub> | $6 \text{C} + \text{LaB}_6 + 0.5714 \text{B}_5\text{H}_7 + 1.929 \text{N}_2 \rightarrow 2.857 \text{BN} + \text{LaB}_6\text{H}_4\text{C}_6\text{N}$                                             | -0.2593             |
| LaNH <sub>4</sub> B <sub>6</sub> C <sub>6</sub> | $3 \text{LaC}_2 + 0.7727 \text{B}_9\text{H}_{11} + 0.9773 \text{N}_2 \rightarrow 0.9545 \text{BN} + 0.5 \text{La}_4\text{H}_9 + \text{LaB}_6\text{H}_4\text{C}_6\text{N}$                       | -0.2571             |
| LaNH <sub>4</sub> B <sub>6</sub> C <sub>6</sub> | $3 \text{LaC}_2 + 21 \text{B} + \text{BN} + 2 \text{LaH}_2 \rightarrow 4 \text{LaB}_4 + \text{LaB}_6\text{H}_4\text{C}_6\text{N}$                                                               | -0.2521             |
| LaNH <sub>4</sub> B <sub>6</sub> C <sub>6</sub> | $\text{LaN} + 16.75 \text{B}_9\text{H}_{11} + 2 \text{La}_2\text{C}_3 \rightarrow 25.75 \text{B}_5\text{H}_7 + 4 \text{LaB}_4 + \text{LaB}_6\text{H}_4\text{C}_6\text{N}$                       | -0.2299             |
| LaNH <sub>4</sub> B <sub>6</sub> C <sub>6</sub> | $3 \text{LaC}_2 + 10.73 \text{B} + 0.3636 \text{B}_9\text{H}_{11} + 0.5 \text{N}_2 \rightarrow 2 \text{LaB}_4 + \text{LaB}_6\text{H}_4\text{C}_6\text{N}$                                       | -0.2293             |
| LaNH <sub>4</sub> B <sub>6</sub> C <sub>6</sub> | $1.333 \text{LaH}_3 + 0.9841 \text{La}_2\text{C}_3 + 0.5 \text{N}_2 + 1.524 \text{B}_{13}\text{C}_2 \rightarrow 2.302 \text{LaB}_6 + \text{LaB}_6\text{H}_4\text{C}_6\text{N}$                  | -0.2279             |
| LaNH <sub>4</sub> B <sub>6</sub> C <sub>6</sub> | $3 \text{LaC}_2 + 2 \text{H}_2 + 2.25 \text{N}_2 + 1.5 \text{LaB}_4 \rightarrow 3.5 \text{LaN} + \text{LaB}_6\text{H}_4\text{C}_6\text{N}$                                                      | -0.2273             |
| LaNH <sub>4</sub> B <sub>6</sub> C <sub>6</sub> | $2 \text{La}_2\text{C}_3 + 1.541 \text{B}_5\text{H}_7 + 0.5 \text{N}_2 \rightarrow 0.2844 \text{LaB}_6 + 1.358 \text{La}_2\text{H}_5 + \text{LaB}_6\text{H}_4\text{C}_6\text{N}$                | -0.2231             |
| LaNH <sub>4</sub> B <sub>6</sub> C <sub>6</sub> | $7.625 \text{H}_2 + 2 \text{La}_2\text{C}_3 + 0.5 \text{N}_2 + 1.5 \text{LaB}_4 \rightarrow 2.25 \text{La}_2\text{H}_5 + \text{LaB}_6\text{H}_4\text{C}_6\text{N}$                              | -0.2209             |
| LaNH <sub>4</sub> B <sub>6</sub> C <sub>6</sub> | $3 \text{LaC}_2 + 13.25 \text{B}_9\text{H}_{11} + 0.5 \text{N}_2 \rightarrow 2 \text{LaB}_6 + 20.25 \text{B}_5\text{H}_7 + \text{LaB}_6\text{H}_4\text{C}_6\text{N}$                            | -0.2039             |
| LaNH <sub>4</sub> B <sub>6</sub> C <sub>6</sub> | $2 \text{H}_2 + 1.238 \text{La}_2\text{C}_3 + 0.5 \text{N}_2 + 1.143 \text{B}_{13}\text{C}_2 \rightarrow 1.476 \text{LaB}_6 + \text{LaB}_6\text{H}_4\text{C}_6\text{N}$                         | -0.1944             |
| LaNH <sub>4</sub> B <sub>6</sub> C <sub>6</sub> | $2.139 \text{La}_2\text{C}_3 + 1.742 \text{B}_5\text{H}_7 + 0.5 \text{N}_2 \rightarrow 0.2085 \text{B}_{13}\text{C}_2 + 1.639 \text{La}_2\text{H}_5 + \text{LaB}_6\text{H}_4\text{C}_6\text{N}$ | -0.1904             |
| LaNH <sub>4</sub> B <sub>6</sub> C <sub>6</sub> | $\text{LaN} + 3 \text{B}_{13}\text{C}_2 + 2.254 \text{La}_2\text{H}_5 \rightarrow 4.508 \text{LaB}_6 + 0.661 \text{B}_9\text{H}_{11} + \text{LaB}_6\text{H}_4\text{C}_6\text{N}$                | -0.1829             |
| LaNH <sub>4</sub> B <sub>6</sub> C <sub>6</sub> | $\text{H}_2 + \text{B} + 0.01195 \text{LaN} + 0.03586 \text{B}_{13}\text{C}_2 \rightarrow 0.2789 \text{B}_5\text{H}_7 + 0.01195 \text{LaB}_6\text{H}_4\text{C}_6\text{N}$                       | -0.1812             |
| LaNH <sub>4</sub> B <sub>6</sub> C <sub>6</sub> | $2.538 \text{LaC}_2 + 0.4444 \text{La}_4\text{H}_9 + 2.158 \text{N}_2 + 0.4615 \text{B}_{13}\text{C}_2 \rightarrow 3.316 \text{LaN} + \text{LaB}_6\text{H}_4\text{C}_6\text{N}$                 | -0.1708             |
| LaNH <sub>4</sub> B <sub>6</sub> C <sub>6</sub> | $4.333 \text{H}_2 + \text{LaN} + 0.6667 \text{B}_9\text{H}_{11} + 2 \text{La}_2\text{C}_3 \rightarrow 4 \text{LaH}_3 + \text{LaB}_6\text{H}_4\text{C}_6\text{N}$                                | -0.1646             |
| LaNH <sub>4</sub> B <sub>6</sub> C <sub>6</sub> | $3 \text{LaC}_2 + 7.833 \text{B} + 2.833 \text{H}_3\text{N} \rightarrow 1.833 \text{BN} + 0.5 \text{La}_4\text{H}_9 + \text{LaB}_6\text{H}_4\text{C}_6\text{N}$                                 | -0.1625             |
| LaNH <sub>4</sub> B <sub>6</sub> C <sub>6</sub> | $2.97 \text{H}_3\text{N} + 1.591 \text{La}_2\text{C}_3 + 0.6131 \text{B}_{13}\text{C}_2 \rightarrow 1.97 \text{BN} + 0.5456 \text{La}_4\text{H}_9 + \text{LaB}_6\text{H}_4\text{C}_6\text{N}$   | -0.1564             |
| LaNH <sub>4</sub> B <sub>6</sub> C <sub>6</sub> | $\text{H}_2 + \text{B} + 0.01754 \text{LaN} + 0.05263 \text{B}_{13}\text{C}_2 \rightarrow 0.1754 \text{B}_9\text{H}_{11} + 0.01754 \text{LaB}_6\text{H}_4\text{C}_6\text{N}$                    | -0.1563             |
| LaNH <sub>4</sub> B <sub>6</sub> C <sub>6</sub> | $5.577 \text{H}_2 + 1.692 \text{La}_2\text{C}_3 + 0.5 \text{N}_2 + 0.4615 \text{B}_{13}\text{C}_2 \rightarrow 2.385 \text{LaH}_3 + \text{LaB}_6\text{H}_4\text{C}_6\text{N}$                    | -0.1346             |
| LaNH <sub>4</sub> B <sub>6</sub> C <sub>6</sub> | $6 \text{C} + 2.956 \text{La} + 1.2 \text{B}_5\text{H}_7 + 0.5 \text{N}_2 \rightarrow 0.4889 \text{La}_4\text{H}_9 + \text{LaB}_6\text{H}_4\text{C}_6\text{N}$                                  | -0.1288             |
| LaNH <sub>4</sub> B <sub>6</sub> C <sub>6</sub> | $3.8 \text{H}_2 + \text{LaN} + 2 \text{La}_2\text{C}_3 + 1.2 \text{B}_5\text{H}_7 \rightarrow 4 \text{LaH}_3 + \text{LaB}_6\text{H}_4\text{C}_6\text{N}$                                        | -0.1196             |
| LaNH <sub>4</sub> B <sub>6</sub> C <sub>6</sub> | $\text{LaN} + 0.7429 \text{La}_2\text{C}_3 + 1.886 \text{B}_{13}\text{C}_2 + 0.8 \text{La}_2\text{H}_5 \rightarrow 3.086 \text{LaB}_6 + \text{LaB}_6\text{H}_4\text{C}_6\text{N}$               | -0.1078             |
| LaNH <sub>4</sub> B <sub>6</sub> C <sub>6</sub> | $3.5 \text{LaN} + 5.75 \text{LaH}_2 + 3 \text{B}_{13}\text{C}_2 \rightarrow 2.5 \text{H}_3\text{N} + 8.25 \text{LaB}_4 + \text{LaB}_6\text{H}_4\text{C}_6\text{N}$                              | -0.1073             |
| LaNH <sub>4</sub> B <sub>6</sub> C <sub>6</sub> | $2.083 \text{H}_2 + 0.6667 \text{B}_9\text{H}_{11} + 2 \text{La}_2\text{C}_3 + 0.5 \text{N}_2 \rightarrow 1.5 \text{La}_2\text{H}_5 + \text{LaB}_6\text{H}_4\text{C}_6\text{N}$                 | -0.1071             |
| LaNH <sub>4</sub> B <sub>6</sub> C <sub>6</sub> | $3 \text{LaC}_2 + \text{LaB}_6 + 2.8 \text{N}_2 + 0.8 \text{La}_2\text{H}_5 \rightarrow 4.6 \text{LaN} + \text{LaB}_6\text{H}_4\text{C}_6\text{N}$                                              | -0.0969             |
| LaNH <sub>4</sub> B <sub>6</sub> C <sub>6</sub> | $8 \text{H}_2 + \text{LaB}_6 + 2 \text{La}_2\text{C}_3 + 0.5 \text{N}_2 \rightarrow 4 \text{LaH}_3 + \text{LaB}_6\text{H}_4\text{C}_6\text{N}$                                                  | -0.0940             |
| LaNH <sub>4</sub> B <sub>6</sub> C <sub>6</sub> | $22.17 \text{H}_2 + \text{La} + 0.5 \text{N}_2 + 3 \text{B}_{13}\text{C}_2 \rightarrow 3.667 \text{B}_9\text{H}_{11} + \text{LaB}_6\text{H}_4\text{C}_6\text{N}$                                | -0.0821             |
| LaNH <sub>4</sub> B <sub>6</sub> C <sub>6</sub> | $\text{LaN} + 0.3636 \text{B}_9\text{H}_{11} + 1.152 \text{La}_2\text{C}_3 + 1.273 \text{B}_{13}\text{C}_2 \rightarrow 2.303 \text{LaB}_6 + \text{LaB}_6\text{H}_4\text{C}_6\text{N}$           | -0.0665             |
| LaNH <sub>4</sub> B <sub>6</sub> C <sub>6</sub> | $0.9173 \text{B}_9\text{H}_{11} + 2 \text{La}_2\text{C}_3 + 0.5 \text{N}_2 \rightarrow 1.218 \text{La}_2\text{H}_5 + 0.5639 \text{LaB}_4 + \text{LaB}_6\text{H}_4\text{C}_6\text{N}$            | -0.0643             |
| LaNH <sub>4</sub> B <sub>6</sub> C <sub>6</sub> | $1.55 \text{H}_2 + 2 \text{La}_2\text{C}_3 + 1.2 \text{B}_5\text{H}_7 + 0.5 \text{N}_2 \rightarrow 1.5 \text{La}_2\text{H}_5 + \text{LaB}_6\text{H}_4\text{C}_6\text{N}$                        | -0.0620             |
| LaNH <sub>4</sub> B <sub>6</sub> C <sub>6</sub> | $3 \text{LaC}_2 + 16 \text{B} + \text{H}_3\text{N} + 0.5 \text{LaH}_2 \rightarrow 2.5 \text{LaB}_4 + \text{LaB}_6\text{H}_4\text{C}_6\text{N}$                                                  | -0.0472             |
| LaNH <sub>4</sub> B <sub>6</sub> C <sub>6</sub> | $1.421 \text{LaC}_2 + 2 \text{LaH}_2 + 0.5 \text{N}_2 + 1.579 \text{B}_{13}\text{C}_2 \rightarrow 2.421 \text{LaB}_6 + \text{LaB}_6\text{H}_4\text{C}_6\text{N}$                                | -0.0371             |
| LaNH <sub>4</sub> B <sub>6</sub> C <sub>6</sub> | $0.9043 \text{B}_9\text{H}_{11} + 2 \text{La}_2\text{C}_3 + 0.5 \text{N}_2 \rightarrow 0.3565 \text{LaB}_6 + 0.6609 \text{La}_4\text{H}_9 + \text{LaB}_6\text{H}_4\text{C}_6\text{N}$           | -0.0340             |
| LaNH <sub>4</sub> B <sub>6</sub> C <sub>6</sub> | $2 \text{La}_2\text{C}_3 + 1.506 \text{B}_5\text{H}_7 + 0.5 \text{N}_2 \rightarrow 1.309 \text{La}_2\text{H}_5 + 0.3827 \text{LaB}_4 + \text{LaB}_6\text{H}_4\text{C}_6\text{N}$                | -0.0214             |
| LaNH <sub>4</sub> B <sub>6</sub> C <sub>6</sub> | $\text{LaN} + 1.138 \text{La}_2\text{C}_3 + 0.5714 \text{B}_5\text{H}_7 + 1.293 \text{B}_{13}\text{C}_2 \rightarrow 2.277 \text{LaB}_6 + \text{LaB}_6\text{H}_4\text{C}_6\text{N}$              | -0.0147             |
| LaNH <sub>4</sub> B <sub>6</sub> C <sub>6</sub> | $\text{H}_3\text{N} + 3 \text{B}_{13}\text{C}_2 + 3.25 \text{La}_2\text{H}_5 \rightarrow 7.625 \text{H}_2 + 5.5 \text{LaB}_6 + \text{LaB}_6\text{H}_4\text{C}_6\text{N}$                        | -0.0065             |
| LaNH <sub>4</sub> B <sub>6</sub> C <sub>6</sub> | $0.5 \text{H}_8\text{C}_5 + 14 \text{B} + 1.167 \text{La}_2\text{C}_3 + 0.5 \text{N}_2 \rightarrow 1.333 \text{LaB}_6 + \text{LaB}_6\text{H}_4\text{C}_6\text{N}$                               | -0.0042             |
| LuNH <sub>4</sub> B <sub>6</sub> C <sub>6</sub> | $3 \text{B}_{13}\text{C}_2 + 251 \text{LuB}_2 + 251 \text{H}_3\text{N} \rightarrow 250 \text{LuN} + 107 \text{B}_5\text{H}_7 + \text{LuB}_6\text{H}_4\text{C}_6\text{N}$                        | -149.6356           |
| LuNH <sub>4</sub> B <sub>6</sub> C <sub>6</sub> | $50 \text{Lu} + 3 \text{B}_{13}\text{C}_2 + 34 \text{H}_3\text{N} \rightarrow 33 \text{BN} + 49 \text{LuH}_2 + \text{LuB}_6\text{H}_4\text{C}_6\text{N}$                                        | -127.6214           |
| LuNH <sub>4</sub> B <sub>6</sub> C <sub>6</sub> | $15.5 \text{Lu}_4\text{C}_7 + 56 \text{H}_3\text{N} + 6 \text{BN} \rightarrow 20.5 \text{H}_8\text{C}_5 + 61 \text{LuN} + \text{LuB}_6\text{H}_4\text{C}_6\text{N}$                             | -113.7139           |
| LuNH <sub>4</sub> B <sub>6</sub> C <sub>6</sub> | $24.64 \text{N}_2 + 3 \text{B}_{13}\text{C}_2 + 0.3636 \text{B}_9\text{H}_{11} + \text{LuB}_{12} \rightarrow 48.27 \text{BN} + \text{LuB}_6\text{H}_4\text{C}_6\text{N}$                        | -112.9722           |
| LuNH <sub>4</sub> B <sub>6</sub> C <sub>6</sub> | $24.43 \text{N}_2 + 3 \text{B}_{13}\text{C}_2 + \text{LuB}_{12} + 0.5714 \text{B}_5\text{H}_7 \rightarrow 47.86 \text{BN} + \text{LuB}_6\text{H}_4\text{C}_6\text{N}$                           | -111.9678           |
| LuNH <sub>4</sub> B <sub>6</sub> C <sub>6</sub> | $23 \text{N}_2 + 3 \text{B}_{13}\text{C}_2 + \text{LuB}_{12} + 2 \text{H}_2 \rightarrow 45 \text{BN} + \text{LuB}_6\text{H}_4\text{C}_6\text{N}$                                                | -105.2314           |
| LuNH <sub>4</sub> B <sub>6</sub> C <sub>6</sub> | $22.33 \text{N}_2 + 3 \text{B}_{13}\text{C}_2 + \text{LuB}_{12} + 1.333 \text{H}_3\text{N} \rightarrow 45 \text{BN} + \text{LuB}_6\text{H}_4\text{C}_6\text{N}$                                 | -103.4659           |
| LuNH <sub>4</sub> B <sub>6</sub> C <sub>6</sub> | $22.69 \text{N}_2 + 3.875 \text{B}_{13}\text{C}_2 + 2 \text{LuH}_2 \rightarrow 0.25 \text{Lu}_4\text{C}_7 + 44.38 \text{BN} + \text{LuB}_6\text{H}_4\text{C}_6\text{N}$                         | -102.6011           |
| LuNH <sub>4</sub> B <sub>6</sub> C <sub>6</sub> | $21.33 \text{N}_2 + 3.667 \text{B}_{13}\text{C}_2 + 2 \text{LuH}_2 \rightarrow 0.3333 \text{Lu}_3\text{C}_4 + 41.67 \text{BN} + \text{LuB}_6\text{H}_4\text{C}_6\text{N}$                       | -95.8918            |
| LuNH <sub>4</sub> B <sub>6</sub> C <sub>6</sub> | $20.64 \text{N}_2 + 3 \text{B}_{13}\text{C}_2 + 0.3636 \text{B}_9\text{H}_{11} + \text{LuB}_4 \rightarrow 40.27 \text{BN} + \text{LuB}_6\text{H}_4\text{C}_6\text{N}$                           | -92.8499            |
| LuNH <sub>4</sub> B <sub>6</sub> C <sub>6</sub> | $20.43 \text{N}_2 + 3 \text{B}_{13}\text{C}_2 + \text{LuB}_4 + 0.5714 \text{B}_5\text{H}_7 \rightarrow 39.86 \text{BN} + \text{LuB}_6\text{H}_4\text{C}_6\text{N}$                              | -91.8455            |
| LuNH <sub>4</sub> B <sub>6</sub> C <sub>6</sub> | $1.2 \text{H}_8\text{C}_5 + 20.3 \text{N}_2 + 3.8 \text{LuB}_{12} \rightarrow 39.6 \text{BN} + 2.8 \text{LuH}_2 + \text{LuB}_6\text{H}_4\text{C}_6\text{N}$                                     | -89.2944            |
| LuNH <sub>4</sub> B <sub>6</sub> C <sub>6</sub> | $19.64 \text{N}_2 + 3 \text{B}_{13}\text{C}_2 + 0.3636 \text{B}_9\text{H}_{11} + \text{LuB}_2 \rightarrow 38.27 \text{BN} + \text{LuB}_6\text{H}_4\text{C}_6\text{N}$                           | -88.3289            |
| LuNH <sub>4</sub> B <sub>6</sub> C <sub>6</sub> | $19.43 \text{N}_2 + 3 \text{B}_{13}\text{C}_2 + \text{LuB}_2 + 0.5714 \text{B}_5\text{H}_7 \rightarrow 37.86 \text{BN} + \text{LuB}_6\text{H}_4\text{C}_6\text{N}$                              | -87.3245            |
| LuNH <sub>4</sub> B <sub>6</sub> C <sub>6</sub> | $18.64 \text{N}_2 + \text{Lu} + 3 \text{B}_{13}\text{C}_2 + 0.3636 \text{B}_9\text{H}_{11} \rightarrow 36.27 \text{BN} + \text{LuB}_6\text{H}_4\text{C}_6\text{N}$                              | -85.2207            |
| LuNH <sub>4</sub> B <sub>6</sub> C <sub>6</sub> | $19 \text{N}_2 + 3 \text{B}_{13}\text{C}_2 + \text{LuB}_4 + 2 \text{H}_2 \rightarrow 37 \text{BN} + \text{LuB}_6\text{H}_4\text{C}_6\text{N}$                                                   | -85.1091            |
| LuNH <sub>4</sub> B <sub>6</sub> C <sub>6</sub> | $18.43 \text{N}_2 + \text{Lu} + 3 \text{B}_{13}\text{C}_2 + 0.5714 \text{B}_5\text{H}_7 \rightarrow 35.86 \text{BN} + \text{LuB}_6\text{H}_4\text{C}_6\text{N}$                                 | -84.2163            |

Continued on next page

Continued

| Compound                                        | Chemical reaction                                                                                                                                                                                                | Reaction energy(eV) |
|-------------------------------------------------|------------------------------------------------------------------------------------------------------------------------------------------------------------------------------------------------------------------|---------------------|
| LuNH <sub>4</sub> B <sub>6</sub> C <sub>6</sub> | 18.33 N <sub>2</sub> + 3 B <sub>13</sub> C <sub>2</sub> + LuB <sub>4</sub> + 1.333 H <sub>3</sub> N → 37 BN + LuB <sub>6</sub> H <sub>4</sub> C <sub>6</sub> N                                                   | -83.3436            |
| LuNH <sub>4</sub> B <sub>6</sub> C <sub>6</sub> | 18.14 N <sub>2</sub> + 3 B <sub>13</sub> C <sub>2</sub> + 0.3636 B <sub>9</sub> H <sub>11</sub> + LuN → 36.27 BN + LuB <sub>6</sub> H <sub>4</sub> C <sub>6</sub> N                                              | -81.6778            |
| LuNH <sub>4</sub> B <sub>6</sub> C <sub>6</sub> | 17.93 N <sub>2</sub> + 3 B <sub>13</sub> C <sub>2</sub> + LuN + 0.5714 B <sub>5</sub> H <sub>7</sub> → 35.86 BN + LuB <sub>6</sub> H <sub>4</sub> C <sub>6</sub> N                                               | -80.6734            |
| LuNH <sub>4</sub> B <sub>6</sub> C <sub>6</sub> | 18 N <sub>2</sub> + 3 B <sub>13</sub> C <sub>2</sub> + LuB <sub>2</sub> + 2 H <sub>2</sub> → 35 BN + LuB <sub>6</sub> H <sub>4</sub> C <sub>6</sub> N                                                            | -80.5881            |
| LuNH <sub>4</sub> B <sub>6</sub> C <sub>6</sub> | 17.82 N <sub>2</sub> + 3 B <sub>13</sub> C <sub>2</sub> + 0.1818 B <sub>9</sub> H <sub>11</sub> + LuH <sub>2</sub> → 34.64 BN + LuB <sub>6</sub> H <sub>4</sub> C <sub>6</sub> N                                 | -79.4082            |
| LuNH <sub>4</sub> B <sub>6</sub> C <sub>6</sub> | 17.71 N <sub>2</sub> + 3 B <sub>13</sub> C <sub>2</sub> + 0.2857 B <sub>5</sub> H <sub>7</sub> + LuH <sub>2</sub> → 34.43 BN + LuB <sub>6</sub> H <sub>4</sub> C <sub>6</sub> N                                  | -78.9060            |
| LuNH <sub>4</sub> B <sub>6</sub> C <sub>6</sub> | 17.33 N <sub>2</sub> + 3 B <sub>13</sub> C <sub>2</sub> + LuB <sub>2</sub> + 1.333 H <sub>3</sub> N → 35 BN + LuB <sub>6</sub> H <sub>4</sub> C <sub>6</sub> N                                                   | -78.8226            |
| LuNH <sub>4</sub> B <sub>6</sub> C <sub>6</sub> | 17 N <sub>2</sub> + Lu + 3 B <sub>13</sub> C <sub>2</sub> + 2 H <sub>2</sub> → 33 BN + LuB <sub>6</sub> H <sub>4</sub> C <sub>6</sub> N                                                                          | -77.4798            |
| LuNH <sub>4</sub> B <sub>6</sub> C <sub>6</sub> | 17.5 N <sub>2</sub> + 3 B <sub>13</sub> C <sub>2</sub> + 2 LuH <sub>2</sub> → LuN + 33 BN + LuB <sub>6</sub> H <sub>4</sub> C <sub>6</sub> N                                                                     | -77.1387            |
| LuNH <sub>4</sub> B <sub>6</sub> C <sub>6</sub> | 16.33 N <sub>2</sub> + Lu + 3 B <sub>13</sub> C <sub>2</sub> + 1.333 H <sub>3</sub> N → 33 BN + LuB <sub>6</sub> H <sub>4</sub> C <sub>6</sub> N                                                                 | -75.7144            |
| LuNH <sub>4</sub> B <sub>6</sub> C <sub>6</sub> | 17 N <sub>2</sub> + 3 B <sub>13</sub> C <sub>2</sub> + H <sub>2</sub> + LuH <sub>2</sub> → 33 BN + LuB <sub>6</sub> H <sub>4</sub> C <sub>6</sub> N                                                              | -75.5378            |
| LuNH <sub>4</sub> B <sub>6</sub> C <sub>6</sub> | 16.67 N <sub>2</sub> + 3 B <sub>13</sub> C <sub>2</sub> + 0.6667 H <sub>3</sub> N + LuH <sub>2</sub> → 33 BN + LuB <sub>6</sub> H <sub>4</sub> C <sub>6</sub> N                                                  | -74.6551            |
| LuNH <sub>4</sub> B <sub>6</sub> C <sub>6</sub> | 16.5 N <sub>2</sub> + 3 B <sub>13</sub> C <sub>2</sub> + LuN + 2 H <sub>2</sub> → 33 BN + LuB <sub>6</sub> H <sub>4</sub> C <sub>6</sub> N                                                                       | -73.9369            |
| LuNH <sub>4</sub> B <sub>6</sub> C <sub>6</sub> | 17 N <sub>2</sub> + 3 B <sub>13</sub> C <sub>2</sub> + 2 LuH <sub>2</sub> → Lu + 33 BN + LuB <sub>6</sub> H <sub>4</sub> C <sub>6</sub> N                                                                        | -73.5957            |
| LuNH <sub>4</sub> B <sub>6</sub> C <sub>6</sub> | 15.83 N <sub>2</sub> + 3 B <sub>13</sub> C <sub>2</sub> + LuN + 1.333 H <sub>3</sub> N → 33 BN + LuB <sub>6</sub> H <sub>4</sub> C <sub>6</sub> N                                                                | -72.1715            |
| LuNH <sub>4</sub> B <sub>6</sub> C <sub>6</sub> | 16 N <sub>2</sub> + 3 B <sub>13</sub> C <sub>2</sub> + 2 LuH <sub>2</sub> → LuB <sub>2</sub> + 31 BN + LuB <sub>6</sub> H <sub>4</sub> C <sub>6</sub> N                                                          | -70.4875            |
| LuNH <sub>4</sub> B <sub>6</sub> C <sub>6</sub> | 15 N <sub>2</sub> + 3 B <sub>13</sub> C <sub>2</sub> + 2 LuH <sub>2</sub> → LuB <sub>4</sub> + 29 BN + LuB <sub>6</sub> H <sub>4</sub> C <sub>6</sub> N                                                          | -65.9665            |
| LuNH <sub>4</sub> B <sub>6</sub> C <sub>6</sub> | 0.5 H <sub>8</sub> C <sub>5</sub> + 14.88 N <sub>2</sub> + 1.75 B <sub>13</sub> C <sub>2</sub> + LuB <sub>12</sub> → 28.75 BN + LuB <sub>6</sub> H <sub>4</sub> C <sub>6</sub> N                                 | -63.9485            |
| LuNH <sub>4</sub> B <sub>6</sub> C <sub>6</sub> | 14.3 N <sub>2</sub> + 2.333 B <sub>13</sub> C <sub>2</sub> + 0.3636 B <sub>9</sub> H <sub>11</sub> + 0.3333 Lu <sub>3</sub> C <sub>4</sub> → 27.61 BN + LuB <sub>6</sub> H <sub>4</sub> C <sub>6</sub> N         | -62.9246            |
| LuNH <sub>4</sub> B <sub>6</sub> C <sub>6</sub> | 14.1 N <sub>2</sub> + 2.333 B <sub>13</sub> C <sub>2</sub> + 0.3333 Lu <sub>3</sub> C <sub>4</sub> + 0.5714 B <sub>5</sub> H <sub>7</sub> → 27.19 BN + LuB <sub>6</sub> H <sub>4</sub> C <sub>6</sub> N          | -61.9202            |
| LuNH <sub>4</sub> B <sub>6</sub> C <sub>6</sub> | 0.25 Lu <sub>4</sub> C <sub>7</sub> + 12.95 N <sub>2</sub> + 2.125 B <sub>13</sub> C <sub>2</sub> + 0.3636 B <sub>9</sub> H <sub>11</sub> → 24.9 BN + LuB <sub>6</sub> H <sub>4</sub> C <sub>6</sub> N           | -56.2153            |
| LuNH <sub>4</sub> B <sub>6</sub> C <sub>6</sub> | 0.25 Lu <sub>4</sub> C <sub>7</sub> + 12.74 N <sub>2</sub> + 2.125 B <sub>13</sub> C <sub>2</sub> + 0.5714 B <sub>5</sub> H <sub>7</sub> → 24.48 BN + LuB <sub>6</sub> H <sub>4</sub> C <sub>6</sub> N           | -55.2109            |
| LuNH <sub>4</sub> B <sub>6</sub> C <sub>6</sub> | 12.67 N <sub>2</sub> + 2.333 B <sub>13</sub> C <sub>2</sub> + 0.3333 Lu <sub>3</sub> C <sub>4</sub> + 2 H <sub>2</sub> → 24.33 BN + LuB <sub>6</sub> H <sub>4</sub> C <sub>6</sub> N                             | -55.1837            |
| LuNH <sub>4</sub> B <sub>6</sub> C <sub>6</sub> | 0.25 H <sub>8</sub> C <sub>5</sub> + 12.94 N <sub>2</sub> + 2.375 B <sub>13</sub> C <sub>2</sub> + LuH <sub>2</sub> → 24.88 BN + LuB <sub>6</sub> H <sub>4</sub> C <sub>6</sub> N                                | -54.8963            |
| LuNH <sub>4</sub> B <sub>6</sub> C <sub>6</sub> | 12 N <sub>2</sub> + 2.333 B <sub>13</sub> C <sub>2</sub> + 0.3333 Lu <sub>3</sub> C <sub>4</sub> + 1.333 H <sub>3</sub> N → 24.33 BN + LuB <sub>6</sub> H <sub>4</sub> C <sub>6</sub> N                          | -53.4183            |
| LuNH <sub>4</sub> B <sub>6</sub> C <sub>6</sub> | 0.25 Lu <sub>4</sub> C <sub>7</sub> + 11.31 N <sub>2</sub> + 2.125 B <sub>13</sub> C <sub>2</sub> + 2 H <sub>2</sub> → 21.62 BN + LuB <sub>6</sub> H <sub>4</sub> C <sub>6</sub> N                               | -48.4744            |
| LuNH <sub>4</sub> B <sub>6</sub> C <sub>6</sub> | 9.484 Lu <sub>4</sub> C <sub>7</sub> + 8.875 B <sub>9</sub> H <sub>11</sub> + H <sub>3</sub> N → 12.08 H <sub>8</sub> C <sub>5</sub> + 36.94 LuB <sub>2</sub> + LuB <sub>6</sub> H <sub>4</sub> C <sub>6</sub> N | -47.1189            |
| LuNH <sub>4</sub> B <sub>6</sub> C <sub>6</sub> | 0.25 Lu <sub>4</sub> C <sub>7</sub> + 10.65 N <sub>2</sub> + 2.125 B <sub>13</sub> C <sub>2</sub> + 1.333 H <sub>3</sub> N → 21.63 BN + LuB <sub>6</sub> H <sub>4</sub> C <sub>6</sub> N                         | -46.7090            |
| LuNH <sub>4</sub> B <sub>6</sub> C <sub>6</sub> | 11 N <sub>2</sub> + 3 B <sub>13</sub> C <sub>2</sub> + 2 LuH <sub>2</sub> → LuB <sub>12</sub> + 21 BN + LuB <sub>6</sub> H <sub>4</sub> C <sub>6</sub> N                                                         | -45.8442            |
| LuNH <sub>4</sub> B <sub>6</sub> C <sub>6</sub> | 3 B <sub>13</sub> C <sub>2</sub> + LuB <sub>12</sub> + 46 H <sub>3</sub> N → 67 H <sub>2</sub> + 45 BN + LuB <sub>6</sub> H <sub>4</sub> C <sub>6</sub> N                                                        | -44.3241            |
| LuNH <sub>4</sub> B <sub>6</sub> C <sub>6</sub> | 9.094 Lu <sub>4</sub> C <sub>7</sub> + 8.75 B <sub>9</sub> H <sub>11</sub> + LuN → 11.53 H <sub>8</sub> C <sub>5</sub> + 36.38 LuB <sub>2</sub> + LuB <sub>6</sub> H <sub>4</sub> C <sub>6</sub> N               | -44.1552            |
| LuNH <sub>4</sub> B <sub>6</sub> C <sub>6</sub> | 0.5 H <sub>8</sub> C <sub>5</sub> + 10.87 N <sub>2</sub> + 1.75 B <sub>13</sub> C <sub>2</sub> + LuB <sub>4</sub> → 20.75 BN + LuB <sub>6</sub> H <sub>4</sub> C <sub>6</sub> N                                  | -43.8262            |
| LuNH <sub>4</sub> B <sub>6</sub> C <sub>6</sub> | 3 B <sub>13</sub> C <sub>2</sub> + 79.8 LuB <sub>2</sub> + 79.8 H <sub>3</sub> N → 21.4 B <sub>9</sub> H <sub>11</sub> + 78.8 LuN + LuB <sub>6</sub> H <sub>4</sub> C <sub>6</sub> N                             | -43.4873            |
| LuNH <sub>4</sub> B <sub>6</sub> C <sub>6</sub> | 0.5 H <sub>8</sub> C <sub>5</sub> + 9.875 N <sub>2</sub> + 1.75 B <sub>13</sub> C <sub>2</sub> + LuB <sub>2</sub> → 18.75 BN + LuB <sub>6</sub> H <sub>4</sub> C <sub>6</sub> N                                  | -39.3052            |
| LuNH <sub>4</sub> B <sub>6</sub> C <sub>6</sub> | 12.55 N <sub>2</sub> + 3 B <sub>13</sub> C <sub>2</sub> + 25.1 LuH <sub>2</sub> → 24.1 LuN + 6.6 B <sub>5</sub> H <sub>7</sub> + LuB <sub>6</sub> H <sub>4</sub> C <sub>6</sub> N                                | -36.3129            |
| LuNH <sub>4</sub> B <sub>6</sub> C <sub>6</sub> | 0.5 H <sub>8</sub> C <sub>5</sub> + 8.875 N <sub>2</sub> + Lu + 1.75 B <sub>13</sub> C <sub>2</sub> → 16.75 BN + LuB <sub>6</sub> H <sub>4</sub> C <sub>6</sub> N                                                | -36.1969            |
| LuNH <sub>4</sub> B <sub>6</sub> C <sub>6</sub> | 7.375 Lu <sub>4</sub> C <sub>7</sub> + 0.5 N <sub>2</sub> + 7 B <sub>9</sub> H <sub>11</sub> → 9.125 H <sub>8</sub> C <sub>5</sub> + 28.5 LuB <sub>2</sub> + LuB <sub>6</sub> H <sub>4</sub> C <sub>6</sub> N    | -35.6607            |
| LuNH <sub>4</sub> B <sub>6</sub> C <sub>6</sub> | 3 B <sub>13</sub> C <sub>2</sub> + LuB <sub>4</sub> + 38 H <sub>3</sub> N → 55 H <sub>2</sub> + 37 BN + LuB <sub>6</sub> H <sub>4</sub> C <sub>6</sub> N                                                         | -34.7944            |
| LuNH <sub>4</sub> B <sub>6</sub> C <sub>6</sub> | 16.73 Lu + 3 B <sub>13</sub> C <sub>2</sub> + 16.73 H <sub>3</sub> N → 15.73 LuN + 6.6 B <sub>5</sub> H <sub>7</sub> + LuB <sub>6</sub> H <sub>4</sub> C <sub>6</sub> N                                          | -33.2596            |
| LuNH <sub>4</sub> B <sub>6</sub> C <sub>6</sub> | 3 B <sub>13</sub> C <sub>2</sub> + LuB <sub>2</sub> + 36 H <sub>3</sub> N → 52 H <sub>2</sub> + 35 BN + LuB <sub>6</sub> H <sub>4</sub> C <sub>6</sub> N                                                         | -32.9215            |
| LuNH <sub>4</sub> B <sub>6</sub> C <sub>6</sub> | 0.5 H <sub>8</sub> C <sub>5</sub> + 8.375 N <sub>2</sub> + 1.75 B <sub>13</sub> C <sub>2</sub> + LuN → 16.75 BN + LuB <sub>6</sub> H <sub>4</sub> C <sub>6</sub> N                                               | -32.6540            |
| LuNH <sub>4</sub> B <sub>6</sub> C <sub>6</sub> | Lu + 3 B <sub>13</sub> C <sub>2</sub> + 34 H <sub>3</sub> N → 49 H <sub>2</sub> + 33 BN + LuB <sub>6</sub> H <sub>4</sub> C <sub>6</sub> N                                                                       | -32.4614            |
| LuNH <sub>4</sub> B <sub>6</sub> C <sub>6</sub> | 11.08 N <sub>2</sub> + 3 B <sub>13</sub> C <sub>2</sub> + 22.17 LuH <sub>2</sub> → 3.667 B <sub>9</sub> H <sub>11</sub> + 21.17 LuN + LuB <sub>6</sub> H <sub>4</sub> C <sub>6</sub> N                           | -31.3690            |
| LuNH <sub>4</sub> B <sub>6</sub> C <sub>6</sub> | 3 B <sub>13</sub> C <sub>2</sub> + 34 H <sub>3</sub> N + LuH <sub>2</sub> → 50 H <sub>2</sub> + 33 BN + LuB <sub>6</sub> H <sub>4</sub> C <sub>6</sub> N                                                         | -30.5194            |
| LuNH <sub>4</sub> B <sub>6</sub> C <sub>6</sub> | 3 B <sub>13</sub> C <sub>2</sub> + LuN + 33 H <sub>3</sub> N → 47.5 H <sub>2</sub> + 33 BN + LuB <sub>6</sub> H <sub>4</sub> C <sub>6</sub> N                                                                    | -30.2426            |
| LuNH <sub>4</sub> B <sub>6</sub> C <sub>6</sub> | 0.5 N <sub>2</sub> + 19.14 Lu + 3 B <sub>13</sub> C <sub>2</sub> + 0.3636 B <sub>9</sub> H <sub>11</sub> → 18.14 LuB <sub>2</sub> + LuB <sub>6</sub> H <sub>4</sub> C <sub>6</sub> N                             | -28.8485            |
| LuNH <sub>4</sub> B <sub>6</sub> C <sub>6</sub> | 14.78 Lu + 3 B <sub>13</sub> C <sub>2</sub> + 14.78 H <sub>3</sub> N → 3.667 B <sub>9</sub> H <sub>11</sub> + 13.78 LuN + LuB <sub>6</sub> H <sub>4</sub> C <sub>6</sub> N                                       | -28.6726            |
| LuNH <sub>4</sub> B <sub>6</sub> C <sub>6</sub> | 0.5 N <sub>2</sub> + 18.93 Lu + 3 B <sub>13</sub> C <sub>2</sub> + 0.5714 B <sub>5</sub> H <sub>7</sub> → 17.93 LuB <sub>2</sub> + LuB <sub>6</sub> H <sub>4</sub> C <sub>6</sub> N                              | -28.4900            |
| LuNH <sub>4</sub> B <sub>6</sub> C <sub>6</sub> | 6.516 Lu <sub>4</sub> C <sub>7</sub> + 6.125 B <sub>9</sub> H <sub>11</sub> + BN → 7.922 H <sub>8</sub> C <sub>5</sub> + 25.06 LuB <sub>2</sub> + LuB <sub>6</sub> H <sub>4</sub> C <sub>6</sub> N               | -28.0878            |
| LuNH <sub>4</sub> B <sub>6</sub> C <sub>6</sub> | 19.64 Lu + 3 B <sub>13</sub> C <sub>2</sub> + 0.3636 B <sub>9</sub> H <sub>11</sub> + BN → 18.64 LuB <sub>2</sub> + LuB <sub>6</sub> H <sub>4</sub> C <sub>6</sub> N                                             | -27.2944            |
| LuNH <sub>4</sub> B <sub>6</sub> C <sub>6</sub> | 19.43 Lu + 3 B <sub>13</sub> C <sub>2</sub> + BN + 0.5714 B <sub>5</sub> H <sub>7</sub> → 18.43 LuB <sub>2</sub> + LuB <sub>6</sub> H <sub>4</sub> C <sub>6</sub> N                                              | -26.9358            |
| LuNH <sub>4</sub> B <sub>6</sub> C <sub>6</sub> | 0.5 N <sub>2</sub> + 17.5 Lu + 3 B <sub>13</sub> C <sub>2</sub> + 2 H <sub>2</sub> → 16.5 LuB <sub>2</sub> + LuB <sub>6</sub> H <sub>4</sub> C <sub>6</sub> N                                                    | -26.1939            |
| LuNH <sub>4</sub> B <sub>6</sub> C <sub>6</sub> | 17.83 Lu + 3 B <sub>13</sub> C <sub>2</sub> + 1.333 H <sub>3</sub> N → 0.3333 LuN + 16.5 LuB <sub>2</sub> + LuB <sub>6</sub> H <sub>4</sub> C <sub>6</sub> N                                                     | -25.6094            |
| LuNH <sub>4</sub> B <sub>6</sub> C <sub>6</sub> | 17.91 Lu + 3 B <sub>13</sub> C <sub>2</sub> + 0.09091 B <sub>9</sub> H <sub>11</sub> + H <sub>3</sub> N → 16.91 LuB <sub>2</sub> + LuB <sub>6</sub> H <sub>4</sub> C <sub>6</sub> N                              | -25.5335            |
| LuNH <sub>4</sub> B <sub>6</sub> C <sub>6</sub> | 17.86 Lu + 3 B <sub>13</sub> C <sub>2</sub> + H <sub>3</sub> N + 0.1429 B <sub>5</sub> H <sub>7</sub> → 16.86 LuB <sub>2</sub> + LuB <sub>6</sub> H <sub>4</sub> C <sub>6</sub> N                                | -25.4438            |
| LuNH <sub>4</sub> B <sub>6</sub> C <sub>6</sub> | 18.14 Lu + 3 B <sub>13</sub> C <sub>2</sub> + 0.3636 B <sub>9</sub> H <sub>11</sub> + LuN → 18.14 LuB <sub>2</sub> + LuB <sub>6</sub> H <sub>4</sub> C <sub>6</sub> N                                            | -25.3056            |
| LuNH <sub>4</sub> B <sub>6</sub> C <sub>6</sub> | 3 B <sub>13</sub> C <sub>2</sub> + 20 LuN + 14 H <sub>3</sub> N → 33 BN + 19 LuH <sub>2</sub> + LuB <sub>6</sub> H <sub>4</sub> C <sub>6</sub> N                                                                 | -24.9834            |
| LuNH <sub>4</sub> B <sub>6</sub> C <sub>6</sub> | 17.93 Lu + 3 B <sub>13</sub> C <sub>2</sub> + LuN + 0.5714 B <sub>5</sub> H <sub>7</sub> → 17.93 LuB <sub>2</sub> + LuB <sub>6</sub> H <sub>4</sub> C <sub>6</sub> N                                             | -24.9470            |
| LuNH <sub>4</sub> B <sub>6</sub> C <sub>6</sub> | 17.33 Lu + 3 B <sub>13</sub> C <sub>2</sub> + 1.333 H <sub>3</sub> N → 16.33 LuB <sub>2</sub> + 0.3333 BN + LuB <sub>6</sub> H <sub>4</sub> C <sub>6</sub> N                                                     | -24.9465            |
| LuNH <sub>4</sub> B <sub>6</sub> C <sub>6</sub> | 17.5 Lu + 3 B <sub>13</sub> C <sub>2</sub> + 0.5 H <sub>2</sub> + H <sub>3</sub> N → 16.5 LuB <sub>2</sub> + LuB <sub>6</sub> H <sub>4</sub> C <sub>6</sub> N                                                    | -24.8698            |

Continued on next page

Continued

| Compound                                        | Chemical reaction                                                                                                                                                                                         | Reaction energy(eV) |
|-------------------------------------------------|-----------------------------------------------------------------------------------------------------------------------------------------------------------------------------------------------------------|---------------------|
| LuNH <sub>4</sub> B <sub>6</sub> C <sub>6</sub> | 18 Lu + 3 B <sub>13</sub> C <sub>2</sub> + 2 H <sub>2</sub> + BN → 17 LuB <sub>2</sub> + LuB <sub>6</sub> H <sub>4</sub> C <sub>6</sub> N                                                                 | -24.6397            |
| LuNH <sub>4</sub> B <sub>6</sub> C <sub>6</sub> | 17.5 Lu + 3 B <sub>13</sub> C <sub>2</sub> + 1.333 H <sub>3</sub> N → 0.1667 N <sub>2</sub> + 16.5 LuB <sub>2</sub> + LuB <sub>6</sub> H <sub>4</sub> C <sub>6</sub> N                                    | -24.4284            |
| LuNH <sub>4</sub> B <sub>6</sub> C <sub>6</sub> | 17 Lu + 3 B <sub>13</sub> C <sub>2</sub> + H <sub>3</sub> N + 0.5 LuH <sub>2</sub> → 16.5 LuB <sub>2</sub> + LuB <sub>6</sub> H <sub>4</sub> C <sub>6</sub> N                                             | -23.8988            |
| LuNH <sub>4</sub> B <sub>6</sub> C <sub>6</sub> | 16.5 Lu + 3 B <sub>13</sub> C <sub>2</sub> + LuN + 2 H <sub>2</sub> → 16.5 LuB <sub>2</sub> + LuB <sub>6</sub> H <sub>4</sub> C <sub>6</sub> N                                                            | -22.6510            |
| LuNH <sub>4</sub> B <sub>6</sub> C <sub>6</sub> | 0.5 N <sub>2</sub> + 15.5 Lu + 3 B <sub>13</sub> C <sub>2</sub> + 2 LuH <sub>2</sub> → 16.5 LuB <sub>2</sub> + LuB <sub>6</sub> H <sub>4</sub> C <sub>6</sub> N                                           | -22.3098            |
| LuNH <sub>4</sub> B <sub>6</sub> C <sub>6</sub> | 2.333 B <sub>13</sub> C <sub>2</sub> + 0.3333 Lu <sub>3</sub> C <sub>4</sub> + 25.33 H <sub>3</sub> N → 36 H <sub>2</sub> + 24.33 BN + LuB <sub>6</sub> H <sub>4</sub> C <sub>6</sub> N                   | -21.6406            |
| LuNH <sub>4</sub> B <sub>6</sub> C <sub>6</sub> | 3 B <sub>13</sub> C <sub>2</sub> + 34 LuN + 35 H <sub>2</sub> → 33 BN + 33 LuH <sub>2</sub> + LuB <sub>6</sub> H <sub>4</sub> C <sub>6</sub> N                                                            | -21.1082            |
| LuNH <sub>4</sub> B <sub>6</sub> C <sub>6</sub> | 11.03 N <sub>2</sub> + 1.5 Lu <sub>3</sub> C <sub>4</sub> + 9.6 B <sub>5</sub> H <sub>7</sub> → 3.5 LuB <sub>12</sub> + 21.07 H <sub>3</sub> N + LuB <sub>6</sub> H <sub>4</sub> C <sub>6</sub> N         | -21.0829            |
| LuNH <sub>4</sub> B <sub>6</sub> C <sub>6</sub> | 0.125 H <sub>8</sub> C <sub>5</sub> + 15.47 Lu + 2.688 B <sub>13</sub> C <sub>2</sub> + H <sub>3</sub> N → 14.47 LuB <sub>2</sub> + LuB <sub>6</sub> H <sub>4</sub> C <sub>6</sub> N                      | -20.8627            |
| LuNH <sub>4</sub> B <sub>6</sub> C <sub>6</sub> | 16 Lu + 3 B <sub>13</sub> C <sub>2</sub> + BN + 2 LuH <sub>2</sub> → 17 LuB <sub>2</sub> + LuB <sub>6</sub> H <sub>4</sub> C <sub>6</sub> N                                                               | -20.7557            |
| LuNH <sub>4</sub> B <sub>6</sub> C <sub>6</sub> | 14.5 Lu + 3 B <sub>13</sub> C <sub>2</sub> + LuN + 2 LuH <sub>2</sub> → 16.5 LuB <sub>2</sub> + LuB <sub>6</sub> H <sub>4</sub> C <sub>6</sub> N                                                          | -18.7669            |
| LuNH <sub>4</sub> B <sub>6</sub> C <sub>6</sub> | 0.25 Lu <sub>4</sub> C <sub>7</sub> + 2.125 B <sub>13</sub> C <sub>2</sub> + 22.62 H <sub>3</sub> N → 31.94 H <sub>2</sub> + 21.62 BN + LuB <sub>6</sub> H <sub>4</sub> C <sub>6</sub> N                  | -18.5173            |
| LuNH <sub>4</sub> B <sub>6</sub> C <sub>6</sub> | 9.611 N <sub>2</sub> + 5.333 B <sub>9</sub> H <sub>11</sub> + 1.5 Lu <sub>3</sub> C <sub>4</sub> → 3.5 LuB <sub>12</sub> + 18.22 H <sub>3</sub> N + LuB <sub>6</sub> H <sub>4</sub> C <sub>6</sub> N      | -17.6774            |
| LuNH <sub>4</sub> B <sub>6</sub> C <sub>6</sub> | 5.136 N <sub>2</sub> + 0.3636 B <sub>9</sub> H <sub>11</sub> + 6 C + LuB <sub>12</sub> → 9.273 BN + LuB <sub>6</sub> H <sub>4</sub> C <sub>6</sub> N                                                      | -16.8955            |
| LuNH <sub>4</sub> B <sub>6</sub> C <sub>6</sub> | 0.5 N <sub>2</sub> + 10.07 Lu + 3 B <sub>13</sub> C <sub>2</sub> + 0.3636 B <sub>9</sub> H <sub>11</sub> → 9.068 LuB <sub>4</sub> + LuB <sub>6</sub> H <sub>4</sub> C <sub>6</sub> N                      | -16.0374            |
| LuNH <sub>4</sub> B <sub>6</sub> C <sub>6</sub> | 4.929 N <sub>2</sub> + 6 C + LuB <sub>12</sub> + 0.5714 B <sub>5</sub> H <sub>7</sub> → 8.857 BN + LuB <sub>6</sub> H <sub>4</sub> C <sub>6</sub> N                                                       | -15.8911            |
| LuNH <sub>4</sub> B <sub>6</sub> C <sub>6</sub> | 0.5 N <sub>2</sub> + 9.964 Lu + 3 B <sub>13</sub> C <sub>2</sub> + 0.5714 B <sub>5</sub> H <sub>7</sub> → 8.964 LuB <sub>4</sub> + LuB <sub>6</sub> H <sub>4</sub> C <sub>6</sub> N                       | -15.8256            |
| LuNH <sub>4</sub> B <sub>6</sub> C <sub>6</sub> | 0.5 N <sub>2</sub> + 9.25 Lu + 3 B <sub>13</sub> C <sub>2</sub> + 2 H <sub>2</sub> → 8.25 LuB <sub>4</sub> + LuB <sub>6</sub> H <sub>4</sub> C <sub>6</sub> N                                             | -14.5386            |
| LuNH <sub>4</sub> B <sub>6</sub> C <sub>6</sub> | 10.32 Lu + 3 B <sub>13</sub> C <sub>2</sub> + 0.3636 B <sub>9</sub> H <sub>11</sub> + BN → 9.318 LuB <sub>4</sub> + LuB <sub>6</sub> H <sub>4</sub> C <sub>6</sub> N                                      | -14.1301            |
| LuNH <sub>4</sub> B <sub>6</sub> C <sub>6</sub> | 9.583 Lu + 3 B <sub>13</sub> C <sub>2</sub> + 1.333 H <sub>3</sub> N → 0.3333 LuN + 8.25 LuB <sub>4</sub> + LuB <sub>6</sub> H <sub>4</sub> C <sub>6</sub> N                                              | -13.9541            |
| LuNH <sub>4</sub> B <sub>6</sub> C <sub>6</sub> | 10.21 Lu + 3 B <sub>13</sub> C <sub>2</sub> + BN + 0.5714 B <sub>5</sub> H <sub>7</sub> → 9.214 LuB <sub>4</sub> + LuB <sub>6</sub> H <sub>4</sub> C <sub>6</sub> N                                       | -13.9183            |
| LuNH <sub>4</sub> B <sub>6</sub> C <sub>6</sub> | 0.5 H <sub>8</sub> C <sub>5</sub> + 4.542 N <sub>2</sub> + 1.083 B <sub>13</sub> C <sub>2</sub> + 0.3333 Lu <sub>3</sub> C <sub>4</sub> → 8.083 BN + LuB <sub>6</sub> H <sub>4</sub> C <sub>6</sub> N     | -13.9008            |
| LuNH <sub>4</sub> B <sub>6</sub> C <sub>6</sub> | 9.455 Lu + 3 B <sub>13</sub> C <sub>2</sub> + 0.09091 B <sub>9</sub> H <sub>11</sub> + H <sub>3</sub> N → 8.455 LuB <sub>4</sub> + LuB <sub>6</sub> H <sub>4</sub> C <sub>6</sub> N                       | -13.5892            |
| LuNH <sub>4</sub> B <sub>6</sub> C <sub>6</sub> | 9.429 Lu + 3 B <sub>13</sub> C <sub>2</sub> + H <sub>3</sub> N + 0.1429 B <sub>5</sub> H <sub>7</sub> → 8.429 LuB <sub>4</sub> + LuB <sub>6</sub> H <sub>4</sub> C <sub>6</sub> N                         | -13.5363            |
| LuNH <sub>4</sub> B <sub>6</sub> C <sub>6</sub> | 0.8571 Lu <sub>4</sub> C <sub>7</sub> + 8.033 N <sub>2</sub> + 7.029 B <sub>5</sub> H <sub>7</sub> → 2.429 LuB <sub>12</sub> + 15.07 H <sub>3</sub> N + LuB <sub>6</sub> H <sub>4</sub> C <sub>6</sub> N  | -13.4437            |
| LuNH <sub>4</sub> B <sub>6</sub> C <sub>6</sub> | 9.167 Lu + 3 B <sub>13</sub> C <sub>2</sub> + 1.333 H <sub>3</sub> N → 8.167 LuB <sub>4</sub> + 0.3333 BN + LuB <sub>6</sub> H <sub>4</sub> C <sub>6</sub> N                                              | -13.4089            |
| LuNH <sub>4</sub> B <sub>6</sub> C <sub>6</sub> | 9.25 Lu + 3 B <sub>13</sub> C <sub>2</sub> + 0.5 H <sub>2</sub> + H <sub>3</sub> N → 8.25 LuB <sub>4</sub> + LuB <sub>6</sub> H <sub>4</sub> C <sub>6</sub> N                                             | -13.2145            |
| LuNH <sub>4</sub> B <sub>6</sub> C <sub>6</sub> | 3 B <sub>13</sub> C <sub>2</sub> + LuB <sub>12</sub> + 15.55 H <sub>3</sub> N → 14.55 BN + 6.091 B <sub>5</sub> H <sub>7</sub> + LuB <sub>6</sub> H <sub>4</sub> C <sub>6</sub> N                         | -12.8438            |
| LuNH <sub>4</sub> B <sub>6</sub> C <sub>6</sub> | 1.2 H <sub>8</sub> C <sub>5</sub> + 5.1 N <sub>2</sub> + 3.8 LuB <sub>4</sub> → 9.2 BN + 2.8 LuH <sub>2</sub> + LuB <sub>6</sub> H <sub>4</sub> C <sub>6</sub> N                                          | -12.8297            |
| LuNH <sub>4</sub> B <sub>6</sub> C <sub>6</sub> | 9.25 Lu + 3 B <sub>13</sub> C <sub>2</sub> + 1.333 H <sub>3</sub> N → 0.1667 N <sub>2</sub> + 8.25 LuB <sub>4</sub> + LuB <sub>6</sub> H <sub>4</sub> C <sub>6</sub> N                                    | -12.7732            |
| LuNH <sub>4</sub> B <sub>6</sub> C <sub>6</sub> | 4.75 N <sub>2</sub> + 1.5 Lu <sub>3</sub> C <sub>4</sub> + 3 LuB <sub>2</sub> + 2 LuH <sub>2</sub> → 8.5 LuN + LuB <sub>6</sub> H <sub>4</sub> C <sub>6</sub> N                                           | -12.7028            |
| LuNH <sub>4</sub> B <sub>6</sub> C <sub>6</sub> | 9.5 Lu + 3 B <sub>13</sub> C <sub>2</sub> + 2 H <sub>2</sub> + BN → 8.5 LuB <sub>4</sub> + LuB <sub>6</sub> H <sub>4</sub> C <sub>6</sub> N                                                               | -12.6313            |
| LuNH <sub>4</sub> B <sub>6</sub> C <sub>6</sub> | 9.068 Lu + 3 B <sub>13</sub> C <sub>2</sub> + 0.3636 B <sub>9</sub> H <sub>11</sub> + LuN → 9.068 LuB <sub>4</sub> + LuB <sub>6</sub> H <sub>4</sub> C <sub>6</sub> N                                     | -12.4945            |
| LuNH <sub>4</sub> B <sub>6</sub> C <sub>6</sub> | 8.964 Lu + 3 B <sub>13</sub> C <sub>2</sub> + LuN + 0.5714 B <sub>5</sub> H <sub>7</sub> → 8.964 LuB <sub>4</sub> + LuB <sub>6</sub> H <sub>4</sub> C <sub>6</sub> N                                      | -12.2827            |
| LuNH <sub>4</sub> B <sub>6</sub> C <sub>6</sub> | 8.75 Lu + 3 B <sub>13</sub> C <sub>2</sub> + H <sub>3</sub> N + 0.5 LuH <sub>2</sub> → 8.25 LuB <sub>4</sub> + LuB <sub>6</sub> H <sub>4</sub> C <sub>6</sub> N                                           | -12.2435            |
| LuNH <sub>4</sub> B <sub>6</sub> C <sub>6</sub> | 3 B <sub>13</sub> C <sub>2</sub> + LuB <sub>12</sub> + 14.26 H <sub>3</sub> N → 3.526 B <sub>9</sub> H <sub>11</sub> + 13.26 BN + LuB <sub>6</sub> H <sub>4</sub> C <sub>6</sub> N                        | -11.2798            |
| LuNH <sub>4</sub> B <sub>6</sub> C <sub>6</sub> | 8.25 Lu + 3 B <sub>13</sub> C <sub>2</sub> + LuN + 2 H <sub>2</sub> → 8.25 LuB <sub>4</sub> + LuB <sub>6</sub> H <sub>4</sub> C <sub>6</sub> N                                                            | -10.9957            |
| LuNH <sub>4</sub> B <sub>6</sub> C <sub>6</sub> | 0.8571 Lu <sub>4</sub> C <sub>7</sub> + 6.992 N <sub>2</sub> + 3.905 B <sub>9</sub> H <sub>11</sub> → 2.429 LuB <sub>12</sub> + 12.98 H <sub>3</sub> N + LuB <sub>6</sub> H <sub>4</sub> C <sub>6</sub> N | -10.9503            |
| LuNH <sub>4</sub> B <sub>6</sub> C <sub>6</sub> | 0.5 N <sub>2</sub> + 7.25 Lu + 3 B <sub>13</sub> C <sub>2</sub> + 2 LuH <sub>2</sub> → 8.25 LuB <sub>4</sub> + LuB <sub>6</sub> H <sub>4</sub> C <sub>6</sub> N                                           | -10.6545            |
| LuNH <sub>4</sub> B <sub>6</sub> C <sub>6</sub> | 0.125 H <sub>8</sub> C <sub>5</sub> + 8.234 Lu + 2.688 B <sub>13</sub> C <sub>2</sub> + H <sub>3</sub> N → 7.234 LuB <sub>4</sub> + LuB <sub>6</sub> H <sub>4</sub> C <sub>6</sub> N                      | -10.6422            |
| LuNH <sub>4</sub> B <sub>6</sub> C <sub>6</sub> | 4.769 Lu <sub>3</sub> C <sub>4</sub> + 8.308 H <sub>3</sub> N + 6 BN → 2.615 H <sub>8</sub> C <sub>5</sub> + 13.31 LuN + LuB <sub>6</sub> H <sub>4</sub> C <sub>6</sub> N                                 | -10.5635            |
| LuNH <sub>4</sub> B <sub>6</sub> C <sub>6</sub> | 3.281 N <sub>2</sub> + 2.188 Lu <sub>3</sub> C <sub>4</sub> + 1.2 B <sub>5</sub> H <sub>7</sub> → 0.55 H <sub>8</sub> C <sub>5</sub> + 5.562 LuN + LuB <sub>6</sub> H <sub>4</sub> C <sub>6</sub> N       | -10.4269            |
| LuNH <sub>4</sub> B <sub>6</sub> C <sub>6</sub> | 0.5 H <sub>8</sub> C <sub>5</sub> + 0.5 N <sub>2</sub> + 9.375 Lu + 1.75 B <sub>13</sub> C <sub>2</sub> → 8.375 LuB <sub>2</sub> + LuB <sub>6</sub> H <sub>4</sub> C <sub>6</sub> N                       | -10.1654            |
| LuNH <sub>4</sub> B <sub>6</sub> C <sub>6</sub> | 0.8571 Lu <sub>4</sub> C <sub>7</sub> + 4.214 N <sub>2</sub> + 3 LuB <sub>2</sub> + 2 LuH <sub>2</sub> → 7.429 LuN + LuB <sub>6</sub> H <sub>4</sub> C <sub>6</sub> N                                     | -9.7922             |
| LuNH <sub>4</sub> B <sub>6</sub> C <sub>6</sub> | 4 N <sub>2</sub> + 1.5 Lu <sub>3</sub> C <sub>4</sub> + 1.5 LuB <sub>4</sub> + 2 LuH <sub>2</sub> → 7 LuN + LuB <sub>6</sub> H <sub>4</sub> C <sub>6</sub> N                                              | -9.5076             |
| LuNH <sub>4</sub> B <sub>6</sub> C <sub>6</sub> | 3.75 N <sub>2</sub> + 1.5 Lu <sub>3</sub> C <sub>4</sub> + 3 LuB <sub>2</sub> + 2 H <sub>2</sub> → 6.5 LuN + LuB <sub>6</sub> H <sub>4</sub> C <sub>6</sub> N                                             | -9.5010             |
| LuNH <sub>4</sub> B <sub>6</sub> C <sub>6</sub> | Lu + 3 B <sub>13</sub> C <sub>2</sub> + 11.73 H <sub>3</sub> N → 10.73 BN + 4.455 B <sub>5</sub> H <sub>7</sub> + LuB <sub>6</sub> H <sub>4</sub> C <sub>6</sub> N                                        | -9.4385             |
| LuNH <sub>4</sub> B <sub>6</sub> C <sub>6</sub> | 3.5 N <sub>2</sub> + 6 C + LuB <sub>12</sub> + 2 H <sub>2</sub> → 6 BN + LuB <sub>6</sub> H <sub>4</sub> C <sub>6</sub> N                                                                                 | -9.1546             |
| LuNH <sub>4</sub> B <sub>6</sub> C <sub>6</sub> | 3 B <sub>13</sub> C <sub>2</sub> + LuB <sub>4</sub> + 13 H <sub>3</sub> N → 12 BN + 5 B <sub>5</sub> H <sub>7</sub> + LuB <sub>6</sub> H <sub>4</sub> C <sub>6</sub> N                                    | -8.9523             |
| LuNH <sub>4</sub> B <sub>6</sub> C <sub>6</sub> | 3.031 N <sub>2</sub> + 0.6667 B <sub>9</sub> H <sub>11</sub> + 2.021 Lu <sub>3</sub> C <sub>4</sub> → 0.4167 H <sub>8</sub> C <sub>5</sub> + 5.063 LuN + LuB <sub>6</sub> H <sub>4</sub> C <sub>6</sub> N | -8.8398             |
| LuNH <sub>4</sub> B <sub>6</sub> C <sub>6</sub> | 7.5 Lu + 3 B <sub>13</sub> C <sub>2</sub> + BN + 2 LuH <sub>2</sub> → 8.5 LuB <sub>4</sub> + LuB <sub>6</sub> H <sub>4</sub> C <sub>6</sub> N                                                             | -8.7472             |
| LuNH <sub>4</sub> B <sub>6</sub> C <sub>6</sub> | 1.2 H <sub>8</sub> C <sub>5</sub> + 4.433 N <sub>2</sub> + LuB <sub>12</sub> → 1.867 H <sub>3</sub> N + 6 BN + LuB <sub>6</sub> H <sub>4</sub> C <sub>6</sub> N                                           | -8.6240             |
| LuNH <sub>4</sub> B <sub>6</sub> C <sub>6</sub> | 0.5 H <sub>8</sub> C <sub>5</sub> + 9.875 Lu + 1.75 B <sub>13</sub> C <sub>2</sub> + BN → 8.875 LuB <sub>2</sub> + LuB <sub>6</sub> H <sub>4</sub> C <sub>6</sub> N                                       | -8.6113             |
| LuNH <sub>4</sub> B <sub>6</sub> C <sub>6</sub> | 3 B <sub>13</sub> C <sub>2</sub> + LuB <sub>2</sub> + 12.36 H <sub>3</sub> N → 11.36 BN + 4.727 B <sub>5</sub> H <sub>7</sub> + LuB <sub>6</sub> H <sub>4</sub> C <sub>6</sub> N                          | -8.4890             |
| LuNH <sub>4</sub> B <sub>6</sub> C <sub>6</sub> | 3.5 N <sub>2</sub> + 1.5 Lu <sub>3</sub> C <sub>4</sub> + 0.5 LuB <sub>12</sub> + 2 LuH <sub>2</sub> → 6 LuN + LuB <sub>6</sub> H <sub>4</sub> C <sub>6</sub> N                                           | -8.3966             |
| LuNH <sub>4</sub> B <sub>6</sub> C <sub>6</sub> | Lu + 3 B <sub>13</sub> C <sub>2</sub> + 10.79 H <sub>3</sub> N → 2.579 B <sub>9</sub> H <sub>11</sub> + 9.789 BN + LuB <sub>6</sub> H <sub>4</sub> C <sub>6</sub> N                                       | -8.2947             |
| LuNH <sub>4</sub> B <sub>6</sub> C <sub>6</sub> | 4.5 N <sub>2</sub> + 1.5 Lu <sub>3</sub> C <sub>4</sub> + 4 B <sub>5</sub> H <sub>7</sub> → 3.5 LuB <sub>4</sub> + 8 H <sub>3</sub> N + LuB <sub>6</sub> H <sub>4</sub> C <sub>6</sub> N                  | -8.1927             |
| LuNH <sub>4</sub> B <sub>6</sub> C <sub>6</sub> | 3.25 N <sub>2</sub> + 6 B + 1.5 Lu <sub>3</sub> C <sub>4</sub> + 2 LuH <sub>2</sub> → 5.5 LuN + LuB <sub>6</sub> H <sub>4</sub> C <sub>6</sub> N                                                          | -8.1499             |
| LuNH <sub>4</sub> B <sub>6</sub> C <sub>6</sub> | 3 B <sub>13</sub> C <sub>2</sub> + LuN + 11.41 H <sub>3</sub> N → 11.41 BN + 4.318 B <sub>5</sub> H <sub>7</sub> + LuB <sub>6</sub> H <sub>4</sub> C <sub>6</sub> N                                       | -7.9244             |
| LuNH <sub>4</sub> B <sub>6</sub> C <sub>6</sub> | 0.5 H <sub>8</sub> C <sub>5</sub> + 3.5 N <sub>2</sub> + 3.5 C + LuB <sub>12</sub> → 6 BN + LuB <sub>6</sub> H <sub>4</sub> C <sub>6</sub> N                                                              | -7.9037             |

Continued on next page

Continued

| Compound                                        | Chemical reaction                                                                                                                                                                                     | Reaction energy(eV) |
|-------------------------------------------------|-------------------------------------------------------------------------------------------------------------------------------------------------------------------------------------------------------|---------------------|
| LuNH <sub>4</sub> B <sub>6</sub> C <sub>6</sub> | $3.083 \text{ N}_2 + 1.5 \text{ Lu}_3\text{C}_4 + 3 \text{ LuB}_2 + 1.333 \text{ H}_3\text{N} \rightarrow 6.5 \text{ LuN} + \text{LuB}_6\text{H}_4\text{C}_6\text{N}$                                 | -7.7356             |
| LuNH <sub>4</sub> B <sub>6</sub> C <sub>6</sub> | $1.2 \text{ H}_8\text{C}_5 + 9.5 \text{ Lu} + \text{H}_3\text{N} + 1.2 \text{ B}_5\text{H}_7 \rightarrow 8.5 \text{ LuH}_2 + \text{LuB}_6\text{H}_4\text{C}_6\text{N}$                                | -7.7307             |
| LuNH <sub>4</sub> B <sub>6</sub> C <sub>6</sub> | $3 \text{ B}_{13}\text{C}_2 + \text{LuB}_4 + 11.95 \text{ H}_3\text{N} \rightarrow 2.895 \text{ B}_9\text{H}_{11} + 10.95 \text{ BN} + \text{LuB}_6\text{H}_4\text{C}_6\text{N}$                      | -7.6685             |
| LuNH <sub>4</sub> B <sub>6</sub> C <sub>6</sub> | $2.833 \text{ N}_2 + 6 \text{ C} + \text{LuB}_{12} + 1.333 \text{ H}_3\text{N} \rightarrow 6 \text{ BN} + \text{LuB}_6\text{H}_4\text{C}_6\text{N}$                                                   | -7.3892             |
| LuNH <sub>4</sub> B <sub>6</sub> C <sub>6</sub> | $3 \text{ B}_{13}\text{C}_2 + \text{LuB}_2 + 11.37 \text{ H}_3\text{N} \rightarrow 2.737 \text{ B}_9\text{H}_{11} + 10.37 \text{ BN} + \text{LuB}_6\text{H}_4\text{C}_6\text{N}$                      | -7.2752             |
| LuNH <sub>4</sub> B <sub>6</sub> C <sub>6</sub> | $0.5 \text{ H}_8\text{C}_5 + 0.25 \text{ Lu}_4\text{C}_7 + 3.187 \text{ N}_2 + 0.875 \text{ B}_{13}\text{C}_2 \rightarrow 5.375 \text{ BN} + \text{LuB}_6\text{H}_4\text{C}_6\text{N}$                | -7.1915             |
| LuNH <sub>4</sub> B <sub>6</sub> C <sub>6</sub> | $6.25 \text{ Lu} + 3 \text{ B}_{13}\text{C}_2 + \text{LuN} + 2 \text{ LuH}_2 \rightarrow 8.25 \text{ LuB}_4 + \text{LuB}_6\text{H}_4\text{C}_6\text{N}$                                               | -7.1116             |
| LuNH <sub>4</sub> B <sub>6</sub> C <sub>6</sub> | $3 \text{ B}_{13}\text{C}_2 + 11.27 \text{ H}_3\text{N} + \text{LuH}_2 \rightarrow 10.27 \text{ BN} + 4.545 \text{ B}_5\text{H}_7 + \text{LuB}_6\text{H}_4\text{C}_6\text{N}$                         | -7.0266             |
| LuNH <sub>4</sub> B <sub>6</sub> C <sub>6</sub> | $3 \text{ B}_{13}\text{C}_2 + \text{LuN} + 10.5 \text{ H}_3\text{N} \rightarrow 2.5 \text{ B}_9\text{H}_{11} + 10.5 \text{ BN} + \text{LuB}_6\text{H}_4\text{C}_6\text{N}$                            | -6.8156             |
| LuNH <sub>4</sub> B <sub>6</sub> C <sub>6</sub> | $3.907 \text{ N}_2 + 2.222 \text{ B}_9\text{H}_{11} + 1.5 \text{ Lu}_3\text{C}_4 \rightarrow 3.5 \text{ LuB}_4 + 6.815 \text{ H}_3\text{N} + \text{LuB}_6\text{H}_4\text{C}_6\text{N}$                | -6.7737             |
| LuNH <sub>4</sub> B <sub>6</sub> C <sub>6</sub> | $1.2 \text{ H}_8\text{C}_5 + 8.967 \text{ Lu} + 0.6667 \text{ B}_9\text{H}_{11} + \text{H}_3\text{N} \rightarrow 7.967 \text{ LuH}_2 + \text{LuB}_6\text{H}_4\text{C}_6\text{N}$                      | -6.7400             |
| LuNH <sub>4</sub> B <sub>6</sub> C <sub>6</sub> | $3.036 \text{ N}_2 + 1.5 \text{ Lu}_3\text{C}_4 + 1.571 \text{ LuB}_2 + 0.5714 \text{ B}_5\text{H}_7 \rightarrow 5.071 \text{ LuN} + \text{LuB}_6\text{H}_4\text{C}_6\text{N}$                        | -6.7358             |
| LuNH <sub>4</sub> B <sub>6</sub> C <sub>6</sub> | $1.2 \text{ H}_8\text{C}_5 + 24.33 \text{ LuN} + 5.867 \text{ B}_5\text{H}_7 \rightarrow 23.33 \text{ BN} + 23.33 \text{ LuH}_2 + \text{LuB}_6\text{H}_4\text{C}_6\text{N}$                           | -6.6651             |
| LuNH <sub>4</sub> B <sub>6</sub> C <sub>6</sub> | $0.5 \text{ H}_8\text{C}_5 + 8.375 \text{ Lu} + 1.75 \text{ B}_{13}\text{C}_2 + \text{LuN} \rightarrow 8.375 \text{ LuB}_2 + \text{LuB}_6\text{H}_4\text{C}_6\text{N}$                                | -6.6225             |
| LuNH <sub>4</sub> B <sub>6</sub> C <sub>6</sub> | $0.8571 \text{ Lu}_4\text{C}_7 + 3.464 \text{ N}_2 + 1.5 \text{ LuB}_4 + 2 \text{ LuH}_2 \rightarrow 5.929 \text{ LuN} + \text{LuB}_6\text{H}_4\text{C}_6\text{N}$                                    | -6.5969             |
| LuNH <sub>4</sub> B <sub>6</sub> C <sub>6</sub> | $0.8571 \text{ Lu}_4\text{C}_7 + 3.214 \text{ N}_2 + 3 \text{ LuB}_2 + 2 \text{ H}_2 \rightarrow 5.429 \text{ LuN} + \text{LuB}_6\text{H}_4\text{C}_6\text{N}$                                        | -6.5904             |
| LuNH <sub>4</sub> B <sub>6</sub> C <sub>6</sub> | $2.932 \text{ N}_2 + 0.3636 \text{ B}_9\text{H}_{11} + 1.5 \text{ Lu}_3\text{C}_4 + 1.364 \text{ LuB}_2 \rightarrow 4.864 \text{ LuN} + \text{LuB}_6\text{H}_4\text{C}_6\text{N}$                     | -6.3582             |
| LuNH <sub>4</sub> B <sub>6</sub> C <sub>6</sub> | $3 \text{ N}_2 + 1.5 \text{ Lu}_3\text{C}_4 + 1.5 \text{ LuB}_4 + 2 \text{ H}_2 \rightarrow 5 \text{ LuN} + \text{LuB}_6\text{H}_4\text{C}_6\text{N}$                                                 | -6.3058             |
| LuNH <sub>4</sub> B <sub>6</sub> C <sub>6</sub> | $1.25 \text{ Lu}_4\text{C}_7 + 2.5 \text{ N}_2 + 1.2 \text{ B}_5\text{H}_7 \rightarrow 0.55 \text{ H}_8\text{C}_5 + 4 \text{ LuN} + \text{LuB}_6\text{H}_4\text{C}_6\text{N}$                         | -6.1822             |
| LuNH <sub>4</sub> B <sub>6</sub> C <sub>6</sub> | $1.5 \text{ Lu}_3\text{C}_4 + 6.5 \text{ LuB}_2 + 8 \text{ H}_3\text{N} \rightarrow 7 \text{ BN} + 10 \text{ LuH}_2 + \text{LuB}_6\text{H}_4\text{C}_6\text{N}$                                       | -6.1788             |
| LuNH <sub>4</sub> B <sub>6</sub> C <sub>6</sub> | $1.2 \text{ H}_8\text{C}_5 + 3.5 \text{ N}_2 + \text{LuB}_{12} \rightarrow 2.8 \text{ H}_2 + 6 \text{ BN} + \text{LuB}_6\text{H}_4\text{C}_6\text{N}$                                                 | -6.1524             |
| LuNH <sub>4</sub> B <sub>6</sub> C <sub>6</sub> | $1.2 \text{ H}_8\text{C}_5 + 0.5 \text{ N}_2 + 8 \text{ Lu} + 1.2 \text{ B}_5\text{H}_7 \rightarrow 7 \text{ LuH}_2 + \text{LuB}_6\text{H}_4\text{C}_6\text{N}$                                       | -6.1417             |
| LuNH <sub>4</sub> B <sub>6</sub> C <sub>6</sub> | $5.667 \text{ N}_2 + 3 \text{ B}_{13}\text{C}_2 + 17.5 \text{ LuH}_2 \rightarrow 16.5 \text{ LuB}_2 + 10.33 \text{ H}_3\text{N} + \text{LuB}_6\text{H}_4\text{C}_6\text{N}$                           | -5.8902             |
| LuNH <sub>4</sub> B <sub>6</sub> C <sub>6</sub> | $3 \text{ B}_{13}\text{C}_2 + 10.32 \text{ H}_3\text{N} + \text{LuH}_2 \rightarrow 2.632 \text{ B}_9\text{H}_{11} + 9.316 \text{ BN} + \text{LuB}_6\text{H}_4\text{C}_6\text{N}$                      | -5.8595             |
| LuNH <sub>4</sub> B <sub>6</sub> C <sub>6</sub> | $2.904 \text{ N}_2 + 0.4615 \text{ B}_{13}\text{C}_2 + 1.269 \text{ Lu}_3\text{C}_4 + 2 \text{ LuH}_2 \rightarrow 4.808 \text{ LuN} + \text{LuB}_6\text{H}_4\text{C}_6\text{N}$                       | -5.7323             |
| LuNH <sub>4</sub> B <sub>6</sub> C <sub>6</sub> | $2.983 \text{ N}_2 + 1.5 \text{ Lu}_3\text{C}_4 + 1.2 \text{ B}_5\text{H}_7 \rightarrow 3.5 \text{ LuN} + 1.467 \text{ H}_3\text{N} + \text{LuB}_6\text{H}_4\text{C}_6\text{N}$                       | -5.6361             |
| LuNH <sub>4</sub> B <sub>6</sub> C <sub>6</sub> | $0.8571 \text{ Lu}_4\text{C}_7 + 2.964 \text{ N}_2 + 0.5 \text{ LuB}_{12} + 2 \text{ LuH}_2 \rightarrow 4.929 \text{ LuN} + \text{LuB}_6\text{H}_4\text{C}_6\text{N}$                                 | -5.4859             |
| LuNH <sub>4</sub> B <sub>6</sub> C <sub>6</sub> | $0.5 \text{ N}_2 + 72 \text{ B} + 1.5 \text{ Lu}_3\text{C}_4 + 2 \text{ LuH}_2 \rightarrow 5.5 \text{ LuB}_{12} + \text{LuB}_6\text{H}_4\text{C}_6\text{N}$                                           | -5.4366             |
| LuNH <sub>4</sub> B <sub>6</sub> C <sub>6</sub> | $0.8571 \text{ Lu}_4\text{C}_7 + 2.714 \text{ N}_2 + 6 \text{ B} + 2 \text{ LuH}_2 \rightarrow 4.429 \text{ LuN} + \text{LuB}_6\text{H}_4\text{C}_6\text{N}$                                          | -5.2393             |
| LuNH <sub>4</sub> B <sub>6</sub> C <sub>6</sub> | $2 \text{ N}_2 + \text{B}_9\text{H}_{11} + 1.5 \text{ Lu}_3\text{C}_4 \rightarrow 3 \text{ BN} + 3.5 \text{ LuH}_2 + \text{LuB}_6\text{H}_4\text{C}_6\text{N}$                                        | -5.2320             |
| LuNH <sub>4</sub> B <sub>6</sub> C <sub>6</sub> | $2.806 \text{ N}_2 + 0.6667 \text{ B}_9\text{H}_{11} + 1.5 \text{ Lu}_3\text{C}_4 \rightarrow 3.5 \text{ LuN} + 1.111 \text{ H}_3\text{N} + \text{LuB}_6\text{H}_4\text{C}_6\text{N}$                 | -5.2104             |
| LuNH <sub>4</sub> B <sub>6</sub> C <sub>6</sub> | $16.62 \text{ C} + \text{LuB}_{12} + 7 \text{ H}_3\text{N} \rightarrow 2.125 \text{ H}_8\text{C}_5 + 6 \text{ BN} + \text{LuB}_6\text{H}_4\text{C}_6\text{N}$                                         | -5.2026             |
| LuNH <sub>4</sub> B <sub>6</sub> C <sub>6</sub> | $2.5 \text{ N}_2 + 1.5 \text{ Lu}_3\text{C}_4 + 0.5 \text{ LuB}_{12} + 2 \text{ H}_2 \rightarrow 4 \text{ LuN} + \text{LuB}_6\text{H}_4\text{C}_6\text{N}$                                            | -5.1948             |
| LuNH <sub>4</sub> B <sub>6</sub> C <sub>6</sub> | $1.2 \text{ H}_8\text{C}_5 + 0.5 \text{ N}_2 + 7.467 \text{ Lu} + 0.6667 \text{ B}_9\text{H}_{11} \rightarrow 6.467 \text{ LuH}_2 + \text{LuB}_6\text{H}_4\text{C}_6\text{N}$                         | -5.1510             |
| LuNH <sub>4</sub> B <sub>6</sub> C <sub>6</sub> | $2.643 \text{ N}_2 + 1.5 \text{ Lu}_3\text{C}_4 + 0.7857 \text{ LuB}_4 + 0.5714 \text{ B}_5\text{H}_7 \rightarrow 4.286 \text{ LuN} + \text{LuB}_6\text{H}_4\text{C}_6\text{N}$                       | -5.0621             |
| LuNH <sub>4</sub> B <sub>6</sub> C <sub>6</sub> | $2.25 \text{ N}_2 + 6 \text{ B} + 1.5 \text{ Lu}_3\text{C}_4 + 2 \text{ H}_2 \rightarrow 3.5 \text{ LuN} + \text{LuB}_6\text{H}_4\text{C}_6\text{N}$                                                  | -4.9481             |
| LuNH <sub>4</sub> B <sub>6</sub> C <sub>6</sub> | $84 \text{ B} + \text{LuN} + 1.5 \text{ Lu}_3\text{C}_4 + 2 \text{ LuH}_2 \rightarrow 6.5 \text{ LuB}_{12} + \text{LuB}_6\text{H}_4\text{C}_6\text{N}$                                                | -4.9432             |
| LuNH <sub>4</sub> B <sub>6</sub> C <sub>6</sub> | $1.155 \text{ Lu}_4\text{C}_7 + 2.31 \text{ N}_2 + 0.6667 \text{ B}_9\text{H}_{11} \rightarrow 0.4167 \text{ H}_8\text{C}_5 + 3.619 \text{ LuN} + \text{LuB}_6\text{H}_4\text{C}_6\text{N}$           | -4.9185             |
| LuNH <sub>4</sub> B <sub>6</sub> C <sub>6</sub> | $2.591 \text{ N}_2 + 0.3636 \text{ B}_9\text{H}_{11} + 1.5 \text{ Lu}_3\text{C}_4 + 0.6818 \text{ LuB}_4 \rightarrow 4.182 \text{ LuN} + \text{LuB}_6\text{H}_4\text{C}_6\text{N}$                    | -4.9058             |
| LuNH <sub>4</sub> B <sub>6</sub> C <sub>6</sub> | $0.8571 \text{ Lu}_4\text{C}_7 + 2.548 \text{ N}_2 + 3 \text{ LuB}_2 + 1.333 \text{ H}_3\text{N} \rightarrow 5.429 \text{ LuN} + \text{LuB}_6\text{H}_4\text{C}_6\text{N}$                            | -4.8250             |
| LuNH <sub>4</sub> B <sub>6</sub> C <sub>6</sub> | $2.333 \text{ B}_{13}\text{C}_2 + 0.3333 \text{ Lu}_3\text{C}_4 + 8.97 \text{ H}_3\text{N} \rightarrow 7.97 \text{ BN} + 3.273 \text{ B}_5\text{H}_7 + \text{LuB}_6\text{H}_4\text{C}_6\text{N}$      | -4.7258             |
| LuNH <sub>4</sub> B <sub>6</sub> C <sub>6</sub> | $2.333 \text{ N}_2 + 1.5 \text{ Lu}_3\text{C}_4 + 1.5 \text{ LuB}_4 + 1.333 \text{ H}_3\text{N} \rightarrow 5 \text{ LuN} + \text{LuB}_6\text{H}_4\text{C}_6\text{N}$                                 | -4.5404             |
| LuNH <sub>4</sub> B <sub>6</sub> C <sub>6</sub> | $0.8571 \text{ Lu}_4\text{C}_7 + 3.5 \text{ N}_2 + 3.143 \text{ B}_5\text{H}_7 \rightarrow 2.429 \text{ LuB}_4 + 6 \text{ H}_3\text{N} + \text{LuB}_6\text{H}_4\text{C}_6\text{N}$                    | -4.4994             |
| LuNH <sub>4</sub> B <sub>6</sub> C <sub>6</sub> | $2.381 \text{ N}_2 + 1.5 \text{ Lu}_3\text{C}_4 + 0.2619 \text{ LuB}_{12} + 0.5714 \text{ B}_5\text{H}_7 \rightarrow 3.762 \text{ LuN} + \text{LuB}_6\text{H}_4\text{C}_6\text{N}$                    | -4.4802             |
| LuNH <sub>4</sub> B <sub>6</sub> C <sub>6</sub> | $2.364 \text{ N}_2 + 0.3636 \text{ B}_9\text{H}_{11} + 1.5 \text{ Lu}_3\text{C}_4 + 0.2273 \text{ LuB}_{12} \rightarrow 3.727 \text{ LuN} + \text{LuB}_6\text{H}_4\text{C}_6\text{N}$                 | -4.4008             |
| LuNH <sub>4</sub> B <sub>6</sub> C <sub>6</sub> | $2.25 \text{ N}_2 + 3.143 \text{ B} + 1.5 \text{ Lu}_3\text{C}_4 + 0.5714 \text{ B}_5\text{H}_7 \rightarrow 3.5 \text{ LuN} + \text{LuB}_6\text{H}_4\text{C}_6\text{N}$                               | -4.3510             |
| LuNH <sub>4</sub> B <sub>6</sub> C <sub>6</sub> | $2.25 \text{ N}_2 + 0.3636 \text{ B}_9\text{H}_{11} + 2.727 \text{ B} + 1.5 \text{ Lu}_3\text{C}_4 \rightarrow 3.5 \text{ LuN} + \text{LuB}_6\text{H}_4\text{C}_6\text{N}$                            | -4.2887             |
| LuNH <sub>4</sub> B <sub>6</sub> C <sub>6</sub> | $0.5 \text{ H}_8\text{C}_5 + 0.5 \text{ N}_2 + 5.187 \text{ Lu} + 1.75 \text{ B}_{13}\text{C}_2 \rightarrow 4.187 \text{ LuB}_4 + \text{LuB}_6\text{H}_4\text{C}_6\text{N}$                           | -4.2495             |
| LuNH <sub>4</sub> B <sub>6</sub> C <sub>6</sub> | $2.333 \text{ B}_{13}\text{C}_2 + 0.3333 \text{ Lu}_3\text{C}_4 + 8.281 \text{ H}_3\text{N} \rightarrow 1.895 \text{ B}_9\text{H}_{11} + 7.281 \text{ BN} + \text{LuB}_6\text{H}_4\text{C}_6\text{N}$ | -3.8855             |
| LuNH <sub>4</sub> B <sub>6</sub> C <sub>6</sub> | $2.25 \text{ N}_2 + 2.75 \text{ B}_9\text{H}_{11} + 1.5 \text{ Lu}_3\text{C}_4 \rightarrow 3.5 \text{ LuN} + 3.75 \text{ B}_5\text{H}_7 + \text{LuB}_6\text{H}_4\text{C}_6\text{N}$                   | -3.8801             |
| LuNH <sub>4</sub> B <sub>6</sub> C <sub>6</sub> | $0.8571 \text{ Lu}_4\text{C}_7 + 2.5 \text{ N}_2 + 1.571 \text{ LuB}_2 + 0.5714 \text{ B}_5\text{H}_7 \rightarrow 4 \text{ LuN} + \text{LuB}_6\text{H}_4\text{C}_6\text{N}$                           | -3.8252             |
| LuNH <sub>4</sub> B <sub>6</sub> C <sub>6</sub> | $2.25 \text{ N}_2 + 0.6667 \text{ B}_9\text{H}_{11} + 1.5 \text{ Lu}_3\text{C}_4 \rightarrow 3.5 \text{ LuN} + 1.667 \text{ H}_2 + \text{LuB}_6\text{H}_4\text{C}_6\text{N}$                          | -3.7392             |
| LuNH <sub>4</sub> B <sub>6</sub> C <sub>6</sub> | $0.8571 \text{ Lu}_4\text{C}_7 + 5.964 \text{ LuB}_2 + 6.929 \text{ H}_3\text{N} \rightarrow 5.929 \text{ BN} + 8.393 \text{ LuH}_2 + \text{LuB}_6\text{H}_4\text{C}_6\text{N}$                       | -3.6965             |
| LuNH <sub>4</sub> B <sub>6</sub> C <sub>6</sub> | $2.25 \text{ N}_2 + 1.5 \text{ Lu}_3\text{C}_4 + 1.2 \text{ B}_5\text{H}_7 \rightarrow 3.5 \text{ LuN} + 2.2 \text{ H}_2 + \text{LuB}_6\text{H}_4\text{C}_6\text{N}$                                  | -3.6941             |
| LuNH <sub>4</sub> B <sub>6</sub> C <sub>6</sub> | $0.25 \text{ Lu}_4\text{C}_7 + 2.125 \text{ B}_{13}\text{C}_2 + 8.108 \text{ H}_3\text{N} \rightarrow 7.108 \text{ BN} + 2.903 \text{ B}_5\text{H}_7 + \text{LuB}_6\text{H}_4\text{C}_6\text{N}$      | -3.5113             |
| LuNH <sub>4</sub> B <sub>6</sub> C <sub>6</sub> | $0.8571 \text{ Lu}_4\text{C}_7 + 2.396 \text{ N}_2 + 0.3636 \text{ B}_9\text{H}_{11} + 1.364 \text{ LuB}_2 \rightarrow 3.792 \text{ LuN} + \text{LuB}_6\text{H}_4\text{C}_6\text{N}$                  | -3.4476             |
| LuNH <sub>4</sub> B <sub>6</sub> C <sub>6</sub> | $1.833 \text{ N}_2 + 1.5 \text{ Lu}_3\text{C}_4 + 0.5 \text{ LuB}_{12} + 1.333 \text{ H}_3\text{N} \rightarrow 4 \text{ LuN} + \text{LuB}_6\text{H}_4\text{C}_6\text{N}$                              | -3.4294             |
| LuNH <sub>4</sub> B <sub>6</sub> C <sub>6</sub> | $0.8571 \text{ Lu}_4\text{C}_7 + 2.464 \text{ N}_2 + 1.5 \text{ LuB}_4 + 2 \text{ H}_2 \rightarrow 3.929 \text{ LuN} + \text{LuB}_6\text{H}_4\text{C}_6\text{N}$                                      | -3.3952             |
| LuNH <sub>4</sub> B <sub>6</sub> C <sub>6</sub> | $0.8571 \text{ Lu}_4\text{C}_7 + 3.034 \text{ N}_2 + 1.746 \text{ B}_9\text{H}_{11} \rightarrow 2.429 \text{ LuB}_4 + 5.069 \text{ H}_3\text{N} + \text{LuB}_6\text{H}_4\text{C}_6\text{N}$           | -3.3845             |
| LuNH <sub>4</sub> B <sub>6</sub> C <sub>6</sub> | $0.5 \text{ H}_8\text{C}_5 + 2.813 \text{ N}_2 + 0.875 \text{ Lu}_3\text{C}_4 + 3 \text{ LuB}_2 \rightarrow 4.625 \text{ LuN} + \text{LuB}_6\text{H}_4\text{C}_6\text{N}$                             | -3.3804             |

Continued on next page

Continued

| Compound                                        | Chemical reaction                                                                                                                                                                                          | Reaction energy(eV) |
|-------------------------------------------------|------------------------------------------------------------------------------------------------------------------------------------------------------------------------------------------------------------|---------------------|
| LuNH <sub>4</sub> B <sub>6</sub> C <sub>6</sub> | 0.7253 Lu <sub>4</sub> C <sub>7</sub> + 2.451 N <sub>2</sub> + 0.4615 B <sub>13</sub> C <sub>2</sub> + 2 LuH <sub>2</sub> → 3.901 LuN + LuB <sub>6</sub> H <sub>4</sub> C <sub>6</sub> N                   | -3.2695             |
| LuNH <sub>4</sub> B <sub>6</sub> C <sub>6</sub> | 0.5 N <sub>2</sub> + 48 B + 1.5 Lu <sub>3</sub> C <sub>4</sub> + 2 H <sub>2</sub> → 3.5 LuB <sub>12</sub> + LuB <sub>6</sub> H <sub>4</sub> C <sub>6</sub> N                                               | -3.2215             |
| LuNH <sub>4</sub> B <sub>6</sub> C <sub>6</sub> | 2.093 N <sub>2</sub> + 0.2098 B <sub>13</sub> C <sub>2</sub> + 0.3636 B <sub>9</sub> H <sub>11</sub> + 1.395 Lu <sub>3</sub> C <sub>4</sub> → 3.185 LuN + LuB <sub>6</sub> H <sub>4</sub> C <sub>6</sub> N | -3.1898             |
| LuNH <sub>4</sub> B <sub>6</sub> C <sub>6</sub> | 2.867 N <sub>2</sub> + 1.5 Lu <sub>3</sub> C <sub>4</sub> + 2.6 B <sub>5</sub> H <sub>7</sub> → 3.5 LuB <sub>2</sub> + 4.733 H <sub>3</sub> N + LuB <sub>6</sub> H <sub>4</sub> C <sub>6</sub> N           | -3.1866             |
| LuNH <sub>4</sub> B <sub>6</sub> C <sub>6</sub> | 1.583 N <sub>2</sub> + 6 B + 1.5 Lu <sub>3</sub> C <sub>4</sub> + 1.333 H <sub>3</sub> N → 3.5 LuN + LuB <sub>6</sub> H <sub>4</sub> C <sub>6</sub> N                                                      | -3.1827             |
| LuNH <sub>4</sub> B <sub>6</sub> C <sub>6</sub> | 0.5 N <sub>2</sub> + 28 B + 1.5 Lu <sub>3</sub> C <sub>4</sub> + 2 LuH <sub>2</sub> → 5.5 LuB <sub>4</sub> + LuB <sub>6</sub> H <sub>4</sub> C <sub>6</sub> N                                              | -3.1718             |
| LuNH <sub>4</sub> B <sub>6</sub> C <sub>6</sub> | 2.069 N <sub>2</sub> + 0.2418 B <sub>13</sub> C <sub>2</sub> + 1.379 Lu <sub>3</sub> C <sub>4</sub> + 0.5714 B <sub>5</sub> H <sub>7</sub> → 3.137 LuN + LuB <sub>6</sub> H <sub>4</sub> C <sub>6</sub> N  | -3.0846             |
| LuNH <sub>4</sub> B <sub>6</sub> C <sub>6</sub> | 0.8571 Lu <sub>4</sub> C <sub>7</sub> + 0.5 N <sub>2</sub> + 59.14 B + 2 LuH <sub>2</sub> → 4.429 LuB <sub>12</sub> + LuB <sub>6</sub> H <sub>4</sub> C <sub>6</sub> N                                     | -3.0545             |
| LuNH <sub>4</sub> B <sub>6</sub> C <sub>6</sub> | 2.917 N <sub>2</sub> + 3 B <sub>13</sub> C <sub>2</sub> + 9.25 LuH <sub>2</sub> → 8.25 LuB <sub>4</sub> + 4.833 H <sub>3</sub> N + LuB <sub>6</sub> H <sub>4</sub> C <sub>6</sub> N                        | -2.9744             |
| LuNH <sub>4</sub> B <sub>6</sub> C <sub>6</sub> | 71 B + 1.5 Lu <sub>3</sub> C <sub>4</sub> + BN + 2 LuH <sub>2</sub> → 5.5 LuB <sub>12</sub> + LuB <sub>6</sub> H <sub>4</sub> C <sub>6</sub> N                                                             | -2.8698             |
| LuNH <sub>4</sub> B <sub>6</sub> C <sub>6</sub> | 0.25 Lu <sub>4</sub> C <sub>7</sub> + 2.125 B <sub>13</sub> C <sub>2</sub> + 7.497 H <sub>3</sub> N → 1.681 B <sub>9</sub> H <sub>11</sub> + 6.497 BN + LuB <sub>6</sub> H <sub>4</sub> C <sub>6</sub> N   | -2.7658             |
| LuNH <sub>4</sub> B <sub>6</sub> C <sub>6</sub> | 60 B + LuN + 1.5 Lu <sub>3</sub> C <sub>4</sub> + 2 H <sub>2</sub> → 4.5 LuB <sub>12</sub> + LuB <sub>6</sub> H <sub>4</sub> C <sub>6</sub> N                                                              | -2.7282             |
| LuNH <sub>4</sub> B <sub>6</sub> C <sub>6</sub> | 0.8571 Lu <sub>4</sub> C <sub>7</sub> + 2.448 N <sub>2</sub> + 1.2 B <sub>5</sub> H <sub>7</sub> → 2.429 LuN + 1.467 H <sub>3</sub> N + LuB <sub>6</sub> H <sub>4</sub> C <sub>6</sub> N                   | -2.7255             |
| LuNH <sub>4</sub> B <sub>6</sub> C <sub>6</sub> | 0.5 N <sub>2</sub> + 45.14 B + 1.5 Lu <sub>3</sub> C <sub>4</sub> + 0.5714 B <sub>5</sub> H <sub>7</sub> → 3.5 LuB <sub>12</sub> + LuB <sub>6</sub> H <sub>4</sub> C <sub>6</sub> N                        | -2.6243             |
| LuNH <sub>4</sub> B <sub>6</sub> C <sub>6</sub> | 1.2 H <sub>8</sub> C <sub>5</sub> + 7 Lu + LuN + 1.2 B <sub>5</sub> H <sub>7</sub> → 7 LuH <sub>2</sub> + LuB <sub>6</sub> H <sub>4</sub> C <sub>6</sub> N                                                 | -2.5988             |
| LuNH <sub>4</sub> B <sub>6</sub> C <sub>6</sub> | 0.5 N <sub>2</sub> + 0.3636 B <sub>9</sub> H <sub>11</sub> + 44.73 B + 1.5 Lu <sub>3</sub> C <sub>4</sub> → 3.5 LuB <sub>12</sub> + LuB <sub>6</sub> H <sub>4</sub> C <sub>6</sub> N                       | -2.5621             |
| LuNH <sub>4</sub> B <sub>6</sub> C <sub>6</sub> | 0.8571 Lu <sub>4</sub> C <sub>7</sub> + 71.14 B + LuN + 2 LuH <sub>2</sub> → 5.429 LuB <sub>12</sub> + LuB <sub>6</sub> H <sub>4</sub> C <sub>6</sub> N                                                    | -2.5612             |
| LuNH <sub>4</sub> B <sub>6</sub> C <sub>6</sub> | 1.904 N <sub>2</sub> + 0.4615 B <sub>13</sub> C <sub>2</sub> + 1.269 Lu <sub>3</sub> C <sub>4</sub> + 2 H <sub>2</sub> → 2.808 LuN + LuB <sub>6</sub> H <sub>4</sub> C <sub>6</sub> N                      | -2.5306             |
| LuNH <sub>4</sub> B <sub>6</sub> C <sub>6</sub> | 1.429 N <sub>2</sub> + 1.5 Lu <sub>3</sub> C <sub>4</sub> + 1.571 B <sub>5</sub> H <sub>7</sub> → 1.857 BN + 3.5 LuH <sub>2</sub> + LuB <sub>6</sub> H <sub>4</sub> C <sub>6</sub> N                       | -2.4698             |
| LuNH <sub>4</sub> B <sub>6</sub> C <sub>6</sub> | 54 B + 1.5 Lu <sub>3</sub> C <sub>4</sub> + H <sub>3</sub> N + 0.5 LuH <sub>2</sub> → 4 LuB <sub>12</sub> + LuB <sub>6</sub> H <sub>4</sub> C <sub>6</sub> N                                               | -2.4512             |
| LuNH <sub>4</sub> B <sub>6</sub> C <sub>6</sub> | 1.2 H <sub>8</sub> C <sub>5</sub> + 7.3 Lu + BN + B <sub>5</sub> H <sub>7</sub> → 6.3 LuH <sub>2</sub> + LuB <sub>6</sub> H <sub>4</sub> C <sub>6</sub> N                                                  | -2.4245             |
| LuNH <sub>4</sub> B <sub>6</sub> C <sub>6</sub> | 0.5 H <sub>8</sub> C <sub>5</sub> + 5.437 Lu + 1.75 B <sub>13</sub> C <sub>2</sub> + BN → 4.437 LuB <sub>4</sub> + LuB <sub>6</sub> H <sub>4</sub> C <sub>6</sub> N                                        | -2.3422             |
| LuNH <sub>4</sub> B <sub>6</sub> C <sub>6</sub> | 48.33 B + 1.5 Lu <sub>3</sub> C <sub>4</sub> + 1.333 H <sub>3</sub> N → 3.5 LuB <sub>12</sub> + 0.3333 BN + LuB <sub>6</sub> H <sub>4</sub> C <sub>6</sub> N                                               | -2.3117             |
| LuNH <sub>4</sub> B <sub>6</sub> C <sub>6</sub> | 0.8571 Lu <sub>4</sub> C <sub>7</sub> + 2.27 N <sub>2</sub> + 0.6667 B <sub>9</sub> H <sub>11</sub> → 2.429 LuN + 1.111 H <sub>3</sub> N + LuB <sub>6</sub> H <sub>4</sub> C <sub>6</sub> N                | -2.2998             |
| LuNH <sub>4</sub> B <sub>6</sub> C <sub>6</sub> | 0.8571 Lu <sub>4</sub> C <sub>7</sub> + 1.964 N <sub>2</sub> + 0.5 LuB <sub>12</sub> + 2 H <sub>2</sub> → 2.929 LuN + LuB <sub>6</sub> H <sub>4</sub> C <sub>6</sub> N                                     | -2.2842             |
| LuNH <sub>4</sub> B <sub>6</sub> C <sub>6</sub> | 32 B + LuN + 1.5 Lu <sub>3</sub> C <sub>4</sub> + 2 LuH <sub>2</sub> → 6.5 LuB <sub>4</sub> + LuB <sub>6</sub> H <sub>4</sub> C <sub>6</sub> N                                                             | -2.2667             |
| LuNH <sub>4</sub> B <sub>6</sub> C <sub>6</sub> | 2.481 N <sub>2</sub> + 1.444 B <sub>9</sub> H <sub>11</sub> + 1.5 Lu <sub>3</sub> C <sub>4</sub> → 3.5 LuB <sub>2</sub> + 3.963 H <sub>3</sub> N + LuB <sub>6</sub> H <sub>4</sub> C <sub>6</sub> N        | -2.2643             |
| LuNH <sub>4</sub> B <sub>6</sub> C <sub>6</sub> | 0.8571 Lu <sub>4</sub> C <sub>7</sub> + 2.107 N <sub>2</sub> + 0.7857 LuB <sub>4</sub> + 0.5714 B <sub>5</sub> H <sub>7</sub> → 3.214 LuN + LuB <sub>6</sub> H <sub>4</sub> C <sub>6</sub> N               | -2.1515             |
| LuNH <sub>4</sub> B <sub>6</sub> C <sub>6</sub> | 57.14 B + LuN + 1.5 Lu <sub>3</sub> C <sub>4</sub> + 0.5714 B <sub>5</sub> H <sub>7</sub> → 4.5 LuB <sub>12</sub> + LuB <sub>6</sub> H <sub>4</sub> C <sub>6</sub> N                                       | -2.1310             |
| LuNH <sub>4</sub> B <sub>6</sub> C <sub>6</sub> | 7.333 Lu + 6 C + 1.333 H <sub>3</sub> N + 6 BN → 6.333 LuN + LuB <sub>6</sub> H <sub>4</sub> C <sub>6</sub> N                                                                                              | -2.0761             |
| LuNH <sub>4</sub> B <sub>6</sub> C <sub>6</sub> | 0.3636 B <sub>9</sub> H <sub>11</sub> + 56.73 B + LuN + 1.5 Lu <sub>3</sub> C <sub>4</sub> → 4.5 LuB <sub>12</sub> + LuB <sub>6</sub> H <sub>4</sub> C <sub>6</sub> N                                      | -2.0687             |
| LuNH <sub>4</sub> B <sub>6</sub> C <sub>6</sub> | 0.8571 Lu <sub>4</sub> C <sub>7</sub> + 1.714 N <sub>2</sub> + 6 B + 2 H <sub>2</sub> → 2.429 LuN + LuB <sub>6</sub> H <sub>4</sub> C <sub>6</sub> N                                                       | -2.0375             |
| LuNH <sub>4</sub> B <sub>6</sub> C <sub>6</sub> | 0.8571 Lu <sub>4</sub> C <sub>7</sub> + 2.055 N <sub>2</sub> + 0.3636 B <sub>9</sub> H <sub>11</sub> + 0.6818 LuB <sub>4</sub> → 3.11 LuN + LuB <sub>6</sub> H <sub>4</sub> C <sub>6</sub> N               | -1.9952             |
| LuNH <sub>4</sub> B <sub>6</sub> C <sub>6</sub> | 3 B <sub>13</sub> C <sub>2</sub> + 11.56 LuN + 1.333 H <sub>3</sub> N → 10.56 LuB <sub>2</sub> + 11.89 BN + LuB <sub>6</sub> H <sub>4</sub> C <sub>6</sub> N                                               | -1.9649             |
| LuNH <sub>4</sub> B <sub>6</sub> C <sub>6</sub> | 48 B + 1.5 Lu <sub>3</sub> C <sub>4</sub> + 0.5 H <sub>2</sub> + H <sub>3</sub> N → 3.5 LuB <sub>12</sub> + LuB <sub>6</sub> H <sub>4</sub> C <sub>6</sub> N                                               | -1.8974             |
| LuNH <sub>4</sub> B <sub>6</sub> C <sub>6</sub> | 0.5 N <sub>2</sub> + 3 B <sub>13</sub> C <sub>2</sub> + 0.3636 B <sub>9</sub> H <sub>11</sub> + 20.14 LuB <sub>2</sub> → 19.14 LuB <sub>4</sub> + LuB <sub>6</sub> H <sub>4</sub> C <sub>6</sub> N         | -1.8134             |
| LuNH <sub>4</sub> B <sub>6</sub> C <sub>6</sub> | 0.5 N <sub>2</sub> + 20 B + 1.5 Lu <sub>3</sub> C <sub>4</sub> + 2 H <sub>2</sub> → 3.5 LuB <sub>4</sub> + LuB <sub>6</sub> H <sub>4</sub> C <sub>6</sub> N                                                | -1.7803             |
| LuNH <sub>4</sub> B <sub>6</sub> C <sub>6</sub> | 1.2 H <sub>8</sub> C <sub>5</sub> + 2.514 B <sub>9</sub> H <sub>11</sub> + 17.63 LuN → 16.63 BN + 16.63 LuH <sub>2</sub> + LuB <sub>6</sub> H <sub>4</sub> C <sub>6</sub> N                                | -1.7604             |
| LuNH <sub>4</sub> B <sub>6</sub> C <sub>6</sub> | 0.5 N <sub>2</sub> + 3 B <sub>13</sub> C <sub>2</sub> + 19.93 LuB <sub>2</sub> + 0.5714 B <sub>5</sub> H <sub>7</sub> → 18.93 LuB <sub>4</sub> + LuB <sub>6</sub> H <sub>4</sub> C <sub>6</sub> N          | -1.7484             |
| LuNH <sub>4</sub> B <sub>6</sub> C <sub>6</sub> | 47.29 B + 1.5 Lu <sub>3</sub> C <sub>4</sub> + H <sub>3</sub> N + 0.1429 B <sub>5</sub> H <sub>7</sub> → 3.5 LuB <sub>12</sub> + LuB <sub>6</sub> H <sub>4</sub> C <sub>6</sub> N                          | -1.7481             |
| LuNH <sub>4</sub> B <sub>6</sub> C <sub>6</sub> | 0.09091 B <sub>9</sub> H <sub>11</sub> + 47.18 B + 1.5 Lu <sub>3</sub> C <sub>4</sub> + H <sub>3</sub> N → 3.5 LuB <sub>12</sub> + LuB <sub>6</sub> H <sub>4</sub> C <sub>6</sub> N                        | -1.7326             |
| LuNH <sub>4</sub> B <sub>6</sub> C <sub>6</sub> | 0.5 N <sub>2</sub> + 1.5 Lu <sub>3</sub> C <sub>4</sub> + 3.5 LuB <sub>12</sub> + 2 LuH <sub>2</sub> → 9 LuB <sub>4</sub> + LuB <sub>6</sub> H <sub>4</sub> C <sub>6</sub> N                               | -1.7306             |
| LuNH <sub>4</sub> B <sub>6</sub> C <sub>6</sub> | 0.5 H <sub>8</sub> C <sub>5</sub> + 0.5 Lu <sub>4</sub> C <sub>7</sub> + 2.5 N <sub>2</sub> + 3 LuB <sub>2</sub> → 4 LuN + LuB <sub>6</sub> H <sub>4</sub> C <sub>6</sub> N                                | -1.6825             |
| LuNH <sub>4</sub> B <sub>6</sub> C <sub>6</sub> | 1.5 Lu <sub>3</sub> C <sub>4</sub> + 2.6 LuB <sub>4</sub> + 5.4 H <sub>3</sub> N → 4.4 BN + 6.1 LuH <sub>2</sub> + LuB <sub>6</sub> H <sub>4</sub> C <sub>6</sub> N                                        | -1.6799             |
| LuNH <sub>4</sub> B <sub>6</sub> C <sub>6</sub> | 0.8571 Lu <sub>4</sub> C <sub>7</sub> + 1.798 N <sub>2</sub> + 1.5 LuB <sub>4</sub> + 1.333 H <sub>3</sub> N → 3.929 LuN + LuB <sub>6</sub> H <sub>4</sub> C <sub>6</sub> N                                | -1.6298             |
| LuNH <sub>4</sub> B <sub>6</sub> C <sub>6</sub> | 44 B + 1.5 Lu <sub>3</sub> C <sub>4</sub> + 1.333 H <sub>3</sub> N → 0.3333 LuN + 3.167 LuB <sub>12</sub> + LuB <sub>6</sub> H <sub>4</sub> C <sub>6</sub> N                                               | -1.6205             |
| LuNH <sub>4</sub> B <sub>6</sub> C <sub>6</sub> | 1.2 H <sub>8</sub> C <sub>5</sub> + 6.467 Lu + 0.6667 B <sub>9</sub> H <sub>11</sub> + LuN → 6.467 LuH <sub>2</sub> + LuB <sub>6</sub> H <sub>4</sub> C <sub>6</sub> N                                     | -1.6081             |
| LuNH <sub>4</sub> B <sub>6</sub> C <sub>6</sub> | 1.2 H <sub>8</sub> C <sub>5</sub> + 6.856 Lu + 0.5556 B <sub>9</sub> H <sub>11</sub> + BN → 5.856 LuH <sub>2</sub> + LuB <sub>6</sub> H <sub>4</sub> C <sub>6</sub> N                                      | -1.5989             |
| LuNH <sub>4</sub> B <sub>6</sub> C <sub>6</sub> | 0.8571 Lu <sub>4</sub> C <sub>7</sub> + 1.845 N <sub>2</sub> + 0.2619 LuB <sub>12</sub> + 0.5714 B <sub>5</sub> H <sub>7</sub> → 2.69 LuN + LuB <sub>6</sub> H <sub>4</sub> C <sub>6</sub> N               | -1.5696             |
| LuNH <sub>4</sub> B <sub>6</sub> C <sub>6</sub> | 1.2 H <sub>8</sub> C <sub>5</sub> + 8.8 Lu + 6 BN → 5 LuN + 2.8 LuH <sub>2</sub> + LuB <sub>6</sub> H <sub>4</sub> C <sub>6</sub> N                                                                        | -1.5531             |
| LuNH <sub>4</sub> B <sub>6</sub> C <sub>6</sub> | 1.2 H <sub>8</sub> C <sub>5</sub> + 10.58 Lu + 10.58 BN → 0.5091 B <sub>9</sub> H <sub>11</sub> + 9.582 LuN + LuB <sub>6</sub> H <sub>4</sub> C <sub>6</sub> N                                             | -1.5112             |
| LuNH <sub>4</sub> B <sub>6</sub> C <sub>6</sub> | 0.8571 Lu <sub>4</sub> C <sub>7</sub> + 1.828 N <sub>2</sub> + 0.3636 B <sub>9</sub> H <sub>11</sub> + 0.2273 LuB <sub>12</sub> → 2.656 LuN + LuB <sub>6</sub> H <sub>4</sub> C <sub>6</sub> N             | -1.4902             |
| LuNH <sub>4</sub> B <sub>6</sub> C <sub>6</sub> | 0.5 N <sub>2</sub> + 3 B <sub>13</sub> C <sub>2</sub> + 18.5 LuB <sub>2</sub> + 2 H <sub>2</sub> → 17.5 LuB <sub>4</sub> + LuB <sub>6</sub> H <sub>4</sub> C <sub>6</sub> N                                | -1.4706             |
| LuNH <sub>4</sub> B <sub>6</sub> C <sub>6</sub> | 48 B + 1.5 Lu <sub>3</sub> C <sub>4</sub> + 1.333 H <sub>3</sub> N → 0.1667 N <sub>2</sub> + 3.5 LuB <sub>12</sub> + LuB <sub>6</sub> H <sub>4</sub> C <sub>6</sub> N                                      | -1.4561             |
| LuNH <sub>4</sub> B <sub>6</sub> C <sub>6</sub> | 0.8571 Lu <sub>4</sub> C <sub>7</sub> + 1.714 N <sub>2</sub> + 3.143 B + 0.5714 B <sub>5</sub> H <sub>7</sub> → 2.429 LuN + LuB <sub>6</sub> H <sub>4</sub> C <sub>6</sub> N                               | -1.4404             |
| LuNH <sub>4</sub> B <sub>6</sub> C <sub>6</sub> | 3 B <sub>13</sub> C <sub>2</sub> + 7.333 LuN + 1.333 H <sub>3</sub> N → 6.333 LuB <sub>4</sub> + 7.667 BN + LuB <sub>6</sub> H <sub>4</sub> C <sub>6</sub> N                                               | -1.4145             |
| LuNH <sub>4</sub> B <sub>6</sub> C <sub>6</sub> | 4.7 Lu + 6 C + H <sub>3</sub> N + 1.2 B <sub>5</sub> H <sub>7</sub> → 3.7 LuH <sub>2</sub> + LuB <sub>6</sub> H <sub>4</sub> C <sub>6</sub> N                                                              | -1.4111             |
| LuNH <sub>4</sub> B <sub>6</sub> C <sub>6</sub> | 0.8571 Lu <sub>4</sub> C <sub>7</sub> + 1.714 N <sub>2</sub> + 0.3636 B <sub>9</sub> H <sub>11</sub> + 2.727 B → 2.429 LuN + LuB <sub>6</sub> H <sub>4</sub> C <sub>6</sub> N                              | -1.3781             |
| LuNH <sub>4</sub> B <sub>6</sub> C <sub>6</sub> | 0.5 N <sub>2</sub> + 4.023 Lu + 3 B <sub>13</sub> C <sub>2</sub> + 0.3636 B <sub>9</sub> H <sub>11</sub> → 3.023 LuB <sub>12</sub> + LuB <sub>6</sub> H <sub>4</sub> C <sub>6</sub> N                      | -1.3354             |
| LuNH <sub>4</sub> B <sub>6</sub> C <sub>6</sub> | 8.667 B + 1.5 Lu <sub>3</sub> C <sub>4</sub> + 3.667 H <sub>3</sub> N → 2.667 BN + 3.5 LuH <sub>2</sub> + LuB <sub>6</sub> H <sub>4</sub> C <sub>6</sub> N                                                 | -1.3349             |

Continued on next page

Continued

| Compound                                        | Chemical reaction                                                                                                                                                                                           | Reaction energy(eV) |
|-------------------------------------------------|-------------------------------------------------------------------------------------------------------------------------------------------------------------------------------------------------------------|---------------------|
| LuNH <sub>4</sub> B <sub>6</sub> C <sub>6</sub> | 0.5 N <sub>2</sub> + 3.988 Lu + 3 B <sub>13</sub> C <sub>2</sub> + 0.5714 B <sub>5</sub> H <sub>7</sub> → 2.988 LuB <sub>12</sub> + LuB <sub>6</sub> H <sub>4</sub> C <sub>6</sub> N                        | -1.2920             |
| LuNH <sub>4</sub> B <sub>6</sub> C <sub>6</sub> | 3 B <sub>13</sub> C <sub>2</sub> + 0.3636 B <sub>9</sub> H <sub>11</sub> + 13.09 LuN → 12.09 LuB <sub>2</sub> + 12.09 BN + LuB <sub>6</sub> H <sub>4</sub> C <sub>6</sub> N                                 | -1.2593             |
| LuNH <sub>4</sub> B <sub>6</sub> C <sub>6</sub> | 0.8571 Lu <sub>4</sub> C <sub>7</sub> + 0.5 N <sub>2</sub> + 23.71 B + 2 LuH <sub>2</sub> → 4.429 LuB <sub>4</sub> + LuB <sub>6</sub> H <sub>4</sub> C <sub>6</sub> N                                       | -1.2309             |
| LuNH <sub>4</sub> B <sub>6</sub> C <sub>6</sub> | 1.5 Lu <sub>3</sub> C <sub>4</sub> + 8.912 LuB <sub>4</sub> + 13.41 H <sub>3</sub> N → 3.294 B <sub>9</sub> H <sub>11</sub> + 12.41 LuN + LuB <sub>6</sub> H <sub>4</sub> C <sub>6</sub> N                  | -1.2298             |
| LuNH <sub>4</sub> B <sub>6</sub> C <sub>6</sub> | 0.5 N <sub>2</sub> + 17.14 B + 1.5 Lu <sub>3</sub> C <sub>4</sub> + 0.5714 B <sub>5</sub> H <sub>7</sub> → 3.5 LuB <sub>4</sub> + LuB <sub>6</sub> H <sub>4</sub> C <sub>6</sub> N                          | -1.1831             |
| LuNH <sub>4</sub> B <sub>6</sub> C <sub>6</sub> | 3 B <sub>13</sub> C <sub>2</sub> + 12.95 LuN + 0.5714 B <sub>5</sub> H <sub>7</sub> → 11.95 LuB <sub>2</sub> + 11.95 BN + LuB <sub>6</sub> H <sub>4</sub> C <sub>6</sub> N                                  | -1.1763             |
| LuNH <sub>4</sub> B <sub>6</sub> C <sub>6</sub> | 0.5 N <sub>2</sub> + 3.75 Lu + 3 B <sub>13</sub> C <sub>2</sub> + 2 H <sub>2</sub> → 2.75 LuB <sub>12</sub> + LuB <sub>6</sub> H <sub>4</sub> C <sub>6</sub> N                                              | -1.1631             |
| LuNH <sub>4</sub> B <sub>6</sub> C <sub>6</sub> | 1.5 Lu <sub>3</sub> C <sub>4</sub> + 0.7647 LuB <sub>12</sub> + 4.176 H <sub>3</sub> N → 3.176 BN + 4.265 LuH <sub>2</sub> + LuB <sub>6</sub> H <sub>4</sub> C <sub>6</sub> N                               | -1.1215             |
| LuNH <sub>4</sub> B <sub>6</sub> C <sub>6</sub> | 0.5 N <sub>2</sub> + 0.3636 B <sub>9</sub> H <sub>11</sub> + 16.73 B + 1.5 Lu <sub>3</sub> C <sub>4</sub> → 3.5 LuB <sub>4</sub> + LuB <sub>6</sub> H <sub>4</sub> C <sub>6</sub> N                         | -1.1208             |
| LuNH <sub>4</sub> B <sub>6</sub> C <sub>6</sub> | 1.417 N <sub>2</sub> + 0.6667 B <sub>9</sub> H <sub>11</sub> + 1.5 Lu <sub>3</sub> C <sub>4</sub> → 1.833 LuN + 1.667 LuH <sub>2</sub> + LuB <sub>6</sub> H <sub>4</sub> C <sub>6</sub> N                   | -1.0711             |
| LuNH <sub>4</sub> B <sub>6</sub> C <sub>6</sub> | 0.8571 Lu <sub>4</sub> C <sub>7</sub> + 2.367 N <sub>2</sub> + 2.171 B <sub>5</sub> H <sub>7</sub> → 2.429 LuB <sub>2</sub> + 3.733 H <sub>3</sub> N + LuB <sub>6</sub> H <sub>4</sub> C <sub>6</sub> N     | -1.0258             |
| LuNH <sub>4</sub> B <sub>6</sub> C <sub>6</sub> | 2.5 N <sub>2</sub> + 6 C + 3 LuB <sub>2</sub> + 2 LuH <sub>2</sub> → 4 LuN + LuB <sub>6</sub> H <sub>4</sub> C <sub>6</sub> N                                                                               | -1.0154             |
| LuNH <sub>4</sub> B <sub>6</sub> C <sub>6</sub> | 0.8571 Lu <sub>4</sub> C <sub>7</sub> + 1.714 N <sub>2</sub> + 2.75 B <sub>9</sub> H <sub>11</sub> → 2.429 LuN + 3.75 B <sub>5</sub> H <sub>7</sub> + LuB <sub>6</sub> H <sub>4</sub> C <sub>6</sub> N      | -0.9695             |
| LuNH <sub>4</sub> B <sub>6</sub> C <sub>6</sub> | 24 B + LuN + 1.5 Lu <sub>3</sub> C <sub>4</sub> + 2 H <sub>2</sub> → 4.5 LuB <sub>4</sub> + LuB <sub>6</sub> H <sub>4</sub> C <sub>6</sub> N                                                                | -0.8751             |
| LuNH <sub>4</sub> B <sub>6</sub> C <sub>6</sub> | 20.33 B + 1.5 Lu <sub>3</sub> C <sub>4</sub> + 1.333 H <sub>3</sub> N → 3.5 LuB <sub>4</sub> + 0.3333 BN + LuB <sub>6</sub> H <sub>4</sub> C <sub>6</sub> N                                                 | -0.8704             |
| LuNH <sub>4</sub> B <sub>6</sub> C <sub>6</sub> | 1.2 H <sub>8</sub> C <sub>5</sub> + 10 Lu + 10 BN → 9 LuN + 0.8 B <sub>5</sub> H <sub>7</sub> + LuB <sub>6</sub> H <sub>4</sub> C <sub>6</sub> N                                                            | -0.8560             |
| LuNH <sub>4</sub> B <sub>6</sub> C <sub>6</sub> | 0.8571 Lu <sub>4</sub> C <sub>7</sub> + 0.5 N <sub>2</sub> + 35.14 B + 2 H <sub>2</sub> → 2.429 LuB <sub>12</sub> + LuB <sub>6</sub> H <sub>4</sub> C <sub>6</sub> N                                        | -0.8394             |
| LuNH <sub>4</sub> B <sub>6</sub> C <sub>6</sub> | 0.8571 Lu <sub>4</sub> C <sub>7</sub> + 1.714 N <sub>2</sub> + 0.6667 B <sub>9</sub> H <sub>11</sub> → 2.429 LuN + 1.667 H <sub>2</sub> + LuB <sub>6</sub> H <sub>4</sub> C <sub>6</sub> N                  | -0.8286             |
| LuNH <sub>4</sub> B <sub>6</sub> C <sub>6</sub> | 1.2 H <sub>8</sub> C <sub>5</sub> + 5.3 Lu + 6 B + H <sub>3</sub> N → 4.3 LuH <sub>2</sub> + LuB <sub>6</sub> H <sub>4</sub> C <sub>6</sub> N                                                               | -0.8281             |
| LuNH <sub>4</sub> B <sub>6</sub> C <sub>6</sub> | 22 B + 1.5 Lu <sub>3</sub> C <sub>4</sub> + H <sub>3</sub> N + 0.5 LuH <sub>2</sub> → 4 LuB <sub>4</sub> + LuB <sub>6</sub> H <sub>4</sub> C <sub>6</sub> N                                                 | -0.8041             |
| LuNH <sub>4</sub> B <sub>6</sub> C <sub>6</sub> | 0.8571 Lu <sub>4</sub> C <sub>7</sub> + 1.714 N <sub>2</sub> + 1.2 B <sub>5</sub> H <sub>7</sub> → 2.429 LuN + 2.2 H <sub>2</sub> + LuB <sub>6</sub> H <sub>4</sub> C <sub>6</sub> N                        | -0.7835             |
| LuNH <sub>4</sub> B <sub>6</sub> C <sub>6</sub> | 3 B <sub>13</sub> C <sub>2</sub> + 12 LuN + 2 H <sub>2</sub> → 11 LuB <sub>2</sub> + 11 BN + LuB <sub>6</sub> H <sub>4</sub> C <sub>6</sub> N                                                               | -0.7743             |
| LuNH <sub>4</sub> B <sub>6</sub> C <sub>6</sub> | 1.237 N <sub>2</sub> + 0.4615 B <sub>13</sub> C <sub>2</sub> + 1.269 Lu <sub>3</sub> C <sub>4</sub> + 1.333 H <sub>3</sub> N → 2.808 LuN + LuB <sub>6</sub> H <sub>4</sub> C <sub>6</sub> N                 | -0.7651             |
| LuNH <sub>4</sub> B <sub>6</sub> C <sub>6</sub> | 0.5 N <sub>2</sub> + 1.5 Lu <sub>3</sub> C <sub>4</sub> + 2.5 LuB <sub>12</sub> + 2 H <sub>2</sub> → 6 LuB <sub>4</sub> + LuB <sub>6</sub> H <sub>4</sub> C <sub>6</sub> N                                  | -0.7508             |
| LuNH <sub>4</sub> B <sub>6</sub> C <sub>6</sub> | 0.5 H <sub>8</sub> C <sub>5</sub> + 4.187 Lu + 1.75 B <sub>13</sub> C <sub>2</sub> + LuN → 4.187 LuB <sub>4</sub> + LuB <sub>6</sub> H <sub>4</sub> C <sub>6</sub> N                                        | -0.7066             |
| LuNH <sub>4</sub> B <sub>6</sub> C <sub>6</sub> | 47 B + 1.5 Lu <sub>3</sub> C <sub>4</sub> + 2 H <sub>2</sub> + BN → 3.5 LuB <sub>12</sub> + LuB <sub>6</sub> H <sub>4</sub> C <sub>6</sub> N                                                                | -0.6547             |
| LuNH <sub>4</sub> B <sub>6</sub> C <sub>6</sub> | 3 B <sub>13</sub> C <sub>2</sub> + 0.3636 B <sub>9</sub> H <sub>11</sub> + 8.255 LuN → 7.255 LuB <sub>4</sub> + 7.255 BN + LuB <sub>6</sub> H <sub>4</sub> C <sub>6</sub> N                                 | -0.6289             |
| LuNH <sub>4</sub> B <sub>6</sub> C <sub>6</sub> | LuN + 1.5 Lu <sub>3</sub> C <sub>4</sub> + 4 LuB <sub>12</sub> + 2 LuH <sub>2</sub> → 10.5 LuB <sub>4</sub> + LuB <sub>6</sub> H <sub>4</sub> C <sub>6</sub> N                                              | -0.6195             |
| LuNH <sub>4</sub> B <sub>6</sub> C <sub>6</sub> | 1.5 Lu <sub>3</sub> C <sub>4</sub> + 6.885 LuB <sub>4</sub> + 11.38 H <sub>3</sub> N → 10.38 LuN + 4.308 B <sub>5</sub> H <sub>7</sub> + LuB <sub>6</sub> H <sub>4</sub> C <sub>6</sub> N                   | -0.6071             |
| LuNH <sub>4</sub> B <sub>6</sub> C <sub>6</sub> | 27 B + 1.5 Lu <sub>3</sub> C <sub>4</sub> + BN + 2 LuH <sub>2</sub> → 5.5 LuB <sub>4</sub> + LuB <sub>6</sub> H <sub>4</sub> C <sub>6</sub> N                                                               | -0.6050             |
| LuNH <sub>4</sub> B <sub>6</sub> C <sub>6</sub> | 0.125 H <sub>8</sub> C <sub>5</sub> + 42.37 B + 1.344 Lu <sub>3</sub> C <sub>4</sub> + H <sub>3</sub> N → 3.031 LuB <sub>12</sub> + LuB <sub>6</sub> H <sub>4</sub> C <sub>6</sub> N                        | -0.5985             |
| LuNH <sub>4</sub> B <sub>6</sub> C <sub>6</sub> | 4.083 Lu + 3 B <sub>13</sub> C <sub>2</sub> + 1.333 H <sub>3</sub> N → 0.3333 LuN + 2.75 LuB <sub>12</sub> + LuB <sub>6</sub> H <sub>4</sub> C <sub>6</sub> N                                               | -0.5786             |
| LuNH <sub>4</sub> B <sub>6</sub> C <sub>6</sub> | 13.77 B + 1.5 Lu <sub>3</sub> C <sub>4</sub> + 4.5 H <sub>3</sub> N → 0.8636 B <sub>9</sub> H <sub>11</sub> + 3.5 LuN + LuB <sub>6</sub> H <sub>4</sub> C <sub>6</sub> N                                    | -0.5560             |
| LuNH <sub>4</sub> B <sub>6</sub> C <sub>6</sub> | 3 B <sub>13</sub> C <sub>2</sub> + 8.171 LuN + 0.5714 B <sub>5</sub> H <sub>7</sub> → 7.171 LuB <sub>4</sub> + 7.171 BN + LuB <sub>6</sub> H <sub>4</sub> C <sub>6</sub> N                                  | -0.5531             |
| LuNH <sub>4</sub> B <sub>6</sub> C <sub>6</sub> | 0.8571 Lu <sub>4</sub> C <sub>7</sub> + 1.298 N <sub>2</sub> + 0.5 LuB <sub>12</sub> + 1.333 H <sub>3</sub> N → 2.929 LuN + LuB <sub>6</sub> H <sub>4</sub> C <sub>6</sub> N                                | -0.5188             |
| LuNH <sub>4</sub> B <sub>6</sub> C <sub>6</sub> | 0.8571 Lu <sub>4</sub> C <sub>7</sub> + 58.14 B + BN + 2 LuH <sub>2</sub> → 4.429 LuB <sub>12</sub> + LuB <sub>6</sub> H <sub>4</sub> C <sub>6</sub> N                                                      | -0.4878             |
| LuNH <sub>4</sub> B <sub>6</sub> C <sub>6</sub> | 0.7972 Lu <sub>4</sub> C <sub>7</sub> + 1.594 N <sub>2</sub> + 0.2098 B <sub>13</sub> C <sub>2</sub> + 0.3636 B <sub>9</sub> H <sub>11</sub> → 2.189 LuN + LuB <sub>6</sub> H <sub>4</sub> C <sub>6</sub> N | -0.4827             |
| LuNH <sub>4</sub> B <sub>6</sub> C <sub>6</sub> | 3 B <sub>13</sub> C <sub>2</sub> + 18.33 LuB <sub>2</sub> + 1.333 H <sub>3</sub> N → 17.33 LuB <sub>4</sub> + 0.3333 BN + LuB <sub>6</sub> H <sub>4</sub> C <sub>6</sub> N                                  | -0.4586             |
| LuNH <sub>4</sub> B <sub>6</sub> C <sub>6</sub> | 20 B + 1.5 Lu <sub>3</sub> C <sub>4</sub> + 0.5 H <sub>2</sub> + H <sub>3</sub> N → 3.5 LuB <sub>4</sub> + LuB <sub>6</sub> H <sub>4</sub> C <sub>6</sub> N                                                 | -0.4562             |
| LuNH <sub>4</sub> B <sub>6</sub> C <sub>6</sub> | 4.167 Lu + 0.6667 B <sub>9</sub> H <sub>11</sub> + 6 C + H <sub>3</sub> N → 3.167 LuH <sub>2</sub> + LuB <sub>6</sub> H <sub>4</sub> C <sub>6</sub> N                                                       | -0.4204             |
| LuNH <sub>4</sub> B <sub>6</sub> C <sub>6</sub> | 3 B <sub>13</sub> C <sub>2</sub> + 19.17 LuB <sub>2</sub> + 1.333 H <sub>3</sub> N → 0.3333 LuN + 17.83 LuB <sub>4</sub> + LuB <sub>6</sub> H <sub>4</sub> C <sub>6</sub> N                                 | -0.4152             |
| LuNH <sub>4</sub> B <sub>6</sub> C <sub>6</sub> | 0.5 N <sub>2</sub> + 3 B <sub>13</sub> C <sub>2</sub> + 14.5 LuB <sub>2</sub> + 2 LuH <sub>2</sub> → 15.5 LuB <sub>4</sub> + LuB <sub>6</sub> H <sub>4</sub> C <sub>6</sub> N                               | -0.4120             |
| LuNH <sub>4</sub> B <sub>6</sub> C <sub>6</sub> | 0.7881 Lu <sub>4</sub> C <sub>7</sub> + 1.576 N <sub>2</sub> + 0.2418 B <sub>13</sub> C <sub>2</sub> + 0.5714 B <sub>5</sub> H <sub>7</sub> → 2.152 LuN + LuB <sub>6</sub> H <sub>4</sub> C <sub>6</sub> N  | -0.4086             |
| LuNH <sub>4</sub> B <sub>6</sub> C <sub>6</sub> | 12.79 B + 1.5 Lu <sub>3</sub> C <sub>4</sub> + 4.5 H <sub>3</sub> N → 3.5 LuN + 1.357 B <sub>5</sub> H <sub>7</sub> + LuB <sub>6</sub> H <sub>4</sub> C <sub>6</sub> N                                      | -0.4081             |
| LuNH <sub>4</sub> B <sub>6</sub> C <sub>6</sub> | 0.8571 Lu <sub>4</sub> C <sub>7</sub> + 47.14 B + LuN + 2 H <sub>2</sub> → 3.429 LuB <sub>12</sub> + LuB <sub>6</sub> H <sub>4</sub> C <sub>6</sub> N                                                       | -0.3461             |
| LuNH <sub>4</sub> B <sub>6</sub> C <sub>6</sub> | 0.8571 Lu <sub>4</sub> C <sub>7</sub> + 27.71 B + LuN + 2 LuH <sub>2</sub> → 5.429 LuB <sub>4</sub> + LuB <sub>6</sub> H <sub>4</sub> C <sub>6</sub> N                                                      | -0.3258             |
| LuNH <sub>4</sub> B <sub>6</sub> C <sub>6</sub> | 18.67 B + 1.5 Lu <sub>3</sub> C <sub>4</sub> + 1.333 H <sub>3</sub> N → 0.3333 LuN + 3.167 LuB <sub>4</sub> + LuB <sub>6</sub> H <sub>4</sub> C <sub>6</sub> N                                              | -0.3165             |
| LuNH <sub>4</sub> B <sub>6</sub> C <sub>6</sub> | 19.29 B + 1.5 Lu <sub>3</sub> C <sub>4</sub> + H <sub>3</sub> N + 0.1429 B <sub>5</sub> H <sub>7</sub> → 3.5 LuB <sub>4</sub> + LuB <sub>6</sub> H <sub>4</sub> C <sub>6</sub> N                            | -0.3069             |
| LuNH <sub>4</sub> B <sub>6</sub> C <sub>6</sub> | 0.5 N <sub>2</sub> + 1.5 Lu <sub>3</sub> C <sub>4</sub> + 2.143 LuB <sub>12</sub> + 0.5714 B <sub>5</sub> H <sub>7</sub> → 5.643 LuB <sub>4</sub> + LuB <sub>6</sub> H <sub>4</sub> C <sub>6</sub> N        | -0.3007             |
| LuNH <sub>4</sub> B <sub>6</sub> C <sub>6</sub> | 0.09091 B <sub>9</sub> H <sub>11</sub> + 19.18 B + 1.5 Lu <sub>3</sub> C <sub>4</sub> + H <sub>3</sub> N → 3.5 LuB <sub>4</sub> + LuB <sub>6</sub> H <sub>4</sub> C <sub>6</sub> N                          | -0.2913             |
| LuNH <sub>4</sub> B <sub>6</sub> C <sub>6</sub> | 21.14 B + LuN + 1.5 Lu <sub>3</sub> C <sub>4</sub> + 0.5714 B <sub>5</sub> H <sub>7</sub> → 4.5 LuB <sub>4</sub> + LuB <sub>6</sub> H <sub>4</sub> C <sub>6</sub> N                                         | -0.2780             |
| LuNH <sub>4</sub> B <sub>6</sub> C <sub>6</sub> | 0.8571 Lu <sub>4</sub> C <sub>7</sub> + 1.048 N <sub>2</sub> + 6 B + 1.333 H <sub>3</sub> N → 2.429 LuN + LuB <sub>6</sub> H <sub>4</sub> C <sub>6</sub> N                                                  | -0.2721             |
| LuNH <sub>4</sub> B <sub>6</sub> C <sub>6</sub> | 0.5 N <sub>2</sub> + 0.3636 B <sub>9</sub> H <sub>11</sub> + 1.5 Lu <sub>3</sub> C <sub>4</sub> + 2.091 LuB <sub>12</sub> → 5.591 LuB <sub>4</sub> + LuB <sub>6</sub> H <sub>4</sub> C <sub>6</sub> N       | -0.2598             |
| LuNH <sub>4</sub> B <sub>6</sub> C <sub>6</sub> | 0.8571 Lu <sub>4</sub> C <sub>7</sub> + 2.045 N <sub>2</sub> + 1.206 B <sub>9</sub> H <sub>11</sub> → 2.429 LuB <sub>2</sub> + 3.09 H <sub>3</sub> N + LuB <sub>6</sub> H <sub>4</sub> C <sub>6</sub> N     | -0.2555             |
| LuNH <sub>4</sub> B <sub>6</sub> C <sub>6</sub> | 0.8571 Lu <sub>4</sub> C <sub>7</sub> + 0.5 N <sub>2</sub> + 32.29 B + 0.5714 B <sub>5</sub> H <sub>7</sub> → 2.429 LuB <sub>12</sub> + LuB <sub>6</sub> H <sub>4</sub> C <sub>6</sub> N                    | -0.2423             |
| LuNH <sub>4</sub> B <sub>6</sub> C <sub>6</sub> | 3 B <sub>13</sub> C <sub>2</sub> + 0.09091 B <sub>9</sub> H <sub>11</sub> + 18.91 LuB <sub>2</sub> + H <sub>3</sub> N → 17.91 LuB <sub>4</sub> + LuB <sub>6</sub> H <sub>4</sub> C <sub>6</sub> N           | -0.2322             |
| LuNH <sub>4</sub> B <sub>6</sub> C <sub>6</sub> | 3 B <sub>13</sub> C <sub>2</sub> + 18.86 LuB <sub>2</sub> + H <sub>3</sub> N + 0.1429 B <sub>5</sub> H <sub>7</sub> → 17.86 LuB <sub>4</sub> + LuB <sub>6</sub> H <sub>4</sub> C <sub>6</sub> N             | -0.2160             |
| LuNH <sub>4</sub> B <sub>6</sub> C <sub>6</sub> | 0.3636 B <sub>9</sub> H <sub>11</sub> + 20.73 B + LuN + 1.5 Lu <sub>3</sub> C <sub>4</sub> → 4.5 LuB <sub>4</sub> + LuB <sub>6</sub> H <sub>4</sub> C <sub>6</sub> N                                        | -0.2157             |
| LuNH <sub>4</sub> B <sub>6</sub> C <sub>6</sub> | 3 B <sub>13</sub> C <sub>2</sub> + 7.6 LuN + 2 H <sub>2</sub> → 6.6 LuB <sub>4</sub> + 6.6 BN + LuB <sub>6</sub> H <sub>4</sub> C <sub>6</sub> N                                                            | -0.2007             |
| LuNH <sub>4</sub> B <sub>6</sub> C <sub>6</sub> | 0.5 H <sub>8</sub> C <sub>5</sub> + 2.063 N <sub>2</sub> + 0.875 Lu <sub>3</sub> C <sub>4</sub> + 1.5 LuB <sub>4</sub> → 3.125 LuN + LuB <sub>6</sub> H <sub>4</sub> C <sub>6</sub> N                       | -0.1851             |

Continued on next page

Continued

| Compound                                        | Chemical reaction                                                                                                                                                                                                  | Reaction energy(eV) |
|-------------------------------------------------|--------------------------------------------------------------------------------------------------------------------------------------------------------------------------------------------------------------------|---------------------|
| LuNH <sub>4</sub> B <sub>6</sub> C <sub>6</sub> | 0.8571 Lu <sub>4</sub> C <sub>7</sub> + 0.5 N <sub>2</sub> + 0.3636 B <sub>9</sub> H <sub>11</sub> + 31.87 B → 2.429 LuB <sub>12</sub> + LuB <sub>6</sub> H <sub>4</sub> C <sub>6</sub> N                          | -0.1800             |
| LuNH <sub>4</sub> B <sub>6</sub> C <sub>6</sub> | 1.15 N <sub>2</sub> + 1.5 Lu <sub>3</sub> C <sub>4</sub> + 1.2 B <sub>5</sub> H <sub>7</sub> → 1.3 LuN + 2.2 LuH <sub>2</sub> + LuB <sub>6</sub> H <sub>4</sub> C <sub>6</sub> N                                   | -0.1722             |
| LuNH <sub>4</sub> B <sub>6</sub> C <sub>6</sub> | 3.722 Lu + 3 B <sub>13</sub> C <sub>2</sub> + 1.333 H <sub>3</sub> N → 2.722 LuB <sub>12</sub> + 0.3333 BN + LuB <sub>6</sub> H <sub>4</sub> C <sub>6</sub> N                                                      | -0.1685             |
| LuNH <sub>4</sub> B <sub>6</sub> C <sub>6</sub> | 3 B <sub>13</sub> C <sub>2</sub> + 18.5 LuB <sub>2</sub> + 0.5 H <sub>2</sub> + H <sub>3</sub> N → 17.5 LuB <sub>4</sub> + LuB <sub>6</sub> H <sub>4</sub> C <sub>6</sub> N                                        | -0.1465             |
| LuNH <sub>4</sub> B <sub>6</sub> C <sub>6</sub> | 1.5 Lu <sub>3</sub> C <sub>4</sub> + 1.443 LuB <sub>12</sub> + 5.943 H <sub>3</sub> N → 1.257 B <sub>9</sub> H <sub>11</sub> + 4.943 LuN + LuB <sub>6</sub> H <sub>4</sub> C <sub>6</sub> N                        | -0.0709             |
| LuNH <sub>4</sub> B <sub>6</sub> C <sub>6</sub> | 0.8571 Lu <sub>4</sub> C <sub>7</sub> + 41.14 B + H <sub>3</sub> N + 0.5 LuH <sub>2</sub> → 2.929 LuB <sub>12</sub> + LuB <sub>6</sub> H <sub>4</sub> C <sub>6</sub> N                                             | -0.0691             |
| LuNH <sub>4</sub> B <sub>6</sub> C <sub>6</sub> | 0.7253 Lu <sub>4</sub> C <sub>7</sub> + 1.451 N <sub>2</sub> + 0.4615 B <sub>13</sub> C <sub>2</sub> + 2 H <sub>2</sub> → 1.901 LuN + LuB <sub>6</sub> H <sub>4</sub> C <sub>6</sub> N                             | -0.0677             |
| LuNH <sub>4</sub> B <sub>6</sub> C <sub>6</sub> | 44.14 B + 1.5 Lu <sub>3</sub> C <sub>4</sub> + BN + 0.5714 B <sub>5</sub> H <sub>7</sub> → 3.5 LuB <sub>12</sub> + LuB <sub>6</sub> H <sub>4</sub> C <sub>6</sub> N                                                | -0.0576             |
| LuNH <sub>4</sub> B <sub>6</sub> C <sub>6</sub> | 20 B + 1.5 Lu <sub>3</sub> C <sub>4</sub> + 1.333 H <sub>3</sub> N → 0.1667 N <sub>2</sub> + 3.5 LuB <sub>4</sub> + LuB <sub>6</sub> H <sub>4</sub> C <sub>6</sub> N                                               | -0.0148             |
| LuNH <sub>4</sub> B <sub>6</sub> C <sub>6</sub> | 0.8571 Lu <sub>4</sub> C <sub>7</sub> + 0.5 N <sub>2</sub> + 2.964 LuB <sub>12</sub> + 2 LuH <sub>2</sub> → 7.393 LuB <sub>4</sub> + LuB <sub>6</sub> H <sub>4</sub> C <sub>6</sub> N                              | -0.0103             |
| NaNH <sub>4</sub> B <sub>6</sub> C <sub>6</sub> | 99 B <sub>13</sub> C <sub>2</sub> + 641 N <sub>2</sub> + 4 NaH → 1281 BN + 3 NaC <sub>64</sub> + NaB <sub>6</sub> H <sub>4</sub> C <sub>6</sub> N                                                                  | -3172.0217          |
| NaNH <sub>4</sub> B <sub>6</sub> C <sub>6</sub> | 3 B <sub>13</sub> C <sub>2</sub> + 218.2 B <sub>5</sub> H <sub>7</sub> + 169.6 NaN <sub>3</sub> → 507.8 H <sub>3</sub> N + 56.2 Na <sub>3</sub> B <sub>20</sub> + NaB <sub>6</sub> H <sub>4</sub> C <sub>6</sub> N | -438.7759           |
| NaNH <sub>4</sub> B <sub>6</sub> C <sub>6</sub> | 47 N <sub>2</sub> + 6.6 NaB <sub>15</sub> + 1.2 H <sub>8</sub> C <sub>5</sub> → 5.6 NaH + 93 BN + NaB <sub>6</sub> H <sub>4</sub> C <sub>6</sub> N                                                                 | -226.3743           |
| NaNH <sub>4</sub> B <sub>6</sub> C <sub>6</sub> | 37.1 N <sub>2</sub> + 8.8 B <sub>9</sub> H <sub>11</sub> + NaC <sub>64</sub> → 73.2 BN + 11.6 H <sub>8</sub> C <sub>5</sub> + NaB <sub>6</sub> H <sub>4</sub> C <sub>6</sub> N                                     | -186.6106           |
| NaNH <sub>4</sub> B <sub>6</sub> C <sub>6</sub> | 89.2 N <sub>2</sub> + NaC <sub>64</sub> + 76.6 B <sub>5</sub> H <sub>7</sub> → 177.4 H <sub>3</sub> N + 29 B <sub>13</sub> C <sub>2</sub> + NaB <sub>6</sub> H <sub>4</sub> C <sub>6</sub> N                       | -179.4279           |
| NaNH <sub>4</sub> B <sub>6</sub> C <sub>6</sub> | 32.07 N <sub>2</sub> + NaC <sub>64</sub> + 13.83 B <sub>5</sub> H <sub>7</sub> → 63.14 BN + 11.6 H <sub>8</sub> C <sub>5</sub> + NaB <sub>6</sub> H <sub>4</sub> C <sub>6</sub> N                                  | -162.3032           |
| NaNH <sub>4</sub> B <sub>6</sub> C <sub>6</sub> | 77.85 N <sub>2</sub> + 42.56 B <sub>9</sub> H <sub>11</sub> + NaC <sub>64</sub> → 154.7 H <sub>3</sub> N + 29 B <sub>13</sub> C <sub>2</sub> + NaB <sub>6</sub> H <sub>4</sub> C <sub>6</sub> N                    | -152.2542           |
| NaNH <sub>4</sub> B <sub>6</sub> C <sub>6</sub> | 19 NaH + 6 BN + 1158 C → 5 H <sub>3</sub> N + 18 NaC <sub>64</sub> + NaB <sub>6</sub> H <sub>4</sub> C <sub>6</sub> N                                                                                              | -125.2254           |
| NaNH <sub>4</sub> B <sub>6</sub> C <sub>6</sub> | 3 B <sub>13</sub> C <sub>2</sub> + 26.14 N <sub>2</sub> + 0.3636 B <sub>9</sub> H <sub>11</sub> + NaB <sub>15</sub> → 51.27 BN + NaB <sub>6</sub> H <sub>4</sub> C <sub>6</sub> N                                  | -119.9621           |
| NaNH <sub>4</sub> B <sub>6</sub> C <sub>6</sub> | 3 B <sub>13</sub> C <sub>2</sub> + 25.93 N <sub>2</sub> + NaB <sub>15</sub> + 0.5714 B <sub>5</sub> H <sub>7</sub> → 50.86 BN + NaB <sub>6</sub> H <sub>4</sub> C <sub>6</sub> N                                   | -118.9576           |
| NaNH <sub>4</sub> B <sub>6</sub> C <sub>6</sub> | 3 B <sub>13</sub> C <sub>2</sub> + 24.5 N <sub>2</sub> + NaB <sub>15</sub> + 2 H <sub>2</sub> → 48 BN + NaB <sub>6</sub> H <sub>4</sub> C <sub>6</sub> N                                                           | -112.2212           |
| NaNH <sub>4</sub> B <sub>6</sub> C <sub>6</sub> | 3 B <sub>13</sub> C <sub>2</sub> + 1.792 B <sub>9</sub> H <sub>11</sub> + 16.71 NaN <sub>3</sub> → 15.71 NaH + 49.13 BN + NaB <sub>6</sub> H <sub>4</sub> C <sub>6</sub> N                                         | -111.5114           |
| NaNH <sub>4</sub> B <sub>6</sub> C <sub>6</sub> | 1.333 H <sub>3</sub> N + 3 B <sub>13</sub> C <sub>2</sub> + 23.83 N <sub>2</sub> + NaB <sub>15</sub> → 48 BN + NaB <sub>6</sub> H <sub>4</sub> C <sub>6</sub> N                                                    | -110.4558           |
| NaNH <sub>4</sub> B <sub>6</sub> C <sub>6</sub> | 3 B <sub>13</sub> C <sub>2</sub> + 2.687 B <sub>5</sub> H <sub>7</sub> + 15.81 NaN <sub>3</sub> → 14.81 NaH + 46.44 BN + NaB <sub>6</sub> H <sub>4</sub> C <sub>6</sub> N                                          | -105.0952           |
| NaNH <sub>4</sub> B <sub>6</sub> C <sub>6</sub> | 3 B <sub>13</sub> C <sub>2</sub> + 21.97 N <sub>2</sub> + 0.3636 B <sub>9</sub> H <sub>11</sub> + 0.3333 Na <sub>3</sub> B <sub>20</sub> → 42.94 BN + NaB <sub>6</sub> H <sub>4</sub> C <sub>6</sub> N             | -98.9205            |
| NaNH <sub>4</sub> B <sub>6</sub> C <sub>6</sub> | 3 B <sub>13</sub> C <sub>2</sub> + 21.76 N <sub>2</sub> + 0.5714 B <sub>5</sub> H <sub>7</sub> + 0.3333 Na <sub>3</sub> B <sub>20</sub> → 42.52 BN + NaB <sub>6</sub> H <sub>4</sub> C <sub>6</sub> N              | -97.9161            |
| NaNH <sub>4</sub> B <sub>6</sub> C <sub>6</sub> | 3 B <sub>13</sub> C <sub>2</sub> + 20.33 N <sub>2</sub> + 0.3333 Na <sub>3</sub> B <sub>20</sub> + 2 H <sub>2</sub> → 39.67 BN + NaB <sub>6</sub> H <sub>4</sub> C <sub>6</sub> N                                  | -91.1796            |
| NaNH <sub>4</sub> B <sub>6</sub> C <sub>6</sub> | 1.333 H <sub>3</sub> N + 3 B <sub>13</sub> C <sub>2</sub> + 19.67 N <sub>2</sub> + 0.3333 Na <sub>3</sub> B <sub>20</sub> → 39.67 BN + NaB <sub>6</sub> H <sub>4</sub> C <sub>6</sub> N                            | -89.4142            |
| NaNH <sub>4</sub> B <sub>6</sub> C <sub>6</sub> | 19.5 N <sub>2</sub> + 1.2 H <sub>8</sub> C <sub>5</sub> + 2.2 Na <sub>3</sub> B <sub>20</sub> → 5.6 NaH + 38 BN + NaB <sub>6</sub> H <sub>4</sub> C <sub>6</sub> N                                                 | -87.4999            |
| NaNH <sub>4</sub> B <sub>6</sub> C <sub>6</sub> | 3 B <sub>13</sub> C <sub>2</sub> + 18.64 N <sub>2</sub> + 0.3636 B <sub>9</sub> H <sub>11</sub> + Na → 36.27 BN + NaB <sub>6</sub> H <sub>4</sub> C <sub>6</sub> N                                                 | -82.2654            |
| NaNH <sub>4</sub> B <sub>6</sub> C <sub>6</sub> | 3 B <sub>13</sub> C <sub>2</sub> + 17.14 N <sub>2</sub> + 0.3636 B <sub>9</sub> H <sub>11</sub> + NaN <sub>3</sub> → 36.27 BN + NaB <sub>6</sub> H <sub>4</sub> C <sub>6</sub> N                                   | -81.8387            |
| NaNH <sub>4</sub> B <sub>6</sub> C <sub>6</sub> | 3 B <sub>13</sub> C <sub>2</sub> + 18.43 N <sub>2</sub> + Na + 0.5714 B <sub>5</sub> H <sub>7</sub> → 35.86 BN + NaB <sub>6</sub> H <sub>4</sub> C <sub>6</sub> N                                                  | -81.2610            |
| NaNH <sub>4</sub> B <sub>6</sub> C <sub>6</sub> | 3 B <sub>13</sub> C <sub>2</sub> + 16.93 N <sub>2</sub> + 0.5714 B <sub>5</sub> H <sub>7</sub> + NaN <sub>3</sub> → 35.86 BN + NaB <sub>6</sub> H <sub>4</sub> C <sub>6</sub> N                                    | -80.8342            |
| NaNH <sub>4</sub> B <sub>6</sub> C <sub>6</sub> | 3 B <sub>13</sub> C <sub>2</sub> + 18.23 N <sub>2</sub> + NaH + 0.2727 B <sub>9</sub> H <sub>11</sub> → 35.45 BN + NaB <sub>6</sub> H <sub>4</sub> C <sub>6</sub> N                                                | -79.9497            |
| NaNH <sub>4</sub> B <sub>6</sub> C <sub>6</sub> | 3 B <sub>13</sub> C <sub>2</sub> + 18.07 N <sub>2</sub> + NaH + 0.4286 B <sub>5</sub> H <sub>7</sub> → 35.14 BN + NaB <sub>6</sub> H <sub>4</sub> C <sub>6</sub> N                                                 | -79.1964            |
| NaNH <sub>4</sub> B <sub>6</sub> C <sub>6</sub> | 3 B <sub>13</sub> C <sub>2</sub> + 0.3636 B <sub>9</sub> H <sub>11</sub> + 12.42 NaN <sub>3</sub> → 36.27 BN + 11.42 Na + NaB <sub>6</sub> H <sub>4</sub> C <sub>6</sub> N                                         | -76.9634            |
| NaNH <sub>4</sub> B <sub>6</sub> C <sub>6</sub> | 3 B <sub>13</sub> C <sub>2</sub> + 0.5714 B <sub>5</sub> H <sub>7</sub> + 12.29 NaN <sub>3</sub> → 35.86 BN + 11.29 Na + NaB <sub>6</sub> H <sub>4</sub> C <sub>6</sub> N                                          | -76.0181            |
| NaNH <sub>4</sub> B <sub>6</sub> C <sub>6</sub> | 3 B <sub>13</sub> C <sub>2</sub> + 17 N <sub>2</sub> + Na + 2 H <sub>2</sub> → 33 BN + NaB <sub>6</sub> H <sub>4</sub> C <sub>6</sub> N                                                                            | -74.5245            |
| NaNH <sub>4</sub> B <sub>6</sub> C <sub>6</sub> | 3 B <sub>13</sub> C <sub>2</sub> + 21.5 N <sub>2</sub> + 4 NaH → 33 BN + 3 NaN <sub>3</sub> + NaB <sub>6</sub> H <sub>4</sub> C <sub>6</sub> N                                                                     | -74.2828            |
| NaNH <sub>4</sub> B <sub>6</sub> C <sub>6</sub> | 3 B <sub>13</sub> C <sub>2</sub> + 17 N <sub>2</sub> + NaH + 1.5 H <sub>2</sub> → 33 BN + NaB <sub>6</sub> H <sub>4</sub> C <sub>6</sub> N                                                                         | -74.1440            |
| NaNH <sub>4</sub> B <sub>6</sub> C <sub>6</sub> | 3 B <sub>13</sub> C <sub>2</sub> + 15.5 N <sub>2</sub> + 2 H <sub>2</sub> + NaN <sub>3</sub> → 33 BN + NaB <sub>6</sub> H <sub>4</sub> C <sub>6</sub> N                                                            | -74.0978            |
| NaNH <sub>4</sub> B <sub>6</sub> C <sub>6</sub> | 3 B <sub>13</sub> C <sub>2</sub> + 7.167 H <sub>2</sub> + 11.33 NaN <sub>3</sub> → 10.33 NaH + 33 BN + NaB <sub>6</sub> H <sub>4</sub> C <sub>6</sub> N                                                            | -73.6200            |
| NaNH <sub>4</sub> B <sub>6</sub> C <sub>6</sub> | 3 B <sub>13</sub> C <sub>2</sub> + 17 N <sub>2</sub> + 4 NaH → 33 BN + 3 Na + NaB <sub>6</sub> H <sub>4</sub> C <sub>6</sub> N                                                                                     | -73.0025            |
| NaNH <sub>4</sub> B <sub>6</sub> C <sub>6</sub> | H <sub>3</sub> N + 3 B <sub>13</sub> C <sub>2</sub> + 16.5 N <sub>2</sub> + NaH → 33 BN + NaB <sub>6</sub> H <sub>4</sub> C <sub>6</sub> N                                                                         | -72.8200            |
| NaNH <sub>4</sub> B <sub>6</sub> C <sub>6</sub> | 1.333 H <sub>3</sub> N + 3 B <sub>13</sub> C <sub>2</sub> + 16.33 N <sub>2</sub> + Na → 33 BN + NaB <sub>6</sub> H <sub>4</sub> C <sub>6</sub> N                                                                   | -72.7591            |
| NaNH <sub>4</sub> B <sub>6</sub> C <sub>6</sub> | 1.333 H <sub>3</sub> N + 3 B <sub>13</sub> C <sub>2</sub> + 14.83 N <sub>2</sub> + NaN <sub>3</sub> → 33 BN + NaB <sub>6</sub> H <sub>4</sub> C <sub>6</sub> N                                                     | -72.3324            |
| NaNH <sub>4</sub> B <sub>6</sub> C <sub>6</sub> | 1.75 B <sub>13</sub> C <sub>2</sub> + 16.38 N <sub>2</sub> + NaB <sub>15</sub> + 0.5 H <sub>8</sub> C <sub>5</sub> → 31.75 BN + NaB <sub>6</sub> H <sub>4</sub> C <sub>6</sub> N                                   | -70.9383            |
| NaNH <sub>4</sub> B <sub>6</sub> C <sub>6</sub> | 3 B <sub>13</sub> C <sub>2</sub> + 2 H <sub>2</sub> + 11.33 NaN <sub>3</sub> → 33 BN + 10.33 Na + NaB <sub>6</sub> H <sub>4</sub> C <sub>6</sub> N                                                                 | -69.6880            |
| NaNH <sub>4</sub> B <sub>6</sub> C <sub>6</sub> | 3 B <sub>13</sub> C <sub>2</sub> + 4 NaH + 11.33 NaN <sub>3</sub> → 33 BN + 14.33 Na + NaB <sub>6</sub> H <sub>4</sub> C <sub>6</sub> N                                                                            | -68.1660            |
| NaNH <sub>4</sub> B <sub>6</sub> C <sub>6</sub> | 1.333 H <sub>3</sub> N + 3 B <sub>13</sub> C <sub>2</sub> + 10.89 NaN <sub>3</sub> → 33 BN + 9.889 Na + NaB <sub>6</sub> H <sub>4</sub> C <sub>6</sub> N                                                           | -68.1123            |
| NaNH <sub>4</sub> B <sub>6</sub> C <sub>6</sub> | 4.3 H <sub>3</sub> N + 3 B <sub>13</sub> C <sub>2</sub> + 9.9 NaN <sub>3</sub> → 8.9 NaH + 33 BN + NaB <sub>6</sub> H <sub>4</sub> C <sub>6</sub> N                                                                | -67.9928            |
| NaNH <sub>4</sub> B <sub>6</sub> C <sub>6</sub> | 34 H <sub>3</sub> N + 3 B <sub>13</sub> C <sub>2</sub> + 99 Na → 98 NaH + 33 BN + NaB <sub>6</sub> H <sub>4</sub> C <sub>6</sub> N                                                                                 | -66.7961            |
| NaNH <sub>4</sub> B <sub>6</sub> C <sub>6</sub> | 35.6 H <sub>3</sub> N + 3.123 B <sub>13</sub> C <sub>2</sub> + NaC <sub>64</sub> → 34.6 BN + 12.85 H <sub>8</sub> C <sub>5</sub> + NaB <sub>6</sub> H <sub>4</sub> C <sub>6</sub> N                                | -55.2855            |
| NaNH <sub>4</sub> B <sub>6</sub> C <sub>6</sub> | 32.27 H <sub>3</sub> N + NaC <sub>64</sub> + 37.27 B → 31.27 BN + 11.6 H <sub>8</sub> C <sub>5</sub> + NaB <sub>6</sub> H <sub>4</sub> C <sub>6</sub> N                                                            | -52.2126            |
| NaNH <sub>4</sub> B <sub>6</sub> C <sub>6</sub> | 1.75 B <sub>13</sub> C <sub>2</sub> + 12.21 N <sub>2</sub> + 0.5 H <sub>8</sub> C <sub>5</sub> + 0.3333 Na <sub>3</sub> B <sub>20</sub> → 23.42 BN + NaB <sub>6</sub> H <sub>4</sub> C <sub>6</sub> N              | -49.8967            |
| NaNH <sub>4</sub> B <sub>6</sub> C <sub>6</sub> | 49 H <sub>3</sub> N + 3 B <sub>13</sub> C <sub>2</sub> + NaB <sub>15</sub> → 48 BN + 71.5 H <sub>2</sub> + NaB <sub>6</sub> H <sub>4</sub> C <sub>6</sub> N                                                        | -47.3418            |
| NaNH <sub>4</sub> B <sub>6</sub> C <sub>6</sub> | 2.063 B <sub>13</sub> C <sub>2</sub> + 10.91 N <sub>2</sub> + NaH + 0.375 H <sub>8</sub> C <sub>5</sub> → 20.81 BN + NaB <sub>6</sub> H <sub>4</sub> C <sub>6</sub> N                                              | -43.1819            |
| NaNH <sub>4</sub> B <sub>6</sub> C <sub>6</sub> | 6 BN + 2.667 NaC <sub>64</sub> + 133.7 H <sub>2</sub> → 32.93 H <sub>8</sub> C <sub>5</sub> + 1.667 NaN <sub>3</sub> + NaB <sub>6</sub> H <sub>4</sub> C <sub>6</sub> N                                            | -39.7189            |
| NaNH <sub>4</sub> B <sub>6</sub> C <sub>6</sub> | 1.2 H <sub>8</sub> C <sub>5</sub> + 6.6 NaN <sub>3</sub> + 24.8 B → 5.6 NaH + 18.8 BN + NaB <sub>6</sub> H <sub>4</sub> C <sub>6</sub> N                                                                           | -38.4155            |
| NaNH <sub>4</sub> B <sub>6</sub> C <sub>6</sub> | 40.67 H <sub>3</sub> N + 3 B <sub>13</sub> C <sub>2</sub> + 0.3333 Na <sub>3</sub> B <sub>20</sub> → 39.67 BN + 59 H <sub>2</sub> + NaB <sub>6</sub> H <sub>4</sub> C <sub>6</sub> N                               | -37.3341            |

Continued on next page

Continued

| Compound                                        | Chemical reaction                                                                                                                                                                                                     | Reaction energy(eV) |
|-------------------------------------------------|-----------------------------------------------------------------------------------------------------------------------------------------------------------------------------------------------------------------------|---------------------|
| NaNH <sub>4</sub> B <sub>6</sub> C <sub>6</sub> | 21.48 H <sub>3</sub> N + 2.942 B <sub>9</sub> H <sub>11</sub> + NaC <sub>64</sub> → 20.48 BN + 11.6 H <sub>8</sub> C <sub>5</sub> + NaB <sub>6</sub> H <sub>4</sub> C <sub>6</sub> N                                  | -33.4715            |
| NaNH <sub>4</sub> B <sub>6</sub> C <sub>6</sub> | 1.75 B <sub>13</sub> C <sub>2</sub> + 8.875 N <sub>2</sub> + Na + 0.5 H <sub>8</sub> C <sub>5</sub> → 16.75 BN + NaB <sub>6</sub> H <sub>4</sub> C <sub>6</sub> N                                                     | -33.2417            |
| NaNH <sub>4</sub> B <sub>6</sub> C <sub>6</sub> | 31 H <sub>3</sub> N + 3 B <sub>13</sub> C <sub>2</sub> + NaN <sub>3</sub> → 33 BN + 44.5 H <sub>2</sub> + NaB <sub>6</sub> H <sub>4</sub> C <sub>6</sub> N                                                            | -33.0516            |
| NaNH <sub>4</sub> B <sub>6</sub> C <sub>6</sub> | 1.75 B <sub>13</sub> C <sub>2</sub> + 7.375 N <sub>2</sub> + 0.5 H <sub>8</sub> C <sub>5</sub> + NaN <sub>3</sub> → 16.75 BN + NaB <sub>6</sub> H <sub>4</sub> C <sub>6</sub> N                                       | -32.8149            |
| NaNH <sub>4</sub> B <sub>6</sub> C <sub>6</sub> | 20.41 H <sub>3</sub> N + NaC <sub>64</sub> + 5.082 B <sub>5</sub> H <sub>7</sub> → 19.41 BN + 11.6 H <sub>8</sub> C <sub>5</sub> + NaB <sub>6</sub> H <sub>4</sub> C <sub>6</sub> N                                   | -32.1667            |
| NaNH <sub>4</sub> B <sub>6</sub> C <sub>6</sub> | 1.75 B <sub>13</sub> C <sub>2</sub> + 0.5 H <sub>8</sub> C <sub>5</sub> + 5.917 NaN <sub>3</sub> → 16.75 BN + 4.917 Na + NaB <sub>6</sub> H <sub>4</sub> C <sub>6</sub> N                                             | -30.7167            |
| NaNH <sub>4</sub> B <sub>6</sub> C <sub>6</sub> | 34 H <sub>3</sub> N + 3 B <sub>13</sub> C <sub>2</sub> + Na → 33 BN + 49 H <sub>2</sub> + NaB <sub>6</sub> H <sub>4</sub> C <sub>6</sub> N                                                                            | -29.5062            |
| NaNH <sub>4</sub> B <sub>6</sub> C <sub>6</sub> | 34 H <sub>3</sub> N + 3 B <sub>13</sub> C <sub>2</sub> + NaH → 33 BN + 49.5 H <sub>2</sub> + NaB <sub>6</sub> H <sub>4</sub> C <sub>6</sub> N                                                                         | -29.1257            |
| NaNH <sub>4</sub> B <sub>6</sub> C <sub>6</sub> | 1.378 NaB <sub>15</sub> + 1.2 H <sub>8</sub> C <sub>5</sub> + 5.222 NaN <sub>3</sub> → 5.6 NaH + 14.67 BN + NaB <sub>6</sub> H <sub>4</sub> C <sub>6</sub> N                                                          | -27.2855            |
| NaNH <sub>4</sub> B <sub>6</sub> C <sub>6</sub> | 1.333 H <sub>3</sub> N + 1.111 NaC <sub>64</sub> + 429.2 B → 32.56 B <sub>13</sub> C <sub>2</sub> + 0.1111 NaN <sub>3</sub> + NaB <sub>6</sub> H <sub>4</sub> C <sub>6</sub> N                                        | -26.7321            |
| NaNH <sub>4</sub> B <sub>6</sub> C <sub>6</sub> | 4 NaH + 0.3 Na <sub>3</sub> B <sub>20</sub> + 276.9 C + 0.3333 NaN <sub>3</sub> → 4.233 NaC <sub>64</sub> + NaB <sub>6</sub> H <sub>4</sub> C <sub>6</sub> N                                                          | -26.4363            |
| NaNH <sub>4</sub> B <sub>6</sub> C <sub>6</sub> | 0.5 N <sub>2</sub> + NaC <sub>64</sub> + 0.5 H <sub>8</sub> C <sub>5</sub> + 399.3 B → 30.25 B <sub>13</sub> C <sub>2</sub> + NaB <sub>6</sub> H <sub>4</sub> C <sub>6</sub> N                                        | -25.0142            |
| NaNH <sub>4</sub> B <sub>6</sub> C <sub>6</sub> | 0.5 N <sub>2</sub> + NaC <sub>64</sub> + 2 H <sub>2</sub> + 383 B → 29 B <sub>13</sub> C <sub>2</sub> + NaB <sub>6</sub> H <sub>4</sub> C <sub>6</sub> N                                                              | -24.5872            |
| NaNH <sub>4</sub> B <sub>6</sub> C <sub>6</sub> | 0.5 N <sub>2</sub> + NaC <sub>64</sub> + 0.5714 B <sub>5</sub> H <sub>7</sub> + 380.1 B → 29 B <sub>13</sub> C <sub>2</sub> + NaB <sub>6</sub> H <sub>4</sub> C <sub>6</sub> N                                        | -23.9901            |
| NaNH <sub>4</sub> B <sub>6</sub> C <sub>6</sub> | 0.5 N <sub>2</sub> + 0.3636 B <sub>9</sub> H <sub>11</sub> + NaC <sub>64</sub> + 379.7 B → 29 B <sub>13</sub> C <sub>2</sub> + NaB <sub>6</sub> H <sub>4</sub> C <sub>6</sub> N                                       | -23.9278            |
| NaNH <sub>4</sub> B <sub>6</sub> C <sub>6</sub> | 6.636 N <sub>2</sub> + 0.3636 B <sub>9</sub> H <sub>11</sub> + NaB <sub>15</sub> + 6 C → 12.27 BN + NaB <sub>6</sub> H <sub>4</sub> C <sub>6</sub> N                                                                  | -23.8854            |
| NaNH <sub>4</sub> B <sub>6</sub> C <sub>6</sub> | 0.5 N <sub>2</sub> + 4 NaH + 0.3 Na <sub>3</sub> B <sub>20</sub> + 255.6 C → 3.9 NaC <sub>64</sub> + NaB <sub>6</sub> H <sub>4</sub> C <sub>6</sub> N                                                                 | -23.8492            |
| NaNH <sub>4</sub> B <sub>6</sub> C <sub>6</sub> | 1.333 H <sub>3</sub> N + NaC <sub>64</sub> + 383.3 B → 29 B <sub>13</sub> C <sub>2</sub> + 0.3333 BN + NaB <sub>6</sub> H <sub>4</sub> C <sub>6</sub> N                                                               | -23.6774            |
| NaNH <sub>4</sub> B <sub>6</sub> C <sub>6</sub> | H <sub>3</sub> N + NaC <sub>64</sub> + 0.125 H <sub>8</sub> C <sub>5</sub> + 387.1 B → 29.31 B <sub>13</sub> C <sub>2</sub> + NaB <sub>6</sub> H <sub>4</sub> C <sub>6</sub> N                                        | -23.3699            |
| NaNH <sub>4</sub> B <sub>6</sub> C <sub>6</sub> | H <sub>3</sub> N + NaC <sub>64</sub> + 0.5 H <sub>2</sub> + 383 B → 29 B <sub>13</sub> C <sub>2</sub> + NaB <sub>6</sub> H <sub>4</sub> C <sub>6</sub> N                                                              | -23.2632            |
| NaNH <sub>4</sub> B <sub>6</sub> C <sub>6</sub> | H <sub>3</sub> N + NaC <sub>64</sub> + 0.1429 B <sub>5</sub> H <sub>7</sub> + 382.3 B → 29 B <sub>13</sub> C <sub>2</sub> + NaB <sub>6</sub> H <sub>4</sub> C <sub>6</sub> N                                          | -23.1139            |
| NaNH <sub>4</sub> B <sub>6</sub> C <sub>6</sub> | H <sub>3</sub> N + 0.09091 B <sub>9</sub> H <sub>11</sub> + NaC <sub>64</sub> + 382.2 B → 29 B <sub>13</sub> C <sub>2</sub> + NaB <sub>6</sub> H <sub>4</sub> C <sub>6</sub> N                                        | -23.0983            |
| NaNH <sub>4</sub> B <sub>6</sub> C <sub>6</sub> | 3 B <sub>13</sub> C <sub>2</sub> + 7 N <sub>2</sub> + 4 NaH → 13 BN + Na <sub>3</sub> B <sub>20</sub> + NaB <sub>6</sub> H <sub>4</sub> C <sub>6</sub> N                                                              | -23.0373            |
| NaNH <sub>4</sub> B <sub>6</sub> C <sub>6</sub> | 6.429 N <sub>2</sub> + NaB <sub>15</sub> + 0.5714 B <sub>5</sub> H <sub>7</sub> + 6 C → 11.86 BN + NaB <sub>6</sub> H <sub>4</sub> C <sub>6</sub> N                                                                   | -22.8809            |
| NaNH <sub>4</sub> B <sub>6</sub> C <sub>6</sub> | 1.333 H <sub>3</sub> N + NaC <sub>64</sub> + 383 B → 29 B <sub>13</sub> C <sub>2</sub> + 0.1667 N <sub>2</sub> + NaB <sub>6</sub> H <sub>4</sub> C <sub>6</sub> N                                                     | -22.8218            |
| NaNH <sub>4</sub> B <sub>6</sub> C <sub>6</sub> | BN + NaC <sub>64</sub> + 0.5 H <sub>8</sub> C <sub>5</sub> + 398.3 B → 30.25 B <sub>13</sub> C <sub>2</sub> + NaB <sub>6</sub> H <sub>4</sub> C <sub>6</sub> N                                                        | -22.4474            |
| NaNH <sub>4</sub> B <sub>6</sub> C <sub>6</sub> | 4 NaH + 0.4 NaB <sub>15</sub> + 244.9 C + 0.3333 NaN <sub>3</sub> → 3.733 NaC <sub>64</sub> + NaB <sub>6</sub> H <sub>4</sub> C <sub>6</sub> N                                                                        | -22.4313            |
| NaNH <sub>4</sub> B <sub>6</sub> C <sub>6</sub> | BN + NaC <sub>64</sub> + 2 H <sub>2</sub> + 382 B → 29 B <sub>13</sub> C <sub>2</sub> + NaB <sub>6</sub> H <sub>4</sub> C <sub>6</sub> N                                                                              | -22.0205            |
| NaNH <sub>4</sub> B <sub>6</sub> C <sub>6</sub> | BN + NaC <sub>64</sub> + 0.5714 B <sub>5</sub> H <sub>7</sub> + 379.1 B → 29 B <sub>13</sub> C <sub>2</sub> + NaB <sub>6</sub> H <sub>4</sub> C <sub>6</sub> N                                                        | -21.4233            |
| NaNH <sub>4</sub> B <sub>6</sub> C <sub>6</sub> | BN + 0.3636 B <sub>9</sub> H <sub>11</sub> + NaC <sub>64</sub> + 378.7 B → 29 B <sub>13</sub> C <sub>2</sub> + NaB <sub>6</sub> H <sub>4</sub> C <sub>6</sub> N                                                       | -21.3610            |
| NaNH <sub>4</sub> B <sub>6</sub> C <sub>6</sub> | 3 B <sub>13</sub> C <sub>2</sub> + 0.3636 B <sub>9</sub> H <sub>11</sub> + 4.545 NaN <sub>3</sub> → 12.64 BN + 1.182 Na <sub>3</sub> B <sub>20</sub> + NaB <sub>6</sub> H <sub>4</sub> C <sub>6</sub> N               | -21.2759            |
| NaNH <sub>4</sub> B <sub>6</sub> C <sub>6</sub> | 3 B <sub>13</sub> C <sub>2</sub> + 0.5714 B <sub>5</sub> H <sub>7</sub> + 4.502 NaN <sub>3</sub> → 12.51 BN + 1.167 Na <sub>3</sub> B <sub>20</sub> + NaB <sub>6</sub> H <sub>4</sub> C <sub>6</sub> N                | -21.0058            |
| NaNH <sub>4</sub> B <sub>6</sub> C <sub>6</sub> | 4 NaH + BN + 0.25 Na <sub>3</sub> B <sub>20</sub> + 246 C → 3.75 NaC <sub>64</sub> + NaB <sub>6</sub> H <sub>4</sub> C <sub>6</sub> N                                                                                 | -20.1227            |
| NaNH <sub>4</sub> B <sub>6</sub> C <sub>6</sub> | 1.333 H <sub>3</sub> N + 3 B <sub>13</sub> C <sub>2</sub> + 4.069 NaN <sub>3</sub> → 12.54 BN + 1.023 Na <sub>3</sub> B <sub>20</sub> + NaB <sub>6</sub> H <sub>4</sub> C <sub>6</sub> N                              | -19.9089            |
| NaNH <sub>4</sub> B <sub>6</sub> C <sub>6</sub> | 0.5 N <sub>2</sub> + 4 NaH + 0.4 NaB <sub>15</sub> + 223.6 C → 3.4 NaC <sub>64</sub> + NaB <sub>6</sub> H <sub>4</sub> C <sub>6</sub> N                                                                               | -19.8442            |
| NaNH <sub>4</sub> B <sub>6</sub> C <sub>6</sub> | 5.933 N <sub>2</sub> + 0.3636 B <sub>9</sub> H <sub>11</sub> + 0.09375 NaC <sub>64</sub> + 0.9063 NaB <sub>15</sub> → 10.87 BN + NaB <sub>6</sub> H <sub>4</sub> C <sub>6</sub> N                                     | -19.5837            |
| NaNH <sub>4</sub> B <sub>6</sub> C <sub>6</sub> | 4 NaH + 219.3 C + 0.3333 NaN <sub>3</sub> + 6 B → 3.333 NaC <sub>64</sub> + NaB <sub>6</sub> H <sub>4</sub> C <sub>6</sub> N                                                                                          | -19.4780            |
| NaNH <sub>4</sub> B <sub>6</sub> C <sub>6</sub> | 3 B <sub>13</sub> C <sub>2</sub> + 2 H <sub>2</sub> + 4.207 NaN <sub>3</sub> → 11.62 BN + 1.069 Na <sub>3</sub> B <sub>20</sub> + NaB <sub>6</sub> H <sub>4</sub> C <sub>6</sub> N                                    | -19.3182            |
| NaNH <sub>4</sub> B <sub>6</sub> C <sub>6</sub> | 0.4615 B <sub>13</sub> C <sub>2</sub> + 4 NaH + 218.4 C + 0.3333 NaN <sub>3</sub> → 3.333 NaC <sub>64</sub> + NaB <sub>6</sub> H <sub>4</sub> C <sub>6</sub> N                                                        | -18.8584            |
| NaNH <sub>4</sub> B <sub>6</sub> C <sub>6</sub> | 1.2 H <sub>8</sub> C <sub>5</sub> + 0.8552 Na <sub>3</sub> B <sub>20</sub> + 4.034 NaN <sub>3</sub> → 5.6 NaH + 11.1 BN + NaB <sub>6</sub> H <sub>4</sub> C <sub>6</sub> N                                            | -18.5836            |
| NaNH <sub>4</sub> B <sub>6</sub> C <sub>6</sub> | 5.725 N <sub>2</sub> + 0.09375 NaC <sub>64</sub> + 0.9063 NaB <sub>15</sub> + 0.5714 B <sub>5</sub> H <sub>7</sub> → 10.45 BN + NaB <sub>6</sub> H <sub>4</sub> C <sub>6</sub> N                                      | -18.5792            |
| NaNH <sub>4</sub> B <sub>6</sub> C <sub>6</sub> | 0.5 N <sub>2</sub> + 4 NaH + 198 C + 6 B → 3 NaC <sub>64</sub> + NaB <sub>6</sub> H <sub>4</sub> C <sub>6</sub> N                                                                                                     | -16.8908            |
| NaNH <sub>4</sub> B <sub>6</sub> C <sub>6</sub> | 4 NaH + BN + 0.3333 NaB <sub>15</sub> + 219.3 C → 3.333 NaC <sub>64</sub> + NaB <sub>6</sub> H <sub>4</sub> C <sub>6</sub> N                                                                                          | -16.7852            |
| NaNH <sub>4</sub> B <sub>6</sub> C <sub>6</sub> | 0.4615 B <sub>13</sub> C <sub>2</sub> + 0.5 N <sub>2</sub> + 4 NaH + 197.1 C → 3 NaC <sub>64</sub> + NaB <sub>6</sub> H <sub>4</sub> C <sub>6</sub> N                                                                 | -16.2713            |
| NaNH <sub>4</sub> B <sub>6</sub> C <sub>6</sub> | 5 N <sub>2</sub> + NaB <sub>15</sub> + 6 C + 2 H <sub>2</sub> → 9 BN + NaB <sub>6</sub> H <sub>4</sub> C <sub>6</sub> N                                                                                               | -16.1445            |
| NaNH <sub>4</sub> B <sub>6</sub> C <sub>6</sub> | 5.933 N <sub>2</sub> + NaB <sub>15</sub> + 1.2 H <sub>8</sub> C <sub>5</sub> → 1.867 H <sub>3</sub> N + 9 BN + NaB <sub>6</sub> H <sub>4</sub> C <sub>6</sub> N                                                       | -15.6138            |
| NaNH <sub>4</sub> B <sub>6</sub> C <sub>6</sub> | 5 N <sub>2</sub> + NaB <sub>15</sub> + 0.5 H <sub>8</sub> C <sub>5</sub> + 3.5 C → 9 BN + NaB <sub>6</sub> H <sub>4</sub> C <sub>6</sub> N                                                                            | -14.8936            |
| NaNH <sub>4</sub> B <sub>6</sub> C <sub>6</sub> | 0.5 N <sub>2</sub> + NaC <sub>64</sub> + 48.4 H <sub>2</sub> + 6 B → 11.6 H <sub>8</sub> C <sub>5</sub> + NaB <sub>6</sub> H <sub>4</sub> C <sub>6</sub> N                                                            | -14.6819            |
| NaNH <sub>4</sub> B <sub>6</sub> C <sub>6</sub> | 0.4615 B <sub>13</sub> C <sub>2</sub> + 0.5 N <sub>2</sub> + NaC <sub>64</sub> + 49.14 H <sub>2</sub> → 11.78 H <sub>8</sub> C <sub>5</sub> + NaB <sub>6</sub> H <sub>4</sub> C <sub>6</sub> N                        | -14.5243            |
| NaNH <sub>4</sub> B <sub>6</sub> C <sub>6</sub> | 1.333 H <sub>3</sub> N + 4.333 N <sub>2</sub> + NaB <sub>15</sub> + 6 C → 9 BN + NaB <sub>6</sub> H <sub>4</sub> C <sub>6</sub> N                                                                                     | -14.3791            |
| NaNH <sub>4</sub> B <sub>6</sub> C <sub>6</sub> | 4 NaH + BN + 198 C + 5 B → 3 NaC <sub>64</sub> + NaB <sub>6</sub> H <sub>4</sub> C <sub>6</sub> N                                                                                                                     | -14.3241            |
| NaNH <sub>4</sub> B <sub>6</sub> C <sub>6</sub> | 0.3846 B <sub>13</sub> C <sub>2</sub> + 4 NaH + BN + 197.2 C → 3 NaC <sub>64</sub> + NaB <sub>6</sub> H <sub>4</sub> C <sub>6</sub> N                                                                                 | -13.8078            |
| NaNH <sub>4</sub> B <sub>6</sub> C <sub>6</sub> | 16.5 H <sub>3</sub> N + 3 B <sub>13</sub> C <sub>2</sub> + NaB <sub>15</sub> → 15.5 BN + 6.5 B <sub>5</sub> H <sub>7</sub> + NaB <sub>6</sub> H <sub>4</sub> C <sub>6</sub> N                                         | -13.7470            |
| NaNH <sub>4</sub> B <sub>6</sub> C <sub>6</sub> | 6.696 B <sub>9</sub> H <sub>11</sub> + 1.2 H <sub>8</sub> C <sub>5</sub> + 9.139 NaN <sub>3</sub> → 26.42 H <sub>3</sub> N + 2.713 Na <sub>3</sub> B <sub>20</sub> + NaB <sub>6</sub> H <sub>4</sub> C <sub>6</sub> N | -13.4993            |
| NaNH <sub>4</sub> B <sub>6</sub> C <sub>6</sub> | 0.5 N <sub>2</sub> + 0.6667 B <sub>9</sub> H <sub>11</sub> + NaC <sub>64</sub> + 44.73 H <sub>2</sub> → 11.6 H <sub>8</sub> C <sub>5</sub> + NaB <sub>6</sub> H <sub>4</sub> C <sub>6</sub> N                         | -13.4730            |
| NaNH <sub>4</sub> B <sub>6</sub> C <sub>6</sub> | 0.5 N <sub>2</sub> + NaC <sub>64</sub> + 1.2 B <sub>5</sub> H <sub>7</sub> + 44.2 H <sub>2</sub> → 11.6 H <sub>8</sub> C <sub>5</sub> + NaB <sub>6</sub> H <sub>4</sub> C <sub>6</sub> N                              | -13.4279            |
| NaNH <sub>4</sub> B <sub>6</sub> C <sub>6</sub> | H <sub>3</sub> N + NaC <sub>64</sub> + 46.9 H <sub>2</sub> + 6 B → 11.6 H <sub>8</sub> C <sub>5</sub> + NaB <sub>6</sub> H <sub>4</sub> C <sub>6</sub> N                                                              | -13.3579            |
| NaNH <sub>4</sub> B <sub>6</sub> C <sub>6</sub> | 0.6667 NaC <sub>64</sub> + 0.5 H <sub>8</sub> C <sub>5</sub> + 0.3333 NaN <sub>3</sub> + 260.6 B → 19.58 B <sub>13</sub> C <sub>2</sub> + NaB <sub>6</sub> H <sub>4</sub> C <sub>6</sub> N                            | -13.2833            |
| NaNH <sub>4</sub> B <sub>6</sub> C <sub>6</sub> | H <sub>3</sub> N + 0.4615 B <sub>13</sub> C <sub>2</sub> + NaC <sub>64</sub> + 47.64 H <sub>2</sub> → 11.78 H <sub>8</sub> C <sub>5</sub> + NaB <sub>6</sub> H <sub>4</sub> C <sub>6</sub> N                          | -13.2002            |
| NaNH <sub>4</sub> B <sub>6</sub> C <sub>6</sub> | 5 N <sub>2</sub> + NaB <sub>15</sub> + 1.2 H <sub>8</sub> C <sub>5</sub> → 9 BN + 2.8 H <sub>2</sub> + NaB <sub>6</sub> H <sub>4</sub> C <sub>6</sub> N                                                               | -13.1422            |

Continued on next page



Continued

| Compound                                        | Chemical reaction                                                                                                                                                                                                        | Reaction energy(eV) |
|-------------------------------------------------|--------------------------------------------------------------------------------------------------------------------------------------------------------------------------------------------------------------------------|---------------------|
| NaNH <sub>4</sub> B <sub>6</sub> C <sub>6</sub> | 0.6667 NaC <sub>64</sub> + 2 H <sub>2</sub> + 0.3333 NaN <sub>3</sub> + 244.3 B → 18.33 B <sub>13</sub> C <sub>2</sub> + NaB <sub>6</sub> H <sub>4</sub> C <sub>6</sub> N                                                | -12.8564            |
| NaNH <sub>4</sub> B <sub>6</sub> C <sub>6</sub> | 4.59 N <sub>2</sub> + 0.05469 NaC <sub>64</sub> + 0.9453 NaB <sub>15</sub> + 0.5 H <sub>8</sub> C <sub>5</sub> → 8.18 BN + NaB <sub>6</sub> H <sub>4</sub> C <sub>6</sub> N                                              | -12.3842            |
| NaNH <sub>4</sub> B <sub>6</sub> C <sub>6</sub> | 0.6667 NaC <sub>64</sub> + 0.5714 B <sub>5</sub> H <sub>7</sub> + 0.3333 NaN <sub>3</sub> + 241.5 B → 18.33 B <sub>13</sub> C <sub>2</sub> + NaB <sub>6</sub> H <sub>4</sub> C <sub>6</sub> N                            | -12.2592            |
| NaNH <sub>4</sub> B <sub>6</sub> C <sub>6</sub> | 0.3636 B <sub>9</sub> H <sub>11</sub> + 0.6667 NaC <sub>64</sub> + 0.3333 NaN <sub>3</sub> + 241.1 B → 18.33 B <sub>13</sub> C <sub>2</sub> + NaB <sub>6</sub> H <sub>4</sub> C <sub>6</sub> N                           | -12.1970            |
| NaNH <sub>4</sub> B <sub>6</sub> C <sub>6</sub> | H <sub>3</sub> N + 0.6667 B <sub>9</sub> H <sub>11</sub> + NaC <sub>64</sub> + 43.23 H <sub>2</sub> → 11.6 H <sub>8</sub> C <sub>5</sub> + NaB <sub>6</sub> H <sub>4</sub> C <sub>6</sub> N                              | -12.1489            |
| NaNH <sub>4</sub> B <sub>6</sub> C <sub>6</sub> | 10.77 H <sub>3</sub> N + 3 B <sub>13</sub> C <sub>2</sub> + NaN <sub>3</sub> → 12.77 BN + 4.045 B <sub>5</sub> H <sub>7</sub> + NaB <sub>6</sub> H <sub>4</sub> C <sub>6</sub> N                                         | -12.1430            |
| NaNH <sub>4</sub> B <sub>6</sub> C <sub>6</sub> | BN + NaC <sub>64</sub> + 48.4 H <sub>2</sub> + 5 B → 11.6 H <sub>8</sub> C <sub>5</sub> + NaB <sub>6</sub> H <sub>4</sub> C <sub>6</sub> N                                                                               | -12.1152            |
| NaNH <sub>4</sub> B <sub>6</sub> C <sub>6</sub> | H <sub>3</sub> N + NaC <sub>64</sub> + 1.2 B <sub>5</sub> H <sub>7</sub> + 42.7 H <sub>2</sub> → 11.6 H <sub>8</sub> C <sub>5</sub> + NaB <sub>6</sub> H <sub>4</sub> C <sub>6</sub> N                                   | -12.1038            |
| NaNH <sub>4</sub> B <sub>6</sub> C <sub>6</sub> | 15.13 H <sub>3</sub> N + 3 B <sub>13</sub> C <sub>2</sub> + NaB <sub>15</sub> → 14.13 BN + 3.763 B <sub>9</sub> H <sub>11</sub> + NaB <sub>6</sub> H <sub>4</sub> C <sub>6</sub> N                                       | -12.0780            |
| NaNH <sub>4</sub> B <sub>6</sub> C <sub>6</sub> | 0.3846 B <sub>13</sub> C <sub>2</sub> + BN + NaC <sub>64</sub> + 49.02 H <sub>2</sub> → 11.75 H <sub>8</sub> C <sub>5</sub> + NaB <sub>6</sub> H <sub>4</sub> C <sub>6</sub> N                                           | -11.9838            |
| NaNH <sub>4</sub> B <sub>6</sub> C <sub>6</sub> | 3 B <sub>13</sub> C <sub>2</sub> + 27.27 H <sub>2</sub> + 5.95 NaN <sub>3</sub> → 16.85 H <sub>3</sub> N + 1.65 Na <sub>3</sub> B <sub>20</sub> + NaB <sub>6</sub> H <sub>4</sub> C <sub>6</sub> N                       | -11.8534            |
| NaNH <sub>4</sub> B <sub>6</sub> C <sub>6</sub> | 4.297 N <sub>2</sub> + 0.09375 NaC <sub>64</sub> + 0.9062 NaB <sub>15</sub> + 2 H <sub>2</sub> → 7.594 BN + NaB <sub>6</sub> H <sub>4</sub> C <sub>6</sub> N                                                             | -11.8428            |
| NaNH <sub>4</sub> B <sub>6</sub> C <sub>6</sub> | 1.097 B <sub>13</sub> C <sub>2</sub> + 0.7611 H <sub>8</sub> C <sub>5</sub> + 3.088 NaN <sub>3</sub> → 2.088 NaH + 8.265 BN + NaB <sub>6</sub> H <sub>4</sub> C <sub>6</sub> N                                           | -11.1635            |
| NaNH <sub>4</sub> B <sub>6</sub> C <sub>6</sub> | BN + 0.5556 B <sub>9</sub> H <sub>11</sub> + NaC <sub>64</sub> + 45.34 H <sub>2</sub> → 11.6 H <sub>8</sub> C <sub>5</sub> + NaB <sub>6</sub> H <sub>4</sub> C <sub>6</sub> N                                            | -11.1077            |
| NaNH <sub>4</sub> B <sub>6</sub> C <sub>6</sub> | 9.921 H <sub>3</sub> N + 3 B <sub>13</sub> C <sub>2</sub> + NaN <sub>3</sub> → 11.92 BN + 2.342 B <sub>9</sub> H <sub>11</sub> + NaB <sub>6</sub> H <sub>4</sub> C <sub>6</sub> N                                        | -11.1043            |
| NaNH <sub>4</sub> B <sub>6</sub> C <sub>6</sub> | BN + NaC <sub>64</sub> + B <sub>5</sub> H <sub>7</sub> + 44.9 H <sub>2</sub> → 11.6 H <sub>8</sub> C <sub>5</sub> + NaB <sub>6</sub> H <sub>4</sub> C <sub>6</sub> N                                                     | -11.0701            |
| NaNH <sub>4</sub> B <sub>6</sub> C <sub>6</sub> | 10 H <sub>3</sub> N + NaB <sub>15</sub> + 22.25 C → 9 BN + 3.25 H <sub>8</sub> C <sub>5</sub> + NaB <sub>6</sub> H <sub>4</sub> C <sub>6</sub> N                                                                         | -11.0349            |
| NaNH <sub>4</sub> B <sub>6</sub> C <sub>6</sub> | 1.333 H <sub>3</sub> N + 3.63 N <sub>2</sub> + 0.09375 NaC <sub>64</sub> + 0.9062 NaB <sub>15</sub> → 7.594 BN + NaB <sub>6</sub> H <sub>4</sub> C <sub>6</sub> N                                                        | -10.0774            |
| NaNH <sub>4</sub> B <sub>6</sub> C <sub>6</sub> | 0.5 N <sub>2</sub> + NaC <sub>64</sub> + 100.6 B <sub>5</sub> H <sub>7</sub> → 55.25 B <sub>9</sub> H <sub>11</sub> + 11.6 H <sub>8</sub> C <sub>5</sub> + NaB <sub>6</sub> H <sub>4</sub> C <sub>6</sub> N              | -9.6917             |
| NaNH <sub>4</sub> B <sub>6</sub> C <sub>6</sub> | 13.85 H <sub>3</sub> N + 3 B <sub>13</sub> C <sub>2</sub> + 0.3333 Na <sub>3</sub> B <sub>20</sub> → 12.85 BN + 5.364 B <sub>5</sub> H <sub>7</sub> + NaB <sub>6</sub> H <sub>4</sub> C <sub>6</sub> N                   | -9.6126             |
| NaNH <sub>4</sub> B <sub>6</sub> C <sub>6</sub> | 1.333 H <sub>3</sub> N + 3 B <sub>13</sub> C <sub>2</sub> + 2.648 NaN <sub>3</sub> → 8.278 BN + 1.648 NaB <sub>15</sub> + NaB <sub>6</sub> H <sub>4</sub> C <sub>6</sub> N                                               | -9.4994             |
| NaNH <sub>4</sub> B <sub>6</sub> C <sub>6</sub> | 3 B <sub>13</sub> C <sub>2</sub> + 0.3636 B <sub>9</sub> H <sub>11</sub> + 2.904 NaN <sub>3</sub> → 7.712 BN + 1.904 NaB <sub>15</sub> + NaB <sub>6</sub> H <sub>4</sub> C <sub>6</sub> N                                | -9.2502             |
| NaNH <sub>4</sub> B <sub>6</sub> C <sub>6</sub> | 3 B <sub>13</sub> C <sub>2</sub> + 0.5714 B <sub>5</sub> H <sub>7</sub> + 2.881 NaN <sub>3</sub> → 7.643 BN + 1.881 NaB <sub>15</sub> + NaB <sub>6</sub> H <sub>4</sub> C <sub>6</sub> N                                 | -9.1259             |
| NaNH <sub>4</sub> B <sub>6</sub> C <sub>6</sub> | H <sub>3</sub> N + NaC <sub>64</sub> + 97.27 B <sub>5</sub> H <sub>7</sub> → 53.37 B <sub>9</sub> H <sub>11</sub> + 11.6 H <sub>8</sub> C <sub>5</sub> + NaB <sub>6</sub> H <sub>4</sub> C <sub>6</sub> N                | -8.4944             |
| NaNH <sub>4</sub> B <sub>6</sub> C <sub>6</sub> | 3 B <sub>13</sub> C <sub>2</sub> + 2 H <sub>2</sub> + 2.722 NaN <sub>3</sub> → 7.167 BN + 1.722 NaB <sub>15</sub> + NaB <sub>6</sub> H <sub>4</sub> C <sub>6</sub> N                                                     | -8.4408             |
| NaNH <sub>4</sub> B <sub>6</sub> C <sub>6</sub> | 12.72 H <sub>3</sub> N + 3 B <sub>13</sub> C <sub>2</sub> + 0.3333 Na <sub>3</sub> B <sub>20</sub> → 11.72 BN + 3.105 B <sub>9</sub> H <sub>11</sub> + NaB <sub>6</sub> H <sub>4</sub> C <sub>6</sub> N                  | -8.2354             |
| NaNH <sub>4</sub> B <sub>6</sub> C <sub>6</sub> | 7.6 B <sub>5</sub> H <sub>7</sub> + 6 C + 5.8 NaN <sub>3</sub> → 16.4 H <sub>3</sub> N + 1.6 Na <sub>3</sub> B <sub>20</sub> + NaB <sub>6</sub> H <sub>4</sub> C <sub>6</sub> N                                          | -7.3378             |
| NaNH <sub>4</sub> B <sub>6</sub> C <sub>6</sub> | BN + NaC <sub>64</sub> + 102 B <sub>5</sub> H <sub>7</sub> → 56.13 B <sub>9</sub> H <sub>11</sub> + 11.6 H <sub>8</sub> C <sub>5</sub> + NaB <sub>6</sub> H <sub>4</sub> C <sub>6</sub> N                                | -7.2747             |
| NaNH <sub>4</sub> B <sub>6</sub> C <sub>6</sub> | 1.75 B <sub>13</sub> C <sub>2</sub> + 0.5 H <sub>8</sub> C <sub>5</sub> + 2.526 NaN <sub>3</sub> → 6.578 BN + 0.5086 Na <sub>3</sub> B <sub>20</sub> + NaB <sub>6</sub> H <sub>4</sub> C <sub>6</sub> N                  | -6.7504             |
| NaNH <sub>4</sub> B <sub>6</sub> C <sub>6</sub> | 0.6667 NaC <sub>64</sub> + 31.33 H <sub>2</sub> + 0.3333 NaN <sub>3</sub> + 6 B → 7.333 H <sub>8</sub> C <sub>5</sub> + NaB <sub>6</sub> H <sub>4</sub> C <sub>6</sub> N                                                 | -6.5944             |
| NaNH <sub>4</sub> B <sub>6</sub> C <sub>6</sub> | 11.73 H <sub>3</sub> N + 3 B <sub>13</sub> C <sub>2</sub> + Na → 10.73 BN + 4.455 B <sub>5</sub> H <sub>7</sub> + NaB <sub>6</sub> H <sub>4</sub> C <sub>6</sub> N                                                       | -6.4832             |
| NaNH <sub>4</sub> B <sub>6</sub> C <sub>6</sub> | 0.4615 B <sub>13</sub> C <sub>2</sub> + 0.6667 NaC <sub>64</sub> + 32.07 H <sub>2</sub> + 0.3333 NaN <sub>3</sub> → 7.518 H <sub>8</sub> C <sub>5</sub> + NaB <sub>6</sub> H <sub>4</sub> C <sub>6</sub> N               | -6.4368             |
| NaNH <sub>4</sub> B <sub>6</sub> C <sub>6</sub> | 6 BN + NaC <sub>64</sub> + 55.9 H <sub>2</sub> → 5 H <sub>3</sub> N + 11.6 H <sub>8</sub> C <sub>5</sub> + NaB <sub>6</sub> H <sub>4</sub> C <sub>6</sub> N                                                              | -5.9017             |
| NaNH <sub>4</sub> B <sub>6</sub> C <sub>6</sub> | 11.5 H <sub>3</sub> N + 3 B <sub>13</sub> C <sub>2</sub> + NaH → 10.5 BN + 4.5 B <sub>5</sub> H <sub>7</sub> + NaB <sub>6</sub> H <sub>4</sub> C <sub>6</sub> N                                                          | -5.8678             |
| NaNH <sub>4</sub> B <sub>6</sub> C <sub>6</sub> | 3 B <sub>13</sub> C <sub>2</sub> + 5.321 B <sub>9</sub> H <sub>11</sub> + 6.393 NaN <sub>3</sub> → 18.18 H <sub>3</sub> N + 5.393 NaB <sub>15</sub> + NaB <sub>6</sub> H <sub>4</sub> C <sub>6</sub> N                   | -5.8529             |
| NaNH <sub>4</sub> B <sub>6</sub> C <sub>6</sub> | 0.6667 B <sub>9</sub> H <sub>11</sub> + 0.6667 NaC <sub>64</sub> + 27.67 H <sub>2</sub> + 0.3333 NaN <sub>3</sub> → 7.333 H <sub>8</sub> C <sub>5</sub> + NaB <sub>6</sub> H <sub>4</sub> C <sub>6</sub> N               | -5.3855             |
| NaNH <sub>4</sub> B <sub>6</sub> C <sub>6</sub> | 0.6667 NaC <sub>64</sub> + 1.2 B <sub>5</sub> H <sub>7</sub> + 27.13 H <sub>2</sub> + 0.3333 NaN <sub>3</sub> → 7.333 H <sub>8</sub> C <sub>5</sub> + NaB <sub>6</sub> H <sub>4</sub> C <sub>6</sub> N                   | -5.3404             |
| NaNH <sub>4</sub> B <sub>6</sub> C <sub>6</sub> | 10.79 H <sub>3</sub> N + 3 B <sub>13</sub> C <sub>2</sub> + Na → 9.789 BN + 2.579 B <sub>9</sub> H <sub>11</sub> + NaB <sub>6</sub> H <sub>4</sub> C <sub>6</sub> N                                                      | -5.3394             |
| NaNH <sub>4</sub> B <sub>6</sub> C <sub>6</sub> | 0.5 N <sub>2</sub> + 0.6 NaC <sub>64</sub> + 0.4 NaB <sub>15</sub> + 27.92 H <sub>2</sub> → 6.48 H <sub>8</sub> C <sub>5</sub> + NaB <sub>6</sub> H <sub>4</sub> C <sub>6</sub> N                                        | -4.8257             |
| NaNH <sub>4</sub> B <sub>6</sub> C <sub>6</sub> | 10.55 H <sub>3</sub> N + 3 B <sub>13</sub> C <sub>2</sub> + NaH → 9.553 BN + 2.605 B <sub>9</sub> H <sub>11</sub> + NaB <sub>6</sub> H <sub>4</sub> C <sub>6</sub> N                                                     | -4.7123             |
| NaNH <sub>4</sub> B <sub>6</sub> C <sub>6</sub> | 3 B <sub>13</sub> C <sub>2</sub> + 7.45 B <sub>5</sub> H <sub>7</sub> + 5.683 NaN <sub>3</sub> → 16.05 H <sub>3</sub> N + 4.683 NaB <sub>15</sub> + NaB <sub>6</sub> H <sub>4</sub> C <sub>6</sub> N                     | -4.6309             |
| NaNH <sub>4</sub> B <sub>6</sub> C <sub>6</sub> | BN + 0.6667 NaC <sub>64</sub> + 0.3333 NaB <sub>15</sub> + 31.33 H <sub>2</sub> → 7.333 H <sub>8</sub> C <sub>5</sub> + NaB <sub>6</sub> H <sub>4</sub> C <sub>6</sub> N                                                 | -3.9017             |
| NaNH <sub>4</sub> B <sub>6</sub> C <sub>6</sub> | 3 N <sub>2</sub> + NaB <sub>15</sub> + 1.2 H <sub>8</sub> C <sub>5</sub> → 5 BN + 0.8 B <sub>5</sub> H <sub>7</sub> + NaB <sub>6</sub> H <sub>4</sub> C <sub>6</sub> N                                                   | -3.7112             |
| NaNH <sub>4</sub> B <sub>6</sub> C <sub>6</sub> | 0.5 N <sub>2</sub> + NaC <sub>64</sub> + 11.94 B <sub>5</sub> H <sub>7</sub> → 4.131 B <sub>13</sub> C <sub>2</sub> + 9.948 H <sub>8</sub> C <sub>5</sub> + NaB <sub>6</sub> H <sub>4</sub> C <sub>6</sub> N             | -3.6150             |
| NaNH <sub>4</sub> B <sub>6</sub> C <sub>6</sub> | H <sub>3</sub> N + 0.6 NaC <sub>64</sub> + 0.4 NaB <sub>15</sub> + 26.42 H <sub>2</sub> → 6.48 H <sub>8</sub> C <sub>5</sub> + NaB <sub>6</sub> H <sub>4</sub> C <sub>6</sub> N                                          | -3.5017             |
| NaNH <sub>4</sub> B <sub>6</sub> C <sub>6</sub> | 0.6667 NaC <sub>64</sub> + 62.25 B <sub>5</sub> H <sub>7</sub> + 0.3333 NaN <sub>3</sub> → 33.92 B <sub>9</sub> H <sub>11</sub> + 7.333 H <sub>8</sub> C <sub>5</sub> + NaB <sub>6</sub> H <sub>4</sub> C <sub>6</sub> N | -3.0468             |
| NaNH <sub>4</sub> B <sub>6</sub> C <sub>6</sub> | 10 H <sub>3</sub> N + NaB <sub>15</sub> + 6 C → 9 BN + 13 H <sub>2</sub> + NaB <sub>6</sub> H <sub>4</sub> C <sub>6</sub> N                                                                                              | -2.9038             |
| NaNH <sub>4</sub> B <sub>6</sub> C <sub>6</sub> | 2.47 N <sub>2</sub> + 0.3636 B <sub>9</sub> H <sub>11</sub> + 0.3333 Na <sub>3</sub> B <sub>20</sub> + 6 C → 3.939 BN + NaB <sub>6</sub> H <sub>4</sub> C <sub>6</sub> N                                                 | -2.8438             |
| NaNH <sub>4</sub> B <sub>6</sub> C <sub>6</sub> | 0.5 N <sub>2</sub> + 7.437 B <sub>9</sub> H <sub>11</sub> + NaC <sub>64</sub> → 4.687 B <sub>13</sub> C <sub>2</sub> + 9.725 H <sub>8</sub> C <sub>5</sub> + NaB <sub>6</sub> H <sub>4</sub> C <sub>6</sub> N            | -2.7971             |
| NaNH <sub>4</sub> B <sub>6</sub> C <sub>6</sub> | H <sub>3</sub> N + NaC <sub>64</sub> + 11.58 B <sub>5</sub> H <sub>7</sub> → 3.991 B <sub>13</sub> C <sub>2</sub> + 10 H <sub>8</sub> C <sub>5</sub> + NaB <sub>6</sub> H <sub>4</sub> C <sub>6</sub> N                  | -2.6240             |
| NaNH <sub>4</sub> B <sub>6</sub> C <sub>6</sub> | 2.709 N <sub>2</sub> + NaB <sub>15</sub> + 1.2 H <sub>8</sub> C <sub>5</sub> → 4.418 BN + 0.5091 B <sub>9</sub> H <sub>11</sub> + NaB <sub>6</sub> H <sub>4</sub> C <sub>6</sub> N                                       | -2.3050             |
| NaNH <sub>4</sub> B <sub>6</sub> C <sub>6</sub> | 2.262 N <sub>2</sub> + 0.5714 B <sub>5</sub> H <sub>7</sub> + 0.3333 Na <sub>3</sub> B <sub>20</sub> + 6 C → 3.524 BN + NaB <sub>6</sub> H <sub>4</sub> C <sub>6</sub> N                                                 | -1.8393             |
| NaNH <sub>4</sub> B <sub>6</sub> C <sub>6</sub> | H <sub>3</sub> N + 7.21 B <sub>9</sub> H <sub>11</sub> + NaC <sub>64</sub> → 4.53 B <sub>13</sub> C <sub>2</sub> + 9.788 H <sub>8</sub> C <sub>5</sub> + NaB <sub>6</sub> H <sub>4</sub> C <sub>6</sub> N                | -1.8310             |
| NaNH <sub>4</sub> B <sub>6</sub> C <sub>6</sub> | 3 B <sub>13</sub> C <sub>2</sub> + 14.9 H <sub>2</sub> + 3.2 NaN <sub>3</sub> → 8.6 H <sub>3</sub> N + 2.2 NaB <sub>15</sub> + NaB <sub>6</sub> H <sub>4</sub> C <sub>6</sub> N                                          | -1.6133             |
| NaNH <sub>4</sub> B <sub>6</sub> C <sub>6</sub> | 1.75 B <sub>13</sub> C <sub>2</sub> + 0.5 H <sub>8</sub> C <sub>5</sub> + 1.819 NaN <sub>3</sub> → 4.458 BN + 0.8194 NaB <sub>15</sub> + NaB <sub>6</sub> H <sub>4</sub> C <sub>6</sub> N                                | -1.5749             |
| NaNH <sub>4</sub> B <sub>6</sub> C <sub>6</sub> | 4 NaH + 6 BN + 198 C → 2.5 N <sub>2</sub> + 3 NaC <sub>64</sub> + NaB <sub>6</sub> H <sub>4</sub> C <sub>6</sub> N                                                                                                       | -1.4903             |
| NaNH <sub>4</sub> B <sub>6</sub> C <sub>6</sub> | 6.377 H <sub>3</sub> N + 0.2415 NaC <sub>64</sub> + 0.7585 NaB <sub>15</sub> → 5.377 BN + 1.891 H <sub>8</sub> C <sub>5</sub> + NaB <sub>6</sub> H <sub>4</sub> C <sub>6</sub> N                                         | -1.3507             |
| NaNH <sub>4</sub> B <sub>6</sub> C <sub>6</sub> | BN + NaC <sub>64</sub> + 11.91 B <sub>5</sub> H <sub>7</sub> → 4.196 B <sub>13</sub> C <sub>2</sub> + 9.921 H <sub>8</sub> C <sub>5</sub> + NaB <sub>6</sub> H <sub>4</sub> C <sub>6</sub> N                             | -1.1019             |
| NaNH <sub>4</sub> B <sub>6</sub> C <sub>6</sub> | 3 B <sub>13</sub> C <sub>2</sub> + 23.7 H <sub>2</sub> + NaN <sub>3</sub> → 2 BN + 6.2 B <sub>5</sub> H <sub>7</sub> + NaB <sub>6</sub> H <sub>4</sub> C <sub>6</sub> N                                                  | -1.0074             |
| NaNH <sub>4</sub> B <sub>6</sub> C <sub>6</sub> | 3 B <sub>13</sub> C <sub>2</sub> + 20.94 H <sub>2</sub> + NaN <sub>3</sub> → 2 BN + 3.444 B <sub>9</sub> H <sub>11</sub> + NaB <sub>6</sub> H <sub>4</sub> C <sub>6</sub> N                                              | -0.7745             |

Continued on next page

Continued

| Compound                                        | Chemical reaction                                                                                                                                                                                 | Reaction energy(eV) |
|-------------------------------------------------|---------------------------------------------------------------------------------------------------------------------------------------------------------------------------------------------------|---------------------|
| NaNH <sub>4</sub> B <sub>6</sub> C <sub>6</sub> | 2.157 N <sub>2</sub> + 0.3636 B <sub>9</sub> H <sub>11</sub> + 0.09375 NaC <sub>64</sub> + 0.3021 Na <sub>3</sub> B <sub>20</sub> → 3.314 BN + NaB <sub>6</sub> H <sub>4</sub> C <sub>6</sub> N   | -0.5147             |
| NaNH <sub>4</sub> B <sub>6</sub> C <sub>6</sub> | 8.594 H <sub>3</sub> N + 0.09375 NaC <sub>64</sub> + 0.9062 NaB <sub>15</sub> → 7.594 BN + 10.89 H <sub>2</sub> + NaB <sub>6</sub> H <sub>4</sub> C <sub>6</sub> N                                | -0.4641             |
| NaNH <sub>4</sub> B <sub>6</sub> C <sub>6</sub> | BN + 7.418 B <sub>9</sub> H <sub>11</sub> + NaC <sub>64</sub> → 4.751 B <sub>13</sub> C <sub>2</sub> + 9.7 H <sub>8</sub> C <sub>5</sub> + NaB <sub>6</sub> H <sub>4</sub> C <sub>6</sub> N       | -0.2860             |
| NaNH <sub>4</sub> B <sub>6</sub> C <sub>6</sub> | 0.5 N <sub>2</sub> + NaC <sub>64</sub> + 13.83 B <sub>5</sub> H <sub>7</sub> → 11.6 H <sub>8</sub> C <sub>5</sub> + 63.14 B + NaB <sub>6</sub> H <sub>4</sub> C <sub>6</sub> N                    | -0.2307             |
| NaNH <sub>4</sub> B <sub>6</sub> C <sub>6</sub> | 1.333 H <sub>3</sub> N + 6 C + NaN <sub>3</sub> + 9.333 B → 3.333 BN + NaB <sub>6</sub> H <sub>4</sub> C <sub>6</sub> N                                                                           | -0.2121             |
| PbNH <sub>4</sub> B <sub>6</sub> C <sub>6</sub> | Pb + 3 B <sub>13</sub> C <sub>2</sub> + 0.3636 B <sub>9</sub> H <sub>11</sub> + 18.64 N <sub>2</sub> → 36.27 BN + B <sub>6</sub> H <sub>4</sub> PbC <sub>6</sub> N                                | -79.1596            |
| PbNH <sub>4</sub> B <sub>6</sub> C <sub>6</sub> | Pb + 0.5714 B <sub>5</sub> H <sub>7</sub> + 3 B <sub>13</sub> C <sub>2</sub> + 18.43 N <sub>2</sub> → 35.86 BN + B <sub>6</sub> H <sub>4</sub> PbC <sub>6</sub> N                                 | -78.1552            |
| PbNH <sub>4</sub> B <sub>6</sub> C <sub>6</sub> | Pb + 3 B <sub>13</sub> C <sub>2</sub> + 2 H <sub>2</sub> + 17 N <sub>2</sub> → 33 BN + B <sub>6</sub> H <sub>4</sub> PbC <sub>6</sub> N                                                           | -71.4187            |
| PbNH <sub>4</sub> B <sub>6</sub> C <sub>6</sub> | Pb + 3 B <sub>13</sub> C <sub>2</sub> + 1.333 H <sub>3</sub> N + 16.33 N <sub>2</sub> → 33 BN + B <sub>6</sub> H <sub>4</sub> PbC <sub>6</sub> N                                                  | -69.6533            |
| PbNH <sub>4</sub> B <sub>6</sub> C <sub>6</sub> | Pb + 1.75 B <sub>13</sub> C <sub>2</sub> + 0.5 H <sub>8</sub> C <sub>5</sub> + 8.875 N <sub>2</sub> → 16.75 BN + B <sub>6</sub> H <sub>4</sub> PbC <sub>6</sub> N                                 | -30.1358            |
| PbNH <sub>4</sub> B <sub>6</sub> C <sub>6</sub> | Pb + 3 B <sub>13</sub> C <sub>2</sub> + 34 H <sub>3</sub> N → 33 BN + 49 H <sub>2</sub> + B <sub>6</sub> H <sub>4</sub> PbC <sub>6</sub> N                                                        | -26.4003            |
| PbNH <sub>4</sub> B <sub>6</sub> C <sub>6</sub> | Pb + 3 B <sub>13</sub> C <sub>2</sub> + 11.73 H <sub>3</sub> N → 4.455 B <sub>5</sub> H <sub>7</sub> + 10.73 BN + B <sub>6</sub> H <sub>4</sub> PbC <sub>6</sub> N                                | -3.3774             |
| PbNH <sub>4</sub> B <sub>6</sub> C <sub>6</sub> | Pb + 3 B <sub>13</sub> C <sub>2</sub> + 10.79 H <sub>3</sub> N → 2.579 B <sub>9</sub> H <sub>11</sub> + 9.789 BN + B <sub>6</sub> H <sub>4</sub> PbC <sub>6</sub> N                               | -2.2336             |
| SrNH <sub>4</sub> B <sub>6</sub> C <sub>6</sub> | 3 B <sub>13</sub> C <sub>2</sub> + 98 SrN <sub>2</sub> + 18 B <sub>9</sub> H <sub>11</sub> → 195 BN + 97 SrH <sub>2</sub> + SrB <sub>6</sub> H <sub>4</sub> C <sub>6</sub> N                      | -468.3416           |
| SrNH <sub>4</sub> B <sub>6</sub> C <sub>6</sub> | 3 B <sub>13</sub> C <sub>2</sub> + 62 SrN <sub>2</sub> + 18 B <sub>5</sub> H <sub>7</sub> → 123 BN + 61 SrH <sub>2</sub> + SrB <sub>6</sub> H <sub>4</sub> C <sub>6</sub> N                       | -293.4320           |
| SrNH <sub>4</sub> B <sub>6</sub> C <sub>6</sub> | 3 B <sub>13</sub> C <sub>2</sub> + 69 H <sub>2</sub> + 34 Sr <sub>2</sub> N → 33 BN + 67 SrH <sub>2</sub> + SrB <sub>6</sub> H <sub>4</sub> C <sub>6</sub> N                                      | -126.9347           |
| SrNH <sub>4</sub> B <sub>6</sub> C <sub>6</sub> | 3 B <sub>13</sub> C <sub>2</sub> + 34 H <sub>3</sub> N + 50 Sr → 33 BN + 49 SrH <sub>2</sub> + SrB <sub>6</sub> H <sub>4</sub> C <sub>6</sub> N                                                   | -109.2894           |
| SrNH <sub>4</sub> B <sub>6</sub> C <sub>6</sub> | 3 B <sub>13</sub> C <sub>2</sub> + 36.5 SrN <sub>2</sub> + 20 B <sub>9</sub> H <sub>11</sub> → 72 H <sub>3</sub> N + 35.5 SrB <sub>6</sub> + SrB <sub>6</sub> H <sub>4</sub> C <sub>6</sub> N     | -107.9539           |
| SrNH <sub>4</sub> B <sub>6</sub> C <sub>6</sub> | 4 B <sub>13</sub> C <sub>2</sub> + 23.5 N <sub>2</sub> + 2 SrH <sub>2</sub> → 46 BN + SrC <sub>2</sub> + SrB <sub>6</sub> H <sub>4</sub> C <sub>6</sub> N                                         | -105.0899           |
| SrNH <sub>4</sub> B <sub>6</sub> C <sub>6</sub> | 3 B <sub>13</sub> C <sub>2</sub> + 0.3636 B <sub>9</sub> H <sub>11</sub> + 21.64 N <sub>2</sub> + SrB <sub>6</sub> → 42.27 BN + SrB <sub>6</sub> H <sub>4</sub> C <sub>6</sub> N                  | -96.0468            |
| SrNH <sub>4</sub> B <sub>6</sub> C <sub>6</sub> | 3 B <sub>13</sub> C <sub>2</sub> + 0.5714 B <sub>5</sub> H <sub>7</sub> + 21.43 N <sub>2</sub> + SrB <sub>6</sub> → 41.86 BN + SrB <sub>6</sub> H <sub>4</sub> C <sub>6</sub> N                   | -95.0424            |
| SrNH <sub>4</sub> B <sub>6</sub> C <sub>6</sub> | 3 B <sub>13</sub> C <sub>2</sub> + 35 H <sub>2</sub> + 34 SrN → 33 BN + 33 SrH <sub>2</sub> + SrB <sub>6</sub> H <sub>4</sub> C <sub>6</sub> N                                                    | -93.0918            |
| SrNH <sub>4</sub> B <sub>6</sub> C <sub>6</sub> | 3 B <sub>13</sub> C <sub>2</sub> + 2 H <sub>2</sub> + 20 N <sub>2</sub> + SrB <sub>6</sub> → 39 BN + SrB <sub>6</sub> H <sub>4</sub> C <sub>6</sub> N                                             | -88.3060            |
| SrNH <sub>4</sub> B <sub>6</sub> C <sub>6</sub> | 3 B <sub>13</sub> C <sub>2</sub> + 1.333 H <sub>3</sub> N + 19.33 N <sub>2</sub> + SrB <sub>6</sub> → 39 BN + SrB <sub>6</sub> H <sub>4</sub> C <sub>6</sub> N                                    | -86.5405            |
| SrNH <sub>4</sub> B <sub>6</sub> C <sub>6</sub> | 3 B <sub>13</sub> C <sub>2</sub> + 0.3636 B <sub>9</sub> H <sub>11</sub> + 18.64 N <sub>2</sub> + Sr → 36.27 BN + SrB <sub>6</sub> H <sub>4</sub> C <sub>6</sub> N                                | -83.7966            |
| SrNH <sub>4</sub> B <sub>6</sub> C <sub>6</sub> | 3 B <sub>13</sub> C <sub>2</sub> + 0.3636 B <sub>9</sub> H <sub>11</sub> + 18.39 N <sub>2</sub> + 0.5 Sr <sub>2</sub> N → 36.27 BN + SrB <sub>6</sub> H <sub>4</sub> C <sub>6</sub> N             | -82.9714            |
| SrNH <sub>4</sub> B <sub>6</sub> C <sub>6</sub> | 3 B <sub>13</sub> C <sub>2</sub> + 0.5714 B <sub>5</sub> H <sub>7</sub> + 18.43 N <sub>2</sub> + Sr → 35.86 BN + SrB <sub>6</sub> H <sub>4</sub> C <sub>6</sub> N                                 | -82.7922            |
| SrNH <sub>4</sub> B <sub>6</sub> C <sub>6</sub> | 3 B <sub>13</sub> C <sub>2</sub> + SrN + 0.3636 B <sub>9</sub> H <sub>11</sub> + 18.14 N <sub>2</sub> → 36.27 BN + SrB <sub>6</sub> H <sub>4</sub> C <sub>6</sub> N                               | -82.7477            |
| SrNH <sub>4</sub> B <sub>6</sub> C <sub>6</sub> | 3 B <sub>13</sub> C <sub>2</sub> + SrN <sub>2</sub> + 0.3636 B <sub>9</sub> H <sub>11</sub> + 17.64 N <sub>2</sub> → 36.27 BN + SrB <sub>6</sub> H <sub>4</sub> C <sub>6</sub> N                  | -82.3089            |
| SrNH <sub>4</sub> B <sub>6</sub> C <sub>6</sub> | 3 B <sub>13</sub> C <sub>2</sub> + 0.5714 B <sub>5</sub> H <sub>7</sub> + 18.18 N <sub>2</sub> + 0.5 Sr <sub>2</sub> N → 35.86 BN + SrB <sub>6</sub> H <sub>4</sub> C <sub>6</sub> N              | -81.9669            |
| SrNH <sub>4</sub> B <sub>6</sub> C <sub>6</sub> | 3 B <sub>13</sub> C <sub>2</sub> + SrN + 0.5714 B <sub>5</sub> H <sub>7</sub> + 17.93 N <sub>2</sub> → 35.86 BN + SrB <sub>6</sub> H <sub>4</sub> C <sub>6</sub> N                                | -81.7433            |
| SrNH <sub>4</sub> B <sub>6</sub> C <sub>6</sub> | 3 B <sub>13</sub> C <sub>2</sub> + SrN <sub>2</sub> + 0.5714 B <sub>5</sub> H <sub>7</sub> + 17.43 N <sub>2</sub> → 35.86 BN + SrB <sub>6</sub> H <sub>4</sub> C <sub>6</sub> N                   | -81.3045            |
| SrNH <sub>4</sub> B <sub>6</sub> C <sub>6</sub> | 3 B <sub>13</sub> C <sub>2</sub> + 0.1818 B <sub>9</sub> H <sub>11</sub> + 17.82 N <sub>2</sub> + SrH <sub>2</sub> → 34.64 BN + SrB <sub>6</sub> H <sub>4</sub> C <sub>6</sub> N                  | -78.3292            |
| SrNH <sub>4</sub> B <sub>6</sub> C <sub>6</sub> | 3 B <sub>13</sub> C <sub>2</sub> + 0.2857 B <sub>5</sub> H <sub>7</sub> + 17.71 N <sub>2</sub> + SrH <sub>2</sub> → 34.43 BN + SrB <sub>6</sub> H <sub>4</sub> C <sub>6</sub> N                   | -77.8270            |
| SrNH <sub>4</sub> B <sub>6</sub> C <sub>6</sub> | 3 B <sub>13</sub> C <sub>2</sub> + 17 SrN <sub>2</sub> + 18 H <sub>2</sub> → 33 BN + 16 SrH <sub>2</sub> + SrB <sub>6</sub> H <sub>4</sub> C <sub>6</sub> N                                       | -76.3165            |
| SrNH <sub>4</sub> B <sub>6</sub> C <sub>6</sub> | 3 B <sub>13</sub> C <sub>2</sub> + 2 H <sub>2</sub> + 17 N <sub>2</sub> + Sr → 33 BN + SrB <sub>6</sub> H <sub>4</sub> C <sub>6</sub> N                                                           | -76.0558            |
| SrNH <sub>4</sub> B <sub>6</sub> C <sub>6</sub> | 3 B <sub>13</sub> C <sub>2</sub> + 2 H <sub>2</sub> + 16.75 N <sub>2</sub> + 0.5 Sr <sub>2</sub> N → 33 BN + SrB <sub>6</sub> H <sub>4</sub> C <sub>6</sub> N                                     | -75.2305            |
| SrNH <sub>4</sub> B <sub>6</sub> C <sub>6</sub> | 3 B <sub>13</sub> C <sub>2</sub> + 2 H <sub>2</sub> + SrN + 16.5 N <sub>2</sub> → 33 BN + SrB <sub>6</sub> H <sub>4</sub> C <sub>6</sub> N                                                        | -75.0068            |
| SrNH <sub>4</sub> B <sub>6</sub> C <sub>6</sub> | 3 B <sub>13</sub> C <sub>2</sub> + SrN <sub>2</sub> + 2 H <sub>2</sub> + 16 N <sub>2</sub> → 33 BN + SrB <sub>6</sub> H <sub>4</sub> C <sub>6</sub> N                                             | -74.5681            |
| SrNH <sub>4</sub> B <sub>6</sub> C <sub>6</sub> | 3 B <sub>13</sub> C <sub>2</sub> + H <sub>2</sub> + 17 N <sub>2</sub> + SrH <sub>2</sub> → 33 BN + SrB <sub>6</sub> H <sub>4</sub> C <sub>6</sub> N                                               | -74.4588            |
| SrNH <sub>4</sub> B <sub>6</sub> C <sub>6</sub> | 3 B <sub>13</sub> C <sub>2</sub> + 18 N <sub>2</sub> + 2 SrH <sub>2</sub> → SrN <sub>2</sub> + 33 BN + SrB <sub>6</sub> H <sub>4</sub> C <sub>6</sub> N                                           | -74.3495            |
| SrNH <sub>4</sub> B <sub>6</sub> C <sub>6</sub> | 3 B <sub>13</sub> C <sub>2</sub> + 1.333 H <sub>3</sub> N + 16.33 N <sub>2</sub> + Sr → 33 BN + SrB <sub>6</sub> H <sub>4</sub> C <sub>6</sub> N                                                  | -74.2903            |
| SrNH <sub>4</sub> B <sub>6</sub> C <sub>6</sub> | 3 B <sub>13</sub> C <sub>2</sub> + 17.5 N <sub>2</sub> + 2 SrH <sub>2</sub> → SrN + 33 BN + SrB <sub>6</sub> H <sub>4</sub> C <sub>6</sub> N                                                      | -73.9108            |
| SrNH <sub>4</sub> B <sub>6</sub> C <sub>6</sub> | 3 B <sub>13</sub> C <sub>2</sub> + 17.25 N <sub>2</sub> + 2 SrH <sub>2</sub> → 33 BN + 0.5 Sr <sub>2</sub> N + SrB <sub>6</sub> H <sub>4</sub> C <sub>6</sub> N                                   | -73.6871            |
| SrNH <sub>4</sub> B <sub>6</sub> C <sub>6</sub> | 3 B <sub>13</sub> C <sub>2</sub> + 0.6667 H <sub>3</sub> N + 16.67 N <sub>2</sub> + SrH <sub>2</sub> → 33 BN + SrB <sub>6</sub> H <sub>4</sub> C <sub>6</sub> N                                   | -73.5761            |
| SrNH <sub>4</sub> B <sub>6</sub> C <sub>6</sub> | 3 B <sub>13</sub> C <sub>2</sub> + 1.333 H <sub>3</sub> N + 16.08 N <sub>2</sub> + 0.5 Sr <sub>2</sub> N → 33 BN + SrB <sub>6</sub> H <sub>4</sub> C <sub>6</sub> N                               | -73.4651            |
| SrNH <sub>4</sub> B <sub>6</sub> C <sub>6</sub> | 3 B <sub>13</sub> C <sub>2</sub> + 1.333 H <sub>3</sub> N + SrN + 15.83 N <sub>2</sub> → 33 BN + SrB <sub>6</sub> H <sub>4</sub> C <sub>6</sub> N                                                 | -73.2414            |
| SrNH <sub>4</sub> B <sub>6</sub> C <sub>6</sub> | 3 B <sub>13</sub> C <sub>2</sub> + 17 N <sub>2</sub> + 2 SrH <sub>2</sub> → 33 BN + Sr + SrB <sub>6</sub> H <sub>4</sub> C <sub>6</sub> N                                                         | -72.8618            |
| SrNH <sub>4</sub> B <sub>6</sub> C <sub>6</sub> | 3 B <sub>13</sub> C <sub>2</sub> + SrN <sub>2</sub> + 1.333 H <sub>3</sub> N + 15.33 N <sub>2</sub> → 33 BN + SrB <sub>6</sub> H <sub>4</sub> C <sub>6</sub> N                                    | -72.8026            |
| SrNH <sub>4</sub> B <sub>6</sub> C <sub>6</sub> | 3 B <sub>13</sub> C <sub>2</sub> + 19.71 H <sub>3</sub> N + 14.29 Sr <sub>2</sub> N → 33 BN + 27.57 SrH <sub>2</sub> + SrB <sub>6</sub> H <sub>4</sub> C <sub>6</sub> N                           | -70.4044            |
| SrNH <sub>4</sub> B <sub>6</sub> C <sub>6</sub> | 3 B <sub>13</sub> C <sub>2</sub> + 14 H <sub>3</sub> N + 20 SrN → 33 BN + 19 SrH <sub>2</sub> + SrB <sub>6</sub> H <sub>4</sub> C <sub>6</sub> N                                                  | -66.8824            |
| SrNH <sub>4</sub> B <sub>6</sub> C <sub>6</sub> | 3 B <sub>13</sub> C <sub>2</sub> + 36.27 SrN <sub>2</sub> + 0.3636 B <sub>9</sub> H <sub>11</sub> → 35.27 SrN + 36.27 BN + SrB <sub>6</sub> H <sub>4</sub> C <sub>6</sub> N                       | -66.8330            |
| SrNH <sub>4</sub> B <sub>6</sub> C <sub>6</sub> | 3 B <sub>13</sub> C <sub>2</sub> + 24.52 SrN <sub>2</sub> + 0.3636 B <sub>9</sub> H <sub>11</sub> → 36.27 BN + 11.76 Sr <sub>2</sub> N + SrB <sub>6</sub> H <sub>4</sub> C <sub>6</sub> N         | -66.7319            |
| SrNH <sub>4</sub> B <sub>6</sub> C <sub>6</sub> | 3 B <sub>13</sub> C <sub>2</sub> + 73.55 SrN + 0.3636 B <sub>9</sub> H <sub>11</sub> → 36.27 BN + 36.27 Sr <sub>2</sub> N + SrB <sub>6</sub> H <sub>4</sub> C <sub>6</sub> N                      | -66.5211            |
| SrNH <sub>4</sub> B <sub>6</sub> C <sub>6</sub> | 3 B <sub>13</sub> C <sub>2</sub> + 35.86 SrN <sub>2</sub> + 0.5714 B <sub>5</sub> H <sub>7</sub> → 34.86 SrN + 35.86 BN + SrB <sub>6</sub> H <sub>4</sub> C <sub>6</sub> N                        | -66.0109            |
| SrNH <sub>4</sub> B <sub>6</sub> C <sub>6</sub> | 3 B <sub>13</sub> C <sub>2</sub> + 24.24 SrN <sub>2</sub> + 0.5714 B <sub>5</sub> H <sub>7</sub> → 35.86 BN + 11.62 Sr <sub>2</sub> N + SrB <sub>6</sub> H <sub>4</sub> C <sub>6</sub> N          | -65.9110            |
| SrNH <sub>4</sub> B <sub>6</sub> C <sub>6</sub> | 3 B <sub>13</sub> C <sub>2</sub> + 23.17 SrN <sub>2</sub> + 20 B <sub>5</sub> H <sub>7</sub> → 45.33 H <sub>3</sub> N + 22.17 SrB <sub>6</sub> + SrB <sub>6</sub> H <sub>4</sub> C <sub>6</sub> N | -65.8445            |
| SrNH <sub>4</sub> B <sub>6</sub> C <sub>6</sub> | 3 B <sub>13</sub> C <sub>2</sub> + 72.71 SrN + 0.5714 B <sub>5</sub> H <sub>7</sub> → 35.86 BN + 35.86 Sr <sub>2</sub> N + SrB <sub>6</sub> H <sub>4</sub> C <sub>6</sub> N                       | -65.7026            |
| SrNH <sub>4</sub> B <sub>6</sub> C <sub>6</sub> | 3 B <sub>13</sub> C <sub>2</sub> + 12.5 SrN <sub>2</sub> + 9 H <sub>3</sub> N → 33 BN + 11.5 SrH <sub>2</sub> + SrB <sub>6</sub> H <sub>4</sub> C <sub>6</sub> N                                  | -63.9082            |
| SrNH <sub>4</sub> B <sub>6</sub> C <sub>6</sub> | 3 B <sub>13</sub> C <sub>2</sub> + 14 N <sub>2</sub> + 2 SrH <sub>2</sub> → 27 BN + SrB <sub>6</sub> + SrB <sub>6</sub> H <sub>4</sub> C <sub>6</sub> N                                           | -60.6116            |

Continued on next page

Continued

| Compound                                        | Chemical reaction                                                                                                                                                                          | Reaction energy(eV) |
|-------------------------------------------------|--------------------------------------------------------------------------------------------------------------------------------------------------------------------------------------------|---------------------|
| SrNH <sub>4</sub> B <sub>6</sub> C <sub>6</sub> | $3 \text{ B}_{13}\text{C}_2 + 33 \text{ SrN}_2 + 2 \text{ H}_2 \rightarrow 32 \text{ SrN} + 33 \text{ BN} + \text{SrB}_6\text{H}_4\text{C}_6\text{N}$                                      | -60.5281            |
| SrNH <sub>4</sub> B <sub>6</sub> C <sub>6</sub> | $3 \text{ B}_{13}\text{C}_2 + 22.33 \text{ SrN}_2 + 2 \text{ H}_2 \rightarrow 33 \text{ BN} + 10.67 \text{ Sr}_2\text{N} + \text{SrB}_6\text{H}_4\text{C}_6\text{N}$                       | -60.4363            |
| SrNH <sub>4</sub> B <sub>6</sub> C <sub>6</sub> | $3 \text{ B}_{13}\text{C}_2 + 2 \text{ H}_2 + 67 \text{ SrN} \rightarrow 33 \text{ BN} + 33 \text{ Sr}_2\text{N} + \text{SrB}_6\text{H}_4\text{C}_6\text{N}$                               | -60.2443            |
| SrNH <sub>4</sub> B <sub>6</sub> C <sub>6</sub> | $3 \text{ B}_{13}\text{C}_2 + 31.67 \text{ SrN}_2 + 1.333 \text{ H}_3\text{N} \rightarrow 30.67 \text{ SrN} + 33 \text{ BN} + \text{SrB}_6\text{H}_4\text{C}_6\text{N}$                    | -59.3476            |
| SrNH <sub>4</sub> B <sub>6</sub> C <sub>6</sub> | $3 \text{ B}_{13}\text{C}_2 + 21.44 \text{ SrN}_2 + 1.333 \text{ H}_3\text{N} \rightarrow 33 \text{ BN} + 10.22 \text{ Sr}_2\text{N} + \text{SrB}_6\text{H}_4\text{C}_6\text{N}$           | -59.2597            |
| SrNH <sub>4</sub> B <sub>6</sub> C <sub>6</sub> | $3 \text{ B}_{13}\text{C}_2 + 1.333 \text{ H}_3\text{N} + 64.33 \text{ SrN} \rightarrow 33 \text{ BN} + 31.67 \text{ Sr}_2\text{N} + \text{SrB}_6\text{H}_4\text{C}_6\text{N}$             | -59.0753            |
| SrNH <sub>4</sub> B <sub>6</sub> C <sub>6</sub> | $3 \text{ B}_{13}\text{C}_2 + 35 \text{ SrN}_2 + 2 \text{ SrH}_2 \rightarrow 36 \text{ SrN} + 33 \text{ BN} + \text{SrB}_6\text{H}_4\text{C}_6\text{N}$                                    | -58.5545            |
| SrNH <sub>4</sub> B <sub>6</sub> C <sub>6</sub> | $3 \text{ B}_{13}\text{C}_2 + 23 \text{ SrN}_2 + 2 \text{ SrH}_2 \rightarrow 33 \text{ BN} + 12 \text{ Sr}_2\text{N} + \text{SrB}_6\text{H}_4\text{C}_6\text{N}$                           | -58.4513            |
| SrNH <sub>4</sub> B <sub>6</sub> C <sub>6</sub> | $3 \text{ B}_{13}\text{C}_2 + 69 \text{ SrN} + 2 \text{ SrH}_2 \rightarrow 33 \text{ BN} + 35 \text{ Sr}_2\text{N} + \text{SrB}_6\text{H}_4\text{C}_6\text{N}$                             | -58.2535            |
| SrNH <sub>4</sub> B <sub>6</sub> C <sub>6</sub> | $1.2 \text{ H}_8\text{C}_5 + 24.33 \text{ SrN} + 5.867 \text{ B}_5\text{H}_7 \rightarrow 23.33 \text{ BN} + 23.33 \text{ SrH}_2 + \text{SrB}_6\text{H}_4\text{C}_6\text{N}$                | -57.8760            |
| SrNH <sub>4</sub> B <sub>6</sub> C <sub>6</sub> | $3 \text{ B}_{13}\text{C}_2 + 18.64 \text{ SrN}_2 + 0.3636 \text{ B}_9\text{H}_{11} \rightarrow 36.27 \text{ BN} + 17.64 \text{ Sr} + \text{SrB}_6\text{H}_4\text{C}_6\text{N}$            | -56.0713            |
| SrNH <sub>4</sub> B <sub>6</sub> C <sub>6</sub> | $3 \text{ B}_{13}\text{C}_2 + 18.43 \text{ SrN}_2 + 0.5714 \text{ B}_5\text{H}_7 \rightarrow 35.86 \text{ BN} + 17.43 \text{ Sr} + \text{SrB}_6\text{H}_4\text{C}_6\text{N}$               | -55.3760            |
| SrNH <sub>4</sub> B <sub>6</sub> C <sub>6</sub> | $2.375 \text{ B}_{13}\text{C}_2 + 0.25 \text{ H}_8\text{C}_5 + 12.94 \text{ N}_2 + \text{SrH}_2 \rightarrow 24.88 \text{ BN} + \text{SrB}_6\text{H}_4\text{C}_6\text{N}$                   | -53.8173            |
| SrNH <sub>4</sub> B <sub>6</sub> C <sub>6</sub> | $2 \text{ B}_{13}\text{C}_2 + 0.3636 \text{ B}_9\text{H}_{11} + 12.14 \text{ N}_2 + \text{SrC}_2 \rightarrow 23.27 \text{ BN} + \text{SrB}_6\text{H}_4\text{C}_6\text{N}$                  | -51.5686            |
| SrNH <sub>4</sub> B <sub>6</sub> C <sub>6</sub> | $3 \text{ B}_{13}\text{C}_2 + 17 \text{ SrN}_2 + 2 \text{ H}_2 \rightarrow 33 \text{ BN} + 16 \text{ Sr} + \text{SrB}_6\text{H}_4\text{C}_6\text{N}$                                       | -50.7649            |
| SrNH <sub>4</sub> B <sub>6</sub> C <sub>6</sub> | $2 \text{ B}_{13}\text{C}_2 + 0.5714 \text{ B}_5\text{H}_7 + 11.93 \text{ N}_2 + \text{SrC}_2 \rightarrow 22.86 \text{ BN} + \text{SrB}_6\text{H}_4\text{C}_6\text{N}$                     | -50.5641            |
| SrNH <sub>4</sub> B <sub>6</sub> C <sub>6</sub> | $3 \text{ B}_{13}\text{C}_2 + 16.33 \text{ SrN}_2 + 1.333 \text{ H}_3\text{N} \rightarrow 33 \text{ BN} + 15.33 \text{ Sr} + \text{SrB}_6\text{H}_4\text{C}_6\text{N}$                     | -49.9912            |
| SrNH <sub>4</sub> B <sub>6</sub> C <sub>6</sub> | $3 \text{ B}_{13}\text{C}_2 + 17 \text{ SrN}_2 + 2 \text{ SrH}_2 \rightarrow 33 \text{ BN} + 18 \text{ Sr} + \text{SrB}_6\text{H}_4\text{C}_6\text{N}$                                     | -47.5709            |
| SrNH <sub>4</sub> B <sub>6</sub> C <sub>6</sub> | $1.75 \text{ B}_{13}\text{C}_2 + 0.5 \text{ H}_8\text{C}_5 + 11.88 \text{ N}_2 + \text{SrB}_6 \rightarrow 22.75 \text{ BN} + \text{SrB}_6\text{H}_4\text{C}_6\text{N}$                     | -47.0231            |
| SrNH <sub>4</sub> B <sub>6</sub> C <sub>6</sub> | $3 \text{ B}_{13}\text{C}_2 + 37.27 \text{ SrN} + 0.3636 \text{ B}_9\text{H}_{11} \rightarrow 36.27 \text{ BN} + 36.27 \text{ Sr} + \text{SrB}_6\text{H}_4\text{C}_6\text{N}$              | -44.6994            |
| SrNH <sub>4</sub> B <sub>6</sub> C <sub>6</sub> | $3 \text{ B}_{13}\text{C}_2 + 36.86 \text{ SrN} + 0.5714 \text{ B}_5\text{H}_7 \rightarrow 35.86 \text{ BN} + 35.86 \text{ Sr} + \text{SrB}_6\text{H}_4\text{C}_6\text{N}$                 | -44.1309            |
| SrNH <sub>4</sub> B <sub>6</sub> C <sub>6</sub> | $2 \text{ B}_{13}\text{C}_2 + 2 \text{ H}_2 + 10.5 \text{ N}_2 + \text{SrC}_2 \rightarrow 20 \text{ BN} + \text{SrB}_6\text{H}_4\text{C}_6\text{N}$                                        | -43.8277            |
| SrNH <sub>4</sub> B <sub>6</sub> C <sub>6</sub> | $2 \text{ B}_{13}\text{C}_2 + 1.333 \text{ H}_3\text{N} + 9.833 \text{ N}_2 + \text{SrC}_2 \rightarrow 20 \text{ BN} + \text{SrB}_6\text{H}_4\text{C}_6\text{N}$                           | -42.0623            |
| SrNH <sub>4</sub> B <sub>6</sub> C <sub>6</sub> | $3 \text{ B}_{13}\text{C}_2 + 2 \text{ H}_2 + 34 \text{ SrN} \rightarrow 33 \text{ BN} + 33 \text{ Sr} + \text{SrB}_6\text{H}_4\text{C}_6\text{N}$                                         | -40.3915            |
| SrNH <sub>4</sub> B <sub>6</sub> C <sub>6</sub> | $3 \text{ B}_{13}\text{C}_2 + 1.333 \text{ H}_3\text{N} + 32.67 \text{ SrN} \rightarrow 33 \text{ BN} + 31.67 \text{ Sr} + \text{SrB}_6\text{H}_4\text{C}_6\text{N}$                       | -40.0246            |
| SrNH <sub>4</sub> B <sub>6</sub> C <sub>6</sub> | $1.2 \text{ H}_8\text{C}_5 + 17.63 \text{ SrN} + 2.514 \text{ B}_9\text{H}_{11} \rightarrow 16.63 \text{ BN} + 16.63 \text{ SrH}_2 + \text{SrB}_6\text{H}_4\text{C}_6\text{N}$             | -38.5634            |
| SrNH <sub>4</sub> B <sub>6</sub> C <sub>6</sub> | $3 \text{ B}_{13}\text{C}_2 + 34 \text{ SrN} + 2 \text{ SrH}_2 \rightarrow 33 \text{ BN} + 35 \text{ Sr} + \text{SrB}_6\text{H}_4\text{C}_6\text{N}$                                       | -37.1975            |
| SrNH <sub>4</sub> B <sub>6</sub> C <sub>6</sub> | $3 \text{ B}_{13}\text{C}_2 + 40 \text{ H}_3\text{N} + \text{SrB}_6 \rightarrow 58 \text{ H}_2 + 39 \text{ BN} + \text{SrB}_6\text{H}_4\text{C}_6\text{N}$                                 | -35.3432            |
| SrNH <sub>4</sub> B <sub>6</sub> C <sub>6</sub> | $1.75 \text{ B}_{13}\text{C}_2 + 0.5 \text{ H}_8\text{C}_5 + 8.875 \text{ N}_2 + \text{Sr} \rightarrow 16.75 \text{ BN} + \text{SrB}_6\text{H}_4\text{C}_6\text{N}$                        | -34.7729            |
| SrNH <sub>4</sub> B <sub>6</sub> C <sub>6</sub> | $1.75 \text{ B}_{13}\text{C}_2 + 0.5 \text{ H}_8\text{C}_5 + 8.625 \text{ N}_2 + 0.5 \text{ Sr}_2\text{N} \rightarrow 16.75 \text{ BN} + \text{SrB}_6\text{H}_4\text{C}_6\text{N}$         | -33.9476            |
| SrNH <sub>4</sub> B <sub>6</sub> C <sub>6</sub> | $1.75 \text{ B}_{13}\text{C}_2 + 0.5 \text{ H}_8\text{C}_5 + \text{SrN} + 8.375 \text{ N}_2 \rightarrow 16.75 \text{ BN} + \text{SrB}_6\text{H}_4\text{C}_6\text{N}$                       | -33.7239            |
| SrNH <sub>4</sub> B <sub>6</sub> C <sub>6</sub> | $1.75 \text{ B}_{13}\text{C}_2 + \text{SrN}_2 + 0.5 \text{ H}_8\text{C}_5 + 7.875 \text{ N}_2 \rightarrow 16.75 \text{ BN} + \text{SrB}_6\text{H}_4\text{C}_6\text{N}$                     | -33.2852            |
| SrNH <sub>4</sub> B <sub>6</sub> C <sub>6</sub> | $3 \text{ B}_{13}\text{C}_2 + \text{SrN}_2 + 32 \text{ H}_3\text{N} \rightarrow 46 \text{ H}_2 + 33 \text{ BN} + \text{SrB}_6\text{H}_4\text{C}_6\text{N}$                                 | -32.1978            |
| SrNH <sub>4</sub> B <sub>6</sub> C <sub>6</sub> | $3 \text{ B}_{13}\text{C}_2 + 33 \text{ H}_3\text{N} + \text{SrN} \rightarrow 47.5 \text{ H}_2 + 33 \text{ BN} + \text{SrB}_6\text{H}_4\text{C}_6\text{N}$                                 | -31.3125            |
| SrNH <sub>4</sub> B <sub>6</sub> C <sub>6</sub> | $3 \text{ B}_{13}\text{C}_2 + 34 \text{ H}_3\text{N} + \text{Sr} \rightarrow 49 \text{ H}_2 + 33 \text{ BN} + \text{SrB}_6\text{H}_4\text{C}_6\text{N}$                                    | -31.0374            |
| SrNH <sub>4</sub> B <sub>6</sub> C <sub>6</sub> | $3 \text{ B}_{13}\text{C}_2 + 33.5 \text{ H}_3\text{N} + 0.5 \text{ Sr}_2\text{N} \rightarrow 48.25 \text{ H}_2 + 33 \text{ BN} + \text{SrB}_6\text{H}_4\text{C}_6\text{N}$                | -30.8741            |
| SrNH <sub>4</sub> B <sub>6</sub> C <sub>6</sub> | $3 \text{ B}_{13}\text{C}_2 + 34 \text{ H}_3\text{N} + \text{SrH}_2 \rightarrow 50 \text{ H}_2 + 33 \text{ BN} + \text{SrB}_6\text{H}_4\text{C}_6\text{N}$                                 | -29.4404            |
| SrNH <sub>4</sub> B <sub>6</sub> C <sub>6</sub> | $1.2 \text{ H}_8\text{C}_5 + 8.9 \text{ N}_2 + 3.8 \text{ SrB}_6 \rightarrow 16.8 \text{ BN} + 2.8 \text{ SrH}_2 + \text{SrB}_6\text{H}_4\text{C}_6\text{N}$                               | -27.9991            |
| SrNH <sub>4</sub> B <sub>6</sub> C <sub>6</sub> | $70 \text{ H}_3\text{N} + 1.2 \text{ B}_5\text{H}_7 + 70 \text{ SrC}_2 \rightarrow 26.8 \text{ H}_8\text{C}_5 + 69 \text{ SrN} + \text{SrB}_6\text{H}_4\text{C}_6\text{N}$                 | -26.6947            |
| SrNH <sub>4</sub> B <sub>6</sub> C <sub>6</sub> | $1.75 \text{ B}_{13}\text{C}_2 + 16.75 \text{ SrN}_2 + 0.5 \text{ H}_8\text{C}_5 \rightarrow 15.75 \text{ SrN} + 16.75 \text{ BN} + \text{SrB}_6\text{H}_4\text{C}_6\text{N}$              | -26.3748            |
| SrNH <sub>4</sub> B <sub>6</sub> C <sub>6</sub> | $1.75 \text{ B}_{13}\text{C}_2 + 11.5 \text{ SrN}_2 + 0.5 \text{ H}_8\text{C}_5 \rightarrow 16.75 \text{ BN} + 5.25 \text{ Sr}_2\text{N} + \text{SrB}_6\text{H}_4\text{C}_6\text{N}$       | -26.3297            |
| SrNH <sub>4</sub> B <sub>6</sub> C <sub>6</sub> | $1.75 \text{ B}_{13}\text{C}_2 + 0.5 \text{ H}_8\text{C}_5 + 34.5 \text{ SrN} \rightarrow 16.75 \text{ BN} + 16.75 \text{ Sr}_2\text{N} + \text{SrB}_6\text{H}_4\text{C}_6\text{N}$        | -26.2308            |
| SrNH <sub>4</sub> B <sub>6</sub> C <sub>6</sub> | $64.67 \text{ H}_3\text{N} + 0.6667 \text{ B}_9\text{H}_{11} + 64.67 \text{ SrC}_2 \rightarrow 24.67 \text{ H}_8\text{C}_5 + 63.67 \text{ SrN} + \text{SrB}_6\text{H}_4\text{C}_6\text{N}$ | -23.9497            |
| SrNH <sub>4</sub> B <sub>6</sub> C <sub>6</sub> | $3 \text{ B}_{13}\text{C}_2 + 0.3636 \text{ B}_9\text{H}_{11} + 37.27 \text{ Sr}_2\text{N} \rightarrow 36.27 \text{ BN} + 73.55 \text{ Sr} + \text{SrB}_6\text{H}_4\text{C}_6\text{N}$     | -22.2761            |
| SrNH <sub>4</sub> B <sub>6</sub> C <sub>6</sub> | $3 \text{ B}_{13}\text{C}_2 + 0.5714 \text{ B}_5\text{H}_7 + 36.86 \text{ Sr}_2\text{N} \rightarrow 35.86 \text{ BN} + 72.71 \text{ Sr} + \text{SrB}_6\text{H}_4\text{C}_6\text{N}$        | -21.9576            |
| SrNH <sub>4</sub> B <sub>6</sub> C <sub>6</sub> | $3 \text{ B}_{13}\text{C}_2 + 5.409 \text{ SrN}_2 + 0.3636 \text{ B}_9\text{H}_{11} \rightarrow 9.818 \text{ BN} + 4.409 \text{ SrB}_6 + \text{SrB}_6\text{H}_4\text{C}_6\text{N}$         | -21.7373            |
| SrNH <sub>4</sub> B <sub>6</sub> C <sub>6</sub> | $1.75 \text{ B}_{13}\text{C}_2 + 8.875 \text{ SrN}_2 + 0.5 \text{ H}_8\text{C}_5 \rightarrow 16.75 \text{ BN} + 7.875 \text{ Sr} + \text{SrB}_6\text{H}_4\text{C}_6\text{N}$               | -21.5695            |
| SrNH <sub>4</sub> B <sub>6</sub> C <sub>6</sub> | $3 \text{ B}_{13}\text{C}_2 + 5.357 \text{ SrN}_2 + 0.5714 \text{ B}_5\text{H}_7 \rightarrow 9.714 \text{ BN} + 4.357 \text{ SrB}_6 + \text{SrB}_6\text{H}_4\text{C}_6\text{N}$            | -21.4465            |
| SrNH <sub>4</sub> B <sub>6</sub> C <sub>6</sub> | $3 \text{ B}_{13}\text{C}_2 + 1.333 \text{ H}_3\text{N} + 32.67 \text{ Sr}_2\text{N} \rightarrow 33 \text{ BN} + 64.33 \text{ Sr} + \text{SrB}_6\text{H}_4\text{C}_6\text{N}$              | -20.3724            |
| SrNH <sub>4</sub> B <sub>6</sub> C <sub>6</sub> | $3 \text{ B}_{13}\text{C}_2 + 4.833 \text{ SrN}_2 + 1.333 \text{ H}_3\text{N} \rightarrow 10 \text{ BN} + 3.833 \text{ SrB}_6 + \text{SrB}_6\text{H}_4\text{C}_6\text{N}$                  | -20.1407            |
| SrNH <sub>4</sub> B <sub>6</sub> C <sub>6</sub> | $3 \text{ B}_{13}\text{C}_2 + 2 \text{ H}_2 + 34 \text{ Sr}_2\text{N} \rightarrow 33 \text{ BN} + 67 \text{ Sr} + \text{SrB}_6\text{H}_4\text{C}_6\text{N}$                                | -19.9371            |
| SrNH <sub>4</sub> B <sub>6</sub> C <sub>6</sub> | $3 \text{ B}_{13}\text{C}_2 + 11.23 \text{ SrN} + 3.154 \text{ B}_9\text{H}_{11} \rightarrow 10.23 \text{ H}_3\text{N} + 10.23 \text{ SrB}_6 + \text{SrB}_6\text{H}_4\text{C}_6\text{N}$   | -19.6297            |
| SrNH <sub>4</sub> B <sub>6</sub> C <sub>6</sub> | $3 \text{ B}_{13}\text{C}_2 + 5 \text{ SrN}_2 + 2 \text{ H}_2 \rightarrow 9 \text{ BN} + 4 \text{ SrB}_6 + \text{SrB}_6\text{H}_4\text{C}_6\text{N}$                                       | -19.6165            |
| SrNH <sub>4</sub> B <sub>6</sub> C <sub>6</sub> | $3 \text{ B}_{13}\text{C}_2 + 10.3 \text{ SrN} + 4.556 \text{ B}_5\text{H}_7 \rightarrow 9.296 \text{ H}_3\text{N} + 9.296 \text{ SrB}_6 + \text{SrB}_6\text{H}_4\text{C}_6\text{N}$       | -17.3873            |
| SrNH <sub>4</sub> B <sub>6</sub> C <sub>6</sub> | $3 \text{ B}_{13}\text{C}_2 + 34 \text{ Sr}_2\text{N} + 2 \text{ SrH}_2 \rightarrow 33 \text{ BN} + 69 \text{ Sr} + \text{SrB}_6\text{H}_4\text{C}_6\text{N}$                              | -16.7431            |
| SrNH <sub>4</sub> B <sub>6</sub> C <sub>6</sub> | $1.75 \text{ B}_{13}\text{C}_2 + 0.5 \text{ H}_8\text{C}_5 + 17.75 \text{ SrN} \rightarrow 16.75 \text{ BN} + 16.75 \text{ Sr} + \text{SrB}_6\text{H}_4\text{C}_6\text{N}$                 | -16.1540            |
| SrNH <sub>4</sub> B <sub>6</sub> C <sub>6</sub> | $2 \text{ B}_{13}\text{C}_2 + 21 \text{ H}_3\text{N} + \text{SrC}_2 \rightarrow 29.5 \text{ H}_2 + 20 \text{ BN} + \text{SrB}_6\text{H}_4\text{C}_6\text{N}$                               | -16.0222            |
| SrNH <sub>4</sub> B <sub>6</sub> C <sub>6</sub> | $4.25 \text{ SrN}_2 + 1.5 \text{ B}_9\text{H}_{11} + 3 \text{ SrC}_2 \rightarrow 7.5 \text{ BN} + 6.25 \text{ SrH}_2 + \text{SrB}_6\text{H}_4\text{C}_6\text{N}$                           | -14.9611            |
| SrNH <sub>4</sub> B <sub>6</sub> C <sub>6</sub> | $3 \text{ B}_{13}\text{C}_2 + 6.5 \text{ SrN}_2 + 20 \text{ H}_2 \rightarrow 12 \text{ H}_3\text{N} + 5.5 \text{ SrB}_6 + \text{SrB}_6\text{H}_4\text{C}_6\text{N}$                        | -14.8985            |
| SrNH <sub>4</sub> B <sub>6</sub> C <sub>6</sub> | $6 \text{ C} + 8.333 \text{ SrN} + 2.667 \text{ B}_5\text{H}_7 \rightarrow 7.333 \text{ BN} + 7.333 \text{ SrH}_2 + \text{SrB}_6\text{H}_4\text{C}_6\text{N}$                              | -14.3857            |

Continued on next page

Continued

| Compound                                        | Chemical reaction                                                                                                                                                                                 | Reaction energy(eV) |
|-------------------------------------------------|---------------------------------------------------------------------------------------------------------------------------------------------------------------------------------------------------|---------------------|
| SrNH <sub>4</sub> B <sub>6</sub> C <sub>6</sub> | $3 \text{ B}_{13}\text{C}_2 + 6.182 \text{ SrN} + 0.3636 \text{ B}_9\text{H}_{11} \rightarrow 5.182 \text{ BN} + 5.182 \text{ SrB}_6 + \text{SrB}_6\text{H}_4\text{C}_6\text{N}$                  | -13.8339            |
| SrNH <sub>4</sub> B <sub>6</sub> C <sub>6</sub> | $3 \text{ B}_{13}\text{C}_2 + 6.122 \text{ SrN} + 0.5714 \text{ B}_5\text{H}_7 \rightarrow 5.122 \text{ BN} + 5.122 \text{ SrB}_6 + \text{SrB}_6\text{H}_4\text{C}_6\text{N}$                     | -13.6190            |
| SrNH <sub>4</sub> B <sub>6</sub> C <sub>6</sub> | $3 \text{ B}_{13}\text{C}_2 + 1.333 \text{ H}_3\text{N} + 5.524 \text{ SrN} \rightarrow 5.857 \text{ BN} + 4.524 \text{ SrB}_6 + \text{SrB}_6\text{H}_4\text{C}_6\text{N}$                        | -13.0786            |
| SrNH <sub>4</sub> B <sub>6</sub> C <sub>6</sub> | $3 \text{ B}_{13}\text{C}_2 + 3.5 \text{ SrN}_2 + 2 \text{ SrH}_2 \rightarrow 6 \text{ BN} + 4.5 \text{ SrB}_6 + \text{SrB}_6\text{H}_4\text{C}_6\text{N}$                                        | -12.5289            |
| SrNH <sub>4</sub> B <sub>6</sub> C <sub>6</sub> | $3 \text{ B}_{13}\text{C}_2 + 2 \text{ H}_2 + 5.714 \text{ SrN} \rightarrow 4.714 \text{ BN} + 4.714 \text{ SrB}_6 + \text{SrB}_6\text{H}_4\text{C}_6\text{N}$                                    | -12.3108            |
| SrNH <sub>4</sub> B <sub>6</sub> C <sub>6</sub> | $3 \text{ B}_{13}\text{C}_2 + \text{SrN}_2 + 11.09 \text{ H}_3\text{N} \rightarrow 4.182 \text{ B}_5\text{H}_7 + 12.09 \text{ BN} + \text{SrB}_6\text{H}_4\text{C}_6\text{N}$                     | -10.5844            |
| SrNH <sub>4</sub> B <sub>6</sub> C <sub>6</sub> | $44 \text{ H}_3\text{N} + 43 \text{ SrC}_2 + \text{SrB}_6 \rightarrow 16 \text{ H}_8\text{C}_5 + 43 \text{ SrN} + \text{SrB}_6\text{H}_4\text{C}_6\text{N}$                                       | -10.3983            |
| SrNH <sub>4</sub> B <sub>6</sub> C <sub>6</sub> | $3 \text{ B}_{13}\text{C}_2 + 0.3636 \text{ B}_9\text{H}_{11} + 0.5 \text{ N}_2 + 7.045 \text{ Sr} \rightarrow 6.045 \text{ SrB}_6 + \text{SrB}_6\text{H}_4\text{C}_6\text{N}$                    | -9.7386             |
| SrNH <sub>4</sub> B <sub>6</sub> C <sub>6</sub> | $3 \text{ B}_{13}\text{C}_2 + 0.5714 \text{ B}_5\text{H}_7 + 0.5 \text{ N}_2 + 6.976 \text{ Sr} \rightarrow 5.976 \text{ SrB}_6 + \text{SrB}_6\text{H}_4\text{C}_6\text{N}$                       | -9.5827             |
| SrNH <sub>4</sub> B <sub>6</sub> C <sub>6</sub> | $3 \text{ B}_{13}\text{C}_2 + 1.229 \text{ B}_9\text{H}_{11} + 4.171 \text{ Sr}_2\text{N} \rightarrow 3.171 \text{ H}_3\text{N} + 7.343 \text{ SrB}_6 + \text{SrB}_6\text{H}_4\text{C}_6\text{N}$ | -9.5714             |
| SrNH <sub>4</sub> B <sub>6</sub> C <sub>6</sub> | $3 \text{ B}_{13}\text{C}_2 + \text{SrN}_2 + 10.21 \text{ H}_3\text{N} \rightarrow 2.421 \text{ B}_9\text{H}_{11} + 11.21 \text{ BN} + \text{SrB}_6\text{H}_4\text{C}_6\text{N}$                  | -9.5107             |
| SrNH <sub>4</sub> B <sub>6</sub> C <sub>6</sub> | $3 \text{ B}_{13}\text{C}_2 + 10.25 \text{ H}_2 + 6.5 \text{ SrN} \rightarrow 5.5 \text{ H}_3\text{N} + 5.5 \text{ SrB}_6 + \text{SrB}_6\text{H}_4\text{C}_6\text{N}$                             | -9.1439             |
| SrNH <sub>4</sub> B <sub>6</sub> C <sub>6</sub> | $1.2 \text{ H}_8\text{C}_5 + 2.123 \text{ B}_5\text{H}_7 + 5.615 \text{ Sr}_2\text{N} \rightarrow 4.615 \text{ BN} + 10.23 \text{ SrH}_2 + \text{SrB}_6\text{H}_4\text{C}_6\text{N}$              | -9.0751             |
| SrNH <sub>4</sub> B <sub>6</sub> C <sub>6</sub> | $3 \text{ B}_{13}\text{C}_2 + 0.3636 \text{ B}_9\text{H}_{11} + 3.329 \text{ Sr}_2\text{N} \rightarrow 2.329 \text{ BN} + 5.657 \text{ SrB}_6 + \text{SrB}_6\text{H}_4\text{C}_6\text{N}$         | -8.9989             |
| SrNH <sub>4</sub> B <sub>6</sub> C <sub>6</sub> | $3 \text{ B}_{13}\text{C}_2 + 0.5 \text{ SrN}_2 + 0.3636 \text{ B}_9\text{H}_{11} + 6.545 \text{ Sr} \rightarrow 6.045 \text{ SrB}_6 + \text{SrB}_6\text{H}_4\text{C}_6\text{N}$                  | -8.9948             |
| SrNH <sub>4</sub> B <sub>6</sub> C <sub>6</sub> | $3 \text{ B}_{13}\text{C}_2 + 1.87 \text{ B}_5\text{H}_7 + 4.029 \text{ Sr}_2\text{N} \rightarrow 3.029 \text{ H}_3\text{N} + 7.058 \text{ SrB}_6 + \text{SrB}_6\text{H}_4\text{C}_6\text{N}$     | -8.9946             |
| SrNH <sub>4</sub> B <sub>6</sub> C <sub>6</sub> | $3 \text{ B}_{13}\text{C}_2 + 11.41 \text{ H}_3\text{N} + \text{SrN} \rightarrow 4.318 \text{ B}_5\text{H}_7 + 11.41 \text{ BN} + \text{SrB}_6\text{H}_4\text{C}_6\text{N}$                       | -8.9943             |
| SrNH <sub>4</sub> B <sub>6</sub> C <sub>6</sub> | $3 \text{ B}_{13}\text{C}_2 + 0.5 \text{ SrN}_2 + 0.5714 \text{ B}_5\text{H}_7 + 6.476 \text{ Sr} \rightarrow 5.976 \text{ SrB}_6 + \text{SrB}_6\text{H}_4\text{C}_6\text{N}$                     | -8.8388             |
| SrNH <sub>4</sub> B <sub>6</sub> C <sub>6</sub> | $3 \text{ B}_{13}\text{C}_2 + 0.5714 \text{ B}_5\text{H}_7 + 3.297 \text{ Sr}_2\text{N} \rightarrow 2.297 \text{ BN} + 5.593 \text{ SrB}_6 + \text{SrB}_6\text{H}_4\text{C}_6\text{N}$            | -8.8305             |
| SrNH <sub>4</sub> B <sub>6</sub> C <sub>6</sub> | $\text{Sr}_2\text{N} + 42 \text{ B} + 3 \text{ SrC}_2 + 2 \text{ SrH}_2 \rightarrow 6 \text{ SrB}_6 + \text{SrB}_6\text{H}_4\text{C}_6\text{N}$                                                   | -8.8298             |
| SrNH <sub>4</sub> B <sub>6</sub> C <sub>6</sub> | $3 \text{ B}_{13}\text{C}_2 + 1.333 \text{ H}_3\text{N} + 2.974 \text{ Sr}_2\text{N} \rightarrow 3.308 \text{ BN} + 4.949 \text{ SrB}_6 + \text{SrB}_6\text{H}_4\text{C}_6\text{N}$               | -8.7582             |
| SrNH <sub>4</sub> B <sub>6</sub> C <sub>6</sub> | $3 \text{ B}_{13}\text{C}_2 + \text{SrN} + 0.3636 \text{ B}_9\text{H}_{11} + 6.045 \text{ Sr} \rightarrow 6.045 \text{ SrB}_6 + \text{SrB}_6\text{H}_4\text{C}_6\text{N}$                         | -8.6897             |
| SrNH <sub>4</sub> B <sub>6</sub> C <sub>6</sub> | $3 \text{ B}_{13}\text{C}_2 + 2 \text{ H}_2 + 0.5 \text{ N}_2 + 6.5 \text{ Sr} \rightarrow 5.5 \text{ SrB}_6 + \text{SrB}_6\text{H}_4\text{C}_6\text{N}$                                          | -8.6797             |
| SrNH <sub>4</sub> B <sub>6</sub> C <sub>6</sub> | $3 \text{ B}_{13}\text{C}_2 + \text{SrN} + 0.5714 \text{ B}_5\text{H}_7 + 5.976 \text{ Sr} \rightarrow 5.976 \text{ SrB}_6 + \text{SrB}_6\text{H}_4\text{C}_6\text{N}$                            | -8.5337             |
| SrNH <sub>4</sub> B <sub>6</sub> C <sub>6</sub> | $3 \text{ B}_{13}\text{C}_2 + 11.57 \text{ H}_3\text{N} + 0.5 \text{ Sr}_2\text{N} \rightarrow 4.386 \text{ B}_5\text{H}_7 + 11.07 \text{ BN} + \text{SrB}_6\text{H}_4\text{C}_6\text{N}$         | -8.2036             |
| SrNH <sub>4</sub> B <sub>6</sub> C <sub>6</sub> | $3.8 \text{ SrN}_2 + 1.2 \text{ H}_8\text{C}_5 + 12.6 \text{ B} \rightarrow 6.6 \text{ BN} + 2.8 \text{ SrH}_2 + \text{SrB}_6\text{H}_4\text{C}_6\text{N}$                                        | -8.1363             |
| SrNH <sub>4</sub> B <sub>6</sub> C <sub>6</sub> | $3 \text{ B}_{13}\text{C}_2 + 13.64 \text{ H}_3\text{N} + \text{SrB}_6 \rightarrow 5.273 \text{ B}_5\text{H}_7 + 12.64 \text{ BN} + \text{SrB}_6\text{H}_4\text{C}_6\text{N}$                     | -8.0915             |
| SrNH <sub>4</sub> B <sub>6</sub> C <sub>6</sub> | $3 \text{ B}_{13}\text{C}_2 + 0.3636 \text{ B}_9\text{H}_{11} + \text{Sr}_2\text{N} + 5.045 \text{ Sr} \rightarrow 6.045 \text{ SrB}_6 + \text{SrB}_6\text{H}_4\text{C}_6\text{N}$                | -8.0881             |
| SrNH <sub>4</sub> B <sub>6</sub> C <sub>6</sub> | $3 \text{ B}_{13}\text{C}_2 + 11.73 \text{ H}_3\text{N} + \text{Sr} \rightarrow 4.455 \text{ B}_5\text{H}_7 + 10.73 \text{ BN} + \text{SrB}_6\text{H}_4\text{C}_6\text{N}$                        | -8.0144             |
| SrNH <sub>4</sub> B <sub>6</sub> C <sub>6</sub> | $3 \text{ B}_{13}\text{C}_2 + 0.5 \text{ SrN}_2 + 2 \text{ H}_2 + 6 \text{ Sr} \rightarrow 5.5 \text{ SrB}_6 + \text{SrB}_6\text{H}_4\text{C}_6\text{N}$                                          | -7.9358             |
| SrNH <sub>4</sub> B <sub>6</sub> C <sub>6</sub> | $3 \text{ B}_{13}\text{C}_2 + 0.5714 \text{ B}_5\text{H}_7 + \text{Sr}_2\text{N} + 4.976 \text{ Sr} \rightarrow 5.976 \text{ SrB}_6 + \text{SrB}_6\text{H}_4\text{C}_6\text{N}$                   | -7.9321             |
| SrNH <sub>4</sub> B <sub>6</sub> C <sub>6</sub> | $3 \text{ B}_{13}\text{C}_2 + 10.5 \text{ H}_3\text{N} + \text{SrN} \rightarrow 2.5 \text{ B}_9\text{H}_{11} + 10.5 \text{ BN} + \text{SrB}_6\text{H}_4\text{C}_6\text{N}$                        | -7.8855             |
| SrNH <sub>4</sub> B <sub>6</sub> C <sub>6</sub> | $3 \text{ B}_{13}\text{C}_2 + 2 \text{ H}_2 + 3.077 \text{ Sr}_2\text{N} \rightarrow 2.077 \text{ BN} + 5.154 \text{ SrB}_6 + \text{SrB}_6\text{H}_4\text{C}_6\text{N}$                           | -7.8415             |
| SrNH <sub>4</sub> B <sub>6</sub> C <sub>6</sub> | $3 \text{ B}_{13}\text{C}_2 + 0.3636 \text{ B}_9\text{H}_{11} + \text{BN} + 7.212 \text{ Sr} \rightarrow 6.212 \text{ SrB}_6 + \text{SrB}_6\text{H}_4\text{C}_6\text{N}$                          | -7.6969             |
| SrNH <sub>4</sub> B <sub>6</sub> C <sub>6</sub> | $3 \text{ B}_{13}\text{C}_2 + 2 \text{ H}_2 + \text{SrN} + 5.5 \text{ Sr} \rightarrow 5.5 \text{ SrB}_6 + \text{SrB}_6\text{H}_4\text{C}_6\text{N}$                                               | -7.6307             |
| SrNH <sub>4</sub> B <sub>6</sub> C <sub>6</sub> | $3 \text{ B}_{13}\text{C}_2 + \text{H}_3\text{N} + 0.09091 \text{ B}_9\text{H}_{11} + 6.636 \text{ Sr} \rightarrow 5.636 \text{ SrB}_6 + \text{SrB}_6\text{H}_4\text{C}_6\text{N}$                | -7.6203             |
| SrNH <sub>4</sub> B <sub>6</sub> C <sub>6</sub> | $3 \text{ B}_{13}\text{C}_2 + 1.333 \text{ H}_3\text{N} + 6.444 \text{ Sr} \rightarrow 0.3333 \text{ BN} + 5.444 \text{ SrB}_6 + \text{SrB}_6\text{H}_4\text{C}_6\text{N}$                        | -7.5948             |
| SrNH <sub>4</sub> B <sub>6</sub> C <sub>6</sub> | $3 \text{ B}_{13}\text{C}_2 + \text{H}_3\text{N} + 0.1429 \text{ B}_5\text{H}_7 + 6.619 \text{ Sr} \rightarrow 5.619 \text{ SrB}_6 + \text{SrB}_6\text{H}_4\text{C}_6\text{N}$                    | -7.5813             |
| SrNH <sub>4</sub> B <sub>6</sub> C <sub>6</sub> | $3 \text{ B}_{13}\text{C}_2 + 0.5714 \text{ B}_5\text{H}_7 + \text{BN} + 7.143 \text{ Sr} \rightarrow 6.143 \text{ SrB}_6 + \text{SrB}_6\text{H}_4\text{C}_6\text{N}$                             | -7.5410             |
| SrNH <sub>4</sub> B <sub>6</sub> C <sub>6</sub> | $3 \text{ B}_{13}\text{C}_2 + 1.333 \text{ H}_3\text{N} + 7.167 \text{ Sr} \rightarrow 0.3333 \text{ Sr}_2\text{N} + 5.5 \text{ SrB}_6 + \text{SrB}_6\text{H}_4\text{C}_6\text{N}$                | -7.4644             |
| SrNH <sub>4</sub> B <sub>6</sub> C <sub>6</sub> | $3 \text{ B}_{13}\text{C}_2 + 4 \text{ SrN} + 2 \text{ SrH}_2 \rightarrow 3 \text{ BN} + 5 \text{ SrB}_6 + \text{SrB}_6\text{H}_4\text{C}_6\text{N}$                                              | -7.4150             |
| SrNH <sub>4</sub> B <sub>6</sub> C <sub>6</sub> | $3 \text{ B}_{13}\text{C}_2 + \text{H}_3\text{N} + 0.5 \text{ H}_2 + 6.5 \text{ Sr} \rightarrow 5.5 \text{ SrB}_6 + \text{SrB}_6\text{H}_4\text{C}_6\text{N}$                                     | -7.3556             |
| SrNH <sub>4</sub> B <sub>6</sub> C <sub>6</sub> | $3 \text{ B}_{13}\text{C}_2 + 1.333 \text{ H}_3\text{N} + 6.833 \text{ Sr} \rightarrow 0.3333 \text{ SrN} + 5.5 \text{ SrB}_6 + \text{SrB}_6\text{H}_4\text{C}_6\text{N}$                         | -7.2639             |
| SrNH <sub>4</sub> B <sub>6</sub> C <sub>6</sub> | $3 \text{ B}_{13}\text{C}_2 + 1.333 \text{ H}_3\text{N} + 6.667 \text{ Sr} \rightarrow 0.1667 \text{ SrN}_2 + 5.5 \text{ SrB}_6 + \text{SrB}_6\text{H}_4\text{C}_6\text{N}$                       | -7.1622             |
| SrNH <sub>4</sub> B <sub>6</sub> C <sub>6</sub> | $3 \text{ B}_{13}\text{C}_2 + 10.64 \text{ H}_3\text{N} + 0.5 \text{ Sr}_2\text{N} \rightarrow 2.539 \text{ B}_9\text{H}_{11} + 10.14 \text{ BN} + \text{SrB}_6\text{H}_4\text{C}_6\text{N}$      | -7.0773             |
| SrNH <sub>4</sub> B <sub>6</sub> C <sub>6</sub> | $3 \text{ B}_{13}\text{C}_2 + 2 \text{ H}_2 + \text{Sr}_2\text{N} + 4.5 \text{ Sr} \rightarrow 5.5 \text{ SrB}_6 + \text{SrB}_6\text{H}_4\text{C}_6\text{N}$                                      | -7.0291             |
| SrNH <sub>4</sub> B <sub>6</sub> C <sub>6</sub> | $3 \text{ B}_{13}\text{C}_2 + 1.333 \text{ H}_3\text{N} + 6.5 \text{ Sr} \rightarrow 0.1667 \text{ N}_2 + 5.5 \text{ SrB}_6 + \text{SrB}_6\text{H}_4\text{C}_6\text{N}$                           | -6.9142             |
| SrNH <sub>4</sub> B <sub>6</sub> C <sub>6</sub> | $3 \text{ B}_{13}\text{C}_2 + 10.79 \text{ H}_3\text{N} + \text{Sr} \rightarrow 2.579 \text{ B}_9\text{H}_{11} + 9.789 \text{ BN} + \text{SrB}_6\text{H}_4\text{C}_6\text{N}$                     | -6.8706             |
| SrNH <sub>4</sub> B <sub>6</sub> C <sub>6</sub> | $3 \text{ B}_{13}\text{C}_2 + 12.53 \text{ H}_3\text{N} + \text{SrB}_6 \rightarrow 3.053 \text{ B}_9\text{H}_{11} + 11.53 \text{ BN} + \text{SrB}_6\text{H}_4\text{C}_6\text{N}$                  | -6.7376             |
| SrNH <sub>4</sub> B <sub>6</sub> C <sub>6</sub> | $3.6 \text{ B}_5\text{H}_7 + 4.033 \text{ N}_2 + 3 \text{ SrC}_2 \rightarrow 7.067 \text{ H}_3\text{N} + 2 \text{ SrB}_6 + \text{SrB}_6\text{H}_4\text{C}_6\text{N}$                              | -6.6675             |
| SrNH <sub>4</sub> B <sub>6</sub> C <sub>6</sub> | $3 \text{ B}_{13}\text{C}_2 + 2 \text{ H}_2 + \text{BN} + 6.667 \text{ Sr} \rightarrow 5.667 \text{ SrB}_6 + \text{SrB}_6\text{H}_4\text{C}_6\text{N}$                                            | -6.6380             |
| SrNH <sub>4</sub> B <sub>6</sub> C <sub>6</sub> | $3 \text{ B}_{13}\text{C}_2 + \text{H}_3\text{N} + 6 \text{ Sr} + 0.5 \text{ SrH}_2 \rightarrow 5.5 \text{ SrB}_6 + \text{SrB}_6\text{H}_4\text{C}_6\text{N}$                                     | -6.5571             |
| SrNH <sub>4</sub> B <sub>6</sub> C <sub>6</sub> | $1.2 \text{ H}_8\text{C}_5 + 1.104 \text{ B}_9\text{H}_{11} + 4.936 \text{ Sr}_2\text{N} \rightarrow 3.936 \text{ BN} + 8.872 \text{ SrH}_2 + \text{SrB}_6\text{H}_4\text{C}_6\text{N}$           | -6.4994             |
| SrNH <sub>4</sub> B <sub>6</sub> C <sub>6</sub> | $3 \text{ B}_{13}\text{C}_2 + 5.375 \text{ H}_2 + 3.25 \text{ Sr}_2\text{N} \rightarrow 2.25 \text{ H}_3\text{N} + 5.5 \text{ SrB}_6 + \text{SrB}_6\text{H}_4\text{C}_6\text{N}$                  | -6.2945             |
| SrNH <sub>4</sub> B <sub>6</sub> C <sub>6</sub> | $\text{SrN} + 36 \text{ B} + 3 \text{ SrC}_2 + 2 \text{ SrH}_2 \rightarrow 5 \text{ SrB}_6 + \text{SrB}_6\text{H}_4\text{C}_6\text{N}$                                                            | -6.2811             |
| SrNH <sub>4</sub> B <sub>6</sub> C <sub>6</sub> | $1.75 \text{ B}_{13}\text{C}_2 + 2.969 \text{ SrN}_2 + 0.5 \text{ H}_8\text{C}_5 \rightarrow 4.938 \text{ BN} + 1.969 \text{ SrB}_6 + \text{SrB}_6\text{H}_4\text{C}_6\text{N}$                   | -6.2387             |
| SrNH <sub>4</sub> B <sub>6</sub> C <sub>6</sub> | $28 \text{ H}_3\text{N} + 6 \text{ B} + 28 \text{ SrC}_2 \rightarrow 10 \text{ H}_8\text{C}_5 + 27 \text{ SrN} + \text{SrB}_6\text{H}_4\text{C}_6\text{N}$                                        | -5.9766             |
| SrNH <sub>4</sub> B <sub>6</sub> C <sub>6</sub> | $3 \text{ B}_{13}\text{C}_2 + 11.27 \text{ H}_3\text{N} + \text{SrH}_2 \rightarrow 4.545 \text{ B}_5\text{H}_7 + 10.27 \text{ BN} + \text{SrB}_6\text{H}_4\text{C}_6\text{N}$                     | -5.9476             |
| SrNH <sub>4</sub> B <sub>6</sub> C <sub>6</sub> | $2 \text{ H}_2 + \text{Sr}_2\text{N} + 30 \text{ B} + 3 \text{ SrC}_2 \rightarrow 4 \text{ SrB}_6 + \text{SrB}_6\text{H}_4\text{C}_6\text{N}$                                                     | -5.7231             |
| SrNH <sub>4</sub> B <sub>6</sub> C <sub>6</sub> | $6 \text{ C} + 5.286 \text{ SrN} + 1.143 \text{ B}_9\text{H}_{11} \rightarrow 4.286 \text{ BN} + 4.286 \text{ SrH}_2 + \text{SrB}_6\text{H}_4\text{C}_6\text{N}$                                  | -5.6073             |

Continued on next page

Continued

| Compound                                        | Chemical reaction                                                                                                                                                                            | Reaction energy(eV) |
|-------------------------------------------------|----------------------------------------------------------------------------------------------------------------------------------------------------------------------------------------------|---------------------|
| SrNH <sub>4</sub> B <sub>6</sub> C <sub>6</sub> | $3 \text{ B}_{13}\text{C}_2 + 0.5 \text{ N}_2 + 4.5 \text{ Sr} + 2 \text{ SrH}_2 \rightarrow 5.5 \text{ SrB}_6 + \text{SrB}_6\text{H}_4\text{C}_6\text{N}$                                   | -5.4857             |
| SrNH <sub>4</sub> B <sub>6</sub> C <sub>6</sub> | $1.75 \text{ B}_{13}\text{C}_2 + 0.5 \text{ H}_8\text{C}_5 + 17.75 \text{ Sr}_2\text{N} \rightarrow 16.75 \text{ BN} + 34.5 \text{ Sr} + \text{SrB}_6\text{H}_4\text{C}_6\text{N}$           | -5.4756             |
| SrNH <sub>4</sub> B <sub>6</sub> C <sub>6</sub> | $2 \text{ B}_9\text{H}_{11} + 3.5 \text{ N}_2 + 3 \text{ SrC}_2 \rightarrow 6 \text{ H}_3\text{N} + 2 \text{ SrB}_6 + \text{SrB}_6\text{H}_4\text{C}_6\text{N}$                              | -5.3905             |
| SrNH <sub>4</sub> B <sub>6</sub> C <sub>6</sub> | $2.688 \text{ B}_{13}\text{C}_2 + 0.125 \text{ H}_8\text{C}_5 + \text{H}_3\text{N} + 5.823 \text{ Sr} \rightarrow 4.823 \text{ SrB}_6 + \text{SrB}_6\text{H}_4\text{C}_6\text{N}$            | -5.3293             |
| SrNH <sub>4</sub> B <sub>6</sub> C <sub>6</sub> | $0.5714 \text{ B}_5\text{H}_7 + \text{Sr}_2\text{N} + 27.14 \text{ B} + 3 \text{ SrC}_2 \rightarrow 4 \text{ SrB}_6 + \text{SrB}_6\text{H}_4\text{C}_6\text{N}$                              | -5.1259             |
| SrNH <sub>4</sub> B <sub>6</sub> C <sub>6</sub> | $0.3636 \text{ B}_9\text{H}_{11} + \text{Sr}_2\text{N} + 26.73 \text{ B} + 3 \text{ SrC}_2 \rightarrow 4 \text{ SrB}_6 + \text{SrB}_6\text{H}_4\text{C}_6\text{N}$                           | -5.0636             |
| SrNH <sub>4</sub> B <sub>6</sub> C <sub>6</sub> | $3 \text{ B}_{13}\text{C}_2 + 0.3636 \text{ B}_9\text{H}_{11} + 6.045 \text{ Sr}_2\text{N} \rightarrow 5.045 \text{ SrN} + 6.045 \text{ SrB}_6 + \text{SrB}_6\text{H}_4\text{C}_6\text{N}$   | -5.0527             |
| SrNH <sub>4</sub> B <sub>6</sub> C <sub>6</sub> | $3 \text{ B}_{13}\text{C}_2 + 0.3636 \text{ B}_9\text{H}_{11} + 4.364 \text{ Sr}_2\text{N} \rightarrow 1.682 \text{ SrN}_2 + 6.045 \text{ SrB}_6 + \text{SrB}_6\text{H}_4\text{C}_6\text{N}$ | -5.0382             |
| SrNH <sub>4</sub> B <sub>6</sub> C <sub>6</sub> | $1.2 \text{ H}_8\text{C}_5 + 2.867 \text{ Sr}_2\text{N} + 34.4 \text{ B} \rightarrow 1.867 \text{ H}_3\text{N} + 4.733 \text{ SrB}_6 + \text{SrB}_6\text{H}_4\text{C}_6\text{N}$             | -5.0291             |
| SrNH <sub>4</sub> B <sub>6</sub> C <sub>6</sub> | $0.5 \text{ SrN}_2 + 33 \text{ B} + 3 \text{ SrC}_2 + 2 \text{ SrH}_2 \rightarrow 4.5 \text{ SrB}_6 + \text{SrB}_6\text{H}_4\text{C}_6\text{N}$                                              | -5.0110             |
| SrNH <sub>4</sub> B <sub>6</sub> C <sub>6</sub> | $3 \text{ B}_{13}\text{C}_2 + 13.09 \text{ SrN} + 0.3636 \text{ B}_9\text{H}_{11} \rightarrow 6.045 \text{ SrN}_2 + 6.045 \text{ SrB}_6 + \text{SrB}_6\text{H}_4\text{C}_6\text{N}$          | -5.0007             |
| SrNH <sub>4</sub> B <sub>6</sub> C <sub>6</sub> | $3 \text{ B}_{13}\text{C}_2 + 0.5714 \text{ B}_5\text{H}_7 + 5.976 \text{ Sr}_2\text{N} \rightarrow 4.976 \text{ SrN} + 5.976 \text{ SrB}_6 + \text{SrB}_6\text{H}_4\text{C}_6\text{N}$      | -4.9384             |
| SrNH <sub>4</sub> B <sub>6</sub> C <sub>6</sub> | $3 \text{ B}_{13}\text{C}_2 + 0.5714 \text{ B}_5\text{H}_7 + 4.317 \text{ Sr}_2\text{N} \rightarrow 1.659 \text{ SrN}_2 + 5.976 \text{ SrB}_6 + \text{SrB}_6\text{H}_4\text{C}_6\text{N}$    | -4.9242             |
| SrNH <sub>4</sub> B <sub>6</sub> C <sub>6</sub> | $3 \text{ B}_{13}\text{C}_2 + 12.95 \text{ SrN} + 0.5714 \text{ B}_5\text{H}_7 \rightarrow 5.976 \text{ SrN}_2 + 5.976 \text{ SrB}_6 + \text{SrB}_6\text{H}_4\text{C}_6\text{N}$             | -4.8870             |
| SrNH <sub>4</sub> B <sub>6</sub> C <sub>6</sub> | $3 \text{ B}_{13}\text{C}_2 + 10.32 \text{ H}_3\text{N} + \text{SrH}_2 \rightarrow 2.632 \text{ B}_9\text{H}_{11} + 9.316 \text{ BN} + \text{SrB}_6\text{H}_4\text{C}_6\text{N}$             | -4.7805             |
| SrNH <sub>4</sub> B <sub>6</sub> C <sub>6</sub> | $3 \text{ B}_{13}\text{C}_2 + 0.5 \text{ SrN}_2 + 4 \text{ Sr} + 2 \text{ SrH}_2 \rightarrow 5.5 \text{ SrB}_6 + \text{SrB}_6\text{H}_4\text{C}_6\text{N}$                                   | -4.7418             |
| SrNH <sub>4</sub> B <sub>6</sub> C <sub>6</sub> | $3 \text{ B}_{13}\text{C}_2 + \text{SrN} + 3.5 \text{ Sr} + 2 \text{ SrH}_2 \rightarrow 5.5 \text{ SrB}_6 + \text{SrB}_6\text{H}_4\text{C}_6\text{N}$                                        | -4.4367             |
| SrNH <sub>4</sub> B <sub>6</sub> C <sub>6</sub> | $3 \text{ B}_{13}\text{C}_2 + 2 \text{ H}_2 + 5.5 \text{ Sr}_2\text{N} \rightarrow 4.5 \text{ SrN} + 5.5 \text{ SrB}_6 + \text{SrB}_6\text{H}_4\text{C}_6\text{N}$                           | -4.3219             |
| SrNH <sub>4</sub> B <sub>6</sub> C <sub>6</sub> | $3 \text{ B}_{13}\text{C}_2 + 2 \text{ H}_2 + 4 \text{ Sr}_2\text{N} \rightarrow 1.5 \text{ SrN}_2 + 5.5 \text{ SrB}_6 + \text{SrB}_6\text{H}_4\text{C}_6\text{N}$                           | -4.3090             |
| SrNH <sub>4</sub> B <sub>6</sub> C <sub>6</sub> | $3 \text{ B}_{13}\text{C}_2 + 2.154 \text{ Sr}_2\text{N} + 2 \text{ SrH}_2 \rightarrow 1.154 \text{ BN} + 5.308 \text{ SrB}_6 + \text{SrB}_6\text{H}_4\text{C}_6\text{N}$                    | -4.2865             |
| SrNH <sub>4</sub> B <sub>6</sub> C <sub>6</sub> | $3 \text{ B}_{13}\text{C}_2 + 2 \text{ H}_2 + 12 \text{ SrN} \rightarrow 5.5 \text{ SrN}_2 + 5.5 \text{ SrB}_6 + \text{SrB}_6\text{H}_4\text{C}_6\text{N}$                                   | -4.2746             |
| SrNH <sub>4</sub> B <sub>6</sub> C <sub>6</sub> | $0.5 \text{ N}_2 + 30 \text{ B} + 3 \text{ SrC}_2 + 2 \text{ SrH}_2 \rightarrow 4 \text{ SrB}_6 + \text{SrB}_6\text{H}_4\text{C}_6\text{N}$                                                  | -4.1797             |
| SrNH <sub>4</sub> B <sub>6</sub> C <sub>6</sub> | $3 \text{ B}_{13}\text{C}_2 + 0.3636 \text{ B}_9\text{H}_{11} + 3.523 \text{ Sr}_2\text{N} \rightarrow 1.261 \text{ N}_2 + 6.045 \text{ SrB}_6 + \text{SrB}_6\text{H}_4\text{C}_6\text{N}$   | -3.9242             |
| SrNH <sub>4</sub> B <sub>6</sub> C <sub>6</sub> | $3 \text{ B}_{13}\text{C}_2 + \text{Sr}_2\text{N} + 2.5 \text{ Sr} + 2 \text{ SrH}_2 \rightarrow 5.5 \text{ SrB}_6 + \text{SrB}_6\text{H}_4\text{C}_6\text{N}$                               | -3.8352             |
| SrNH <sub>4</sub> B <sub>6</sub> C <sub>6</sub> | $3 \text{ B}_{13}\text{C}_2 + 0.5714 \text{ B}_5\text{H}_7 + 3.488 \text{ Sr}_2\text{N} \rightarrow 1.244 \text{ N}_2 + 5.976 \text{ SrB}_6 + \text{SrB}_6\text{H}_4\text{C}_6\text{N}$      | -3.8254             |
| SrNH <sub>4</sub> B <sub>6</sub> C <sub>6</sub> | $3 \text{ B}_{13}\text{C}_2 + \text{BN} + 4.667 \text{ Sr} + 2 \text{ SrH}_2 \rightarrow 5.667 \text{ SrB}_6 + \text{SrB}_6\text{H}_4\text{C}_6\text{N}$                                     | -3.4440             |
| SrNH <sub>4</sub> B <sub>6</sub> C <sub>6</sub> | $1.2 \text{ H}_8\text{C}_5 + \text{H}_3\text{N} + 1.2 \text{ B}_5\text{H}_7 + 9.5 \text{ Sr} \rightarrow 8.5 \text{ SrH}_2 + \text{SrB}_6\text{H}_4\text{C}_6\text{N}$                       | -3.3736             |
| SrNH <sub>4</sub> B <sub>6</sub> C <sub>6</sub> | $3 \text{ B}_{13}\text{C}_2 + 2 \text{ H}_2 + 3.25 \text{ Sr}_2\text{N} \rightarrow 1.125 \text{ N}_2 + 5.5 \text{ SrB}_6 + \text{SrB}_6\text{H}_4\text{C}_6\text{N}$                        | -3.3154             |
| SrNH <sub>4</sub> B <sub>6</sub> C <sub>6</sub> | $2 \text{ H}_2 + \text{SrN} + 24 \text{ B} + 3 \text{ SrC}_2 \rightarrow 3 \text{ SrB}_6 + \text{SrB}_6\text{H}_4\text{C}_6\text{N}$                                                         | -3.1743             |
| SrNH <sub>4</sub> B <sub>6</sub> C <sub>6</sub> | $3 \text{ B}_{13}\text{C}_2 + 1.333 \text{ H}_3\text{N} + 6.833 \text{ Sr}_2\text{N} \rightarrow 7.167 \text{ SrN} + 5.5 \text{ SrB}_6 + \text{SrB}_6\text{H}_4\text{C}_6\text{N}$           | -3.1529             |
| SrNH <sub>4</sub> B <sub>6</sub> C <sub>6</sub> | $3 \text{ B}_{13}\text{C}_2 + 1.333 \text{ H}_3\text{N} + 4.444 \text{ Sr}_2\text{N} \rightarrow 2.389 \text{ SrN}_2 + 5.5 \text{ SrB}_6 + \text{SrB}_6\text{H}_4\text{C}_6\text{N}$         | -3.1324             |
| SrNH <sub>4</sub> B <sub>6</sub> C <sub>6</sub> | $3 \text{ B}_{13}\text{C}_2 + 1.333 \text{ H}_3\text{N} + 13.33 \text{ SrN} \rightarrow 6.833 \text{ SrN}_2 + 5.5 \text{ SrB}_6 + \text{SrB}_6\text{H}_4\text{C}_6\text{N}$                  | -3.0942             |
| SrNH <sub>4</sub> B <sub>6</sub> C <sub>6</sub> | $\text{SrN} + 0.5714 \text{ B}_5\text{H}_7 + 21.14 \text{ B} + 3 \text{ SrC}_2 \rightarrow 3 \text{ SrB}_6 + \text{SrB}_6\text{H}_4\text{C}_6\text{N}$                                       | -2.5771             |
| SrNH <sub>4</sub> B <sub>6</sub> C <sub>6</sub> | $1.2 \text{ H}_8\text{C}_5 + \text{H}_3\text{N} + 0.6667 \text{ B}_9\text{H}_{11} + 8.967 \text{ Sr} \rightarrow 7.967 \text{ SrH}_2 + \text{SrB}_6\text{H}_4\text{C}_6\text{N}$             | -2.5669             |
| SrNH <sub>4</sub> B <sub>6</sub> C <sub>6</sub> | $0.75 \text{ B}_{13}\text{C}_2 + 0.5 \text{ H}_8\text{C}_5 + 2.375 \text{ N}_2 + \text{SrC}_2 \rightarrow 3.75 \text{ BN} + \text{SrB}_6\text{H}_4\text{C}_6\text{N}$                        | -2.5448             |
| SrNH <sub>4</sub> B <sub>6</sub> C <sub>6</sub> | $\text{SrN} + 0.3636 \text{ B}_9\text{H}_{11} + 20.73 \text{ B} + 3 \text{ SrC}_2 \rightarrow 3 \text{ SrB}_6 + \text{SrB}_6\text{H}_4\text{C}_6\text{N}$                                    | -2.5149             |
| SrNH <sub>4</sub> B <sub>6</sub> C <sub>6</sub> | $3 \text{ B}_{13}\text{C}_2 + 7.045 \text{ SrN} + 0.3636 \text{ B}_9\text{H}_{11} \rightarrow 3.023 \text{ N}_2 + 6.045 \text{ SrB}_6 + \text{SrB}_6\text{H}_4\text{C}_6\text{N}$            | -2.3483             |
| SrNH <sub>4</sub> B <sub>6</sub> C <sub>6</sub> | $3 \text{ B}_{13}\text{C}_2 + 3.5 \text{ Sr}_2\text{N} + 2 \text{ SrH}_2 \rightarrow 2.5 \text{ SrN} + 5.5 \text{ SrB}_6 + \text{SrB}_6\text{H}_4\text{C}_6\text{N}$                         | -2.3311             |
| SrNH <sub>4</sub> B <sub>6</sub> C <sub>6</sub> | $3 \text{ B}_{13}\text{C}_2 + 2.667 \text{ Sr}_2\text{N} + 2 \text{ SrH}_2 \rightarrow 0.8333 \text{ SrN}_2 + 5.5 \text{ SrB}_6 + \text{SrB}_6\text{H}_4\text{C}_6\text{N}$                  | -2.3240             |
| SrNH <sub>4</sub> B <sub>6</sub> C <sub>6</sub> | $1.2 \text{ H}_8\text{C}_5 + 1.2 \text{ B}_5\text{H}_7 + 0.5 \text{ N}_2 + 8 \text{ Sr} \rightarrow 7 \text{ SrH}_2 + \text{SrB}_6\text{H}_4\text{C}_6\text{N}$                              | -2.3022             |
| SrNH <sub>4</sub> B <sub>6</sub> C <sub>6</sub> | $3 \text{ B}_{13}\text{C}_2 + 8 \text{ SrN} + 2 \text{ SrH}_2 \rightarrow 3.5 \text{ SrN}_2 + 5.5 \text{ SrB}_6 + \text{SrB}_6\text{H}_4\text{C}_6\text{N}$                                  | -2.3010             |
| SrNH <sub>4</sub> B <sub>6</sub> C <sub>6</sub> | $3 \text{ B}_{13}\text{C}_2 + 2 \text{ N}_2 + 6.5 \text{ SrH}_2 \rightarrow 3 \text{ H}_3\text{N} + 5.5 \text{ SrB}_6 + \text{SrB}_6\text{H}_4\text{C}_6\text{N}$                            | -2.2715             |
| SrNH <sub>4</sub> B <sub>6</sub> C <sub>6</sub> | $3 \text{ B}_{13}\text{C}_2 + 6.976 \text{ SrN} + 0.5714 \text{ B}_5\text{H}_7 \rightarrow 2.988 \text{ N}_2 + 5.976 \text{ SrB}_6 + \text{SrB}_6\text{H}_4\text{C}_6\text{N}$               | -2.2650             |
| SrNH <sub>4</sub> B <sub>6</sub> C <sub>6</sub> | $2 \text{ B}_{13}\text{C}_2 + 7.591 \text{ H}_3\text{N} + \text{SrC}_2 \rightarrow 2.682 \text{ B}_5\text{H}_7 + 6.591 \text{ BN} + \text{SrB}_6\text{H}_4\text{C}_6\text{N}$                | -2.1615             |
| SrNH <sub>4</sub> B <sub>6</sub> C <sub>6</sub> | $3 \text{ B}_{13}\text{C}_2 + 16.73 \text{ H}_3\text{N} + 32.47 \text{ Sr} \rightarrow 6.6 \text{ B}_5\text{H}_7 + 15.73 \text{ Sr}_2\text{N} + \text{SrB}_6\text{H}_4\text{C}_6\text{N}$    | -2.0624             |
| SrNH <sub>4</sub> B <sub>6</sub> C <sub>6</sub> | $0.4615 \text{ B}_{13}\text{C}_2 + 20.62 \text{ H}_3\text{N} + 20.62 \text{ SrC}_2 \rightarrow 7.231 \text{ H}_8\text{C}_5 + 19.62 \text{ SrN} + \text{SrB}_6\text{H}_4\text{C}_6\text{N}$   | -1.9557             |
| SrNH <sub>4</sub> B <sub>6</sub> C <sub>6</sub> | $0.5 \text{ SrN}_2 + 2 \text{ H}_2 + 21 \text{ B} + 3 \text{ SrC}_2 \rightarrow 2.5 \text{ SrB}_6 + \text{SrB}_6\text{H}_4\text{C}_6\text{N}$                                                | -1.9042             |
| SrNH <sub>4</sub> B <sub>6</sub> C <sub>6</sub> | $1.75 \text{ B}_{13}\text{C}_2 + 0.5 \text{ H}_8\text{C}_5 + 3.393 \text{ SrN} \rightarrow 2.393 \text{ BN} + 2.393 \text{ SrB}_6 + \text{SrB}_6\text{H}_4\text{C}_6\text{N}$                | -1.9009             |
| SrNH <sub>4</sub> B <sub>6</sub> C <sub>6</sub> | $3 \text{ B}_{13}\text{C}_2 + 1.714 \text{ Sr}_2\text{N} + 3.071 \text{ SrH}_2 \rightarrow 0.7143 \text{ H}_3\text{N} + 5.5 \text{ SrB}_6 + \text{SrB}_6\text{H}_4\text{C}_6\text{N}$        | -1.8909             |
| SrNH <sub>4</sub> B <sub>6</sub> C <sub>6</sub> | $3 \text{ B}_{13}\text{C}_2 + 2 \text{ H}_2 + 6.5 \text{ SrN} \rightarrow 2.75 \text{ N}_2 + 5.5 \text{ SrB}_6 + \text{SrB}_6\text{H}_4\text{C}_6\text{N}$                                   | -1.8615             |
| SrNH <sub>4</sub> B <sub>6</sub> C <sub>6</sub> | $3 \text{ B}_{13}\text{C}_2 + 2.25 \text{ Sr}_2\text{N} + 2 \text{ SrH}_2 \rightarrow 0.625 \text{ N}_2 + 5.5 \text{ SrB}_6 + \text{SrB}_6\text{H}_4\text{C}_6\text{N}$                      | -1.7720             |
| SrNH <sub>4</sub> B <sub>6</sub> C <sub>6</sub> | $\text{BN} + 29 \text{ B} + 3 \text{ SrC}_2 + 2 \text{ SrH}_2 \rightarrow 4 \text{ SrB}_6 + \text{SrB}_6\text{H}_4\text{C}_6\text{N}$                                                        | -1.6129             |
| SrNH <sub>4</sub> B <sub>6</sub> C <sub>6</sub> | $0.5 \text{ SrN}_2 + 1.2 \text{ H}_8\text{C}_5 + 1.2 \text{ B}_5\text{H}_7 + 7.5 \text{ Sr} \rightarrow 7 \text{ SrH}_2 + \text{SrB}_6\text{H}_4\text{C}_6\text{N}$                          | -1.5583             |
| SrNH <sub>4</sub> B <sub>6</sub> C <sub>6</sub> | $3 \text{ B}_{13}\text{C}_2 + 1.333 \text{ H}_3\text{N} + 3.25 \text{ Sr}_2\text{N} \rightarrow 1.792 \text{ N}_2 + 5.5 \text{ SrB}_6 + \text{SrB}_6\text{H}_4\text{C}_6\text{N}$            | -1.5499             |
| SrNH <sub>4</sub> B <sub>6</sub> C <sub>6</sub> | $1.2 \text{ H}_8\text{C}_5 + 0.6667 \text{ B}_9\text{H}_{11} + 0.5 \text{ N}_2 + 7.467 \text{ Sr} \rightarrow 6.467 \text{ SrH}_2 + \text{SrB}_6\text{H}_4\text{C}_6\text{N}$                | -1.4956             |
| SrNH <sub>4</sub> B <sub>6</sub> C <sub>6</sub> | $2 \text{ B}_{13}\text{C}_2 + 7.026 \text{ H}_3\text{N} + \text{SrC}_2 \rightarrow 1.553 \text{ B}_9\text{H}_{11} + 6.026 \text{ BN} + \text{SrB}_6\text{H}_4\text{C}_6\text{N}$             | -1.4729             |
| SrNH <sub>4</sub> B <sub>6</sub> C <sub>6</sub> | $3 \text{ B}_{13}\text{C}_2 + 2.4 \text{ SrN} + 4.1 \text{ SrH}_2 \rightarrow 1.4 \text{ H}_3\text{N} + 5.5 \text{ SrB}_6 + \text{SrB}_6\text{H}_4\text{C}_6\text{N}$                        | -1.4683             |
| SrNH <sub>4</sub> B <sub>6</sub> C <sub>6</sub> | $0.7778 \text{ B}_{13}\text{C}_2 + 2.556 \text{ SrN}_2 + 0.8889 \text{ H}_8\text{C}_5 \rightarrow 4.111 \text{ BN} + 1.556 \text{ SrH}_2 + \text{SrB}_6\text{H}_4\text{C}_6\text{N}$         | -1.3462             |
| SrNH <sub>4</sub> B <sub>6</sub> C <sub>6</sub> | $0.5 \text{ SrN}_2 + 0.5714 \text{ B}_5\text{H}_7 + 18.14 \text{ B} + 3 \text{ SrC}_2 \rightarrow 2.5 \text{ SrB}_6 + \text{SrB}_6\text{H}_4\text{C}_6\text{N}$                              | -1.3071             |
| SrNH <sub>4</sub> B <sub>6</sub> C <sub>6</sub> | $1.2 \text{ H}_8\text{C}_5 + \text{SrN} + 1.2 \text{ B}_5\text{H}_7 + 7 \text{ Sr} \rightarrow 7 \text{ SrH}_2 + \text{SrB}_6\text{H}_4\text{C}_6\text{N}$                                   | -1.2532             |

Continued on next page

Continued

| Compound                                        | Chemical reaction                                                                                                                                                                                          | Reaction energy(eV) |
|-------------------------------------------------|------------------------------------------------------------------------------------------------------------------------------------------------------------------------------------------------------------|---------------------|
| SrNH <sub>4</sub> B <sub>6</sub> C <sub>6</sub> | 0.5 SrN <sub>2</sub> + 0.3636 B <sub>9</sub> H <sub>11</sub> + 17.73 B + 3 SrC <sub>2</sub> → 2.5 SrB <sub>6</sub> + SrB <sub>6</sub> H <sub>4</sub> C <sub>6</sub> N                                      | -1.2448             |
| SrNH <sub>4</sub> B <sub>6</sub> C <sub>6</sub> | 3 B <sub>13</sub> C <sub>2</sub> + 14.78 H <sub>3</sub> N + 28.56 Sr → 3.667 B <sub>9</sub> H <sub>11</sub> + 13.78 Sr <sub>2</sub> N + SrB <sub>6</sub> H <sub>4</sub> C <sub>6</sub> N                   | -1.1760             |
| SrNH <sub>4</sub> B <sub>6</sub> C <sub>6</sub> | 3 B <sub>13</sub> C <sub>2</sub> + 1.5 SrN <sub>2</sub> + 5 SrH <sub>2</sub> → 2 H <sub>3</sub> N + 5.5 SrB <sub>6</sub> + SrB <sub>6</sub> H <sub>4</sub> C <sub>6</sub> N                                | -1.1113             |
| SrNH <sub>4</sub> B <sub>6</sub> C <sub>6</sub> | 2 H <sub>2</sub> + 0.5 N <sub>2</sub> + 18 B + 3 SrC <sub>2</sub> → 2 SrB <sub>6</sub> + SrB <sub>6</sub> H <sub>4</sub> C <sub>6</sub> N                                                                  | -1.0729             |
| SrNH <sub>4</sub> B <sub>6</sub> C <sub>6</sub> | 23.75 B <sub>9</sub> H <sub>11</sub> + Sr <sub>2</sub> N + 3 SrC <sub>2</sub> → 36.75 B <sub>5</sub> H <sub>7</sub> + 4 SrB <sub>6</sub> + SrB <sub>6</sub> H <sub>4</sub> C <sub>6</sub> N                | -1.0590             |
| SrNH <sub>4</sub> B <sub>6</sub> C <sub>6</sub> | 0.5 H <sub>8</sub> C <sub>5</sub> + Sr <sub>2</sub> N + 22.5 B + 1.75 SrC <sub>2</sub> → 2.75 SrB <sub>6</sub> + SrB <sub>6</sub> H <sub>4</sub> C <sub>6</sub> N                                          | -0.7873             |
| SrNH <sub>4</sub> B <sub>6</sub> C <sub>6</sub> | 3 B <sub>13</sub> C <sub>2</sub> + 4.5 SrN + 2 SrH <sub>2</sub> → 1.75 N <sub>2</sub> + 5.5 SrB <sub>6</sub> + SrB <sub>6</sub> H <sub>4</sub> C <sub>6</sub> N                                            | -0.7654             |
| SrNH <sub>4</sub> B <sub>6</sub> C <sub>6</sub> | 0.5 SrN <sub>2</sub> + 1.2 H <sub>8</sub> C <sub>5</sub> + 0.6667 B <sub>9</sub> H <sub>11</sub> + 6.967 Sr → 6.467 SrH <sub>2</sub> + SrB <sub>6</sub> H <sub>4</sub> C <sub>6</sub> N                    | -0.7517             |
| SrNH <sub>4</sub> B <sub>6</sub> C <sub>6</sub> | 1.2 H <sub>8</sub> C <sub>5</sub> + 1.2 B <sub>5</sub> H <sub>7</sub> + Sr <sub>2</sub> N + 6 Sr → 7 SrH <sub>2</sub> + SrB <sub>6</sub> H <sub>4</sub> C <sub>6</sub> N                                   | -0.6516             |
| SrNH <sub>4</sub> B <sub>6</sub> C <sub>6</sub> | 1.75 B <sub>13</sub> C <sub>2</sub> + 0.5 H <sub>8</sub> C <sub>5</sub> + 0.5 N <sub>2</sub> + 3.792 Sr → 2.792 SrB <sub>6</sub> + SrB <sub>6</sub> H <sub>4</sub> C <sub>6</sub> N                        | -0.5744             |
| SrNH <sub>4</sub> B <sub>6</sub> C <sub>6</sub> | H <sub>3</sub> N + 21 B + 3 SrC <sub>2</sub> + 0.5 SrH <sub>2</sub> → 2.5 SrB <sub>6</sub> + SrB <sub>6</sub> H <sub>4</sub> C <sub>6</sub> N                                                              | -0.5255             |
| SrNH <sub>4</sub> B <sub>6</sub> C <sub>6</sub> | 0.5714 B <sub>5</sub> H <sub>7</sub> + 0.5 N <sub>2</sub> + 15.14 B + 3 SrC <sub>2</sub> → 2 SrB <sub>6</sub> + SrB <sub>6</sub> H <sub>4</sub> C <sub>6</sub> N                                           | -0.4757             |
| SrNH <sub>4</sub> B <sub>6</sub> C <sub>6</sub> | 1.2 H <sub>8</sub> C <sub>5</sub> + SrN + 0.6667 B <sub>9</sub> H <sub>11</sub> + 6.467 Sr → 6.467 SrH <sub>2</sub> + SrB <sub>6</sub> H <sub>4</sub> C <sub>6</sub> N                                     | -0.4466             |
| SrNH <sub>4</sub> B <sub>6</sub> C <sub>6</sub> | 0.3636 B <sub>9</sub> H <sub>11</sub> + 0.5 N <sub>2</sub> + 14.73 B + 3 SrC <sub>2</sub> → 2 SrB <sub>6</sub> + SrB <sub>6</sub> H <sub>4</sub> C <sub>6</sub> N                                          | -0.4135             |
| SrNH <sub>4</sub> B <sub>6</sub> C <sub>6</sub> | 1.25 SrN <sub>2</sub> + 1.5 B <sub>5</sub> H <sub>7</sub> + 3 SrC <sub>2</sub> → 1.5 BN + 3.25 SrH <sub>2</sub> + SrB <sub>6</sub> H <sub>4</sub> C <sub>6</sub> N                                         | -0.3853             |
| SrNH <sub>4</sub> B <sub>6</sub> C <sub>6</sub> | 1.333 H <sub>3</sub> N + 18.33 B + 3 SrC <sub>2</sub> → 0.3333 BN + 2 SrB <sub>6</sub> + SrB <sub>6</sub> H <sub>4</sub> C <sub>6</sub> N                                                                  | -0.1631             |
| SrNH <sub>4</sub> B <sub>6</sub> C <sub>6</sub> | 3 B <sub>13</sub> C <sub>2</sub> + 1.333 H <sub>3</sub> N + 6.5 SrN → 3.417 N <sub>2</sub> + 5.5 SrB <sub>6</sub> + SrB <sub>6</sub> H <sub>4</sub> C <sub>6</sub> N                                       | -0.0961             |
| SrNH <sub>4</sub> B <sub>6</sub> C <sub>6</sub> | 1.2 H <sub>8</sub> C <sub>5</sub> + 3.8 SrN + 8.8 B → 2.8 BN + 2.8 SrH <sub>2</sub> + SrB <sub>6</sub> H <sub>4</sub> C <sub>6</sub> N                                                                     | -0.0498             |
| ThNH <sub>4</sub> B <sub>6</sub> C <sub>6</sub> | 1.2 B <sub>5</sub> H <sub>7</sub> + 70 ThC <sub>2</sub> + 70 H <sub>3</sub> N → 26.8 H <sub>8</sub> C <sub>5</sub> + 69 ThN + ThB <sub>6</sub> H <sub>4</sub> C <sub>6</sub> N                             | -117.0136           |
| ThNH <sub>4</sub> B <sub>6</sub> C <sub>6</sub> | 2 ThH <sub>2</sub> + 4 B <sub>13</sub> C <sub>2</sub> + 23.5 N <sub>2</sub> → 46 BN + ThC <sub>2</sub> + ThB <sub>6</sub> H <sub>4</sub> C <sub>6</sub> N                                                  | -109.2371           |
| ThNH <sub>4</sub> B <sub>6</sub> C <sub>6</sub> | 64.67 ThC <sub>2</sub> + 0.6667 B <sub>9</sub> H <sub>11</sub> + 64.67 H <sub>3</sub> N → 24.67 H <sub>8</sub> C <sub>5</sub> + 63.67 ThN + ThB <sub>6</sub> H <sub>4</sub> C <sub>6</sub> N               | -107.4563           |
| ThNH <sub>4</sub> B <sub>6</sub> C <sub>6</sub> | 3 B <sub>13</sub> C <sub>2</sub> + 50 Th + 34 H <sub>3</sub> N → 49 ThH <sub>2</sub> + 33 BN + ThB <sub>6</sub> H <sub>4</sub> C <sub>6</sub> N                                                            | -104.4706           |
| ThNH <sub>4</sub> B <sub>6</sub> C <sub>6</sub> | 2 ThH <sub>2</sub> + 3.75 B <sub>13</sub> C <sub>2</sub> + 21.88 N <sub>2</sub> → 42.75 BN + 0.5 Th <sub>2</sub> C <sub>3</sub> + ThB <sub>6</sub> H <sub>4</sub> C <sub>6</sub> N                         | -101.0736           |
| ThNH <sub>4</sub> B <sub>6</sub> C <sub>6</sub> | 0.3636 B <sub>9</sub> H <sub>11</sub> + 3 B <sub>13</sub> C <sub>2</sub> + 21.64 N <sub>2</sub> + ThB <sub>6</sub> → 42.27 BN + ThB <sub>6</sub> H <sub>4</sub> C <sub>6</sub> N                           | -98.8171            |
| ThNH <sub>4</sub> B <sub>6</sub> C <sub>6</sub> | 0.5714 B <sub>5</sub> H <sub>7</sub> + 3 B <sub>13</sub> C <sub>2</sub> + 21.43 N <sub>2</sub> + ThB <sub>6</sub> → 41.86 BN + ThB <sub>6</sub> H <sub>4</sub> C <sub>6</sub> N                            | -97.8127            |
| ThNH <sub>4</sub> B <sub>6</sub> C <sub>6</sub> | ThB <sub>4</sub> + 0.3636 B <sub>9</sub> H <sub>11</sub> + 3 B <sub>13</sub> C <sub>2</sub> + 20.64 N <sub>2</sub> → 40.27 BN + ThB <sub>6</sub> H <sub>4</sub> C <sub>6</sub> N                           | -93.9722            |
| ThNH <sub>4</sub> B <sub>6</sub> C <sub>6</sub> | ThB <sub>4</sub> + 0.5714 B <sub>5</sub> H <sub>7</sub> + 3 B <sub>13</sub> C <sub>2</sub> + 20.43 N <sub>2</sub> → 39.86 BN + ThB <sub>6</sub> H <sub>4</sub> C <sub>6</sub> N                            | -92.9678            |
| ThNH <sub>4</sub> B <sub>6</sub> C <sub>6</sub> | 2 ThH <sub>2</sub> + 3.5 B <sub>13</sub> C <sub>2</sub> + 20.25 N <sub>2</sub> → ThC + 39.5 BN + ThB <sub>6</sub> H <sub>4</sub> C <sub>6</sub> N                                                          | -92.9028            |
| ThNH <sub>4</sub> B <sub>6</sub> C <sub>6</sub> | 3 B <sub>13</sub> C <sub>2</sub> + 27.13 Th + 34 H <sub>3</sub> N → 6.533 Th <sub>4</sub> H <sub>15</sub> + 33 BN + ThB <sub>6</sub> H <sub>4</sub> C <sub>6</sub> N                                       | -91.3079            |
| ThNH <sub>4</sub> B <sub>6</sub> C <sub>6</sub> | 2 H <sub>2</sub> + 3 B <sub>13</sub> C <sub>2</sub> + 20 N <sub>2</sub> + ThB <sub>6</sub> → 39 BN + ThB <sub>6</sub> H <sub>4</sub> C <sub>6</sub> N                                                      | -91.0763            |
| ThNH <sub>4</sub> B <sub>6</sub> C <sub>6</sub> | 3 B <sub>13</sub> C <sub>2</sub> + 1.333 H <sub>3</sub> N + 19.33 N <sub>2</sub> + ThB <sub>6</sub> → 39 BN + ThB <sub>6</sub> H <sub>4</sub> C <sub>6</sub> N                                             | -89.3108            |
| ThNH <sub>4</sub> B <sub>6</sub> C <sub>6</sub> | 0.3636 B <sub>9</sub> H <sub>11</sub> + 3 B <sub>13</sub> C <sub>2</sub> + Th + 18.64 N <sub>2</sub> → 36.27 BN + ThB <sub>6</sub> H <sub>4</sub> C <sub>6</sub> N                                         | -86.8031            |
| ThNH <sub>4</sub> B <sub>6</sub> C <sub>6</sub> | ThB <sub>4</sub> + 2 H <sub>2</sub> + 3 B <sub>13</sub> C <sub>2</sub> + 19 N <sub>2</sub> → 37 BN + ThB <sub>6</sub> H <sub>4</sub> C <sub>6</sub> N                                                      | -86.2314            |
| ThNH <sub>4</sub> B <sub>6</sub> C <sub>6</sub> | 0.5714 B <sub>5</sub> H <sub>7</sub> + 3 B <sub>13</sub> C <sub>2</sub> + Th + 18.43 N <sub>2</sub> → 35.86 BN + ThB <sub>6</sub> H <sub>4</sub> C <sub>6</sub> N                                          | -85.7987            |
| ThNH <sub>4</sub> B <sub>6</sub> C <sub>6</sub> | ThB <sub>4</sub> + 3 B <sub>13</sub> C <sub>2</sub> + 1.333 H <sub>3</sub> N + 18.33 N <sub>2</sub> → 37 BN + ThB <sub>6</sub> H <sub>4</sub> C <sub>6</sub> N                                             | -84.4659            |
| ThNH <sub>4</sub> B <sub>6</sub> C <sub>6</sub> | 0.3636 B <sub>9</sub> H <sub>11</sub> + 3 B <sub>13</sub> C <sub>2</sub> + 18.14 N <sub>2</sub> + ThN → 36.27 BN + ThB <sub>6</sub> H <sub>4</sub> C <sub>6</sub> N                                        | -83.6556            |
| ThNH <sub>4</sub> B <sub>6</sub> C <sub>6</sub> | 0.3333 Th <sub>3</sub> N <sub>4</sub> + 0.3636 B <sub>9</sub> H <sub>11</sub> + 3 B <sub>13</sub> C <sub>2</sub> + 17.97 N <sub>2</sub> → 36.27 BN + ThB <sub>6</sub> H <sub>4</sub> C <sub>6</sub> N      | -83.0336            |
| ThNH <sub>4</sub> B <sub>6</sub> C <sub>6</sub> | 0.5714 B <sub>5</sub> H <sub>7</sub> + 3 B <sub>13</sub> C <sub>2</sub> + 17.93 N <sub>2</sub> + ThN → 35.86 BN + ThB <sub>6</sub> H <sub>4</sub> C <sub>6</sub> N                                         | -82.6512            |
| ThNH <sub>4</sub> B <sub>6</sub> C <sub>6</sub> | 0.5714 B <sub>5</sub> H <sub>7</sub> + 0.3333 Th <sub>3</sub> N <sub>4</sub> + 3 B <sub>13</sub> C <sub>2</sub> + 17.76 N <sub>2</sub> → 35.86 BN + ThB <sub>6</sub> H <sub>4</sub> C <sub>6</sub> N       | -82.0292            |
| ThNH <sub>4</sub> B <sub>6</sub> C <sub>6</sub> | ThH <sub>2</sub> + 0.1818 B <sub>9</sub> H <sub>11</sub> + 3 B <sub>13</sub> C <sub>2</sub> + 17.82 N <sub>2</sub> → 34.64 BN + ThB <sub>6</sub> H <sub>4</sub> C <sub>6</sub> N                           | -81.4954            |
| ThNH <sub>4</sub> B <sub>6</sub> C <sub>6</sub> | 1.5 ThB <sub>4</sub> + 50.5 ThC <sub>2</sub> + 52 H <sub>3</sub> N → 19 H <sub>8</sub> C <sub>5</sub> + 51 ThN + ThB <sub>6</sub> H <sub>4</sub> C <sub>6</sub> N                                          | -81.2472            |
| ThNH <sub>4</sub> B <sub>6</sub> C <sub>6</sub> | ThH <sub>2</sub> + 0.2857 B <sub>5</sub> H <sub>7</sub> + 3 B <sub>13</sub> C <sub>2</sub> + 17.71 N <sub>2</sub> → 34.43 BN + ThB <sub>6</sub> H <sub>4</sub> C <sub>6</sub> N                            | -80.9932            |
| ThNH <sub>4</sub> B <sub>6</sub> C <sub>6</sub> | 2 ThH <sub>2</sub> + 3 B <sub>13</sub> C <sub>2</sub> + 17.67 N <sub>2</sub> → 0.3333 Th <sub>3</sub> N <sub>4</sub> + 33 BN + ThB <sub>6</sub> H <sub>4</sub> C <sub>6</sub> N                            | -79.9572            |
| ThNH <sub>4</sub> B <sub>6</sub> C <sub>6</sub> | 2 ThH <sub>2</sub> + 3 B <sub>13</sub> C <sub>2</sub> + 17.5 N <sub>2</sub> → 33 BN + ThN + ThB <sub>6</sub> H <sub>4</sub> C <sub>6</sub> N                                                               | -79.3353            |
| ThNH <sub>4</sub> B <sub>6</sub> C <sub>6</sub> | 30.2 B <sub>5</sub> H <sub>7</sub> + 36.5 Th <sub>3</sub> N <sub>4</sub> + 1.2 H <sub>8</sub> C <sub>5</sub> → 108.5 ThH <sub>2</sub> + 145 BN + ThB <sub>6</sub> H <sub>4</sub> C <sub>6</sub> N          | -79.1851            |
| ThNH <sub>4</sub> B <sub>6</sub> C <sub>6</sub> | 2 H <sub>2</sub> + 3 B <sub>13</sub> C <sub>2</sub> + Th + 17 N <sub>2</sub> → 33 BN + ThB <sub>6</sub> H <sub>4</sub> C <sub>6</sub> N                                                                    | -79.0623            |
| ThNH <sub>4</sub> B <sub>6</sub> C <sub>6</sub> | 0.2667 Th <sub>4</sub> H <sub>15</sub> + 3.067 B <sub>13</sub> C <sub>2</sub> + 17.43 N <sub>2</sub> → 33.87 BN + 0.06667 ThC <sub>2</sub> + ThB <sub>6</sub> H <sub>4</sub> C <sub>6</sub> N              | -78.9282            |
| ThNH <sub>4</sub> B <sub>6</sub> C <sub>6</sub> | 0.2667 Th <sub>4</sub> H <sub>15</sub> + 3.05 B <sub>13</sub> C <sub>2</sub> + 17.32 N <sub>2</sub> → 33.65 BN + 0.03333 Th <sub>2</sub> C <sub>3</sub> + ThB <sub>6</sub> H <sub>4</sub> C <sub>6</sub> N | -78.3840            |
| ThNH <sub>4</sub> B <sub>6</sub> C <sub>6</sub> | 0.2667 Th <sub>4</sub> H <sub>15</sub> + 3.033 B <sub>13</sub> C <sub>2</sub> + 17.22 N <sub>2</sub> → 0.06667 ThC + 33.43 BN + ThB <sub>6</sub> H <sub>4</sub> C <sub>6</sub> N                           | -77.8393            |
| ThNH <sub>4</sub> B <sub>6</sub> C <sub>6</sub> | ThH <sub>2</sub> + H <sub>2</sub> + 3 B <sub>13</sub> C <sub>2</sub> + 17 N <sub>2</sub> → 33 BN + ThB <sub>6</sub> H <sub>4</sub> C <sub>6</sub> N                                                        | -77.6250            |
| ThNH <sub>4</sub> B <sub>6</sub> C <sub>6</sub> | 0.25 Th <sub>4</sub> H <sub>15</sub> + 0.02273 B <sub>9</sub> H <sub>11</sub> + 3 B <sub>13</sub> C <sub>2</sub> + 17.1 N <sub>2</sub> → 33.2 BN + ThB <sub>6</sub> H <sub>4</sub> C <sub>6</sub> N        | -77.3548            |
| ThNH <sub>4</sub> B <sub>6</sub> C <sub>6</sub> | 3 B <sub>13</sub> C <sub>2</sub> + Th + 1.333 H <sub>3</sub> N + 16.33 N <sub>2</sub> → 33 BN + ThB <sub>6</sub> H <sub>4</sub> C <sub>6</sub> N                                                           | -77.2968            |
| ThNH <sub>4</sub> B <sub>6</sub> C <sub>6</sub> | 0.03571 B <sub>5</sub> H <sub>7</sub> + 0.25 Th <sub>4</sub> H <sub>15</sub> + 3 B <sub>13</sub> C <sub>2</sub> + 17.09 N <sub>2</sub> → 33.18 BN + ThB <sub>6</sub> H <sub>4</sub> C <sub>6</sub> N       | -77.2921            |
| ThNH <sub>4</sub> B <sub>6</sub> C <sub>6</sub> | 0.2667 Th <sub>4</sub> H <sub>15</sub> + 3 B <sub>13</sub> C <sub>2</sub> + 17.04 N <sub>2</sub> → 0.02222 Th <sub>3</sub> N <sub>4</sub> + 33 BN + ThB <sub>6</sub> H <sub>4</sub> C <sub>6</sub> N       | -76.9763            |
| ThNH <sub>4</sub> B <sub>6</sub> C <sub>6</sub> | 0.2667 Th <sub>4</sub> H <sub>15</sub> + 3 B <sub>13</sub> C <sub>2</sub> + 17.03 N <sub>2</sub> → 33 BN + 0.06667 ThN + ThB <sub>6</sub> H <sub>4</sub> C <sub>6</sub> N                                  | -76.9348            |
| ThNH <sub>4</sub> B <sub>6</sub> C <sub>6</sub> | 0.125 H <sub>2</sub> + 0.25 Th <sub>4</sub> H <sub>15</sub> + 3 B <sub>13</sub> C <sub>2</sub> + 17 N <sub>2</sub> → 33 BN + ThB <sub>6</sub> H <sub>4</sub> C <sub>6</sub> N                              | -76.8710            |
| ThNH <sub>4</sub> B <sub>6</sub> C <sub>6</sub> | 0.2857 Th <sub>4</sub> H <sub>15</sub> + 3 B <sub>13</sub> C <sub>2</sub> + 17 N <sub>2</sub> → 0.1429 ThH <sub>2</sub> + 33 BN + ThB <sub>6</sub> H <sub>4</sub> C <sub>6</sub> N                         | -76.7633            |
| ThNH <sub>4</sub> B <sub>6</sub> C <sub>6</sub> | 0.25 Th <sub>4</sub> H <sub>15</sub> + 3 B <sub>13</sub> C <sub>2</sub> + 0.08333 H <sub>3</sub> N + 16.96 N <sub>2</sub> → 33 BN + ThB <sub>6</sub> H <sub>4</sub> C <sub>6</sub> N                       | -76.7607            |
| ThNH <sub>4</sub> B <sub>6</sub> C <sub>6</sub> | ThH <sub>2</sub> + 3 B <sub>13</sub> C <sub>2</sub> + 0.6667 H <sub>3</sub> N + 16.67 N <sub>2</sub> → 33 BN + ThB <sub>6</sub> H <sub>4</sub> C <sub>6</sub> N                                            | -76.7423            |
| ThNH <sub>4</sub> B <sub>6</sub> C <sub>6</sub> | 0.2667 Th <sub>4</sub> H <sub>15</sub> + 3 B <sub>13</sub> C <sub>2</sub> + 17 N <sub>2</sub> → 33 BN + 0.06667 Th + ThB <sub>6</sub> H <sub>4</sub> C <sub>6</sub> N                                      | -76.7250            |

Continued on next page

Continued

| Compound                                        | Chemical reaction                                                                                                                                                                                                 | Reaction energy(eV) |
|-------------------------------------------------|-------------------------------------------------------------------------------------------------------------------------------------------------------------------------------------------------------------------|---------------------|
| ThNH <sub>4</sub> B <sub>6</sub> C <sub>6</sub> | 0.2667 Th <sub>4</sub> H <sub>15</sub> + 3 B <sub>13</sub> C <sub>2</sub> + 16.87 N <sub>2</sub> → 0.06667 ThB <sub>4</sub> + 32.73 BN + ThB <sub>6</sub> H <sub>4</sub> C <sub>6</sub> N                         | -76.2470            |
| ThNH <sub>4</sub> B <sub>6</sub> C <sub>6</sub> | 2 ThH <sub>2</sub> + 3 B <sub>13</sub> C <sub>2</sub> + 17 N <sub>2</sub> → 33 BN + Th + ThB <sub>6</sub> H <sub>4</sub> C <sub>6</sub> N                                                                         | -76.1877            |
| ThNH <sub>4</sub> B <sub>6</sub> C <sub>6</sub> | 0.2667 Th <sub>4</sub> H <sub>15</sub> + 3 B <sub>13</sub> C <sub>2</sub> + 16.8 N <sub>2</sub> → 32.6 BN + 0.06667 ThB <sub>6</sub> + ThB <sub>6</sub> H <sub>4</sub> C <sub>6</sub> N                           | -75.9240            |
| ThNH <sub>4</sub> B <sub>6</sub> C <sub>6</sub> | 2 H <sub>2</sub> + 3 B <sub>13</sub> C <sub>2</sub> + 16.5 N <sub>2</sub> + ThN → 33 BN + ThB <sub>6</sub> H <sub>4</sub> C <sub>6</sub> N                                                                        | -75.9147            |
| ThNH <sub>4</sub> B <sub>6</sub> C <sub>6</sub> | 58.14 ThH <sub>2</sub> + 3 B <sub>13</sub> C <sub>2</sub> + 34 H <sub>3</sub> N → 14.29 Th <sub>4</sub> H <sub>15</sub> + 33 BN + ThB <sub>6</sub> H <sub>4</sub> C <sub>6</sub> N                                | -75.6892            |
| ThNH <sub>4</sub> B <sub>6</sub> C <sub>6</sub> | 0.3333 Th <sub>3</sub> N <sub>4</sub> + 2 H <sub>2</sub> + 3 B <sub>13</sub> C <sub>2</sub> + 16.33 N <sub>2</sub> → 33 BN + ThB <sub>6</sub> H <sub>4</sub> C <sub>6</sub> N                                     | -75.2927            |
| ThNH <sub>4</sub> B <sub>6</sub> C <sub>6</sub> | 0.25 Th <sub>4</sub> H <sub>15</sub> + 2.922 B <sub>13</sub> C <sub>2</sub> + 0.03125 H <sub>8</sub> C <sub>5</sub> + 16.49 N <sub>2</sub> → 31.98 BN + ThB <sub>6</sub> H <sub>4</sub> C <sub>6</sub> N          | -74.2909            |
| ThNH <sub>4</sub> B <sub>6</sub> C <sub>6</sub> | 3 B <sub>13</sub> C <sub>2</sub> + 1.333 H <sub>3</sub> N + 15.83 N <sub>2</sub> + ThN → 33 BN + ThB <sub>6</sub> H <sub>4</sub> C <sub>6</sub> N                                                                 | -74.1493            |
| ThNH <sub>4</sub> B <sub>6</sub> C <sub>6</sub> | 0.3333 Th <sub>3</sub> N <sub>4</sub> + 3 B <sub>13</sub> C <sub>2</sub> + 1.333 H <sub>3</sub> N + 15.67 N <sub>2</sub> → 33 BN + ThB <sub>6</sub> H <sub>4</sub> C <sub>6</sub> N                               | -73.5273            |
| ThNH <sub>4</sub> B <sub>6</sub> C <sub>6</sub> | ThC + 0.3636 B <sub>9</sub> H <sub>11</sub> + 2.5 B <sub>13</sub> C <sub>2</sub> + 15.39 N <sub>2</sub> → 29.77 BN + ThB <sub>6</sub> H <sub>4</sub> C <sub>6</sub> N                                             | -70.0881            |
| ThNH <sub>4</sub> B <sub>6</sub> C <sub>6</sub> | 0.5714 B <sub>5</sub> H <sub>7</sub> + ThC + 2.5 B <sub>13</sub> C <sub>2</sub> + 15.18 N <sub>2</sub> → 29.36 BN + ThB <sub>6</sub> H <sub>4</sub> C <sub>6</sub> N                                              | -69.0836            |
| ThNH <sub>4</sub> B <sub>6</sub> C <sub>6</sub> | 2 ThH <sub>2</sub> + 3 B <sub>13</sub> C <sub>2</sub> + 15 N <sub>2</sub> → ThB <sub>4</sub> + 29 BN + ThB <sub>6</sub> H <sub>4</sub> C <sub>6</sub> N                                                           | -69.0186            |
| ThNH <sub>4</sub> B <sub>6</sub> C <sub>6</sub> | 43 ThC <sub>2</sub> + 44 H <sub>3</sub> N + ThB <sub>6</sub> → 16 H <sub>8</sub> C <sub>5</sub> + 43 ThN + ThB <sub>6</sub> H <sub>4</sub> C <sub>6</sub> N                                                       | -68.0925            |
| ThNH <sub>4</sub> B <sub>6</sub> C <sub>6</sub> | 2 ThH <sub>2</sub> + 3 B <sub>13</sub> C <sub>2</sub> + 14 N <sub>2</sub> → 27 BN + ThB <sub>6</sub> + ThB <sub>6</sub> H <sub>4</sub> C <sub>6</sub> N                                                           | -64.1737            |
| ThNH <sub>4</sub> B <sub>6</sub> C <sub>6</sub> | ThC + 2 H <sub>2</sub> + 2.5 B <sub>13</sub> C <sub>2</sub> + 13.75 N <sub>2</sub> → 26.5 BN + ThB <sub>6</sub> H <sub>4</sub> C <sub>6</sub> N                                                                   | -62.3472            |
| ThNH <sub>4</sub> B <sub>6</sub> C <sub>6</sub> | 0.3636 B <sub>9</sub> H <sub>11</sub> + 2.25 B <sub>13</sub> C <sub>2</sub> + 0.5 Th <sub>2</sub> C <sub>3</sub> + 13.76 N <sub>2</sub> → 26.52 BN + ThB <sub>6</sub> H <sub>4</sub> C <sub>6</sub> N             | -61.9173            |
| ThNH <sub>4</sub> B <sub>6</sub> C <sub>6</sub> | 0.5714 B <sub>5</sub> H <sub>7</sub> + 2.25 B <sub>13</sub> C <sub>2</sub> + 0.5 Th <sub>2</sub> C <sub>3</sub> + 13.55 N <sub>2</sub> → 26.11 BN + ThB <sub>6</sub> H <sub>4</sub> C <sub>6</sub> N              | -60.9128            |
| ThNH <sub>4</sub> B <sub>6</sub> C <sub>6</sub> | ThC + 2.5 B <sub>13</sub> C <sub>2</sub> + 1.333 H <sub>3</sub> N + 13.08 N <sub>2</sub> → 26.5 BN + ThB <sub>6</sub> H <sub>4</sub> C <sub>6</sub> N                                                             | -60.5818            |
| ThNH <sub>4</sub> B <sub>6</sub> C <sub>6</sub> | ThH <sub>2</sub> + 2.375 B <sub>13</sub> C <sub>2</sub> + 0.25 H <sub>8</sub> C <sub>5</sub> + 12.94 N <sub>2</sub> → 24.87 BN + ThB <sub>6</sub> H <sub>4</sub> C <sub>6</sub> N                                 | -56.9835            |
| ThNH <sub>4</sub> B <sub>6</sub> C <sub>6</sub> | 25.1 ThH <sub>2</sub> + 3 B <sub>13</sub> C <sub>2</sub> + 16.57 N <sub>2</sub> → 6.6 B <sub>5</sub> H <sub>7</sub> + 8.033 Th <sub>3</sub> N <sub>4</sub> + ThB <sub>6</sub> H <sub>4</sub> C <sub>6</sub> N     | -56.0264            |
| ThNH <sub>4</sub> B <sub>6</sub> C <sub>6</sub> | 2 H <sub>2</sub> + 2.25 B <sub>13</sub> C <sub>2</sub> + 0.5 Th <sub>2</sub> C <sub>3</sub> + 12.12 N <sub>2</sub> → 23.25 BN + ThB <sub>6</sub> H <sub>4</sub> C <sub>6</sub> N                                  | -54.1764            |
| ThNH <sub>4</sub> B <sub>6</sub> C <sub>6</sub> | ThC <sub>2</sub> + 0.3636 B <sub>9</sub> H <sub>11</sub> + 2 B <sub>13</sub> C <sub>2</sub> + 12.14 N <sub>2</sub> → 23.27 BN + ThB <sub>6</sub> H <sub>4</sub> C <sub>6</sub> N                                  | -53.7538            |
| ThNH <sub>4</sub> B <sub>6</sub> C <sub>6</sub> | 0.5714 B <sub>5</sub> H <sub>7</sub> + ThC <sub>2</sub> + 2 B <sub>13</sub> C <sub>2</sub> + 11.93 N <sub>2</sub> → 22.86 BN + ThB <sub>6</sub> H <sub>4</sub> C <sub>6</sub> N                                   | -52.7494            |
| ThNH <sub>4</sub> B <sub>6</sub> C <sub>6</sub> | 2.25 B <sub>13</sub> C <sub>2</sub> + 0.5 Th <sub>2</sub> C <sub>3</sub> + 1.333 H <sub>3</sub> N + 11.46 N <sub>2</sub> → 23.25 BN + ThB <sub>6</sub> H <sub>4</sub> C <sub>6</sub> N                            | -52.4110            |
| ThNH <sub>4</sub> B <sub>6</sub> C <sub>6</sub> | 1.75 B <sub>13</sub> C <sub>2</sub> + 0.5 H <sub>8</sub> C <sub>5</sub> + 11.88 N <sub>2</sub> + ThB <sub>6</sub> → 22.75 BN + ThB <sub>6</sub> H <sub>4</sub> C <sub>6</sub> N                                   | -49.7934            |
| ThNH <sub>4</sub> B <sub>6</sub> C <sub>6</sub> | 22.17 ThH <sub>2</sub> + 3 B <sub>13</sub> C <sub>2</sub> + 14.61 N <sub>2</sub> → 7.056 Th <sub>3</sub> N <sub>4</sub> + 3.667 B <sub>9</sub> H <sub>11</sub> + ThB <sub>6</sub> H <sub>4</sub> C <sub>6</sub> N | -48.9372            |
| ThNH <sub>4</sub> B <sub>6</sub> C <sub>6</sub> | 2 H <sub>2</sub> + ThC <sub>2</sub> + 2 B <sub>13</sub> C <sub>2</sub> + 10.5 N <sub>2</sub> → 20 BN + ThB <sub>6</sub> H <sub>4</sub> C <sub>6</sub> N                                                           | -46.0129            |
| ThNH <sub>4</sub> B <sub>6</sub> C <sub>6</sub> | ThB <sub>4</sub> + 1.75 B <sub>13</sub> C <sub>2</sub> + 0.5 H <sub>8</sub> C <sub>5</sub> + 10.87 N <sub>2</sub> → 20.75 BN + ThB <sub>6</sub> H <sub>4</sub> C <sub>6</sub> N                                   | -44.9485            |
| ThNH <sub>4</sub> B <sub>6</sub> C <sub>6</sub> | 63.87 H <sub>2</sub> + 3 B <sub>13</sub> C <sub>2</sub> + 34 ThN → 8.25 Th <sub>4</sub> H <sub>15</sub> + 33 BN + ThB <sub>6</sub> H <sub>4</sub> C <sub>6</sub> N                                                | -44.3560            |
| ThNH <sub>4</sub> B <sub>6</sub> C <sub>6</sub> | ThC <sub>2</sub> + 2 B <sub>13</sub> C <sub>2</sub> + 1.333 H <sub>3</sub> N + 9.833 N <sub>2</sub> → 20 BN + ThB <sub>6</sub> H <sub>4</sub> C <sub>6</sub> N                                                    | -44.2475            |
| ThNH <sub>4</sub> B <sub>6</sub> C <sub>6</sub> | 28 ThC <sub>2</sub> + 6 B + 28 H <sub>3</sub> N → 10 H <sub>8</sub> C <sub>5</sub> + 27 ThN + ThB <sub>6</sub> H <sub>4</sub> C <sub>6</sub> N                                                                    | -42.6489            |
| ThNH <sub>4</sub> B <sub>6</sub> C <sub>6</sub> | 25.1 ThH <sub>2</sub> + 3 B <sub>13</sub> C <sub>2</sub> + 12.55 N <sub>2</sub> → 6.6 B <sub>5</sub> H <sub>7</sub> + 24.1 ThN + ThB <sub>6</sub> H <sub>4</sub> C <sub>6</sub> N                                 | -41.0366            |
| ThNH <sub>4</sub> B <sub>6</sub> C <sub>6</sub> | 3 B <sub>13</sub> C <sub>2</sub> + 40 H <sub>3</sub> N + ThB <sub>6</sub> → 58 H <sub>2</sub> + 39 BN + ThB <sub>6</sub> H <sub>4</sub> C <sub>6</sub> N                                                          | -38.1135            |
| ThNH <sub>4</sub> B <sub>6</sub> C <sub>6</sub> | 1.75 B <sub>13</sub> C <sub>2</sub> + Th + 0.5 H <sub>8</sub> C <sub>5</sub> + 8.875 N <sub>2</sub> → 16.75 BN + ThB <sub>6</sub> H <sub>4</sub> C <sub>6</sub> N                                                 | -37.7794            |
| ThNH <sub>4</sub> B <sub>6</sub> C <sub>6</sub> | 3 B <sub>13</sub> C <sub>2</sub> + 18.93 H <sub>3</sub> N + 15.07 ThN → 3.519 Th <sub>4</sub> H <sub>15</sub> + 33 BN + ThB <sub>6</sub> H <sub>4</sub> C <sub>6</sub> N                                          | -37.3961            |
| ThNH <sub>4</sub> B <sub>6</sub> C <sub>6</sub> | 8.5 Th <sub>3</sub> N <sub>4</sub> + 47.94 H <sub>2</sub> + 3 B <sub>13</sub> C <sub>2</sub> → 6.125 Th <sub>4</sub> H <sub>15</sub> + 33 BN + ThB <sub>6</sub> H <sub>4</sub> C <sub>6</sub> N                   | -36.6242            |
| ThNH <sub>4</sub> B <sub>6</sub> C <sub>6</sub> | ThB <sub>4</sub> + 3 B <sub>13</sub> C <sub>2</sub> + 38 H <sub>3</sub> N → 55 H <sub>2</sub> + 37 BN + ThB <sub>6</sub> H <sub>4</sub> C <sub>6</sub> N                                                          | -35.9167            |
| ThNH <sub>4</sub> B <sub>6</sub> C <sub>6</sub> | 22.17 ThH <sub>2</sub> + 3 B <sub>13</sub> C <sub>2</sub> + 11.08 N <sub>2</sub> → 3.667 B <sub>9</sub> H <sub>11</sub> + 21.17 ThN + ThB <sub>6</sub> H <sub>4</sub> C <sub>6</sub> N                            | -35.7719            |
| ThNH <sub>4</sub> B <sub>6</sub> C <sub>6</sub> | 1.75 B <sub>13</sub> C <sub>2</sub> + 0.5 H <sub>8</sub> C <sub>5</sub> + 8.375 N <sub>2</sub> + ThN → 16.75 BN + ThB <sub>6</sub> H <sub>4</sub> C <sub>6</sub> N                                                | -34.6318            |
| ThNH <sub>4</sub> B <sub>6</sub> C <sub>6</sub> | 4.376 Th <sub>3</sub> N <sub>4</sub> + 3 B <sub>13</sub> C <sub>2</sub> + 16.49 H <sub>3</sub> N → 3.032 Th <sub>4</sub> H <sub>15</sub> + 33 BN + ThB <sub>6</sub> H <sub>4</sub> C <sub>6</sub> N               | -34.3093            |
| ThNH <sub>4</sub> B <sub>6</sub> C <sub>6</sub> | 3 B <sub>13</sub> C <sub>2</sub> + Th + 34 H <sub>3</sub> N → 49 H <sub>2</sub> + 33 BN + ThB <sub>6</sub> H <sub>4</sub> C <sub>6</sub> N                                                                        | -34.0439            |
| ThNH <sub>4</sub> B <sub>6</sub> C <sub>6</sub> | 0.3333 Th <sub>3</sub> N <sub>4</sub> + 1.75 B <sub>13</sub> C <sub>2</sub> + 0.5 H <sub>8</sub> C <sub>5</sub> + 8.208 N <sub>2</sub> → 16.75 BN + ThB <sub>6</sub> H <sub>4</sub> C <sub>6</sub> N              | -34.0098            |
| ThNH <sub>4</sub> B <sub>6</sub> C <sub>6</sub> | 6 ThC + 2.068 B <sub>9</sub> H <sub>11</sub> + 6.807 N <sub>2</sub> → 1.25 Th <sub>4</sub> H <sub>15</sub> + 12.61 BN + ThB <sub>6</sub> H <sub>4</sub> C <sub>6</sub> N                                          | -33.7542            |
| ThNH <sub>4</sub> B <sub>6</sub> C <sub>6</sub> | ThH <sub>2</sub> + 3 B <sub>13</sub> C <sub>2</sub> + 34 H <sub>3</sub> N → 50 H <sub>2</sub> + 33 BN + ThB <sub>6</sub> H <sub>4</sub> C <sub>6</sub> N                                                          | -32.6066            |
| ThNH <sub>4</sub> B <sub>6</sub> C <sub>6</sub> | 3 B <sub>13</sub> C <sub>2</sub> + 33 H <sub>3</sub> N + ThN → 47.5 H <sub>2</sub> + 33 BN + ThB <sub>6</sub> H <sub>4</sub> C <sub>6</sub> N                                                                     | -32.2204            |
| ThNH <sub>4</sub> B <sub>6</sub> C <sub>6</sub> | 0.3333 Th <sub>3</sub> N <sub>4</sub> + 3 B <sub>13</sub> C <sub>2</sub> + 32.67 H <sub>3</sub> N → 47 H <sub>2</sub> + 33 BN + ThB <sub>6</sub> H <sub>4</sub> C <sub>6</sub> N                                  | -32.0398            |
| ThNH <sub>4</sub> B <sub>6</sub> C <sub>6</sub> | 0.25 Th <sub>4</sub> H <sub>15</sub> + 3 B <sub>13</sub> C <sub>2</sub> + 34 H <sub>3</sub> N → 50.87 H <sub>2</sub> + 33 BN + ThB <sub>6</sub> H <sub>4</sub> C <sub>6</sub> N                                   | -31.8527            |
| ThNH <sub>4</sub> B <sub>6</sub> C <sub>6</sub> | 1.2 H <sub>8</sub> C <sub>5</sub> + 8.9 N <sub>2</sub> + 3.8 ThB <sub>6</sub> → 2.8 ThH <sub>2</sub> + 16.8 BN + ThB <sub>6</sub> H <sub>4</sub> C <sub>6</sub> N                                                 | -29.6609            |
| ThNH <sub>4</sub> B <sub>6</sub> C <sub>6</sub> | 20.62 ThC <sub>2</sub> + 0.4615 B <sub>13</sub> C <sub>2</sub> + 20.62 H <sub>3</sub> N → 7.231 H <sub>8</sub> C <sub>5</sub> + 19.62 ThN + ThB <sub>6</sub> H <sub>4</sub> C <sub>6</sub> N                      | -29.1956            |
| ThNH <sub>4</sub> B <sub>6</sub> C <sub>6</sub> | 3 B <sub>13</sub> C <sub>2</sub> + 16.73 Th + 16.73 H <sub>3</sub> N → 6.6 B <sub>5</sub> H <sub>7</sub> + 15.73 ThN + ThB <sub>6</sub> H <sub>4</sub> C <sub>6</sub> N                                           | -28.6217            |
| ThNH <sub>4</sub> B <sub>6</sub> C <sub>6</sub> | 3.25 B <sub>5</sub> H <sub>7</sub> + 6 ThC + 5.625 N <sub>2</sub> → 1.25 Th <sub>4</sub> H <sub>15</sub> + 10.25 BN + ThB <sub>6</sub> H <sub>4</sub> C <sub>6</sub> N                                            | -28.0414            |
| ThNH <sub>4</sub> B <sub>6</sub> C <sub>6</sub> | ThC + 2.5 B <sub>13</sub> C <sub>2</sub> + 27.5 H <sub>3</sub> N → 39.25 H <sub>2</sub> + 26.5 BN + ThB <sub>6</sub> H <sub>4</sub> C <sub>6</sub> N                                                              | -25.9353            |
| ThNH <sub>4</sub> B <sub>6</sub> C <sub>6</sub> | 3 B <sub>13</sub> C <sub>2</sub> + 14 H <sub>3</sub> N + 20 ThN → 19 ThH <sub>2</sub> + 33 BN + ThB <sub>6</sub> H <sub>4</sub> C <sub>6</sub> N                                                                  | -24.8826            |
| ThNH <sub>4</sub> B <sub>6</sub> C <sub>6</sub> | 3 B <sub>13</sub> C <sub>2</sub> + 14.78 Th + 14.78 H <sub>3</sub> N → 3.667 B <sub>9</sub> H <sub>11</sub> + 13.78 ThN + ThB <sub>6</sub> H <sub>4</sub> C <sub>6</sub> N                                        | -24.8079            |
| ThNH <sub>4</sub> B <sub>6</sub> C <sub>6</sub> | 7.2 B <sub>5</sub> H <sub>7</sub> + 6 ThC + 8.233 N <sub>2</sub> → 15.47 H <sub>3</sub> N + 5 ThB <sub>6</sub> + ThB <sub>6</sub> H <sub>4</sub> C <sub>6</sub> N                                                 | -24.0599            |
| ThNH <sub>4</sub> B <sub>6</sub> C <sub>6</sub> | 11 B <sub>5</sub> H <sub>7</sub> + 6 C + 12.5 Th <sub>3</sub> N <sub>4</sub> → 36.5 ThH <sub>2</sub> + 49 BN + ThB <sub>6</sub> H <sub>4</sub> C <sub>6</sub> N                                                   | -23.7652            |
| ThNH <sub>4</sub> B <sub>6</sub> C <sub>6</sub> | 3 B <sub>13</sub> C <sub>2</sub> + 12.8 Th + 16.73 H <sub>3</sub> N → 6.6 B <sub>5</sub> H <sub>7</sub> + 3.933 Th <sub>3</sub> N <sub>4</sub> + ThB <sub>6</sub> H <sub>4</sub> C <sub>6</sub> N                 | -23.5808            |
| ThNH <sub>4</sub> B <sub>6</sub> C <sub>6</sub> | 5.556 Th <sub>3</sub> N <sub>4</sub> + 3 B <sub>13</sub> C <sub>2</sub> + 11.78 H <sub>3</sub> N → 15.67 ThH <sub>2</sub> + 33 BN + ThB <sub>6</sub> H <sub>4</sub> C <sub>6</sub> N                              | -23.1595            |
| ThNH <sub>4</sub> B <sub>6</sub> C <sub>6</sub> | 2.25 B <sub>13</sub> C <sub>2</sub> + 0.5 Th <sub>2</sub> C <sub>3</sub> + 24.25 H <sub>3</sub> N → 34.38 H <sub>2</sub> + 23.25 BN + ThB <sub>6</sub> H <sub>4</sub> C <sub>6</sub> N                            | -22.0677            |
| ThNH <sub>4</sub> B <sub>6</sub> C <sub>6</sub> | 0.3636 B <sub>9</sub> H <sub>11</sub> + 3 B <sub>13</sub> C <sub>2</sub> + 10.07 Th + 0.5 N <sub>2</sub> → 9.068 ThB <sub>4</sub> + ThB <sub>6</sub> H <sub>4</sub> C <sub>6</sub> N                              | -21.7924            |

Continued on next page

Continued

| Compound                                        | Chemical reaction                                                                                                                                                                                                                | Reaction energy(eV) |
|-------------------------------------------------|----------------------------------------------------------------------------------------------------------------------------------------------------------------------------------------------------------------------------------|---------------------|
| ThNH <sub>4</sub> B <sub>6</sub> C <sub>6</sub> | 1.2 B <sub>5</sub> H <sub>7</sub> + 8.75 ThC + 5.667 N <sub>2</sub> → 2.583 Th <sub>3</sub> N <sub>4</sub> + 0.55 H <sub>8</sub> C <sub>5</sub> + ThB <sub>6</sub> H <sub>4</sub> C <sub>6</sub> N                               | -21.5769            |
| ThNH <sub>4</sub> B <sub>6</sub> C <sub>6</sub> | 0.5714 B <sub>5</sub> H <sub>7</sub> + 3 B <sub>13</sub> C <sub>2</sub> + 9.964 Th + 0.5 N <sub>2</sub> → 8.964 ThB <sub>4</sub> + ThB <sub>6</sub> H <sub>4</sub> C <sub>6</sub> N                                              | -21.5328            |
| ThNH <sub>4</sub> B <sub>6</sub> C <sub>6</sub> | 6 ThC + 4 B <sub>9</sub> H <sub>11</sub> + 7.167 N <sub>2</sub> → 13.33 H <sub>3</sub> N + 5 ThB <sub>6</sub> + ThB <sub>6</sub> H <sub>4</sub> C <sub>6</sub> N                                                                 | -21.5057            |
| ThNH <sub>4</sub> B <sub>6</sub> C <sub>6</sub> | ThC + 1.25 B <sub>13</sub> C <sub>2</sub> + 0.5 H <sub>8</sub> C <sub>5</sub> + 5.625 N <sub>2</sub> → 10.25 BN + ThB <sub>6</sub> H <sub>4</sub> C <sub>6</sub> N                                                               | -21.0643            |
| ThNH <sub>4</sub> B <sub>6</sub> C <sub>6</sub> | 12.34 Th <sub>3</sub> N <sub>4</sub> + 6.04 B <sub>9</sub> H <sub>11</sub> + 1.2 H <sub>8</sub> C <sub>5</sub> → 36.02 ThH <sub>2</sub> + 48.36 BN + ThB <sub>6</sub> H <sub>4</sub> C <sub>6</sub> N                            | -20.7820            |
| ThNH <sub>4</sub> B <sub>6</sub> C <sub>6</sub> | 3 B <sub>13</sub> C <sub>2</sub> + 11.33 Th + 14.78 H <sub>3</sub> N → 3.444 Th <sub>3</sub> N <sub>4</sub> + 3.667 B <sub>9</sub> H <sub>11</sub> + ThB <sub>6</sub> H <sub>4</sub> C <sub>6</sub> N                            | -20.3935            |
| ThNH <sub>4</sub> B <sub>6</sub> C <sub>6</sub> | 6 BN + 10.33 Th <sub>2</sub> C <sub>3</sub> + 14.67 H <sub>3</sub> N → 5 H <sub>8</sub> C <sub>5</sub> + 19.67 ThN + ThB <sub>6</sub> H <sub>4</sub> C <sub>6</sub> N                                                            | -20.0655            |
| ThNH <sub>4</sub> B <sub>6</sub> C <sub>6</sub> | BN + 0.3636 B <sub>9</sub> H <sub>11</sub> + 3 B <sub>13</sub> C <sub>2</sub> + 10.32 Th → 9.318 ThB <sub>4</sub> + ThB <sub>6</sub> H <sub>4</sub> C <sub>6</sub> N                                                             | -20.0002            |
| ThNH <sub>4</sub> B <sub>6</sub> C <sub>6</sub> | 2 H <sub>2</sub> + 3 B <sub>13</sub> C <sub>2</sub> + 9.25 Th + 0.5 N <sub>2</sub> → 8.25 ThB <sub>4</sub> + ThB <sub>6</sub> H <sub>4</sub> C <sub>6</sub> N                                                                    | -19.9172            |
| ThNH <sub>4</sub> B <sub>6</sub> C <sub>6</sub> | 0.5714 B <sub>5</sub> H <sub>7</sub> + BN + 3 B <sub>13</sub> C <sub>2</sub> + 10.21 Th → 9.214 ThB <sub>4</sub> + ThB <sub>6</sub> H <sub>4</sub> C <sub>6</sub> N                                                              | -19.7406            |
| ThNH <sub>4</sub> B <sub>6</sub> C <sub>6</sub> | 35 H <sub>2</sub> + 3 B <sub>13</sub> C <sub>2</sub> + 34 ThN → 33 ThH <sub>2</sub> + 33 BN + ThB <sub>6</sub> H <sub>4</sub> C <sub>6</sub> N                                                                                   | -19.4758            |
| ThNH <sub>4</sub> B <sub>6</sub> C <sub>6</sub> | 8.083 ThC + 0.6667 B <sub>9</sub> H <sub>11</sub> + 5.222 N <sub>2</sub> → 2.361 Th <sub>3</sub> N <sub>4</sub> + 0.4167 H <sub>8</sub> C <sub>5</sub> + ThB <sub>6</sub> H <sub>4</sub> C <sub>6</sub> N                        | -19.2436            |
| ThNH <sub>4</sub> B <sub>6</sub> C <sub>6</sub> | 3 B <sub>13</sub> C <sub>2</sub> + 9.583 Th + 1.333 H <sub>3</sub> N → 8.25 ThB <sub>4</sub> + 0.3333 ThN + ThB <sub>6</sub> H <sub>4</sub> C <sub>6</sub> N                                                                     | -19.2009            |
| ThNH <sub>4</sub> B <sub>6</sub> C <sub>6</sub> | 3 B <sub>13</sub> C <sub>2</sub> + 9.5 Th + 1.333 H <sub>3</sub> N → 8.25 ThB <sub>4</sub> + 0.08333 Th <sub>3</sub> N <sub>4</sub> + ThB <sub>6</sub> H <sub>4</sub> C <sub>6</sub> N                                           | -19.0941            |
| ThNH <sub>4</sub> B <sub>6</sub> C <sub>6</sub> | 0.09091 B <sub>9</sub> H <sub>11</sub> + 3 B <sub>13</sub> C <sub>2</sub> + 9.455 Th + H <sub>3</sub> N → 8.455 ThB <sub>4</sub> + ThB <sub>6</sub> H <sub>4</sub> C <sub>6</sub> N                                              | -19.0619            |
| ThNH <sub>4</sub> B <sub>6</sub> C <sub>6</sub> | 0.1429 B <sub>5</sub> H <sub>7</sub> + 3 B <sub>13</sub> C <sub>2</sub> + 9.429 Th + H <sub>3</sub> N → 8.429 ThB <sub>4</sub> + ThB <sub>6</sub> H <sub>4</sub> C <sub>6</sub> N                                                | -18.9970            |
| ThNH <sub>4</sub> B <sub>6</sub> C <sub>6</sub> | 0.25 Th <sub>3</sub> N <sub>4</sub> + 0.3636 B <sub>9</sub> H <sub>11</sub> + 3 B <sub>13</sub> C <sub>2</sub> + 9.318 Th → 9.068 ThB <sub>4</sub> + ThB <sub>6</sub> H <sub>4</sub> C <sub>6</sub> N                            | -18.9653            |
| ThNH <sub>4</sub> B <sub>6</sub> C <sub>6</sub> | 3 B <sub>13</sub> C <sub>2</sub> + 9.167 Th + 1.333 H <sub>3</sub> N → 8.167 ThB <sub>4</sub> + 0.3333 BN + ThB <sub>6</sub> H <sub>4</sub> C <sub>6</sub> N                                                                     | -18.7492            |
| ThNH <sub>4</sub> B <sub>6</sub> C <sub>6</sub> | 0.5714 B <sub>5</sub> H <sub>7</sub> + 0.25 Th <sub>3</sub> N <sub>4</sub> + 3 B <sub>13</sub> C <sub>2</sub> + 9.214 Th → 8.964 ThB <sub>4</sub> + ThB <sub>6</sub> H <sub>4</sub> C <sub>6</sub> N                             | -18.7057            |
| ThNH <sub>4</sub> B <sub>6</sub> C <sub>6</sub> | 2 ThH <sub>2</sub> + 1.5 ThB <sub>4</sub> + 6 ThC + 6.167 N <sub>2</sub> → 2.833 Th <sub>3</sub> N <sub>4</sub> + ThB <sub>6</sub> H <sub>4</sub> C <sub>6</sub> N                                                               | -18.6919            |
| ThNH <sub>4</sub> B <sub>6</sub> C <sub>6</sub> | 0.3636 B <sub>9</sub> H <sub>11</sub> + 3 B <sub>13</sub> C <sub>2</sub> + 9.068 Th + ThN → 9.068 ThB <sub>4</sub> + ThB <sub>6</sub> H <sub>4</sub> C <sub>6</sub> N                                                            | -18.6449            |
| ThNH <sub>4</sub> B <sub>6</sub> C <sub>6</sub> | 3.347 Th <sub>4</sub> H <sub>15</sub> + 3 B <sub>13</sub> C <sub>2</sub> + 8.758 N <sub>2</sub> → 6.6 B <sub>5</sub> H <sub>7</sub> + 4.129 Th <sub>3</sub> N <sub>4</sub> + ThB <sub>6</sub> H <sub>4</sub> C <sub>6</sub> N    | -18.6151            |
| ThNH <sub>4</sub> B <sub>6</sub> C <sub>6</sub> | 0.5 H <sub>2</sub> + 3 B <sub>13</sub> C <sub>2</sub> + 9.25 Th + H <sub>3</sub> N → 8.25 ThB <sub>4</sub> + ThB <sub>6</sub> H <sub>4</sub> C <sub>6</sub> N                                                                    | -18.5931            |
| ThNH <sub>4</sub> B <sub>6</sub> C <sub>6</sub> | 5.2 B <sub>5</sub> H <sub>7</sub> + 6 ThC + 5.9 N <sub>2</sub> → 5 ThB <sub>4</sub> + 10.8 H <sub>3</sub> N + ThB <sub>6</sub> H <sub>4</sub> C <sub>6</sub> N                                                                   | -18.5279            |
| ThNH <sub>4</sub> B <sub>6</sub> C <sub>6</sub> | 0.5714 B <sub>5</sub> H <sub>7</sub> + 3 B <sub>13</sub> C <sub>2</sub> + 8.964 Th + ThN → 8.964 ThB <sub>4</sub> + ThB <sub>6</sub> H <sub>4</sub> C <sub>6</sub> N                                                             | -18.3853            |
| ThNH <sub>4</sub> B <sub>6</sub> C <sub>6</sub> | ThC <sub>2</sub> + 2 B <sub>13</sub> C <sub>2</sub> + 21 H <sub>3</sub> N → 29.5 H <sub>2</sub> + 20 BN + ThB <sub>6</sub> H <sub>4</sub> C <sub>6</sub> N                                                                       | -18.2074            |
| ThNH <sub>4</sub> B <sub>6</sub> C <sub>6</sub> | 8.5 Th <sub>3</sub> N <sub>4</sub> + 26.5 H <sub>2</sub> + 3 B <sub>13</sub> C <sub>2</sub> → 24.5 ThH <sub>2</sub> + 33 BN + ThB <sub>6</sub> H <sub>4</sub> C <sub>6</sub> N                                                   | -18.1525            |
| ThNH <sub>4</sub> B <sub>6</sub> C <sub>6</sub> | 3 B <sub>13</sub> C <sub>2</sub> + 9.25 Th + 1.333 H <sub>3</sub> N → 8.25 ThB <sub>4</sub> + 0.1667 N <sub>2</sub> + ThB <sub>6</sub> H <sub>4</sub> C <sub>6</sub> N                                                           | -18.1518            |
| ThNH <sub>4</sub> B <sub>6</sub> C <sub>6</sub> | 2 H <sub>2</sub> + BN + 3 B <sub>13</sub> C <sub>2</sub> + 9.5 Th → 8.5 ThB <sub>4</sub> + ThB <sub>6</sub> H <sub>4</sub> C <sub>6</sub> N                                                                                      | -18.1249            |
| ThNH <sub>4</sub> B <sub>6</sub> C <sub>6</sub> | 2 ThH <sub>2</sub> + 6 ThC + 5.833 N <sub>2</sub> + ThB <sub>6</sub> → 2.667 Th <sub>3</sub> N <sub>4</sub> + ThB <sub>6</sub> H <sub>4</sub> C <sub>6</sub> N                                                                   | -18.0675            |
| ThNH <sub>4</sub> B <sub>6</sub> C <sub>6</sub> | 0.06667 Th <sub>4</sub> H <sub>15</sub> + 3 B <sub>13</sub> C <sub>2</sub> + 8.983 Th + H <sub>3</sub> N → 8.25 ThB <sub>4</sub> + ThB <sub>6</sub> H <sub>4</sub> C <sub>6</sub> N                                              | -18.0088            |
| ThNH <sub>4</sub> B <sub>6</sub> C <sub>6</sub> | 0.5 ThH <sub>2</sub> + 3 B <sub>13</sub> C <sub>2</sub> + 8.75 Th + H <sub>3</sub> N → 8.25 ThB <sub>4</sub> + ThB <sub>6</sub> H <sub>4</sub> C <sub>6</sub> N                                                                  | -17.7845            |
| ThNH <sub>4</sub> B <sub>6</sub> C <sub>6</sub> | 6 BN + 16.75 ThC <sub>2</sub> + 16 H <sub>3</sub> N → 5.25 Th <sub>3</sub> N <sub>4</sub> + 5.5 H <sub>8</sub> C <sub>5</sub> + ThB <sub>6</sub> H <sub>4</sub> C <sub>6</sub> N                                                 | -17.7826            |
| ThNH <sub>4</sub> B <sub>6</sub> C <sub>6</sub> | 2 ThH <sub>2</sub> + 6 ThC + 6 B + 5.167 N <sub>2</sub> → 2.333 Th <sub>3</sub> N <sub>4</sub> + ThB <sub>6</sub> H <sub>4</sub> C <sub>6</sub> N                                                                                | -17.6845            |
| ThNH <sub>4</sub> B <sub>6</sub> C <sub>6</sub> | 0.2667 Th <sub>4</sub> H <sub>15</sub> + 3 B <sub>13</sub> C <sub>2</sub> + 8.183 Th + 0.5 N <sub>2</sub> → 8.25 ThB <sub>4</sub> + ThB <sub>6</sub> H <sub>4</sub> C <sub>6</sub> N                                             | -17.5799            |
| ThNH <sub>4</sub> B <sub>6</sub> C <sub>6</sub> | 0.25 Th <sub>3</sub> N <sub>4</sub> + 2 H <sub>2</sub> + 3 B <sub>13</sub> C <sub>2</sub> + 8.5 Th → 8.25 ThB <sub>4</sub> + ThB <sub>6</sub> H <sub>4</sub> C <sub>6</sub> N                                                    | -17.0900            |
| ThNH <sub>4</sub> B <sub>6</sub> C <sub>6</sub> | 2 ThH <sub>2</sub> + 3 B <sub>13</sub> C <sub>2</sub> + 7.25 Th + 0.5 N <sub>2</sub> → 8.25 ThB <sub>4</sub> + ThB <sub>6</sub> H <sub>4</sub> C <sub>6</sub> N                                                                  | -17.0426            |
| ThNH <sub>4</sub> B <sub>6</sub> C <sub>6</sub> | 2 H <sub>2</sub> + 3 B <sub>13</sub> C <sub>2</sub> + 8.25 Th + ThN → 8.25 ThB <sub>4</sub> + ThB <sub>6</sub> H <sub>4</sub> C <sub>6</sub> N                                                                                   | -16.7696            |
| ThNH <sub>4</sub> B <sub>6</sub> C <sub>6</sub> | 1.2 B <sub>5</sub> H <sub>7</sub> + 8.75 ThC + 4.375 N <sub>2</sub> → 0.55 H <sub>8</sub> C <sub>5</sub> + 7.75 ThN + ThB <sub>6</sub> H <sub>4</sub> C <sub>6</sub> N                                                           | -16.7566            |
| ThNH <sub>4</sub> B <sub>6</sub> C <sub>6</sub> | 6 ThC + 2.889 B <sub>9</sub> H <sub>11</sub> + 5.13 N <sub>2</sub> → 5 ThB <sub>4</sub> + 9.259 H <sub>3</sub> N + ThB <sub>6</sub> H <sub>4</sub> C <sub>6</sub> N                                                              | -16.6832            |
| ThNH <sub>4</sub> B <sub>6</sub> C <sub>6</sub> | 36.27 Th <sub>3</sub> N <sub>4</sub> + 0.3636 B <sub>9</sub> H <sub>11</sub> + 3 B <sub>13</sub> C <sub>2</sub> → 36.27 BN + 107.8 ThN + ThB <sub>6</sub> H <sub>4</sub> C <sub>6</sub> N                                        | -15.9725            |
| ThNH <sub>4</sub> B <sub>6</sub> C <sub>6</sub> | 2.956 Th <sub>4</sub> H <sub>15</sub> + 3 B <sub>13</sub> C <sub>2</sub> + 7.715 N <sub>2</sub> → 3.607 Th <sub>3</sub> N <sub>4</sub> + 3.667 B <sub>9</sub> H <sub>11</sub> + ThB <sub>6</sub> H <sub>4</sub> C <sub>6</sub> N | -15.8980            |
| ThNH <sub>4</sub> B <sub>6</sub> C <sub>6</sub> | 0.2667 Th <sub>4</sub> H <sub>15</sub> + BN + 3 B <sub>13</sub> C <sub>2</sub> + 8.433 Th → 8.5 ThB <sub>4</sub> + ThB <sub>6</sub> H <sub>4</sub> C <sub>6</sub> N                                                              | -15.7876            |
| ThNH <sub>4</sub> B <sub>6</sub> C <sub>6</sub> | 0.5714 B <sub>5</sub> H <sub>7</sub> + 35.86 Th <sub>3</sub> N <sub>4</sub> + 3 B <sub>13</sub> C <sub>2</sub> → 35.86 BN + 106.6 ThN + ThB <sub>6</sub> H <sub>4</sub> C <sub>6</sub> N                                         | -15.7435            |
| ThNH <sub>4</sub> B <sub>6</sub> C <sub>6</sub> | 1.5 ThB <sub>4</sub> + 6 ThC + 0.2667 Th <sub>4</sub> H <sub>15</sub> + 5.544 N <sub>2</sub> → 2.522 Th <sub>3</sub> N <sub>4</sub> + ThB <sub>6</sub> H <sub>4</sub> C <sub>6</sub> N                                           | -15.7110            |
| ThNH <sub>4</sub> B <sub>6</sub> C <sub>6</sub> | 1.386 B <sub>9</sub> H <sub>11</sub> + 2 Th <sub>2</sub> C <sub>3</sub> + 3.739 N <sub>2</sub> → 0.75 Th <sub>4</sub> H <sub>15</sub> + 6.477 BN + ThB <sub>6</sub> H <sub>4</sub> C <sub>6</sub> N                              | -15.6046            |
| ThNH <sub>4</sub> B <sub>6</sub> C <sub>6</sub> | 2.687 B <sub>13</sub> C <sub>2</sub> + 8.234 Th + H <sub>3</sub> N + 0.125 H <sub>8</sub> C <sub>5</sub> → 7.234 ThB <sub>4</sub> + ThB <sub>6</sub> H <sub>4</sub> C <sub>6</sub> N                                             | -15.5535            |
| ThNH <sub>4</sub> B <sub>6</sub> C <sub>6</sub> | 2 ThH <sub>2</sub> + BN + 3 B <sub>13</sub> C <sub>2</sub> + 7.5 Th → 8.5 ThB <sub>4</sub> + ThB <sub>6</sub> H <sub>4</sub> C <sub>6</sub> N                                                                                    | -15.2503            |
| ThNH <sub>4</sub> B <sub>6</sub> C <sub>6</sub> | 2 ThH <sub>2</sub> + 6 ThC + 54 B + ThN → 8 ThB <sub>6</sub> + ThB <sub>6</sub> H <sub>4</sub> C <sub>6</sub> N                                                                                                                  | -15.2427            |
| ThNH <sub>4</sub> B <sub>6</sub> C <sub>6</sub> | 6 ThC + 0.2667 Th <sub>4</sub> H <sub>15</sub> + 5.211 N <sub>2</sub> + ThB <sub>6</sub> → 2.356 Th <sub>3</sub> N <sub>4</sub> + ThB <sub>6</sub> H <sub>4</sub> C <sub>6</sub> N                                               | -15.0865            |
| ThNH <sub>4</sub> B <sub>6</sub> C <sub>6</sub> | 31.67 Th <sub>3</sub> N <sub>4</sub> + 3 B <sub>13</sub> C <sub>2</sub> + 1.333 H <sub>3</sub> N → 33 BN + 94 ThN + ThB <sub>6</sub> H <sub>4</sub> C <sub>6</sub> N                                                             | -15.0609            |
| ThNH <sub>4</sub> B <sub>6</sub> C <sub>6</sub> | 2 ThH <sub>2</sub> + 6 ThC + 48 B + 0.5 N <sub>2</sub> → 7 ThB <sub>6</sub> + ThB <sub>6</sub> H <sub>4</sub> C <sub>6</sub> N                                                                                                   | -15.0037            |
| ThNH <sub>4</sub> B <sub>6</sub> C <sub>6</sub> | 4.576 ThB <sub>4</sub> + 6 ThC + 13.3 H <sub>3</sub> N → 2.394 Th <sub>4</sub> H <sub>15</sub> + 12.3 BN + ThB <sub>6</sub> H <sub>4</sub> C <sub>6</sub> N                                                                      | -14.9444            |
| ThNH <sub>4</sub> B <sub>6</sub> C <sub>6</sub> | 8.083 ThC + 0.6667 B <sub>9</sub> H <sub>11</sub> + 4.042 N <sub>2</sub> → 0.4167 H <sub>8</sub> C <sub>5</sub> + 7.083 ThN + ThB <sub>6</sub> H <sub>4</sub> C <sub>6</sub> N                                                   | -14.8379            |
| ThNH <sub>4</sub> B <sub>6</sub> C <sub>6</sub> | 0.25 Th <sub>3</sub> N <sub>4</sub> + 0.2667 Th <sub>4</sub> H <sub>15</sub> + 3 B <sub>13</sub> C <sub>2</sub> + 7.433 Th → 8.25 ThB <sub>4</sub> + ThB <sub>6</sub> H <sub>4</sub> C <sub>6</sub> N                            | -14.7527            |
| ThNH <sub>4</sub> B <sub>6</sub> C <sub>6</sub> | 2 ThH <sub>2</sub> + 0.25 Th <sub>3</sub> N <sub>4</sub> + 6 ThC + 52.5 B → 7.75 ThB <sub>6</sub> + ThB <sub>6</sub> H <sub>4</sub> C <sub>6</sub> N                                                                             | -14.7165            |
| ThNH <sub>4</sub> B <sub>6</sub> C <sub>6</sub> | 6 ThC + 0.2667 Th <sub>4</sub> H <sub>15</sub> + 6 B + 4.544 N <sub>2</sub> → 2.022 Th <sub>3</sub> N <sub>4</sub> + ThB <sub>6</sub> H <sub>4</sub> C <sub>6</sub> N                                                            | -14.7036            |
| ThNH <sub>4</sub> B <sub>6</sub> C <sub>6</sub> | 0.2667 Th <sub>4</sub> H <sub>15</sub> + 3 B <sub>13</sub> C <sub>2</sub> + 7.183 Th + ThN → 8.25 ThB <sub>4</sub> + ThB <sub>6</sub> H <sub>4</sub> C <sub>6</sub> N                                                            | -14.4323            |
| ThNH <sub>4</sub> B <sub>6</sub> C <sub>6</sub> | 33 Th <sub>3</sub> N <sub>4</sub> + 2 H <sub>2</sub> + 3 B <sub>13</sub> C <sub>2</sub> → 33 BN + 98 ThN + ThB <sub>6</sub> H <sub>4</sub> C <sub>6</sub> N                                                                      | -14.3384            |
| ThNH <sub>4</sub> B <sub>6</sub> C <sub>6</sub> | 2 ThH <sub>2</sub> + 5.077 ThC + 0.4615 B <sub>13</sub> C <sub>2</sub> + 4.551 N <sub>2</sub> → 2.026 Th <sub>3</sub> N <sub>4</sub> + ThB <sub>6</sub> H <sub>4</sub> C <sub>6</sub> N                                          | -14.2337            |

Continued on next page



Continued

| Compound                                        | Chemical reaction                                                                                                                                                                               | Reaction energy(eV) |
|-------------------------------------------------|-------------------------------------------------------------------------------------------------------------------------------------------------------------------------------------------------|---------------------|
| ThNH <sub>4</sub> B <sub>6</sub> C <sub>6</sub> | $2 \text{ ThH}_2 + 0.25 \text{ Th}_3\text{N}_4 + 3 \text{ B}_{13}\text{C}_2 + 6.5 \text{ Th} \rightarrow 8.25 \text{ ThB}_4 + \text{ThB}_6\text{H}_4\text{C}_6\text{N}$                         | -14.2155            |
| ThNH <sub>4</sub> B <sub>6</sub> C <sub>6</sub> | $0.3636 \text{ B}_9\text{H}_{11} + 3 \text{ B}_{13}\text{C}_2 + 7.045 \text{ Th} + 0.5 \text{ N}_2 \rightarrow 6.045 \text{ ThB}_6 + \text{ThB}_6\text{H}_4\text{C}_6\text{N}$                  | -14.1730            |
| ThNH <sub>4</sub> B <sub>6</sub> C <sub>6</sub> | $1.5 \text{ ThB}_4 + 6 \text{ ThC} + 2 \text{ H}_2 + 4.833 \text{ N}_2 \rightarrow 2.167 \text{ Th}_3\text{N}_4 + \text{ThB}_6\text{H}_4\text{C}_6\text{N}$                                     | -14.0274            |
| ThNH <sub>4</sub> B <sub>6</sub> C <sub>6</sub> | $2 \text{ ThH}_2 + 35 \text{ Th}_3\text{N}_4 + 3 \text{ B}_{13}\text{C}_2 \rightarrow 33 \text{ BN} + 106 \text{ ThN} + \text{ThB}_6\text{H}_4\text{C}_6\text{N}$                               | -14.0270            |
| ThNH <sub>4</sub> B <sub>6</sub> C <sub>6</sub> | $0.5714 \text{ B}_5\text{H}_7 + 3 \text{ B}_{13}\text{C}_2 + 6.976 \text{ Th} + 0.5 \text{ N}_2 \rightarrow 5.976 \text{ ThB}_6 + \text{ThB}_6\text{H}_4\text{C}_6\text{N}$                     | -14.0007            |
| ThNH <sub>4</sub> B <sub>6</sub> C <sub>6</sub> | $2 \text{ ThH}_2 + 3 \text{ B}_{13}\text{C}_2 + 6.25 \text{ Th} + \text{ThN} \rightarrow 8.25 \text{ ThB}_4 + \text{ThB}_6\text{H}_4\text{C}_6\text{N}$                                         | -13.8951            |
| ThNH <sub>4</sub> B <sub>6</sub> C <sub>6</sub> | $1.2 \text{ B}_5\text{H}_7 + 6 \text{ ThC} + 4.567 \text{ N}_2 \rightarrow 1.667 \text{ Th}_3\text{N}_4 + 1.467 \text{ H}_3\text{N} + \text{ThB}_6\text{H}_4\text{C}_6\text{N}$                 | -13.7080            |
| ThNH <sub>4</sub> B <sub>6</sub> C <sub>6</sub> | $2 \text{ ThH}_2 + 1.5 \text{ ThB}_4 + 6 \text{ ThC} + 4.75 \text{ N}_2 \rightarrow 8.5 \text{ ThN} + \text{ThB}_6\text{H}_4\text{C}_6\text{N}$                                                 | -13.4051            |
| ThNH <sub>4</sub> B <sub>6</sub> C <sub>6</sub> | $6 \text{ ThC} + 2 \text{ H}_2 + 4.5 \text{ N}_2 + \text{ThB}_6 \rightarrow 2 \text{ Th}_3\text{N}_4 + \text{ThB}_6\text{H}_4\text{C}_6\text{N}$                                                | -13.4030            |
| ThNH <sub>4</sub> B <sub>6</sub> C <sub>6</sub> | $34.07 \text{ Th}_3\text{N}_4 + 0.2667 \text{ Th}_4\text{H}_{15} + 3 \text{ B}_{13}\text{C}_2 \rightarrow 33 \text{ BN} + 102.3 \text{ ThN} + \text{ThB}_6\text{H}_4\text{C}_6\text{N}$         | -13.3681            |
| ThNH <sub>4</sub> B <sub>6</sub> C <sub>6</sub> | $2 \text{ ThH}_2 + 6 \text{ ThC} + 6 \text{ B} + 4 \text{ N}_2 \rightarrow 7 \text{ ThN} + \text{ThB}_6\text{H}_4\text{C}_6\text{N}$                                                            | -13.3307            |
| ThNH <sub>4</sub> B <sub>6</sub> C <sub>6</sub> | $6 \text{ ThC} + 0.6667 \text{ B}_9\text{H}_{11} + 4.389 \text{ N}_2 \rightarrow 1.667 \text{ Th}_3\text{N}_4 + 1.111 \text{ H}_3\text{N} + \text{ThB}_6\text{H}_4\text{C}_6\text{N}$           | -13.2823            |
| ThNH <sub>4</sub> B <sub>6</sub> C <sub>6</sub> | $1.2 \text{ H}_8\text{C}_5 + 4.98 \text{ N}_2 + 2.493 \text{ ThB}_6 \rightarrow 0.3733 \text{ Th}_4\text{H}_{15} + 8.96 \text{ BN} + \text{ThB}_6\text{H}_4\text{C}_6\text{N}$                  | -13.2104            |
| ThNH <sub>4</sub> B <sub>6</sub> C <sub>6</sub> | $2.313 \text{ Th}_4\text{H}_{15} + 3 \text{ B}_{13}\text{C}_2 + 5.615 \text{ N}_2 \rightarrow 8.25 \text{ ThB}_4 + 10.23 \text{ H}_3\text{N} + \text{ThB}_6\text{H}_4\text{C}_6\text{N}$        | -13.1925            |
| ThNH <sub>4</sub> B <sub>6</sub> C <sub>6</sub> | $4.8 \text{ B}_5\text{H}_7 + 2 \text{ Th}_2\text{C}_3 + 5.433 \text{ N}_2 \rightarrow 9.867 \text{ H}_3\text{N} + 3 \text{ ThB}_6 + \text{ThB}_6\text{H}_4\text{C}_6\text{N}$                   | -13.1271            |
| ThNH <sub>4</sub> B <sub>6</sub> C <sub>6</sub> | $2 \text{ ThH}_2 + 6 \text{ ThC} + 4.5 \text{ N}_2 + \text{ThB}_6 \rightarrow 8 \text{ ThN} + \text{ThB}_6\text{H}_4\text{C}_6\text{N}$                                                         | -13.0917            |
| ThNH <sub>4</sub> B <sub>6</sub> C <sub>6</sub> | $6 \text{ ThC} + 1.273 \text{ B}_9\text{H}_{11} + 3.227 \text{ N}_2 \rightarrow 5 \text{ ThH}_2 + 5.455 \text{ BN} + \text{ThB}_6\text{H}_4\text{C}_6\text{N}$                                  | -13.0513            |
| ThNH <sub>4</sub> B <sub>6</sub> C <sub>6</sub> | $9.25 \text{ ThH}_2 + 3 \text{ B}_{13}\text{C}_2 + 2.917 \text{ N}_2 \rightarrow 8.25 \text{ ThB}_4 + 4.833 \text{ H}_3\text{N} + \text{ThB}_6\text{H}_4\text{C}_6\text{N}$                     | -13.0220            |
| ThNH <sub>4</sub> B <sub>6</sub> C <sub>6</sub> | $6 \text{ ThC} + 2 \text{ H}_2 + 6 \text{ B} + 3.833 \text{ N}_2 \rightarrow 1.667 \text{ Th}_3\text{N}_4 + \text{ThB}_6\text{H}_4\text{C}_6\text{N}$                                           | -13.0200            |
| ThNH <sub>4</sub> B <sub>6</sub> C <sub>6</sub> | $2 \text{ H}_2 + 3 \text{ B}_{13}\text{C}_2 + 6.5 \text{ Th} + 0.5 \text{ N}_2 \rightarrow 5.5 \text{ ThB}_6 + \text{ThB}_6\text{H}_4\text{C}_6\text{N}$                                        | -12.9853            |
| ThNH <sub>4</sub> B <sub>6</sub> C <sub>6</sub> | $2 \text{ ThH}_2 + 6 \text{ ThC} + 34 \text{ B} + 0.5 \text{ N}_2 \rightarrow 7 \text{ ThB}_4 + \text{ThB}_6\text{H}_4\text{C}_6\text{N}$                                                       | -12.9834            |
| ThNH <sub>4</sub> B <sub>6</sub> C <sub>6</sub> | $0.7857 \text{ ThB}_4 + 0.5714 \text{ B}_5\text{H}_7 + 6 \text{ ThC} + 4.357 \text{ N}_2 \rightarrow 1.929 \text{ Th}_3\text{N}_4 + \text{ThB}_6\text{H}_4\text{C}_6\text{N}$                   | -12.9506            |
| ThNH <sub>4</sub> B <sub>6</sub> C <sub>6</sub> | $6 \text{ ThC} + 10.89 \text{ H}_3\text{N} + 2.649 \text{ ThB}_6 \rightarrow 1.912 \text{ Th}_4\text{H}_{15} + 9.895 \text{ BN} + \text{ThB}_6\text{H}_4\text{C}_6\text{N}$                     | -12.9339            |
| ThNH <sub>4</sub> B <sub>6</sub> C <sub>6</sub> | $2 \text{ ThH}_2 + 6 \text{ ThC} + 38 \text{ B} + \text{ThN} \rightarrow 8 \text{ ThB}_4 + \text{ThB}_6\text{H}_4\text{C}_6\text{N}$                                                            | -12.9338            |
| ThNH <sub>4</sub> B <sub>6</sub> C <sub>6</sub> | $\text{B}_{13}\text{C}_2 + 0.5 \text{ Th}_2\text{C}_3 + 0.5 \text{ H}_8\text{C}_5 + 4 \text{ N}_2 \rightarrow 7 \text{ BN} + \text{ThB}_6\text{H}_4\text{C}_6\text{N}$                          | -12.8935            |
| ThNH <sub>4</sub> B <sub>6</sub> C <sub>6</sub> | $17.54 \text{ ThH}_2 + 3 \text{ B}_{13}\text{C}_2 + 0.5 \text{ N}_2 \rightarrow 8.25 \text{ ThB}_4 + 2.071 \text{ Th}_4\text{H}_{15} + \text{ThB}_6\text{H}_4\text{C}_6\text{N}$                | -12.8693            |
| ThNH <sub>4</sub> B <sub>6</sub> C <sub>6</sub> | $19.25 \text{ ThH}_2 + 3 \text{ B}_{13}\text{C}_2 + \text{H}_3\text{N} \rightarrow 8.25 \text{ ThB}_4 + 2.5 \text{ Th}_4\text{H}_{15} + \text{ThB}_6\text{H}_4\text{C}_6\text{N}$               | -12.8377            |
| ThNH <sub>4</sub> B <sub>6</sub> C <sub>6</sub> | $0.6818 \text{ ThB}_4 + 6 \text{ ThC} + 0.3636 \text{ B}_9\text{H}_{11} + 4.288 \text{ N}_2 \rightarrow 1.894 \text{ Th}_3\text{N}_4 + \text{ThB}_6\text{H}_4\text{C}_6\text{N}$                | -12.8185            |
| ThNH <sub>4</sub> B <sub>6</sub> C <sub>6</sub> | $0.5714 \text{ B}_5\text{H}_7 + 6 \text{ ThC} + 4.183 \text{ N}_2 + 0.5238 \text{ ThB}_6 \rightarrow 1.841 \text{ Th}_3\text{N}_4 + \text{ThB}_6\text{H}_4\text{C}_6\text{N}$                   | -12.6235            |
| ThNH <sub>4</sub> B <sub>6</sub> C <sub>6</sub> | $6 \text{ ThC} + 0.2667 \text{ Th}_4\text{H}_{15} + 48.4 \text{ B} + \text{ThN} \rightarrow 7.067 \text{ ThB}_6 + \text{ThB}_6\text{H}_4\text{C}_6\text{N}$                                     | -12.6192            |
| ThNH <sub>4</sub> B <sub>6</sub> C <sub>6</sub> | $6 \text{ ThC} + 0.3636 \text{ B}_9\text{H}_{11} + 4.136 \text{ N}_2 + 0.4545 \text{ ThB}_6 \rightarrow 1.818 \text{ Th}_3\text{N}_4 + \text{ThB}_6\text{H}_4\text{C}_6\text{N}$                | -12.5347            |
| ThNH <sub>4</sub> B <sub>6</sub> C <sub>6</sub> | $2 \text{ ThH}_2 + 0.25 \text{ Th}_3\text{N}_4 + 6 \text{ ThC} + 37 \text{ B} \rightarrow 7.75 \text{ ThB}_4 + \text{ThB}_6\text{H}_4\text{C}_6\text{N}$                                        | -12.4797            |
| ThNH <sub>4</sub> B <sub>6</sub> C <sub>6</sub> | $2 \text{ ThH}_2 + 6 \text{ ThC} + \text{BN} + 47 \text{ B} \rightarrow 7 \text{ ThB}_6 + \text{ThB}_6\text{H}_4\text{C}_6\text{N}$                                                             | -12.4370            |
| ThNH <sub>4</sub> B <sub>6</sub> C <sub>6</sub> | $0.5714 \text{ B}_5\text{H}_7 + 6 \text{ ThC} + 3.143 \text{ B} + 3.833 \text{ N}_2 \rightarrow 1.667 \text{ Th}_3\text{N}_4 + \text{ThB}_6\text{H}_4\text{C}_6\text{N}$                        | -12.4229            |
| ThNH <sub>4</sub> B <sub>6</sub> C <sub>6</sub> | $6 \text{ ThC} + 0.2667 \text{ Th}_4\text{H}_{15} + 42.4 \text{ B} + 0.5 \text{ N}_2 \rightarrow 6.067 \text{ ThB}_6 + \text{ThB}_6\text{H}_4\text{C}_6\text{N}$                                | -12.3802            |
| ThNH <sub>4</sub> B <sub>6</sub> C <sub>6</sub> | $17.33 \text{ Th}_3\text{N}_4 + 19 \text{ B}_9\text{H}_{11} + 3 \text{ B}_{13}\text{C}_2 \rightarrow 51 \text{ ThB}_4 + 68.33 \text{ H}_3\text{N} + \text{ThB}_6\text{H}_4\text{C}_6\text{N}$   | -12.3613            |
| ThNH <sub>4</sub> B <sub>6</sub> C <sub>6</sub> | $6 \text{ ThC} + 0.3636 \text{ B}_9\text{H}_{11} + 2.727 \text{ B} + 3.833 \text{ N}_2 \rightarrow 1.667 \text{ Th}_3\text{N}_4 + \text{ThB}_6\text{H}_4\text{C}_6\text{N}$                     | -12.3606            |
| ThNH <sub>4</sub> B <sub>6</sub> C <sub>6</sub> | $3 \text{ B}_{13}\text{C}_2 + 6.833 \text{ Th} + 1.333 \text{ H}_3\text{N} \rightarrow 5.5 \text{ ThB}_6 + 0.3333 \text{ ThN} + \text{ThB}_6\text{H}_4\text{C}_6\text{N}$                       | -12.2690            |
| ThNH <sub>4</sub> B <sub>6</sub> C <sub>6</sub> | $1.5 \text{ ThB}_4 + 6 \text{ ThC} + 1.333 \text{ H}_3\text{N} + 4.167 \text{ N}_2 \rightarrow 2.167 \text{ Th}_3\text{N}_4 + \text{ThB}_6\text{H}_4\text{C}_6\text{N}$                         | -12.2620            |
| ThNH <sub>4</sub> B <sub>6</sub> C <sub>6</sub> | $\text{BN} + 0.3636 \text{ B}_9\text{H}_{11} + 3 \text{ B}_{13}\text{C}_2 + 7.212 \text{ Th} \rightarrow 6.212 \text{ ThB}_6 + \text{ThB}_6\text{H}_4\text{C}_6\text{N}$                        | -12.1707            |
| ThNH <sub>4</sub> B <sub>6</sub> C <sub>6</sub> | $3 \text{ B}_{13}\text{C}_2 + 6.75 \text{ Th} + 1.333 \text{ H}_3\text{N} \rightarrow 0.08333 \text{ Th}_3\text{N}_4 + 5.5 \text{ ThB}_6 + \text{ThB}_6\text{H}_4\text{C}_6\text{N}$            | -12.1622            |
| ThNH <sub>4</sub> B <sub>6</sub> C <sub>6</sub> | $0.25 \text{ Th}_3\text{N}_4 + 6 \text{ ThC} + 0.2667 \text{ Th}_4\text{H}_{15} + 46.9 \text{ B} \rightarrow 6.817 \text{ ThB}_6 + \text{ThB}_6\text{H}_4\text{C}_6\text{N}$                    | -12.0930            |
| ThNH <sub>4</sub> B <sub>6</sub> C <sub>6</sub> | $0.5714 \text{ B}_5\text{H}_7 + \text{BN} + 3 \text{ B}_{13}\text{C}_2 + 7.143 \text{ Th} \rightarrow 6.143 \text{ ThB}_6 + \text{ThB}_6\text{H}_4\text{C}_6\text{N}$                           | -11.9984            |
| ThNH <sub>4</sub> B <sub>6</sub> C <sub>6</sub> | $6 \text{ ThC} + 12.58 \text{ B} + 7.583 \text{ H}_3\text{N} \rightarrow 1.25 \text{ Th}_4\text{H}_{15} + 6.583 \text{ BN} + \text{ThB}_6\text{H}_4\text{C}_6\text{N}$                          | -11.9855            |
| ThNH <sub>4</sub> B <sub>6</sub> C <sub>6</sub> | $0.09091 \text{ B}_9\text{H}_{11} + 3 \text{ B}_{13}\text{C}_2 + 6.636 \text{ Th} + \text{H}_3\text{N} \rightarrow 5.636 \text{ ThB}_6 + \text{ThB}_6\text{H}_4\text{C}_6\text{N}$              | -11.9581            |
| ThNH <sub>4</sub> B <sub>6</sub> C <sub>6</sub> | $6 \text{ ThC} + 2.75 \text{ B}_9\text{H}_{11} + 3.833 \text{ N}_2 \rightarrow 3.75 \text{ B}_5\text{H}_7 + 1.667 \text{ Th}_3\text{N}_4 + \text{ThB}_6\text{H}_4\text{C}_6\text{N}$            | -11.9520            |
| ThNH <sub>4</sub> B <sub>6</sub> C <sub>6</sub> | $0.1429 \text{ B}_5\text{H}_7 + 3 \text{ B}_{13}\text{C}_2 + 6.619 \text{ Th} + \text{H}_3\text{N} \rightarrow 5.619 \text{ ThB}_6 + \text{ThB}_6\text{H}_4\text{C}_6\text{N}$                  | -11.9151            |
| ThNH <sub>4</sub> B <sub>6</sub> C <sub>6</sub> | $2 \text{ ThH}_2 + 1.5 \text{ ThB}_4 + 2 \text{ Th}_2\text{C}_3 + 4.833 \text{ N}_2 \rightarrow 2.167 \text{ Th}_3\text{N}_4 + \text{ThB}_6\text{H}_4\text{C}_6\text{N}$                        | -11.8999            |
| ThNH <sub>4</sub> B <sub>6</sub> C <sub>6</sub> | $3 \text{ B}_{13}\text{C}_2 + 6.444 \text{ Th} + 1.333 \text{ H}_3\text{N} \rightarrow 0.3333 \text{ BN} + 5.444 \text{ ThB}_6 + \text{ThB}_6\text{H}_4\text{C}_6\text{N}$                      | -11.8873            |
| ThNH <sub>4</sub> B <sub>6</sub> C <sub>6</sub> | $6 \text{ ThC} + 0.6667 \text{ B}_9\text{H}_{11} + 3.833 \text{ N}_2 \rightarrow 1.667 \text{ Th}_3\text{N}_4 + 1.667 \text{ H}_2 + \text{ThB}_6\text{H}_4\text{C}_6\text{N}$                   | -11.8111            |
| ThNH <sub>4</sub> B <sub>6</sub> C <sub>6</sub> | $2.179 \text{ B}_5\text{H}_7 + 2 \text{ Th}_2\text{C}_3 + 2.946 \text{ N}_2 \rightarrow 0.75 \text{ Th}_4\text{H}_{15} + 4.893 \text{ BN} + \text{ThB}_6\text{H}_4\text{C}_6\text{N}$           | -11.7752            |
| ThNH <sub>4</sub> B <sub>6</sub> C <sub>6</sub> | $1.2 \text{ B}_5\text{H}_7 + 6 \text{ ThC} + 3.833 \text{ N}_2 \rightarrow 1.667 \text{ Th}_3\text{N}_4 + 2.2 \text{ H}_2 + \text{ThB}_6\text{H}_4\text{C}_6\text{N}$                           | -11.7660            |
| ThNH <sub>4</sub> B <sub>6</sub> C <sub>6</sub> | $1.2 \text{ B}_5\text{H}_7 + 2.917 \text{ Th}_2\text{C}_3 + 3.722 \text{ N}_2 \rightarrow 1.611 \text{ Th}_3\text{N}_4 + 0.55 \text{ H}_8\text{C}_5 + \text{ThB}_6\text{H}_4\text{C}_6\text{N}$ | -11.6719            |
| ThNH <sub>4</sub> B <sub>6</sub> C <sub>6</sub> | $0.5 \text{ H}_2 + 3 \text{ B}_{13}\text{C}_2 + 6.5 \text{ Th} + \text{H}_3\text{N} \rightarrow 5.5 \text{ ThB}_6 + \text{ThB}_6\text{H}_4\text{C}_6\text{N}$                                   | -11.6612            |
| ThNH <sub>4</sub> B <sub>6</sub> C <sub>6</sub> | $6 \text{ ThC} + 1.333 \text{ H}_3\text{N} + 3.833 \text{ N}_2 + \text{ThB}_6 \rightarrow 2 \text{ Th}_3\text{N}_4 + \text{ThB}_6\text{H}_4\text{C}_6\text{N}$                                  | -11.6376            |
| ThNH <sub>4</sub> B <sub>6</sub> C <sub>6</sub> | $2.667 \text{ B}_9\text{H}_{11} + 2 \text{ Th}_2\text{C}_3 + 4.722 \text{ N}_2 \rightarrow 8.444 \text{ H}_3\text{N} + 3 \text{ ThB}_6 + \text{ThB}_6\text{H}_4\text{C}_6\text{N}$              | -11.4243            |
| ThNH <sub>4</sub> B <sub>6</sub> C <sub>6</sub> | $0.25 \text{ Th}_3\text{N}_4 + 0.3636 \text{ B}_9\text{H}_{11} + 3 \text{ B}_{13}\text{C}_2 + 6.295 \text{ Th} \rightarrow 6.045 \text{ ThB}_6 + \text{ThB}_6\text{H}_4\text{C}_6\text{N}$      | -11.3459            |
| ThNH <sub>4</sub> B <sub>6</sub> C <sub>6</sub> | $6 \text{ ThC} + 2 \text{ H}_2 + 42 \text{ B} + \text{ThN} \rightarrow 6 \text{ ThB}_6 + \text{ThB}_6\text{H}_4\text{C}_6\text{N}$                                                              | -11.3442            |
| ThNH <sub>4</sub> B <sub>6</sub> C <sub>6</sub> | $2 \text{ ThH}_2 + 2 \text{ Th}_2\text{C}_3 + 4.5 \text{ N}_2 + \text{ThB}_6 \rightarrow 2 \text{ Th}_3\text{N}_4 + \text{ThB}_6\text{H}_4\text{C}_6\text{N}$                                   | -11.2754            |
| ThNH <sub>4</sub> B <sub>6</sub> C <sub>6</sub> | $6 \text{ ThC} + 6 \text{ B} + 1.333 \text{ H}_3\text{N} + 3.167 \text{ N}_2 \rightarrow 1.667 \text{ Th}_3\text{N}_4 + \text{ThB}_6\text{H}_4\text{C}_6\text{N}$                               | -11.2546            |

Continued on next page

Continued

| Compound                                        | Chemical reaction                                                                                                                                                                                                                    | Reaction energy(eV) |
|-------------------------------------------------|--------------------------------------------------------------------------------------------------------------------------------------------------------------------------------------------------------------------------------------|---------------------|
| ThNH <sub>4</sub> B <sub>6</sub> C <sub>6</sub> | 5.077 ThC + 0.2667 Th <sub>4</sub> H <sub>15</sub> + 0.4615 B <sub>13</sub> C <sub>2</sub> + 3.929 N <sub>2</sub> → 1.715 Th <sub>3</sub> N <sub>4</sub> + ThB <sub>6</sub> H <sub>4</sub> C <sub>6</sub> N                          | -11.2527            |
| ThNH <sub>4</sub> B <sub>6</sub> C <sub>6</sub> | 3.8 ThB <sub>4</sub> + 1.2 H <sub>8</sub> C <sub>5</sub> + 5.1 N <sub>2</sub> → 2.8 ThH <sub>2</sub> + 9.2 BN + ThB <sub>6</sub> H <sub>4</sub> C <sub>6</sub> N                                                                     | -11.2503            |
| ThNH <sub>4</sub> B <sub>6</sub> C <sub>6</sub> | 3 B <sub>13</sub> C <sub>2</sub> + 6.5 Th + 1.333 H <sub>3</sub> N → 0.1667 N <sub>2</sub> + 5.5 ThB <sub>6</sub> + ThB <sub>6</sub> H <sub>4</sub> C <sub>6</sub> N                                                                 | -11.2198            |
| ThNH <sub>4</sub> B <sub>6</sub> C <sub>6</sub> | 0.5714 B <sub>5</sub> H <sub>7</sub> + 0.25 Th <sub>3</sub> N <sub>4</sub> + 3 B <sub>13</sub> C <sub>2</sub> + 6.226 Th → 5.976 ThB <sub>6</sub> + ThB <sub>6</sub> H <sub>4</sub> C <sub>6</sub> N                                 | -11.1736            |
| ThNH <sub>4</sub> B <sub>6</sub> C <sub>6</sub> | 6 ThC + 2 H <sub>2</sub> + 36 B + 0.5 N <sub>2</sub> → 5 ThB <sub>6</sub> + ThB <sub>6</sub> H <sub>4</sub> C <sub>6</sub> N                                                                                                         | -11.1052            |
| ThNH <sub>4</sub> B <sub>6</sub> C <sub>6</sub> | 0.06667 Th <sub>4</sub> H <sub>15</sub> + 3 B <sub>13</sub> C <sub>2</sub> + 6.233 Th + H <sub>3</sub> N → 5.5 ThB <sub>6</sub> + ThB <sub>6</sub> H <sub>4</sub> C <sub>6</sub> N                                                   | -11.0769            |
| ThNH <sub>4</sub> B <sub>6</sub> C <sub>6</sub> | 0.3636 B <sub>9</sub> H <sub>11</sub> + 3 B <sub>13</sub> C <sub>2</sub> + 6.045 Th + ThN → 6.045 ThB <sub>6</sub> + ThB <sub>6</sub> H <sub>4</sub> C <sub>6</sub> N                                                                | -11.0255            |
| ThNH <sub>4</sub> B <sub>6</sub> C <sub>6</sub> | 3 B <sub>13</sub> C <sub>2</sub> + Th + 11.73 H <sub>3</sub> N → 4.455 B <sub>5</sub> H <sub>7</sub> + 10.73 BN + ThB <sub>6</sub> H <sub>4</sub> C <sub>6</sub> N                                                                   | -11.0209            |
| ThNH <sub>4</sub> B <sub>6</sub> C <sub>6</sub> | 1.5 ThB <sub>4</sub> + 6 ThC + 0.2667 Th <sub>4</sub> H <sub>15</sub> + 4.283 N <sub>2</sub> → 7.567 ThN + ThB <sub>6</sub> H <sub>4</sub> C <sub>6</sub> N                                                                          | -11.0046            |
| ThNH <sub>4</sub> B <sub>6</sub> C <sub>6</sub> | 2 H <sub>2</sub> + BN + 3 B <sub>13</sub> C <sub>2</sub> + 6.667 Th → 5.667 ThB <sub>6</sub> + ThB <sub>6</sub> H <sub>4</sub> C <sub>6</sub> N                                                                                      | -10.9829            |
| ThNH <sub>4</sub> B <sub>6</sub> C <sub>6</sub> | 0.5 ThH <sub>2</sub> + 3 B <sub>13</sub> C <sub>2</sub> + 6 Th + H <sub>3</sub> N → 5.5 ThB <sub>6</sub> + ThB <sub>6</sub> H <sub>4</sub> C <sub>6</sub> N                                                                          | -10.9426            |
| ThNH <sub>4</sub> B <sub>6</sub> C <sub>6</sub> | 18.07 ThH <sub>2</sub> + BN + 3 B <sub>13</sub> C <sub>2</sub> → 8.5 ThB <sub>4</sub> + 2.143 Th <sub>4</sub> H <sub>15</sub> + ThB <sub>6</sub> H <sub>4</sub> C <sub>6</sub> N                                                     | -10.9331            |
| ThNH <sub>4</sub> B <sub>6</sub> C <sub>6</sub> | 6 ThC + 0.2667 Th <sub>4</sub> H <sub>15</sub> + 6 B + 3.533 N <sub>2</sub> → 6.067 ThN + ThB <sub>6</sub> H <sub>4</sub> C <sub>6</sub> N                                                                                           | -10.9302            |
| ThNH <sub>4</sub> B <sub>6</sub> C <sub>6</sub> | 3.347 Th <sub>4</sub> H <sub>15</sub> + 3 B <sub>13</sub> C <sub>2</sub> + 6.693 N <sub>2</sub> → 6.6 B <sub>5</sub> H <sub>7</sub> + 12.39 ThN + ThB <sub>6</sub> H <sub>4</sub> C <sub>6</sub> N                                   | -10.9108            |
| ThNH <sub>4</sub> B <sub>6</sub> C <sub>6</sub> | 2 ThH <sub>2</sub> + 2 Th <sub>2</sub> C <sub>3</sub> + 6 B + 3.833 N <sub>2</sub> → 1.667 Th <sub>3</sub> N <sub>4</sub> + ThB <sub>6</sub> H <sub>4</sub> C <sub>6</sub> N                                                         | -10.8925            |
| ThNH <sub>4</sub> B <sub>6</sub> C <sub>6</sub> | 3 B <sub>13</sub> C <sub>2</sub> + 13.64 H <sub>3</sub> N + ThB <sub>6</sub> → 5.273 B <sub>5</sub> H <sub>7</sub> + 12.64 BN + ThB <sub>6</sub> H <sub>4</sub> C <sub>6</sub> N                                                     | -10.8618            |
| ThNH <sub>4</sub> B <sub>6</sub> C <sub>6</sub> | 0.5714 B <sub>5</sub> H <sub>7</sub> + 3 B <sub>13</sub> C <sub>2</sub> + 5.976 Th + ThN → 5.976 ThB <sub>6</sub> + ThB <sub>6</sub> H <sub>4</sub> C <sub>6</sub> N                                                                 | -10.8532            |
| ThNH <sub>4</sub> B <sub>6</sub> C <sub>6</sub> | 0.25 Th <sub>3</sub> N <sub>4</sub> + 6 ThC + 2 H <sub>2</sub> + 40.5 B → 5.75 ThB <sub>6</sub> + ThB <sub>6</sub> H <sub>4</sub> C <sub>6</sub> N                                                                                   | -10.8179            |
| ThNH <sub>4</sub> B <sub>6</sub> C <sub>6</sub> | 5.58 ThC + 0.3636 B <sub>9</sub> H <sub>11</sub> + 0.2098 B <sub>13</sub> C <sub>2</sub> + 3.554 N <sub>2</sub> → 1.527 Th <sub>3</sub> N <sub>4</sub> + ThB <sub>6</sub> H <sub>4</sub> C <sub>6</sub> N                            | -10.7920            |
| ThNH <sub>4</sub> B <sub>6</sub> C <sub>6</sub> | 0.5 ThH <sub>2</sub> + 6 ThC + 39 B + H <sub>3</sub> N → 5.5 ThB <sub>6</sub> + ThB <sub>6</sub> H <sub>4</sub> C <sub>6</sub> N                                                                                                     | -10.7557            |
| ThNH <sub>4</sub> B <sub>6</sub> C <sub>6</sub> | 0.5714 B <sub>5</sub> H <sub>7</sub> + 6 ThC + 39.14 B + ThN → 6 ThB <sub>6</sub> + ThB <sub>6</sub> H <sub>4</sub> C <sub>6</sub> N                                                                                                 | -10.7470            |
| ThNH <sub>4</sub> B <sub>6</sub> C <sub>6</sub> | 6 ThC + 0.2667 Th <sub>4</sub> H <sub>15</sub> + 4.033 N <sub>2</sub> + ThB <sub>6</sub> → 7.067 ThN + ThB <sub>6</sub> H <sub>4</sub> C <sub>6</sub> N                                                                              | -10.6912            |
| ThNH <sub>4</sub> B <sub>6</sub> C <sub>6</sub> | 6 ThC + 0.3636 B <sub>9</sub> H <sub>11</sub> + 38.73 B + ThN → 6 ThB <sub>6</sub> + ThB <sub>6</sub> H <sub>4</sub> C <sub>6</sub> N                                                                                                | -10.6848            |
| ThNH <sub>4</sub> B <sub>6</sub> C <sub>6</sub> | 0.2667 Th <sub>4</sub> H <sub>15</sub> + 3 B <sub>13</sub> C <sub>2</sub> + 5.433 Th + 0.5 N <sub>2</sub> → 5.5 ThB <sub>6</sub> + ThB <sub>6</sub> H <sub>4</sub> C <sub>6</sub> N                                                  | -10.6480            |
| ThNH <sub>4</sub> B <sub>6</sub> C <sub>6</sub> | 6 ThC + 0.2667 Th <sub>4</sub> H <sub>15</sub> + 30.27 B + 0.5 N <sub>2</sub> → 6.067 ThB <sub>4</sub> + ThB <sub>6</sub> H <sub>4</sub> C <sub>6</sub> N                                                                            | -10.6292            |
| ThNH <sub>4</sub> B <sub>6</sub> C <sub>6</sub> | 0.5714 B <sub>5</sub> H <sub>7</sub> + 5.516 ThC + 0.2418 B <sub>13</sub> C <sub>2</sub> + 3.511 N <sub>2</sub> → 1.505 Th <sub>3</sub> N <sub>4</sub> + ThB <sub>6</sub> H <sub>4</sub> C <sub>6</sub> N                            | -10.6153            |
| ThNH <sub>4</sub> B <sub>6</sub> C <sub>6</sub> | 1.2 B <sub>5</sub> H <sub>7</sub> + 6 ThC + 3.733 N <sub>2</sub> → 1.467 H <sub>3</sub> N + 5 ThN + ThB <sub>6</sub> H <sub>4</sub> C <sub>6</sub> N                                                                                 | -10.5981            |
| ThNH <sub>4</sub> B <sub>6</sub> C <sub>6</sub> | 6 ThC + 0.2667 Th <sub>4</sub> H <sub>15</sub> + 34.27 B + ThN → 7.067 ThB <sub>4</sub> + ThB <sub>6</sub> H <sub>4</sub> C <sub>6</sub> N                                                                                           | -10.5796            |
| ThNH <sub>4</sub> B <sub>6</sub> C <sub>6</sub> | 0.5714 B <sub>5</sub> H <sub>7</sub> + 6 ThC + 33.14 B + 0.5 N <sub>2</sub> → 5 ThB <sub>6</sub> + ThB <sub>6</sub> H <sub>4</sub> C <sub>6</sub> N                                                                                  | -10.5080            |
| ThNH <sub>4</sub> B <sub>6</sub> C <sub>6</sub> | 15.93 ThH <sub>2</sub> + 0.25 Th <sub>3</sub> N <sub>4</sub> + 3 B <sub>13</sub> C <sub>2</sub> → 8.25 ThB <sub>4</sub> + 1.857 Th <sub>4</sub> H <sub>15</sub> + ThB <sub>6</sub> H <sub>4</sub> C <sub>6</sub> N                   | -10.4739            |
| ThNH <sub>4</sub> B <sub>6</sub> C <sub>6</sub> | 2 ThH <sub>2</sub> + 5.077 ThC + 0.4615 B <sub>13</sub> C <sub>2</sub> + 3.538 N <sub>2</sub> → 6.077 ThN + ThB <sub>6</sub> H <sub>4</sub> C <sub>6</sub> N                                                                         | -10.4540            |
| ThNH <sub>4</sub> B <sub>6</sub> C <sub>6</sub> | 6 ThC + 0.3636 B <sub>9</sub> H <sub>11</sub> + 32.73 B + 0.5 N <sub>2</sub> → 5 ThB <sub>6</sub> + ThB <sub>6</sub> H <sub>4</sub> C <sub>6</sub> N                                                                                 | -10.4457            |
| ThNH <sub>4</sub> B <sub>6</sub> C <sub>6</sub> | 2 ThH <sub>2</sub> + 6 ThC + BN + 33 B → 7 ThB <sub>4</sub> + ThB <sub>6</sub> H <sub>4</sub> C <sub>6</sub> N                                                                                                                       | -10.4166            |
| ThNH <sub>4</sub> B <sub>6</sub> C <sub>6</sub> | 6 ThC + 0.6667 B <sub>9</sub> H <sub>11</sub> + 3.241 N <sub>2</sub> → 1.37 Th <sub>3</sub> N <sub>4</sub> + 0.2222 Th <sub>4</sub> H <sub>15</sub> + ThB <sub>6</sub> H <sub>4</sub> C <sub>6</sub> N                               | -10.4081            |
| ThNH <sub>4</sub> B <sub>6</sub> C <sub>6</sub> | 15.39 ThH <sub>2</sub> + 3 B <sub>13</sub> C <sub>2</sub> + ThN → 8.25 ThB <sub>4</sub> + 1.786 Th <sub>4</sub> H <sub>15</sub> + ThB <sub>6</sub> H <sub>4</sub> C <sub>6</sub> N                                                   | -10.2974            |
| ThNH <sub>4</sub> B <sub>6</sub> C <sub>6</sub> | 0.5714 B <sub>5</sub> H <sub>7</sub> + 0.25 Th <sub>3</sub> N <sub>4</sub> + 6 ThC + 37.64 B → 5.75 ThB <sub>6</sub> + ThB <sub>6</sub> H <sub>4</sub> C <sub>6</sub> N                                                              | -10.2208            |
| ThNH <sub>4</sub> B <sub>6</sub> C <sub>6</sub> | 6 ThC + 36.33 B + 1.333 H <sub>3</sub> N → 0.3333 BN + 5 ThB <sub>6</sub> + ThB <sub>6</sub> H <sub>4</sub> C <sub>6</sub> N                                                                                                         | -10.1953            |
| ThNH <sub>4</sub> B <sub>6</sub> C <sub>6</sub> | 6 ThC + 0.6667 B <sub>9</sub> H <sub>11</sub> + 3.556 N <sub>2</sub> → 1.111 H <sub>3</sub> N + 5 ThN + ThB <sub>6</sub> H <sub>4</sub> C <sub>6</sub> N                                                                             | -10.1724            |
| ThNH <sub>4</sub> B <sub>6</sub> C <sub>6</sub> | 0.25 Th <sub>3</sub> N <sub>4</sub> + 6 ThC + 0.3636 B <sub>9</sub> H <sub>11</sub> + 37.23 B → 5.75 ThB <sub>6</sub> + ThB <sub>6</sub> H <sub>4</sub> C <sub>6</sub> N                                                             | -10.1585            |
| ThNH <sub>4</sub> B <sub>6</sub> C <sub>6</sub> | 0.25 Th <sub>3</sub> N <sub>4</sub> + 2 H <sub>2</sub> + 3 B <sub>13</sub> C <sub>2</sub> + 5.75 Th → 5.5 ThB <sub>6</sub> + ThB <sub>6</sub> H <sub>4</sub> C <sub>6</sub> N                                                        | -10.1581            |
| ThNH <sub>4</sub> B <sub>6</sub> C <sub>6</sub> | 0.25 Th <sub>3</sub> N <sub>4</sub> + 6 ThC + 0.2667 Th <sub>4</sub> H <sub>15</sub> + 33.27 B → 6.817 ThB <sub>4</sub> + ThB <sub>6</sub> H <sub>4</sub> C <sub>6</sub> N                                                           | -10.1255            |
| ThNH <sub>4</sub> B <sub>6</sub> C <sub>6</sub> | 2 ThH <sub>2</sub> + 3 B <sub>13</sub> C <sub>2</sub> + 4.5 Th + 0.5 N <sub>2</sub> → 5.5 ThB <sub>6</sub> + ThB <sub>6</sub> H <sub>4</sub> C <sub>6</sub> N                                                                        | -10.1107            |
| ThNH <sub>4</sub> B <sub>6</sub> C <sub>6</sub> | 6 ThC + 0.06667 Th <sub>4</sub> H <sub>15</sub> + 37.6 B + H <sub>3</sub> N → 5.267 ThB <sub>6</sub> + ThB <sub>6</sub> H <sub>4</sub> C <sub>6</sub> N                                                                              | -10.0999            |
| ThNH <sub>4</sub> B <sub>6</sub> C <sub>6</sub> | 0.6667 B <sub>9</sub> H <sub>11</sub> + 2.694 Th <sub>2</sub> C <sub>3</sub> + 3.426 N <sub>2</sub> → 1.463 Th <sub>3</sub> N <sub>4</sub> + 0.4167 H <sub>8</sub> C <sub>5</sub> + ThB <sub>6</sub> H <sub>4</sub> C <sub>6</sub> N | -10.0932            |
| ThNH <sub>4</sub> B <sub>6</sub> C <sub>6</sub> | ThB <sub>4</sub> + 3 B <sub>13</sub> C <sub>2</sub> + 13 H <sub>3</sub> N → 5 B <sub>5</sub> H <sub>7</sub> + 12 BN + ThB <sub>6</sub> H <sub>4</sub> C <sub>6</sub> N                                                               | -10.0746            |
| ThNH <sub>4</sub> B <sub>6</sub> C <sub>6</sub> | 1.5 ThB <sub>4</sub> + 6 ThC + 2 H <sub>2</sub> + 3.75 N <sub>2</sub> → 6.5 ThN + ThB <sub>6</sub> H <sub>4</sub> C <sub>6</sub> N                                                                                                   | -9.9845             |
| ThNH <sub>4</sub> B <sub>6</sub> C <sub>6</sub> | 0.3333 Th <sub>3</sub> N <sub>4</sub> + 3 B <sub>13</sub> C <sub>2</sub> + 11.3 H <sub>3</sub> N → 4.273 B <sub>5</sub> H <sub>7</sub> + 11.64 BN + ThB <sub>6</sub> H <sub>4</sub> C <sub>6</sub> N                                 | -9.9565             |
| ThNH <sub>4</sub> B <sub>6</sub> C <sub>6</sub> | 1.2 B <sub>5</sub> H <sub>7</sub> + 6 ThC + 3.051 N <sub>2</sub> → 1.276 Th <sub>3</sub> N <sub>4</sub> + 0.2933 Th <sub>4</sub> H <sub>15</sub> + ThB <sub>6</sub> H <sub>4</sub> C <sub>6</sub> N                                  | -9.9141             |
| ThNH <sub>4</sub> B <sub>6</sub> C <sub>6</sub> | 6 ThC + 2 H <sub>2</sub> + 6 B + 3 N <sub>2</sub> → 5 ThN + ThB <sub>6</sub> H <sub>4</sub> C <sub>6</sub> N                                                                                                                         | -9.9101             |
| ThNH <sub>4</sub> B <sub>6</sub> C <sub>6</sub> | 3 B <sub>13</sub> C <sub>2</sub> + 11.41 H <sub>3</sub> N + ThN → 4.318 B <sub>5</sub> H <sub>7</sub> + 11.41 BN + ThB <sub>6</sub> H <sub>4</sub> C <sub>6</sub> N                                                                  | -9.9022             |
| ThNH <sub>4</sub> B <sub>6</sub> C <sub>6</sub> | 3 B <sub>13</sub> C <sub>2</sub> + Th + 10.79 H <sub>3</sub> N → 9.789 BN + 2.579 B <sub>9</sub> H <sub>11</sub> + ThB <sub>6</sub> H <sub>4</sub> C <sub>6</sub> N                                                                  | -9.8771             |
| ThNH <sub>4</sub> B <sub>6</sub> C <sub>6</sub> | 2 H <sub>2</sub> + 3 B <sub>13</sub> C <sub>2</sub> + 5.5 Th + ThN → 5.5 ThB <sub>6</sub> + ThB <sub>6</sub> H <sub>4</sub> C <sub>6</sub> N                                                                                         | -9.8377             |
| ThNH <sub>4</sub> B <sub>6</sub> C <sub>6</sub> | 6 ThC + 0.2667 Th <sub>4</sub> H <sub>15</sub> + BN + 41.4 B → 6.067 ThB <sub>6</sub> + ThB <sub>6</sub> H <sub>4</sub> C <sub>6</sub> N                                                                                             | -9.8134             |
| ThNH <sub>4</sub> B <sub>6</sub> C <sub>6</sub> | 3.6 B <sub>5</sub> H <sub>7</sub> + 2 Th <sub>2</sub> C <sub>3</sub> + 4.033 N <sub>2</sub> → 3 ThB <sub>4</sub> + 7.067 H <sub>3</sub> N + ThB <sub>6</sub> H <sub>4</sub> C <sub>6</sub> N                                         | -9.8078             |
| ThNH <sub>4</sub> B <sub>6</sub> C <sub>6</sub> | 6 ThC + 0.5 H <sub>2</sub> + 36 B + H <sub>3</sub> N → 5 ThB <sub>6</sub> + ThB <sub>6</sub> H <sub>4</sub> C <sub>6</sub> N                                                                                                         | -9.7811             |
| ThNH <sub>4</sub> B <sub>6</sub> C <sub>6</sub> | 6 ThC + 2 H <sub>2</sub> + 3.5 N <sub>2</sub> + ThB <sub>6</sub> → 6 ThN + ThB <sub>6</sub> H <sub>4</sub> C <sub>6</sub> N                                                                                                          | -9.6711             |
| ThNH <sub>4</sub> B <sub>6</sub> C <sub>6</sub> | 6 ThC + 2 H <sub>2</sub> + 26 B + 0.5 N <sub>2</sub> → 5 ThB <sub>4</sub> + ThB <sub>6</sub> H <sub>4</sub> C <sub>6</sub> N                                                                                                         | -9.6621             |
| ThNH <sub>4</sub> B <sub>6</sub> C <sub>6</sub> | 0.1429 B <sub>5</sub> H <sub>7</sub> + 6 ThC + 35.29 B + H <sub>3</sub> N → 5 ThB <sub>6</sub> + ThB <sub>6</sub> H <sub>4</sub> C <sub>6</sub> N                                                                                    | -9.6318             |
| ThNH <sub>4</sub> B <sub>6</sub> C <sub>6</sub> | 6 ThC + 0.09091 B <sub>9</sub> H <sub>11</sub> + 35.18 B + H <sub>3</sub> N → 5 ThB <sub>6</sub> + ThB <sub>6</sub> H <sub>4</sub> C <sub>6</sub> N                                                                                  | -9.6162             |
| ThNH <sub>4</sub> B <sub>6</sub> C <sub>6</sub> | 6 ThC + 2 H <sub>2</sub> + 30 B + ThN → 6 ThB <sub>4</sub> + ThB <sub>6</sub> H <sub>4</sub> C <sub>6</sub> N                                                                                                                        | -9.6125             |

Continued on next page

Continued

| Compound                                        | Chemical reaction                                                                                                                                                                                                  | Reaction energy(eV) |
|-------------------------------------------------|--------------------------------------------------------------------------------------------------------------------------------------------------------------------------------------------------------------------|---------------------|
| ThNH <sub>4</sub> B <sub>6</sub> C <sub>6</sub> | 5.077 ThC + 2 H <sub>2</sub> + 0.4615 B <sub>13</sub> C <sub>2</sub> + 3.218 N <sub>2</sub> → 1.359 Th <sub>3</sub> N <sub>4</sub> + ThB <sub>6</sub> H <sub>4</sub> C <sub>6</sub> N                              | -9.5692             |
| ThNH <sub>4</sub> B <sub>6</sub> C <sub>6</sub> | 2 B <sub>5</sub> H <sub>7</sub> + 6 ThC + 2.5 N <sub>2</sub> → 5 ThH <sub>2</sub> + 4 BN + ThB <sub>6</sub> H <sub>4</sub> C <sub>6</sub> N                                                                        | -9.5358             |
| ThNH <sub>4</sub> B <sub>6</sub> C <sub>6</sub> | 3 B <sub>13</sub> C <sub>2</sub> + 12.53 H <sub>3</sub> N + ThB <sub>6</sub> → 11.53 BN + 3.053 B <sub>9</sub> H <sub>11</sub> + ThB <sub>6</sub> H <sub>4</sub> C <sub>6</sub> N                                  | -9.5079             |
| ThNH <sub>4</sub> B <sub>6</sub> C <sub>6</sub> | 2.687 B <sub>13</sub> C <sub>2</sub> + 5.823 Th + H <sub>3</sub> N + 0.125 H <sub>8</sub> C <sub>5</sub> → 4.823 ThB <sub>6</sub> + ThB <sub>6</sub> H <sub>4</sub> C <sub>6</sub> N                               | -9.4749             |
| ThNH <sub>4</sub> B <sub>6</sub> C <sub>6</sub> | 6 ThC + 34.5 B + 1.333 H <sub>3</sub> N → 0.08333 Th <sub>3</sub> N <sub>4</sub> + 4.75 ThB <sub>6</sub> + ThB <sub>6</sub> H <sub>4</sub> C <sub>6</sub> N                                                        | -9.4355             |
| ThNH <sub>4</sub> B <sub>6</sub> C <sub>6</sub> | 0.7857 ThB <sub>4</sub> + 0.5714 B <sub>5</sub> H <sub>7</sub> + 6 ThC + 3.393 N <sub>2</sub> → 5.786 ThN + ThB <sub>6</sub> H <sub>4</sub> C <sub>6</sub> N                                                       | -9.3519             |
| ThNH <sub>4</sub> B <sub>6</sub> C <sub>6</sub> | 6 ThC + 36 B + 1.333 H <sub>3</sub> N → 0.1667 N <sub>2</sub> + 5 ThB <sub>6</sub> + ThB <sub>6</sub> H <sub>4</sub> C <sub>6</sub> N                                                                              | -9.3397             |
| ThNH <sub>4</sub> B <sub>6</sub> C <sub>6</sub> | 2.58 Th <sub>3</sub> N <sub>4</sub> + 0.3636 B <sub>9</sub> H <sub>11</sub> + 3 B <sub>13</sub> C <sub>2</sub> → 6.739 ThB <sub>4</sub> + 9.318 BN + ThB <sub>6</sub> H <sub>4</sub> C <sub>6</sub> N              | -9.3221             |
| ThNH <sub>4</sub> B <sub>6</sub> C <sub>6</sub> | 0.5714 B <sub>5</sub> H <sub>7</sub> + 6 ThC + 3.143 B + 3 N <sub>2</sub> → 5 ThN + ThB <sub>6</sub> H <sub>4</sub> C <sub>6</sub> N                                                                               | -9.3130             |
| ThNH <sub>4</sub> B <sub>6</sub> C <sub>6</sub> | 0.6818 ThB <sub>4</sub> + 6 ThC + 0.3636 B <sub>9</sub> H <sub>11</sub> + 3.341 N <sub>2</sub> → 5.682 ThN + ThB <sub>6</sub> H <sub>4</sub> C <sub>6</sub> N                                                      | -9.2845             |
| ThNH <sub>4</sub> B <sub>6</sub> C <sub>6</sub> | 2.292 Th <sub>3</sub> N <sub>4</sub> + 3 B <sub>13</sub> C <sub>2</sub> + 1.333 H <sub>3</sub> N → 5.875 ThB <sub>4</sub> + 9.5 BN + ThB <sub>6</sub> H <sub>4</sub> C <sub>6</sub> N                              | -9.2628             |
| ThNH <sub>4</sub> B <sub>6</sub> C <sub>6</sub> | 6 ThC + 34 B + 1.333 H <sub>3</sub> N → 4.667 ThB <sub>6</sub> + 0.3333 ThN + ThB <sub>6</sub> H <sub>4</sub> C <sub>6</sub> N                                                                                     | -9.2601             |
| ThNH <sub>4</sub> B <sub>6</sub> C <sub>6</sub> | 6 ThC + 0.3636 B <sub>9</sub> H <sub>11</sub> + 2.727 B + 3 N <sub>2</sub> → 5 ThN + ThB <sub>6</sub> H <sub>4</sub> C <sub>6</sub> N                                                                              | -9.2507             |
| ThNH <sub>4</sub> B <sub>6</sub> C <sub>6</sub> | 2 ThH <sub>2</sub> + 2 Th <sub>2</sub> C <sub>3</sub> + 42 B + ThN → 6 ThB <sub>6</sub> + ThB <sub>6</sub> H <sub>4</sub> C <sub>6</sub> N                                                                         | -9.2166             |
| ThNH <sub>4</sub> B <sub>6</sub> C <sub>6</sub> | 0.5714 B <sub>5</sub> H <sub>7</sub> + 6 ThC + 3.262 N <sub>2</sub> + 0.5238 ThB <sub>6</sub> → 5.524 ThN + ThB <sub>6</sub> H <sub>4</sub> C <sub>6</sub> N                                                       | -9.1878             |
| ThNH <sub>4</sub> B <sub>6</sub> C <sub>6</sub> | 0.5714 B <sub>5</sub> H <sub>7</sub> + 2.554 Th <sub>3</sub> N <sub>4</sub> + 3 B <sub>13</sub> C <sub>2</sub> → 6.661 ThB <sub>4</sub> + 9.214 BN + ThB <sub>6</sub> H <sub>4</sub> C <sub>6</sub> N              | -9.1701             |
| ThNH <sub>4</sub> B <sub>6</sub> C <sub>6</sub> | 0.5 ThH <sub>2</sub> + 6 ThC + 28 B + H <sub>3</sub> N → 5.5 ThB <sub>4</sub> + ThB <sub>6</sub> H <sub>4</sub> C <sub>6</sub> N                                                                                   | -9.1683             |
| ThNH <sub>4</sub> B <sub>6</sub> C <sub>6</sub> | 2.956 Th <sub>4</sub> H <sub>15</sub> + 3 B <sub>13</sub> C <sub>2</sub> + 5.911 N <sub>2</sub> → 3.667 B <sub>9</sub> H <sub>11</sub> + 10.82 ThN + ThB <sub>6</sub> H <sub>4</sub> C <sub>6</sub> N              | -9.1668             |
| ThNH <sub>4</sub> B <sub>6</sub> C <sub>6</sub> | 0.25 Th <sub>3</sub> N <sub>4</sub> + 6 ThC + 2 H <sub>2</sub> + 29 B → 5.75 ThB <sub>4</sub> + ThB <sub>6</sub> H <sub>4</sub> C <sub>6</sub> N                                                                   | -9.1584             |
| ThNH <sub>4</sub> B <sub>6</sub> C <sub>6</sub> | 6 ThC + 0.3636 B <sub>9</sub> H <sub>11</sub> + 3.227 N <sub>2</sub> + 0.4545 ThB <sub>6</sub> → 5.455 ThN + ThB <sub>6</sub> H <sub>4</sub> C <sub>6</sub> N                                                      | -9.1421             |
| ThNH <sub>4</sub> B <sub>6</sub> C <sub>6</sub> | ThH <sub>2</sub> + 3 B <sub>13</sub> C <sub>2</sub> + 11.27 H <sub>3</sub> N → 4.545 B <sub>5</sub> H <sub>7</sub> + 10.27 BN + ThB <sub>6</sub> H <sub>4</sub> C <sub>6</sub> N                                   | -9.1138             |
| ThNH <sub>4</sub> B <sub>6</sub> C <sub>6</sub> | 0.5714 B <sub>5</sub> H <sub>7</sub> + 6 ThC + 23.14 B + 0.5 N <sub>2</sub> → 5 ThB <sub>4</sub> + ThB <sub>6</sub> H <sub>4</sub> C <sub>6</sub> N                                                                | -9.0649             |
| ThNH <sub>4</sub> B <sub>6</sub> C <sub>6</sub> | 0.5714 B <sub>5</sub> H <sub>7</sub> + 6 ThC + 27.14 B + ThN → 6 ThB <sub>4</sub> + ThB <sub>6</sub> H <sub>4</sub> C <sub>6</sub> N                                                                               | -9.0153             |
| ThNH <sub>4</sub> B <sub>6</sub> C <sub>6</sub> | 6 ThC + 0.3636 B <sub>9</sub> H <sub>11</sub> + 22.73 B + 0.5 N <sub>2</sub> → 5 ThB <sub>4</sub> + ThB <sub>6</sub> H <sub>4</sub> C <sub>6</sub> N                                                               | -9.0026             |
| ThNH <sub>4</sub> B <sub>6</sub> C <sub>6</sub> | 2 ThH <sub>2</sub> + 2 Th <sub>2</sub> C <sub>3</sub> + 36 B + 0.5 N <sub>2</sub> → 5 ThB <sub>6</sub> + ThB <sub>6</sub> H <sub>4</sub> C <sub>6</sub> N                                                          | -8.9776             |
| ThNH <sub>4</sub> B <sub>6</sub> C <sub>6</sub> | 6 ThC + 0.3636 B <sub>9</sub> H <sub>11</sub> + 26.73 B + ThN → 6 ThB <sub>4</sub> + ThB <sub>6</sub> H <sub>4</sub> C <sub>6</sub> N                                                                              | -8.9530             |
| ThNH <sub>4</sub> B <sub>6</sub> C <sub>6</sub> | 1.5 ThB <sub>4</sub> + 0.2667 Th <sub>4</sub> H <sub>15</sub> + 2 Th <sub>2</sub> C <sub>3</sub> + 4.211 N <sub>2</sub> → 1.856 Th <sub>3</sub> N <sub>4</sub> + ThB <sub>6</sub> H <sub>4</sub> C <sub>6</sub> N  | -8.9189             |
| ThNH <sub>4</sub> B <sub>6</sub> C <sub>6</sub> | 0.3333 Th <sub>3</sub> N <sub>4</sub> + 3 B <sub>13</sub> C <sub>2</sub> + 10.4 H <sub>3</sub> N → 10.74 BN + 2.474 B <sub>9</sub> H <sub>11</sub> + ThB <sub>6</sub> H <sub>4</sub> C <sub>6</sub> N              | -8.8594             |
| ThNH <sub>4</sub> B <sub>6</sub> C <sub>6</sub> | 6.765 B <sub>9</sub> H <sub>11</sub> + 3 B <sub>13</sub> C <sub>2</sub> + 24.47 ThN → 23.47 ThB <sub>4</sub> + 23.47 H <sub>3</sub> N + ThB <sub>6</sub> H <sub>4</sub> C <sub>6</sub> N                           | -8.8566             |
| ThNH <sub>4</sub> B <sub>6</sub> C <sub>6</sub> | 6 ThC + 2.75 B <sub>9</sub> H <sub>11</sub> + 3 N <sub>2</sub> → 3.75 B <sub>5</sub> H <sub>7</sub> + 5 ThN + ThB <sub>6</sub> H <sub>4</sub> C <sub>6</sub> N                                                     | -8.8421             |
| ThNH <sub>4</sub> B <sub>6</sub> C <sub>6</sub> | 0.3636 B <sub>9</sub> H <sub>11</sub> + 3 B <sub>13</sub> C <sub>2</sub> + 8.255 ThN → 7.255 ThB <sub>4</sub> + 7.255 BN + ThB <sub>6</sub> H <sub>4</sub> C <sub>6</sub> N                                        | -8.8130             |
| ThNH <sub>4</sub> B <sub>6</sub> C <sub>6</sub> | 3 B <sub>13</sub> C <sub>2</sub> + 1.333 H <sub>3</sub> N + 7.333 ThN → 6.333 ThB <sub>4</sub> + 7.667 BN + ThB <sub>6</sub> H <sub>4</sub> C <sub>6</sub> N                                                       | -8.8105             |
| ThNH <sub>4</sub> B <sub>6</sub> C <sub>6</sub> | 3 B <sub>13</sub> C <sub>2</sub> + 10.5 H <sub>3</sub> N + ThN → 10.5 BN + 2.5 B <sub>9</sub> H <sub>11</sub> + ThB <sub>6</sub> H <sub>4</sub> C <sub>6</sub> N                                                   | -8.7935             |
| ThNH <sub>4</sub> B <sub>6</sub> C <sub>6</sub> | ThB <sub>4</sub> + 3 B <sub>13</sub> C <sub>2</sub> + 11.95 H <sub>3</sub> N → 10.95 BN + 2.895 B <sub>9</sub> H <sub>11</sub> + ThB <sub>6</sub> H <sub>4</sub> C <sub>6</sub> N                                  | -8.7908             |
| ThNH <sub>4</sub> B <sub>6</sub> C <sub>6</sub> | 6 ThC + 26.33 B + 1.333 H <sub>3</sub> N → 5 ThB <sub>4</sub> + 0.3333 BN + ThB <sub>6</sub> H <sub>4</sub> C <sub>6</sub> N                                                                                       | -8.7522             |
| ThNH <sub>4</sub> B <sub>6</sub> C <sub>6</sub> | 6 ThC + 0.6667 B <sub>9</sub> H <sub>11</sub> + 3 N <sub>2</sub> → 1.667 H <sub>2</sub> + 5 ThN + ThB <sub>6</sub> H <sub>4</sub> C <sub>6</sub> N                                                                 | -8.7012             |
| ThNH <sub>4</sub> B <sub>6</sub> C <sub>6</sub> | 2 ThH <sub>2</sub> + 0.25 Th <sub>3</sub> N <sub>4</sub> + 2 Th <sub>2</sub> C <sub>3</sub> + 40.5 B → 5.75 ThB <sub>6</sub> + ThB <sub>6</sub> H <sub>4</sub> C <sub>6</sub> N                                    | -8.6904             |
| ThNH <sub>4</sub> B <sub>6</sub> C <sub>6</sub> | 0.5714 B <sub>5</sub> H <sub>7</sub> + 3 B <sub>13</sub> C <sub>2</sub> + 8.171 ThN → 7.171 ThB <sub>4</sub> + 7.171 BN + ThB <sub>6</sub> H <sub>4</sub> C <sub>6</sub> N                                         | -8.6660             |
| ThNH <sub>4</sub> B <sub>6</sub> C <sub>6</sub> | 1.2 B <sub>5</sub> H <sub>7</sub> + 2.917 Th <sub>2</sub> C <sub>3</sub> + 2.917 N <sub>2</sub> → 0.55 H <sub>8</sub> C <sub>5</sub> + 4.833 ThN + ThB <sub>6</sub> H <sub>4</sub> C <sub>6</sub> N                | -8.6656             |
| ThNH <sub>4</sub> B <sub>6</sub> C <sub>6</sub> | 1.2 B <sub>5</sub> H <sub>7</sub> + 6 ThC + 3 N <sub>2</sub> → 2.2 H <sub>2</sub> + 5 ThN + ThB <sub>6</sub> H <sub>4</sub> C <sub>6</sub> N                                                                       | -8.6561             |
| ThNH <sub>4</sub> B <sub>6</sub> C <sub>6</sub> | 0.2667 Th <sub>4</sub> H <sub>15</sub> + BN + 3 B <sub>13</sub> C <sub>2</sub> + 5.6 Th → 5.667 ThB <sub>6</sub> + ThB <sub>6</sub> H <sub>4</sub> C <sub>6</sub> N                                                | -8.6456             |
| ThNH <sub>4</sub> B <sub>6</sub> C <sub>6</sub> | 6 ThC + 0.06667 Th <sub>4</sub> H <sub>15</sub> + 27.07 B + H <sub>3</sub> N → 5.267 ThB <sub>4</sub> + ThB <sub>6</sub> H <sub>4</sub> C <sub>6</sub> N                                                           | -8.5798             |
| ThNH <sub>4</sub> B <sub>6</sub> C <sub>6</sub> | 0.5714 B <sub>5</sub> H <sub>7</sub> + 0.25 Th <sub>3</sub> N <sub>4</sub> + 6 ThC + 26.14 B → 5.75 ThB <sub>4</sub> + ThB <sub>6</sub> H <sub>4</sub> C <sub>6</sub> N                                            | -8.5612             |
| ThNH <sub>4</sub> B <sub>6</sub> C <sub>6</sub> | 6 ThC + 2 H <sub>2</sub> + BN + 35 B → 5 ThB <sub>6</sub> + ThB <sub>6</sub> H <sub>4</sub> C <sub>6</sub> N                                                                                                       | -8.5384             |
| ThNH <sub>4</sub> B <sub>6</sub> C <sub>6</sub> | 2 B <sub>9</sub> H <sub>11</sub> + 2 Th <sub>2</sub> C <sub>3</sub> + 3.5 N <sub>2</sub> → 3 ThB <sub>4</sub> + 6 H <sub>3</sub> N + ThB <sub>6</sub> H <sub>4</sub> C <sub>6</sub> N                              | -8.5308             |
| ThNH <sub>4</sub> B <sub>6</sub> C <sub>6</sub> | 2 ThH <sub>2</sub> + 1.5 ThB <sub>4</sub> + 3 ThC <sub>2</sub> + 4.167 N <sub>2</sub> → 1.833 Th <sub>3</sub> N <sub>4</sub> + ThB <sub>6</sub> H <sub>4</sub> C <sub>6</sub> N                                    | -8.5257             |
| ThNH <sub>4</sub> B <sub>6</sub> C <sub>6</sub> | 0.25 Th <sub>3</sub> N <sub>4</sub> + 6 ThC + 0.3636 B <sub>9</sub> H <sub>11</sub> + 25.73 B → 5.75 ThB <sub>4</sub> + ThB <sub>6</sub> H <sub>4</sub> C <sub>6</sub> N                                           | -8.4989             |
| ThNH <sub>4</sub> B <sub>6</sub> C <sub>6</sub> | 2 ThH <sub>2</sub> + 0.4615 B <sub>13</sub> C <sub>2</sub> + 1.692 Th <sub>2</sub> C <sub>3</sub> + 3.423 N <sub>2</sub> → 1.462 Th <sub>3</sub> N <sub>4</sub> + ThB <sub>6</sub> H <sub>4</sub> C <sub>6</sub> N | -8.4866             |
| ThNH <sub>4</sub> B <sub>6</sub> C <sub>6</sub> | 6 ThC + 0.5 H <sub>2</sub> + 26 B + H <sub>3</sub> N → 5 ThB <sub>4</sub> + ThB <sub>6</sub> H <sub>4</sub> C <sub>6</sub> N                                                                                       | -8.3380             |
| ThNH <sub>4</sub> B <sub>6</sub> C <sub>6</sub> | 0.2667 Th <sub>4</sub> H <sub>15</sub> + 2 Th <sub>2</sub> C <sub>3</sub> + 3.878 N <sub>2</sub> + ThB <sub>6</sub> → 1.689 Th <sub>3</sub> N <sub>4</sub> + ThB <sub>6</sub> H <sub>4</sub> C <sub>6</sub> N      | -8.2945             |
| ThNH <sub>4</sub> B <sub>6</sub> C <sub>6</sub> | 2.375 Th <sub>3</sub> N <sub>4</sub> + 2 H <sub>2</sub> + 3 B <sub>13</sub> C <sub>2</sub> → 6.125 ThB <sub>4</sub> + 8.5 BN + ThB <sub>6</sub> H <sub>4</sub> C <sub>6</sub> N                                    | -8.2936             |
| ThNH <sub>4</sub> B <sub>6</sub> C <sub>6</sub> | 1.5 ThB <sub>4</sub> + 6 ThC + 1.333 H <sub>3</sub> N + 3.083 N <sub>2</sub> → 6.5 ThN + ThB <sub>6</sub> H <sub>4</sub> C <sub>6</sub> N                                                                          | -8.2191             |
| ThNH <sub>4</sub> B <sub>6</sub> C <sub>6</sub> | 0.1429 B <sub>5</sub> H <sub>7</sub> + 6 ThC + 25.29 B + H <sub>3</sub> N → 5 ThB <sub>4</sub> + ThB <sub>6</sub> H <sub>4</sub> C <sub>6</sub> N                                                                  | -8.1887             |
| ThNH <sub>4</sub> B <sub>6</sub> C <sub>6</sub> | 6 ThC + 0.09091 B <sub>9</sub> H <sub>11</sub> + 25.18 B + H <sub>3</sub> N → 5 ThB <sub>4</sub> + ThB <sub>6</sub> H <sub>4</sub> C <sub>6</sub> N                                                                | -8.1731             |
| ThNH <sub>4</sub> B <sub>6</sub> C <sub>6</sub> | 6 ThC + 6 B + 1.333 H <sub>3</sub> N + 2.333 N <sub>2</sub> → 5 ThN + ThB <sub>6</sub> H <sub>4</sub> C <sub>6</sub> N                                                                                             | -8.1447             |
| ThNH <sub>4</sub> B <sub>6</sub> C <sub>6</sub> | 2 ThH <sub>2</sub> + BN + 3 B <sub>13</sub> C <sub>2</sub> + 4.667 Th → 5.667 ThB <sub>6</sub> + ThB <sub>6</sub> H <sub>4</sub> C <sub>6</sub> N                                                                  | -8.1084             |
| ThNH <sub>4</sub> B <sub>6</sub> C <sub>6</sub> | 2 ThH <sub>2</sub> + 6 ThC + 0.5 N <sub>2</sub> + 17 ThB <sub>6</sub> → 24 ThB <sub>4</sub> + ThB <sub>6</sub> H <sub>4</sub> C <sub>6</sub> N                                                                     | -8.0769             |
| ThNH <sub>4</sub> B <sub>6</sub> C <sub>6</sub> | 6 ThC + 25 B + 1.333 H <sub>3</sub> N → 4.75 ThB <sub>4</sub> + 0.08333 Th <sub>3</sub> N <sub>4</sub> + ThB <sub>6</sub> H <sub>4</sub> C <sub>6</sub> N                                                          | -8.0645             |
| ThNH <sub>4</sub> B <sub>6</sub> C <sub>6</sub> | 6 ThC + 0.2667 Th <sub>4</sub> H <sub>15</sub> + BN + 29.27 B → 6.067 ThB <sub>4</sub> + ThB <sub>6</sub> H <sub>4</sub> C <sub>6</sub> N                                                                          | -8.0625             |
| ThNH <sub>4</sub> B <sub>6</sub> C <sub>6</sub> | 5.077 ThC + 0.2667 Th <sub>4</sub> H <sub>15</sub> + 0.4615 B <sub>13</sub> C <sub>2</sub> + 3.072 N <sub>2</sub> → 5.144 ThN + ThB <sub>6</sub> H <sub>4</sub> C <sub>6</sub> N                                   | -8.0535             |

Continued on next page

Continued

| Compound                                        | Chemical reaction                                                                                                                                                                                               | Reaction energy(eV) |
|-------------------------------------------------|-----------------------------------------------------------------------------------------------------------------------------------------------------------------------------------------------------------------|---------------------|
| ThNH <sub>4</sub> B <sub>6</sub> C <sub>6</sub> | 0.25 Th <sub>4</sub> H <sub>15</sub> + 3 B <sub>13</sub> C <sub>2</sub> + 10.88 H <sub>3</sub> N → 4.625 B <sub>5</sub> H <sub>7</sub> + 9.875 BN + ThB <sub>6</sub> H <sub>4</sub> C <sub>6</sub> N            | -7.9487             |
| ThNH <sub>4</sub> B <sub>6</sub> C <sub>6</sub> | ThH <sub>2</sub> + 3 B <sub>13</sub> C <sub>2</sub> + 10.32 H <sub>3</sub> N → 9.316 BN + 2.632 B <sub>9</sub> H <sub>11</sub> + ThB <sub>6</sub> H <sub>4</sub> C <sub>6</sub> N                               | -7.9467             |
| ThNH <sub>4</sub> B <sub>6</sub> C <sub>6</sub> | 5.58 ThC + 0.3636 B <sub>9</sub> H <sub>11</sub> + 0.2098 B <sub>13</sub> C <sub>2</sub> + 2.79 N <sub>2</sub> → 4.58 ThN + ThB <sub>6</sub> H <sub>4</sub> C <sub>6</sub> N                                    | -7.9431             |
| ThNH <sub>4</sub> B <sub>6</sub> C <sub>6</sub> | 0.5714 B <sub>5</sub> H <sub>7</sub> + 6 ThC + BN + 32.14 B → 5 ThB <sub>6</sub> + ThB <sub>6</sub> H <sub>4</sub> C <sub>6</sub> N                                                                             | -7.9412             |
| ThNH <sub>4</sub> B <sub>6</sub> C <sub>6</sub> | 6 ThC + 0.6667 B <sub>9</sub> H <sub>11</sub> + 2.722 N <sub>2</sub> → 1.667 ThH <sub>2</sub> + 1.111 Th <sub>3</sub> N <sub>4</sub> + ThB <sub>6</sub> H <sub>4</sub> C <sub>6</sub> N                         | -7.9240             |
| ThNH <sub>4</sub> B <sub>6</sub> C <sub>6</sub> | 6 ThC + 24.67 B + 1.333 H <sub>3</sub> N → 4.667 ThB <sub>4</sub> + 0.3333 ThN + ThB <sub>6</sub> H <sub>4</sub> C <sub>6</sub> N                                                                               | -7.9132             |
| ThNH <sub>4</sub> B <sub>6</sub> C <sub>6</sub> | 0.2667 Th <sub>4</sub> H <sub>15</sub> + 2 Th <sub>2</sub> C <sub>3</sub> + 6 B + 3.211 N <sub>2</sub> → 1.356 Th <sub>3</sub> N <sub>4</sub> + ThB <sub>6</sub> H <sub>4</sub> C <sub>6</sub> N                | -7.9115             |
| ThNH <sub>4</sub> B <sub>6</sub> C <sub>6</sub> | 6 ThC + 1.333 H <sub>3</sub> N + 2.833 N <sub>2</sub> + ThB <sub>6</sub> → 6 ThN + ThB <sub>6</sub> H <sub>4</sub> C <sub>6</sub> N                                                                             | -7.9057             |
| ThNH <sub>4</sub> B <sub>6</sub> C <sub>6</sub> | 2 ThH <sub>2</sub> + 3 ThC <sub>2</sub> + 3.833 N <sub>2</sub> + ThB <sub>6</sub> → 1.667 Th <sub>3</sub> N <sub>4</sub> + ThB <sub>6</sub> H <sub>4</sub> C <sub>6</sub> N                                     | -7.9013             |
| ThNH <sub>4</sub> B <sub>6</sub> C <sub>6</sub> | 6 ThC + 26 B + 1.333 H <sub>3</sub> N → 5 ThB <sub>4</sub> + 0.1667 N <sub>2</sub> + ThB <sub>6</sub> H <sub>4</sub> C <sub>6</sub> N                                                                           | -7.8966             |
| ThNH <sub>4</sub> B <sub>6</sub> C <sub>6</sub> | 6 ThC + BN + 0.3636 B <sub>9</sub> H <sub>11</sub> + 31.73 B → 5 ThB <sub>6</sub> + ThB <sub>6</sub> H <sub>4</sub> C <sub>6</sub> N                                                                            | -7.8790             |
| ThNH <sub>4</sub> B <sub>6</sub> C <sub>6</sub> | 2 ThH <sub>2</sub> + 1.5 ThB <sub>4</sub> + 2 Th <sub>2</sub> C <sub>3</sub> + 3.75 N <sub>2</sub> → 6.5 ThN + ThB <sub>6</sub> H <sub>4</sub> C <sub>6</sub> N                                                 | -7.8570             |
| ThNH <sub>4</sub> B <sub>6</sub> C <sub>6</sub> | 6 ThC + 0.6667 B <sub>9</sub> H <sub>11</sub> + 2.556 N <sub>2</sub> → 0.2222 Th <sub>4</sub> H <sub>15</sub> + 4.111 ThN + ThB <sub>6</sub> H <sub>4</sub> C <sub>6</sub> N                                    | -7.8511             |
| ThNH <sub>4</sub> B <sub>6</sub> C <sub>6</sub> | 2 H <sub>2</sub> + 3 B <sub>13</sub> C <sub>2</sub> + 7.6 ThN → 6.6 ThB <sub>4</sub> + 6.6 BN + ThB <sub>6</sub> H <sub>4</sub> C <sub>6</sub> N                                                                | -7.8248             |
| ThNH <sub>4</sub> B <sub>6</sub> C <sub>6</sub> | 0.25 Th <sub>3</sub> N <sub>4</sub> + 0.2667 Th <sub>4</sub> H <sub>15</sub> + 3 B <sub>13</sub> C <sub>2</sub> + 4.683 Th → 5.5 ThB <sub>6</sub> + ThB <sub>6</sub> H <sub>4</sub> C <sub>6</sub> N            | -7.8208             |
| ThNH <sub>4</sub> B <sub>6</sub> C <sub>6</sub> | 0.5714 B <sub>5</sub> H <sub>7</sub> + 5.516 ThC + 0.2418 B <sub>13</sub> C <sub>2</sub> + 2.758 N <sub>2</sub> → 4.516 ThN + ThB <sub>6</sub> H <sub>4</sub> C <sub>6</sub> N                                  | -7.8061             |
| ThNH <sub>4</sub> B <sub>6</sub> C <sub>6</sub> | 5.077 ThC + 0.4615 B <sub>13</sub> C <sub>2</sub> + 1.333 H <sub>3</sub> N + 2.551 N <sub>2</sub> → 1.359 Th <sub>3</sub> N <sub>4</sub> + ThB <sub>6</sub> H <sub>4</sub> C <sub>6</sub> N                     | -7.8038             |
| ThNH <sub>4</sub> B <sub>6</sub> C <sub>6</sub> | 5.375 ThC + 32.25 B + H <sub>3</sub> N + 0.125 H <sub>8</sub> C <sub>5</sub> → 4.375 ThB <sub>6</sub> + ThB <sub>6</sub> H <sub>4</sub> C <sub>6</sub> N                                                        | -7.7907             |
| ThNH <sub>4</sub> B <sub>6</sub> C <sub>6</sub> | 2 ThH <sub>2</sub> + 2 Th <sub>2</sub> C <sub>3</sub> + 6 B + 3 N <sub>2</sub> → 5 ThN + ThB <sub>6</sub> H <sub>4</sub> C <sub>6</sub> N                                                                       | -7.7826             |
| ThNH <sub>4</sub> B <sub>6</sub> C <sub>6</sub> | 1.75 B <sub>13</sub> C <sub>2</sub> + 5.188 Th + 0.5 H <sub>8</sub> C <sub>5</sub> + 0.5 N <sub>2</sub> → 4.187 ThB <sub>4</sub> + ThB <sub>6</sub> H <sub>4</sub> C <sub>6</sub> N                             | -7.7588             |
| ThNH <sub>4</sub> B <sub>6</sub> C <sub>6</sub> | 1.625 Th <sub>4</sub> H <sub>15</sub> + 3 B <sub>13</sub> C <sub>2</sub> + 3.896 N <sub>2</sub> → 6.792 H <sub>3</sub> N + 5.5 ThB <sub>6</sub> + ThB <sub>6</sub> H <sub>4</sub> C <sub>6</sub> N              | -7.7349             |
| ThNH <sub>4</sub> B <sub>6</sub> C <sub>6</sub> | 3.6 B <sub>5</sub> H <sub>7</sub> + 3 ThC <sub>2</sub> + 4.033 N <sub>2</sub> → 7.067 H <sub>3</sub> N + 2 ThB <sub>6</sub> + ThB <sub>6</sub> H <sub>4</sub> C <sub>6</sub> N                                  | -7.6825             |
| ThNH <sub>4</sub> B <sub>6</sub> C <sub>6</sub> | 6.5 ThH <sub>2</sub> + 3 B <sub>13</sub> C <sub>2</sub> + 2 N <sub>2</sub> → 3 H <sub>3</sub> N + 5.5 ThB <sub>6</sub> + ThB <sub>6</sub> H <sub>4</sub> C <sub>6</sub> N                                       | -7.6151             |
| ThNH <sub>4</sub> B <sub>6</sub> C <sub>6</sub> | 3.667 ThB <sub>4</sub> + 2 Th <sub>2</sub> C <sub>3</sub> + 9.667 H <sub>3</sub> N → 1.667 Th <sub>4</sub> H <sub>15</sub> + 8.667 BN + ThB <sub>6</sub> H <sub>4</sub> C <sub>6</sub> N                        | -7.6143             |
| ThNH <sub>4</sub> B <sub>6</sub> C <sub>6</sub> | 2 ThH <sub>2</sub> + 2 Th <sub>2</sub> C <sub>3</sub> + 3.5 N <sub>2</sub> + ThB <sub>6</sub> → 6 ThN + ThB <sub>6</sub> H <sub>4</sub> C <sub>6</sub> N                                                        | -7.5436             |
| ThNH <sub>4</sub> B <sub>6</sub> C <sub>6</sub> | 2 ThH <sub>2</sub> + 2 Th <sub>2</sub> C <sub>3</sub> + 26 B + 0.5 N <sub>2</sub> → 5 ThB <sub>4</sub> + ThB <sub>6</sub> H <sub>4</sub> C <sub>6</sub> N                                                       | -7.5345             |
| ThNH <sub>4</sub> B <sub>6</sub> C <sub>6</sub> | 1.2 B <sub>5</sub> H <sub>7</sub> + 6 ThC + 2.413 N <sub>2</sub> → 0.2933 Th <sub>4</sub> H <sub>15</sub> + 3.827 ThN + ThB <sub>6</sub> H <sub>4</sub> C <sub>6</sub> N                                        | -7.5340             |
| ThNH <sub>4</sub> B <sub>6</sub> C <sub>6</sub> | 11.64 ThH <sub>2</sub> + 3 B <sub>13</sub> C <sub>2</sub> + 0.5 N <sub>2</sub> → 1.286 Th <sub>4</sub> H <sub>15</sub> + 5.5 ThB <sub>6</sub> + ThB <sub>6</sub> H <sub>4</sub> C <sub>6</sub> N                | -7.5204             |
| ThNH <sub>4</sub> B <sub>6</sub> C <sub>6</sub> | 2 ThH <sub>2</sub> + 3 ThC <sub>2</sub> + 6 B + 3.167 N <sub>2</sub> → 1.333 Th <sub>3</sub> N <sub>4</sub> + ThB <sub>6</sub> H <sub>4</sub> C <sub>6</sub> N                                                  | -7.5183             |
| ThNH <sub>4</sub> B <sub>6</sub> C <sub>6</sub> | 0.2667 Th <sub>4</sub> H <sub>15</sub> + 3 B <sub>13</sub> C <sub>2</sub> + 4.433 Th + ThN → 5.5 ThB <sub>6</sub> + ThB <sub>6</sub> H <sub>4</sub> C <sub>6</sub> N                                            | -7.5004             |
| ThNH <sub>4</sub> B <sub>6</sub> C <sub>6</sub> | ThC + 2.5 B <sub>13</sub> C <sub>2</sub> + 9.659 H <sub>3</sub> N → 3.568 B <sub>5</sub> H <sub>7</sub> + 8.659 BN + ThB <sub>6</sub> H <sub>4</sub> C <sub>6</sub> N                                           | -7.4934             |
| ThNH <sub>4</sub> B <sub>6</sub> C <sub>6</sub> | 2 ThH <sub>2</sub> + 1.875 Th <sub>3</sub> N <sub>4</sub> + 3 B <sub>13</sub> C <sub>2</sub> → 6.625 ThB <sub>4</sub> + 6.5 BN + ThB <sub>6</sub> H <sub>4</sub> C <sub>6</sub> N                               | -7.4888             |
| ThNH <sub>4</sub> B <sub>6</sub> C <sub>6</sub> | 13.36 ThH <sub>2</sub> + 3 B <sub>13</sub> C <sub>2</sub> + H <sub>3</sub> N → 1.714 Th <sub>4</sub> H <sub>15</sub> + 5.5 ThB <sub>6</sub> + ThB <sub>6</sub> H <sub>4</sub> C <sub>6</sub> N                  | -7.4888             |
| ThNH <sub>4</sub> B <sub>6</sub> C <sub>6</sub> | 2 ThH <sub>2</sub> + 2 Th <sub>2</sub> C <sub>3</sub> + 30 B + ThN → 6 ThB <sub>4</sub> + ThB <sub>6</sub> H <sub>4</sub> C <sub>6</sub> N                                                                      | -7.4849             |
| ThNH <sub>4</sub> B <sub>6</sub> C <sub>6</sub> | 2 ThH <sub>2</sub> + 6 ThC + 19 ThB <sub>6</sub> + ThN → 27 ThB <sub>4</sub> + ThB <sub>6</sub> H <sub>4</sub> C <sub>6</sub> N                                                                                 | -7.4500             |
| ThNH <sub>4</sub> B <sub>6</sub> C <sub>6</sub> | 0.6667 B <sub>9</sub> H <sub>11</sub> + 2.694 Th <sub>2</sub> C <sub>3</sub> + 2.694 N <sub>2</sub> → 0.4167 H <sub>8</sub> C <sub>5</sub> + 4.389 ThN + ThB <sub>6</sub> H <sub>4</sub> C <sub>6</sub> N       | -7.3634             |
| ThNH <sub>4</sub> B <sub>6</sub> C <sub>6</sub> | 2 ThH <sub>2</sub> + 0.25 Th <sub>3</sub> N <sub>4</sub> + 3 B <sub>13</sub> C <sub>2</sub> + 3.75 Th → 5.5 ThB <sub>6</sub> + ThB <sub>6</sub> H <sub>4</sub> C <sub>6</sub> N                                 | -7.2836             |
| ThNH <sub>4</sub> B <sub>6</sub> C <sub>6</sub> | 1.5 ThB <sub>4</sub> + 2 H <sub>2</sub> + 2 Th <sub>2</sub> C <sub>3</sub> + 3.5 N <sub>2</sub> → 1.5 Th <sub>3</sub> N <sub>4</sub> + ThB <sub>6</sub> H <sub>4</sub> C <sub>6</sub> N                         | -7.2354             |
| ThNH <sub>4</sub> B <sub>6</sub> C <sub>6</sub> | 3 B <sub>13</sub> C <sub>2</sub> + 16.73 H <sub>3</sub> N + 51.2 ThN → 6.6 B <sub>5</sub> H <sub>7</sub> + 16.73 Th <sub>3</sub> N <sub>4</sub> + ThB <sub>6</sub> H <sub>4</sub> C <sub>6</sub> N              | -7.1763             |
| ThNH <sub>4</sub> B <sub>6</sub> C <sub>6</sub> | 2 ThH <sub>2</sub> + 0.25 Th <sub>3</sub> N <sub>4</sub> + 6 ThC + 18.5 ThB <sub>6</sub> → 26.25 ThB <sub>4</sub> + ThB <sub>6</sub> H <sub>4</sub> C <sub>6</sub> N                                            | -7.1402             |
| ThNH <sub>4</sub> B <sub>6</sub> C <sub>6</sub> | 2 ThH <sub>2</sub> + 3 B <sub>13</sub> C <sub>2</sub> + 6 ThN → 7 ThB <sub>4</sub> + 5 BN + ThB <sub>6</sub> H <sub>4</sub> C <sub>6</sub> N                                                                    | -7.1187             |
| ThNH <sub>4</sub> B <sub>6</sub> C <sub>6</sub> | 6 ThC + 2 H <sub>2</sub> + BN + 25 B → 5 ThB <sub>4</sub> + ThB <sub>6</sub> H <sub>4</sub> C <sub>6</sub> N                                                                                                    | -7.0953             |
| ThNH <sub>4</sub> B <sub>6</sub> C <sub>6</sub> | 2.108 Th <sub>3</sub> N <sub>4</sub> + 0.2667 Th <sub>4</sub> H <sub>15</sub> + 3 B <sub>13</sub> C <sub>2</sub> → 6.392 ThB <sub>4</sub> + 7.433 BN + ThB <sub>6</sub> H <sub>4</sub> C <sub>6</sub> N         | -7.0602             |
| ThNH <sub>4</sub> B <sub>6</sub> C <sub>6</sub> | 9.675 ThC + 3.321 B <sub>9</sub> H <sub>11</sub> + 0.5 N <sub>2</sub> → 2.169 Th <sub>4</sub> H <sub>15</sub> + 1.838 B <sub>13</sub> C <sub>2</sub> + ThB <sub>6</sub> H <sub>4</sub> C <sub>6</sub> N         | -7.0451             |
| ThNH <sub>4</sub> B <sub>6</sub> C <sub>6</sub> | 5.077 ThC + 2 H <sub>2</sub> + 0.4615 B <sub>13</sub> C <sub>2</sub> + 2.538 N <sub>2</sub> → 4.077 ThN + ThB <sub>6</sub> H <sub>4</sub> C <sub>6</sub> N                                                      | -7.0334             |
| ThNH <sub>4</sub> B <sub>6</sub> C <sub>6</sub> | 2 ThH <sub>2</sub> + 0.25 Th <sub>3</sub> N <sub>4</sub> + 2 Th <sub>2</sub> C <sub>3</sub> + 29 B → 5.75 ThB <sub>4</sub> + ThB <sub>6</sub> H <sub>4</sub> C <sub>6</sub> N                                   | -7.0308             |
| ThNH <sub>4</sub> B <sub>6</sub> C <sub>6</sub> | 0.3636 B <sub>9</sub> H <sub>11</sub> + 3 B <sub>13</sub> C <sub>2</sub> + 37.27 ThN → 9.068 ThB <sub>4</sub> + 9.068 Th <sub>3</sub> N <sub>4</sub> + ThB <sub>6</sub> H <sub>4</sub> C <sub>6</sub> N         | -7.0231             |
| ThNH <sub>4</sub> B <sub>6</sub> C <sub>6</sub> | 2 ThH <sub>2</sub> + 3 B <sub>13</sub> C <sub>2</sub> + 3.5 Th + ThN → 5.5 ThB <sub>6</sub> + ThB <sub>6</sub> H <sub>4</sub> C <sub>6</sub> N                                                                  | -6.9632             |
| ThNH <sub>4</sub> B <sub>6</sub> C <sub>6</sub> | 3 B <sub>13</sub> C <sub>2</sub> + 1.333 H <sub>3</sub> N + 38 ThN → 8.25 ThB <sub>4</sub> + 9.583 Th <sub>3</sub> N <sub>4</sub> + ThB <sub>6</sub> H <sub>4</sub> C <sub>6</sub> N                            | -6.9189             |
| ThNH <sub>4</sub> B <sub>6</sub> C <sub>6</sub> | 1.2 B <sub>5</sub> H <sub>7</sub> + 2 Th <sub>2</sub> C <sub>3</sub> + 3.233 N <sub>2</sub> → Th <sub>3</sub> N <sub>4</sub> + 1.467 H <sub>3</sub> N + ThB <sub>6</sub> H <sub>4</sub> C <sub>6</sub> N        | -6.9159             |
| ThNH <sub>4</sub> B <sub>6</sub> C <sub>6</sub> | 0.5714 B <sub>5</sub> H <sub>7</sub> + 3 B <sub>13</sub> C <sub>2</sub> + 36.86 ThN → 8.964 ThB <sub>4</sub> + 8.964 Th <sub>3</sub> N <sub>4</sub> + ThB <sub>6</sub> H <sub>4</sub> C <sub>6</sub> N          | -6.8967             |
| ThNH <sub>4</sub> B <sub>6</sub> C <sub>6</sub> | 10.57 ThC + 3.967 B <sub>9</sub> H <sub>11</sub> + ThN → 2.642 Th <sub>4</sub> H <sub>15</sub> + 2.285 B <sub>13</sub> C <sub>2</sub> + ThB <sub>6</sub> H <sub>4</sub> C <sub>6</sub> N                        | -6.8491             |
| ThNH <sub>4</sub> B <sub>6</sub> C <sub>6</sub> | 0.25 Th <sub>4</sub> H <sub>15</sub> + 3 B <sub>13</sub> C <sub>2</sub> + 9.901 H <sub>3</sub> N → 8.901 BN + 2.678 B <sub>9</sub> H <sub>11</sub> + ThB <sub>6</sub> H <sub>4</sub> C <sub>6</sub> N           | -6.7612             |
| ThNH <sub>4</sub> B <sub>6</sub> C <sub>6</sub> | 1.2 B <sub>5</sub> H <sub>7</sub> + 4.375 ThC <sub>2</sub> + 2.75 N <sub>2</sub> → 1.125 Th <sub>3</sub> N <sub>4</sub> + 0.55 H <sub>8</sub> C <sub>5</sub> + ThB <sub>6</sub> H <sub>4</sub> C <sub>6</sub> N | -6.7512             |
| ThNH <sub>4</sub> B <sub>6</sub> C <sub>6</sub> | 0.2667 Th <sub>4</sub> H <sub>15</sub> + 3 B <sub>13</sub> C <sub>2</sub> + 6.747 ThN → 6.813 ThB <sub>4</sub> + 5.747 BN + ThB <sub>6</sub> H <sub>4</sub> C <sub>6</sub> N                                    | -6.6440             |
| ThNH <sub>4</sub> B <sub>6</sub> C <sub>6</sub> | 1.2 B <sub>5</sub> H <sub>7</sub> + 6 ThC + 2.367 N <sub>2</sub> → 2.2 ThH <sub>2</sub> + 0.9333 Th <sub>3</sub> N <sub>4</sub> + ThB <sub>6</sub> H <sub>4</sub> C <sub>6</sub> N                              | -6.6350             |
| ThNH <sub>4</sub> B <sub>6</sub> C <sub>6</sub> | 9.25 ThH <sub>2</sub> + 3 B <sub>13</sub> C <sub>2</sub> + 0.5 N <sub>2</sub> → 8.25 ThB <sub>4</sub> + 7.25 H <sub>2</sub> + ThB <sub>6</sub> H <sub>4</sub> C <sub>6</sub> N                                  | -6.6223             |
| ThNH <sub>4</sub> B <sub>6</sub> C <sub>6</sub> | 2 H <sub>2</sub> + 2 Th <sub>2</sub> C <sub>3</sub> + 3.167 N <sub>2</sub> + ThB <sub>6</sub> → 1.333 Th <sub>3</sub> N <sub>4</sub> + ThB <sub>6</sub> H <sub>4</sub> C <sub>6</sub> N                         | -6.6109             |
| ThNH <sub>4</sub> B <sub>6</sub> C <sub>6</sub> | 0.2667 Th <sub>4</sub> H <sub>15</sub> + 2 Th <sub>2</sub> C <sub>3</sub> + 36.4 B + ThN → 5.067 ThB <sub>6</sub> + ThB <sub>6</sub> H <sub>4</sub> C <sub>6</sub> N                                            | -6.5931             |
| ThNH <sub>4</sub> B <sub>6</sub> C <sub>6</sub> | ThC + 2.5 B <sub>13</sub> C <sub>2</sub> + 8.908 H <sub>3</sub> N → 7.908 BN + 2.066 B <sub>9</sub> H <sub>11</sub> + ThB <sub>6</sub> H <sub>4</sub> C <sub>6</sub> N                                          | -6.5772             |

Continued on next page

Continued

| Compound                                        | Chemical reaction                                                                                                                                                                                                                     | Reaction energy(eV) |
|-------------------------------------------------|---------------------------------------------------------------------------------------------------------------------------------------------------------------------------------------------------------------------------------------|---------------------|
| ThNH <sub>4</sub> B <sub>6</sub> C <sub>6</sub> | 8.846 B <sub>5</sub> H <sub>7</sub> + 3 B <sub>13</sub> C <sub>2</sub> + 20.31 ThN → 19.31 ThB <sub>4</sub> + 19.31 H <sub>3</sub> N + ThB <sub>6</sub> H <sub>4</sub> C <sub>6</sub> N                                               | -6.5740             |
| ThNH <sub>4</sub> B <sub>6</sub> C <sub>6</sub> | 3 ThC <sub>2</sub> + 1.045 B <sub>9</sub> H <sub>11</sub> + 2.205 N <sub>2</sub> → 0.5 Th <sub>4</sub> H <sub>15</sub> + 3.409 BN + ThB <sub>6</sub> H <sub>4</sub> C <sub>6</sub> N                                                  | -6.5517             |
| ThNH <sub>4</sub> B <sub>6</sub> C <sub>6</sub> | 5.375 ThC + 23.5 B + H <sub>3</sub> N + 0.125 H <sub>8</sub> C <sub>5</sub> → 4.375 ThB <sub>4</sub> + ThB <sub>6</sub> H <sub>4</sub> C <sub>6</sub> N                                                                               | -6.5280             |
| ThNH <sub>4</sub> B <sub>6</sub> C <sub>6</sub> | 0.5714 B <sub>5</sub> H <sub>7</sub> + 6 ThC + BN + 22.14 B → 5 ThB <sub>4</sub> + ThB <sub>6</sub> H <sub>4</sub> C <sub>6</sub> N                                                                                                   | -6.4982             |
| ThNH <sub>4</sub> B <sub>6</sub> C <sub>6</sub> | 0.6667 B <sub>9</sub> H <sub>11</sub> + 2 Th <sub>2</sub> C <sub>3</sub> + 3.056 N <sub>2</sub> → Th <sub>3</sub> N <sub>4</sub> + 1.111 H <sub>3</sub> N + ThB <sub>6</sub> H <sub>4</sub> C <sub>6</sub> N                          | -6.4902             |
| ThNH <sub>4</sub> B <sub>6</sub> C <sub>6</sub> | 6 ThC + BN + 0.3636 B <sub>9</sub> H <sub>11</sub> + 21.73 B → 5 ThB <sub>4</sub> + ThB <sub>6</sub> H <sub>4</sub> C <sub>6</sub> N                                                                                                  | -6.4359             |
| ThNH <sub>4</sub> B <sub>6</sub> C <sub>6</sub> | 0.25 Th <sub>3</sub> N <sub>4</sub> + 10.35 ThC + 3.805 B <sub>9</sub> H <sub>11</sub> → 2.524 Th <sub>4</sub> H <sub>15</sub> + 2.173 B <sub>13</sub> C <sub>2</sub> + ThB <sub>6</sub> H <sub>4</sub> C <sub>6</sub> N              | -6.4316             |
| ThNH <sub>4</sub> B <sub>6</sub> C <sub>6</sub> | 2 ThH <sub>2</sub> + BN + 2 Th <sub>2</sub> C <sub>3</sub> + 35 B → 5 ThB <sub>6</sub> + ThB <sub>6</sub> H <sub>4</sub> C <sub>6</sub> N                                                                                             | -6.4108             |
| ThNH <sub>4</sub> B <sub>6</sub> C <sub>6</sub> | 3 ThC <sub>2</sub> + 2 B <sub>9</sub> H <sub>11</sub> + 3.5 N <sub>2</sub> → 6 H <sub>3</sub> N + 2 ThB <sub>6</sub> + ThB <sub>6</sub> H <sub>4</sub> C <sub>6</sub> N                                                               | -6.4054             |
| ThNH <sub>4</sub> B <sub>6</sub> C <sub>6</sub> | 0.2667 Th <sub>4</sub> H <sub>15</sub> + 2 Th <sub>2</sub> C <sub>3</sub> + 30.4 B + 0.5 N <sub>2</sub> → 4.067 ThB <sub>6</sub> + ThB <sub>6</sub> H <sub>4</sub> C <sub>6</sub> N                                                   | -6.3541             |
| ThNH <sub>4</sub> B <sub>6</sub> C <sub>6</sub> | 6 ThC + 0.2667 Th <sub>4</sub> H <sub>15</sub> + 0.5 N <sub>2</sub> + 15.13 ThB <sub>6</sub> → 21.2 ThB <sub>4</sub> + ThB <sub>6</sub> H <sub>4</sub> C <sub>6</sub> N                                                               | -6.2614             |
| ThNH <sub>4</sub> B <sub>6</sub> C <sub>6</sub> | 2 H <sub>2</sub> + 2 Th <sub>2</sub> C <sub>3</sub> + 6 B + 2.5 N <sub>2</sub> → Th <sub>3</sub> N <sub>4</sub> + ThB <sub>6</sub> H <sub>4</sub> C <sub>6</sub> N                                                                    | -6.2280             |
| ThNH <sub>4</sub> B <sub>6</sub> C <sub>6</sub> | 2 ThH <sub>2</sub> + 3 ThC <sub>2</sub> + 36 B + ThN → 5 ThB <sub>6</sub> + ThB <sub>6</sub> H <sub>4</sub> C <sub>6</sub> N                                                                                                          | -6.2255             |
| ThNH <sub>4</sub> B <sub>6</sub> C <sub>6</sub> | 2 H <sub>2</sub> + 3 B <sub>13</sub> C <sub>2</sub> + 34 ThN → 8.25 ThB <sub>4</sub> + 8.25 Th <sub>3</sub> N <sub>4</sub> + ThB <sub>6</sub> H <sub>4</sub> C <sub>6</sub> N                                                         | -6.1964             |
| ThNH <sub>4</sub> B <sub>6</sub> C <sub>6</sub> | 19 B <sub>5</sub> H <sub>7</sub> + 11 Th <sub>3</sub> N <sub>4</sub> + 3 B <sub>13</sub> C <sub>2</sub> → 32 ThB <sub>4</sub> + 43 H <sub>3</sub> N + ThB <sub>6</sub> H <sub>4</sub> C <sub>6</sub> N                                | -6.1781             |
| ThNH <sub>4</sub> B <sub>6</sub> C <sub>6</sub> | 0.7857 ThB <sub>4</sub> + 0.5714 B <sub>5</sub> H <sub>7</sub> + 2 Th <sub>2</sub> C <sub>3</sub> + 3.024 N <sub>2</sub> → 1.262 Th <sub>3</sub> N <sub>4</sub> + ThB <sub>6</sub> H <sub>4</sub> C <sub>6</sub> N                    | -6.1585             |
| ThNH <sub>4</sub> B <sub>6</sub> C <sub>6</sub> | 5.867 B <sub>5</sub> H <sub>7</sub> + 1.2 H <sub>8</sub> C <sub>5</sub> + 24.33 ThN → 23.33 ThH <sub>2</sub> + 23.33 BN + ThB <sub>6</sub> H <sub>4</sub> C <sub>6</sub> N                                                            | -6.0902             |
| ThNH <sub>4</sub> B <sub>6</sub> C <sub>6</sub> | 1.758 Th <sub>3</sub> N <sub>4</sub> + 3 B <sub>13</sub> C <sub>2</sub> + 1.333 H <sub>3</sub> N → 7.364 BN + 4.273 ThB <sub>6</sub> + ThB <sub>6</sub> H <sub>4</sub> C <sub>6</sub> N                                               | -6.0886             |
| ThNH <sub>4</sub> B <sub>6</sub> C <sub>6</sub> | 0.25 Th <sub>3</sub> N <sub>4</sub> + 0.2667 Th <sub>4</sub> H <sub>15</sub> + 2 Th <sub>2</sub> C <sub>3</sub> + 34.9 B → 4.817 ThB <sub>6</sub> + ThB <sub>6</sub> H <sub>4</sub> C <sub>6</sub> N                                  | -6.0668             |
| ThNH <sub>4</sub> B <sub>6</sub> C <sub>6</sub> | 0.6818 ThB <sub>4</sub> + 0.3636 B <sub>9</sub> H <sub>11</sub> + 2 Th <sub>2</sub> C <sub>3</sub> + 2.955 N <sub>2</sub> → 1.227 Th <sub>3</sub> N <sub>4</sub> + ThB <sub>6</sub> H <sub>4</sub> C <sub>6</sub> N                   | -6.0264             |
| ThNH <sub>4</sub> B <sub>6</sub> C <sub>6</sub> | 4.687 B <sub>5</sub> H <sub>7</sub> + 8.682 ThC + 0.5 N <sub>2</sub> → 1.921 Th <sub>4</sub> H <sub>15</sub> + 1.341 B <sub>13</sub> C <sub>2</sub> + ThB <sub>6</sub> H <sub>4</sub> C <sub>6</sub> N                                | -6.0244             |
| ThNH <sub>4</sub> B <sub>6</sub> C <sub>6</sub> | 2 Th <sub>2</sub> C <sub>3</sub> + 7.737 H <sub>3</sub> N + 2.123 ThB <sub>6</sub> → 1.281 Th <sub>4</sub> H <sub>15</sub> + 6.737 BN + ThB <sub>6</sub> H <sub>4</sub> C <sub>6</sub> N                                              | -6.0033             |
| ThNH <sub>4</sub> B <sub>6</sub> C <sub>6</sub> | 6 ThC + 21.55 B + 7.667 H <sub>3</sub> N → 1.667 Th <sub>3</sub> N <sub>4</sub> + 1.727 B <sub>9</sub> H <sub>11</sub> + ThB <sub>6</sub> H <sub>4</sub> C <sub>6</sub> N                                                             | -6.0011             |
| ThNH <sub>4</sub> B <sub>6</sub> C <sub>6</sub> | 2 ThH <sub>2</sub> + 3 ThC <sub>2</sub> + 30 B + 0.5 N <sub>2</sub> → 4 ThB <sub>6</sub> + ThB <sub>6</sub> H <sub>4</sub> C <sub>6</sub> N                                                                                           | -5.9864             |
| ThNH <sub>4</sub> B <sub>6</sub> C <sub>6</sub> | BN + 1.75 B <sub>13</sub> C <sub>2</sub> + 5.437 Th + 0.5 H <sub>8</sub> C <sub>5</sub> → 4.437 ThB <sub>4</sub> + ThB <sub>6</sub> H <sub>4</sub> C <sub>6</sub> N                                                                   | -5.9665             |
| ThNH <sub>4</sub> B <sub>6</sub> C <sub>6</sub> | 4.376 ThC + 0.8118 B <sub>13</sub> C <sub>2</sub> + 5.554 H <sub>3</sub> N → 0.8441 Th <sub>4</sub> H <sub>15</sub> + 4.554 BN + ThB <sub>6</sub> H <sub>4</sub> C <sub>6</sub> N                                                     | -5.9561             |
| ThNH <sub>4</sub> B <sub>6</sub> C <sub>6</sub> | 2.25 B <sub>13</sub> C <sub>2</sub> + 0.5 Th <sub>2</sub> C <sub>3</sub> + 8.625 H <sub>3</sub> N → 3.125 B <sub>5</sub> H <sub>7</sub> + 7.625 BN + ThB <sub>6</sub> H <sub>4</sub> C <sub>6</sub> N                                 | -5.9164             |
| ThNH <sub>4</sub> B <sub>6</sub> C <sub>6</sub> | 6 ThC + 2 H <sub>2</sub> + 0.5 N <sub>2</sub> + 13 ThB <sub>6</sub> → 18 ThB <sub>4</sub> + ThB <sub>6</sub> H <sub>4</sub> C <sub>6</sub> N                                                                                          | -5.9100             |
| ThNH <sub>4</sub> B <sub>6</sub> C <sub>6</sub> | 2 ThH <sub>2</sub> + 3 B <sub>13</sub> C <sub>2</sub> + 26 ThN → 8.25 ThB <sub>4</sub> + 6.25 Th <sub>3</sub> N <sub>4</sub> + ThB <sub>6</sub> H <sub>4</sub> C <sub>6</sub> N                                                       | -5.8851             |
| ThNH <sub>4</sub> B <sub>6</sub> C <sub>6</sub> | 3 B <sub>13</sub> C <sub>2</sub> + 14.78 H <sub>3</sub> N + 45.33 ThN → 14.78 Th <sub>3</sub> N <sub>4</sub> + 3.667 B <sub>9</sub> H <sub>11</sub> + ThB <sub>6</sub> H <sub>4</sub> C <sub>6</sub> N                                | -5.8687             |
| ThNH <sub>4</sub> B <sub>6</sub> C <sub>6</sub> | 6 ThC + 0.6667 B <sub>9</sub> H <sub>11</sub> + 2.167 N <sub>2</sub> → 1.667 ThH <sub>2</sub> + 3.333 ThN + ThB <sub>6</sub> H <sub>4</sub> C <sub>6</sub> N                                                                          | -5.8507             |
| ThNH <sub>4</sub> B <sub>6</sub> C <sub>6</sub> | 0.5714 B <sub>5</sub> H <sub>7</sub> + 2 Th <sub>2</sub> C <sub>3</sub> + 2.849 N <sub>2</sub> + 0.5238 ThB <sub>6</sub> → 1.175 Th <sub>3</sub> N <sub>4</sub> + ThB <sub>6</sub> H <sub>4</sub> C <sub>6</sub> N                    | -5.8314             |
| ThNH <sub>4</sub> B <sub>6</sub> C <sub>6</sub> | 2 ThH <sub>2</sub> + 0.4615 B <sub>13</sub> C <sub>2</sub> + 1.692 Th <sub>2</sub> C <sub>3</sub> + 2.692 N <sub>2</sub> → 4.385 ThN + ThB <sub>6</sub> H <sub>4</sub> C <sub>6</sub> N                                               | -5.7594             |
| ThNH <sub>4</sub> B <sub>6</sub> C <sub>6</sub> | 0.3636 B <sub>9</sub> H <sub>11</sub> + 2 Th <sub>2</sub> C <sub>3</sub> + 2.803 N <sub>2</sub> + 0.4545 ThB <sub>6</sub> → 1.152 Th <sub>3</sub> N <sub>4</sub> + ThB <sub>6</sub> H <sub>4</sub> C <sub>6</sub> N                   | -5.7426             |
| ThNH <sub>4</sub> B <sub>6</sub> C <sub>6</sub> | 0.5714 B <sub>5</sub> H <sub>7</sub> + 6 ThC + 0.5 N <sub>2</sub> + 11.57 ThB <sub>6</sub> → 16.57 ThB <sub>4</sub> + ThB <sub>6</sub> H <sub>4</sub> C <sub>6</sub> N                                                                | -5.7252             |
| ThNH <sub>4</sub> B <sub>6</sub> C <sub>6</sub> | 6 ThC + 0.3636 B <sub>9</sub> H <sub>11</sub> + 0.5 N <sub>2</sub> + 11.36 ThB <sub>6</sub> → 16.36 ThB <sub>4</sub> + ThB <sub>6</sub> H <sub>4</sub> C <sub>6</sub> N                                                               | -5.7229             |
| ThNH <sub>4</sub> B <sub>6</sub> C <sub>6</sub> | 6 ThC + 19.57 B + 7.667 H <sub>3</sub> N → 2.714 B <sub>5</sub> H <sub>7</sub> + 1.667 Th <sub>3</sub> N <sub>4</sub> + ThB <sub>6</sub> H <sub>4</sub> C <sub>6</sub> N                                                              | -5.7053             |
| ThNH <sub>4</sub> B <sub>6</sub> C <sub>6</sub> | 2 ThH <sub>2</sub> + 0.25 Th <sub>3</sub> N <sub>4</sub> + 3 ThC <sub>2</sub> + 34.5 B → 4.75 ThB <sub>6</sub> + ThB <sub>6</sub> H <sub>4</sub> C <sub>6</sub> N                                                                     | -5.6992             |
| ThNH <sub>4</sub> B <sub>6</sub> C <sub>6</sub> | 1.967 Th <sub>3</sub> N <sub>4</sub> + 0.3636 B <sub>9</sub> H <sub>11</sub> + 3 B <sub>13</sub> C <sub>2</sub> → 6.868 BN + 4.901 ThB <sub>6</sub> + ThB <sub>6</sub> H <sub>4</sub> C <sub>6</sub> N                                | -5.6812             |
| ThNH <sub>4</sub> B <sub>6</sub> C <sub>6</sub> | 6 ThC + 0.9934 B <sub>9</sub> H <sub>11</sub> + 3.941 H <sub>3</sub> N → 1.25 Th <sub>4</sub> H <sub>15</sub> + 2.941 BN + ThB <sub>6</sub> H <sub>4</sub> C <sub>6</sub> N                                                           | -5.6574             |
| ThNH <sub>4</sub> B <sub>6</sub> C <sub>6</sub> | 2 ThH <sub>2</sub> + 6 ThC + BN + 16.5 ThB <sub>6</sub> → 23.5 ThB <sub>4</sub> + ThB <sub>6</sub> H <sub>4</sub> C <sub>6</sub> N                                                                                                    | -5.6544             |
| ThNH <sub>4</sub> B <sub>6</sub> C <sub>6</sub> | 6 ThC + 0.2667 Th <sub>4</sub> H <sub>15</sub> + 17.13 ThB <sub>6</sub> + ThN → 24.2 ThB <sub>4</sub> + ThB <sub>6</sub> H <sub>4</sub> C <sub>6</sub> N                                                                              | -5.6346             |
| ThNH <sub>4</sub> B <sub>6</sub> C <sub>6</sub> | 2 ThH <sub>2</sub> + 2.538 ThC <sub>2</sub> + 0.4615 B <sub>13</sub> C <sub>2</sub> + 2.859 N <sub>2</sub> → 1.179 Th <sub>3</sub> N <sub>4</sub> + ThB <sub>6</sub> H <sub>4</sub> C <sub>6</sub> N                                  | -5.6315             |
| ThNH <sub>4</sub> B <sub>6</sub> C <sub>6</sub> | 0.5714 B <sub>5</sub> H <sub>7</sub> + 2 Th <sub>2</sub> C <sub>3</sub> + 3.143 B + 2.5 N <sub>2</sub> → Th <sub>3</sub> N <sub>4</sub> + ThB <sub>6</sub> H <sub>4</sub> C <sub>6</sub> N                                            | -5.6308             |
| ThNH <sub>4</sub> B <sub>6</sub> C <sub>6</sub> | 5.598 B <sub>5</sub> H <sub>7</sub> + 9.383 ThC + ThN → 2.346 Th <sub>4</sub> H <sub>15</sub> + 1.692 B <sub>13</sub> C <sub>2</sub> + ThB <sub>6</sub> H <sub>4</sub> C <sub>6</sub> N                                               | -5.6299             |
| ThNH <sub>4</sub> B <sub>6</sub> C <sub>6</sub> | 6 ThC + 20.25 B <sub>9</sub> H <sub>11</sub> + 0.5 N <sub>2</sub> → 5 ThB <sub>4</sub> + 31.25 B <sub>5</sub> H <sub>7</sub> + ThB <sub>6</sub> H <sub>4</sub> C <sub>6</sub> N                                                       | -5.5973             |
| ThNH <sub>4</sub> B <sub>6</sub> C <sub>6</sub> | 0.5714 B <sub>5</sub> H <sub>7</sub> + 1.948 Th <sub>3</sub> N <sub>4</sub> + 3 B <sub>13</sub> C <sub>2</sub> → 6.792 BN + 4.844 ThB <sub>6</sub> + ThB <sub>6</sub> H <sub>4</sub> C <sub>6</sub> N                                 | -5.5713             |
| ThNH <sub>4</sub> B <sub>6</sub> C <sub>6</sub> | 0.3636 B <sub>9</sub> H <sub>11</sub> + 2 Th <sub>2</sub> C <sub>3</sub> + 2.727 B + 2.5 N <sub>2</sub> → Th <sub>3</sub> N <sub>4</sub> + ThB <sub>6</sub> H <sub>4</sub> C <sub>6</sub> N                                           | -5.5685             |
| ThNH <sub>4</sub> B <sub>6</sub> C <sub>6</sub> | 3 B <sub>13</sub> C <sub>2</sub> + 1.333 H <sub>3</sub> N + 5.524 ThN → 5.857 BN + 4.524 ThB <sub>6</sub> + ThB <sub>6</sub> H <sub>4</sub> C <sub>6</sub> N                                                                          | -5.5613             |
| ThNH <sub>4</sub> B <sub>6</sub> C <sub>6</sub> | 4.042 ThC <sub>2</sub> + 0.6667 B <sub>9</sub> H <sub>11</sub> + 2.528 N <sub>2</sub> → 1.014 Th <sub>3</sub> N <sub>4</sub> + 0.4167 H <sub>8</sub> C <sub>5</sub> + ThB <sub>6</sub> H <sub>4</sub> C <sub>6</sub> N                | -5.5475             |
| ThNH <sub>4</sub> B <sub>6</sub> C <sub>6</sub> | 1.5 ThB <sub>4</sub> + 0.2667 Th <sub>4</sub> H <sub>15</sub> + 3 ThC <sub>2</sub> + 3.544 N <sub>2</sub> → 1.522 Th <sub>3</sub> N <sub>4</sub> + ThB <sub>6</sub> H <sub>4</sub> C <sub>6</sub> N                                   | -5.5448             |
| ThNH <sub>4</sub> B <sub>6</sub> C <sub>6</sub> | 6 ThC + 29 B <sub>9</sub> H <sub>11</sub> + 0.5 N <sub>2</sub> → 45 B <sub>5</sub> H <sub>7</sub> + 5 ThB <sub>6</sub> + ThB <sub>6</sub> H <sub>4</sub> C <sub>6</sub> N                                                             | -5.5420             |
| ThNH <sub>4</sub> B <sub>6</sub> C <sub>6</sub> | 0.2667 Th <sub>4</sub> H <sub>15</sub> + 0.4615 B <sub>13</sub> C <sub>2</sub> + 1.692 Th <sub>2</sub> C <sub>3</sub> + 2.801 N <sub>2</sub> → 1.15 Th <sub>3</sub> N <sub>4</sub> + ThB <sub>6</sub> H <sub>4</sub> C <sub>6</sub> N | -5.5056             |
| ThNH <sub>4</sub> B <sub>6</sub> C <sub>6</sub> | 1.5 ThB <sub>4</sub> + 2 Th <sub>2</sub> C <sub>3</sub> + 1.333 H <sub>3</sub> N + 2.833 N <sub>2</sub> → 1.5 Th <sub>3</sub> N <sub>4</sub> + ThB <sub>6</sub> H <sub>4</sub> C <sub>6</sub> N                                       | -5.4699             |
| ThNH <sub>4</sub> B <sub>6</sub> C <sub>6</sub> | 2.8 B <sub>5</sub> H <sub>7</sub> + 3 ThC <sub>2</sub> + 3.1 N <sub>2</sub> → 2 ThB <sub>4</sub> + 5.2 H <sub>3</sub> N + ThB <sub>6</sub> H <sub>4</sub> C <sub>6</sub> N                                                            | -5.4697             |
| ThNH <sub>4</sub> B <sub>6</sub> C <sub>6</sub> | 1.5 ThB <sub>4</sub> + 0.2667 Th <sub>4</sub> H <sub>15</sub> + 2 Th <sub>2</sub> C <sub>3</sub> + 3.283 N <sub>2</sub> → 5.567 ThN + ThB <sub>6</sub> H <sub>4</sub> C <sub>6</sub> N                                                | -5.4565             |
| ThNH <sub>4</sub> B <sub>6</sub> C <sub>6</sub> | 12 ThH <sub>2</sub> + BN + 3 B <sub>13</sub> C <sub>2</sub> → 1.333 Th <sub>4</sub> H <sub>15</sub> + 5.667 ThB <sub>6</sub> + ThB <sub>6</sub> H <sub>4</sub> C <sub>6</sub> N                                                       | -5.4221             |
| ThNH <sub>4</sub> B <sub>6</sub> C <sub>6</sub> | 0.2667 Th <sub>4</sub> H <sub>15</sub> + 2 Th <sub>2</sub> C <sub>3</sub> + 6 B + 2.533 N <sub>2</sub> → 4.067 ThN + ThB <sub>6</sub> H <sub>4</sub> C <sub>6</sub> N                                                                 | -5.3821             |
| ThNH <sub>4</sub> B <sub>6</sub> C <sub>6</sub> | 6 ThC + 2.727 BN + 0.3636 B <sub>9</sub> H <sub>11</sub> + 2.47 N <sub>2</sub> → 1.667 Th <sub>3</sub> N <sub>4</sub> + ThB <sub>6</sub> H <sub>4</sub> C <sub>6</sub> N                                                              | -5.3604             |
| ThNH <sub>4</sub> B <sub>6</sub> C <sub>6</sub> | 0.25 Th <sub>3</sub> N <sub>4</sub> + 6 ThC + 0.2667 Th <sub>4</sub> H <sub>15</sub> + 16.63 ThB <sub>6</sub> → 23.45 ThB <sub>4</sub> + ThB <sub>6</sub> H <sub>4</sub> C <sub>6</sub> N                                             | -5.3248             |

Continued on next page

Continued

| Compound                                        | Chemical reaction                                                                                                                                                                            | Reaction energy(eV) |
|-------------------------------------------------|----------------------------------------------------------------------------------------------------------------------------------------------------------------------------------------------|---------------------|
| ThNH <sub>4</sub> B <sub>6</sub> C <sub>6</sub> | $2\text{H}_2 + 2\text{Th}_2\text{C}_3 + 30\text{B} + \text{ThN} \rightarrow 4\text{ThB}_6 + \text{ThB}_6\text{H}_4\text{C}_6\text{N}$                                                        | -5.3181             |
| ThNH <sub>4</sub> B <sub>6</sub> C <sub>6</sub> | $9.25\text{ThH}_2 + 3\text{B}_{13}\text{C}_2 + \text{H}_3\text{N} \rightarrow 8.25\text{ThB}_4 + 8.75\text{H}_2 + \text{ThB}_6\text{H}_4\text{C}_6\text{N}$                                  | -5.2983             |
| ThNH <sub>4</sub> B <sub>6</sub> C <sub>6</sub> | $6\text{ThC} + 2\text{H}_2 + 15\text{ThB}_6 + \text{ThN} \rightarrow 21\text{ThB}_4 + \text{ThB}_6\text{H}_4\text{C}_6\text{N}$                                                              | -5.2832             |
| ThNH <sub>4</sub> B <sub>6</sub> C <sub>6</sub> | $5.077\text{ThC} + 0.4615\text{B}_{13}\text{C}_2 + 1.333\text{H}_3\text{N} + 1.872\text{N}_2 \rightarrow 4.077\text{ThN} + \text{ThB}_6\text{H}_4\text{C}_6\text{N}$                         | -5.2680             |
| ThNH <sub>4</sub> B <sub>6</sub> C <sub>6</sub> | $5.37\text{B}_5\text{H}_7 + 0.25\text{Th}_3\text{N}_4 + 9.208\text{ThC} \rightarrow 2.239\text{Th}_4\text{H}_{15} + 1.604\text{B}_{13}\text{C}_2 + \text{ThB}_6\text{H}_4\text{C}_6\text{N}$ | -5.2621             |
| ThNH <sub>4</sub> B <sub>6</sub> C <sub>6</sub> | $2\text{Th}_2\text{C}_3 + 10.08\text{B} + 5.083\text{H}_3\text{N} \rightarrow 0.75\text{Th}_4\text{H}_{15} + 4.083\text{BN} + \text{ThB}_6\text{H}_4\text{C}_6\text{N}$                      | -5.2433             |
| ThNH <sub>4</sub> B <sub>6</sub> C <sub>6</sub> | $0.2667\text{Th}_4\text{H}_{15} + 3\text{B}_{13}\text{C}_2 + 29.73\text{ThN} \rightarrow 8.25\text{ThB}_4 + 7.183\text{Th}_3\text{N}_4 + \text{ThB}_6\text{H}_4\text{C}_6\text{N}$           | -5.2262             |
| ThNH <sub>4</sub> B <sub>6</sub> C <sub>6</sub> | $1.716\text{B}_5\text{H}_7 + 6\text{ThC} + 3.58\text{H}_3\text{N} \rightarrow 1.25\text{Th}_4\text{H}_{15} + 2.58\text{BN} + \text{ThB}_6\text{H}_4\text{C}_6\text{N}$                       | -5.2168             |
| ThNH <sub>4</sub> B <sub>6</sub> C <sub>6</sub> | $0.2667\text{Th}_4\text{H}_{15} + 2\text{Th}_2\text{C}_3 + 22.27\text{B} + 0.5\text{N}_2 \rightarrow 4.067\text{ThB}_4 + \text{ThB}_6\text{H}_4\text{C}_6\text{N}$                           | -5.1804             |
| ThNH <sub>4</sub> B <sub>6</sub> C <sub>6</sub> | $2.75\text{B}_9\text{H}_{11} + 2\text{Th}_2\text{C}_3 + 2.5\text{N}_2 \rightarrow 3.75\text{B}_5\text{H}_7 + \text{Th}_3\text{N}_4 + \text{ThB}_6\text{H}_4\text{C}_6\text{N}$               | -5.1599             |
| ThNH <sub>4</sub> B <sub>6</sub> C <sub>6</sub> | $0.2667\text{Th}_4\text{H}_{15} + 2\text{Th}_2\text{C}_3 + 3.033\text{N}_2 + \text{ThB}_6 \rightarrow 5.067\text{ThN} + \text{ThB}_6\text{H}_4\text{C}_6\text{N}$                            | -5.1431             |
| ThNH <sub>4</sub> B <sub>6</sub> C <sub>6</sub> | $0.2667\text{Th}_4\text{H}_{15} + 2\text{Th}_2\text{C}_3 + 26.27\text{B} + \text{ThN} \rightarrow 5.067\text{ThB}_4 + \text{ThB}_6\text{H}_4\text{C}_6\text{N}$                              | -5.1307             |
| ThNH <sub>4</sub> B <sub>6</sub> C <sub>6</sub> | $6\text{ThC} + 11.37\text{H}_2 + 6\text{B} + 0.5\text{N}_2 \rightarrow 1.25\text{Th}_4\text{H}_{15} + \text{ThB}_6\text{H}_4\text{C}_6\text{N}$                                              | -5.1285             |
| ThNH <sub>4</sub> B <sub>6</sub> C <sub>6</sub> | $0.5\text{ThH}_2 + 6\text{ThC} + \text{H}_3\text{N} + 14\text{ThB}_6 \rightarrow 19.5\text{ThB}_4 + \text{ThB}_6\text{H}_4\text{C}_6\text{N}$                                                | -5.1277             |
| ThNH <sub>4</sub> B <sub>6</sub> C <sub>6</sub> | $10.04\text{ThH}_2 + 0.25\text{Th}_3\text{N}_4 + 3\text{B}_{13}\text{C}_2 \rightarrow 1.071\text{Th}_4\text{H}_{15} + 5.5\text{ThB}_6 + \text{ThB}_6\text{H}_4\text{C}_6\text{N}$            | -5.1249             |
| ThNH <sub>4</sub> B <sub>6</sub> C <sub>6</sub> | $2.25\text{B}_{13}\text{C}_2 + 0.5\text{Th}_2\text{C}_3 + 7.967\text{H}_3\text{N} \rightarrow 6.967\text{BN} + 1.809\text{B}_9\text{H}_{11} + \text{ThB}_6\text{H}_4\text{C}_6\text{N}$      | -5.1140             |
| ThNH <sub>4</sub> B <sub>6</sub> C <sub>6</sub> | $8.96\text{ThC} + 2.805\text{B}_9\text{H}_{11} + \text{H}_3\text{N} \rightarrow 1.99\text{Th}_4\text{H}_{15} + 1.48\text{B}_{13}\text{C}_2 + \text{ThB}_6\text{H}_4\text{C}_6\text{N}$       | -5.1129             |
| ThNH <sub>4</sub> B <sub>6</sub> C <sub>6</sub> | $1.5\text{ThB}_4 + 3.5\text{ThC} + 0.5\text{H}_8\text{C}_5 + 3.167\text{N}_2 \rightarrow 1.333\text{Th}_3\text{N}_4 + \text{ThB}_6\text{H}_4\text{C}_6\text{N}$                              | -5.1084             |
| ThNH <sub>4</sub> B <sub>6</sub> C <sub>6</sub> | $2\text{ThH}_2 + 1.5\text{ThB}_4 + 3\text{ThC}_2 + 3.25\text{N}_2 \rightarrow 5.5\text{ThN} + \text{ThB}_6\text{H}_4\text{C}_6\text{N}$                                                      | -5.1048             |
| ThNH <sub>4</sub> B <sub>6</sub> C <sub>6</sub> | $0.5714\text{B}_5\text{H}_7 + 6\text{ThC} + 13.57\text{ThB}_6 + \text{ThN} \rightarrow 19.57\text{ThB}_4 + \text{ThB}_6\text{H}_4\text{C}_6\text{N}$                                         | -5.0983             |
| ThNH <sub>4</sub> B <sub>6</sub> C <sub>6</sub> | $6\text{ThC} + 0.3636\text{B}_9\text{H}_{11} + 13.36\text{ThB}_6 + \text{ThN} \rightarrow 19.36\text{ThB}_4 + \text{ThB}_6\text{H}_4\text{C}_6\text{N}$                                      | -5.0960             |
| ThNH <sub>4</sub> B <sub>6</sub> C <sub>6</sub> | $0.3636\text{B}_9\text{H}_{11} + 3\text{B}_{13}\text{C}_2 + 6.182\text{ThN} \rightarrow 5.182\text{BN} + 5.182\text{ThB}_6 + \text{ThB}_6\text{H}_4\text{C}_6\text{N}$                       | -5.0912             |
| ThNH <sub>4</sub> B <sub>6</sub> C <sub>6</sub> | $2\text{H}_2 + 2\text{Th}_2\text{C}_3 + 24\text{B} + 0.5\text{N}_2 \rightarrow 3\text{ThB}_6 + \text{ThB}_6\text{H}_4\text{C}_6\text{N}$                                                     | -5.0791             |
| ThNH <sub>4</sub> B <sub>6</sub> C <sub>6</sub> | $1.2\text{B}_5\text{H}_7 + 2\text{Th}_2\text{C}_3 + 2.733\text{N}_2 \rightarrow 1.467\text{H}_3\text{N} + 3\text{ThN} + \text{ThB}_6\text{H}_4\text{C}_6\text{N}$                            | -5.0500             |
| ThNH <sub>4</sub> B <sub>6</sub> C <sub>6</sub> | $7.342\text{ThH}_2 + 3\text{B}_{13}\text{C}_2 + 0.5\text{N}_2 \rightarrow 6.342\text{ThB}_4 + 1.526\text{B}_5\text{H}_7 + \text{ThB}_6\text{H}_4\text{C}_6\text{N}$                          | -5.0490             |
| ThNH <sub>4</sub> B <sub>6</sub> C <sub>6</sub> | $2\text{ThH}_2 + 3\text{ThC}_2 + 6\text{B} + 2.5\text{N}_2 \rightarrow 4\text{ThN} + \text{ThB}_6\text{H}_4\text{C}_6\text{N}$                                                               | -5.0304             |
| ThNH <sub>4</sub> B <sub>6</sub> C <sub>6</sub> | $1.2\text{B}_5\text{H}_7 + 9.5\text{Th} + \text{H}_3\text{N} + 1.2\text{H}_8\text{C}_5 \rightarrow 8.5\text{ThH}_2 + \text{ThB}_6\text{H}_4\text{C}_6\text{N}$                               | -5.0226             |
| ThNH <sub>4</sub> B <sub>6</sub> C <sub>6</sub> | $0.6667\text{B}_9\text{H}_{11} + 2\text{Th}_2\text{C}_3 + 2.5\text{N}_2 \rightarrow \text{Th}_3\text{N}_4 + 1.667\text{H}_2 + \text{ThB}_6\text{H}_4\text{C}_6\text{N}$                      | -5.0190             |
| ThNH <sub>4</sub> B <sub>6</sub> C <sub>6</sub> | $0.5714\text{B}_5\text{H}_7 + 3\text{B}_{13}\text{C}_2 + 6.122\text{ThN} \rightarrow 5.122\text{BN} + 5.122\text{ThB}_6 + \text{ThB}_6\text{H}_4\text{C}_6\text{N}$                          | -4.9869             |
| ThNH <sub>4</sub> B <sub>6</sub> C <sub>6</sub> | $1.818\text{Th}_3\text{N}_4 + 2\text{H}_2 + 3\text{B}_{13}\text{C}_2 \rightarrow 6.273\text{BN} + 4.455\text{ThB}_6 + \text{ThB}_6\text{H}_4\text{C}_6\text{N}$                              | -4.9843             |
| ThNH <sub>4</sub> B <sub>6</sub> C <sub>6</sub> | $1.2\text{B}_5\text{H}_7 + 2\text{Th}_2\text{C}_3 + 2.5\text{N}_2 \rightarrow \text{Th}_3\text{N}_4 + 2.2\text{H}_2 + \text{ThB}_6\text{H}_4\text{C}_6\text{N}$                              | -4.9739             |
| ThNH <sub>4</sub> B <sub>6</sub> C <sub>6</sub> | $0.25\text{Th}_3\text{N}_4 + 6\text{ThC} + 2\text{H}_2 + 14.5\text{ThB}_6 \rightarrow 20.25\text{ThB}_4 + \text{ThB}_6\text{H}_4\text{C}_6\text{N}$                                          | -4.9734             |
| ThNH <sub>4</sub> B <sub>6</sub> C <sub>6</sub> | $2\text{ThH}_2 + \text{BN} + 2\text{Th}_2\text{C}_3 + 25\text{B} \rightarrow 5\text{ThB}_4 + \text{ThB}_6\text{H}_4\text{C}_6\text{N}$                                                       | -4.9678             |
| ThNH <sub>4</sub> B <sub>6</sub> C <sub>6</sub> | $6\text{ThC} + 1.333\text{H}_3\text{N} + 13.17\text{ThB}_6 \rightarrow 18.17\text{ThB}_4 + 0.3333\text{BN} + \text{ThB}_6\text{H}_4\text{C}_6\text{N}$                                       | -4.9521             |
| ThNH <sub>4</sub> B <sub>6</sub> C <sub>6</sub> | $9.5\text{ThH}_2 + 3\text{B}_{13}\text{C}_2 + \text{ThN} \rightarrow \text{Th}_4\text{H}_{15} + 5.5\text{ThB}_6 + \text{ThB}_6\text{H}_4\text{C}_6\text{N}$                                  | -4.9484             |
| ThNH <sub>4</sub> B <sub>6</sub> C <sub>6</sub> | $6\text{ThC} + 23.75\text{B}_9\text{H}_{11} + \text{ThN} \rightarrow 6\text{ThB}_4 + 36.75\text{B}_5\text{H}_7 + \text{ThB}_6\text{H}_4\text{C}_6\text{N}$                                   | -4.9484             |
| ThNH <sub>4</sub> B <sub>6</sub> C <sub>6</sub> | $0.25\text{Th}_3\text{N}_4 + 1.75\text{B}_{13}\text{C}_2 + 4.437\text{Th} + 0.5\text{H}_8\text{C}_5 \rightarrow 4.187\text{ThB}_4 + \text{ThB}_6\text{H}_4\text{C}_6\text{N}$                | -4.9316             |
| ThNH <sub>4</sub> B <sub>6</sub> C <sub>6</sub> | $9.967\text{ThC} + \text{BN} + 3.421\text{B}_9\text{H}_{11} \rightarrow 2.242\text{Th}_4\text{H}_{15} + 1.983\text{B}_{13}\text{C}_2 + \text{ThB}_6\text{H}_4\text{C}_6\text{N}$             | -4.9277             |
| ThNH <sub>4</sub> B <sub>6</sub> C <sub>6</sub> | $0.2667\text{Th}_4\text{H}_{15} + 3\text{ThC}_2 + 3.211\text{N}_2 + \text{ThB}_6 \rightarrow 1.356\text{Th}_3\text{N}_4 + \text{ThB}_6\text{H}_4\text{C}_6\text{N}$                          | -4.9203             |
| ThNH <sub>4</sub> B <sub>6</sub> C <sub>6</sub> | $8.25\text{ThH}_2 + 3\text{B}_{13}\text{C}_2 + \text{ThN} \rightarrow 8.25\text{ThB}_4 + 6.25\text{H}_2 + \text{ThB}_6\text{H}_4\text{C}_6\text{N}$                                          | -4.9121             |
| ThNH <sub>4</sub> B <sub>6</sub> C <sub>6</sub> | $1.2\text{B}_5\text{H}_7 + 6\text{ThC} + 1.9\text{N}_2 \rightarrow 2.2\text{ThH}_2 + 2.8\text{ThN} + \text{ThB}_6\text{H}_4\text{C}_6\text{N}$                                               | -4.8935             |
| ThNH <sub>4</sub> B <sub>6</sub> C <sub>6</sub> | $6\text{ThC} + 34.25\text{B}_9\text{H}_{11} + \text{ThN} \rightarrow 53.25\text{B}_5\text{H}_7 + 6\text{ThB}_6 + \text{ThB}_6\text{H}_4\text{C}_6\text{N}$                                   | -4.8820             |
| ThNH <sub>4</sub> B <sub>6</sub> C <sub>6</sub> | $8.5\text{ThH}_2 + 0.25\text{Th}_3\text{N}_4 + 3\text{B}_{13}\text{C}_2 \rightarrow 8.25\text{ThB}_4 + 6.5\text{H}_2 + \text{ThB}_6\text{H}_4\text{C}_6\text{N}$                             | -4.8732             |
| ThNH <sub>4</sub> B <sub>6</sub> C <sub>6</sub> | $2\text{Th}_2\text{C}_3 + 1.333\text{H}_3\text{N} + 2.5\text{N}_2 + \text{ThB}_6 \rightarrow 1.333\text{Th}_3\text{N}_4 + \text{ThB}_6\text{H}_4\text{C}_6\text{N}$                          | -4.8455             |
| ThNH <sub>4</sub> B <sub>6</sub> C <sub>6</sub> | $2\text{ThH}_2 + 3\text{ThC}_2 + 22\text{B} + 0.5\text{N}_2 \rightarrow 4\text{ThB}_4 + \text{ThB}_6\text{H}_4\text{C}_6\text{N}$                                                            | -4.8320             |
| ThNH <sub>4</sub> B <sub>6</sub> C <sub>6</sub> | $7.145\text{ThH}_2 + 3\text{B}_{13}\text{C}_2 + 0.5\text{N}_2 \rightarrow 6.145\text{ThB}_4 + 0.9355\text{B}_9\text{H}_{11} + \text{ThB}_6\text{H}_4\text{C}_6\text{N}$                      | -4.8234             |
| ThNH <sub>4</sub> B <sub>6</sub> C <sub>6</sub> | $0.25\text{Th}_3\text{N}_4 + 2\text{H}_2 + 2\text{Th}_2\text{C}_3 + 28.5\text{B} \rightarrow 3.75\text{ThB}_6 + \text{ThB}_6\text{H}_4\text{C}_6\text{N}$                                    | -4.7918             |
| ThNH <sub>4</sub> B <sub>6</sub> C <sub>6</sub> | $2\text{ThH}_2 + 3\text{ThC}_2 + 3\text{N}_2 + \text{ThB}_6 \rightarrow 5\text{ThN} + \text{ThB}_6\text{H}_4\text{C}_6\text{N}$                                                              | -4.7914             |
| ThNH <sub>4</sub> B <sub>6</sub> C <sub>6</sub> | $0.5714\text{B}_5\text{H}_7 + 0.25\text{Th}_3\text{N}_4 + 6\text{ThC} + 13.07\text{ThB}_6 \rightarrow 18.82\text{ThB}_4 + \text{ThB}_6\text{H}_4\text{C}_6\text{N}$                          | -4.7885             |
| ThNH <sub>4</sub> B <sub>6</sub> C <sub>6</sub> | $0.25\text{Th}_3\text{N}_4 + 6\text{ThC} + 0.3636\text{B}_9\text{H}_{11} + 12.86\text{ThB}_6 \rightarrow 18.61\text{ThB}_4 + \text{ThB}_6\text{H}_4\text{C}_6\text{N}$                       | -4.7862             |
| ThNH <sub>4</sub> B <sub>6</sub> C <sub>6</sub> | $2\text{ThH}_2 + 3\text{ThC}_2 + 26\text{B} + \text{ThN} \rightarrow 5\text{ThB}_4 + \text{ThB}_6\text{H}_4\text{C}_6\text{N}$                                                               | -4.7824             |
| ThNH <sub>4</sub> B <sub>6</sub> C <sub>6</sub> | $\text{ThC}_2 + 0.75\text{B}_{13}\text{C}_2 + 0.5\text{H}_8\text{C}_5 + 2.375\text{N}_2 \rightarrow 3.75\text{BN} + \text{ThB}_6\text{H}_4\text{C}_6\text{N}$                                | -4.7300             |
| ThNH <sub>4</sub> B <sub>6</sub> C <sub>6</sub> | $0.5\text{ThH}_2 + 2\text{Th}_2\text{C}_3 + 27\text{B} + \text{H}_3\text{N} \rightarrow 3.5\text{ThB}_6 + \text{ThB}_6\text{H}_4\text{C}_6\text{N}$                                          | -4.7296             |
| ThNH <sub>4</sub> B <sub>6</sub> C <sub>6</sub> | $0.5714\text{B}_5\text{H}_7 + 2\text{Th}_2\text{C}_3 + 27.14\text{B} + \text{ThN} \rightarrow 4\text{ThB}_6 + \text{ThB}_6\text{H}_4\text{C}_6\text{N}$                                      | -4.7209             |
| ThNH <sub>4</sub> B <sub>6</sub> C <sub>6</sub> | $0.25\text{Th}_3\text{N}_4 + 0.2667\text{Th}_4\text{H}_{15} + 2\text{Th}_2\text{C}_3 + 25.27\text{B} \rightarrow 4.817\text{ThB}_4 + \text{ThB}_6\text{H}_4\text{C}_6\text{N}$               | -4.6767             |
| ThNH <sub>4</sub> B <sub>6</sub> C <sub>6</sub> | $6\text{ThC} + 0.06667\text{Th}_4\text{H}_{15} + \text{H}_3\text{N} + 13.53\text{ThB}_6 \rightarrow 18.8\text{ThB}_4 + \text{ThB}_6\text{H}_4\text{C}_6\text{N}$                             | -4.6738             |
| ThNH <sub>4</sub> B <sub>6</sub> C <sub>6</sub> | $0.3636\text{B}_9\text{H}_{11} + 2\text{Th}_2\text{C}_3 + 26.73\text{B} + \text{ThN} \rightarrow 4\text{ThB}_6 + \text{ThB}_6\text{H}_4\text{C}_6\text{N}$                                   | -4.6586             |
| ThNH <sub>4</sub> B <sub>6</sub> C <sub>6</sub> | $1.2\text{B}_5\text{H}_7 + 4.375\text{ThC}_2 + 2.187\text{N}_2 \rightarrow 0.55\text{H}_8\text{C}_5 + 3.375\text{ThN} + \text{ThB}_6\text{H}_4\text{C}_6\text{N}$                            | -4.6520             |
| ThNH <sub>4</sub> B <sub>6</sub> C <sub>6</sub> | $0.25\text{Th}_3\text{N}_4 + 6\text{ThC} + 22.88\text{B}_9\text{H}_{11} \rightarrow 5.75\text{ThB}_4 + 35.38\text{B}_5\text{H}_7 + \text{ThB}_6\text{H}_4\text{C}_6\text{N}$                 | -4.6441             |
| ThNH <sub>4</sub> B <sub>6</sub> C <sub>6</sub> | $0.6667\text{B}_9\text{H}_{11} + 2\text{Th}_2\text{C}_3 + 2.556\text{N}_2 \rightarrow 1.111\text{H}_3\text{N} + 3\text{ThN} + \text{ThB}_6\text{H}_4\text{C}_6\text{N}$                      | -4.6243             |

Continued on next page

Continued

| Compound                                        | Chemical reaction                                                                                                                                                                                                                     | Reaction energy(eV) |
|-------------------------------------------------|---------------------------------------------------------------------------------------------------------------------------------------------------------------------------------------------------------------------------------------|---------------------|
| ThNH <sub>4</sub> B <sub>6</sub> C <sub>6</sub> | 1.75 B <sub>13</sub> C <sub>2</sub> + 4.187 Th + 0.5 H <sub>8</sub> C <sub>5</sub> + ThN → 4.187 ThB <sub>4</sub> + ThB <sub>6</sub> H <sub>4</sub> C <sub>6</sub> N                                                                  | -4.6112             |
| ThNH <sub>4</sub> B <sub>6</sub> C <sub>6</sub> | 6 ThC + 9.667 B + 4.667 H <sub>3</sub> N → 5 ThH <sub>2</sub> + 3.667 BN + ThB <sub>6</sub> H <sub>4</sub> C <sub>6</sub> N                                                                                                           | -4.5912             |
| ThNH <sub>4</sub> B <sub>6</sub> C <sub>6</sub> | 6 ThC + 0.5 H <sub>2</sub> + H <sub>3</sub> N + 13 ThB <sub>6</sub> → 18 ThB <sub>4</sub> + ThB <sub>6</sub> H <sub>4</sub> C <sub>6</sub> N                                                                                          | -4.5859             |
| ThNH <sub>4</sub> B <sub>6</sub> C <sub>6</sub> | 0.25 Th <sub>3</sub> N <sub>4</sub> + 6 ThC + 32.94 B <sub>9</sub> H <sub>11</sub> → 51.19 B <sub>5</sub> H <sub>7</sub> + 5.75 ThB <sub>6</sub> + ThB <sub>6</sub> H <sub>4</sub> C <sub>6</sub> N                                   | -4.5806             |
| ThNH <sub>4</sub> B <sub>6</sub> C <sub>6</sub> | 0.1429 B <sub>5</sub> H <sub>7</sub> + 6 ThC + H <sub>3</sub> N + 12.64 ThB <sub>6</sub> → 17.64 ThB <sub>4</sub> + ThB <sub>6</sub> H <sub>4</sub> C <sub>6</sub> N                                                                  | -4.5397             |
| ThNH <sub>4</sub> B <sub>6</sub> C <sub>6</sub> | 6 ThC + 0.09091 B <sub>9</sub> H <sub>11</sub> + H <sub>3</sub> N + 12.59 ThB <sub>6</sub> → 17.59 ThB <sub>4</sub> + ThB <sub>6</sub> H <sub>4</sub> C <sub>6</sub> N                                                                | -4.5392             |
| ThNH <sub>4</sub> B <sub>6</sub> C <sub>6</sub> | 0.2667 Th <sub>4</sub> H <sub>15</sub> + 3 ThC <sub>2</sub> + 6 B + 2.544 N <sub>2</sub> → 1.022 Th <sub>3</sub> N <sub>4</sub> + ThB <sub>6</sub> H <sub>4</sub> C <sub>6</sub> N                                                    | -4.5374             |
| ThNH <sub>4</sub> B <sub>6</sub> C <sub>6</sub> | 3.5 ThC + 0.5 H <sub>8</sub> C <sub>5</sub> + 2.833 N <sub>2</sub> + ThB <sub>6</sub> → 1.167 Th <sub>3</sub> N <sub>4</sub> + ThB <sub>6</sub> H <sub>4</sub> C <sub>6</sub> N                                                       | -4.4840             |
| ThNH <sub>4</sub> B <sub>6</sub> C <sub>6</sub> | 0.5714 B <sub>5</sub> H <sub>7</sub> + 2 Th <sub>2</sub> C <sub>3</sub> + 21.14 B + 0.5 N <sub>2</sub> → 3 ThB <sub>6</sub> + ThB <sub>6</sub> H <sub>4</sub> C <sub>6</sub> N                                                        | -4.4819             |
| ThNH <sub>4</sub> B <sub>6</sub> C <sub>6</sub> | 3 ThC <sub>2</sub> + 1.556 B <sub>9</sub> H <sub>11</sub> + 2.685 N <sub>2</sub> → 2 ThB <sub>4</sub> + 4.37 H <sub>3</sub> N + ThB <sub>6</sub> H <sub>4</sub> C <sub>6</sub> N                                                      | -4.4764             |
| ThNH <sub>4</sub> B <sub>6</sub> C <sub>6</sub> | 0.3636 B <sub>9</sub> H <sub>11</sub> + 0.2098 B <sub>13</sub> C <sub>2</sub> + 1.86 Th <sub>2</sub> C <sub>3</sub> + 2.314 N <sub>2</sub> → 0.9068 Th <sub>3</sub> N <sub>4</sub> + ThB <sub>6</sub> H <sub>4</sub> C <sub>6</sub> N | -4.4750             |
| ThNH <sub>4</sub> B <sub>6</sub> C <sub>6</sub> | 9.5 ThH <sub>2</sub> + BN + 3 B <sub>13</sub> C <sub>2</sub> → 8.5 ThB <sub>4</sub> + 7.5 H <sub>2</sub> + ThB <sub>6</sub> H <sub>4</sub> C <sub>6</sub> N                                                                           | -4.4708             |
| ThNH <sub>4</sub> B <sub>6</sub> C <sub>6</sub> | 2 Th <sub>2</sub> C <sub>3</sub> + 6 B + 1.333 H <sub>3</sub> N + 1.833 N <sub>2</sub> → Th <sub>3</sub> N <sub>4</sub> + ThB <sub>6</sub> H <sub>4</sub> C <sub>6</sub> N                                                            | -4.4625             |
| ThNH <sub>4</sub> B <sub>6</sub> C <sub>6</sub> | 6 ThC + 1.333 H <sub>3</sub> N + 12.5 ThB <sub>6</sub> → 17.25 ThB <sub>4</sub> + 0.08333 Th <sub>3</sub> N <sub>4</sub> + ThB <sub>6</sub> H <sub>4</sub> C <sub>6</sub> N                                                           | -4.4568             |
| ThNH <sub>4</sub> B <sub>6</sub> C <sub>6</sub> | 2 H <sub>2</sub> + 3 B <sub>13</sub> C <sub>2</sub> + 5.714 ThN → 4.714 BN + 4.714 ThB <sub>6</sub> + ThB <sub>6</sub> H <sub>4</sub> C <sub>6</sub> N                                                                                | -4.4388             |
| ThNH <sub>4</sub> B <sub>6</sub> C <sub>6</sub> | 1.5 ThB <sub>4</sub> + 2 H <sub>2</sub> + 2 Th <sub>2</sub> C <sub>3</sub> + 2.75 N <sub>2</sub> → 4.5 ThN + ThB <sub>6</sub> H <sub>4</sub> C <sub>6</sub> N                                                                         | -4.4364             |
| ThNH <sub>4</sub> B <sub>6</sub> C <sub>6</sub> | 6 ThC + 2.889 B <sub>9</sub> H <sub>11</sub> + 0.5 N <sub>2</sub> → 5 ThB <sub>4</sub> + 13.89 H <sub>2</sub> + ThB <sub>6</sub> H <sub>4</sub> C <sub>6</sub> N                                                                      | -4.4233             |
| ThNH <sub>4</sub> B <sub>6</sub> C <sub>6</sub> | 0.3636 B <sub>9</sub> H <sub>11</sub> + 2 Th <sub>2</sub> C <sub>3</sub> + 20.73 B + 0.5 N <sub>2</sub> → 3 ThB <sub>6</sub> + ThB <sub>6</sub> H <sub>4</sub> C <sub>6</sub> N                                                       | -4.4196             |
| ThNH <sub>4</sub> B <sub>6</sub> C <sub>6</sub> | 6 ThC + 22.12 B <sub>9</sub> H <sub>11</sub> + H <sub>3</sub> N → 5 ThB <sub>4</sub> + 34.62 B <sub>5</sub> H <sub>7</sub> + ThB <sub>6</sub> H <sub>4</sub> C <sub>6</sub> N                                                         | -4.4000             |
| ThNH <sub>4</sub> B <sub>6</sub> C <sub>6</sub> | 0.5714 B <sub>5</sub> H <sub>7</sub> + 0.2418 B <sub>13</sub> C <sub>2</sub> + 1.839 Th <sub>2</sub> C <sub>3</sub> + 2.285 N <sub>2</sub> → 0.8926 Th <sub>3</sub> N <sub>4</sub> + ThB <sub>6</sub> H <sub>4</sub> C <sub>6</sub> N | -4.3706             |
| ThNH <sub>4</sub> B <sub>6</sub> C <sub>6</sub> | 2 H <sub>2</sub> + 2 Th <sub>2</sub> C <sub>3</sub> + 6 B + 2 N <sub>2</sub> → 3 ThN + ThB <sub>6</sub> H <sub>4</sub> C <sub>6</sub> N                                                                                               | -4.3620             |
| ThNH <sub>4</sub> B <sub>6</sub> C <sub>6</sub> | 0.5714 B <sub>5</sub> H <sub>7</sub> + 6 ThC + 3.143 BN + 2.262 N <sub>2</sub> → 1.667 Th <sub>3</sub> N <sub>4</sub> + ThB <sub>6</sub> H <sub>4</sub> C <sub>6</sub> N                                                              | -4.3559             |
| ThNH <sub>4</sub> B <sub>6</sub> C <sub>6</sub> | 6 ThC + 1.333 H <sub>3</sub> N + 12.33 ThB <sub>6</sub> → 17 ThB <sub>4</sub> + 0.3333 ThN + ThB <sub>6</sub> H <sub>4</sub> C <sub>6</sub> N                                                                                         | -4.3535             |
| ThNH <sub>4</sub> B <sub>6</sub> C <sub>6</sub> | ThC <sub>2</sub> + 2 B <sub>13</sub> C <sub>2</sub> + 7.591 H <sub>3</sub> N → 2.682 B <sub>5</sub> H <sub>7</sub> + 6.591 BN + ThB <sub>6</sub> H <sub>4</sub> C <sub>6</sub> N                                                      | -4.3467             |
| ThNH <sub>4</sub> B <sub>6</sub> C <sub>6</sub> | 6 ThC + 30.88 B <sub>9</sub> H <sub>11</sub> + H <sub>3</sub> N → 48.38 B <sub>5</sub> H <sub>7</sub> + 5 ThB <sub>6</sub> + ThB <sub>6</sub> H <sub>4</sub> C <sub>6</sub> N                                                         | -4.3448             |
| ThNH <sub>4</sub> B <sub>6</sub> C <sub>6</sub> | 2 ThH <sub>2</sub> + 0.25 Th <sub>3</sub> N <sub>4</sub> + 3 ThC <sub>2</sub> + 25 B → 4.75 ThB <sub>4</sub> + ThB <sub>6</sub> H <sub>4</sub> C <sub>6</sub> N                                                                       | -4.3283             |
| ThNH <sub>4</sub> B <sub>6</sub> C <sub>6</sub> | 0.6667 B <sub>9</sub> H <sub>11</sub> + 8.967 Th + H <sub>3</sub> N + 1.2 H <sub>8</sub> C <sub>5</sub> → 7.967 ThH <sub>2</sub> + ThB <sub>6</sub> H <sub>4</sub> C <sub>6</sub> N                                                   | -4.3012             |
| ThNH <sub>4</sub> B <sub>6</sub> C <sub>6</sub> | 6 ThC + 17.45 B + 6 H <sub>3</sub> N → 1.273 B <sub>9</sub> H <sub>11</sub> + 5 ThN + ThB <sub>6</sub> H <sub>4</sub> C <sub>6</sub> N                                                                                                | -4.2737             |
| ThNH <sub>4</sub> B <sub>6</sub> C <sub>6</sub> | 3.958 B <sub>5</sub> H <sub>7</sub> + 8.121 ThC + H <sub>3</sub> N → 1.78 Th <sub>4</sub> H <sub>15</sub> + 1.061 B <sub>13</sub> C <sub>2</sub> + ThB <sub>6</sub> H <sub>4</sub> C <sub>6</sub> N                                   | -4.2509             |
| ThNH <sub>4</sub> B <sub>6</sub> C <sub>6</sub> | 1.75 B <sub>13</sub> C <sub>2</sub> + 3.792 Th + 0.5 H <sub>8</sub> C <sub>5</sub> + 0.5 N <sub>2</sub> → 2.792 ThB <sub>6</sub> + ThB <sub>6</sub> H <sub>4</sub> C <sub>6</sub> N                                                   | -4.2403             |
| ThNH <sub>4</sub> B <sub>6</sub> C <sub>6</sub> | 5.2 B <sub>5</sub> H <sub>7</sub> + 6 ThC + 0.5 N <sub>2</sub> → 5 ThB <sub>4</sub> + 16.2 H <sub>2</sub> + ThB <sub>6</sub> H <sub>4</sub> C <sub>6</sub> N                                                                          | -4.2279             |
| ThNH <sub>4</sub> B <sub>6</sub> C <sub>6</sub> | 2 H <sub>2</sub> + 2 Th <sub>2</sub> C <sub>3</sub> + 18 B + 0.5 N <sub>2</sub> → 3 ThB <sub>4</sub> + ThB <sub>6</sub> H <sub>4</sub> C <sub>6</sub> N                                                                               | -4.2132             |
| ThNH <sub>4</sub> B <sub>6</sub> C <sub>6</sub> | 0.5714 B <sub>5</sub> H <sub>7</sub> + 0.25 Th <sub>3</sub> N <sub>4</sub> + 2 Th <sub>2</sub> C <sub>3</sub> + 25.64 B → 3.75 ThB <sub>6</sub> + ThB <sub>6</sub> H <sub>4</sub> C <sub>6</sub> N                                    | -4.1947             |
| ThNH <sub>4</sub> B <sub>6</sub> C <sub>6</sub> | 1.2 B <sub>5</sub> H <sub>7</sub> + 8 Th + 1.2 H <sub>8</sub> C <sub>5</sub> + 0.5 N <sub>2</sub> → 7 ThH <sub>2</sub> + ThB <sub>6</sub> H <sub>4</sub> C <sub>6</sub> N                                                             | -4.1908             |
| ThNH <sub>4</sub> B <sub>6</sub> C <sub>6</sub> | 6 ThC + 13.25 H <sub>2</sub> + 6 B + ThN → 1.5 Th <sub>4</sub> H <sub>15</sub> + ThB <sub>6</sub> H <sub>4</sub> C <sub>6</sub> N                                                                                                     | -4.1722             |
| ThNH <sub>4</sub> B <sub>6</sub> C <sub>6</sub> | 2 Th <sub>2</sub> C <sub>3</sub> + 24.33 B + 1.333 H <sub>3</sub> N → 0.3333 BN + 3 ThB <sub>6</sub> + ThB <sub>6</sub> H <sub>4</sub> C <sub>6</sub> N                                                                               | -4.1692             |
| ThNH <sub>4</sub> B <sub>6</sub> C <sub>6</sub> | 2 H <sub>2</sub> + 2 Th <sub>2</sub> C <sub>3</sub> + 22 B + ThN → 4 ThB <sub>4</sub> + ThB <sub>6</sub> H <sub>4</sub> C <sub>6</sub> N                                                                                              | -4.1636             |
| ThNH <sub>4</sub> B <sub>6</sub> C <sub>6</sub> | 6 ThC + 1.333 H <sub>3</sub> N + 13 ThB <sub>6</sub> → 18 ThB <sub>4</sub> + 0.1667 N <sub>2</sub> + ThB <sub>6</sub> H <sub>4</sub> C <sub>6</sub> N                                                                                 | -4.1446             |
| ThNH <sub>4</sub> B <sub>6</sub> C <sub>6</sub> | 0.25 Th <sub>3</sub> N <sub>4</sub> + 0.3636 B <sub>9</sub> H <sub>11</sub> + 2 Th <sub>2</sub> C <sub>3</sub> + 25.23 B → 3.75 ThB <sub>6</sub> + ThB <sub>6</sub> H <sub>4</sub> C <sub>6</sub> N                                   | -4.1324             |
| ThNH <sub>4</sub> B <sub>6</sub> C <sub>6</sub> | 2 H <sub>2</sub> + 2 Th <sub>2</sub> C <sub>3</sub> + 2.5 N <sub>2</sub> + ThB <sub>6</sub> → 4 ThN + ThB <sub>6</sub> H <sub>4</sub> C <sub>6</sub> N                                                                                | -4.1230             |
| ThNH <sub>4</sub> B <sub>6</sub> C <sub>6</sub> | 3.5 ThC + 6 B + 0.5 H <sub>8</sub> C <sub>5</sub> + 2.167 N <sub>2</sub> → 0.8333 Th <sub>3</sub> N <sub>4</sub> + ThB <sub>6</sub> H <sub>4</sub> C <sub>6</sub> N                                                                   | -4.1010             |
| ThNH <sub>4</sub> B <sub>6</sub> C <sub>6</sub> | 6 ThC + 1.46 B <sub>9</sub> H <sub>11</sub> + 0.5 N <sub>2</sub> → 1.785 ThB <sub>4</sub> + 0.8039 Th <sub>4</sub> H <sub>15</sub> + ThB <sub>6</sub> H <sub>4</sub> C <sub>6</sub> N                                                 | -4.0993             |
| ThNH <sub>4</sub> B <sub>6</sub> C <sub>6</sub> | 0.06667 Th <sub>4</sub> H <sub>15</sub> + 2 Th <sub>2</sub> C <sub>3</sub> + 25.6 B + H <sub>3</sub> N → 3.267 ThB <sub>6</sub> + ThB <sub>6</sub> H <sub>4</sub> C <sub>6</sub> N                                                    | -4.0737             |
| ThNH <sub>4</sub> B <sub>6</sub> C <sub>6</sub> | 6 ThC + 16 B + 6 H <sub>3</sub> N → 2 B <sub>5</sub> H <sub>7</sub> + 5 ThN + ThB <sub>6</sub> H <sub>4</sub> C <sub>6</sub> N                                                                                                        | -4.0558             |
| ThNH <sub>4</sub> B <sub>6</sub> C <sub>6</sub> | 2.428 B <sub>5</sub> H <sub>7</sub> + 6 ThC + 0.5 N <sub>2</sub> → 1.535 ThB <sub>4</sub> + 0.8663 Th <sub>4</sub> H <sub>15</sub> + ThB <sub>6</sub> H <sub>4</sub> C <sub>6</sub> N                                                 | -3.9830             |
| ThNH <sub>4</sub> B <sub>6</sub> C <sub>6</sub> | 3.212 ThB <sub>4</sub> + 3 ThC <sub>2</sub> + 7.848 H <sub>3</sub> N → 1.303 Th <sub>4</sub> H <sub>15</sub> + 6.848 BN + ThB <sub>6</sub> H <sub>4</sub> C <sub>6</sub> N                                                            | -3.9712             |
| ThNH <sub>4</sub> B <sub>6</sub> C <sub>6</sub> | 5.75 ThH <sub>2</sub> + 3 B <sub>13</sub> C <sub>2</sub> + 3.5 ThN → 8.25 ThB <sub>4</sub> + 2.5 H <sub>3</sub> N + ThB <sub>6</sub> H <sub>4</sub> C <sub>6</sub> N                                                                  | -3.9466             |
| ThNH <sub>4</sub> B <sub>6</sub> C <sub>6</sub> | 0.25 Th <sub>3</sub> N <sub>4</sub> + 6 ThC + 12.78 H <sub>2</sub> + 6 B → 1.437 Th <sub>4</sub> H <sub>15</sub> + ThB <sub>6</sub> H <sub>4</sub> C <sub>6</sub> N                                                                   | -3.9448             |
| ThNH <sub>4</sub> B <sub>6</sub> C <sub>6</sub> | 6 ThC + 13.25 H <sub>2</sub> + 0.5 N <sub>2</sub> + ThB <sub>6</sub> → 1.5 Th <sub>4</sub> H <sub>15</sub> + ThB <sub>6</sub> H <sub>4</sub> C <sub>6</sub> N                                                                         | -3.9332             |
| ThNH <sub>4</sub> B <sub>6</sub> C <sub>6</sub> | 6 ThC + 7.708 H <sub>2</sub> + 0.6667 B <sub>9</sub> H <sub>11</sub> + 0.5 N <sub>2</sub> → 1.25 Th <sub>4</sub> H <sub>15</sub> + ThB <sub>6</sub> H <sub>4</sub> C <sub>6</sub> N                                                   | -3.9195             |
| ThNH <sub>4</sub> B <sub>6</sub> C <sub>6</sub> | 2 ThH <sub>2</sub> + 1.273 Th <sub>3</sub> N <sub>4</sub> + 3 B <sub>13</sub> C <sub>2</sub> → 4.091 BN + 4.818 ThB <sub>6</sub> + ThB <sub>6</sub> H <sub>4</sub> C <sub>6</sub> N                                                   | -3.9093             |
| ThNH <sub>4</sub> B <sub>6</sub> C <sub>6</sub> | 6 ThC + 1.594 B <sub>9</sub> H <sub>11</sub> + 0.5 N <sub>2</sub> → 0.9023 Th <sub>4</sub> H <sub>15</sub> + 1.391 ThB <sub>6</sub> + ThB <sub>6</sub> H <sub>4</sub> C <sub>6</sub> N                                                | -3.9006             |
| ThNH <sub>4</sub> B <sub>6</sub> C <sub>6</sub> | 4.827 B <sub>5</sub> H <sub>7</sub> + 8.944 ThC + BN → 1.986 Th <sub>4</sub> H <sub>15</sub> + 1.472 B <sub>13</sub> C <sub>2</sub> + ThB <sub>6</sub> H <sub>4</sub> C <sub>6</sub> N                                                | -3.8764             |
| ThNH <sub>4</sub> B <sub>6</sub> C <sub>6</sub> | 1.2 B <sub>5</sub> H <sub>7</sub> + 6 ThC + 7.175 H <sub>2</sub> + 0.5 N <sub>2</sub> → 1.25 Th <sub>4</sub> H <sub>15</sub> + ThB <sub>6</sub> H <sub>4</sub> C <sub>6</sub> N                                                       | -3.8745             |
| ThNH <sub>4</sub> B <sub>6</sub> C <sub>6</sub> | 1.5 ThB <sub>4</sub> + 2 H <sub>2</sub> + 3 ThC <sub>2</sub> + 2.833 N <sub>2</sub> → 1.167 Th <sub>3</sub> N <sub>4</sub> + ThB <sub>6</sub> H <sub>4</sub> C <sub>6</sub> N                                                         | -3.8612             |
| ThNH <sub>4</sub> B <sub>6</sub> C <sub>6</sub> | 6 ThC + 4 B <sub>9</sub> H <sub>11</sub> + 0.5 N <sub>2</sub> → 20 H <sub>2</sub> + 5 ThB <sub>6</sub> + ThB <sub>6</sub> H <sub>4</sub> C <sub>6</sub> N                                                                             | -3.8515             |
| ThNH <sub>4</sub> B <sub>6</sub> C <sub>6</sub> | 6 ThC + 0.2667 Th <sub>4</sub> H <sub>15</sub> + BN + 14.63 ThB <sub>6</sub> → 20.7 ThB <sub>4</sub> + ThB <sub>6</sub> H <sub>4</sub> C <sub>6</sub> N                                                                               | -3.8390             |
| ThNH <sub>4</sub> B <sub>6</sub> C <sub>6</sub> | 2 H <sub>2</sub> + 0.4615 B <sub>13</sub> C <sub>2</sub> + 1.692 Th <sub>2</sub> C <sub>3</sub> + 2.09 N <sub>2</sub> → 0.7949 Th <sub>3</sub> N <sub>4</sub> + ThB <sub>6</sub> H <sub>4</sub> C <sub>6</sub> N                      | -3.8221             |
| ThNH <sub>4</sub> B <sub>6</sub> C <sub>6</sub> | 2.617 B <sub>5</sub> H <sub>7</sub> + 6 ThC + 0.5 N <sub>2</sub> → 0.9547 Th <sub>4</sub> H <sub>15</sub> + 1.181 ThB <sub>6</sub> + ThB <sub>6</sub> H <sub>4</sub> C <sub>6</sub> N                                                 | -3.8051             |
| ThNH <sub>4</sub> B <sub>6</sub> C <sub>6</sub> | 6 ThC + 9.875 H <sub>2</sub> + 6 B + H <sub>3</sub> N → 1.25 Th <sub>4</sub> H <sub>15</sub> + ThB <sub>6</sub> H <sub>4</sub> C <sub>6</sub> N                                                                                       | -3.8044             |

Continued on next page

Continued

| Compound                                        | Chemical reaction                                                                                                                                                                                                                   | Reaction energy(eV) |
|-------------------------------------------------|-------------------------------------------------------------------------------------------------------------------------------------------------------------------------------------------------------------------------------------|---------------------|
| ThNH <sub>4</sub> B <sub>6</sub> C <sub>6</sub> | 0.7857 ThB <sub>4</sub> + 0.5714 B <sub>5</sub> H <sub>7</sub> + 2 Th <sub>2</sub> C <sub>3</sub> + 2.393 N <sub>2</sub> → 3.786 ThN + ThB <sub>6</sub> H <sub>4</sub> C <sub>6</sub> N                                             | -3.8038             |
| ThNH <sub>4</sub> B <sub>6</sub> C <sub>6</sub> | 0.2667 Th <sub>4</sub> H <sub>15</sub> + BN + 2 Th <sub>2</sub> C <sub>3</sub> + 29.4 B → 4.067 ThB <sub>6</sub> + ThB <sub>6</sub> H <sub>4</sub> C <sub>6</sub> N                                                                 | -3.7873             |
| ThNH <sub>4</sub> B <sub>6</sub> C <sub>6</sub> | 2 ThH <sub>2</sub> + 2 Th <sub>2</sub> C <sub>3</sub> + 0.5 N <sub>2</sub> + 13 ThB <sub>6</sub> → 18 ThB <sub>4</sub> + ThB <sub>6</sub> H <sub>4</sub> C <sub>6</sub> N                                                           | -3.7825             |
| ThNH <sub>4</sub> B <sub>6</sub> C <sub>6</sub> | 1.5 ThB <sub>4</sub> + 6 ThC + 14.19 H <sub>2</sub> + 0.5 N <sub>2</sub> → 1.625 Th <sub>4</sub> H <sub>15</sub> + ThB <sub>6</sub> H <sub>4</sub> C <sub>6</sub> N                                                                 | -3.7684             |
| ThNH <sub>4</sub> B <sub>6</sub> C <sub>6</sub> | 0.5714 B <sub>5</sub> H <sub>7</sub> + 2 Th <sub>2</sub> C <sub>3</sub> + 3.143 B + 2 N <sub>2</sub> → 3 ThN + ThB <sub>6</sub> H <sub>4</sub> C <sub>6</sub> N                                                                     | -3.7649             |
| ThNH <sub>4</sub> B <sub>6</sub> C <sub>6</sub> | 0.5 H <sub>2</sub> + 2 Th <sub>2</sub> C <sub>3</sub> + 24 B + H <sub>3</sub> N → 3 ThB <sub>6</sub> + ThB <sub>6</sub> H <sub>4</sub> C <sub>6</sub> N                                                                             | -3.7550             |
| ThNH <sub>4</sub> B <sub>6</sub> C <sub>6</sub> | 0.6818 ThB <sub>4</sub> + 0.3636 B <sub>9</sub> H <sub>11</sub> + 2 Th <sub>2</sub> C <sub>3</sub> + 2.341 N <sub>2</sub> → 3.682 ThN + ThB <sub>6</sub> H <sub>4</sub> C <sub>6</sub> N                                            | -3.7364             |
| ThNH <sub>4</sub> B <sub>6</sub> C <sub>6</sub> | 0.5 ThH <sub>2</sub> + 2 Th <sub>2</sub> C <sub>3</sub> + 20 B + H <sub>3</sub> N → 3.5 ThB <sub>4</sub> + ThB <sub>6</sub> H <sub>4</sub> C <sub>6</sub> N                                                                         | -3.7194             |
| ThNH <sub>4</sub> B <sub>6</sub> C <sub>6</sub> | 0.25 Th <sub>3</sub> N <sub>4</sub> + 2 H <sub>2</sub> + 2 Th <sub>2</sub> C <sub>3</sub> + 21 B → 3.75 ThB <sub>4</sub> + ThB <sub>6</sub> H <sub>4</sub> C <sub>6</sub> N                                                         | -3.7095             |
| ThNH <sub>4</sub> B <sub>6</sub> C <sub>6</sub> | 0.3636 B <sub>9</sub> H <sub>11</sub> + 2 Th <sub>2</sub> C <sub>3</sub> + 2.727 B + 2 N <sub>2</sub> → 3 ThN + ThB <sub>6</sub> H <sub>4</sub> C <sub>6</sub> N                                                                    | -3.7026             |
| ThNH <sub>4</sub> B <sub>6</sub> C <sub>6</sub> | 1.643 B <sub>5</sub> H <sub>7</sub> + 3 ThC <sub>2</sub> + 1.607 N <sub>2</sub> → 0.5 Th <sub>4</sub> H <sub>15</sub> + 2.214 BN + ThB <sub>6</sub> H <sub>4</sub> C <sub>6</sub> N                                                 | -3.6639             |
| ThNH <sub>4</sub> B <sub>6</sub> C <sub>6</sub> | ThC <sub>2</sub> + 2 B <sub>13</sub> C <sub>2</sub> + 7.026 H <sub>3</sub> N → 6.026 BN + 1.553 B <sub>9</sub> H <sub>11</sub> + ThB <sub>6</sub> H <sub>4</sub> C <sub>6</sub> N                                                   | -3.6581             |
| ThNH <sub>4</sub> B <sub>6</sub> C <sub>6</sub> | 4.042 ThC <sub>2</sub> + 0.6667 B <sub>9</sub> H <sub>11</sub> + 2.021 N <sub>2</sub> → 0.4167 H <sub>8</sub> C <sub>5</sub> + 3.042 ThN + ThB <sub>6</sub> H <sub>4</sub> C <sub>6</sub> N                                         | -3.6556             |
| ThNH <sub>4</sub> B <sub>6</sub> C <sub>6</sub> | 6.333 ThH <sub>2</sub> + 0.9722 Th <sub>3</sub> N <sub>4</sub> + 3 B <sub>13</sub> C <sub>2</sub> → 8.25 ThB <sub>4</sub> + 2.889 H <sub>3</sub> N + ThB <sub>6</sub> H <sub>4</sub> C <sub>6</sub> N                               | -3.6450             |
| ThNH <sub>4</sub> B <sub>6</sub> C <sub>6</sub> | 6.5 ThH <sub>2</sub> + 3 B <sub>13</sub> C <sub>2</sub> + 0.5 N <sub>2</sub> → 4.5 H <sub>2</sub> + 5.5 ThB <sub>6</sub> + ThB <sub>6</sub> H <sub>4</sub> C <sub>6</sub> N                                                         | -3.6429             |
| ThNH <sub>4</sub> B <sub>6</sub> C <sub>6</sub> | 0.5714 B <sub>5</sub> H <sub>7</sub> + 2 Th <sub>2</sub> C <sub>3</sub> + 2.262 N <sub>2</sub> + 0.5238 ThB <sub>6</sub> → 3.524 ThN + ThB <sub>6</sub> H <sub>4</sub> C <sub>6</sub> N                                             | -3.6397             |
| ThNH <sub>4</sub> B <sub>6</sub> C <sub>6</sub> | 0.6667 B <sub>9</sub> H <sub>11</sub> + 2 Th <sub>2</sub> C <sub>3</sub> + 1.907 N <sub>2</sub> → 0.7037 Th <sub>3</sub> N <sub>4</sub> + 0.2222 Th <sub>4</sub> H <sub>15</sub> + ThB <sub>6</sub> H <sub>4</sub> C <sub>6</sub> N | -3.6161             |
| ThNH <sub>4</sub> B <sub>6</sub> C <sub>6</sub> | 0.5714 B <sub>5</sub> H <sub>7</sub> + 2 Th <sub>2</sub> C <sub>3</sub> + 15.14 B + 0.5 N <sub>2</sub> → 3 ThB <sub>4</sub> + ThB <sub>6</sub> H <sub>4</sub> C <sub>6</sub> N                                                      | -3.6160             |
| ThNH <sub>4</sub> B <sub>6</sub> C <sub>6</sub> | 1.527 Th <sub>3</sub> N <sub>4</sub> + 0.2667 Th <sub>4</sub> H <sub>15</sub> + 3 B <sub>13</sub> C <sub>2</sub> → 5.109 BN + 4.648 ThB <sub>6</sub> + ThB <sub>6</sub> H <sub>4</sub> C <sub>6</sub> N                             | -3.6067             |
| ThNH <sub>4</sub> B <sub>6</sub> C <sub>6</sub> | 0.1429 B <sub>5</sub> H <sub>7</sub> + 2 Th <sub>2</sub> C <sub>3</sub> + 23.29 B + H <sub>3</sub> N → 3 ThB <sub>6</sub> + ThB <sub>6</sub> H <sub>4</sub> C <sub>6</sub> N                                                        | -3.6057             |
| ThNH <sub>4</sub> B <sub>6</sub> C <sub>6</sub> | 0.2667 Th <sub>4</sub> H <sub>15</sub> + 3 ThC <sub>2</sub> + 30.4 B + ThN → 4.067 ThB <sub>6</sub> + ThB <sub>6</sub> H <sub>4</sub> C <sub>6</sub> N                                                                              | -3.6019             |
| ThNH <sub>4</sub> B <sub>6</sub> C <sub>6</sub> | 0.3636 B <sub>9</sub> H <sub>11</sub> + 2 Th <sub>2</sub> C <sub>3</sub> + 2.227 N <sub>2</sub> + 0.4545 ThB <sub>6</sub> → 3.455 ThN + ThB <sub>6</sub> H <sub>4</sub> C <sub>6</sub> N                                            | -3.5940             |
| ThNH <sub>4</sub> B <sub>6</sub> C <sub>6</sub> | 0.09091 B <sub>9</sub> H <sub>11</sub> + 2 Th <sub>2</sub> C <sub>3</sub> + 23.18 B + H <sub>3</sub> N → 3 ThB <sub>6</sub> + ThB <sub>6</sub> H <sub>4</sub> C <sub>6</sub> N                                                      | -3.5901             |
| ThNH <sub>4</sub> B <sub>6</sub> C <sub>6</sub> | 7.2 B <sub>5</sub> H <sub>7</sub> + 6 ThC + 0.5 N <sub>2</sub> → 23.2 H <sub>2</sub> + 5 ThB <sub>6</sub> + ThB <sub>6</sub> H <sub>4</sub> C <sub>6</sub> N                                                                        | -3.5810             |
| ThNH <sub>4</sub> B <sub>6</sub> C <sub>6</sub> | 6 ThC + 3.333 B <sub>9</sub> H <sub>11</sub> + ThN → 6 ThB <sub>4</sub> + 16.33 H <sub>2</sub> + ThB <sub>6</sub> H <sub>4</sub> C <sub>6</sub> N                                                                                   | -3.5677             |
| ThNH <sub>4</sub> B <sub>6</sub> C <sub>6</sub> | 0.5714 B <sub>5</sub> H <sub>7</sub> + 2 Th <sub>2</sub> C <sub>3</sub> + 19.14 B + ThN → 4 ThB <sub>4</sub> + ThB <sub>6</sub> H <sub>4</sub> C <sub>6</sub> N                                                                     | -3.5664             |
| ThNH <sub>4</sub> B <sub>6</sub> C <sub>6</sub> | 6.605 ThH <sub>2</sub> + 3 B <sub>13</sub> C <sub>2</sub> + ThN → 6.605 ThB <sub>4</sub> + 1.316 B <sub>5</sub> H <sub>7</sub> + ThB <sub>6</sub> H <sub>4</sub> C <sub>6</sub> N                                                   | -3.5558             |
| ThNH <sub>4</sub> B <sub>6</sub> C <sub>6</sub> | 0.3636 B <sub>9</sub> H <sub>11</sub> + 2 Th <sub>2</sub> C <sub>3</sub> + 14.73 B + 0.5 N <sub>2</sub> → 3 ThB <sub>4</sub> + ThB <sub>6</sub> H <sub>4</sub> C <sub>6</sub> N                                                     | -3.5538             |
| ThNH <sub>4</sub> B <sub>6</sub> C <sub>6</sub> | 1.2 B <sub>5</sub> H <sub>7</sub> + 3 ThC <sub>2</sub> + 2.567 N <sub>2</sub> → 0.6667 Th <sub>3</sub> N <sub>4</sub> + 1.467 H <sub>3</sub> N + ThB <sub>6</sub> H <sub>4</sub> C <sub>6</sub> N                                   | -3.5418             |
| ThNH <sub>4</sub> B <sub>6</sub> C <sub>6</sub> | 2 ThH <sub>2</sub> + 3 B <sub>13</sub> C <sub>2</sub> + 4 ThN → 3 BN + 5 ThB <sub>6</sub> + ThB <sub>6</sub> H <sub>4</sub> C <sub>6</sub> N                                                                                        | -3.5275             |
| ThNH <sub>4</sub> B <sub>6</sub> C <sub>6</sub> | 3 B <sub>13</sub> C <sub>2</sub> + 1.333 H <sub>3</sub> N + 27 ThN → 6.833 Th <sub>3</sub> N <sub>4</sub> + 5.5 ThB <sub>6</sub> + ThB <sub>6</sub> H <sub>4</sub> C <sub>6</sub> N                                                 | -3.5114             |
| ThNH <sub>4</sub> B <sub>6</sub> C <sub>6</sub> | 0.3636 B <sub>9</sub> H <sub>11</sub> + 2 Th <sub>2</sub> C <sub>3</sub> + 18.73 B + ThN → 4 ThB <sub>4</sub> + ThB <sub>6</sub> H <sub>4</sub> C <sub>6</sub> N                                                                    | -3.5042             |
| ThNH <sub>4</sub> B <sub>6</sub> C <sub>6</sub> | 6 ThC + 2 H <sub>2</sub> + BN + 12.5 ThB <sub>6</sub> → 17.5 ThB <sub>4</sub> + ThB <sub>6</sub> H <sub>4</sub> C <sub>6</sub> N                                                                                                    | -3.4876             |
| ThNH <sub>4</sub> B <sub>6</sub> C <sub>6</sub> | 0.6667 B <sub>9</sub> H <sub>11</sub> + 7.467 Th + 1.2 H <sub>8</sub> C <sub>5</sub> + 0.5 N <sub>2</sub> → 6.467 ThH <sub>2</sub> + ThB <sub>6</sub> H <sub>4</sub> C <sub>6</sub> N                                               | -3.4693             |
| ThNH <sub>4</sub> B <sub>6</sub> C <sub>6</sub> | 6.789 ThH <sub>2</sub> + 0.25 Th <sub>3</sub> N <sub>4</sub> + 3 B <sub>13</sub> C <sub>2</sub> → 6.539 ThB <sub>4</sub> + 1.368 B <sub>5</sub> H <sub>7</sub> + ThB <sub>6</sub> H <sub>4</sub> C <sub>6</sub> N                   | -3.4626             |
| ThNH <sub>4</sub> B <sub>6</sub> C <sub>6</sub> | 2 ThH <sub>2</sub> + 2.538 ThC <sub>2</sub> + 0.4615 B <sub>13</sub> C <sub>2</sub> + 2.269 N <sub>2</sub> → 3.538 ThN + ThB <sub>6</sub> H <sub>4</sub> C <sub>6</sub> N                                                           | -3.4307             |
| ThNH <sub>4</sub> B <sub>6</sub> C <sub>6</sub> | 2 ThH <sub>2</sub> + BN + 3 ThC <sub>2</sub> + 29 B → 4 ThB <sub>6</sub> + ThB <sub>6</sub> H <sub>4</sub> C <sub>6</sub> N                                                                                                         | -3.4197             |
| ThNH <sub>4</sub> B <sub>6</sub> C <sub>6</sub> | 2 Th <sub>2</sub> C <sub>3</sub> + 22.5 B + 1.333 H <sub>3</sub> N → 0.08333 Th <sub>3</sub> N <sub>4</sub> + 2.75 ThB <sub>6</sub> + ThB <sub>6</sub> H <sub>4</sub> C <sub>6</sub> N                                              | -3.4094             |
| ThNH <sub>4</sub> B <sub>6</sub> C <sub>6</sub> | 6.947 ThH <sub>2</sub> + 3 B <sub>13</sub> C <sub>2</sub> + H <sub>3</sub> N → 5.947 ThB <sub>4</sub> + 1.842 B <sub>5</sub> H <sub>7</sub> + ThB <sub>6</sub> H <sub>4</sub> C <sub>6</sub> N                                      | -3.3994             |
| ThNH <sub>4</sub> B <sub>6</sub> C <sub>6</sub> | 3.5 ThC + 27 B + 0.5 H <sub>8</sub> C <sub>5</sub> + ThN → 3.5 ThB <sub>6</sub> + ThB <sub>6</sub> H <sub>4</sub> C <sub>6</sub> N                                                                                                  | -3.3826             |
| ThNH <sub>4</sub> B <sub>6</sub> C <sub>6</sub> | 16.75 Th <sub>3</sub> N <sub>4</sub> + 1.75 B <sub>13</sub> C <sub>2</sub> + 0.5 H <sub>8</sub> C <sub>5</sub> → 16.75 BN + 49.25 ThN + ThB <sub>6</sub> H <sub>4</sub> C <sub>6</sub> N                                            | -3.3772             |
| ThNH <sub>4</sub> B <sub>6</sub> C <sub>6</sub> | 0.2667 Th <sub>4</sub> H <sub>15</sub> + 3 ThC <sub>2</sub> + 24.4 B + 0.5 N <sub>2</sub> → 3.067 ThB <sub>6</sub> + ThB <sub>6</sub> H <sub>4</sub> C <sub>6</sub> N                                                               | -3.3629             |
| ThNH <sub>4</sub> B <sub>6</sub> C <sub>6</sub> | 6.435 ThH <sub>2</sub> + 3 B <sub>13</sub> C <sub>2</sub> + ThN → 6.435 ThB <sub>4</sub> + 0.8065 B <sub>9</sub> H <sub>11</sub> + ThB <sub>6</sub> H <sub>4</sub> C <sub>6</sub> N                                                 | -3.3612             |
| ThNH <sub>4</sub> B <sub>6</sub> C <sub>6</sub> | 0.2667 Th <sub>4</sub> H <sub>15</sub> + 0.4615 B <sub>13</sub> C <sub>2</sub> + 1.692 Th <sub>2</sub> C <sub>3</sub> + 2.226 N <sub>2</sub> → 3.451 ThN + ThB <sub>6</sub> H <sub>4</sub> C <sub>6</sub> N                         | -3.3590             |
| ThNH <sub>4</sub> B <sub>6</sub> C <sub>6</sub> | 6 B <sub>5</sub> H <sub>7</sub> + 6 ThC + ThN → 6 ThB <sub>4</sub> + 19 H <sub>2</sub> + ThB <sub>6</sub> H <sub>4</sub> C <sub>6</sub> N                                                                                           | -3.3423             |
| ThNH <sub>4</sub> B <sub>6</sub> C <sub>6</sub> | 6 ThC + 6 B + 4.398 H <sub>3</sub> N → 0.8495 Th <sub>3</sub> N <sub>4</sub> + 0.6129 Th <sub>4</sub> H <sub>15</sub> + ThB <sub>6</sub> H <sub>4</sub> C <sub>6</sub> N                                                            | -3.3276             |
| ThNH <sub>4</sub> B <sub>6</sub> C <sub>6</sub> | 0.25 Th <sub>3</sub> N <sub>4</sub> + 6 ThC + 3.222 B <sub>9</sub> H <sub>11</sub> → 5.75 ThB <sub>4</sub> + 15.72 H <sub>2</sub> + ThB <sub>6</sub> H <sub>4</sub> C <sub>6</sub> N                                                | -3.3151             |
| ThNH <sub>4</sub> B <sub>6</sub> C <sub>6</sub> | 2 Th <sub>2</sub> C <sub>3</sub> + 24 B + 1.333 H <sub>3</sub> N → 0.1667 N <sub>2</sub> + 3 ThB <sub>6</sub> + ThB <sub>6</sub> H <sub>4</sub> C <sub>6</sub> N                                                                    | -3.3136             |
| ThNH <sub>4</sub> B <sub>6</sub> C <sub>6</sub> | 2 Th <sub>2</sub> C <sub>3</sub> + 18.33 B + 1.333 H <sub>3</sub> N → 3 ThB <sub>4</sub> + 0.3333 BN + ThB <sub>6</sub> H <sub>4</sub> C <sub>6</sub> N                                                                             | -3.3033             |
| ThNH <sub>4</sub> B <sub>6</sub> C <sub>6</sub> | 0.5714 B <sub>5</sub> H <sub>7</sub> + 6 ThC + BN + 11.07 ThB <sub>6</sub> → 16.07 ThB <sub>4</sub> + ThB <sub>6</sub> H <sub>4</sub> C <sub>6</sub> N                                                                              | -3.3027             |
| ThNH <sub>4</sub> B <sub>6</sub> C <sub>6</sub> | 6 ThC + BN + 0.3636 B <sub>9</sub> H <sub>11</sub> + 10.86 ThB <sub>6</sub> → 15.86 ThB <sub>4</sub> + ThB <sub>6</sub> H <sub>4</sub> C <sub>6</sub> N                                                                             | -3.3004             |
| ThNH <sub>4</sub> B <sub>6</sub> C <sub>6</sub> | 2.75 B <sub>9</sub> H <sub>11</sub> + 2 Th <sub>2</sub> C <sub>3</sub> + 2 N <sub>2</sub> → 3.75 B <sub>5</sub> H <sub>7</sub> + 3 ThN + ThB <sub>6</sub> H <sub>4</sub> C <sub>6</sub> N                                           | -3.2940             |
| ThNH <sub>4</sub> B <sub>6</sub> C <sub>6</sub> | 0.3636 B <sub>9</sub> H <sub>11</sub> + 3 B <sub>13</sub> C <sub>2</sub> + 25.18 ThN → 6.045 Th <sub>3</sub> N <sub>4</sub> + 6.045 ThB <sub>6</sub> + ThB <sub>6</sub> H <sub>4</sub> C <sub>6</sub> N                             | -3.2776             |
| ThNH <sub>4</sub> B <sub>6</sub> C <sub>6</sub> | 17.34 B <sub>5</sub> H <sub>7</sub> + 6 ThC + 0.5 N <sub>2</sub> → 1.25 Th <sub>4</sub> H <sub>15</sub> + 8.969 B <sub>9</sub> H <sub>11</sub> + ThB <sub>6</sub> H <sub>4</sub> C <sub>6</sub> N                                   | -3.2680             |
| ThNH <sub>4</sub> B <sub>6</sub> C <sub>6</sub> | 6.613 ThH <sub>2</sub> + 0.25 Th <sub>3</sub> N <sub>4</sub> + 3 B <sub>13</sub> C <sub>2</sub> → 6.363 ThB <sub>4</sub> + 0.8387 B <sub>9</sub> H <sub>11</sub> + ThB <sub>6</sub> H <sub>4</sub> C <sub>6</sub> N                 | -3.2603             |
| ThNH <sub>4</sub> B <sub>6</sub> C <sub>6</sub> | 2 H <sub>2</sub> + 3 ThC <sub>2</sub> + 2.5 N <sub>2</sub> + ThB <sub>6</sub> → Th <sub>3</sub> N <sub>4</sub> + ThB <sub>6</sub> H <sub>4</sub> C <sub>6</sub> N                                                                   | -3.2368             |
| ThNH <sub>4</sub> B <sub>6</sub> C <sub>6</sub> | 2 Th <sub>2</sub> C <sub>3</sub> + 22 B + 1.333 H <sub>3</sub> N → 2.667 ThB <sub>6</sub> + 0.3333 ThN + ThB <sub>6</sub> H <sub>4</sub> C <sub>6</sub> N                                                                           | -3.2340             |
| ThNH <sub>4</sub> B <sub>6</sub> C <sub>6</sub> | 0.5714 B <sub>5</sub> H <sub>7</sub> + 3 B <sub>13</sub> C <sub>2</sub> + 24.9 ThN → 5.976 Th <sub>3</sub> N <sub>4</sub> + 5.976 ThB <sub>6</sub> + ThB <sub>6</sub> H <sub>4</sub> C <sub>6</sub> N                               | -3.1941             |
| ThNH <sub>4</sub> B <sub>6</sub> C <sub>6</sub> | 6 ThC + 1.653 B <sub>9</sub> H <sub>11</sub> + ThN → 2.219 ThB <sub>4</sub> + 0.9453 Th <sub>4</sub> H <sub>15</sub> + ThB <sub>6</sub> H <sub>4</sub> C <sub>6</sub> N                                                             | -3.1867             |
| ThNH <sub>4</sub> B <sub>6</sub> C <sub>6</sub> | 0.9091 B <sub>9</sub> H <sub>11</sub> + 2 Th <sub>2</sub> C <sub>3</sub> + 1.591 N <sub>2</sub> → 3 ThH <sub>2</sub> + 2.182 BN + ThB <sub>6</sub> H <sub>4</sub> C <sub>6</sub> N                                                  | -3.1828             |

Continued on next page



Continued

| Compound                                        | Chemical reaction                                                                                                                                                                                                               | Reaction energy(eV) |
|-------------------------------------------------|---------------------------------------------------------------------------------------------------------------------------------------------------------------------------------------------------------------------------------|---------------------|
| ThNH <sub>4</sub> B <sub>6</sub> C <sub>6</sub> | 6 ThC + BN + 19.37 B <sub>9</sub> H <sub>11</sub> → 5 ThB <sub>4</sub> + 29.87 B <sub>5</sub> H <sub>7</sub> + ThB <sub>6</sub> H <sub>4</sub> C <sub>6</sub> N                                                                 | -3.1804             |
| ThNH <sub>4</sub> B <sub>6</sub> C <sub>6</sub> | 3.315 B <sub>5</sub> H <sub>7</sub> + 2.894 Th <sub>3</sub> N <sub>4</sub> + 1.2 H <sub>8</sub> C <sub>5</sub> → 1.92 Th <sub>4</sub> H <sub>15</sub> + 10.58 BN + ThB <sub>6</sub> H <sub>4</sub> C <sub>6</sub> N             | -3.1704             |
| ThNH <sub>4</sub> B <sub>6</sub> C <sub>6</sub> | 2 ThH <sub>2</sub> + 2 Th <sub>2</sub> C <sub>3</sub> + 15 ThB <sub>6</sub> + ThN → 21 ThB <sub>4</sub> + ThB <sub>6</sub> H <sub>4</sub> C <sub>6</sub> N                                                                      | -3.1556             |
| ThNH <sub>4</sub> B <sub>6</sub> C <sub>6</sub> | 0.6667 B <sub>9</sub> H <sub>11</sub> + 2 Th <sub>2</sub> C <sub>3</sub> + 2 N <sub>2</sub> → 1.667 H <sub>2</sub> + 3 ThN + ThB <sub>6</sub> H <sub>4</sub> C <sub>6</sub> N                                                   | -3.1531             |
| ThNH <sub>4</sub> B <sub>6</sub> C <sub>6</sub> | 0.2667 Th <sub>4</sub> H <sub>15</sub> + 3 B <sub>13</sub> C <sub>2</sub> + 4.8 ThN → 3.8 BN + 4.867 ThB <sub>6</sub> + ThB <sub>6</sub> H <sub>4</sub> C <sub>6</sub> N                                                        | -3.1486             |
| ThNH <sub>4</sub> B <sub>6</sub> C <sub>6</sub> | 3.5 ThC + 21 B + 0.5 H <sub>8</sub> C <sub>5</sub> + 0.5 N <sub>2</sub> → 2.5 ThB <sub>6</sub> + ThB <sub>6</sub> H <sub>4</sub> C <sub>6</sub> N                                                                               | -3.1436             |
| ThNH <sub>4</sub> B <sub>6</sub> C <sub>6</sub> | 5.375 ThC + H <sub>3</sub> N + 0.125 H <sub>8</sub> C <sub>5</sub> + 11.75 ThB <sub>6</sub> → 16.12 ThB <sub>4</sub> + ThB <sub>6</sub> H <sub>4</sub> C <sub>6</sub> N                                                         | -3.1367             |
| ThNH <sub>4</sub> B <sub>6</sub> C <sub>6</sub> | 5.077 ThC + 9.644 H <sub>2</sub> + 0.4615 B <sub>13</sub> C <sub>2</sub> + 0.5 N <sub>2</sub> → 1.019 Th <sub>4</sub> H <sub>15</sub> + ThB <sub>6</sub> H <sub>4</sub> C <sub>6</sub> N                                        | -3.1346             |
| ThNH <sub>4</sub> B <sub>6</sub> C <sub>6</sub> | 0.06667 Th <sub>4</sub> H <sub>15</sub> + 2 Th <sub>2</sub> C <sub>3</sub> + 19.07 B + H <sub>3</sub> N → 3.267 ThB <sub>4</sub> + ThB <sub>6</sub> H <sub>4</sub> C <sub>6</sub> N                                             | -3.1309             |
| ThNH <sub>4</sub> B <sub>6</sub> C <sub>6</sub> | 6.71 ThH <sub>2</sub> + 3 B <sub>13</sub> C <sub>2</sub> + H <sub>3</sub> N → 5.71 ThB <sub>4</sub> + 1.129 B <sub>9</sub> H <sub>11</sub> + ThB <sub>6</sub> H <sub>4</sub> C <sub>6</sub> N                                   | -3.1271             |
| ThNH <sub>4</sub> B <sub>6</sub> C <sub>6</sub> | 6 ThC + BN + 28.13 B <sub>9</sub> H <sub>11</sub> → 43.63 B <sub>5</sub> H <sub>7</sub> + 5 ThB <sub>6</sub> + ThB <sub>6</sub> H <sub>4</sub> C <sub>6</sub> N                                                                 | -3.1251             |
| ThNH <sub>4</sub> B <sub>6</sub> C <sub>6</sub> | 1.2 B <sub>5</sub> H <sub>7</sub> + 2 Th <sub>2</sub> C <sub>3</sub> + 1.718 N <sub>2</sub> → 0.6089 Th <sub>3</sub> N <sub>4</sub> + 0.2933 Th <sub>4</sub> H <sub>15</sub> + ThB <sub>6</sub> H <sub>4</sub> C <sub>6</sub> N | -3.1221             |
| ThNH <sub>4</sub> B <sub>6</sub> C <sub>6</sub> | 3 ThC <sub>2</sub> + 0.6667 B <sub>9</sub> H <sub>11</sub> + 2.389 N <sub>2</sub> → 0.6667 Th <sub>3</sub> N <sub>4</sub> + 1.111 H <sub>3</sub> N + ThB <sub>6</sub> H <sub>4</sub> C <sub>6</sub> N                           | -3.1161             |
| ThNH <sub>4</sub> B <sub>6</sub> C <sub>6</sub> | 0.5714 B <sub>5</sub> H <sub>7</sub> + 0.25 Th <sub>3</sub> N <sub>4</sub> + 2 Th <sub>2</sub> C <sub>3</sub> + 18.14 B → 3.75 ThB <sub>4</sub> + ThB <sub>6</sub> H <sub>4</sub> C <sub>6</sub> N                              | -3.1123             |
| ThNH <sub>4</sub> B <sub>6</sub> C <sub>6</sub> | 1.2 B <sub>5</sub> H <sub>7</sub> + 2 Th <sub>2</sub> C <sub>3</sub> + 2 N <sub>2</sub> → 2.2 H <sub>2</sub> + 3 ThN + ThB <sub>6</sub> H <sub>4</sub> C <sub>6</sub> N                                                         | -3.1080             |
| ThNH <sub>4</sub> B <sub>6</sub> C <sub>6</sub> | 6 ThC + 2.889 B <sub>9</sub> H <sub>11</sub> + H <sub>3</sub> N → 5 ThB <sub>4</sub> + 15.39 H <sub>2</sub> + ThB <sub>6</sub> H <sub>4</sub> C <sub>6</sub> N                                                                  | -3.0992             |
| ThNH <sub>4</sub> B <sub>6</sub> C <sub>6</sub> | 5.8 B <sub>5</sub> H <sub>7</sub> + 0.25 Th <sub>3</sub> N <sub>4</sub> + 6 ThC → 5.75 ThB <sub>4</sub> + 18.3 H <sub>2</sub> + ThB <sub>6</sub> H <sub>4</sub> C <sub>6</sub> N                                                | -3.0972             |
| ThNH <sub>4</sub> B <sub>6</sub> C <sub>6</sub> | 0.25 Th <sub>3</sub> N <sub>4</sub> + 0.2667 Th <sub>4</sub> H <sub>15</sub> + 3 ThC <sub>2</sub> + 28.9 B → 3.817 ThB <sub>6</sub> + ThB <sub>6</sub> H <sub>4</sub> C <sub>6</sub> N                                          | -3.0757             |
| ThNH <sub>4</sub> B <sub>6</sub> C <sub>6</sub> | 2.749 B <sub>5</sub> H <sub>7</sub> + 6 ThC + ThN → 1.936 ThB <sub>4</sub> + 1.016 Th <sub>4</sub> H <sub>15</sub> + ThB <sub>6</sub> H <sub>4</sub> C <sub>6</sub> N                                                           | -3.0550             |
| ThNH <sub>4</sub> B <sub>6</sub> C <sub>6</sub> | 2 ThH <sub>2</sub> + 2.762 ThC + 1.619 B <sub>13</sub> C <sub>2</sub> + 0.5 N <sub>2</sub> → 3.762 ThB <sub>4</sub> + ThB <sub>6</sub> H <sub>4</sub> C <sub>6</sub> N                                                          | -3.0528             |
| ThNH <sub>4</sub> B <sub>6</sub> C <sub>6</sub> | 0.25 Th <sub>3</sub> N <sub>4</sub> + 0.3636 B <sub>9</sub> H <sub>11</sub> + 2 Th <sub>2</sub> C <sub>3</sub> + 17.73 B → 3.75 ThB <sub>4</sub> + ThB <sub>6</sub> H <sub>4</sub> C <sub>6</sub> N                             | -3.0501             |
| ThNH <sub>4</sub> B <sub>6</sub> C <sub>6</sub> | 5.635 ThH <sub>2</sub> + 3 B <sub>13</sub> C <sub>2</sub> + 0.5 N <sub>2</sub> → 1.038 B <sub>5</sub> H <sub>7</sub> + 4.635 ThB <sub>6</sub> + ThB <sub>6</sub> H <sub>4</sub> C <sub>6</sub> N                                | -3.0413             |
| ThNH <sub>4</sub> B <sub>6</sub> C <sub>6</sub> | 6 ThC + 15.12 H <sub>2</sub> + ThB <sub>6</sub> + ThN → 1.75 Th <sub>4</sub> H <sub>15</sub> + ThB <sub>6</sub> H <sub>4</sub> C <sub>6</sub> N                                                                                 | -2.9768             |
| ThNH <sub>4</sub> B <sub>6</sub> C <sub>6</sub> | 6 ThC + 9.583 H <sub>2</sub> + 0.6667 B <sub>9</sub> H <sub>11</sub> + ThN → 1.5 Th <sub>4</sub> H <sub>15</sub> + ThB <sub>6</sub> H <sub>4</sub> C <sub>6</sub> N                                                             | -2.9632             |
| ThNH <sub>4</sub> B <sub>6</sub> C <sub>6</sub> | 0.25 Th <sub>3</sub> N <sub>4</sub> + 6 ThC + 1.605 B <sub>9</sub> H <sub>11</sub> → 2.11 ThB <sub>4</sub> + 0.91 Th <sub>4</sub> H <sub>15</sub> + ThB <sub>6</sub> H <sub>4</sub> C <sub>6</sub> N                            | -2.9484             |
| ThNH <sub>4</sub> B <sub>6</sub> C <sub>6</sub> | 6 ThC + 1.82 B <sub>9</sub> H <sub>11</sub> + ThN → 1.068 Th <sub>4</sub> H <sub>15</sub> + 1.729 ThB <sub>6</sub> + ThB <sub>6</sub> H <sub>4</sub> C <sub>6</sub> N                                                           | -2.9397             |
| ThNH <sub>4</sub> B <sub>6</sub> C <sub>6</sub> | 5.536 ThH <sub>2</sub> + 3 B <sub>13</sub> C <sub>2</sub> + 0.5 N <sub>2</sub> → 0.6429 B <sub>9</sub> H <sub>11</sub> + 4.536 ThB <sub>6</sub> + ThB <sub>6</sub> H <sub>4</sub> C <sub>6</sub> N                              | -2.9291             |
| ThNH <sub>4</sub> B <sub>6</sub> C <sub>6</sub> | 1.2 B <sub>5</sub> H <sub>7</sub> + 6 ThC + 9.05 H <sub>2</sub> + ThN → 1.5 Th <sub>4</sub> H <sub>15</sub> + ThB <sub>6</sub> H <sub>4</sub> C <sub>6</sub> N                                                                  | -2.9181             |
| ThNH <sub>4</sub> B <sub>6</sub> C <sub>6</sub> | 5.2 B <sub>5</sub> H <sub>7</sub> + 6 ThC + H <sub>3</sub> N → 5 ThB <sub>4</sub> + 17.7 H <sub>2</sub> + ThB <sub>6</sub> H <sub>4</sub> C <sub>6</sub> N                                                                      | -2.9038             |
| ThNH <sub>4</sub> B <sub>6</sub> C <sub>6</sub> | 0.5 H <sub>2</sub> + 2 Th <sub>2</sub> C <sub>3</sub> + 18 B + H <sub>3</sub> N → 3 ThB <sub>4</sub> + ThB <sub>6</sub> H <sub>4</sub> C <sub>6</sub> N                                                                         | -2.8891             |
| ThNH <sub>4</sub> B <sub>6</sub> C <sub>6</sub> | 6 ThC + 4.667 B <sub>9</sub> H <sub>11</sub> + ThN → 23.67 H <sub>2</sub> + 6 ThB <sub>6</sub> + ThB <sub>6</sub> H <sub>4</sub> C <sub>6</sub> N                                                                               | -2.8815             |
| ThNH <sub>4</sub> B <sub>6</sub> C <sub>6</sub> | 6 ThC + 6 B + 7.667 H <sub>3</sub> N → 1.667 Th <sub>3</sub> N <sub>4</sub> + 9.5 H <sub>2</sub> + ThB <sub>6</sub> H <sub>4</sub> C <sub>6</sub> N                                                                             | -2.8688             |
| ThNH <sub>4</sub> B <sub>6</sub> C <sub>6</sub> | 0.25 Th <sub>3</sub> N <sub>4</sub> + 3.5 ThC + 25.5 B + 0.5 H <sub>8</sub> C <sub>5</sub> → 3.25 ThB <sub>6</sub> + ThB <sub>6</sub> H <sub>4</sub> C <sub>6</sub> N                                                           | -2.8563             |
| ThNH <sub>4</sub> B <sub>6</sub> C <sub>6</sub> | 2 H <sub>2</sub> + 3 ThC <sub>2</sub> + 6 B + 1.833 N <sub>2</sub> → 0.6667 Th <sub>3</sub> N <sub>4</sub> + ThB <sub>6</sub> H <sub>4</sub> C <sub>6</sub> N                                                                   | -2.8538             |
| ThNH <sub>4</sub> B <sub>6</sub> C <sub>6</sub> | 2 ThH <sub>2</sub> + 0.25 Th <sub>3</sub> N <sub>4</sub> + 2 Th <sub>2</sub> C <sub>3</sub> + 14.5 ThB <sub>6</sub> → 20.25 ThB <sub>4</sub> + ThB <sub>6</sub> H <sub>4</sub> C <sub>6</sub> N                                 | -2.8458             |
| ThNH <sub>4</sub> B <sub>6</sub> C <sub>6</sub> | 7.526 ThH <sub>2</sub> + BN + 3 B <sub>13</sub> C <sub>2</sub> → 6.526 ThB <sub>4</sub> + 1.579 B <sub>5</sub> H <sub>7</sub> + ThB <sub>6</sub> H <sub>4</sub> C <sub>6</sub> N                                                | -2.8432             |
| ThNH <sub>4</sub> B <sub>6</sub> C <sub>6</sub> | 2.988 B <sub>5</sub> H <sub>7</sub> + 6 ThC + ThN → 1.128 Th <sub>4</sub> H <sub>15</sub> + 1.49 ThB <sub>6</sub> + ThB <sub>6</sub> H <sub>4</sub> C <sub>6</sub> N                                                            | -2.8307             |
| ThNH <sub>4</sub> B <sub>6</sub> C <sub>6</sub> | 2.668 B <sub>5</sub> H <sub>7</sub> + 0.25 Th <sub>3</sub> N <sub>4</sub> + 6 ThC → 1.836 ThB <sub>4</sub> + 0.9786 Th <sub>4</sub> H <sub>15</sub> + ThB <sub>6</sub> H <sub>4</sub> C <sub>6</sub> N                          | -2.8205             |
| ThNH <sub>4</sub> B <sub>6</sub> C <sub>6</sub> | 1.5 ThB <sub>4</sub> + 6 ThC + 16.06 H <sub>2</sub> + ThN → 1.875 Th <sub>4</sub> H <sub>15</sub> + ThB <sub>6</sub> H <sub>4</sub> C <sub>6</sub> N                                                                            | -2.8121             |
| ThNH <sub>4</sub> B <sub>6</sub> C <sub>6</sub> | 2 H <sub>2</sub> + 3 B <sub>13</sub> C <sub>2</sub> + 23 ThN → 5.5 Th <sub>3</sub> N <sub>4</sub> + 5.5 ThB <sub>6</sub> + ThB <sub>6</sub> H <sub>4</sub> C <sub>6</sub> N                                                     | -2.7889             |
| ThNH <sub>4</sub> B <sub>6</sub> C <sub>6</sub> | 0.7857 ThB <sub>4</sub> + 0.5714 B <sub>5</sub> H <sub>7</sub> + 3 ThC <sub>2</sub> + 2.357 N <sub>2</sub> → 0.9286 Th <sub>3</sub> N <sub>4</sub> + ThB <sub>6</sub> H <sub>4</sub> C <sub>6</sub> N                           | -2.7844             |
| ThNH <sub>4</sub> B <sub>6</sub> C <sub>6</sub> | 0.3636 B <sub>9</sub> H <sub>11</sub> + 0.2098 B <sub>13</sub> C <sub>2</sub> + 1.86 Th <sub>2</sub> C <sub>3</sub> + 1.86 N <sub>2</sub> → 2.72 ThN + ThB <sub>6</sub> H <sub>4</sub> C <sub>6</sub> N                         | -2.7830             |
| ThNH <sub>4</sub> B <sub>6</sub> C <sub>6</sub> | 6 ThC + 17.13 B <sub>9</sub> H <sub>11</sub> + 7.667 H <sub>3</sub> N → 29.63 B <sub>5</sub> H <sub>7</sub> + 1.667 Th <sub>3</sub> N <sub>4</sub> + ThB <sub>6</sub> H <sub>4</sub> C <sub>6</sub> N                           | -2.7729             |
| ThNH <sub>4</sub> B <sub>6</sub> C <sub>6</sub> | 8.533 ThH <sub>2</sub> + 3 B <sub>13</sub> C <sub>2</sub> + 11.04 H <sub>3</sub> N → 6.6 B <sub>5</sub> H <sub>7</sub> + 2.511 Th <sub>3</sub> N <sub>4</sub> + ThB <sub>6</sub> H <sub>4</sub> C <sub>6</sub> N                | -2.7651             |
| ThNH <sub>4</sub> B <sub>6</sub> C <sub>6</sub> | 0.25 Th <sub>3</sub> N <sub>4</sub> + 6 ThC + 14.66 H <sub>2</sub> + ThB <sub>6</sub> → 1.688 Th <sub>4</sub> H <sub>15</sub> + ThB <sub>6</sub> H <sub>4</sub> C <sub>6</sub> N                                                | -2.7494             |
| ThNH <sub>4</sub> B <sub>6</sub> C <sub>6</sub> | 6 C + 0.3636 B <sub>9</sub> H <sub>11</sub> + 2.136 N <sub>2</sub> + ThB <sub>6</sub> → 3.273 BN + ThB <sub>6</sub> H <sub>4</sub> C <sub>6</sub> N                                                                             | -2.7404             |
| ThNH <sub>4</sub> B <sub>6</sub> C <sub>6</sub> | 6 ThC + 1.305 B <sub>9</sub> H <sub>11</sub> + H <sub>3</sub> N → 1.437 ThB <sub>4</sub> + 0.8907 Th <sub>4</sub> H <sub>15</sub> + ThB <sub>6</sub> H <sub>4</sub> C <sub>6</sub> N                                            | -2.7403             |
| ThNH <sub>4</sub> B <sub>6</sub> C <sub>6</sub> | 0.1429 B <sub>5</sub> H <sub>7</sub> + 2 Th <sub>2</sub> C <sub>3</sub> + 17.29 B + H <sub>3</sub> N → 3 ThB <sub>4</sub> + ThB <sub>6</sub> H <sub>4</sub> C <sub>6</sub> N                                                    | -2.7398             |
| ThNH <sub>4</sub> B <sub>6</sub> C <sub>6</sub> | 1.2 B <sub>5</sub> H <sub>7</sub> + 5.533 Th + H <sub>3</sub> N + 1.2 H <sub>8</sub> C <sub>5</sub> → 1.133 Th <sub>4</sub> H <sub>15</sub> + ThB <sub>6</sub> H <sub>4</sub> C <sub>6</sub> N                                  | -2.7393             |
| ThNH <sub>4</sub> B <sub>6</sub> C <sub>6</sub> | 0.25 Th <sub>3</sub> N <sub>4</sub> + 6 ThC + 9.115 H <sub>2</sub> + 0.6667 B <sub>9</sub> H <sub>11</sub> → 1.438 Th <sub>4</sub> H <sub>15</sub> + ThB <sub>6</sub> H <sub>4</sub> C <sub>6</sub> N                           | -2.7358             |
| ThNH <sub>4</sub> B <sub>6</sub> C <sub>6</sub> | 6 ThC + 6 B + 3.926 H <sub>3</sub> N → 0.5185 Th <sub>4</sub> H <sub>15</sub> + 2.926 ThN + ThB <sub>6</sub> H <sub>4</sub> C <sub>6</sub> N                                                                                    | -2.7284             |
| ThNH <sub>4</sub> B <sub>6</sub> C <sub>6</sub> | 0.09091 B <sub>9</sub> H <sub>11</sub> + 2 Th <sub>2</sub> C <sub>3</sub> + 17.18 B + H <sub>3</sub> N → 3 ThB <sub>4</sub> + ThB <sub>6</sub> H <sub>4</sub> C <sub>6</sub> N                                                  | -2.7243             |
| ThNH <sub>4</sub> B <sub>6</sub> C <sub>6</sub> | 0.25 Th <sub>3</sub> N <sub>4</sub> + 6 ThC + 1.763 B <sub>9</sub> H <sub>11</sub> → 1.026 Th <sub>4</sub> H <sub>15</sub> + 1.645 ThB <sub>6</sub> + ThB <sub>6</sub> H <sub>4</sub> C <sub>6</sub> N                          | -2.7134             |
| ThNH <sub>4</sub> B <sub>6</sub> C <sub>6</sub> | 0.5714 B <sub>5</sub> H <sub>7</sub> + 0.2418 B <sub>13</sub> C <sub>2</sub> + 1.839 Th <sub>2</sub> C <sub>3</sub> + 1.839 N <sub>2</sub> → 2.678 ThN + ThB <sub>6</sub> H <sub>4</sub> C <sub>6</sub> N                       | -2.7051             |
| ThNH <sub>4</sub> B <sub>6</sub> C <sub>6</sub> | 1.5 ThB <sub>4</sub> + 0.2667 Th <sub>4</sub> H <sub>15</sub> + 3 ThC <sub>2</sub> + 2.783 N <sub>2</sub> → 4.567 ThN + ThB <sub>6</sub> H <sub>4</sub> C <sub>6</sub> N                                                        | -2.7044             |
| ThNH <sub>4</sub> B <sub>6</sub> C <sub>6</sub> | 1.2 B <sub>5</sub> H <sub>7</sub> + 0.25 Th <sub>3</sub> N <sub>4</sub> + 6 ThC + 8.581 H <sub>2</sub> → 1.437 Th <sub>4</sub> H <sub>15</sub> + ThB <sub>6</sub> H <sub>4</sub> C <sub>6</sub> N                               | -2.6907             |
| ThNH <sub>4</sub> B <sub>6</sub> C <sub>6</sub> | 1.5 ThB <sub>4</sub> + 2 Th <sub>2</sub> C <sub>3</sub> + 1.333 H <sub>3</sub> N + 2.083 N <sub>2</sub> → 4.5 ThN + ThB <sub>6</sub> H <sub>4</sub> C <sub>6</sub> N                                                            | -2.6710             |
| ThNH <sub>4</sub> B <sub>6</sub> C <sub>6</sub> | 0.25 Th <sub>3</sub> N <sub>4</sub> + 6 ThC + 4.5 B <sub>9</sub> H <sub>11</sub> → 22.75 H <sub>2</sub> + 5.75 ThB <sub>6</sub> + ThB <sub>6</sub> H <sub>4</sub> C <sub>6</sub> N                                              | -2.6575             |
| ThNH <sub>4</sub> B <sub>6</sub> C <sub>6</sub> | 0.6818 ThB <sub>4</sub> + 3 ThC <sub>2</sub> + 0.3636 B <sub>9</sub> H <sub>11</sub> + 2.288 N <sub>2</sub> → 0.8939 Th <sub>3</sub> N <sub>4</sub> + ThB <sub>6</sub> H <sub>4</sub> C <sub>6</sub> N                          | -2.6523             |
| ThNH <sub>4</sub> B <sub>6</sub> C <sub>6</sub> | 0.2667 Th <sub>4</sub> H <sub>15</sub> + 2.538 ThC <sub>2</sub> + 0.4615 B <sub>13</sub> C <sub>2</sub> + 2.237 N <sub>2</sub> → 0.8684 Th <sub>3</sub> N <sub>4</sub> + ThB <sub>6</sub> H <sub>4</sub> C <sub>6</sub> N       | -2.6506             |

Continued on next page

Continued

| Compound                                        | Chemical reaction                                                                                                                                                                                               | Reaction energy(eV) |
|-------------------------------------------------|-----------------------------------------------------------------------------------------------------------------------------------------------------------------------------------------------------------------|---------------------|
| ThNH <sub>4</sub> B <sub>6</sub> C <sub>6</sub> | 2.171 B <sub>5</sub> H <sub>7</sub> + 6 ThC + H <sub>3</sub> N → 1.214 ThB <sub>4</sub> + 0.9465 Th <sub>4</sub> H <sub>15</sub> + ThB <sub>6</sub> H <sub>4</sub> C <sub>6</sub> N                             | -2.6362             |
| ThNH <sub>4</sub> B <sub>6</sub> C <sub>6</sub> | 0.2667 Th <sub>4</sub> H <sub>15</sub> + 3 ThC <sub>2</sub> + 6 B + 2.033 N <sub>2</sub> → 3.067 ThN + ThB <sub>6</sub> H <sub>4</sub> C <sub>6</sub> N                                                         | -2.6299             |
| ThNH <sub>4</sub> B <sub>6</sub> C <sub>6</sub> | 1.5 ThB <sub>4</sub> + 3.5 ThC + 0.5 H <sub>8</sub> C <sub>5</sub> + 2.5 N <sub>2</sub> → 4 ThN + ThB <sub>6</sub> H <sub>4</sub> C <sub>6</sub> N                                                              | -2.6204             |
| ThNH <sub>4</sub> B <sub>6</sub> C <sub>6</sub> | 2 Th <sub>2</sub> C <sub>3</sub> + 17 B + 1.333 H <sub>3</sub> N → 2.75 ThB <sub>4</sub> + 0.08333 Th <sub>3</sub> N <sub>4</sub> + ThB <sub>6</sub> H <sub>4</sub> C <sub>6</sub> N                            | -2.6157             |
| ThNH <sub>4</sub> B <sub>6</sub> C <sub>6</sub> | 0.2667 Th <sub>4</sub> H <sub>15</sub> + BN + 2 Th <sub>2</sub> C <sub>3</sub> + 21.27 B → 4.067 ThB <sub>4</sub> + ThB <sub>6</sub> H <sub>4</sub> C <sub>6</sub> N                                            | -2.6136             |
| ThNH <sub>4</sub> B <sub>6</sub> C <sub>6</sub> | 7.323 ThH <sub>2</sub> + BN + 3 B <sub>13</sub> C <sub>2</sub> → 6.323 ThB <sub>4</sub> + 0.9677 B <sub>9</sub> H <sub>11</sub> + ThB <sub>6</sub> H <sub>4</sub> C <sub>6</sub> N                              | -2.6097             |
| ThNH <sub>4</sub> B <sub>6</sub> C <sub>6</sub> | 6 ThC + 11.75 H <sub>2</sub> + H <sub>3</sub> N + ThB <sub>6</sub> → 1.5 Th <sub>4</sub> H <sub>15</sub> + ThB <sub>6</sub> H <sub>4</sub> C <sub>6</sub> N                                                     | -2.6091             |
| ThNH <sub>4</sub> B <sub>6</sub> C <sub>6</sub> | 2.895 B <sub>5</sub> H <sub>7</sub> + 0.25 Th <sub>3</sub> N <sub>4</sub> + 6 ThC → 1.084 Th <sub>4</sub> H <sub>15</sub> + 1.413 ThB <sub>6</sub> + ThB <sub>6</sub> H <sub>4</sub> C <sub>6</sub> N           | -2.6078             |
| ThNH <sub>4</sub> B <sub>6</sub> C <sub>6</sub> | 2 Th <sub>2</sub> C <sub>3</sub> + 6 B + 1.333 H <sub>3</sub> N + 1.333 N <sub>2</sub> → 3 ThN + ThB <sub>6</sub> H <sub>4</sub> C <sub>6</sub> N                                                               | -2.5966             |
| ThNH <sub>4</sub> B <sub>6</sub> C <sub>6</sub> | 6 ThC + 6.208 H <sub>2</sub> + 0.6667 B <sub>9</sub> H <sub>11</sub> + H <sub>3</sub> N → 1.25 Th <sub>4</sub> H <sub>15</sub> + ThB <sub>6</sub> H <sub>4</sub> C <sub>6</sub> N                               | -2.5955             |
| ThNH <sub>4</sub> B <sub>6</sub> C <sub>6</sub> | 1.5 ThB <sub>4</sub> + 0.25 Th <sub>3</sub> N <sub>4</sub> + 6 ThC + 15.59 H <sub>2</sub> → 1.812 Th <sub>4</sub> H <sub>15</sub> + ThB <sub>6</sub> H <sub>4</sub> C <sub>6</sub> N                            | -2.5847             |
| ThNH <sub>4</sub> B <sub>6</sub> C <sub>6</sub> | 6 ThC + 1.414 B <sub>9</sub> H <sub>11</sub> + H <sub>3</sub> N → 0.9699 Th <sub>4</sub> H <sub>15</sub> + 1.12 ThB <sub>6</sub> + ThB <sub>6</sub> H <sub>4</sub> C <sub>6</sub> N                             | -2.5802             |
| ThNH <sub>4</sub> B <sub>6</sub> C <sub>6</sub> | 8.4 B <sub>5</sub> H <sub>7</sub> + 6 ThC + ThN → 27.4 H <sub>2</sub> + 6 ThB <sub>6</sub> + ThB <sub>6</sub> H <sub>4</sub> C <sub>6</sub> N                                                                   | -2.5659             |
| ThNH <sub>4</sub> B <sub>6</sub> C <sub>6</sub> | 6 ThC + 11.38 H <sub>2</sub> + BN + 5 B → 1.25 Th <sub>4</sub> H <sub>15</sub> + ThB <sub>6</sub> H <sub>4</sub> C <sub>6</sub> N                                                                               | -2.5617             |
| ThNH <sub>4</sub> B <sub>6</sub> C <sub>6</sub> | 3 ThC <sub>2</sub> + 6.158 H <sub>3</sub> N + 1.86 ThB <sub>6</sub> → 0.9649 Th <sub>4</sub> H <sub>15</sub> + 5.158 BN + ThB <sub>6</sub> H <sub>4</sub> C <sub>6</sub> N                                      | -2.5599             |
| ThNH <sub>4</sub> B <sub>6</sub> C <sub>6</sub> | 6 ThC + 5.875 H <sub>3</sub> N + 1.813 ThB <sub>6</sub> → 6.813 ThH <sub>2</sub> + 4.875 BN + ThB <sub>6</sub> H <sub>4</sub> C <sub>6</sub> N                                                                  | -2.5597             |
| ThNH <sub>4</sub> B <sub>6</sub> C <sub>6</sub> | 1.2 B <sub>5</sub> H <sub>7</sub> + 6 ThC + 5.675 H <sub>2</sub> + H <sub>3</sub> N → 1.25 Th <sub>4</sub> H <sub>15</sub> + ThB <sub>6</sub> H <sub>4</sub> C <sub>6</sub> N                                   | -2.5504             |
| ThNH <sub>4</sub> B <sub>6</sub> C <sub>6</sub> | 3.5 ThC + 6 B + 0.5 H <sub>8</sub> C <sub>5</sub> + 1.75 N <sub>2</sub> → 2.5 ThN + ThB <sub>6</sub> H <sub>4</sub> C <sub>6</sub> N                                                                            | -2.5460             |
| ThNH <sub>4</sub> B <sub>6</sub> C <sub>6</sub> | 6 ThC + 4 B <sub>9</sub> H <sub>11</sub> + H <sub>3</sub> N → 21.5 H <sub>2</sub> + 5 ThB <sub>6</sub> + ThB <sub>6</sub> H <sub>4</sub> C <sub>6</sub> N                                                       | -2.5274             |
| ThNH <sub>4</sub> B <sub>6</sub> C <sub>6</sub> | 2 H <sub>2</sub> + BN + 2 Th <sub>2</sub> C <sub>3</sub> + 23 B → 3 ThB <sub>6</sub> + ThB <sub>6</sub> H <sub>4</sub> C <sub>6</sub> N                                                                         | -2.5123             |
| ThNH <sub>4</sub> B <sub>6</sub> C <sub>6</sub> | 2.321 B <sub>5</sub> H <sub>7</sub> + 6 ThC + H <sub>3</sub> N → 1.016 Th <sub>4</sub> H <sub>15</sub> + 0.9342 ThB <sub>6</sub> + ThB <sub>6</sub> H <sub>4</sub> C <sub>6</sub> N                             | -2.4956             |
| ThNH <sub>4</sub> B <sub>6</sub> C <sub>6</sub> | 6 C + 3.7 Th <sub>3</sub> N <sub>4</sub> + 2.2 B <sub>9</sub> H <sub>11</sub> → 10.1 ThH <sub>2</sub> + 13.8 BN + ThB <sub>6</sub> H <sub>4</sub> C <sub>6</sub> N                                              | -2.4926             |
| ThNH <sub>4</sub> B <sub>6</sub> C <sub>6</sub> | 0.2667 Th <sub>4</sub> H <sub>15</sub> + 3 ThC <sub>2</sub> + 18.27 B + 0.5 N <sub>2</sub> → 3.067 ThB <sub>4</sub> + ThB <sub>6</sub> H <sub>4</sub> C <sub>6</sub> N                                          | -2.4778             |
| ThNH <sub>4</sub> B <sub>6</sub> C <sub>6</sub> | 2 ThH <sub>2</sub> + 3 B <sub>13</sub> C <sub>2</sub> + 15 ThN → 3.5 Th <sub>3</sub> N <sub>4</sub> + 5.5 ThB <sub>6</sub> + ThB <sub>6</sub> H <sub>4</sub> C <sub>6</sub> N                                   | -2.4775             |
| ThNH <sub>4</sub> B <sub>6</sub> C <sub>6</sub> | 2 Th <sub>2</sub> C <sub>3</sub> + 16.67 B + 1.333 H <sub>3</sub> N → 2.667 ThB <sub>4</sub> + 0.3333 ThN + ThB <sub>6</sub> H <sub>4</sub> C <sub>6</sub> N                                                    | -2.4643             |
| ThNH <sub>4</sub> B <sub>6</sub> C <sub>6</sub> | 0.5714 B <sub>5</sub> H <sub>7</sub> + 3 ThC <sub>2</sub> + 2.183 N <sub>2</sub> + 0.5238 ThB <sub>6</sub> → 0.8413 Th <sub>3</sub> N <sub>4</sub> + ThB <sub>6</sub> H <sub>4</sub> C <sub>6</sub> N           | -2.4573             |
| ThNH <sub>4</sub> B <sub>6</sub> C <sub>6</sub> | 2 Th <sub>2</sub> C <sub>3</sub> + 18 B + 1.333 H <sub>3</sub> N → 3 ThB <sub>4</sub> + 0.1667 N <sub>2</sub> + ThB <sub>6</sub> H <sub>4</sub> C <sub>6</sub> N                                                | -2.4478             |
| ThNH <sub>4</sub> B <sub>6</sub> C <sub>6</sub> | 1.5 ThB <sub>4</sub> + 6 ThC + 12.69 H <sub>2</sub> + H <sub>3</sub> N → 1.625 Th <sub>4</sub> H <sub>15</sub> + ThB <sub>6</sub> H <sub>4</sub> C <sub>6</sub> N                                               | -2.4444             |
| ThNH <sub>4</sub> B <sub>6</sub> C <sub>6</sub> | 0.2667 Th <sub>4</sub> H <sub>15</sub> + 3 ThC <sub>2</sub> + 22.27 B + ThN → 4.067 ThB <sub>4</sub> + ThB <sub>6</sub> H <sub>4</sub> C <sub>6</sub> N                                                         | -2.4282             |
| ThNH <sub>4</sub> B <sub>6</sub> C <sub>6</sub> | 3.5 ThC + 16 B + 0.5 H <sub>8</sub> C <sub>5</sub> + 0.5 N <sub>2</sub> → 2.5 ThB <sub>4</sub> + ThB <sub>6</sub> H <sub>4</sub> C <sub>6</sub> N                                                               | -2.4220             |
| ThNH <sub>4</sub> B <sub>6</sub> C <sub>6</sub> | 1.792 Th <sub>2</sub> C <sub>3</sub> + 21.5 B + H <sub>3</sub> N + 0.125 H <sub>8</sub> C <sub>5</sub> → 2.583 ThB <sub>6</sub> + ThB <sub>6</sub> H <sub>4</sub> C <sub>6</sub> N                              | -2.3923             |
| ThNH <sub>4</sub> B <sub>6</sub> C <sub>6</sub> | 0.2667 Th <sub>4</sub> H <sub>15</sub> + 3 ThC <sub>2</sub> + 2.533 N <sub>2</sub> + ThB <sub>6</sub> → 4.067 ThN + ThB <sub>6</sub> H <sub>4</sub> C <sub>6</sub> N                                            | -2.3909             |
| ThNH <sub>4</sub> B <sub>6</sub> C <sub>6</sub> | 3.5 ThC + 20 B + 0.5 H <sub>8</sub> C <sub>5</sub> + ThN → 3.5 ThB <sub>4</sub> + ThB <sub>6</sub> H <sub>4</sub> C <sub>6</sub> N                                                                              | -2.3724             |
| ThNH <sub>4</sub> B <sub>6</sub> C <sub>6</sub> | 3 ThC <sub>2</sub> + 0.3636 B <sub>9</sub> H <sub>11</sub> + 2.136 N <sub>2</sub> + 0.4545 ThB <sub>6</sub> → 0.8182 Th <sub>3</sub> N <sub>4</sub> + ThB <sub>6</sub> H <sub>4</sub> C <sub>6</sub> N          | -2.3685             |
| ThNH <sub>4</sub> B <sub>6</sub> C <sub>6</sub> | 3.835 ThC + 0.3636 B <sub>9</sub> H <sub>11</sub> + 1.082 B <sub>13</sub> C <sub>2</sub> + 0.5 N <sub>2</sub> → 2.835 ThB <sub>4</sub> + ThB <sub>6</sub> H <sub>4</sub> C <sub>6</sub> N                       | -2.3645             |
| ThNH <sub>4</sub> B <sub>6</sub> C <sub>6</sub> | 2 Th <sub>2</sub> C <sub>3</sub> + 1.333 H <sub>3</sub> N + 1.833 N <sub>2</sub> + ThB <sub>6</sub> → 4 ThN + ThB <sub>6</sub> H <sub>4</sub> C <sub>6</sub> N                                                  | -2.3576             |
| ThNH <sub>4</sub> B <sub>6</sub> C <sub>6</sub> | 8.1 B <sub>5</sub> H <sub>7</sub> + 0.25 Th <sub>3</sub> N <sub>4</sub> + 6 ThC → 26.35 H <sub>2</sub> + 5.75 ThB <sub>6</sub> + ThB <sub>6</sub> H <sub>4</sub> C <sub>6</sub> N                               | -2.3532             |
| ThNH <sub>4</sub> B <sub>6</sub> C <sub>6</sub> | 2 H <sub>2</sub> + 0.4615 B <sub>13</sub> C <sub>2</sub> + 1.692 Th <sub>2</sub> C <sub>3</sub> + 1.692 N <sub>2</sub> → 2.385 ThN + ThB <sub>6</sub> H <sub>4</sub> C <sub>6</sub> N                           | -2.3389             |
| ThNH <sub>4</sub> B <sub>6</sub> C <sub>6</sub> | 2 H <sub>2</sub> + 3 ThC <sub>2</sub> + 24 B + ThN → 3 ThB <sub>6</sub> + ThB <sub>6</sub> H <sub>4</sub> C <sub>6</sub> N                                                                                      | -2.3269             |
| ThNH <sub>4</sub> B <sub>6</sub> C <sub>6</sub> | 6.5 ThH <sub>2</sub> + 3 B <sub>13</sub> C <sub>2</sub> + H <sub>3</sub> N → 6 H <sub>2</sub> + 5.5 ThB <sub>6</sub> + ThB <sub>6</sub> H <sub>4</sub> C <sub>6</sub> N                                         | -2.3189             |
| ThNH <sub>4</sub> B <sub>6</sub> C <sub>6</sub> | 1.2 B <sub>5</sub> H <sub>7</sub> + 4.733 ThH <sub>2</sub> + 1.2 H <sub>8</sub> C <sub>5</sub> + 0.5 N <sub>2</sub> → 0.9333 Th <sub>4</sub> H <sub>15</sub> + ThB <sub>6</sub> H <sub>4</sub> C <sub>6</sub> N | -2.3104             |
| ThNH <sub>4</sub> B <sub>6</sub> C <sub>6</sub> | 3.5 ThC + 0.5 H <sub>8</sub> C <sub>5</sub> + 2.25 N <sub>2</sub> + ThB <sub>6</sub> → 3.5 ThN + ThB <sub>6</sub> H <sub>4</sub> C <sub>6</sub> N                                                               | -2.3070             |
| ThNH <sub>4</sub> B <sub>6</sub> C <sub>6</sub> | 0.5714 B <sub>5</sub> H <sub>7</sub> + 3.796 ThC + 1.102 B <sub>13</sub> C <sub>2</sub> + 0.5 N <sub>2</sub> → 2.796 ThB <sub>4</sub> + ThB <sub>6</sub> H <sub>4</sub> C <sub>6</sub> N                        | -2.3054             |
| ThNH <sub>4</sub> B <sub>6</sub> C <sub>6</sub> | 0.6667 B <sub>9</sub> H <sub>11</sub> + 2 Th <sub>2</sub> C <sub>3</sub> + 1.556 N <sub>2</sub> → 0.2222 Th <sub>4</sub> H <sub>15</sub> + 2.111 ThN + ThB <sub>6</sub> H <sub>4</sub> C <sub>6</sub> N         | -2.3030             |
| ThNH <sub>4</sub> B <sub>6</sub> C <sub>6</sub> | 1.2 B <sub>5</sub> H <sub>7</sub> + 3 ThC <sub>2</sub> + 2.233 N <sub>2</sub> → 1.467 H <sub>3</sub> N + 2 ThN + ThB <sub>6</sub> H <sub>4</sub> C <sub>6</sub> N                                               | -2.2978             |
| ThNH <sub>4</sub> B <sub>6</sub> C <sub>6</sub> | 6 ThC + 0.6667 B <sub>9</sub> H <sub>11</sub> + 3.136 H <sub>3</sub> N → 0.5341 Th <sub>3</sub> N <sub>4</sub> + 0.8495 Th <sub>4</sub> H <sub>15</sub> + ThB <sub>6</sub> H <sub>4</sub> C <sub>6</sub> N      | -2.2957             |
| ThNH <sub>4</sub> B <sub>6</sub> C <sub>6</sub> | 2 ThH <sub>2</sub> + 6 ThC + 6 BN + 2.167 N <sub>2</sub> → 2.333 Th <sub>3</sub> N <sub>4</sub> + ThB <sub>6</sub> H <sub>4</sub> C <sub>6</sub> N                                                              | -2.2840             |
| ThNH <sub>4</sub> B <sub>6</sub> C <sub>6</sub> | 1.2 B <sub>5</sub> H <sub>7</sub> + 6 ThC + 2.953 H <sub>3</sub> N → 0.4882 Th <sub>3</sub> N <sub>4</sub> + 0.8839 Th <sub>4</sub> H <sub>15</sub> + ThB <sub>6</sub> H <sub>4</sub> C <sub>6</sub> N          | -2.2764             |
| ThNH <sub>4</sub> B <sub>6</sub> C <sub>6</sub> | 2 ThH <sub>2</sub> + BN + 3 ThC <sub>2</sub> + 21 B → 4 ThB <sub>4</sub> + ThB <sub>6</sub> H <sub>4</sub> C <sub>6</sub> N                                                                                     | -2.2652             |
| ThNH <sub>4</sub> B <sub>6</sub> C <sub>6</sub> | 7.2 B <sub>5</sub> H <sub>7</sub> + 6 ThC + H <sub>3</sub> N → 24.7 H <sub>2</sub> + 5 ThB <sub>6</sub> + ThB <sub>6</sub> H <sub>4</sub> C <sub>6</sub> N                                                      | -2.2569             |
| ThNH <sub>4</sub> B <sub>6</sub> C <sub>6</sub> | 0.5714 B <sub>5</sub> H <sub>7</sub> + 3 ThC <sub>2</sub> + 3.143 B + 1.833 N <sub>2</sub> → 0.6667 Th <sub>3</sub> N <sub>4</sub> + ThB <sub>6</sub> H <sub>4</sub> C <sub>6</sub> N                           | -2.2567             |
| ThNH <sub>4</sub> B <sub>6</sub> C <sub>6</sub> | 6 ThC + 2.727 BN + 0.3636 B <sub>9</sub> H <sub>11</sub> + 1.636 N <sub>2</sub> → 5 ThN + ThB <sub>6</sub> H <sub>4</sub> C <sub>6</sub> N                                                                      | -2.2504             |
| ThNH <sub>4</sub> B <sub>6</sub> C <sub>6</sub> | BN + 1.75 B <sub>13</sub> C <sub>2</sub> + 3.958 Th + 0.5 H <sub>8</sub> C <sub>5</sub> → 2.958 ThB <sub>6</sub> + ThB <sub>6</sub> H <sub>4</sub> C <sub>6</sub> N                                             | -2.2379             |
| ThNH <sub>4</sub> B <sub>6</sub> C <sub>6</sub> | 3 ThC <sub>2</sub> + 0.3636 B <sub>9</sub> H <sub>11</sub> + 2.727 B + 1.833 N <sub>2</sub> → 0.6667 Th <sub>3</sub> N <sub>4</sub> + ThB <sub>6</sub> H <sub>4</sub> C <sub>6</sub> N                          | -2.1944             |
| ThNH <sub>4</sub> B <sub>6</sub> C <sub>6</sub> | 5.077 ThC + 11.52 H <sub>2</sub> + 0.4615 B <sub>13</sub> C <sub>2</sub> + ThN → 1.269 Th <sub>4</sub> H <sub>15</sub> + ThB <sub>6</sub> H <sub>4</sub> C <sub>6</sub> N                                       | -2.1782             |
| ThNH <sub>4</sub> B <sub>6</sub> C <sub>6</sub> | 2.9 ThB <sub>4</sub> + 6 ThC + 6.6 H <sub>3</sub> N → 7.9 ThH <sub>2</sub> + 5.6 BN + ThB <sub>6</sub> H <sub>4</sub> C <sub>6</sub> N                                                                          | -2.1779             |
| ThNH <sub>4</sub> B <sub>6</sub> C <sub>6</sub> | 0.6667 B <sub>9</sub> H <sub>11</sub> + 5.249 Th + H <sub>3</sub> N + 1.2 H <sub>8</sub> C <sub>5</sub> → 1.062 Th <sub>4</sub> H <sub>15</sub> + ThB <sub>6</sub> H <sub>4</sub> C <sub>6</sub> N              | -2.1611             |
| ThNH <sub>4</sub> B <sub>6</sub> C <sub>6</sub> | 21.56 B <sub>5</sub> H <sub>7</sub> + 6 ThC + ThN → 1.5 Th <sub>4</sub> H <sub>15</sub> + 11.31 B <sub>9</sub> H <sub>11</sub> + ThB <sub>6</sub> H <sub>4</sub> C <sub>6</sub> N                               | -2.1531             |
| ThNH <sub>4</sub> B <sub>6</sub> C <sub>6</sub> | 2 ThH <sub>2</sub> + 2.16 ThC + 1.92 B <sub>13</sub> C <sub>2</sub> + 0.5 N <sub>2</sub> → 3.16 ThB <sub>6</sub> + ThB <sub>6</sub> H <sub>4</sub> C <sub>6</sub> N                                             | -2.1189             |
| ThNH <sub>4</sub> B <sub>6</sub> C <sub>6</sub> | 1.5 ThB <sub>4</sub> + 3 ThC <sub>2</sub> + 1.333 H <sub>3</sub> N + 2.167 N <sub>2</sub> → 1.167 Th <sub>3</sub> N <sub>4</sub> + ThB <sub>6</sub> H <sub>4</sub> C <sub>6</sub> N                             | -2.0958             |

Continued on next page

Continued

| Compound                                        | Chemical reaction                                                                                                                                                                             | Reaction energy(eV) |
|-------------------------------------------------|-----------------------------------------------------------------------------------------------------------------------------------------------------------------------------------------------|---------------------|
| ThNH <sub>4</sub> B <sub>6</sub> C <sub>6</sub> | $2\text{H}_2 + 3\text{ThC}_2 + 18\text{B} + 0.5\text{N}_2 \rightarrow 2\text{ThB}_6 + \text{ThB}_6\text{H}_4\text{C}_6\text{N}$                                                               | -2.0879             |
| ThNH <sub>4</sub> B <sub>6</sub> C <sub>6</sub> | $13.97\text{B}_5\text{H}_7 + 6\text{ThC} + \text{H}_3\text{N} \rightarrow 1.25\text{Th}_4\text{H}_{15} + 7.094\text{B}_9\text{H}_{11} + \text{ThB}_6\text{H}_4\text{C}_6\text{N}$             | -2.0707             |
| ThNH <sub>4</sub> B <sub>6</sub> C <sub>6</sub> | $3.524\text{ThC} + 2\text{H}_2 + 1.238\text{B}_{13}\text{C}_2 + 0.5\text{N}_2 \rightarrow 2.524\text{ThB}_4 + \text{ThB}_6\text{H}_4\text{C}_6\text{N}$                                       | -2.0681             |
| ThNH <sub>4</sub> B <sub>6</sub> C <sub>6</sub> | $6\text{ThC} + \text{BN} + 2.778\text{B}_9\text{H}_{11} \rightarrow 5\text{ThB}_4 + 13.28\text{H}_2 + \text{ThB}_6\text{H}_4\text{C}_6\text{N}$                                               | -2.0580             |
| ThNH <sub>4</sub> B <sub>6</sub> C <sub>6</sub> | $0.4615\text{B}_{13}\text{C}_2 + 1.692\text{Th}_2\text{C}_3 + 1.333\text{H}_3\text{N} + 1.423\text{N}_2 \rightarrow 0.7949\text{Th}_3\text{N}_4 + \text{ThB}_6\text{H}_4\text{C}_6\text{N}$   | -2.0566             |
| ThNH <sub>4</sub> B <sub>6</sub> C <sub>6</sub> | $6\text{ThC} + 5.043\text{H}_3\text{N} + \text{ThB}_6 \rightarrow 1.011\text{Th}_3\text{N}_4 + 0.7419\text{Th}_4\text{H}_{15} + \text{ThB}_6\text{H}_4\text{C}_6\text{N}$                     | -2.0417             |
| ThNH <sub>4</sub> B <sub>6</sub> C <sub>6</sub> | $10.04\text{ThH}_2 + 3\text{B}_{13}\text{C}_2 + 10.04\text{H}_3\text{N} \rightarrow 6.6\text{B}_5\text{H}_7 + 9.04\text{ThN} + \text{ThB}_6\text{H}_4\text{C}_6\text{N}$                      | -1.9863             |
| ThNH <sub>4</sub> B <sub>6</sub> C <sub>6</sub> | $1.2\text{B}_5\text{H}_7 + 2\text{Th}_2\text{C}_3 + 1.413\text{N}_2 \rightarrow 0.2933\text{Th}_4\text{H}_{15} + 1.827\text{ThN} + \text{ThB}_6\text{H}_4\text{C}_6\text{N}$                  | -1.9859             |
| ThNH <sub>4</sub> B <sub>6</sub> C <sub>6</sub> | $0.25\text{Th}_3\text{N}_4 + 0.2667\text{Th}_4\text{H}_{15} + 3\text{ThC}_2 + 21.27\text{B} \rightarrow 3.817\text{ThB}_4 + \text{ThB}_6\text{H}_4\text{C}_6\text{N}$                         | -1.9741             |
| ThNH <sub>4</sub> B <sub>6</sub> C <sub>6</sub> | $0.2667\text{Th}_4\text{H}_{15} + 2\text{Th}_2\text{C}_3 + 0.5\text{N}_2 + 11.13\text{ThB}_6 \rightarrow 15.2\text{ThB}_4 + \text{ThB}_6\text{H}_4\text{C}_6\text{N}$                         | -1.9670             |
| ThNH <sub>4</sub> B <sub>6</sub> C <sub>6</sub> | $6\text{ThC} + 6\text{B} + 6\text{H}_3\text{N} \rightarrow 7\text{H}_2 + 5\text{ThN} + \text{ThB}_6\text{H}_4\text{C}_6\text{N}$                                                              | -1.9657             |
| ThNH <sub>4</sub> B <sub>6</sub> C <sub>6</sub> | $20.51\text{B}_5\text{H}_7 + 0.25\text{Th}_3\text{N}_4 + 6\text{ThC} \rightarrow 1.437\text{Th}_4\text{H}_{15} + 10.73\text{B}_9\text{H}_{11} + \text{ThB}_6\text{H}_4\text{C}_6\text{N}$     | -1.9654             |
| ThNH <sub>4</sub> B <sub>6</sub> C <sub>6</sub> | $7.556\text{ThH}_2 + 3\text{B}_{13}\text{C}_2 + 9.741\text{H}_3\text{N} \rightarrow 2.185\text{Th}_3\text{N}_4 + 3.667\text{B}_9\text{H}_{11} + \text{ThB}_6\text{H}_4\text{C}_6\text{N}$     | -1.9629             |
| ThNH <sub>4</sub> B <sub>6</sub> C <sub>6</sub> | $0.25\text{Th}_3\text{N}_4 + 5.077\text{ThC} + 11.05\text{H}_2 + 0.4615\text{B}_{13}\text{C}_2 \rightarrow 1.207\text{Th}_4\text{H}_{15} + \text{ThB}_6\text{H}_4\text{C}_6\text{N}$          | -1.9508             |
| ThNH <sub>4</sub> B <sub>6</sub> C <sub>6</sub> | $5.5\text{ThH}_2 + 3\text{B}_{13}\text{C}_2 + \text{ThN} \rightarrow 3.5\text{H}_2 + 5.5\text{ThB}_6 + \text{ThB}_6\text{H}_4\text{C}_6\text{N}$                                              | -1.9327             |
| ThNH <sub>4</sub> B <sub>6</sub> C <sub>6</sub> | $1.2\text{B}_5\text{H}_7 + 6\text{ThC} + 2.681\text{H}_3\text{N} \rightarrow 0.8296\text{Th}_4\text{H}_{15} + 1.681\text{ThN} + \text{ThB}_6\text{H}_4\text{C}_6\text{N}$                     | -1.9320             |
| ThNH <sub>4</sub> B <sub>6</sub> C <sub>6</sub> | $2.514\text{B}_9\text{H}_{11} + 1.2\text{H}_8\text{C}_5 + 17.63\text{ThN} \rightarrow 16.63\text{ThH}_2 + 16.63\text{BN} + \text{ThB}_6\text{H}_4\text{C}_6\text{N}$                          | -1.9190             |
| ThNH <sub>4</sub> B <sub>6</sub> C <sub>6</sub> | $6\text{ThC} + 0.6667\text{B}_9\text{H}_{11} + 2.84\text{H}_3\text{N} \rightarrow 0.7901\text{Th}_4\text{H}_{15} + 1.84\text{ThN} + \text{ThB}_6\text{H}_4\text{C}_6\text{N}$                 | -1.9190             |
| ThNH <sub>4</sub> B <sub>6</sub> C <sub>6</sub> | $0.25\text{Th}_3\text{N}_4 + 3.5\text{ThC} + 19\text{B} + 0.5\text{H}_8\text{C}_5 \rightarrow 3.25\text{ThB}_4 + \text{ThB}_6\text{H}_4\text{C}_6\text{N}$                                    | -1.9183             |
| ThNH <sub>4</sub> B <sub>6</sub> C <sub>6</sub> | $0.5714\text{B}_5\text{H}_7 + \text{BN} + 2\text{Th}_2\text{C}_3 + 20.14\text{B} \rightarrow 3\text{ThB}_6 + \text{ThB}_6\text{H}_4\text{C}_6\text{N}$                                        | -1.9151             |
| ThNH <sub>4</sub> B <sub>6</sub> C <sub>6</sub> | $3\text{ThC}_2 + 8.833\text{B} + 3.833\text{H}_3\text{N} \rightarrow 0.5\text{Th}_4\text{H}_{15} + 2.833\text{BN} + \text{ThB}_6\text{H}_4\text{C}_6\text{N}$                                 | -1.8941             |
| ThNH <sub>4</sub> B <sub>6</sub> C <sub>6</sub> | $5.75\text{ThH}_2 + 0.25\text{Th}_3\text{N}_4 + 3\text{B}_{13}\text{C}_2 \rightarrow 3.75\text{H}_2 + 5.5\text{ThB}_6 + \text{ThB}_6\text{H}_4\text{C}_6\text{N}$                             | -1.8938             |
| ThNH <sub>4</sub> B <sub>6</sub> C <sub>6</sub> | $3\text{ThC}_2 + 0.6667\text{B}_9\text{H}_{11} + 2.056\text{N}_2 \rightarrow 1.111\text{H}_3\text{N} + 2\text{ThN} + \text{ThB}_6\text{H}_4\text{C}_6\text{N}$                                | -1.8721             |
| ThNH <sub>4</sub> B <sub>6</sub> C <sub>6</sub> | $5\text{B}_5\text{H}_7 + 6\text{ThC} + \text{BN} \rightarrow 5\text{ThB}_4 + 15.5\text{H}_2 + \text{ThB}_6\text{H}_4\text{C}_6\text{N}$                                                       | -1.8702             |
| ThNH <sub>4</sub> B <sub>6</sub> C <sub>6</sub> | $\text{BN} + 0.3636\text{B}_9\text{H}_{11} + 2\text{Th}_2\text{C}_3 + 19.73\text{B} \rightarrow 3\text{ThB}_6 + \text{ThB}_6\text{H}_4\text{C}_6\text{N}$                                     | -1.8529             |
| ThNH <sub>4</sub> B <sub>6</sub> C <sub>6</sub> | $2\text{ThH}_2 + 2.381\text{ThC} + 1.81\text{B}_{13}\text{C}_2 + \text{ThN} \rightarrow 4.381\text{ThB}_4 + \text{ThB}_6\text{H}_4\text{C}_6\text{N}$                                         | -1.8349             |
| ThNH <sub>4</sub> B <sub>6</sub> C <sub>6</sub> | $1.5\text{ThB}_4 + 6\text{ThC} + 5.366\text{H}_3\text{N} \rightarrow 1.091\text{Th}_3\text{N}_4 + 0.8065\text{Th}_4\text{H}_{15} + \text{ThB}_6\text{H}_4\text{C}_6\text{N}$                  | -1.8317             |
| ThNH <sub>4</sub> B <sub>6</sub> C <sub>6</sub> | $0.2667\text{Th}_4\text{H}_{15} + 3\text{B}_{13}\text{C}_2 + 18.73\text{ThN} \rightarrow 4.433\text{Th}_3\text{N}_4 + 5.5\text{ThB}_6 + \text{ThB}_6\text{H}_4\text{C}_6\text{N}$             | -1.8186             |
| ThNH <sub>4</sub> B <sub>6</sub> C <sub>6</sub> | $5.077\text{ThC} + 8.144\text{H}_2 + 0.4615\text{B}_{13}\text{C}_2 + \text{H}_3\text{N} \rightarrow 1.019\text{Th}_4\text{H}_{15} + \text{ThB}_6\text{H}_4\text{C}_6\text{N}$                 | -1.8105             |
| ThNH <sub>4</sub> B <sub>6</sub> C <sub>6</sub> | $0.25\text{Th}_3\text{N}_4 + 2\text{H}_2 + 3\text{ThC}_2 + 22.5\text{B} \rightarrow 2.75\text{ThB}_6 + \text{ThB}_6\text{H}_4\text{C}_6\text{N}$                                              | -1.8007             |
| ThNH <sub>4</sub> B <sub>6</sub> C <sub>6</sub> | $3.117\text{ThC} + 0.2667\text{Th}_4\text{H}_{15} + 1.441\text{B}_{13}\text{C}_2 + 0.5\text{N}_2 \rightarrow 3.184\text{ThB}_4 + \text{ThB}_6\text{H}_4\text{C}_6\text{N}$                    | -1.7890             |
| ThNH <sub>4</sub> B <sub>6</sub> C <sub>6</sub> | $3\text{ThC}_2 + 2.75\text{B}_9\text{H}_{11} + 1.833\text{N}_2 \rightarrow 3.75\text{B}_5\text{H}_7 + 0.6667\text{Th}_3\text{N}_4 + \text{ThB}_6\text{H}_4\text{C}_6\text{N}$                 | -1.7858             |
| ThNH <sub>4</sub> B <sub>6</sub> C <sub>6</sub> | $6\text{ThC} + \text{BN} + 1.412\text{B}_9\text{H}_{11} \rightarrow 1.926\text{ThB}_4 + 0.7685\text{Th}_4\text{H}_{15} + \text{ThB}_6\text{H}_4\text{C}_6\text{N}$                            | -1.7483             |
| ThNH <sub>4</sub> B <sub>6</sub> C <sub>6</sub> | $0.5\text{ThH}_2 + 3\text{ThC}_2 + 21\text{B} + \text{H}_3\text{N} \rightarrow 2.5\text{ThB}_6 + \text{ThB}_6\text{H}_4\text{C}_6\text{N}$                                                    | -1.7385             |
| ThNH <sub>4</sub> B <sub>6</sub> C <sub>6</sub> | $0.5714\text{B}_5\text{H}_7 + 6\text{C} + 1.929\text{N}_2 + \text{ThB}_6 \rightarrow 2.857\text{BN} + \text{ThB}_6\text{H}_4\text{C}_6\text{N}$                                               | -1.7360             |
| ThNH <sub>4</sub> B <sub>6</sub> C <sub>6</sub> | $0.6667\text{B}_9\text{H}_{11} + 4.449\text{Th} + 1.2\text{H}_8\text{C}_5 + 0.5\text{N}_2 \rightarrow 0.8622\text{Th}_4\text{H}_{15} + \text{ThB}_6\text{H}_4\text{C}_6\text{N}$              | -1.7322             |
| ThNH <sub>4</sub> B <sub>6</sub> C <sub>6</sub> | $3.25\text{B}_5\text{H}_7 + 6\text{ThC} + 0.5\text{N}_2 \rightarrow 1.25\text{Th}_4\text{H}_{15} + 10.25\text{B} + \text{ThB}_6\text{H}_4\text{C}_6\text{N}$                                  | -1.7321             |
| ThNH <sub>4</sub> B <sub>6</sub> C <sub>6</sub> | $0.5714\text{B}_5\text{H}_7 + 3\text{ThC}_2 + 21.14\text{B} + \text{ThN} \rightarrow 3\text{ThB}_6 + \text{ThB}_6\text{H}_4\text{C}_6\text{N}$                                                | -1.7297             |
| ThNH <sub>4</sub> B <sub>6</sub> C <sub>6</sub> | $14.38\text{H}_2 + 3\text{B}_{13}\text{C}_2 + 9.25\text{ThN} \rightarrow 8.25\text{ThB}_4 + 8.25\text{H}_3\text{N} + \text{ThB}_6\text{H}_4\text{C}_6\text{N}$                                | -1.7259             |
| ThNH <sub>4</sub> B <sub>6</sub> C <sub>6</sub> | $1.5\text{ThB}_4 + 2\text{H}_2 + 3\text{ThC}_2 + 2.25\text{N}_2 \rightarrow 3.5\text{ThN} + \text{ThB}_6\text{H}_4\text{C}_6\text{N}$                                                         | -1.6843             |
| ThNH <sub>4</sub> B <sub>6</sub> C <sub>6</sub> | $0.6875\text{B}_{13}\text{C}_2 + 1.542\text{Th}_2\text{C}_3 + 3.937\text{H}_3\text{N} \rightarrow 0.5208\text{Th}_4\text{H}_{15} + 2.937\text{BN} + \text{ThB}_6\text{H}_4\text{C}_6\text{N}$ | -1.6824             |
| ThNH <sub>4</sub> B <sub>6</sub> C <sub>6</sub> | $2\text{ThH}_2 + 0.25\text{Th}_3\text{N}_4 + 2.476\text{ThC} + 1.762\text{B}_{13}\text{C}_2 \rightarrow 4.226\text{ThB}_4 + \text{ThB}_6\text{H}_4\text{C}_6\text{N}$                         | -1.6729             |
| ThNH <sub>4</sub> B <sub>6</sub> C <sub>6</sub> | $3\text{ThC}_2 + 0.3636\text{B}_9\text{H}_{11} + 20.73\text{B} + \text{ThN} \rightarrow 3\text{ThB}_6 + \text{ThB}_6\text{H}_4\text{C}_6\text{N}$                                             | -1.6675             |
| ThNH <sub>4</sub> B <sub>6</sub> C <sub>6</sub> | $3.382\text{ThC} + 0.3636\text{B}_9\text{H}_{11} + 1.309\text{B}_{13}\text{C}_2 + 0.5\text{N}_2 \rightarrow 2.382\text{ThB}_6 + \text{ThB}_6\text{H}_4\text{C}_6\text{N}$                     | -1.6606             |
| ThNH <sub>4</sub> B <sub>6</sub> C <sub>6</sub> | $6\text{ThC} + 0.6667\text{B}_9\text{H}_{11} + 7.667\text{H}_3\text{N} \rightarrow 1.667\text{Th}_3\text{N}_4 + 13.17\text{H}_2 + \text{ThB}_6\text{H}_4\text{C}_6\text{N}$                   | -1.6599             |
| ThNH <sub>4</sub> B <sub>6</sub> C <sub>6</sub> | $6\text{ThC} + 14\text{B}_9\text{H}_{11} + 6\text{H}_3\text{N} \rightarrow 24\text{B}_5\text{H}_7 + 5\text{ThN} + \text{ThB}_6\text{H}_4\text{C}_6\text{N}$                                   | -1.6584             |
| ThNH <sub>4</sub> B <sub>6</sub> C <sub>6</sub> | $2\text{ThH}_2 + 3\text{ThC}_2 + 0.5\text{N}_2 + 11\text{ThB}_6 \rightarrow 15\text{ThB}_4 + \text{ThB}_6\text{H}_4\text{C}_6\text{N}$                                                        | -1.6571             |
| ThNH <sub>4</sub> B <sub>6</sub> C <sub>6</sub> | $1.792\text{Th}_2\text{C}_3 + 16.33\text{B} + \text{H}_3\text{N} + 0.125\text{H}_8\text{C}_5 \rightarrow 2.583\text{ThB}_4 + \text{ThB}_6\text{H}_4\text{C}_6\text{N}$                        | -1.6467             |
| ThNH <sub>4</sub> B <sub>6</sub> C <sub>6</sub> | $2\text{H}_2 + \text{BN} + 2\text{Th}_2\text{C}_3 + 17\text{B} \rightarrow 3\text{ThB}_4 + \text{ThB}_6\text{H}_4\text{C}_6\text{N}$                                                          | -1.6464             |
| ThNH <sub>4</sub> B <sub>6</sub> C <sub>6</sub> | $3\text{ThC}_2 + 0.6667\text{B}_9\text{H}_{11} + 1.833\text{N}_2 \rightarrow 0.6667\text{Th}_3\text{N}_4 + 1.667\text{H}_2 + \text{ThB}_6\text{H}_4\text{C}_6\text{N}$                        | -1.6449             |
| ThNH <sub>4</sub> B <sub>6</sub> C <sub>6</sub> | $2.348\text{B}_5\text{H}_7 + 6\text{ThC} + \text{BN} \rightarrow 1.684\text{ThB}_4 + 0.8289\text{Th}_4\text{H}_{15} + \text{ThB}_6\text{H}_4\text{C}_6\text{N}$                               | -1.6358             |
| ThNH <sub>4</sub> B <sub>6</sub> C <sub>6</sub> | $2\text{H}_2 + 2\text{Th}_2\text{C}_3 + 0.5\text{N}_2 + 9\text{ThB}_6 \rightarrow 12\text{ThB}_4 + \text{ThB}_6\text{H}_4\text{C}_6\text{N}$                                                  | -1.6156             |
| ThNH <sub>4</sub> B <sub>6</sub> C <sub>6</sub> | $1.2\text{B}_5\text{H}_7 + 6\text{ThC} + 7.667\text{H}_3\text{N} \rightarrow 1.667\text{Th}_3\text{N}_4 + 13.7\text{H}_2 + \text{ThB}_6\text{H}_4\text{C}_6\text{N}$                          | -1.6148             |
| ThNH <sub>4</sub> B <sub>6</sub> C <sub>6</sub> | $0.5714\text{B}_5\text{H}_7 + 3.349\text{ThC} + 1.326\text{B}_{13}\text{C}_2 + 0.5\text{N}_2 \rightarrow 2.349\text{ThB}_6 + \text{ThB}_6\text{H}_4\text{C}_6\text{N}$                        | -1.6113             |
| ThNH <sub>4</sub> B <sub>6</sub> C <sub>6</sub> | $2\text{H}_2 + 3\text{ThC}_2 + 6\text{B} + 1.5\text{N}_2 \rightarrow 2\text{ThN} + \text{ThB}_6\text{H}_4\text{C}_6\text{N}$                                                                  | -1.6099             |
| ThNH <sub>4</sub> B <sub>6</sub> C <sub>6</sub> | $1.2\text{B}_5\text{H}_7 + 3\text{ThC}_2 + 1.833\text{N}_2 \rightarrow 0.6667\text{Th}_3\text{N}_4 + 2.2\text{H}_2 + \text{ThB}_6\text{H}_4\text{C}_6\text{N}$                                | -1.5998             |
| ThNH <sub>4</sub> B <sub>6</sub> C <sub>6</sub> | $4.651\text{ThC} + 0.6744\text{B}_{13}\text{C}_2 + 3.767\text{H}_3\text{N} \rightarrow 3.651\text{ThH}_2 + 2.767\text{BN} + \text{ThB}_6\text{H}_4\text{C}_6\text{N}$                         | -1.5771             |
| ThNH <sub>4</sub> B <sub>6</sub> C <sub>6</sub> | $6\text{ThC} + 12.94\text{H}_2 + \text{BN} + 0.8333\text{ThB}_6 \rightarrow 1.458\text{Th}_4\text{H}_{15} + \text{ThB}_6\text{H}_4\text{C}_6\text{N}$                                         | -1.5656             |
| ThNH <sub>4</sub> B <sub>6</sub> C <sub>6</sub> | $6\text{ThC} + 8.319\text{H}_2 + \text{BN} + 0.5556\text{B}_9\text{H}_{11} \rightarrow 1.25\text{Th}_4\text{H}_{15} + \text{ThB}_6\text{H}_4\text{C}_6\text{N}$                               | -1.5543             |
| ThNH <sub>4</sub> B <sub>6</sub> C <sub>6</sub> | $6\text{ThC} + \text{BN} + 1.556\text{B}_9\text{H}_{11} \rightarrow 0.8747\text{Th}_4\text{H}_{15} + 1.501\text{ThB}_6 + \text{ThB}_6\text{H}_4\text{C}_6\text{N}$                            | -1.5338             |

Continued on next page

Continued

| Compound                                        | Chemical reaction                                                                                                                                                                                                       | Reaction energy(eV) |
|-------------------------------------------------|-------------------------------------------------------------------------------------------------------------------------------------------------------------------------------------------------------------------------|---------------------|
| ThNH <sub>4</sub> B <sub>6</sub> C <sub>6</sub> | B <sub>5</sub> H <sub>7</sub> + 6 ThC + 7.875 H <sub>2</sub> + BN → 1.25 Th <sub>4</sub> H <sub>15</sub> + ThB <sub>6</sub> H <sub>4</sub> C <sub>6</sub> N                                                             | -1.5167             |
| ThNH <sub>4</sub> B <sub>6</sub> C <sub>6</sub> | 5.346 ThH <sub>2</sub> + 3 B <sub>13</sub> C <sub>2</sub> + H <sub>3</sub> N → 1.385 B <sub>5</sub> H <sub>7</sub> + 4.346 ThB <sub>6</sub> + ThB <sub>6</sub> H <sub>4</sub> C <sub>6</sub> N                          | -1.5167             |
| ThNH <sub>4</sub> B <sub>6</sub> C <sub>6</sub> | 2 H <sub>2</sub> + 3 ThC <sub>2</sub> + 14 B + 0.5 N <sub>2</sub> → 2 ThB <sub>4</sub> + ThB <sub>6</sub> H <sub>4</sub> C <sub>6</sub> N                                                                               | -1.5107             |
| ThNH <sub>4</sub> B <sub>6</sub> C <sub>6</sub> | 7.625 H <sub>2</sub> + 2 Th <sub>2</sub> C <sub>3</sub> + 6 B + 0.5 N <sub>2</sub> → 0.75 Th <sub>4</sub> H <sub>15</sub> + ThB <sub>6</sub> H <sub>4</sub> C <sub>6</sub> N                                            | -1.4930             |
| ThNH <sub>4</sub> B <sub>6</sub> C <sub>6</sub> | 0.5714 B <sub>5</sub> H <sub>7</sub> + 3 ThC <sub>2</sub> + 15.14 B + 0.5 N <sub>2</sub> → 2 ThB <sub>6</sub> + ThB <sub>6</sub> H <sub>4</sub> C <sub>6</sub> N                                                        | -1.4907             |
| ThNH <sub>4</sub> B <sub>6</sub> C <sub>6</sub> | 6 ThC + 9 H <sub>3</sub> N + ThB <sub>6</sub> → 2 Th <sub>3</sub> N <sub>4</sub> + 11.5 H <sub>2</sub> + ThB <sub>6</sub> H <sub>4</sub> C <sub>6</sub> N                                                               | -1.4864             |
| ThNH <sub>4</sub> B <sub>6</sub> C <sub>6</sub> | 6 ThC + BN + 3.889 B <sub>9</sub> H <sub>11</sub> → 19.39 H <sub>2</sub> + 5 ThB <sub>6</sub> + ThB <sub>6</sub> H <sub>4</sub> C <sub>6</sub> N                                                                        | -1.4862             |
| ThNH <sub>4</sub> B <sub>6</sub> C <sub>6</sub> | 3.154 B <sub>9</sub> H <sub>11</sub> + 3 B <sub>13</sub> C <sub>2</sub> + 11.23 ThN → 10.23 H <sub>3</sub> N + 10.23 ThB <sub>6</sub> + ThB <sub>6</sub> H <sub>4</sub> C <sub>6</sub> N                                | -1.4839             |
| ThNH <sub>4</sub> B <sub>6</sub> C <sub>6</sub> | 3 ThC <sub>2</sub> + 1.333 H <sub>3</sub> N + 1.833 N <sub>2</sub> + ThB <sub>6</sub> → Th <sub>3</sub> N <sub>4</sub> + ThB <sub>6</sub> H <sub>4</sub> C <sub>6</sub> N                                               | -1.4714             |
| ThNH <sub>4</sub> B <sub>6</sub> C <sub>6</sub> | 4.827 ThH <sub>2</sub> + 3 B <sub>13</sub> C <sub>2</sub> + ThN → 0.8077 B <sub>5</sub> H <sub>7</sub> + 4.827 ThB <sub>6</sub> + ThB <sub>6</sub> H <sub>4</sub> C <sub>6</sub> N                                      | -1.4647             |
| ThNH <sub>4</sub> B <sub>6</sub> C <sub>6</sub> | 2 H <sub>2</sub> + 3 ThC <sub>2</sub> + 18 B + ThN → 3 ThB <sub>4</sub> + ThB <sub>6</sub> H <sub>4</sub> C <sub>6</sub> N                                                                                              | -1.4610             |
| ThNH <sub>4</sub> B <sub>6</sub> C <sub>6</sub> | 3.12 ThC + 2 H <sub>2</sub> + 1.44 B <sub>13</sub> C <sub>2</sub> + 0.5 N <sub>2</sub> → 2.12 ThB <sub>6</sub> + ThB <sub>6</sub> H <sub>4</sub> C <sub>6</sub> N                                                       | -1.4415             |
| ThNH <sub>4</sub> B <sub>6</sub> C <sub>6</sub> | 2.556 B <sub>5</sub> H <sub>7</sub> + 6 ThC + BN → 0.9259 Th <sub>4</sub> H <sub>15</sub> + 1.296 ThB <sub>6</sub> + ThB <sub>6</sub> H <sub>4</sub> C <sub>6</sub> N                                                   | -1.4406             |
| ThNH <sub>4</sub> B <sub>6</sub> C <sub>6</sub> | 0.5714 B <sub>5</sub> H <sub>7</sub> + 2 Th <sub>2</sub> C <sub>3</sub> + 0.5 N <sub>2</sub> + 7.571 ThB <sub>6</sub> → 10.57 ThB <sub>4</sub> + ThB <sub>6</sub> H <sub>4</sub> C <sub>6</sub> N                       | -1.4308             |
| ThNH <sub>4</sub> B <sub>6</sub> C <sub>6</sub> | 0.3636 B <sub>9</sub> H <sub>11</sub> + 2 Th <sub>2</sub> C <sub>3</sub> + 0.5 N <sub>2</sub> + 7.364 ThB <sub>6</sub> → 10.36 ThB <sub>4</sub> + ThB <sub>6</sub> H <sub>4</sub> C <sub>6</sub> N                      | -1.4285             |
| ThNH <sub>4</sub> B <sub>6</sub> C <sub>6</sub> | 3 ThC <sub>2</sub> + 0.3636 B <sub>9</sub> H <sub>11</sub> + 14.73 B + 0.5 N <sub>2</sub> → 2 ThB <sub>6</sub> + ThB <sub>6</sub> H <sub>4</sub> C <sub>6</sub> N                                                       | -1.4285             |
| ThNH <sub>4</sub> B <sub>6</sub> C <sub>6</sub> | 1.25 ThB <sub>4</sub> + 6 ThC + 13.72 H <sub>2</sub> + BN → 1.562 Th <sub>4</sub> H <sub>15</sub> + ThB <sub>6</sub> H <sub>4</sub> C <sub>6</sub> N                                                                    | -1.4283             |
| ThNH <sub>4</sub> B <sub>6</sub> C <sub>6</sub> | 2 Th <sub>2</sub> C <sub>3</sub> + 15 B + 5 H <sub>3</sub> N → Th <sub>3</sub> N <sub>4</sub> + B <sub>9</sub> H <sub>11</sub> + ThB <sub>6</sub> H <sub>4</sub> C <sub>6</sub> N                                       | -1.4210             |
| ThNH <sub>4</sub> B <sub>6</sub> C <sub>6</sub> | 5.077 ThC + 0.4615 B <sub>13</sub> C <sub>2</sub> + 3.802 H <sub>3</sub> N → 0.7006 Th <sub>3</sub> N <sub>4</sub> + 0.4938 Th <sub>4</sub> H <sub>15</sub> + ThB <sub>6</sub> H <sub>4</sub> C <sub>6</sub> N          | -1.4172             |
| ThNH <sub>4</sub> B <sub>6</sub> C <sub>6</sub> | 0.25 Th <sub>3</sub> N <sub>4</sub> + 1.75 B <sub>13</sub> C <sub>2</sub> + 3.042 Th + 0.5 H <sub>8</sub> C <sub>5</sub> → 2.792 ThB <sub>6</sub> + ThB <sub>6</sub> H <sub>4</sub> C <sub>6</sub> N                    | -1.4131             |
| ThNH <sub>4</sub> B <sub>6</sub> C <sub>6</sub> | 2 ThH <sub>2</sub> + 1.418 B <sub>13</sub> C <sub>2</sub> + 1.055 Th <sub>2</sub> C <sub>3</sub> + 0.5 N <sub>2</sub> → 3.109 ThB <sub>4</sub> + ThB <sub>6</sub> H <sub>4</sub> C <sub>6</sub> N                       | -1.4118             |
| ThNH <sub>4</sub> B <sub>6</sub> C <sub>6</sub> | 6.667 ThH <sub>2</sub> + BN + 3 B <sub>13</sub> C <sub>2</sub> → 4.667 H <sub>2</sub> + 5.667 ThB <sub>6</sub> + ThB <sub>6</sub> H <sub>4</sub> C <sub>6</sub> N                                                       | -1.4011             |
| ThNH <sub>4</sub> B <sub>6</sub> C <sub>6</sub> | 5.029 ThH <sub>2</sub> + 0.25 Th <sub>3</sub> N <sub>4</sub> + 3 B <sub>13</sub> C <sub>2</sub> → 0.8654 B <sub>5</sub> H <sub>7</sub> + 4.779 ThB <sub>6</sub> + ThB <sub>6</sub> H <sub>4</sub> C <sub>6</sub> N      | -1.3924             |
| ThNH <sub>4</sub> B <sub>6</sub> C <sub>6</sub> | 4.1 ThH <sub>2</sub> + 3 B <sub>13</sub> C <sub>2</sub> + 2.4 ThN → 1.4 H <sub>3</sub> N + 5.5 ThB <sub>6</sub> + ThB <sub>6</sub> H <sub>4</sub> C <sub>6</sub> N                                                      | -1.3920             |
| ThNH <sub>4</sub> B <sub>6</sub> C <sub>6</sub> | 6 ThC + 2.068 B <sub>9</sub> H <sub>11</sub> + 0.5 N <sub>2</sub> → 1.25 Th <sub>4</sub> H <sub>15</sub> + 12.61 B + ThB <sub>6</sub> H <sub>4</sub> C <sub>6</sub> N                                                   | -1.3780             |
| ThNH <sub>4</sub> B <sub>6</sub> C <sub>6</sub> | 4.75 ThH <sub>2</sub> + 3 B <sub>13</sub> C <sub>2</sub> + ThN → 0.5 B <sub>9</sub> H <sub>11</sub> + 4.75 ThB <sub>6</sub> + ThB <sub>6</sub> H <sub>4</sub> C <sub>6</sub> N                                          | -1.3774             |
| ThNH <sub>4</sub> B <sub>6</sub> C <sub>6</sub> | 2 H <sub>2</sub> + 3 ThC <sub>2</sub> + 2 N <sub>2</sub> + ThB <sub>6</sub> → 3 ThN + ThB <sub>6</sub> H <sub>4</sub> C <sub>6</sub> N                                                                                  | -1.3709             |
| ThNH <sub>4</sub> B <sub>6</sub> C <sub>6</sub> | 5.214 ThH <sub>2</sub> + 3 B <sub>13</sub> C <sub>2</sub> + H <sub>3</sub> N → 0.8571 B <sub>9</sub> H <sub>11</sub> + 4.214 ThB <sub>6</sub> + ThB <sub>6</sub> H <sub>4</sub> C <sub>6</sub> N                        | -1.3670             |
| ThNH <sub>4</sub> B <sub>6</sub> C <sub>6</sub> | 1.2 B <sub>5</sub> H <sub>7</sub> + 0.25 Th <sub>3</sub> N <sub>4</sub> + 7.25 Th + 1.2 H <sub>8</sub> C <sub>5</sub> → 7 ThH <sub>2</sub> + ThB <sub>6</sub> H <sub>4</sub> C <sub>6</sub> N                           | -1.3636             |
| ThNH <sub>4</sub> B <sub>6</sub> C <sub>6</sub> | 2 ThH <sub>2</sub> + BN + 2 Th <sub>2</sub> C <sub>3</sub> + 12.5 ThB <sub>6</sub> → 17.5 ThB <sub>4</sub> + ThB <sub>6</sub> H <sub>4</sub> C <sub>6</sub> N                                                           | -1.3600             |
| ThNH <sub>4</sub> B <sub>6</sub> C <sub>6</sub> | 6 ThC + 7 H <sub>2</sub> + 6 B + 0.5 N <sub>2</sub> → 5 ThH <sub>2</sub> + ThB <sub>6</sub> H <sub>4</sub> C <sub>6</sub> N                                                                                             | -1.3588             |
| ThNH <sub>4</sub> B <sub>6</sub> C <sub>6</sub> | 13.25 B <sub>9</sub> H <sub>11</sub> + 2 Th <sub>2</sub> C <sub>3</sub> + 0.5 N <sub>2</sub> → 3 ThB <sub>4</sub> + 20.25 B <sub>5</sub> H <sub>7</sub> + ThB <sub>6</sub> H <sub>4</sub> C <sub>6</sub> N              | -1.3471             |
| ThNH <sub>4</sub> B <sub>6</sub> C <sub>6</sub> | 0.2667 Th <sub>4</sub> H <sub>15</sub> + 2 Th <sub>2</sub> C <sub>3</sub> + 13.13 ThB <sub>6</sub> + ThN → 18.2 ThB <sub>4</sub> + ThB <sub>6</sub> H <sub>4</sub> C <sub>6</sub> N                                     | -1.3402             |
| ThNH <sub>4</sub> B <sub>6</sub> C <sub>6</sub> | 2.79 ThC <sub>2</sub> + 0.3636 B <sub>9</sub> H <sub>11</sub> + 0.2098 B <sub>13</sub> C <sub>2</sub> + 1.693 N <sub>2</sub> → 0.5967 Th <sub>3</sub> N <sub>4</sub> + ThB <sub>6</sub> H <sub>4</sub> C <sub>6</sub> N | -1.3368             |
| ThNH <sub>4</sub> B <sub>6</sub> C <sub>6</sub> | 6 ThC + 4.481 H <sub>3</sub> N + ThB <sub>6</sub> → 0.6296 Th <sub>4</sub> H <sub>15</sub> + 3.481 ThN + ThB <sub>6</sub> H <sub>4</sub> C <sub>6</sub> N                                                               | -1.3288             |
| ThNH <sub>4</sub> B <sub>6</sub> C <sub>6</sub> | 18.5 B <sub>9</sub> H <sub>11</sub> + 2 Th <sub>2</sub> C <sub>3</sub> + 0.5 N <sub>2</sub> → 28.5 B <sub>5</sub> H <sub>7</sub> + 3 ThB <sub>6</sub> + ThB <sub>6</sub> H <sub>4</sub> C <sub>6</sub> N                | -1.3140             |
| ThNH <sub>4</sub> B <sub>6</sub> C <sub>6</sub> | 4.946 ThH <sub>2</sub> + 0.25 Th <sub>3</sub> N <sub>4</sub> + 3 B <sub>13</sub> C <sub>2</sub> → 0.5357 B <sub>9</sub> H <sub>11</sub> + 4.696 ThB <sub>6</sub> + ThB <sub>6</sub> H <sub>4</sub> C <sub>6</sub> N     | -1.2988             |
| ThNH <sub>4</sub> B <sub>6</sub> C <sub>6</sub> | 8.867 ThH <sub>2</sub> + 3 B <sub>13</sub> C <sub>2</sub> + 8.867 H <sub>3</sub> N → 3.667 B <sub>9</sub> H <sub>11</sub> + 7.867 ThN + ThB <sub>6</sub> H <sub>4</sub> C <sub>6</sub> N                                | -1.2852             |
| ThNH <sub>4</sub> B <sub>6</sub> C <sub>6</sub> | 0.5714 B <sub>5</sub> H <sub>7</sub> + 2.758 ThC <sub>2</sub> + 0.2418 B <sub>13</sub> C <sub>2</sub> + 1.672 N <sub>2</sub> → 0.5861 Th <sub>3</sub> N <sub>4</sub> + ThB <sub>6</sub> H <sub>4</sub> C <sub>6</sub> N | -1.2684             |
| ThNH <sub>4</sub> B <sub>6</sub> C <sub>6</sub> | 25.1 H <sub>2</sub> + 3 B <sub>13</sub> C <sub>2</sub> + Th + 0.5 N <sub>2</sub> → 6.6 B <sub>5</sub> H <sub>7</sub> + ThB <sub>6</sub> H <sub>4</sub> C <sub>6</sub> N                                                 | -1.2564             |
| ThNH <sub>4</sub> B <sub>6</sub> C <sub>6</sub> | 2 Th <sub>2</sub> C <sub>3</sub> + 13.86 B + 5 H <sub>3</sub> N → 1.571 B <sub>5</sub> H <sub>7</sub> + Th <sub>3</sub> N <sub>4</sub> + ThB <sub>6</sub> H <sub>4</sub> C <sub>6</sub> N                               | -1.2498             |
| ThNH <sub>4</sub> B <sub>6</sub> C <sub>6</sub> | 0.5714 B <sub>5</sub> H <sub>7</sub> + 6 ThC + 3.143 BN + 1.429 N <sub>2</sub> → 5 ThN + ThB <sub>6</sub> H <sub>4</sub> C <sub>6</sub> N                                                                               | -1.2460             |
| ThNH <sub>4</sub> B <sub>6</sub> C <sub>6</sub> | 1.5 ThB <sub>4</sub> + 6 ThC + 9.667 H <sub>3</sub> N → 2.167 Th <sub>3</sub> N <sub>4</sub> + 12.5 H <sub>2</sub> + ThB <sub>6</sub> H <sub>4</sub> C <sub>6</sub> N                                                   | -1.2281             |
| ThNH <sub>4</sub> B <sub>6</sub> C <sub>6</sub> | 7 B <sub>5</sub> H <sub>7</sub> + 6 ThC + BN → 22.5 H <sub>2</sub> + 5 ThB <sub>6</sub> + ThB <sub>6</sub> H <sub>4</sub> C <sub>6</sub> N                                                                              | -1.2232             |
| ThNH <sub>4</sub> B <sub>6</sub> C <sub>6</sub> | 0.5714 B <sub>5</sub> H <sub>7</sub> + 0.25 Th <sub>3</sub> N <sub>4</sub> + 3 ThC <sub>2</sub> + 19.64 B → 2.75 ThB <sub>6</sub> + ThB <sub>6</sub> H <sub>4</sub> C <sub>6</sub> N                                    | -1.2035             |
| ThNH <sub>4</sub> B <sub>6</sub> C <sub>6</sub> | 4.5 ThH <sub>2</sub> + 0.6667 Th <sub>3</sub> N <sub>4</sub> + 3 B <sub>13</sub> C <sub>2</sub> → 1.667 H <sub>3</sub> N + 5.5 ThB <sub>6</sub> + ThB <sub>6</sub> H <sub>4</sub> C <sub>6</sub> N                      | -1.1852             |
| ThNH <sub>4</sub> B <sub>6</sub> C <sub>6</sub> | 3 ThC <sub>2</sub> + 18.33 B + 1.333 H <sub>3</sub> N → 0.3333 BN + 2 ThB <sub>6</sub> + ThB <sub>6</sub> H <sub>4</sub> C <sub>6</sub> N                                                                               | -1.1780             |
| ThNH <sub>4</sub> B <sub>6</sub> C <sub>6</sub> | 6 C + 6 BN + 7.333 Th + 1.333 H <sub>3</sub> N → 6.333 ThN + ThB <sub>6</sub> H <sub>4</sub> C <sub>6</sub> N                                                                                                           | -1.1546             |
| ThNH <sub>4</sub> B <sub>6</sub> C <sub>6</sub> | 3.455 ThC + 0.3636 B <sub>9</sub> H <sub>11</sub> + 1.273 B <sub>13</sub> C <sub>2</sub> + ThN → 3.455 ThB <sub>4</sub> + ThB <sub>6</sub> H <sub>4</sub> C <sub>6</sub> N                                              | -1.1466             |
| ThNH <sub>4</sub> B <sub>6</sub> C <sub>6</sub> | 1.5 ThB <sub>4</sub> + 1.167 Th <sub>2</sub> C <sub>3</sub> + 0.5 H <sub>8</sub> C <sub>5</sub> + 2.389 N <sub>2</sub> → 0.9444 Th <sub>3</sub> N <sub>4</sub> + ThB <sub>6</sub> H <sub>4</sub> C <sub>6</sub> N       | -1.1463             |
| ThNH <sub>4</sub> B <sub>6</sub> C <sub>6</sub> | 0.25 Th <sub>3</sub> N <sub>4</sub> + 3 ThC <sub>2</sub> + 0.3636 B <sub>9</sub> H <sub>11</sub> + 19.23 B → 2.75 ThB <sub>6</sub> + ThB <sub>6</sub> H <sub>4</sub> C <sub>6</sub> N                                   | -1.1412             |
| ThNH <sub>4</sub> B <sub>6</sub> C <sub>6</sub> | 0.6667 B <sub>9</sub> H <sub>11</sub> + 2 Th <sub>2</sub> C <sub>3</sub> + 1.389 N <sub>2</sub> → 1.667 ThH <sub>2</sub> + 0.4444 Th <sub>3</sub> N <sub>4</sub> + ThB <sub>6</sub> H <sub>4</sub> C <sub>6</sub> N     | -1.1319             |
| ThNH <sub>4</sub> B <sub>6</sub> C <sub>6</sub> | 2.493 ThB <sub>4</sub> + 1.2 H <sub>8</sub> C <sub>5</sub> + 2.487 N <sub>2</sub> → 0.3733 Th <sub>4</sub> H <sub>15</sub> + 3.973 BN + ThB <sub>6</sub> H <sub>4</sub> C <sub>6</sub> N                                | -1.1305             |
| ThNH <sub>4</sub> B <sub>6</sub> C <sub>6</sub> | 1.2 B <sub>5</sub> H <sub>7</sub> + 6 C + 4.7 Th + H <sub>3</sub> N → 3.7 ThH <sub>2</sub> + ThB <sub>6</sub> H <sub>4</sub> C <sub>6</sub> N                                                                           | -1.1259             |
| ThNH <sub>4</sub> B <sub>6</sub> C <sub>6</sub> | 2.431 Th <sub>3</sub> N <sub>4</sub> + 1.636 B <sub>9</sub> H <sub>11</sub> + 1.2 H <sub>8</sub> C <sub>5</sub> → 1.573 Th <sub>4</sub> H <sub>15</sub> + 8.722 BN + ThB <sub>6</sub> H <sub>4</sub> C <sub>6</sub> N   | -1.1056             |
| ThNH <sub>4</sub> B <sub>6</sub> C <sub>6</sub> | 1.75 B <sub>13</sub> C <sub>2</sub> + 2.792 Th + 0.5 H <sub>8</sub> C <sub>5</sub> + ThN → 2.792 ThB <sub>6</sub> + ThB <sub>6</sub> H <sub>4</sub> C <sub>6</sub> N                                                    | -1.0927             |
| ThNH <sub>4</sub> B <sub>6</sub> C <sub>6</sub> | 3 ThC <sub>2</sub> + 6 B + 1.333 H <sub>3</sub> N + 1.167 N <sub>2</sub> → 0.6667 Th <sub>3</sub> N <sub>4</sub> + ThB <sub>6</sub> H <sub>4</sub> C <sub>6</sub> N                                                     | -1.0884             |
| ThNH <sub>4</sub> B <sub>6</sub> C <sub>6</sub> | 0.5714 B <sub>5</sub> H <sub>7</sub> + 3.415 ThC + 1.293 B <sub>13</sub> C <sub>2</sub> + ThN → 3.415 ThB <sub>4</sub> + ThB <sub>6</sub> H <sub>4</sub> C <sub>6</sub> N                                               | -1.0875             |
| ThNH <sub>4</sub> B <sub>6</sub> C <sub>6</sub> | 0.06667 Th <sub>4</sub> H <sub>15</sub> + 3 ThC <sub>2</sub> + 19.6 B + H <sub>3</sub> N → 2.267 ThB <sub>6</sub> + ThB <sub>6</sub> H <sub>4</sub> C <sub>6</sub> N                                                    | -1.0826             |
| ThNH <sub>4</sub> B <sub>6</sub> C <sub>6</sub> | 6 ThC + 6 B + 3.444 H <sub>3</sub> N → 3.167 ThH <sub>2</sub> + 0.6111 Th <sub>3</sub> N <sub>4</sub> + ThB <sub>6</sub> H <sub>4</sub> C <sub>6</sub> N                                                                | -1.0739             |

Continued on next page

Continued

| Compound                                        | Chemical reaction                                                                                                                                                                                                    | Reaction energy(eV) |
|-------------------------------------------------|----------------------------------------------------------------------------------------------------------------------------------------------------------------------------------------------------------------------|---------------------|
| ThNH <sub>4</sub> B <sub>6</sub> C <sub>6</sub> | 1.5 ThB <sub>4</sub> + 6 ThC + 4.759 H <sub>3</sub> N → 0.6852 Th <sub>4</sub> H <sub>15</sub> + 3.759 ThN + ThB <sub>6</sub> H <sub>4</sub> C <sub>6</sub> N                                                        | -1.0619             |
| ThNH <sub>4</sub> B <sub>6</sub> C <sub>6</sub> | 3.492 ThC + 1.254 B <sub>13</sub> C <sub>2</sub> + 1.333 H <sub>3</sub> N → 2.492 ThB <sub>4</sub> + 0.3333 BN + ThB <sub>6</sub> H <sub>4</sub> C <sub>6</sub> N                                                    | -1.0609             |
| ThNH <sub>4</sub> B <sub>6</sub> C <sub>6</sub> | 0.7857 ThB <sub>4</sub> + 0.5714 B <sub>5</sub> H <sub>7</sub> + 3 ThC <sub>2</sub> + 1.893 N <sub>2</sub> → 2.786 ThN + ThB <sub>6</sub> H <sub>4</sub> C <sub>6</sub> N                                            | -1.0517             |
| ThNH <sub>4</sub> B <sub>6</sub> C <sub>6</sub> | 0.5714 B <sub>5</sub> H <sub>7</sub> + BN + 2 Th <sub>2</sub> C <sub>3</sub> + 14.14 B → 3 ThB <sub>4</sub> + ThB <sub>6</sub> H <sub>4</sub> C <sub>6</sub> N                                                       | -1.0493             |
| ThNH <sub>4</sub> B <sub>6</sub> C <sub>6</sub> | 5.077 ThC + 0.4615 B <sub>13</sub> C <sub>2</sub> + 6.436 H <sub>3</sub> N → 1.359 Th <sub>3</sub> N <sub>4</sub> + 7.654 H <sub>2</sub> + ThB <sub>6</sub> H <sub>4</sub> C <sub>6</sub> N                          | -1.0476             |
| ThNH <sub>4</sub> B <sub>6</sub> C <sub>6</sub> | 1.2 B <sub>5</sub> H <sub>7</sub> + 7 Th + 1.2 H <sub>8</sub> C <sub>5</sub> + ThN → 7 ThH <sub>2</sub> + ThB <sub>6</sub> H <sub>4</sub> C <sub>6</sub> N                                                           | -1.0432             |
| ThNH <sub>4</sub> B <sub>6</sub> C <sub>6</sub> | 0.25 Th <sub>3</sub> N <sub>4</sub> + 0.2667 Th <sub>4</sub> H <sub>15</sub> + 2 Th <sub>2</sub> C <sub>3</sub> + 12.63 ThB <sub>6</sub> → 17.45 ThB <sub>4</sub> + ThB <sub>6</sub> H <sub>4</sub> C <sub>6</sub> N | -1.0304             |
| ThNH <sub>4</sub> B <sub>6</sub> C <sub>6</sub> | 2 ThH <sub>2</sub> + 3 ThC <sub>2</sub> + 13 ThB <sub>6</sub> + ThN → 18 ThB <sub>4</sub> + ThB <sub>6</sub> H <sub>4</sub> C <sub>6</sub> N                                                                         | -1.0303             |
| ThNH <sub>4</sub> B <sub>6</sub> C <sub>6</sub> | 0.2667 Th <sub>4</sub> H <sub>15</sub> + 2.538 ThC <sub>2</sub> + 0.4615 B <sub>13</sub> C <sub>2</sub> + 1.803 N <sub>2</sub> → 2.605 ThN + ThB <sub>6</sub> H <sub>4</sub> C <sub>6</sub> N                        | -1.0302             |
| ThNH <sub>4</sub> B <sub>6</sub> C <sub>6</sub> | 0.5 ThH <sub>2</sub> + 3 ThC <sub>2</sub> + 16 B + H <sub>3</sub> N → 2.5 ThB <sub>4</sub> + ThB <sub>6</sub> H <sub>4</sub> C <sub>6</sub> N                                                                        | -1.0169             |
| ThNH <sub>4</sub> B <sub>6</sub> C <sub>6</sub> | 0.5714 B <sub>5</sub> H <sub>7</sub> + 3 ThC <sub>2</sub> + 3.143 B + 1.5 N <sub>2</sub> → 2 ThN + ThB <sub>6</sub> H <sub>4</sub> C <sub>6</sub> N                                                                  | -1.0127             |
| ThNH <sub>4</sub> B <sub>6</sub> C <sub>6</sub> | 22.17 H <sub>2</sub> + 3 B <sub>13</sub> C <sub>2</sub> + Th + 0.5 N <sub>2</sub> → 3.667 B <sub>9</sub> H <sub>11</sub> + ThB <sub>6</sub> H <sub>4</sub> C <sub>6</sub> N                                          | -1.0084             |
| ThNH <sub>4</sub> B <sub>6</sub> C <sub>6</sub> | 0.25 Th <sub>3</sub> N <sub>4</sub> + 2 H <sub>2</sub> + 3 ThC <sub>2</sub> + 17 B → 2.75 ThB <sub>4</sub> + ThB <sub>6</sub> H <sub>4</sub> C <sub>6</sub> N                                                        | -1.0070             |
| ThNH <sub>4</sub> B <sub>6</sub> C <sub>6</sub> | 2.608 ThC + 0.2667 Th <sub>4</sub> H <sub>15</sub> + 1.696 B <sub>13</sub> C <sub>2</sub> + 0.5 N <sub>2</sub> → 2.675 ThB <sub>6</sub> + ThB <sub>6</sub> H <sub>4</sub> C <sub>6</sub> N                           | -0.9986             |
| ThNH <sub>4</sub> B <sub>6</sub> C <sub>6</sub> | 0.5 ThH <sub>2</sub> + 3.333 ThC + 1.333 B <sub>13</sub> C <sub>2</sub> + H <sub>3</sub> N → 2.833 ThB <sub>4</sub> + ThB <sub>6</sub> H <sub>4</sub> C <sub>6</sub> N                                               | -0.9902             |
| ThNH <sub>4</sub> B <sub>6</sub> C <sub>6</sub> | 2 H <sub>2</sub> + 2 Th <sub>2</sub> C <sub>3</sub> + 11 ThB <sub>6</sub> + ThN → 15 ThB <sub>4</sub> + ThB <sub>6</sub> H <sub>4</sub> C <sub>6</sub> N                                                             | -0.9888             |
| ThNH <sub>4</sub> B <sub>6</sub> C <sub>6</sub> | BN + 0.3636 B <sub>9</sub> H <sub>11</sub> + 2 Th <sub>2</sub> C <sub>3</sub> + 13.73 B → 3 ThB <sub>4</sub> + ThB <sub>6</sub> H <sub>4</sub> C <sub>6</sub> N                                                      | -0.9870             |
| ThNH <sub>4</sub> B <sub>6</sub> C <sub>6</sub> | 0.25 Th <sub>3</sub> N <sub>4</sub> + 3.55 ThC + 0.3636 B <sub>9</sub> H <sub>11</sub> + 1.225 B <sub>13</sub> C <sub>2</sub> → 3.3 ThB <sub>4</sub> + ThB <sub>6</sub> H <sub>4</sub> C <sub>6</sub> N              | -0.9846             |
| ThNH <sub>4</sub> B <sub>6</sub> C <sub>6</sub> | 0.6818 ThB <sub>4</sub> + 3 ThC <sub>2</sub> + 0.3636 B <sub>9</sub> H <sub>11</sub> + 1.841 N <sub>2</sub> → 2.682 ThN + ThB <sub>6</sub> H <sub>4</sub> C <sub>6</sub> N                                           | -0.9843             |
| ThNH <sub>4</sub> B <sub>6</sub> C <sub>6</sub> | 4.556 B <sub>5</sub> H <sub>7</sub> + 3 B <sub>13</sub> C <sub>2</sub> + 10.3 ThN → 9.296 H <sub>3</sub> N + 9.296 ThB <sub>6</sub> + ThB <sub>6</sub> H <sub>4</sub> C <sub>6</sub> N                               | -0.9818             |
| ThNH <sub>4</sub> B <sub>6</sub> C <sub>6</sub> | 6 ThC + 1.097 B <sub>9</sub> H <sub>11</sub> + 0.5 N <sub>2</sub> → 4.032 ThH <sub>2</sub> + 0.9677 ThB <sub>4</sub> + ThB <sub>6</sub> H <sub>4</sub> C <sub>6</sub> N                                              | -0.9769             |
| ThNH <sub>4</sub> B <sub>6</sub> C <sub>6</sub> | 2 H <sub>2</sub> + 2.538 ThC <sub>2</sub> + 0.4615 B <sub>13</sub> C <sub>2</sub> + 1.526 N <sub>2</sub> → 0.5128 Th <sub>3</sub> N <sub>4</sub> + ThB <sub>6</sub> H <sub>4</sub> C <sub>6</sub> N                  | -0.9670             |
| ThNH <sub>4</sub> B <sub>6</sub> C <sub>6</sub> | 3 ThC <sub>2</sub> + 0.3636 B <sub>9</sub> H <sub>11</sub> + 2.727 B + 1.5 N <sub>2</sub> → 2 ThN + ThB <sub>6</sub> H <sub>4</sub> C <sub>6</sub> N                                                                 | -0.9504             |
| ThNH <sub>4</sub> B <sub>6</sub> C <sub>6</sub> | 0.5714 B <sub>5</sub> H <sub>7</sub> + 0.25 Th <sub>3</sub> N <sub>4</sub> + 3.51 ThC + 1.245 B <sub>13</sub> C <sub>2</sub> → 3.26 ThB <sub>4</sub> + ThB <sub>6</sub> H <sub>4</sub> C <sub>6</sub> N              | -0.9255             |
| ThNH <sub>4</sub> B <sub>6</sub> C <sub>6</sub> | 5.077 ThC + 0.4615 B <sub>13</sub> C <sub>2</sub> + 3.413 H <sub>3</sub> N → 0.416 Th <sub>4</sub> H <sub>15</sub> + 2.413 ThN + ThB <sub>6</sub> H <sub>4</sub> C <sub>6</sub> N                                    | -0.9231             |
| ThNH <sub>4</sub> B <sub>6</sub> C <sub>6</sub> | 2 ThH <sub>2</sub> + 1.714 B <sub>13</sub> C <sub>2</sub> + 0.8571 Th <sub>2</sub> C <sub>3</sub> + 0.5 N <sub>2</sub> → 2.714 ThB <sub>6</sub> + ThB <sub>6</sub> H <sub>4</sub> C <sub>6</sub> N                   | -0.9168             |
| ThNH <sub>4</sub> B <sub>6</sub> C <sub>6</sub> | 0.5714 B <sub>5</sub> H <sub>7</sub> + 3 ThC <sub>2</sub> + 11.14 B + 0.5 N <sub>2</sub> → 2 ThB <sub>4</sub> + ThB <sub>6</sub> H <sub>4</sub> C <sub>6</sub> N                                                     | -0.9135             |
| ThNH <sub>4</sub> B <sub>6</sub> C <sub>6</sub> | 5.231 ThC + 9.933 H <sub>2</sub> + BN + 0.3846 B <sub>13</sub> C <sub>2</sub> → 1.058 Th <sub>4</sub> H <sub>15</sub> + ThB <sub>6</sub> H <sub>4</sub> C <sub>6</sub> N                                             | -0.9001             |
| ThNH <sub>4</sub> B <sub>6</sub> C <sub>6</sub> | 0.5714 B <sub>5</sub> H <sub>7</sub> + 3 ThC <sub>2</sub> + 1.762 N <sub>2</sub> + 0.5238 ThB <sub>6</sub> → 2.524 ThN + ThB <sub>6</sub> H <sub>4</sub> C <sub>6</sub> N                                            | -0.8875             |
| ThNH <sub>4</sub> B <sub>6</sub> C <sub>6</sub> | 6 ThC + 6 B + 3.2 H <sub>3</sub> N → 2.8 ThH <sub>2</sub> + 2.2 ThN + ThB <sub>6</sub> H <sub>4</sub> C <sub>6</sub> N                                                                                               | -0.8843             |
| ThNH <sub>4</sub> B <sub>6</sub> C <sub>6</sub> | 0.5714 B <sub>5</sub> H <sub>7</sub> + 3 ThC <sub>2</sub> + 15.14 B + ThN → 3 ThB <sub>4</sub> + ThB <sub>6</sub> H <sub>4</sub> C <sub>6</sub> N                                                                    | -0.8639             |
| ThNH <sub>4</sub> B <sub>6</sub> C <sub>6</sub> | 2.821 B <sub>5</sub> H <sub>7</sub> + 6 ThC + H <sub>3</sub> N → 1.25 Th <sub>4</sub> H <sub>15</sub> + 8.107 B + ThB <sub>6</sub> H <sub>4</sub> C <sub>6</sub> N                                                   | -0.8559             |
| ThNH <sub>4</sub> B <sub>6</sub> C <sub>6</sub> | 3 ThC <sub>2</sub> + 0.3636 B <sub>9</sub> H <sub>11</sub> + 10.73 B + 0.5 N <sub>2</sub> → 2 ThB <sub>4</sub> + ThB <sub>6</sub> H <sub>4</sub> C <sub>6</sub> N                                                    | -0.8512             |
| ThNH <sub>4</sub> B <sub>6</sub> C <sub>6</sub> | 18.72 B <sub>5</sub> H <sub>7</sub> + 6 ThC + BN → 1.25 Th <sub>4</sub> H <sub>15</sub> + 9.844 B <sub>9</sub> H <sub>11</sub> + ThB <sub>6</sub> H <sub>4</sub> C <sub>6</sub> N                                    | -0.8510             |
| ThNH <sub>4</sub> B <sub>6</sub> C <sub>6</sub> | 3.143 ThC + 2 H <sub>2</sub> + 1.429 B <sub>13</sub> C <sub>2</sub> + ThN → 3.143 ThB <sub>4</sub> + ThB <sub>6</sub> H <sub>4</sub> C <sub>6</sub> N                                                                | -0.8502             |
| ThNH <sub>4</sub> B <sub>6</sub> C <sub>6</sub> | 3 ThC <sub>2</sub> + 0.3636 B <sub>9</sub> H <sub>11</sub> + 1.727 N <sub>2</sub> + 0.4545 ThB <sub>6</sub> → 2.455 ThN + ThB <sub>6</sub> H <sub>4</sub> C <sub>6</sub> N                                           | -0.8418             |
| ThNH <sub>4</sub> B <sub>6</sub> C <sub>6</sub> | 0.5 ThH <sub>2</sub> + 2 Th <sub>2</sub> C <sub>3</sub> + H <sub>3</sub> N + 10 ThB <sub>6</sub> → 13.5 ThB <sub>4</sub> + ThB <sub>6</sub> H <sub>4</sub> C <sub>6</sub> N                                          | -0.8333             |
| ThNH <sub>4</sub> B <sub>6</sub> C <sub>6</sub> | B <sub>5</sub> H <sub>7</sub> + BN + 7.3 Th + 1.2 H <sub>8</sub> C <sub>5</sub> → 6.3 ThH <sub>2</sub> + ThB <sub>6</sub> H <sub>4</sub> C <sub>6</sub> N                                                            | -0.8269             |
| ThNH <sub>4</sub> B <sub>6</sub> C <sub>6</sub> | 3.602 ThC + 0.09091 B <sub>9</sub> H <sub>11</sub> + 1.199 B <sub>13</sub> C <sub>2</sub> + H <sub>3</sub> N → 2.602 ThB <sub>4</sub> + ThB <sub>6</sub> H <sub>4</sub> C <sub>6</sub> N                             | -0.8181             |
| ThNH <sub>4</sub> B <sub>6</sub> C <sub>6</sub> | 6 ThC + 15.97 H <sub>3</sub> N + 6.227 ThB <sub>6</sub> → 6.273 B <sub>5</sub> H <sub>7</sub> + 3.742 Th <sub>3</sub> N <sub>4</sub> + ThB <sub>6</sub> H <sub>4</sub> C <sub>6</sub> N                              | -0.8151             |
| ThNH <sub>4</sub> B <sub>6</sub> C <sub>6</sub> | 2 Th <sub>2</sub> C <sub>3</sub> + 8.333 B + 3.333 H <sub>3</sub> N → 3 ThH <sub>2</sub> + 2.333 BN + ThB <sub>6</sub> H <sub>4</sub> C <sub>6</sub> N                                                               | -0.8067             |
| ThNH <sub>4</sub> B <sub>6</sub> C <sub>6</sub> | 0.5714 B <sub>5</sub> H <sub>7</sub> + 2 Th <sub>2</sub> C <sub>3</sub> + 9.571 ThB <sub>6</sub> + ThN → 13.57 ThB <sub>4</sub> + ThB <sub>6</sub> H <sub>4</sub> C <sub>6</sub> N                                   | -0.8039             |
| ThNH <sub>4</sub> B <sub>6</sub> C <sub>6</sub> | 0.1429 B <sub>5</sub> H <sub>7</sub> + 3.592 ThC + 1.204 B <sub>13</sub> C <sub>2</sub> + H <sub>3</sub> N → 2.592 ThB <sub>4</sub> + ThB <sub>6</sub> H <sub>4</sub> C <sub>6</sub> N                               | -0.8033             |
| ThNH <sub>4</sub> B <sub>6</sub> C <sub>6</sub> | 0.3636 B <sub>9</sub> H <sub>11</sub> + 2 Th <sub>2</sub> C <sub>3</sub> + 9.364 ThB <sub>6</sub> + ThN → 13.36 ThB <sub>4</sub> + ThB <sub>6</sub> H <sub>4</sub> C <sub>6</sub> N                                  | -0.8016             |
| ThNH <sub>4</sub> B <sub>6</sub> C <sub>6</sub> | 3 ThC <sub>2</sub> + 0.3636 B <sub>9</sub> H <sub>11</sub> + 14.73 B + ThN → 3 ThB <sub>4</sub> + ThB <sub>6</sub> H <sub>4</sub> C <sub>6</sub> N                                                                   | -0.8016             |
| ThNH <sub>4</sub> B <sub>6</sub> C <sub>6</sub> | 0.2667 Th <sub>4</sub> H <sub>15</sub> + BN + 3 ThC <sub>2</sub> + 23.4 B → 3.067 ThB <sub>6</sub> + ThB <sub>6</sub> H <sub>4</sub> C <sub>6</sub> N                                                                | -0.7962             |
| ThNH <sub>4</sub> B <sub>6</sub> C <sub>6</sub> | 2 ThH <sub>2</sub> + 2.857 ThC + BN + 1.571 B <sub>13</sub> C <sub>2</sub> → 3.857 ThB <sub>4</sub> + ThB <sub>6</sub> H <sub>4</sub> C <sub>6</sub> N                                                               | -0.7781             |
| ThNH <sub>4</sub> B <sub>6</sub> C <sub>6</sub> | 5.769 ThH <sub>2</sub> + BN + 3 B <sub>13</sub> C <sub>2</sub> → 1.077 B <sub>5</sub> H <sub>7</sub> + 4.769 ThB <sub>6</sub> + ThB <sub>6</sub> H <sub>4</sub> C <sub>6</sub> N                                     | -0.7771             |
| ThNH <sub>4</sub> B <sub>6</sub> C <sub>6</sub> | 0.5 H <sub>2</sub> + 3 ThC <sub>2</sub> + 18 B + H <sub>3</sub> N → 2 ThB <sub>6</sub> + ThB <sub>6</sub> H <sub>4</sub> C <sub>6</sub> N                                                                            | -0.7638             |
| ThNH <sub>4</sub> B <sub>6</sub> C <sub>6</sub> | 3.619 ThC + 1.19 B <sub>13</sub> C <sub>2</sub> + 1.333 H <sub>3</sub> N → 2.369 ThB <sub>4</sub> + 0.08333 Th <sub>3</sub> N <sub>4</sub> + ThB <sub>6</sub> H <sub>4</sub> C <sub>6</sub> N                        | -0.7626             |
| ThNH <sub>4</sub> B <sub>6</sub> C <sub>6</sub> | 6 ThC + 0.6667 B <sub>9</sub> H <sub>11</sub> + 6 H <sub>3</sub> N → 10.67 H <sub>2</sub> + 5 ThN + ThB <sub>6</sub> H <sub>4</sub> C <sub>6</sub> N                                                                 | -0.7567             |
| ThNH <sub>4</sub> B <sub>6</sub> C <sub>6</sub> | 2 ThH <sub>2</sub> + 1.68 ThC + 2.16 B <sub>13</sub> C <sub>2</sub> + ThN → 3.68 ThB <sub>6</sub> + ThB <sub>6</sub> H <sub>4</sub> C <sub>6</sub> N                                                                 | -0.7473             |
| ThNH <sub>4</sub> B <sub>6</sub> C <sub>6</sub> | 3.524 ThC + 0.5 H <sub>2</sub> + 1.238 B <sub>13</sub> C <sub>2</sub> + H <sub>3</sub> N → 2.524 ThB <sub>4</sub> + ThB <sub>6</sub> H <sub>4</sub> C <sub>6</sub> N                                                 | -0.7440             |
| ThNH <sub>4</sub> B <sub>6</sub> C <sub>6</sub> | 2 ThH <sub>2</sub> + 0.25 Th <sub>3</sub> N <sub>4</sub> + 3 ThC <sub>2</sub> + 12.5 ThB <sub>6</sub> → 17.25 ThB <sub>4</sub> + ThB <sub>6</sub> H <sub>4</sub> C <sub>6</sub> N                                    | -0.7205             |
| ThNH <sub>4</sub> B <sub>6</sub> C <sub>6</sub> | 1.789 B <sub>5</sub> H <sub>7</sub> + 6 ThC + 0.5 N <sub>2</sub> → 4.263 ThH <sub>2</sub> + 0.7368 ThB <sub>4</sub> + ThB <sub>6</sub> H <sub>4</sub> C <sub>6</sub> N                                               | -0.7124             |
| ThNH <sub>4</sub> B <sub>6</sub> C <sub>6</sub> | 1.2 B <sub>5</sub> H <sub>7</sub> + 6 ThC + 6 H <sub>3</sub> N → 11.2 H <sub>2</sub> + 5 ThN + ThB <sub>6</sub> H <sub>4</sub> C <sub>6</sub> N                                                                      | -0.7117             |
| ThNH <sub>4</sub> B <sub>6</sub> C <sub>6</sub> | 3.651 ThC + 1.175 B <sub>13</sub> C <sub>2</sub> + 1.333 H <sub>3</sub> N → 2.317 ThB <sub>4</sub> + 0.3333 ThN + ThB <sub>6</sub> H <sub>4</sub> C <sub>6</sub> N                                                   | -0.7086             |
| ThNH <sub>4</sub> B <sub>6</sub> C <sub>6</sub> | 16.75 B <sub>9</sub> H <sub>11</sub> + 2 Th <sub>2</sub> C <sub>3</sub> + ThN → 4 ThB <sub>4</sub> + 25.75 B <sub>5</sub> H <sub>7</sub> + ThB <sub>6</sub> H <sub>4</sub> C <sub>6</sub> N                          | -0.6982             |
| ThNH <sub>4</sub> B <sub>6</sub> C <sub>6</sub> | 0.25 Th <sub>3</sub> N <sub>4</sub> + 3.238 ThC + 2 H <sub>2</sub> + 1.381 B <sub>13</sub> C <sub>2</sub> → 2.988 ThB <sub>4</sub> + ThB <sub>6</sub> H <sub>4</sub> C <sub>6</sub> N                                | -0.6882             |
| ThNH <sub>4</sub> B <sub>6</sub> C <sub>6</sub> | 0.25 Th <sub>3</sub> N <sub>4</sub> + 2 H <sub>2</sub> + 2 Th <sub>2</sub> C <sub>3</sub> + 10.5 ThB <sub>6</sub> → 14.25 ThB <sub>4</sub> + ThB <sub>6</sub> H <sub>4</sub> C <sub>6</sub> N                        | -0.6790             |

Continued on next page

Continued

| Compound                                        | Chemical reaction                                                                                                                                                                                                                   | Reaction energy(eV) |
|-------------------------------------------------|-------------------------------------------------------------------------------------------------------------------------------------------------------------------------------------------------------------------------------------|---------------------|
| ThNH <sub>4</sub> B <sub>6</sub> C <sub>6</sub> | 6 ThC + 1.143 B <sub>9</sub> H <sub>11</sub> + 0.5 N <sub>2</sub> → 4.286 ThH <sub>2</sub> + 0.7143 ThB <sub>6</sub> + ThB <sub>6</sub> H <sub>4</sub> C <sub>6</sub> N                                                             | -0.6786             |
| ThNH <sub>4</sub> B <sub>6</sub> C <sub>6</sub> | 3.422 ThC + 0.06667 Th <sub>4</sub> H <sub>15</sub> + 1.289 B <sub>13</sub> C <sub>2</sub> + H <sub>3</sub> N → 2.689 ThB <sub>4</sub> + ThB <sub>6</sub> H <sub>4</sub> C <sub>6</sub> N                                           | -0.6742             |
| ThNH <sub>4</sub> B <sub>6</sub> C <sub>6</sub> | 1.429 B <sub>5</sub> H <sub>7</sub> + 2 Th <sub>2</sub> C <sub>3</sub> + 1.071 N <sub>2</sub> → 3 ThH <sub>2</sub> + 1.143 BN + ThB <sub>6</sub> H <sub>4</sub> C <sub>6</sub> N                                                    | -0.6717             |
| ThNH <sub>4</sub> B <sub>6</sub> C <sub>6</sub> | 5.667 ThH <sub>2</sub> + BN + 3 B <sub>13</sub> C <sub>2</sub> → 0.6667 B <sub>9</sub> H <sub>11</sub> + 4.667 ThB <sub>6</sub> + ThB <sub>6</sub> H <sub>4</sub> C <sub>6</sub> N                                                  | -0.6607             |
| ThNH <sub>4</sub> B <sub>6</sub> C <sub>6</sub> | 2 Th <sub>2</sub> C <sub>3</sub> + 1.333 H <sub>3</sub> N + 9.167 ThB <sub>6</sub> → 12.17 ThB <sub>4</sub> + 0.3333 BN + ThB <sub>6</sub> H <sub>4</sub> C <sub>6</sub> N                                                          | -0.6577             |
| ThNH <sub>4</sub> B <sub>6</sub> C <sub>6</sub> | 23.75 B <sub>9</sub> H <sub>11</sub> + 2 Th <sub>2</sub> C <sub>3</sub> + ThN → 36.75 B <sub>5</sub> H <sub>7</sub> + 4 ThB <sub>6</sub> + ThB <sub>6</sub> H <sub>4</sub> C <sub>6</sub> N                                         | -0.6540             |
| ThNH <sub>4</sub> B <sub>6</sub> C <sub>6</sub> | 2.577 ThC + 0.4615 B <sub>13</sub> C <sub>2</sub> + 0.5 H <sub>8</sub> C <sub>5</sub> + 1.551 N <sub>2</sub> → 0.5256 Th <sub>3</sub> N <sub>4</sub> + ThB <sub>6</sub> H <sub>4</sub> C <sub>6</sub> N                             | -0.6502             |
| ThNH <sub>4</sub> B <sub>6</sub> C <sub>6</sub> | 0.25 Th <sub>3</sub> N <sub>4</sub> + 0.6667 B <sub>9</sub> H <sub>11</sub> + 6.717 Th + 1.2 H <sub>8</sub> C <sub>5</sub> → 6.467 ThH <sub>2</sub> + ThB <sub>6</sub> H <sub>4</sub> C <sub>6</sub> N                              | -0.6422             |
| ThNH <sub>4</sub> B <sub>6</sub> C <sub>6</sub> | 1.717 B <sub>9</sub> H <sub>11</sub> + 2.485 Th <sub>2</sub> C <sub>3</sub> + 0.5 N <sub>2</sub> → 0.9923 Th <sub>4</sub> H <sub>15</sub> + 0.727 B <sub>13</sub> C <sub>2</sub> + ThB <sub>6</sub> H <sub>4</sub> C <sub>6</sub> N | -0.6396             |
| ThNH <sub>4</sub> B <sub>6</sub> C <sub>6</sub> | 2 ThH <sub>2</sub> + 0.25 Th <sub>3</sub> N <sub>4</sub> + 1.8 ThC + 2.1 B <sub>13</sub> C <sub>2</sub> → 3.55 ThB <sub>6</sub> + ThB <sub>6</sub> H <sub>4</sub> C <sub>6</sub> N                                                  | -0.6237             |
| ThNH <sub>4</sub> B <sub>6</sub> C <sub>6</sub> | 0.1429 B <sub>5</sub> H <sub>7</sub> + 3 ThC <sub>2</sub> + 17.29 B + H <sub>3</sub> N → 2 ThB <sub>6</sub> + ThB <sub>6</sub> H <sub>4</sub> C <sub>6</sub> N                                                                      | -0.6145             |
| ThNH <sub>4</sub> B <sub>6</sub> C <sub>6</sub> | 3 ThC <sub>2</sub> + 14.33 B + 1.333 H <sub>3</sub> N → 2 ThB <sub>4</sub> + 0.3333 BN + ThB <sub>6</sub> H <sub>4</sub> C <sub>6</sub> N                                                                                           | -0.6008             |
| ThNH <sub>4</sub> B <sub>6</sub> C <sub>6</sub> | 3 ThC <sub>2</sub> + 0.09091 B <sub>9</sub> H <sub>11</sub> + 17.18 B + H <sub>3</sub> N → 2 ThB <sub>6</sub> + ThB <sub>6</sub> H <sub>4</sub> C <sub>6</sub> N                                                                    | -0.5990             |
| ThNH <sub>4</sub> B <sub>6</sub> C <sub>6</sub> | 2 B <sub>9</sub> H <sub>11</sub> + 2 Th <sub>2</sub> C <sub>3</sub> + 0.5 N <sub>2</sub> → 3 ThB <sub>4</sub> + 9 H <sub>2</sub> + ThB <sub>6</sub> H <sub>4</sub> C <sub>6</sub> N                                                 | -0.5863             |
| ThNH <sub>4</sub> B <sub>6</sub> C <sub>6</sub> | 3.5 ThC + BN + 20 B + 0.5 H <sub>8</sub> C <sub>5</sub> → 2.5 ThB <sub>6</sub> + ThB <sub>6</sub> H <sub>4</sub> C <sub>6</sub> N                                                                                                   | -0.5768             |
| ThNH <sub>4</sub> B <sub>6</sub> C <sub>6</sub> | 0.4615 B <sub>13</sub> C <sub>2</sub> + 1.692 Th <sub>2</sub> C <sub>3</sub> + 1.333 H <sub>3</sub> N + 1.026 N <sub>2</sub> → 2.385 ThN + ThB <sub>6</sub> H <sub>4</sub> C <sub>6</sub> N                                         | -0.5735             |
| ThNH <sub>4</sub> B <sub>6</sub> C <sub>6</sub> | 2.737 ThC + 0.2667 Th <sub>4</sub> H <sub>15</sub> + 1.632 B <sub>13</sub> C <sub>2</sub> + ThN → 3.803 ThB <sub>4</sub> + ThB <sub>6</sub> H <sub>4</sub> C <sub>6</sub> N                                                         | -0.5711             |
| ThNH <sub>4</sub> B <sub>6</sub> C <sub>6</sub> | 6 ThC + 1.795 B <sub>9</sub> H <sub>11</sub> + H <sub>3</sub> N → 1.25 Th <sub>4</sub> H <sub>15</sub> + 10.16 B + ThB <sub>6</sub> H <sub>4</sub> C <sub>6</sub> N                                                                 | -0.5485             |
| ThNH <sub>4</sub> B <sub>6</sub> C <sub>6</sub> | 3 ThC <sub>2</sub> + 2.75 B <sub>9</sub> H <sub>11</sub> + 1.5 N <sub>2</sub> → 3.75 B <sub>5</sub> H <sub>7</sub> + 2 ThN + ThB <sub>6</sub> H <sub>4</sub> C <sub>6</sub> N                                                       | -0.5418             |
| ThNH <sub>4</sub> B <sub>6</sub> C <sub>6</sub> | 9.5 H <sub>2</sub> + 2 Th <sub>2</sub> C <sub>3</sub> + 6 B + ThN → Th <sub>4</sub> H <sub>15</sub> + ThB <sub>6</sub> H <sub>4</sub> C <sub>6</sub> N                                                                              | -0.5367             |
| ThNH <sub>4</sub> B <sub>6</sub> C <sub>6</sub> | 1.167 Th <sub>2</sub> C <sub>3</sub> + 0.5 H <sub>8</sub> C <sub>5</sub> + 2.056 N <sub>2</sub> + ThB <sub>6</sub> → 0.7778 Th <sub>3</sub> N <sub>4</sub> + ThB <sub>6</sub> H <sub>4</sub> C <sub>6</sub> N                       | -0.5219             |
| ThNH <sub>4</sub> B <sub>6</sub> C <sub>6</sub> | 0.5714 B <sub>5</sub> H <sub>7</sub> + 0.25 Th <sub>3</sub> N <sub>4</sub> + 2 Th <sub>2</sub> C <sub>3</sub> + 9.071 ThB <sub>6</sub> → 12.82 ThB <sub>4</sub> + ThB <sub>6</sub> H <sub>4</sub> C <sub>6</sub> N                  | -0.4941             |
| ThNH <sub>4</sub> B <sub>6</sub> C <sub>6</sub> | 0.25 Th <sub>3</sub> N <sub>4</sub> + 0.3636 B <sub>9</sub> H <sub>11</sub> + 2 Th <sub>2</sub> C <sub>3</sub> + 8.864 ThB <sub>6</sub> → 12.61 ThB <sub>4</sub> + ThB <sub>6</sub> H <sub>4</sub> C <sub>6</sub> N                 | -0.4918             |
| ThNH <sub>4</sub> B <sub>6</sub> C <sub>6</sub> | 1.846 B <sub>5</sub> H <sub>7</sub> + 6 ThC + 0.5 N <sub>2</sub> → 4.462 ThH <sub>2</sub> + 0.5385 ThB <sub>6</sub> + ThB <sub>6</sub> H <sub>4</sub> C <sub>6</sub> N                                                              | -0.4791             |
| ThNH <sub>4</sub> B <sub>6</sub> C <sub>6</sub> | 3.6 B <sub>5</sub> H <sub>7</sub> + 2 Th <sub>2</sub> C <sub>3</sub> + 0.5 N <sub>2</sub> → 3 ThB <sub>4</sub> + 10.6 H <sub>2</sub> + ThB <sub>6</sub> H <sub>4</sub> C <sub>6</sub> N                                             | -0.4511             |
| ThNH <sub>4</sub> B <sub>6</sub> C <sub>6</sub> | 3.093 ThC + 1.453 B <sub>13</sub> C <sub>2</sub> + 1.333 H <sub>3</sub> N → 0.3333 BN + 2.093 ThB <sub>6</sub> + ThB <sub>6</sub> H <sub>4</sub> C <sub>6</sub> N                                                                   | -0.4422             |
| ThNH <sub>4</sub> B <sub>6</sub> C <sub>6</sub> | 2.549 B <sub>5</sub> H <sub>7</sub> + 2.346 Th <sub>2</sub> C <sub>3</sub> + 0.5 N <sub>2</sub> → 0.923 Th <sub>4</sub> H <sub>15</sub> + 0.5189 B <sub>13</sub> C <sub>2</sub> + ThB <sub>6</sub> H <sub>4</sub> C <sub>6</sub> N  | -0.4421             |
| ThNH <sub>4</sub> B <sub>6</sub> C <sub>6</sub> | 1.2 B <sub>5</sub> H <sub>7</sub> + 8.75 Th <sub>3</sub> N <sub>4</sub> + 8.75 ThC → 0.55 H <sub>8</sub> C <sub>5</sub> + 34 ThN + ThB <sub>6</sub> H <sub>4</sub> C <sub>6</sub> N                                                 | -0.4295             |
| ThNH <sub>4</sub> B <sub>6</sub> C <sub>6</sub> | 0.06667 Th <sub>4</sub> H <sub>15</sub> + 3 ThC <sub>2</sub> + 15.07 B + H <sub>3</sub> N → 2.267 ThB <sub>4</sub> + ThB <sub>6</sub> H <sub>4</sub> C <sub>6</sub> N                                                               | -0.4284             |
| ThNH <sub>4</sub> B <sub>6</sub> C <sub>6</sub> | 2 ThH <sub>2</sub> + 1.636 B <sub>13</sub> C <sub>2</sub> + 0.9091 Th <sub>2</sub> C <sub>3</sub> + ThN → 3.818 ThB <sub>4</sub> + ThB <sub>6</sub> H <sub>4</sub> C <sub>6</sub> N                                                 | -0.4202             |
| ThNH <sub>4</sub> B <sub>6</sub> C <sub>6</sub> | 3 ThC <sub>2</sub> + 16.5 B + 1.333 H <sub>3</sub> N → 0.08333 Th <sub>3</sub> N <sub>4</sub> + 1.75 ThB <sub>6</sub> + ThB <sub>6</sub> H <sub>4</sub> C <sub>6</sub> N                                                            | -0.4182             |
| ThNH <sub>4</sub> B <sub>6</sub> C <sub>6</sub> | 6 BN + 4.188 Th <sub>2</sub> C <sub>3</sub> + 4.833 H <sub>3</sub> N → 2.458 Th <sub>3</sub> N <sub>4</sub> + 1.313 H <sub>8</sub> C <sub>5</sub> + ThB <sub>6</sub> H <sub>4</sub> C <sub>6</sub> N                                | -0.4114             |
| ThNH <sub>4</sub> B <sub>6</sub> C <sub>6</sub> | 2 ThH <sub>2</sub> + 1.706 ThC <sub>2</sub> + 1.294 B <sub>13</sub> C <sub>2</sub> + 0.5 N <sub>2</sub> → 2.706 ThB <sub>4</sub> + ThB <sub>6</sub> H <sub>4</sub> C <sub>6</sub> N                                                 | -0.4107             |
| ThNH <sub>4</sub> B <sub>6</sub> C <sub>6</sub> | 0.5714 B <sub>5</sub> H <sub>7</sub> + 0.25 Th <sub>3</sub> N <sub>4</sub> + 3 ThC <sub>2</sub> + 14.14 B → 2.75 ThB <sub>4</sub> + ThB <sub>6</sub> H <sub>4</sub> C <sub>6</sub> N                                                | -0.4098             |
| ThNH <sub>4</sub> B <sub>6</sub> C <sub>6</sub> | 0.25 Th <sub>3</sub> N <sub>4</sub> + 2.832 ThC + 0.2667 Th <sub>4</sub> H <sub>15</sub> + 1.584 B <sub>13</sub> C <sub>2</sub> → 3.648 ThB <sub>4</sub> + ThB <sub>6</sub> H <sub>4</sub> C <sub>6</sub> N                         | -0.4091             |
| ThNH <sub>4</sub> B <sub>6</sub> C <sub>6</sub> | 6 C + 0.6667 B <sub>9</sub> H <sub>11</sub> + 4.167 Th + H <sub>3</sub> N → 3.167 ThH <sub>2</sub> + ThB <sub>6</sub> H <sub>4</sub> C <sub>6</sub> N                                                                               | -0.4045             |
| ThNH <sub>4</sub> B <sub>6</sub> C <sub>6</sub> | 6 ThC + 7 H <sub>3</sub> N + ThB <sub>6</sub> → 8.5 H <sub>2</sub> + 6 ThN + ThB <sub>6</sub> H <sub>4</sub> C <sub>6</sub> N                                                                                                       | -0.4026             |
| ThNH <sub>4</sub> B <sub>6</sub> C <sub>6</sub> | 3 ThC <sub>2</sub> + 0.6667 B <sub>9</sub> H <sub>11</sub> + 1.5 N <sub>2</sub> → 1.667 H <sub>2</sub> + 2 ThN + ThB <sub>6</sub> H <sub>4</sub> C <sub>6</sub> N                                                                   | -0.4009             |
| ThNH <sub>4</sub> B <sub>6</sub> C <sub>6</sub> | 0.25 Th <sub>3</sub> N <sub>4</sub> + 15.87 B <sub>9</sub> H <sub>11</sub> + 2 Th <sub>2</sub> C <sub>3</sub> → 3.75 ThB <sub>4</sub> + 24.37 B <sub>5</sub> H <sub>7</sub> + ThB <sub>6</sub> H <sub>4</sub> C <sub>6</sub> N      | -0.3939             |
| ThNH <sub>4</sub> B <sub>6</sub> C <sub>6</sub> | 2 Th <sub>2</sub> C <sub>3</sub> + 12.55 B + 4 H <sub>3</sub> N → 0.7273 B <sub>9</sub> H <sub>11</sub> + 3 ThN + ThB <sub>6</sub> H <sub>4</sub> C <sub>6</sub> N                                                                  | -0.3846             |
| ThNH <sub>4</sub> B <sub>6</sub> C <sub>6</sub> | 0.06667 Th <sub>4</sub> H <sub>15</sub> + 2 Th <sub>2</sub> C <sub>3</sub> + H <sub>3</sub> N + 9.533 ThB <sub>6</sub> → 12.8 ThB <sub>4</sub> + ThB <sub>6</sub> H <sub>4</sub> C <sub>6</sub> N                                   | -0.3794             |
| ThNH <sub>4</sub> B <sub>6</sub> C <sub>6</sub> | 1.074 B <sub>9</sub> H <sub>11</sub> + 2 Th <sub>2</sub> C <sub>3</sub> + 0.5 N <sub>2</sub> → 0.9164 ThB <sub>4</sub> + 0.5209 Th <sub>4</sub> H <sub>15</sub> + ThB <sub>6</sub> H <sub>4</sub> C <sub>6</sub> N                  | -0.3764             |
| ThNH <sub>4</sub> B <sub>6</sub> C <sub>6</sub> | 1.2 B <sub>5</sub> H <sub>7</sub> + 3 ThC <sub>2</sub> + 1.5 N <sub>2</sub> → 2.2 H <sub>2</sub> + 2 ThN + ThB <sub>6</sub> H <sub>4</sub> C <sub>6</sub> N                                                                         | -0.3558             |
| ThNH <sub>4</sub> B <sub>6</sub> C <sub>6</sub> | 0.25 Th <sub>3</sub> N <sub>4</sub> + 22.44 B <sub>9</sub> H <sub>11</sub> + 2 Th <sub>2</sub> C <sub>3</sub> → 34.69 B <sub>5</sub> H <sub>7</sub> + 3.75 ThB <sub>6</sub> + ThB <sub>6</sub> H <sub>4</sub> C <sub>6</sub> N      | -0.3525             |
| ThNH <sub>4</sub> B <sub>6</sub> C <sub>6</sub> | 0.25 Th <sub>3</sub> N <sub>4</sub> + 3 ThC <sub>2</sub> + 0.3636 B <sub>9</sub> H <sub>11</sub> + 13.73 B → 2.75 ThB <sub>4</sub> + ThB <sub>6</sub> H <sub>4</sub> C <sub>6</sub> N                                               | -0.3475             |
| ThNH <sub>4</sub> B <sub>6</sub> C <sub>6</sub> | 1.359 Th <sub>3</sub> N <sub>4</sub> + 1.75 B <sub>13</sub> C <sub>2</sub> + 0.5 H <sub>8</sub> C <sub>5</sub> → 3.078 ThB <sub>4</sub> + 4.438 BN + ThB <sub>6</sub> H <sub>4</sub> C <sub>6</sub> N                               | -0.3393             |
| ThNH <sub>4</sub> B <sub>6</sub> C <sub>6</sub> | 3.908 ThC + 1.046 B <sub>13</sub> C <sub>2</sub> + 4.878 H <sub>3</sub> N → 1.519 B <sub>5</sub> H <sub>7</sub> + 0.9695 Th <sub>3</sub> N <sub>4</sub> + ThB <sub>6</sub> H <sub>4</sub> C <sub>6</sub> N                          | -0.3296             |
| ThNH <sub>4</sub> B <sub>6</sub> C <sub>6</sub> | 3 ThC <sub>2</sub> + 18 B + 1.333 H <sub>3</sub> N → 0.1667 N <sub>2</sub> + 2 ThB <sub>6</sub> + ThB <sub>6</sub> H <sub>4</sub> C <sub>6</sub> N                                                                                  | -0.3225             |
| ThNH <sub>4</sub> B <sub>6</sub> C <sub>6</sub> | 0.6667 B <sub>9</sub> H <sub>11</sub> + 6.467 Th + 1.2 H <sub>8</sub> C <sub>5</sub> + ThN → 6.467 ThH <sub>2</sub> + ThB <sub>6</sub> H <sub>4</sub> C <sub>6</sub> N                                                              | -0.3218             |
| ThNH <sub>4</sub> B <sub>6</sub> C <sub>6</sub> | 5.077 ThC + 0.4615 B <sub>13</sub> C <sub>2</sub> + 5.077 H <sub>3</sub> N → 5.615 H <sub>2</sub> + 4.077 ThN + ThB <sub>6</sub> H <sub>4</sub> C <sub>6</sub> N                                                                    | -0.3112             |
| ThNH <sub>4</sub> B <sub>6</sub> C <sub>6</sub> | 0.25 Th <sub>3</sub> N <sub>4</sub> + 9.031 H <sub>2</sub> + 2 Th <sub>2</sub> C <sub>3</sub> + 6 B → 0.9375 Th <sub>4</sub> H <sub>15</sub> + ThB <sub>6</sub> H <sub>4</sub> C <sub>6</sub> N                                     | -0.3093             |
| ThNH <sub>4</sub> B <sub>6</sub> C <sub>6</sub> | 1.2 B <sub>5</sub> H <sub>7</sub> + Th + 1.2 H <sub>8</sub> C <sub>5</sub> + 2.833 N <sub>2</sub> → 4.667 H <sub>3</sub> N + ThB <sub>6</sub> H <sub>4</sub> C <sub>6</sub> N                                                       | -0.3088             |
| ThNH <sub>4</sub> B <sub>6</sub> C <sub>6</sub> | 3.524 ThC + 1.238 B <sub>13</sub> C <sub>2</sub> + 1.333 H <sub>3</sub> N → 2.524 ThB <sub>4</sub> + 0.1667 N <sub>2</sub> + ThB <sub>6</sub> H <sub>4</sub> C <sub>6</sub> N                                                       | -0.3026             |
| ThNH <sub>4</sub> B <sub>6</sub> C <sub>6</sub> | 0.6667 B <sub>9</sub> H <sub>11</sub> + 2 Th <sub>2</sub> C <sub>3</sub> + 1.167 N <sub>2</sub> → 1.667 ThH <sub>2</sub> + 1.333 ThN + ThB <sub>6</sub> H <sub>4</sub> C <sub>6</sub> N                                             | -0.3026             |
| ThNH <sub>4</sub> B <sub>6</sub> C <sub>6</sub> | 9.5 H <sub>2</sub> + 2 Th <sub>2</sub> C <sub>3</sub> + 0.5 N <sub>2</sub> + ThB <sub>6</sub> → Th <sub>4</sub> H <sub>15</sub> + ThB <sub>6</sub> H <sub>4</sub> C <sub>6</sub> N                                                  | -0.2977             |
| ThNH <sub>4</sub> B <sub>6</sub> C <sub>6</sub> | 1.2 B <sub>5</sub> H <sub>7</sub> + 6 C + 3.2 Th + 0.5 N <sub>2</sub> → 2.2 ThH <sub>2</sub> + ThB <sub>6</sub> H <sub>4</sub> C <sub>6</sub> N                                                                                     | -0.2941             |
| ThNH <sub>4</sub> B <sub>6</sub> C <sub>6</sub> | 0.5 H <sub>2</sub> + 2 Th <sub>2</sub> C <sub>3</sub> + H <sub>3</sub> N + 9 ThB <sub>6</sub> → 12 ThB <sub>4</sub> + ThB <sub>6</sub> H <sub>4</sub> C <sub>6</sub> N                                                              | -0.2915             |
| ThNH <sub>4</sub> B <sub>6</sub> C <sub>6</sub> | 1.786 B <sub>5</sub> H <sub>7</sub> + 2 Th <sub>2</sub> C <sub>3</sub> + 0.5 N <sub>2</sub> → 0.7326 ThB <sub>4</sub> + 0.5668 Th <sub>4</sub> H <sub>15</sub> + ThB <sub>6</sub> H <sub>4</sub> C <sub>6</sub> N                   | -0.2908             |
| ThNH <sub>4</sub> B <sub>6</sub> C <sub>6</sub> | 6 ThC + 18.2 H <sub>3</sub> N + 7.9 ThB <sub>6</sub> → 4.3 Th <sub>3</sub> N <sub>4</sub> + 4.6 B <sub>9</sub> H <sub>11</sub> + ThB <sub>6</sub> H <sub>4</sub> C <sub>6</sub> N                                                   | -0.2892             |
| ThNH <sub>4</sub> B <sub>6</sub> C <sub>6</sub> | 2.902 ThC + 0.3636 B <sub>9</sub> H <sub>11</sub> + 1.549 B <sub>13</sub> C <sub>2</sub> + ThN → 2.902 ThB <sub>6</sub> + ThB <sub>6</sub> H <sub>4</sub> C <sub>6</sub> N                                                          | -0.2890             |

Continued on next page

Continued

| Compound                                        | Chemical reaction                                                                                                                                                                                                     | Reaction energy(eV) |
|-------------------------------------------------|-----------------------------------------------------------------------------------------------------------------------------------------------------------------------------------------------------------------------|---------------------|
| ThNH <sub>4</sub> B <sub>6</sub> C <sub>6</sub> | 2 ThH <sub>2</sub> + 1.5 ThB <sub>4</sub> + 6 C + 2.167 N <sub>2</sub> → 0.8333 Th <sub>3</sub> N <sub>4</sub> + ThB <sub>6</sub> H <sub>4</sub> C <sub>6</sub> N                                                     | -0.2885             |
| ThNH <sub>4</sub> B <sub>6</sub> C <sub>6</sub> | 0.5 ThH <sub>2</sub> + 2.88 ThC + 1.56 B <sub>13</sub> C <sub>2</sub> + H <sub>3</sub> N → 2.38 ThB <sub>6</sub> + ThB <sub>6</sub> H <sub>4</sub> C <sub>6</sub> N                                                   | -0.2868             |
| ThNH <sub>4</sub> B <sub>6</sub> C <sub>6</sub> | 3.958 H <sub>2</sub> + 0.6667 B <sub>9</sub> H <sub>11</sub> + 2 Th <sub>2</sub> C <sub>3</sub> + 0.5 N <sub>2</sub> → 0.75 Th <sub>4</sub> H <sub>15</sub> + ThB <sub>6</sub> H <sub>4</sub> C <sub>6</sub> N        | -0.2841             |
| ThNH <sub>4</sub> B <sub>6</sub> C <sub>6</sub> | 1.143 B <sub>9</sub> H <sub>11</sub> + 2 Th <sub>2</sub> C <sub>3</sub> + 0.5 N <sub>2</sub> → 0.5714 Th <sub>4</sub> H <sub>15</sub> + 0.7143 ThB <sub>6</sub> + ThB <sub>6</sub> H <sub>4</sub> C <sub>6</sub> N    | -0.2744             |
| ThNH <sub>4</sub> B <sub>6</sub> C <sub>6</sub> | 2 Th <sub>2</sub> C <sub>3</sub> + 11.71 B + 4 H <sub>3</sub> N → 1.143 B <sub>5</sub> H <sub>7</sub> + 3 ThN + ThB <sub>6</sub> H <sub>4</sub> C <sub>6</sub> N                                                      | -0.2601             |
| ThNH <sub>4</sub> B <sub>6</sub> C <sub>6</sub> | 7.121 ThC + 1.477 B <sub>9</sub> H <sub>11</sub> + 0.5 N <sub>2</sub> → 6.121 ThH <sub>2</sub> + 0.5607 B <sub>13</sub> C <sub>2</sub> + ThB <sub>6</sub> H <sub>4</sub> C <sub>6</sub> N                             | -0.2580             |
| ThNH <sub>4</sub> B <sub>6</sub> C <sub>6</sub> | 0.1429 B <sub>5</sub> H <sub>7</sub> + 2 Th <sub>2</sub> C <sub>3</sub> + H <sub>3</sub> N + 8.643 ThB <sub>6</sub> → 11.64 ThB <sub>4</sub> + ThB <sub>6</sub> H <sub>4</sub> C <sub>6</sub> N                       | -0.2453             |
| ThNH <sub>4</sub> B <sub>6</sub> C <sub>6</sub> | 0.09091 B <sub>9</sub> H <sub>11</sub> + 2 Th <sub>2</sub> C <sub>3</sub> + H <sub>3</sub> N + 8.591 ThB <sub>6</sub> → 11.59 ThB <sub>4</sub> + ThB <sub>6</sub> H <sub>4</sub> C <sub>6</sub> N                     | -0.2448             |
| ThNH <sub>4</sub> B <sub>6</sub> C <sub>6</sub> | 2.667 B <sub>9</sub> H <sub>11</sub> + 2 Th <sub>2</sub> C <sub>3</sub> + 0.5 N <sub>2</sub> → 12.67 H <sub>2</sub> + 3 ThB <sub>6</sub> + ThB <sub>6</sub> H <sub>4</sub> C <sub>6</sub> N                           | -0.2432             |
| ThNH <sub>4</sub> B <sub>6</sub> C <sub>6</sub> | 3 ThC <sub>2</sub> + 16 B + 1.333 H <sub>3</sub> N → 1.667 ThB <sub>6</sub> + 0.3333 ThN + ThB <sub>6</sub> H <sub>4</sub> C <sub>6</sub> N                                                                           | -0.2428             |
| ThNH <sub>4</sub> B <sub>6</sub> C <sub>6</sub> | 3 ThC <sub>2</sub> + 0.6667 B <sub>9</sub> H <sub>11</sub> + 1.241 N <sub>2</sub> → 0.3704 Th <sub>3</sub> N <sub>4</sub> + 0.2222 Th <sub>4</sub> H <sub>15</sub> + ThB <sub>6</sub> H <sub>4</sub> C <sub>6</sub> N | -0.2419             |
| ThNH <sub>4</sub> B <sub>6</sub> C <sub>6</sub> | 6 B + 5.3 Th + H <sub>3</sub> N + 1.2 H <sub>8</sub> C <sub>5</sub> → 4.3 ThH <sub>2</sub> + ThB <sub>6</sub> H <sub>4</sub> C <sub>6</sub> N                                                                         | -0.2401             |
| ThNH <sub>4</sub> B <sub>6</sub> C <sub>6</sub> | 0.5714 B <sub>5</sub> H <sub>7</sub> + 2.869 ThC + 1.566 B <sub>13</sub> C <sub>2</sub> + ThN → 2.869 ThB <sub>6</sub> + ThB <sub>6</sub> H <sub>4</sub> C <sub>6</sub> N                                             | -0.2397             |
| ThNH <sub>4</sub> B <sub>6</sub> C <sub>6</sub> | 1.2 B <sub>5</sub> H <sub>7</sub> + 3.425 H <sub>2</sub> + 2 Th <sub>2</sub> C <sub>3</sub> + 0.5 N <sub>2</sub> → 0.75 Th <sub>4</sub> H <sub>15</sub> + ThB <sub>6</sub> H <sub>4</sub> C <sub>6</sub> N            | -0.2390             |
| ThNH <sub>4</sub> B <sub>6</sub> C <sub>6</sub> | BN + 0.5556 B <sub>9</sub> H <sub>11</sub> + 6.856 Th + 1.2 H <sub>8</sub> C <sub>5</sub> → 5.856 ThH <sub>2</sub> + ThB <sub>6</sub> H <sub>4</sub> C <sub>6</sub> N                                                 | -0.2257             |
| ThNH <sub>4</sub> B <sub>6</sub> C <sub>6</sub> | 2.79 ThC <sub>2</sub> + 0.3636 B <sub>9</sub> H <sub>11</sub> + 0.2098 B <sub>13</sub> C <sub>2</sub> + 1.395 N <sub>2</sub> → 1.79 ThN + ThB <sub>6</sub> H <sub>4</sub> C <sub>6</sub> N                            | -0.2233             |
| ThNH <sub>4</sub> B <sub>6</sub> C <sub>6</sub> | 3.786 B <sub>5</sub> H <sub>7</sub> + 6 ThC + ThN → 1.5 Th <sub>4</sub> H <sub>15</sub> + 12.93 B + ThB <sub>6</sub> H <sub>4</sub> C <sub>6</sub> N                                                                  | -0.2160             |
| ThNH <sub>4</sub> B <sub>6</sub> C <sub>6</sub> | 1.877 B <sub>5</sub> H <sub>7</sub> + 2 Th <sub>2</sub> C <sub>3</sub> + 0.5 N <sub>2</sub> → 0.6091 Th <sub>4</sub> H <sub>15</sub> + 0.5638 ThB <sub>6</sub> + ThB <sub>6</sub> H <sub>4</sub> C <sub>6</sub> N     | -0.2059             |
| ThNH <sub>4</sub> B <sub>6</sub> C <sub>6</sub> | 2 ThH <sub>2</sub> + 0.25 Th <sub>3</sub> N <sub>4</sub> + 1.582 B <sub>13</sub> C <sub>2</sub> + 0.9455 Th <sub>2</sub> C <sub>3</sub> → 3.641 ThB <sub>4</sub> + ThB <sub>6</sub> H <sub>4</sub> C <sub>6</sub> N   | -0.2016             |
| ThNH <sub>4</sub> B <sub>6</sub> C <sub>6</sub> | 3.795 ThC + 1.102 B <sub>13</sub> C <sub>2</sub> + 4.727 H <sub>3</sub> N → 0.9318 Th <sub>3</sub> N <sub>4</sub> + 0.9256 B <sub>9</sub> H <sub>11</sub> + ThB <sub>6</sub> H <sub>4</sub> C <sub>6</sub> N          | -0.1976             |
| ThNH <sub>4</sub> B <sub>6</sub> C <sub>6</sub> | 0.5 H <sub>2</sub> + 3 ThC <sub>2</sub> + 14 B + H <sub>3</sub> N → 2 ThB <sub>4</sub> + ThB <sub>6</sub> H <sub>4</sub> C <sub>6</sub> N                                                                             | -0.1866             |
| ThNH <sub>4</sub> B <sub>6</sub> C <sub>6</sub> | 0.5714 B <sub>5</sub> H <sub>7</sub> + 2.758 ThC <sub>2</sub> + 0.2418 B <sub>13</sub> C <sub>2</sub> + 1.379 N <sub>2</sub> → 1.758 ThN + ThB <sub>6</sub> H <sub>4</sub> C <sub>6</sub> N                           | -0.1748             |
| ThNH <sub>4</sub> B <sub>6</sub> C <sub>6</sub> | 3.24 ThC + 1.38 B <sub>13</sub> C <sub>2</sub> + 1.333 H <sub>3</sub> N → 0.08333 Th <sub>3</sub> N <sub>4</sub> + 1.99 ThB <sub>6</sub> + ThB <sub>6</sub> H <sub>4</sub> C <sub>6</sub> N                           | -0.1745             |
| ThNH <sub>4</sub> B <sub>6</sub> C <sub>6</sub> | 0.7961 B <sub>9</sub> H <sub>11</sub> + 2 Th <sub>2</sub> C <sub>3</sub> + 2.164 H <sub>3</sub> N → 0.75 Th <sub>4</sub> H <sub>15</sub> + 1.164 BN + ThB <sub>6</sub> H <sub>4</sub> C <sub>6</sub> N                | -0.1725             |
| ThNH <sub>4</sub> B <sub>6</sub> C <sub>6</sub> | 3.185 ThC + 0.09091 B <sub>9</sub> H <sub>11</sub> + 1.407 B <sub>13</sub> C <sub>2</sub> + H <sub>3</sub> N → 2.185 ThB <sub>6</sub> + ThB <sub>6</sub> H <sub>4</sub> C <sub>6</sub> N                              | -0.1722             |
| ThNH <sub>4</sub> B <sub>6</sub> C <sub>6</sub> | 6.125 H <sub>2</sub> + 2 Th <sub>2</sub> C <sub>3</sub> + 6 B + H <sub>3</sub> N → 0.75 Th <sub>4</sub> H <sub>15</sub> + ThB <sub>6</sub> H <sub>4</sub> C <sub>6</sub> N                                            | -0.1690             |
| ThNH <sub>4</sub> B <sub>6</sub> C <sub>6</sub> | 0.25 Th <sub>3</sub> N <sub>4</sub> + 3.022 ThC + 0.3636 B <sub>9</sub> H <sub>11</sub> + 1.489 B <sub>13</sub> C <sub>2</sub> → 2.772 ThB <sub>6</sub> + ThB <sub>6</sub> H <sub>4</sub> C <sub>6</sub> N            | -0.1654             |
| ThNH <sub>4</sub> B <sub>6</sub> C <sub>6</sub> | 2 Th <sub>2</sub> C <sub>3</sub> + 1.333 H <sub>3</sub> N + 8.5 ThB <sub>6</sub> → 11.25 ThB <sub>4</sub> + 0.08333 Th <sub>3</sub> N <sub>4</sub> + ThB <sub>6</sub> H <sub>4</sub> C <sub>6</sub> N                 | -0.1624             |
| ThNH <sub>4</sub> B <sub>6</sub> C <sub>6</sub> | 0.1429 B <sub>5</sub> H <sub>7</sub> + 3.177 ThC + 1.411 B <sub>13</sub> C <sub>2</sub> + H <sub>3</sub> N → 2.177 ThB <sub>6</sub> + ThB <sub>6</sub> H <sub>4</sub> C <sub>6</sub> N                                | -0.1599             |
| ThNH <sub>4</sub> B <sub>6</sub> C <sub>6</sub> | 1.065 Th <sub>4</sub> H <sub>15</sub> + 3 B <sub>13</sub> C <sub>2</sub> + 4.991 ThN → 8.25 ThB <sub>4</sub> + 3.991 H <sub>3</sub> N + ThB <sub>6</sub> H <sub>4</sub> C <sub>6</sub> N                              | -0.1596             |
| ThNH <sub>4</sub> B <sub>6</sub> C <sub>6</sub> | 15.12 B <sub>9</sub> H <sub>11</sub> + 2 Th <sub>2</sub> C <sub>3</sub> + H <sub>3</sub> N → 3 ThB <sub>4</sub> + 23.62 B <sub>5</sub> H <sub>7</sub> + ThB <sub>6</sub> H <sub>4</sub> C <sub>6</sub> N              | -0.1498             |
| ThNH <sub>4</sub> B <sub>6</sub> C <sub>6</sub> | 6 ThC + 3.333 H <sub>2</sub> + 0.6667 B <sub>9</sub> H <sub>11</sub> + 0.5 N <sub>2</sub> → 5 ThH <sub>2</sub> + ThB <sub>6</sub> H <sub>4</sub> C <sub>6</sub> N                                                     | -0.1498             |
| ThNH <sub>4</sub> B <sub>6</sub> C <sub>6</sub> | 2.225 B <sub>5</sub> H <sub>7</sub> + 6.789 ThC + 0.5 N <sub>2</sub> → 5.789 ThH <sub>2</sub> + 0.3944 B <sub>13</sub> C <sub>2</sub> + ThB <sub>6</sub> H <sub>4</sub> C <sub>6</sub> N                              | -0.1423             |
| ThNH <sub>4</sub> B <sub>6</sub> C <sub>6</sub> | 1.167 Th <sub>2</sub> C <sub>3</sub> + 6 B + 0.5 H <sub>8</sub> C <sub>5</sub> + 1.389 N <sub>2</sub> → 0.4444 Th <sub>3</sub> N <sub>4</sub> + ThB <sub>6</sub> H <sub>4</sub> C <sub>6</sub> N                      | -0.1390             |
| ThNH <sub>4</sub> B <sub>6</sub> C <sub>6</sub> | 2 ThH <sub>2</sub> + 1.421 ThC <sub>2</sub> + 1.579 B <sub>13</sub> C <sub>2</sub> + 0.5 N <sub>2</sub> → 2.421 ThB <sub>6</sub> + ThB <sub>6</sub> H <sub>4</sub> C <sub>6</sub> N                                   | -0.1363             |
| ThNH <sub>4</sub> B <sub>6</sub> C <sub>6</sub> | 3.28 ThC + 1.36 B <sub>13</sub> C <sub>2</sub> + 1.333 H <sub>3</sub> N → 1.947 ThB <sub>6</sub> + 0.3333 ThN + ThB <sub>6</sub> H <sub>4</sub> C <sub>6</sub> N                                                      | -0.1333             |
| ThNH <sub>4</sub> B <sub>6</sub> C <sub>6</sub> | 1.5 ThB <sub>4</sub> + 10.44 H <sub>2</sub> + 2 Th <sub>2</sub> C <sub>3</sub> + 0.5 N <sub>2</sub> → 1.125 Th <sub>4</sub> H <sub>15</sub> + ThB <sub>6</sub> H <sub>4</sub> C <sub>6</sub> N                        | -0.1330             |
| ThNH <sub>4</sub> B <sub>6</sub> C <sub>6</sub> | 1.2 B <sub>5</sub> H <sub>7</sub> + 6 C + 2.973 Th + H <sub>3</sub> N → 0.4933 Th <sub>4</sub> H <sub>15</sub> + ThB <sub>6</sub> H <sub>4</sub> C <sub>6</sub> N                                                     | -0.1320             |
| ThNH <sub>4</sub> B <sub>6</sub> C <sub>6</sub> | 3.652 B <sub>5</sub> H <sub>7</sub> + 0.25 Th <sub>3</sub> N <sub>4</sub> + 6 ThC → 1.438 Th <sub>4</sub> H <sub>15</sub> + 12.26 B + ThB <sub>6</sub> H <sub>4</sub> C <sub>6</sub> N                                | -0.1285             |
| ThNH <sub>4</sub> B <sub>6</sub> C <sub>6</sub> | 3.12 ThC + 0.5 H <sub>2</sub> + 1.44 B <sub>13</sub> C <sub>2</sub> + H <sub>3</sub> N → 2.12 ThB <sub>6</sub> + ThB <sub>6</sub> H <sub>4</sub> C <sub>6</sub> N                                                     | -0.1175             |
| ThNH <sub>4</sub> B <sub>6</sub> C <sub>6</sub> | 20.38 B <sub>9</sub> H <sub>11</sub> + 2 Th <sub>2</sub> C <sub>3</sub> + H <sub>3</sub> N → 31.88 B <sub>5</sub> H <sub>7</sub> + 3 ThB <sub>6</sub> + ThB <sub>6</sub> H <sub>4</sub> C <sub>6</sub> N              | -0.1167             |
| ThNH <sub>4</sub> B <sub>6</sub> C <sub>6</sub> | 0.5714 B <sub>5</sub> H <sub>7</sub> + 0.25 Th <sub>3</sub> N <sub>4</sub> + 2.989 ThC + 1.506 B <sub>13</sub> C <sub>2</sub> → 2.739 ThB <sub>6</sub> + ThB <sub>6</sub> H <sub>4</sub> C <sub>6</sub> N             | -0.1162             |
| ThNH <sub>4</sub> B <sub>6</sub> C <sub>6</sub> | 3.5 ThC + 0.5 H <sub>8</sub> C <sub>5</sub> + 0.5 N <sub>2</sub> + 8 ThB <sub>6</sub> → 10.5 ThB <sub>4</sub> + ThB <sub>6</sub> H <sub>4</sub> C <sub>6</sub> N                                                      | -0.1131             |
| ThNH <sub>4</sub> B <sub>6</sub> C <sub>6</sub> | 1.2 B <sub>5</sub> H <sub>7</sub> + 6 ThC + 2.8 H <sub>2</sub> + 0.5 N <sub>2</sub> → 5 ThH <sub>2</sub> + ThB <sub>6</sub> H <sub>4</sub> C <sub>6</sub> N                                                           | -0.1047             |
| ThNH <sub>4</sub> B <sub>6</sub> C <sub>6</sub> | 3.931 ThC + BN + 0.3636 B <sub>9</sub> H <sub>11</sub> + 1.035 B <sub>13</sub> C <sub>2</sub> → 2.931 ThB <sub>4</sub> + ThB <sub>6</sub> H <sub>4</sub> C <sub>6</sub> N                                             | -0.0899             |
| ThNH <sub>4</sub> B <sub>6</sub> C <sub>6</sub> | 0.3636 B <sub>9</sub> H <sub>11</sub> + 0.8033 B <sub>13</sub> C <sub>2</sub> + 1.464 Th <sub>2</sub> C <sub>3</sub> + 0.5 N <sub>2</sub> → 1.929 ThB <sub>4</sub> + ThB <sub>6</sub> H <sub>4</sub> C <sub>6</sub> N | -0.0856             |
| ThNH <sub>4</sub> B <sub>6</sub> C <sub>6</sub> | 1.75 B <sub>13</sub> C <sub>2</sub> + 0.5 H <sub>8</sub> C <sub>5</sub> + 4.35 ThN → 3.35 ThB <sub>4</sub> + 3.35 BN + ThB <sub>6</sub> H <sub>4</sub> C <sub>6</sub> N                                               | -0.0710             |
| ThNH <sub>4</sub> B <sub>6</sub> C <sub>6</sub> | 2.64 ThC + 2 H <sub>2</sub> + 1.68 B <sub>13</sub> C <sub>2</sub> + ThN → 2.64 ThB <sub>6</sub> + ThB <sub>6</sub> H <sub>4</sub> C <sub>6</sub> N                                                                    | -0.0700             |
| ThNH <sub>4</sub> B <sub>6</sub> C <sub>6</sub> | 4.8 B <sub>5</sub> H <sub>7</sub> + 2 Th <sub>2</sub> C <sub>3</sub> + 0.5 N <sub>2</sub> → 14.8 H <sub>2</sub> + 3 ThB <sub>6</sub> + ThB <sub>6</sub> H <sub>4</sub> C <sub>6</sub> N                               | -0.0629             |
| ThNH <sub>4</sub> B <sub>6</sub> C <sub>6</sub> | 5.077 ThC + 6.077 H <sub>2</sub> + 0.4615 B <sub>13</sub> C <sub>2</sub> + 0.5 N <sub>2</sub> → 4.077 ThH <sub>2</sub> + ThB <sub>6</sub> H <sub>4</sub> C <sub>6</sub> N                                             | -0.0608             |
| ThNH <sub>4</sub> B <sub>6</sub> C <sub>6</sub> | 2 Th <sub>2</sub> C <sub>3</sub> + 1.333 H <sub>3</sub> N + 8.333 ThB <sub>6</sub> → 11 ThB <sub>4</sub> + 0.3333 ThN + ThB <sub>6</sub> H <sub>4</sub> C <sub>6</sub> N                                              | -0.0591             |
| ThNH <sub>4</sub> B <sub>6</sub> C <sub>6</sub> | 6.471 H <sub>2</sub> + 0.4615 B <sub>13</sub> C <sub>2</sub> + 1.692 Th <sub>2</sub> C <sub>3</sub> + 0.5 N <sub>2</sub> → 0.5962 Th <sub>4</sub> H <sub>15</sub> + ThB <sub>6</sub> H <sub>4</sub> C <sub>6</sub> N  | -0.0584             |
| ThNH <sub>4</sub> B <sub>6</sub> C <sub>6</sub> | 3.083 Th <sub>3</sub> N <sub>4</sub> + 19 H <sub>2</sub> + 3 B <sub>13</sub> C <sub>2</sub> → 8.25 ThB <sub>4</sub> + 11.33 H <sub>3</sub> N + ThB <sub>6</sub> H <sub>4</sub> C <sub>6</sub> N                       | -0.0551             |
| ThNH <sub>4</sub> B <sub>6</sub> C <sub>6</sub> | 1.5 ThB <sub>4</sub> + 6 ThC + 7.5 H <sub>3</sub> N → 9.25 H <sub>2</sub> + 6.5 ThN + ThB <sub>6</sub> H <sub>4</sub> C <sub>6</sub> N                                                                                | -0.0540             |
| ThNH <sub>4</sub> B <sub>6</sub> C <sub>6</sub> | 0.5714 B <sub>5</sub> H <sub>7</sub> + 0.826 B <sub>13</sub> C <sub>2</sub> + 1.449 Th <sub>2</sub> C <sub>3</sub> + 0.5 N <sub>2</sub> → 1.899 ThB <sub>4</sub> + ThB <sub>6</sub> H <sub>4</sub> C <sub>6</sub> N   | -0.0500             |
| ThNH <sub>4</sub> B <sub>6</sub> C <sub>6</sub> | 4.867 Th <sub>3</sub> N <sub>4</sub> + 5.4 B <sub>9</sub> H <sub>11</sub> + 3 B <sub>13</sub> C <sub>2</sub> → 18.47 H <sub>3</sub> N + 13.6 ThB <sub>6</sub> + ThB <sub>6</sub> H <sub>4</sub> C <sub>6</sub> N      | -0.0398             |
| ThNH <sub>4</sub> B <sub>6</sub> C <sub>6</sub> | 0.1429 B <sub>5</sub> H <sub>7</sub> + 3 ThC <sub>2</sub> + 13.29 B + H <sub>3</sub> N → 2 ThB <sub>4</sub> + ThB <sub>6</sub> H <sub>4</sub> C <sub>6</sub> N                                                        | -0.0373             |
| ThNH <sub>4</sub> B <sub>6</sub> C <sub>6</sub> | 6 ThC + 5.5 H <sub>2</sub> + 6 B + H <sub>3</sub> N → 5 ThH <sub>2</sub> + ThB <sub>6</sub> H <sub>4</sub> C <sub>6</sub> N                                                                                           | -0.0347             |
| ThNH <sub>4</sub> B <sub>6</sub> C <sub>6</sub> | 0.5714 B <sub>5</sub> H <sub>7</sub> + 3.891 ThC + BN + 1.054 B <sub>13</sub> C <sub>2</sub> → 2.891 ThB <sub>4</sub> + ThB <sub>6</sub> H <sub>4</sub> C <sub>6</sub> N                                              | -0.0307             |
| ThNH <sub>4</sub> B <sub>6</sub> C <sub>6</sub> | 3 ThC <sub>2</sub> + 0.09091 B <sub>9</sub> H <sub>11</sub> + 13.18 B + H <sub>3</sub> N → 2 ThB <sub>4</sub> + ThB <sub>6</sub> H <sub>4</sub> C <sub>6</sub> N                                                      | -0.0217             |

Continued on next page

Continued

| Compound                                        | Chemical reaction                                                                                                                                                                                         | Reaction energy(eV) |
|-------------------------------------------------|-----------------------------------------------------------------------------------------------------------------------------------------------------------------------------------------------------------|---------------------|
| ThNH <sub>4</sub> B <sub>6</sub> C <sub>6</sub> | 2 H <sub>2</sub> + 2.538 ThC <sub>2</sub> + 0.4615 B <sub>13</sub> C <sub>2</sub> + 1.269 N <sub>2</sub> $\longrightarrow$ 1.538 ThN + ThB <sub>6</sub> H <sub>4</sub> C <sub>6</sub> N                   | -0.0101             |
| ThNH <sub>4</sub> B <sub>6</sub> C <sub>6</sub> | 2.992 ThC + 0.06667 Th <sub>4</sub> H <sub>15</sub> + 1.504 B <sub>13</sub> C <sub>2</sub> + H <sub>3</sub> N $\longrightarrow$ 2.259 ThB <sub>6</sub> + ThB <sub>6</sub> H <sub>4</sub> C <sub>6</sub> N | -0.0067             |



---

\* [li.zhu@rutgers.edu](mailto:li.zhu@rutgers.edu)

- [1] G. Bergerhoff, R. Hundt, R. Sievers, and I. D. Brown, The inorganic crystal structure data base, *J. Chem. Inf. Comput. Sci.* **23**, 66 (1983).
